# Supplementary material for: Exploring Consequences of Simulation Design for Apparent Performance of Statistical Methods. 2: Results from simulations with normally and uniformly distributed sample sizes
Source: arXiv:2007.05354 ancillary file (2020-07-07)
Supplement: Supplementary file 1 [file Appendix_A.pdf]

## Appendix A.

Results from simulations with normally distributed  
sample sizes

July 7, 2020

## A1.1 Results from simulations with normally distributed sample sizes

### Plots of bias of estimators of $\tau^2$ for log-odds-ratio

Each figure corresponds to a value of  $\theta$  ( $= 0, 0.5, 1, 1.5, 2$ ), a value of  $p_C$  ( $= .1, .4$ ), and a value of  $\sigma^2$  ( $= 0.1, 0.4$ ).

Each panel of a figure corresponds to a value of  $n$  ( $= 40, 100, 250, 1000$ ) and a value of  $K$  ( $= 5, 10, 30$ ) and has  $\tau^2 = 0.0(0.1)1.0$  on the horizontal axis.

The data-generation mechanisms are

- FIM1 - Fixed-intercept model with  $c = 0$
- FIM2 - Fixed-intercept model with  $c = 1/2$
- RIM1 - Random-intercept model with  $c = 0$
- RIM2 - Random-intercept model with  $c = 1/2$
- URIM1 - Random-intercept model with  $c = 0$  and  $p_{iC}$  uniformly distributed on  $[p_C - \sigma\sqrt{3}p_C(1 - p_C), p_C + \sigma\sqrt{3}p_C(1 - p_C)]$

The point estimators of  $\tau^2$  are

- $\hat{\tau}_{DL}^2$  - DerSimonian-Laird
- $\hat{\tau}_{REML}^2$  - Restricted maximum-likelihood
- $\hat{\tau}_{MP}^2$  - Mandel-Paule
- $\hat{\tau}_{KD}^2$  - Kulinskaya-Dollinger
- $\hat{\tau}_{FIM2}^2$  - Estimator of  $\tau^2$  in the FIM2 GLMM
- $\hat{\tau}_{RIM2}^2$  - Estimator of  $\tau^2$  in the RIM2 GLMM

### A1.1 Bias of $\hat{\tau}_{DL}^2$

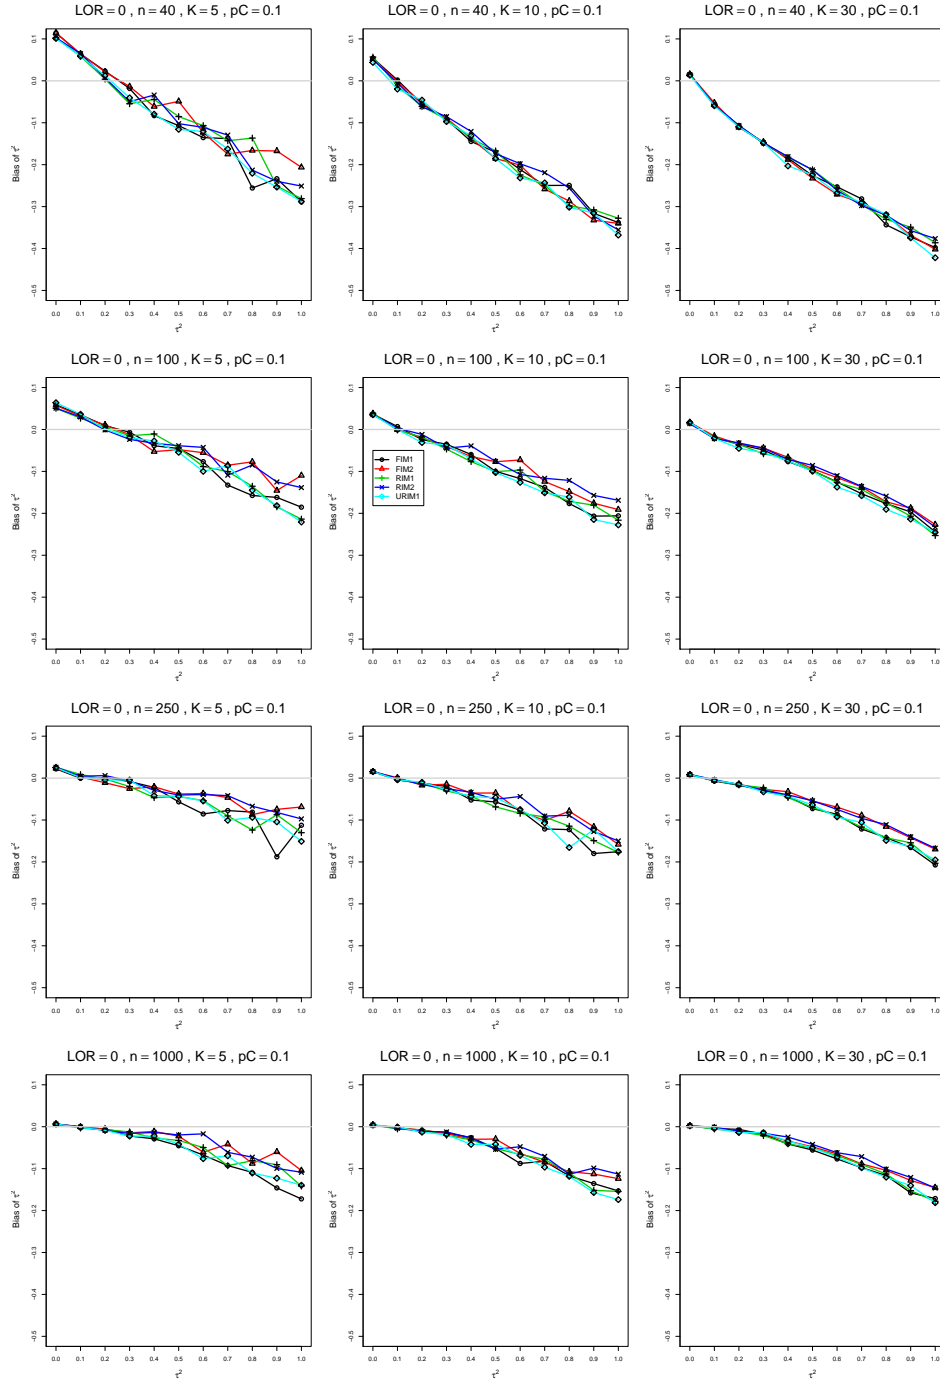

Figure A1.1.1: Bias of between-studies variance  $\hat{\tau}_{DL}^2$  for  $\theta = 0$ ,  $p_C = 0.1$ ,  $\sigma^2 = 0.1$ , constant sample sizes  $n = 40, 100, 250, 1000$ . The data-generation mechanisms are FIM1 ( $\circ$ ), FIM2 ( $\triangle$ ), RIM1 ( $+$ ), RIM2 ( $\times$ ), and URIM1 ( $\diamond$ ).



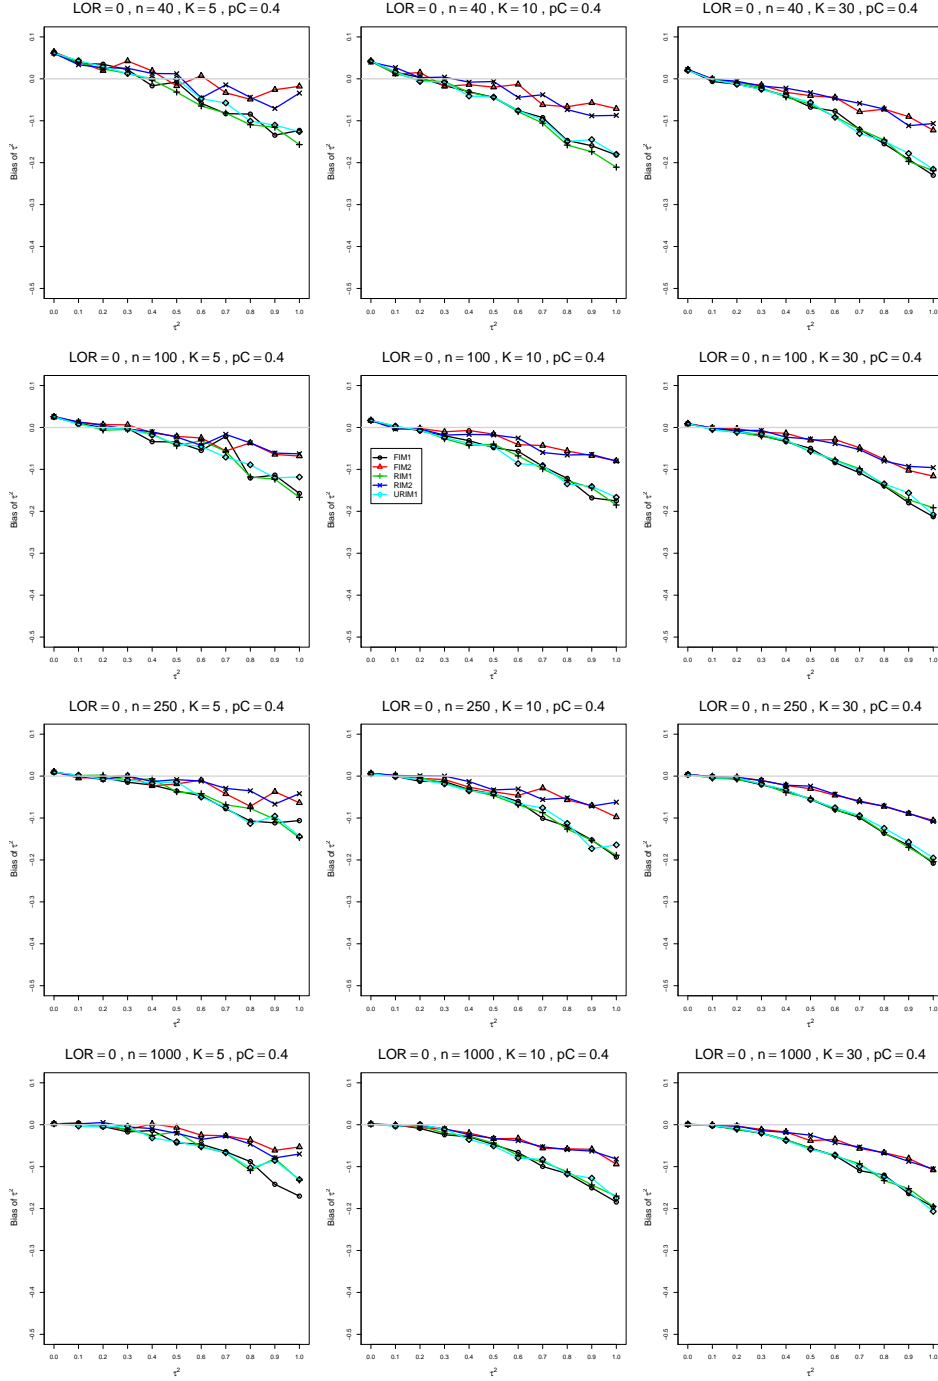

Figure A1.1.2: Bias of between-studies variance  $\hat{\tau}_{DL}^2$  for  $\theta = 0$ ,  $p_C = 0.4$ ,  $\sigma^2 = 0.1$ , constant sample sizes  $n = 40, 100, 250, 1000$ . The data-generation mechanisms are FIM1 ( $\circ$ ), FIM2 ( $\triangle$ ), RIM1 ( $+$ ), RIM2 ( $\times$ ), and URIM1 ( $\diamond$ ).

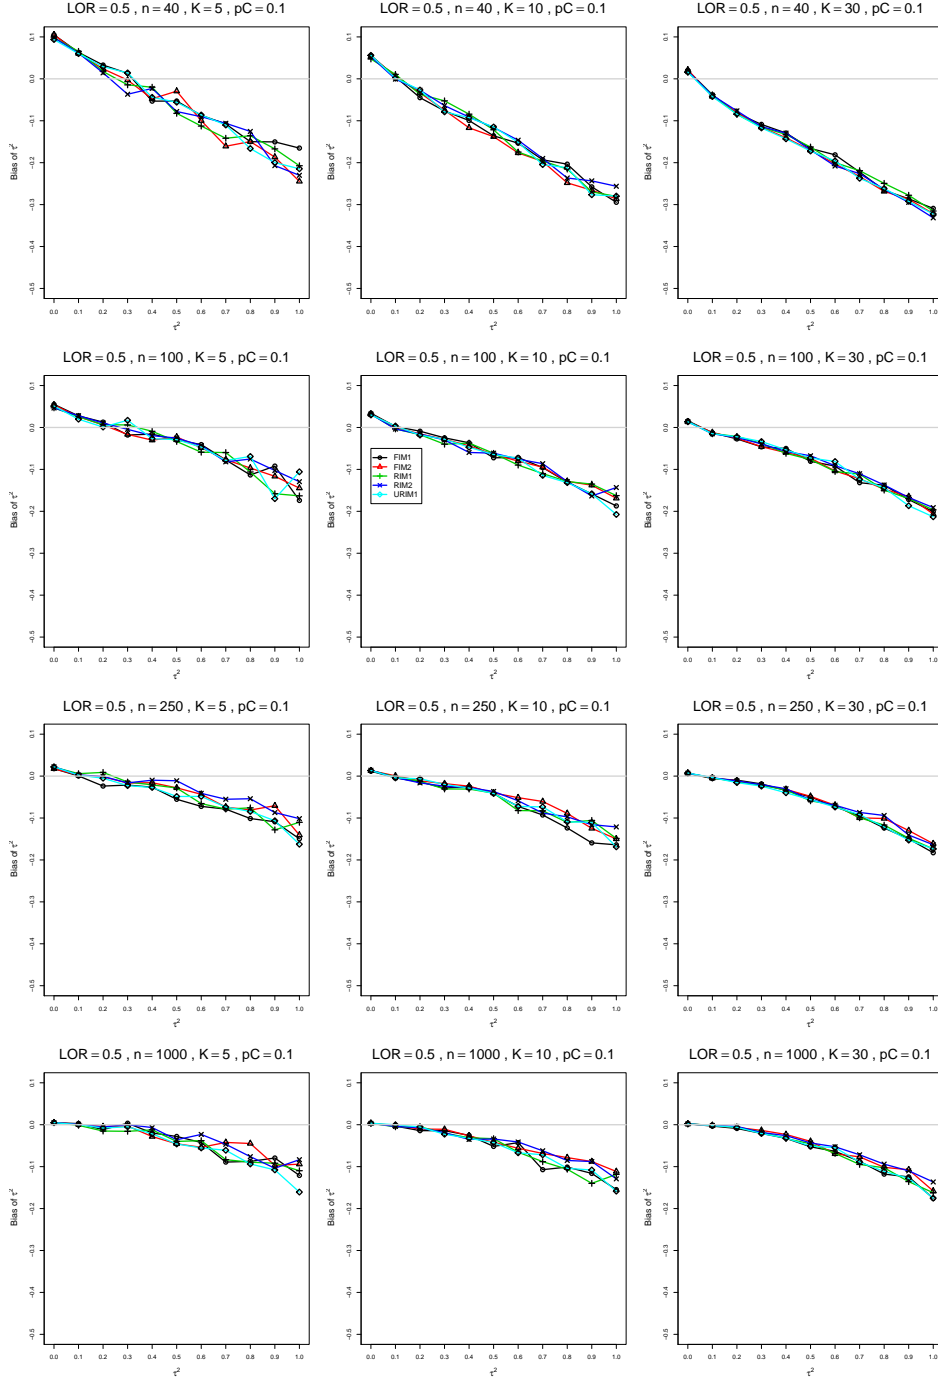

Figure A1.1.3: Bias of between-studies variance  $\hat{\tau}_{DL}^2$  for  $\theta = 0.5$ ,  $p_C = 0.1$ ,  $\sigma^2 = 0.1$ , constant sample sizes  $n = 40, 100, 250, 1000$ . The data-generation mechanisms are FIM1 ( $\circ$ ), FIM2 ( $\triangle$ ), RIM1 ( $+$ ), RIM2 ( $\times$ ), and URIM1 ( $\diamond$ ).

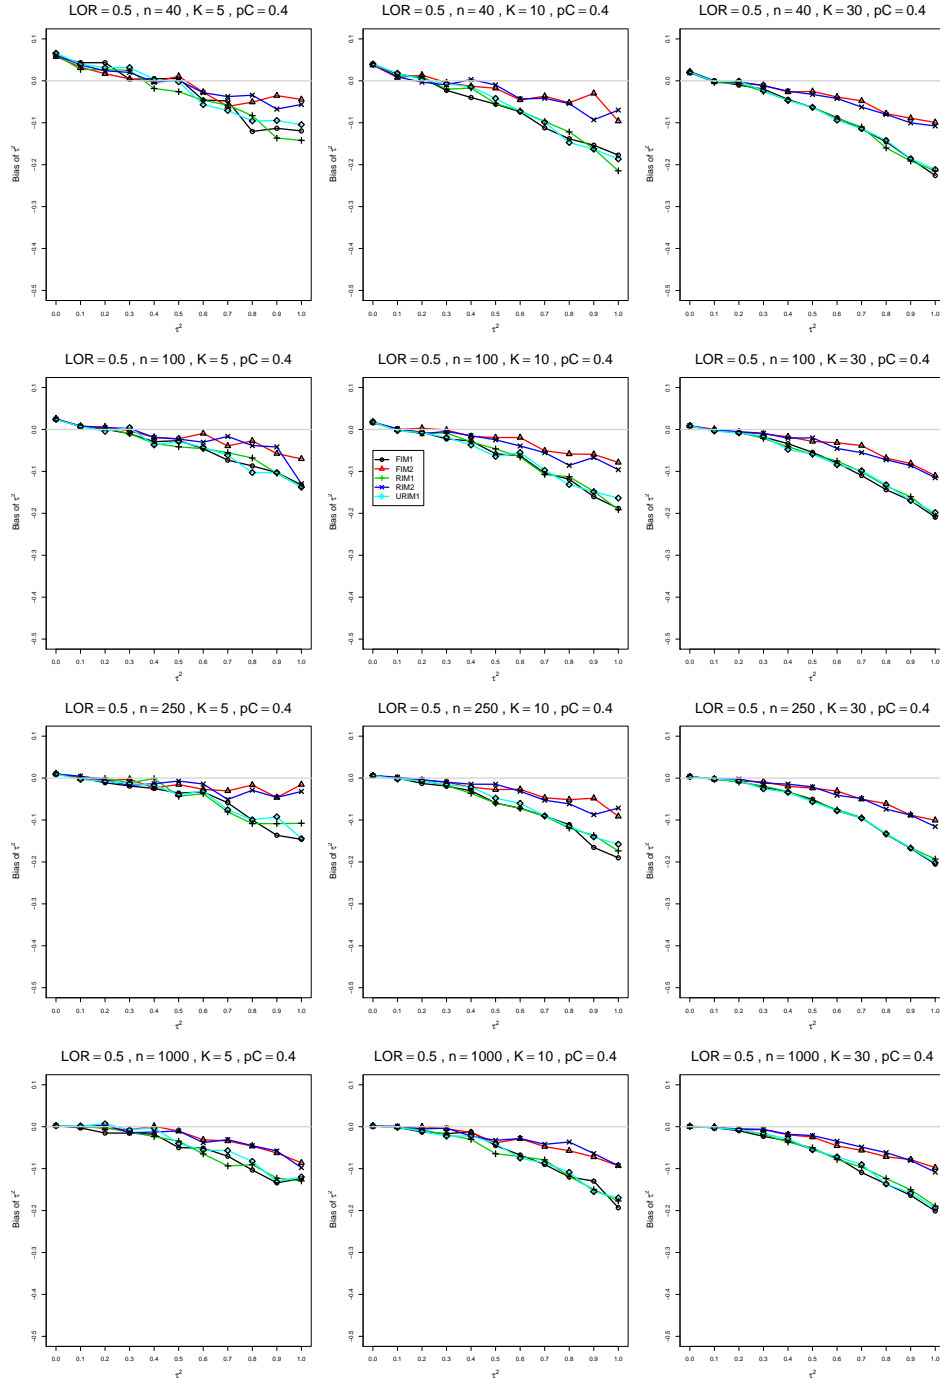

Figure A1.1.4: Bias of between-studies variance  $\hat{\tau}_{DL}^2$  for  $\theta = 0.5$ ,  $p_C = 0.4$ ,  $\sigma^2 = 0.1$ , constant sample sizes  $n = 40, 100, 250, 1000$ . The data-generation mechanisms are FIM1 ( $\circ$ ), FIM2 ( $\triangle$ ), RIM1 ( $+$ ), RIM2 ( $\times$ ), and URIM1 ( $\diamond$ ).

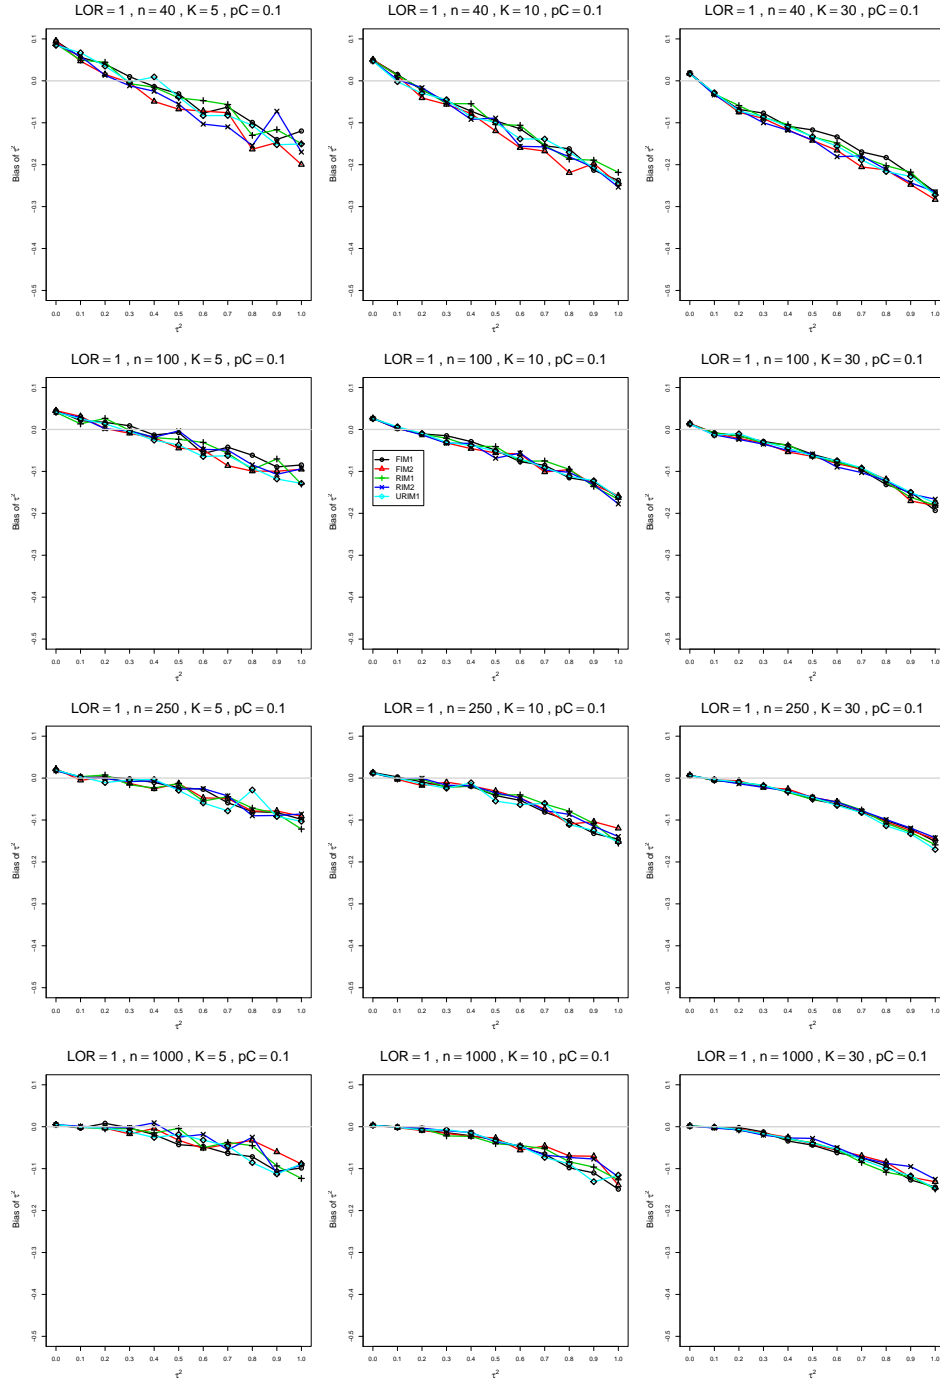

Figure A1.1.5: Bias of between-studies variance  $\hat{\tau}_{DL}^2$  for  $\theta = 1$ ,  $p_C = 0.1$ ,  $\sigma^2 = 0.1$ , constant sample sizes  $n = 40, 100, 250, 1000$ . The data-generation mechanisms are FIM1 ( $\circ$ ), FIM2 ( $\triangle$ ), RIM1 ( $+$ ), RIM2 ( $\times$ ), and URIM1 ( $\diamond$ ).

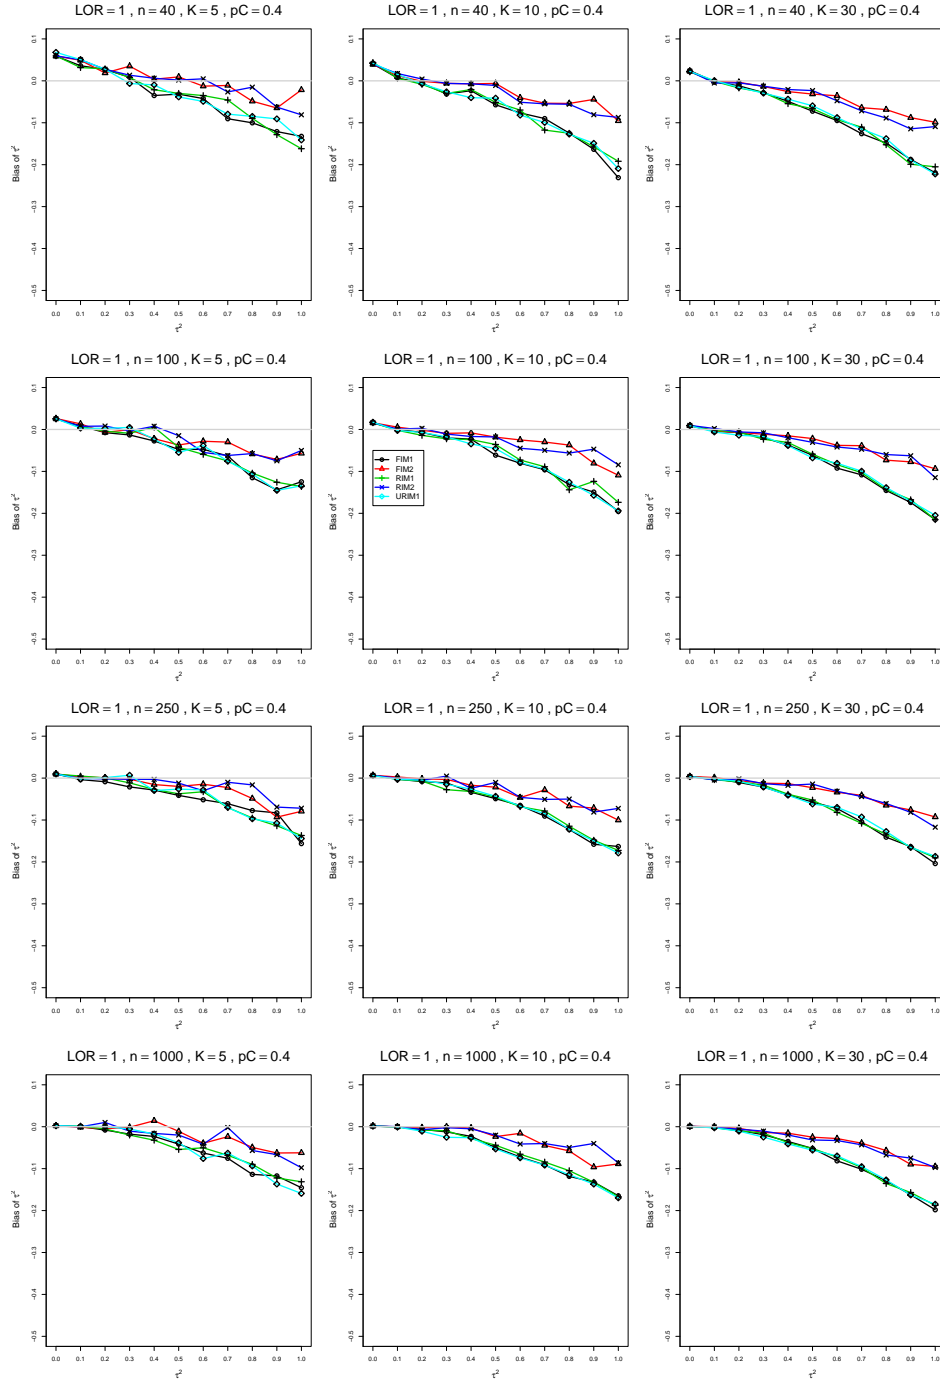

Figure A1.1.6: Bias of between-studies variance  $\hat{\tau}_{DL}^2$  for  $\theta = 1$ ,  $p_C = 0.4$ ,  $\sigma^2 = 0.1$ , constant sample sizes  $n = 40, 100, 250, 1000$ . The data-generation mechanisms are FIM1 ( $\circ$ ), FIM2 ( $\triangle$ ), RIM1 ( $+$ ), RIM2 ( $\times$ ), and URIM1 ( $\diamond$ ).

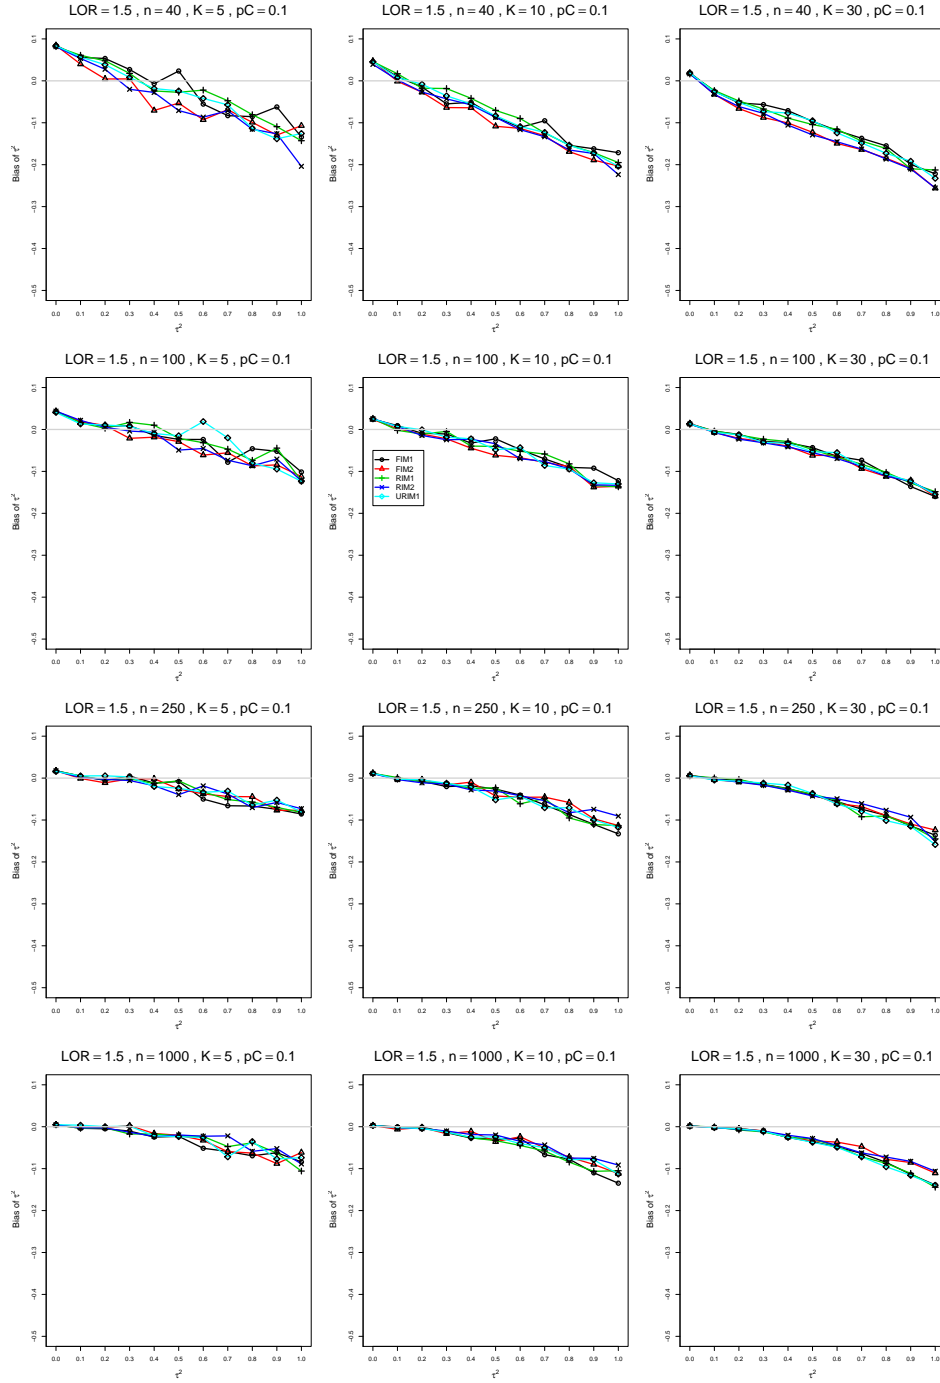

Figure A1.1.7: Bias of between-studies variance  $\hat{\tau}_{DL}^2$  for  $\theta = 1.5$ ,  $p_C = 0.1$ ,  $\sigma^2 = 0.1$ , constant sample sizes  $n = 40, 100, 250, 1000$ . The data-generation mechanisms are FIM1 ( $\circ$ ), FIM2 ( $\triangle$ ), RIM1 ( $+$ ), RIM2 ( $\times$ ), and URIM1 ( $\diamond$ ).

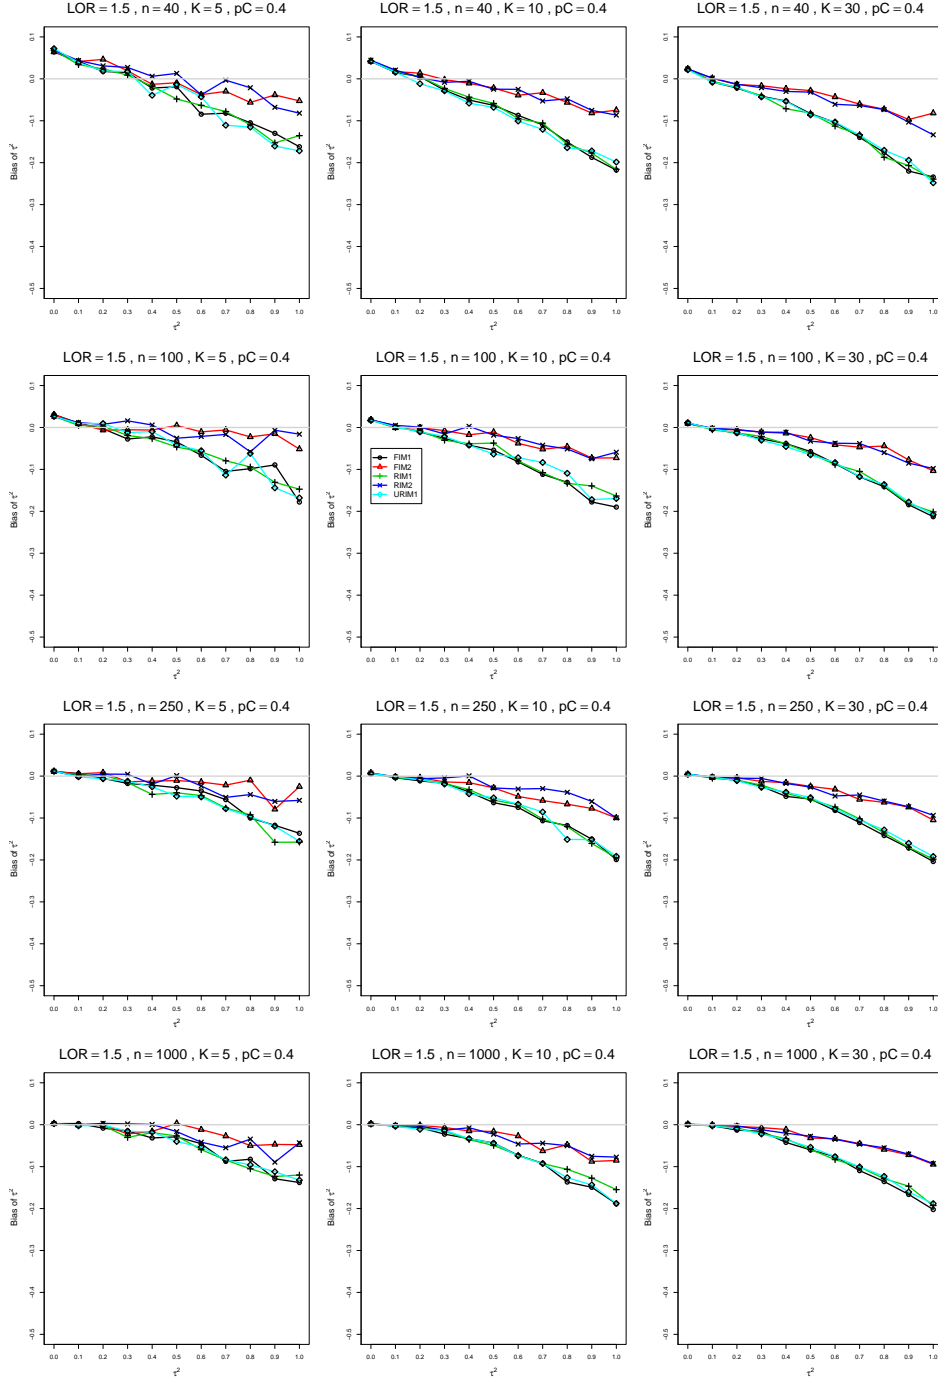

Figure A1.1.8: Bias of between-studies variance  $\hat{\tau}_{DL}^2$  for  $\theta = 1.5$ ,  $p_C = 0.4$ ,  $\sigma^2 = 0.1$ , constant sample sizes  $n = 40, 100, 250, 1000$ . The data-generation mechanisms are FIM1 ( $\circ$ ), FIM2 ( $\triangle$ ), RIM1 ( $+$ ), RIM2 ( $\times$ ), and URIM1 ( $\diamond$ ).

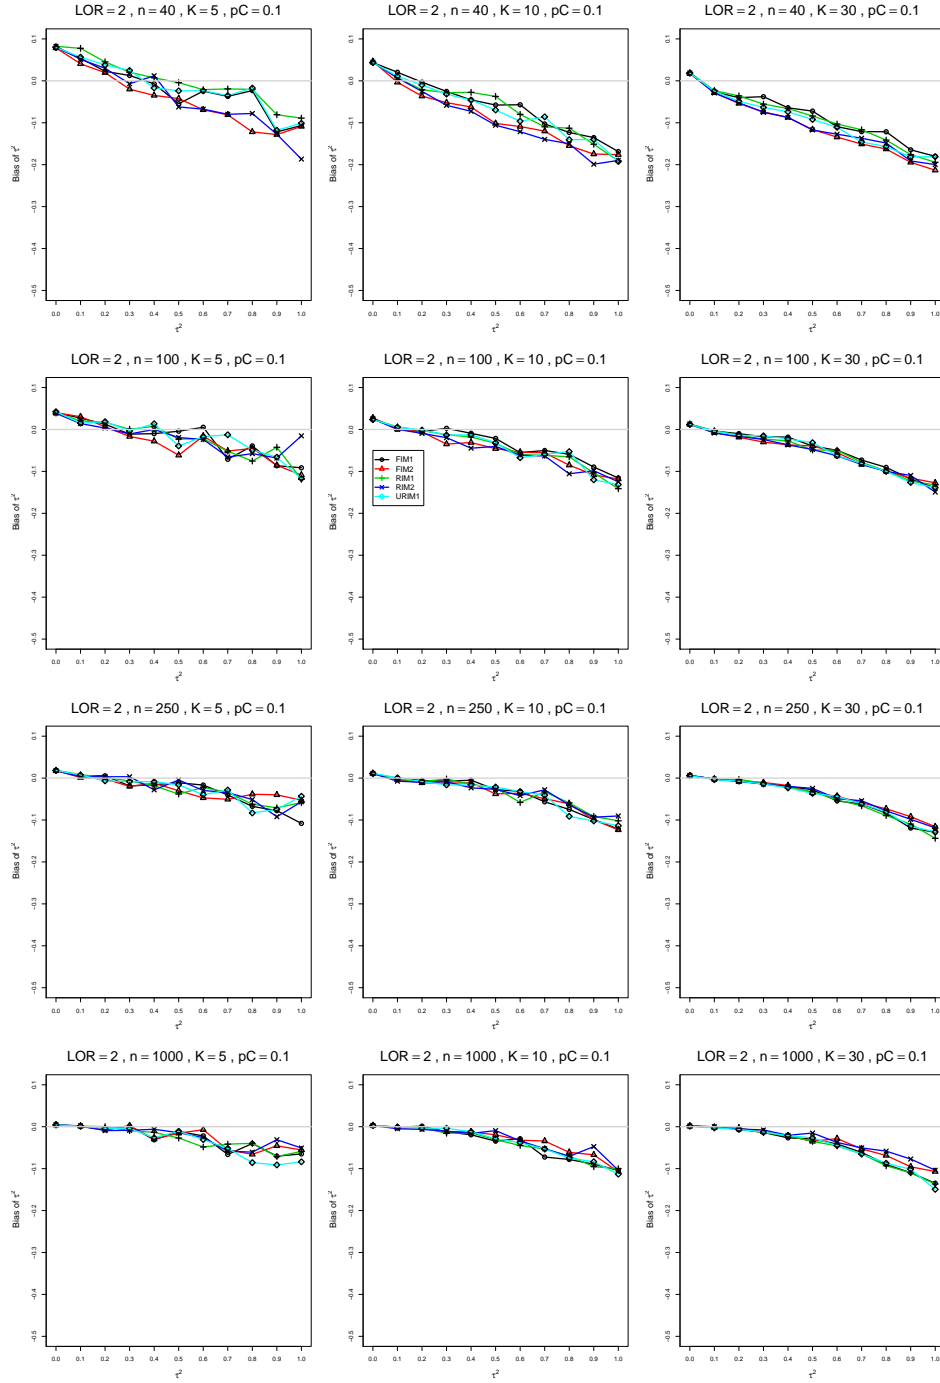

Figure A1.1.9: Bias of between-studies variance  $\hat{\tau}_{DL}^2$  for  $\theta = 2$ ,  $p_C = 0.1$ ,  $\sigma^2 = 0.1$ , constant sample sizes  $n = 40, 100, 250, 1000$ . The data-generation mechanisms are FIM1 ( $\circ$ ), FIM2 ( $\triangle$ ), RIM1 ( $+$ ), RIM2 ( $\times$ ), and URIM1 ( $\diamond$ ).



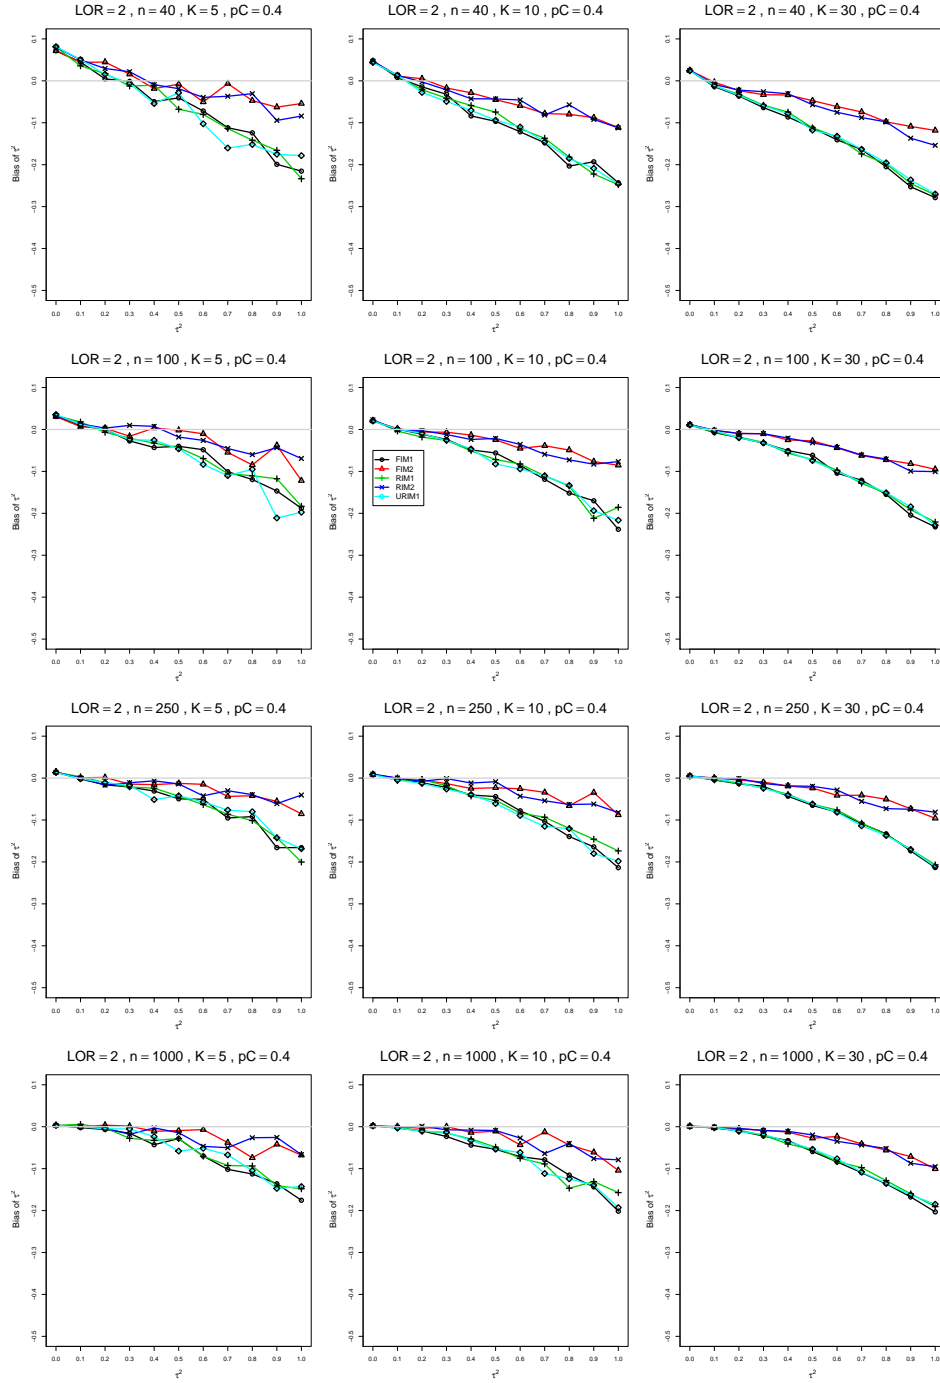

Figure A1.1.10: Bias of between-studies variance  $\hat{\tau}_{DL}^2$  for  $\theta = 2$ ,  $p_C = 0.4$ ,  $\sigma^2 = 0.1$ , constant sample sizes  $n = 40, 100, 250, 1000$ . The data-generation mechanisms are FIM1 ( $\circ$ ), FIM2 ( $\triangle$ ), RIM1 ( $+$ ), RIM2 ( $\times$ ), and URIM1 ( $\diamond$ ).

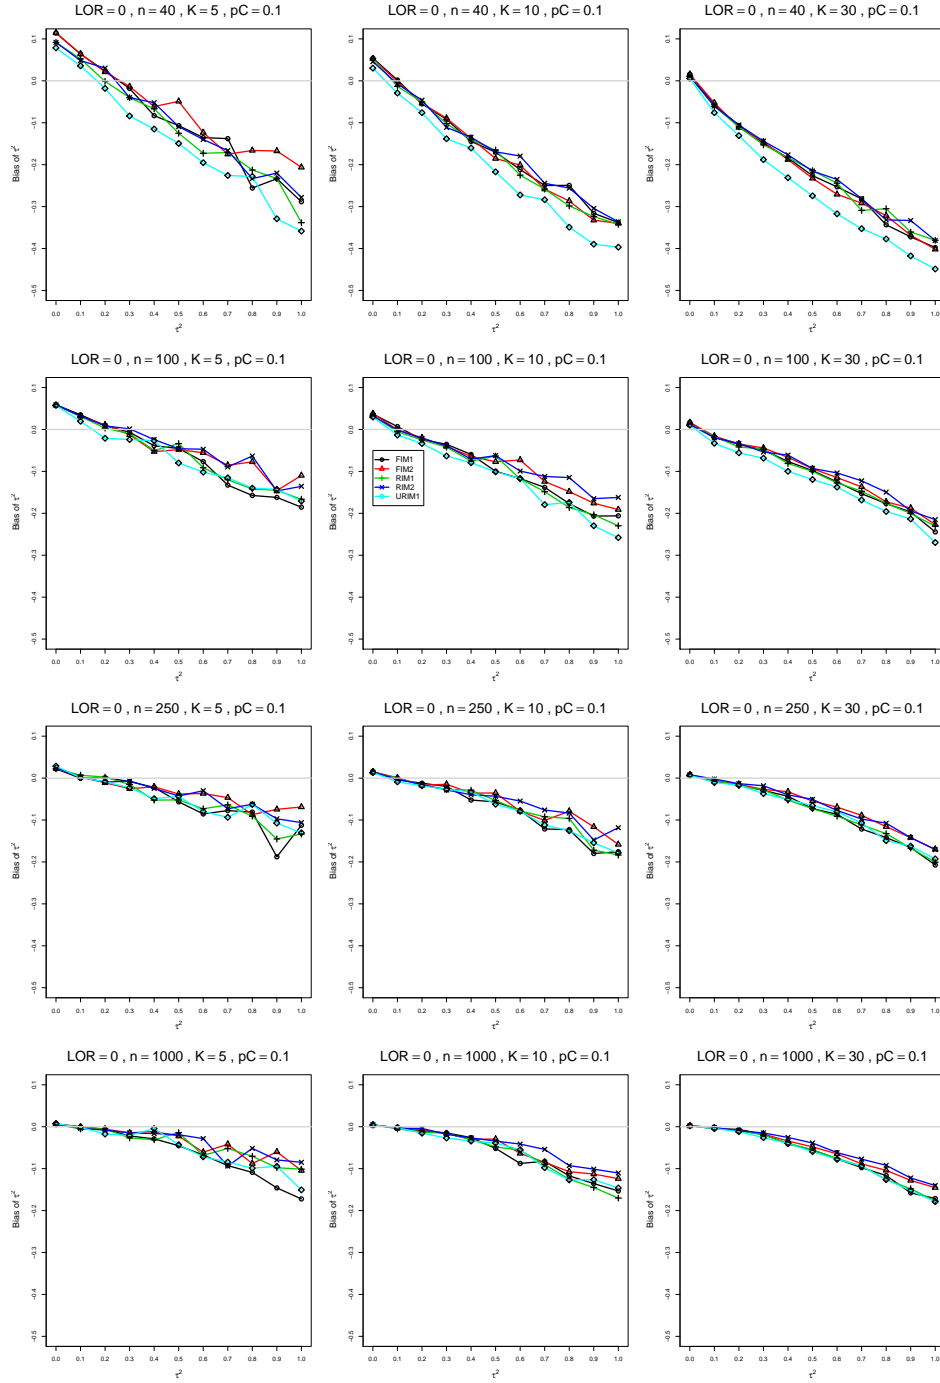

Figure A1.1.11: Bias of between-studies variance  $\hat{\tau}_{DL}^2$  for  $\theta = 0$ ,  $p_C = 0.1$ ,  $\sigma^2 = 0.4$ , constant sample sizes  $n = 40, 100, 250, 1000$ . The data-generation mechanisms are FIM1 ( $\circ$ ), FIM2 ( $\triangle$ ), RIM1 ( $+$ ), RIM2 ( $\times$ ), and URIM1 ( $\diamond$ ).

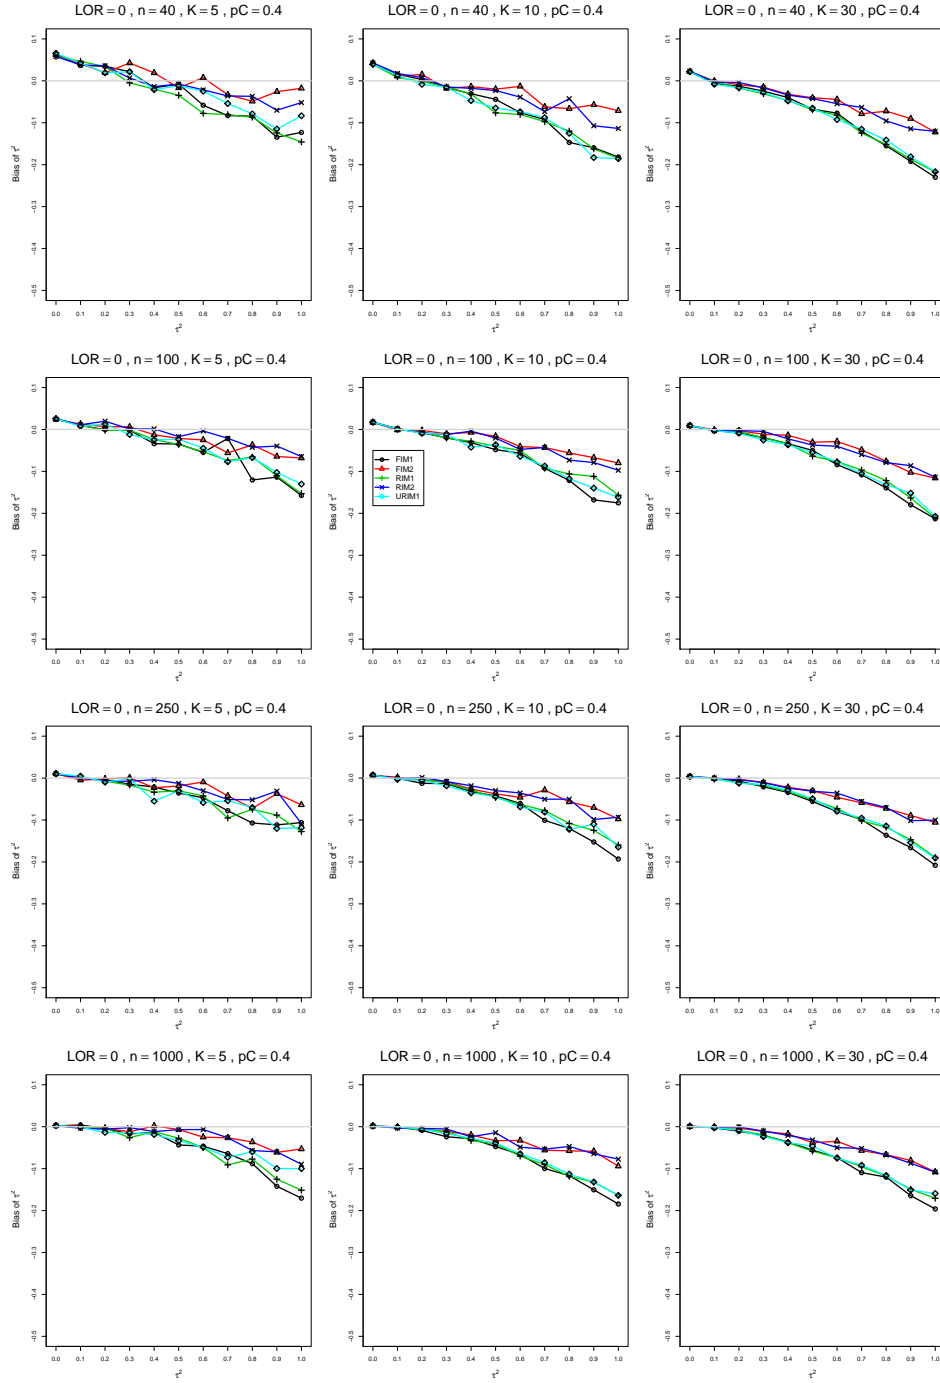

Figure A1.1.12: Bias of between-studies variance  $\hat{\tau}_{DL}^2$  for  $\theta = 0$ ,  $p_C = 0.4$ ,  $\sigma^2 = 0.4$ , constant sample sizes  $n = 40, 100, 250, 1000$ . The data-generation mechanisms are FIM1 ( $\circ$ ), FIM2 ( $\triangle$ ), RIM1 ( $+$ ), RIM2 ( $\times$ ), and URIM1 ( $\diamond$ ).

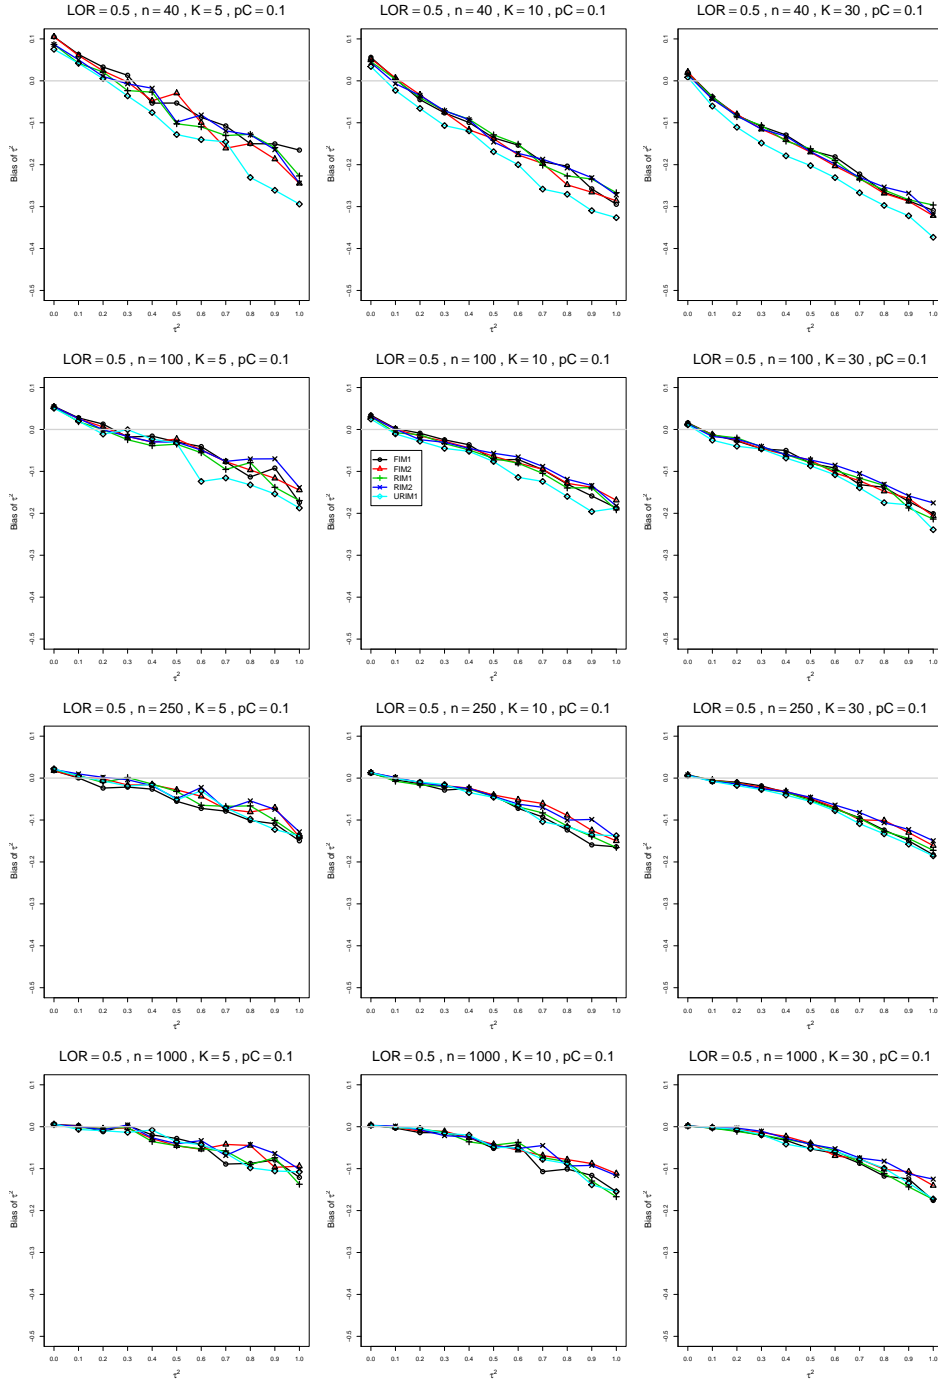

Figure A1.1.13: Bias of between-studies variance  $\hat{\tau}_{DL}^2$  for  $\theta = 0.5$ ,  $p_C = 0.1$ ,  $\sigma^2 = 0.4$ , constant sample sizes  $n = 40, 100, 250, 1000$ . The data-generation mechanisms are FIM1 ( $\circ$ ), FIM2 ( $\triangle$ ), RIM1 ( $+$ ), RIM2 ( $\times$ ), and URIM1 ( $\diamond$ ).

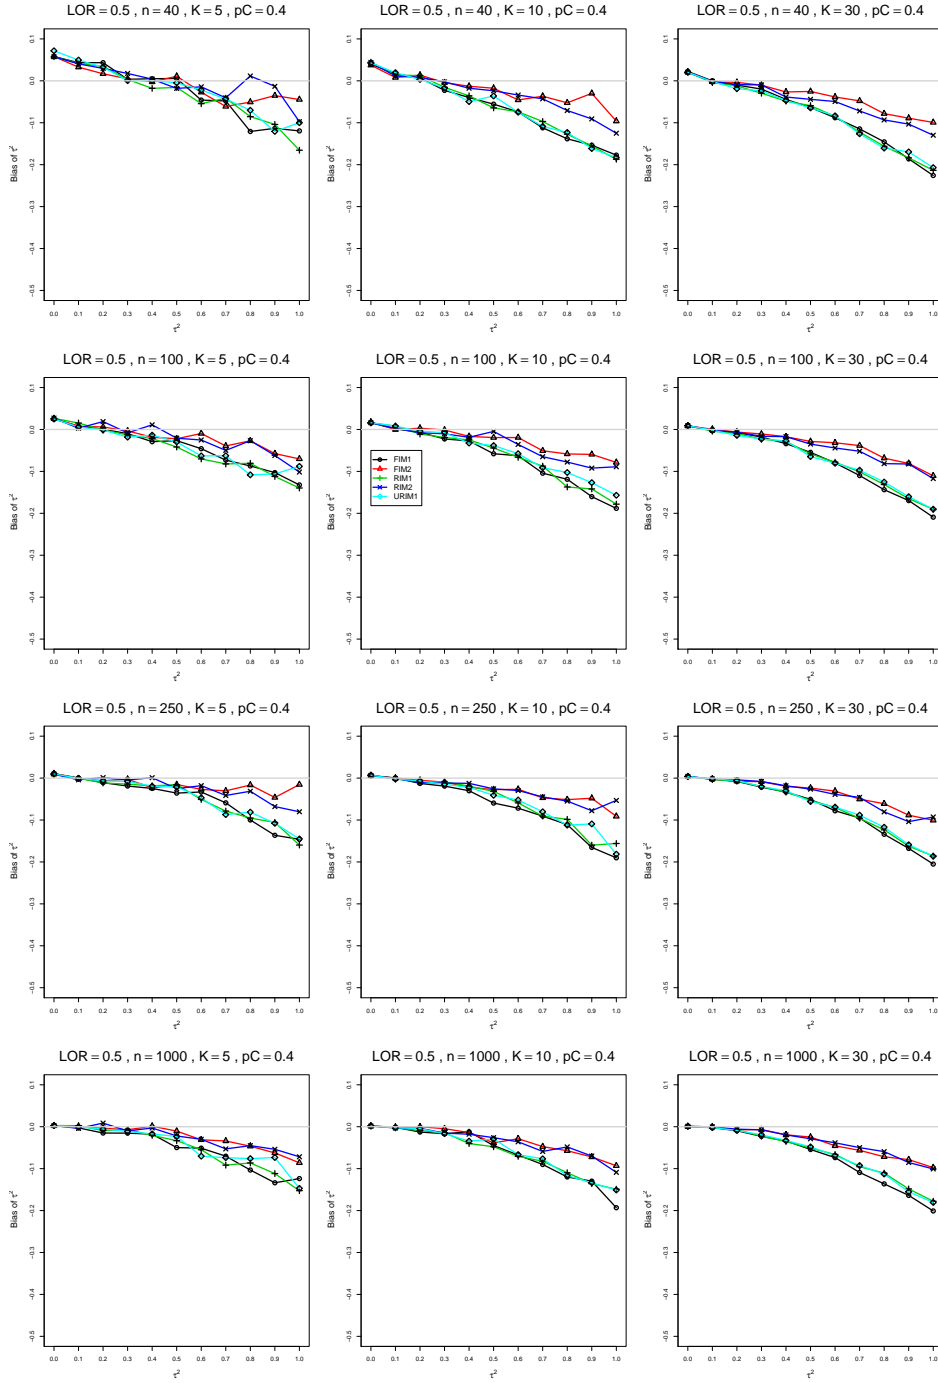

Figure A1.1.14: Bias of between-studies variance  $\hat{\tau}_{DL}^2$  for  $\theta = 0.5$ ,  $p_C = 0.4$ ,  $\sigma^2 = 0.4$ , constant sample sizes  $n = 40, 100, 250, 1000$ . The data-generation mechanisms are FIM1 ( $\circ$ ), FIM2 ( $\triangle$ ), RIM1 ( $+$ ), RIM2 ( $\times$ ), and URIM1 ( $\diamond$ ).

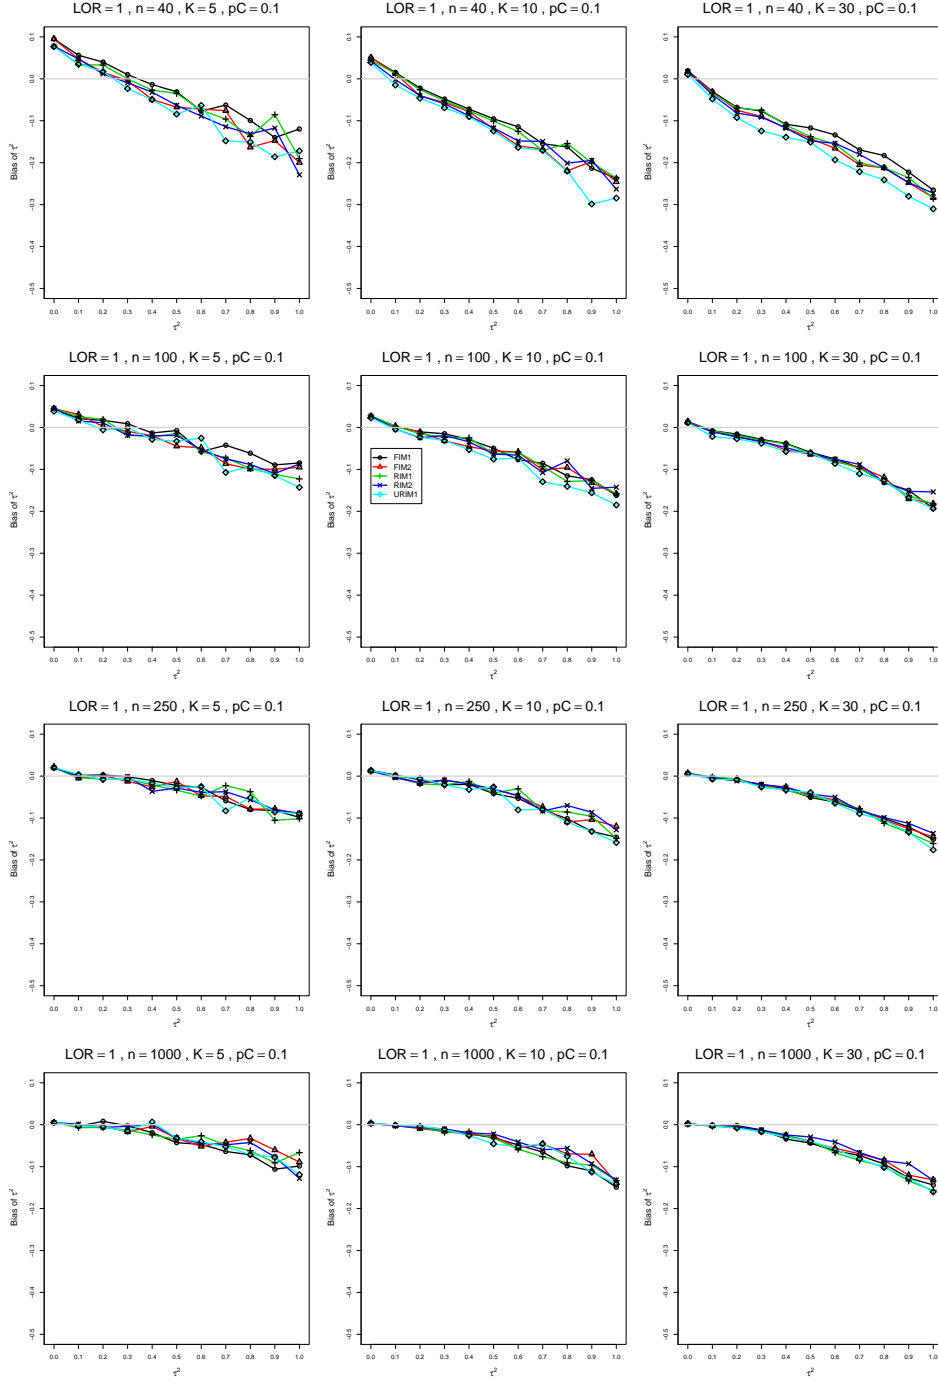

Figure A1.1.15: Bias of between-studies variance  $\hat{\tau}_{DL}^2$  for  $\theta = 1$ ,  $p_C = 0.1$ ,  $\sigma^2 = 0.4$ , constant sample sizes  $n = 40, 100, 250, 1000$ . The data-generation mechanisms are FIM1 ( $\circ$ ), FIM2 ( $\triangle$ ), RIM1 ( $+$ ), RIM2 ( $\times$ ), and URIM1 ( $\diamond$ ).

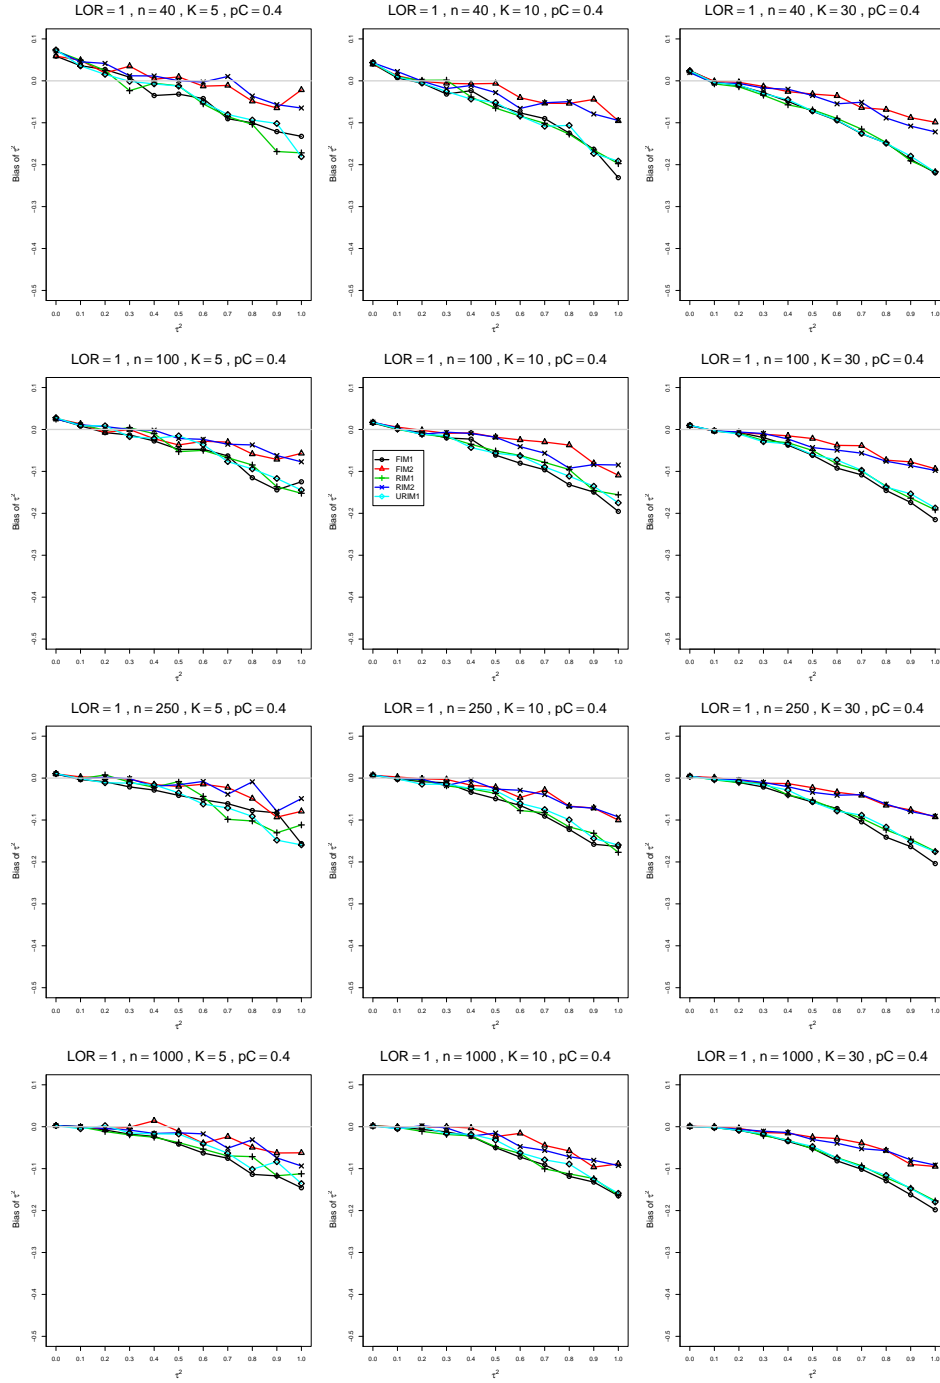

Figure A1.1.16: Bias of between-studies variance  $\hat{\tau}_{DL}^2$  for  $\theta = 1$ ,  $p_C = 0.4$ ,  $\sigma^2 = 0.4$ , constant sample sizes  $n = 40, 100, 250, 1000$ . The data-generation mechanisms are FIM1 ( $\circ$ ), FIM2 ( $\triangle$ ), RIM1 ( $+$ ), RIM2 ( $\times$ ), and URIM1 ( $\diamond$ ).

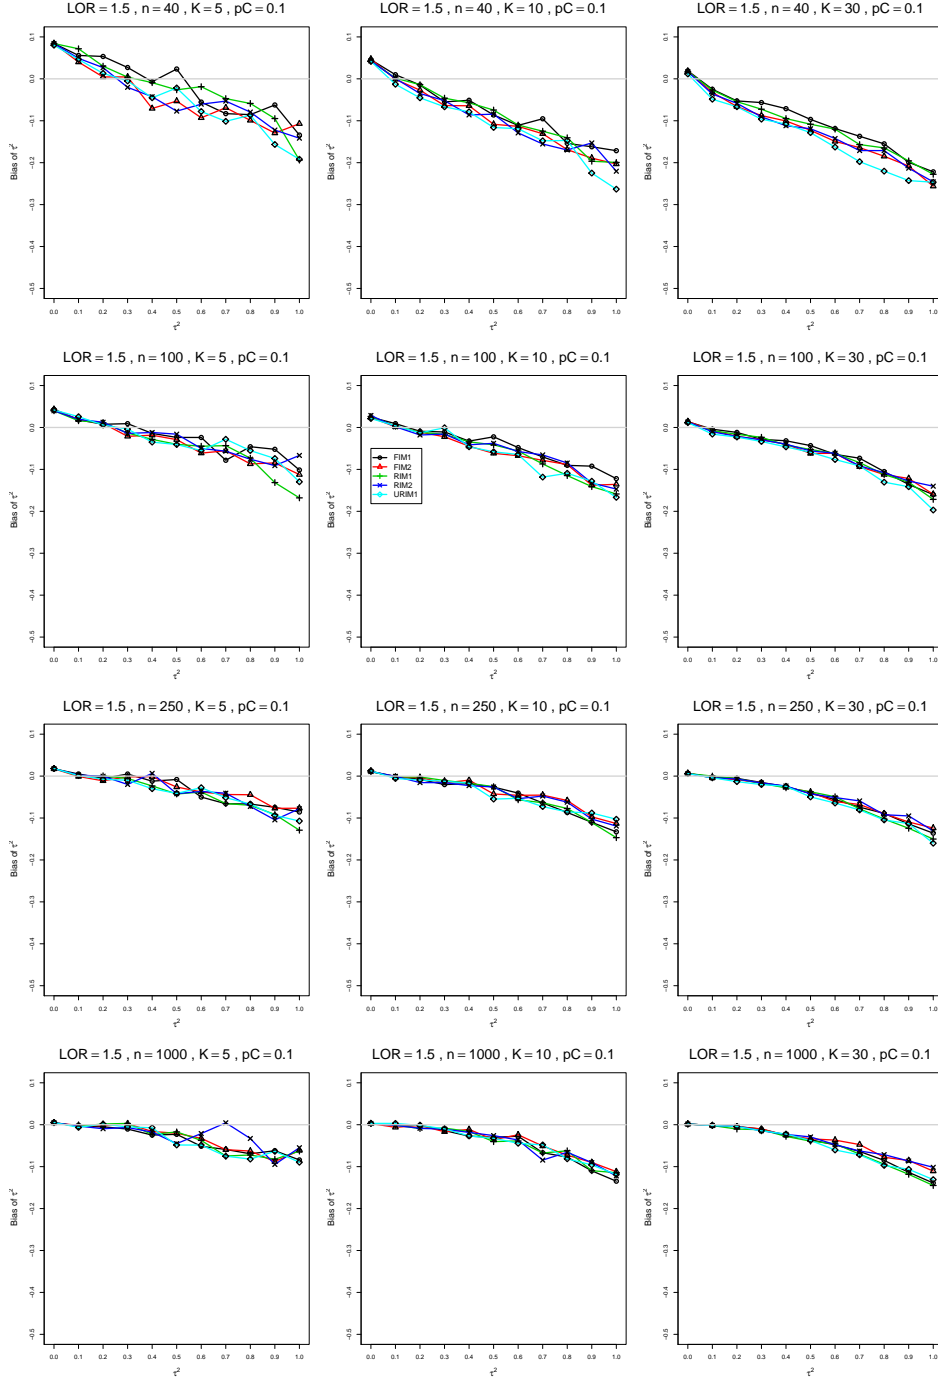

Figure A1.1.17: Bias of between-studies variance  $\hat{\tau}_{DL}^2$  for  $\theta = 1.5$ ,  $p_C = 0.1$ ,  $\sigma^2 = 0.4$ , constant sample sizes  $n = 40, 100, 250, 1000$ . The data-generation mechanisms are FIM1 ( $\circ$ ), FIM2 ( $\triangle$ ), RIM1 ( $+$ ), RIM2 ( $\times$ ), and URIM1 ( $\diamond$ ).



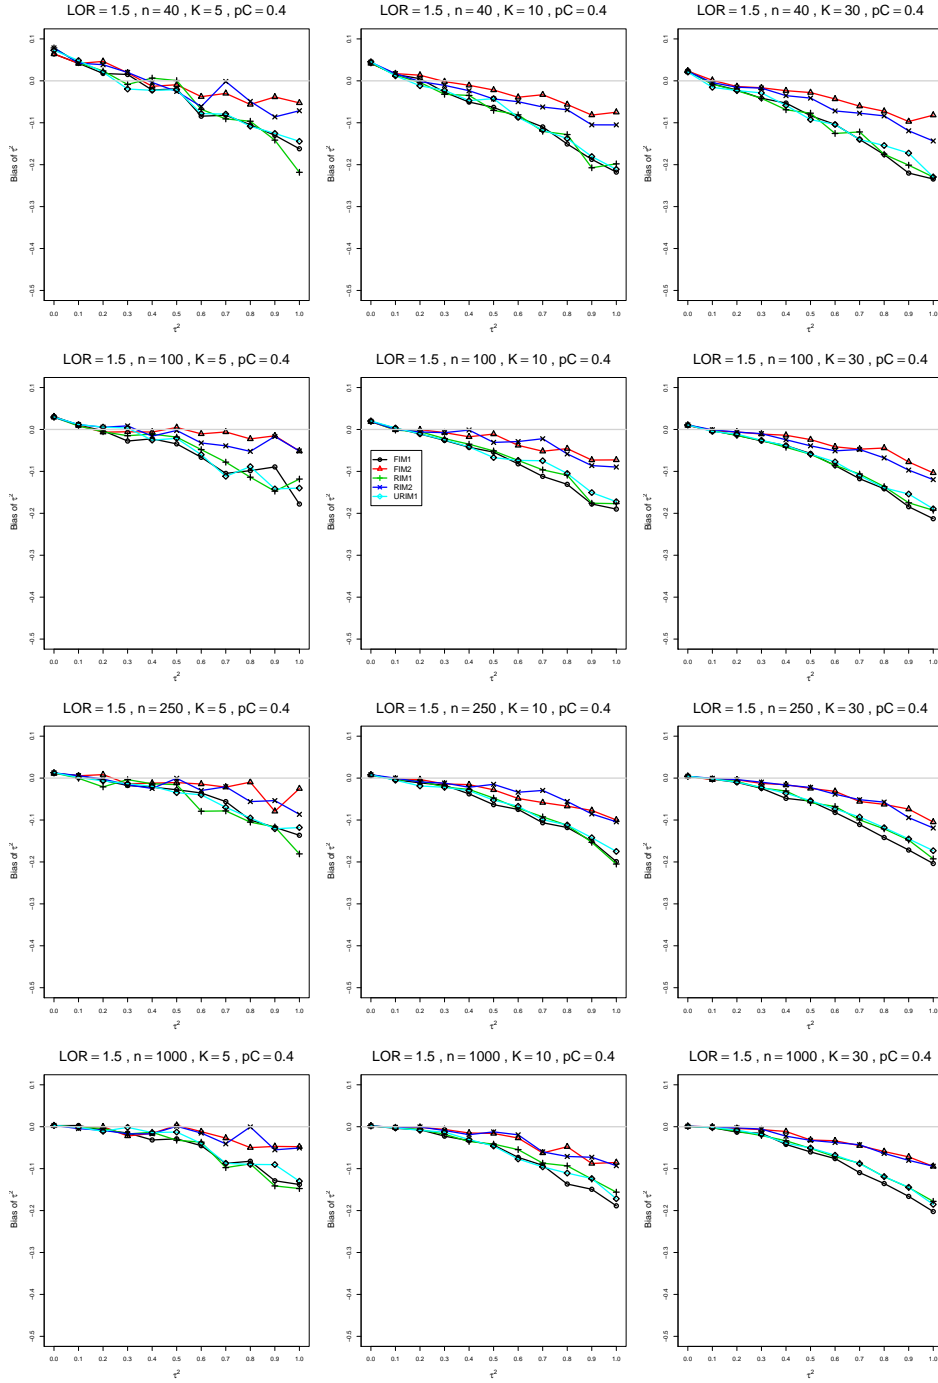

Figure A1.1.18: Bias of between-studies variance  $\hat{\tau}_{DL}^2$  for  $\theta = 1.5$ ,  $p_C = 0.4$ ,  $\sigma^2 = 0.4$ , constant sample sizes  $n = 40, 100, 250, 1000$ . The data-generation mechanisms are FIM1 ( $\circ$ ), FIM2 ( $\triangle$ ), RIM1 ( $+$ ), RIM2 ( $\times$ ), and URIM1 ( $\diamond$ ).

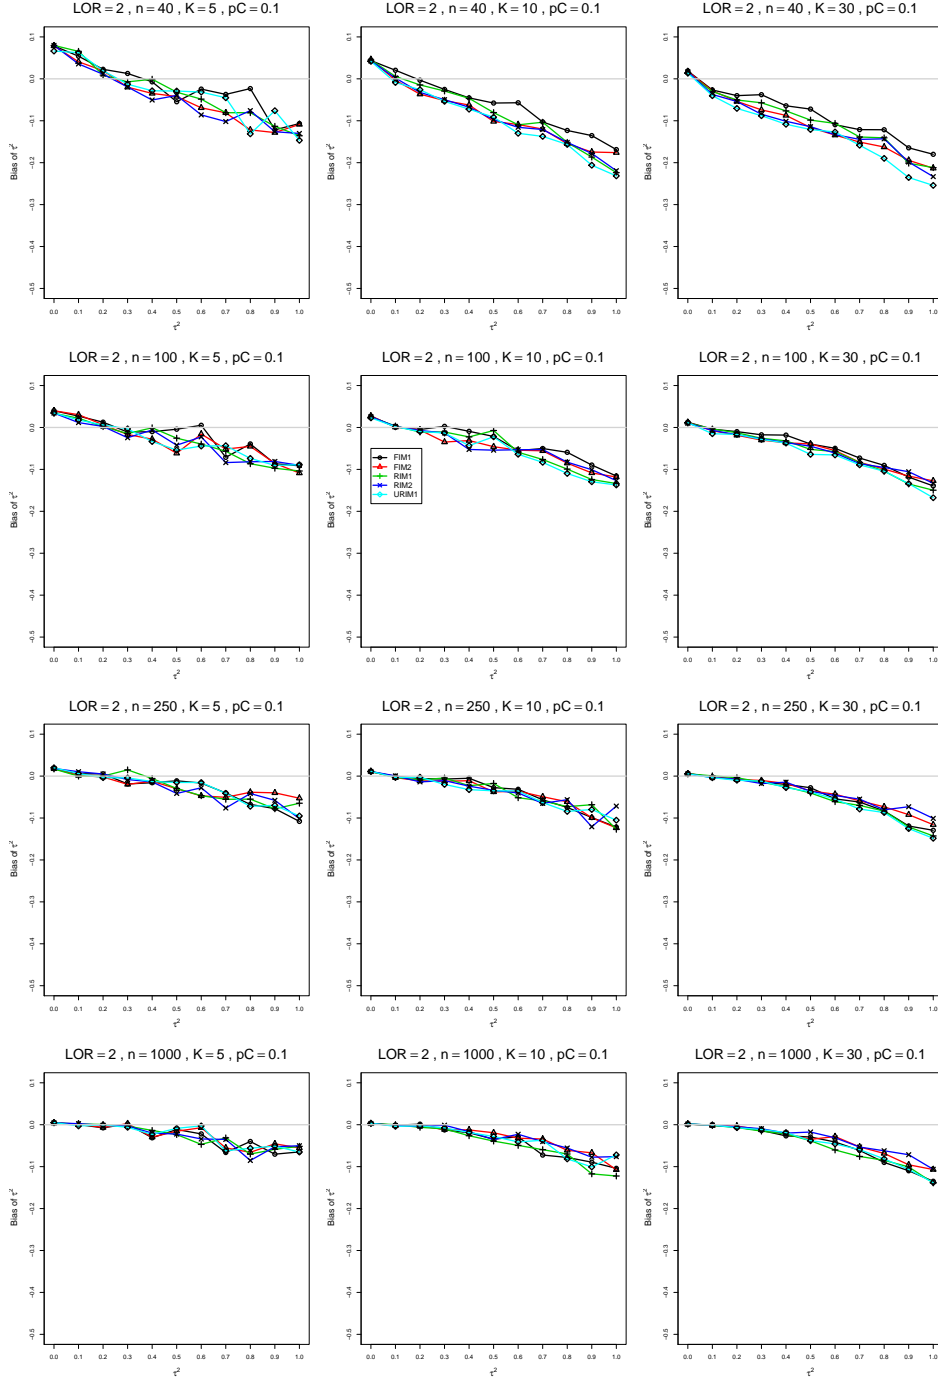

Figure A1.1.19: Bias of between-studies variance  $\hat{\tau}_{DL}^2$  for  $\theta = 2$ ,  $p_C = 0.1$ ,  $\sigma^2 = 0.4$ , constant sample sizes  $n = 40, 100, 250, 1000$ . The data-generation mechanisms are FIM1 ( $\circ$ ), FIM2 ( $\triangle$ ), RIM1 ( $+$ ), RIM2 ( $\times$ ), and URIM1 ( $\diamond$ ).

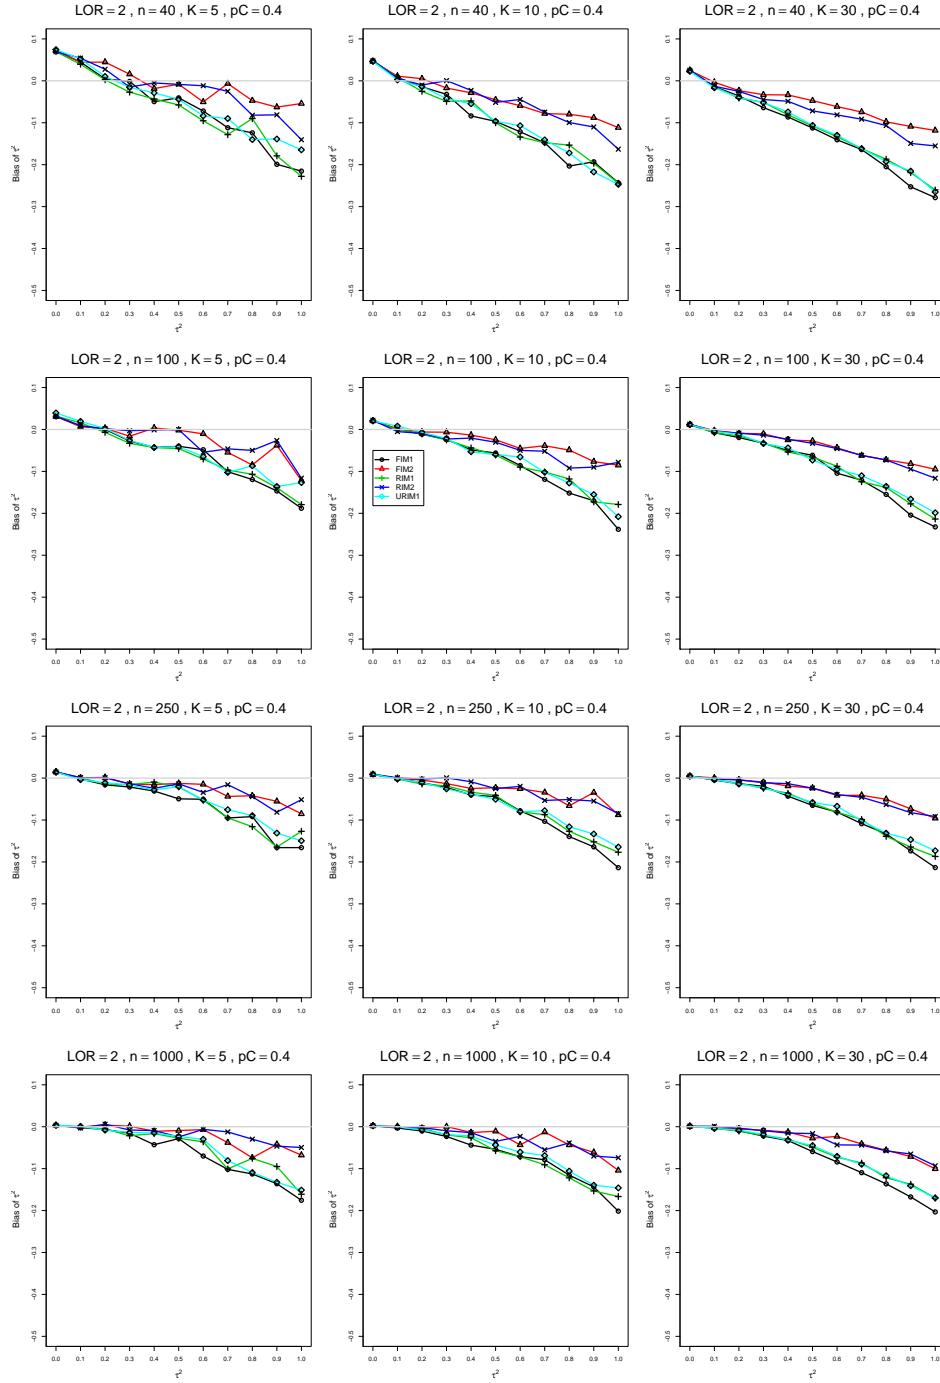

Figure A1.1.20: Bias of between-studies variance  $\hat{\tau}_{DL}^2$  for  $\theta = 2$ ,  $p_C = 0.4$ ,  $\sigma^2 = 0.4$ , constant sample sizes  $n = 40, 100, 250, 1000$ . The data-generation mechanisms are FIM1 ( $\circ$ ), FIM2 ( $\triangle$ ), RIM1 ( $+$ ), RIM2 ( $\times$ ), and URIM1 ( $\diamond$ ).

## A1.2 Bias of $\hat{\tau}_{REML}^2$

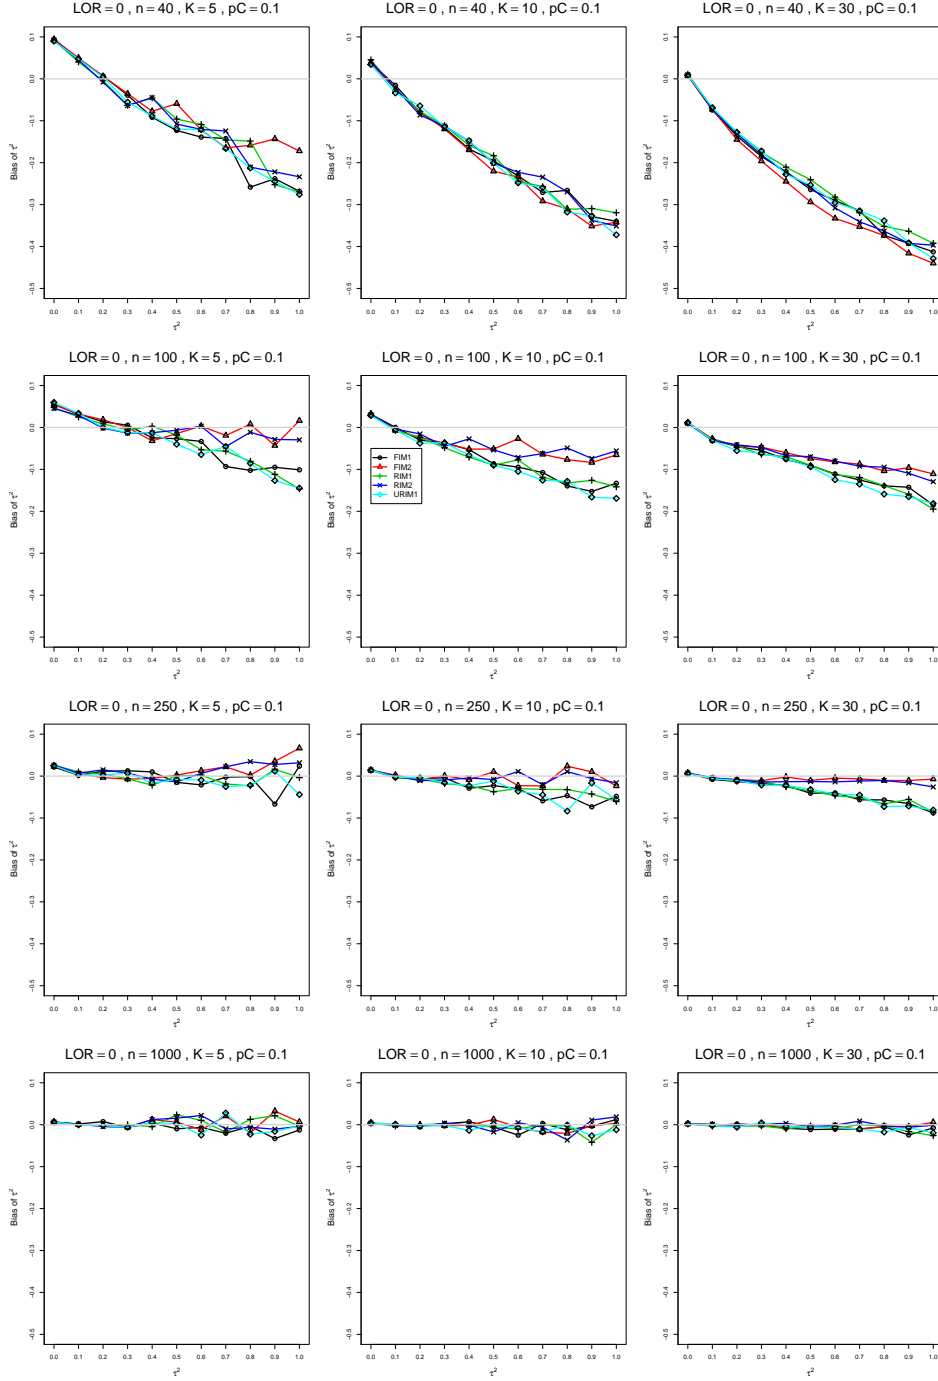

Figure A1.2.1: Bias of between-studies variance  $\hat{\tau}_{REML}^2$  for  $\theta = 0$ ,  $p_C = 0.1$ ,  $\sigma^2 = 0.1$ , constant sample sizes  $n = 40, 100, 250, 1000$ . The data-generation mechanisms are FIM1 ( $\circ$ ), FIM2 ( $\triangle$ ), RIM1 ( $+$ ), RIM2 ( $\times$ ), and URIM1 ( $\diamond$ ).

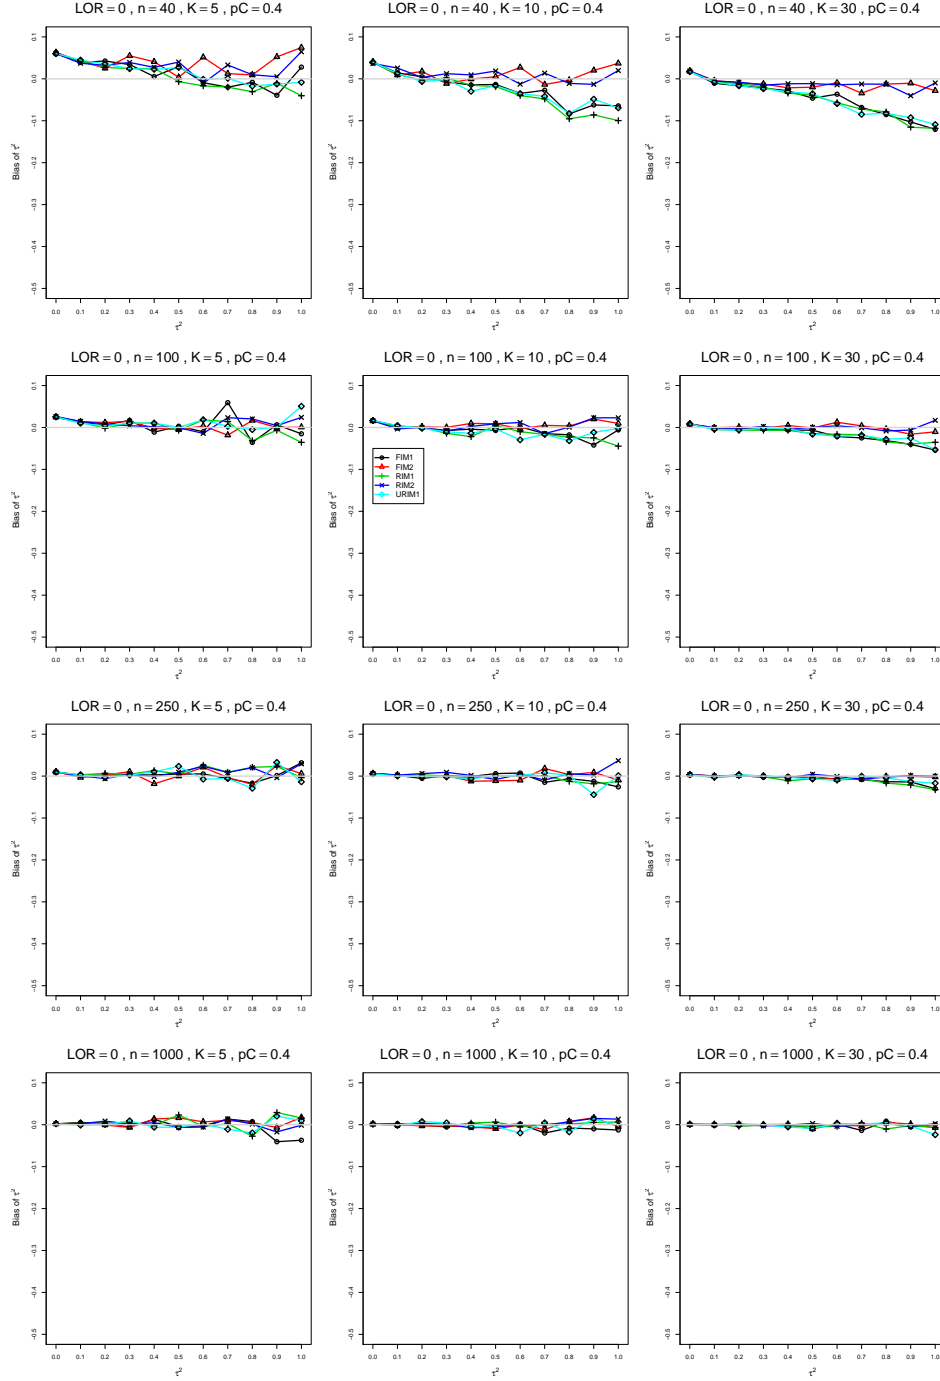

Figure A1.2.2: Bias of between-studies variance  $\hat{\tau}_{REML}^2$  for  $\theta = 0$ ,  $p_C = 0.4$ ,  $\sigma^2 = 0.1$ , constant sample sizes  $n = 40, 100, 250, 1000$ . The data-generation mechanisms are FIM1 ( $\circ$ ), FIM2 ( $\triangle$ ), RIM1 ( $+$ ), RIM2 ( $\times$ ), and URIM1 ( $\diamond$ ).

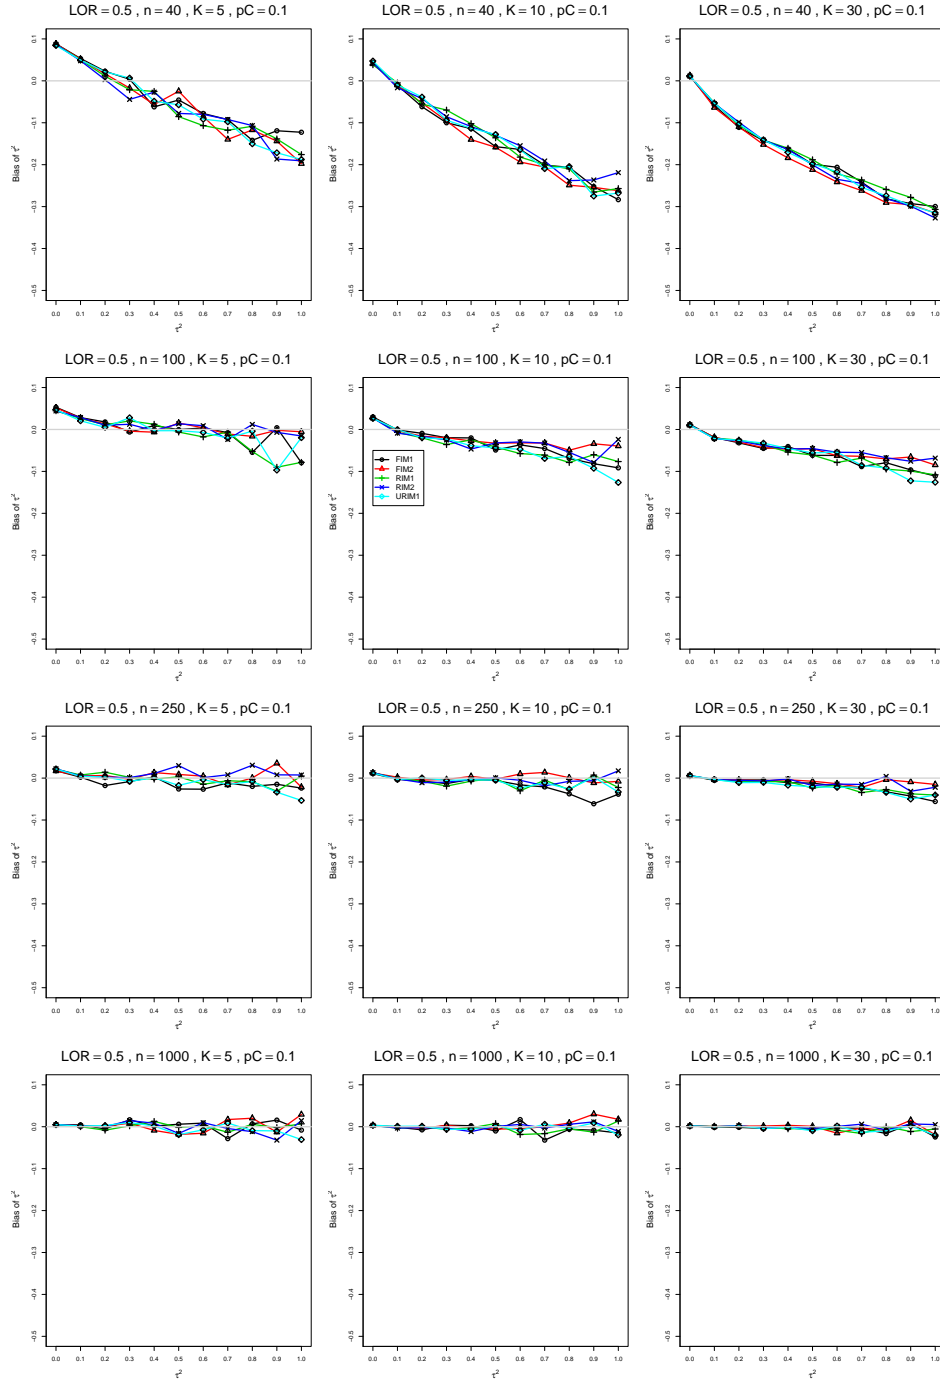

Figure A1.2.3: Bias of between-studies variance  $\hat{\tau}_{REML}^2$  for  $\theta = 0.5$ ,  $p_C = 0.1$ ,  $\sigma^2 = 0.1$ , constant sample sizes  $n = 40, 100, 250, 1000$ . The data-generation mechanisms are FIM1 ( $\circ$ ), FIM2 ( $\triangle$ ), RIM1 ( $+$ ), RIM2 ( $\times$ ), and URIM1 ( $\diamond$ ).

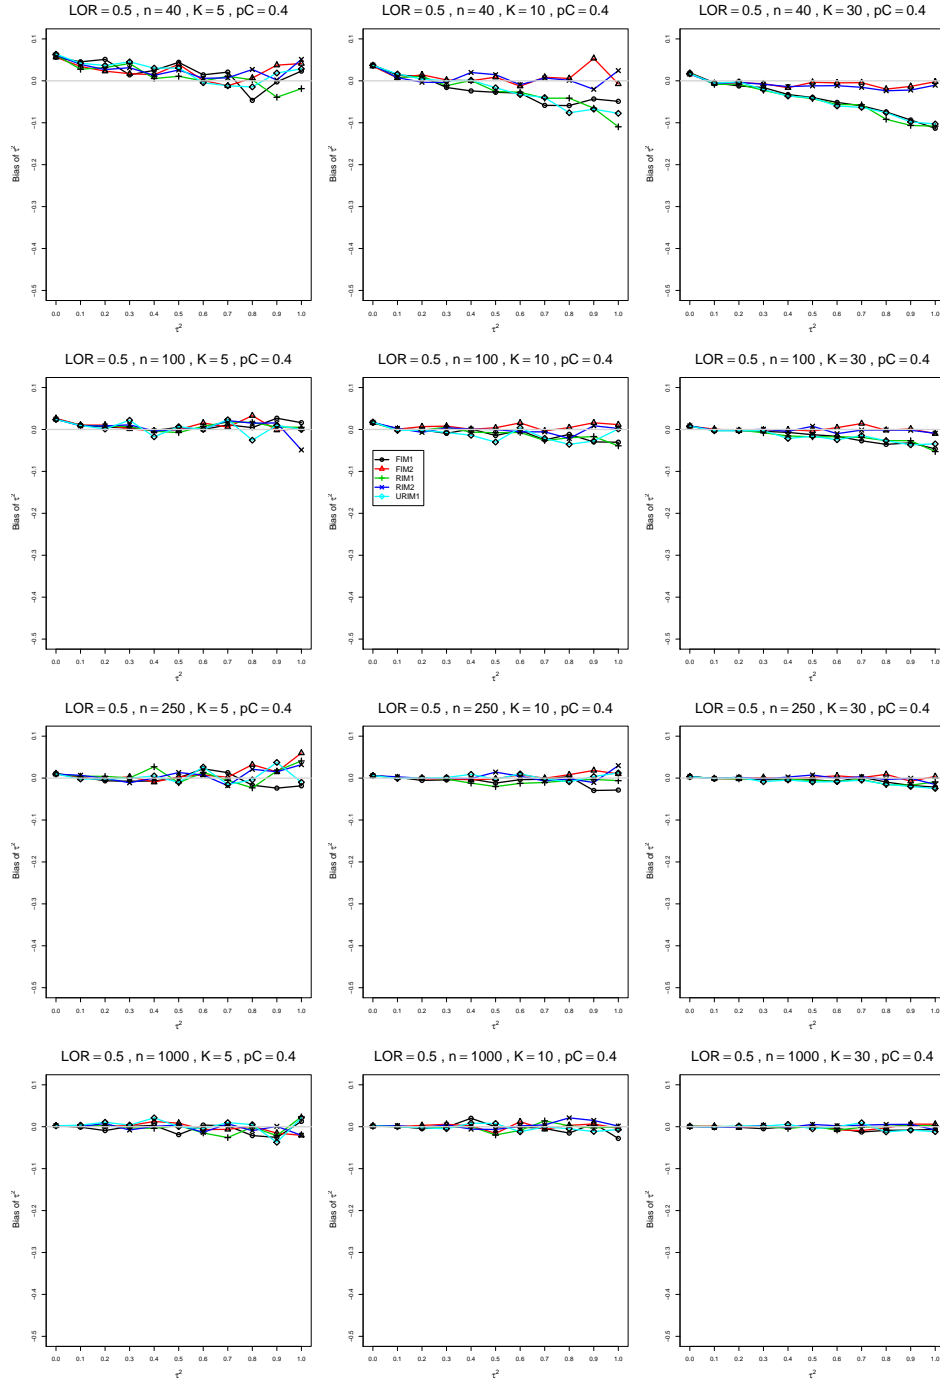

Figure A1.2.4: Bias of between-studies variance  $\hat{\tau}_{REML}^2$  for  $\theta = 0.5$ ,  $p_C = 0.4$ ,  $\sigma^2 = 0.1$ , constant sample sizes  $n = 40, 100, 250, 1000$ . The data-generation mechanisms are FIM1 ( $\circ$ ), FIM2 ( $\triangle$ ), RIM1 ( $+$ ), RIM2 ( $\times$ ), and URIM1 ( $\diamond$ ).



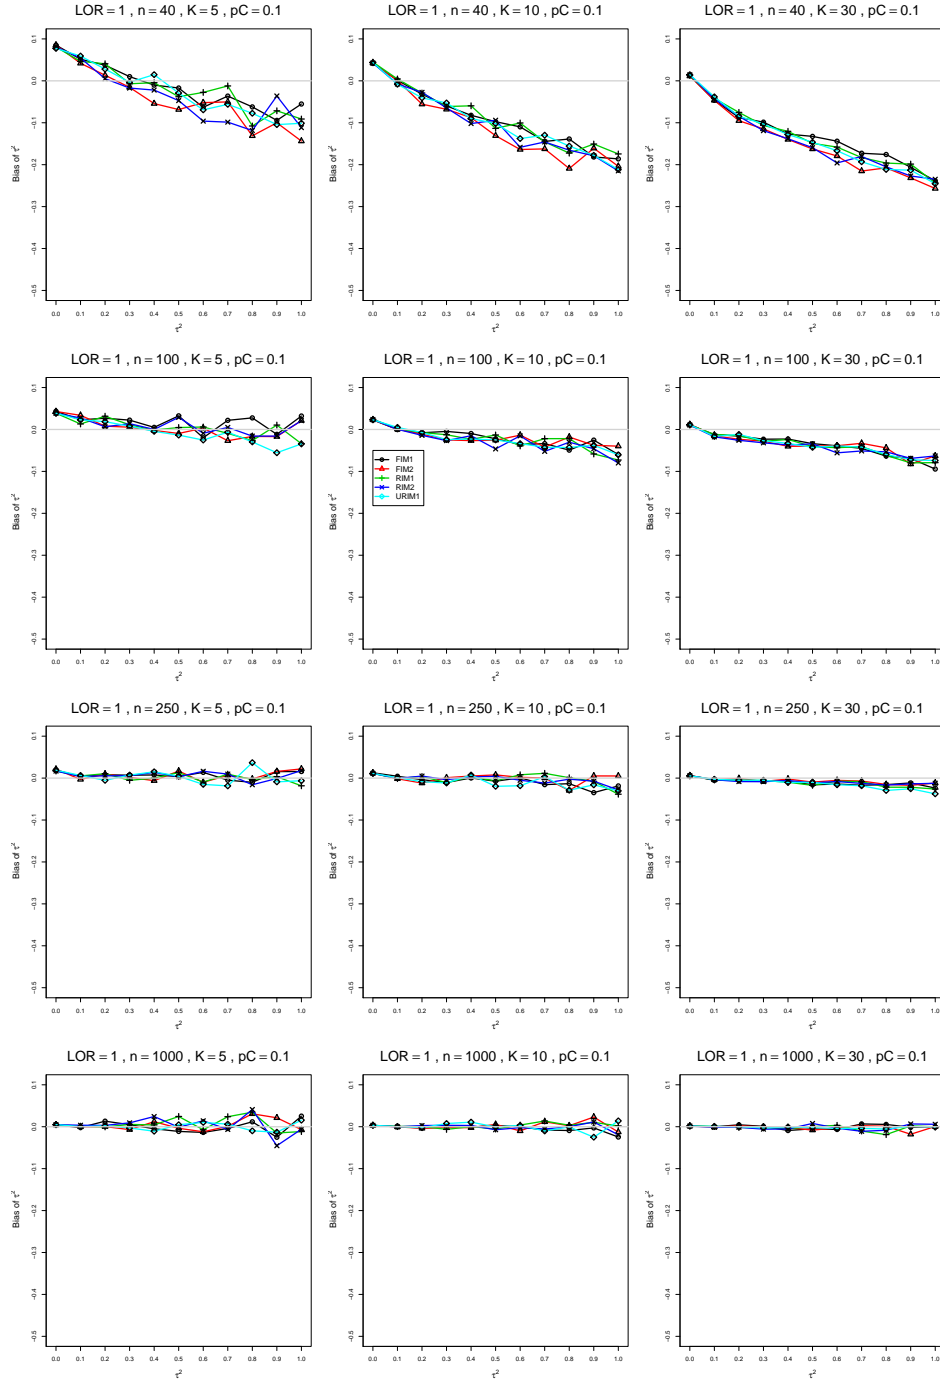

Figure A1.2.5: Bias of between-studies variance  $\hat{\tau}_{REML}^2$  for  $\theta = 1$ ,  $p_C = 0.1$ ,  $\sigma^2 = 0.1$ , constant sample sizes  $n = 40, 100, 250, 1000$ . The data-generation mechanisms are FIM1 ( $\circ$ ), FIM2 ( $\triangle$ ), RIM1 ( $+$ ), RIM2 ( $\times$ ), and URIM1 ( $\diamond$ ).

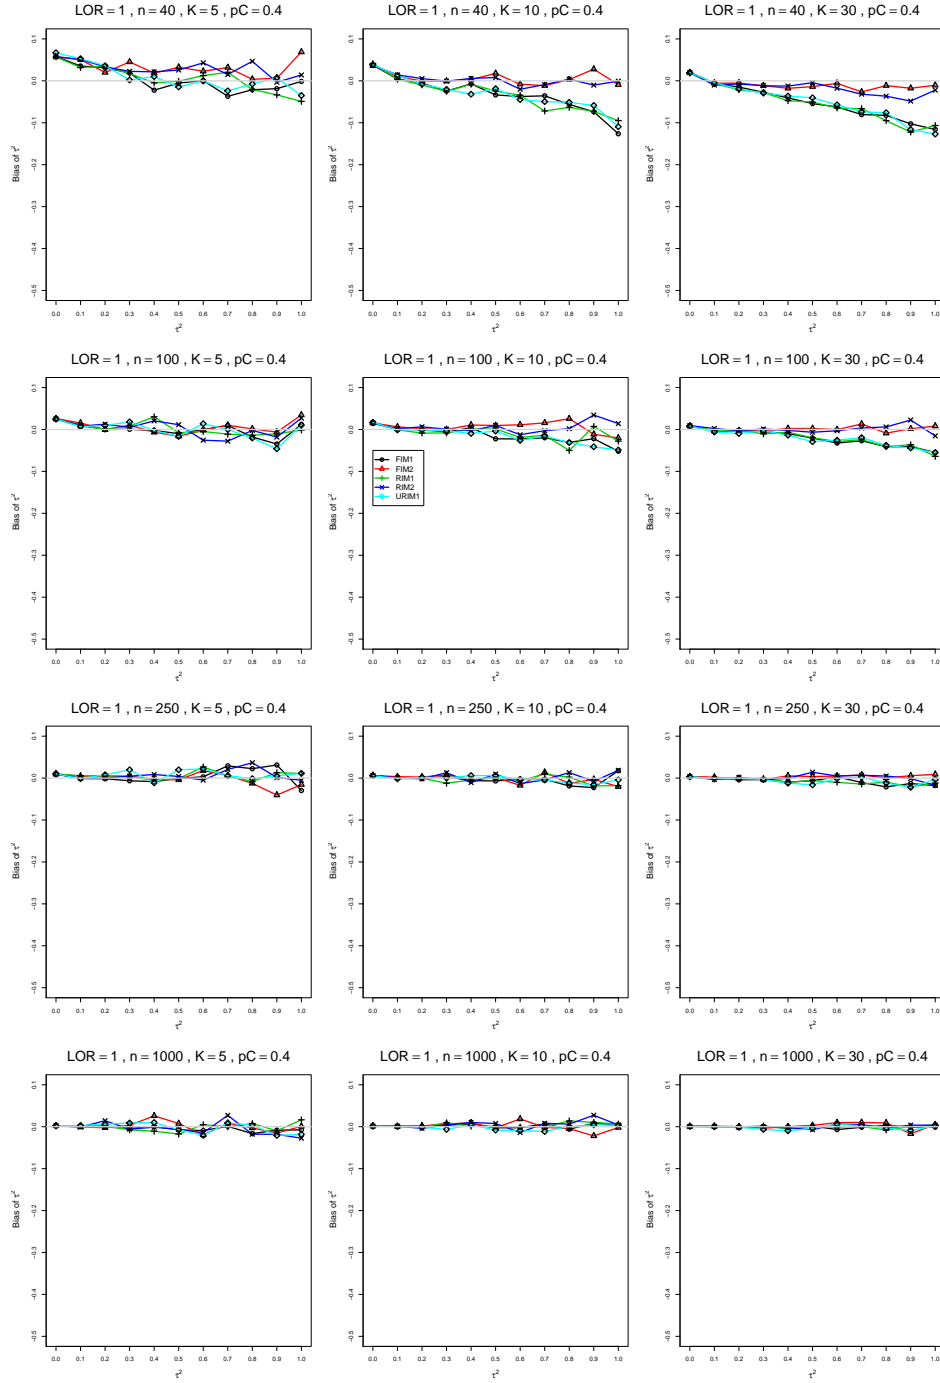

Figure A1.2.6: Bias of between-studies variance  $\hat{\tau}_{REML}^2$  for  $\theta = 1$ ,  $p_C = 0.4$ ,  $\sigma^2 = 0.1$ , constant sample sizes  $n = 40, 100, 250, 1000$ . The data-generation mechanisms are FIM1 ( $\circ$ ), FIM2 ( $\triangle$ ), RIM1 ( $+$ ), RIM2 ( $\times$ ), and URIM1 ( $\diamond$ ).

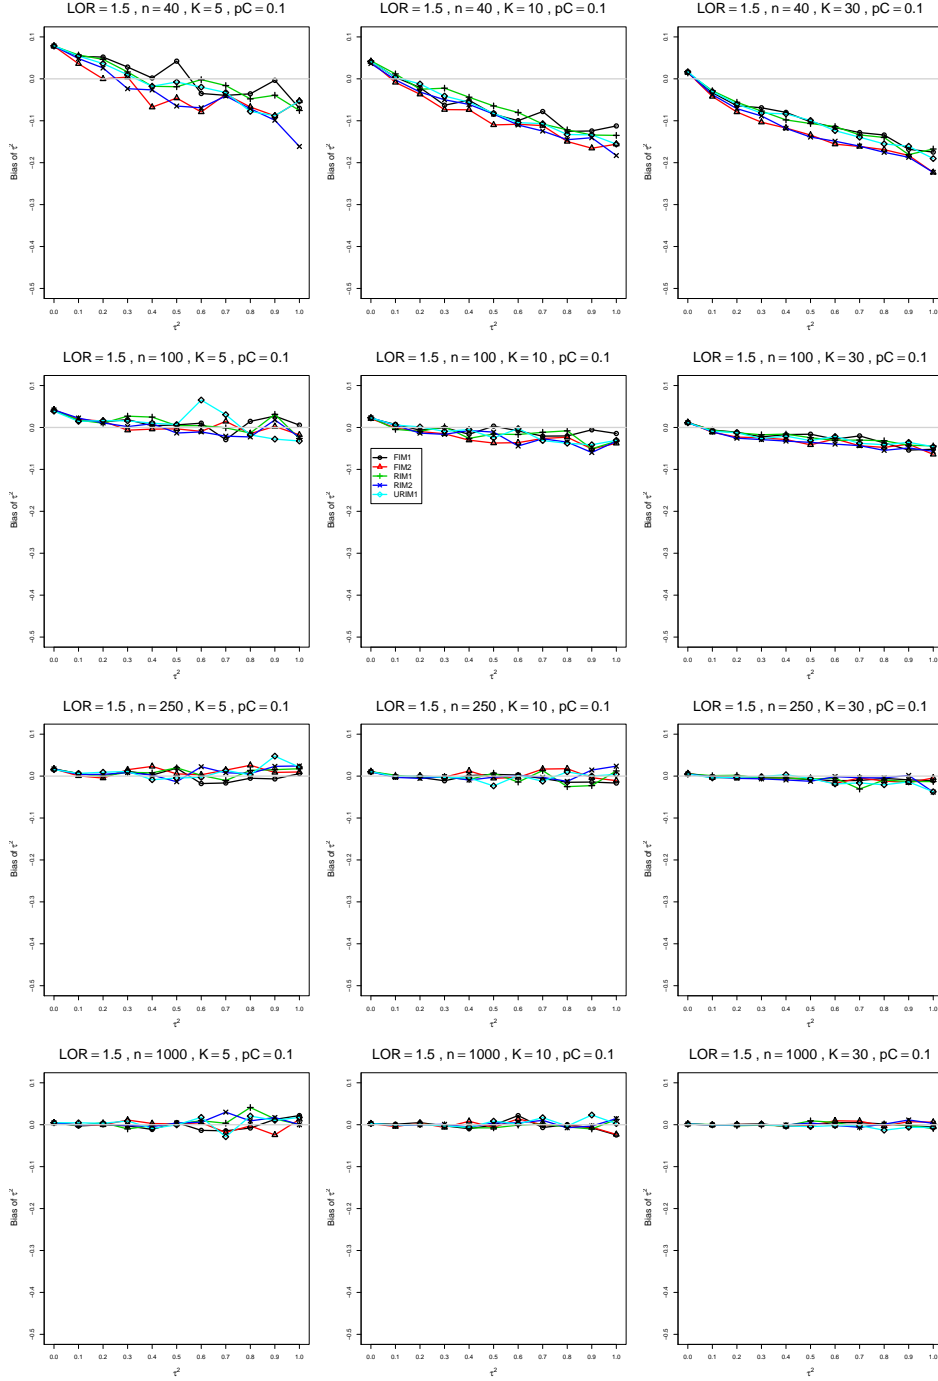

Figure A1.2.7: Bias of between-studies variance  $\hat{\tau}_{REML}^2$  for  $\theta = 1.5$ ,  $p_C = 0.1$ ,  $\sigma^2 = 0.1$ , constant sample sizes  $n = 40, 100, 250, 1000$ . The data-generation mechanisms are FIM1 ( $\circ$ ), FIM2 ( $\triangle$ ), RIM1 ( $+$ ), RIM2 ( $\times$ ), and URIM1 ( $\diamond$ ).

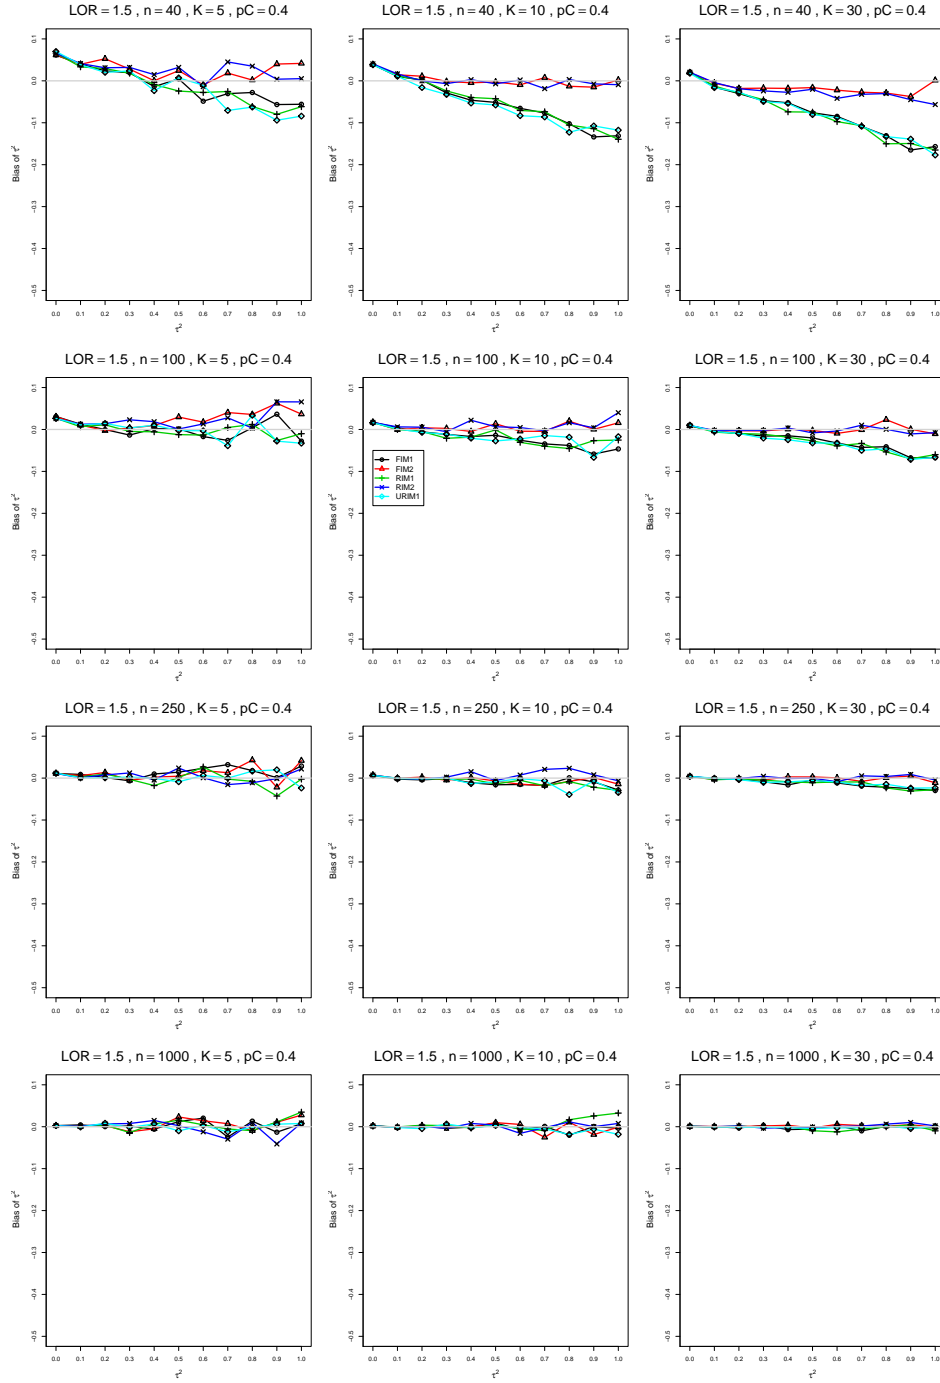

Figure A1.2.8: Bias of between-studies variance  $\hat{\tau}_{REML}^2$  for  $\theta = 1.5$ ,  $p_C = 0.4$ ,  $\sigma^2 = 0.1$ , constant sample sizes  $n = 40, 100, 250, 1000$ . The data-generation mechanisms are FIM1 ( $\circ$ ), FIM2 ( $\triangle$ ), RIM1 ( $+$ ), RIM2 ( $\times$ ), and URIM1 ( $\diamond$ ).

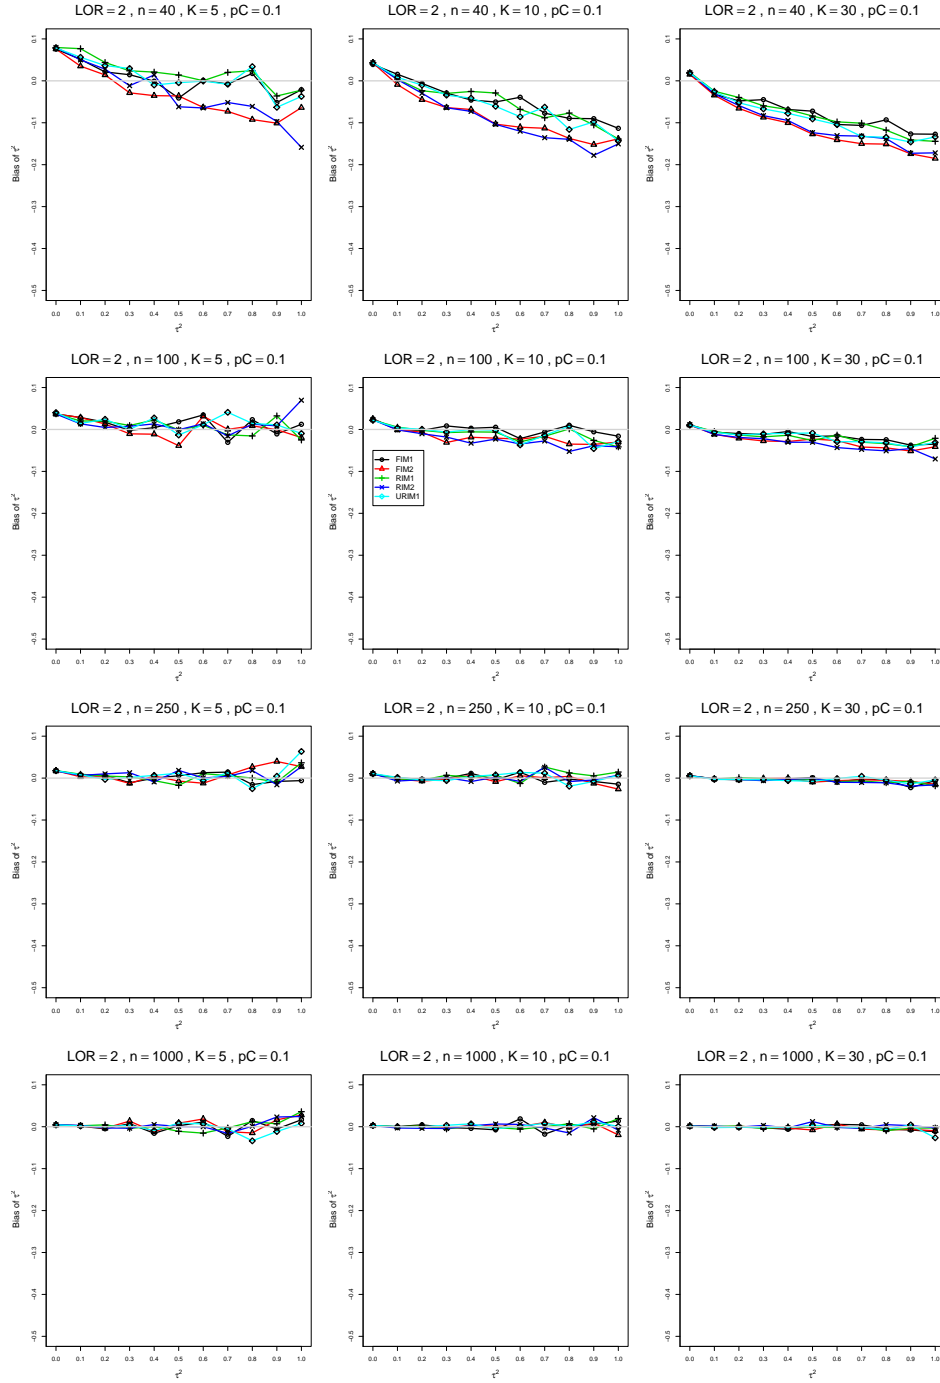

Figure A1.2.9: Bias of between-studies variance  $\hat{\tau}_{REML}^2$  for  $\theta = 2$ ,  $p_C = 0.1$ ,  $\sigma^2 = 0.1$ , constant sample sizes  $n = 40, 100, 250, 1000$ . The data-generation mechanisms are FIM1 ( $\circ$ ), FIM2 ( $\triangle$ ), RIM1 ( $+$ ), RIM2 ( $\times$ ), and URIM1 ( $\diamond$ ).

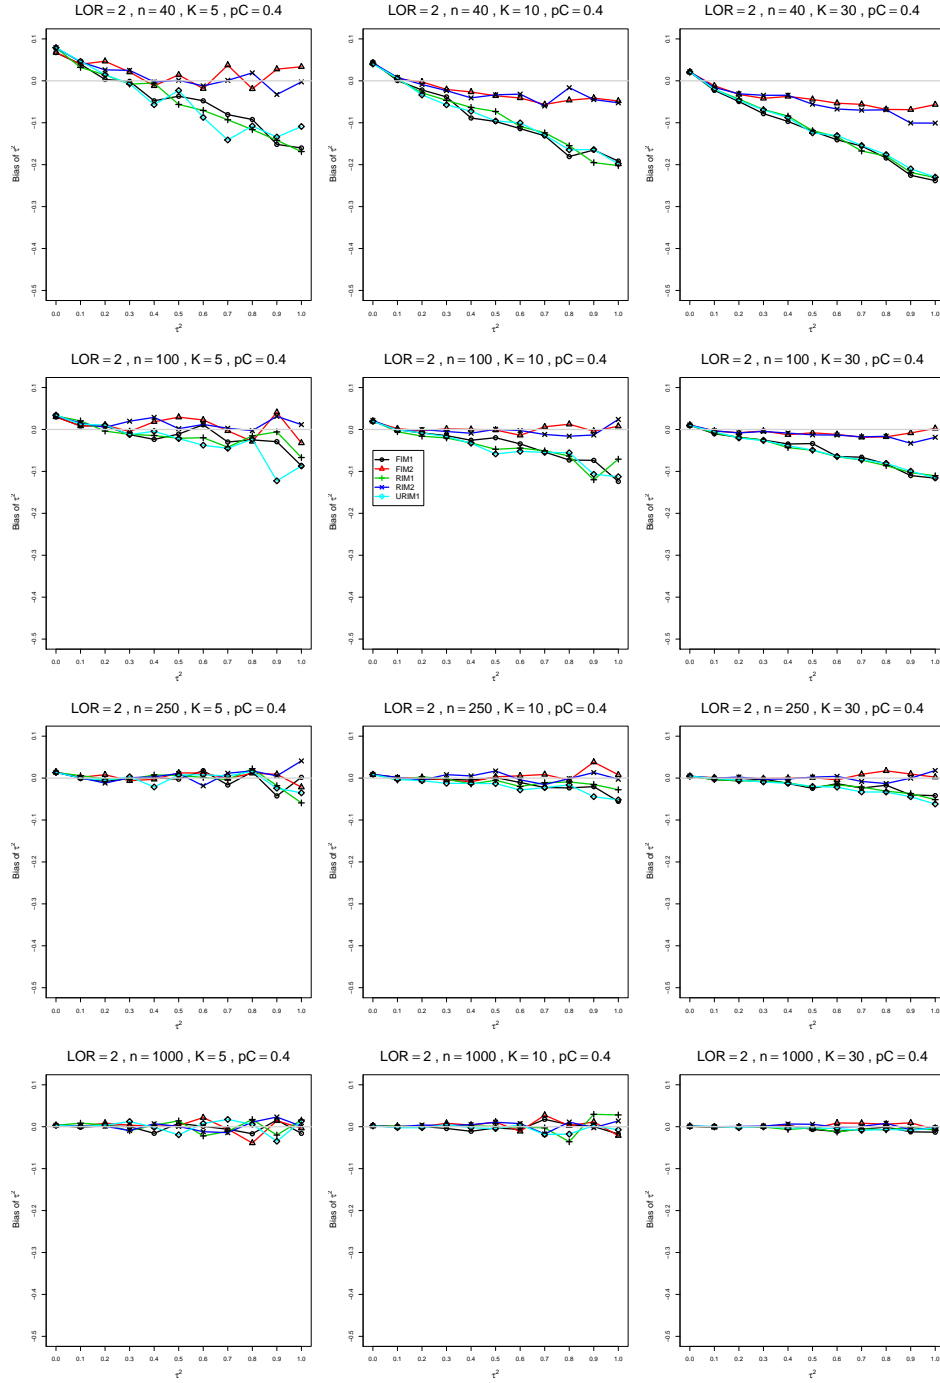

Figure A1.2.10: Bias of between-studies variance  $\hat{\tau}_{REML}^2$  for  $\theta = 2$ ,  $p_C = 0.4$ ,  $\sigma^2 = 0.1$ , constant sample sizes  $n = 40, 100, 250, 1000$ . The data-generation mechanisms are FIM1 ( $\circ$ ), FIM2 ( $\triangle$ ), RIM1 ( $+$ ), RIM2 ( $\times$ ), and URIM1 ( $\diamond$ ).

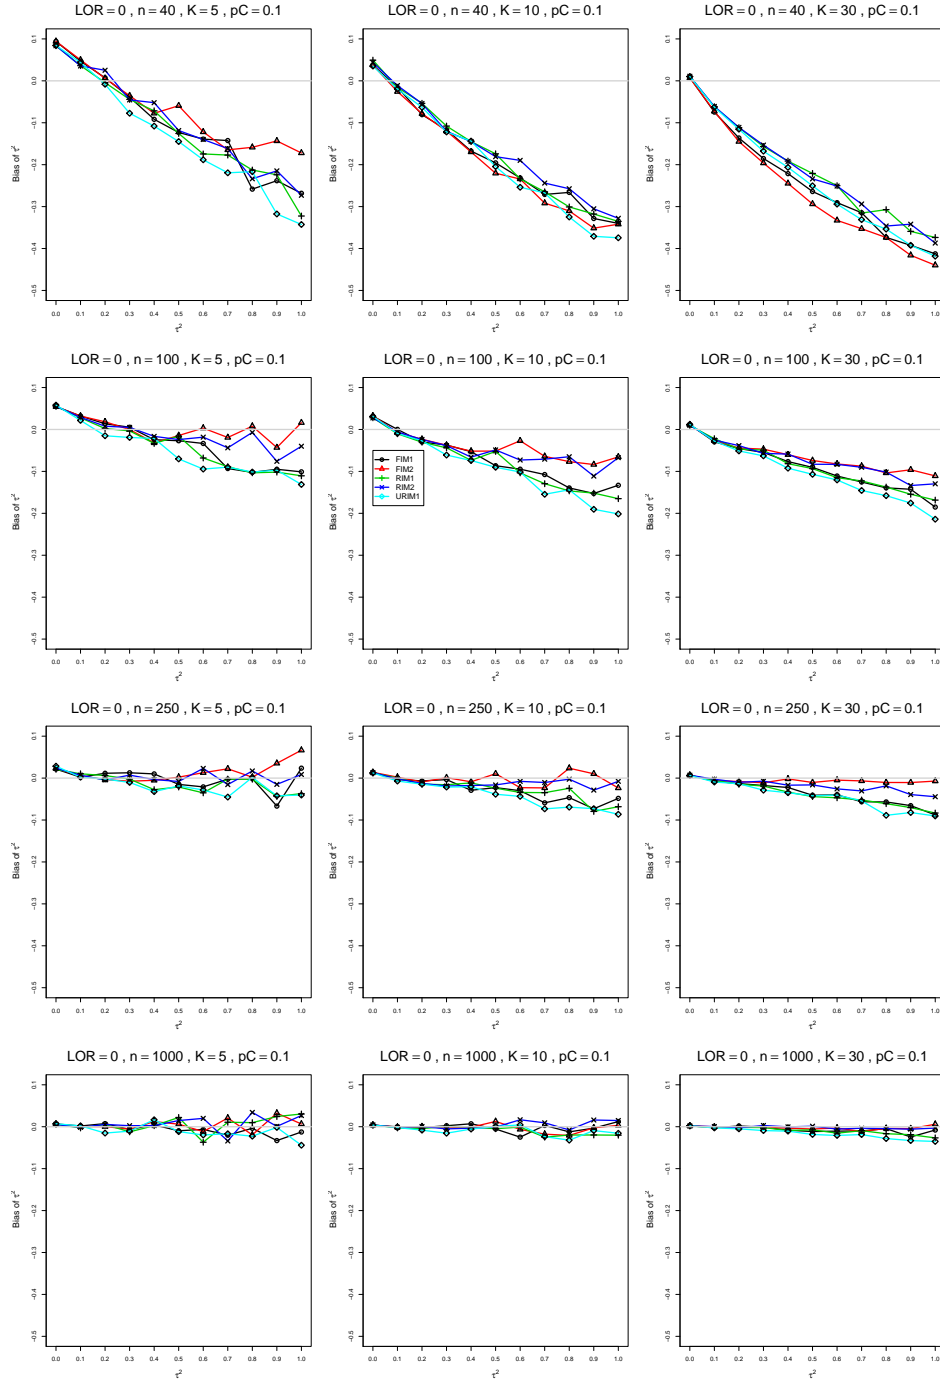

Figure A1.2.11: Bias of between-studies variance  $\hat{\tau}_{REML}^2$  for  $\theta = 0$ ,  $p_C = 0.1$ ,  $\sigma^2 = 0.4$ , constant sample sizes  $n = 40, 100, 250, 1000$ . The data-generation mechanisms are FIM1 ( $\circ$ ), FIM2 ( $\triangle$ ), RIM1 ( $+$ ), RIM2 ( $\times$ ), and URIM1 ( $\diamond$ ).

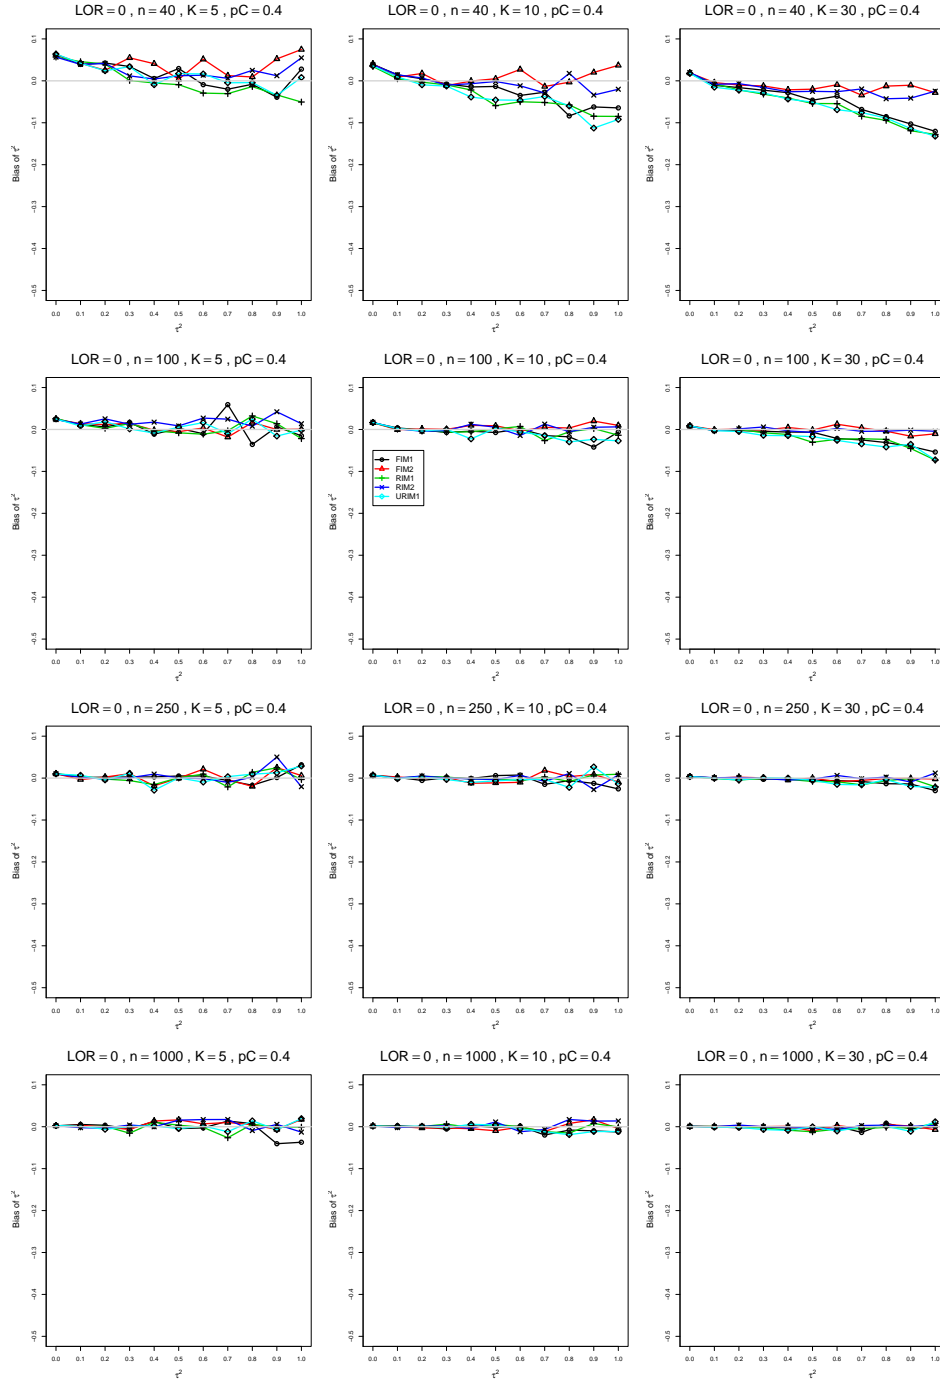

Figure A1.2.12: Bias of between-studies variance  $\hat{\tau}_{REML}^2$  for  $\theta = 0$ ,  $p_C = 0.4$ ,  $\sigma^2 = 0.4$ , constant sample sizes  $n = 40, 100, 250, 1000$ . The data-generation mechanisms are FIM1 ( $\circ$ ), FIM2 ( $\triangle$ ), RIM1 ( $+$ ), RIM2 ( $\times$ ), and URIM1 ( $\diamond$ ).



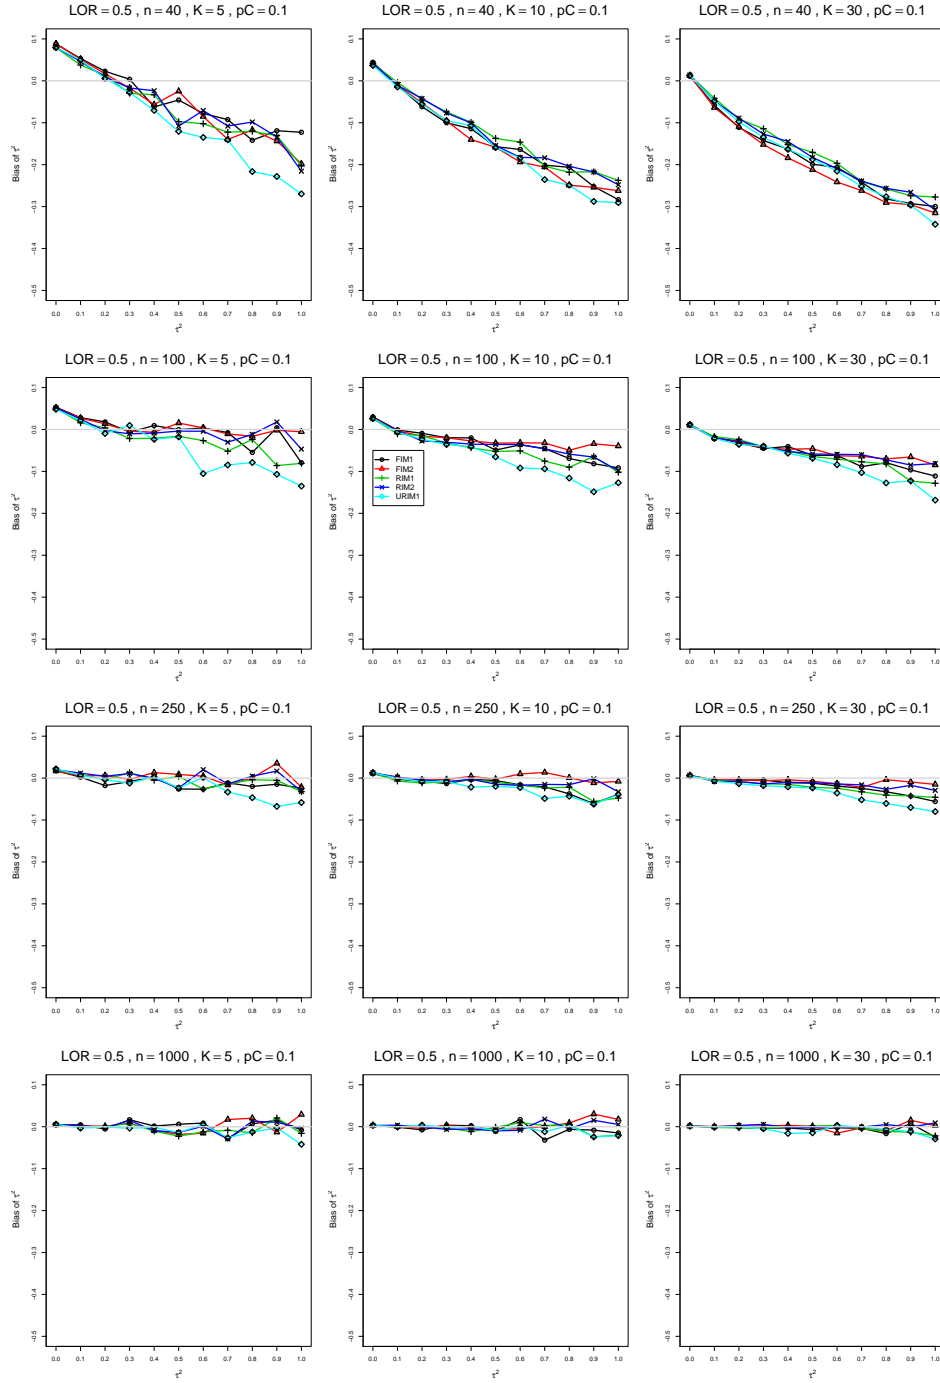

Figure A1.2.13: Bias of between-studies variance  $\hat{\tau}_{REML}^2$  for  $\theta = 0.5$ ,  $p_C = 0.1$ ,  $\sigma^2 = 0.4$ , constant sample sizes  $n = 40, 100, 250, 1000$ . The data-generation mechanisms are FIM1 ( $\circ$ ), FIM2 ( $\triangle$ ), RIM1 ( $+$ ), RIM2 ( $\times$ ), and URIM1 ( $\diamond$ ).

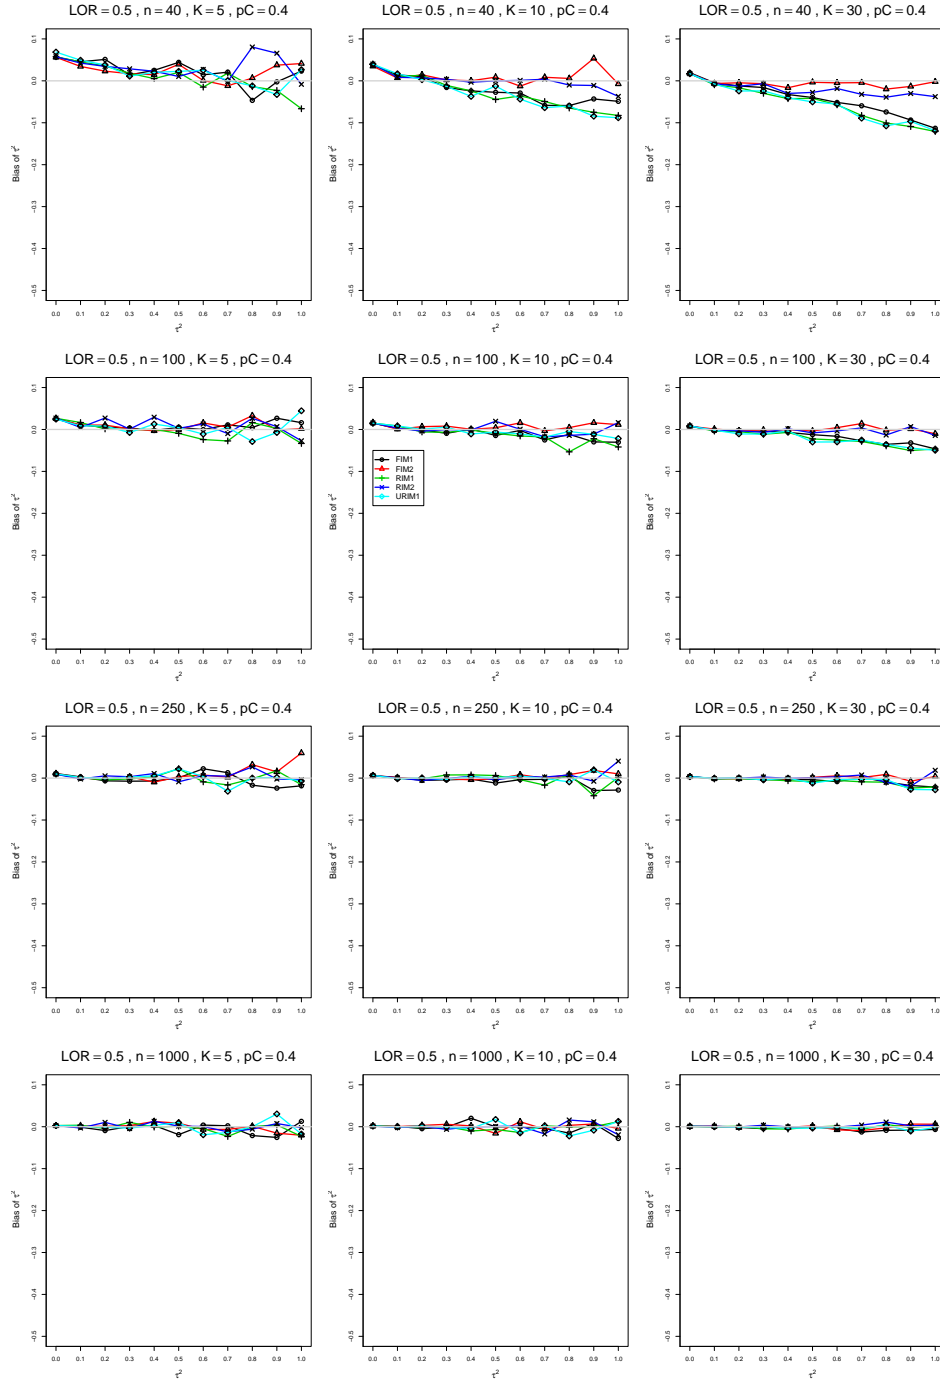

Figure A1.2.14: Bias of between-studies variance  $\hat{\tau}_{REML}^2$  for  $\theta = 0.5$ ,  $p_C = 0.4$ ,  $\sigma^2 = 0.4$ , constant sample sizes  $n = 40, 100, 250, 1000$ . The data-generation mechanisms are FIM1 ( $\circ$ ), FIM2 ( $\triangle$ ), RIM1 ( $+$ ), RIM2 ( $\times$ ), and URIM1 ( $\diamond$ ).

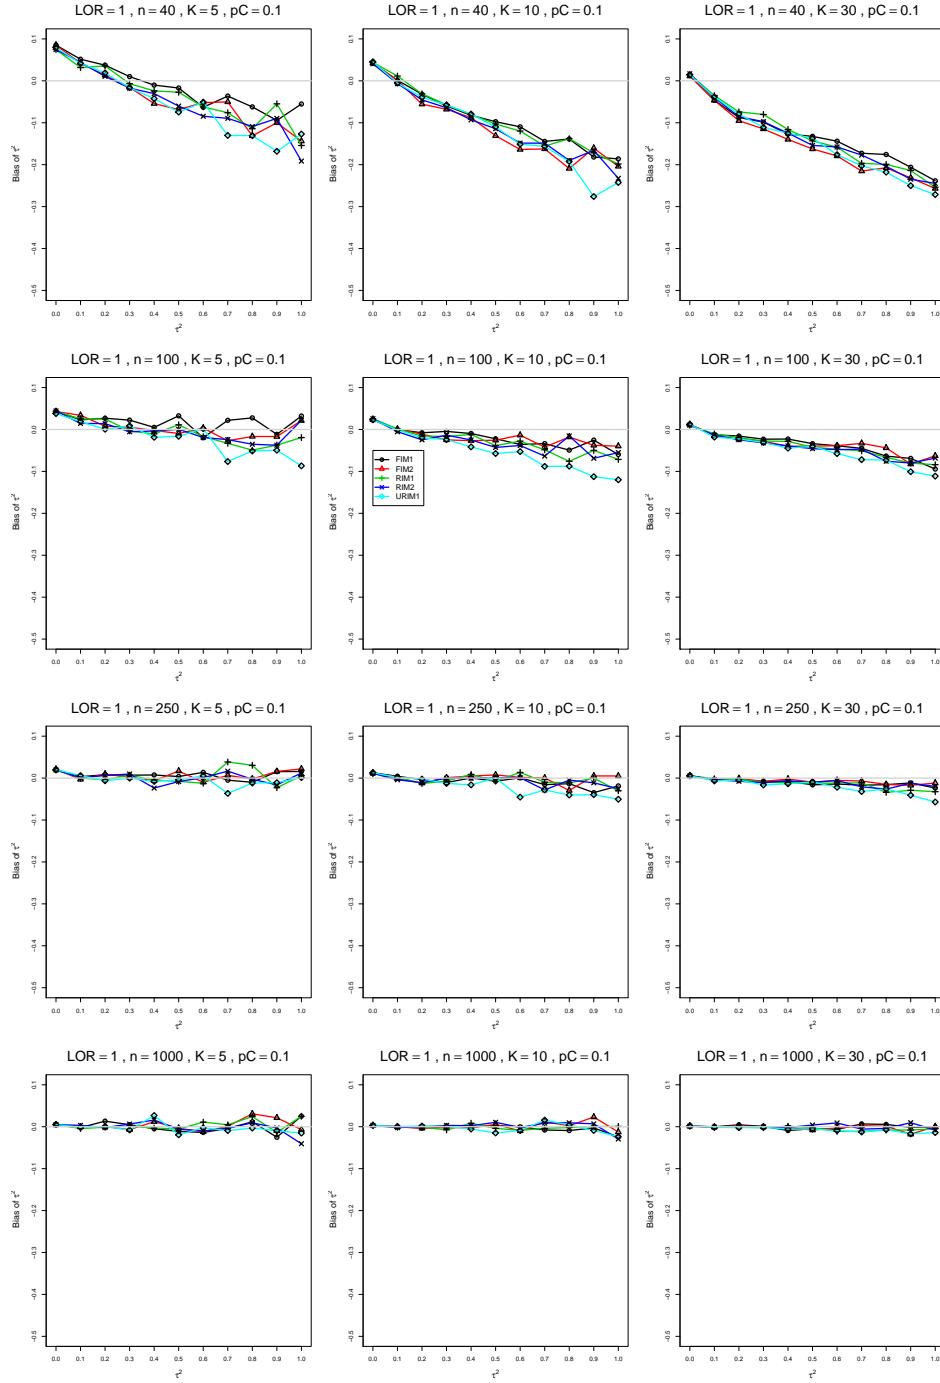

Figure A1.2.15: Bias of between-studies variance  $\hat{\tau}_{REML}^2$  for  $\theta = 1$ ,  $p_C = 0.1$ ,  $\sigma^2 = 0.4$ , constant sample sizes  $n = 40, 100, 250, 1000$ . The data-generation mechanisms are FIM1 ( $\circ$ ), FIM2 ( $\triangle$ ), RIM1 ( $+$ ), RIM2 ( $\times$ ), and URIM1 ( $\diamond$ ).

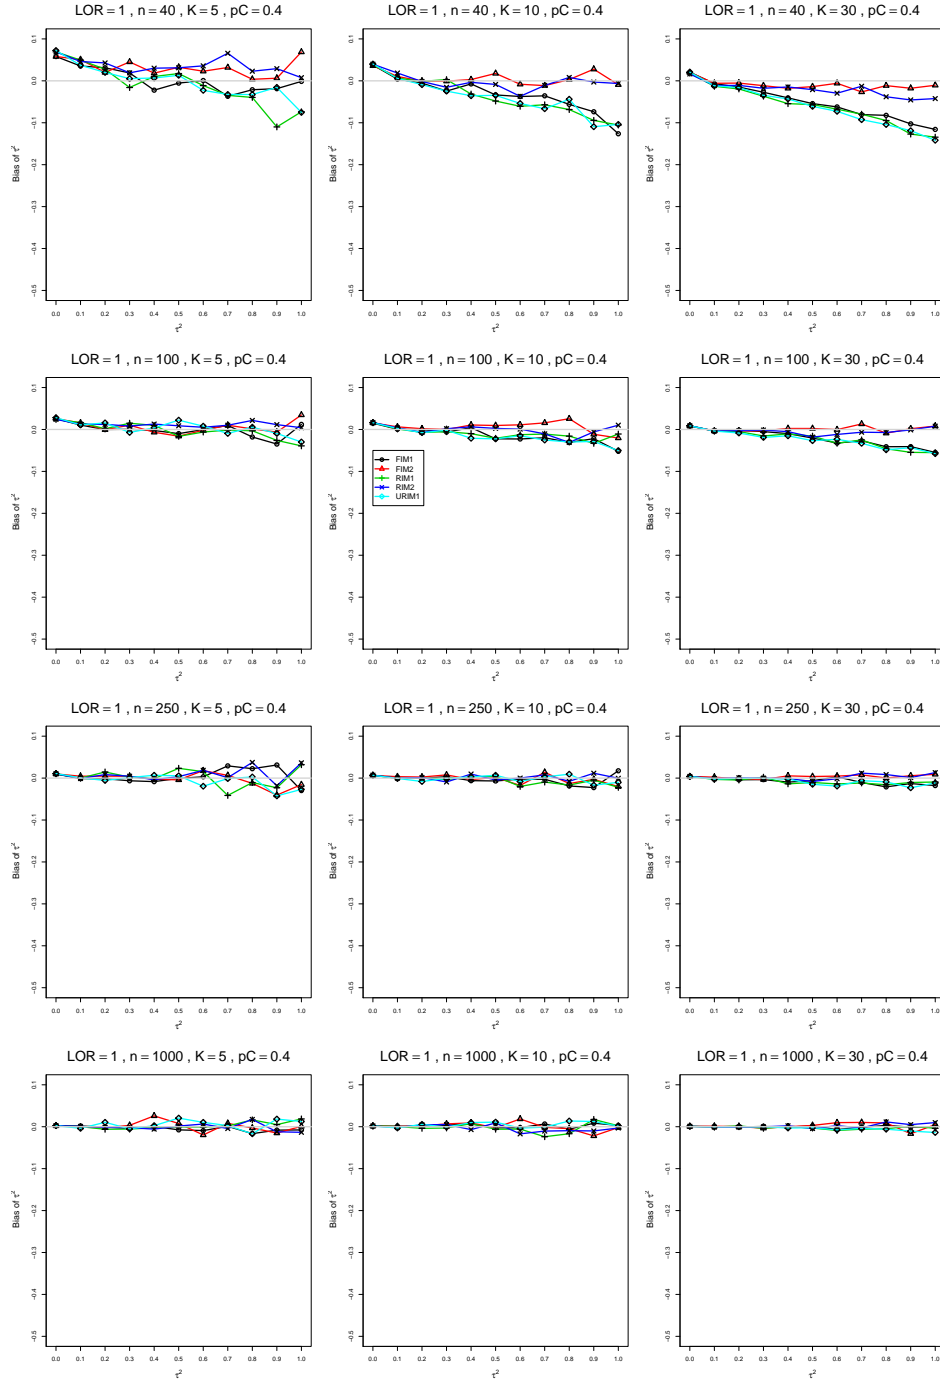

Figure A1.2.16: Bias of between-studies variance  $\hat{\tau}_{REML}^2$  for  $\theta = 1$ ,  $p_C = 0.4$ ,  $\sigma^2 = 0.4$ , constant sample sizes  $n = 40, 100, 250, 1000$ . The data-generation mechanisms are FIM1 ( $\circ$ ), FIM2 ( $\triangle$ ), RIM1 ( $+$ ), RIM2 ( $\times$ ), and URIM1 ( $\diamond$ ).

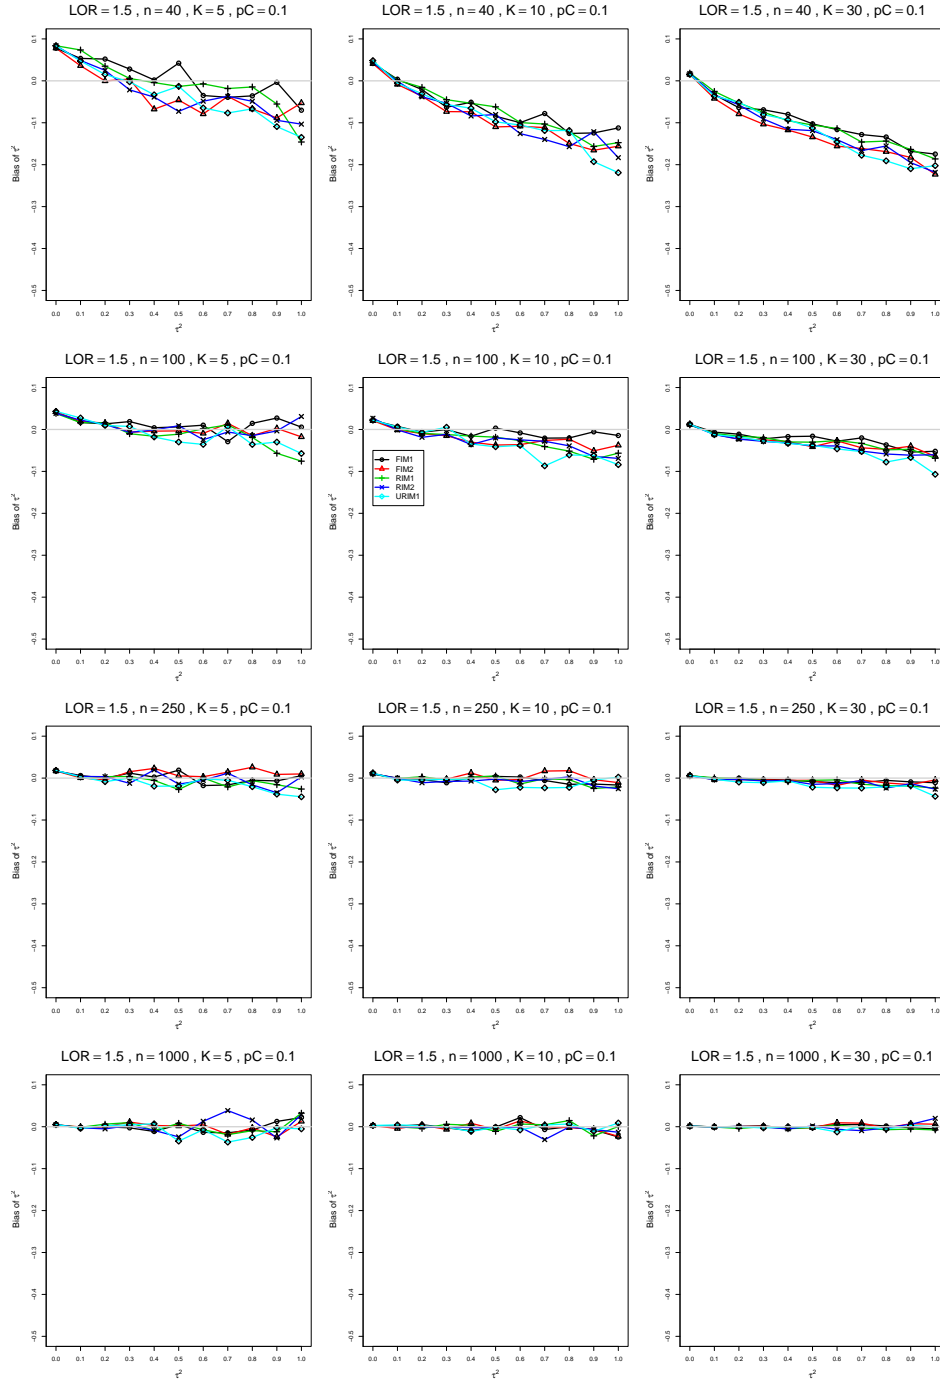

Figure A1.2.17: Bias of between-studies variance  $\hat{\tau}_{REML}^2$  for  $\theta = 1.5$ ,  $p_C = 0.1$ ,  $\sigma^2 = 0.4$ , constant sample sizes  $n = 40, 100, 250, 1000$ . The data-generation mechanisms are FIM1 ( $\circ$ ), FIM2 ( $\triangle$ ), RIM1 ( $+$ ), RIM2 ( $\times$ ), and URIM1 ( $\diamond$ ).

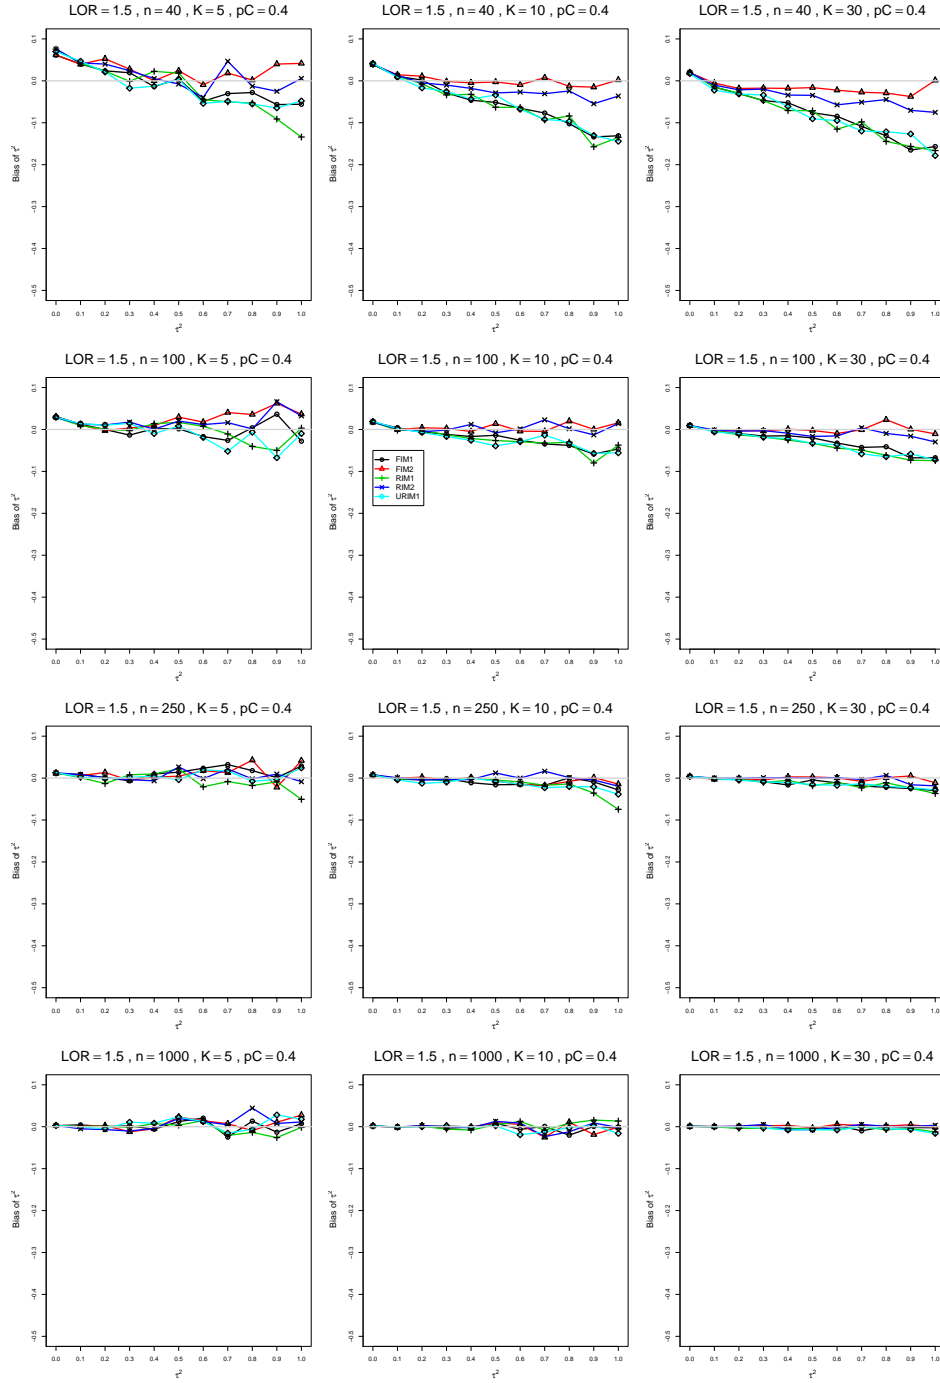

Figure A1.2.18: Bias of between-studies variance  $\hat{\tau}_{REML}^2$  for  $\theta = 1.5$ ,  $p_C = 0.4$ ,  $\sigma^2 = 0.4$ , constant sample sizes  $n = 40, 100, 250, 1000$ . The data-generation mechanisms are FIM1 ( $\circ$ ), FIM2 ( $\triangle$ ), RIM1 ( $+$ ), RIM2 ( $\times$ ), and URIM1 ( $\diamond$ ).

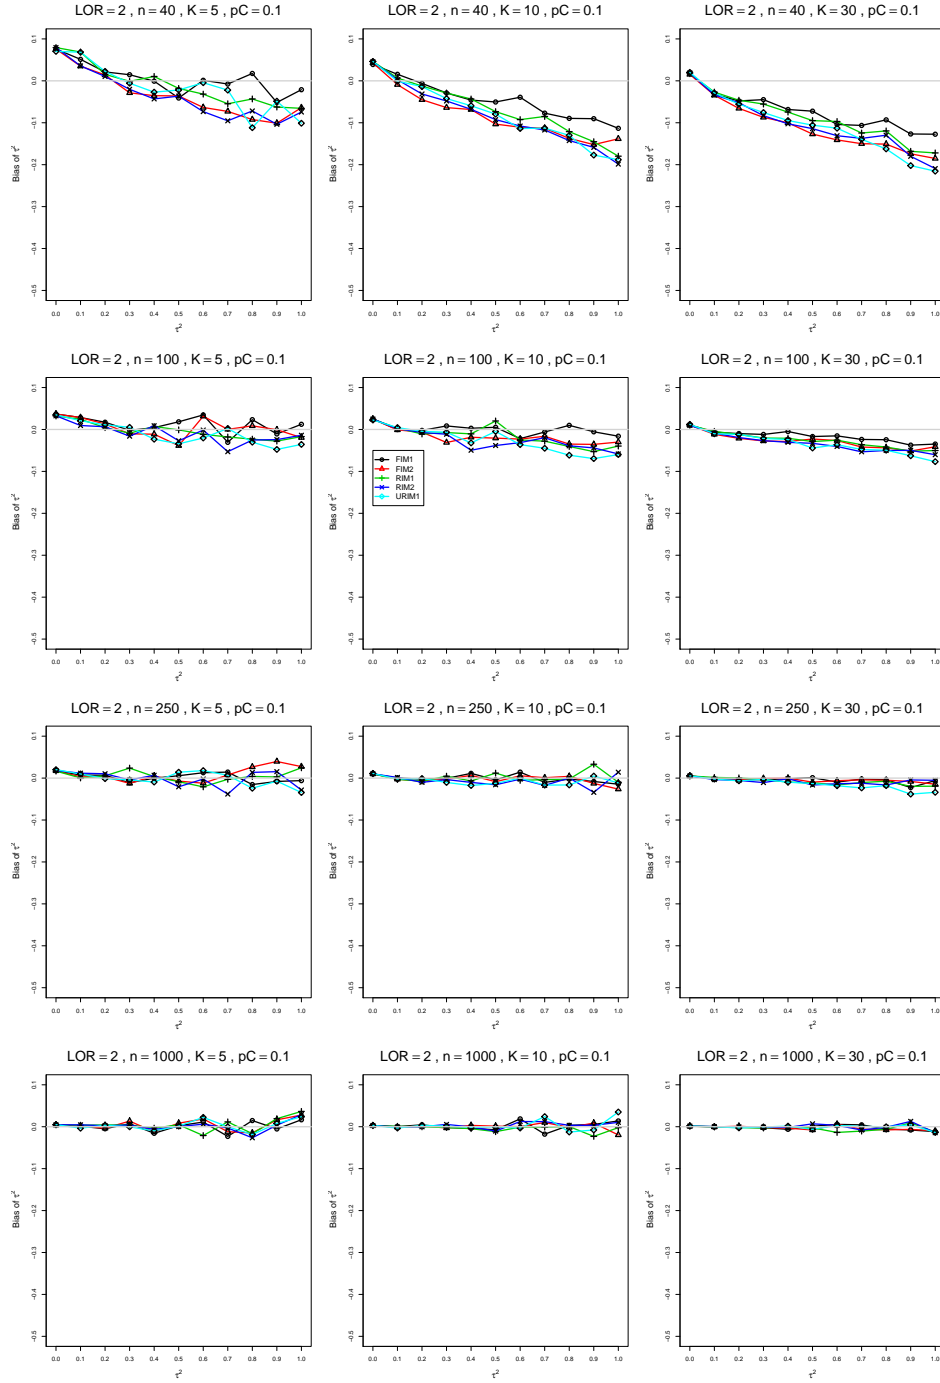

Figure A1.2.19: Bias of between-studies variance  $\hat{\tau}_{REML}^2$  for  $\theta = 2$ ,  $p_C = 0.1$ ,  $\sigma^2 = 0.4$ , constant sample sizes  $n = 40, 100, 250, 1000$ . The data-generation mechanisms are FIM1 ( $\circ$ ), FIM2 ( $\triangle$ ), RIM1 ( $+$ ), RIM2 ( $\times$ ), and URIM1 ( $\diamond$ ).

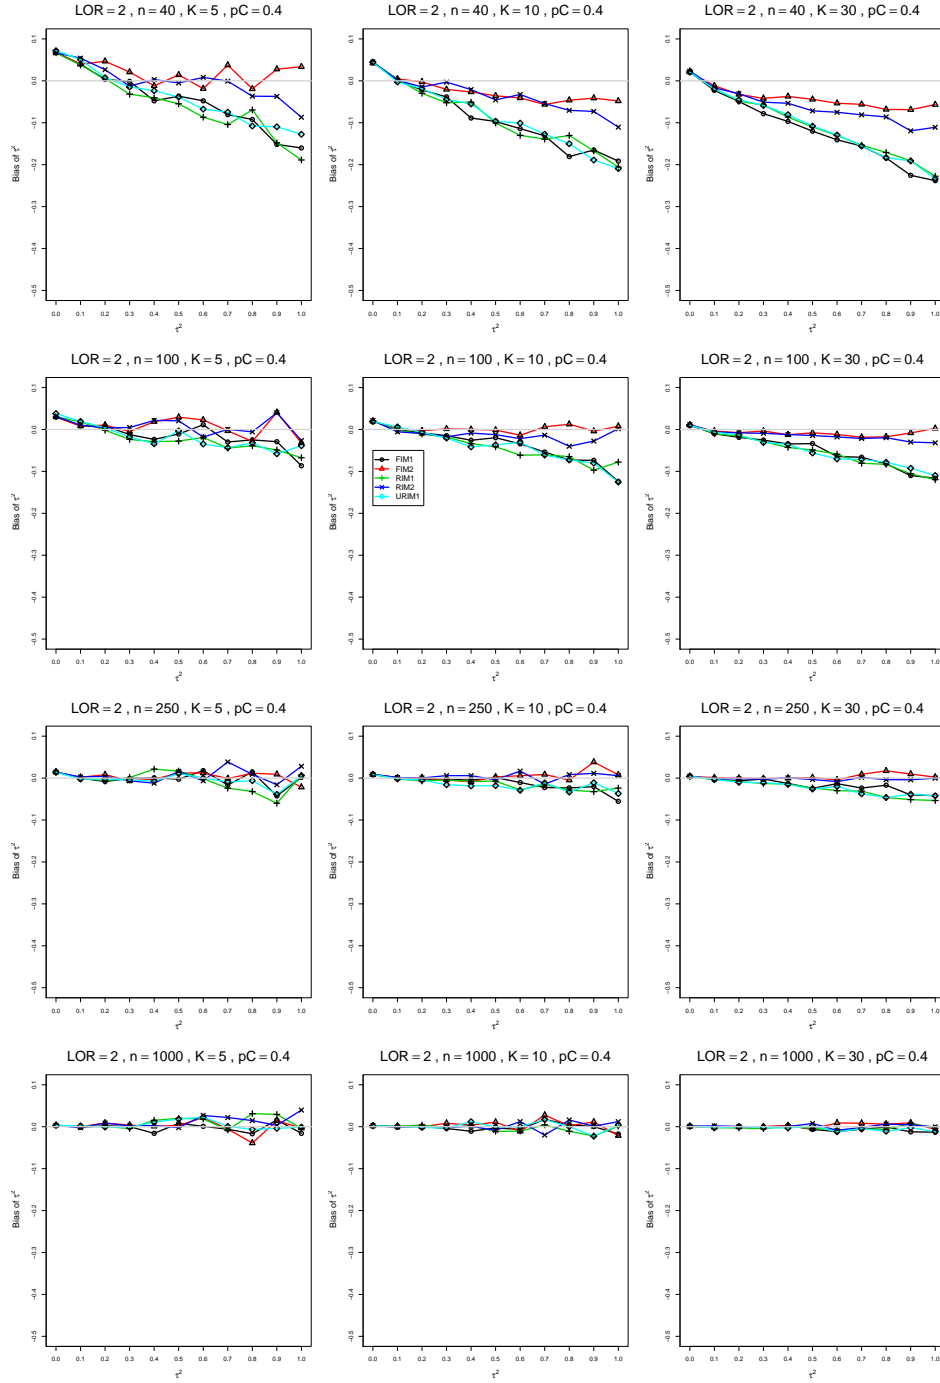

Figure A1.2.20: Bias of between-studies variance  $\hat{\tau}_{REML}^2$  for  $\theta = 2$ ,  $p_C = 0.4$ ,  $\sigma^2 = 0.4$ , constant sample sizes  $n = 40, 100, 250, 1000$ . The data-generation mechanisms are FIM1 ( $\circ$ ), FIM2 ( $\triangle$ ), RIM1 ( $+$ ), RIM2 ( $\times$ ), and URIM1 ( $\diamond$ ).



### A1.3 Bias of $\hat{\tau}_{MP}^2$

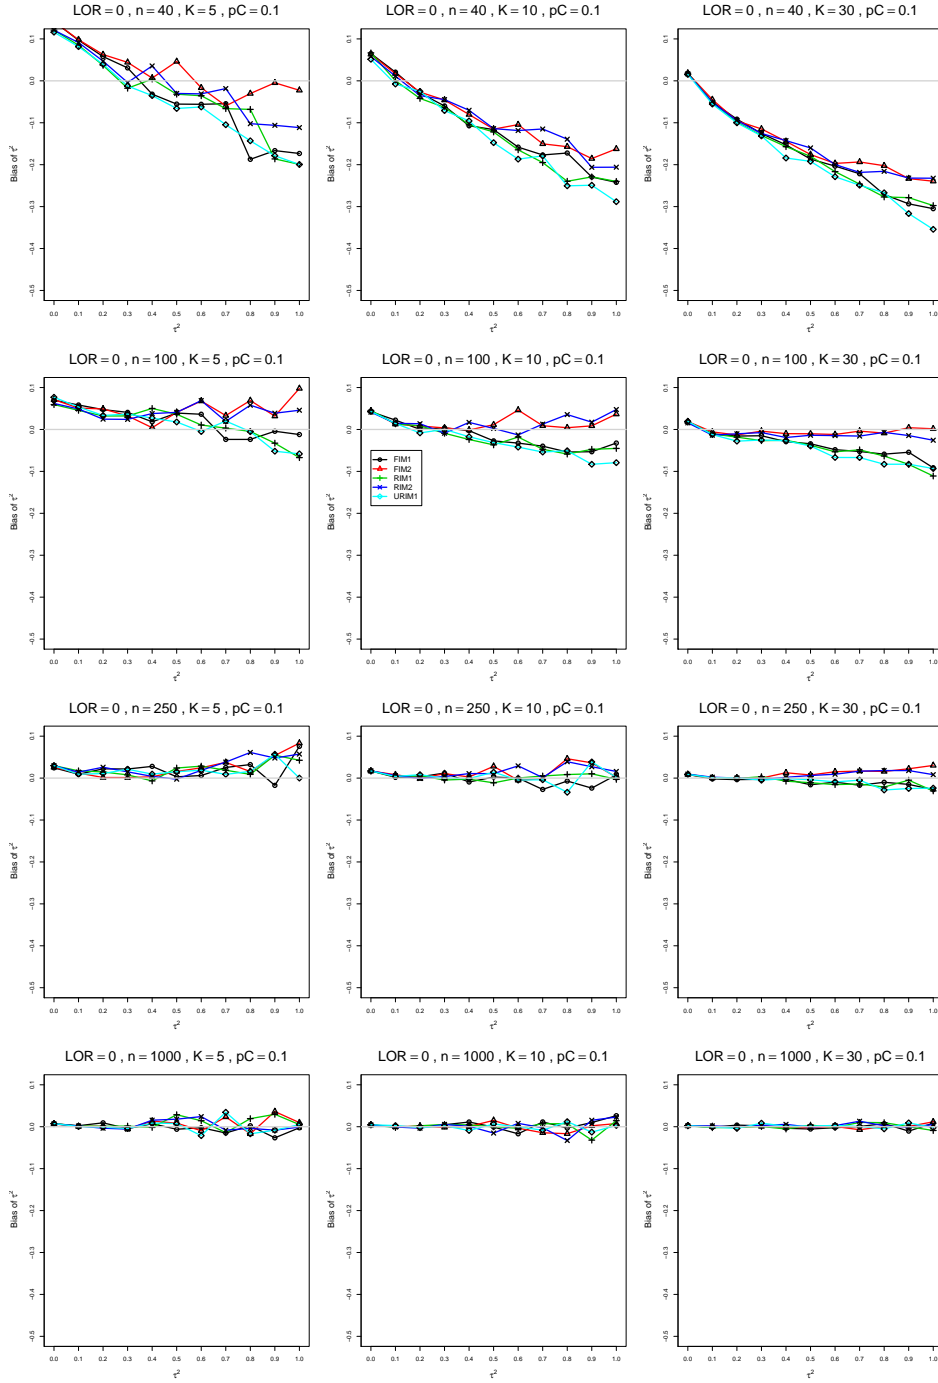

Figure A1.3.1: Bias of between-studies variance  $\hat{\tau}_{MP}^2$  for  $\theta = 0$ ,  $p_C = 0.1$ ,  $\sigma^2 = 0.1$ , constant sample sizes  $n = 40, 100, 250, 1000$ . The data-generation mechanisms are FIM1 ( $\circ$ ), FIM2 ( $\triangle$ ), RIM1 ( $+$ ), RIM2 ( $\times$ ), and URIM1 ( $\diamond$ ).

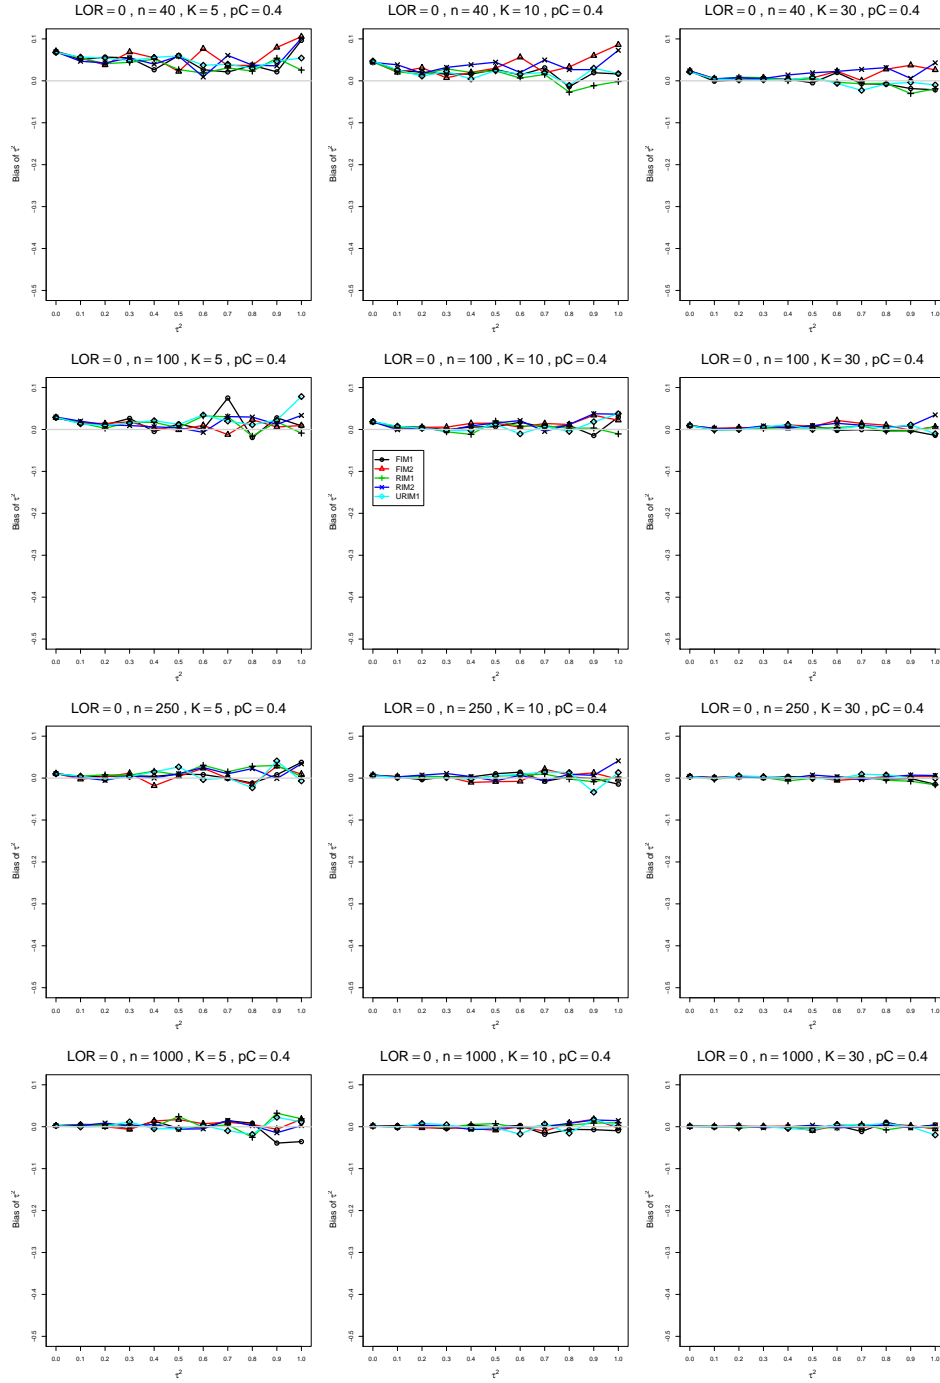

Figure A1.3.2: Bias of between-studies variance  $\hat{\tau}_{MP}^2$  for  $\theta = 0$ ,  $p_C = 0.4$ ,  $\sigma^2 = 0.1$ , constant sample sizes  $n = 40, 100, 250, 1000$ . The data-generation mechanisms are FIM1 ( $\circ$ ), FIM2 ( $\triangle$ ), RIM1 ( $+$ ), RIM2 ( $\times$ ), and URIM1 ( $\diamond$ ).

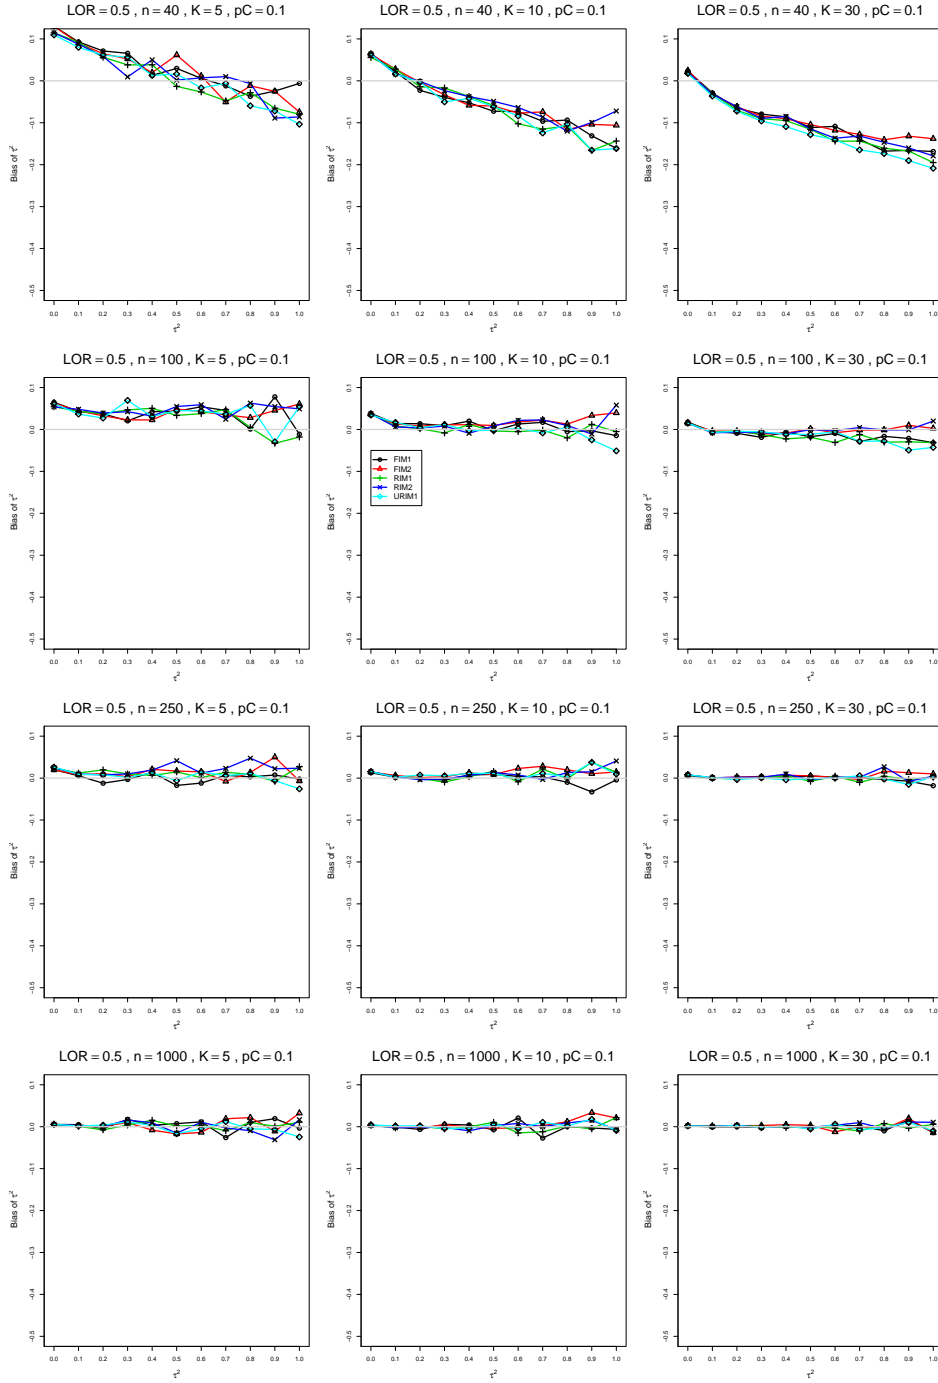

Figure A1.3.3: Bias of between-studies variance  $\hat{\tau}_{MP}^2$  for  $\theta = 0.5$ ,  $p_C = 0.1$ ,  $\sigma^2 = 0.1$ , constant sample sizes  $n = 40, 100, 250, 1000$ . The data-generation mechanisms are FIM1 ( $\circ$ ), FIM2 ( $\triangle$ ), RIM1 ( $+$ ), RIM2 ( $\times$ ), and URIM1 ( $\diamond$ ).

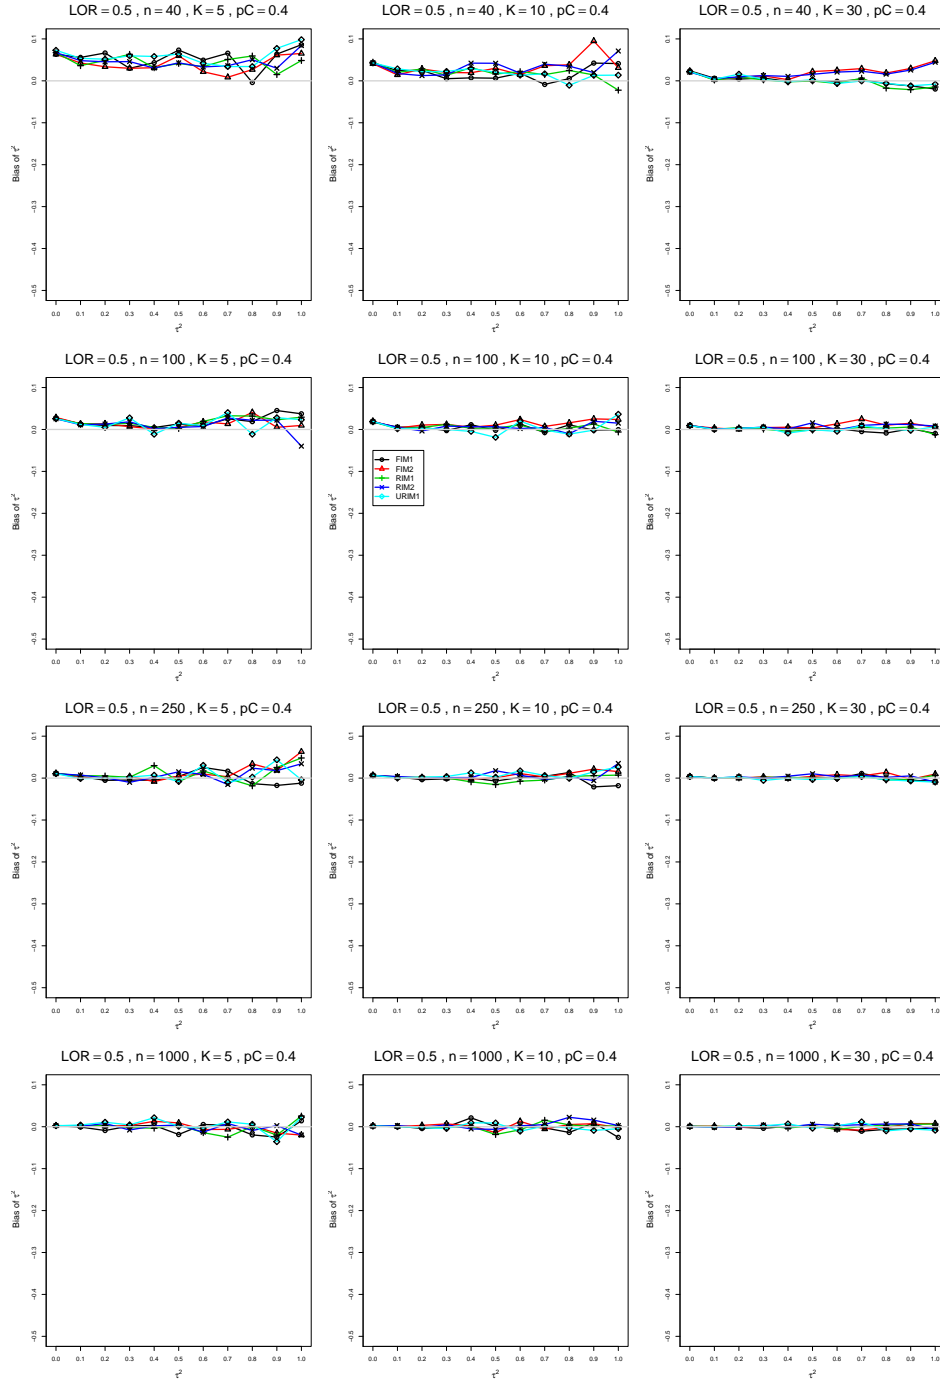

Figure A1.3.4: Bias of between-studies variance  $\hat{\tau}_{MP}^2$  for  $\theta = 0.5$ ,  $p_C = 0.4$ ,  $\sigma^2 = 0.1$ , constant sample sizes  $n = 40, 100, 250, 1000$ . The data-generation mechanisms are FIM1 ( $\circ$ ), FIM2 ( $\triangle$ ), RIM1 ( $+$ ), RIM2 ( $\times$ ), and URIM1 ( $\diamond$ ).

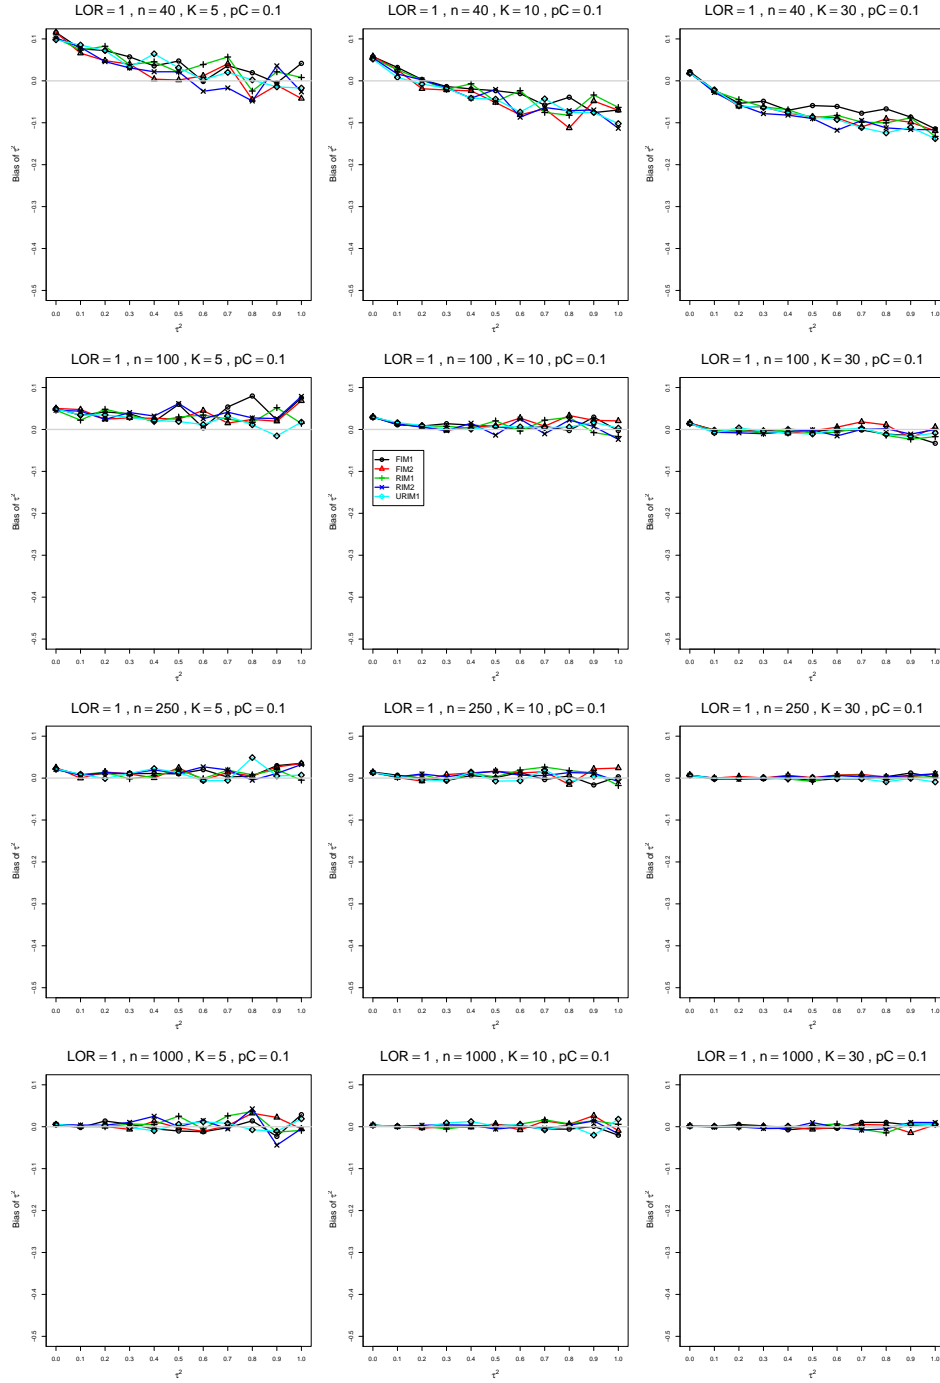

Figure A1.3.5: Bias of between-studies variance  $\hat{\tau}_{MP}^2$  for  $\theta = 1$ ,  $p_C = 0.1$ ,  $\sigma^2 = 0.1$ , constant sample sizes  $n = 40, 100, 250, 1000$ . The data-generation mechanisms are FIM1 ( $\circ$ ), FIM2 ( $\triangle$ ), RIM1 ( $+$ ), RIM2 ( $\times$ ), and URIM1 ( $\diamond$ ).

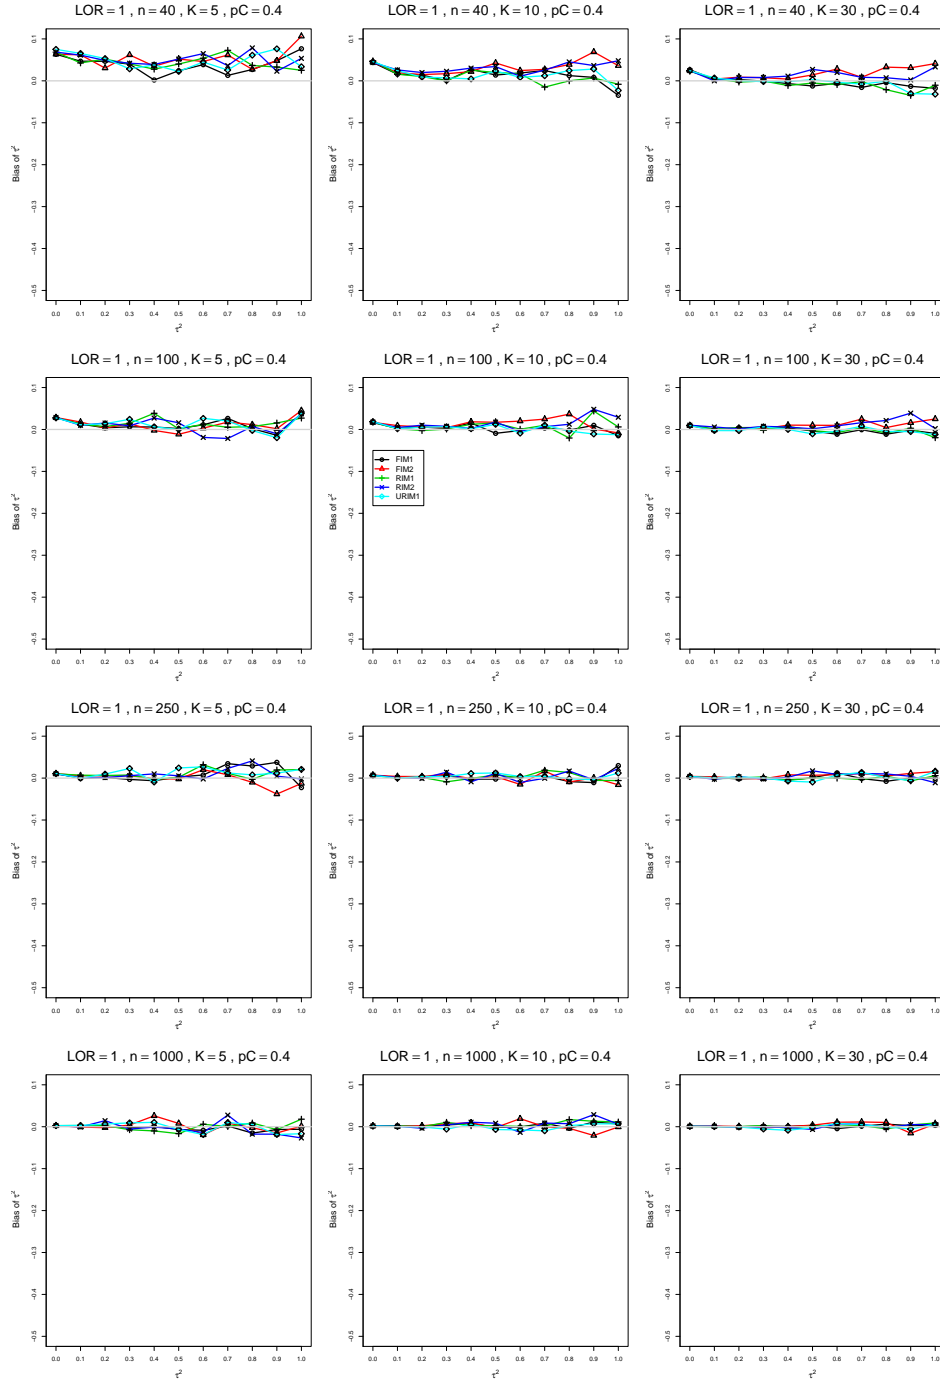

Figure A1.3.6: Bias of between-studies variance  $\hat{\tau}_{MP}^2$  for  $\theta = 1$ ,  $p_C = 0.4$ ,  $\sigma^2 = 0.1$ , constant sample sizes  $n = 40, 100, 250, 1000$ . The data-generation mechanisms are FIM1 ( $\circ$ ), FIM2 ( $\triangle$ ), RIM1 ( $+$ ), RIM2 ( $\times$ ), and URIM1 ( $\diamond$ ).

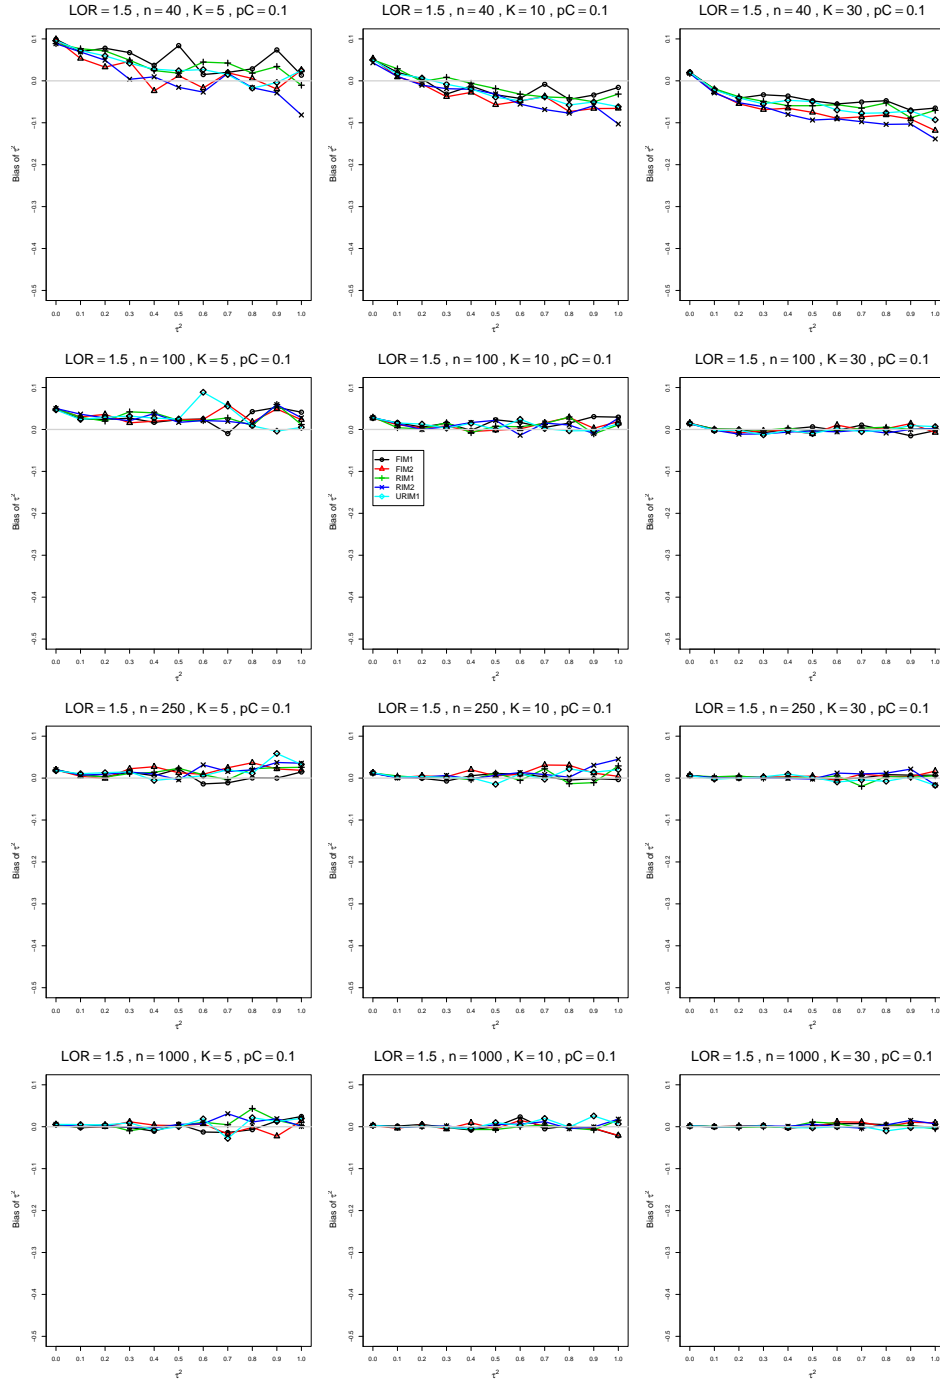

Figure A1.3.7: Bias of between-studies variance  $\hat{\tau}_{MP}^2$  for  $\theta = 1.5$ ,  $p_C = 0.1$ ,  $\sigma^2 = 0.1$ , constant sample sizes  $n = 40, 100, 250, 1000$ . The data-generation mechanisms are FIM1 ( $\circ$ ), FIM2 ( $\triangle$ ), RIM1 ( $+$ ), RIM2 ( $\times$ ), and URIM1 ( $\diamond$ ).



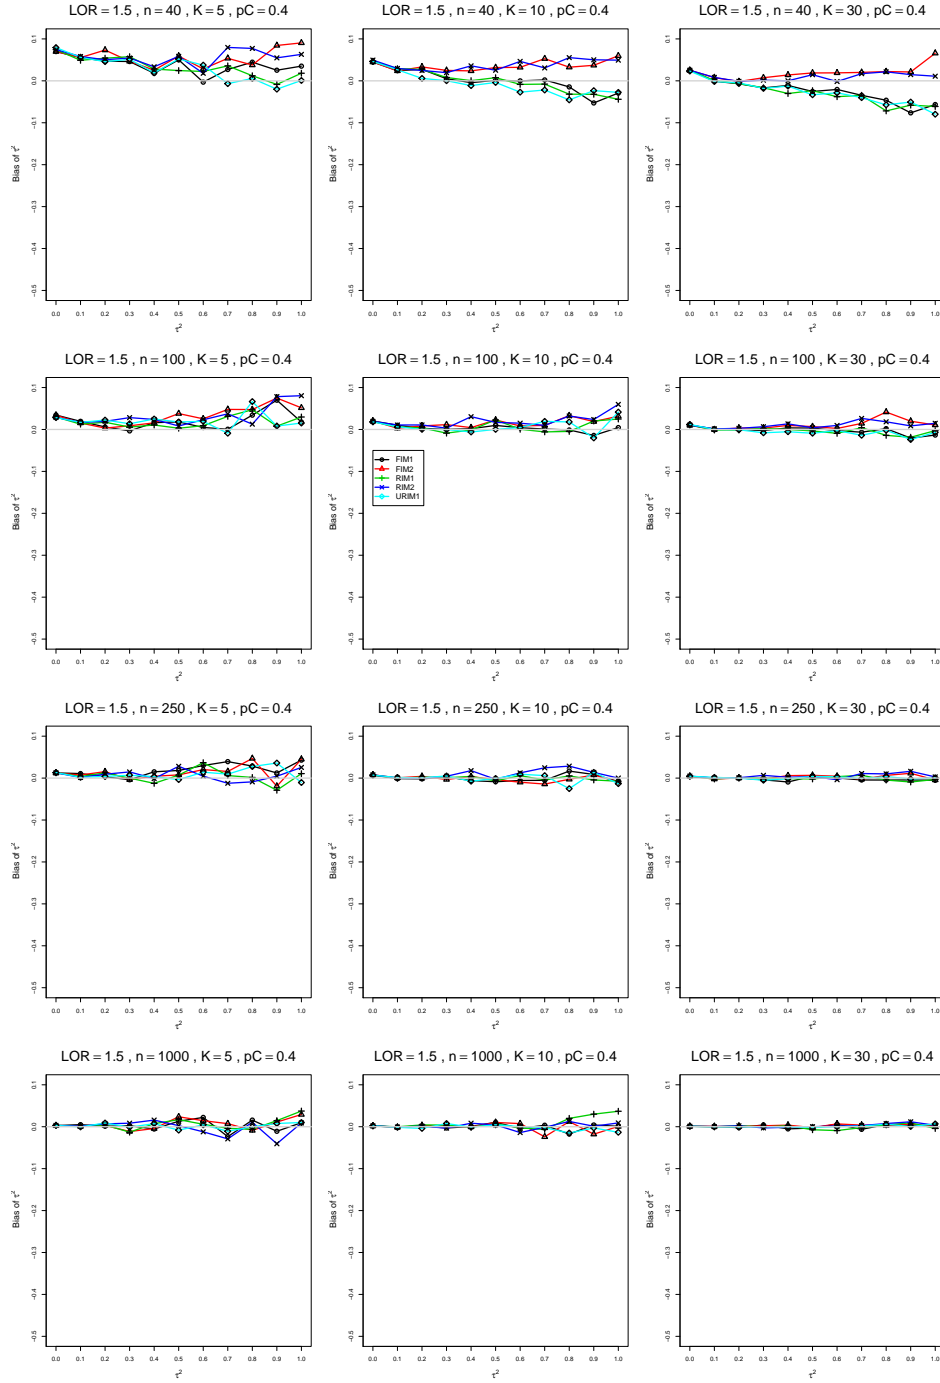

Figure A1.3.8: Bias of between-studies variance  $\hat{\tau}_{MP}^2$  for  $\theta = 1.5$ ,  $p_C = 0.4$ ,  $\sigma^2 = 0.1$ , constant sample sizes  $n = 40, 100, 250, 1000$ . The data-generation mechanisms are FIM1 ( $\circ$ ), FIM2 ( $\triangle$ ), RIM1 ( $+$ ), RIM2 ( $\times$ ), and URIM1 ( $\diamond$ ).

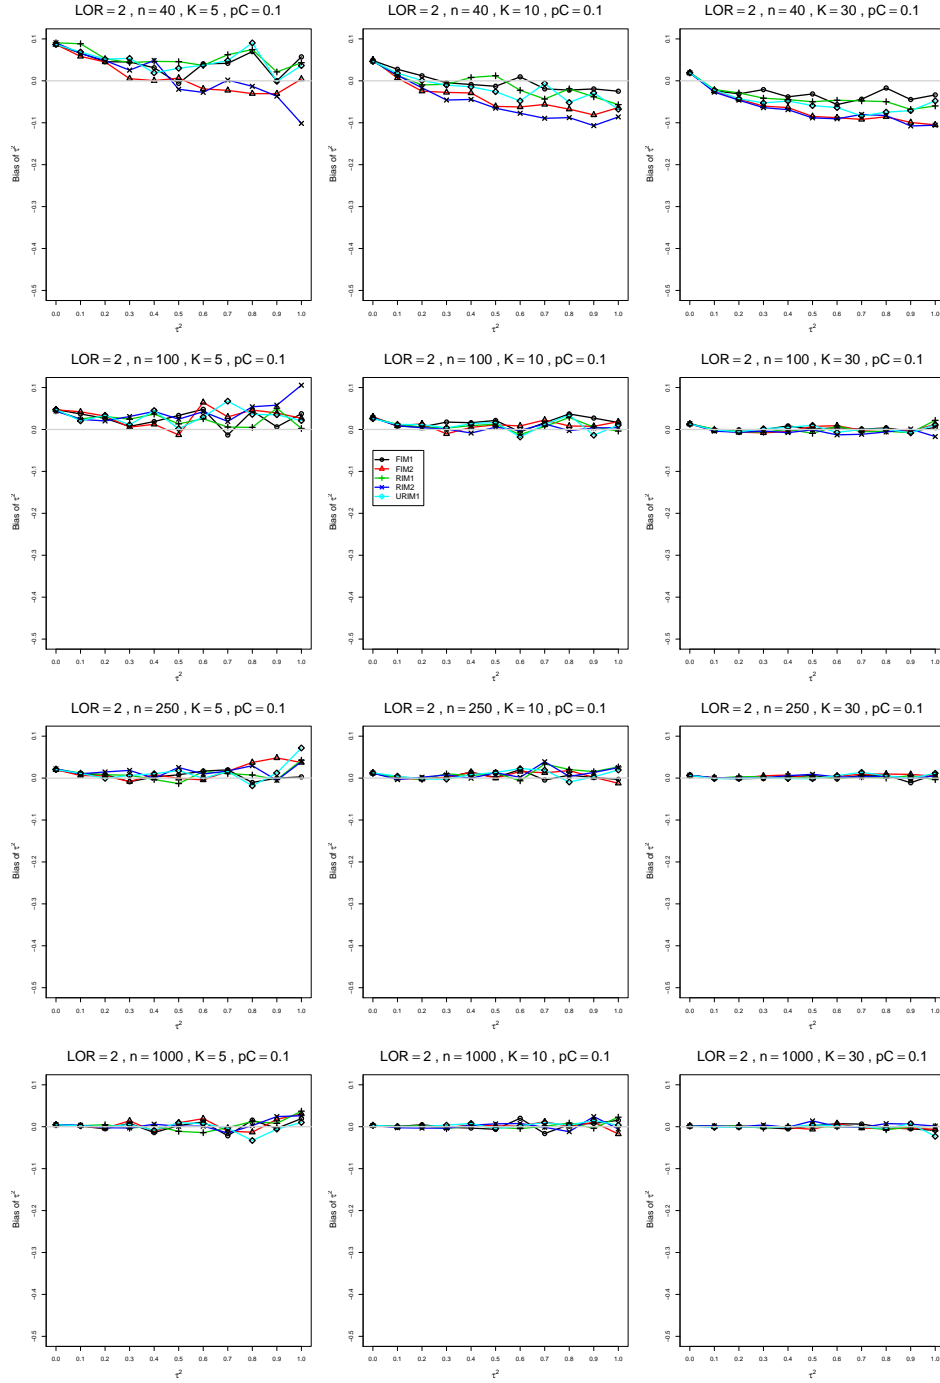

Figure A1.3.9: Bias of between-studies variance  $\hat{\tau}_{MP}^2$  for  $\theta = 2$ ,  $p_C = 0.1$ ,  $\sigma^2 = 0.1$ , constant sample sizes  $n = 40, 100, 250, 1000$ . The data-generation mechanisms are FIM1 ( $\circ$ ), FIM2 ( $\triangle$ ), RIM1 ( $+$ ), RIM2 ( $\times$ ), and URIM1 ( $\diamond$ ).

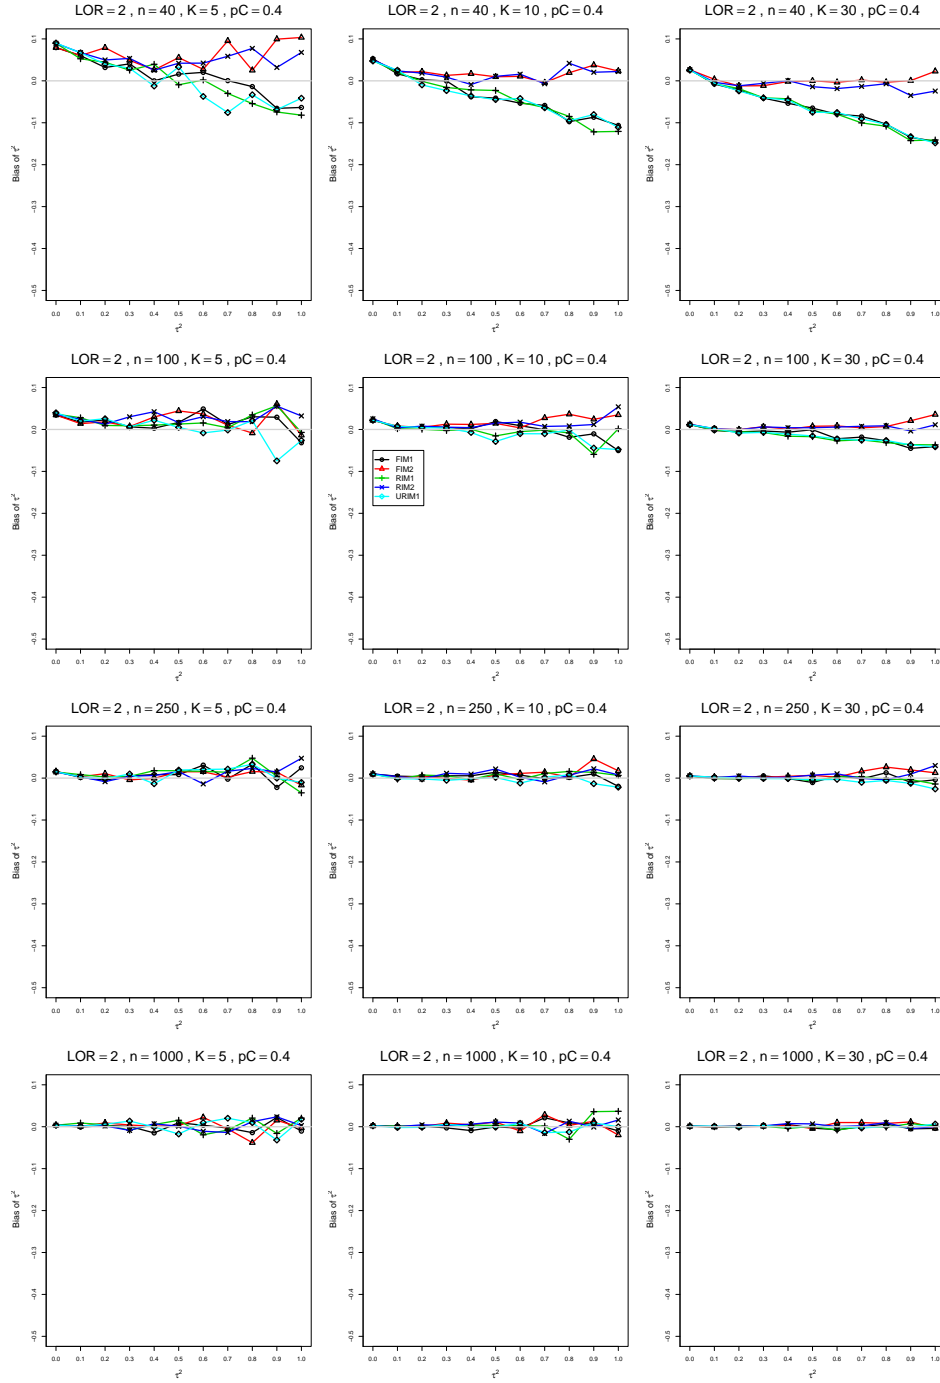

Figure A1.3.10: Bias of between-studies variance  $\hat{\tau}_{MP}^2$  for  $\theta = 2$ ,  $p_C = 0.4$ ,  $\sigma^2 = 0.1$ , constant sample sizes  $n = 40, 100, 250, 1000$ . The data-generation mechanisms are FIM1 ( $\circ$ ), FIM2 ( $\triangle$ ), RIM1 ( $+$ ), RIM2 ( $\times$ ), and URIM1 ( $\diamond$ ).

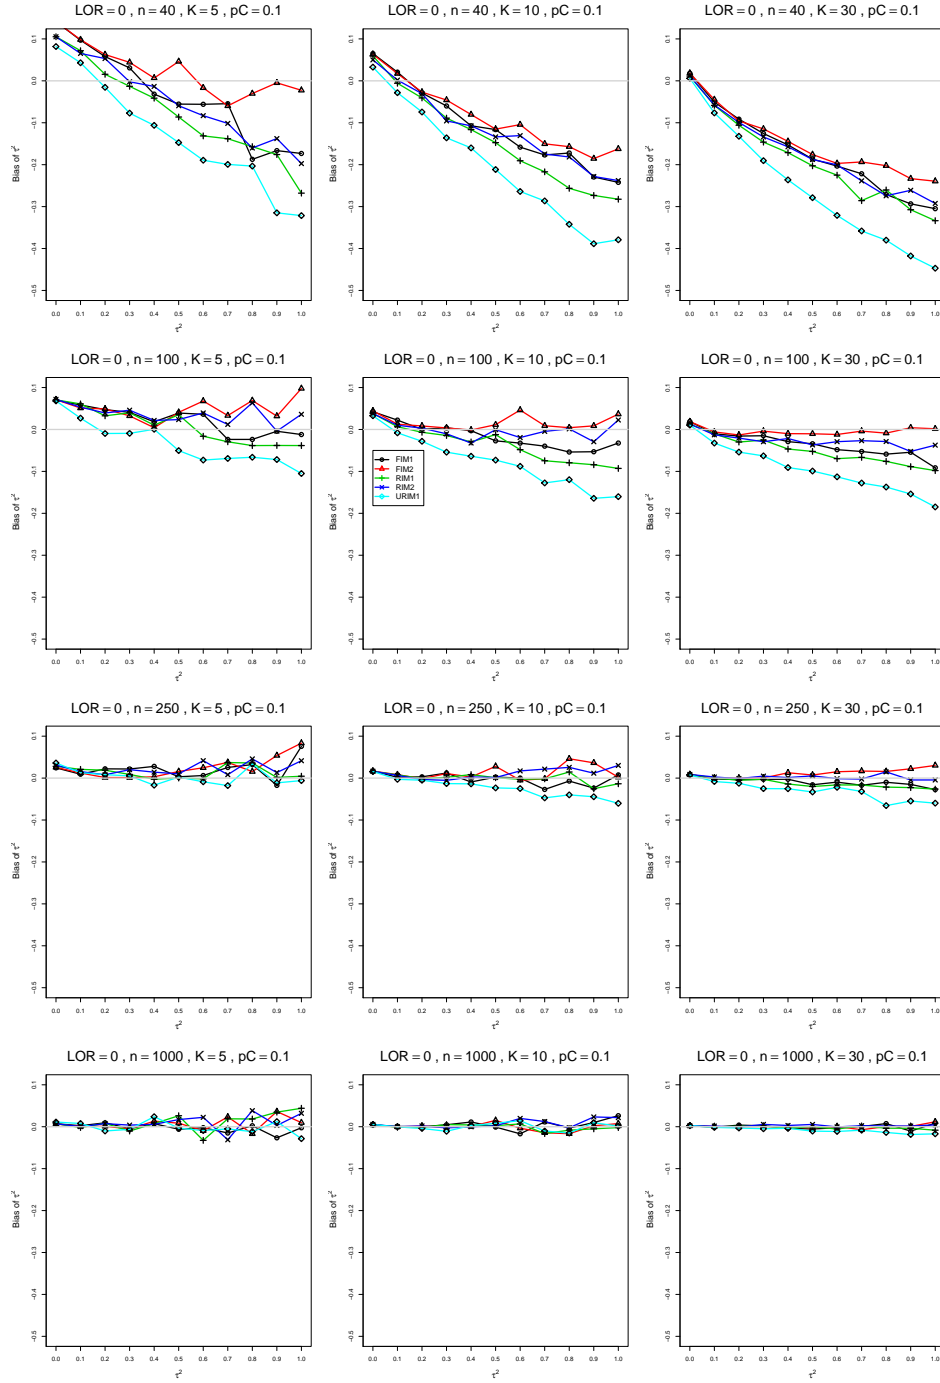

Figure A1.3.11: Bias of between-studies variance  $\hat{\tau}_{MP}^2$  for  $\theta = 0$ ,  $p_C = 0.1$ ,  $\sigma^2 = 0.4$ , constant sample sizes  $n = 40, 100, 250, 1000$ . The data-generation mechanisms are FIM1 ( $\circ$ ), FIM2 ( $\triangle$ ), RIM1 ( $+$ ), RIM2 ( $\times$ ), and URIM1 ( $\diamond$ ).

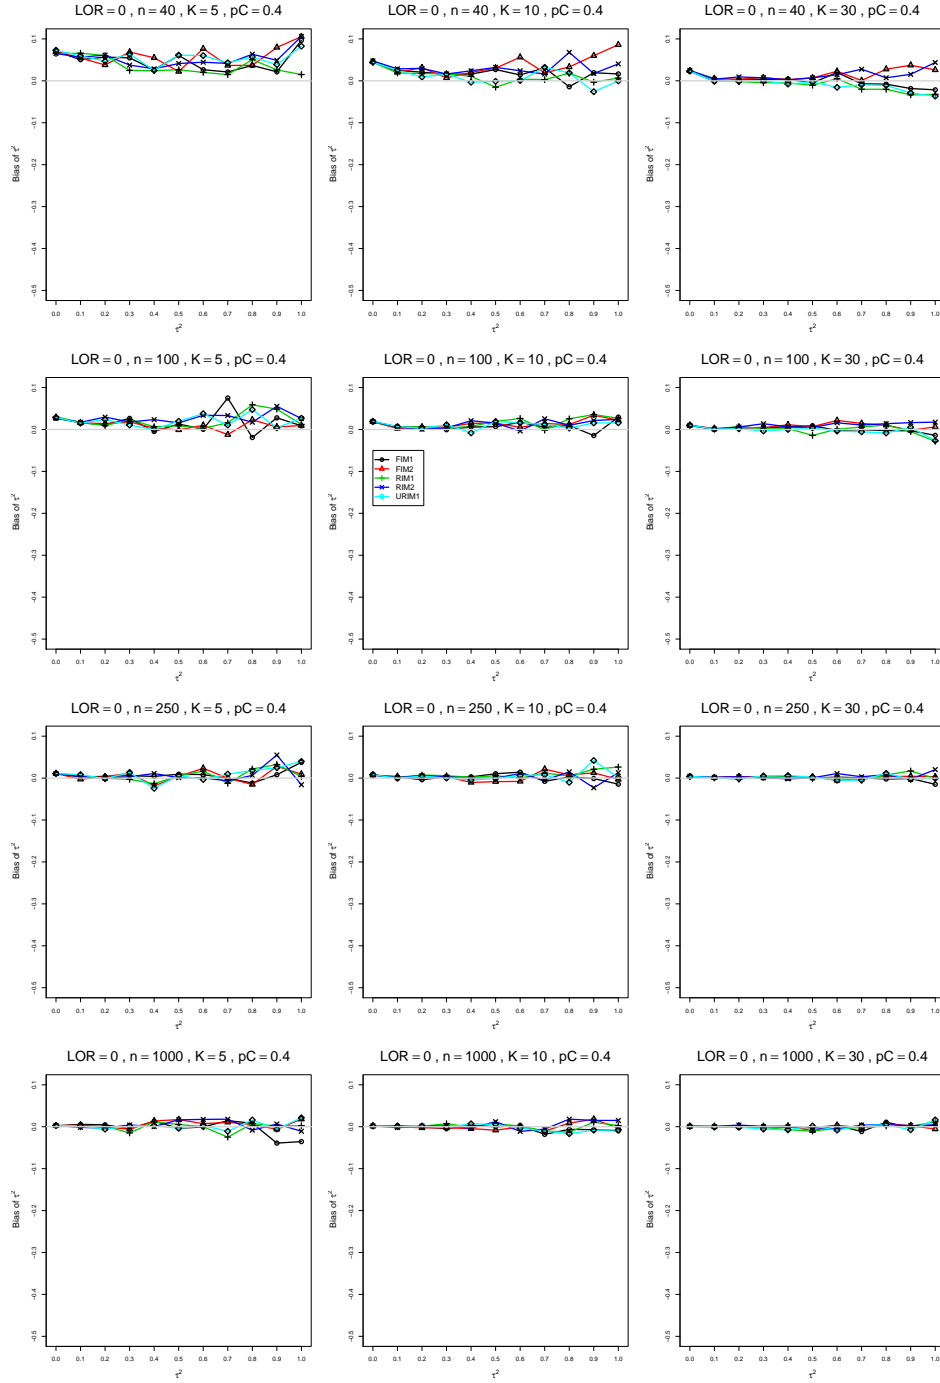

Figure A1.3.12: Bias of between-studies variance  $\hat{\tau}_{MP}^2$  for  $\theta = 0$ ,  $p_C = 0.4$ ,  $\sigma^2 = 0.4$ , constant sample sizes  $n = 40, 100, 250, 1000$ . The data-generation mechanisms are FIM1 ( $\circ$ ), FIM2 ( $\triangle$ ), RIM1 ( $+$ ), RIM2 ( $\times$ ), and URIM1 ( $\diamond$ ).

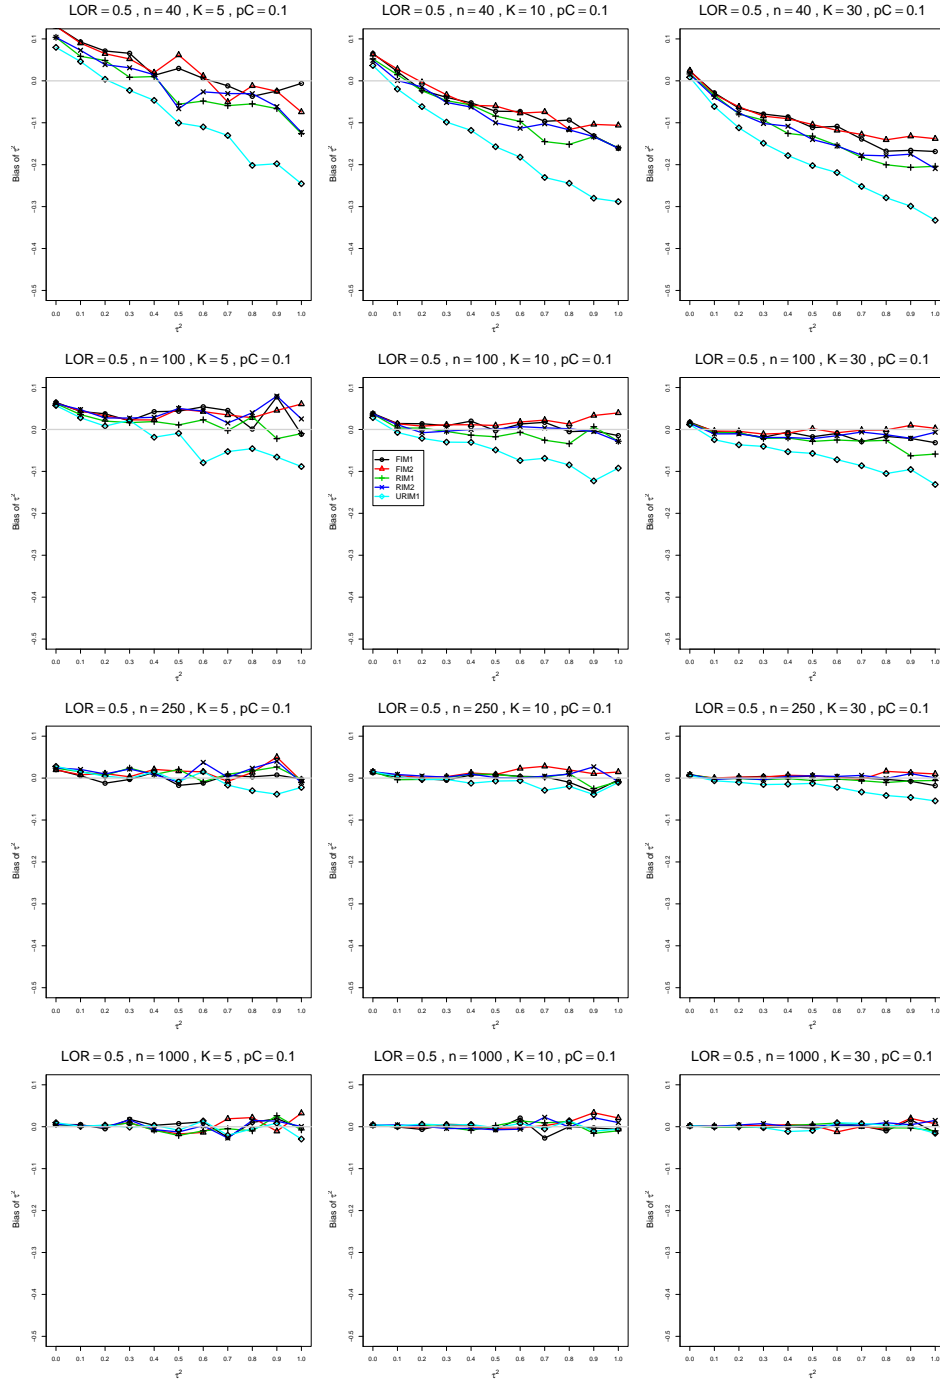

Figure A1.3.13: Bias of between-studies variance  $\hat{\tau}_{MP}^2$  for  $\theta = 0.5$ ,  $p_C = 0.1$ ,  $\sigma^2 = 0.4$ , constant sample sizes  $n = 40, 100, 250, 1000$ . The data-generation mechanisms are FIM1 ( $\circ$ ), FIM2 ( $\triangle$ ), RIM1 ( $+$ ), RIM2 ( $\times$ ), and URIM1 ( $\diamond$ ).

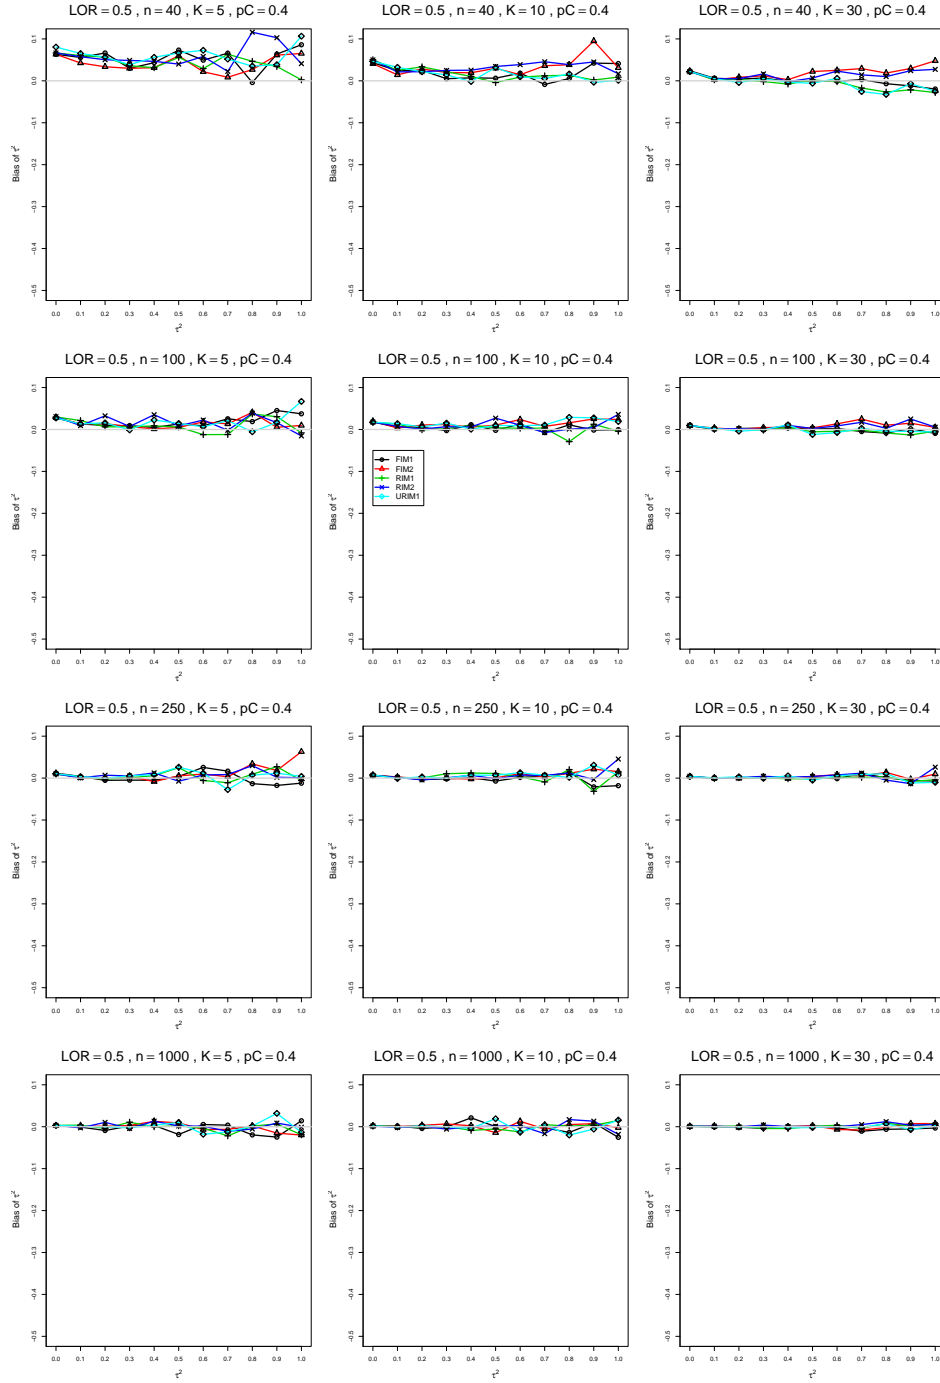

Figure A1.3.14: Bias of between-studies variance  $\hat{\tau}_{MP}^2$  for  $\theta = 0.5$ ,  $p_C = 0.4$ ,  $\sigma^2 = 0.4$ , constant sample sizes  $n = 40, 100, 250, 1000$ . The data-generation mechanisms are FIM1 ( $\circ$ ), FIM2 ( $\triangle$ ), RIM1 ( $+$ ), RIM2 ( $\times$ ), and URIM1 ( $\diamond$ ).

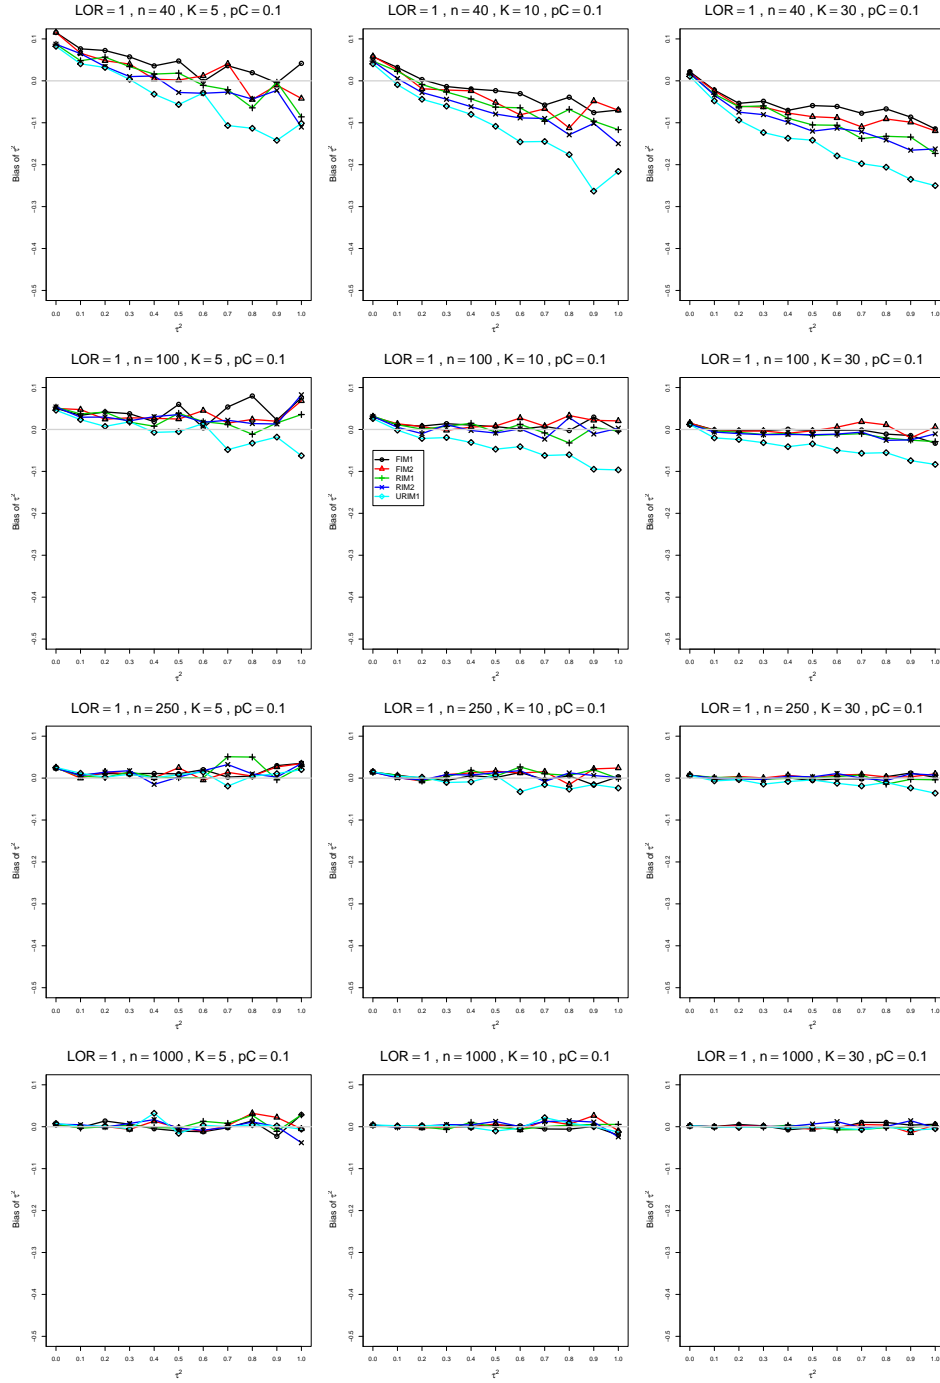

Figure A1.3.15: Bias of between-studies variance  $\hat{\tau}_{MP}^2$  for  $\theta = 1$ ,  $p_C = 0.1$ ,  $\sigma^2 = 0.4$ , constant sample sizes  $n = 40, 100, 250, 1000$ . The data-generation mechanisms are FIM1 ( $\circ$ ), FIM2 ( $\triangle$ ), RIM1 ( $+$ ), RIM2 ( $\times$ ), and URIM1 ( $\diamond$ ).



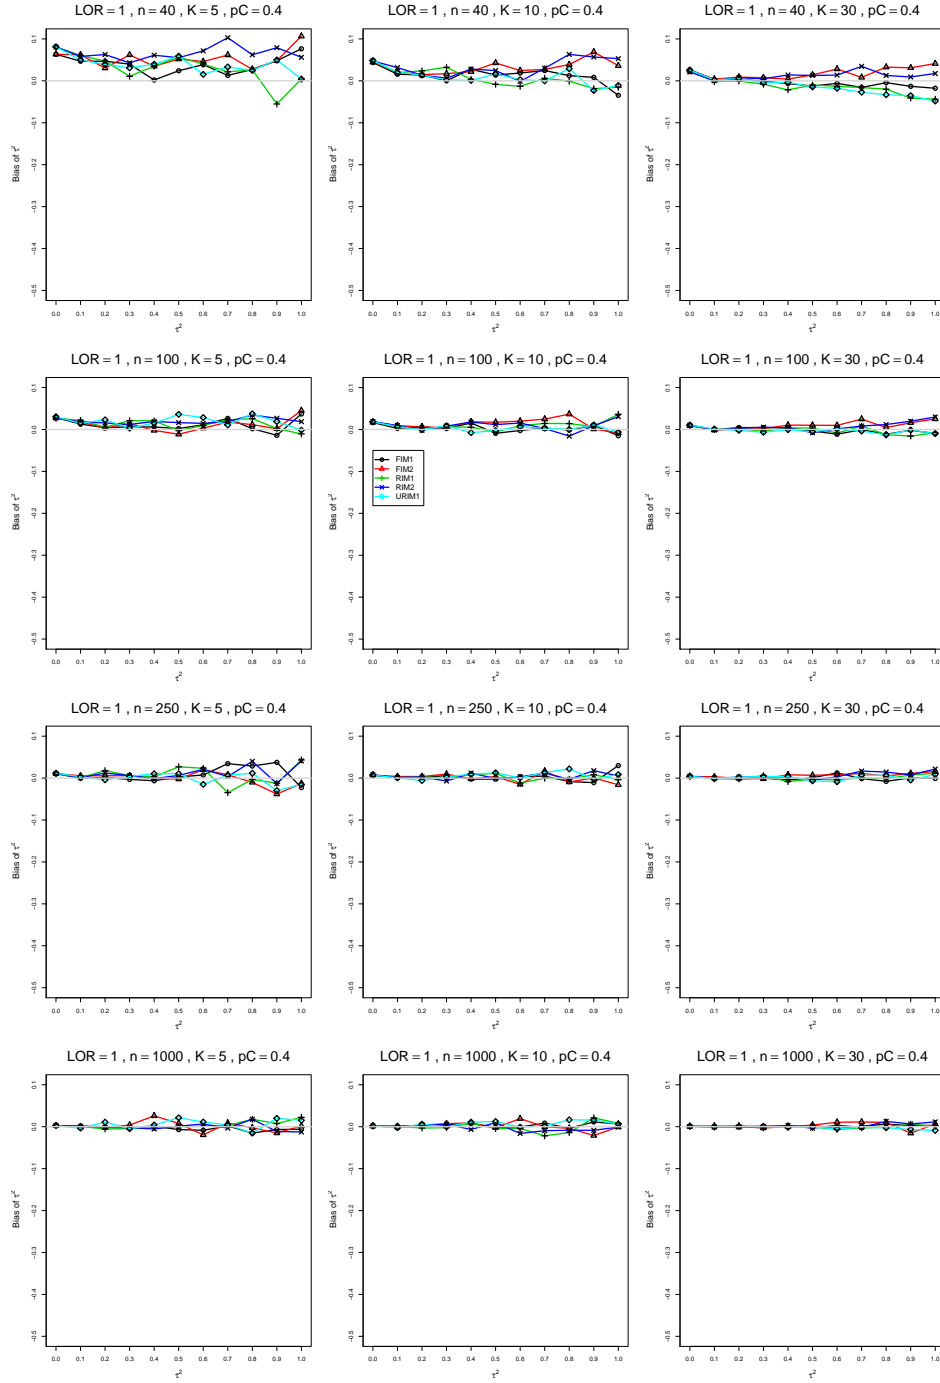

Figure A1.3.16: Bias of between-studies variance  $\hat{\tau}_{MP}^2$  for  $\theta = 1$ ,  $p_C = 0.4$ ,  $\sigma^2 = 0.4$ , constant sample sizes  $n = 40, 100, 250, 1000$ . The data-generation mechanisms are FIM1 ( $\circ$ ), FIM2 ( $\triangle$ ), RIM1 ( $+$ ), RIM2 ( $\times$ ), and URIM1 ( $\diamond$ ).

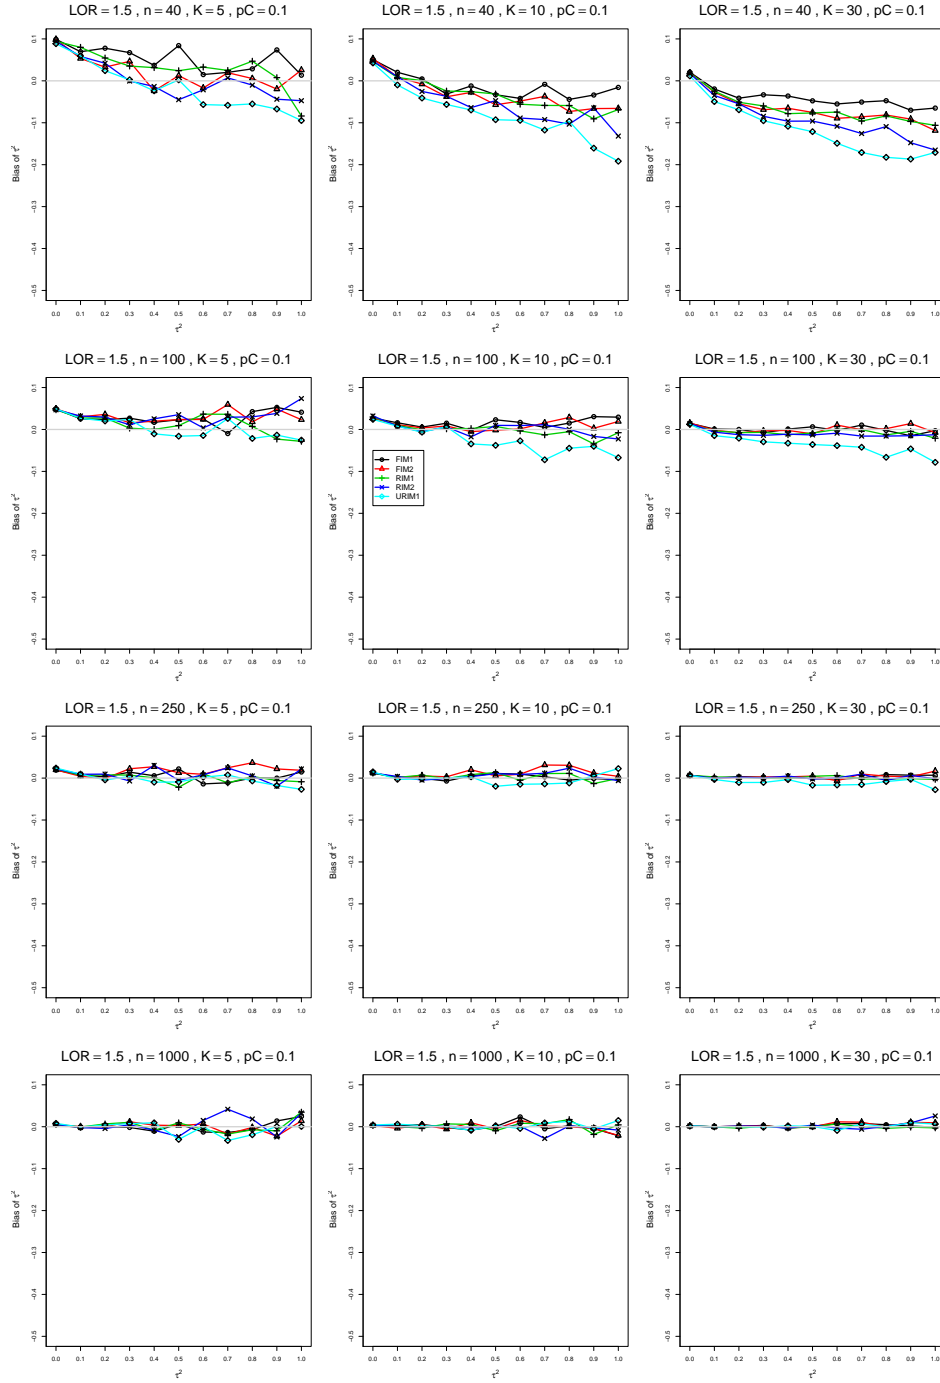

Figure A1.3.17: Bias of between-studies variance  $\hat{\tau}_{MP}^2$  for  $\theta = 1.5$ ,  $p_C = 0.1$ ,  $\sigma^2 = 0.4$ , constant sample sizes  $n = 40, 100, 250, 1000$ . The data-generation mechanisms are FIM1 ( $\circ$ ), FIM2 ( $\triangle$ ), RIM1 ( $+$ ), RIM2 ( $\times$ ), and URIM1 ( $\diamond$ ).

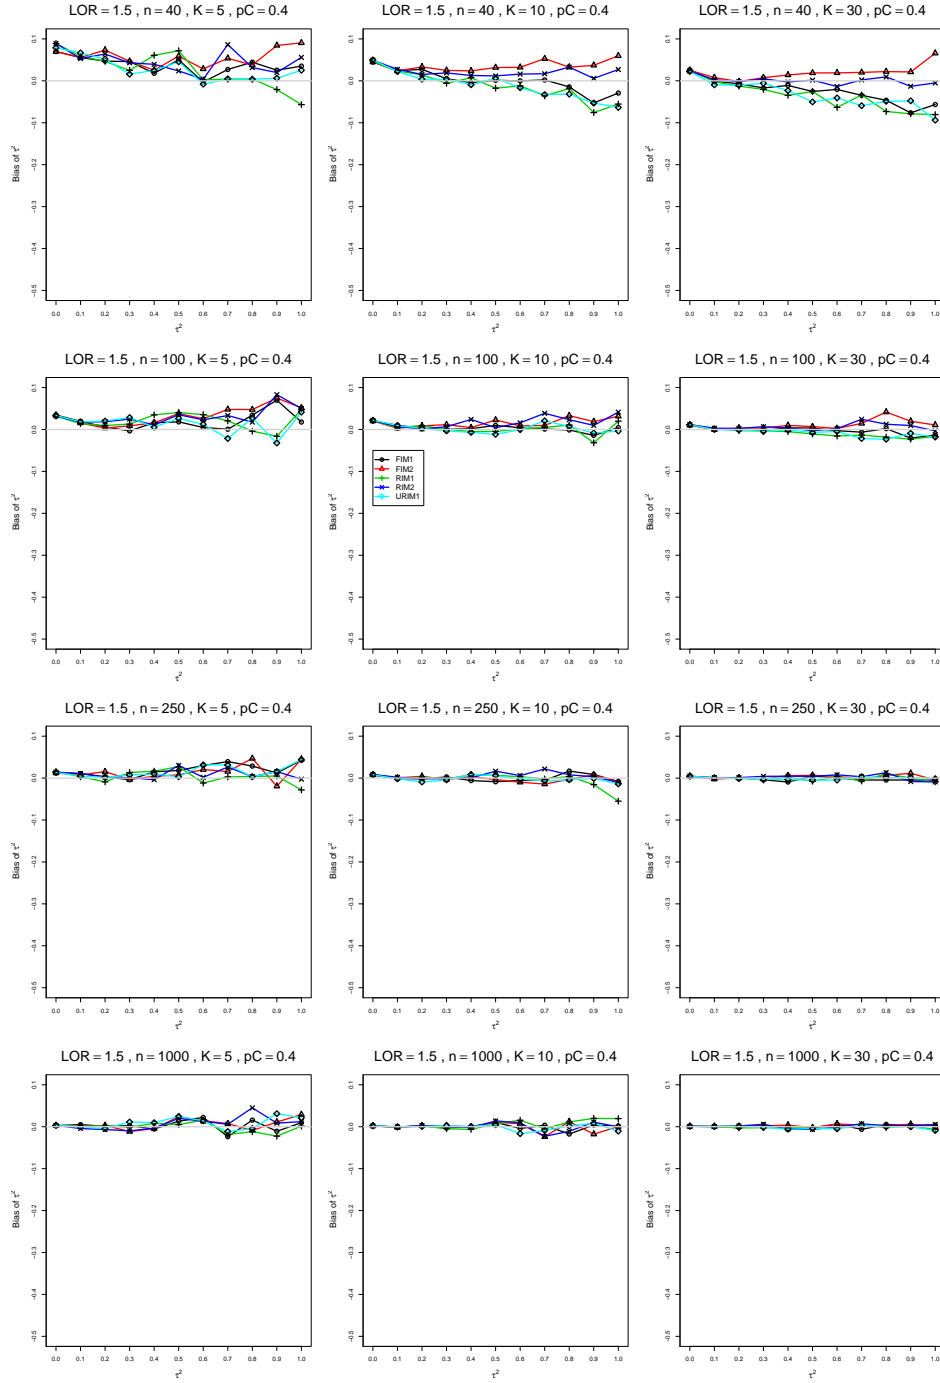

Figure A1.3.18: Bias of between-studies variance  $\hat{\tau}_{MP}^2$  for  $\theta = 1.5$ ,  $p_C = 0.4$ ,  $\sigma^2 = 0.4$ , constant sample sizes  $n = 40, 100, 250, 1000$ . The data-generation mechanisms are FIM1 ( $\circ$ ), FIM2 ( $\triangle$ ), RIM1 ( $+$ ), RIM2 ( $\times$ ), and URIM1 ( $\diamond$ ).

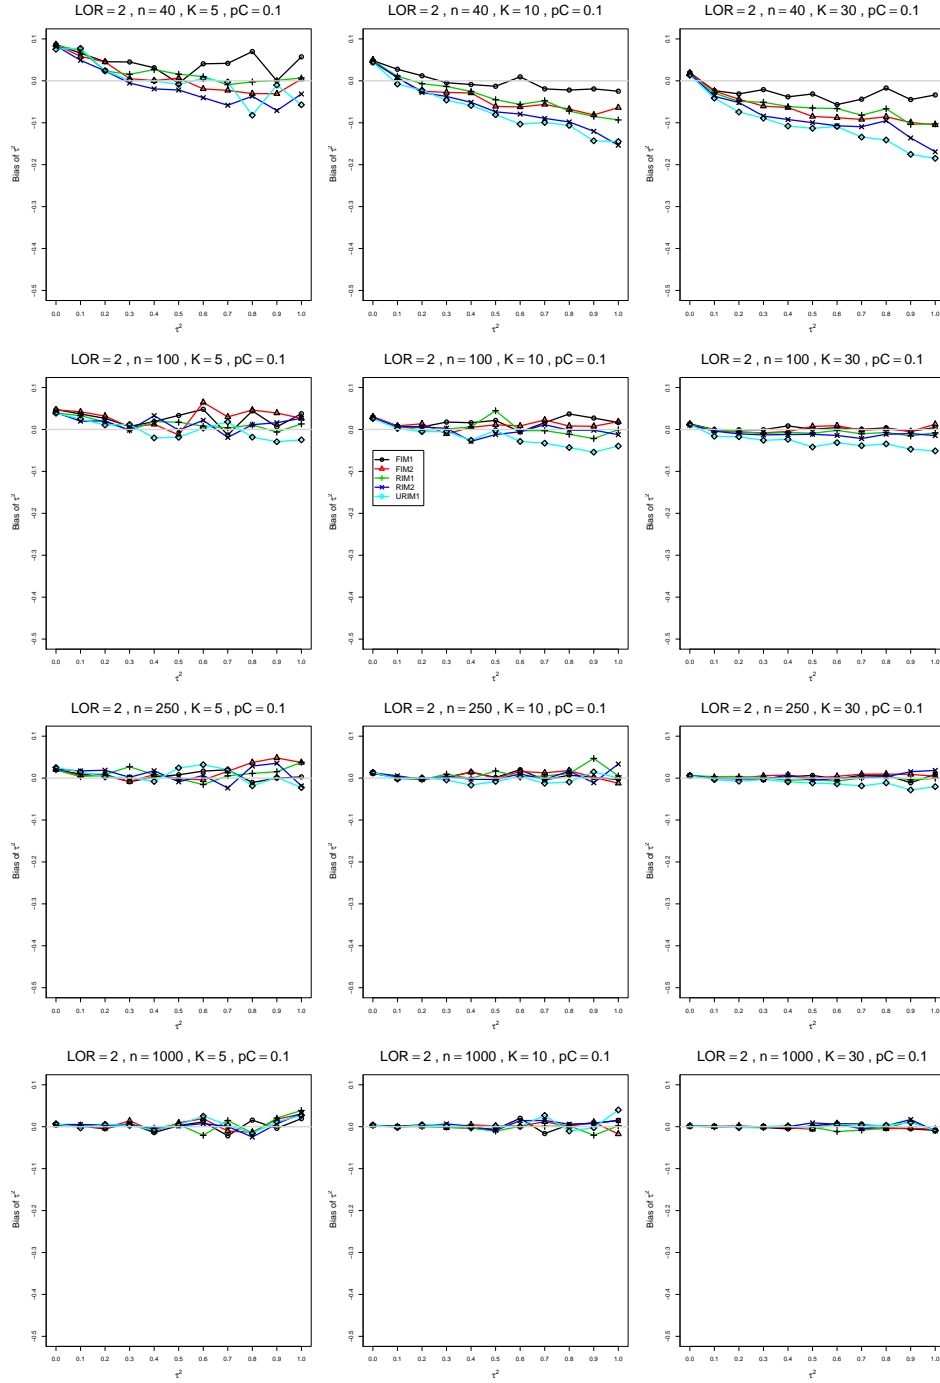

Figure A1.3.19: Bias of between-studies variance  $\hat{\tau}_{MP}^2$  for  $\theta = 2$ ,  $p_C = 0.1$ ,  $\sigma^2 = 0.4$ , constant sample sizes  $n = 40, 100, 250, 1000$ . The data-generation mechanisms are FIM1 ( $\circ$ ), FIM2 ( $\triangle$ ), RIM1 ( $+$ ), RIM2 ( $\times$ ), and URIM1 ( $\diamond$ ).

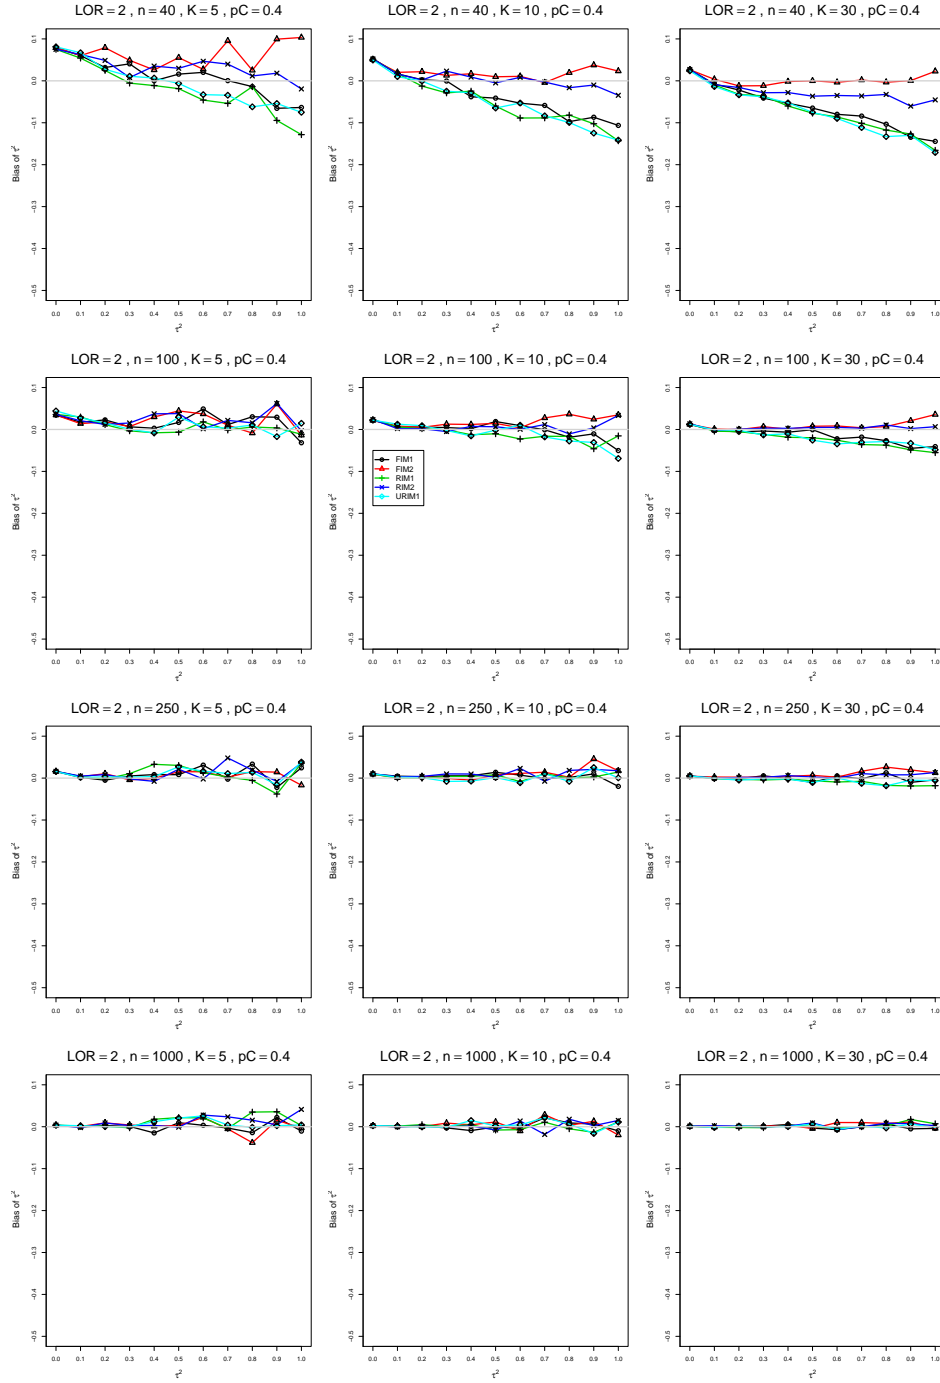

Figure A1.3.20: Bias of between-studies variance  $\hat{\tau}_{MP}^2$  for  $\theta = 2$ ,  $p_C = 0.4$ ,  $\sigma^2 = 0.4$ , constant sample sizes  $n = 40, 100, 250, 1000$ . The data-generation mechanisms are FIM1 ( $\circ$ ), FIM2 ( $\triangle$ ), RIM1 ( $+$ ), RIM2 ( $\times$ ), and URIM1 ( $\diamond$ ).

#### A1.4 Bias of $\hat{\tau}_{KD}^2$

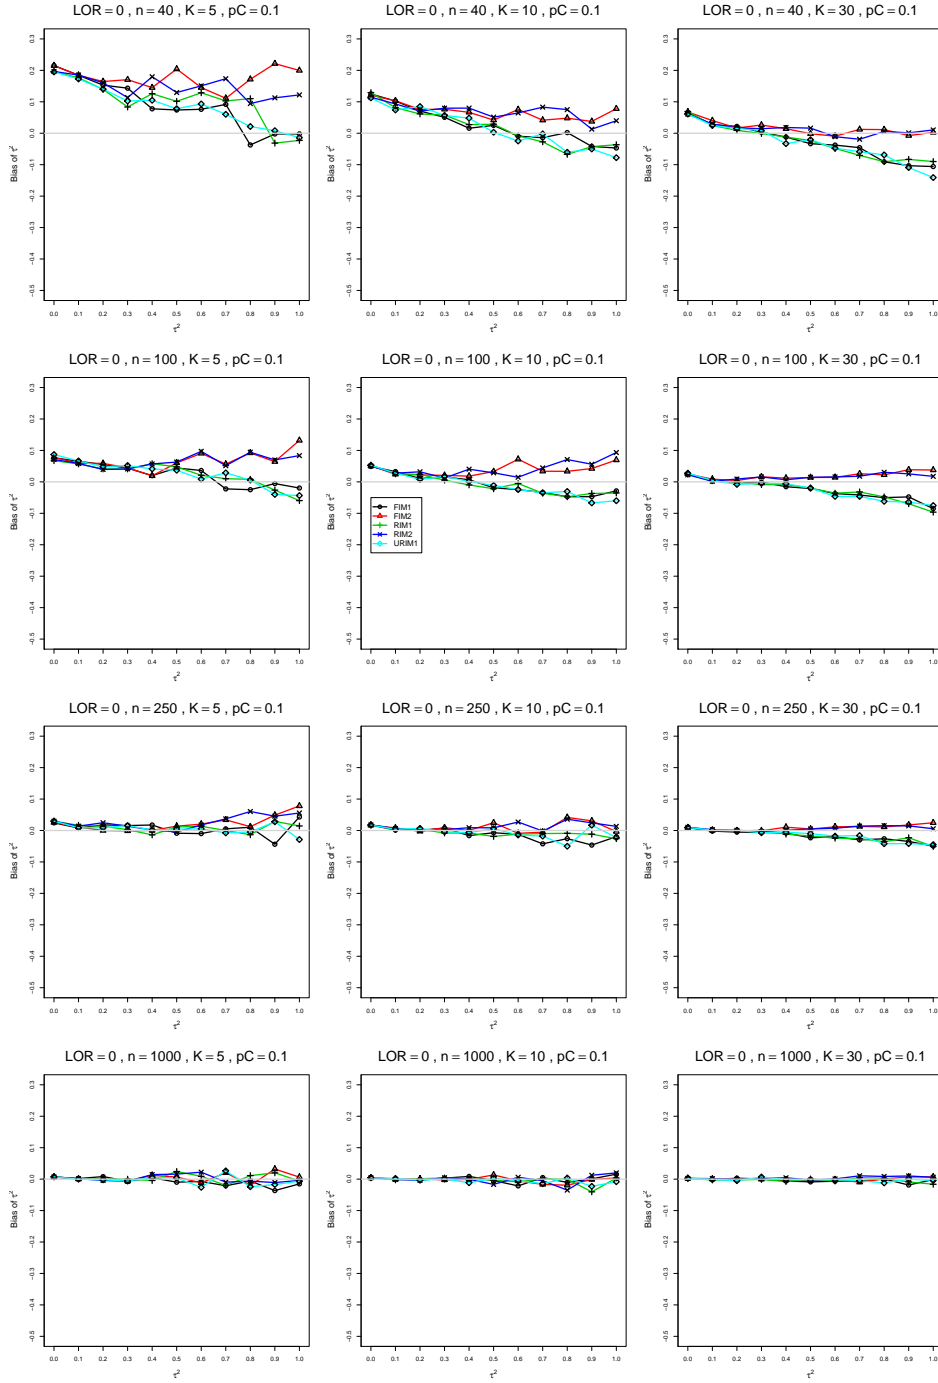

Figure A1.4.1: Bias of between-studies variance  $\hat{\tau}_{KD}^2$  for  $\theta = 0$ ,  $p_C = 0.1$ ,  $\sigma^2 = 0.1$ , constant sample sizes  $n = 40, 100, 250, 1000$ . The data-generation mechanisms are FIM1 ( $\circ$ ), FIM2 ( $\triangle$ ), RIM1 ( $+$ ), RIM2 ( $\times$ ), and URIM1 ( $\diamond$ ).

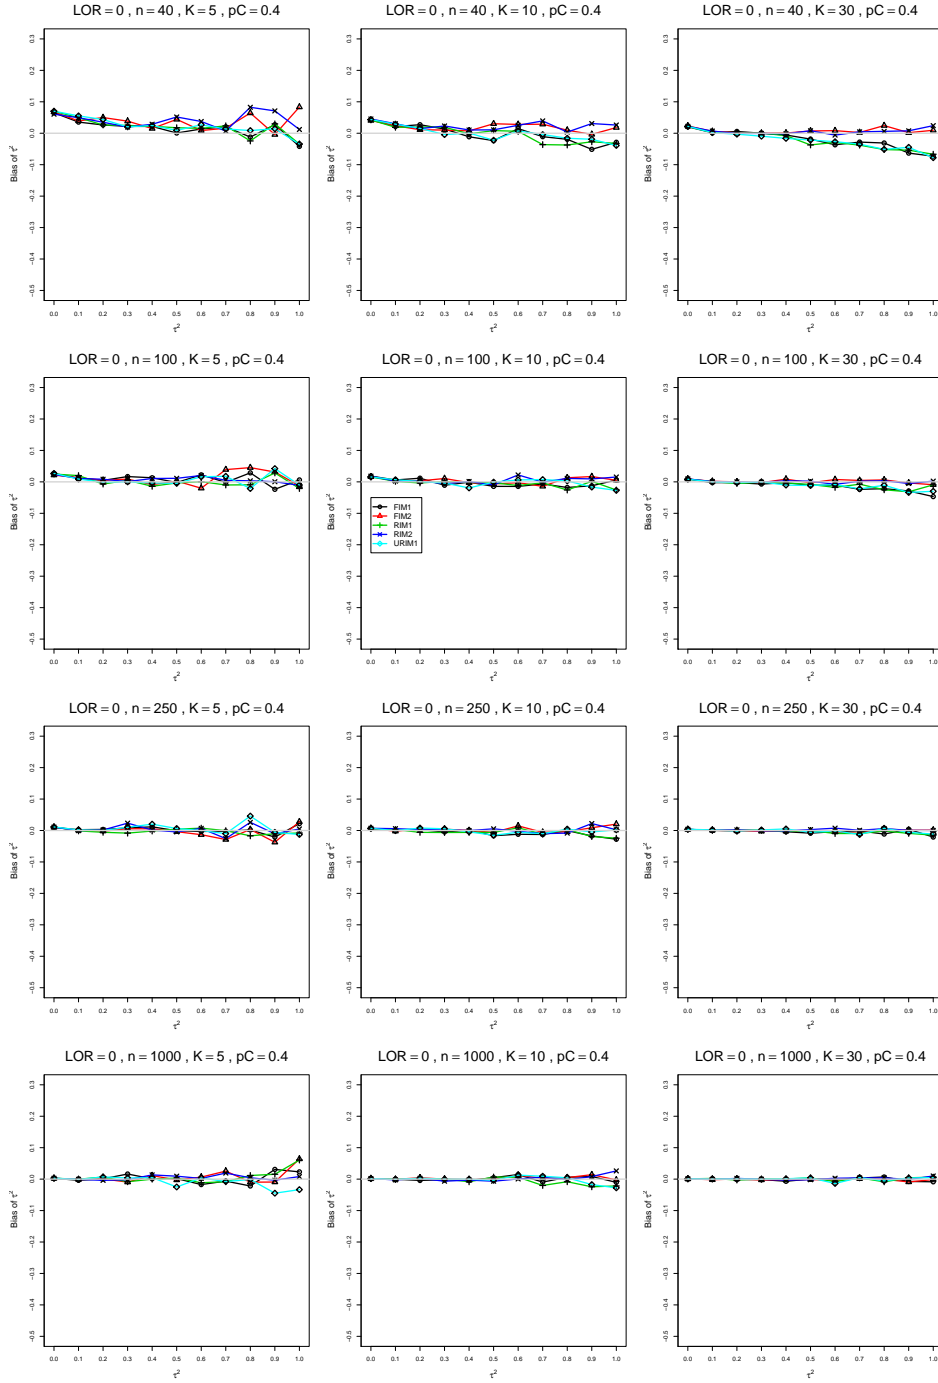

Figure A1.4.2: Bias of between-studies variance  $\hat{\tau}_{KD}^2$  for  $\theta = 0$ ,  $p_C = 0.4$ ,  $\sigma^2 = 0.1$ , constant sample sizes  $n = 40, 100, 250, 1000$ . The data-generation mechanisms are FIM1 ( $\circ$ ), FIM2 ( $\triangle$ ), RIM1 ( $+$ ), RIM2 ( $\times$ ), and URIM1 ( $\diamond$ ).



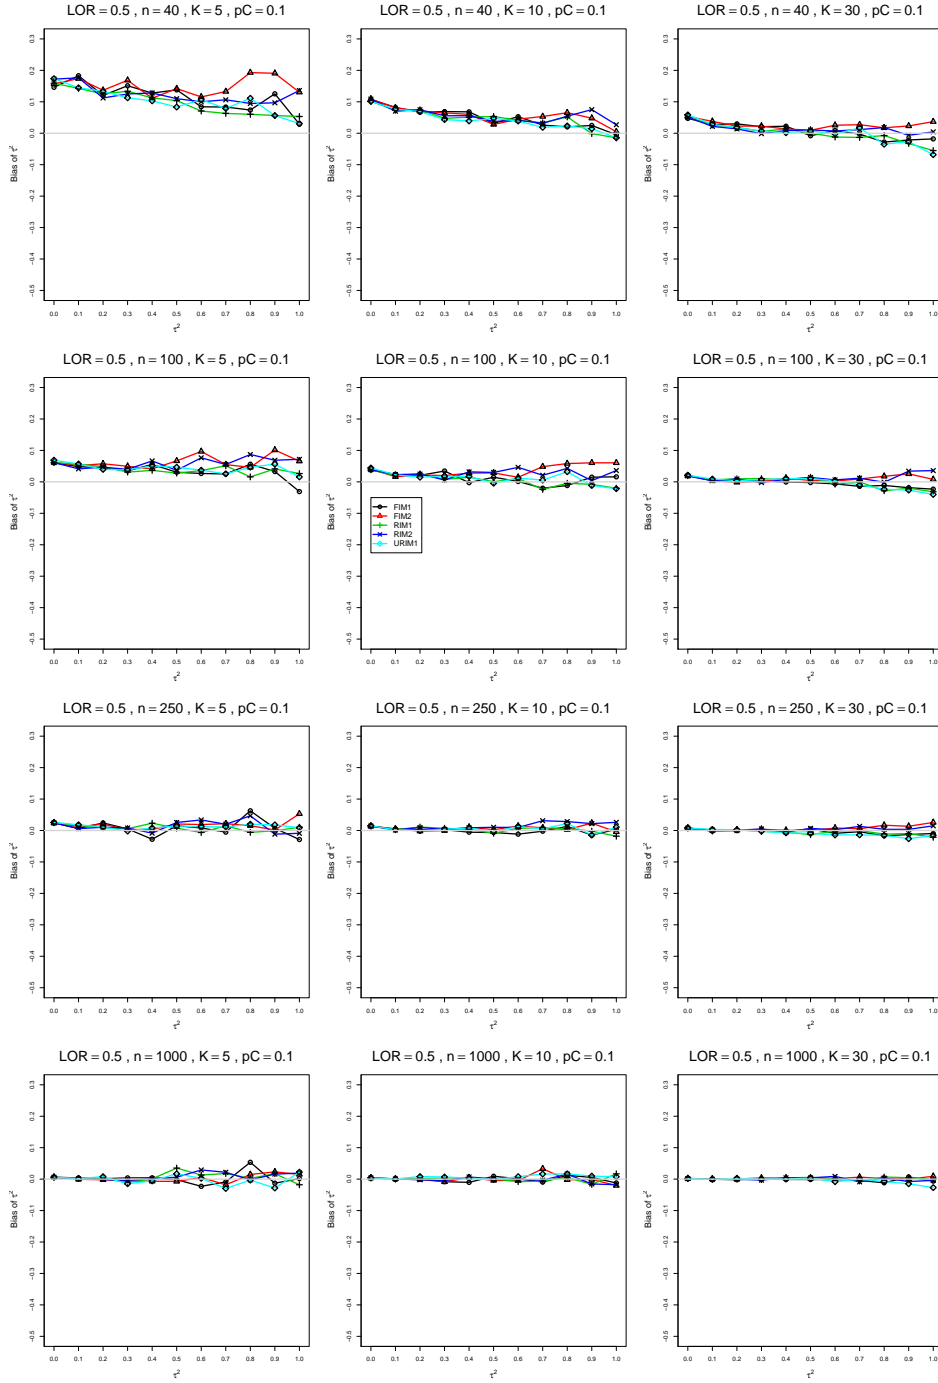

Figure A1.4.3: Bias of between-studies variance  $\hat{\tau}_{KD}^2$  for  $\theta = 0.5$ ,  $p_C = 0.1$ ,  $\sigma^2 = 0.1$ , constant sample sizes  $n = 40, 100, 250, 1000$ . The data-generation mechanisms are FIM1 ( $\circ$ ), FIM2 ( $\triangle$ ), RIM1 ( $+$ ), RIM2 ( $\times$ ), and URIM1 ( $\diamond$ ).

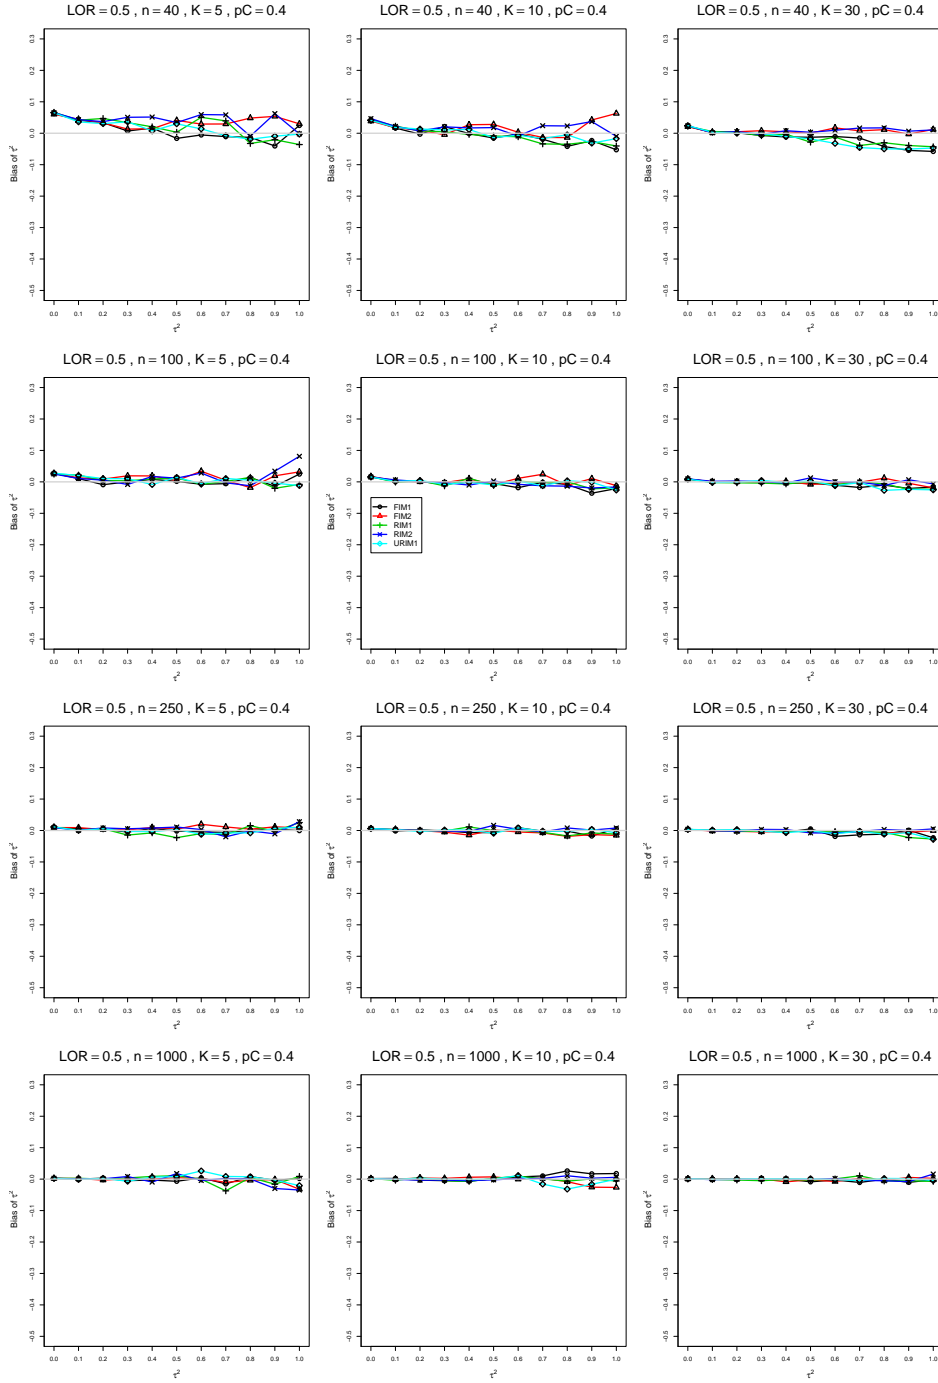

Figure A1.4.4: Bias of between-studies variance  $\hat{\tau}_{KD}^2$  for  $\theta = 0.5$ ,  $p_C = 0.4$ ,  $\sigma^2 = 0.1$ , constant sample sizes  $n = 40, 100, 250, 1000$ . The data-generation mechanisms are FIM1 ( $\circ$ ), FIM2 ( $\triangle$ ), RIM1 ( $+$ ), RIM2 ( $\times$ ), and URIM1 ( $\diamond$ ).

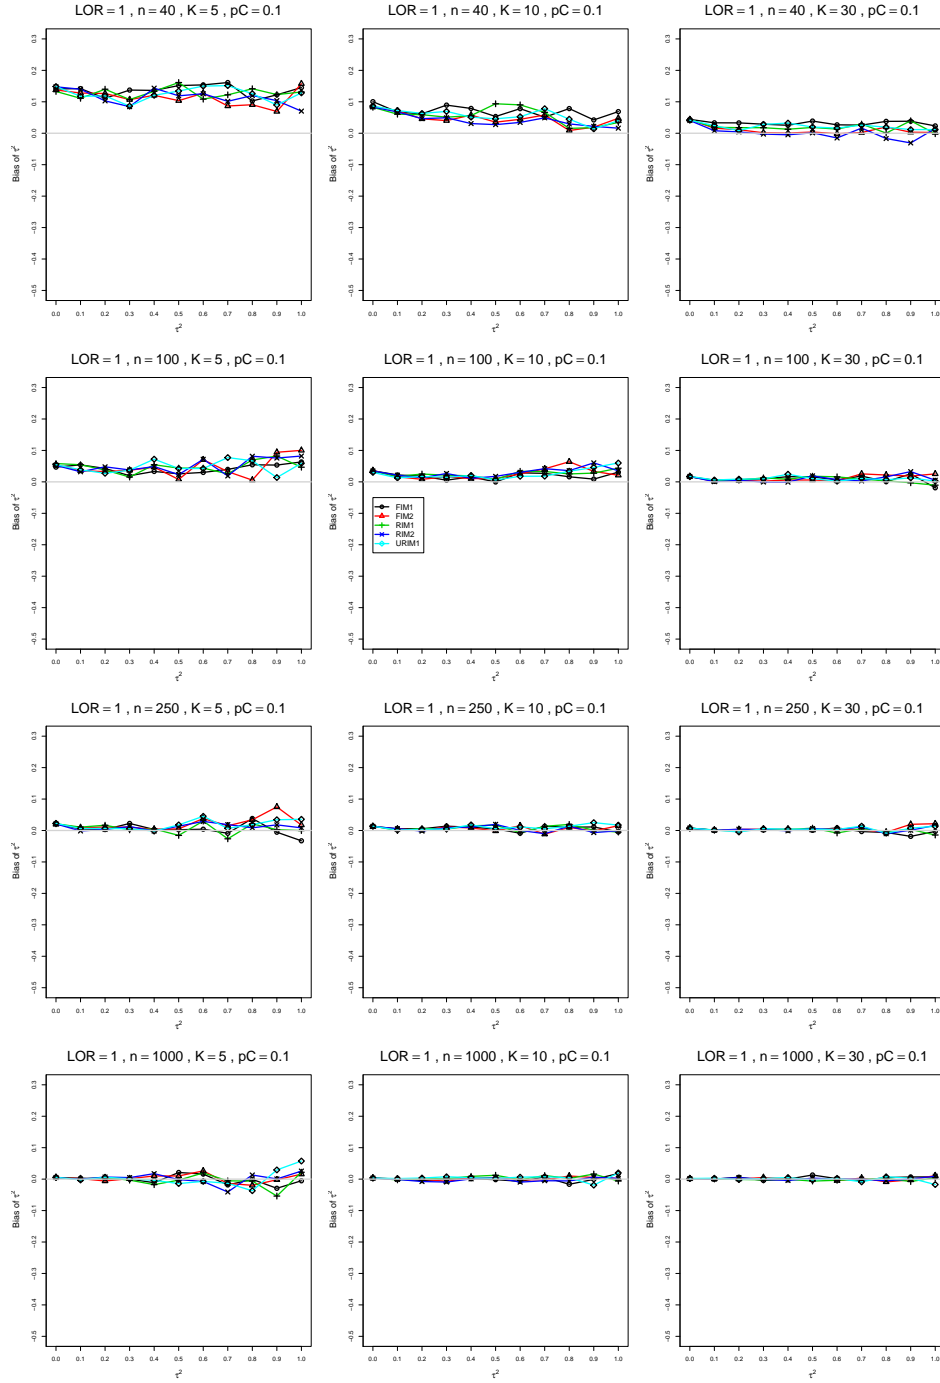

Figure A1.4.5: Bias of between-studies variance  $\hat{\tau}_{KD}^2$  for  $\theta = 1$ ,  $p_C = 0.1$ ,  $\sigma^2 = 0.1$ , constant sample sizes  $n = 40, 100, 250, 1000$ . The data-generation mechanisms are FIM1 ( $\circ$ ), FIM2 ( $\triangle$ ), RIM1 ( $+$ ), RIM2 ( $\times$ ), and URIM1 ( $\diamond$ ).

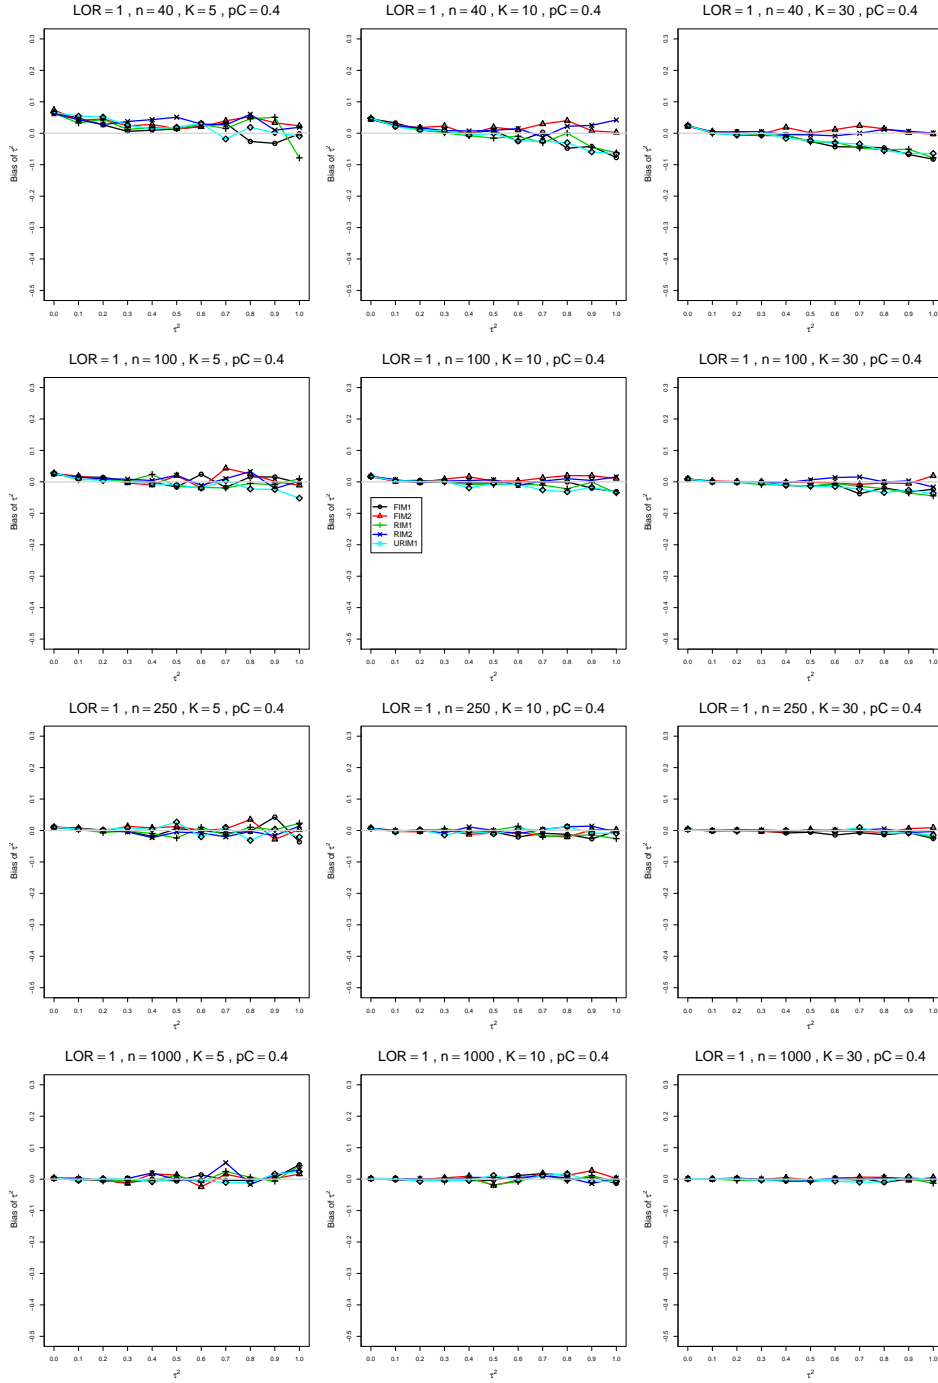

Figure A1.4.6: Bias of between-studies variance  $\hat{\tau}_{KD}^2$  for  $\theta = 1$ ,  $p_C = 0.4$ ,  $\sigma^2 = 0.1$ , constant sample sizes  $n = 40, 100, 250, 1000$ . The data-generation mechanisms are FIM1 ( $\circ$ ), FIM2 ( $\triangle$ ), RIM1 ( $+$ ), RIM2 ( $\times$ ), and URIM1 ( $\diamond$ ).

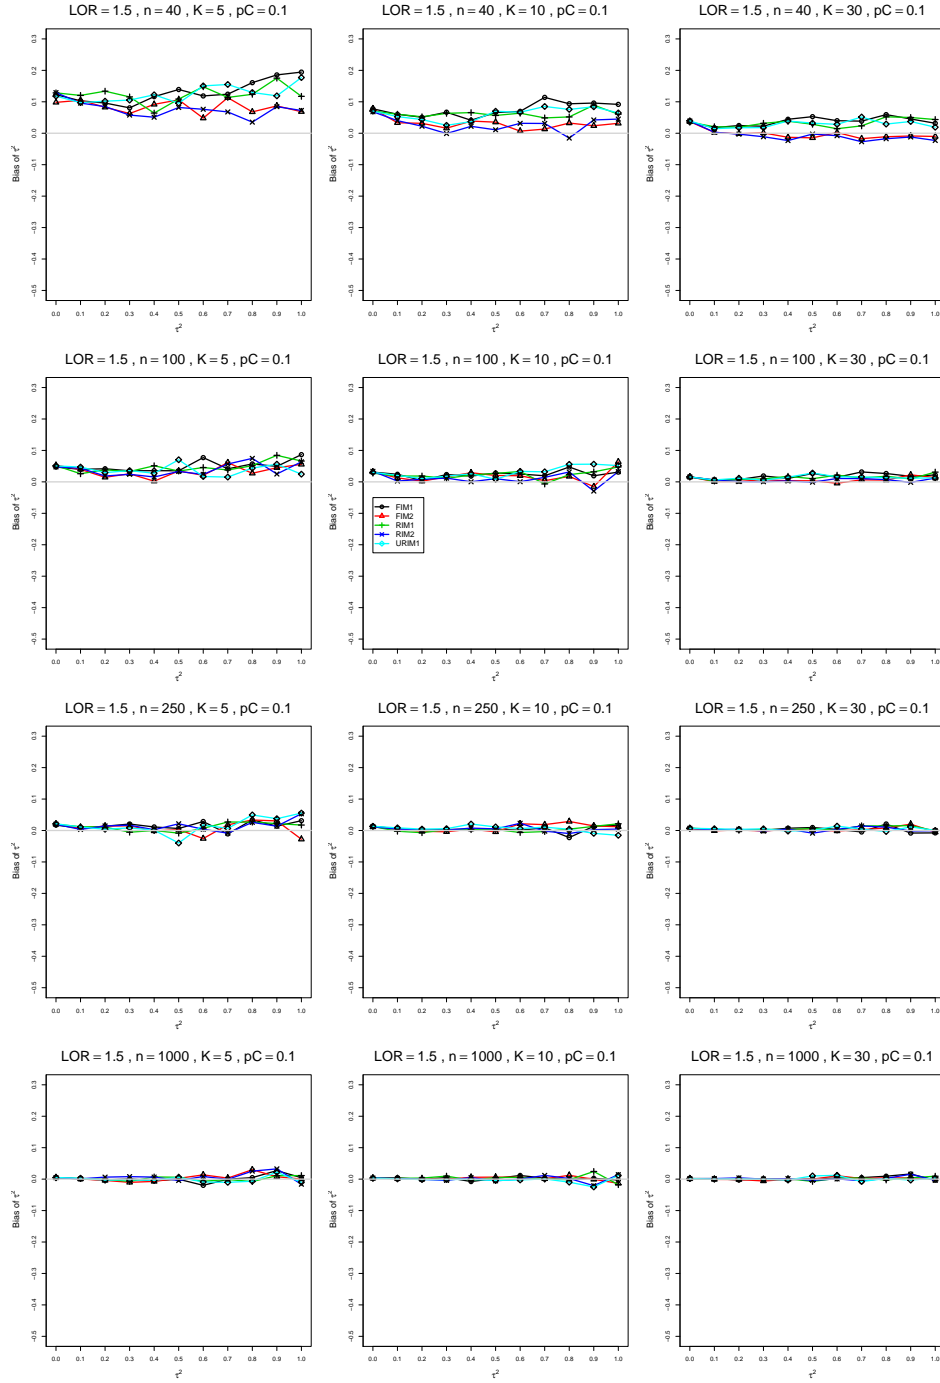

Figure A1.4.7: Bias of between-studies variance  $\hat{\tau}_{KD}^2$  for  $\theta = 1.5$ ,  $p_C = 0.1$ ,  $\sigma^2 = 0.1$ , constant sample sizes  $n = 40, 100, 250, 1000$ . The data-generation mechanisms are FIM1 ( $\circ$ ), FIM2 ( $\triangle$ ), RIM1 ( $+$ ), RIM2 ( $\times$ ), and URIM1 ( $\diamond$ ).

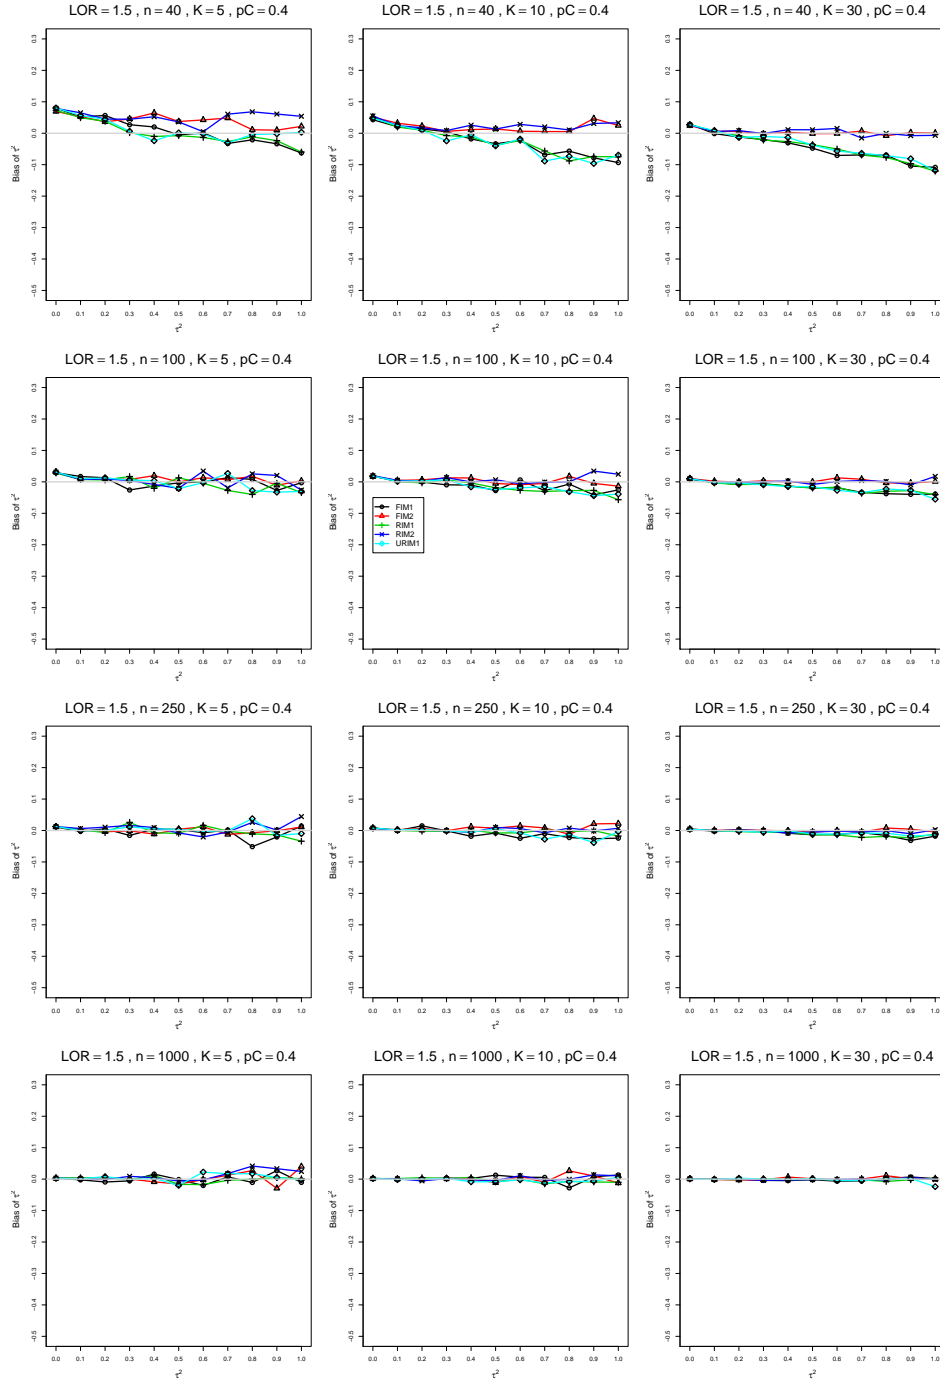

Figure A1.4.8: Bias of between-studies variance  $\hat{\tau}_{KD}^2$  for  $\theta = 1.5$ ,  $p_C = 0.4$ ,  $\sigma^2 = 0.1$ , constant sample sizes  $n = 40, 100, 250, 1000$ . The data-generation mechanisms are FIM1 ( $\circ$ ), FIM2 ( $\triangle$ ), RIM1 ( $+$ ), RIM2 ( $\times$ ), and URIM1 ( $\diamond$ ).

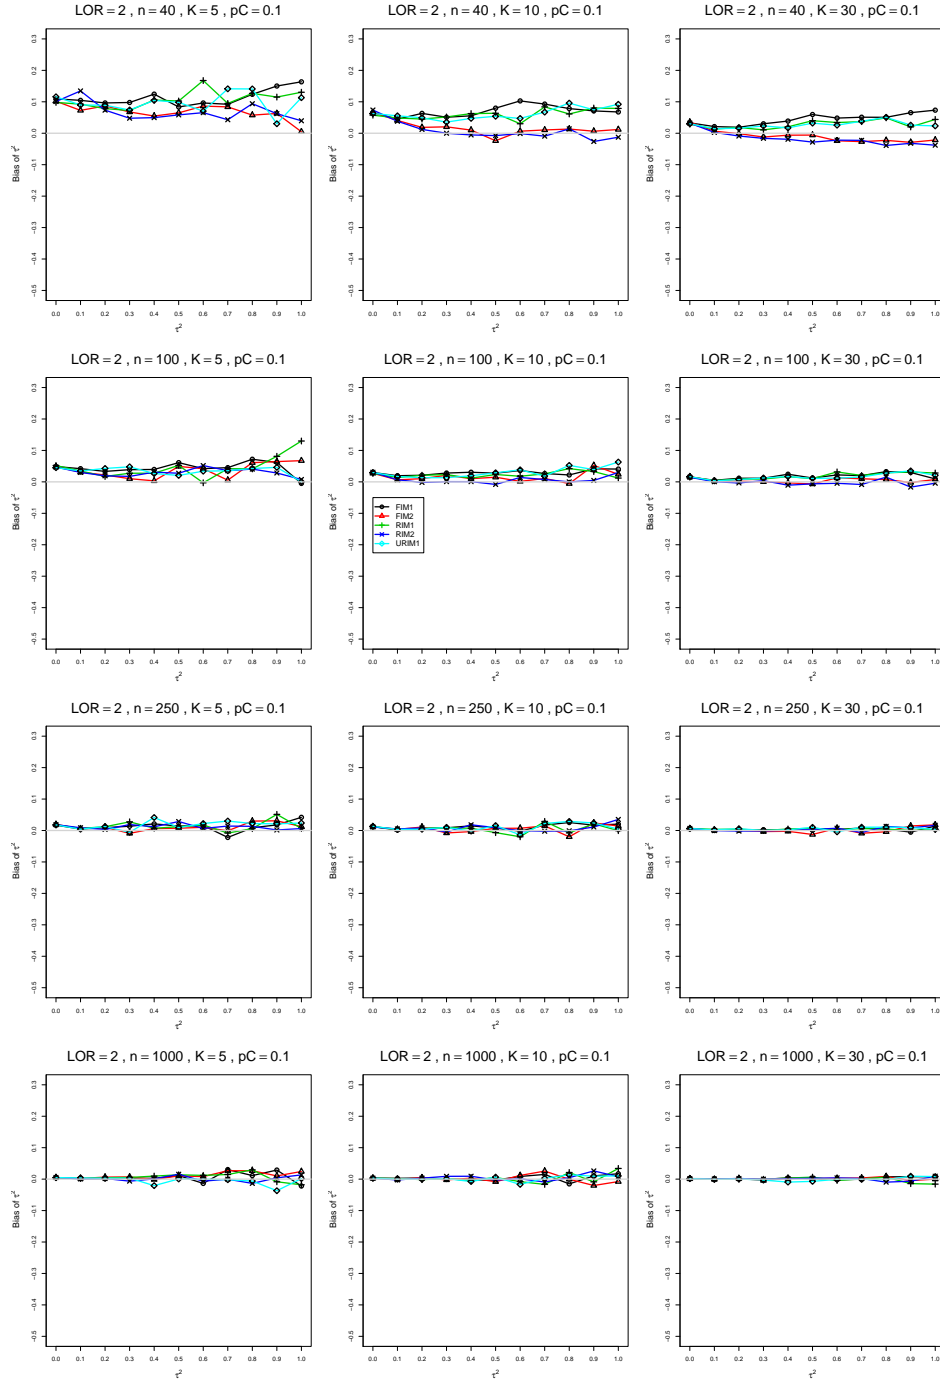

Figure A1.4.9: Bias of between-studies variance  $\hat{\tau}_{KD}^2$  for  $\theta = 2$ ,  $p_C = 0.1$ ,  $\sigma^2 = 0.1$ , constant sample sizes  $n = 40, 100, 250, 1000$ . The data-generation mechanisms are FIM1 ( $\circ$ ), FIM2 ( $\triangle$ ), RIM1 ( $+$ ), RIM2 ( $\times$ ), and URIM1 ( $\diamond$ ).

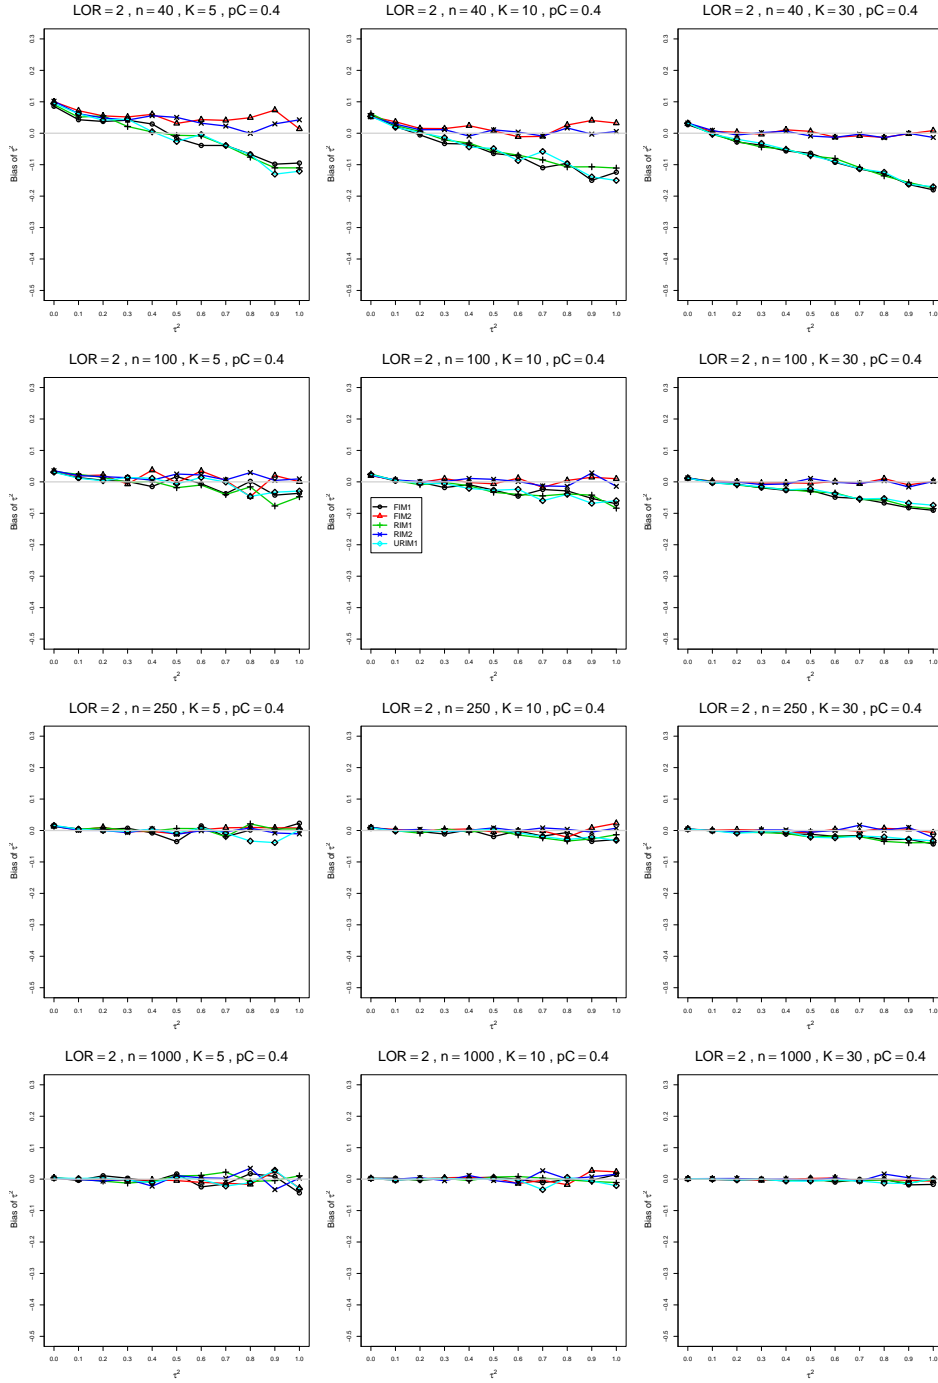

Figure A1.4.10: Bias of between-studies variance  $\hat{\tau}_{KD}^2$  for  $\theta = 2$ ,  $p_C = 0.4$ ,  $\sigma^2 = 0.1$ , constant sample sizes  $n = 40, 100, 250, 1000$ . The data-generation mechanisms are FIM1 ( $\circ$ ), FIM2 ( $\triangle$ ), RIM1 ( $+$ ), RIM2 ( $\times$ ), and URIM1 ( $\diamond$ ).



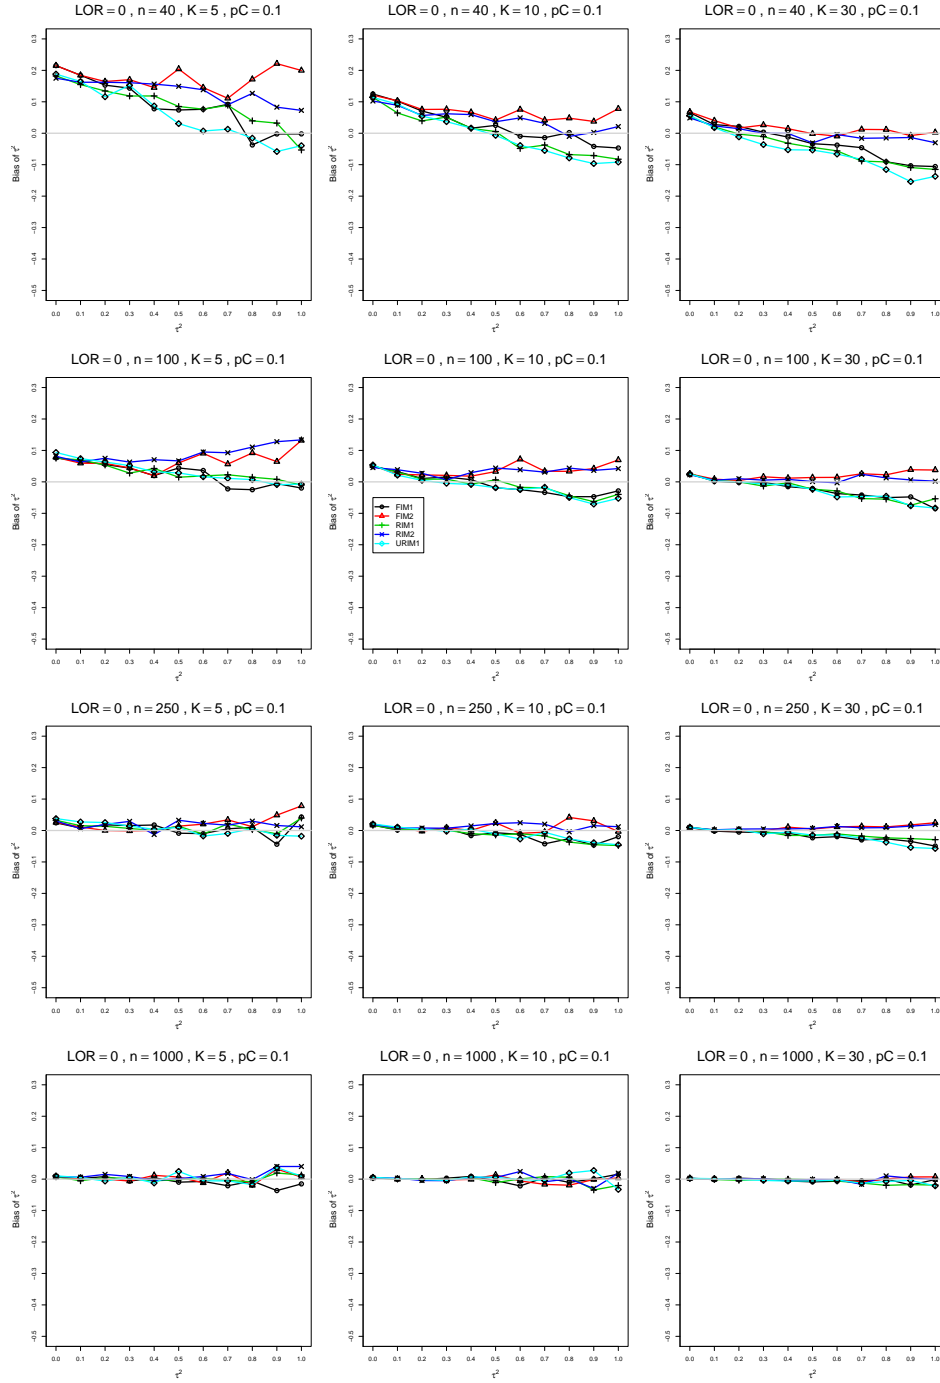

Figure A1.4.11: Bias of between-studies variance  $\hat{\tau}_{KD}^2$  for  $\theta = 0$ ,  $p_C = 0.1$ ,  $\sigma^2 = 0.4$ , constant sample sizes  $n = 40, 100, 250, 1000$ . The data-generation mechanisms are FIM1 ( $\circ$ ), FIM2 ( $\triangle$ ), RIM1 ( $+$ ), RIM2 ( $\times$ ), and URIM1 ( $\diamond$ ).

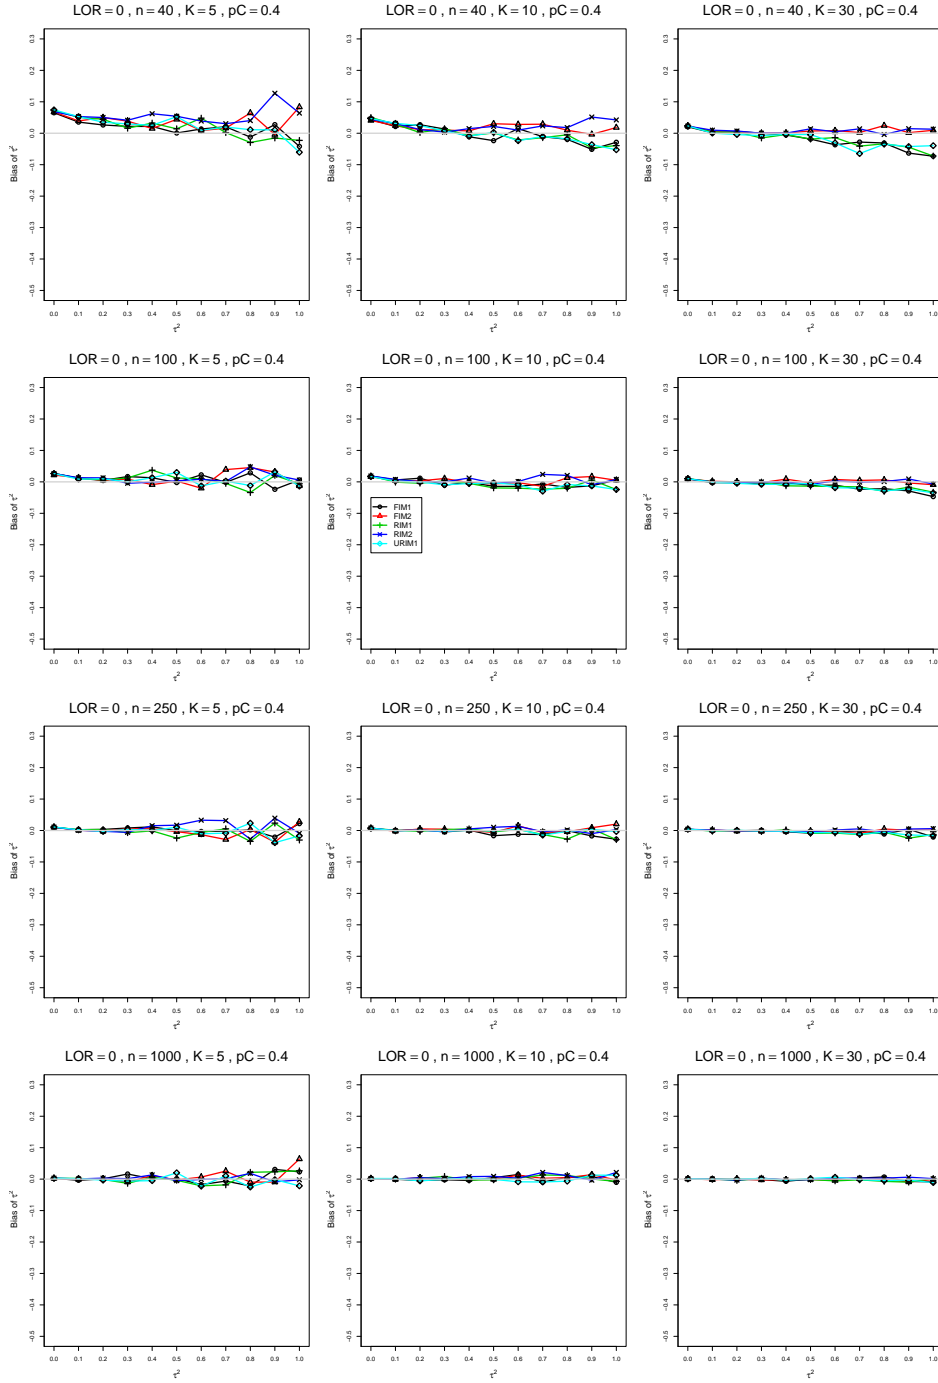

Figure A1.4.12: Bias of between-studies variance  $\hat{\tau}_{KD}^2$  for  $\theta = 0$ ,  $p_C = 0.4$ ,  $\sigma^2 = 0.4$ , constant sample sizes  $n = 40, 100, 250, 1000$ . The data-generation mechanisms are FIM1 ( $\circ$ ), FIM2 ( $\triangle$ ), RIM1 ( $+$ ), RIM2 ( $\times$ ), and URIM1 ( $\diamond$ ).

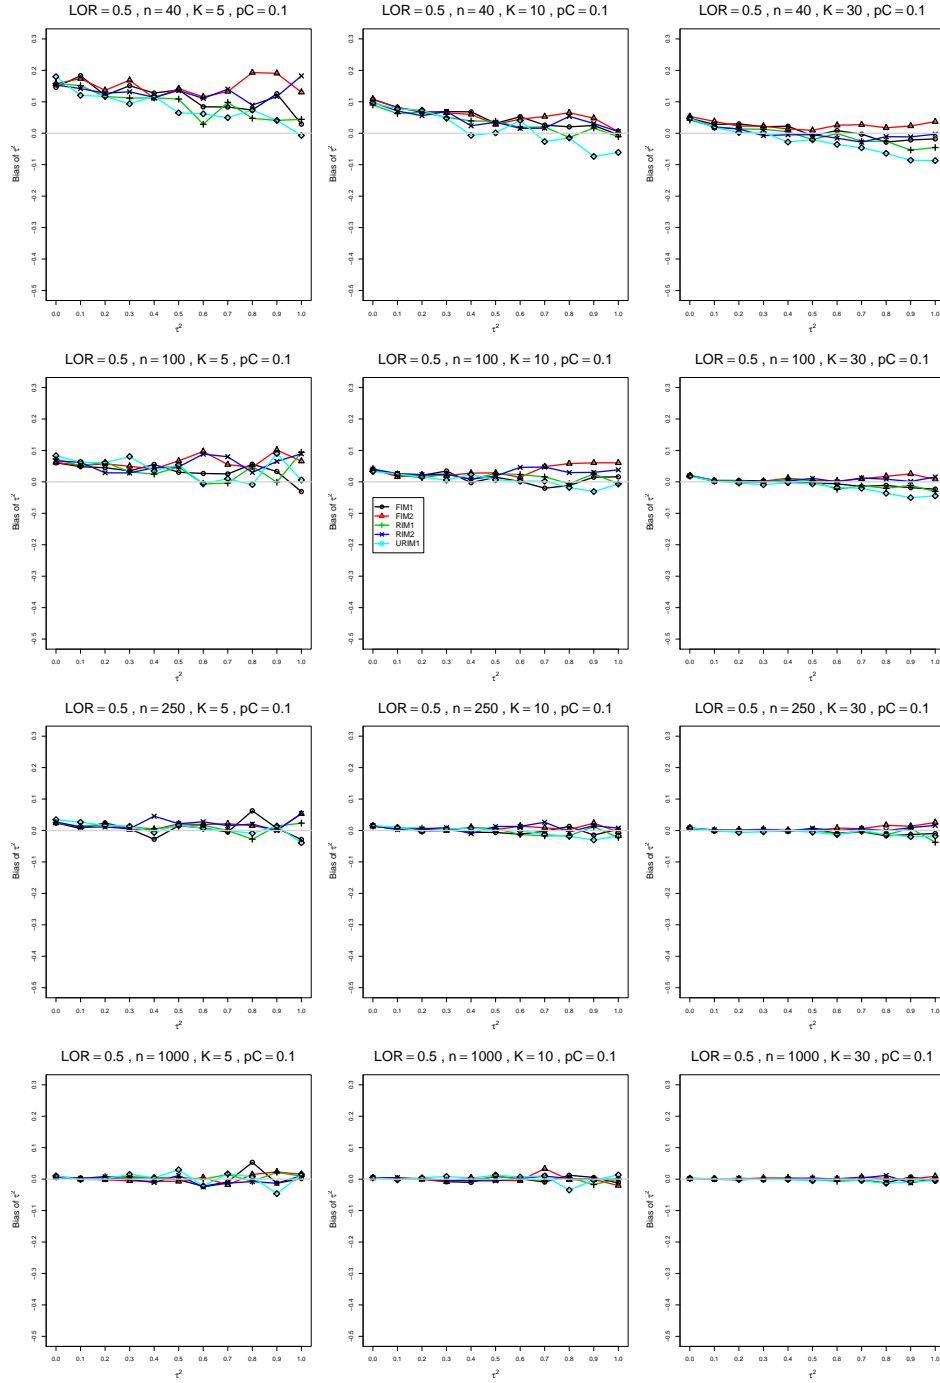

Figure A1.4.13: Bias of between-studies variance  $\hat{\tau}_{KD}^2$  for  $\theta = 0.5$ ,  $p_C = 0.1$ ,  $\sigma^2 = 0.4$ , constant sample sizes  $n = 40, 100, 250, 1000$ . The data-generation mechanisms are FIM1 ( $\circ$ ), FIM2 ( $\triangle$ ), RIM1 ( $+$ ), RIM2 ( $\times$ ), and URIM1 ( $\diamond$ ).

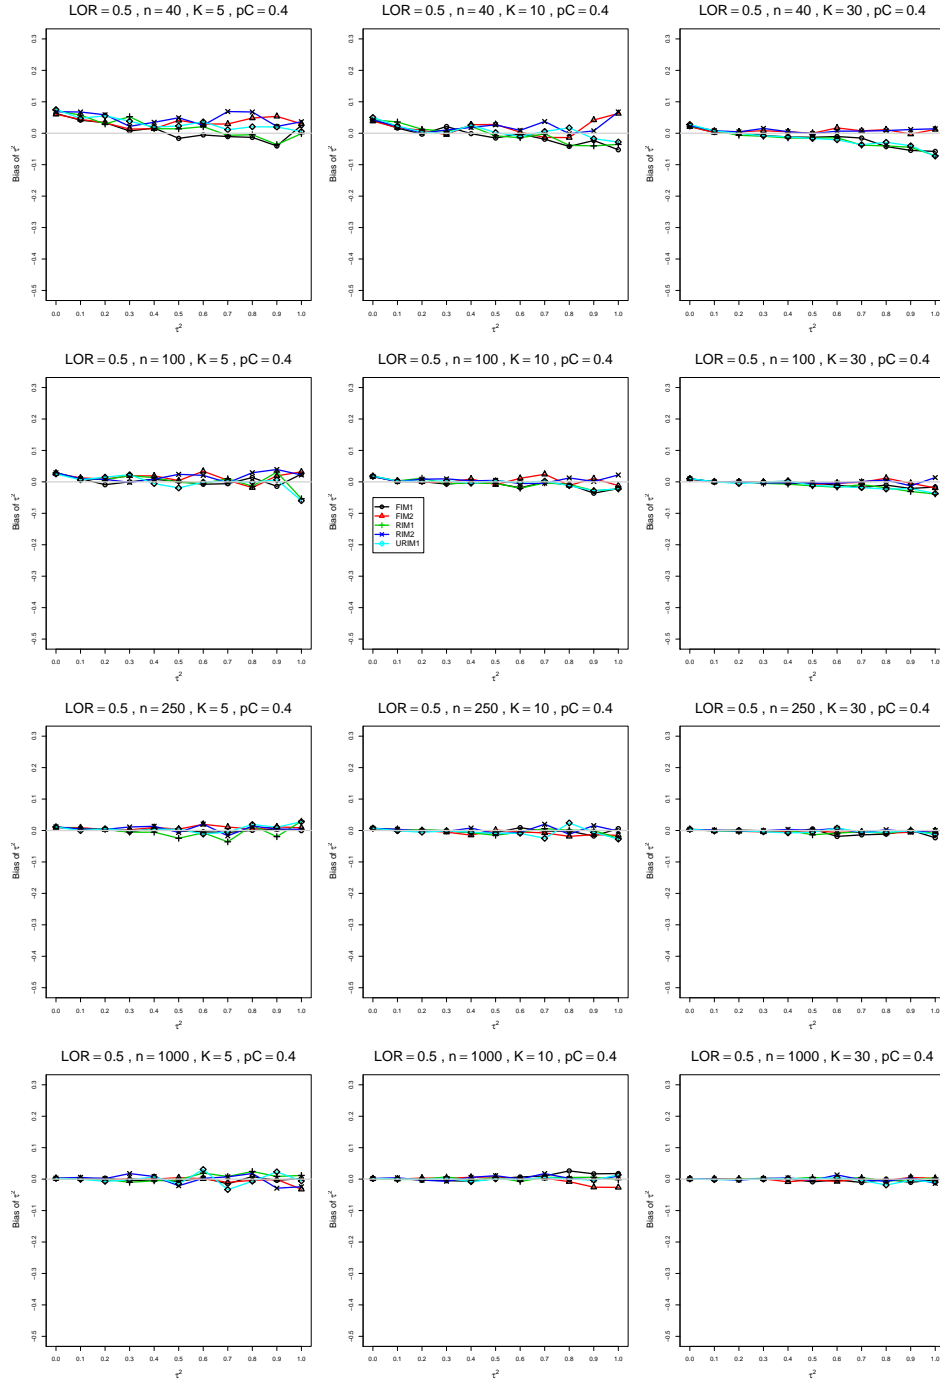

Figure A1.4.14: Bias of between-studies variance  $\hat{\tau}_{KD}^2$  for  $\theta = 0.5$ ,  $p_C = 0.4$ ,  $\sigma^2 = 0.4$ , constant sample sizes  $n = 40, 100, 250, 1000$ . The data-generation mechanisms are FIM1 ( $\circ$ ), FIM2 ( $\triangle$ ), RIM1 ( $+$ ), RIM2 ( $\times$ ), and URIM1 ( $\diamond$ ).

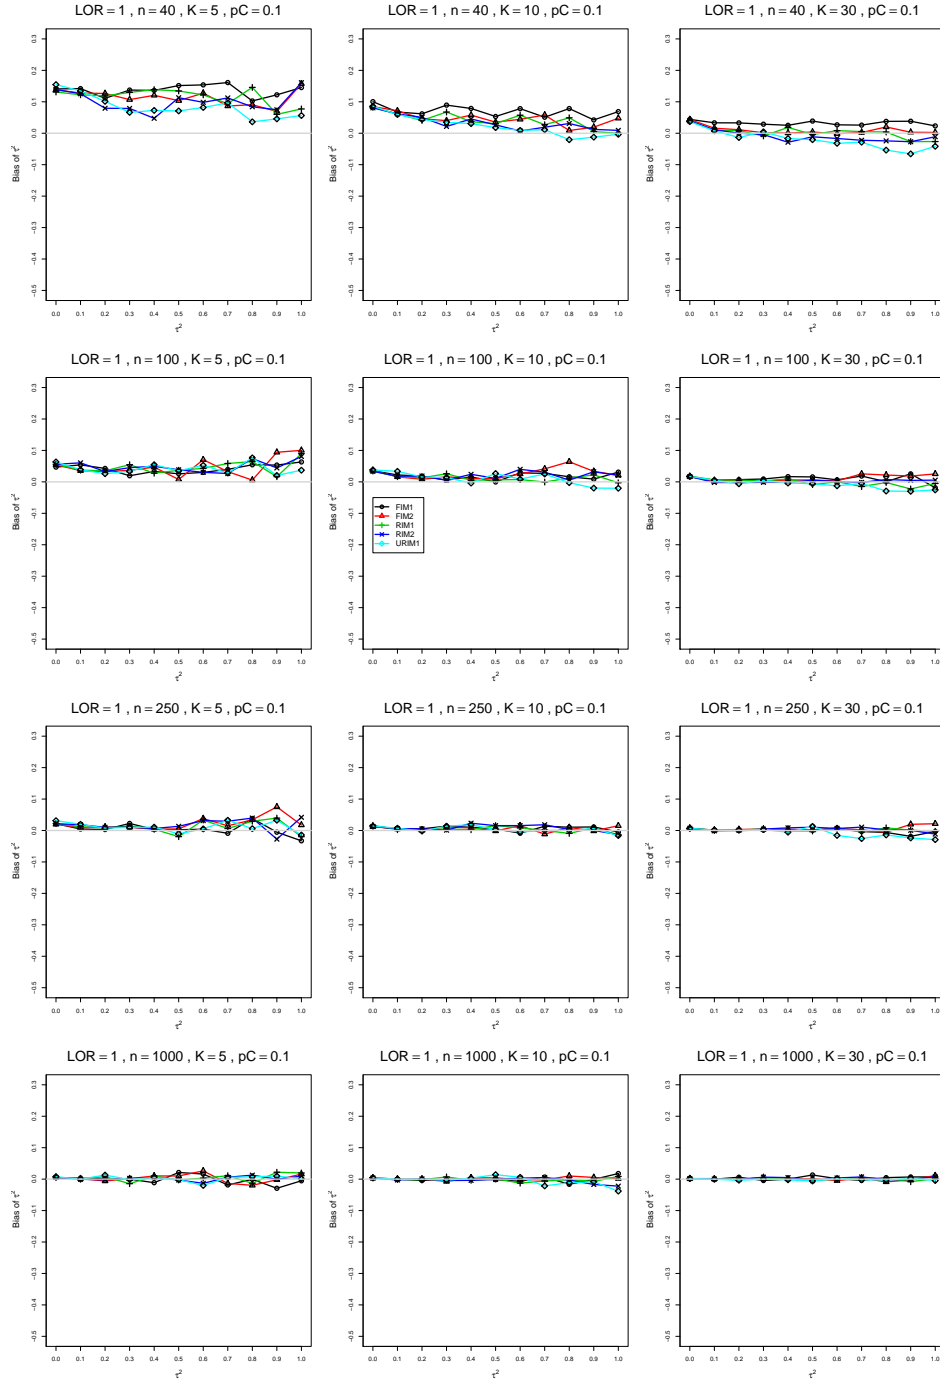

Figure A1.4.15: Bias of between-studies variance  $\hat{\tau}_{KD}^2$  for  $\theta = 1$ ,  $p_C = 0.1$ ,  $\sigma^2 = 0.4$ , constant sample sizes  $n = 40, 100, 250, 1000$ . The data-generation mechanisms are FIM1 ( $\circ$ ), FIM2 ( $\triangle$ ), RIM1 ( $+$ ), RIM2 ( $\times$ ), and URIM1 ( $\diamond$ ).

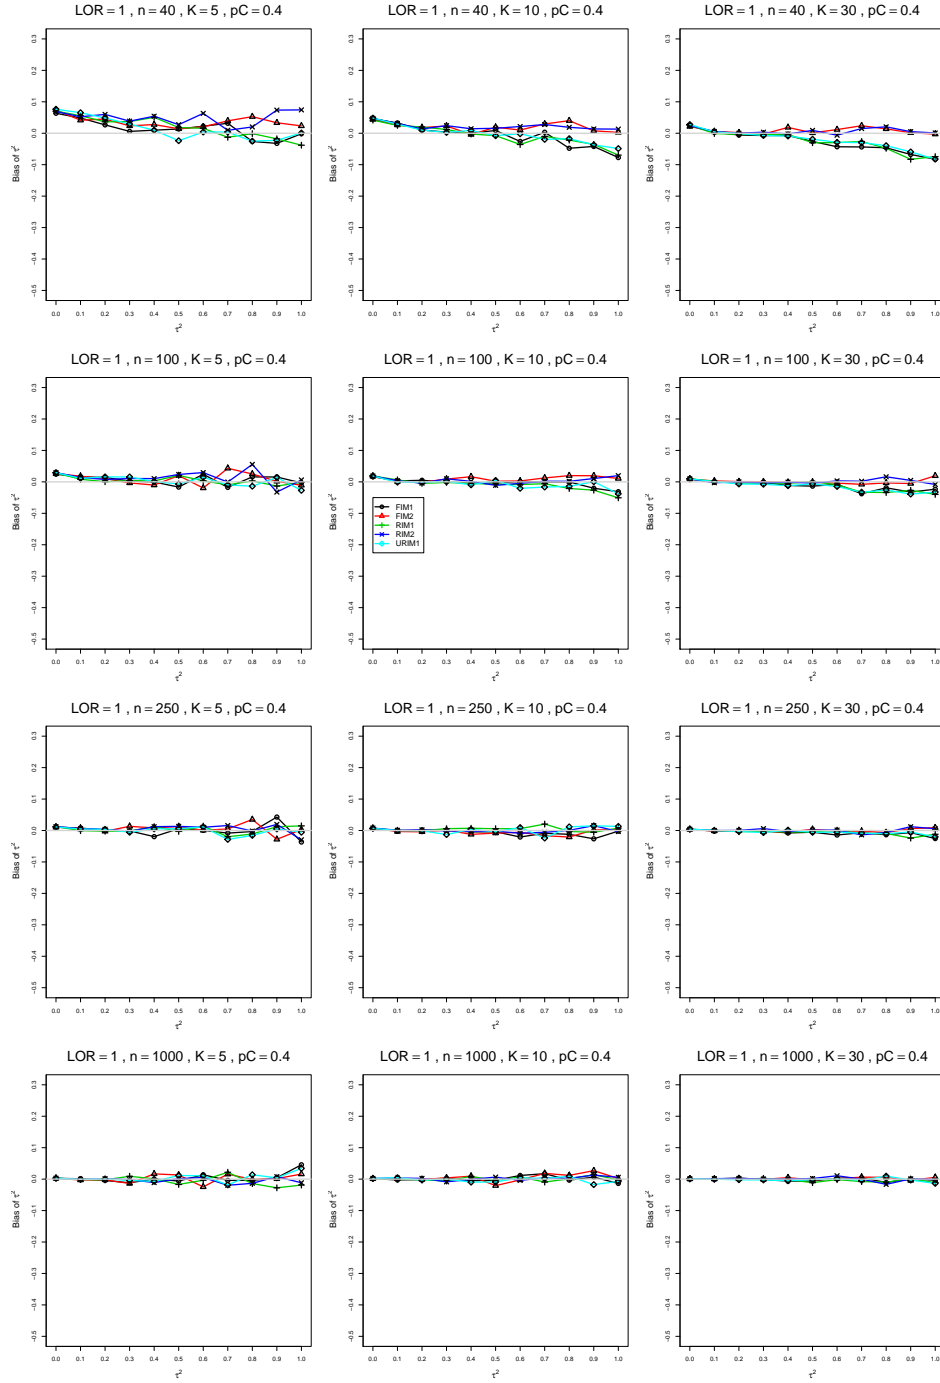

Figure A1.4.16: Bias of between-studies variance  $\hat{\tau}_{KD}^2$  for  $\theta = 1$ ,  $p_C = 0.4$ ,  $\sigma^2 = 0.4$ , constant sample sizes  $n = 40, 100, 250, 1000$ . The data-generation mechanisms are FIM1 ( $\circ$ ), FIM2 ( $\triangle$ ), RIM1 ( $+$ ), RIM2 ( $\times$ ), and URIM1 ( $\diamond$ ).

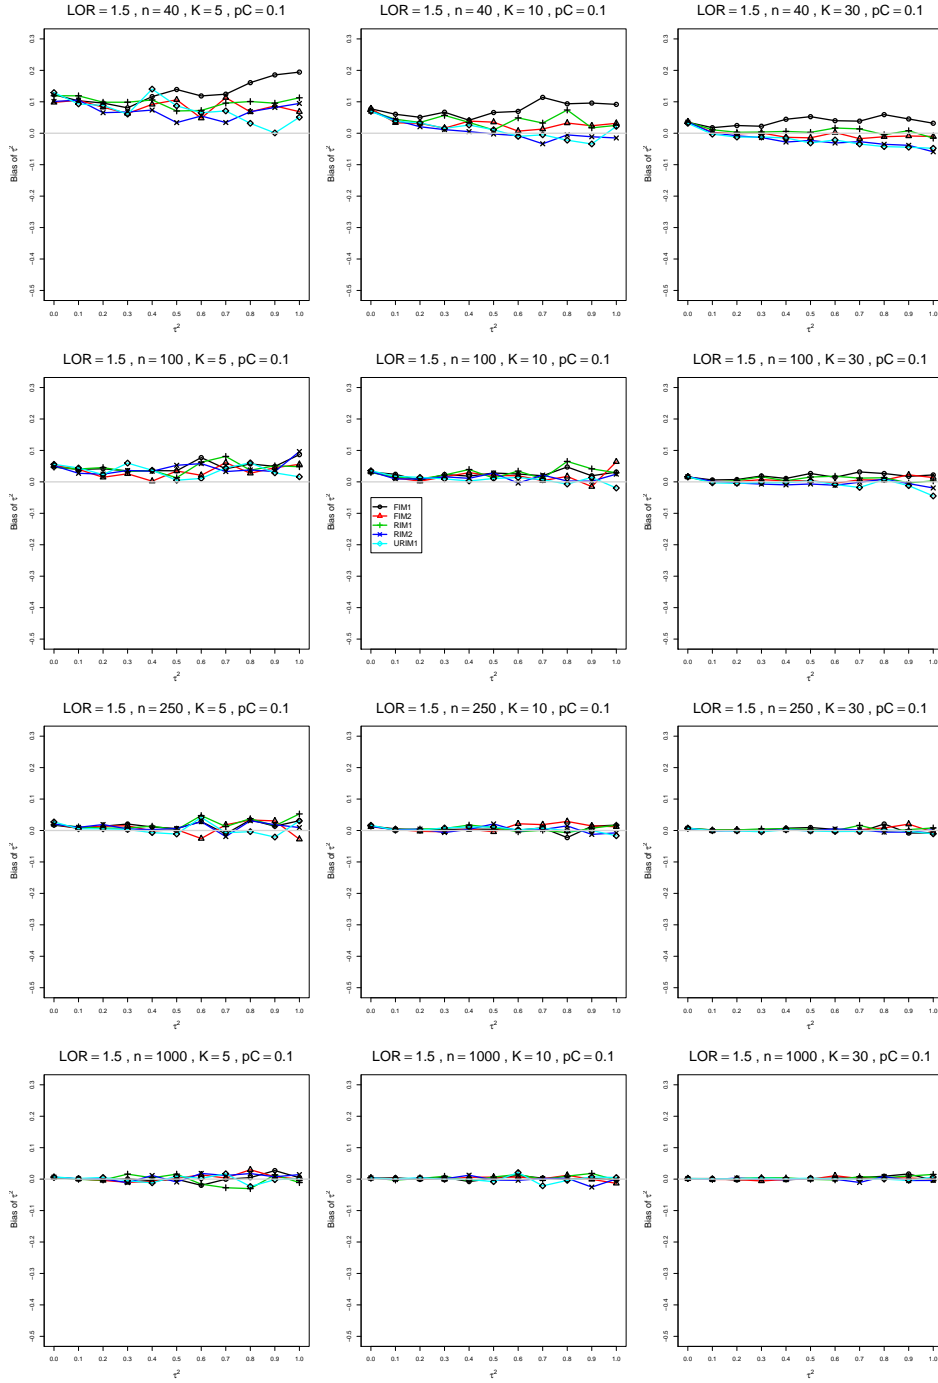

Figure A1.4.17: Bias of between-studies variance  $\hat{\tau}_{KD}^2$  for  $\theta = 1.5$ ,  $p_C = 0.1$ ,  $\sigma^2 = 0.4$ , constant sample sizes  $n = 40, 100, 250, 1000$ . The data-generation mechanisms are FIM1 ( $\circ$ ), FIM2 ( $\triangle$ ), RIM1 ( $+$ ), RIM2 ( $\times$ ), and URIM1 ( $\diamond$ ).

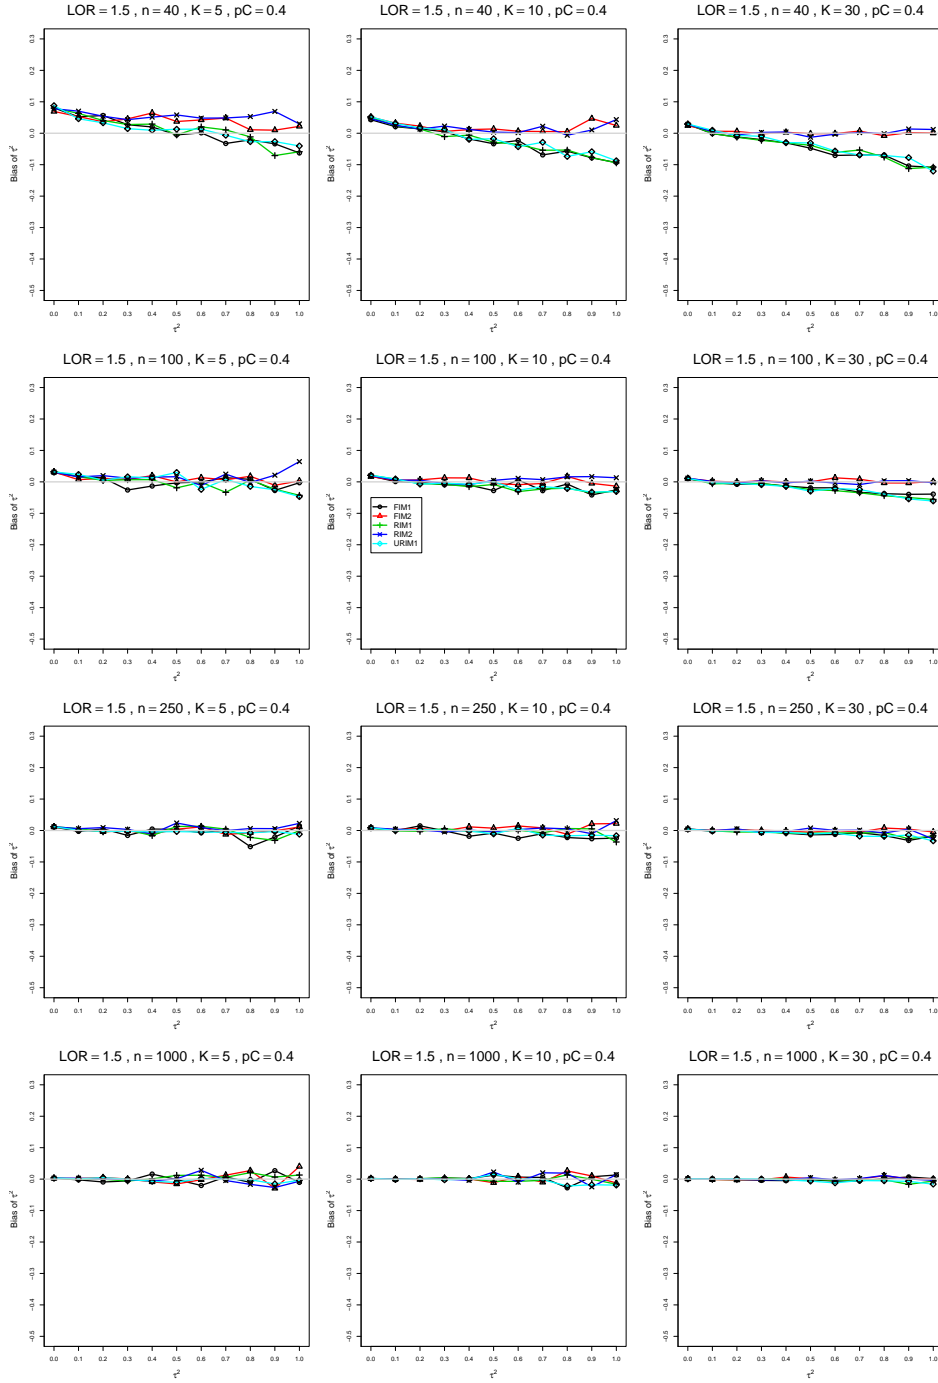

Figure A1.4.18: Bias of between-studies variance  $\hat{\tau}_{KD}^2$  for  $\theta = 1.5$ ,  $p_C = 0.4$ ,  $\sigma^2 = 0.4$ , constant sample sizes  $n = 40, 100, 250, 1000$ . The data-generation mechanisms are FIM1 ( $\circ$ ), FIM2 ( $\triangle$ ), RIM1 ( $+$ ), RIM2 ( $\times$ ), and URIM1 ( $\diamond$ ).



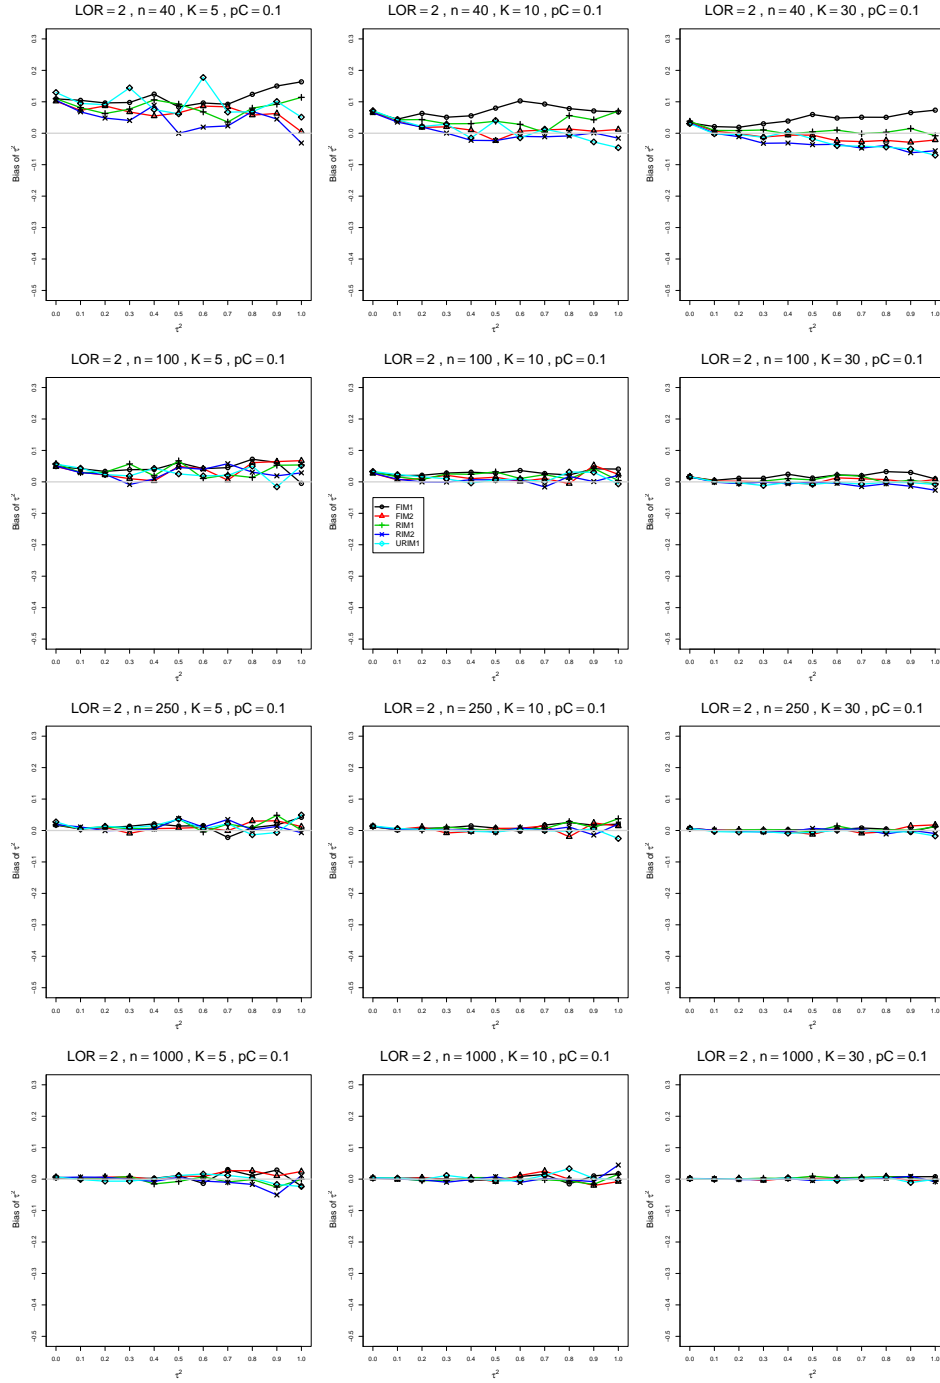

Figure A1.4.19: Bias of between-studies variance  $\hat{\tau}_{KD}^2$  for  $\theta = 2$ ,  $p_C = 0.1$ ,  $\sigma^2 = 0.4$ , constant sample sizes  $n = 40, 100, 250, 1000$ . The data-generation mechanisms are FIM1 ( $\circ$ ), FIM2 ( $\triangle$ ), RIM1 ( $+$ ), RIM2 ( $\times$ ), and URIM1 ( $\diamond$ ).

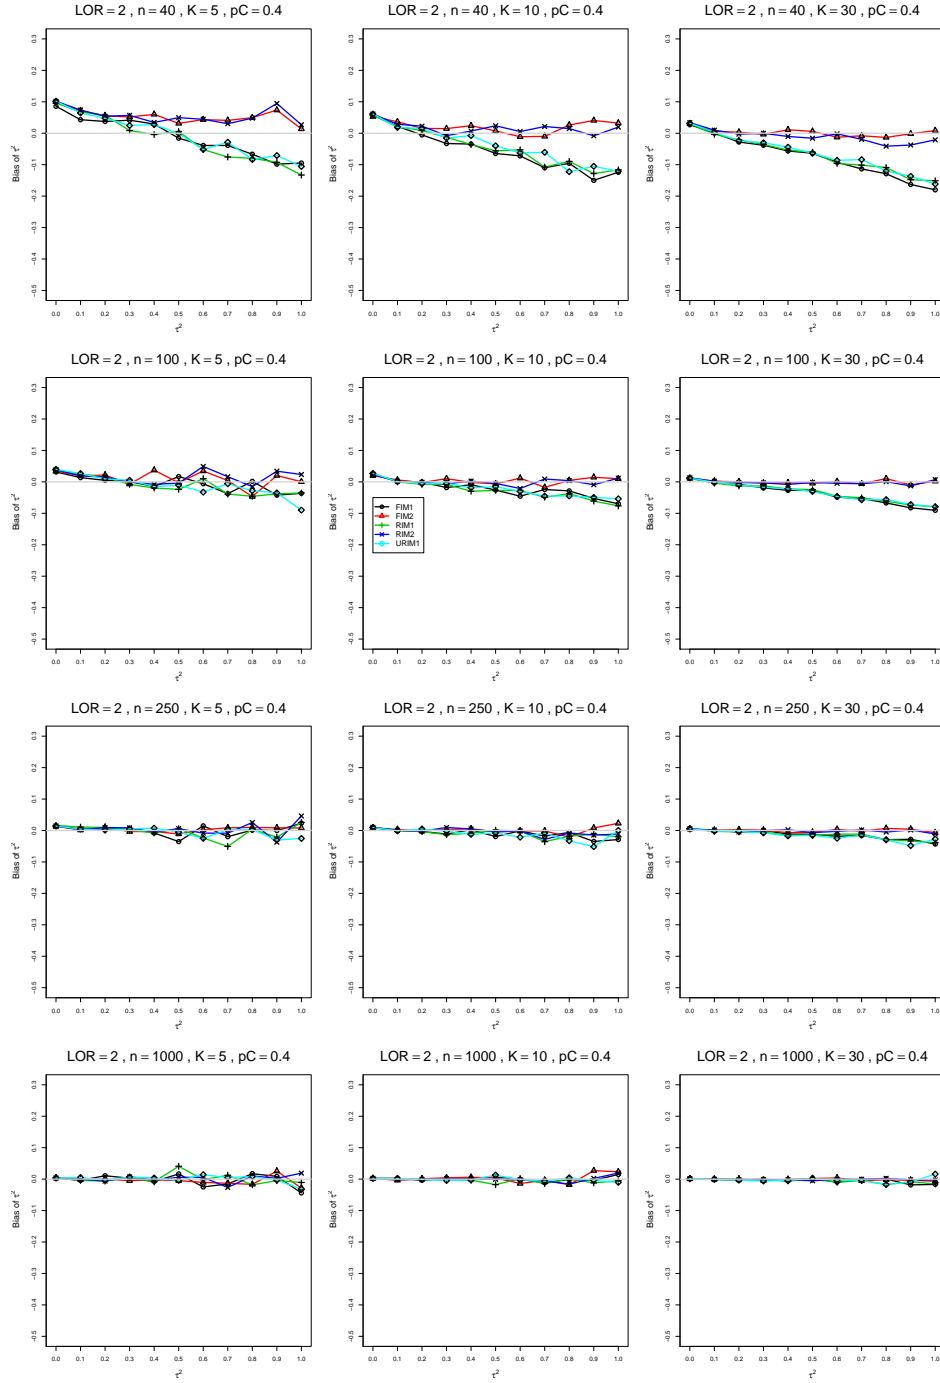

Figure A1.4.20: Bias of between-studies variance  $\hat{\tau}_{KD}^2$  for  $\theta = 2$ ,  $p_C = 0.4$ ,  $\sigma^2 = 0.4$ , constant sample sizes  $n = 40, 100, 250, 1000$ . The data-generation mechanisms are FIM1 ( $\circ$ ), FIM2 ( $\triangle$ ), RIM1 ( $+$ ), RIM2 ( $\times$ ), and URIM1 ( $\diamond$ ).

### A1.5 Bias of $\hat{\tau}_{FIM2}^2$

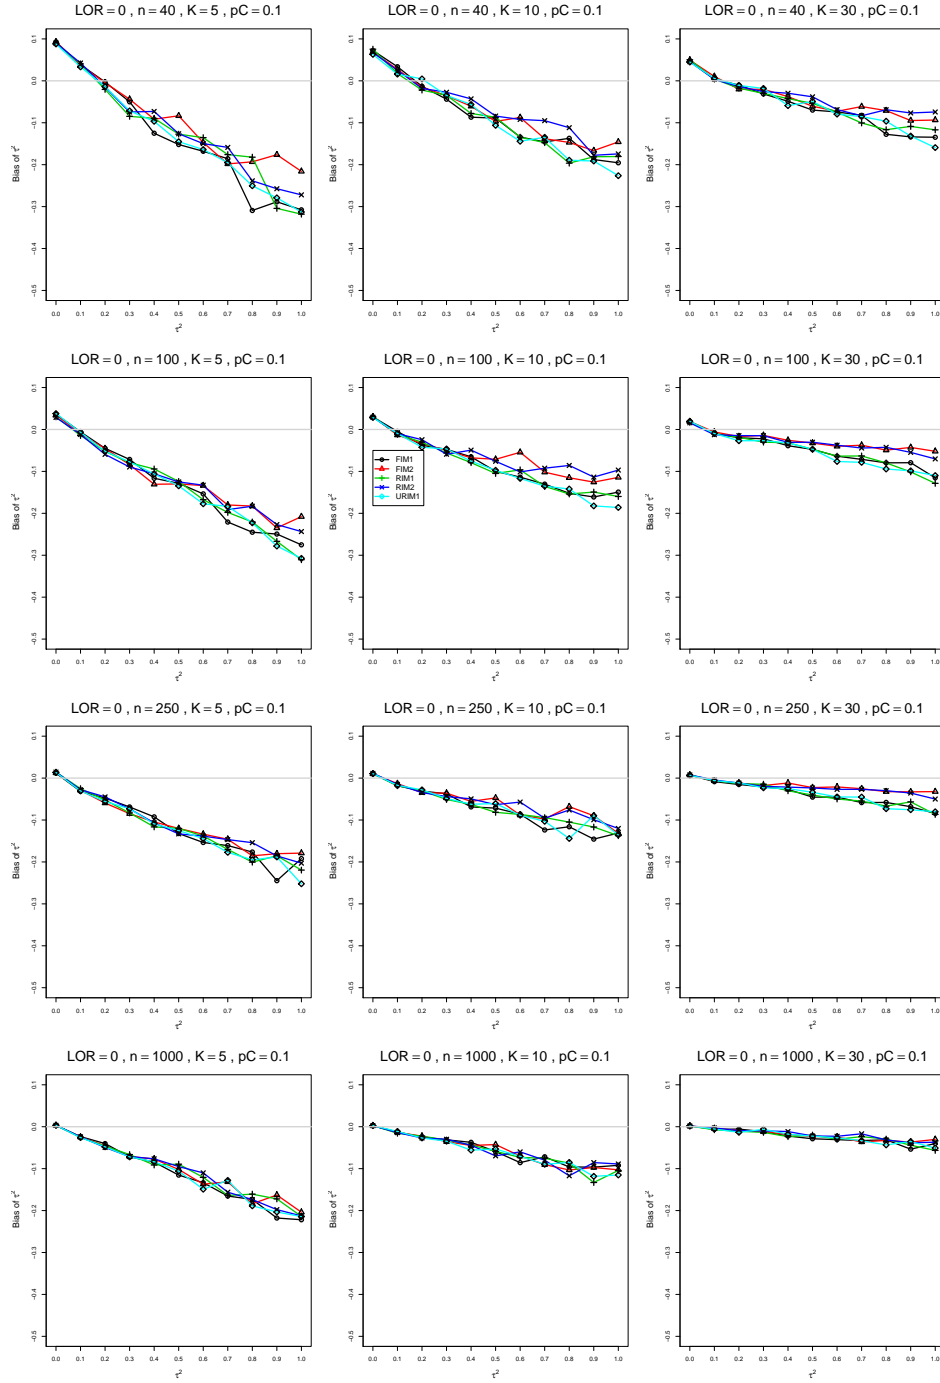

Figure A1.5.1: Bias of between-studies variance  $\hat{\tau}_{FIM2}^2$  for  $\theta = 0$ ,  $p_C = 0.1$ ,  $\sigma^2 = 0.1$ , constant sample sizes  $n = 40, 100, 250, 1000$ . The data-generation mechanisms are FIM1 ( $\circ$ ), FIM2 ( $\triangle$ ), RIM1 ( $+$ ), RIM2 ( $\times$ ), and URIM1 ( $\diamond$ ).

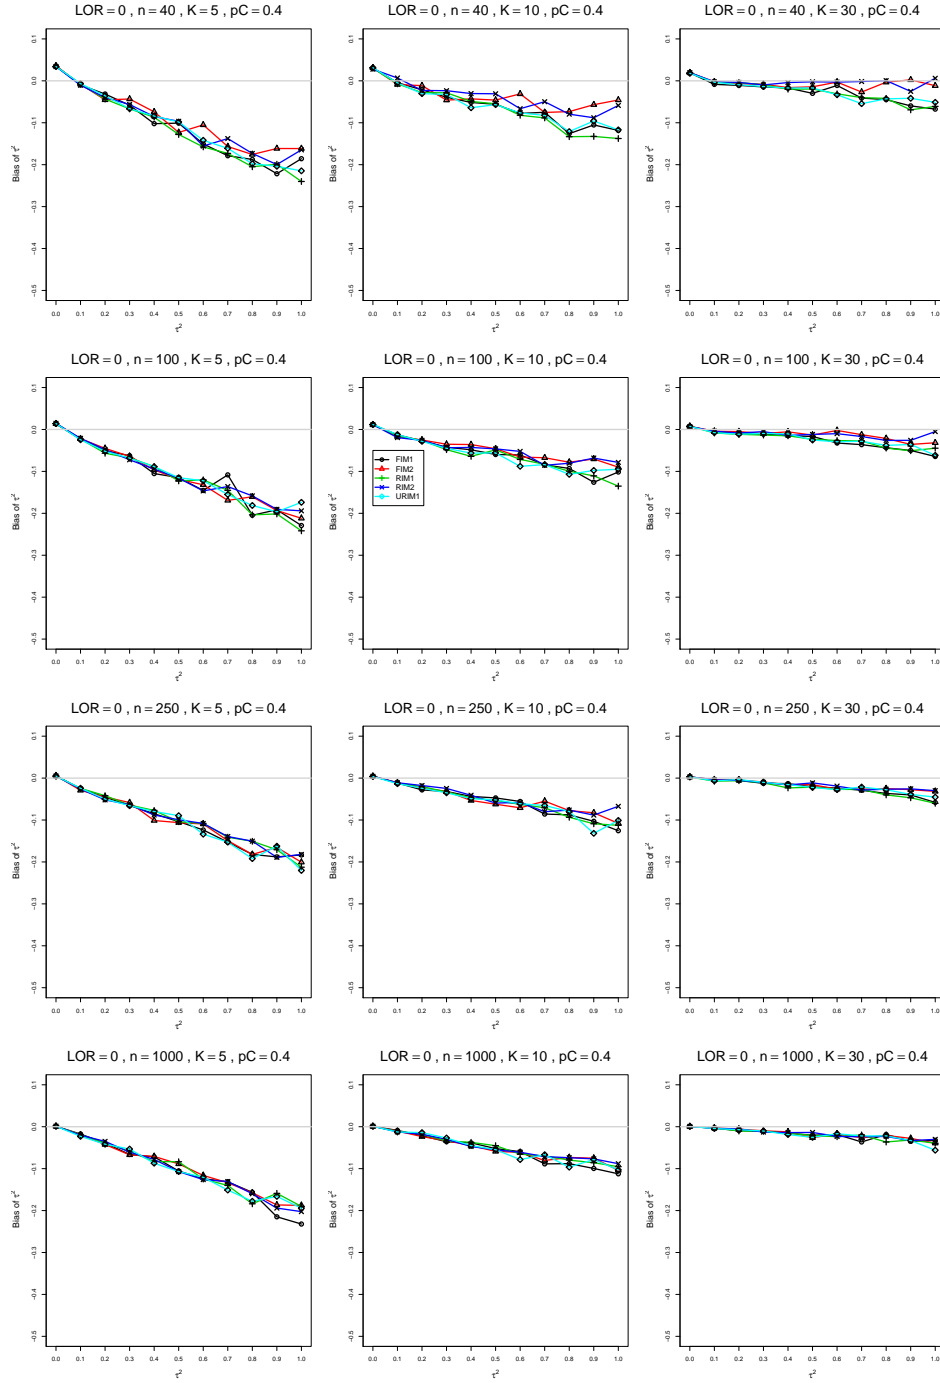

Figure A1.5.2: Bias of between-studies variance  $\hat{\tau}_{FIM2}^2$  for  $\theta = 0$ ,  $p_C = 0.4$ ,  $\sigma^2 = 0.1$ , constant sample sizes  $n = 40, 100, 250, 1000$ . The data-generation mechanisms are FIM1 ( $\circ$ ), FIM2 ( $\triangle$ ), RIM1 ( $+$ ), RIM2 ( $\times$ ), and URIM1 ( $\diamond$ ).

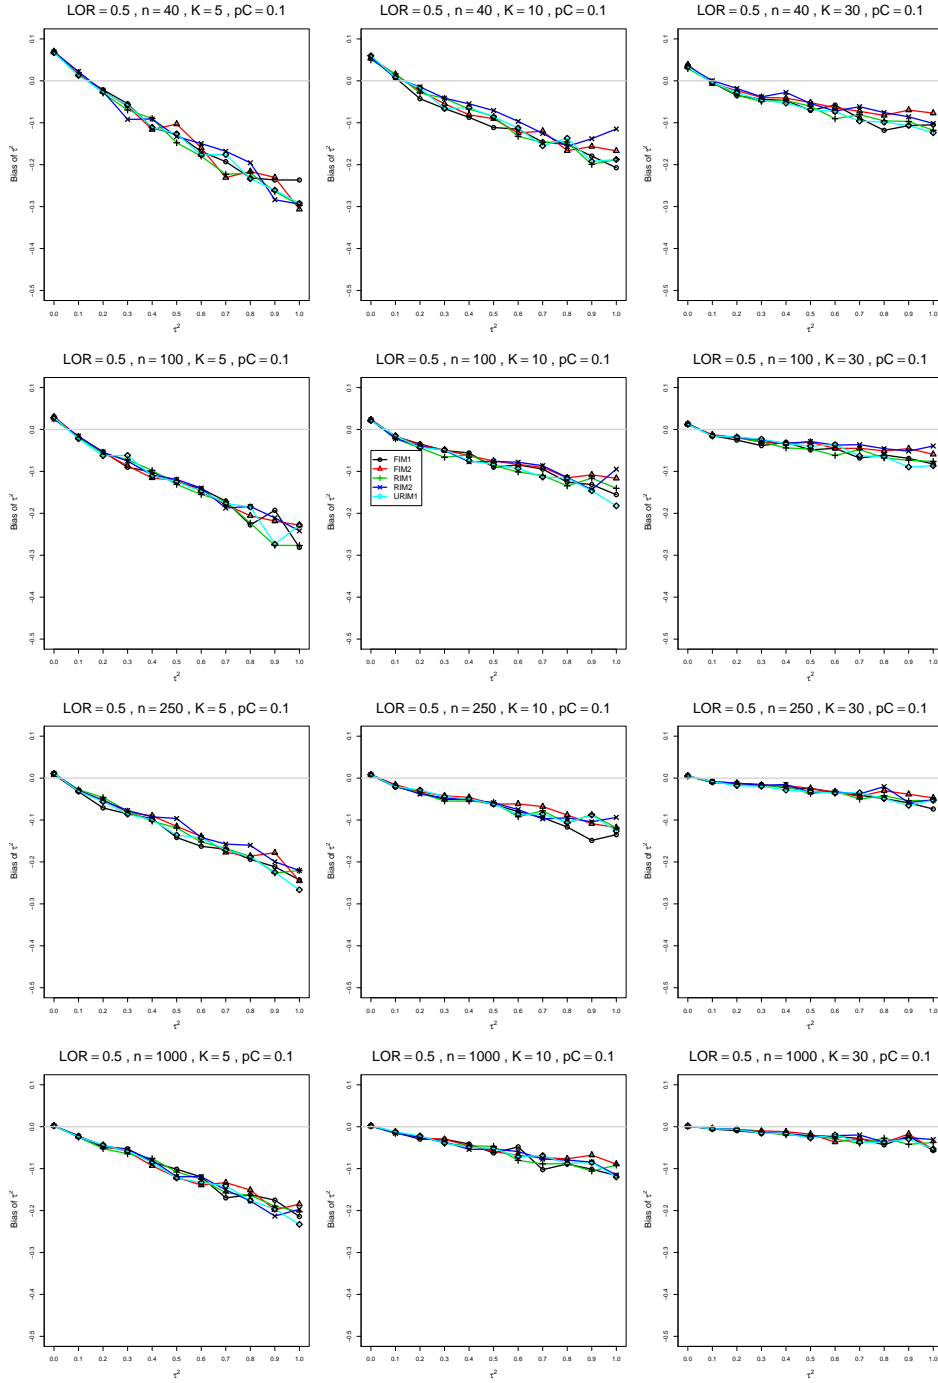

Figure A1.5.3: Bias of between-studies variance  $\hat{\tau}_{FIM2}^2$  for  $\theta = 0.5$ ,  $p_C = 0.1$ ,  $\sigma^2 = 0.1$ , constant sample sizes  $n = 40, 100, 250, 1000$ . The data-generation mechanisms are FIM1 ( $\circ$ ), FIM2 ( $\triangle$ ), RIM1 ( $+$ ), RIM2 ( $\times$ ), and URIM1 ( $\diamond$ ).

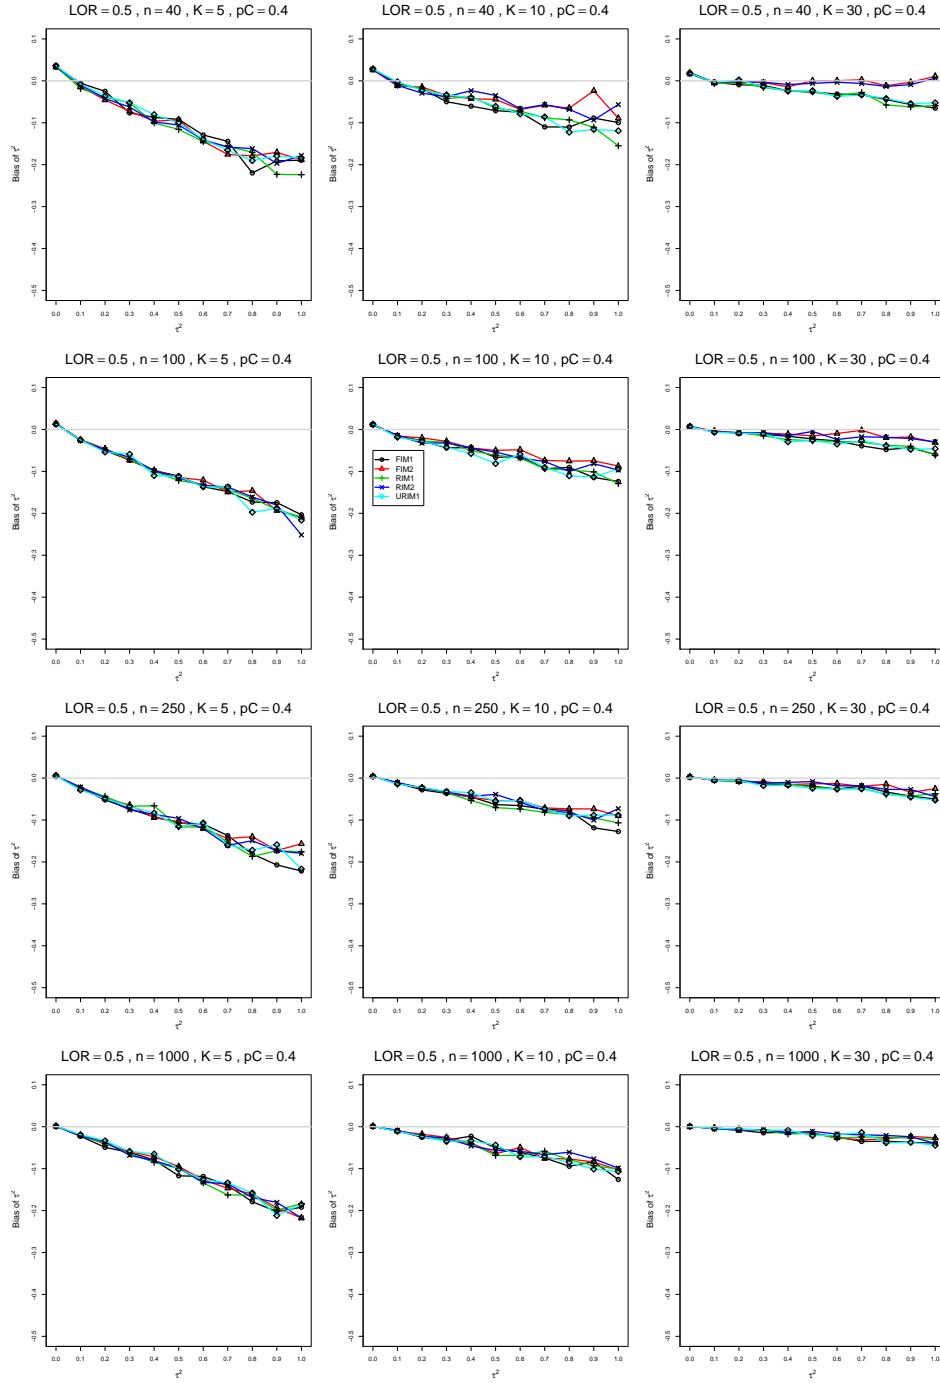

Figure A1.5.4: Bias of between-studies variance  $\hat{\tau}_{FIM2}^2$  for  $\theta = 0.5$ ,  $p_C = 0.4$ ,  $\sigma^2 = 0.1$ , constant sample sizes  $n = 40, 100, 250, 1000$ . The data-generation mechanisms are FIM1 ( $\circ$ ), FIM2 ( $\triangle$ ), RIM1 ( $+$ ), RIM2 ( $\times$ ), and URIM1 ( $\diamond$ ).

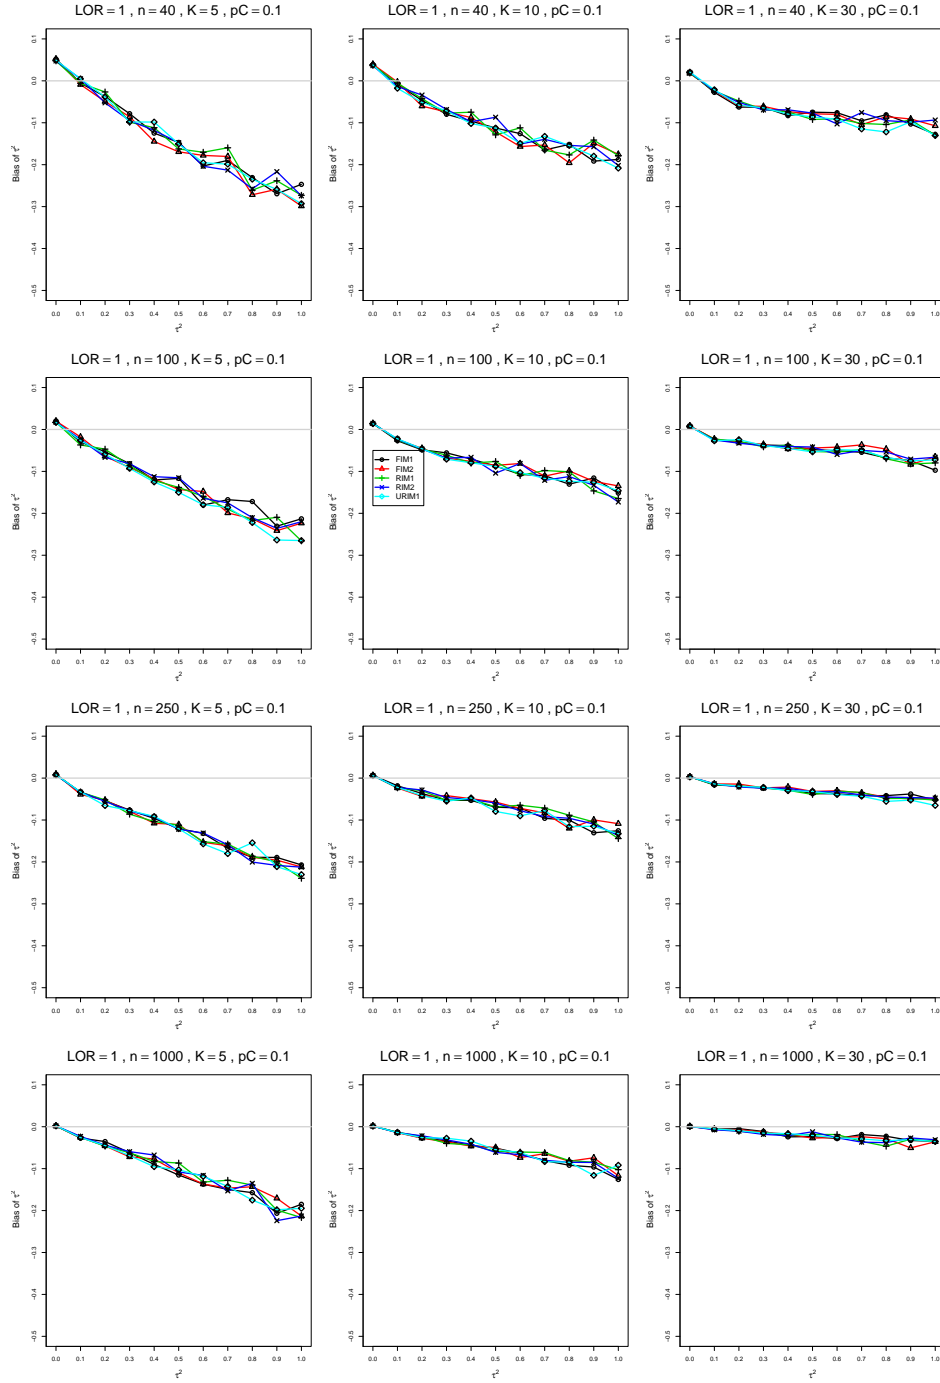

Figure A1.5.5: Bias of between-studies variance  $\hat{\tau}_{FIM2}^2$  for  $\theta = 1$ ,  $p_C = 0.1$ ,  $\sigma^2 = 0.1$ , constant sample sizes  $n = 40, 100, 250, 1000$ . The data-generation mechanisms are FIM1 ( $\circ$ ), FIM2 ( $\triangle$ ), RIM1 ( $+$ ), RIM2 ( $\times$ ), and URIM1 ( $\diamond$ ).



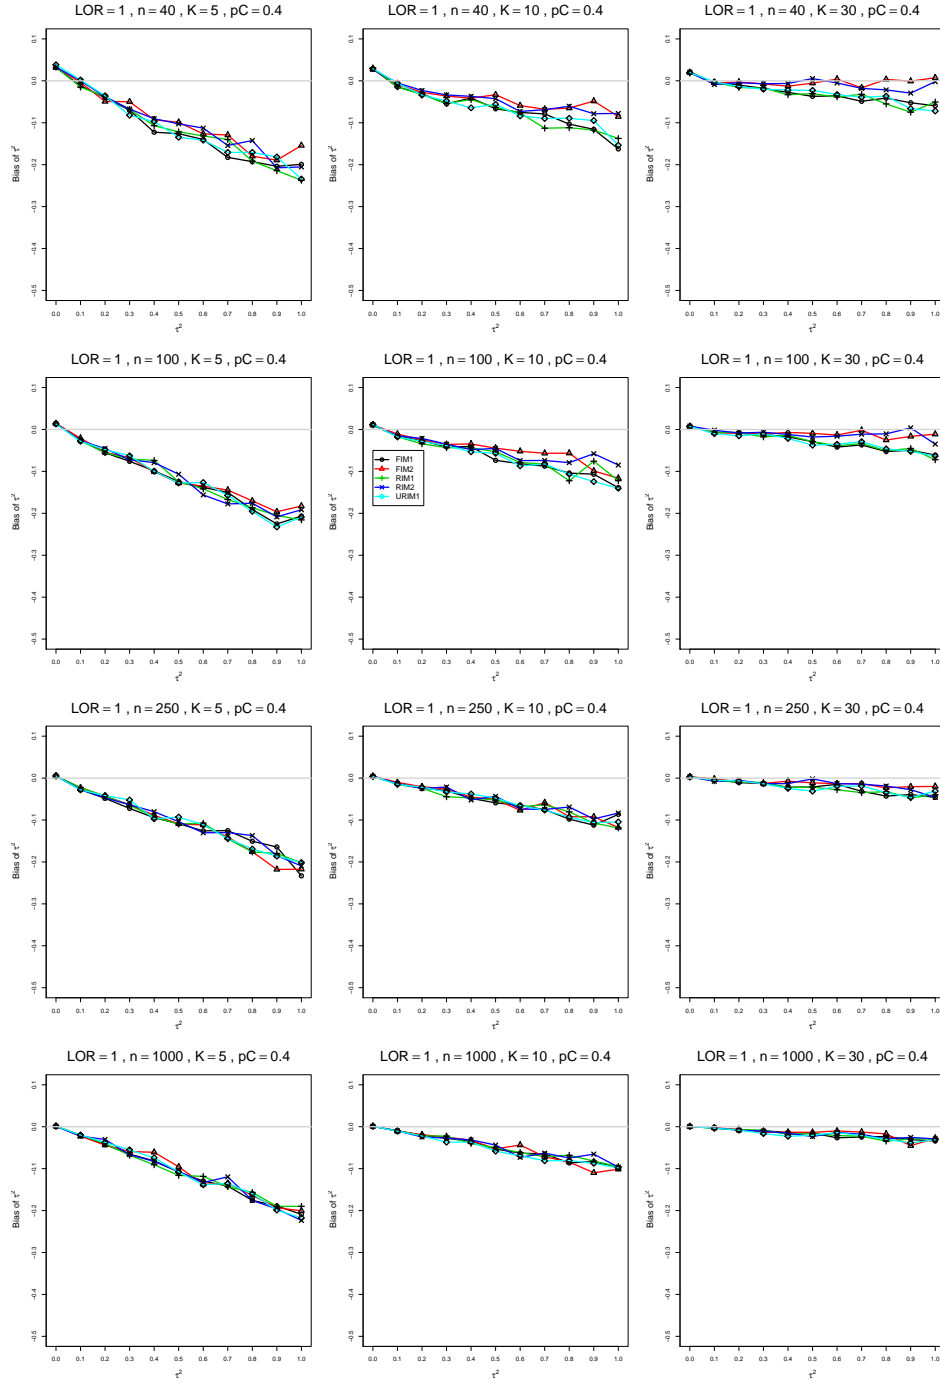

Figure A1.5.6: Bias of between-studies variance  $\hat{\tau}_{FIM2}^2$  for  $\theta = 1$ ,  $p_C = 0.4$ ,  $\sigma^2 = 0.1$ , constant sample sizes  $n = 40, 100, 250, 1000$ . The data-generation mechanisms are FIM1 ( $\circ$ ), FIM2 ( $\triangle$ ), RIM1 ( $+$ ), RIM2 ( $\times$ ), and URIM1 ( $\diamond$ ).

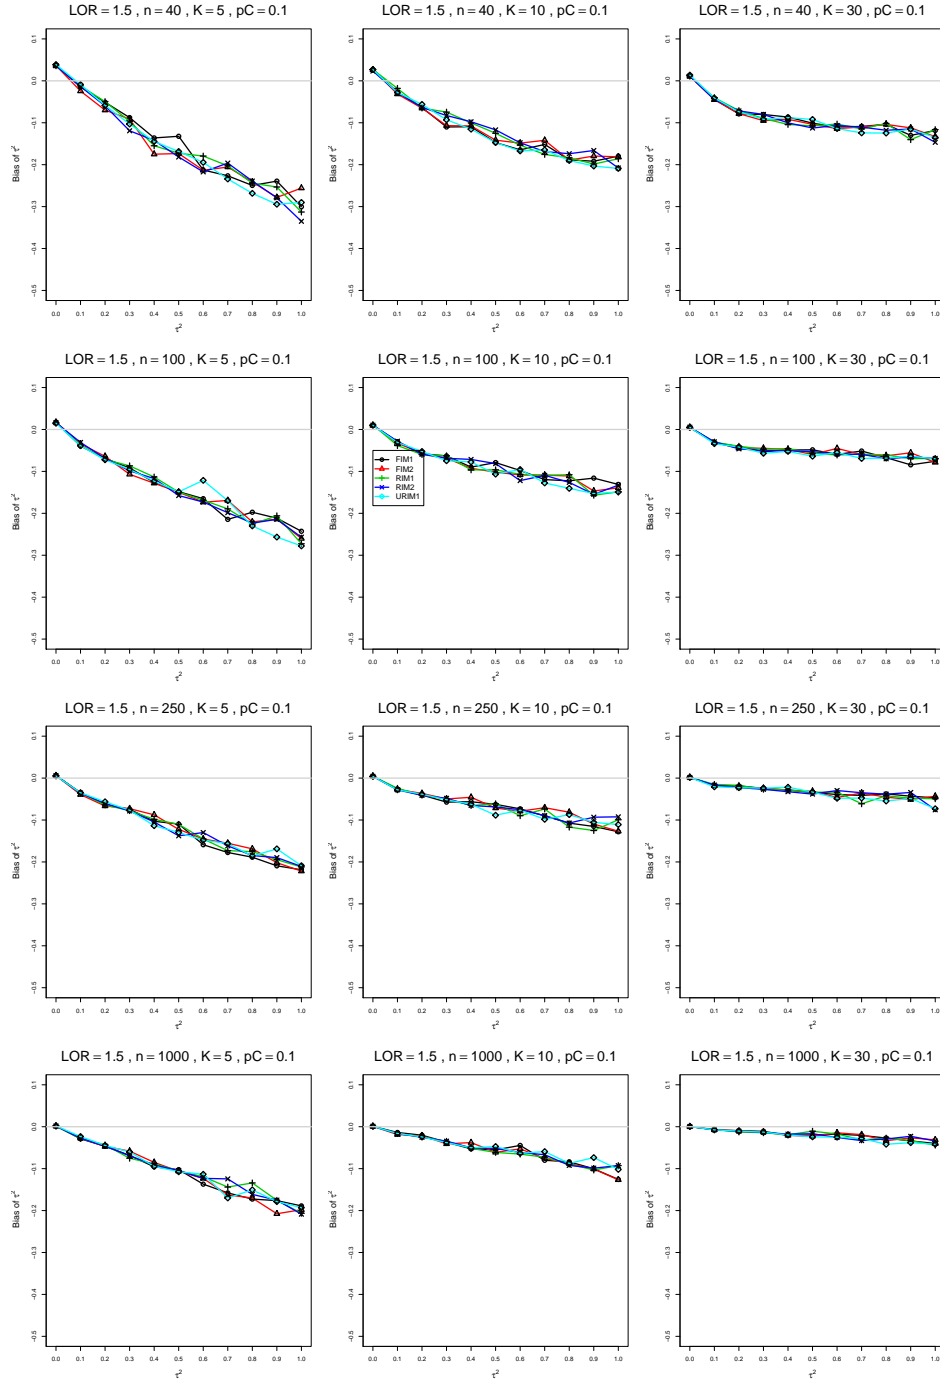

Figure A1.5.7: Bias of between-studies variance  $\hat{\tau}_{FIM2}^2$  for  $\theta = 1.5$ ,  $p_C = 0.1$ ,  $\sigma^2 = 0.1$ , constant sample sizes  $n = 40, 100, 250, 1000$ . The data-generation mechanisms are FIM1 ( $\circ$ ), FIM2 ( $\triangle$ ), RIM1 ( $+$ ), RIM2 ( $\times$ ), and URIM1 ( $\diamond$ ).

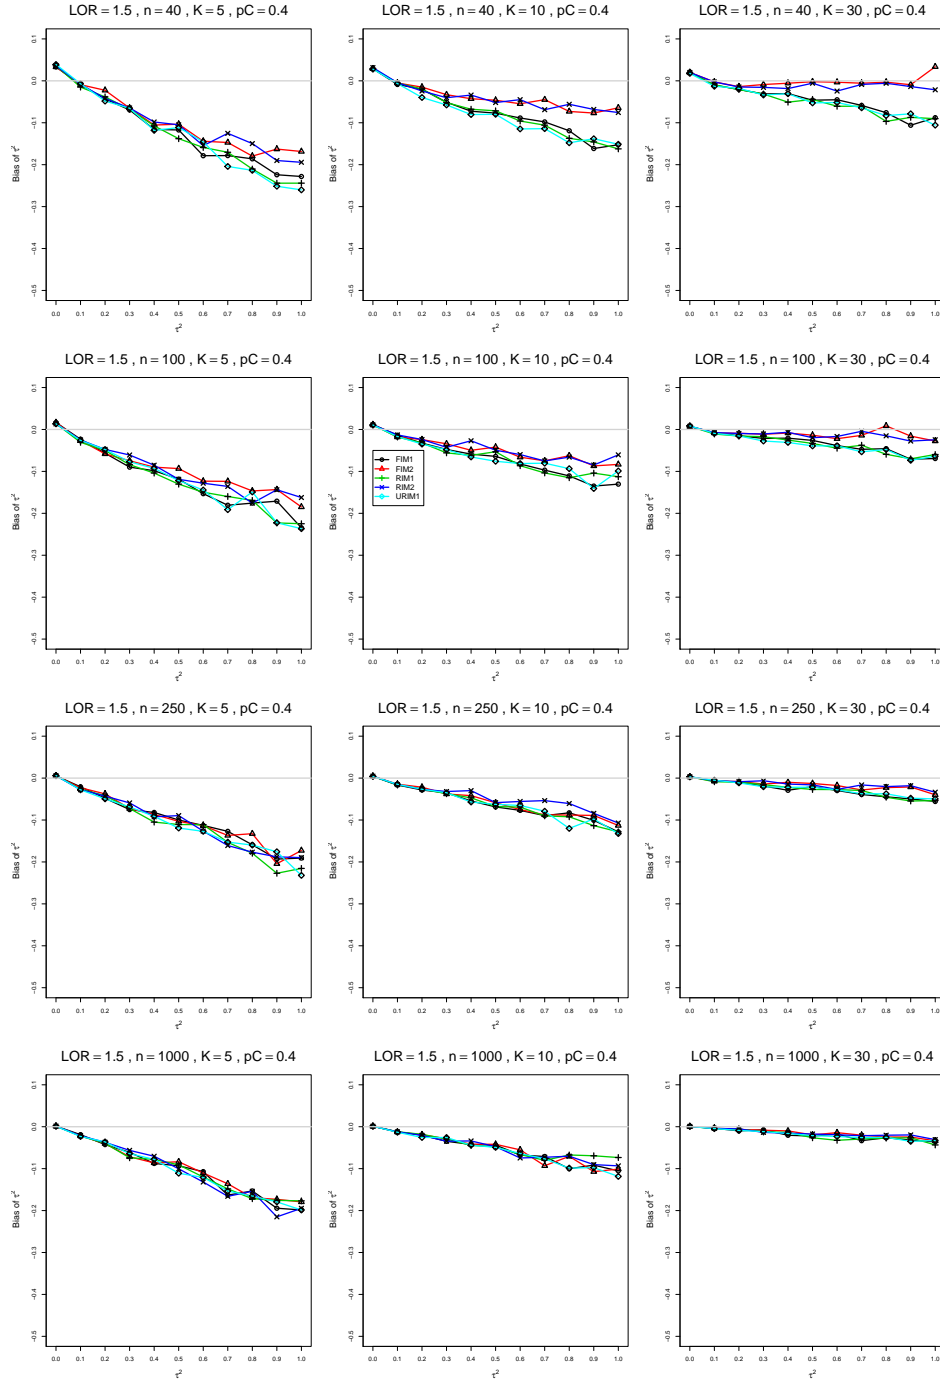

Figure A1.5.8: Bias of between-studies variance  $\hat{\tau}_{FIM2}^2$  for  $\theta = 1.5$ ,  $p_C = 0.4$ ,  $\sigma^2 = 0.1$ , constant sample sizes  $n = 40, 100, 250, 1000$ . The data-generation mechanisms are FIM1 ( $\circ$ ), FIM2 ( $\triangle$ ), RIM1 (+), RIM2 ( $\times$ ), and URIM1 ( $\diamond$ ).

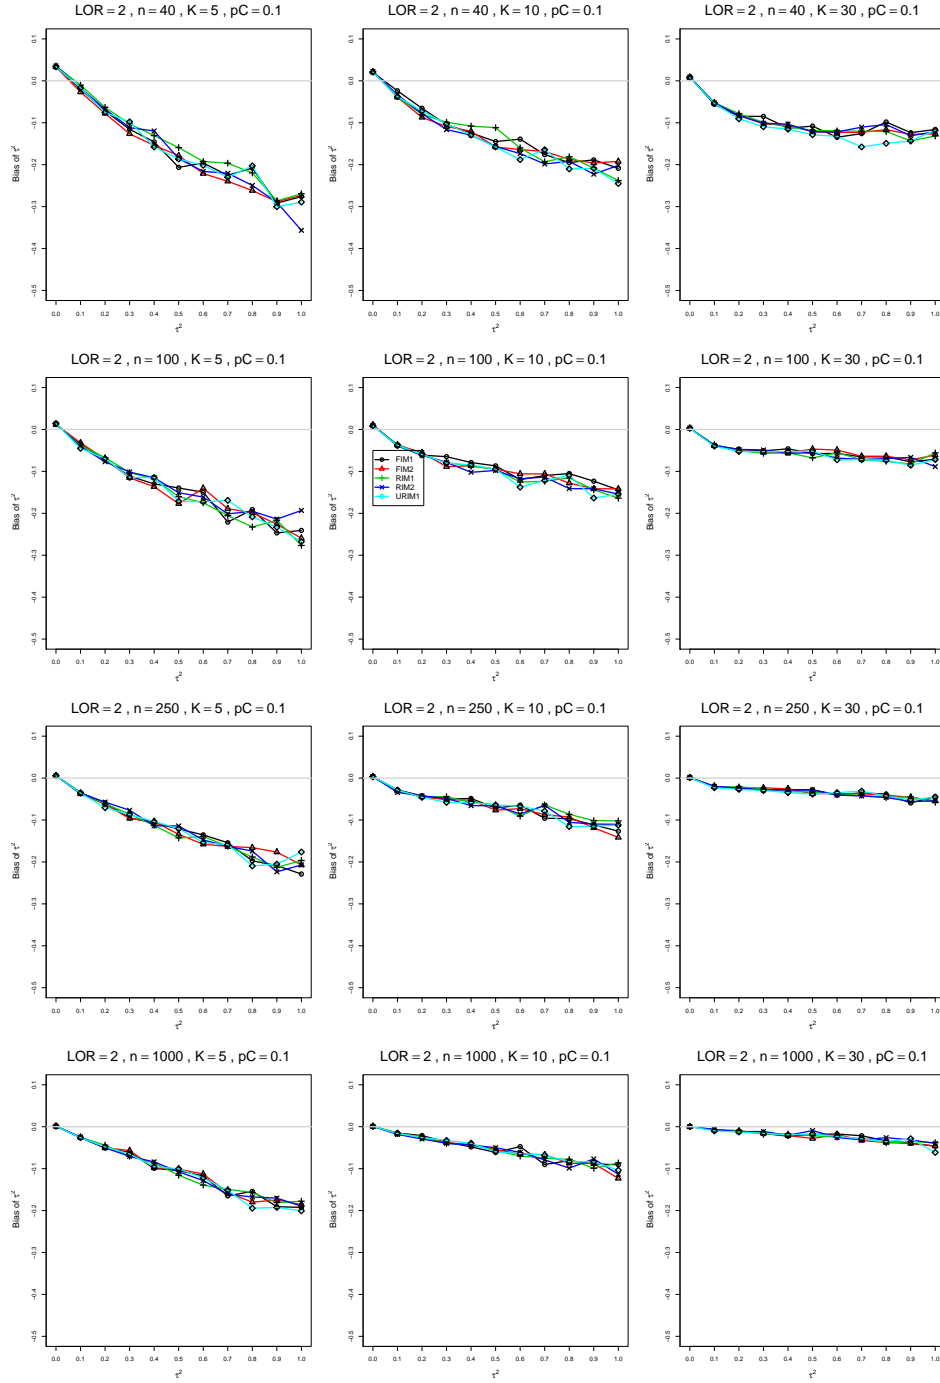

Figure A1.5.9: Bias of between-studies variance  $\hat{\tau}_{FIM2}^2$  for  $\theta = 2$ ,  $p_C = 0.1$ ,  $\sigma^2 = 0.1$ , constant sample sizes  $n = 40, 100, 250, 1000$ . The data-generation mechanisms are FIM1 ( $\circ$ ), FIM2 ( $\triangle$ ), RIM1 ( $+$ ), RIM2 ( $\times$ ), and URIM1 ( $\diamond$ ).

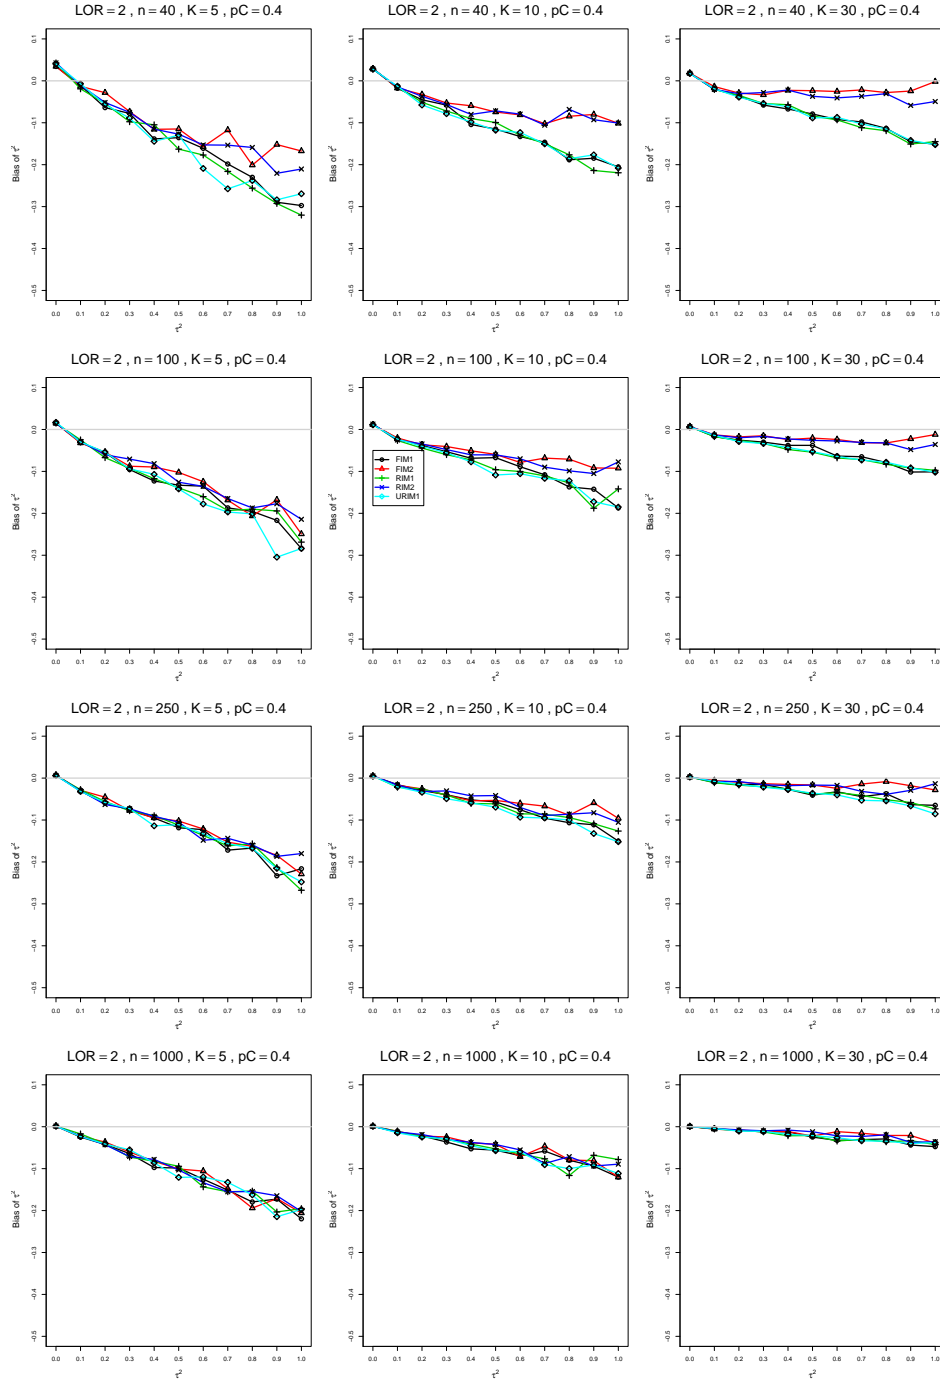

Figure A1.5.10: Bias of between-studies variance  $\hat{\tau}_{FIM2}^2$  for  $\theta = 2$ ,  $p_C = 0.4$ ,  $\sigma^2 = 0.1$ , constant sample sizes  $n = 40, 100, 250, 1000$ . The data-generation mechanisms are FIM1 ( $\circ$ ), FIM2 ( $\triangle$ ), RIM1 ( $+$ ), RIM2 ( $\times$ ), and URIM1 ( $\diamond$ ).

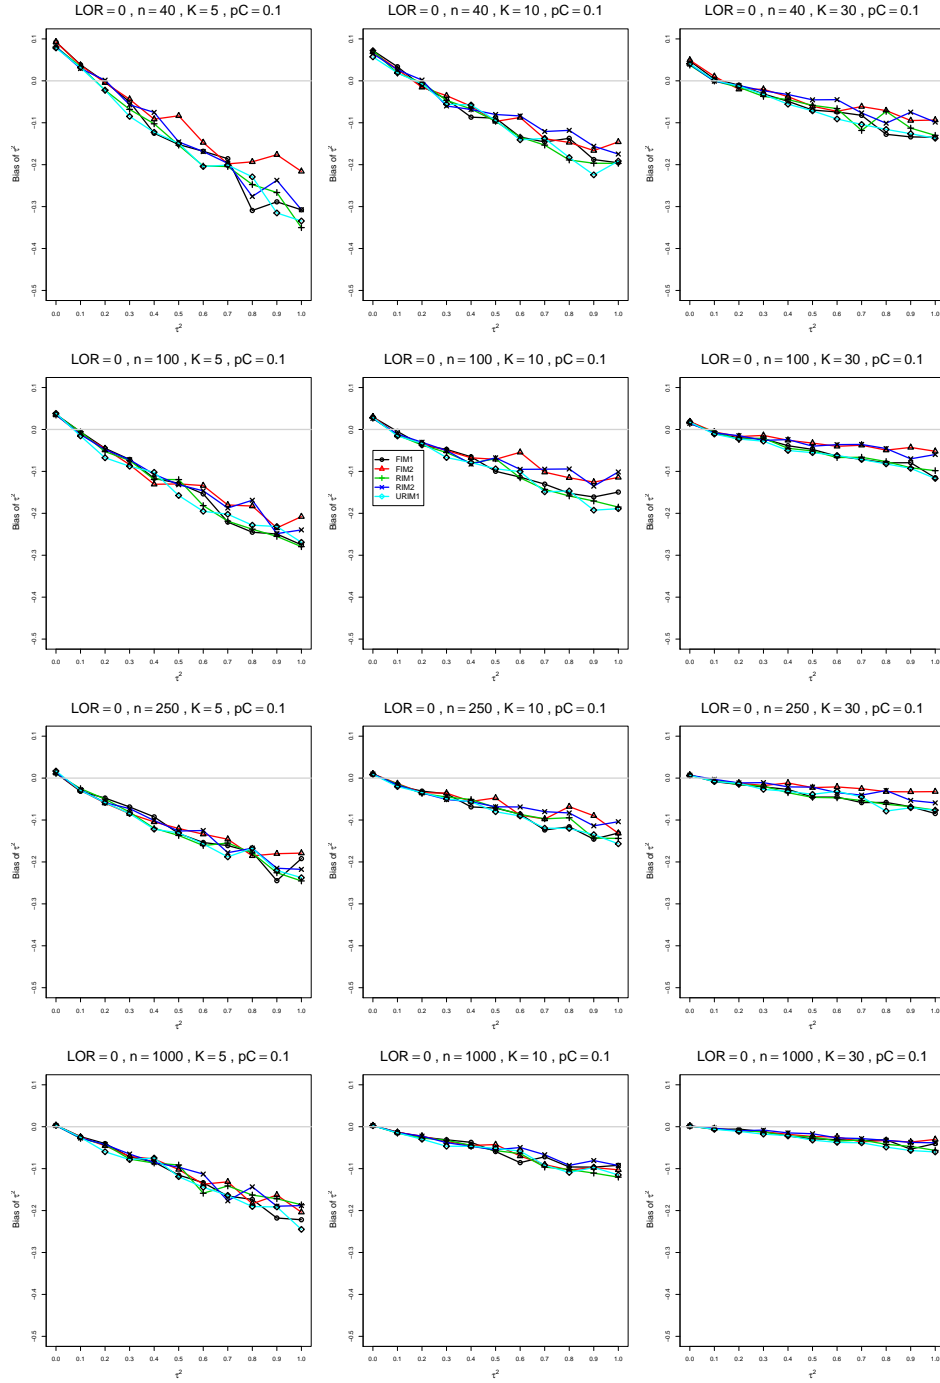

Figure A1.5.11: Bias of between-studies variance  $\hat{\tau}_{FIM2}^2$  for  $\theta = 0$ ,  $p_C = 0.1$ ,  $\sigma^2 = 0.4$ , constant sample sizes  $n = 40, 100, 250, 1000$ . The data-generation mechanisms are FIM1 ( $\circ$ ), FIM2 ( $\triangle$ ), RIM1 ( $+$ ), RIM2 ( $\times$ ), and URIM1 ( $\diamond$ ).

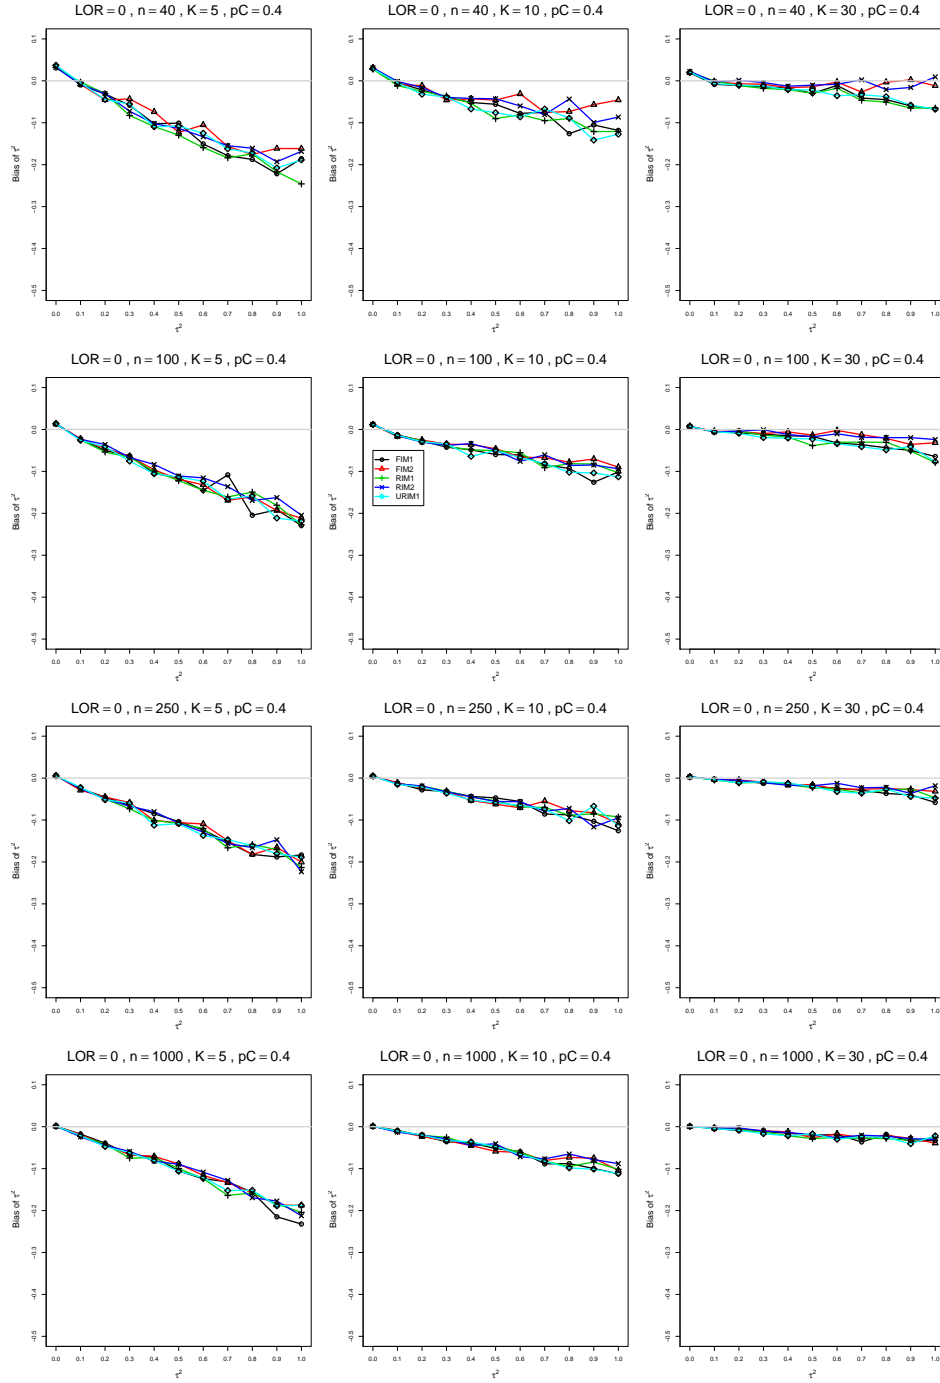

Figure A1.5.12: Bias of between-studies variance  $\hat{\tau}_{FIM2}^2$  for  $\theta = 0$ ,  $p_C = 0.4$ ,  $\sigma^2 = 0.4$ , constant sample sizes  $n = 40, 100, 250, 1000$ . The data-generation mechanisms are FIM1 ( $\circ$ ), FIM2 ( $\triangle$ ), RIM1 ( $+$ ), RIM2 ( $\times$ ), and URIM1 ( $\diamond$ ).

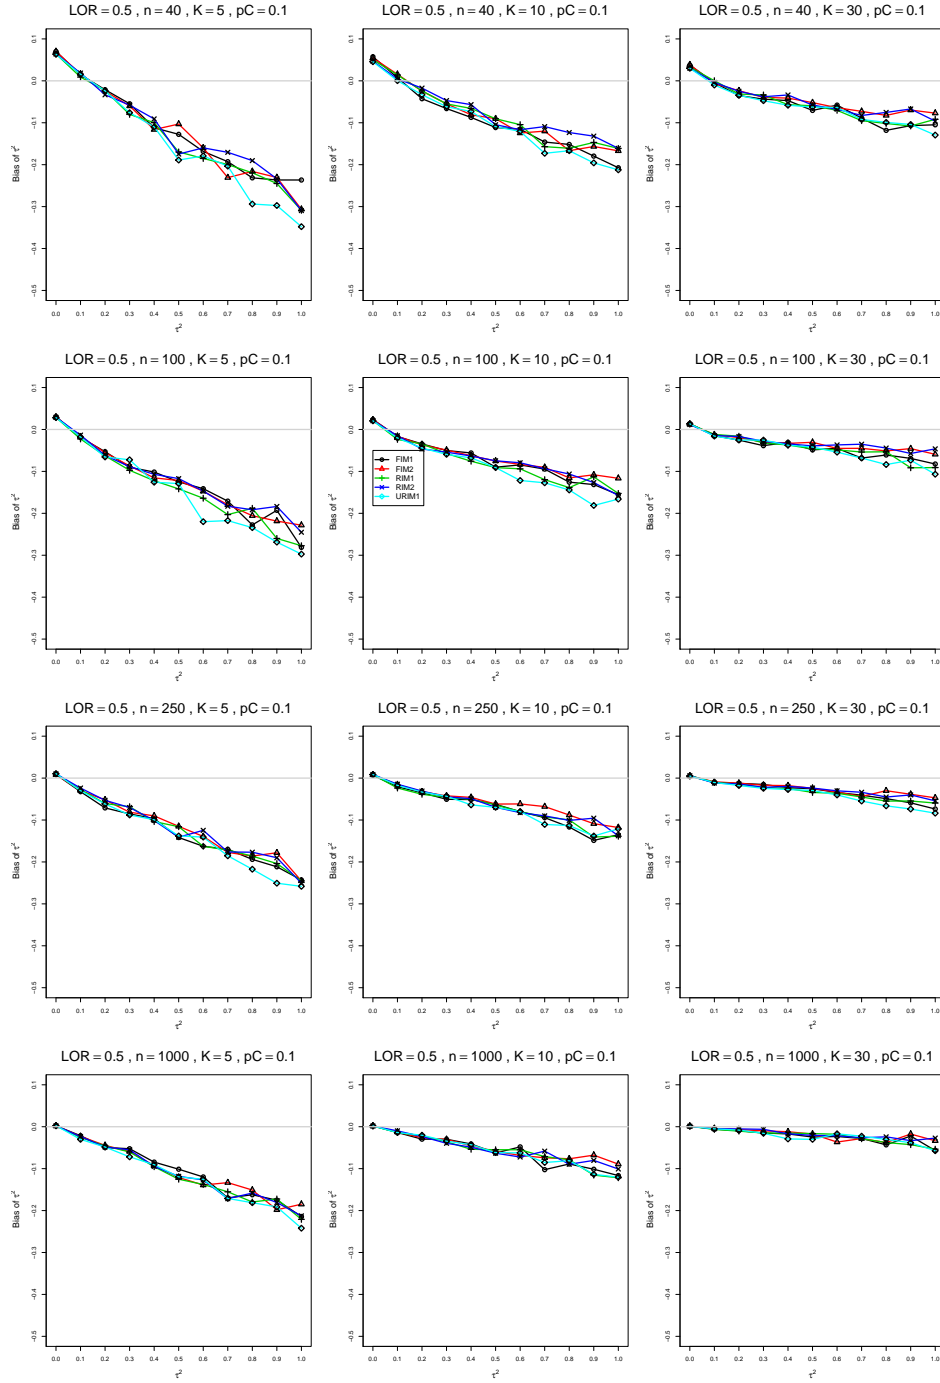

Figure A1.5.13: Bias of between-studies variance  $\hat{\tau}_{FIM2}^2$  for  $\theta = 0.5$ ,  $p_C = 0.1$ ,  $\sigma^2 = 0.4$ , constant sample sizes  $n = 40, 100, 250, 1000$ . The data-generation mechanisms are FIM1 ( $\circ$ ), FIM2 ( $\triangle$ ), RIM1 ( $+$ ), RIM2 ( $\times$ ), and URIM1 ( $\diamond$ ).



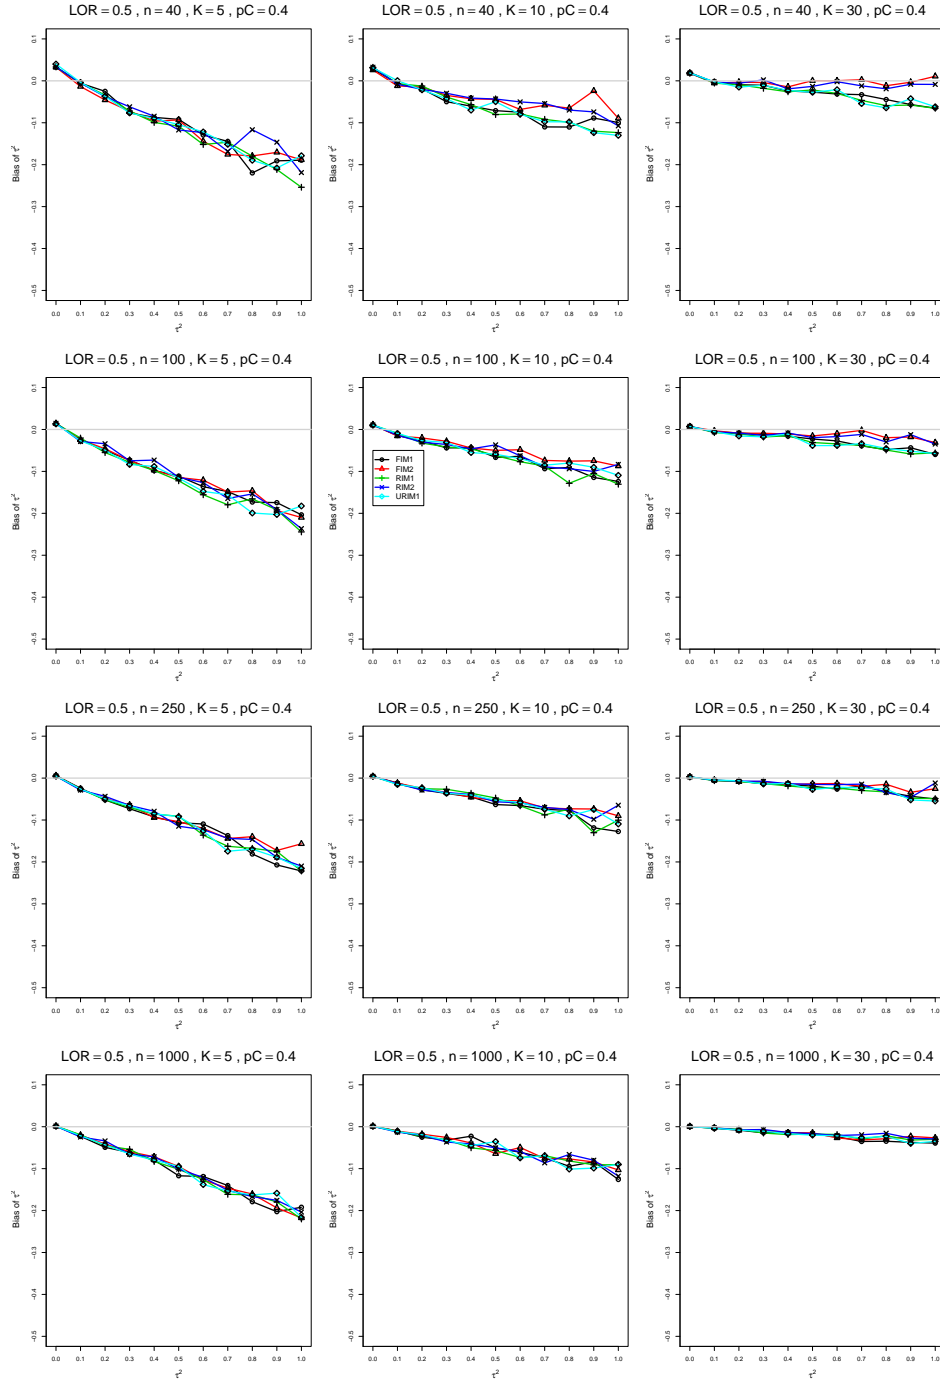

Figure A1.5.14: Bias of between-studies variance  $\hat{\tau}_{FIM2}^2$  for  $\theta = 0.5$ ,  $p_C = 0.4$ ,  $\sigma^2 = 0.4$ , constant sample sizes  $n = 40, 100, 250, 1000$ . The data-generation mechanisms are FIM1 ( $\circ$ ), FIM2 ( $\triangle$ ), RIM1 ( $+$ ), RIM2 ( $\times$ ), and URIM1 ( $\diamond$ ).

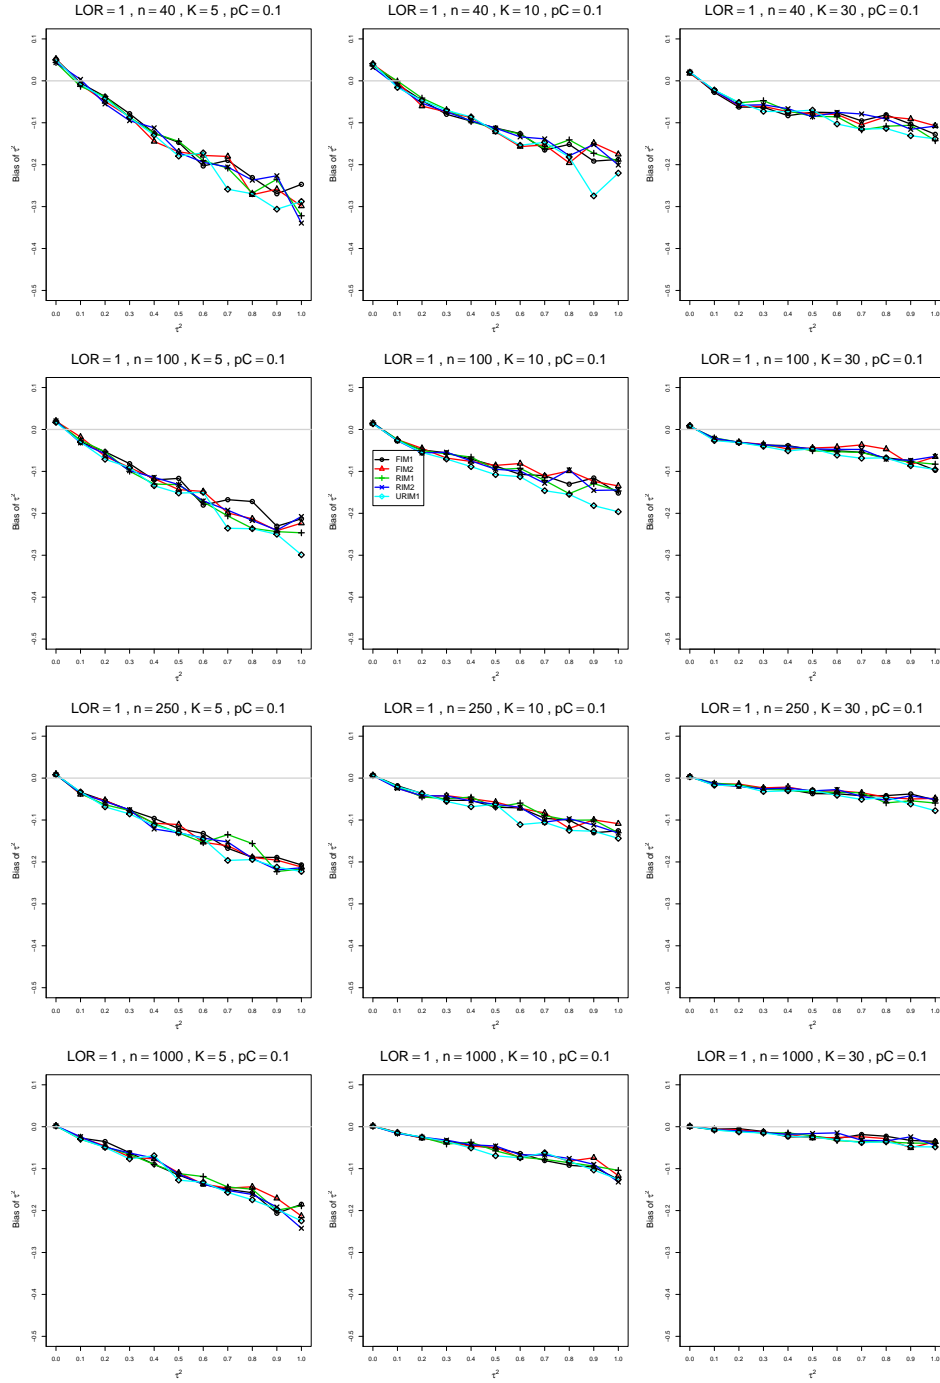

Figure A1.5.15: Bias of between-studies variance  $\hat{\tau}_{FIM2}^2$  for  $\theta = 1$ ,  $p_C = 0.1$ ,  $\sigma^2 = 0.4$ , constant sample sizes  $n = 40, 100, 250, 1000$ . The data-generation mechanisms are FIM1 ( $\circ$ ), FIM2 ( $\triangle$ ), RIM1 ( $+$ ), RIM2 ( $\times$ ), and URIM1 ( $\diamond$ ).

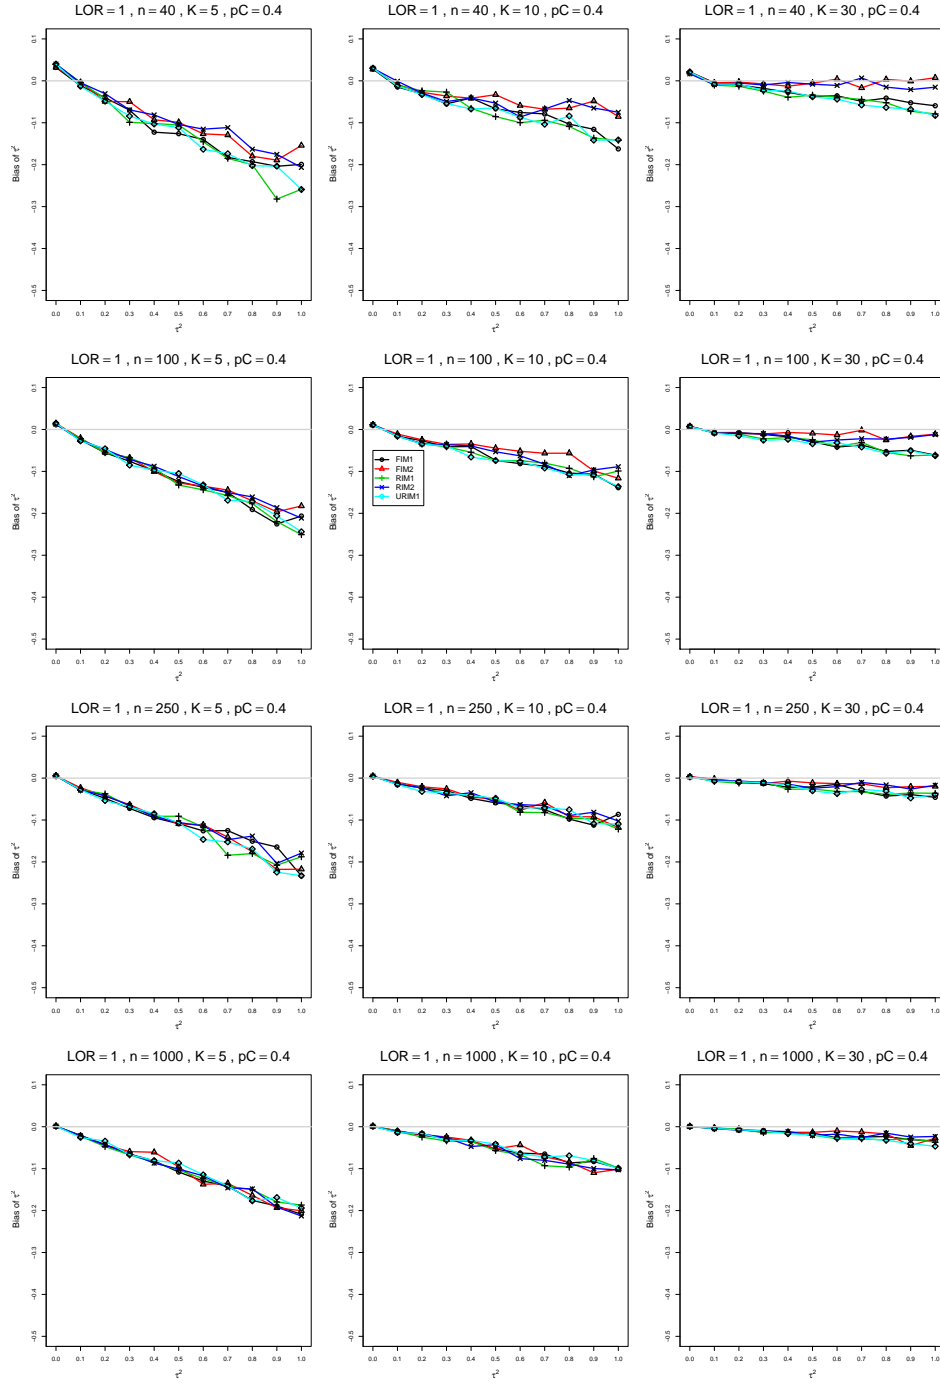

Figure A1.5.16: Bias of between-studies variance  $\hat{\tau}_{FIM2}^2$  for  $\theta = 1$ ,  $p_C = 0.4$ ,  $\sigma^2 = 0.4$ , constant sample sizes  $n = 40, 100, 250, 1000$ . The data-generation mechanisms are FIM1 ( $\circ$ ), FIM2 ( $\triangle$ ), RIM1 ( $+$ ), RIM2 ( $\times$ ), and URIM1 ( $\diamond$ ).

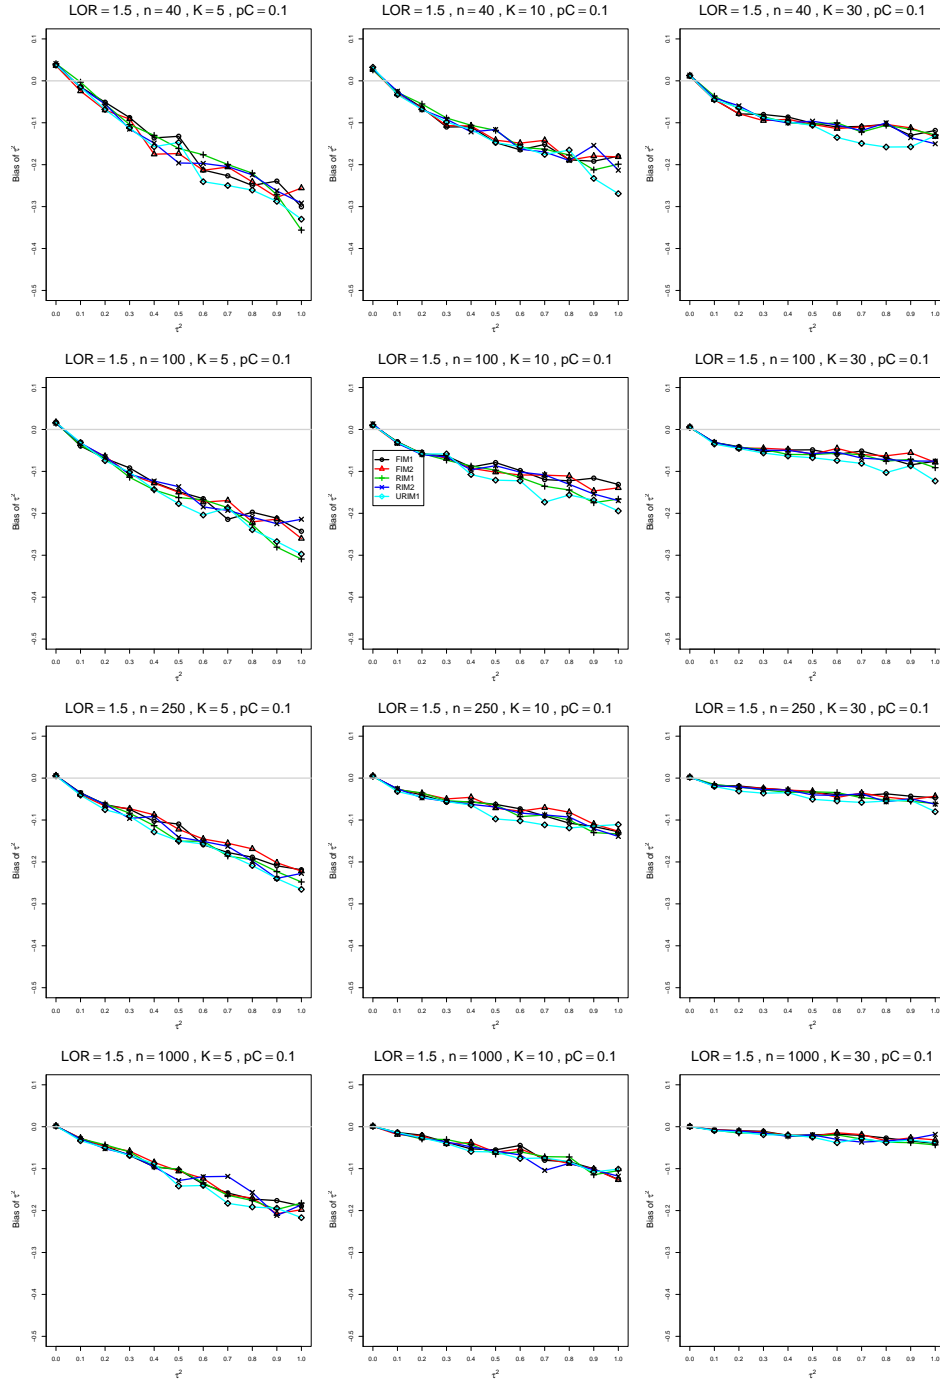

Figure A1.5.17: Bias of between-studies variance  $\hat{\tau}_{FIM2}^2$  for  $\theta = 1.5$ ,  $p_C = 0.1$ ,  $\sigma^2 = 0.4$ , constant sample sizes  $n = 40, 100, 250, 1000$ . The data-generation mechanisms are FIM1 ( $\circ$ ), FIM2 ( $\triangle$ ), RIM1 ( $+$ ), RIM2 ( $\times$ ), and URIM1 ( $\diamond$ ).

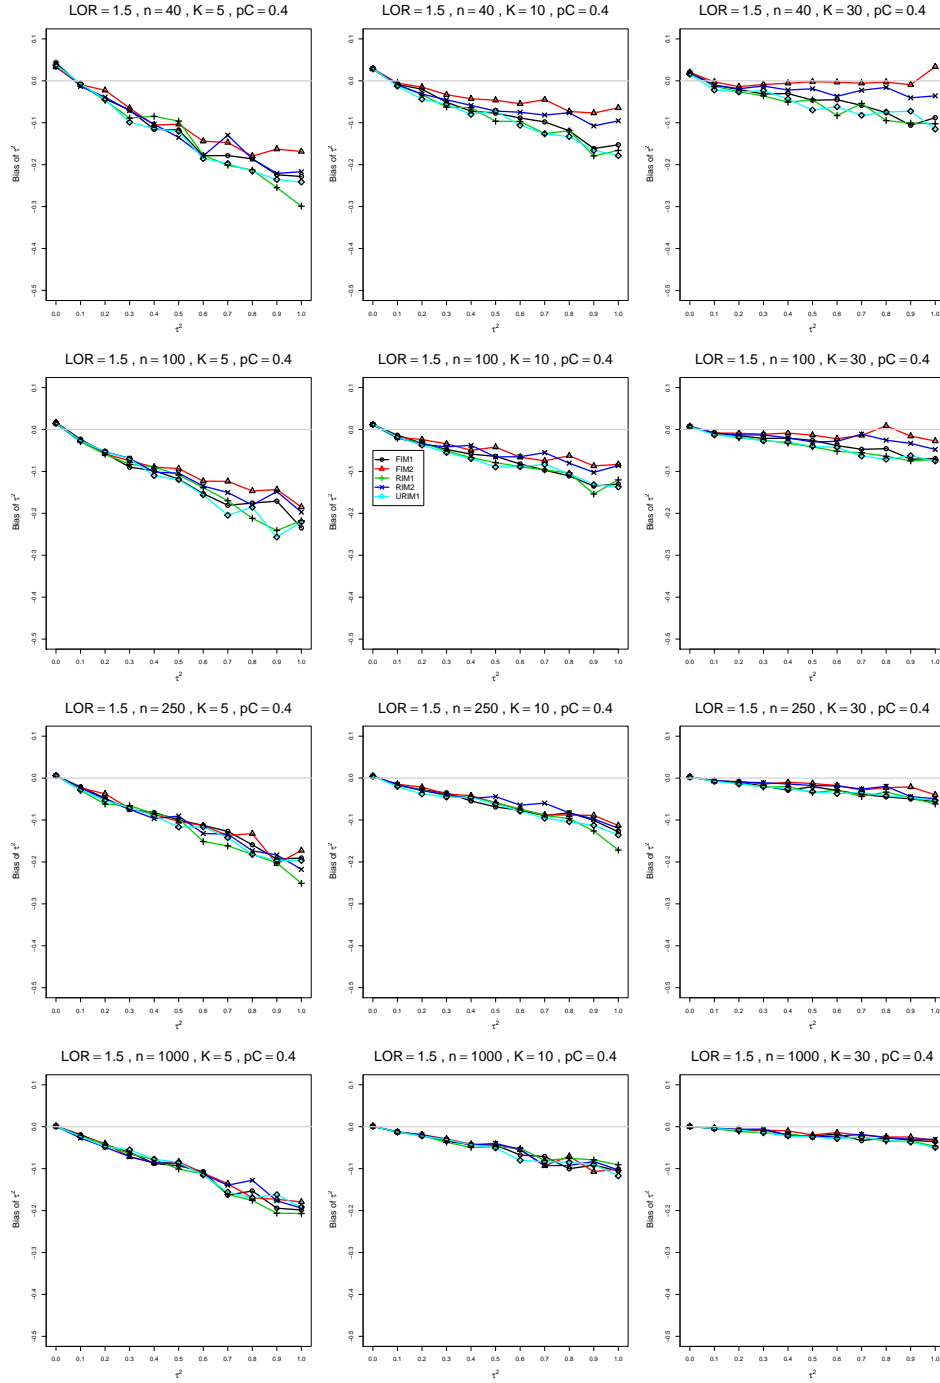

Figure A1.5.18: Bias of between-studies variance  $\hat{\tau}_{FIM2}^2$  for  $\theta = 1.5$ ,  $p_C = 0.4$ ,  $\sigma^2 = 0.4$ , constant sample sizes  $n = 40, 100, 250, 1000$ . The data-generation mechanisms are FIM1 ( $\circ$ ), FIM2 ( $\triangle$ ), RIM1 ( $+$ ), RIM2 ( $\times$ ), and URIM1 ( $\diamond$ ).

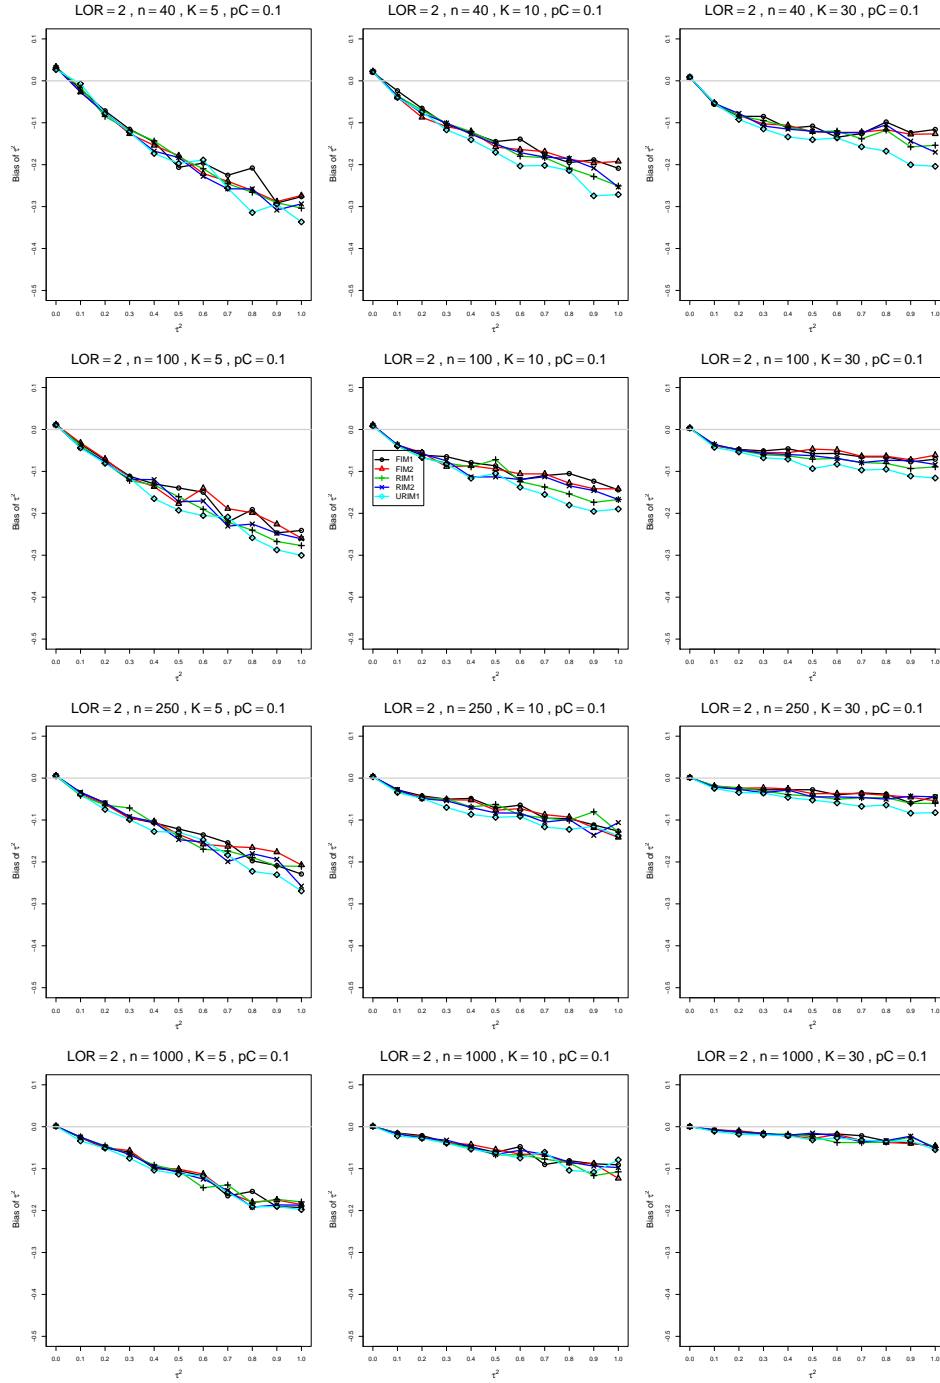

Figure A1.5.19: Bias of between-studies variance  $\hat{\tau}_{FIM2}^2$  for  $\theta = 2$ ,  $p_C = 0.1$ ,  $\sigma^2 = 0.4$ , constant sample sizes  $n = 40, 100, 250, 1000$ . The data-generation mechanisms are FIM1 ( $\circ$ ), FIM2 ( $\triangle$ ), RIM1 ( $+$ ), RIM2 ( $\times$ ), and URIM1 ( $\diamond$ ).

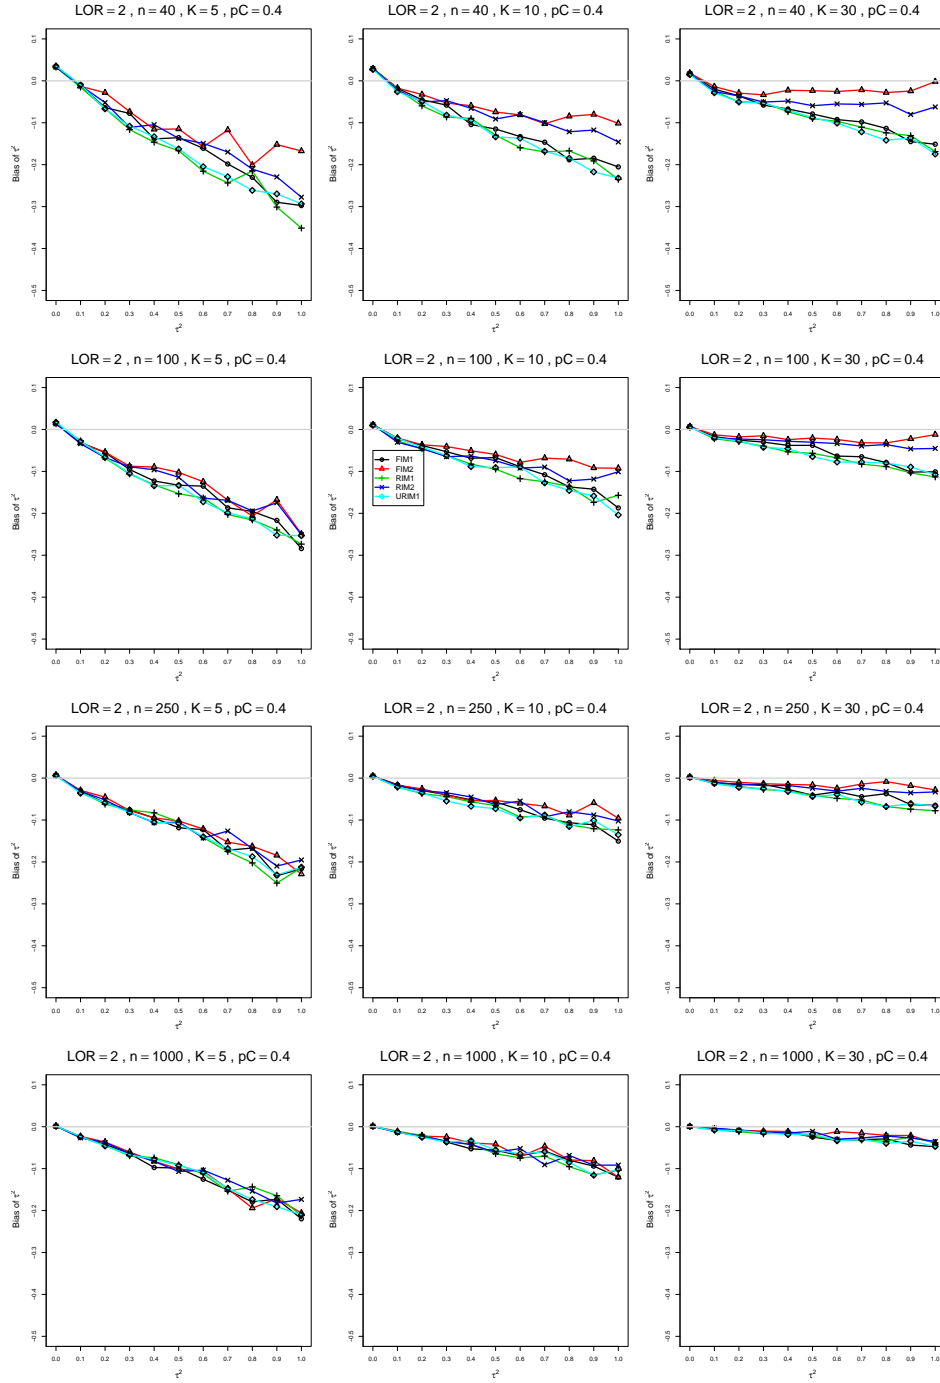

Figure A1.5.20: Bias of between-studies variance  $\hat{\tau}_{FIM2}^2$  for  $\theta = 2$ ,  $p_C = 0.4$ ,  $\sigma^2 = 0.4$ , constant sample sizes  $n = 40, 100, 250, 1000$ . The data-generation mechanisms are FIM1 ( $\circ$ ), FIM2 ( $\triangle$ ), RIM1 ( $+$ ), RIM2 ( $\times$ ), and URIM1 ( $\diamond$ ).

## A1.6 Bias of $\hat{\tau}_{RIM2}^2$



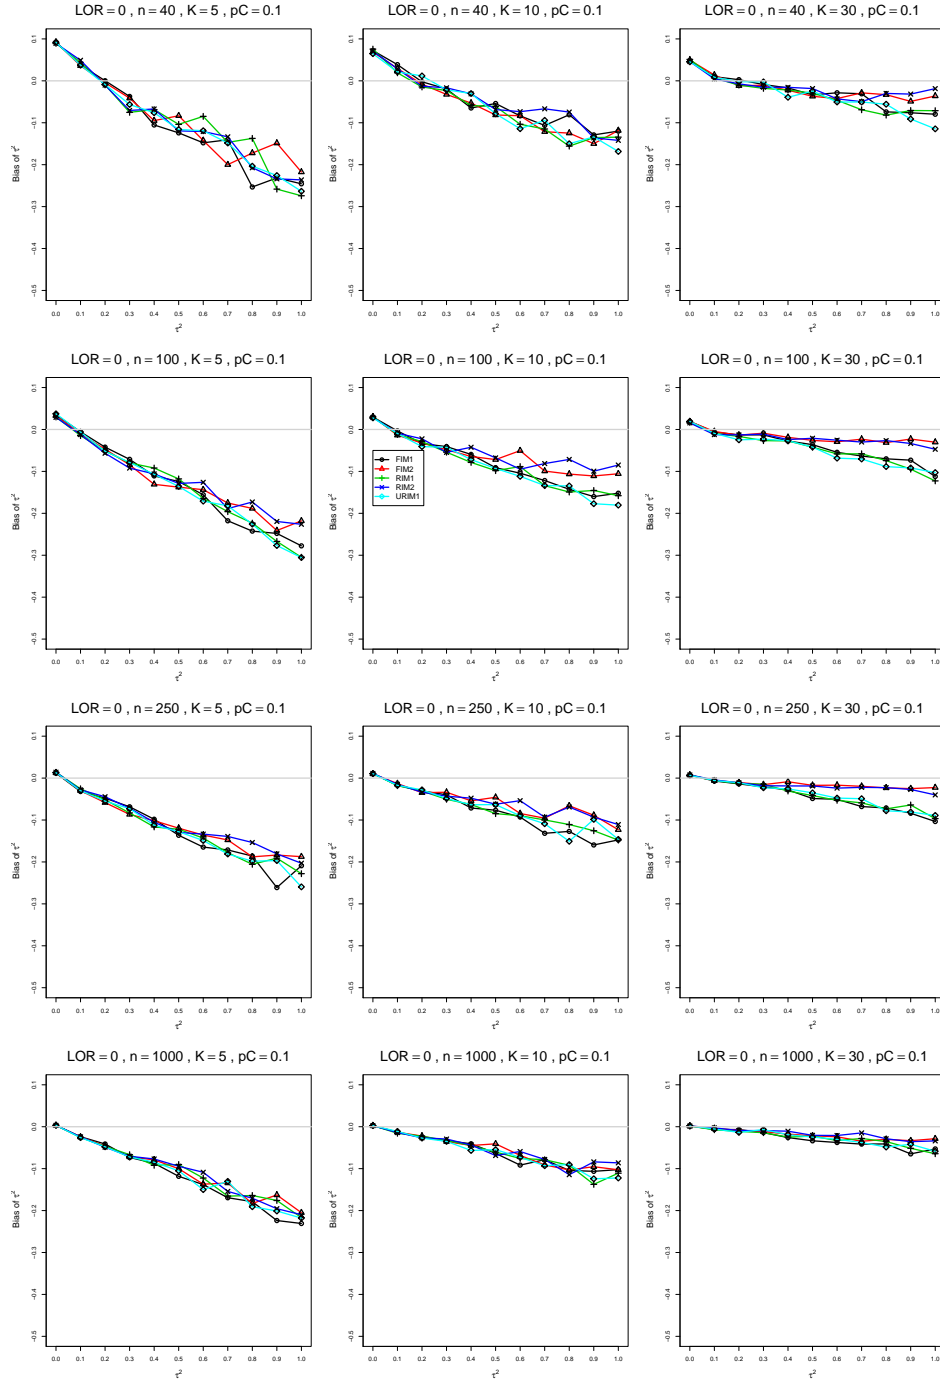

Figure A1.6.1: Bias of between-studies variance  $\hat{\tau}_{RIM2}^2$  for  $\theta = 0$ ,  $p_C = 0.1$ ,  $\sigma^2 = 0.1$ , constant sample sizes  $n = 40, 100, 250, 1000$ . The data-generation mechanisms are FIM1 ( $\circ$ ), FIM2 ( $\triangle$ ), RIM1 ( $+$ ), RIM2 ( $\times$ ), and URIM1 ( $\diamond$ ).

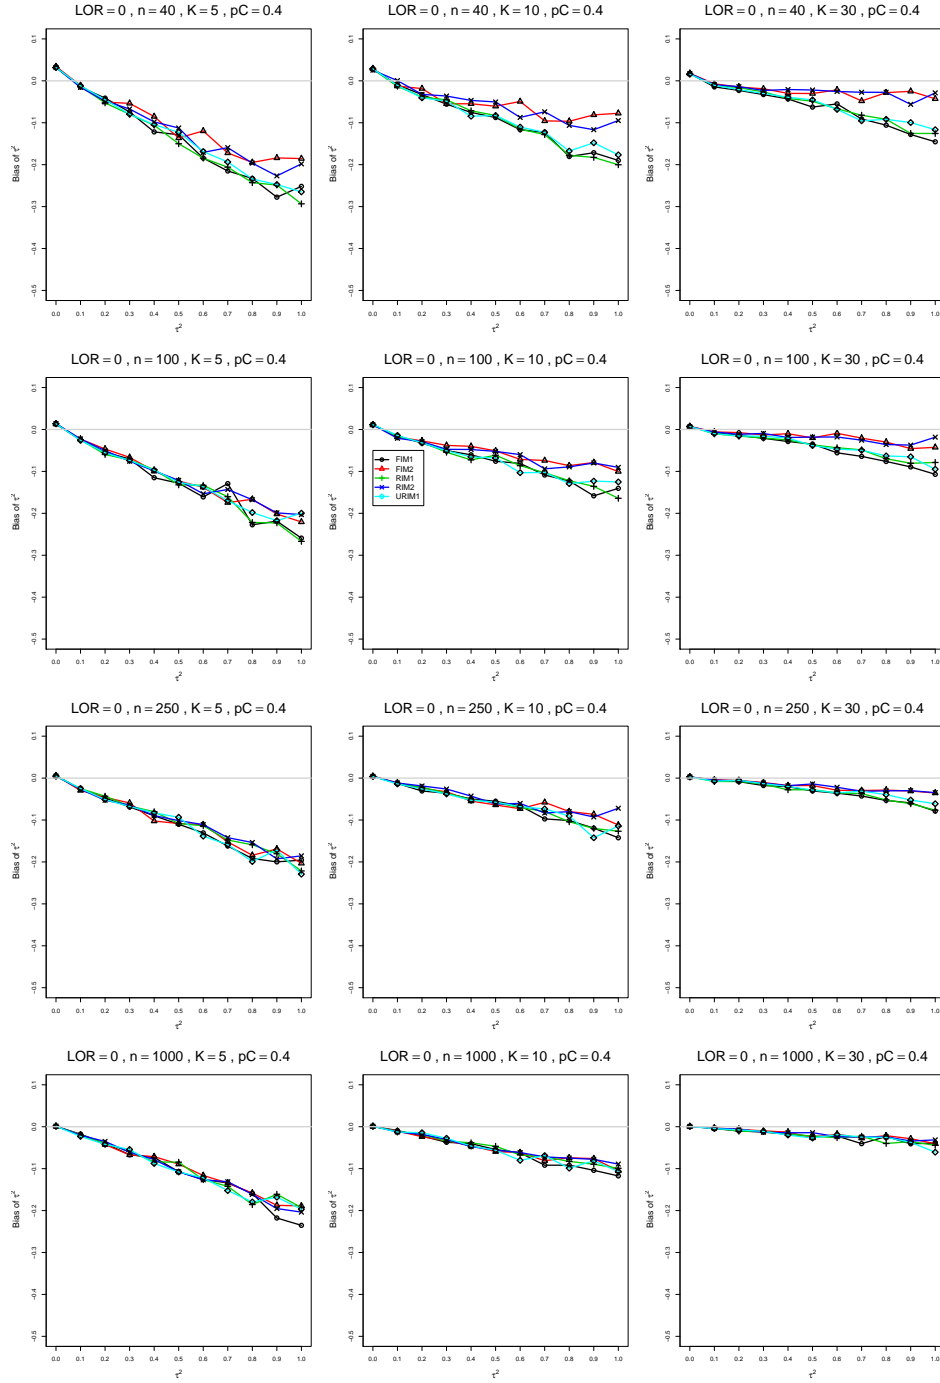

Figure A1.6.2: Bias of between-studies variance  $\hat{\tau}_{RIM2}^2$  for  $\theta = 0$ ,  $p_C = 0.4$ ,  $\sigma^2 = 0.1$ , constant sample sizes  $n = 40, 100, 250, 1000$ . The data-generation mechanisms are FIM1 ( $\circ$ ), FIM2 ( $\triangle$ ), RIM1 ( $+$ ), RIM2 ( $\times$ ), and URIM1 ( $\diamond$ ).

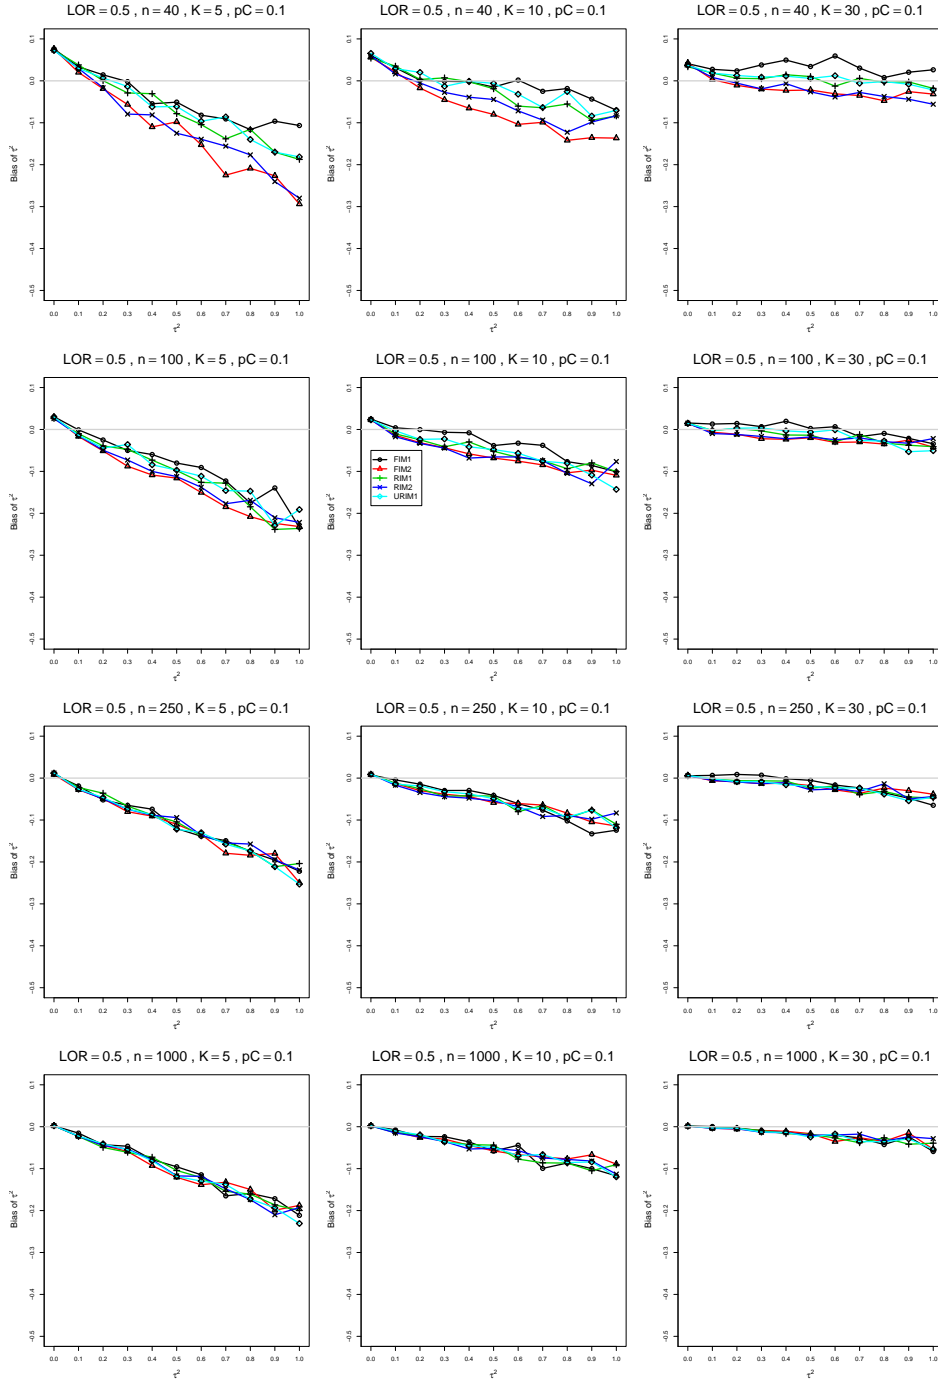

Figure A1.6.3: Bias of between-studies variance  $\hat{\tau}_{RIM2}^2$  for  $\theta = 0.5$ ,  $p_C = 0.1$ ,  $\sigma^2 = 0.1$ , constant sample sizes  $n = 40, 100, 250, 1000$ . The data-generation mechanisms are FIM1 ( $\circ$ ), FIM2 ( $\triangle$ ), RIM1 ( $+$ ), RIM2 ( $\times$ ), and URIM1 ( $\diamond$ ).

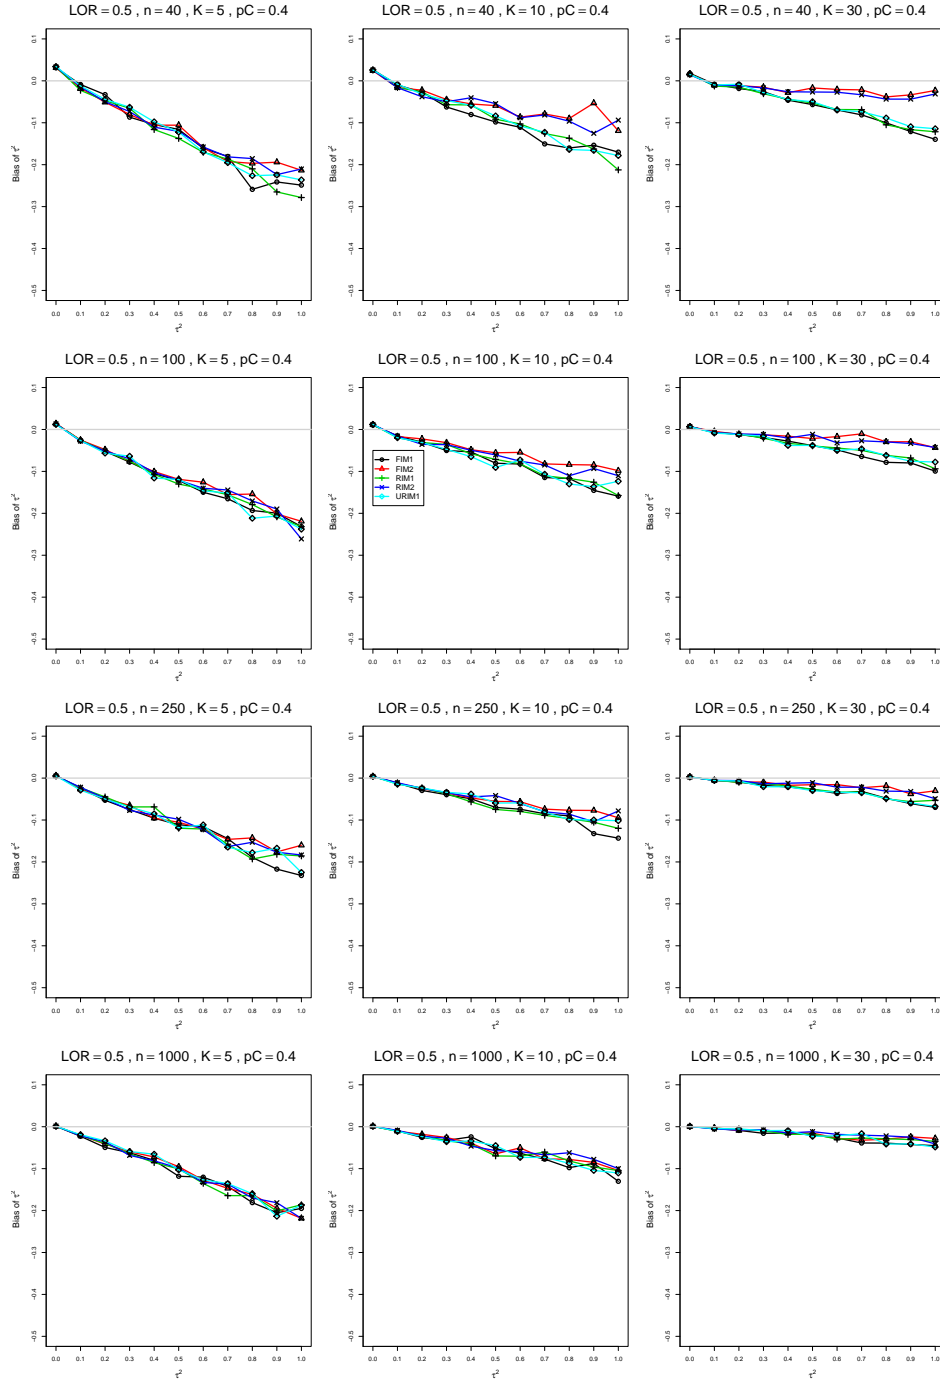

Figure A1.6.4: Bias of between-studies variance  $\hat{\tau}_{RIM2}^2$  for  $\theta = 0.5$ ,  $p_C = 0.4$ ,  $\sigma^2 = 0.1$ , constant sample sizes  $n = 40, 100, 250, 1000$ . The data-generation mechanisms are FIM1 ( $\circ$ ), FIM2 ( $\triangle$ ), RIM1 ( $+$ ), RIM2 ( $\times$ ), and URIM1 ( $\diamond$ ).

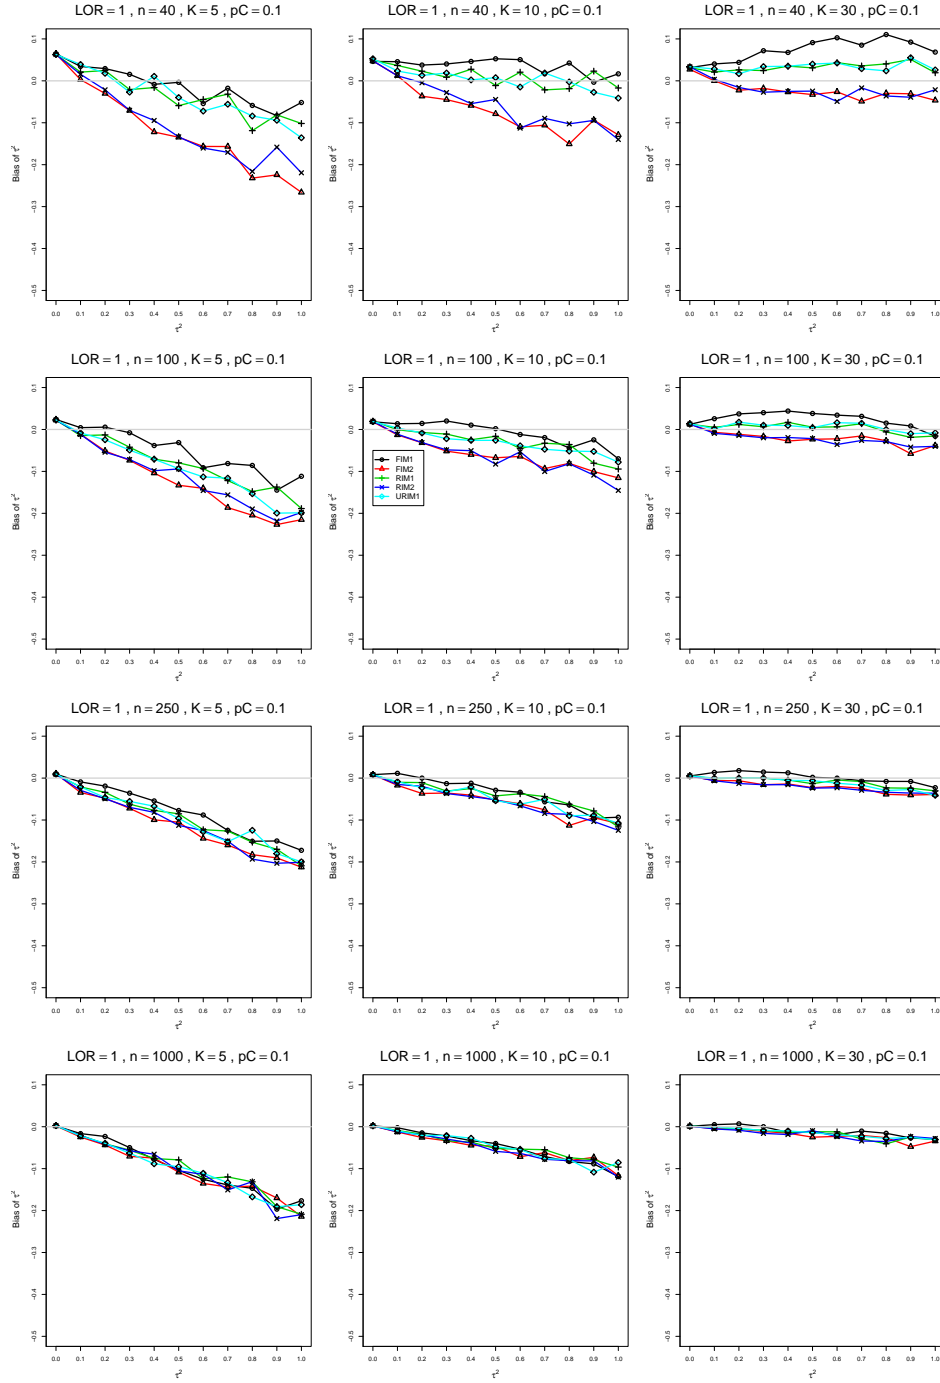

Figure A1.6.5: Bias of between-studies variance  $\hat{\tau}_{RIM2}^2$  for  $\theta = 1$ ,  $p_C = 0.1$ ,  $\sigma^2 = 0.1$ , constant sample sizes  $n = 40, 100, 250, 1000$ . The data-generation mechanisms are FIM1 ( $\circ$ ), FIM2 ( $\triangle$ ), RIM1 ( $+$ ), RIM2 ( $\times$ ), and URIM1 ( $\diamond$ ).

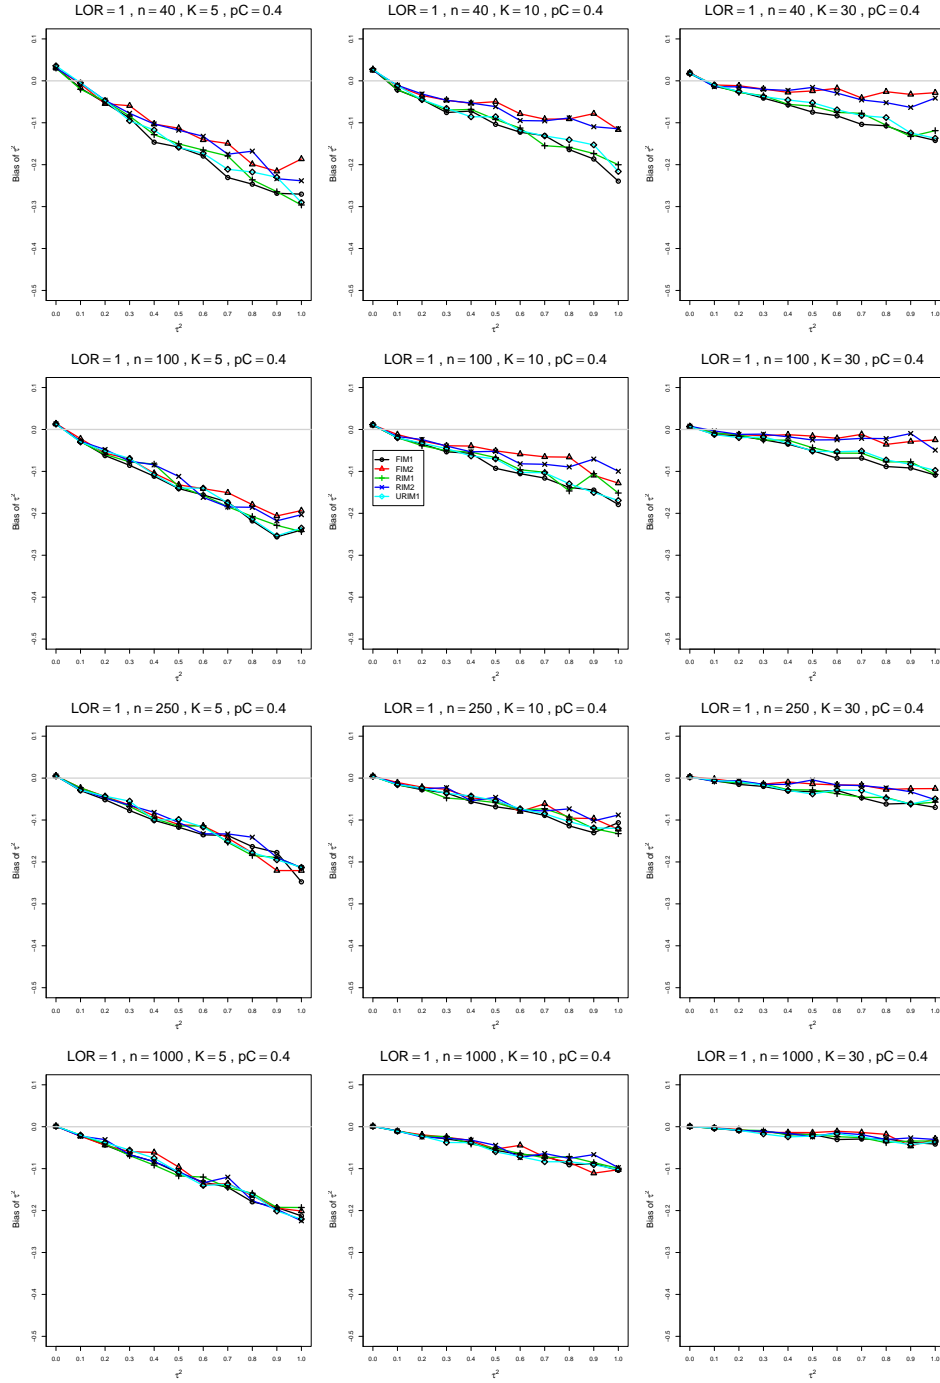

Figure A1.6.6: Bias of between-studies variance  $\hat{\tau}_{RIM2}^2$  for  $\theta = 1$ ,  $p_C = 0.4$ ,  $\sigma^2 = 0.1$ , constant sample sizes  $n = 40, 100, 250, 1000$ . The data-generation mechanisms are FIM1 ( $\circ$ ), FIM2 ( $\triangle$ ), RIM1 ( $+$ ), RIM2 ( $\times$ ), and URIM1 ( $\diamond$ ).

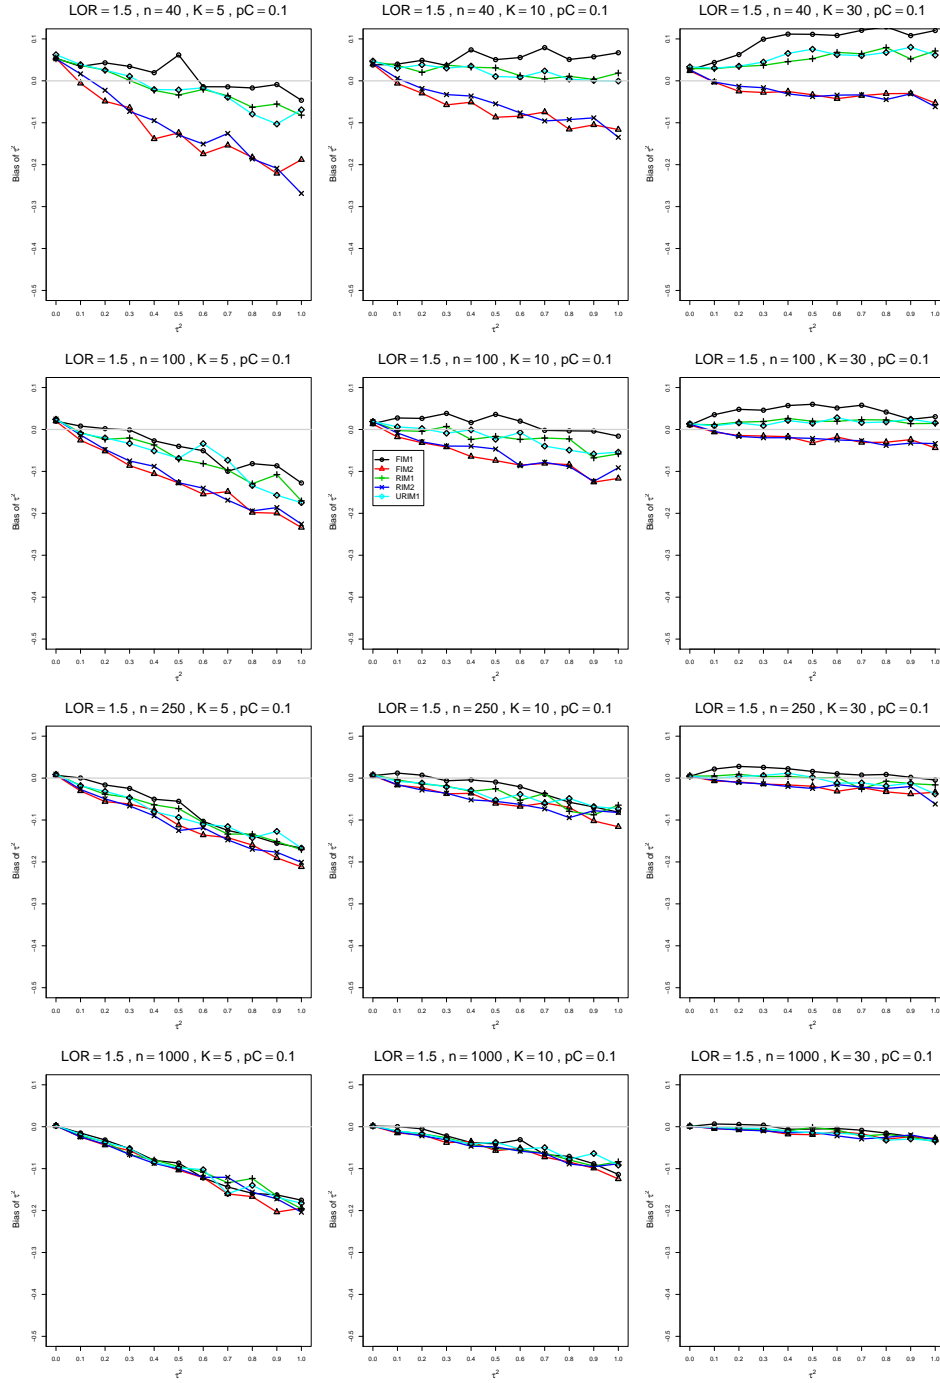

Figure A1.6.7: Bias of between-studies variance  $\hat{\tau}_{RIM2}^2$  for  $\theta = 1.5$ ,  $p_C = 0.1$ ,  $\sigma^2 = 0.1$ , constant sample sizes  $n = 40, 100, 250, 1000$ . The data-generation mechanisms are FIM1 ( $\circ$ ), FIM2 ( $\triangle$ ), RIM1 ( $+$ ), RIM2 ( $\times$ ), and URIM1 ( $\diamond$ ).

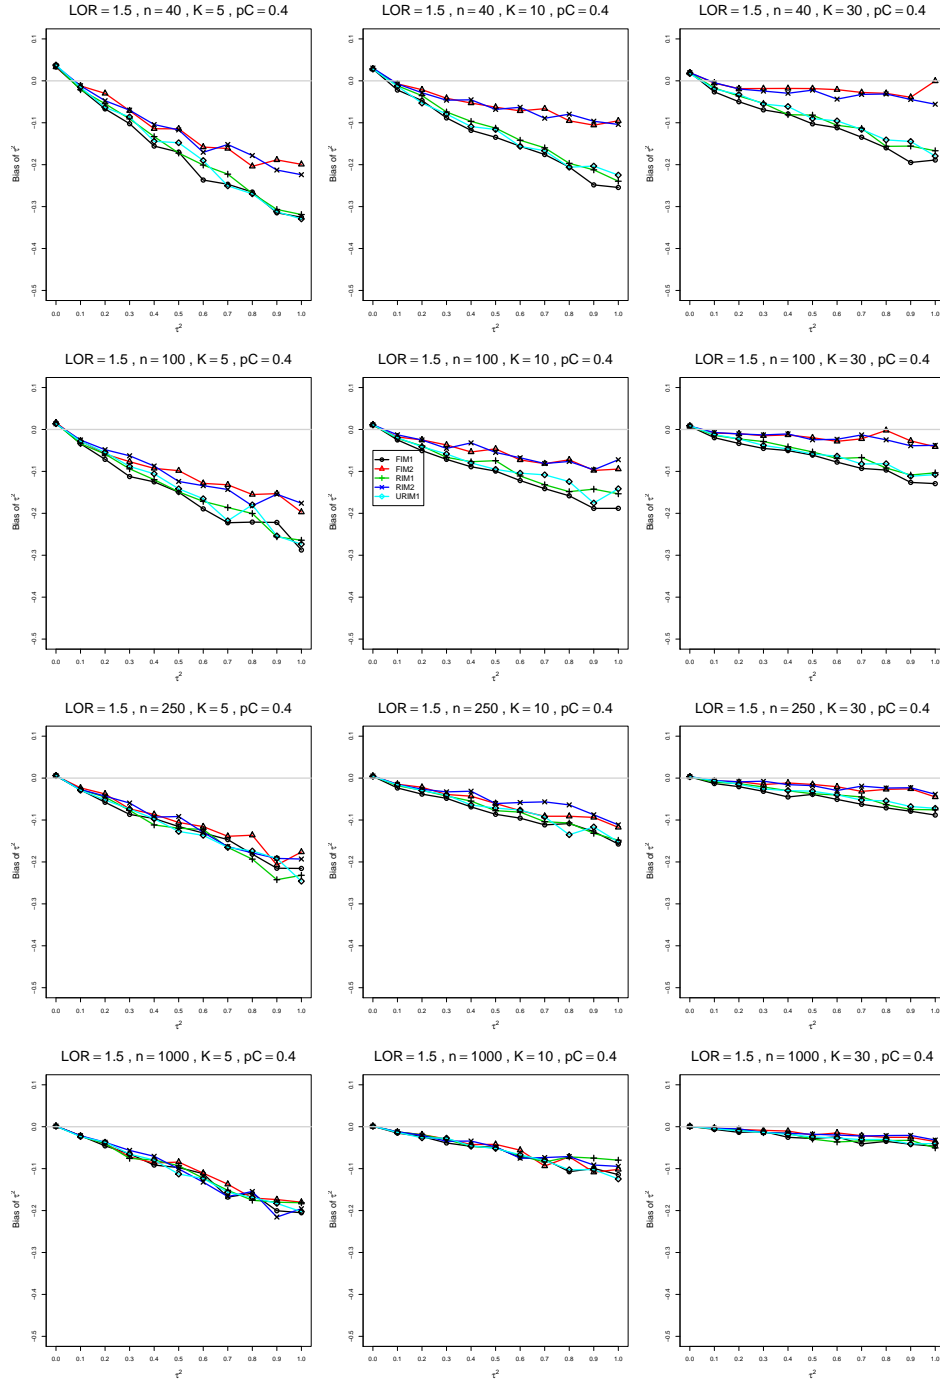

Figure A1.6.8: Bias of between-studies variance  $\hat{\tau}_{RIM2}^2$  for  $\theta = 1.5$ ,  $p_C = 0.4$ ,  $\sigma^2 = 0.1$ , constant sample sizes  $n = 40, 100, 250, 1000$ . The data-generation mechanisms are FIM1 ( $\circ$ ), FIM2 ( $\triangle$ ), RIM1 ( $+$ ), RIM2 ( $\times$ ), and URIM1 ( $\diamond$ ).



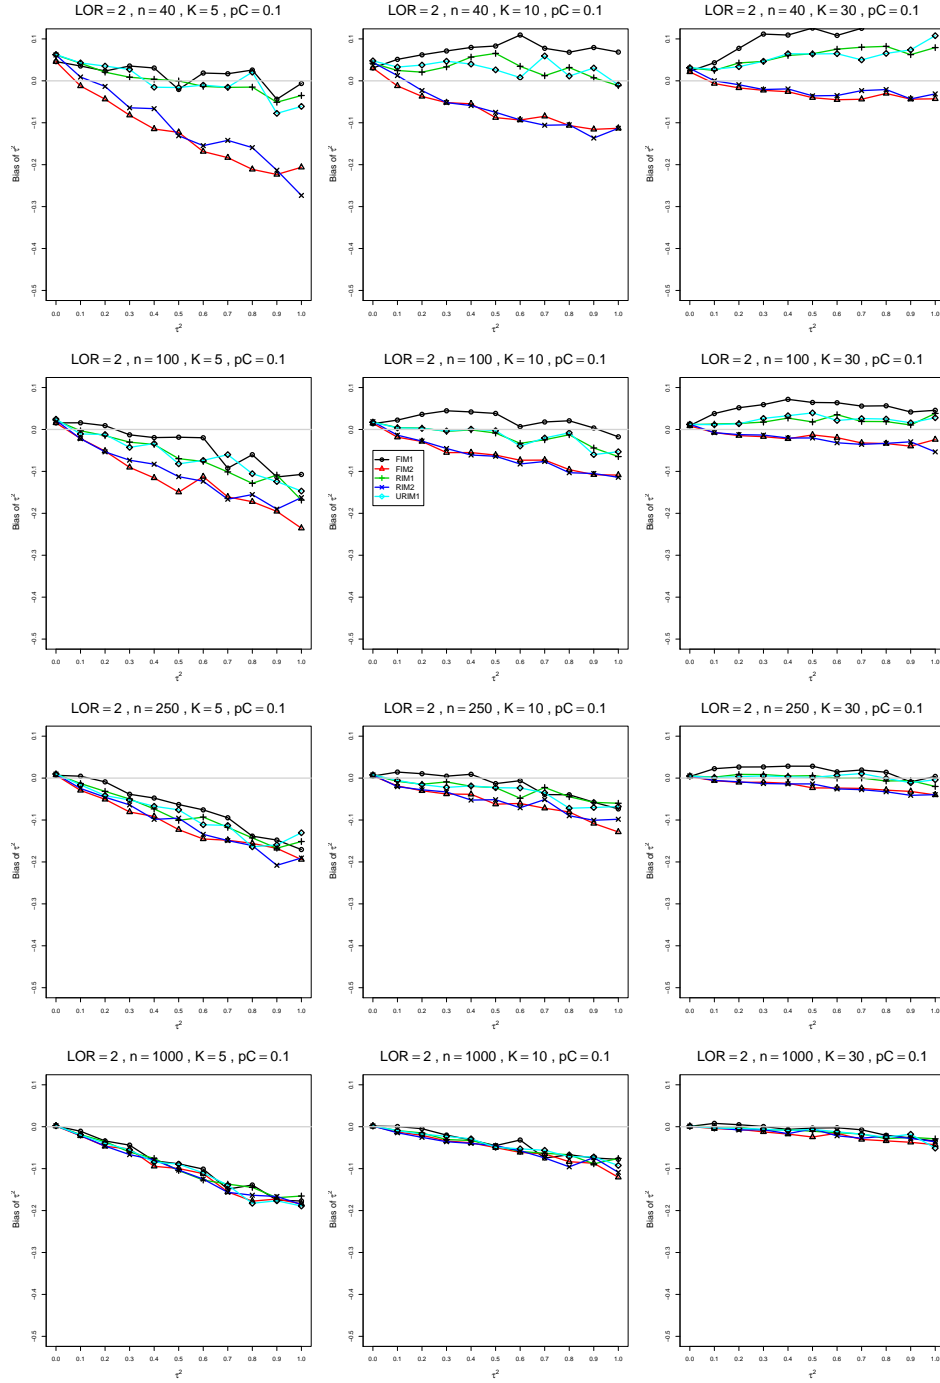

Figure A1.6.9: Bias of between-studies variance  $\hat{\tau}_{RIM2}^2$  for  $\theta = 2$ ,  $p_C = 0.1$ ,  $\sigma^2 = 0.1$ , constant sample sizes  $n = 40, 100, 250, 1000$ . The data-generation mechanisms are FIM1 ( $\circ$ ), FIM2 ( $\triangle$ ), RIM1 ( $+$ ), RIM2 ( $\times$ ), and URIM1 ( $\diamond$ ).

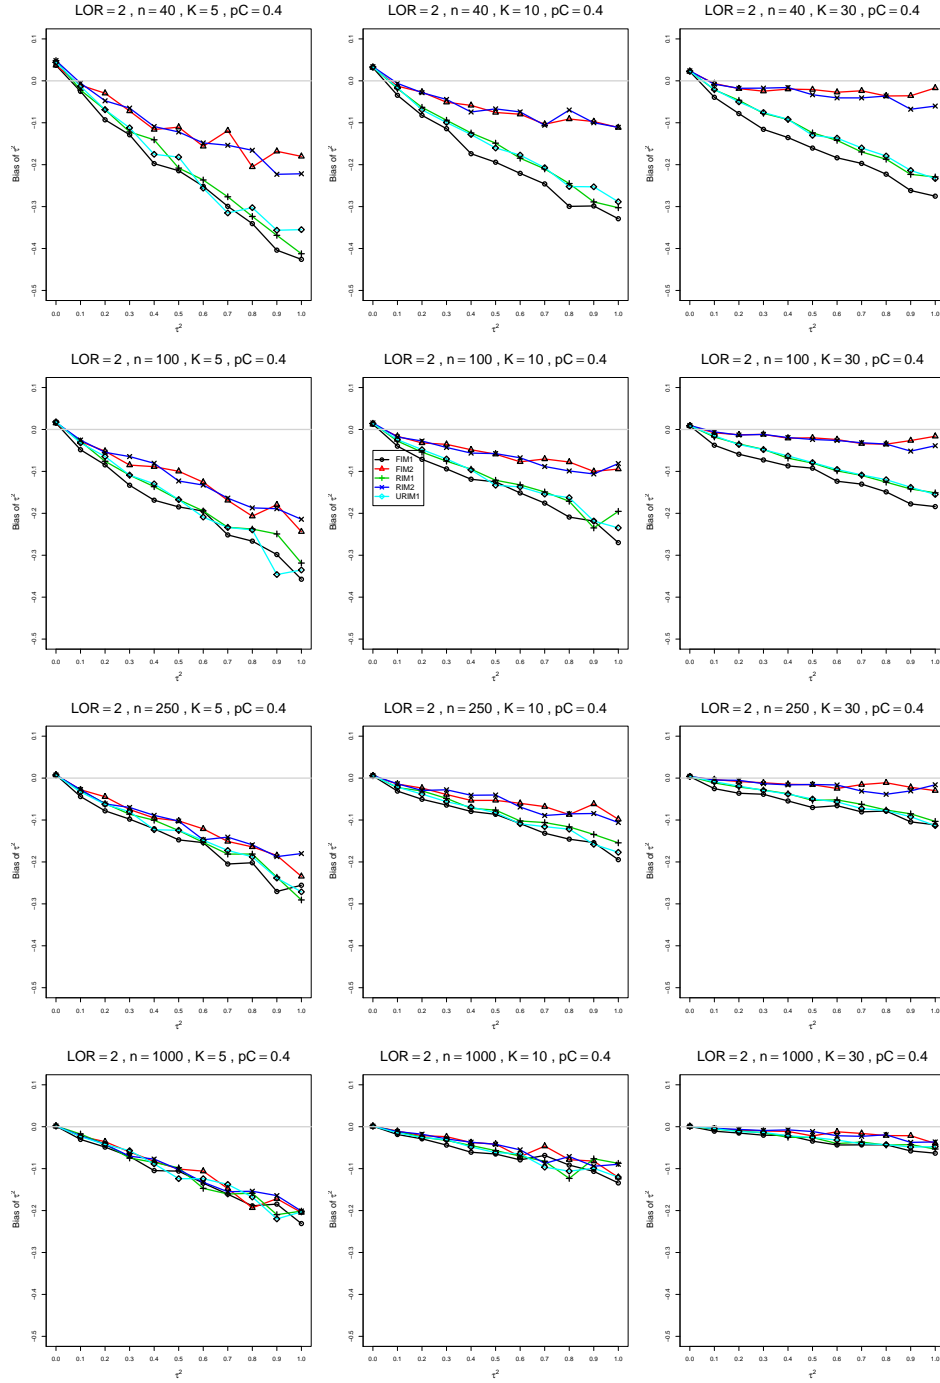

Figure A1.6.10: Bias of between-studies variance  $\hat{\tau}_{RIM2}^2$  for  $\theta = 2$ ,  $p_C = 0.4$ ,  $\sigma^2 = 0.1$ , constant sample sizes  $n = 40, 100, 250, 1000$ . The data-generation mechanisms are FIM1 ( $\circ$ ), FIM2 ( $\triangle$ ), RIM1 ( $+$ ), RIM2 ( $\times$ ), and URIM1 ( $\diamond$ ).

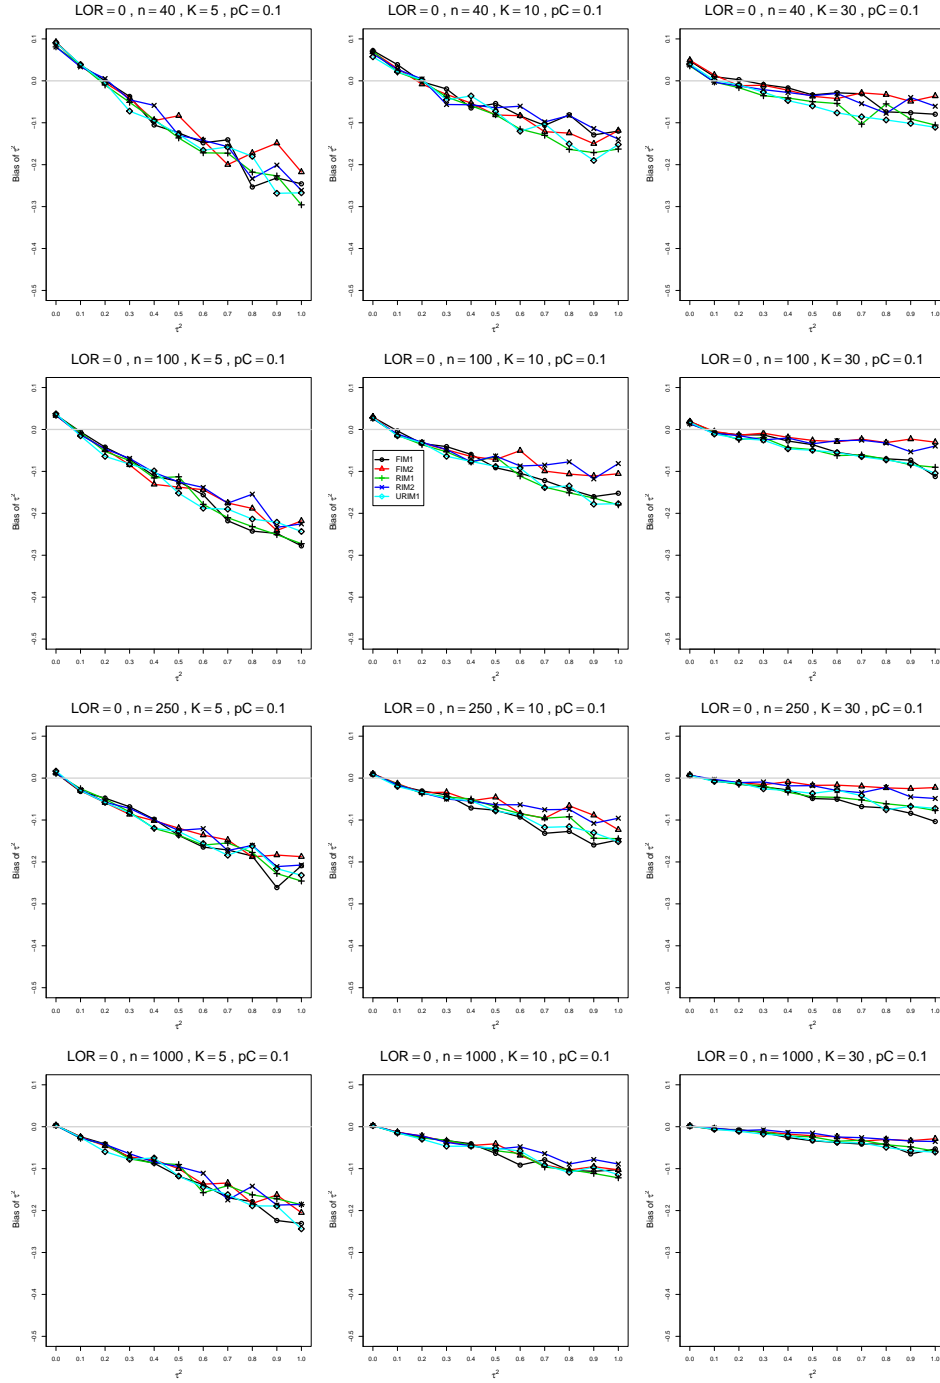

Figure A1.6.11: Bias of between-studies variance  $\hat{\tau}_{RIM2}^2$  for  $\theta = 0$ ,  $p_C = 0.1$ ,  $\sigma^2 = 0.4$ , constant sample sizes  $n = 40, 100, 250, 1000$ . The data-generation mechanisms are FIM1 ( $\circ$ ), FIM2 ( $\triangle$ ), RIM1 ( $+$ ), RIM2 ( $\times$ ), and URIM1 ( $\diamond$ ).

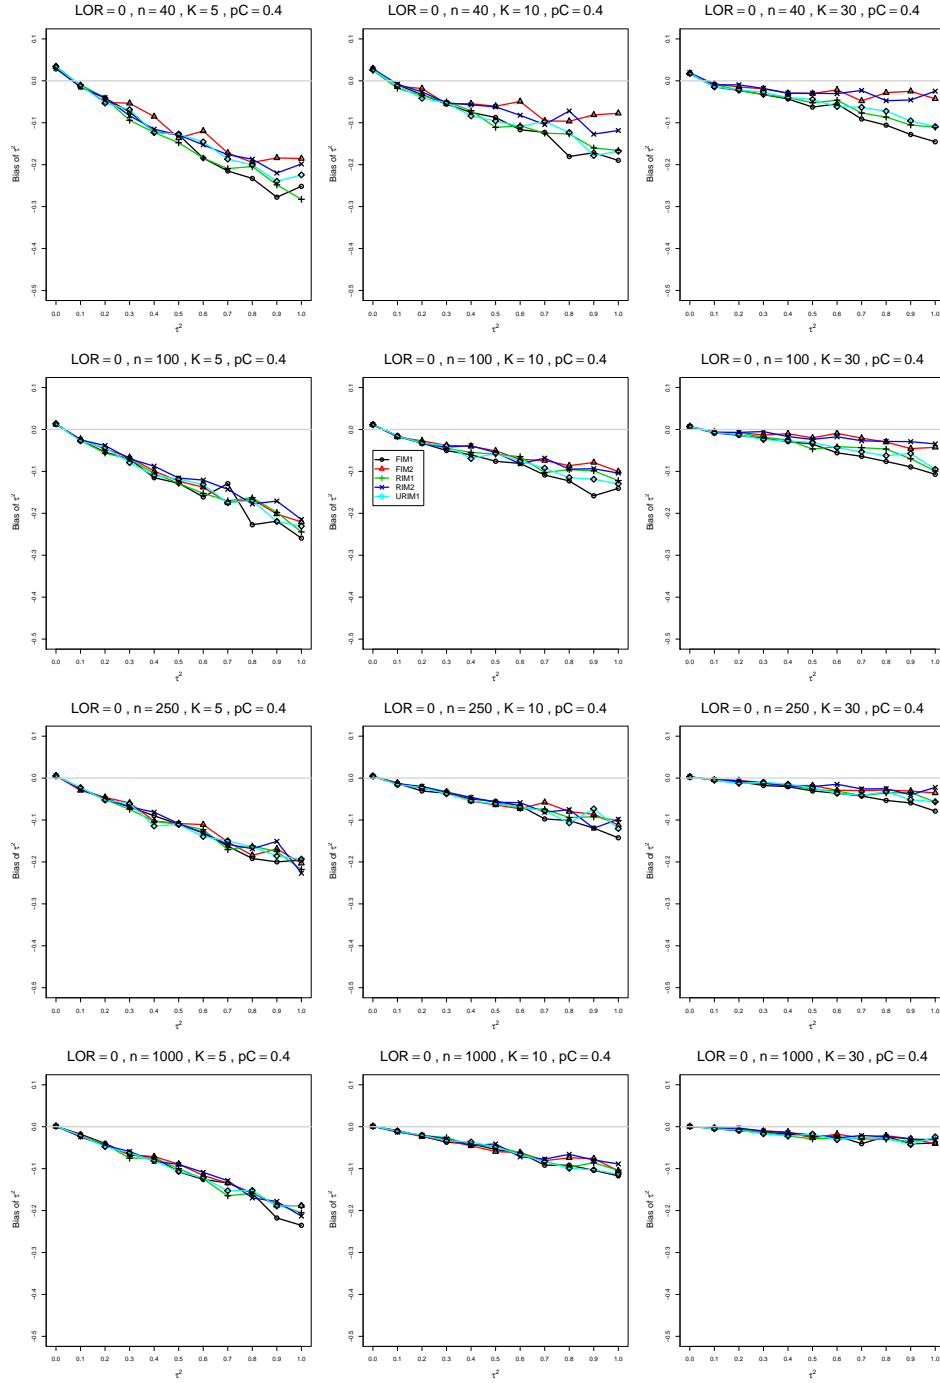

Figure A1.6.12: Bias of between-studies variance  $\hat{\tau}_{RIM2}^2$  for  $\theta = 0$ ,  $p_C = 0.4$ ,  $\sigma^2 = 0.4$ , constant sample sizes  $n = 40, 100, 250, 1000$ . The data-generation mechanisms are FIM1 ( $\circ$ ), FIM2 ( $\triangle$ ), RIM1 ( $+$ ), RIM2 ( $\times$ ), and URIM1 ( $\diamond$ ).

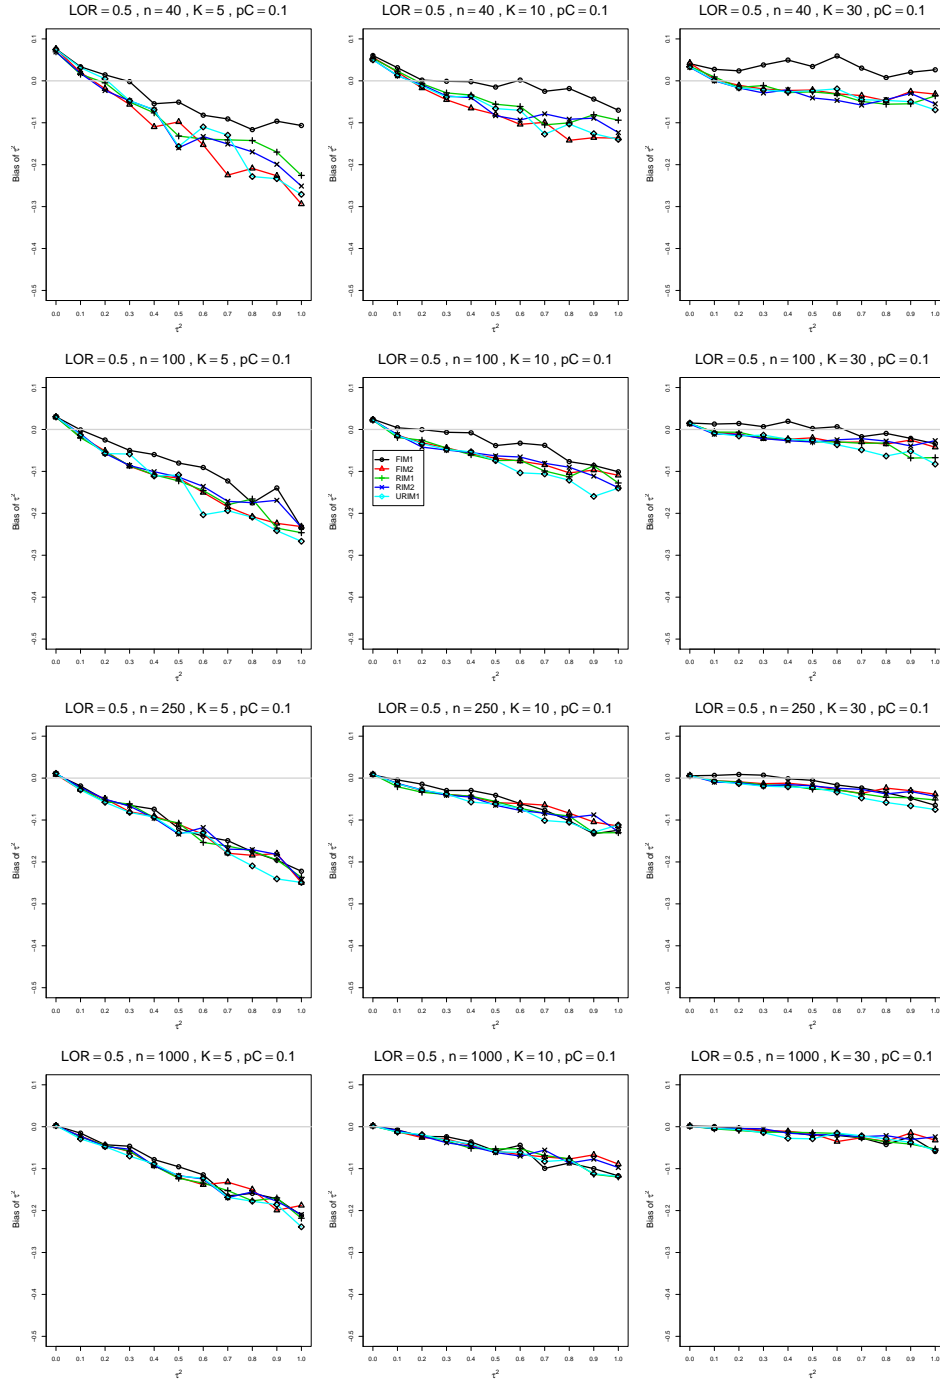

Figure A1.6.13: Bias of between-studies variance  $\hat{\tau}_{RIM2}^2$  for  $\theta = 0.5$ ,  $p_C = 0.1$ ,  $\sigma^2 = 0.4$ , constant sample sizes  $n = 40, 100, 250, 1000$ . The data-generation mechanisms are FIM1 ( $\circ$ ), FIM2 ( $\triangle$ ), RIM1 ( $+$ ), RIM2 ( $\times$ ), and URIM1 ( $\diamond$ ).

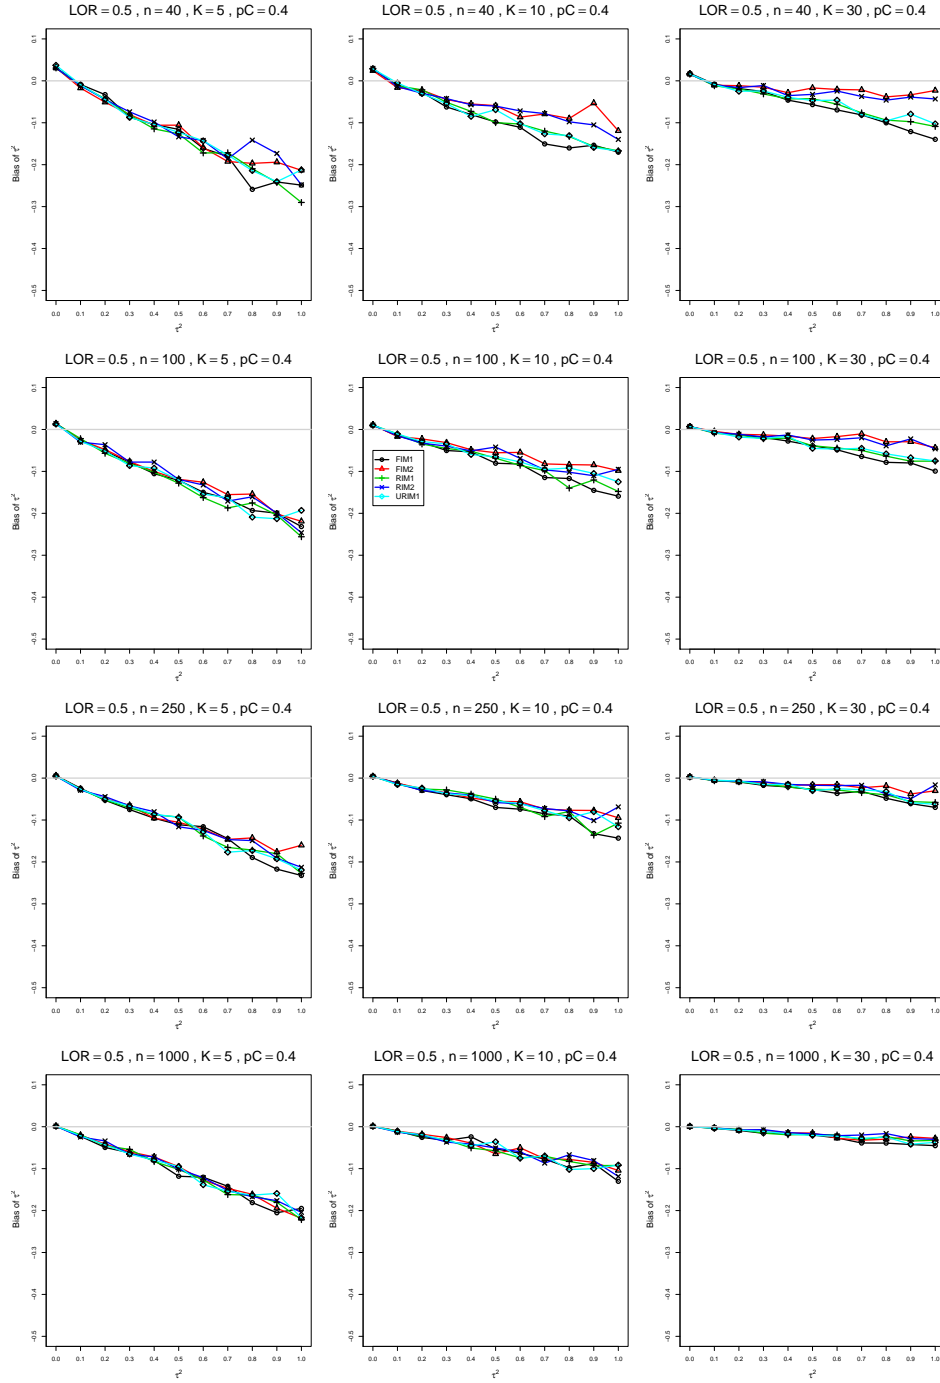

Figure A1.6.14: Bias of between-studies variance  $\hat{\tau}_{RIM2}^2$  for  $\theta = 0.5$ ,  $p_C = 0.4$ ,  $\sigma^2 = 0.4$ , constant sample sizes  $n = 40, 100, 250, 1000$ . The data-generation mechanisms are FIM1 ( $\circ$ ), FIM2 ( $\triangle$ ), RIM1 ( $+$ ), RIM2 ( $\times$ ), and URIM1 ( $\diamond$ ).

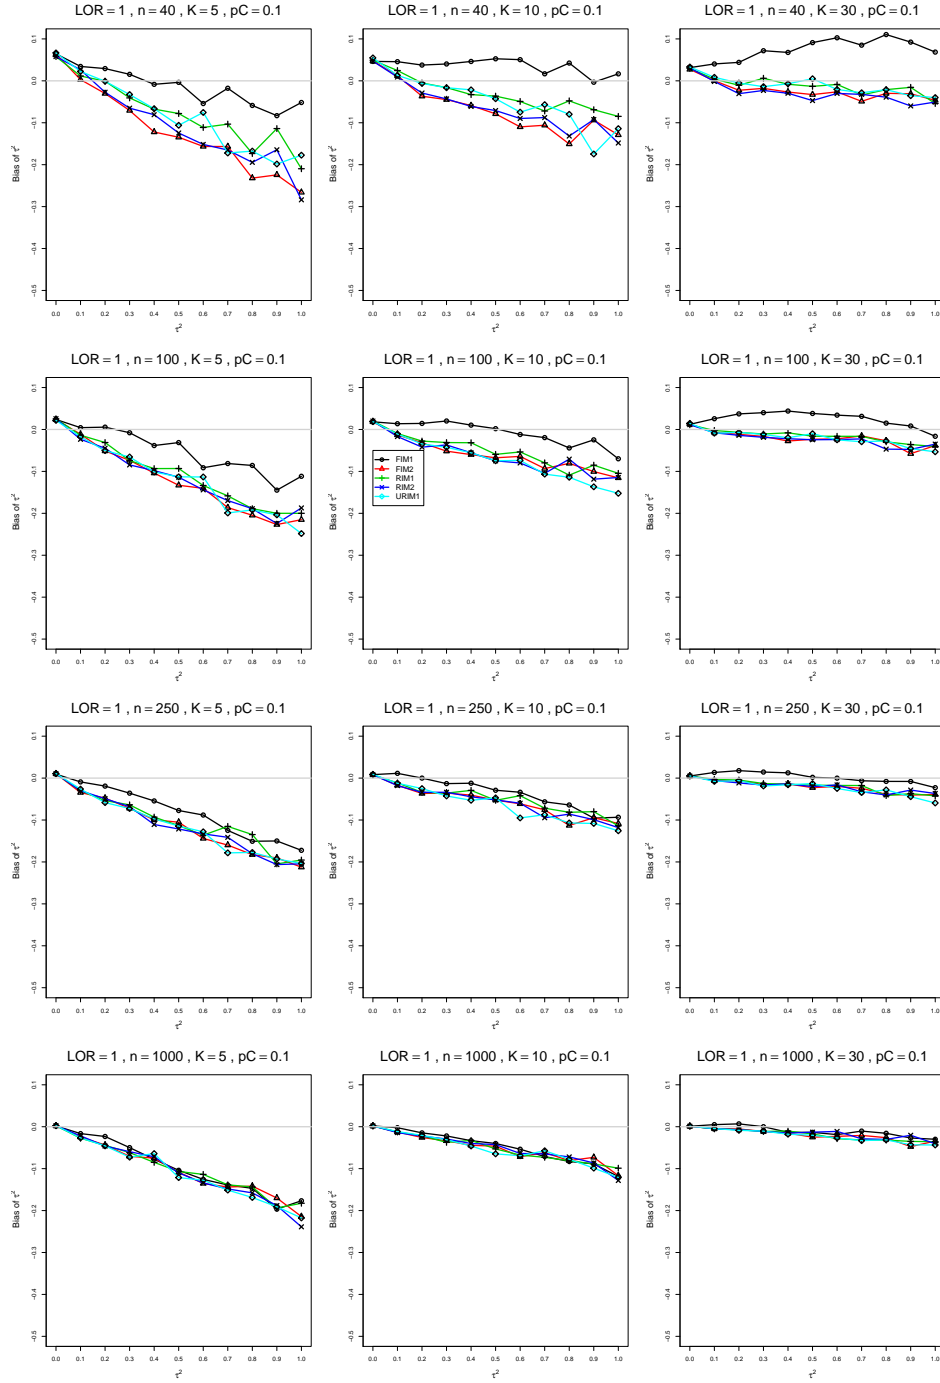

Figure A1.6.15: Bias of between-studies variance  $\hat{\tau}_{RIM2}^2$  for  $\theta = 1$ ,  $p_C = 0.1$ ,  $\sigma^2 = 0.4$ , constant sample sizes  $n = 40, 100, 250, 1000$ . The data-generation mechanisms are FIM1 ( $\circ$ ), FIM2 ( $\triangle$ ), RIM1 ( $+$ ), RIM2 ( $\times$ ), and URIM1 ( $\diamond$ ).

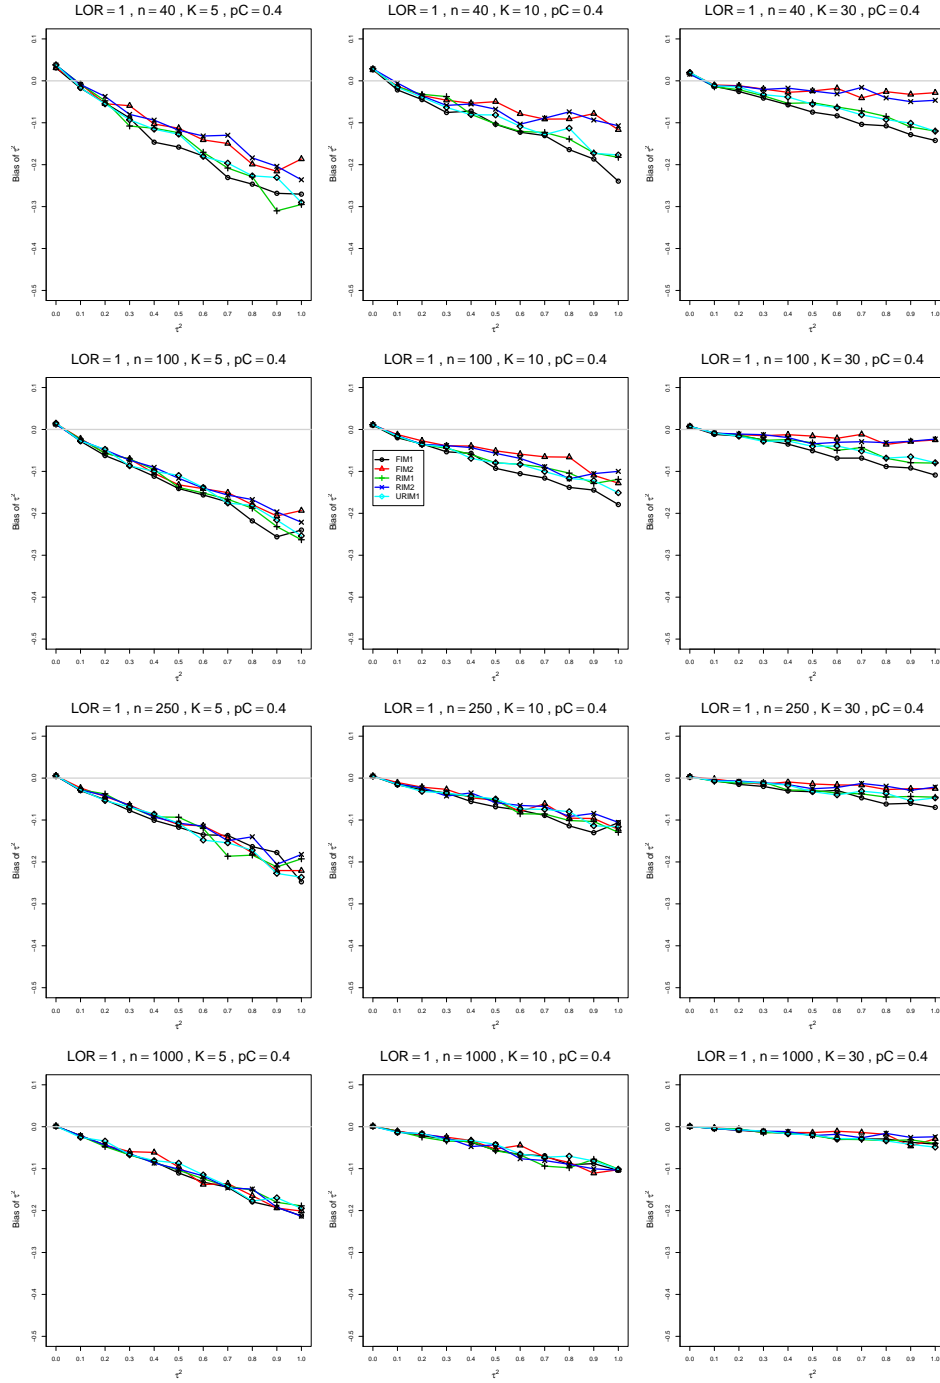

Figure A1.6.16: Bias of between-studies variance  $\hat{\tau}_{RIM2}^2$  for  $\theta = 1$ ,  $p_C = 0.4$ ,  $\sigma^2 = 0.4$ , constant sample sizes  $n = 40, 100, 250, 1000$ . The data-generation mechanisms are FIM1 ( $\circ$ ), FIM2 ( $\triangle$ ), RIM1 ( $+$ ), RIM2 ( $\times$ ), and URIM1 ( $\diamond$ ).



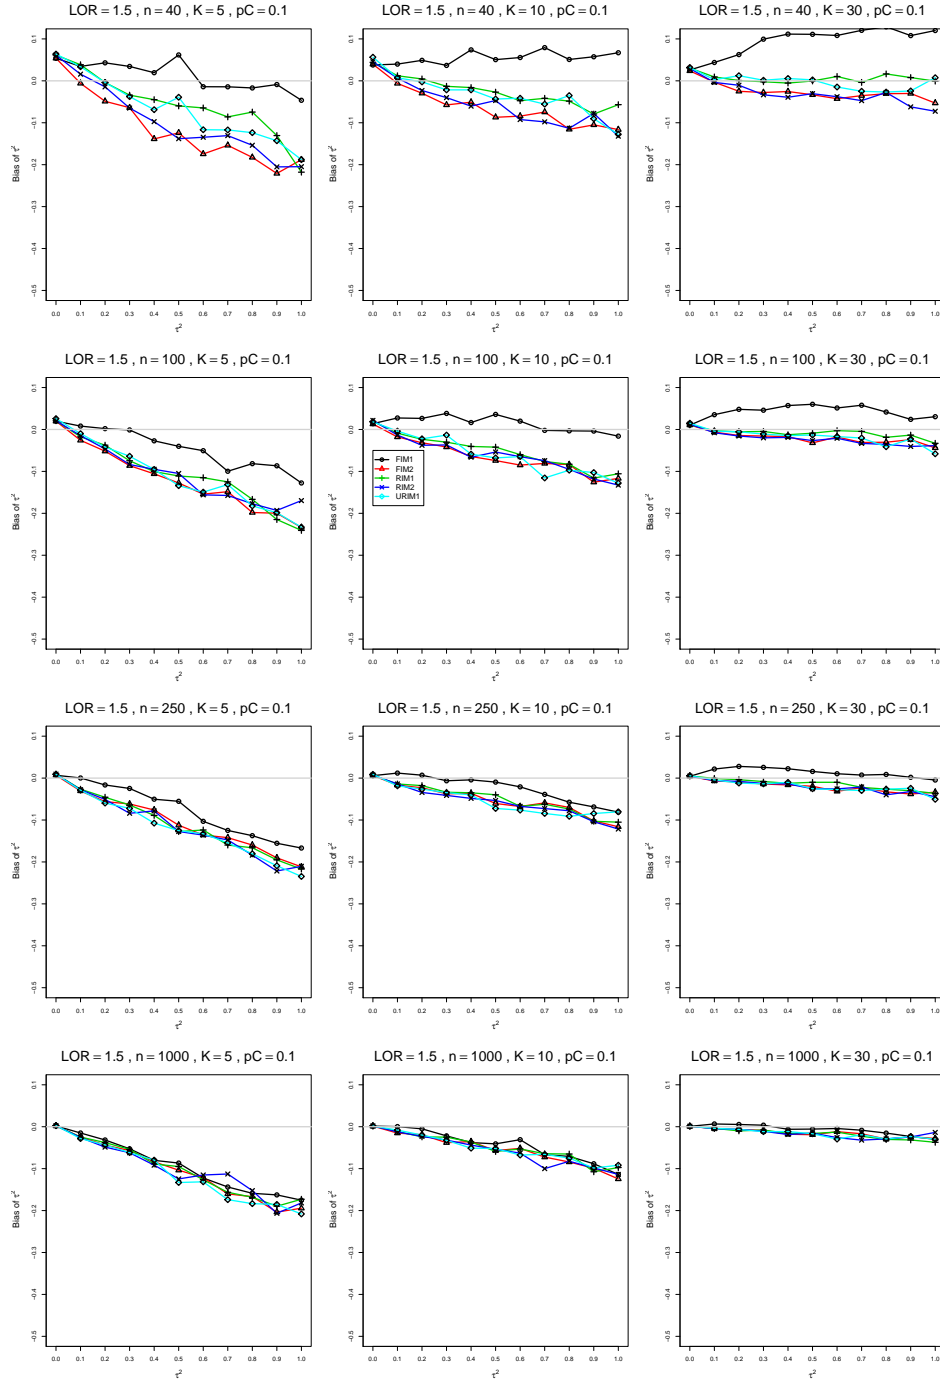

Figure A1.6.17: Bias of between-studies variance  $\hat{\tau}_{RIM2}^2$  for  $\theta = 1.5$ ,  $p_C = 0.1$ ,  $\sigma^2 = 0.4$ , constant sample sizes  $n = 40, 100, 250, 1000$ . The data-generation mechanisms are FIM1 ( $\circ$ ), FIM2 ( $\triangle$ ), RIM1 ( $+$ ), RIM2 ( $\times$ ), and URIM1 ( $\diamond$ ).

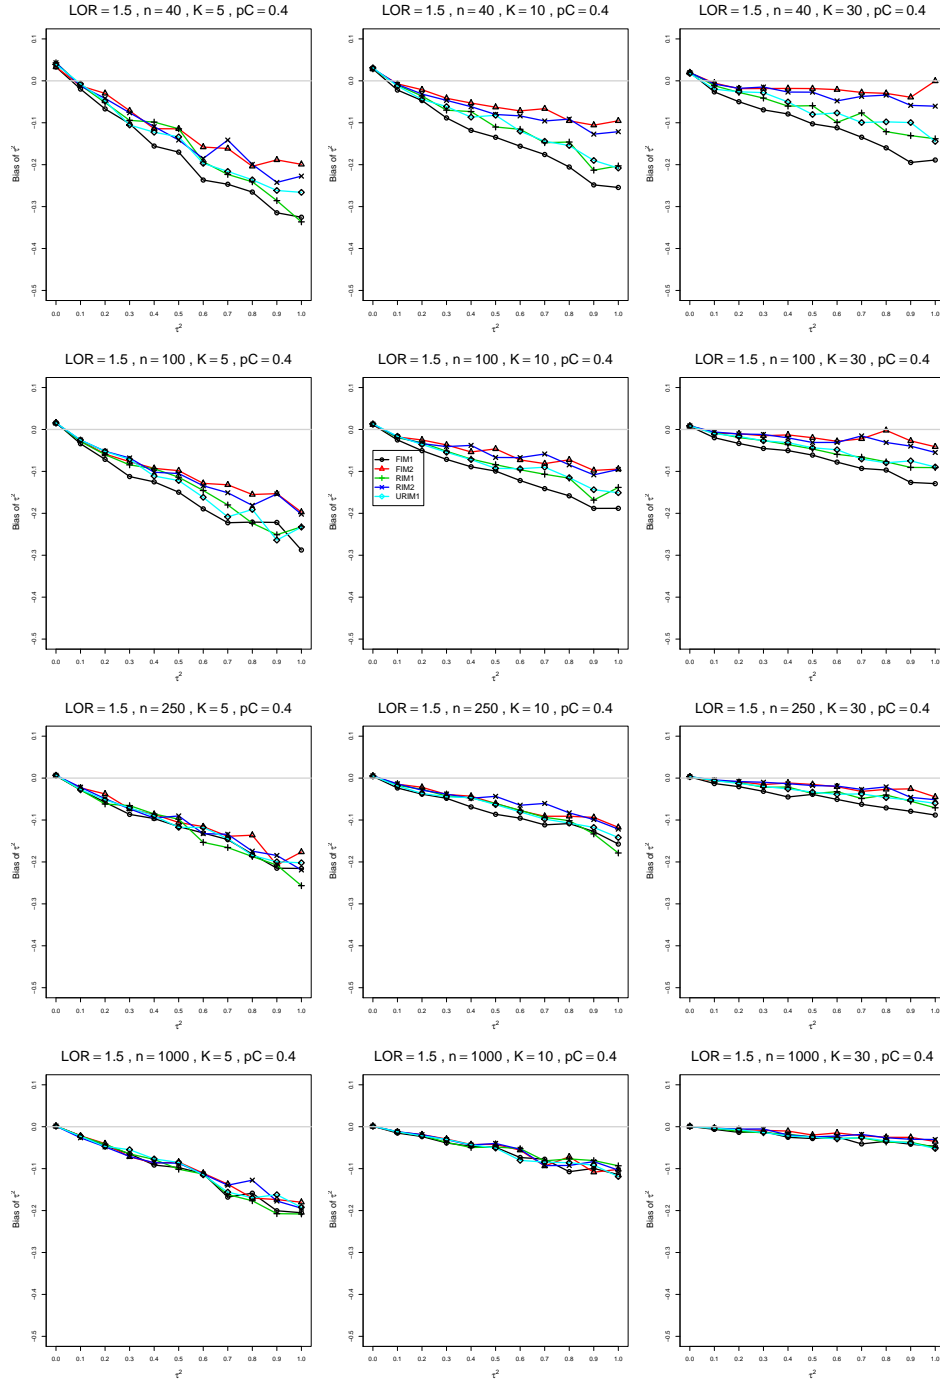

Figure A1.6.18: Bias of between-studies variance  $\hat{\tau}_{RIM2}^2$  for  $\theta = 1.5$ ,  $p_C = 0.4$ ,  $\sigma^2 = 0.4$ , constant sample sizes  $n = 40, 100, 250, 1000$ . The data-generation mechanisms are FIM1 ( $\circ$ ), FIM2 ( $\triangle$ ), RIM1 ( $+$ ), RIM2 ( $\times$ ), and URIM1 ( $\diamond$ ).

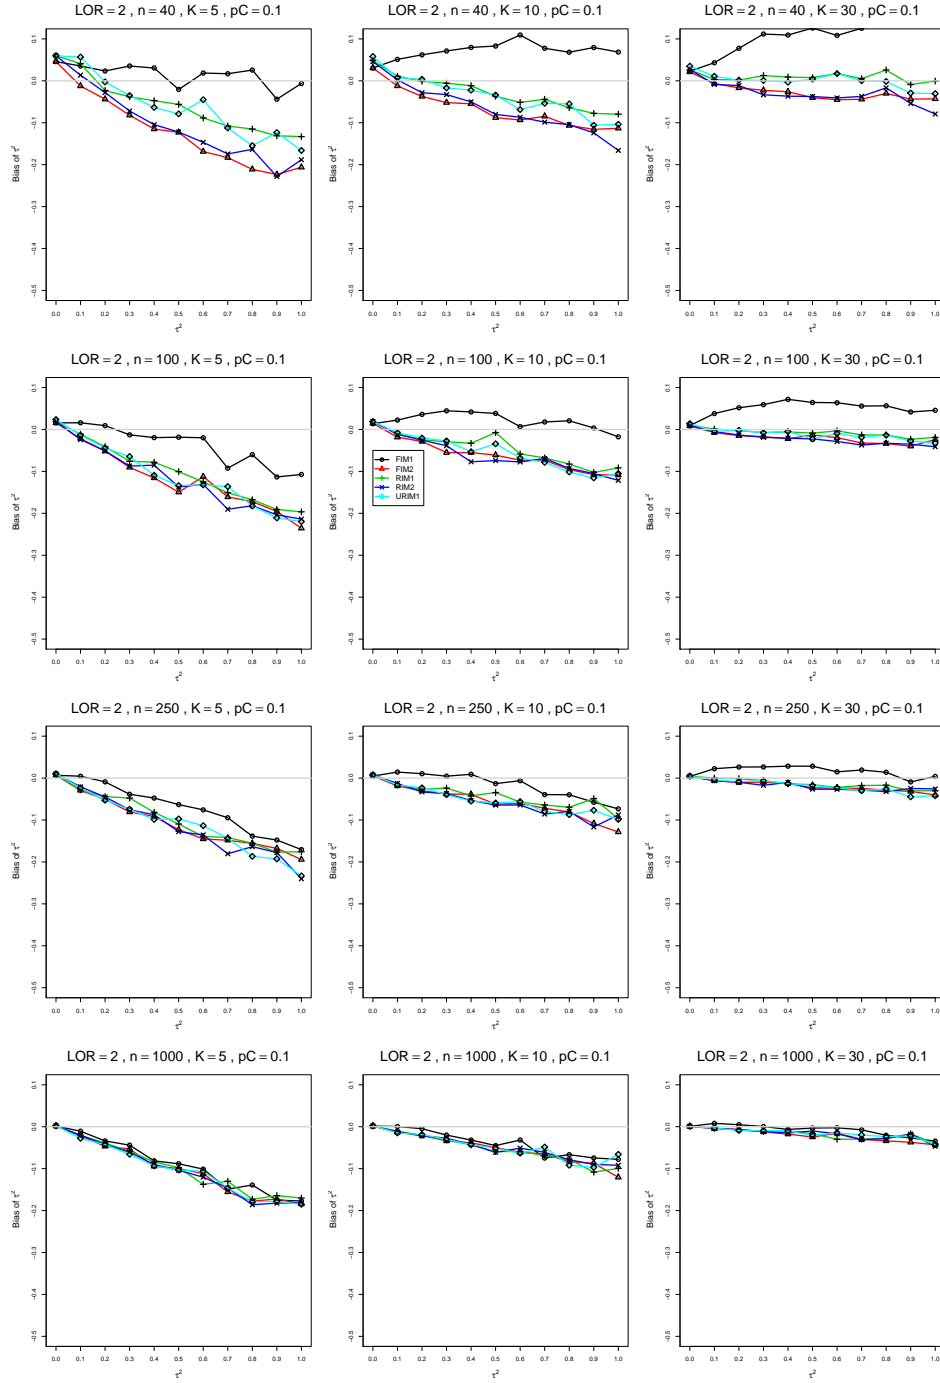

Figure A1.6.19: Bias of between-studies variance  $\hat{\tau}_{RIM2}^2$  for  $\theta = 2$ ,  $p_C = 0.1$ ,  $\sigma^2 = 0.4$ , constant sample sizes  $n = 40, 100, 250, 1000$ . The data-generation mechanisms are FIM1 ( $\circ$ ), FIM2 ( $\triangle$ ), RIM1 ( $+$ ), RIM2 ( $\times$ ), and URIM1 ( $\diamond$ ).

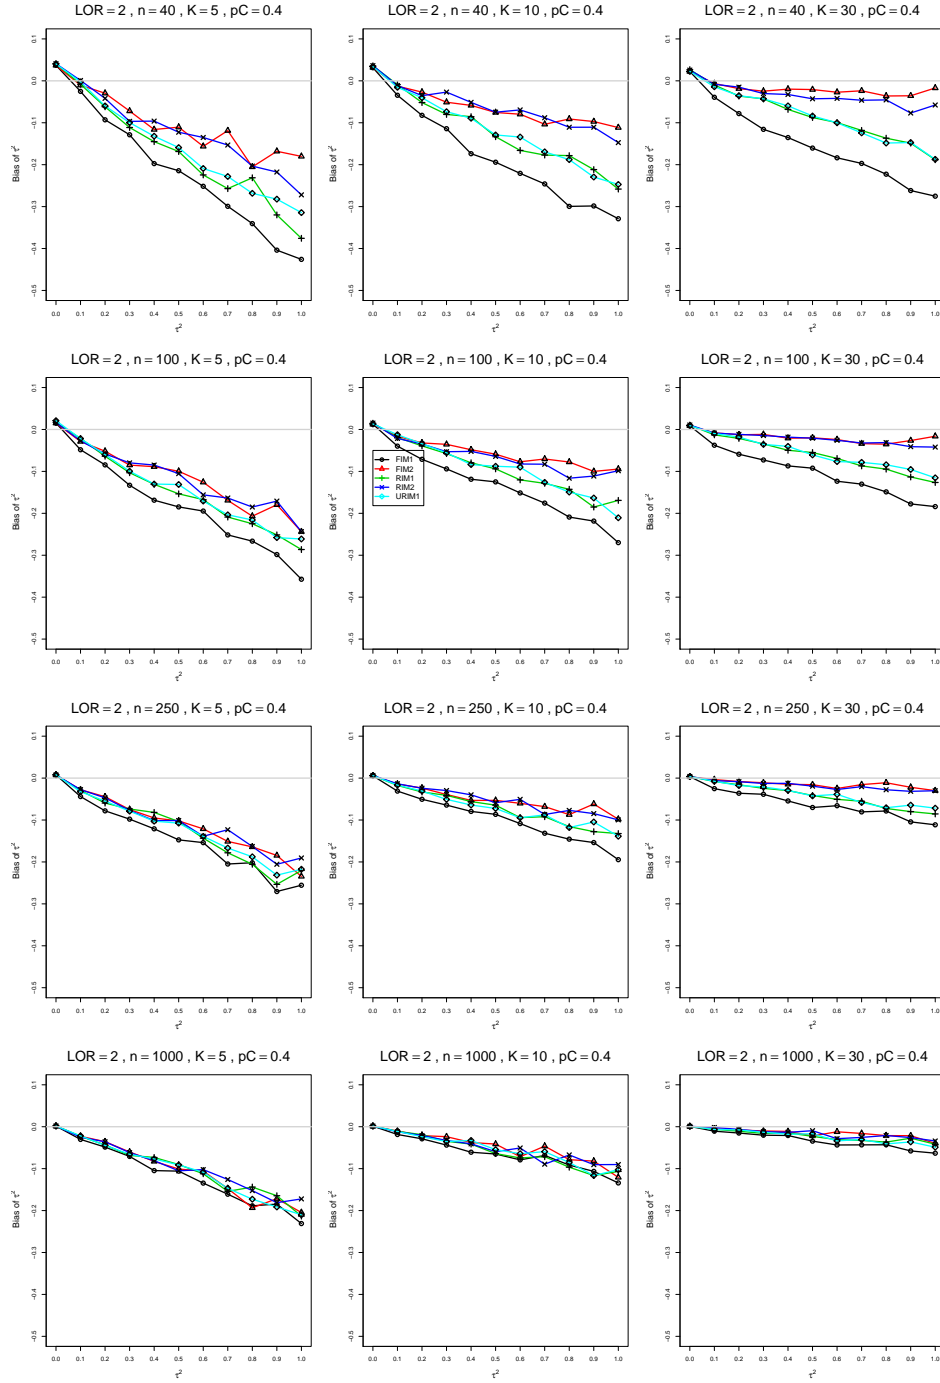

Figure A1.6.20: Bias of between-studies variance  $\hat{\tau}_{RIM2}^2$  for  $\theta = 2$ ,  $p_C = 0.4$ ,  $\sigma^2 = 0.4$ , constant sample sizes  $n = 40, 100, 250, 1000$ . The data-generation mechanisms are FIM1 ( $\circ$ ), FIM2 ( $\triangle$ ), RIM1 ( $+$ ), RIM2 ( $\times$ ), and URIM1 ( $\diamond$ ).

## A2: Plots of bias of estimators of $\theta$ for log-odds-ratio

Each panel of a figure corresponds to a value of  $n$  ( $= 40, 100, 250, 1000$ ) and a value of  $K$  ( $= 5, 10, 30$ ) and has  $\tau^2 = 0.0(0.1)1.0$  on the horizontal axis.

The data-generation mechanisms are

- FIM1 - Fixed-intercept model with  $c = 0$
- FIM2 - Fixed-intercept model with  $c = 1/2$
- RIM1 - Random-intercept model with  $c = 0$
- RIM2 - Random-intercept model with  $c = 1/2$
- URIM1 - Random-intercept model with  $c = 0$  and  $p_{iC}$  is uniformly distributed on  $[p_{iC} - \sigma\sqrt{3}p_{iC}(1 - p_{iC}), p_{iC} + \sigma\sqrt{3}p_{iC}(1 - p_{iC})]$

The point estimators of  $\theta$  are

- $\hat{\theta}_{DL}$  - DerSimonian-Laird
- $\hat{\theta}_{REML}$  - Restricted maximum-likelihood
- $\hat{\theta}_{MP}$  - Mandel-Paule
- $\hat{\theta}_{KD}$  - Kulinskaya-Dollinger
- $\hat{\theta}_{FIM2}$  - Estimator of  $\theta$  in the FIM2 GLMM
- $\hat{\theta}_{RIM2}$  - Estimator of  $\theta$  in the RIM2 GLMM
- $\hat{\theta}_{SSW}$  - sample-size-weighted estimator of  $\theta$

### A2.1 Bias of $\hat{\theta}_{DL}$

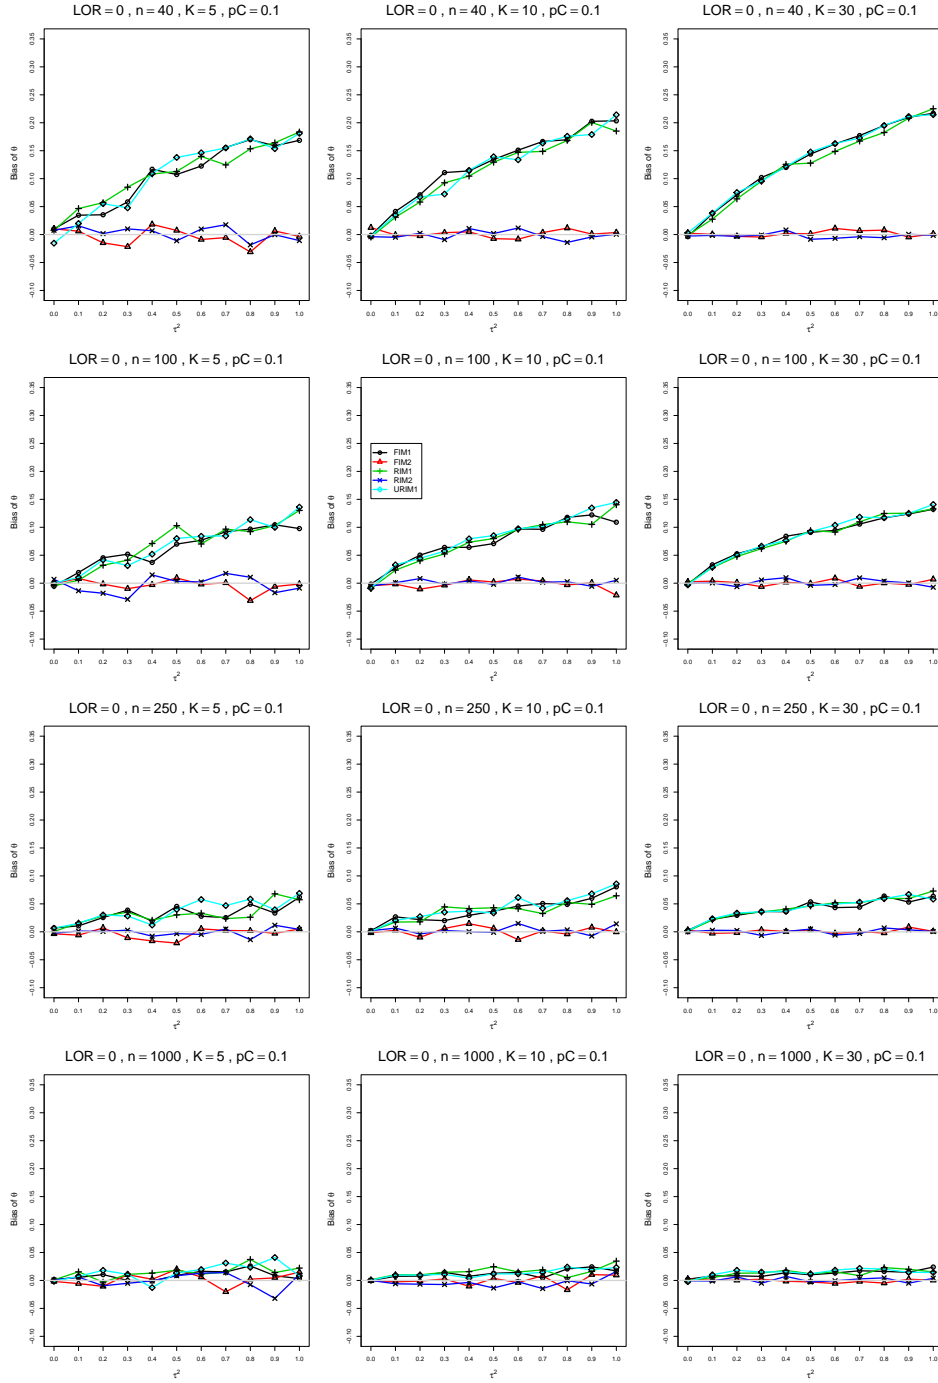

Figure A2.1.1: Bias of overall log-odds ratio  $\hat{\theta}_{DL}$  for  $\theta = 0$ ,  $p_C = 0.1$ ,  $\sigma^2 = 0.1$ , constant sample sizes  $n = 40, 100, 250, 1000$ . The data-generation mechanisms are FIM1 ( $\circ$ ), FIM2 ( $\triangle$ ), RIM1 ( $+$ ), RIM2 ( $\times$ ), and URIM1 ( $\diamond$ ).

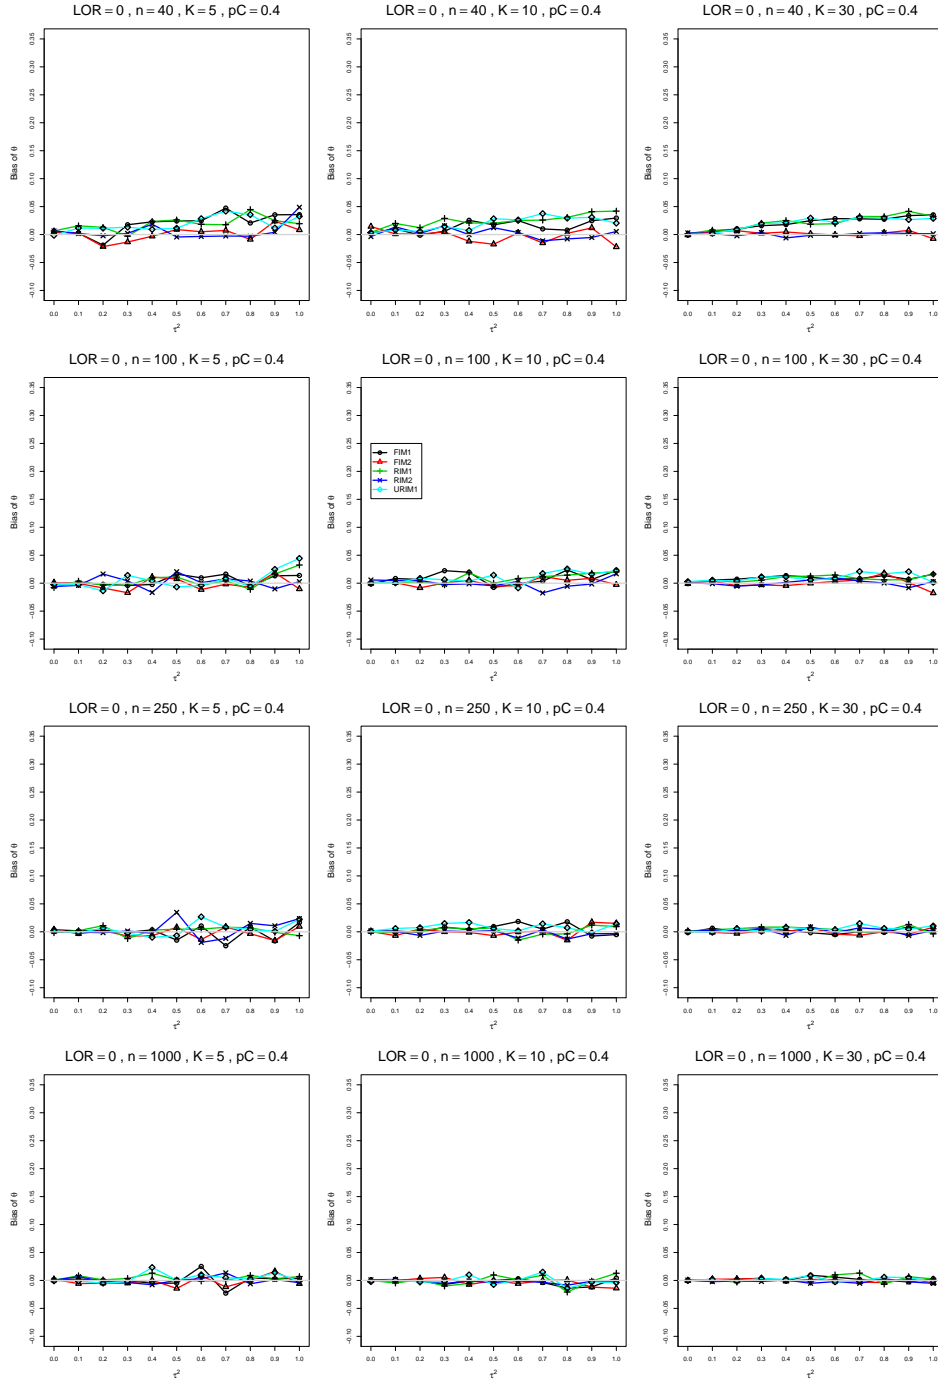

Figure A2.1.2: Bias of overall log-odds ratio  $\hat{\theta}_{DL}$  for  $\theta = 0$ ,  $p_C = 0.4$ ,  $\sigma^2 = 0.1$ , constant sample sizes  $n = 40, 100, 250, 1000$ . The data-generation mechanisms are FIM1 ( $\circ$ ), FIM2 ( $\triangle$ ), RIM1 ( $+$ ), RIM2 ( $\times$ ), and URIM1 ( $\diamond$ ).



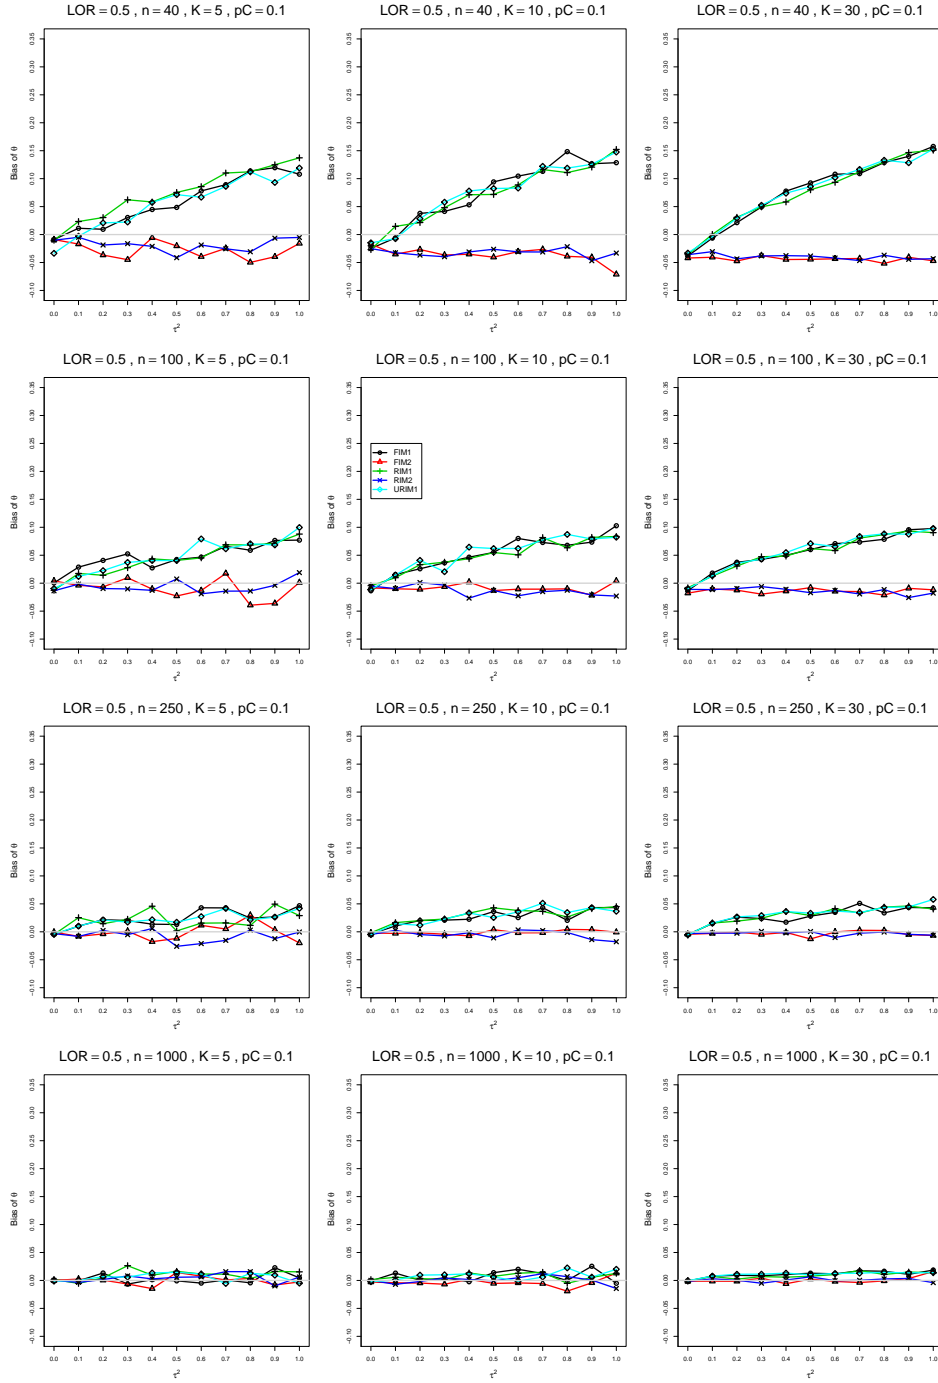

Figure A2.1.3: Bias of overall log-odds ratio  $\hat{\theta}_{DL}$  for  $\theta = 0.5$ ,  $p_C = 0.1$ ,  $\sigma^2 = 0.1$ , constant sample sizes  $n = 40, 100, 250, 1000$ . The data-generation mechanisms are FIM1 ( $\circ$ ), FIM2 ( $\triangle$ ), RIM1 ( $+$ ), RIM2 ( $\times$ ), and URIM1 ( $\diamond$ ).

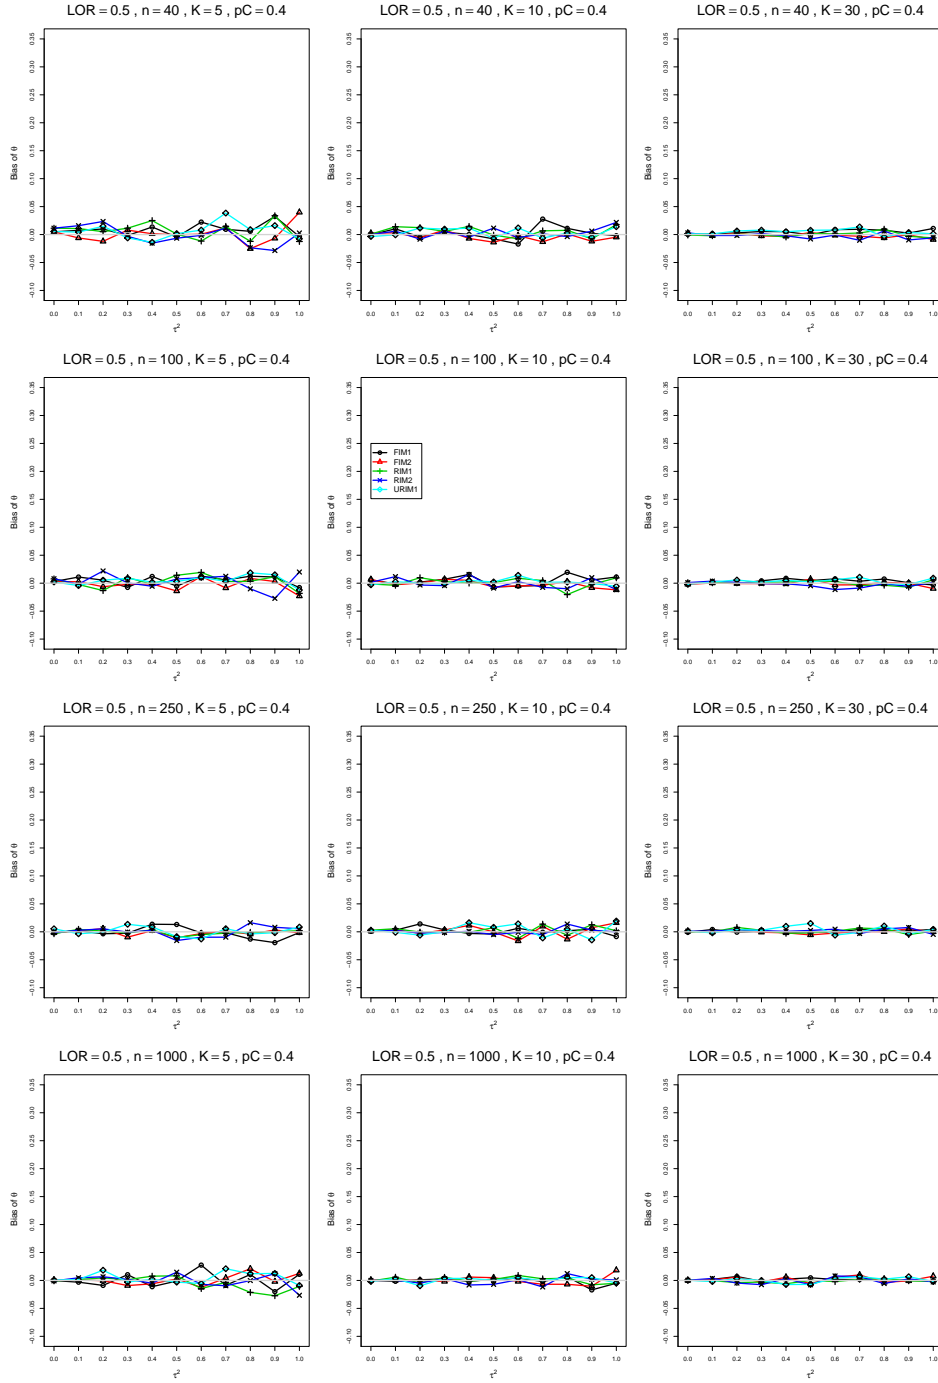

Figure A2.1.4: Bias of overall log-odds ratio  $\hat{\theta}_{DL}$  for  $\theta = 0.5$ ,  $p_C = 0.4$ ,  $\sigma^2 = 0.1$ , constant sample sizes  $n = 40, 100, 250, 1000$ . The data-generation mechanisms are FIM1 ( $\circ$ ), FIM2 ( $\triangle$ ), RIM1 ( $+$ ), RIM2 ( $\times$ ), and URIM1 ( $\diamond$ ).

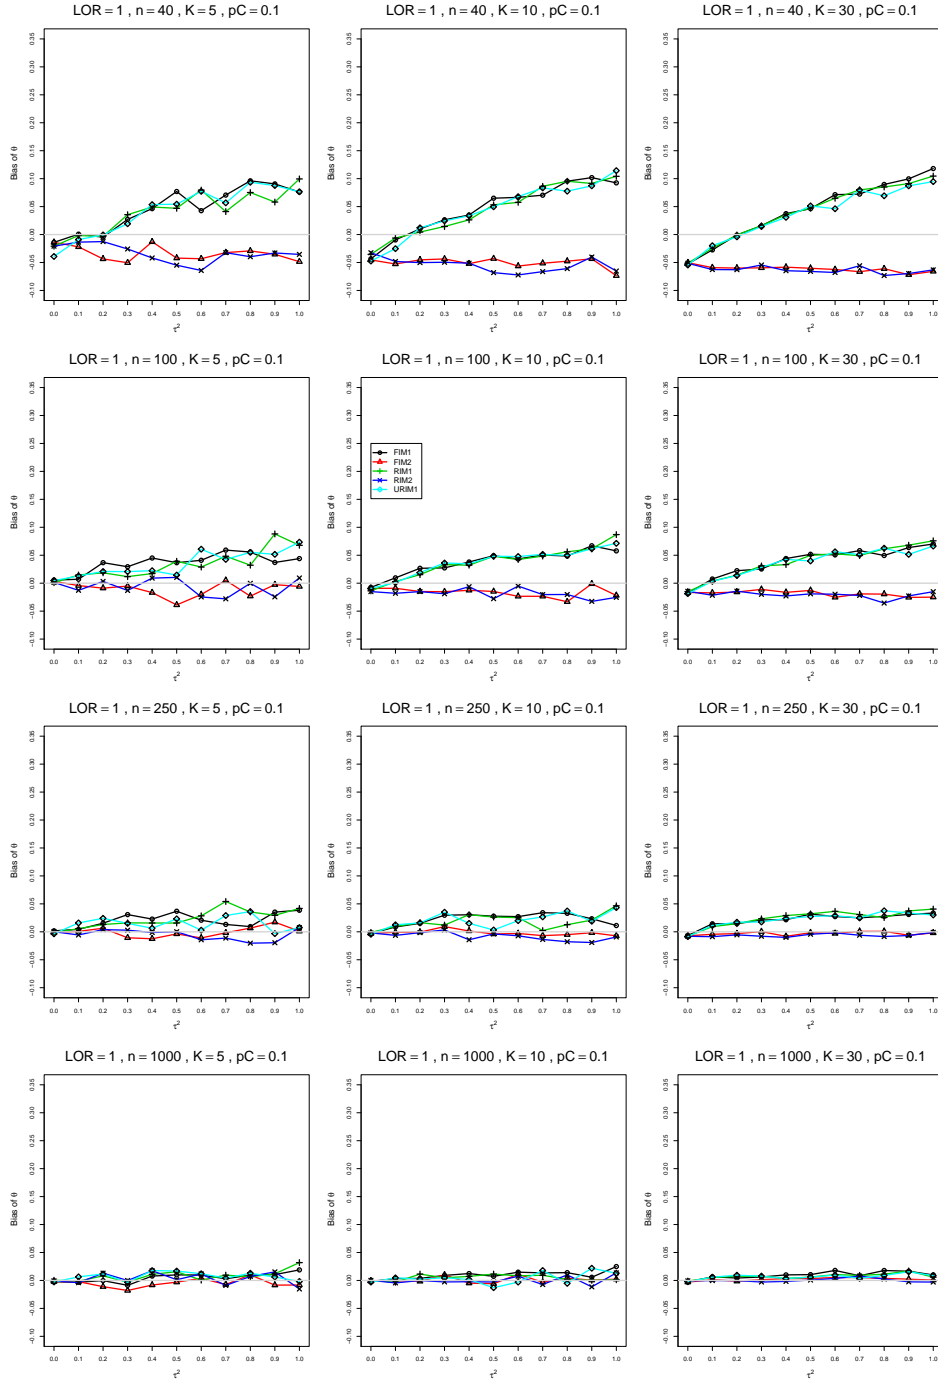

Figure A2.1.5: Bias of overall log-odds ratio  $\hat{\theta}_{DL}$  for  $\theta = 1$ ,  $p_C = 0.1$ ,  $\sigma^2 = 0.1$ , constant sample sizes  $n = 40, 100, 250, 1000$ . The data-generation mechanisms are FIM1 ( $\circ$ ), FIM2 ( $\triangle$ ), RIM1 ( $+$ ), RIM2 ( $\times$ ), and URIM1 ( $\diamond$ ).

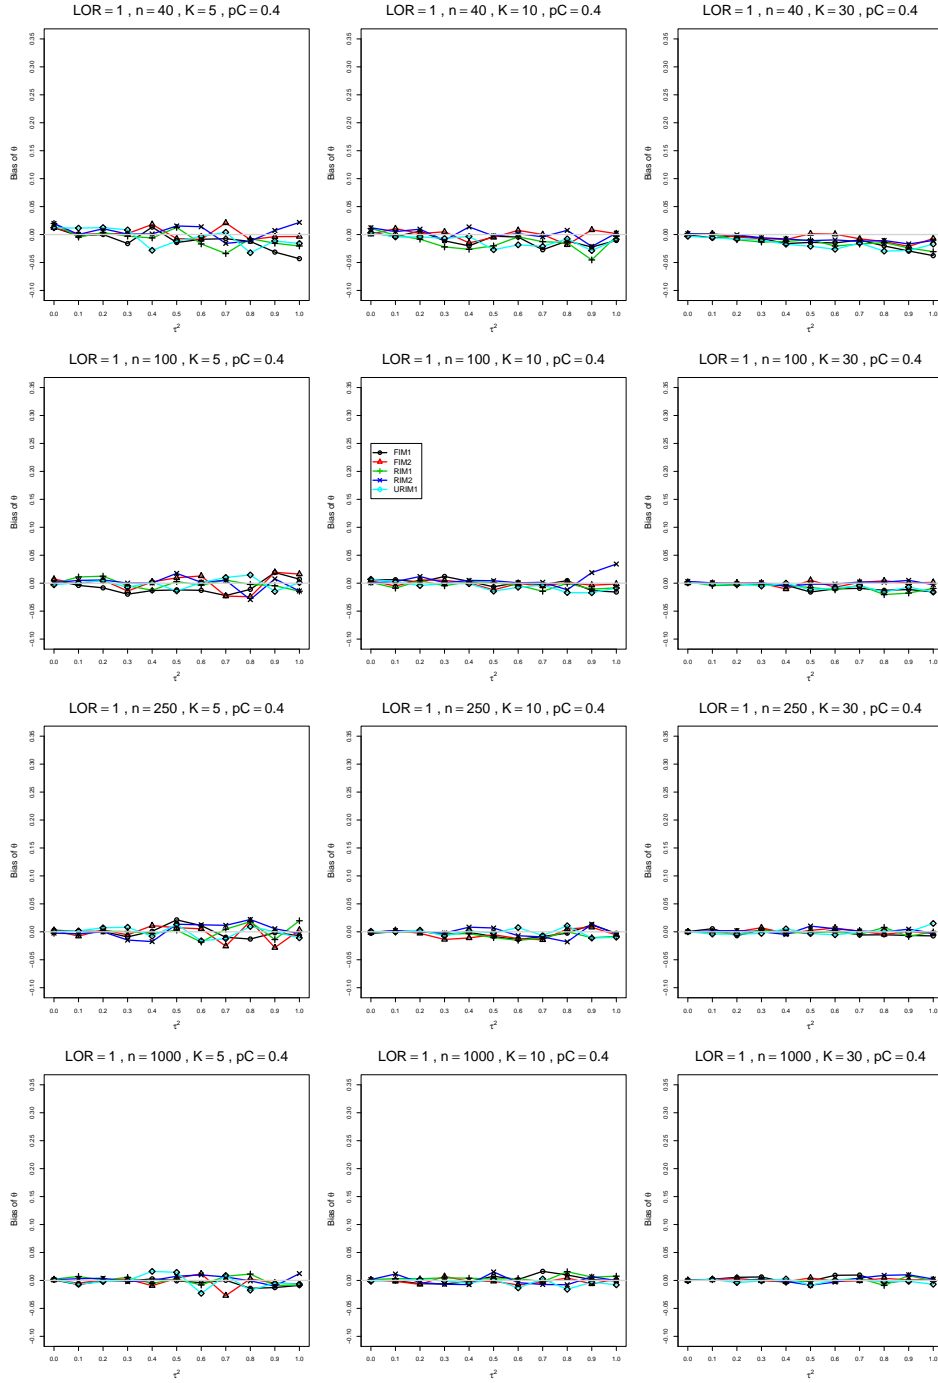

Figure A2.1.6: Bias of overall log-odds ratio  $\hat{\theta}_{DL}$  for  $\theta = 1$ ,  $p_C = 0.4$ ,  $\sigma^2 = 0.1$ , constant sample sizes  $n = 40, 100, 250, 1000$ . The data-generation mechanisms are FIM1 ( $\circ$ ), FIM2 ( $\triangle$ ), RIM1 ( $+$ ), RIM2 ( $\times$ ), and URIM1 ( $\diamond$ ).

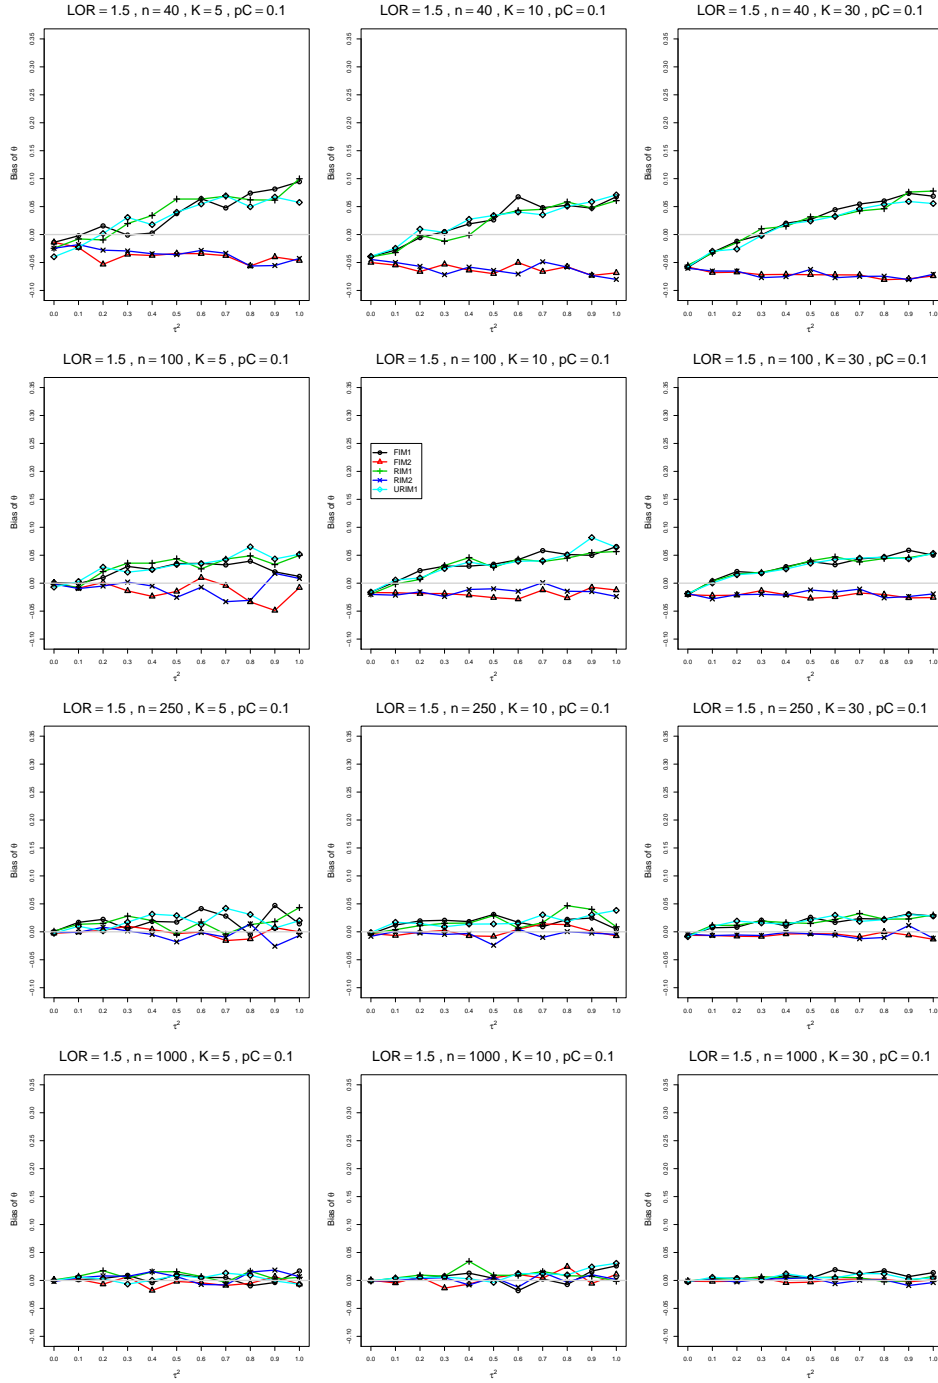

Figure A2.1.7: Bias of overall log-odds ratio  $\hat{\theta}_{DL}$  for  $\theta = 1.5$ ,  $p_C = 0.1$ ,  $\sigma^2 = 0.1$ , constant sample sizes  $n = 40, 100, 250, 1000$ . The data-generation mechanisms are FIM1 ( $\circ$ ), FIM2 ( $\triangle$ ), RIM1 ( $+$ ), RIM2 ( $\times$ ), and URIM1 ( $\diamond$ ).

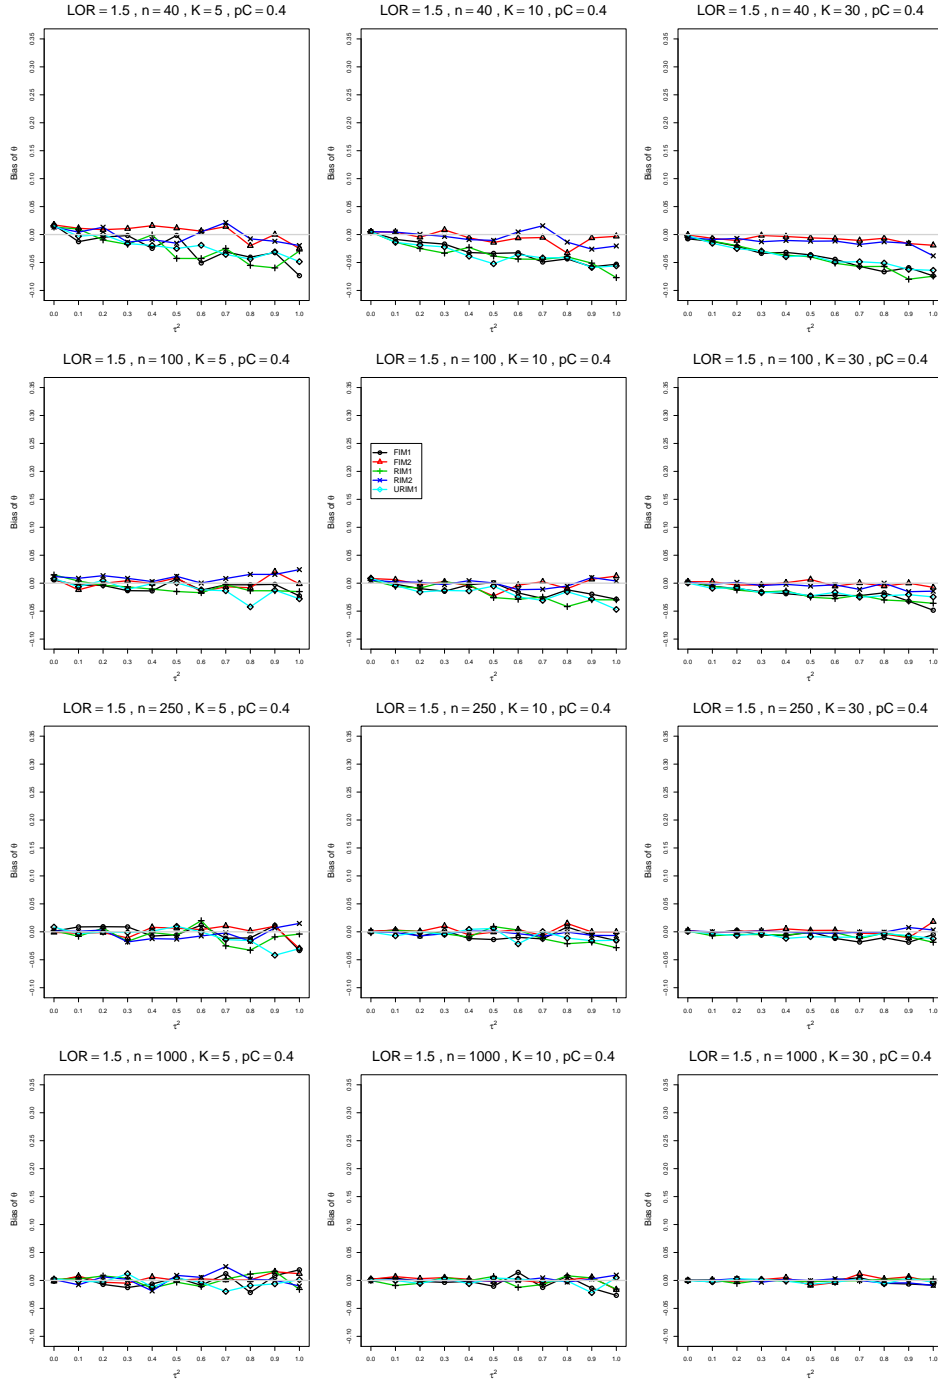

Figure A2.1.8: Bias of overall log-odds ratio  $\hat{\theta}_{DL}$  for  $\theta = 1.5$ ,  $p_C = 0.4$ ,  $\sigma^2 = 0.1$ , constant sample sizes  $n = 40, 100, 250, 1000$ . The data-generation mechanisms are FIM1 ( $\circ$ ), FIM2 ( $\triangle$ ), RIM1 ( $+$ ), RIM2 ( $\times$ ), and URIM1 ( $\diamond$ ).

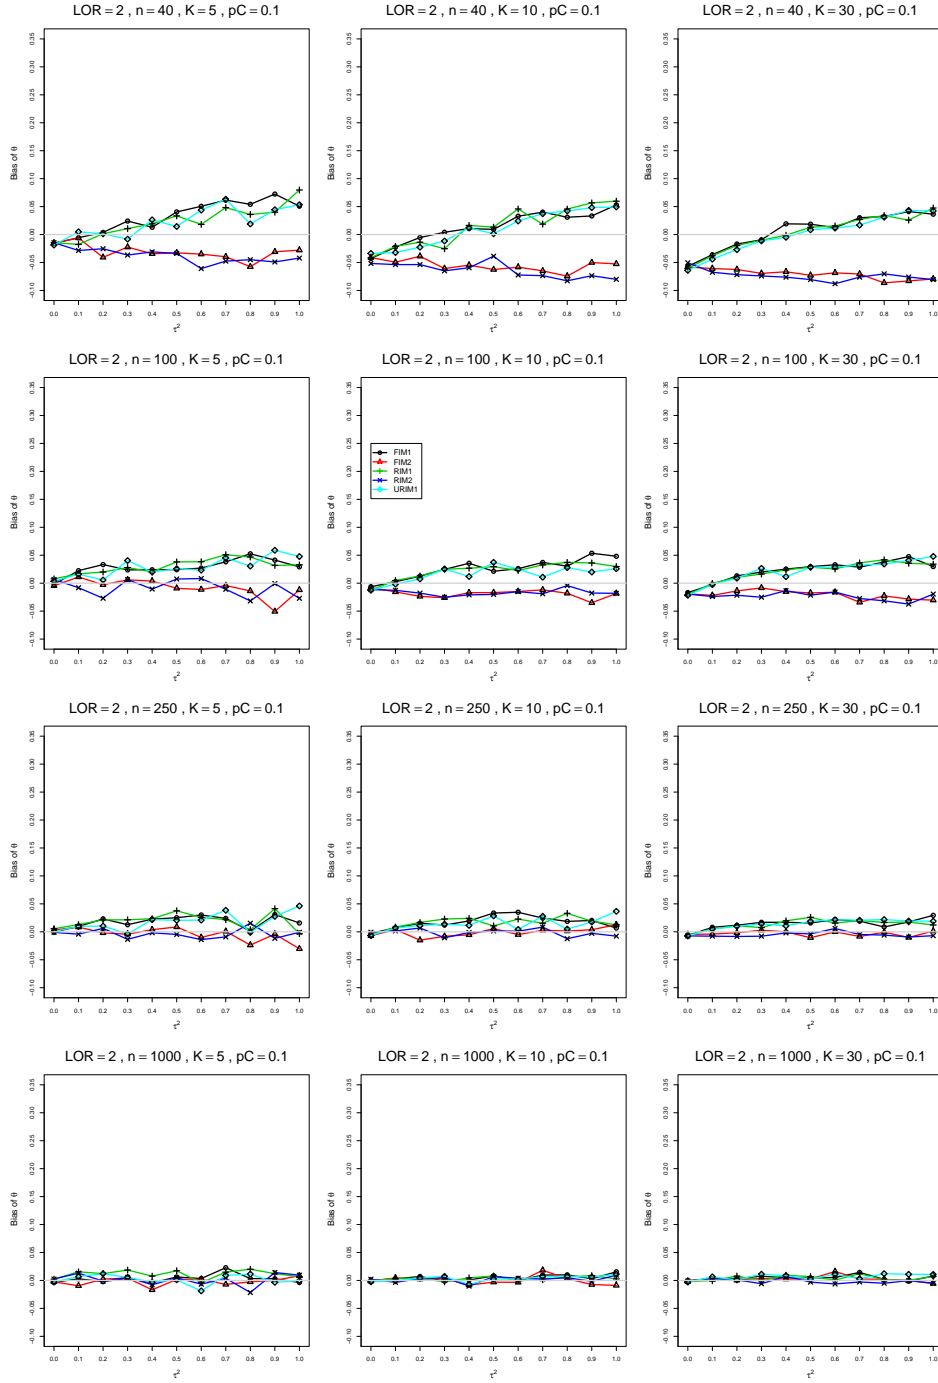

Figure A2.1.9: Bias of overall log-odds ratio  $\hat{\theta}_{DL}$  for  $\theta = 2$ ,  $p_C = 0.1$ ,  $\sigma^2 = 0.1$ , constant sample sizes  $n = 40, 100, 250, 1000$ . The data-generation mechanisms are FIM1 ( $\circ$ ), FIM2 ( $\triangle$ ), RIM1 ( $+$ ), RIM2 ( $\times$ ), and URIM1 ( $\diamond$ ).

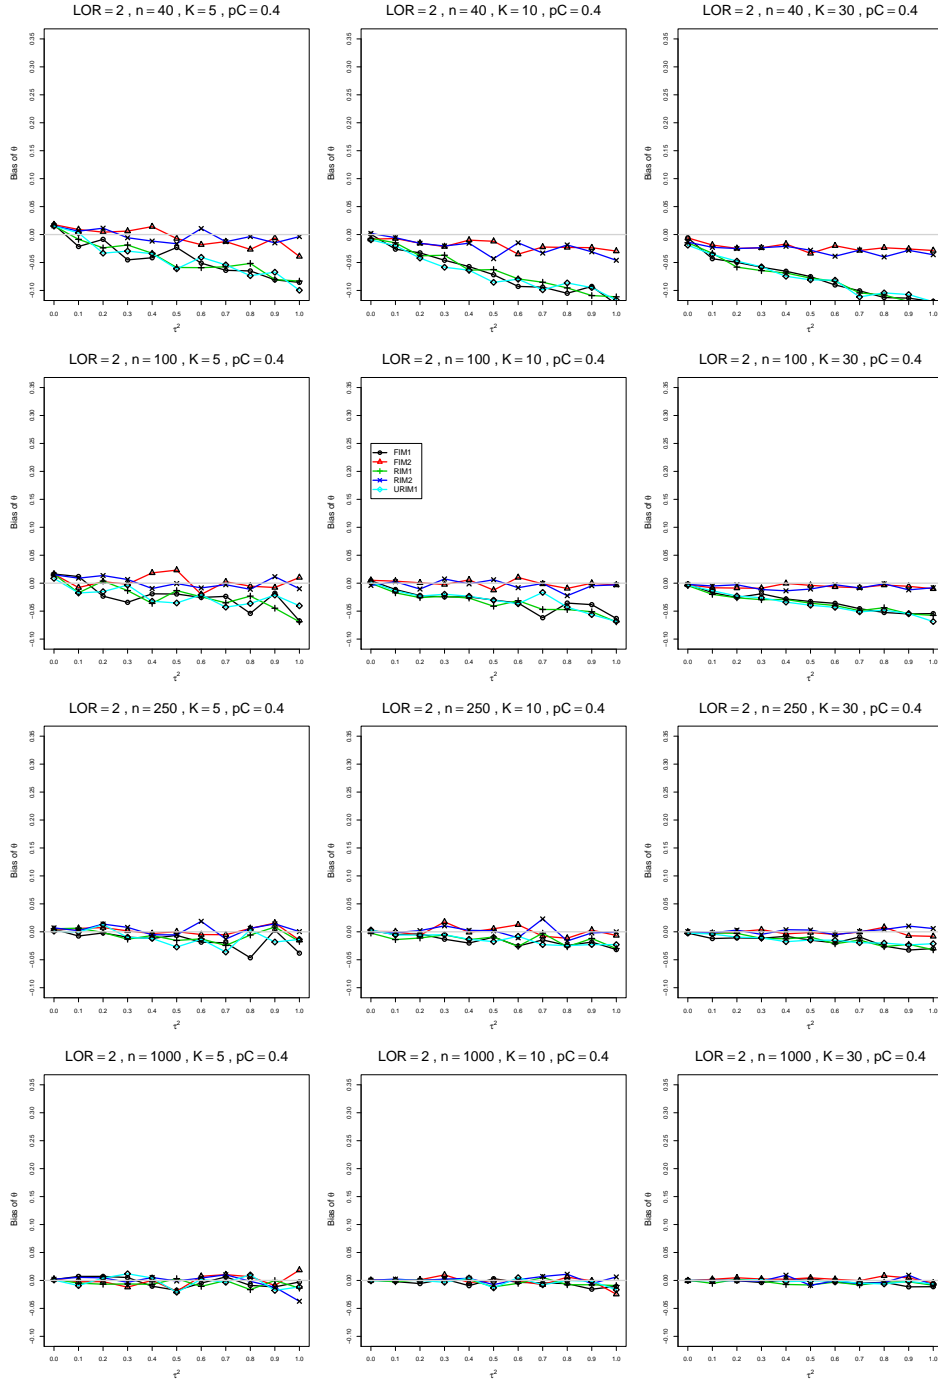

Figure A2.1.10: Bias of overall log-odds ratio  $\hat{\theta}_{DL}$  for  $\theta = 2$ ,  $p_C = 0.4$ ,  $\sigma^2 = 0.1$ , constant sample sizes  $n = 40, 100, 250, 1000$ . The data-generation mechanisms are FIM1 ( $\circ$ ), FIM2 ( $\triangle$ ), RIM1 ( $+$ ), RIM2 ( $\times$ ), and URIM1 ( $\diamond$ ).



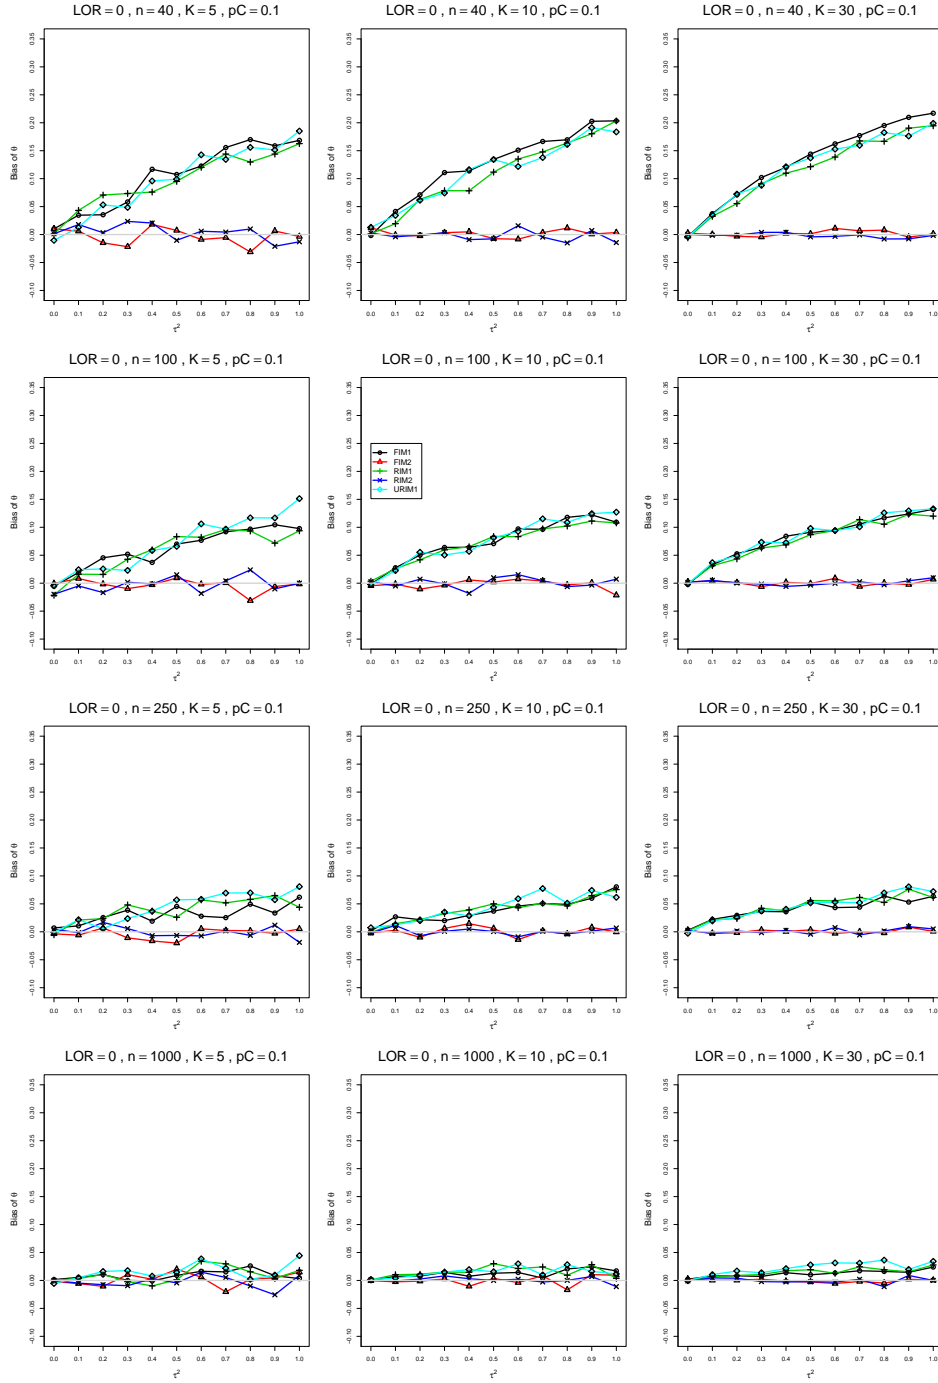

Figure A2.1.11: Bias of overall log-odds ratio  $\hat{\theta}_{DL}$  for  $\theta = 0$ ,  $p_C = 0.1$ ,  $\sigma^2 = 0.4$ , constant sample sizes  $n = 40, 100, 250, 1000$ . The data-generation mechanisms are FIM1 ( $\circ$ ), FIM2 ( $\triangle$ ), RIM1 ( $+$ ), RIM2 ( $\times$ ), and URIM1 ( $\diamond$ ).

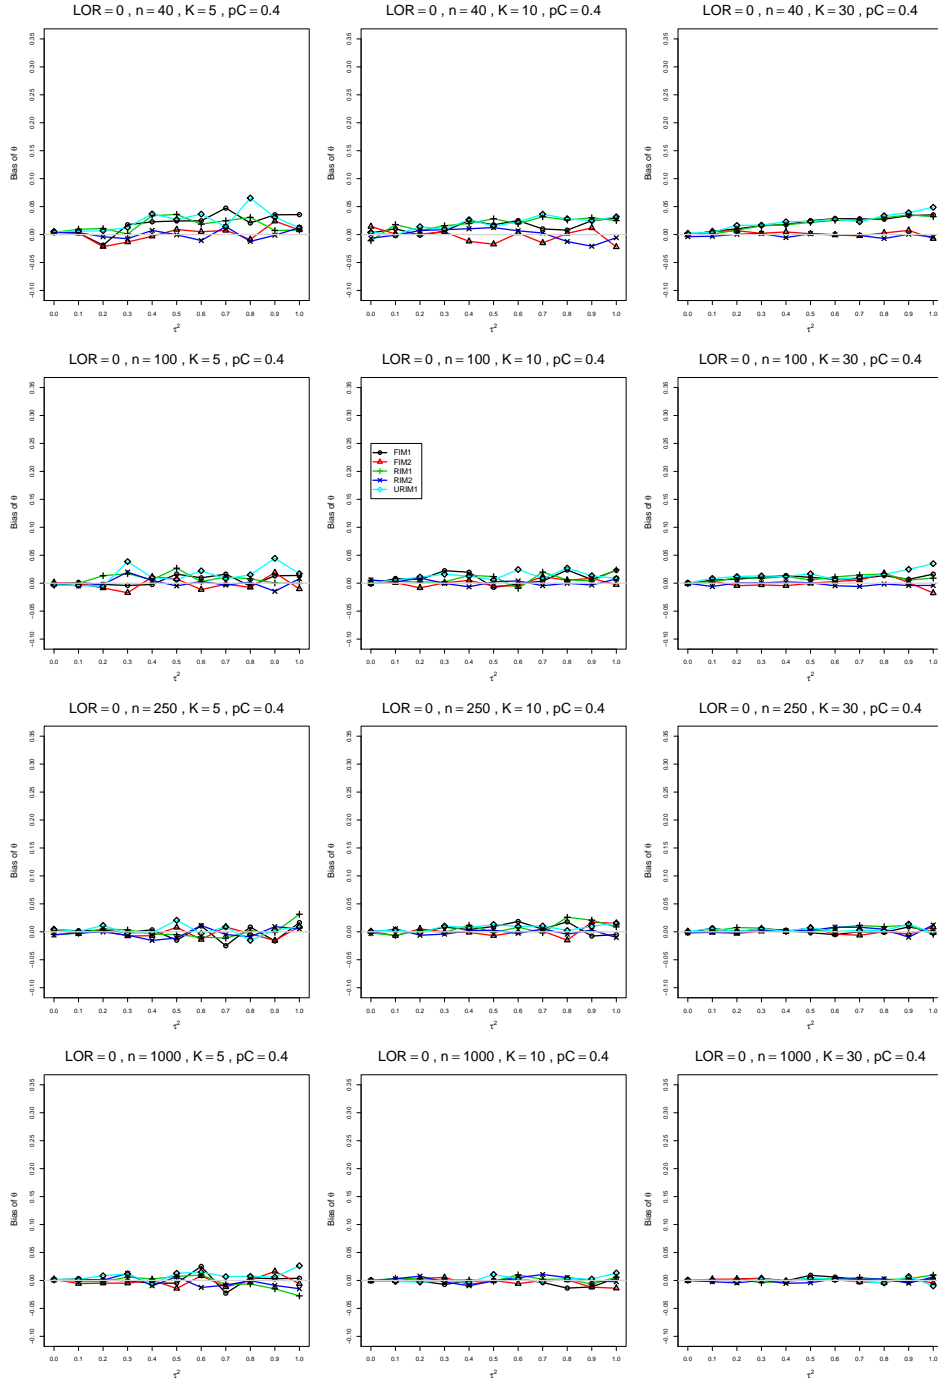

Figure A2.1.12: Bias of overall log-odds ratio  $\hat{\theta}_{DL}$  for  $\theta = 0$ ,  $p_C = 0.4$ ,  $\sigma^2 = 0.4$ , constant sample sizes  $n = 40, 100, 250, 1000$ . The data-generation mechanisms are FIM1 ( $\circ$ ), FIM2 ( $\triangle$ ), RIM1 ( $+$ ), RIM2 ( $\times$ ), and URIM1 ( $\diamond$ ).

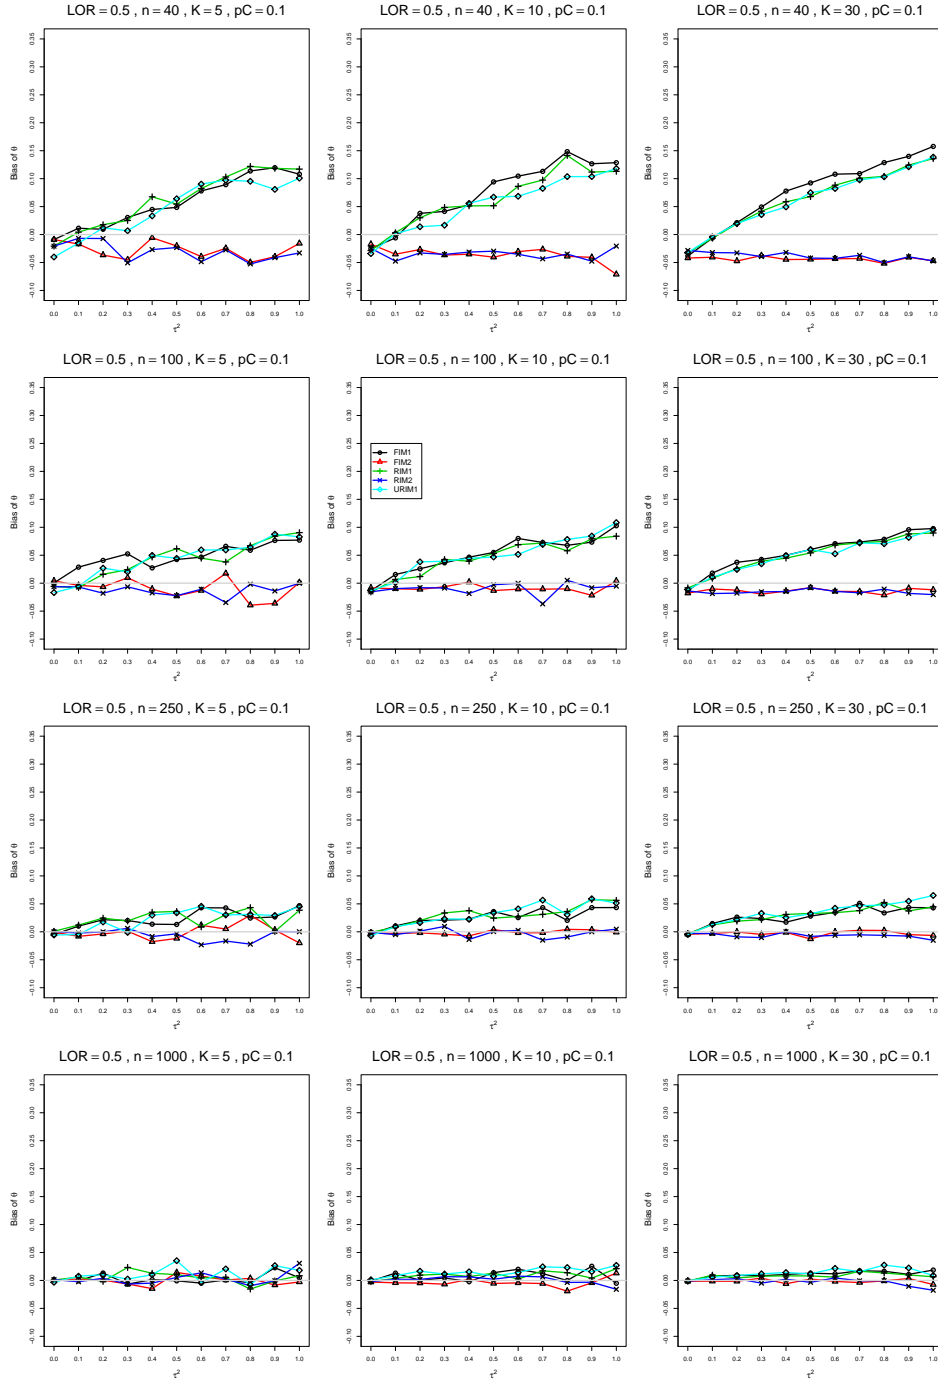

Figure A2.1.13: Bias of overall log-odds ratio  $\hat{\theta}_{DL}$  for  $\theta = 0.5$ ,  $p_C = 0.1$ ,  $\sigma^2 = 0.4$ , constant sample sizes  $n = 40, 100, 250, 1000$ . The data-generation mechanisms are FIM1 ( $\circ$ ), FIM2 ( $\triangle$ ), RIM1 ( $+$ ), RIM2 ( $\times$ ), and URIM1 ( $\diamond$ ).

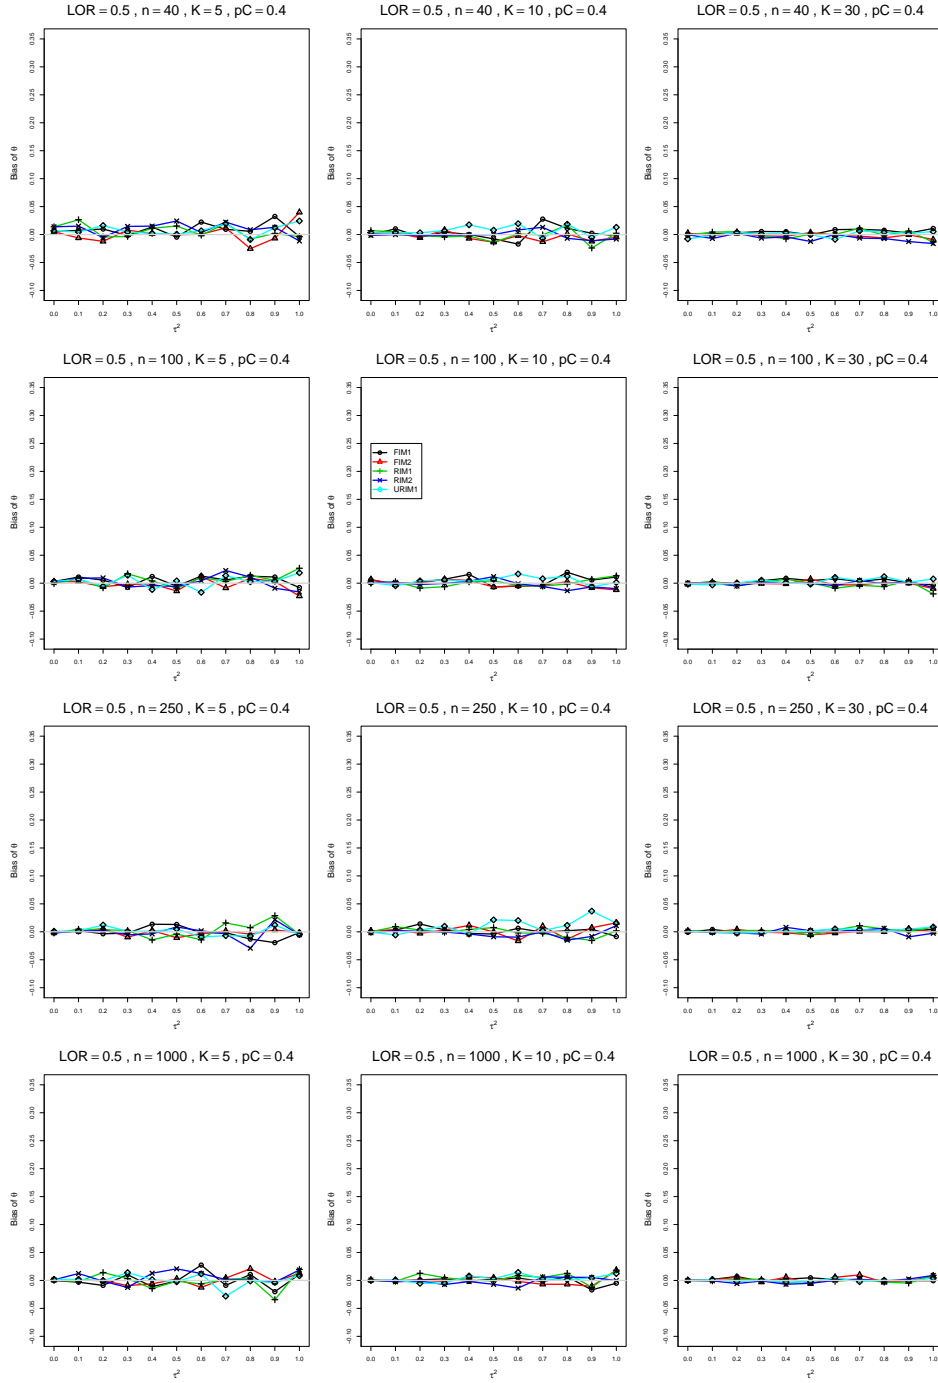

Figure A2.1.14: Bias of overall log-odds ratio  $\hat{\theta}_{DL}$  for  $\theta = 0.5$ ,  $p_C = 0.4$ ,  $\sigma^2 = 0.4$ , constant sample sizes  $n = 40, 100, 250, 1000$ . The data-generation mechanisms are FIM1 ( $\circ$ ), FIM2 ( $\triangle$ ), RIM1 ( $+$ ), RIM2 ( $\times$ ), and URIM1 ( $\diamond$ ).

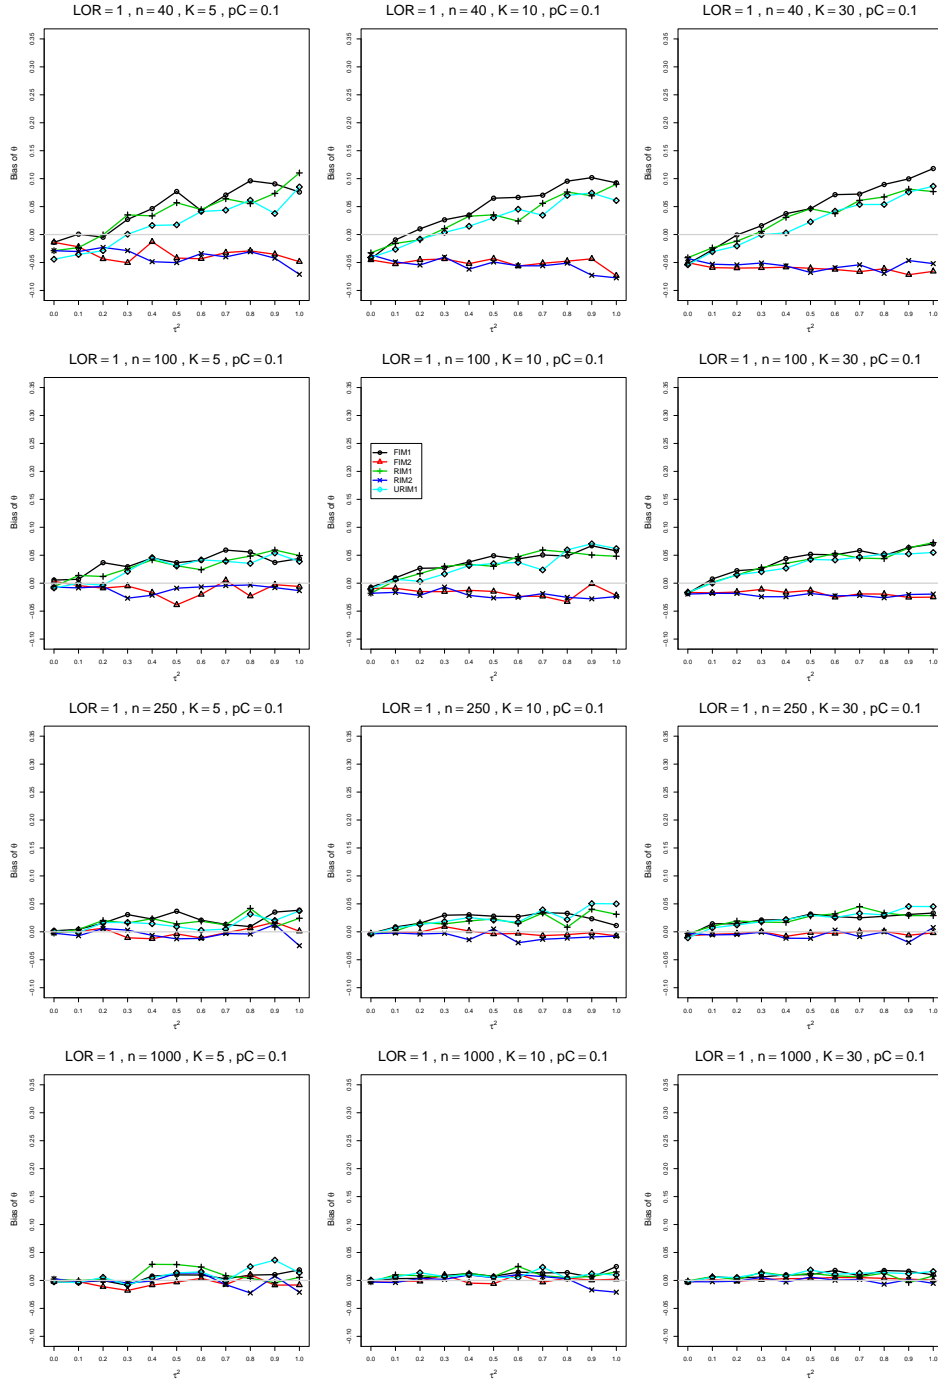

Figure A2.1.15: Bias of overall log-odds ratio  $\hat{\theta}_{DL}$  for  $\theta = 1$ ,  $p_C = 0.1$ ,  $\sigma^2 = 0.4$ , constant sample sizes  $n = 40, 100, 250, 1000$ . The data-generation mechanisms are FIM1 ( $\circ$ ), FIM2 ( $\triangle$ ), RIM1 ( $+$ ), RIM2 ( $\times$ ), and URIM1 ( $\diamond$ ).

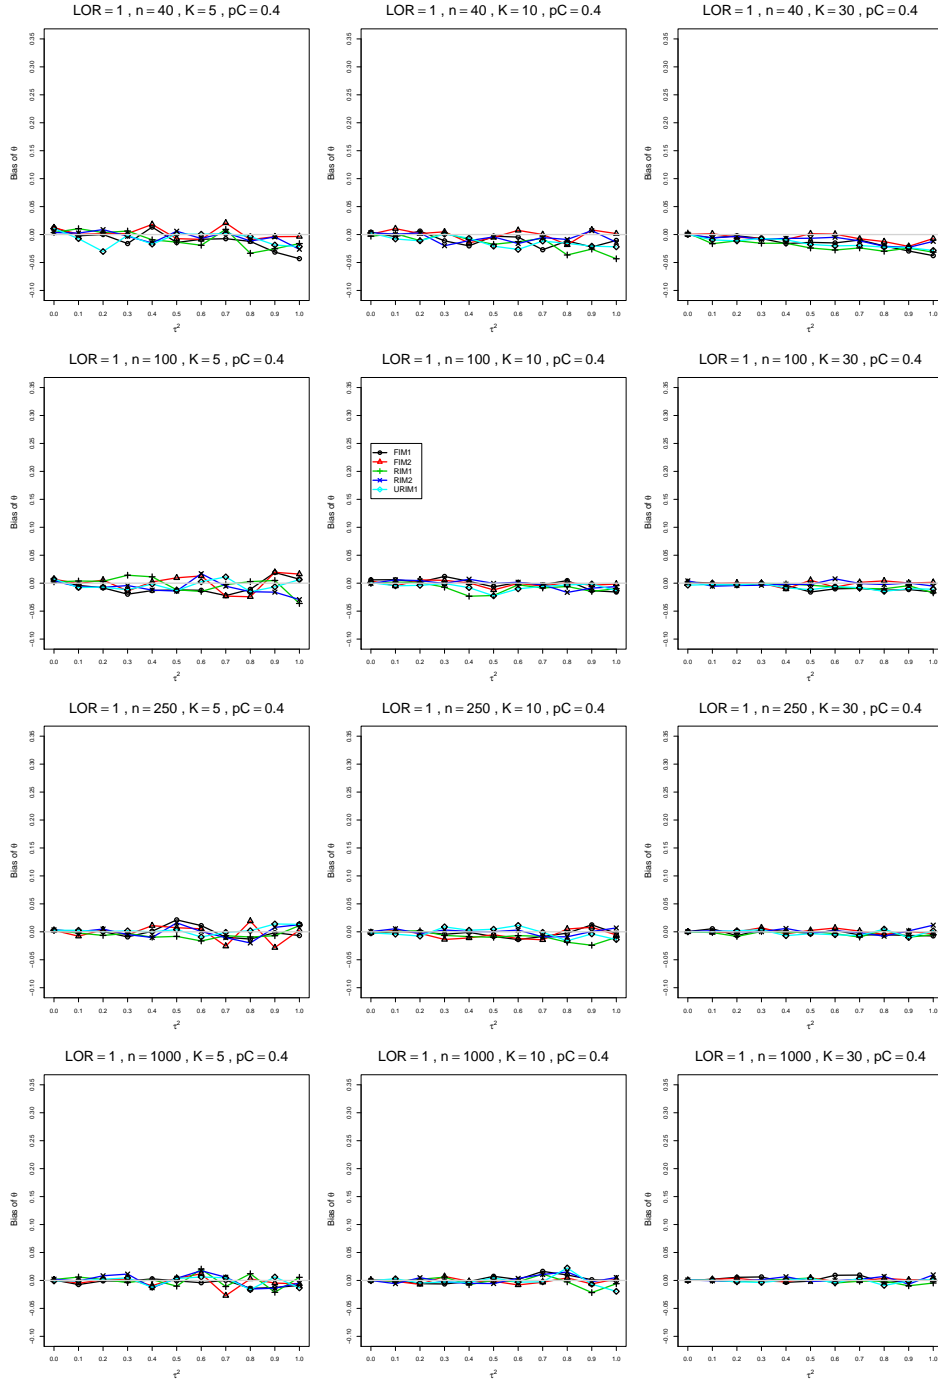

Figure A2.1.16: Bias of overall log-odds ratio  $\hat{\theta}_{DL}$  for  $\theta = 1$ ,  $p_C = 0.4$ ,  $\sigma^2 = 0.4$ , constant sample sizes  $n = 40, 100, 250, 1000$ . The data-generation mechanisms are FIM1 ( $\circ$ ), FIM2 ( $\triangle$ ), RIM1 ( $+$ ), RIM2 ( $\times$ ), and URIM1 ( $\diamond$ ).

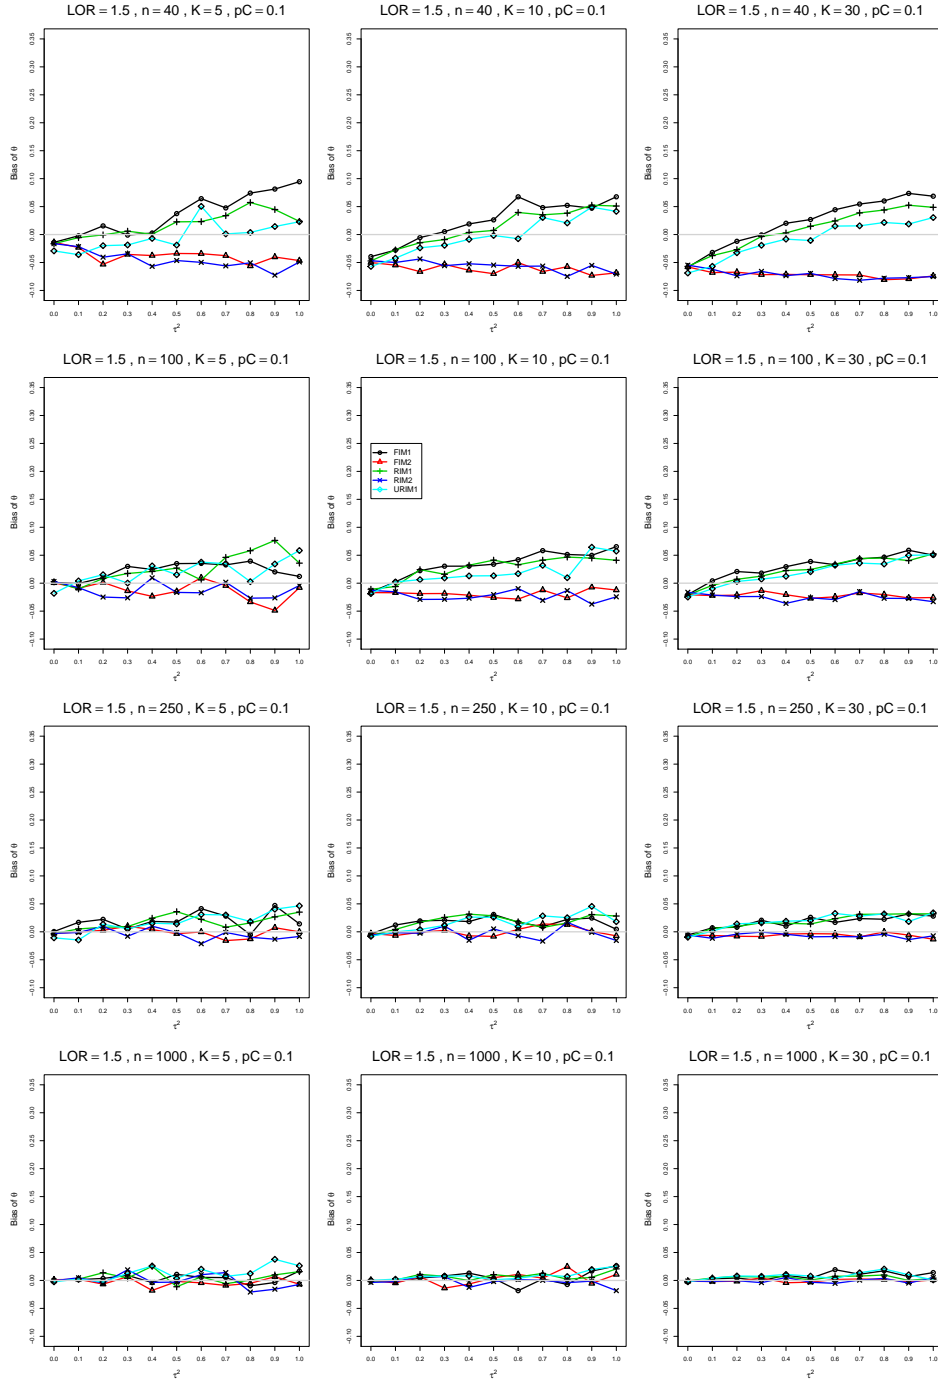

Figure A2.1.17: Bias of overall log-odds ratio  $\hat{\theta}_{DL}$  for  $\theta = 1.5$ ,  $p_C = 0.1$ ,  $\sigma^2 = 0.4$ , constant sample sizes  $n = 40, 100, 250, 1000$ . The data-generation mechanisms are FIM1 ( $\circ$ ), FIM2 ( $\triangle$ ), RIM1 ( $+$ ), RIM2 ( $\times$ ), and URIM1 ( $\diamond$ ).

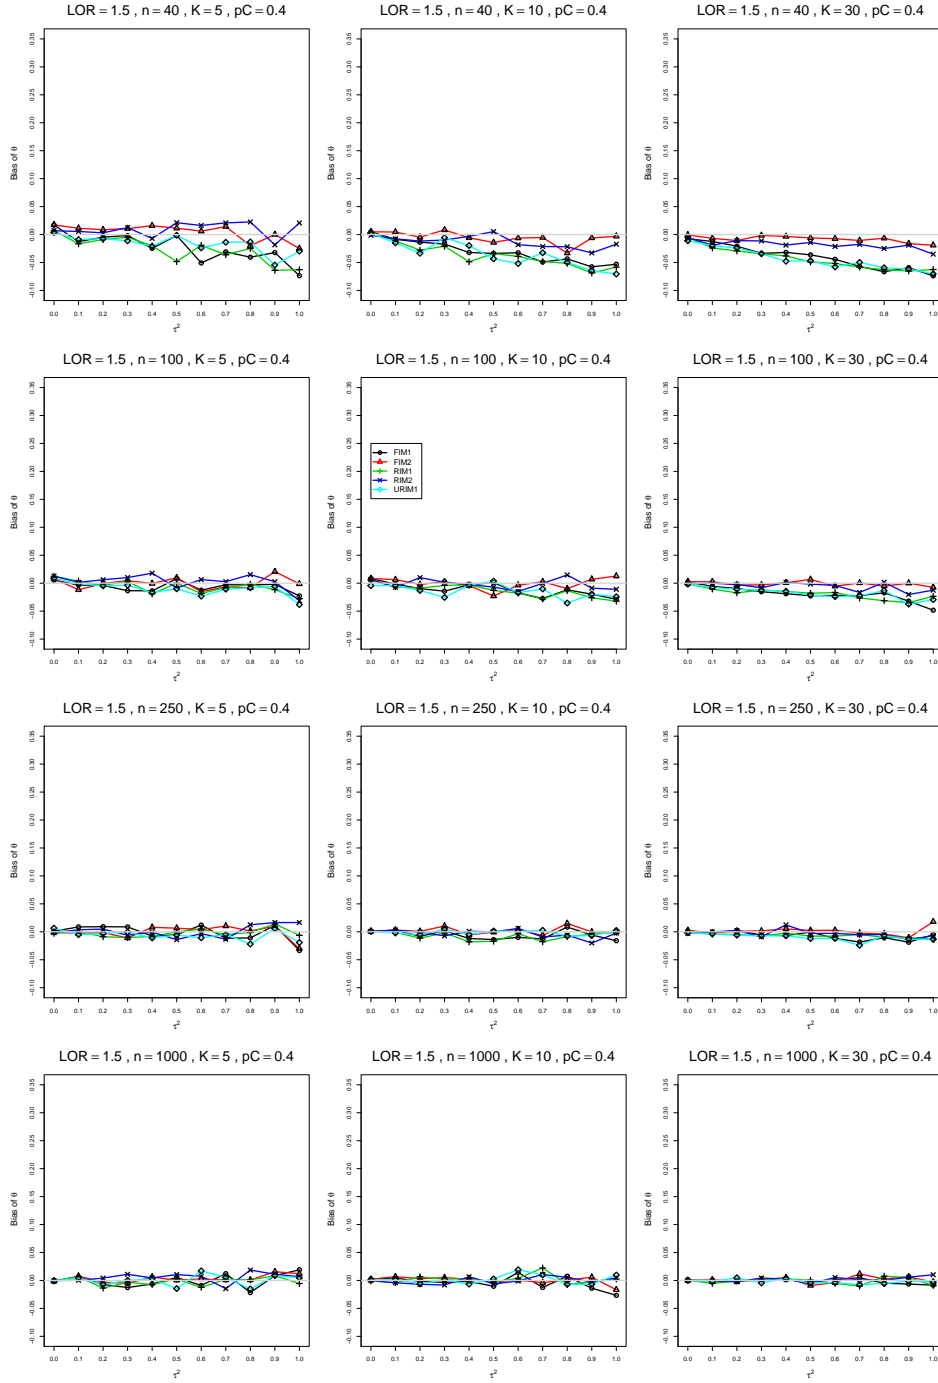

Figure A2.1.18: Bias of overall log-odds ratio  $\hat{\theta}_{DL}$  for  $\theta = 1.5$ ,  $p_C = 0.4$ ,  $\sigma^2 = 0.4$ , constant sample sizes  $n = 40, 100, 250, 1000$ . The data-generation mechanisms are FIM1 ( $\circ$ ), FIM2 ( $\triangle$ ), RIM1 ( $+$ ), RIM2 ( $\times$ ), and URIM1 ( $\diamond$ ).



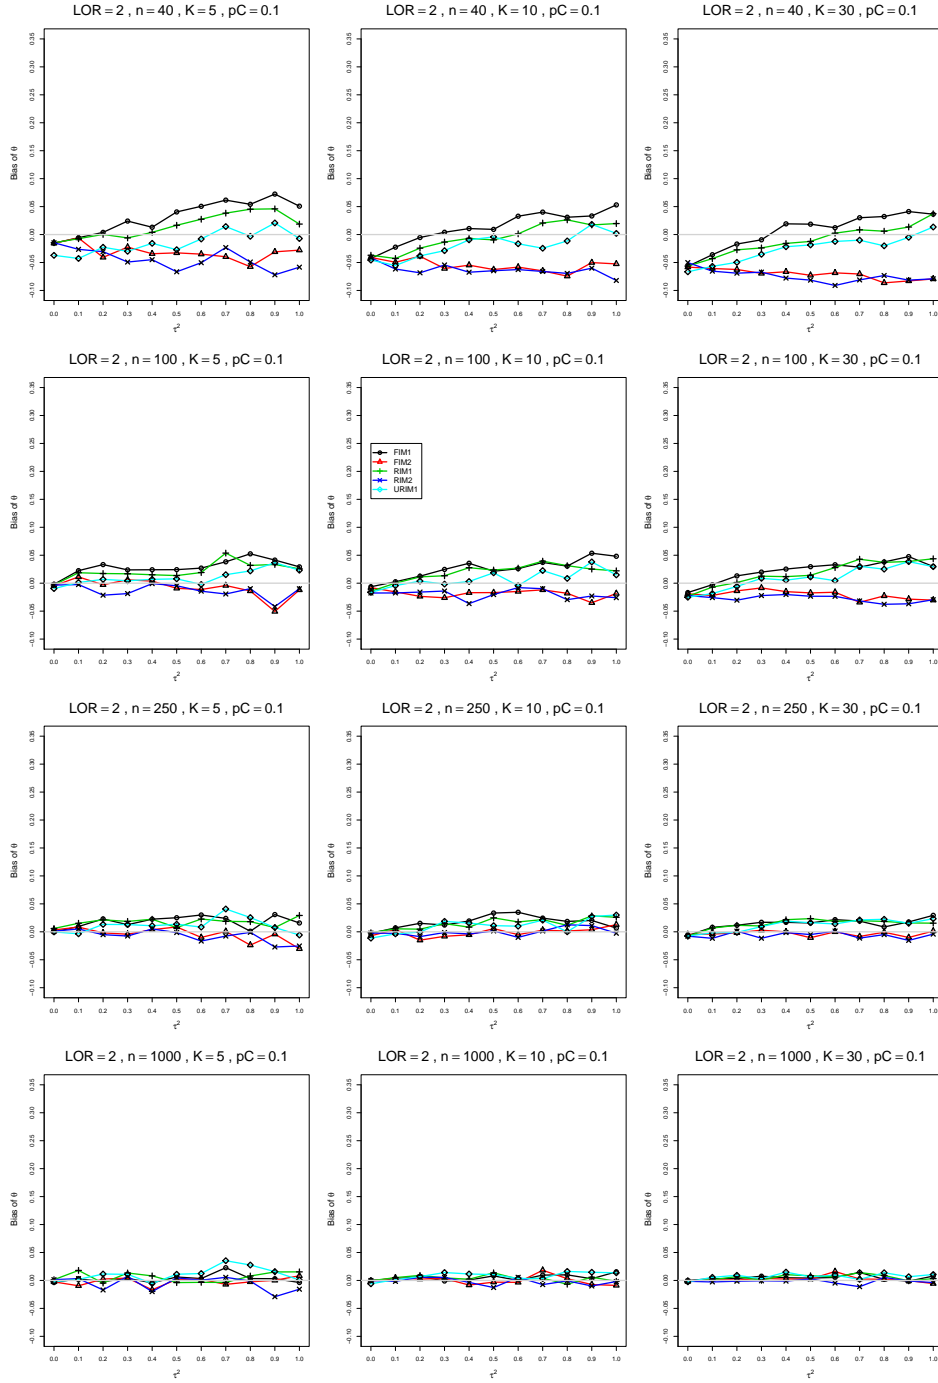

Figure A2.1.19: Bias of overall log-odds ratio  $\hat{\theta}_{DL}$  for  $\theta = 2$ ,  $p_C = 0.1$ ,  $\sigma^2 = 0.4$ , constant sample sizes  $n = 40, 100, 250, 1000$ . The data-generation mechanisms are FIM1 ( $\circ$ ), FIM2 ( $\triangle$ ), RIM1 ( $+$ ), RIM2 ( $\times$ ), and URIM1 ( $\diamond$ ).

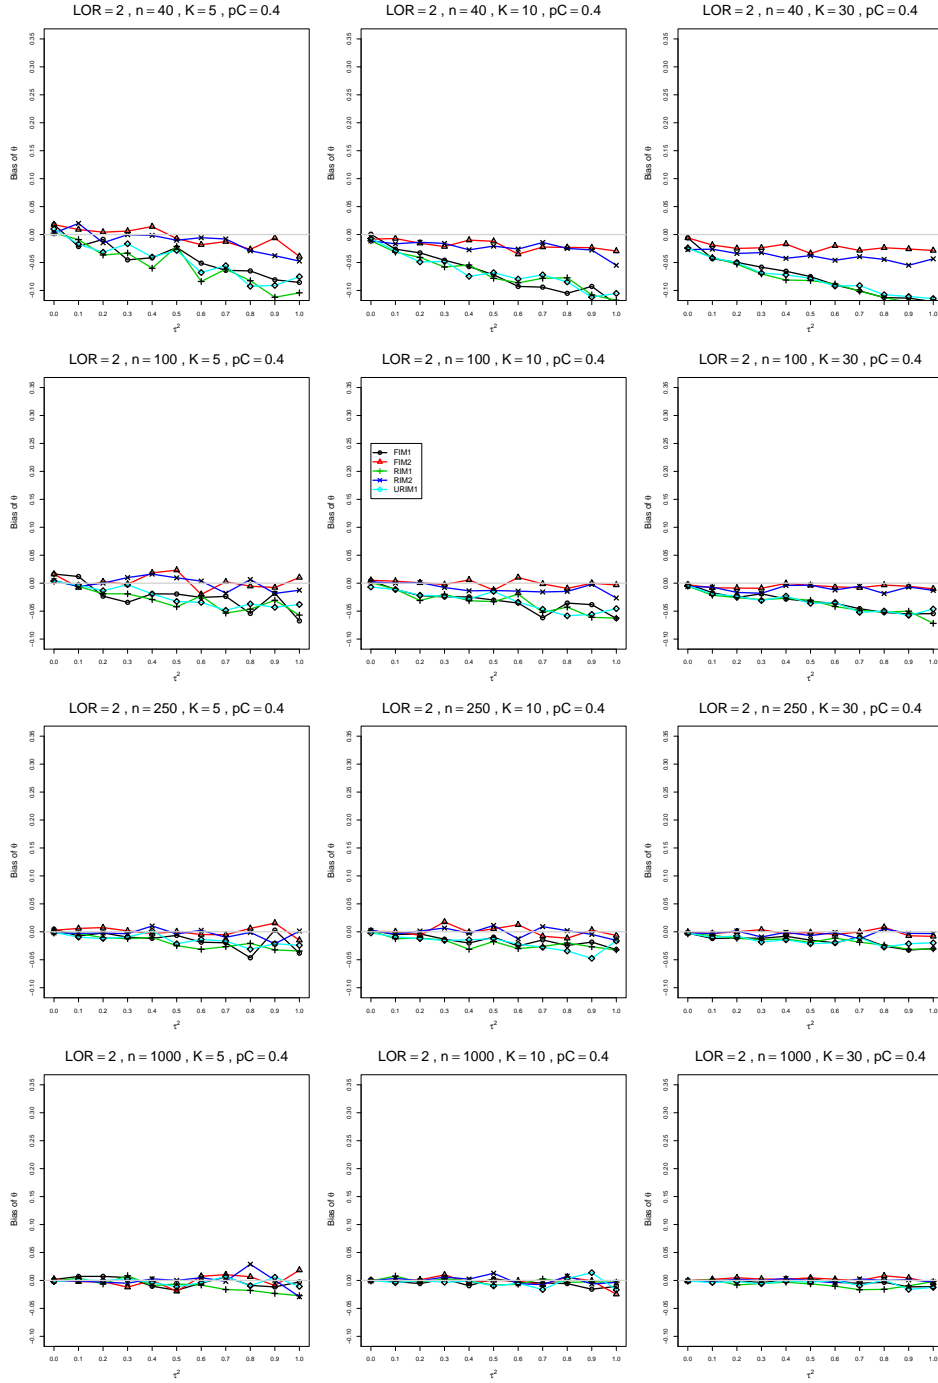

Figure A2.1.20: Bias of overall log-odds ratio  $\hat{\theta}_{DL}$  for  $\theta = 2$ ,  $p_C = 0.4$ ,  $\sigma^2 = 0.4$ , constant sample sizes  $n = 40, 100, 250, 1000$ . The data-generation mechanisms are FIM1 ( $\circ$ ), FIM2 ( $\triangle$ ), RIM1 ( $+$ ), RIM2 ( $\times$ ), and URIM1 ( $\diamond$ ).

## A2.2 Bias of $\hat{\theta}_{REML}$

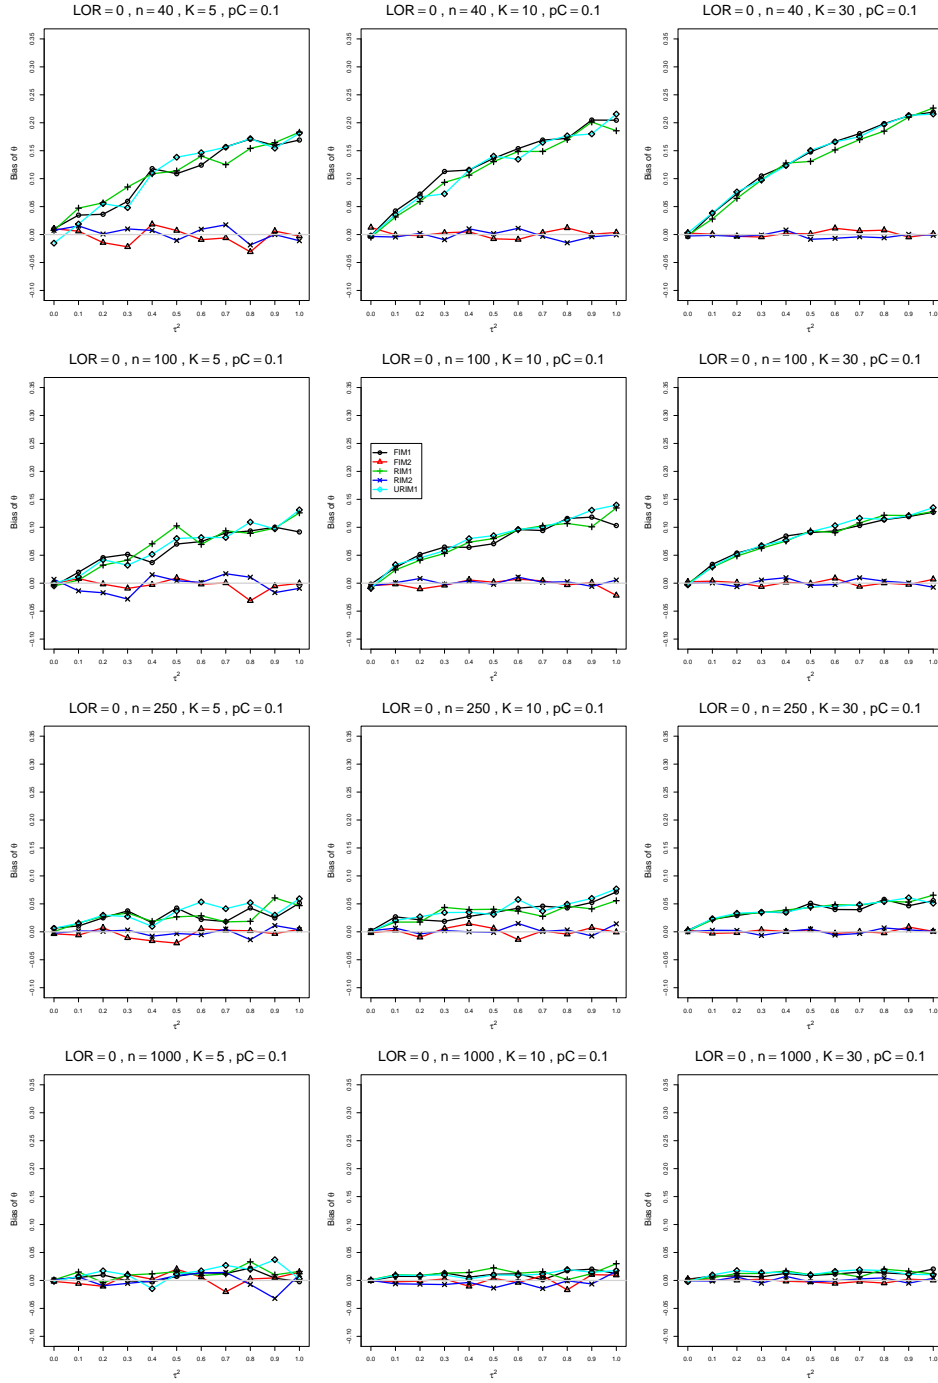

Figure A2.2.1: Bias of overall log-odds ratio  $\hat{\theta}_{REML}$  for  $\theta = 0$ ,  $p_C = 0.1$ ,  $\sigma^2 = 0.1$ , constant sample sizes  $n = 40, 100, 250, 1000$ . The data-generation mechanisms are FIM1 ( $\circ$ ), FIM2 ( $\triangle$ ), RIM1 ( $+$ ), RIM2 ( $\times$ ), and URIM1 ( $\diamond$ ).

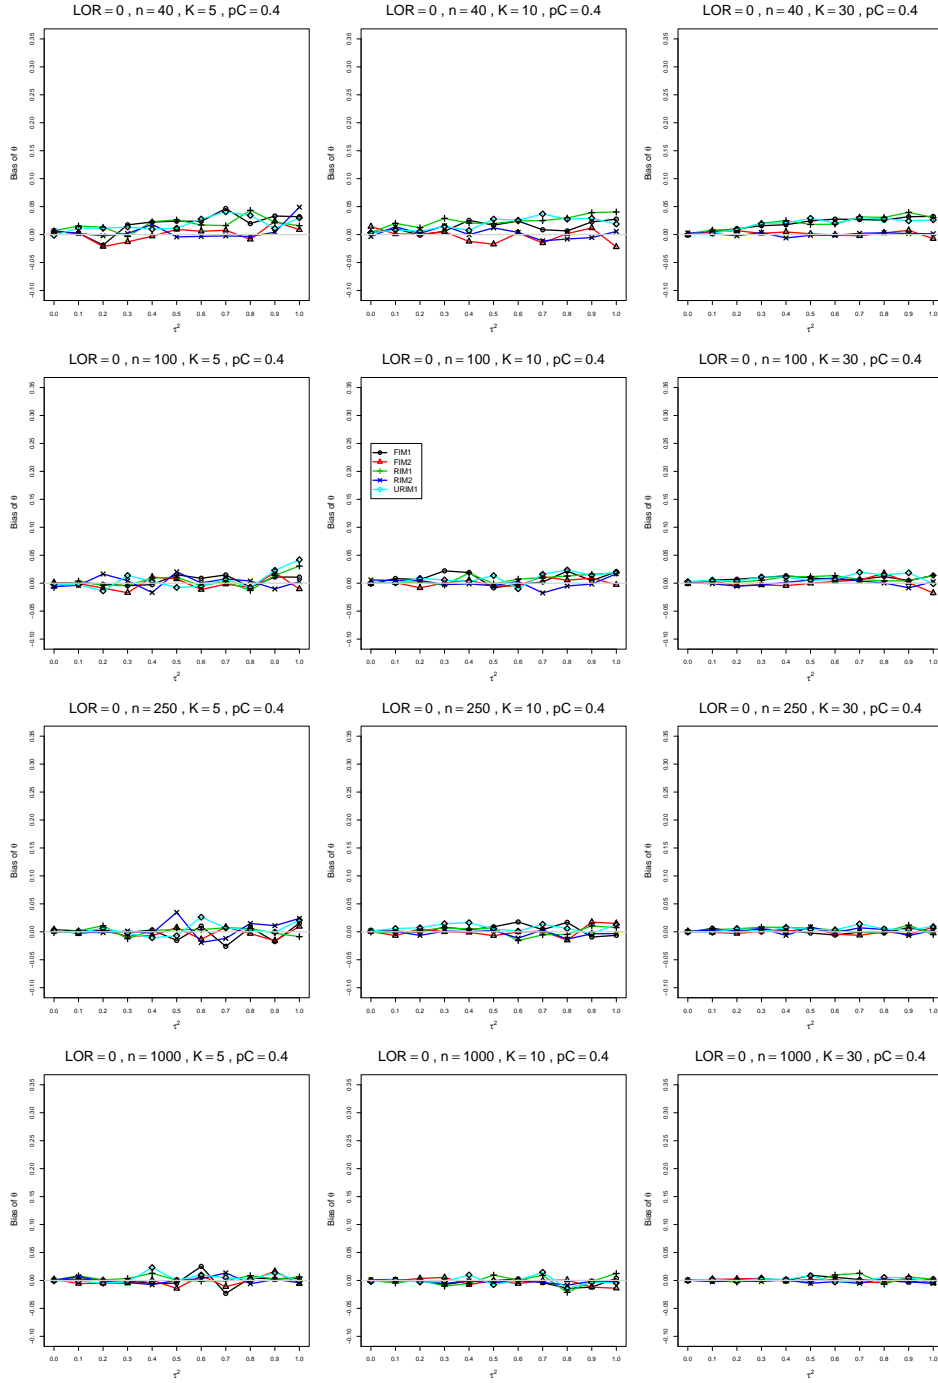

Figure A2.2.2: Bias of overall log-odds ratio  $\hat{\theta}_{REML}$  for  $\theta = 0$ ,  $p_C = 0.4$ ,  $\sigma^2 = 0.1$ , constant sample sizes  $n = 40, 100, 250, 1000$ . The data-generation mechanisms are FIM1 ( $\circ$ ), FIM2 ( $\triangle$ ), RIM1 ( $+$ ), RIM2 ( $\times$ ), and URIM1 ( $\diamond$ ).

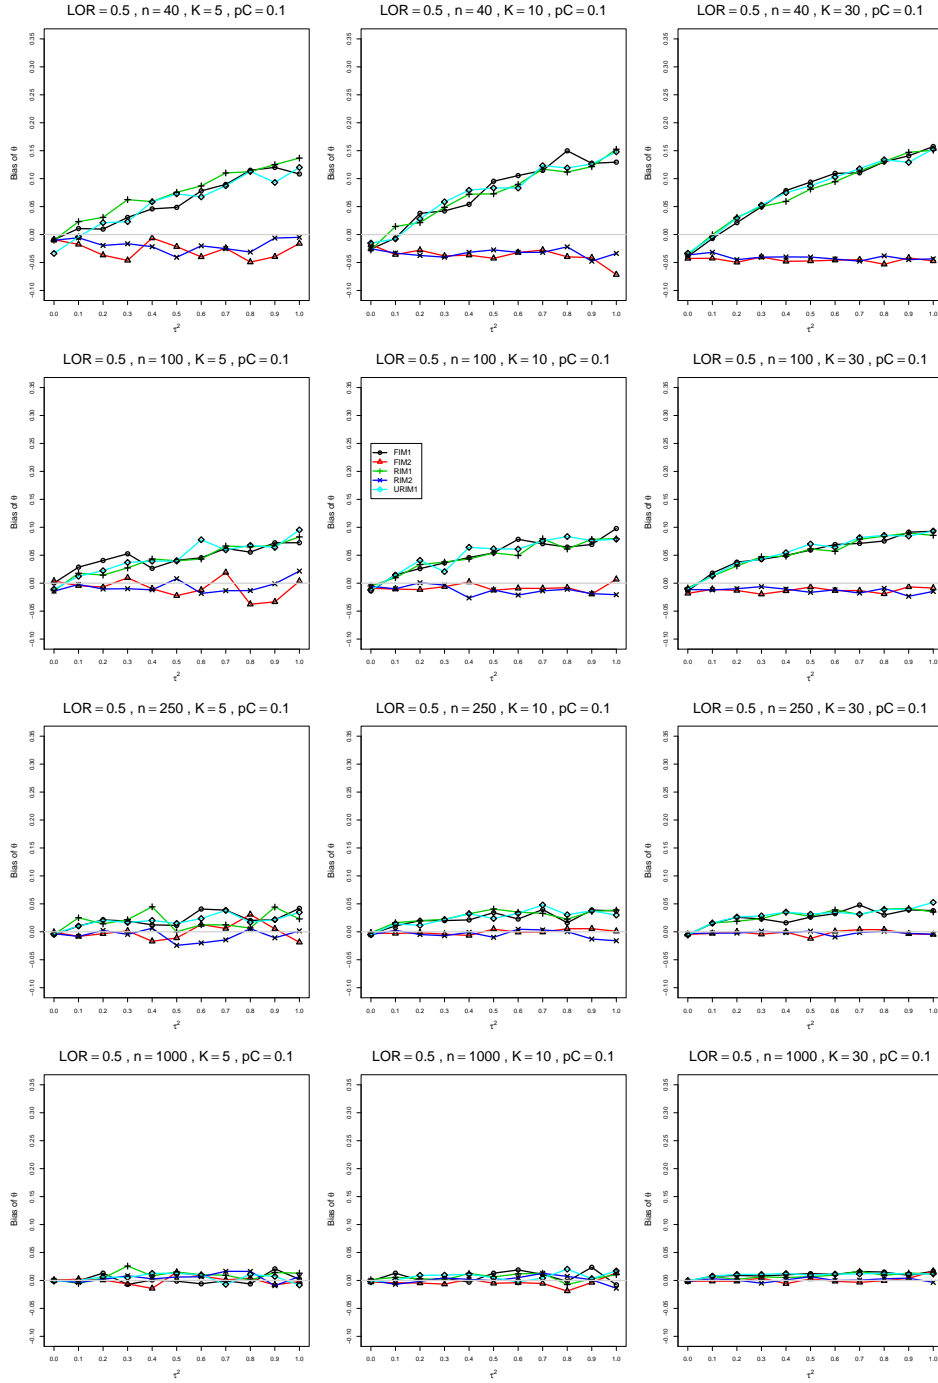

Figure A2.2.3: Bias of overall log-odds ratio  $\hat{\theta}_{REML}$  for  $\theta = 0.5$ ,  $p_C = 0.1$ ,  $\sigma^2 = 0.1$ , constant sample sizes  $n = 40, 100, 250, 1000$ . The data-generation mechanisms are FIM1 ( $\circ$ ), FIM2 ( $\triangle$ ), RIM1 ( $+$ ), RIM2 ( $\times$ ), and URIM1 ( $\diamond$ ).

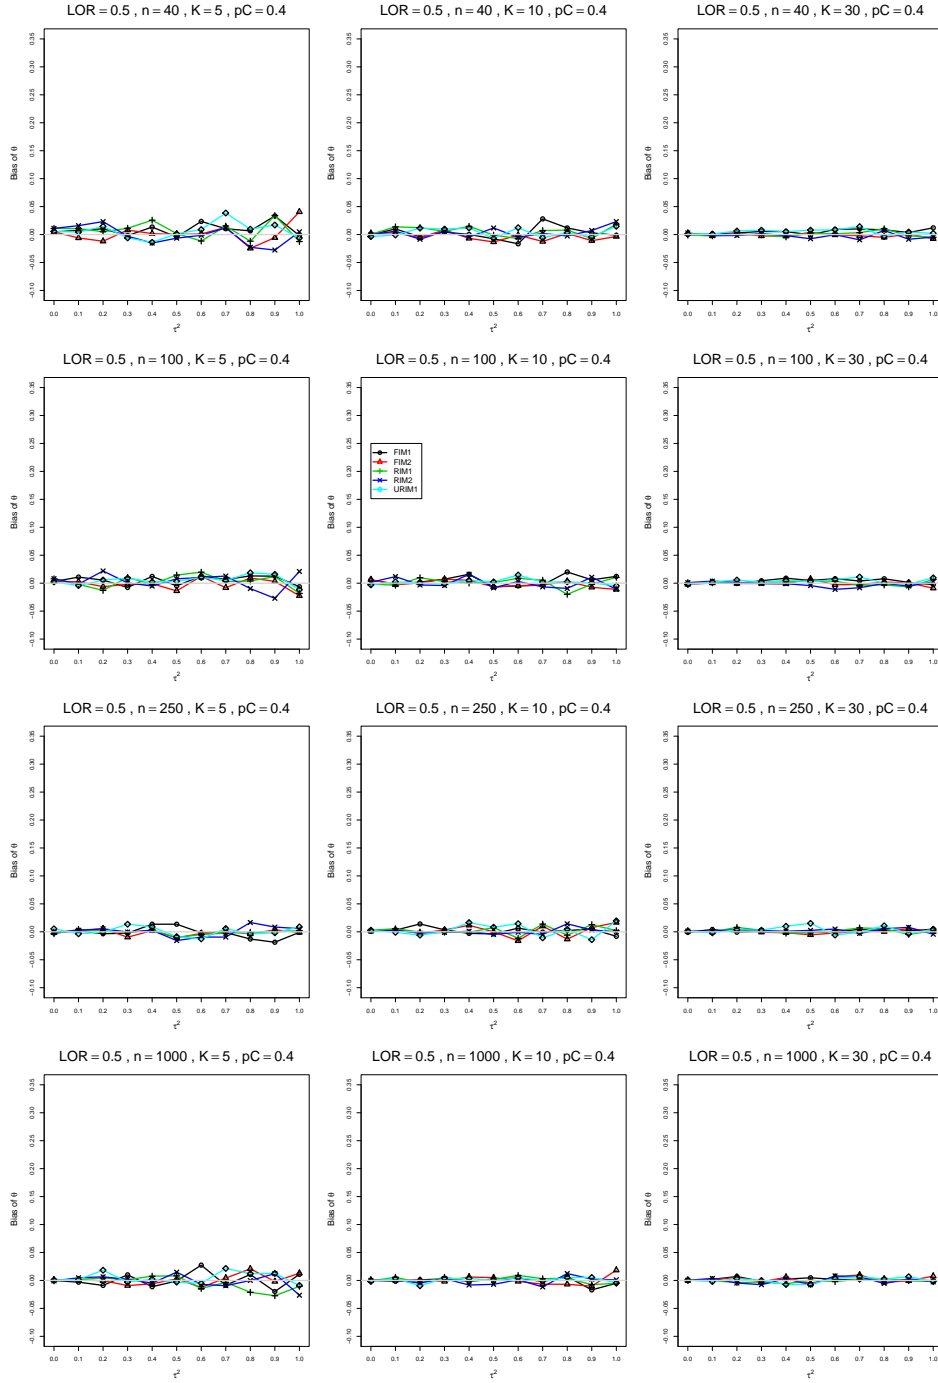

Figure A2.2.4: Bias of overall log-odds ratio  $\hat{\theta}_{REML}$  for  $\theta = 0.5$ ,  $p_C = 0.4$ ,  $\sigma^2 = 0.1$ , constant sample sizes  $n = 40, 100, 250, 1000$ . The data-generation mechanisms are FIM1 ( $\circ$ ), FIM2 ( $\triangle$ ), RIM1 ( $+$ ), RIM2 ( $\times$ ), and URIM1 ( $\diamond$ ).

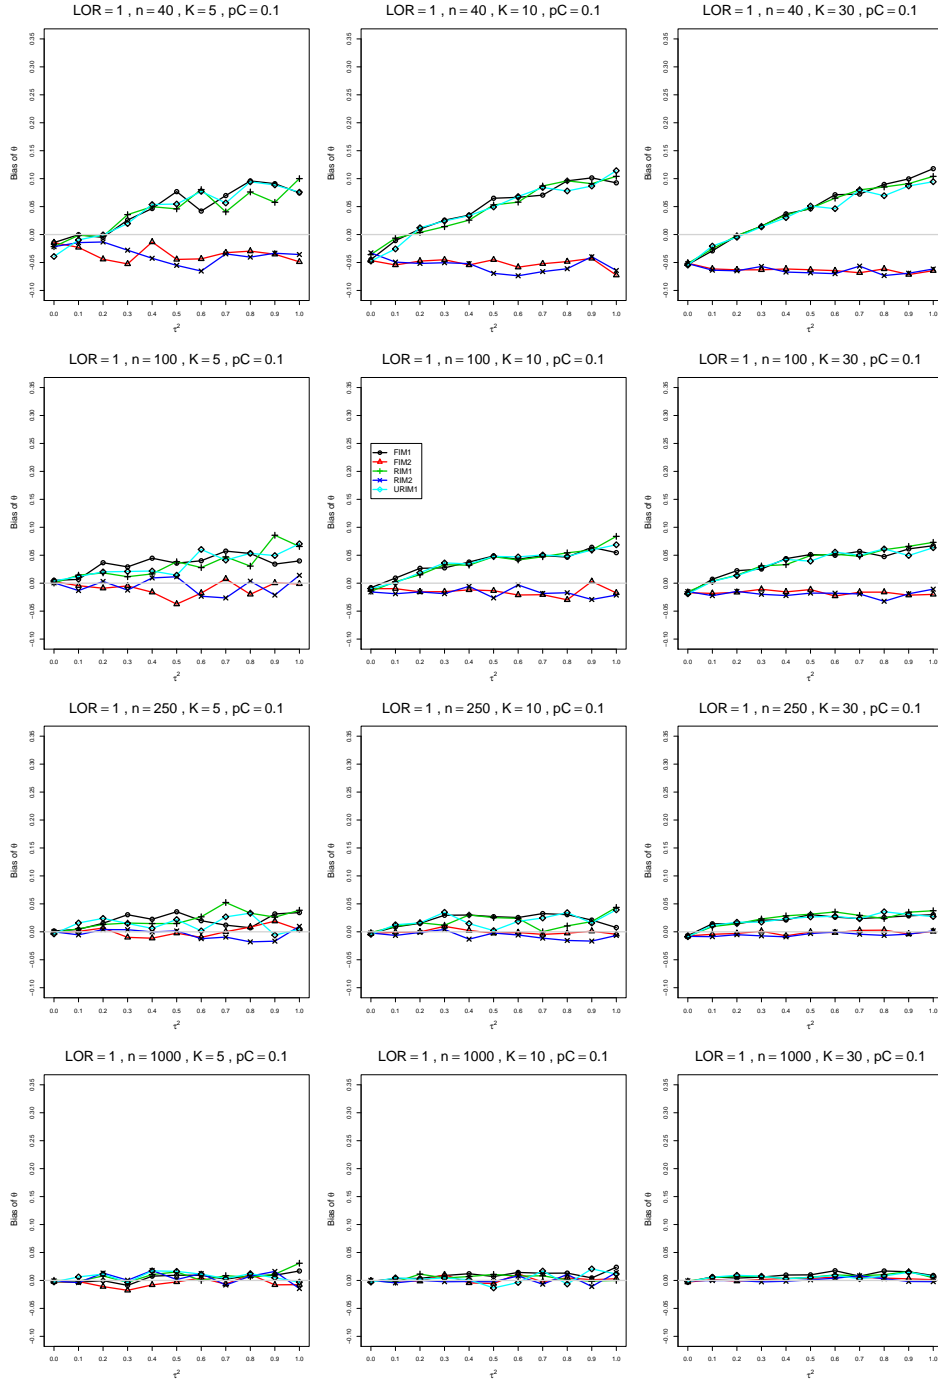

Figure A2.2.5: Bias of overall log-odds ratio  $\hat{\theta}_{REML}$  for  $\theta = 1$ ,  $p_C = 0.1$ ,  $\sigma^2 = 0.1$ , constant sample sizes  $n = 40, 100, 250, 1000$ . The data-generation mechanisms are FIM1 ( $\circ$ ), FIM2 ( $\triangle$ ), RIM1 ( $+$ ), RIM2 ( $\times$ ), and URIM1 ( $\diamond$ ).



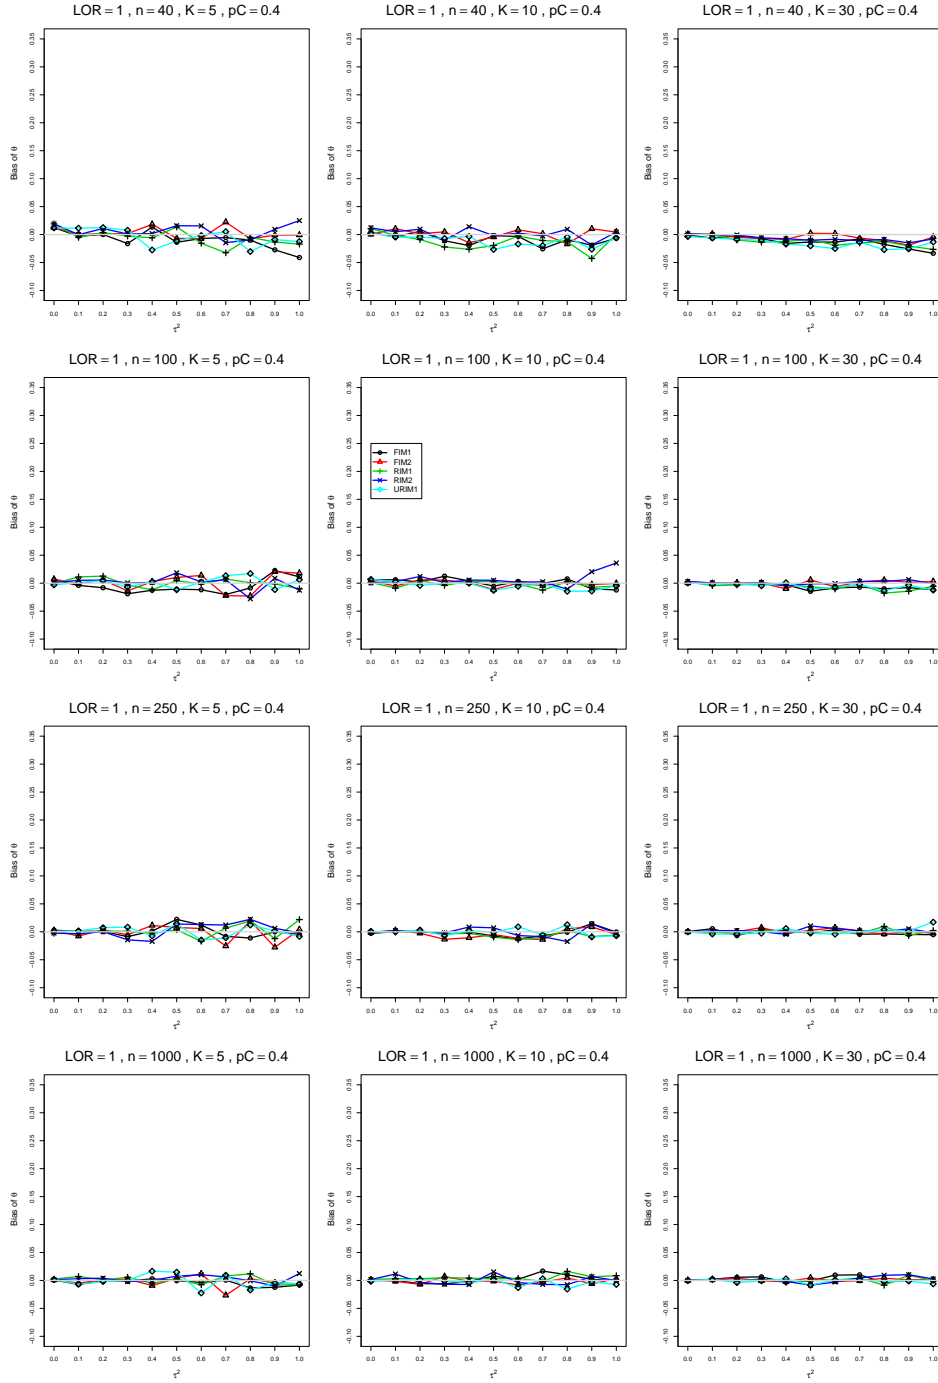

Figure A2.2.6: Bias of overall log-odds ratio  $\hat{\theta}_{REML}$  for  $\theta = 1$ ,  $p_C = 0.4$ ,  $\sigma^2 = 0.1$ , constant sample sizes  $n = 40, 100, 250, 1000$ . The data-generation mechanisms are FIM1 ( $\circ$ ), FIM2 ( $\triangle$ ), RIM1 ( $+$ ), RIM2 ( $\times$ ), and URIM1 ( $\diamond$ ).

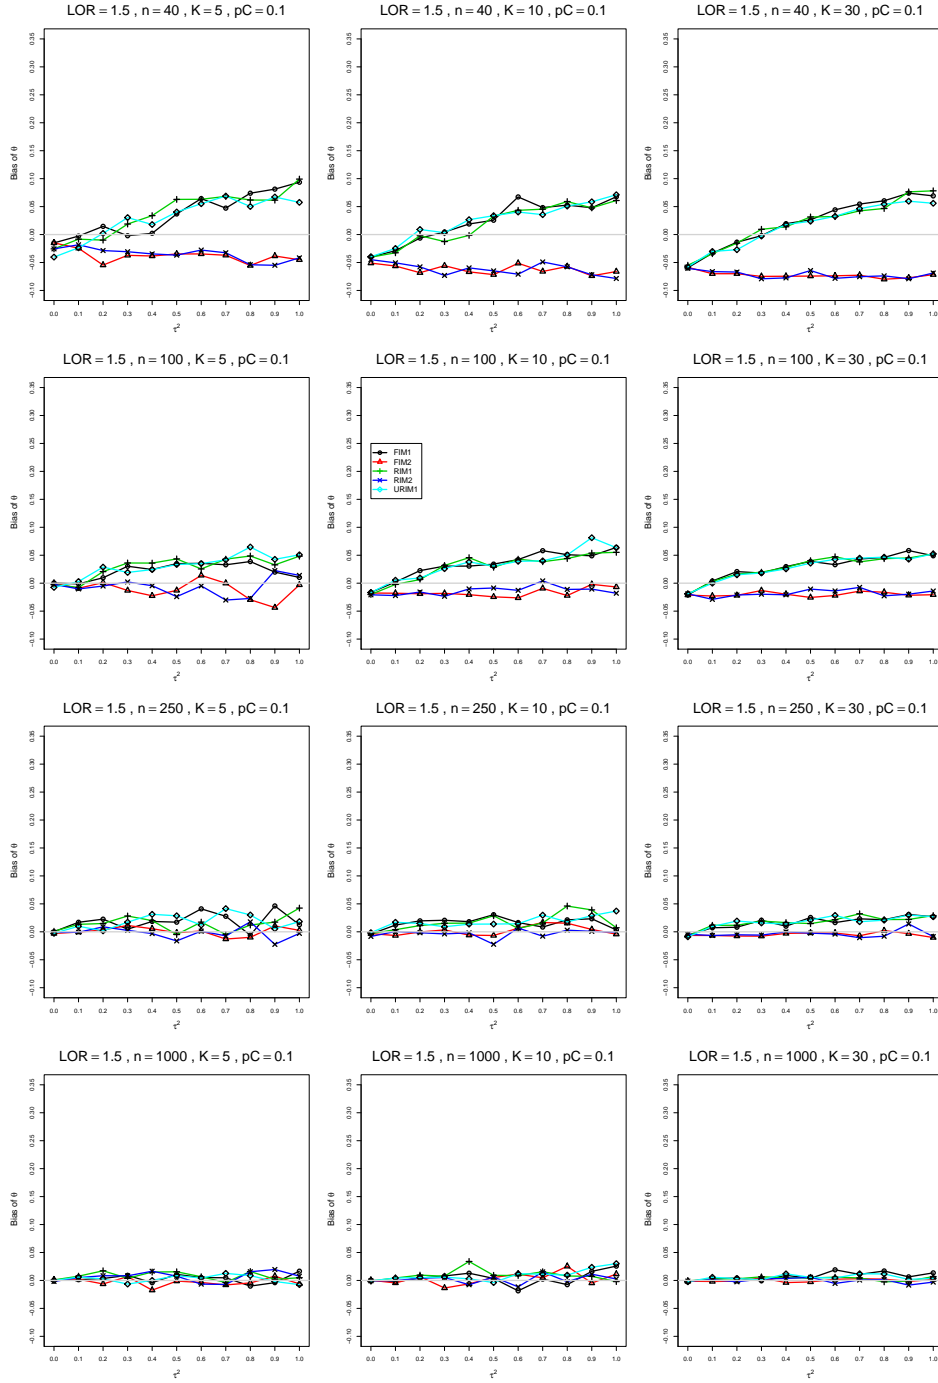

Figure A2.2.7: Bias of overall log-odds ratio  $\hat{\theta}_{REML}$  for  $\theta = 1.5$ ,  $p_C = 0.1$ ,  $\sigma^2 = 0.1$ , constant sample sizes  $n = 40, 100, 250, 1000$ . The data-generation mechanisms are FIM1 ( $\circ$ ), FIM2 ( $\triangle$ ), RIM1 (+), RIM2 ( $\times$ ), and URIM1 ( $\diamond$ ).

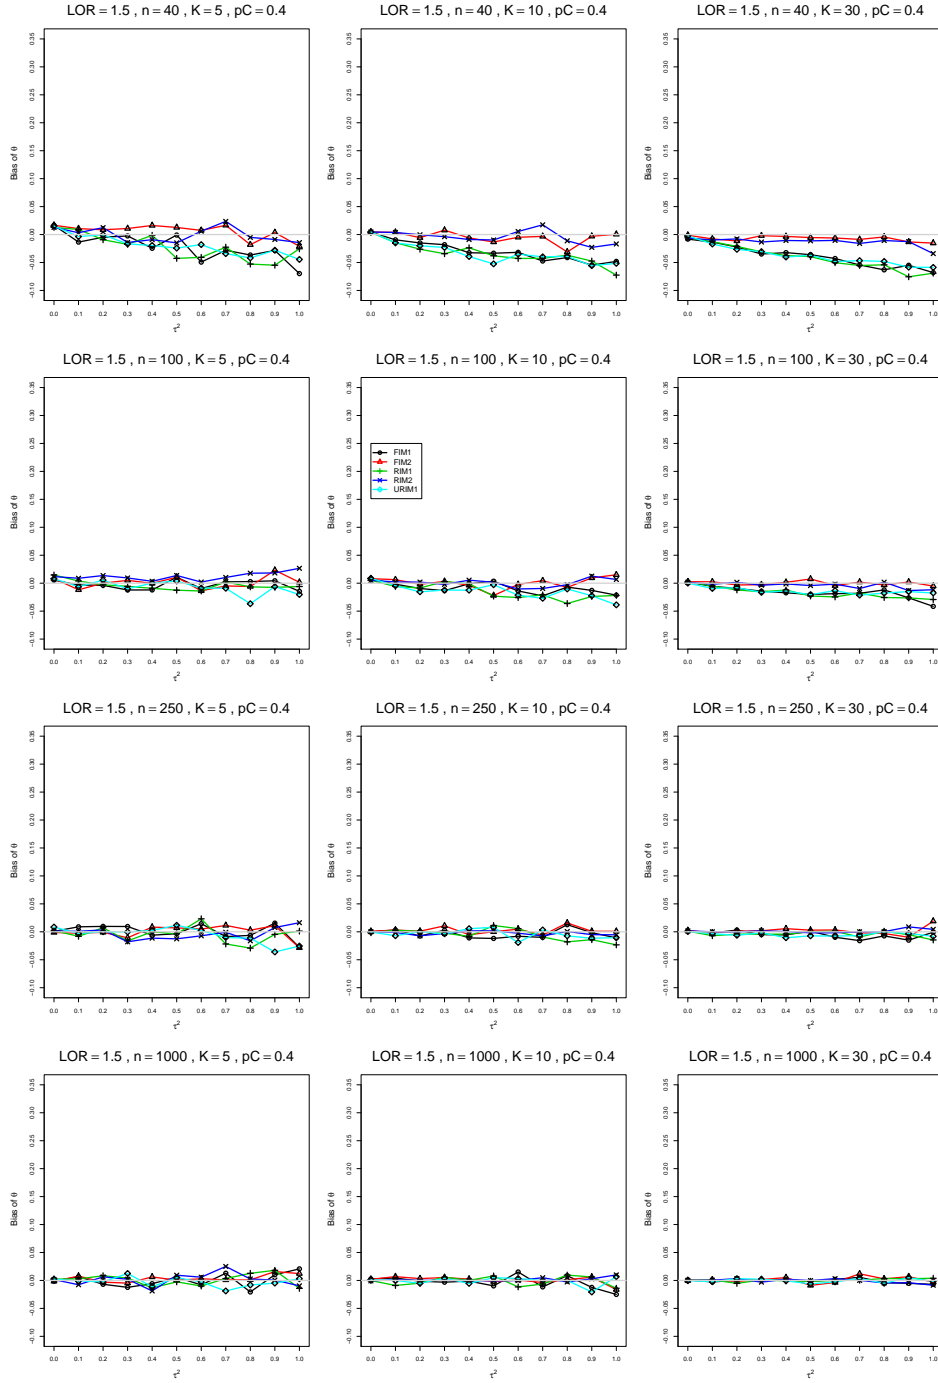

Figure A2.2.8: Bias of overall log-odds ratio  $\hat{\theta}_{REML}$  for  $\theta = 1.5$ ,  $p_C = 0.4$ ,  $\sigma^2 = 0.1$ , constant sample sizes  $n = 40, 100, 250, 1000$ . The data-generation mechanisms are FIM1 ( $\circ$ ), FIM2 ( $\triangle$ ), RIM1 ( $+$ ), RIM2 ( $\times$ ), and URIM1 ( $\diamond$ ).

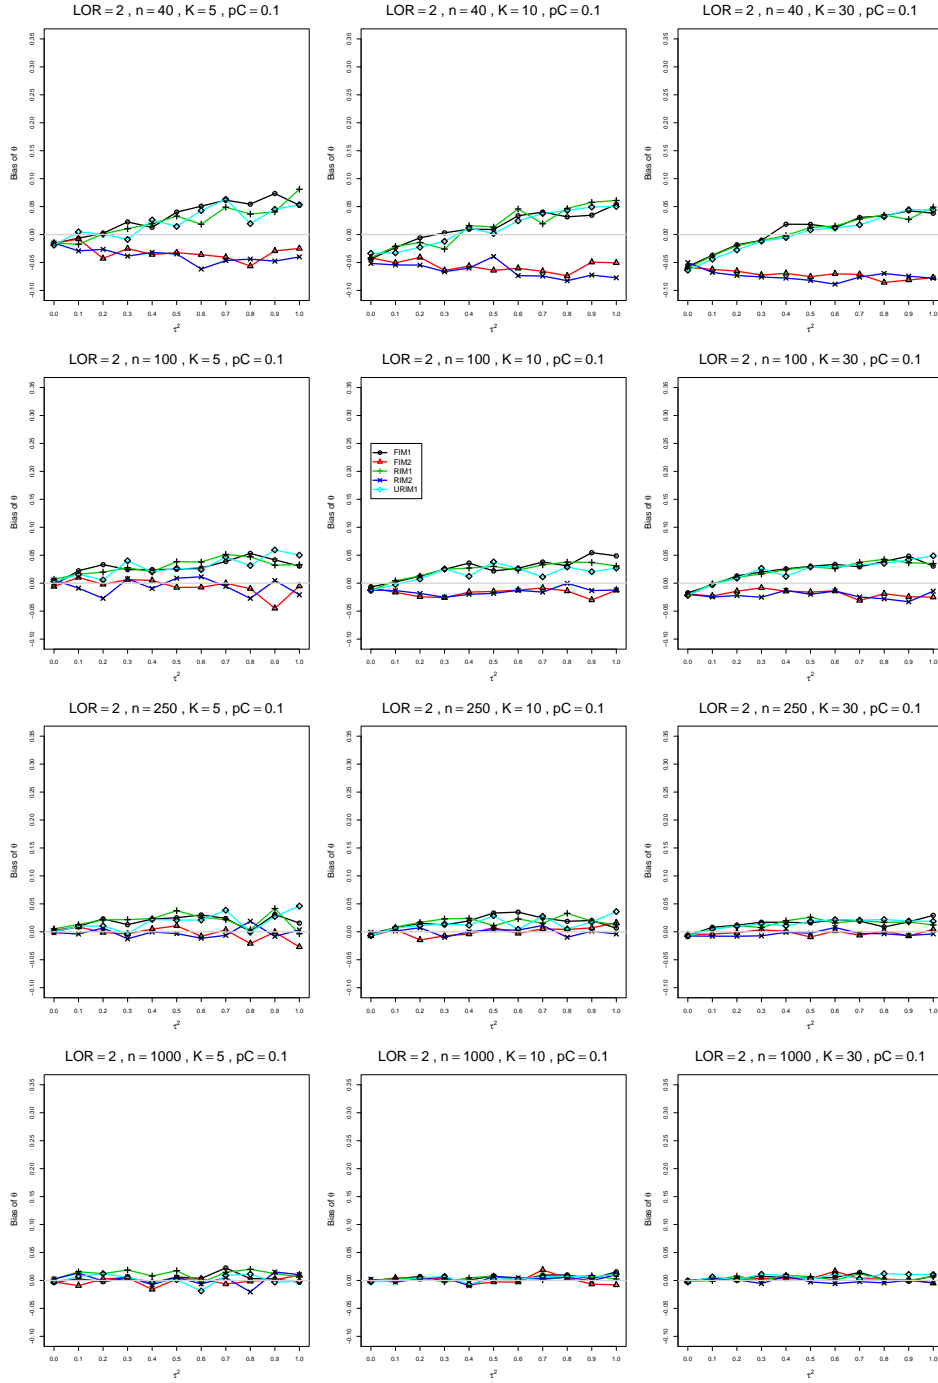

Figure A2.2.9: Bias of overall log-odds ratio  $\hat{\theta}_{REML}$  for  $\theta = 2$ ,  $p_C = 0.1$ ,  $\sigma^2 = 0.1$ , constant sample sizes  $n = 40, 100, 250, 1000$ . The data-generation mechanisms are FIM1 ( $\circ$ ), FIM2 ( $\triangle$ ), RIM1 ( $+$ ), RIM2 ( $\times$ ), and URIM1 ( $\diamond$ ).

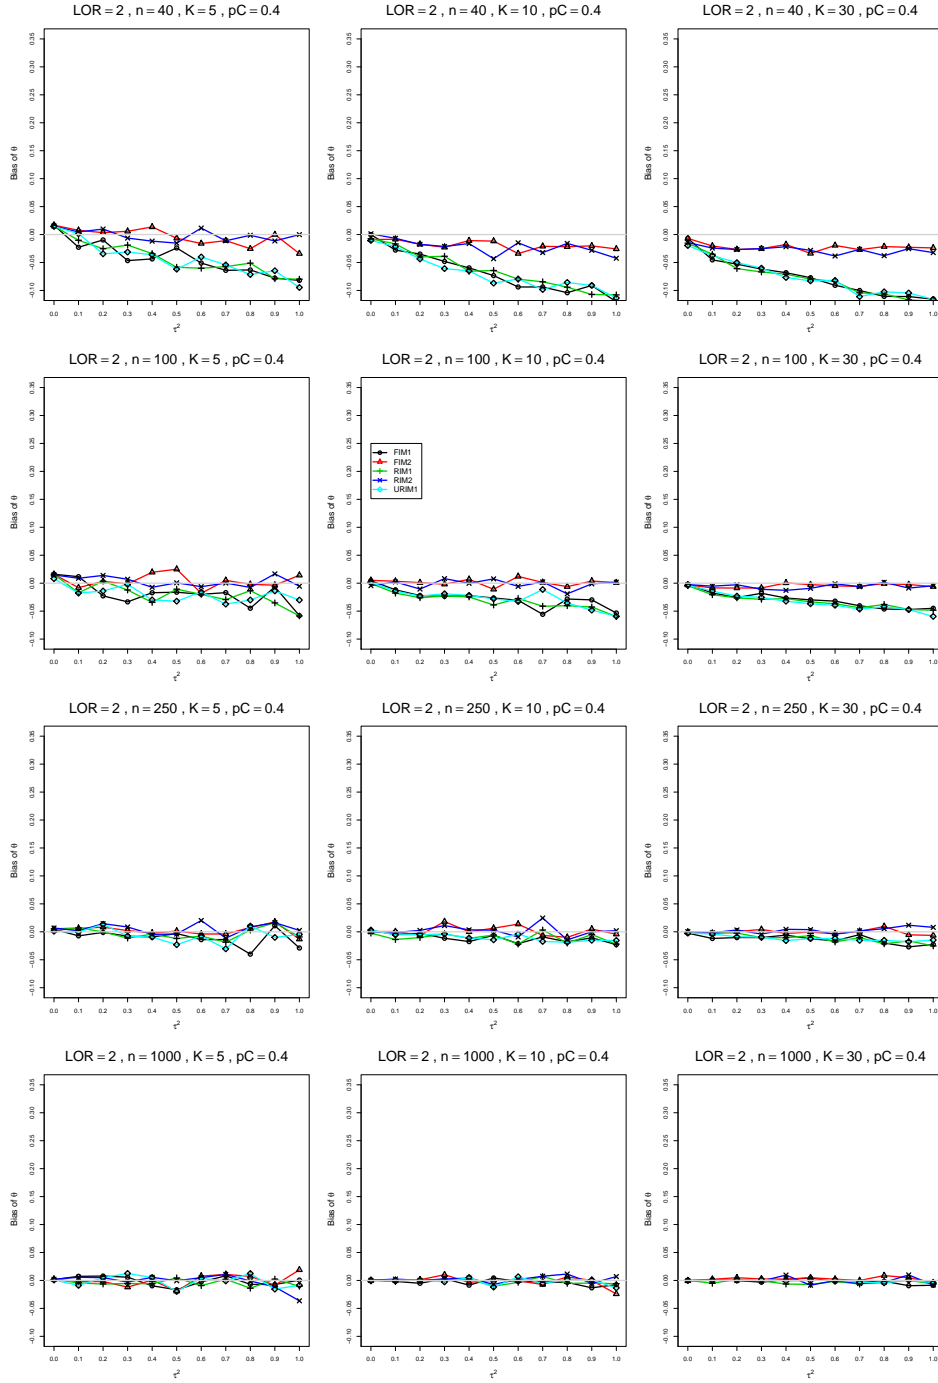

Figure A2.2.10: Bias of overall log-odds ratio  $\hat{\theta}_{REML}$  for  $\theta = 2$ ,  $p_C = 0.4$ ,  $\sigma^2 = 0.1$ , constant sample sizes  $n = 40, 100, 250, 1000$ . The data-generation mechanisms are FIM1 ( $\circ$ ), FIM2 ( $\triangle$ ), RIM1 ( $+$ ), RIM2 ( $\times$ ), and URIM1 ( $\diamond$ ).

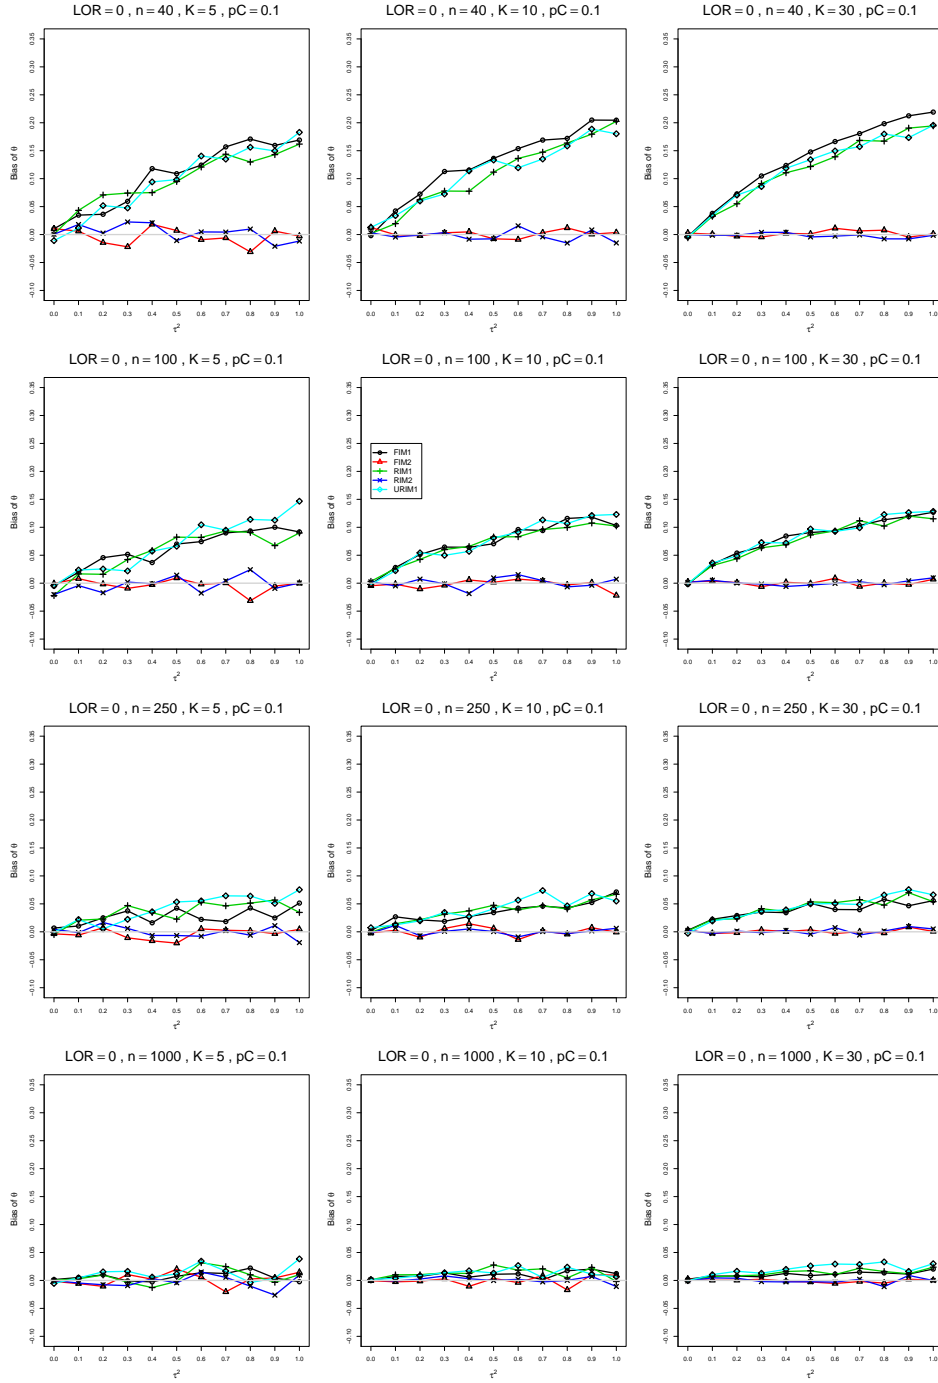

Figure A2.2.11: Bias of overall log-odds ratio  $\hat{\theta}_{REML}$  for  $\theta = 0$ ,  $p_C = 0.1$ ,  $\sigma^2 = 0.4$ , constant sample sizes  $n = 40, 100, 250, 1000$ . The data-generation mechanisms are FIM1 ( $\circ$ ), FIM2 ( $\triangle$ ), RIM1 ( $+$ ), RIM2 ( $\times$ ), and URIM1 ( $\diamond$ ).

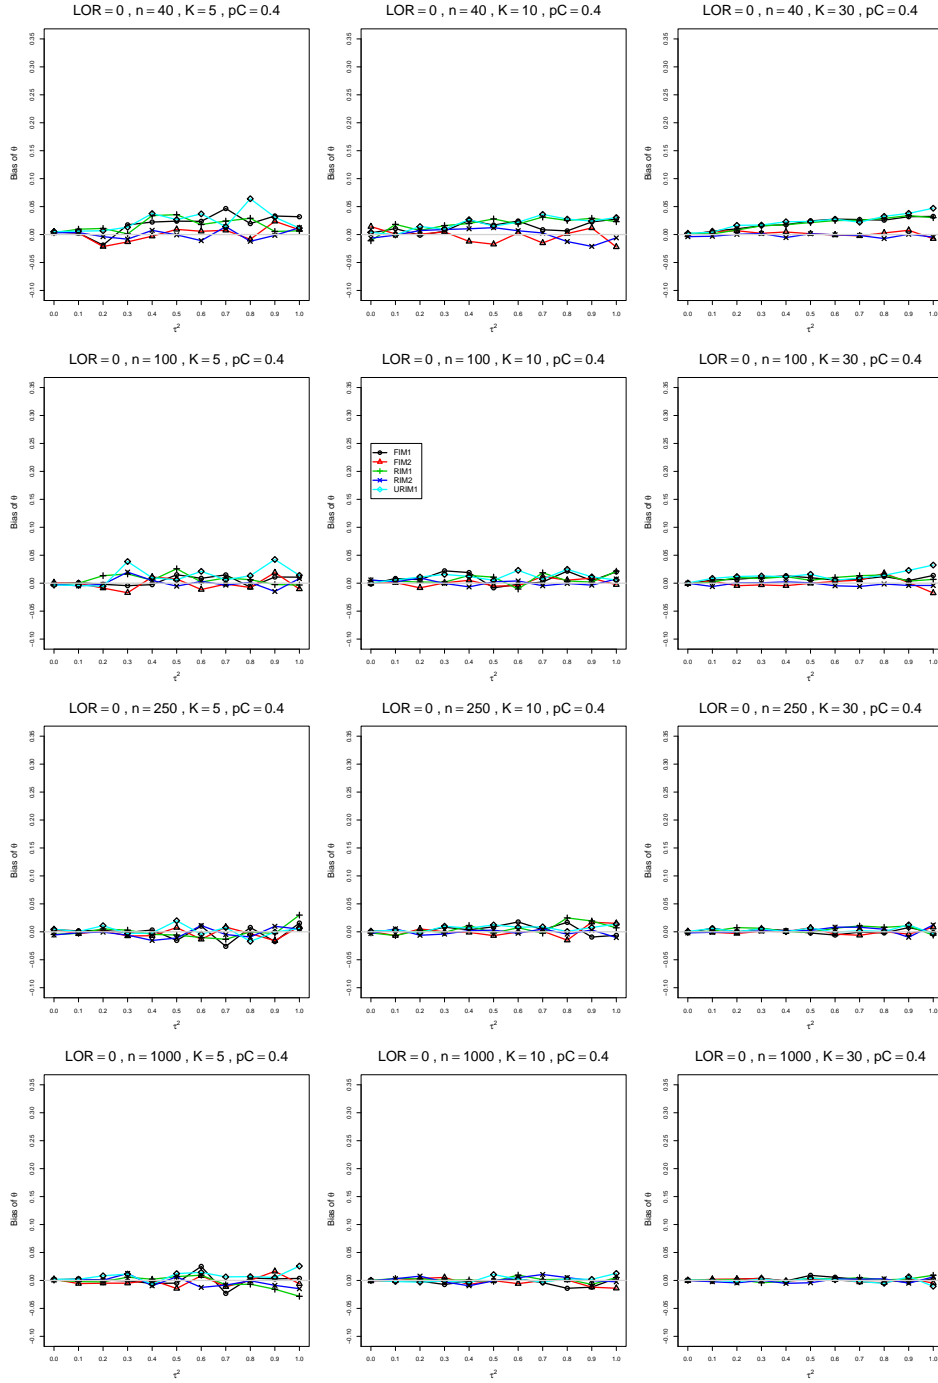

Figure A2.2.12: Bias of overall log-odds ratio  $\hat{\theta}_{REML}$  for  $\theta = 0$ ,  $p_C = 0.4$ ,  $\sigma^2 = 0.4$ , constant sample sizes  $n = 40, 100, 250, 1000$ . The data-generation mechanisms are FIM1 ( $\circ$ ), FIM2 ( $\triangle$ ), RIM1 ( $+$ ), RIM2 ( $\times$ ), and URIM1 ( $\diamond$ ).

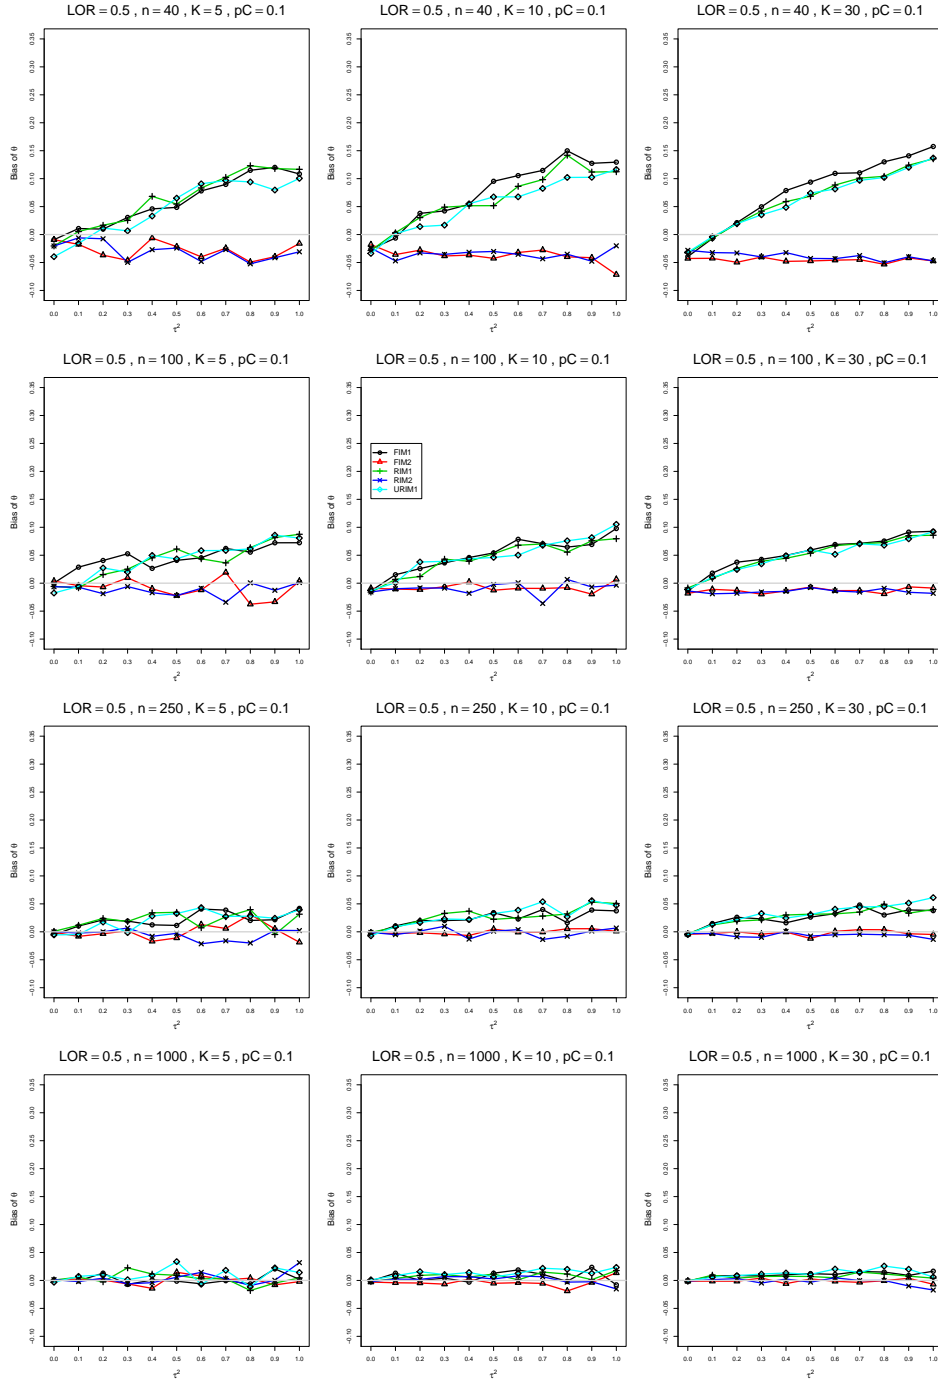

Figure A2.2.13: Bias of overall log-odds ratio  $\hat{\theta}_{REML}$  for  $\theta = 0.5$ ,  $p_C = 0.1$ ,  $\sigma^2 = 0.4$ , constant sample sizes  $n = 40, 100, 250, 1000$ . The data-generation mechanisms are FIM1 ( $\circ$ ), FIM2 ( $\triangle$ ), RIM1 ( $+$ ), RIM2 ( $\times$ ), and URIM1 ( $\diamond$ ).



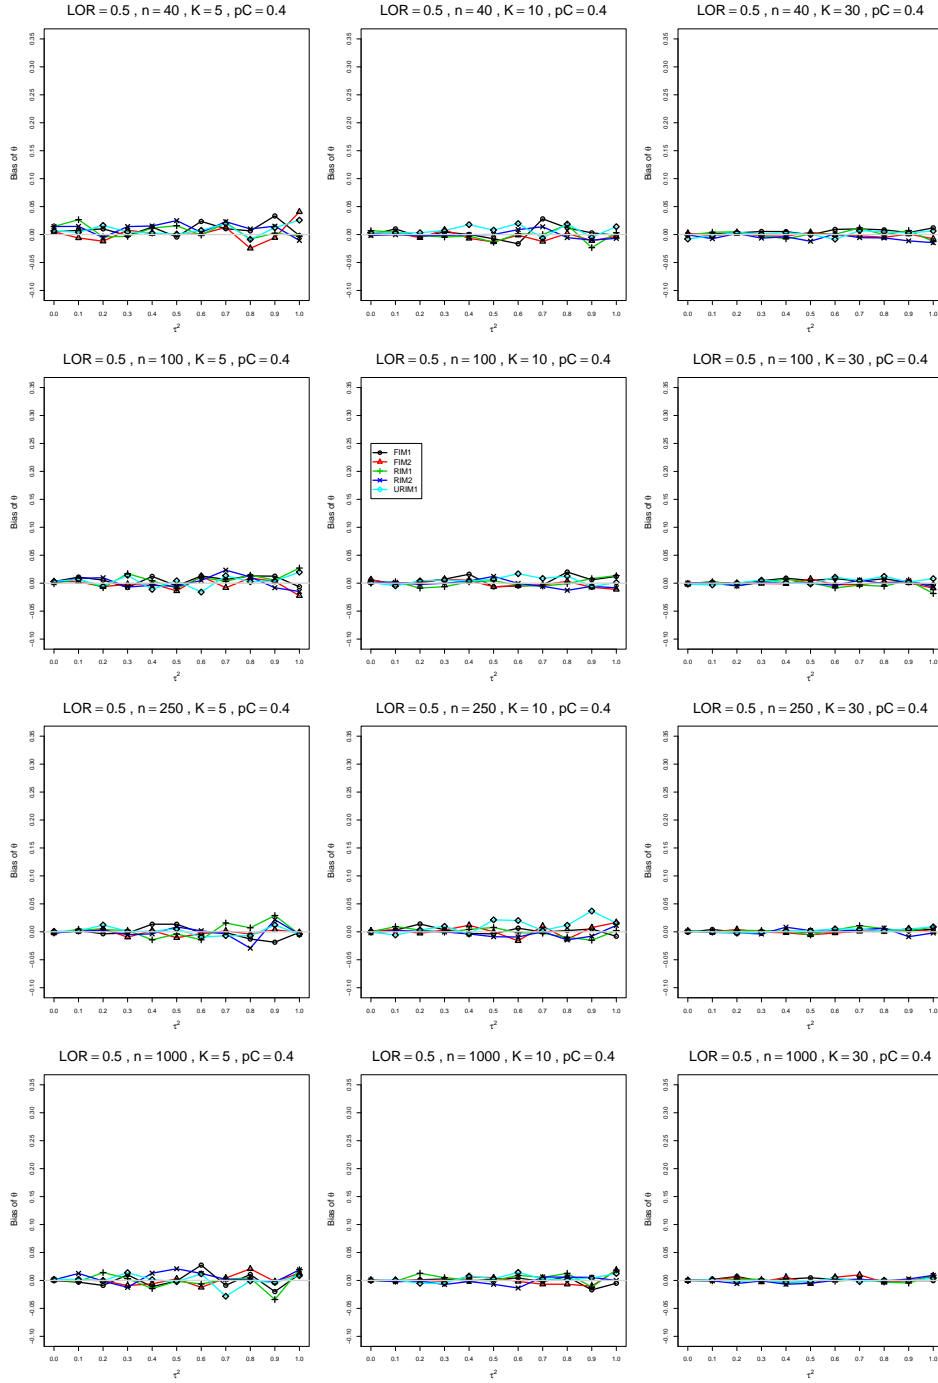

Figure A2.2.14: Bias of overall log-odds ratio  $\hat{\theta}_{REML}$  for  $\theta = 0.5$ ,  $p_C = 0.4$ ,  $\sigma^2 = 0.4$ , constant sample sizes  $n = 40, 100, 250, 1000$ . The data-generation mechanisms are FIM1 ( $\circ$ ), FIM2 ( $\triangle$ ), RIM1 ( $+$ ), RIM2 ( $\times$ ), and URIM1 ( $\diamond$ ).

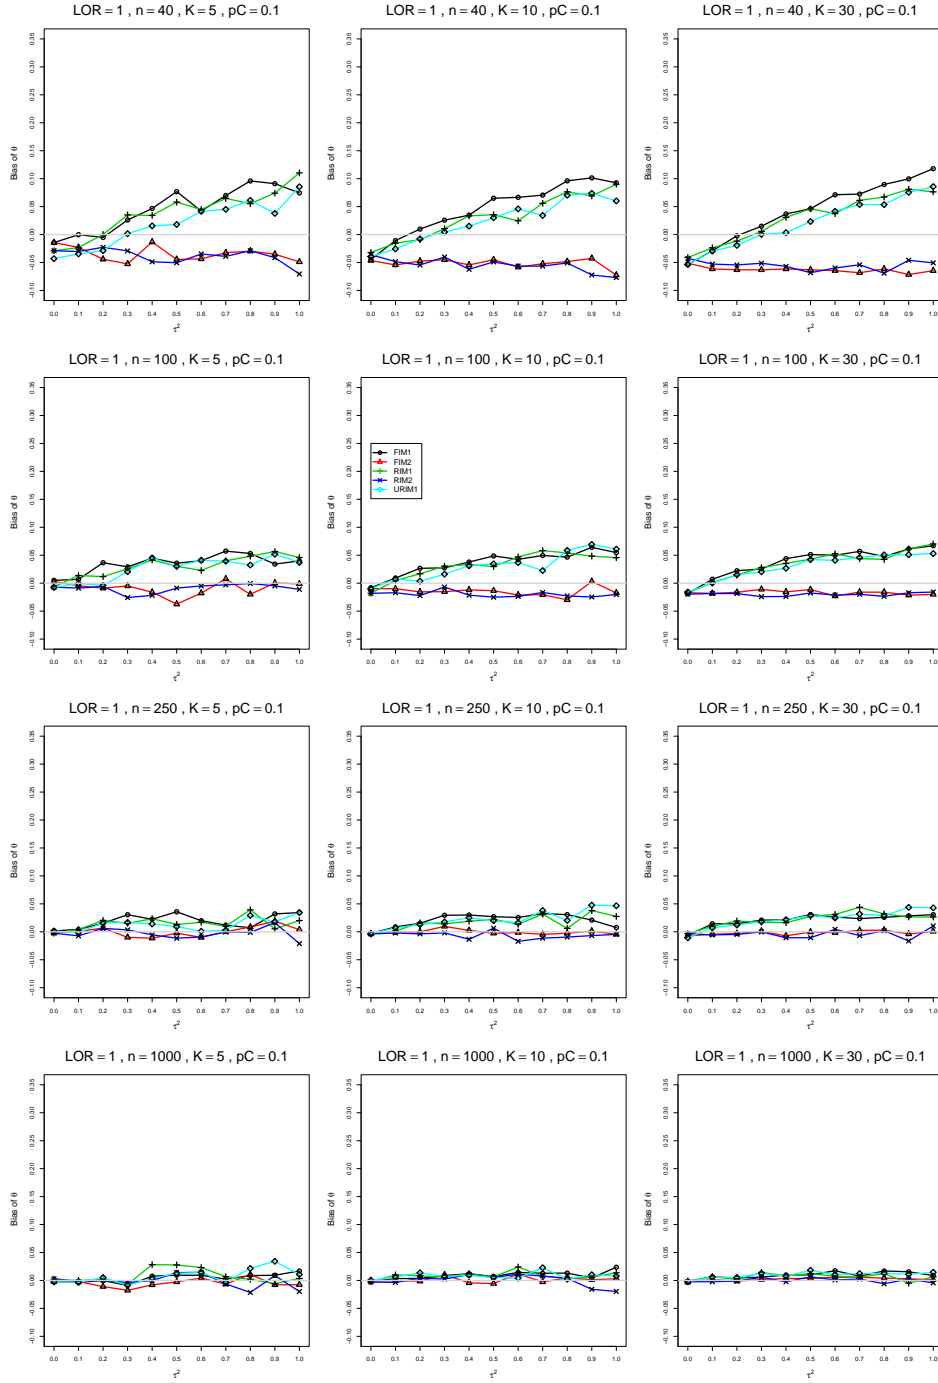

Figure A2.2.15: Bias of overall log-odds ratio  $\hat{\theta}_{REML}$  for  $\theta = 1$ ,  $p_C = 0.1$ ,  $\sigma^2 = 0.4$ , constant sample sizes  $n = 40, 100, 250, 1000$ . The data-generation mechanisms are FIM1 ( $\circ$ ), FIM2 ( $\triangle$ ), RIM1 ( $+$ ), RIM2 ( $\times$ ), and URIM1 ( $\diamond$ ).

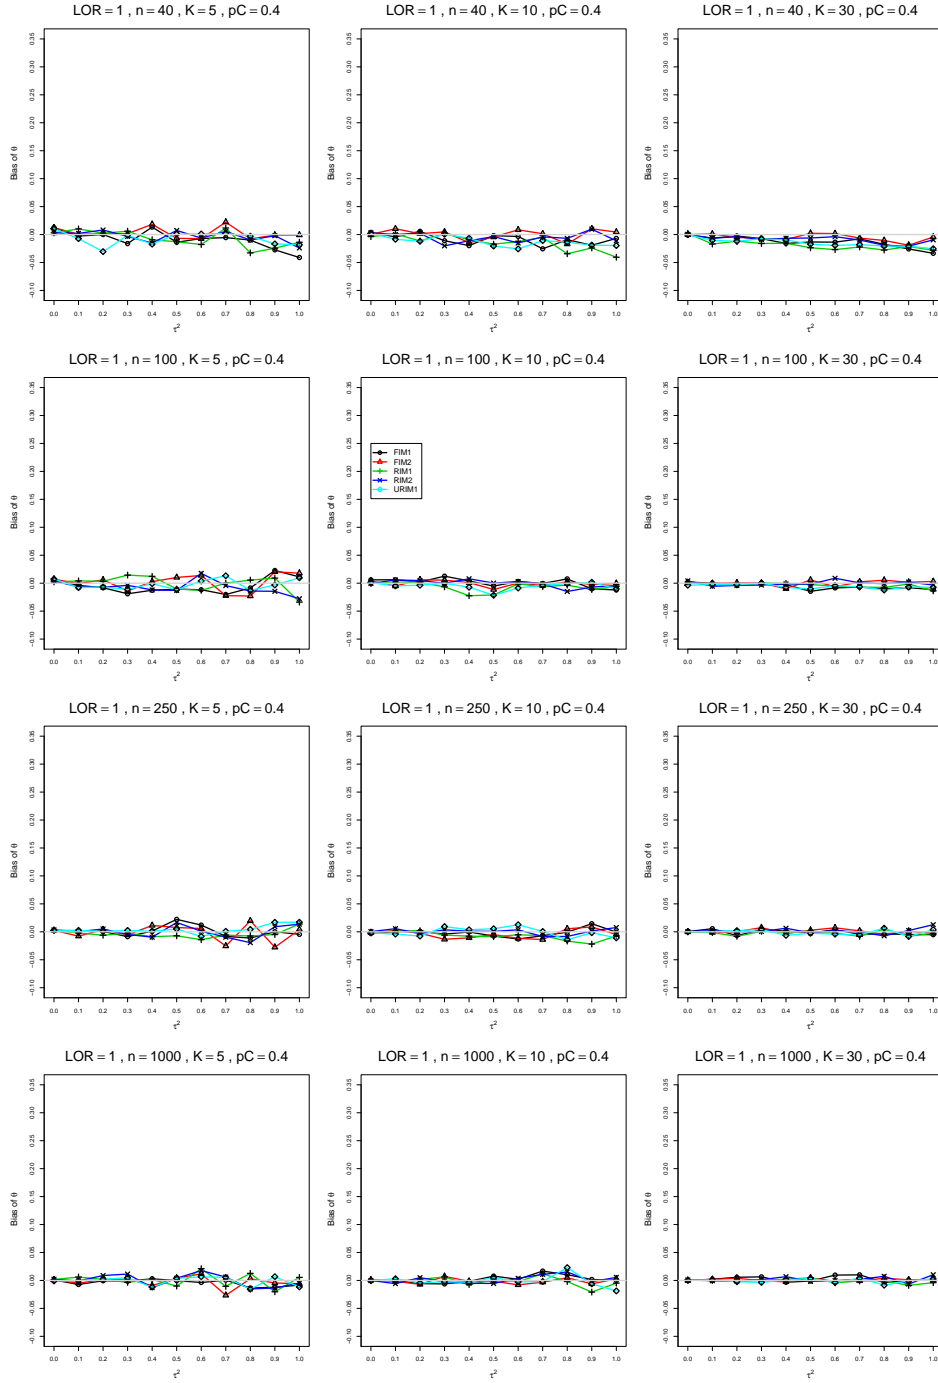

Figure A2.2.16: Bias of overall log-odds ratio  $\hat{\theta}_{REML}$  for  $\theta = 1$ ,  $p_C = 0.4$ ,  $\sigma^2 = 0.4$ , constant sample sizes  $n = 40, 100, 250, 1000$ . The data-generation mechanisms are FIM1 ( $\circ$ ), FIM2 ( $\triangle$ ), RIM1 ( $+$ ), RIM2 ( $\times$ ), and URIM1 ( $\diamond$ ).

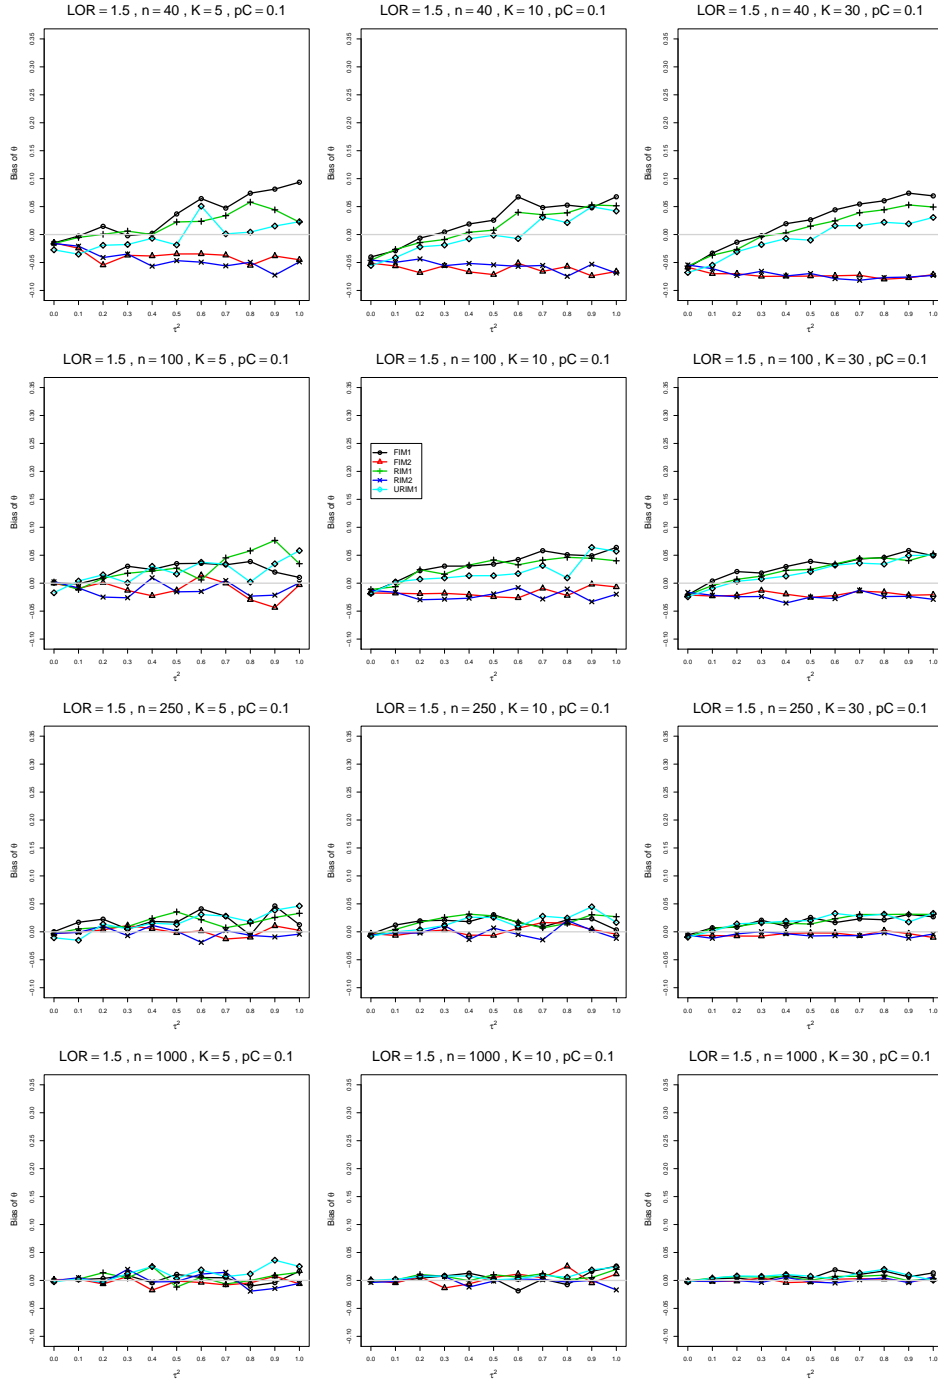

Figure A2.2.17: Bias of overall log-odds ratio  $\hat{\theta}_{REML}$  for  $\theta = 1.5$ ,  $p_C = 0.1$ ,  $\sigma^2 = 0.4$ , constant sample sizes  $n = 40, 100, 250, 1000$ . The data-generation mechanisms are FIM1 ( $\circ$ ), FIM2 ( $\triangle$ ), RIM1 ( $+$ ), RIM2 ( $\times$ ), and URIM1 ( $\diamond$ ).

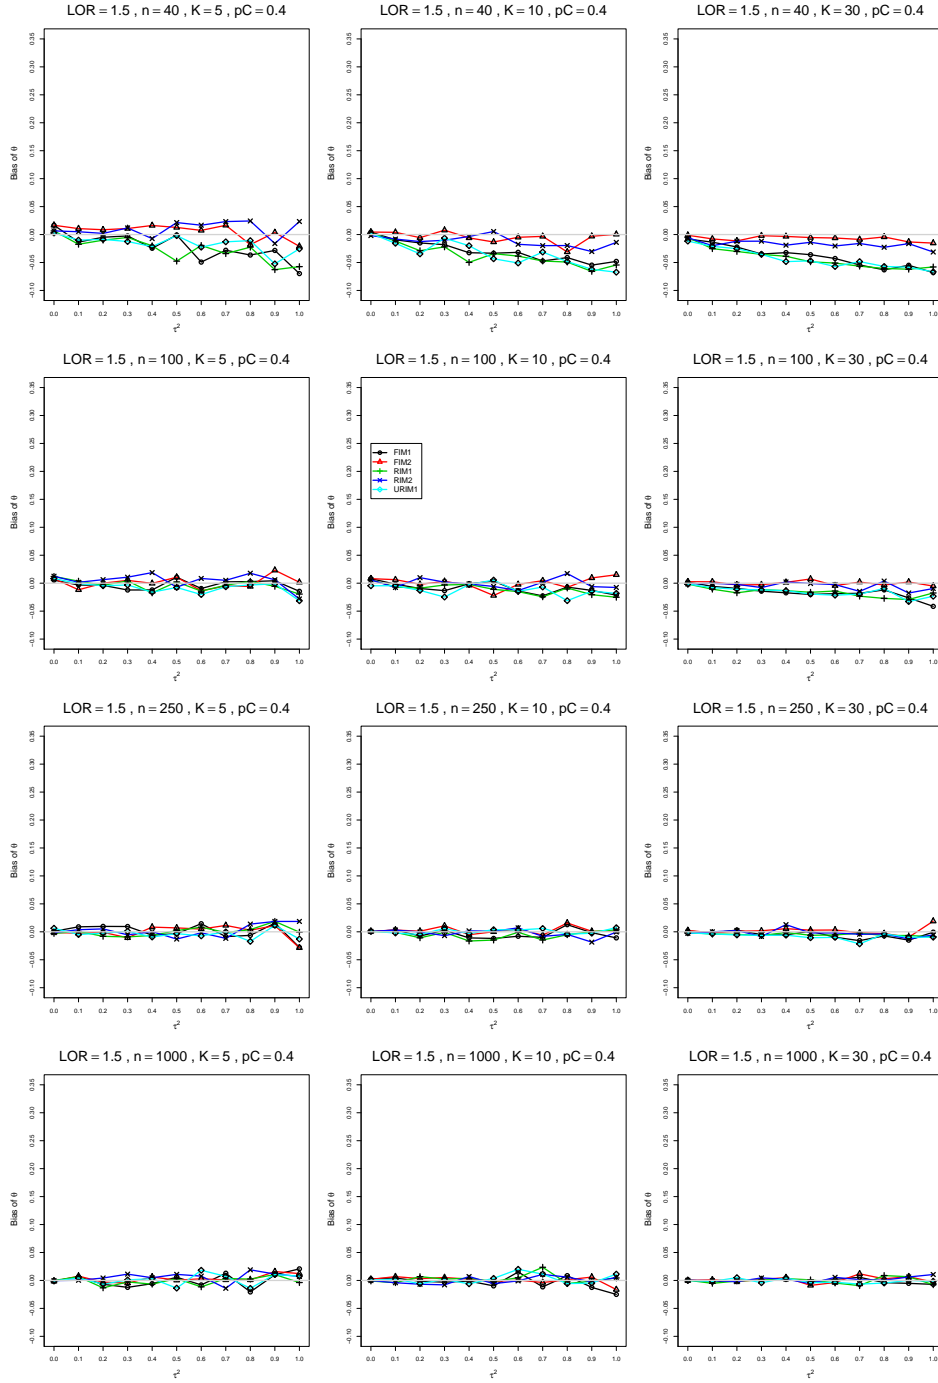

Figure A2.2.18: Bias of overall log-odds ratio  $\hat{\theta}_{REML}$  for  $\theta = 1.5$ ,  $p_C = 0.4$ ,  $\sigma^2 = 0.4$ , constant sample sizes  $n = 40, 100, 250, 1000$ . The data-generation mechanisms are FIM1 ( $\circ$ ), FIM2 ( $\triangle$ ), RIM1 ( $+$ ), RIM2 ( $\times$ ), and URIM1 ( $\diamond$ ).

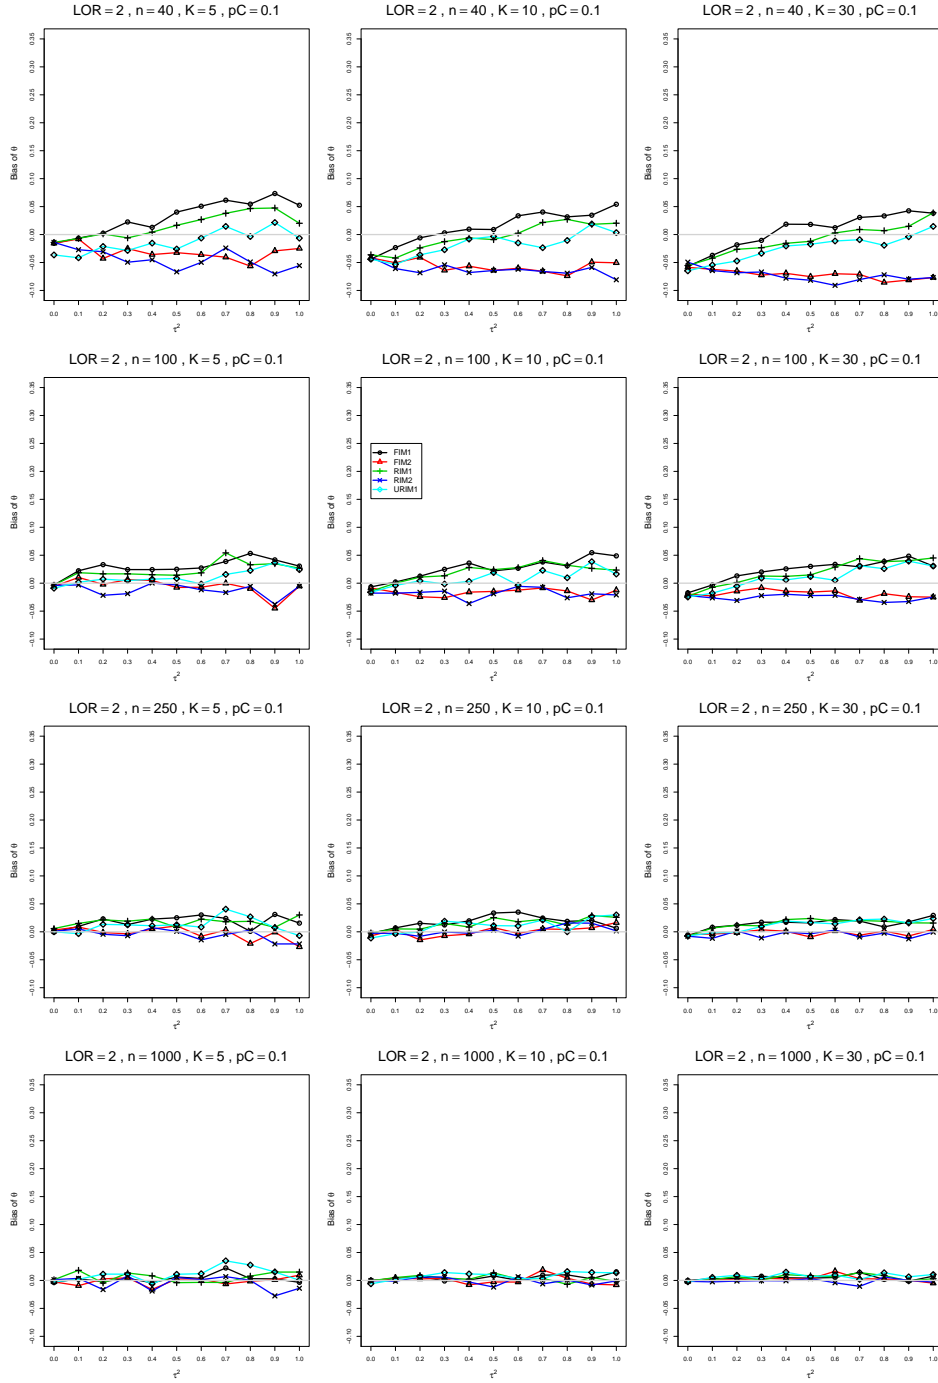

Figure A2.2.19: Bias of overall log-odds ratio  $\hat{\theta}_{REML}$  for  $\theta = 2$ ,  $p_C = 0.1$ ,  $\sigma^2 = 0.4$ , constant sample sizes  $n = 40, 100, 250, 1000$ . The data-generation mechanisms are FIM1 ( $\circ$ ), FIM2 ( $\triangle$ ), RIM1 ( $+$ ), RIM2 ( $\times$ ), and URIM1 ( $\diamond$ ).

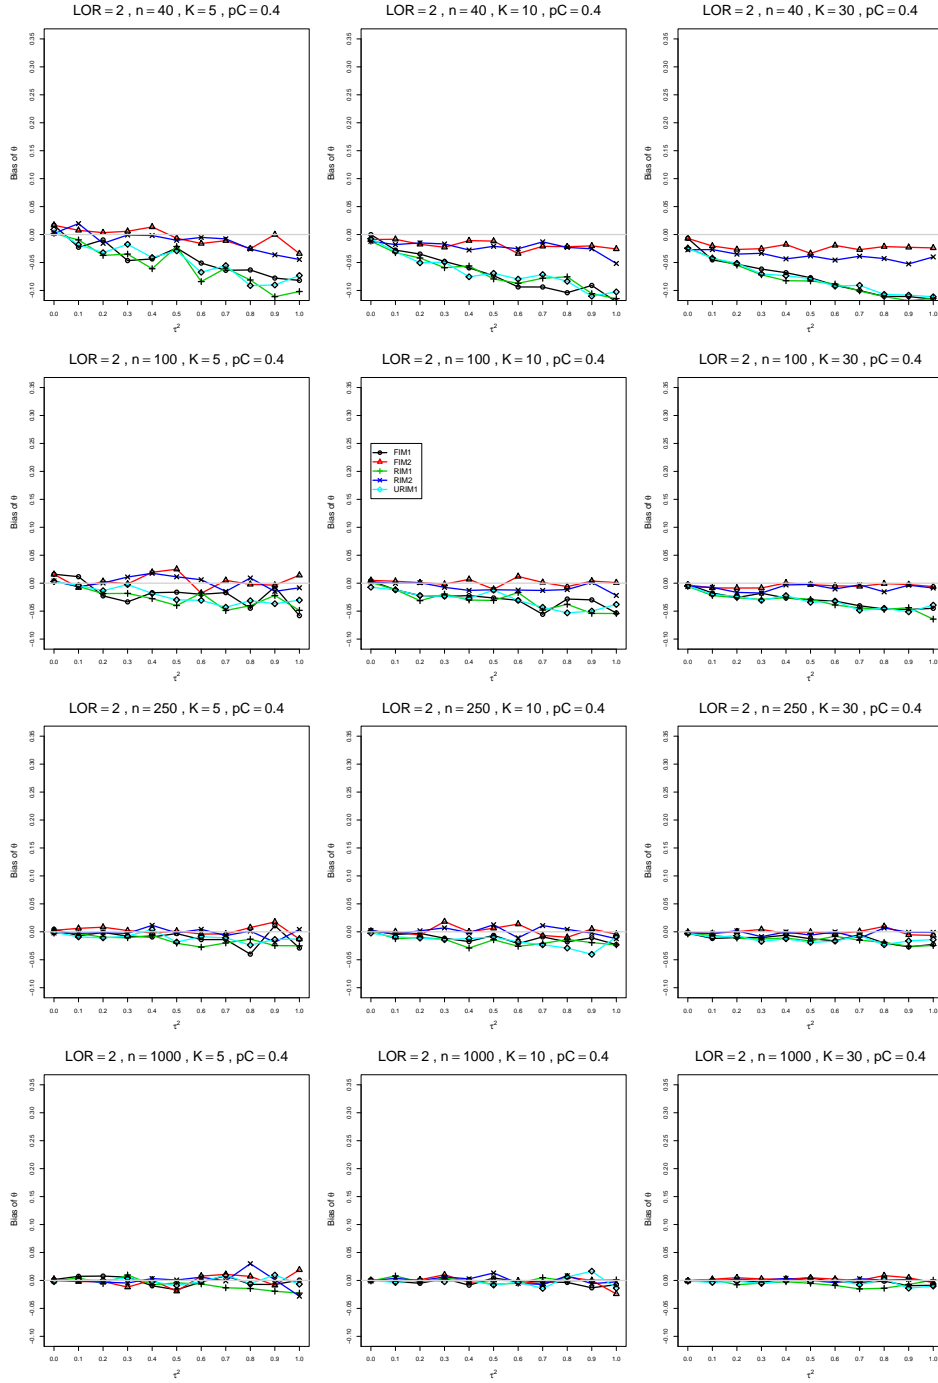

Figure A2.2.20: Bias of overall log-odds ratio  $\hat{\theta}_{REML}$  for  $\theta = 2$ ,  $p_C = 0.4$ ,  $\sigma^2 = 0.4$ , constant sample sizes  $n = 40, 100, 250, 1000$ . The data-generation mechanisms are FIM1 ( $\circ$ ), FIM2 ( $\triangle$ ), RIM1 ( $+$ ), RIM2 ( $\times$ ), and URIM1 ( $\diamond$ ).

### A2.3 Bias of $\hat{\theta}_{MP}$



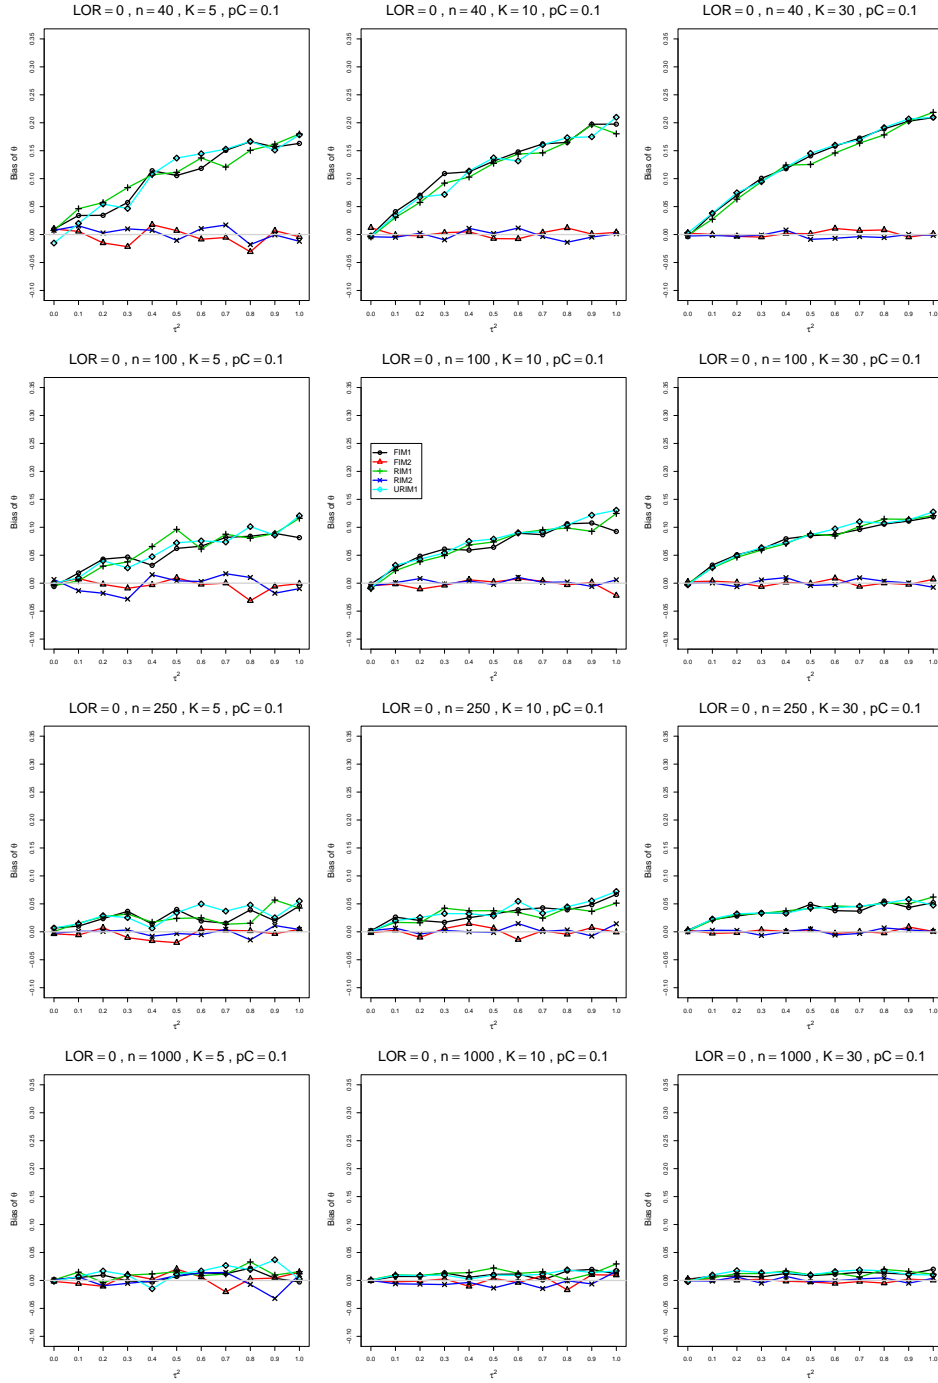

Figure A2.3.1: Bias of overall log-odds ratio  $\hat{\theta}_{MP}$  for  $\theta = 0$ ,  $p_C = 0.1$ ,  $\sigma^2 = 0.1$ , constant sample sizes  $n = 40, 100, 250, 1000$ . The data-generation mechanisms are FIM1 ( $\circ$ ), FIM2 ( $\triangle$ ), RIM1 ( $+$ ), RIM2 ( $\times$ ), and URIM1 ( $\diamond$ ).

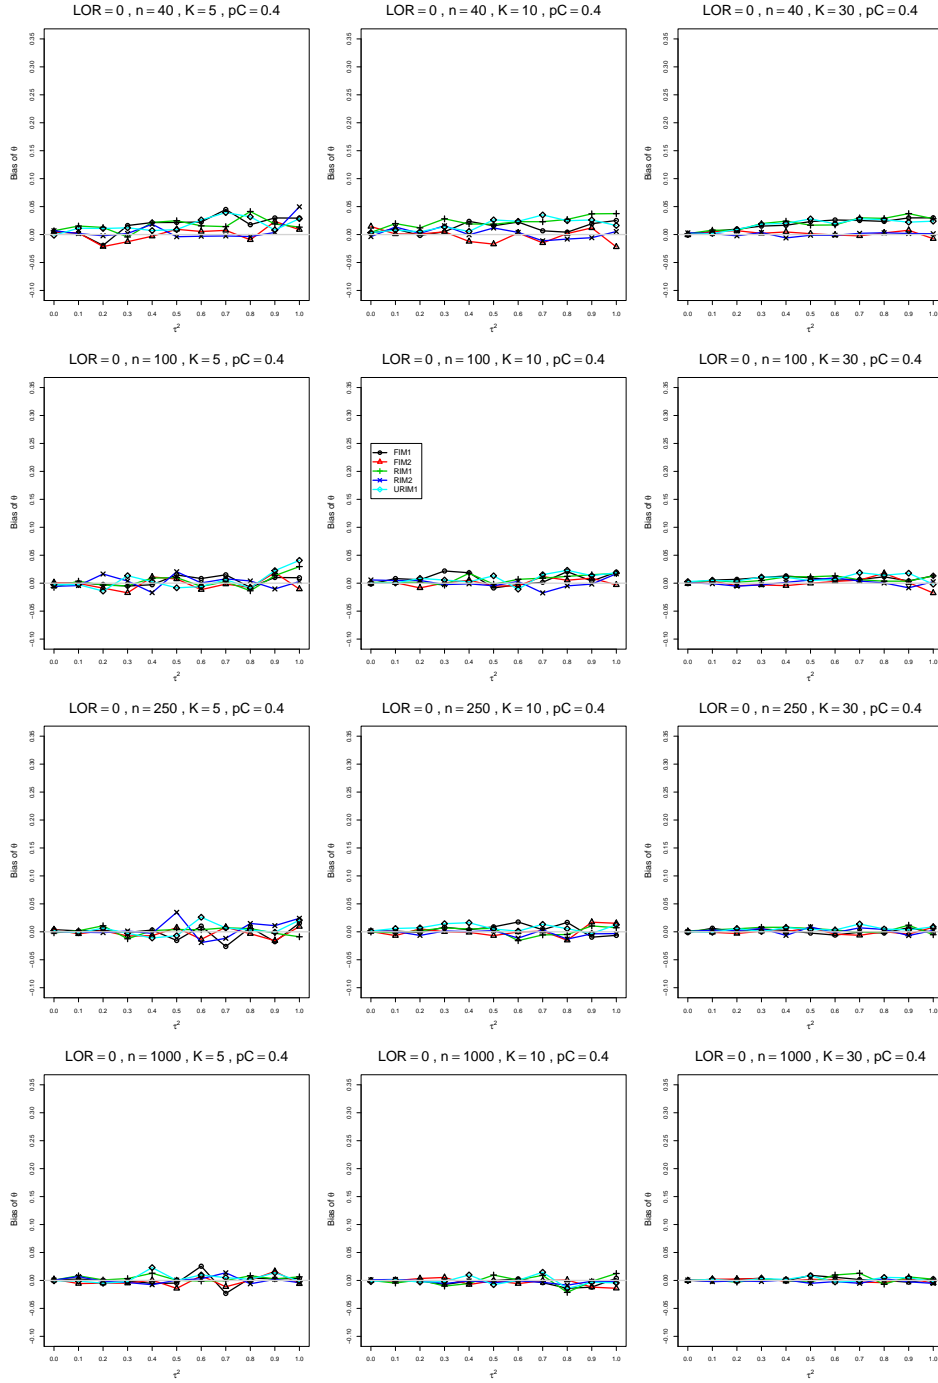

Figure A2.3.2: Bias of overall log-odds ratio  $\hat{\theta}_{MP}$  for  $\theta = 0$ ,  $p_C = 0.4$ ,  $\sigma^2 = 0.1$ , constant sample sizes  $n = 40, 100, 250, 1000$ . The data-generation mechanisms are FIM1 ( $\circ$ ), FIM2 ( $\triangle$ ), RIM1 ( $+$ ), RIM2 ( $\times$ ), and URIM1 ( $\diamond$ ).

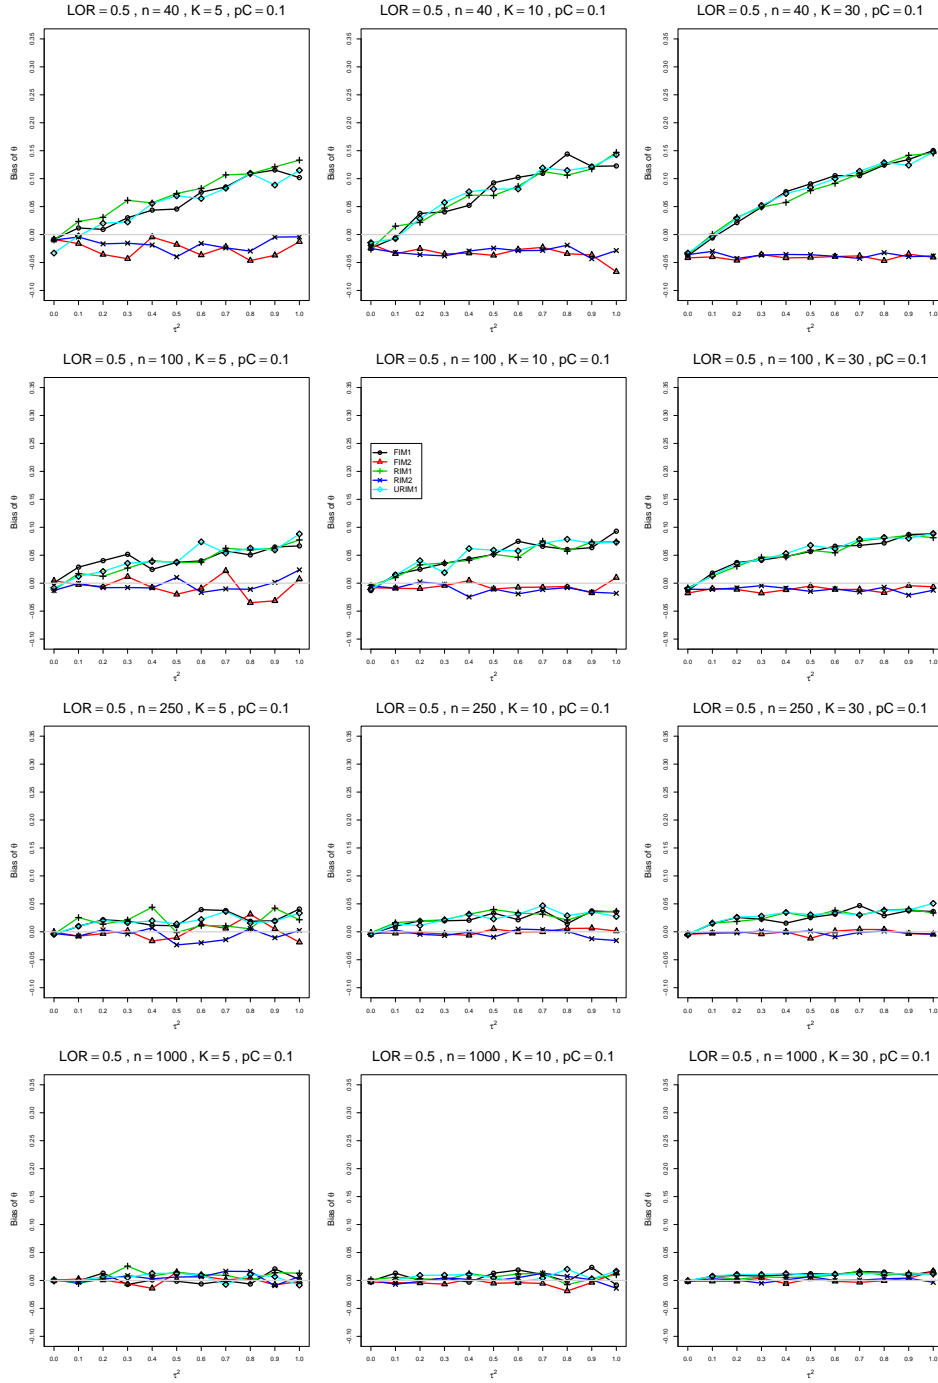

Figure A2.3.3: Bias of overall log-odds ratio  $\hat{\theta}_{MP}$  for  $\theta = 0.5$ ,  $p_C = 0.1$ ,  $\sigma^2 = 0.1$ , constant sample sizes  $n = 40, 100, 250, 1000$ . The data-generation mechanisms are FIM1 ( $\circ$ ), FIM2 ( $\triangle$ ), RIM1 ( $+$ ), RIM2 ( $\times$ ), and URIM1 ( $\diamond$ ).

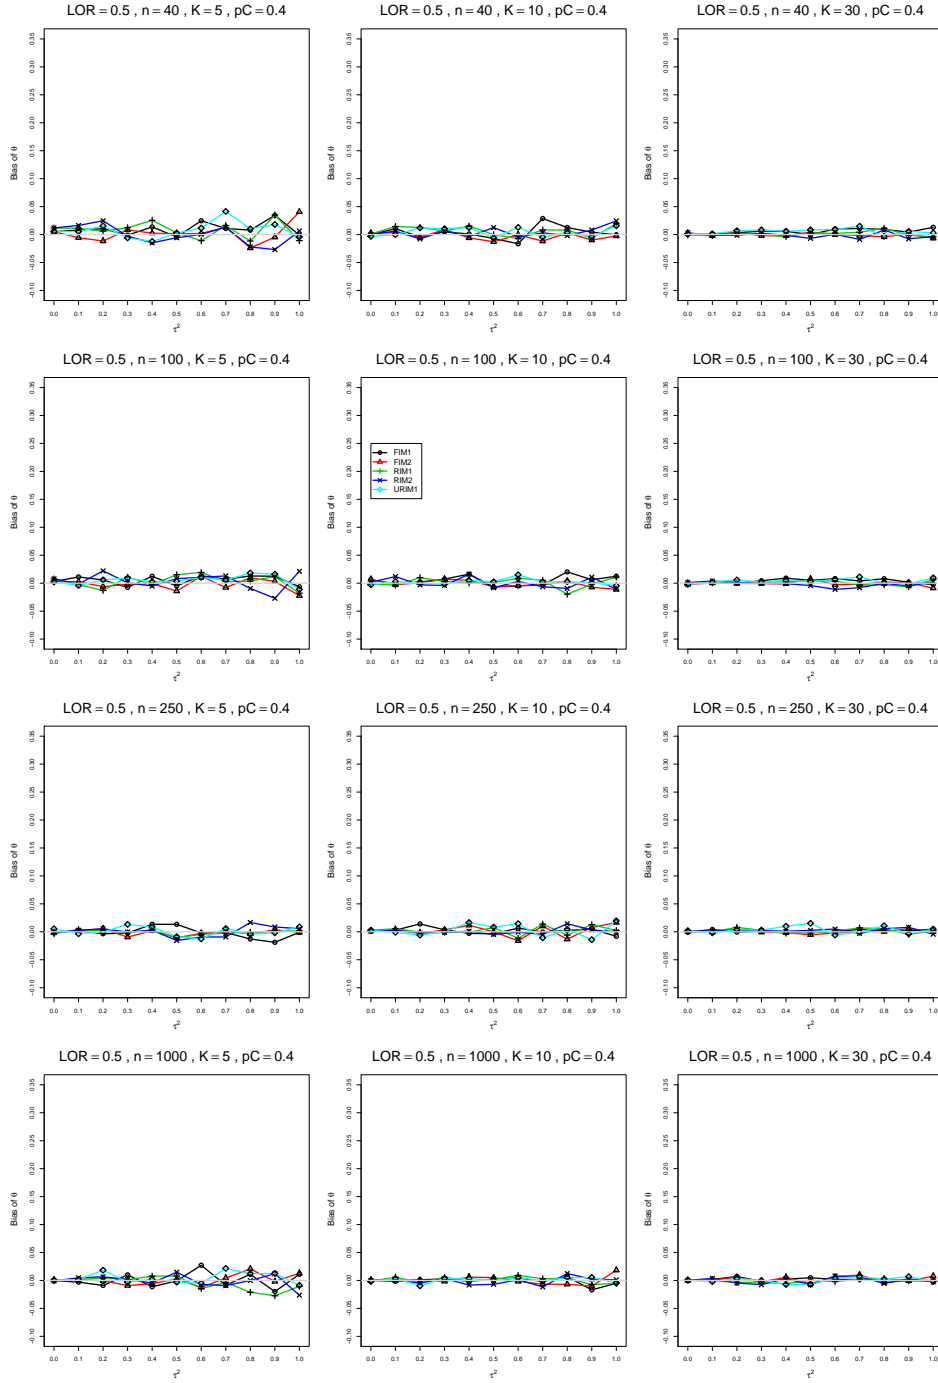

Figure A2.3.4: Bias of overall log-odds ratio  $\hat{\theta}_{MP}$  for  $\theta = 0.5$ ,  $p_C = 0.4$ ,  $\sigma^2 = 0.1$ , constant sample sizes  $n = 40, 100, 250, 1000$ . The data-generation mechanisms are FIM1 ( $\circ$ ), FIM2 ( $\triangle$ ), RIM1 ( $+$ ), RIM2 ( $\times$ ), and URIM1 ( $\diamond$ ).

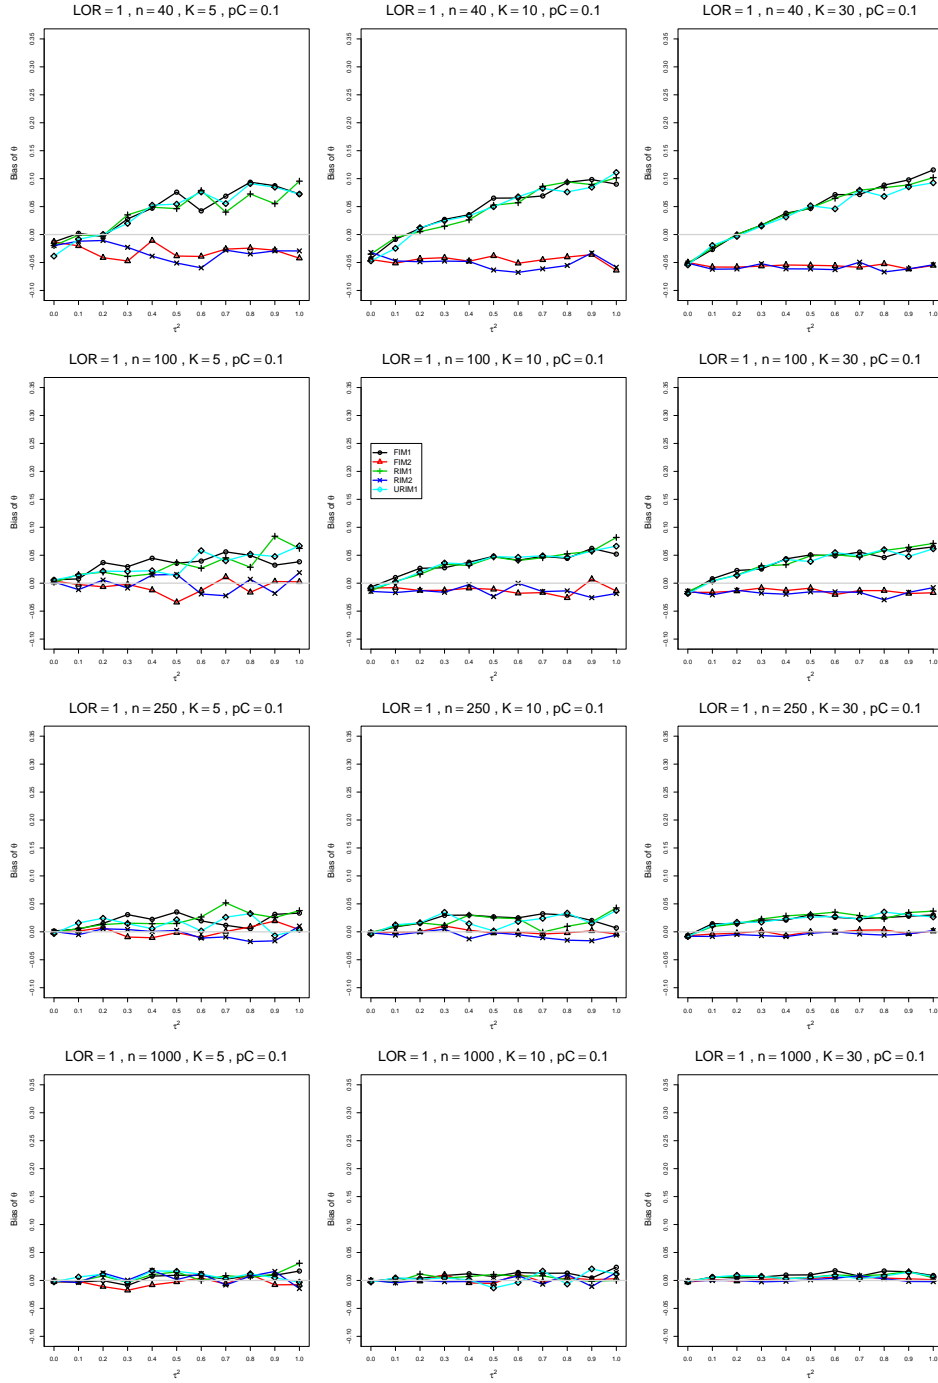

Figure A2.3.5: Bias of overall log-odds ratio  $\hat{\theta}_{MP}$  for  $\theta = 1$ ,  $p_C = 0.1$ ,  $\sigma^2 = 0.1$ , constant sample sizes  $n = 40, 100, 250, 1000$ . The data-generation mechanisms are FIM1 ( $\circ$ ), FIM2 ( $\triangle$ ), RIM1 ( $+$ ), RIM2 ( $\times$ ), and URIM1 ( $\diamond$ ).

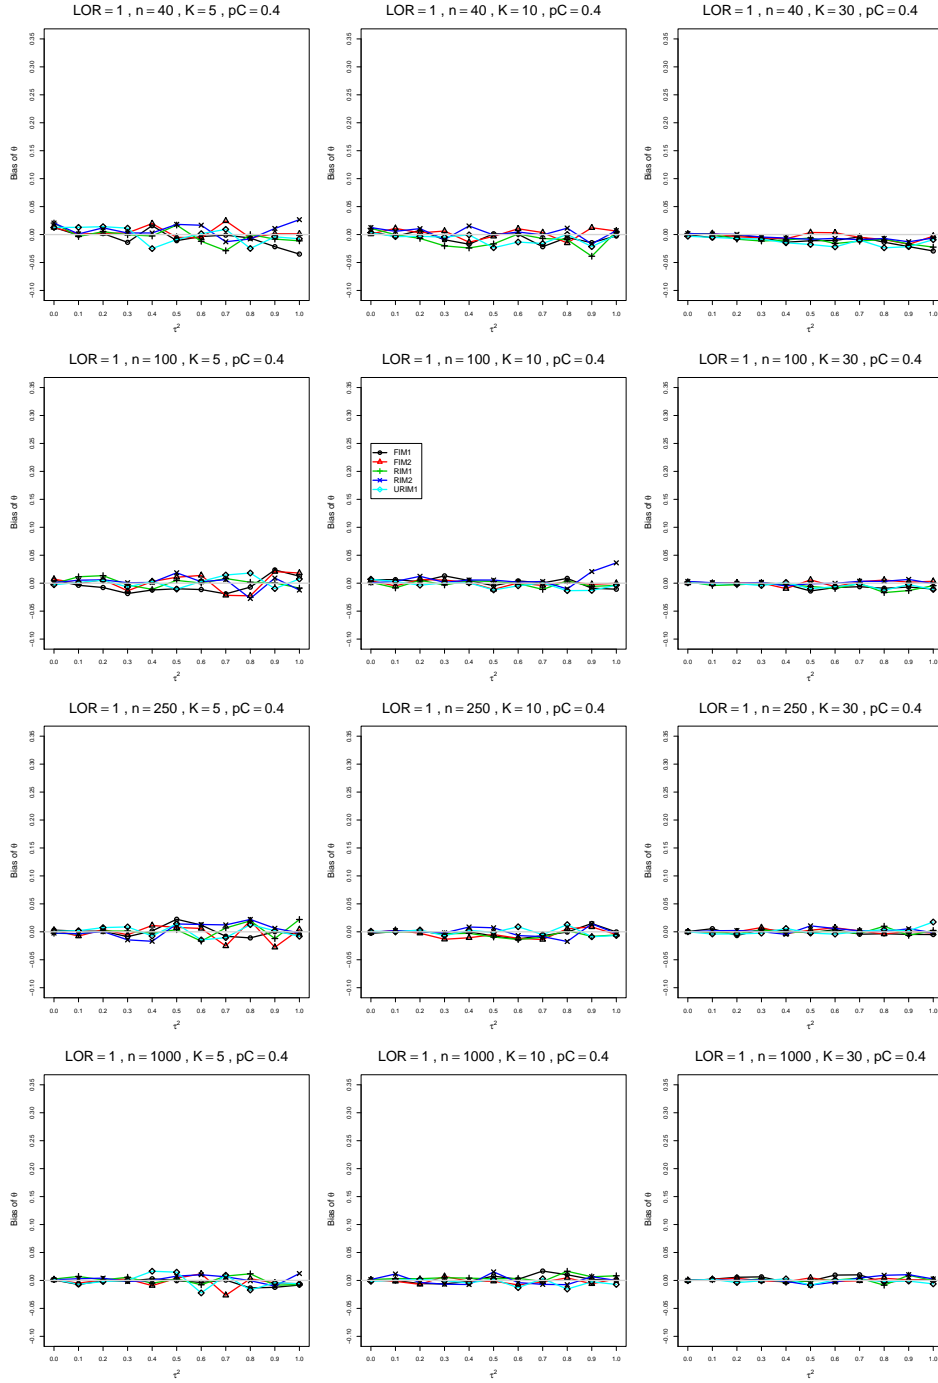

Figure A2.3.6: Bias of overall log-odds ratio  $\hat{\theta}_{MP}$  for  $\theta = 1$ ,  $p_C = 0.4$ ,  $\sigma^2 = 0.1$ , constant sample sizes  $n = 40, 100, 250, 1000$ . The data-generation mechanisms are FIM1 ( $\circ$ ), FIM2 ( $\triangle$ ), RIM1 ( $+$ ), RIM2 ( $\times$ ), and URIM1 ( $\diamond$ ).

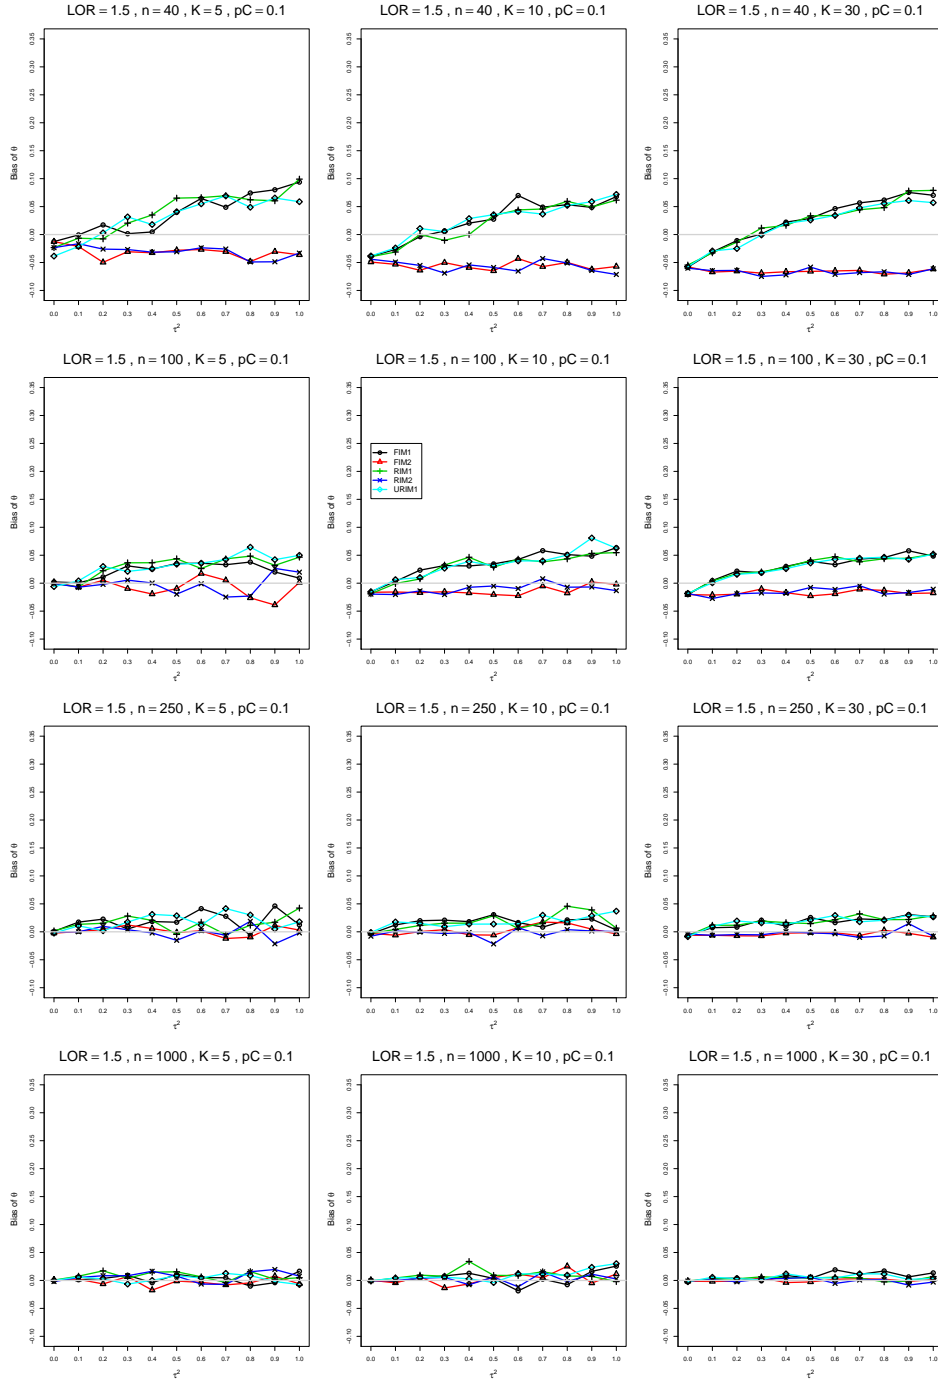

Figure A2.3.7: Bias of overall log-odds ratio  $\hat{\theta}_{MP}$  for  $\theta = 1.5$ ,  $p_C = 0.1$ ,  $\sigma^2 = 0.1$ , constant sample sizes  $n = 40, 100, 250, 1000$ . The data-generation mechanisms are FIM1 ( $\circ$ ), FIM2 ( $\triangle$ ), RIM1 ( $+$ ), RIM2 ( $\times$ ), and URIM1 ( $\diamond$ ).

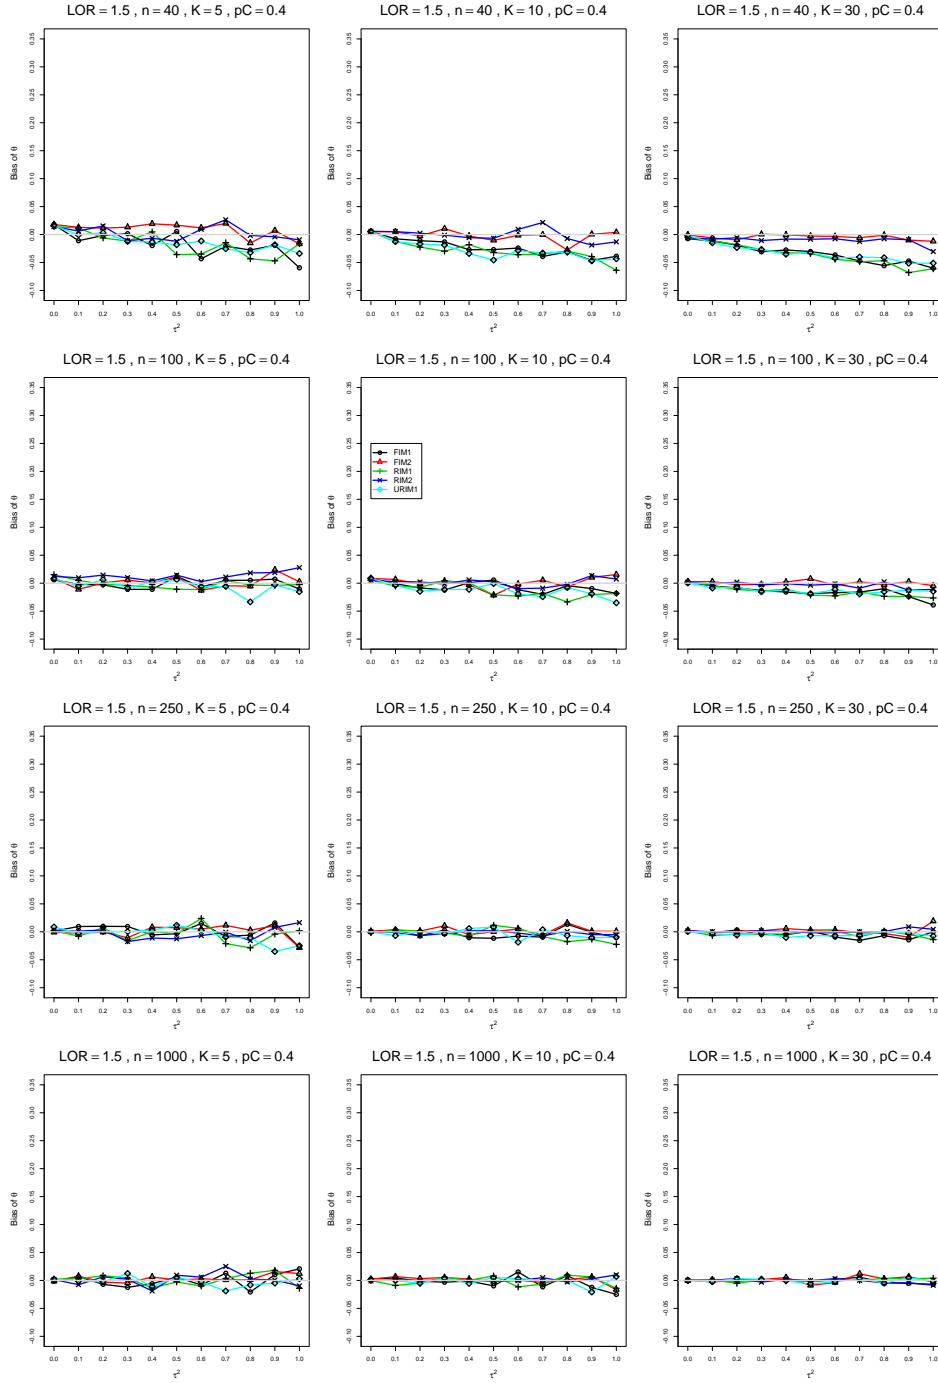

Figure A2.3.8: Bias of overall log-odds ratio  $\hat{\theta}_{MP}$  for  $\theta = 1.5$ ,  $p_C = 0.4$ ,  $\sigma^2 = 0.1$ , constant sample sizes  $n = 40, 100, 250, 1000$ . The data-generation mechanisms are FIM1 ( $\circ$ ), FIM2 ( $\triangle$ ), RIM1 ( $+$ ), RIM2 ( $\times$ ), and URIM1 ( $\diamond$ ).



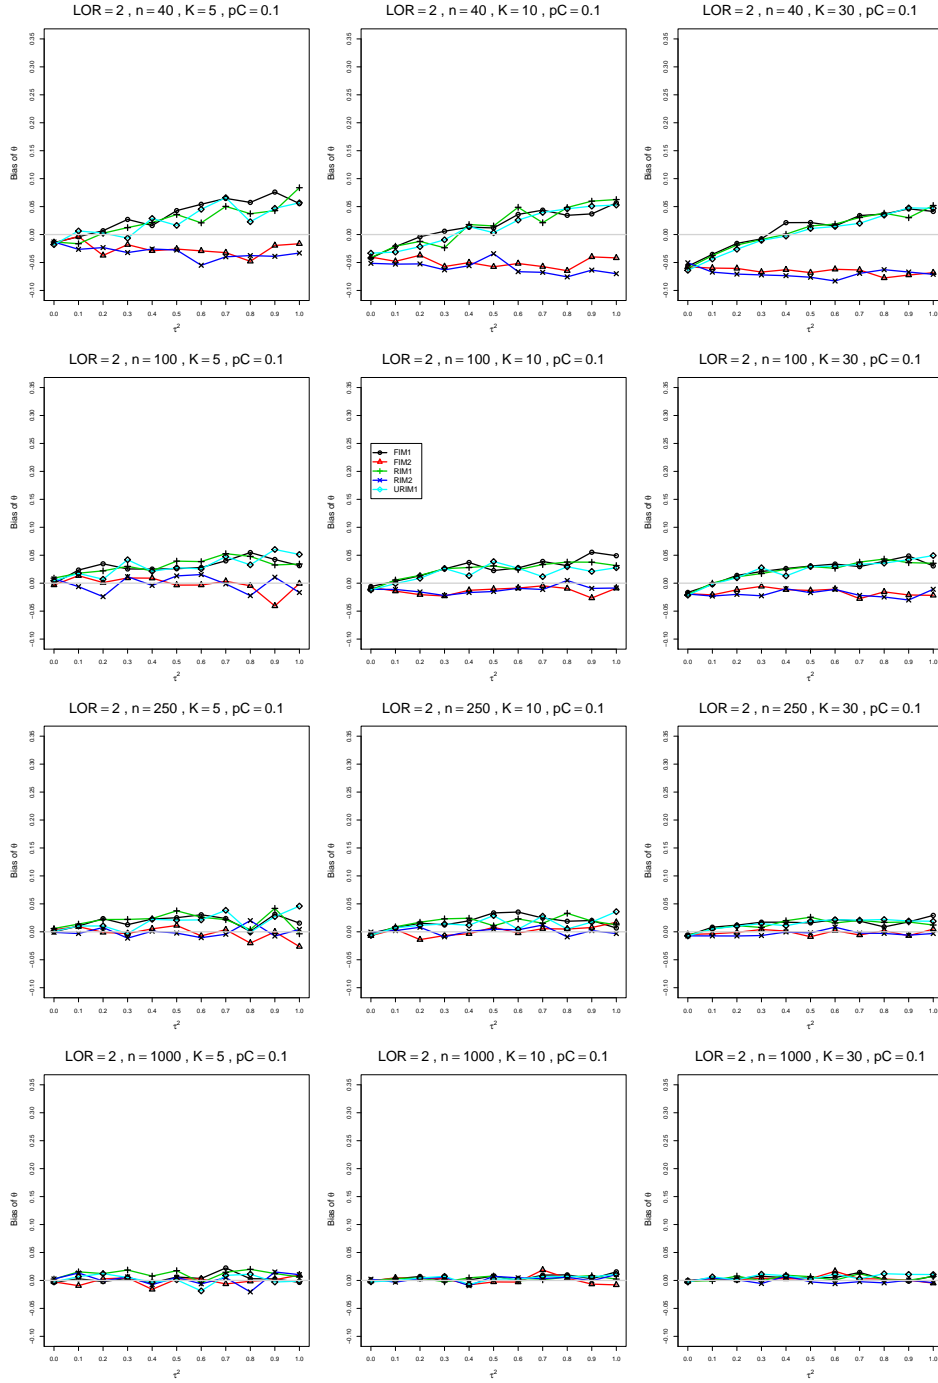

Figure A2.3.9: Bias of overall log-odds ratio  $\hat{\theta}_{MP}$  for  $\theta = 2$ ,  $p_C = 0.1$ ,  $\sigma^2 = 0.1$ , constant sample sizes  $n = 40, 100, 250, 1000$ . The data-generation mechanisms are FIM1 ( $\circ$ ), FIM2 ( $\triangle$ ), RIM1 ( $+$ ), RIM2 ( $\times$ ), and URIM1 ( $\diamond$ ).

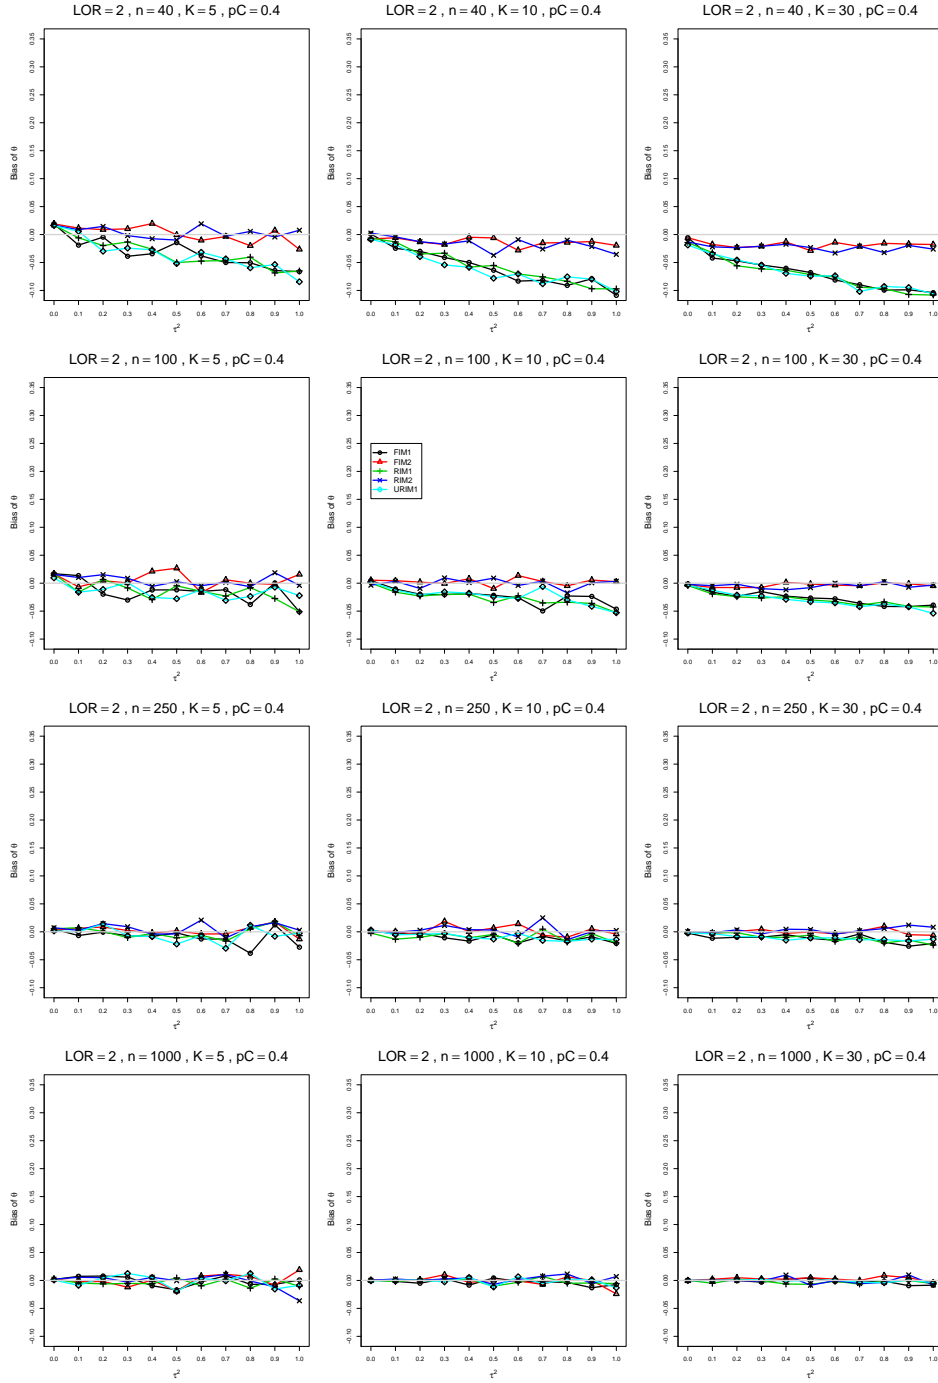

Figure A2.3.10: Bias of overall log-odds ratio  $\hat{\theta}_{MP}$  for  $\theta = 2$ ,  $p_C = 0.4$ ,  $\sigma^2 = 0.1$ , constant sample sizes  $n = 40, 100, 250, 1000$ . The data-generation mechanisms are FIM1 ( $\circ$ ), FIM2 ( $\triangle$ ), RIM1 ( $+$ ), RIM2 ( $\times$ ), and URIM1 ( $\diamond$ ).

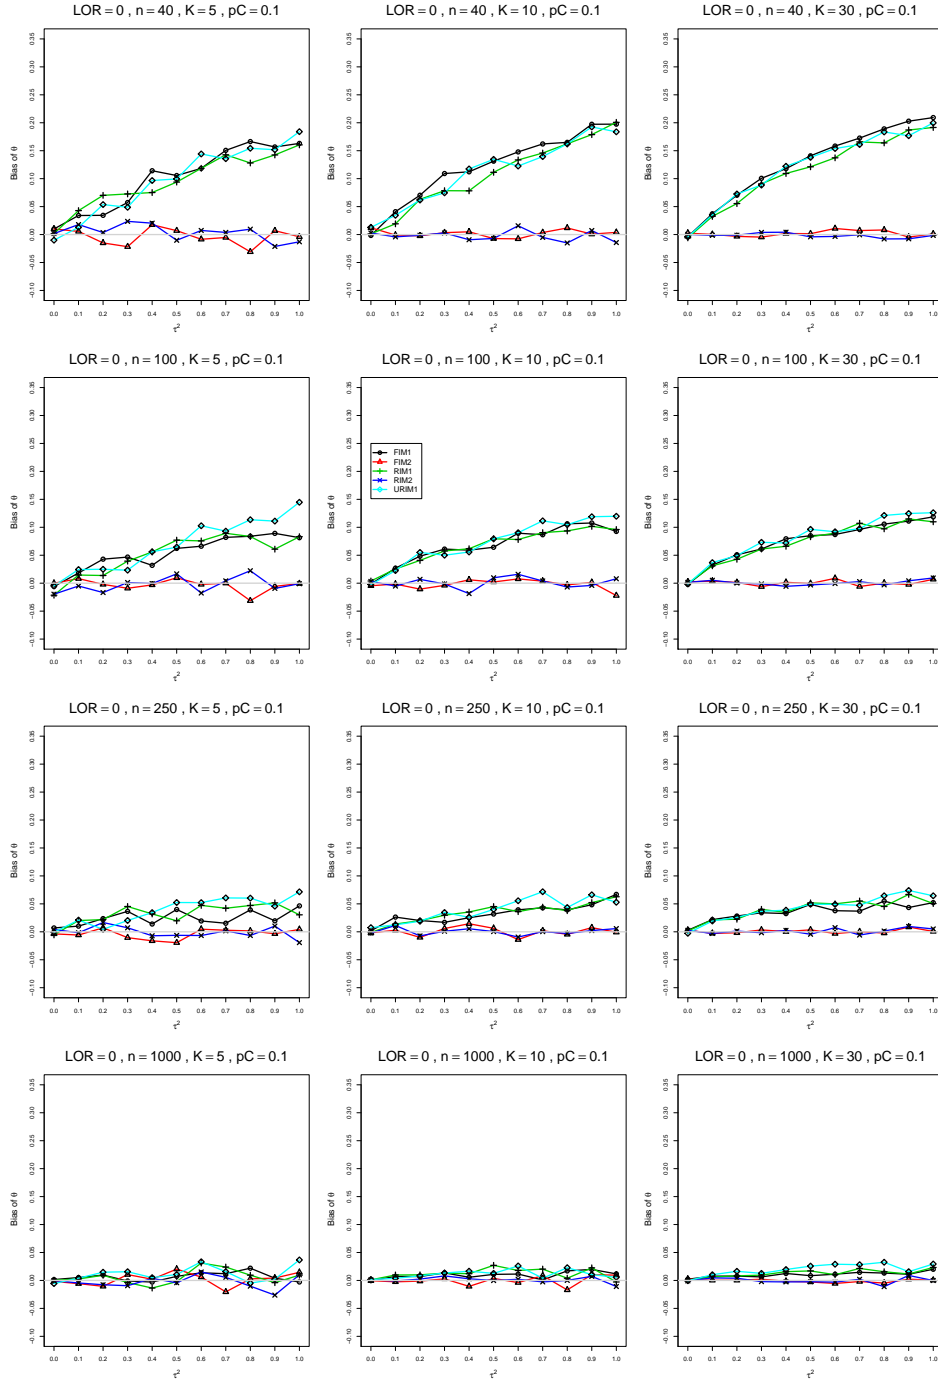

Figure A2.3.11: Bias of overall log-odds ratio  $\hat{\theta}_{MP}$  for  $\theta = 0$ ,  $p_C = 0.1$ ,  $\sigma^2 = 0.4$ , constant sample sizes  $n = 40, 100, 250, 1000$ . The data-generation mechanisms are FIM1 ( $\circ$ ), FIM2 ( $\triangle$ ), RIM1 ( $+$ ), RIM2 ( $\times$ ), and URIM1 ( $\diamond$ ).

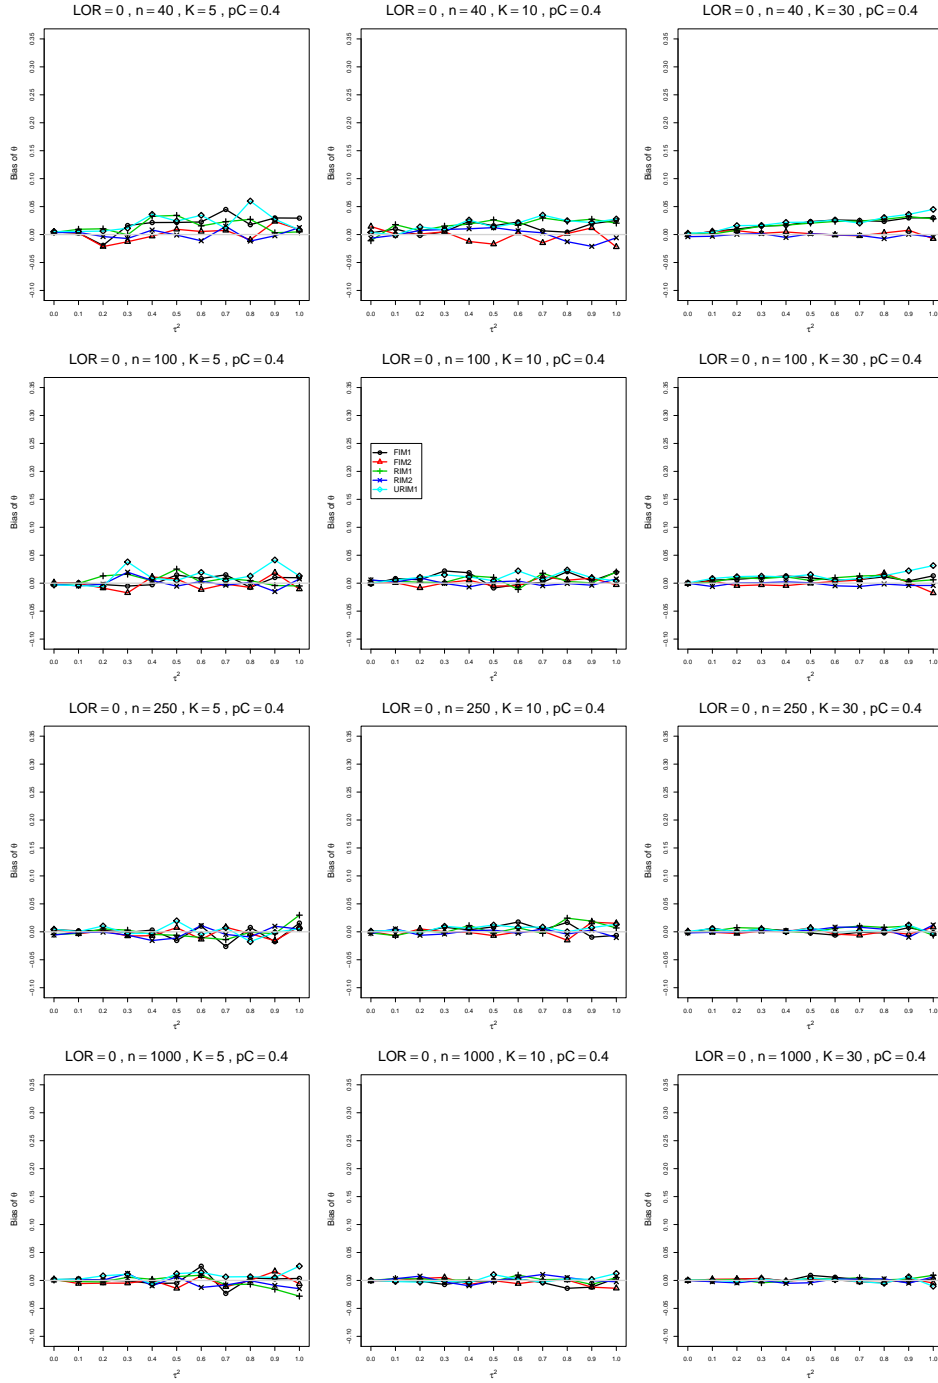

Figure A2.3.12: Bias of overall log-odds ratio  $\hat{\theta}_{MP}$  for  $\theta = 0$ ,  $p_C = 0.4$ ,  $\sigma^2 = 0.4$ , constant sample sizes  $n = 40, 100, 250, 1000$ . The data-generation mechanisms are FIM1 ( $\circ$ ), FIM2 ( $\triangle$ ), RIM1 ( $+$ ), RIM2 ( $\times$ ), and URIM1 ( $\diamond$ ).

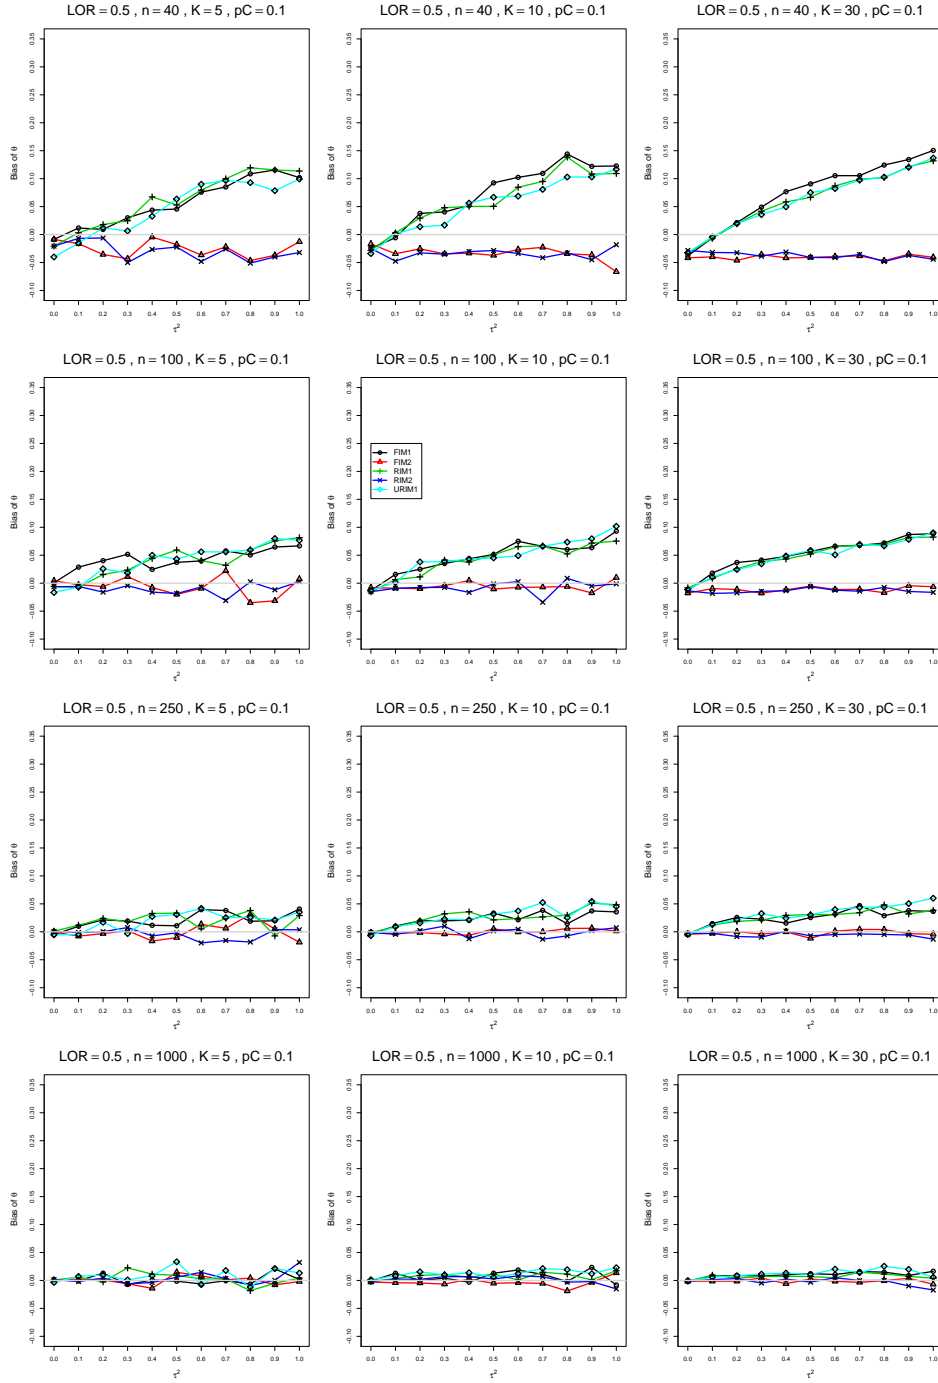

Figure A2.3.13: Bias of overall log-odds ratio  $\hat{\theta}_{MP}$  for  $\theta = 0.5$ ,  $p_C = 0.1$ ,  $\sigma^2 = 0.4$ , constant sample sizes  $n = 40, 100, 250, 1000$ . The data-generation mechanisms are FIM1 ( $\circ$ ), FIM2 ( $\triangle$ ), RIM1 ( $+$ ), RIM2 ( $\times$ ), and URIM1 ( $\diamond$ ).

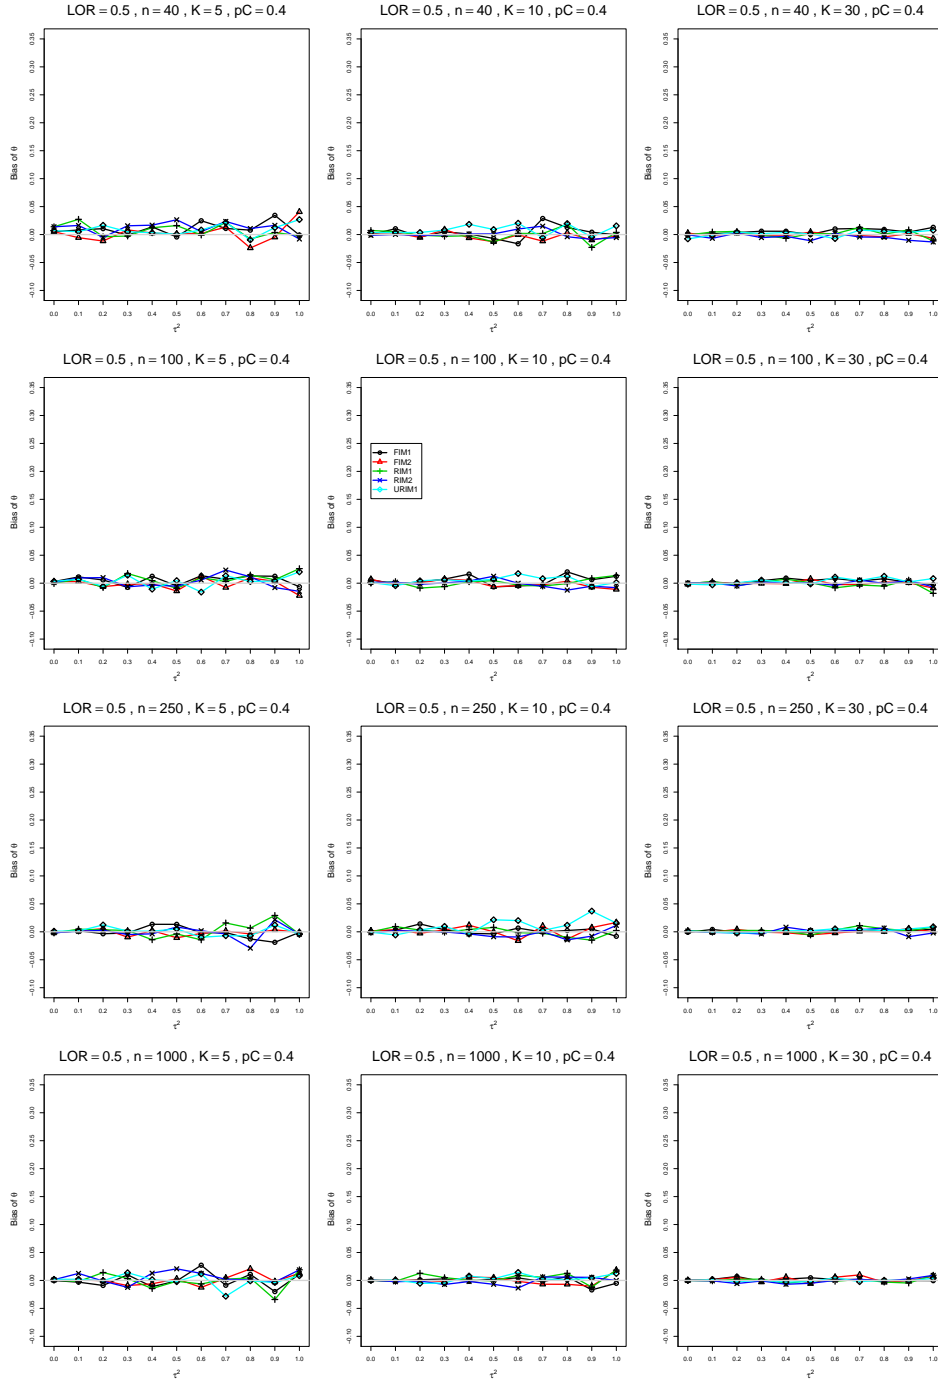

Figure A2.3.14: Bias of overall log-odds ratio  $\hat{\theta}_{MP}$  for  $\theta = 0.5$ ,  $p_C = 0.4$ ,  $\sigma^2 = 0.4$ , constant sample sizes  $n = 40, 100, 250, 1000$ . The data-generation mechanisms are FIM1 ( $\circ$ ), FIM2 ( $\triangle$ ), RIM1 ( $+$ ), RIM2 ( $\times$ ), and URIM1 ( $\diamond$ ).

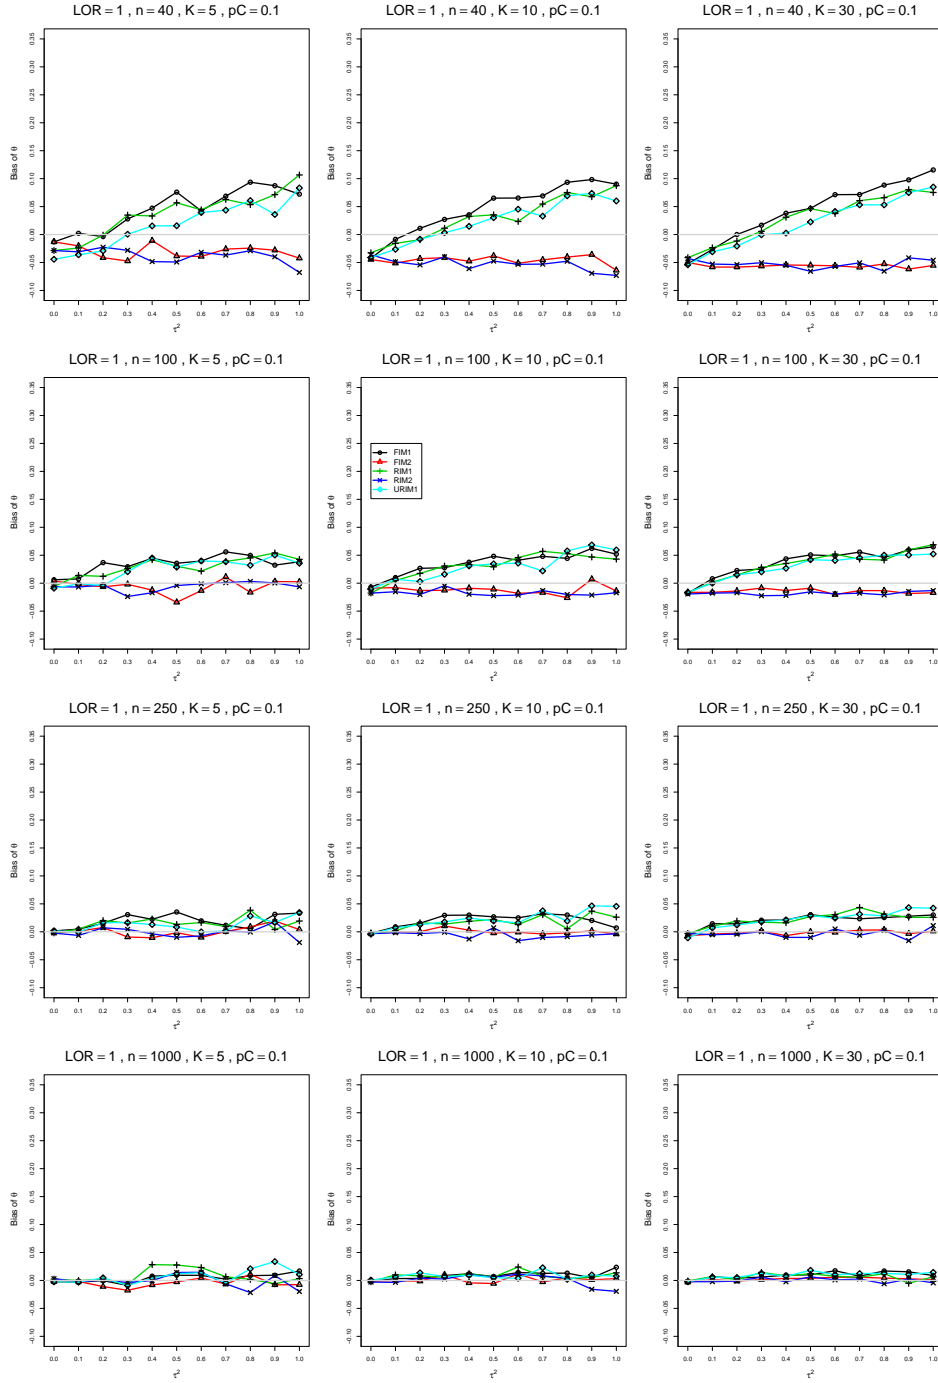

Figure A2.3.15: Bias of overall log-odds ratio  $\hat{\theta}_{MP}$  for  $\theta = 1$ ,  $p_C = 0.1$ ,  $\sigma^2 = 0.4$ , constant sample sizes  $n = 40, 100, 250, 1000$ . The data-generation mechanisms are FIM1 ( $\circ$ ), FIM2 ( $\triangle$ ), RIM1 ( $+$ ), RIM2 ( $\times$ ), and URIM1 ( $\diamond$ ).

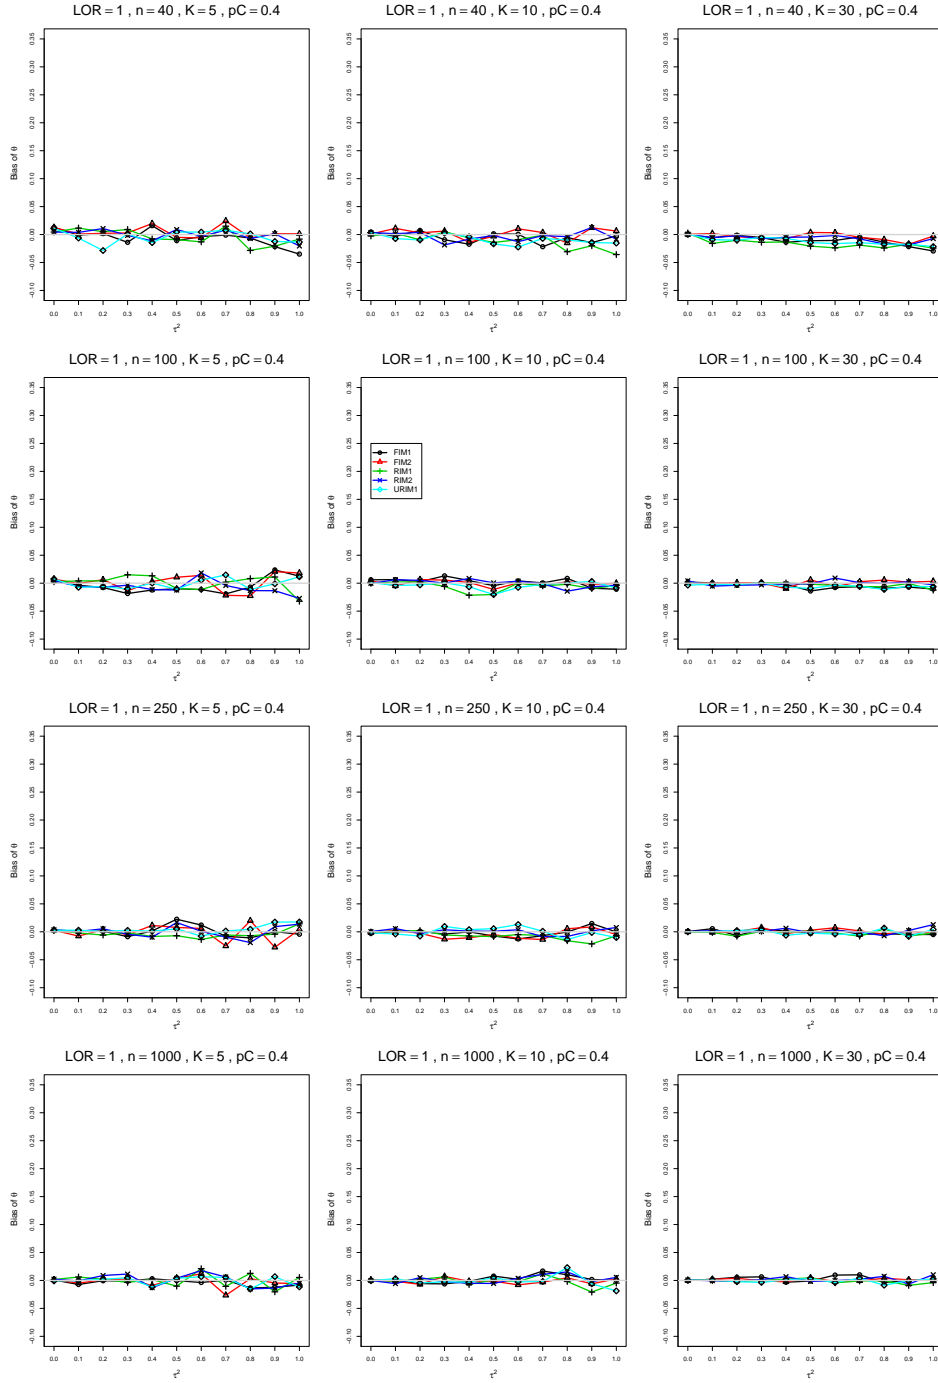

Figure A2.3.16: Bias of overall log-odds ratio  $\hat{\theta}_{MP}$  for  $\theta = 1$ ,  $p_C = 0.4$ ,  $\sigma^2 = 0.4$ , constant sample sizes  $n = 40, 100, 250, 1000$ . The data-generation mechanisms are FIM1 ( $\circ$ ), FIM2 ( $\triangle$ ), RIM1 ( $+$ ), RIM2 ( $\times$ ), and URIM1 ( $\diamond$ ).



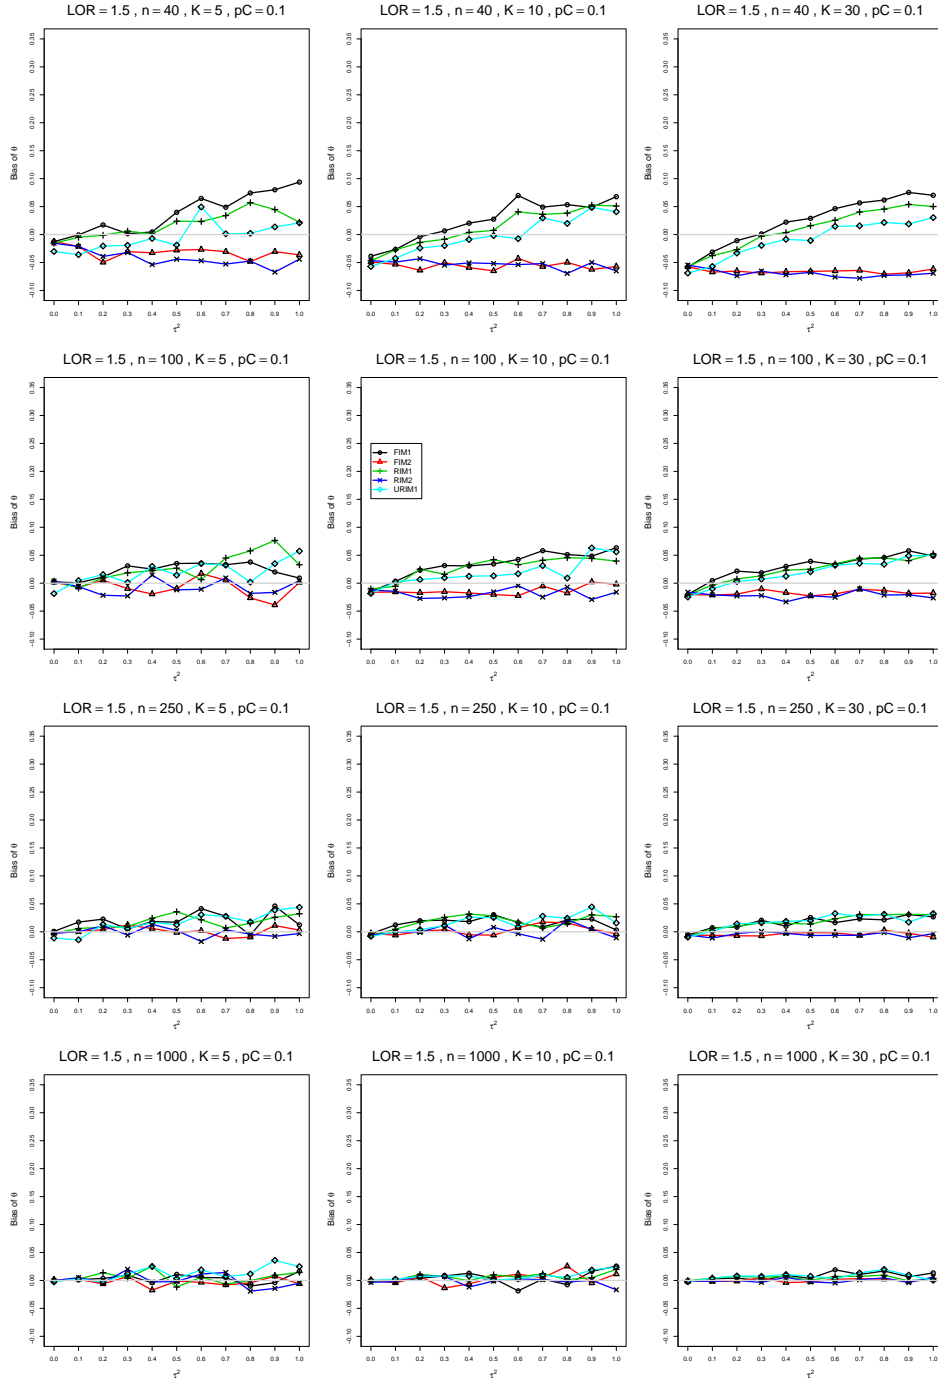

Figure A2.3.17: Bias of overall log-odds ratio  $\hat{\theta}_{MP}$  for  $\theta = 1.5$ ,  $p_C = 0.1$ ,  $\sigma^2 = 0.4$ , constant sample sizes  $n = 40, 100, 250, 1000$ . The data-generation mechanisms are FIM1 ( $\circ$ ), FIM2 ( $\triangle$ ), RIM1 ( $+$ ), RIM2 ( $\times$ ), and URIM1 ( $\diamond$ ).

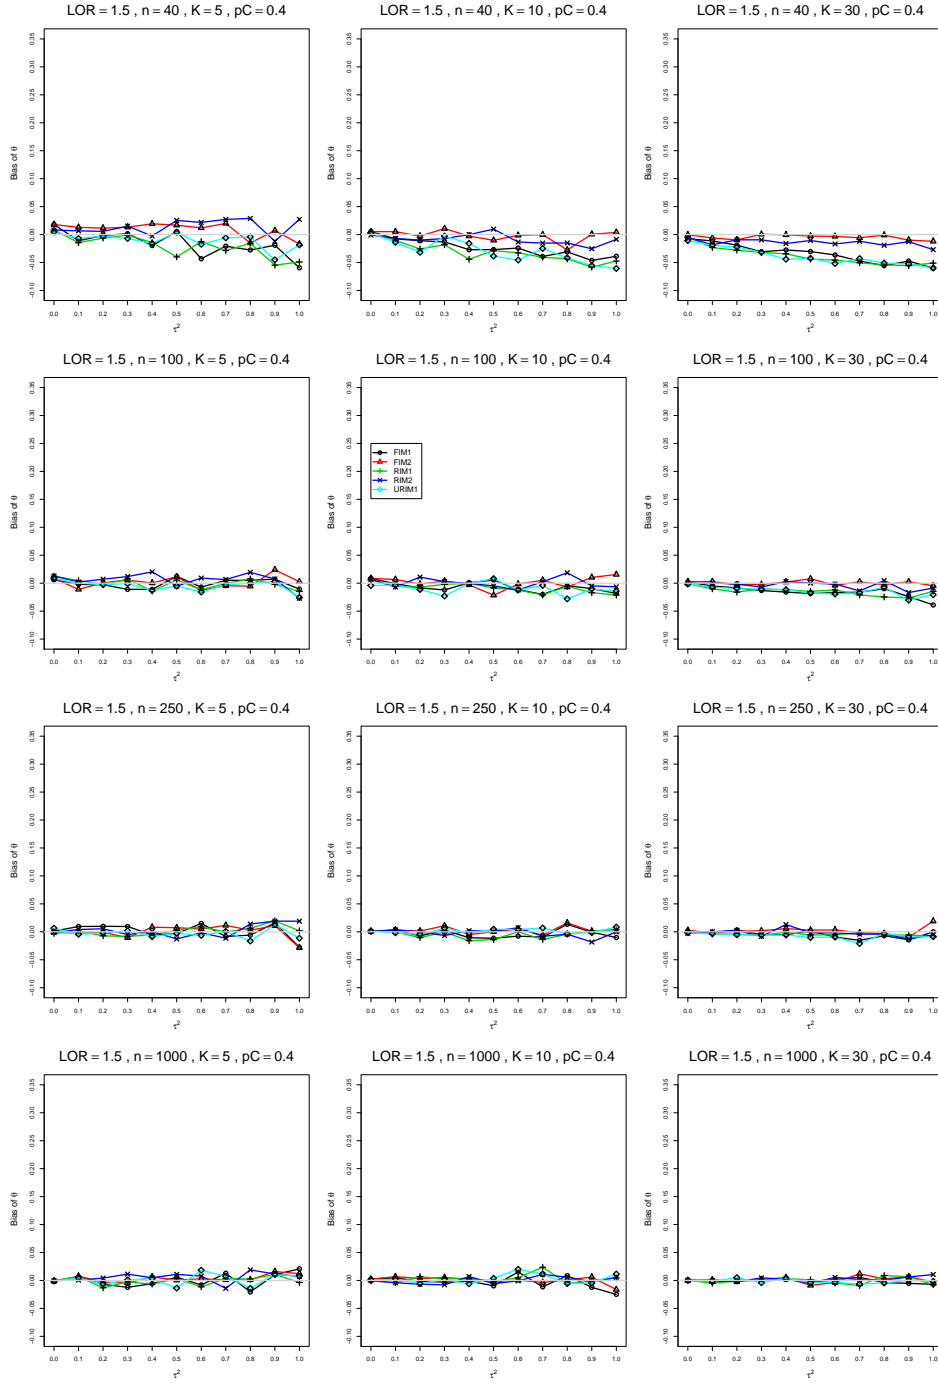

Figure A2.3.18: Bias of overall log-odds ratio  $\hat{\theta}_{MP}$  for  $\theta = 1.5$ ,  $p_C = 0.4$ ,  $\sigma^2 = 0.4$ , constant sample sizes  $n = 40, 100, 250, 1000$ . The data-generation mechanisms are FIM1 ( $\circ$ ), FIM2 ( $\triangle$ ), RIM1 ( $+$ ), RIM2 ( $\times$ ), and URIM1 ( $\diamond$ ).

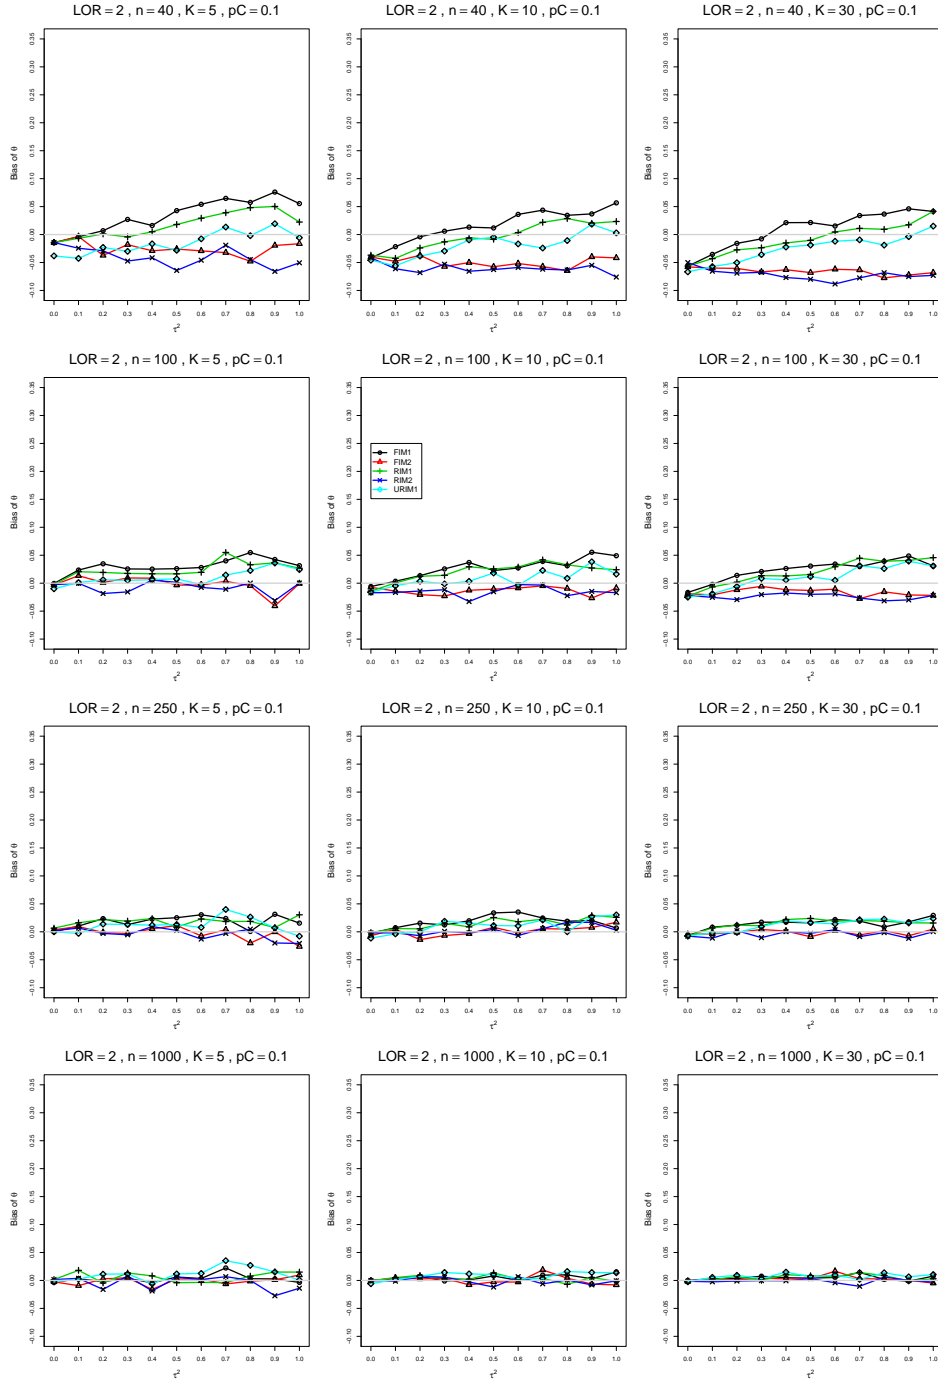

Figure A2.3.19: Bias of overall log-odds ratio  $\hat{\theta}_{MP}$  for  $\theta = 2$ ,  $p_C = 0.1$ ,  $\sigma^2 = 0.4$ , constant sample sizes  $n = 40, 100, 250, 1000$ . The data-generation mechanisms are FIM1 ( $\circ$ ), FIM2 ( $\triangle$ ), RIM1 ( $+$ ), RIM2 ( $\times$ ), and URIM1 ( $\diamond$ ).

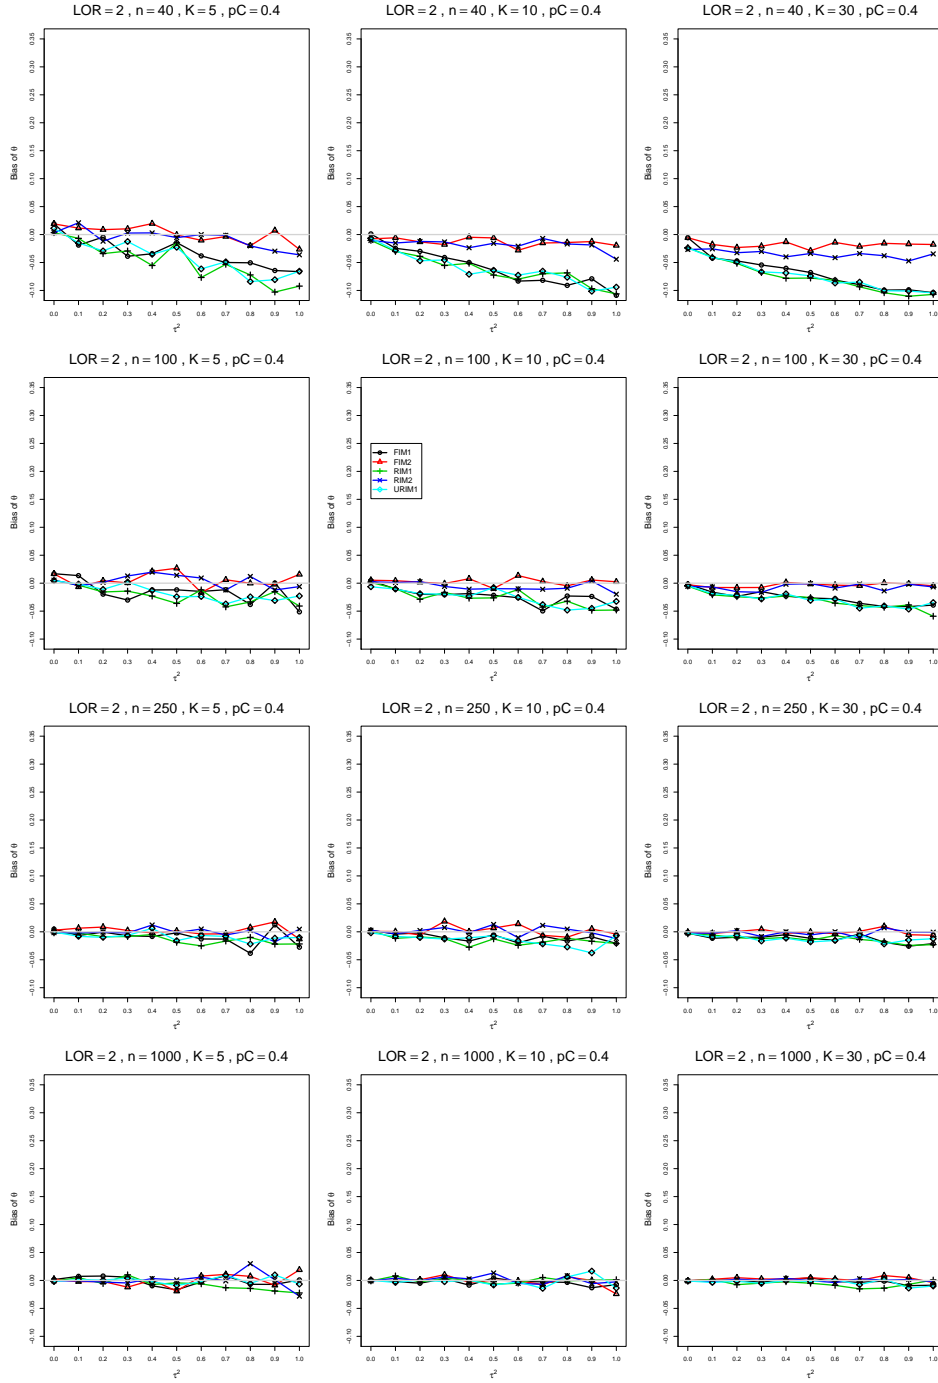

Figure A2.3.20: Bias of overall log-odds ratio  $\hat{\theta}_{MP}$  for  $\theta = 2$ ,  $p_C = 0.4$ ,  $\sigma^2 = 0.4$ , constant sample sizes  $n = 40, 100, 250, 1000$ . The data-generation mechanisms are FIM1 ( $\circ$ ), FIM2 ( $\triangle$ ), RIM1 ( $+$ ), RIM2 ( $\times$ ), and URIM1 ( $\diamond$ ).

#### A2.4 Bias of $\hat{\theta}_{KD}$

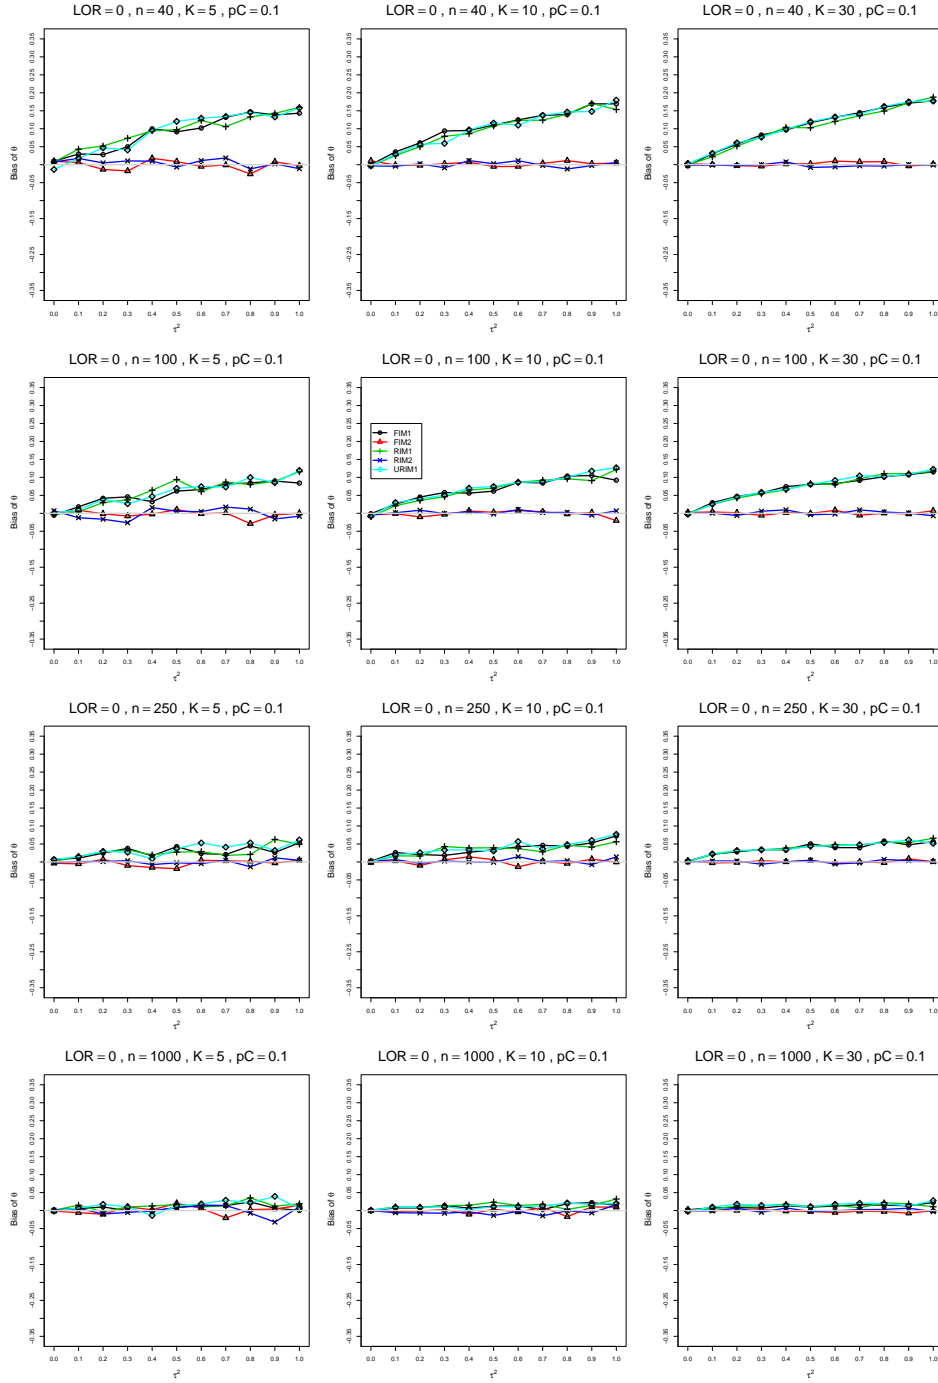

Figure A2.4.1: Bias of overall log-odds ratio  $\hat{\theta}_{KD}$  for  $\theta = 0$ ,  $p_C = 0.1$ ,  $\sigma^2 = 0.1$ , constant sample sizes  $n = 40, 100, 250, 1000$ . The data-generation mechanisms are FIM1 ( $\circ$ ), FIM2 ( $\triangle$ ), RIM1 ( $+$ ), RIM2 ( $\times$ ), and URIM1 ( $\diamond$ ).

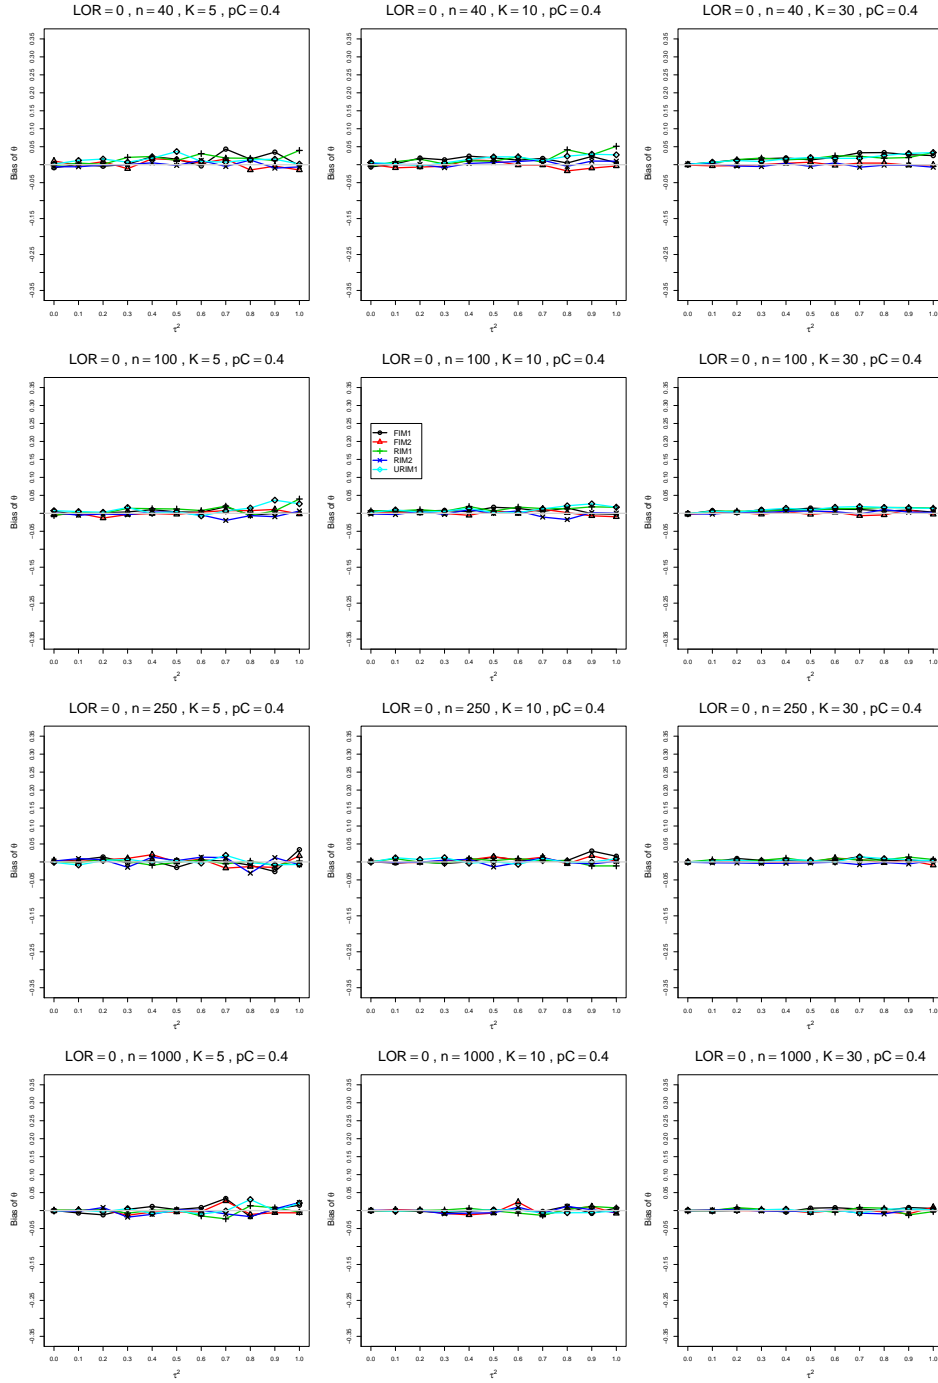

Figure A2.4.2: Bias of overall log-odds ratio  $\hat{\theta}_{KD}$  for  $\theta = 0$ ,  $p_C = 0.4$ ,  $\sigma^2 = 0.1$ , constant sample sizes  $n = 40, 100, 250, 1000$ . The data-generation mechanisms are FIM1 ( $\circ$ ), FIM2 ( $\triangle$ ), RIM1 ( $+$ ), RIM2 ( $\times$ ), and URIM1 ( $\diamond$ ).

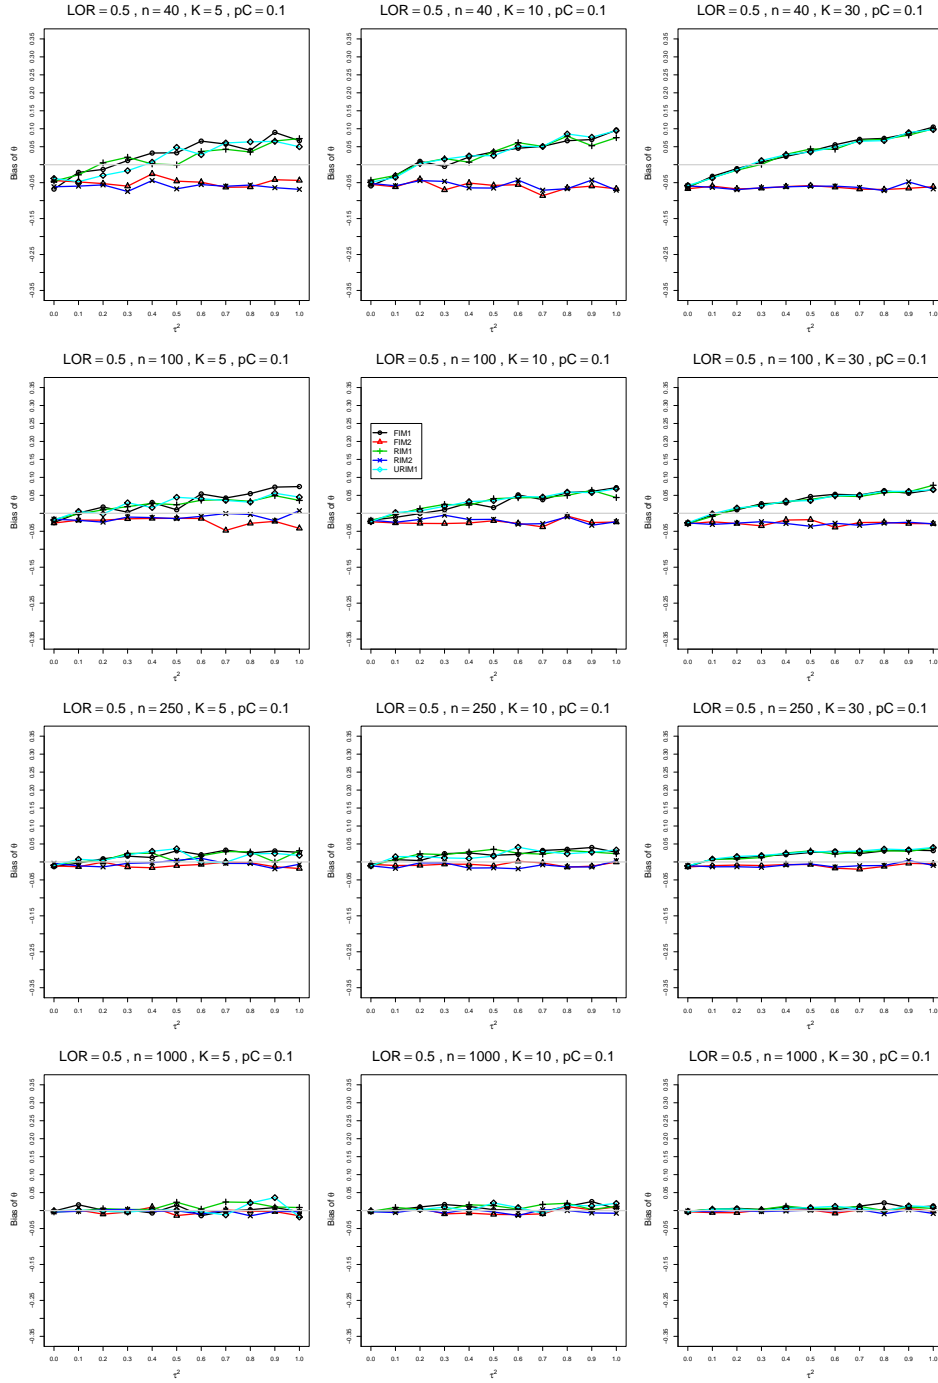

Figure A2.4.3: Bias of overall log-odds ratio  $\hat{\theta}_{KD}$  for  $\theta = 0.5$ ,  $p_C = 0.1$ ,  $\sigma^2 = 0.1$ , constant sample sizes  $n = 40, 100, 250, 1000$ . The data-generation mechanisms are FIM1 ( $\circ$ ), FIM2 ( $\triangle$ ), RIM1 ( $+$ ), RIM2 ( $\times$ ), and URIM1 ( $\diamond$ ).



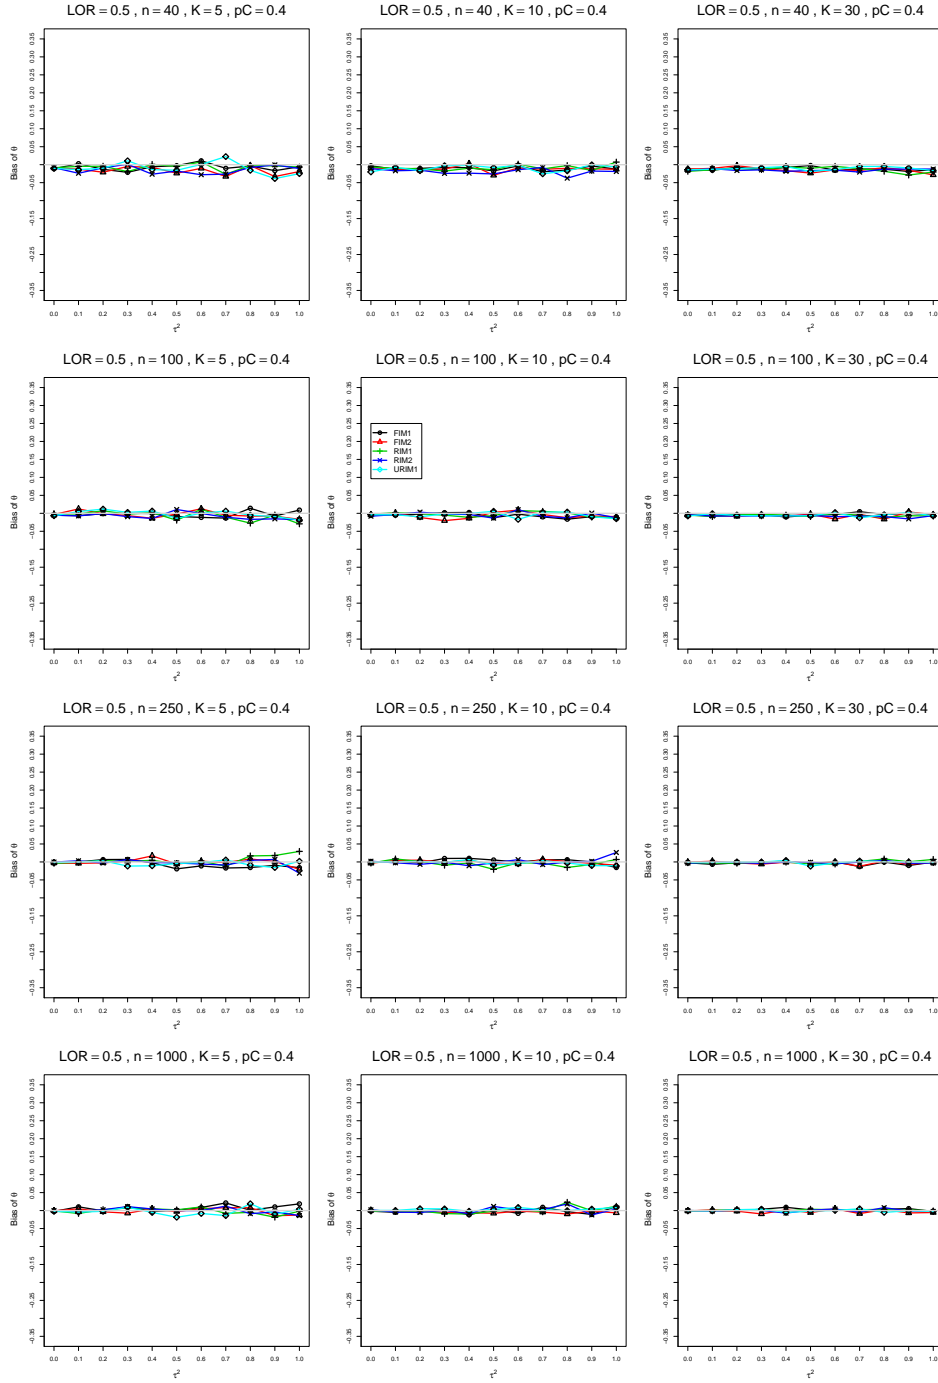

Figure A2.4.4: Bias of overall log-odds ratio  $\hat{\theta}_{KD}$  for  $\theta = 0.5$ ,  $p_C = 0.4$ ,  $\sigma^2 = 0.1$ , constant sample sizes  $n = 40, 100, 250, 1000$ . The data-generation mechanisms are FIM1 ( $\circ$ ), FIM2 ( $\triangle$ ), RIM1 ( $+$ ), RIM2 ( $\times$ ), and URIM1 ( $\diamond$ ).

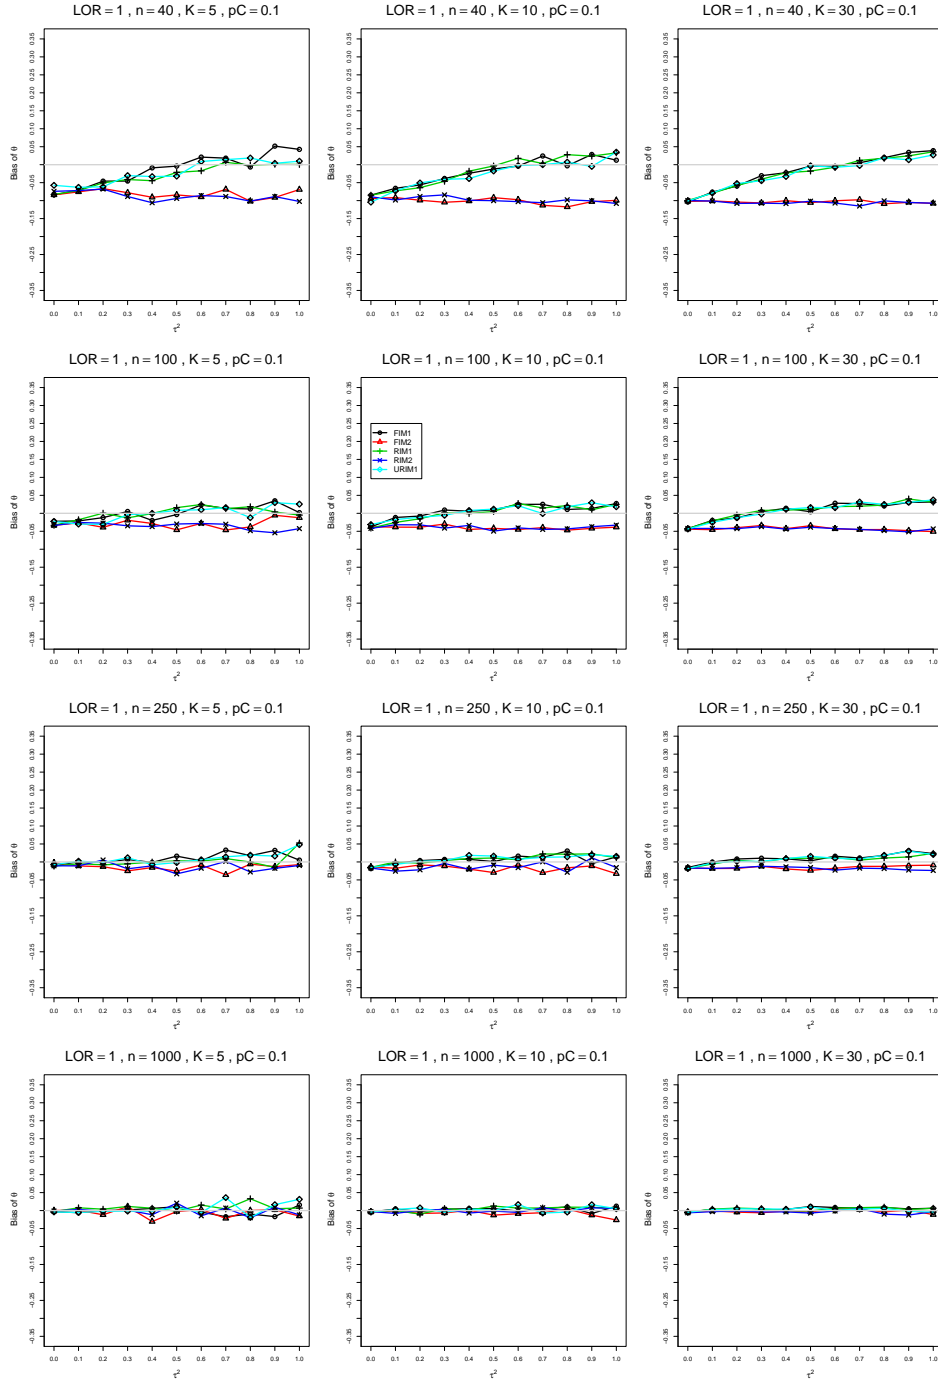

Figure A2.4.5: Bias of overall log-odds ratio  $\hat{\theta}_{KD}$  for  $\theta = 1$ ,  $p_C = 0.1$ ,  $\sigma^2 = 0.1$ , constant sample sizes  $n = 40, 100, 250, 1000$ . The data-generation mechanisms are FIM1 ( $\circ$ ), FIM2 ( $\triangle$ ), RIM1 ( $+$ ), RIM2 ( $\times$ ), and URIM1 ( $\diamond$ ).

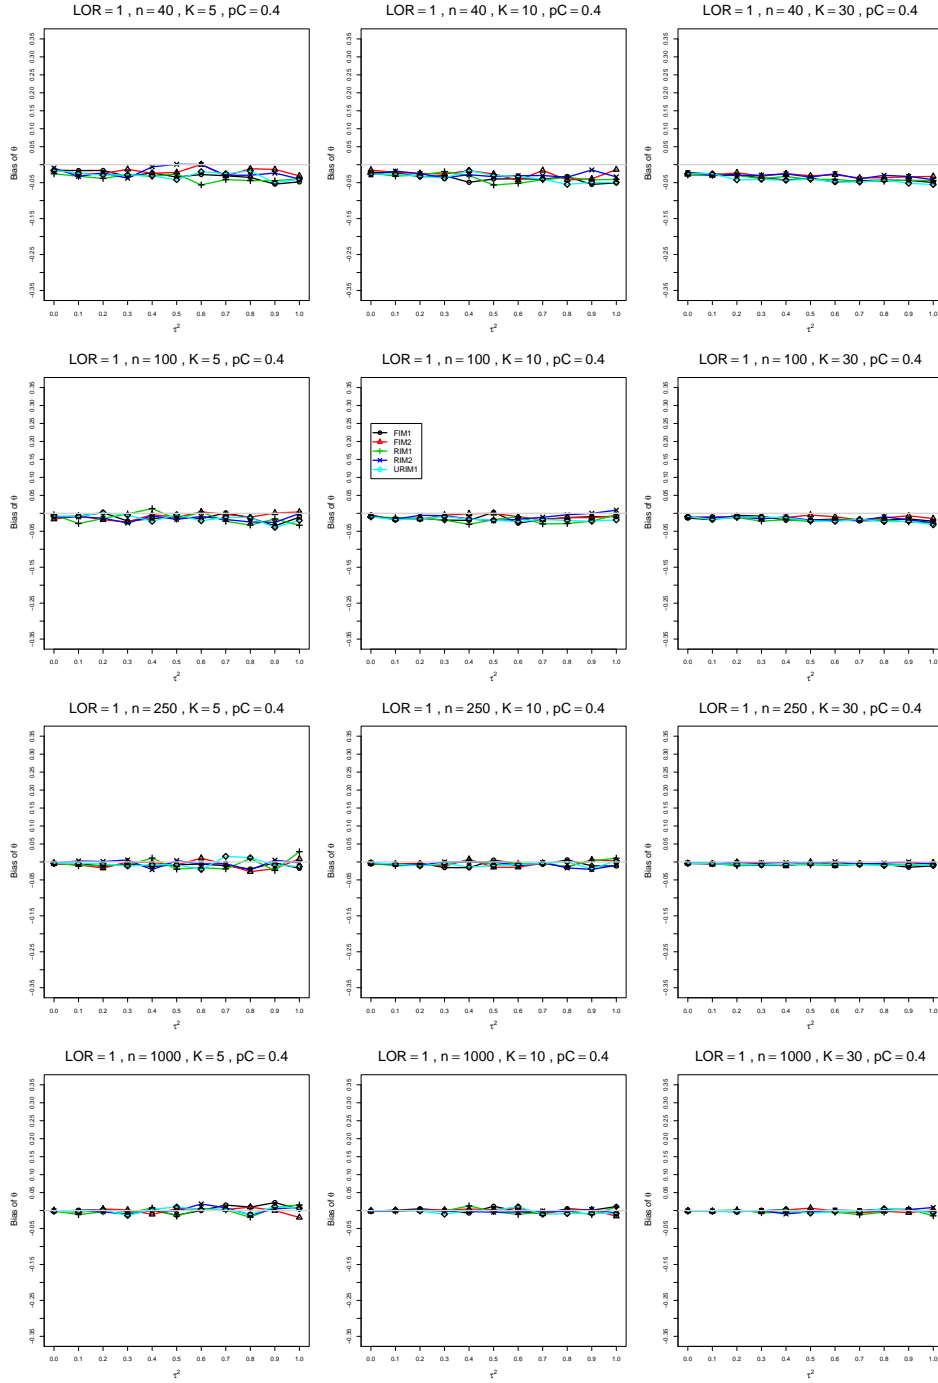

Figure A2.4.6: Bias of overall log-odds ratio  $\hat{\theta}_{KD}$  for  $\theta = 1$ ,  $p_C = 0.4$ ,  $\sigma^2 = 0.1$ , constant sample sizes  $n = 40, 100, 250, 1000$ . The data-generation mechanisms are FIM1 ( $\circ$ ), FIM2 ( $\triangle$ ), RIM1 ( $+$ ), RIM2 ( $\times$ ), and URIM1 ( $\diamond$ ).

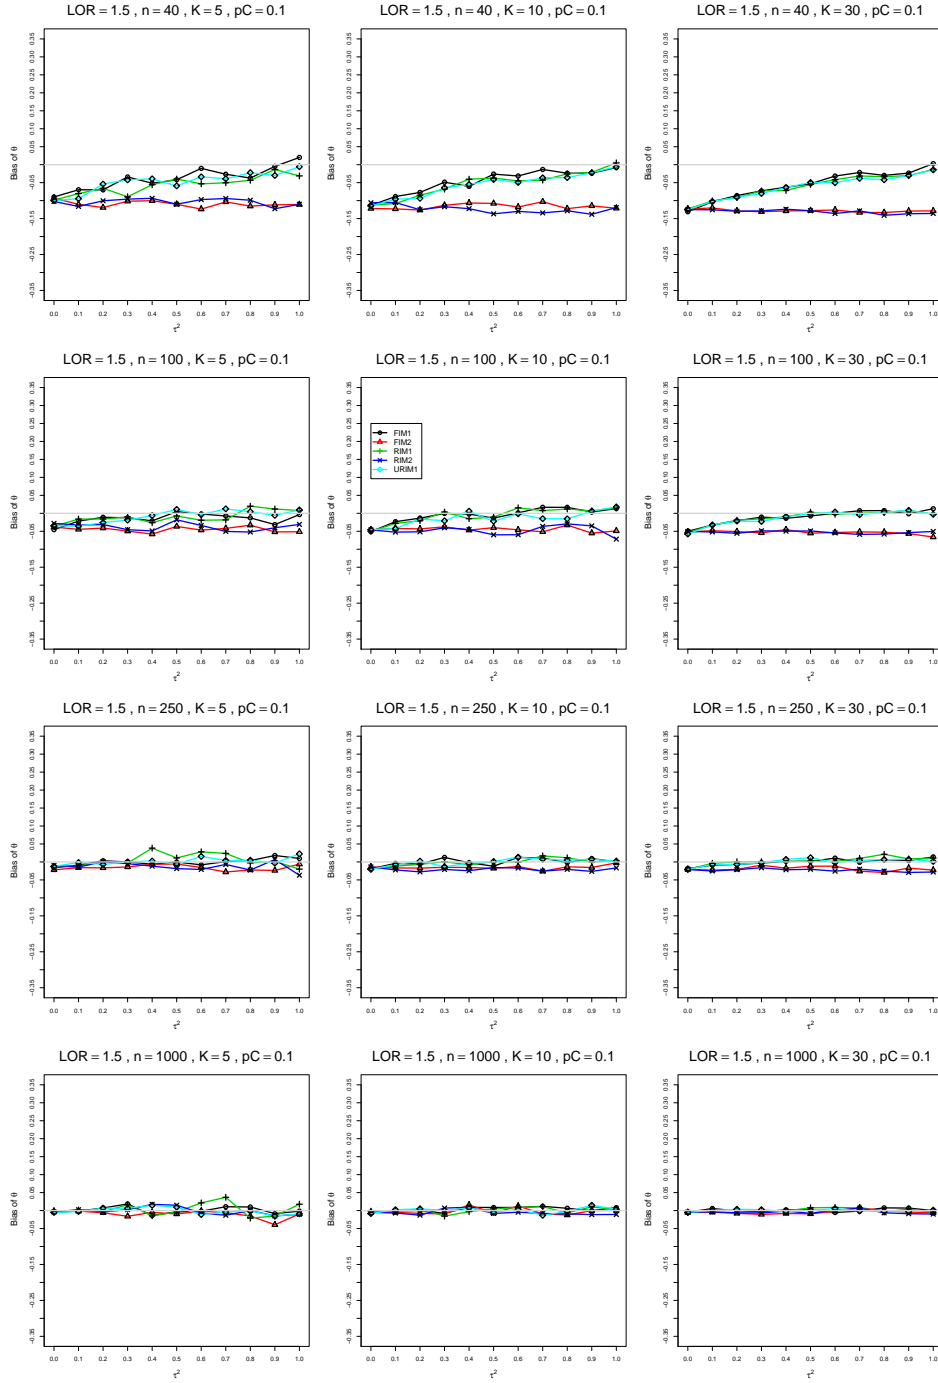

Figure A2.4.7: Bias of overall log-odds ratio  $\hat{\theta}_{KD}$  for  $\theta = 1.5$ ,  $p_C = 0.1$ ,  $\sigma^2 = 0.1$ , constant sample sizes  $n = 40, 100, 250, 1000$ . The data-generation mechanisms are FIM1 ( $\circ$ ), FIM2 ( $\triangle$ ), RIM1 ( $+$ ), RIM2 ( $\times$ ), and URIM1 ( $\diamond$ ).

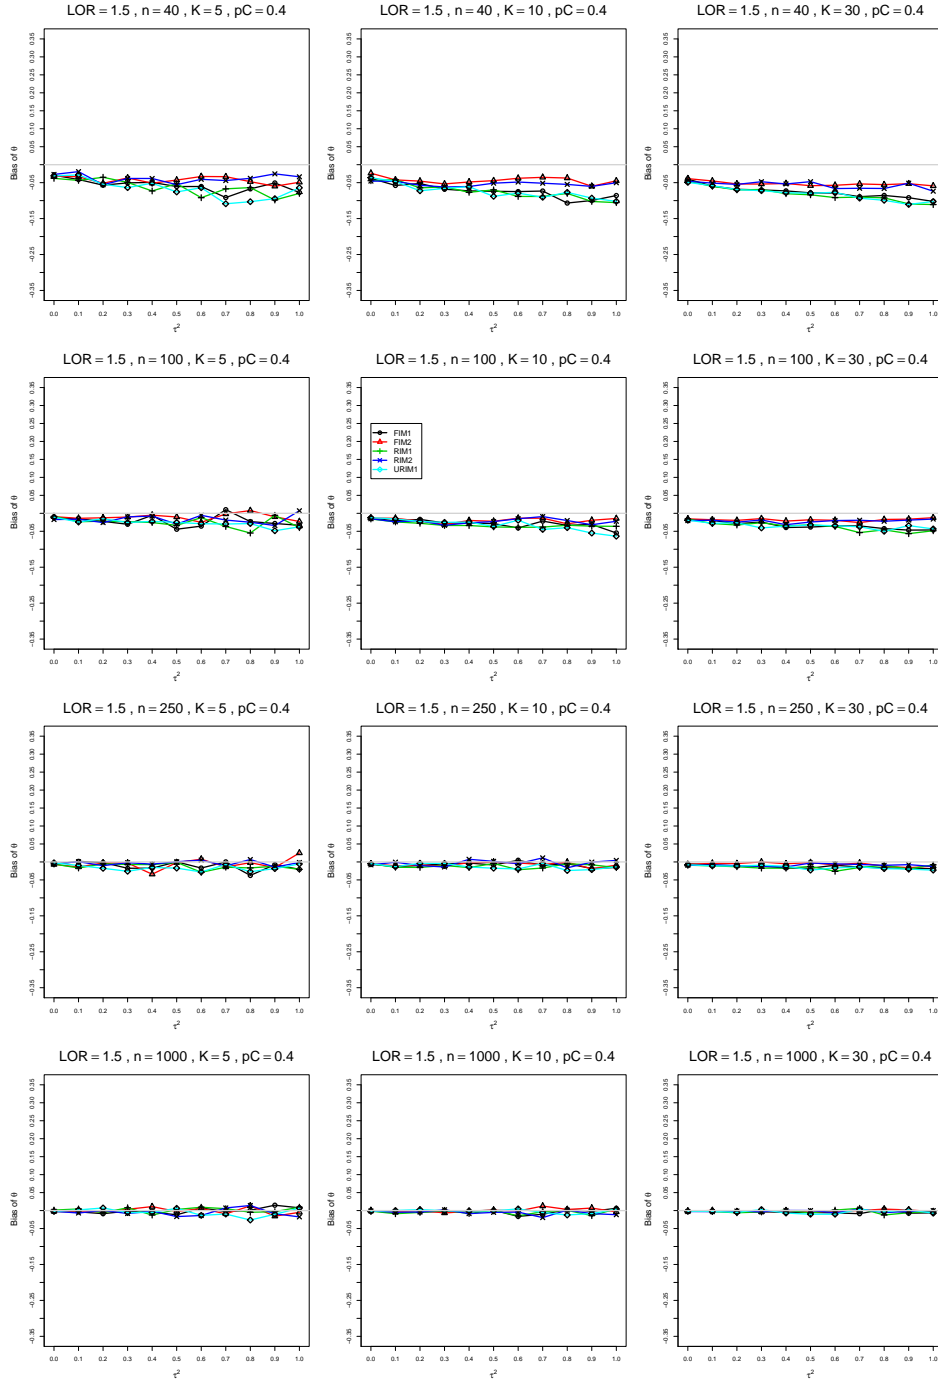

Figure A2.4.8: Bias of overall log-odds ratio  $\hat{\theta}_{KD}$  for  $\theta = 1.5$ ,  $p_C = 0.4$ ,  $\sigma^2 = 0.1$ , constant sample sizes  $n = 40, 100, 250, 1000$ . The data-generation mechanisms are FIM1 ( $\circ$ ), FIM2 ( $\triangle$ ), RIM1 ( $+$ ), RIM2 ( $\times$ ), and URIM1 ( $\diamond$ ).

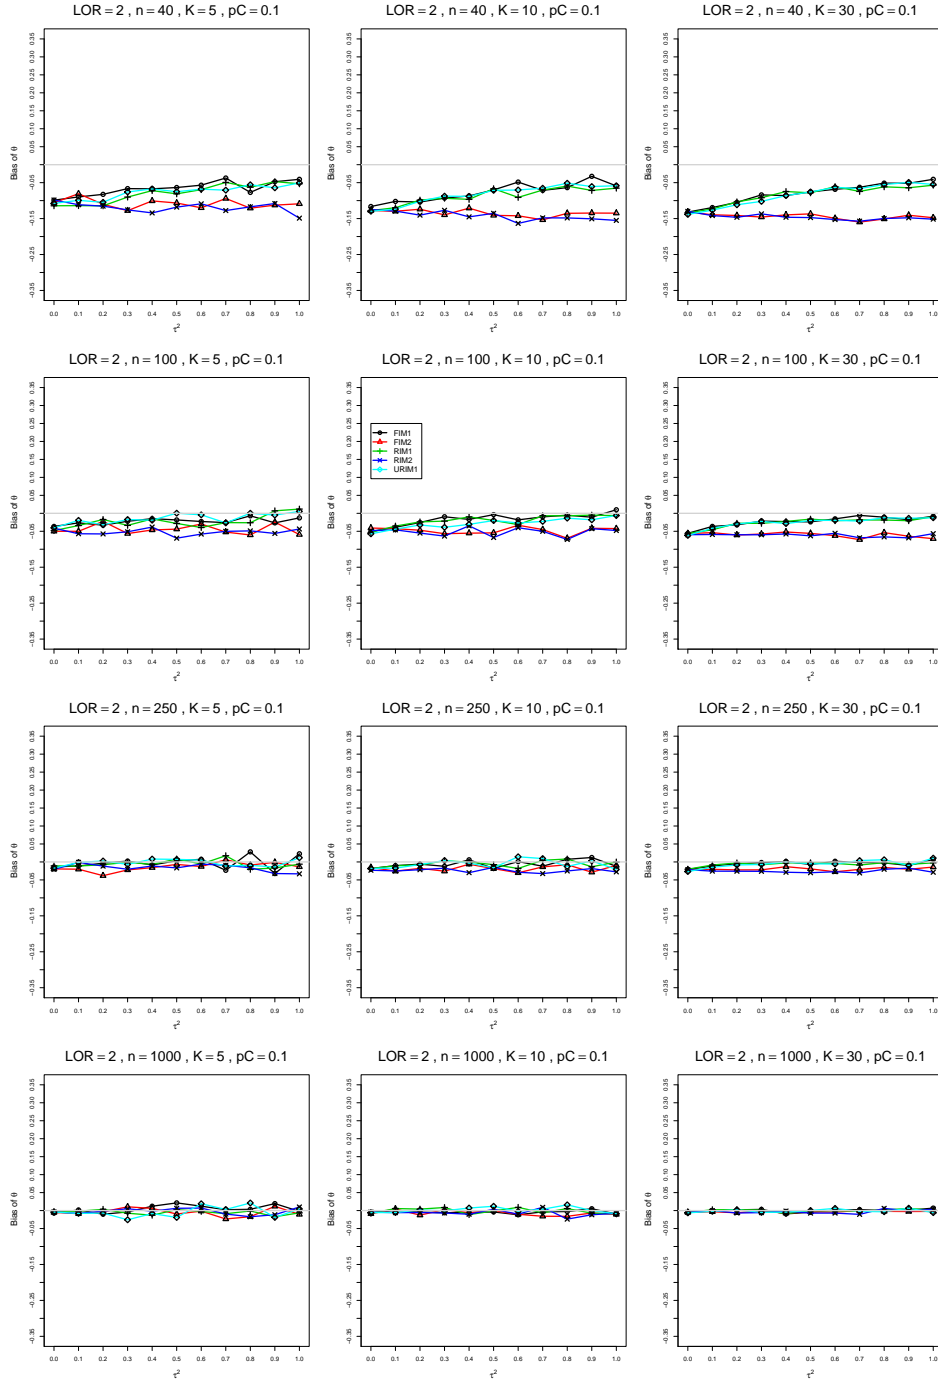

Figure A2.4.9: Bias of overall log-odds ratio  $\hat{\theta}_{KD}$  for  $\theta = 2$ ,  $p_C = 0.1$ ,  $\sigma^2 = 0.1$ , constant sample sizes  $n = 40, 100, 250, 1000$ . The data-generation mechanisms are FIM1 ( $\circ$ ), FIM2 ( $\triangle$ ), RIM1 ( $+$ ), RIM2 ( $\times$ ), and URIM1 ( $\diamond$ ).

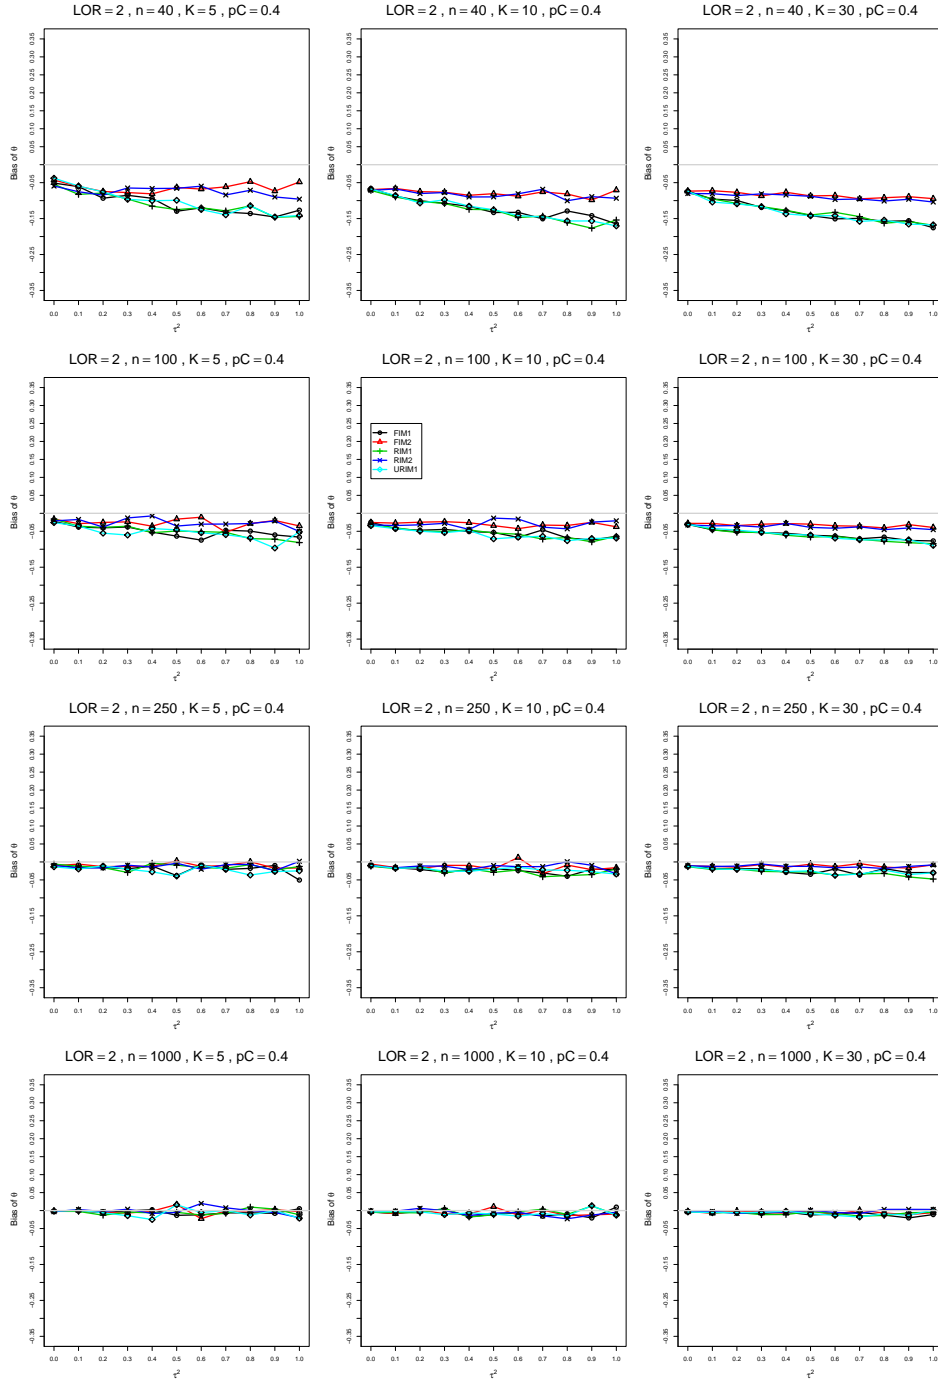

Figure A2.4.10: Bias of overall log-odds ratio  $\hat{\theta}_{KD}$  for  $\theta = 2$ ,  $p_C = 0.4$ ,  $\sigma^2 = 0.1$ , constant sample sizes  $n = 40, 100, 250, 1000$ . The data-generation mechanisms are FIM1 ( $\circ$ ), FIM2 ( $\triangle$ ), RIM1 ( $+$ ), RIM2 ( $\times$ ), and URIM1 ( $\diamond$ ).

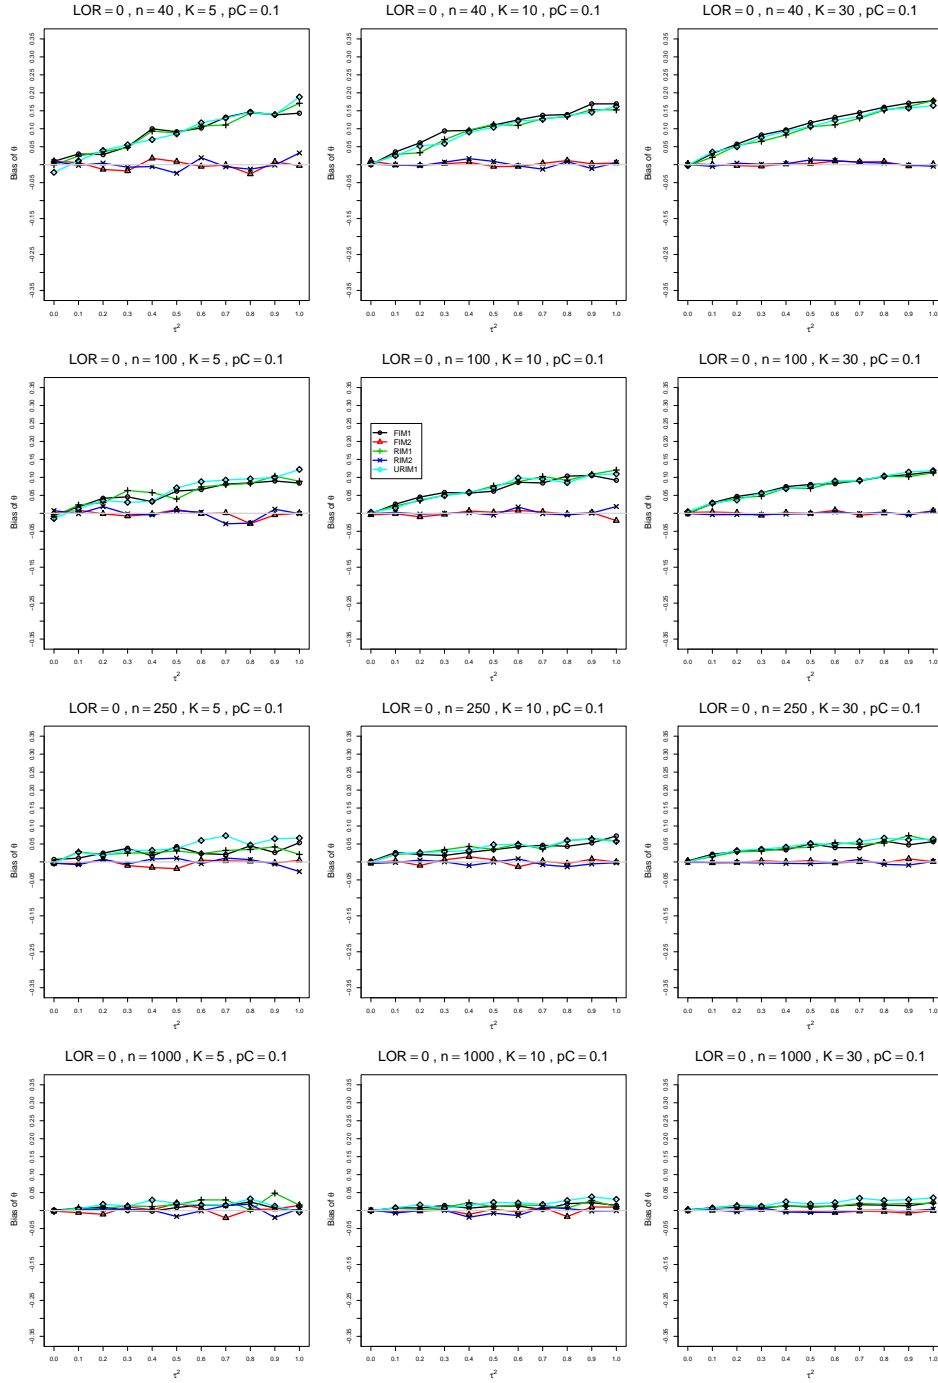

Figure A2.4.11: Bias of overall log-odds ratio  $\hat{\theta}_{KD}$  for  $\theta = 0$ ,  $p_C = 0.1$ ,  $\sigma^2 = 0.4$ , constant sample sizes  $n = 40, 100, 250, 1000$ . The data-generation mechanisms are FIM1 ( $\circ$ ), FIM2 ( $\triangle$ ), RIM1 ( $+$ ), RIM2 ( $\times$ ), and URIM1 ( $\diamond$ ).



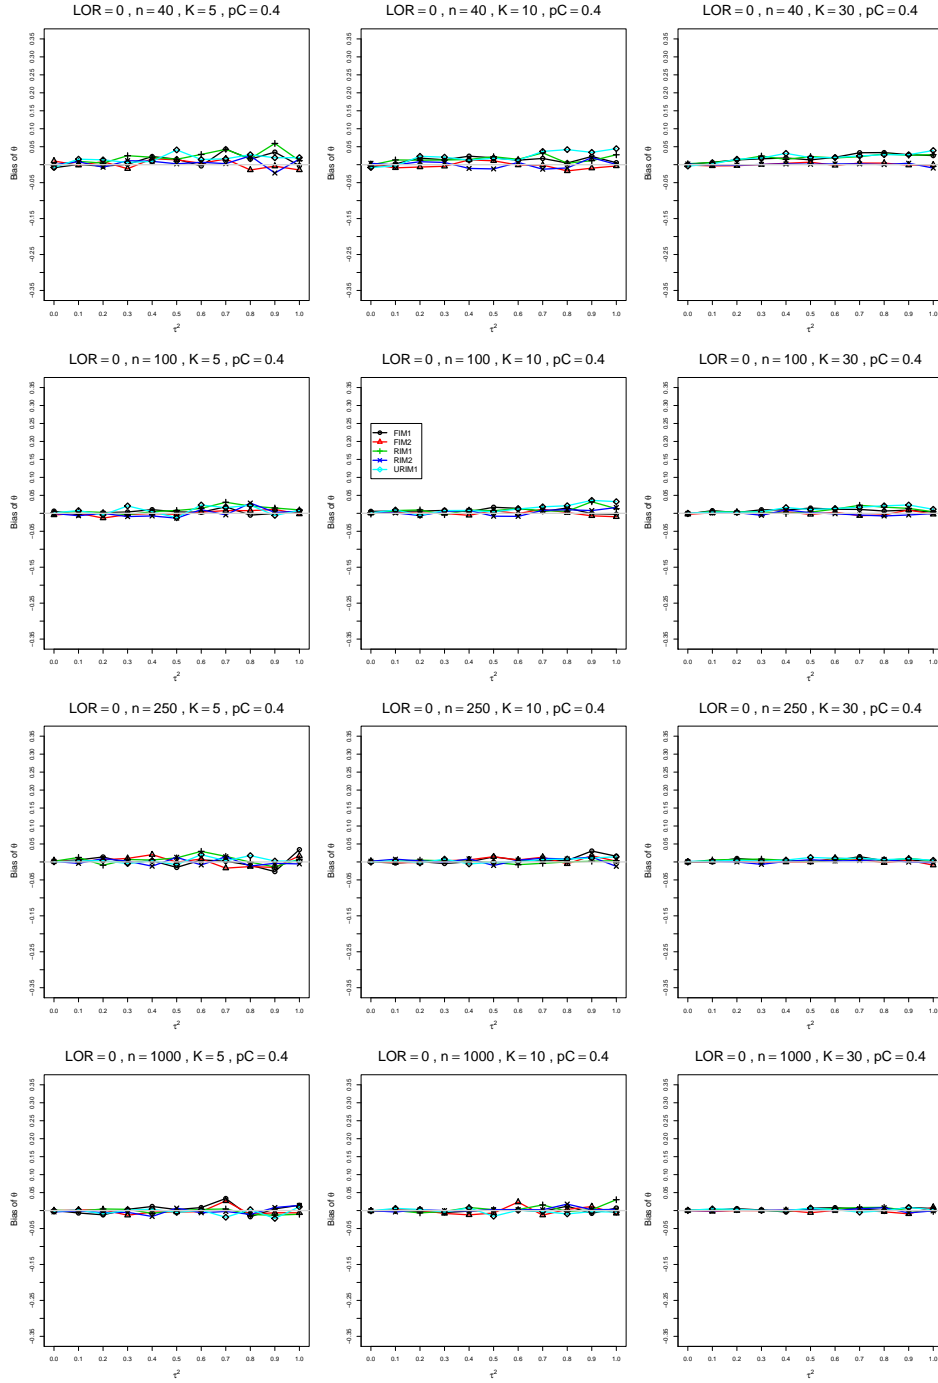

Figure A2.4.12: Bias of overall log-odds ratio  $\hat{\theta}_{KD}$  for  $\theta = 0$ ,  $p_C = 0.4$ ,  $\sigma^2 = 0.4$ , constant sample sizes  $n = 40, 100, 250, 1000$ . The data-generation mechanisms are FIM1 ( $\circ$ ), FIM2 ( $\triangle$ ), RIM1 ( $+$ ), RIM2 ( $\times$ ), and URIM1 ( $\diamond$ ).

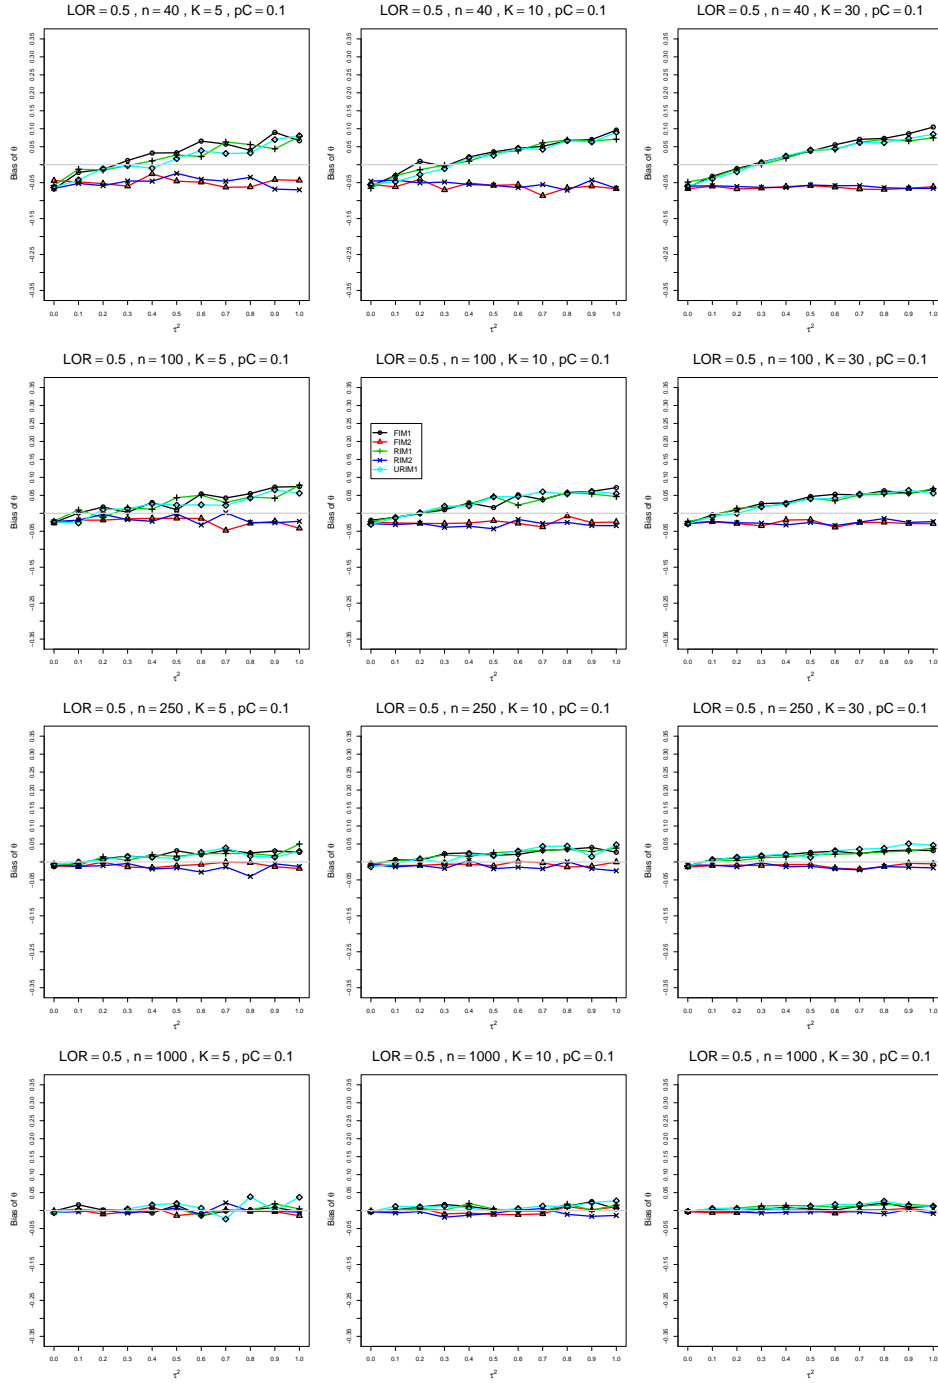

Figure A2.4.13: Bias of overall log-odds ratio  $\hat{\theta}_{KD}$  for  $\theta = 0.5$ ,  $p_C = 0.1$ ,  $\sigma^2 = 0.4$ , constant sample sizes  $n = 40, 100, 250, 1000$ . The data-generation mechanisms are FIM1 ( $\circ$ ), FIM2 ( $\triangle$ ), RIM1 ( $+$ ), RIM2 ( $\times$ ), and URIM1 ( $\diamond$ ).

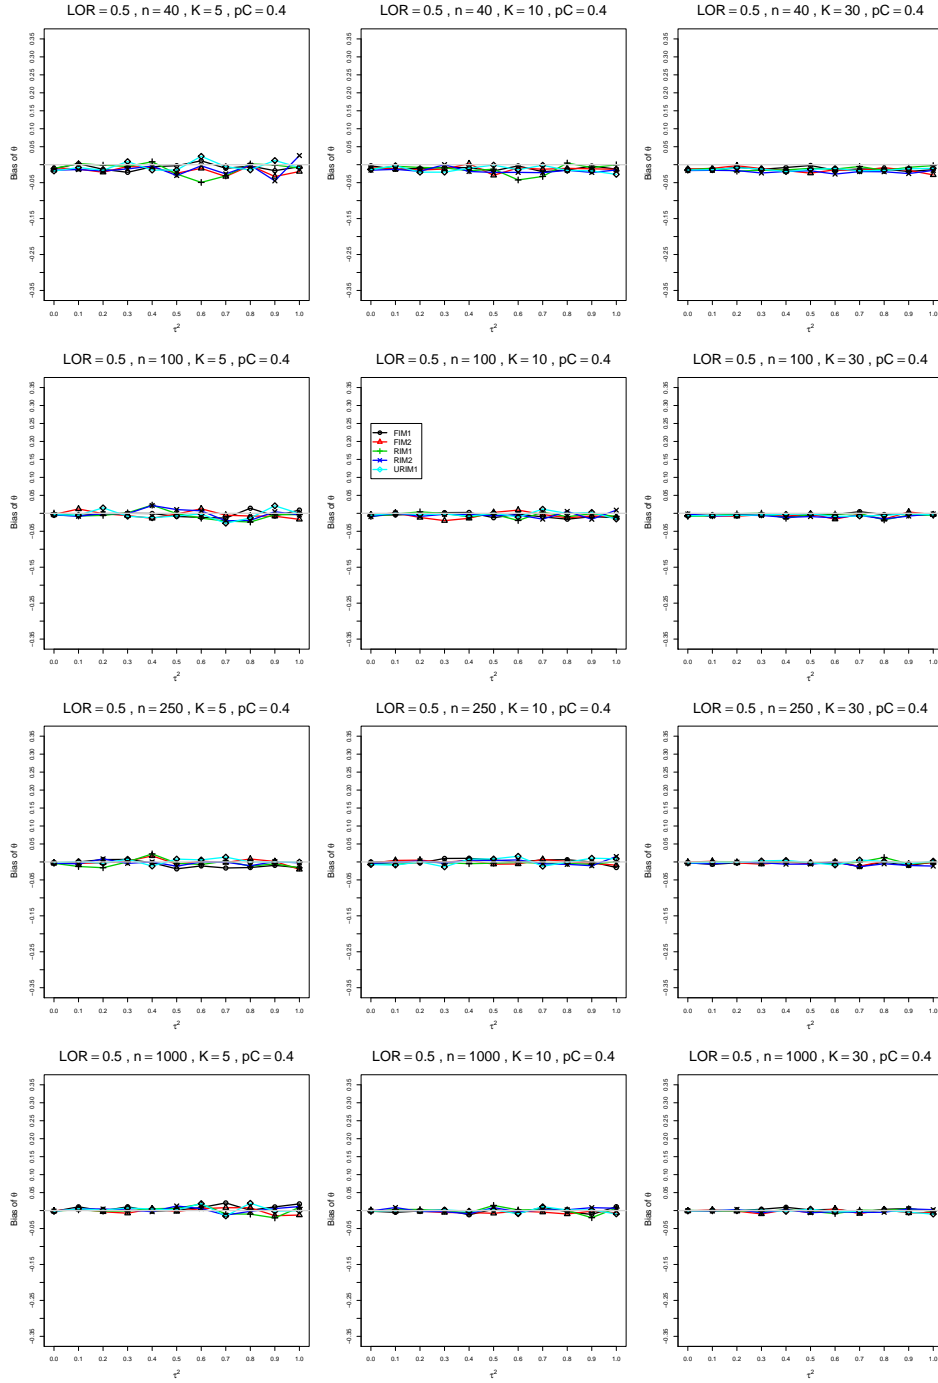

Figure A2.4.14: Bias of overall log-odds ratio  $\hat{\theta}_{KD}$  for  $\theta = 0.5$ ,  $p_C = 0.4$ ,  $\sigma^2 = 0.4$ , constant sample sizes  $n = 40, 100, 250, 1000$ . The data-generation mechanisms are FIM1 ( $\circ$ ), FIM2 ( $\triangle$ ), RIM1 ( $+$ ), RIM2 ( $\times$ ), and URIM1 ( $\diamond$ ).

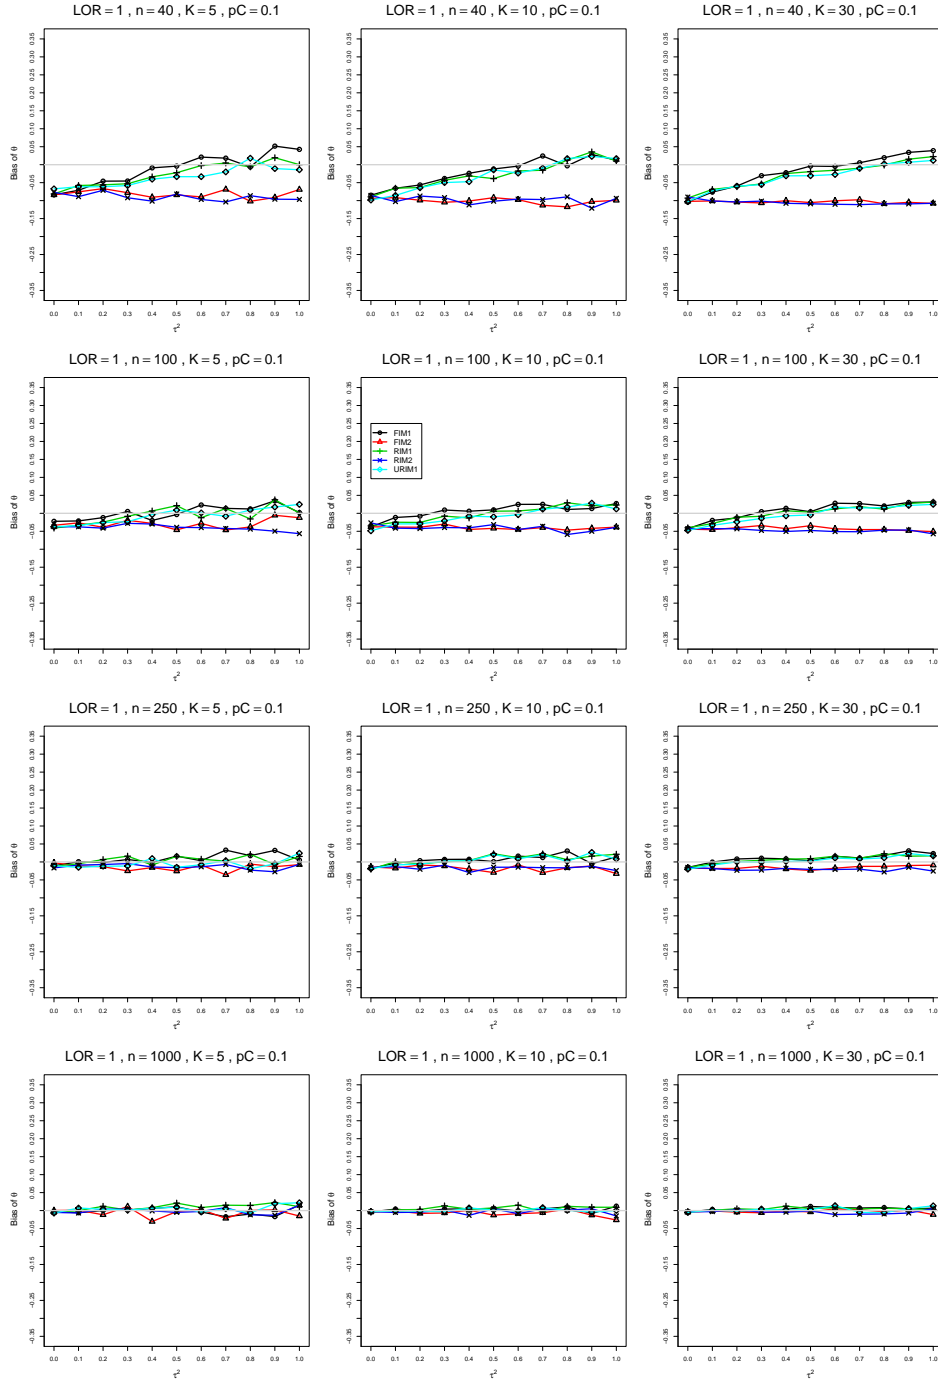

Figure A2.4.15: Bias of overall log-odds ratio  $\hat{\theta}_{KD}$  for  $\theta = 1$ ,  $p_C = 0.1$ ,  $\sigma^2 = 0.4$ , constant sample sizes  $n = 40, 100, 250, 1000$ . The data-generation mechanisms are FIM1 ( $\circ$ ), FIM2 ( $\triangle$ ), RIM1 ( $+$ ), RIM2 ( $\times$ ), and URIM1 ( $\diamond$ ).

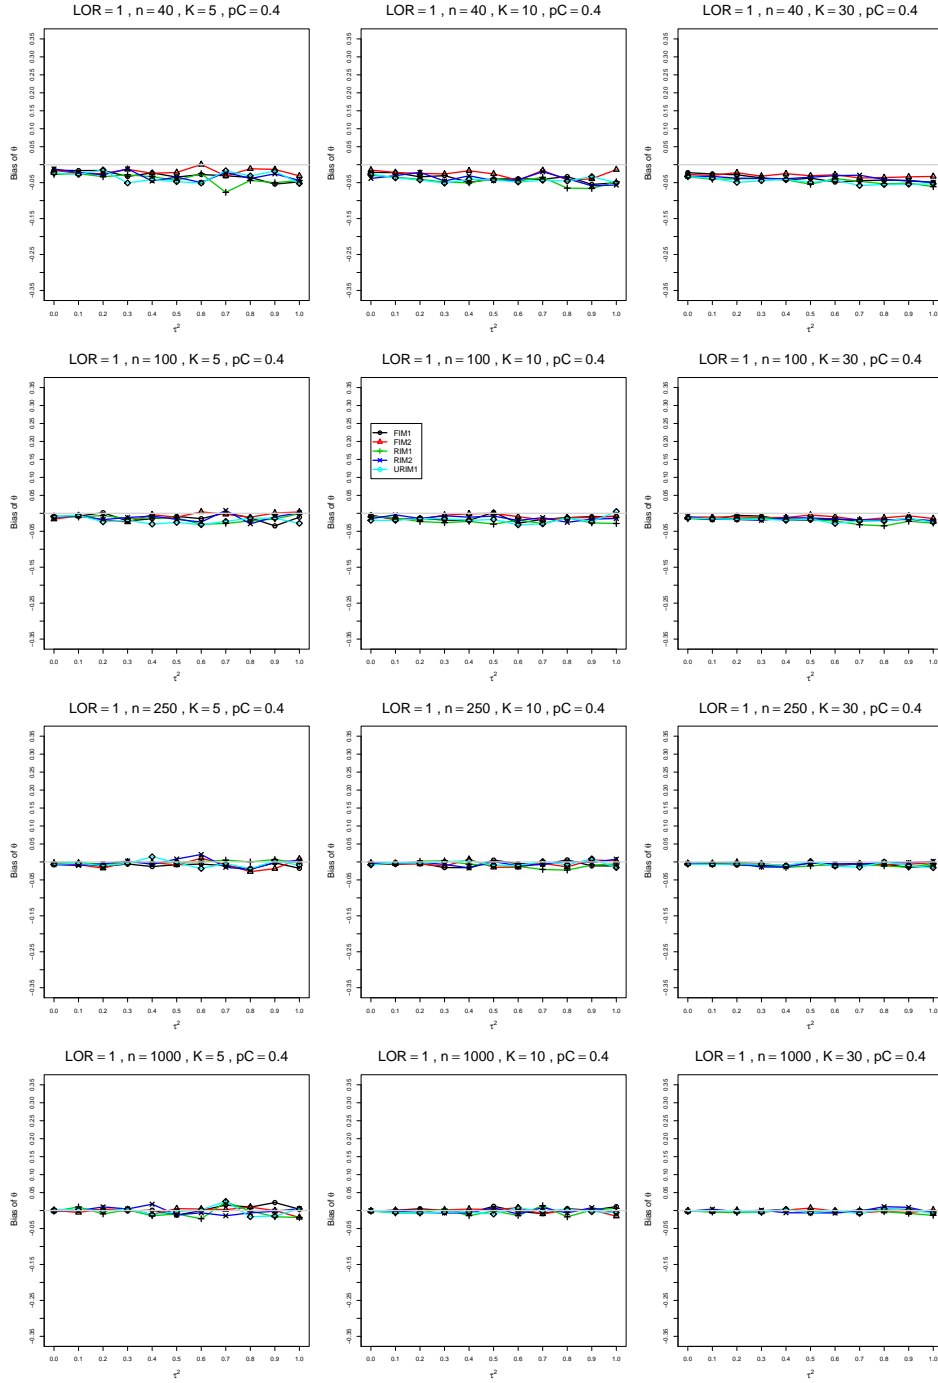

Figure A2.4.16: Bias of overall log-odds ratio  $\hat{\theta}_{KD}$  for  $\theta = 1$ ,  $p_C = 0.4$ ,  $\sigma^2 = 0.4$ , constant sample sizes  $n = 40, 100, 250, 1000$ . The data-generation mechanisms are FIM1 ( $\circ$ ), FIM2 ( $\triangle$ ), RIM1 ( $+$ ), RIM2 ( $\times$ ), and URIM1 ( $\diamond$ ).

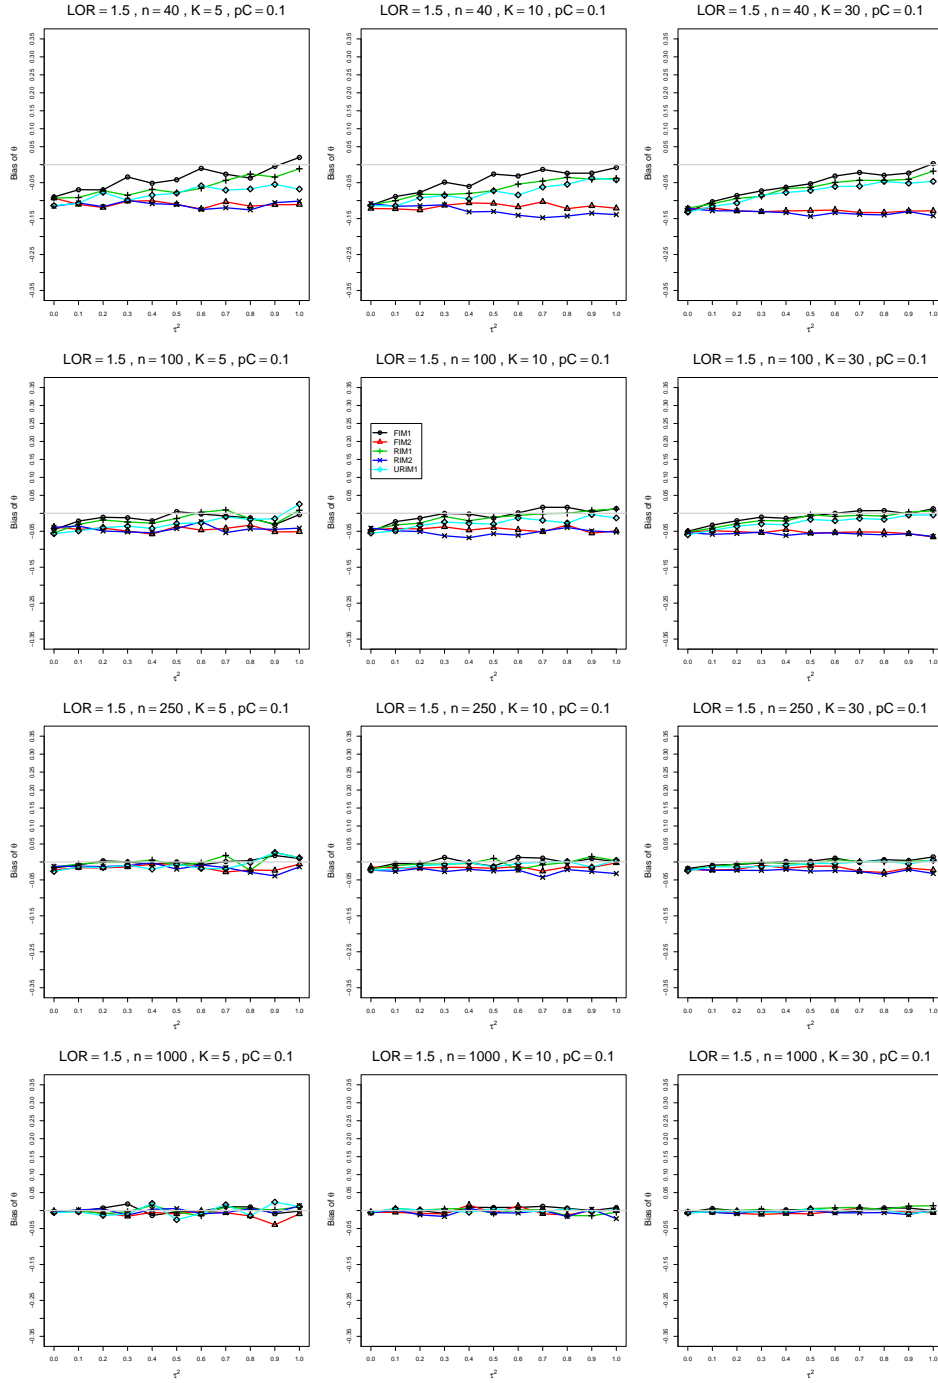

Figure A2.4.17: Bias of overall log-odds ratio  $\hat{\theta}_{KD}$  for  $\theta = 1.5$ ,  $p_C = 0.1$ ,  $\sigma^2 = 0.4$ , constant sample sizes  $n = 40, 100, 250, 1000$ . The data-generation mechanisms are FIM1 ( $\circ$ ), FIM2 ( $\triangle$ ), RIM1 ( $+$ ), RIM2 ( $\times$ ), and URIM1 ( $\diamond$ ).

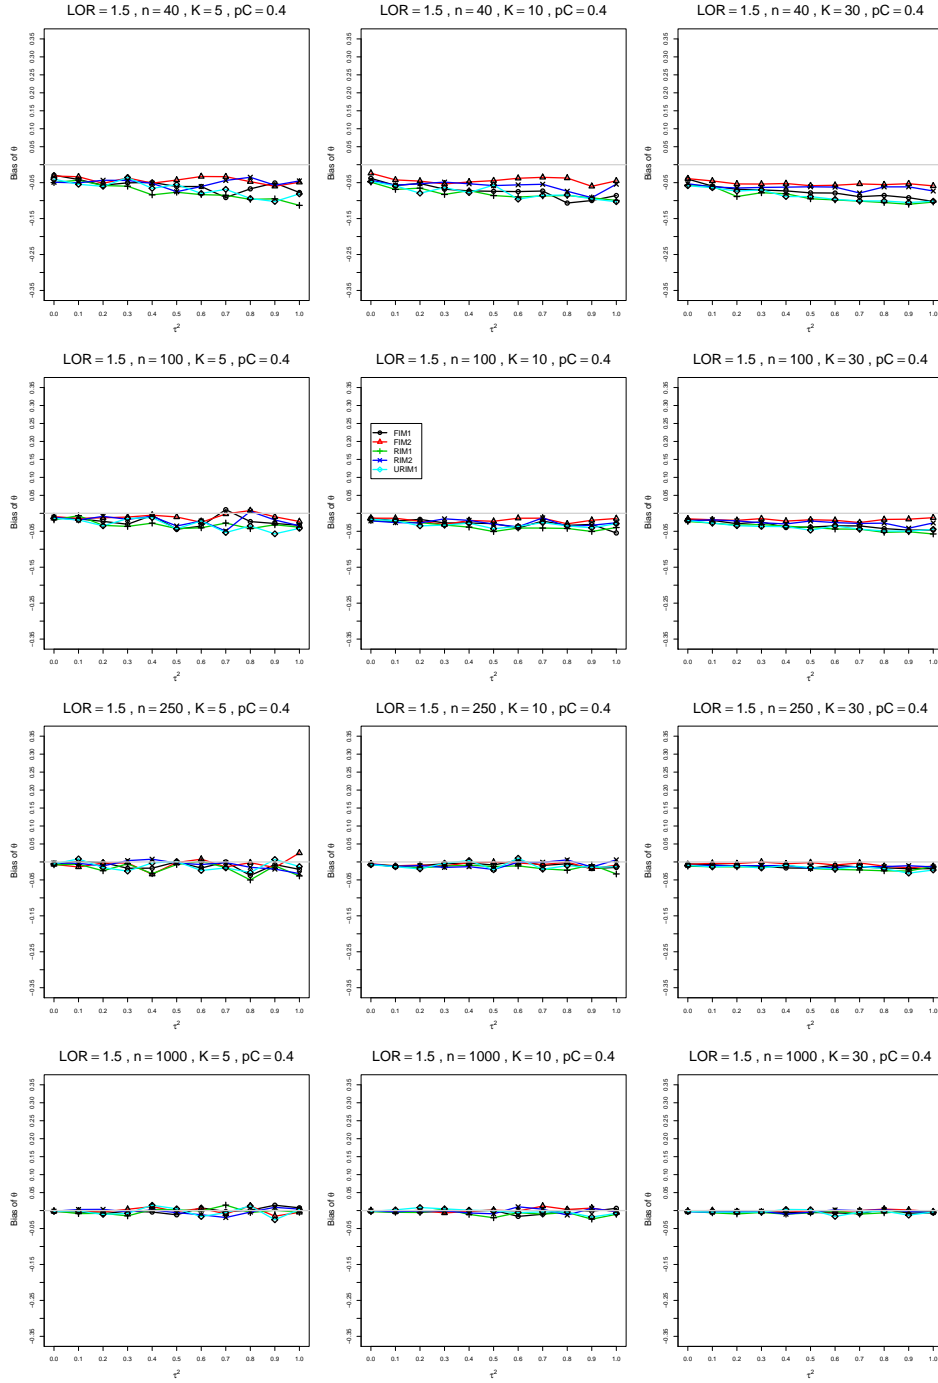

Figure A2.4.18: Bias of overall log-odds ratio  $\hat{\theta}_{KD}$  for  $\theta = 1.5$ ,  $p_C = 0.4$ ,  $\sigma^2 = 0.4$ , constant sample sizes  $n = 40, 100, 250, 1000$ . The data-generation mechanisms are FIM1 ( $\circ$ ), FIM2 ( $\triangle$ ), RIM1 ( $+$ ), RIM2 ( $\times$ ), and URIM1 ( $\diamond$ ).

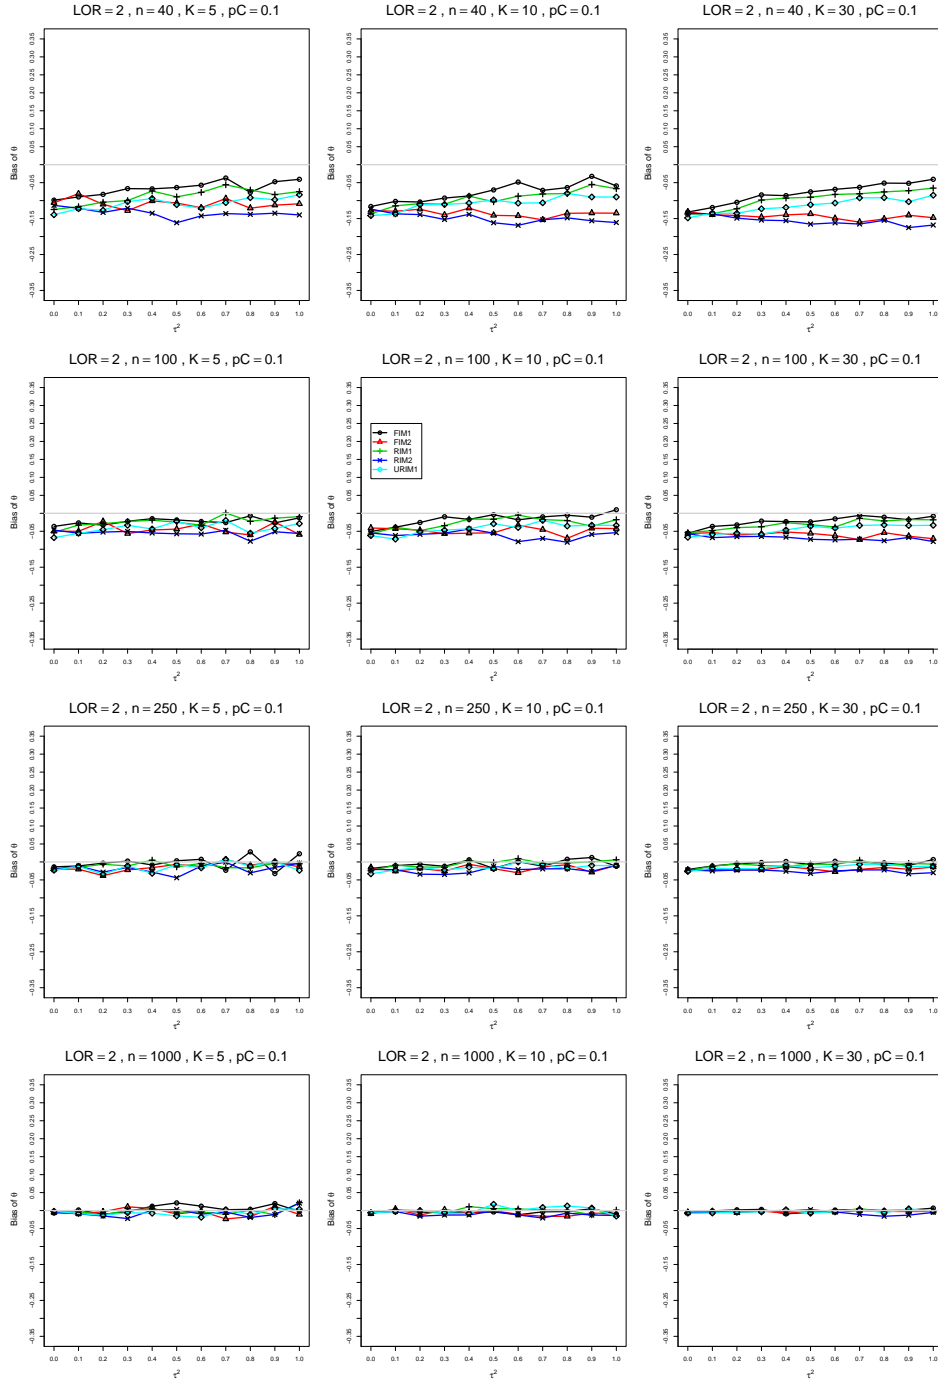

Figure A2.4.19: Bias of overall log-odds ratio  $\hat{\theta}_{KD}$  for  $\theta = 2$ ,  $p_C = 0.1$ ,  $\sigma^2 = 0.4$ , constant sample sizes  $n = 40, 100, 250, 1000$ . The data-generation mechanisms are FIM1 ( $\circ$ ), FIM2 ( $\triangle$ ), RIM1 ( $+$ ), RIM2 ( $\times$ ), and URIM1 ( $\diamond$ ).



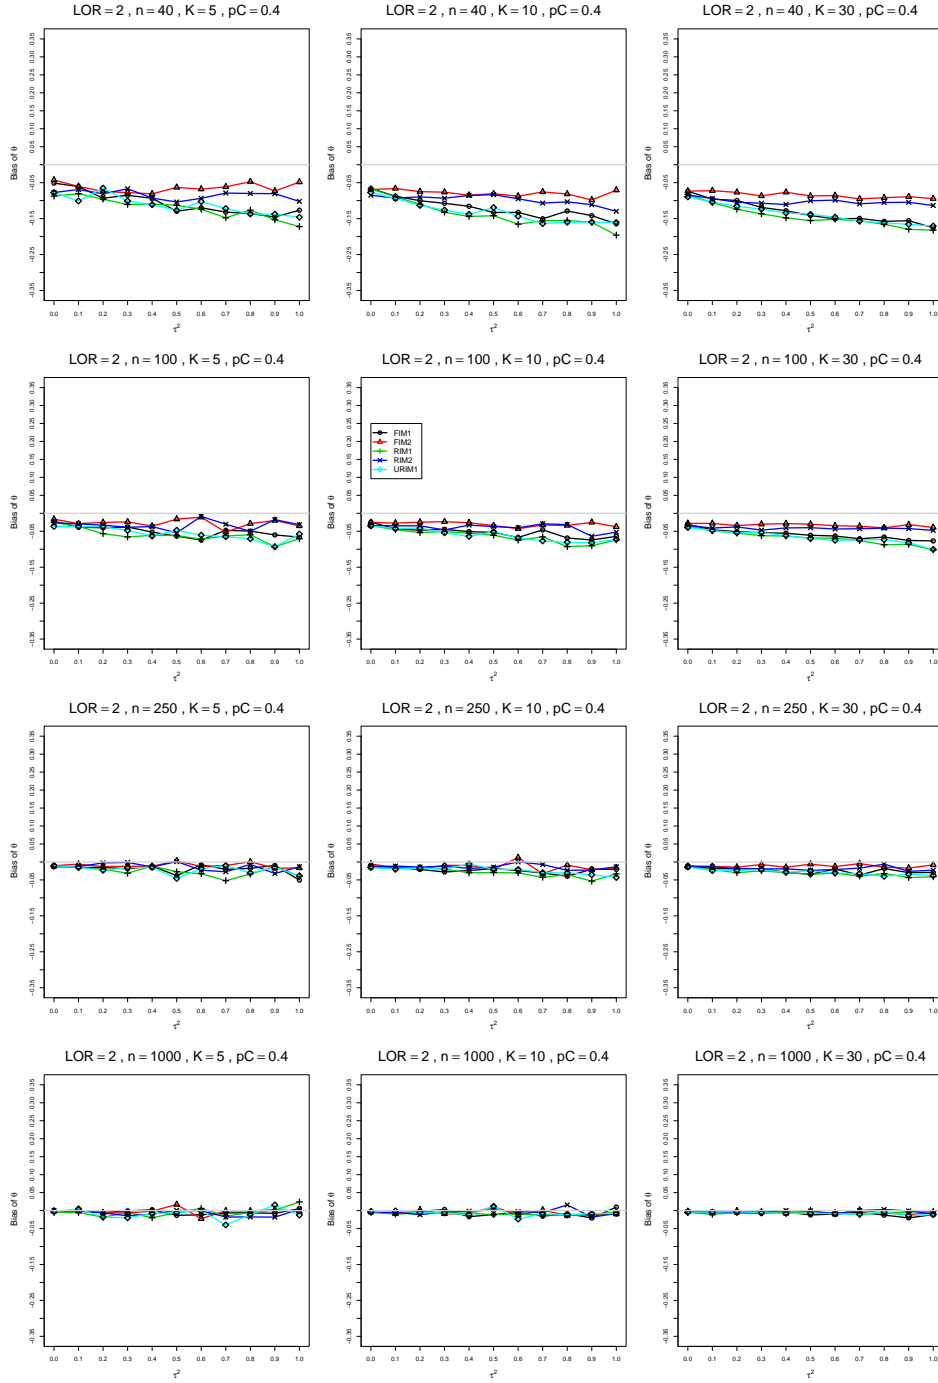

Figure A2.4.20: Bias of overall log-odds ratio  $\hat{\theta}_{KD}$  for  $\theta = 2$ ,  $p_C = 0.4$ ,  $\sigma^2 = 0.4$ , constant sample sizes  $n = 40, 100, 250, 1000$ . The data-generation mechanisms are FIM1 ( $\circ$ ), FIM2 ( $\triangle$ ), RIM1 ( $+$ ), RIM2 ( $\times$ ), and URIM1 ( $\diamond$ ).

## A2.5 Bias of $\hat{\theta}_{FIM2}$

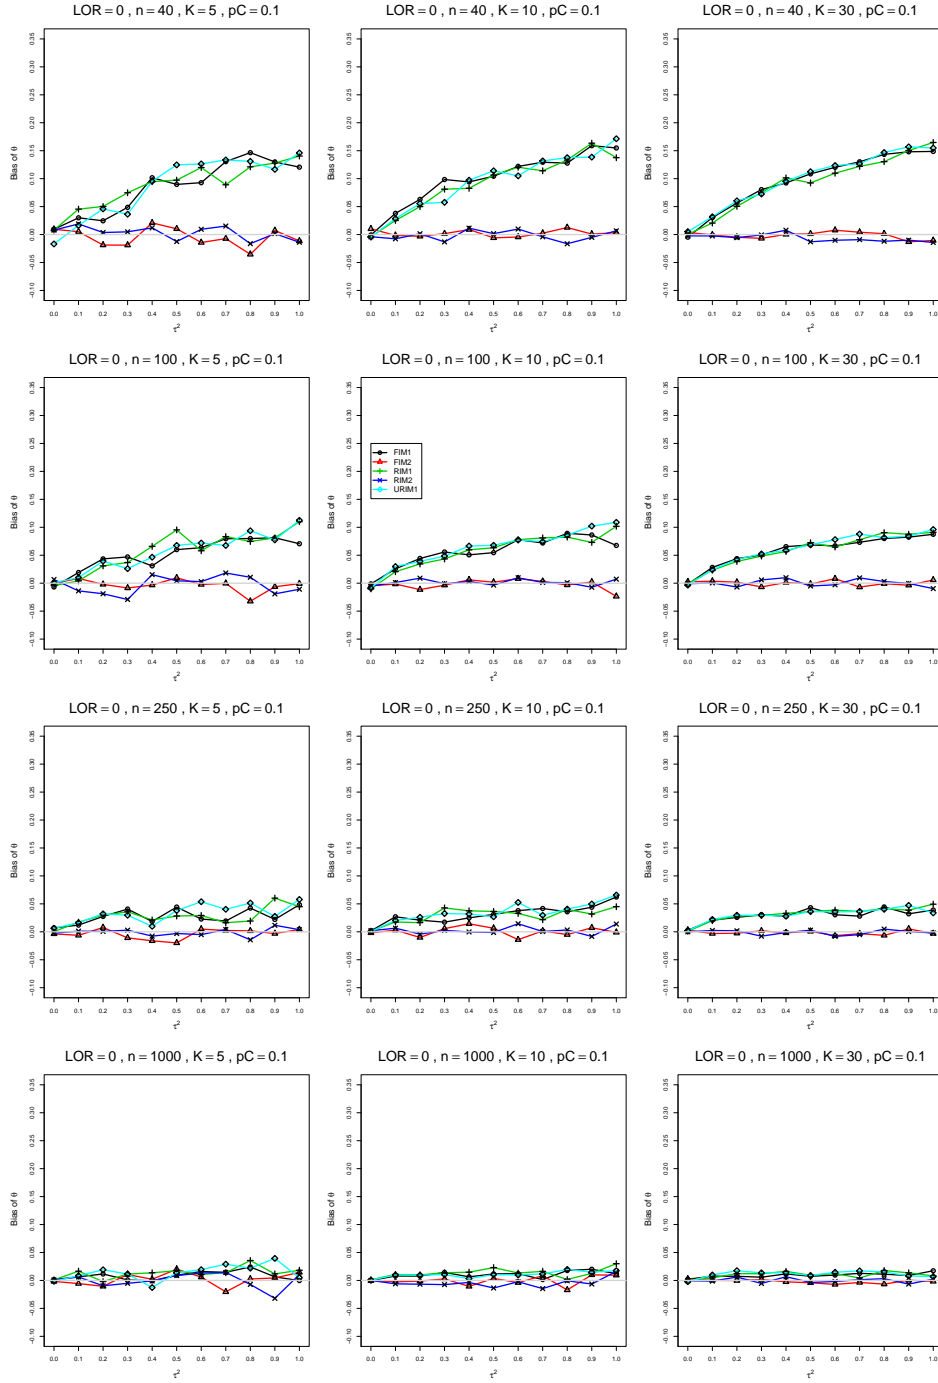

Figure A2.5.1: Bias of overall log-odds ratio  $\hat{\theta}_{FIM2}$  for  $\theta = 0$ ,  $p_C = 0.1$ ,  $\sigma^2 = 0.1$ , constant sample sizes  $n = 40, 100, 250, 1000$ . The data-generation mechanisms are FIM1 ( $\circ$ ), FIM2 ( $\triangle$ ), RIM1 ( $+$ ), RIM2 ( $\times$ ), and URIM1 ( $\diamond$ ).

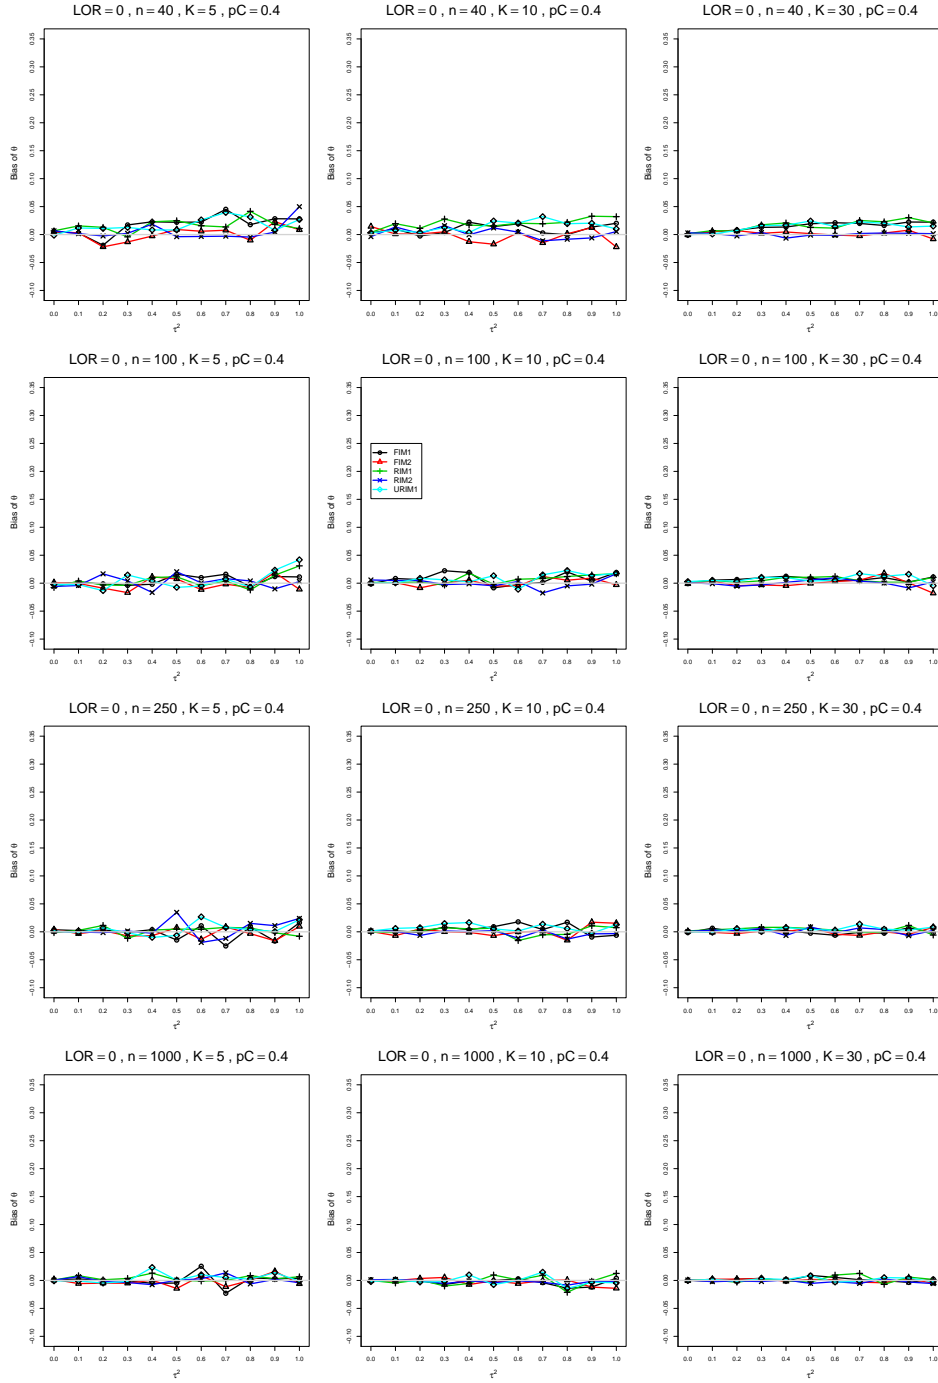

Figure A2.5.2: Bias of overall log-odds ratio  $\hat{\theta}_{FIM2}$  for  $\theta = 0$ ,  $p_C = 0.4$ ,  $\sigma^2 = 0.1$ , constant sample sizes  $n = 40, 100, 250, 1000$ . The data-generation mechanisms are FIM1 ( $\circ$ ), FIM2 ( $\triangle$ ), RIM1 ( $+$ ), RIM2 ( $\times$ ), and URIM1 ( $\diamond$ ).

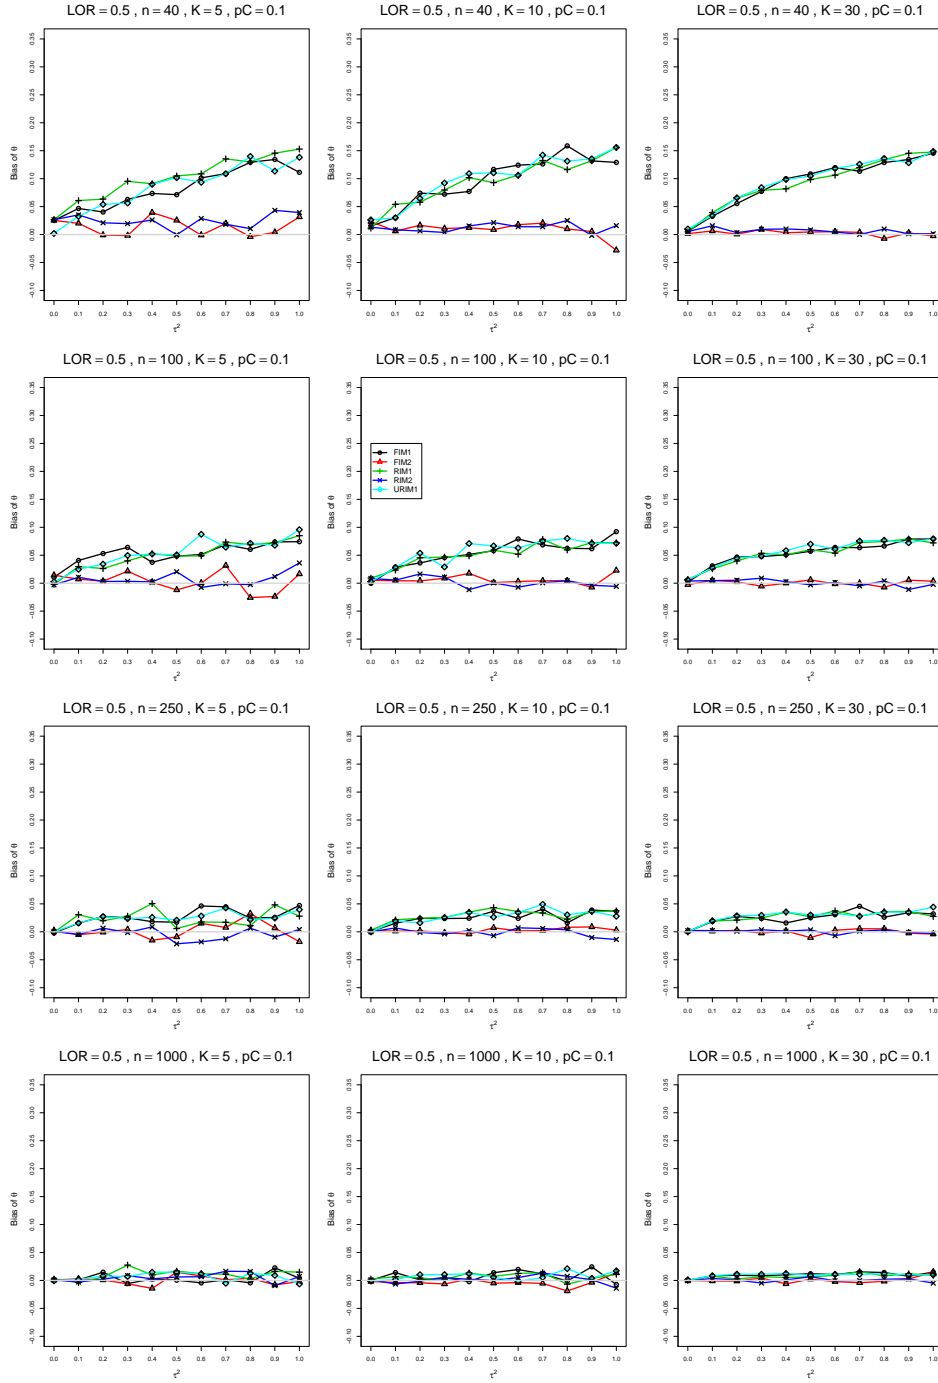

Figure A2.5.3: Bias of overall log-odds ratio  $\hat{\theta}_{FIM2}$  for  $\theta = 0.5$ ,  $p_C = 0.1$ ,  $\sigma^2 = 0.1$ , constant sample sizes  $n = 40, 100, 250, 1000$ . The data-generation mechanisms are FIM1 ( $\circ$ ), FIM2 ( $\triangle$ ), RIM1 (+), RIM2 ( $\times$ ), and URIM1 ( $\diamond$ ).

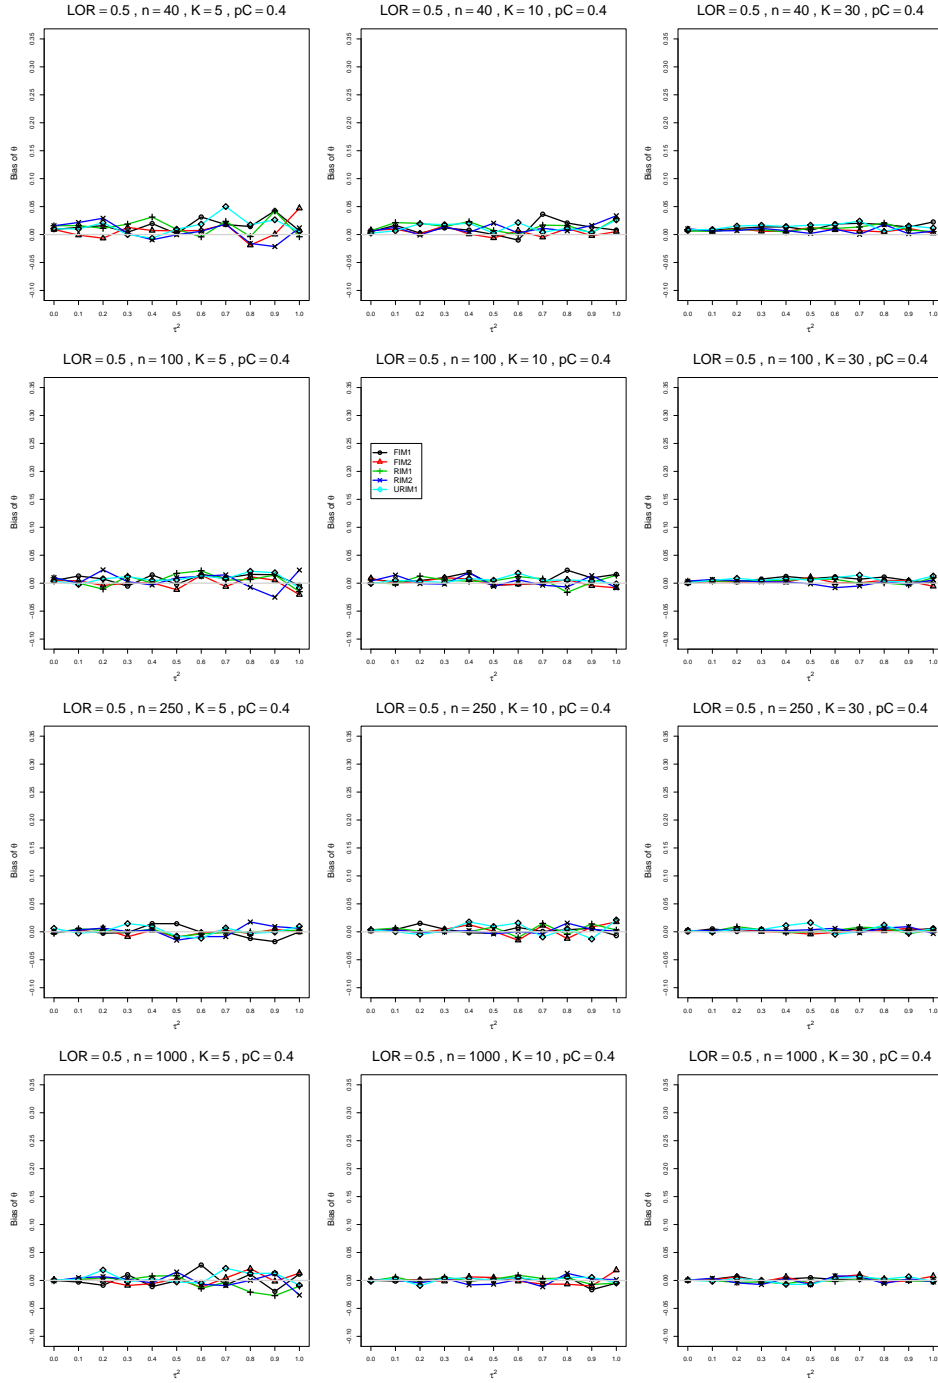

Figure A2.5.4: Bias of overall log-odds ratio  $\hat{\theta}_{FIM2}$  for  $\theta = 0.5$ ,  $p_C = 0.4$ ,  $\sigma^2 = 0.1$ , constant sample sizes  $n = 40, 100, 250, 1000$ . The data-generation mechanisms are FIM1 ( $\circ$ ), FIM2 ( $\triangle$ ), RIM1 ( $+$ ), RIM2 ( $\times$ ), and URIM1 ( $\diamond$ ).

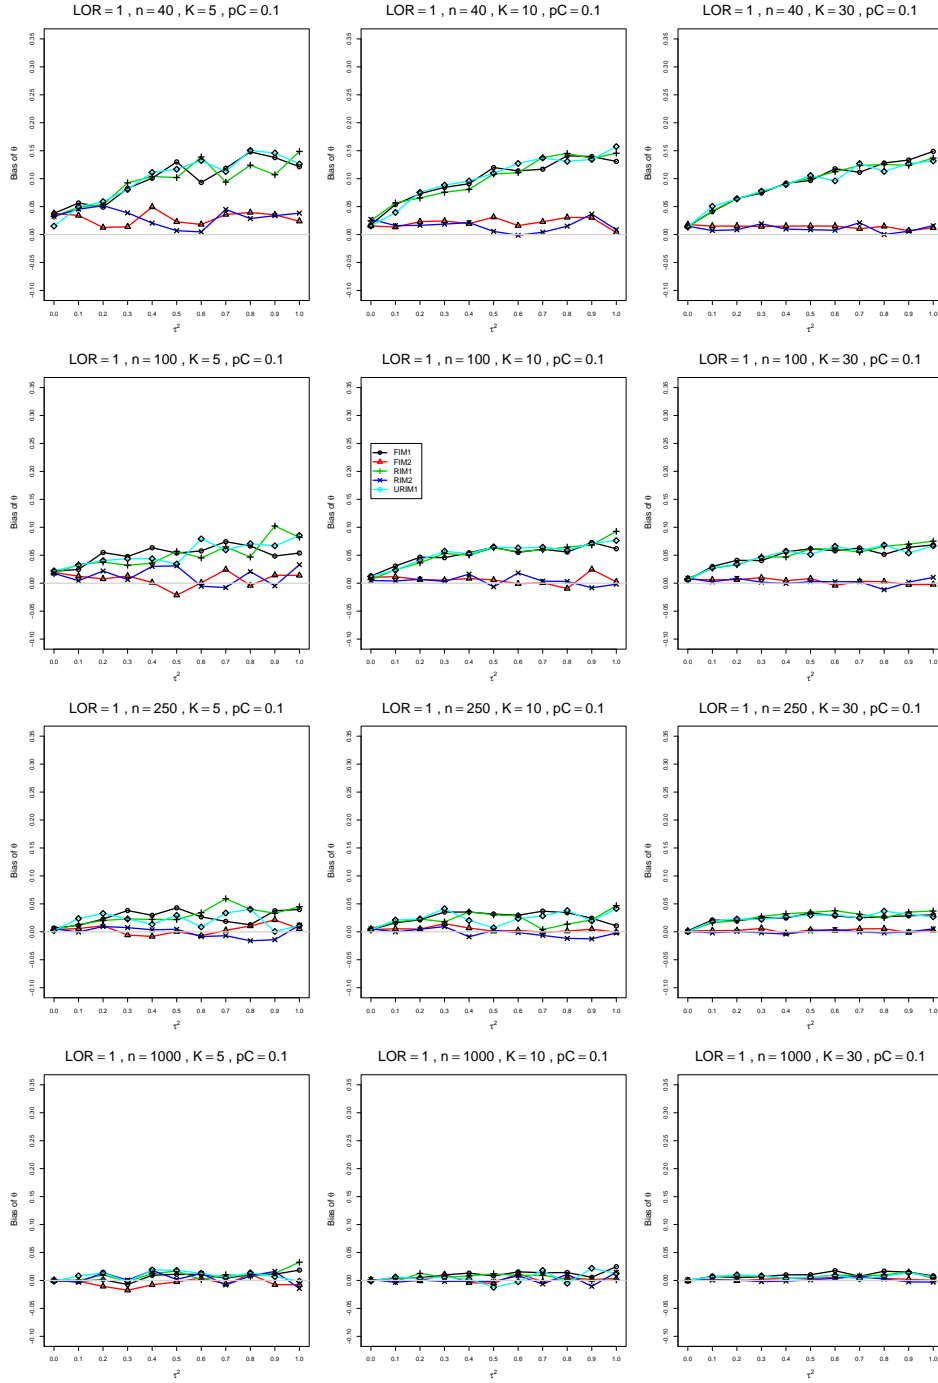

Figure A2.5.5: Bias of overall log-odds ratio  $\hat{\theta}_{FIM2}$  for  $\theta = 1$ ,  $p_C = 0.1$ ,  $\sigma^2 = 0.1$ , constant sample sizes  $n = 40, 100, 250, 1000$ . The data-generation mechanisms are FIM1 ( $\circ$ ), FIM2 ( $\triangle$ ), RIM1 ( $+$ ), RIM2 ( $\times$ ), and URIM1 ( $\diamond$ ).

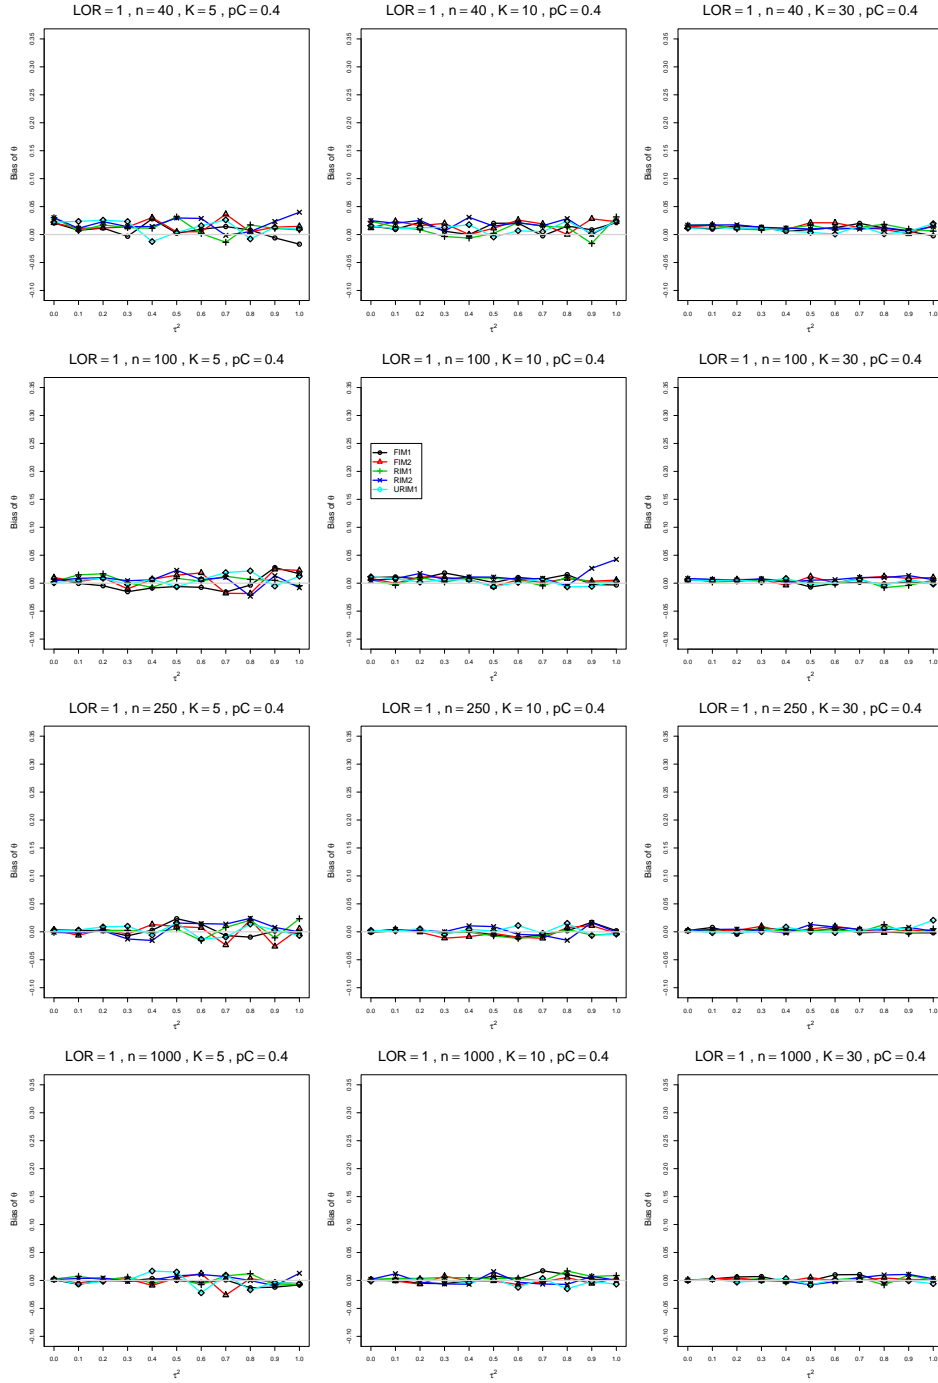

Figure A2.5.6: Bias of overall log-odds ratio  $\hat{\theta}_{FIM2}$  for  $\theta = 1$ ,  $p_C = 0.4$ ,  $\sigma^2 = 0.1$ , constant sample sizes  $n = 40, 100, 250, 1000$ . The data-generation mechanisms are FIM1 ( $\circ$ ), FIM2 ( $\triangle$ ), RIM1 ( $+$ ), RIM2 ( $\times$ ), and URIM1 ( $\diamond$ ).



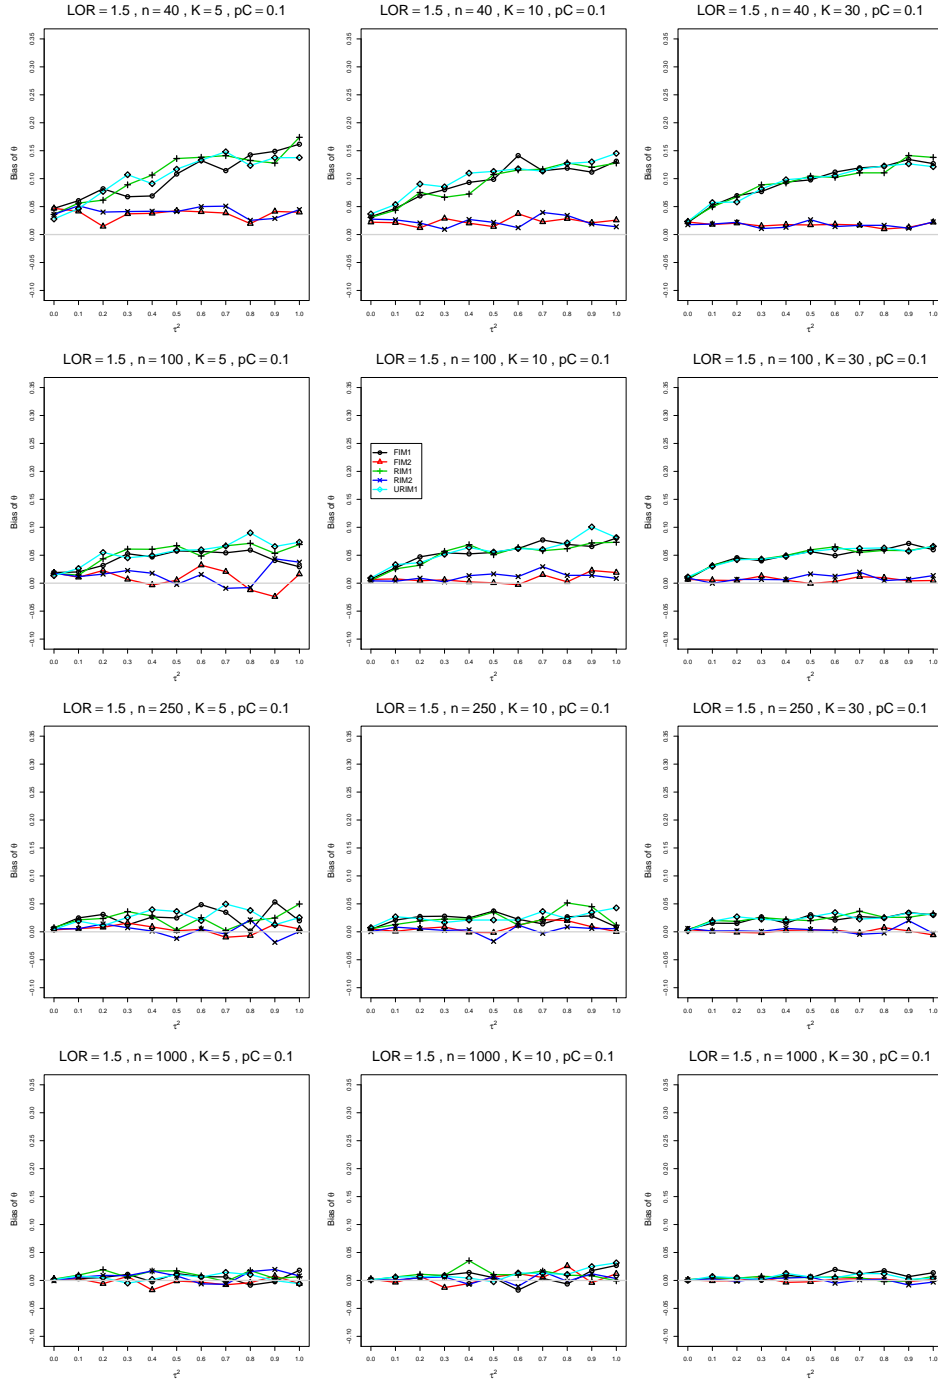

Figure A2.5.7: Bias of overall log-odds ratio  $\hat{\theta}_{FIM2}$  for  $\theta = 1.5$ ,  $p_C = 0.1$ ,  $\sigma^2 = 0.1$ , constant sample sizes  $n = 40, 100, 250, 1000$ . The data-generation mechanisms are FIM1 ( $\circ$ ), FIM2 ( $\triangle$ ), RIM1 ( $+$ ), RIM2 ( $\times$ ), and URIM1 ( $\diamond$ ).

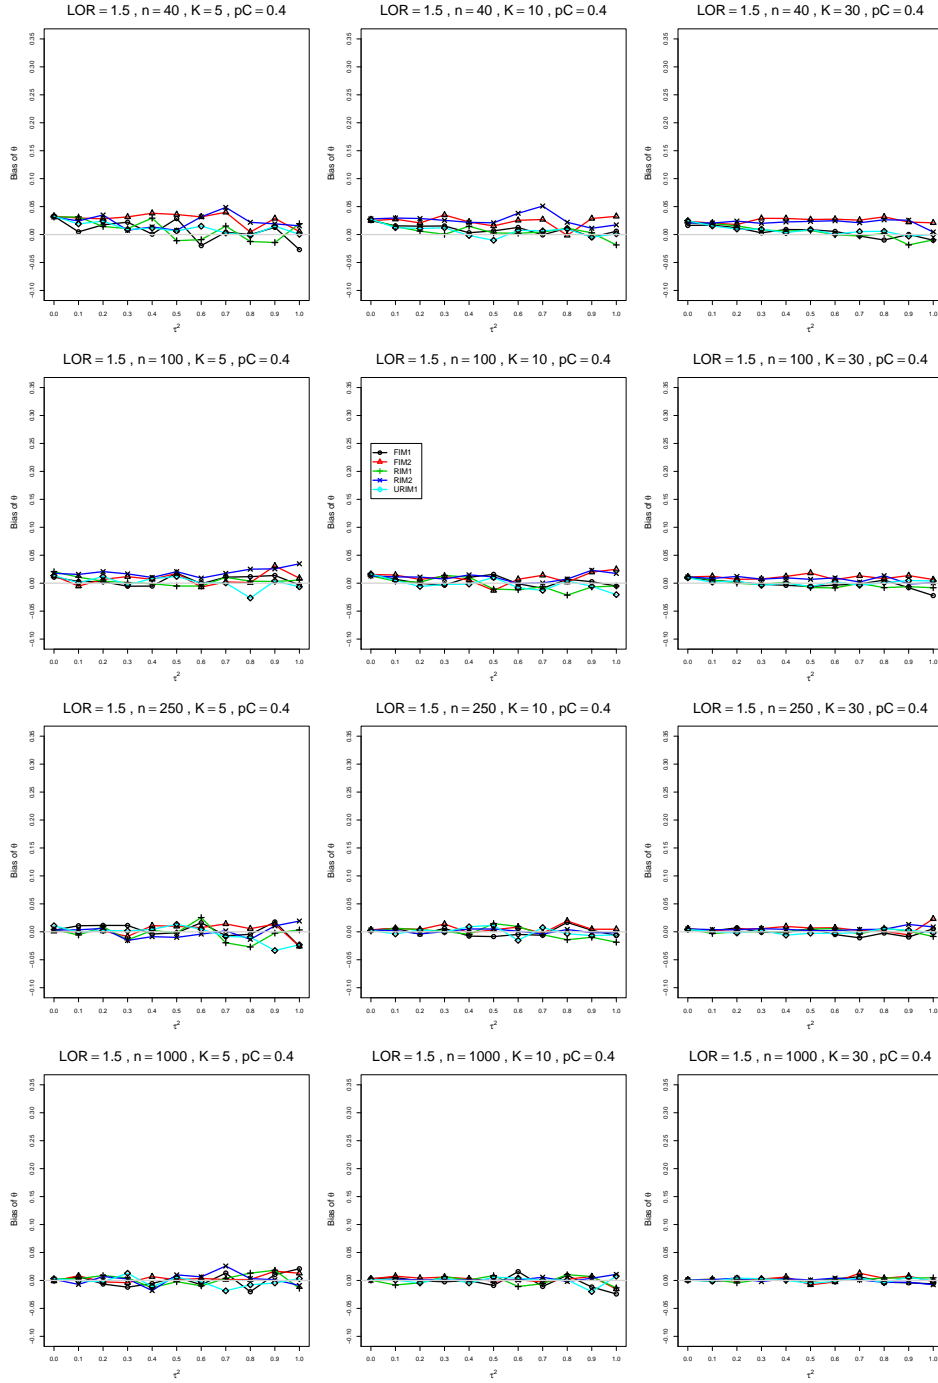

Figure A2.5.8: Bias of overall log-odds ratio  $\hat{\theta}_{FIM2}$  for  $\theta = 1.5$ ,  $p_C = 0.4$ ,  $\sigma^2 = 0.1$ , constant sample sizes  $n = 40, 100, 250, 1000$ . The data-generation mechanisms are FIM1 ( $\circ$ ), FIM2 ( $\triangle$ ), RIM1 ( $+$ ), RIM2 ( $\times$ ), and URIM1 ( $\diamond$ ).

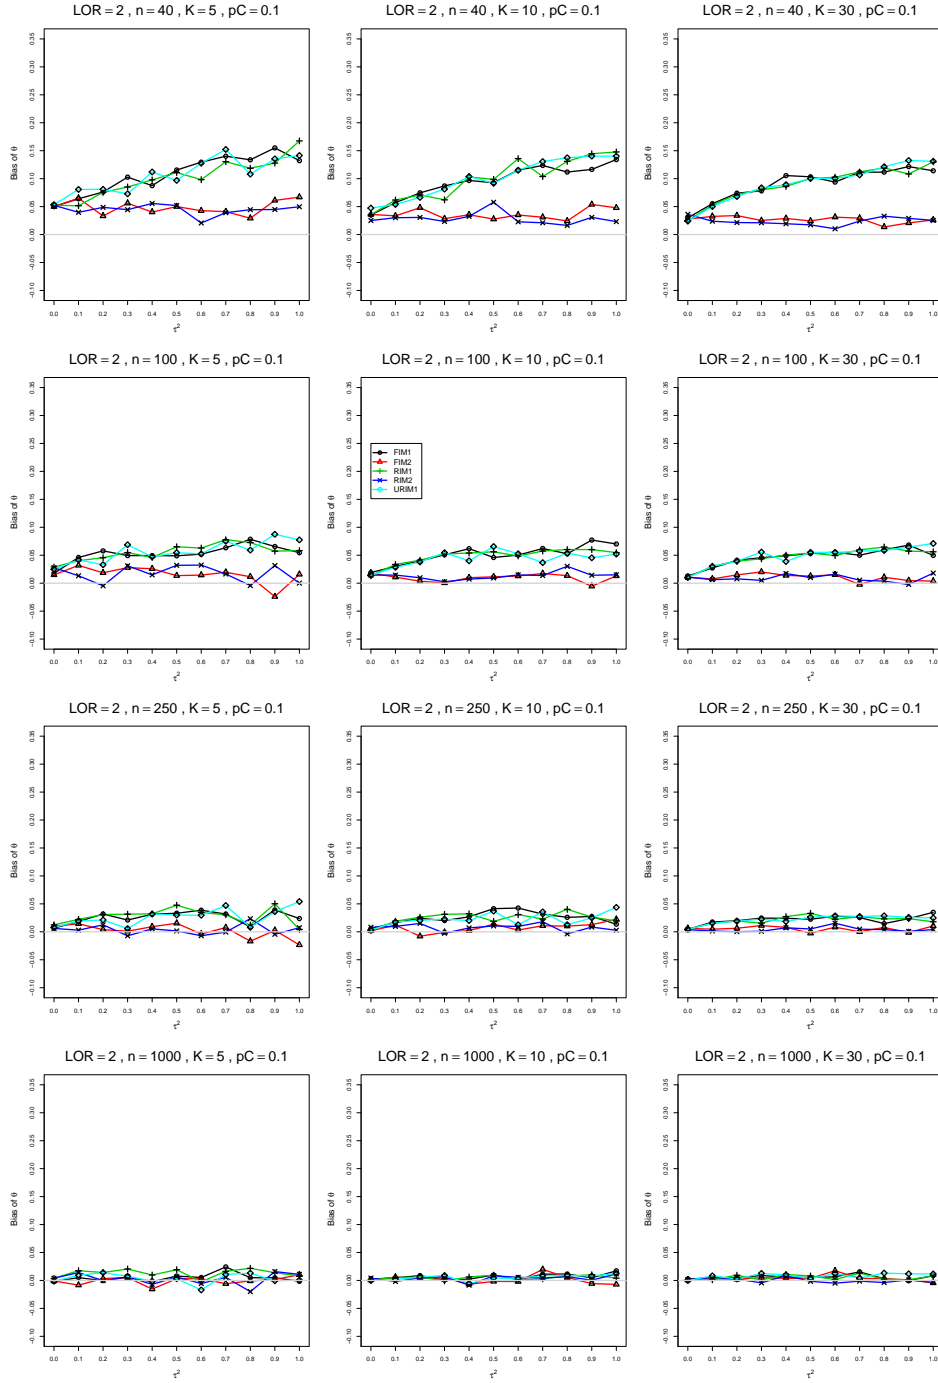

Figure A2.5.9: Bias of overall log-odds ratio  $\hat{\theta}_{FIM2}$  for  $\theta = 2$ ,  $p_C = 0.1$ ,  $\sigma^2 = 0.1$ , constant sample sizes  $n = 40, 100, 250, 1000$ . The data-generation mechanisms are FIM1 ( $\circ$ ), FIM2 ( $\triangle$ ), RIM1 ( $+$ ), RIM2 ( $\times$ ), and URIM1 ( $\diamond$ ).

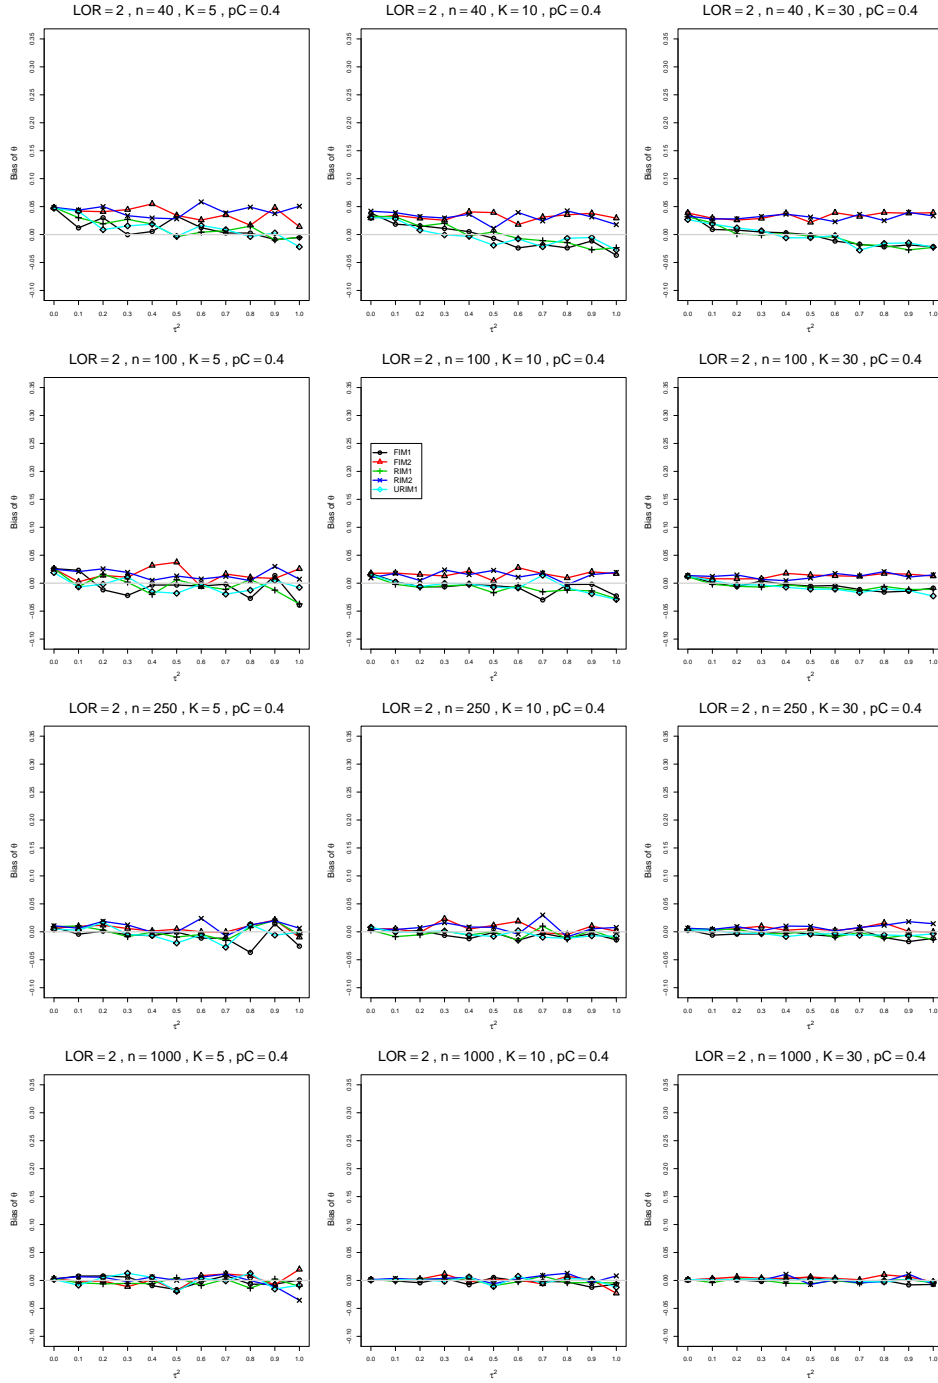

Figure A2.5.10: Bias of overall log-odds ratio  $\hat{\theta}_{FIM2}$  for  $\theta = 2$ ,  $p_C = 0.4$ ,  $\sigma^2 = 0.1$ , constant sample sizes  $n = 40, 100, 250, 1000$ . The data-generation mechanisms are FIM1 ( $\circ$ ), FIM2 ( $\triangle$ ), RIM1 ( $+$ ), RIM2 ( $\times$ ), and URIM1 ( $\diamond$ ).

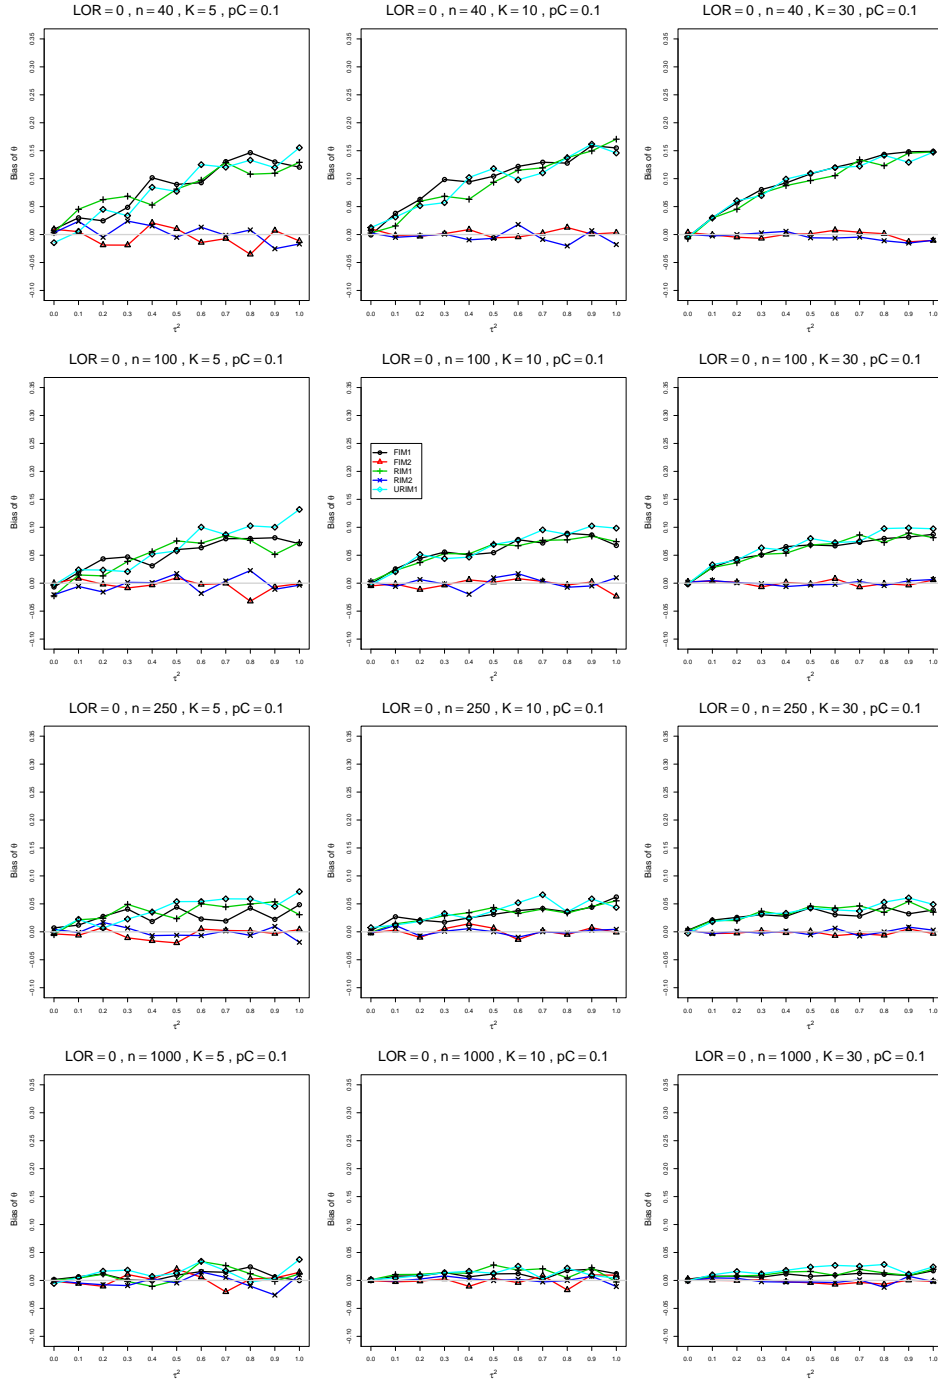

Figure A2.5.11: Bias of overall log-odds ratio  $\hat{\theta}_{FIM2}$  for  $\theta = 0$ ,  $p_C = 0.1$ ,  $\sigma^2 = 0.4$ , constant sample sizes  $n = 40, 100, 250, 1000$ . The data-generation mechanisms are FIM1 ( $\circ$ ), FIM2 ( $\triangle$ ), RIM1 ( $+$ ), RIM2 ( $\times$ ), and URIM1 ( $\diamond$ ).

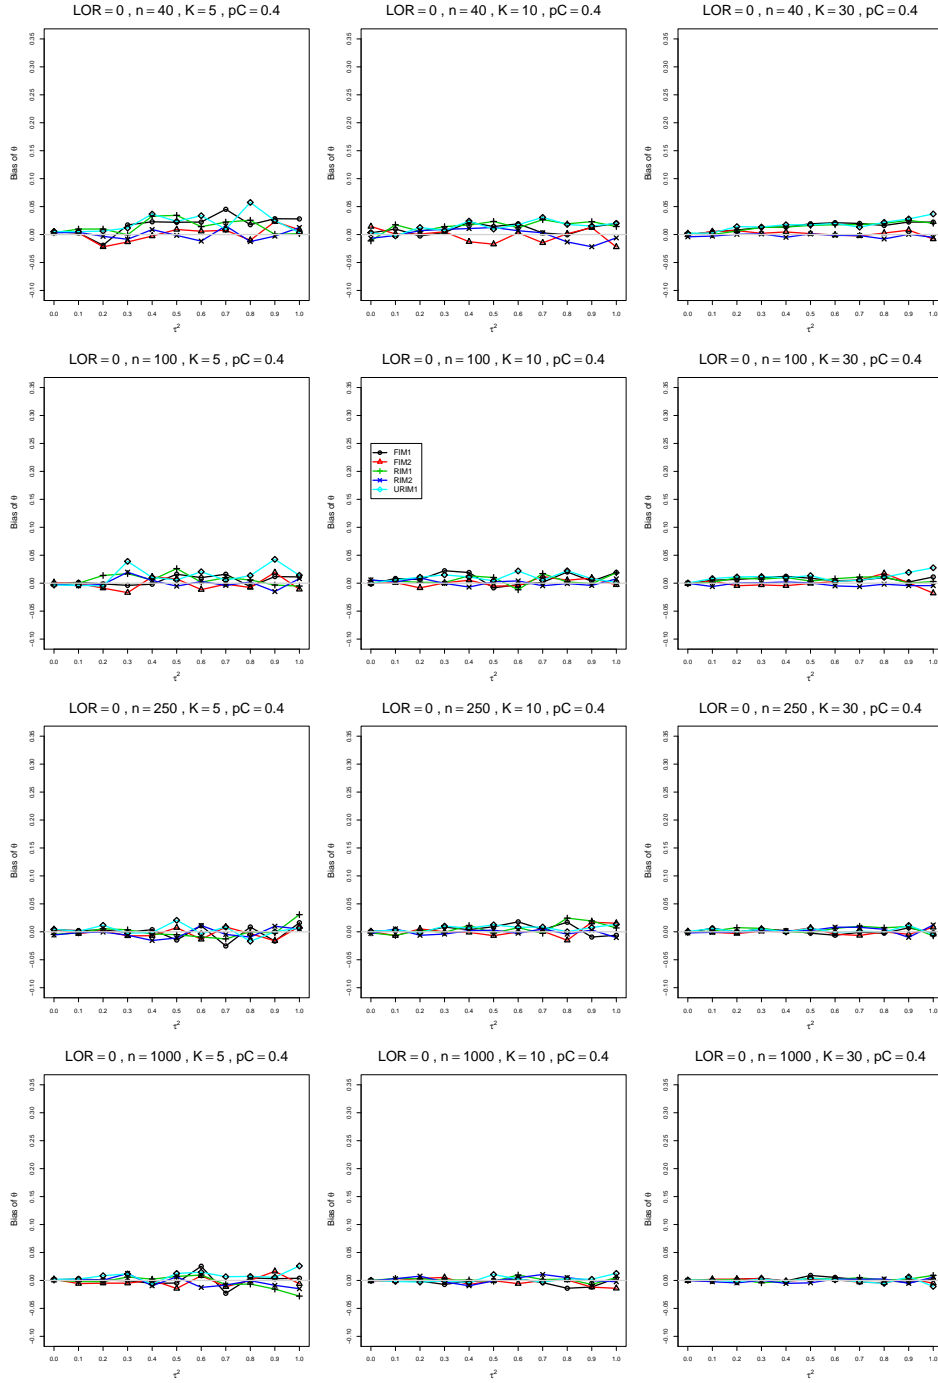

Figure A2.5.12: Bias of overall log-odds ratio  $\hat{\theta}_{FIM2}$  for  $\theta = 0$ ,  $p_C = 0.4$ ,  $\sigma^2 = 0.4$ , constant sample sizes  $n = 40, 100, 250, 1000$ . The data-generation mechanisms are FIM1 ( $\circ$ ), FIM2 ( $\triangle$ ), RIM1 ( $+$ ), RIM2 ( $\times$ ), and URIM1 ( $\diamond$ ).

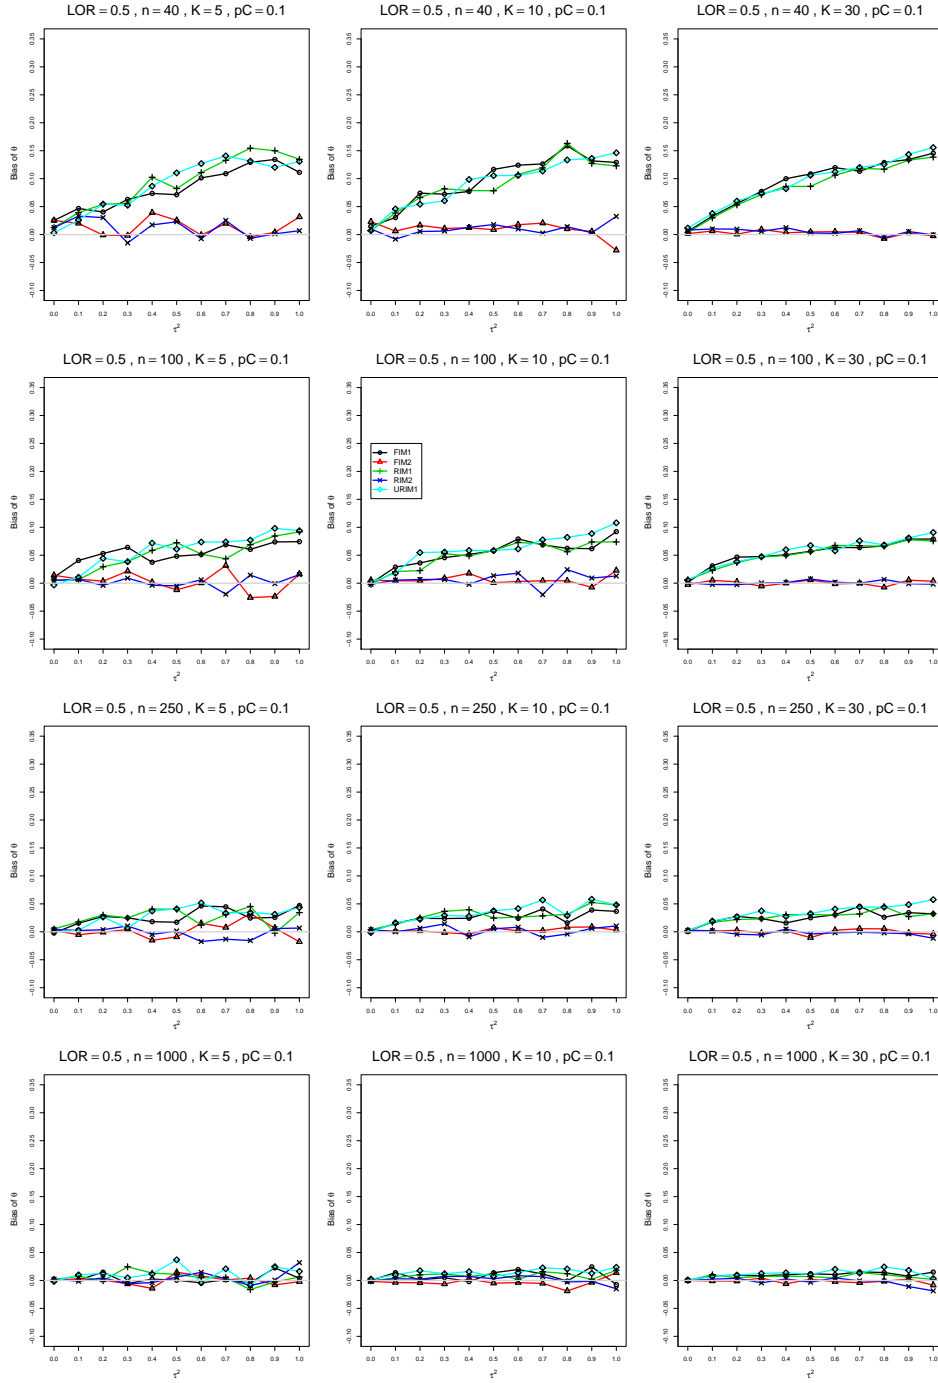

Figure A2.5.13: Bias of overall log-odds ratio  $\hat{\theta}_{FIM2}$  for  $\theta = 0.5$ ,  $p_C = 0.1$ ,  $\sigma^2 = 0.4$ , constant sample sizes  $n = 40, 100, 250, 1000$ . The data-generation mechanisms are FIM1 ( $\circ$ ), FIM2 ( $\triangle$ ), RIM1 ( $+$ ), RIM2 ( $\times$ ), and URIM1 ( $\diamond$ ).

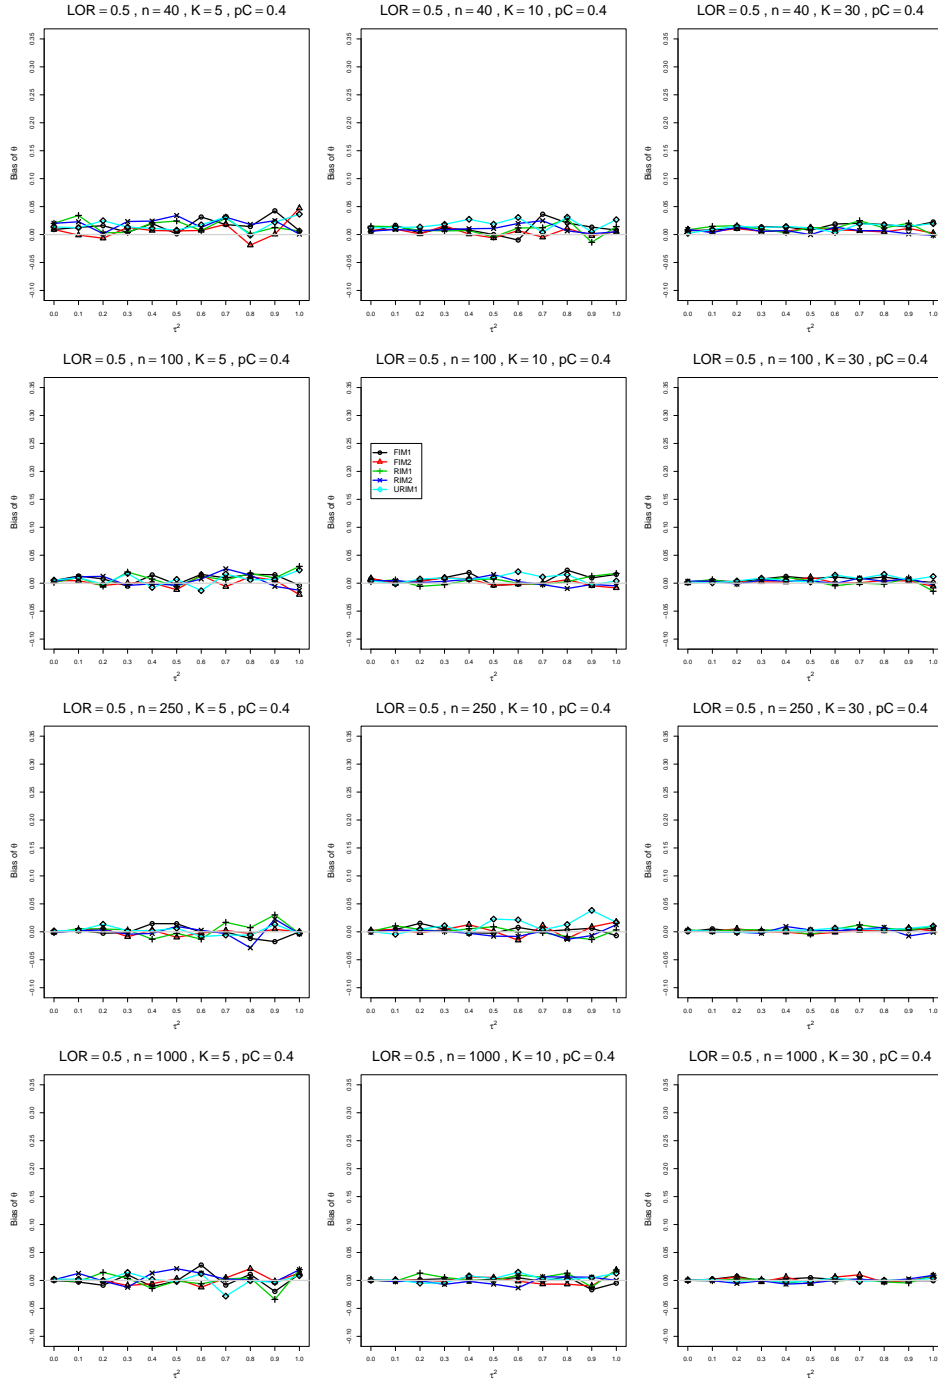

Figure A2.5.14: Bias of overall log-odds ratio  $\hat{\theta}_{FIM2}$  for  $\theta = 0.5$ ,  $p_C = 0.4$ ,  $\sigma^2 = 0.4$ , constant sample sizes  $n = 40, 100, 250, 1000$ . The data-generation mechanisms are FIM1 ( $\circ$ ), FIM2 ( $\triangle$ ), RIM1 ( $+$ ), RIM2 ( $\times$ ), and URIM1 ( $\diamond$ ).



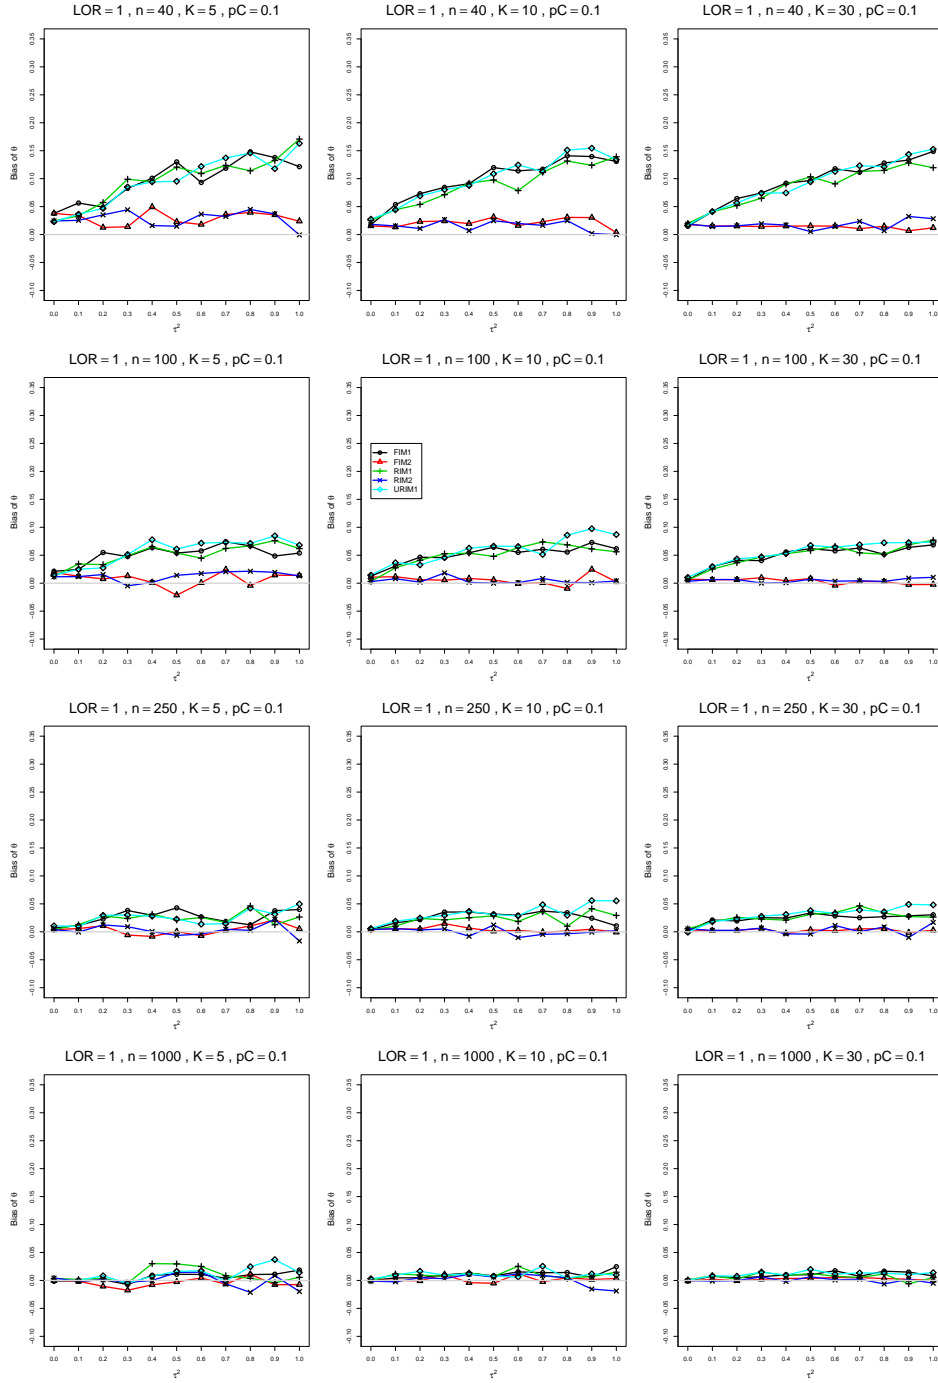

Figure A2.5.15: Bias of overall log-odds ratio  $\hat{\theta}_{FIM2}$  for  $\theta = 1$ ,  $p_C = 0.1$ ,  $\sigma^2 = 0.4$ , constant sample sizes  $n = 40, 100, 250, 1000$ . The data-generation mechanisms are FIM1 ( $\circ$ ), FIM2 ( $\triangle$ ), RIM1 ( $+$ ), RIM2 ( $\times$ ), and URIM1 ( $\diamond$ ).

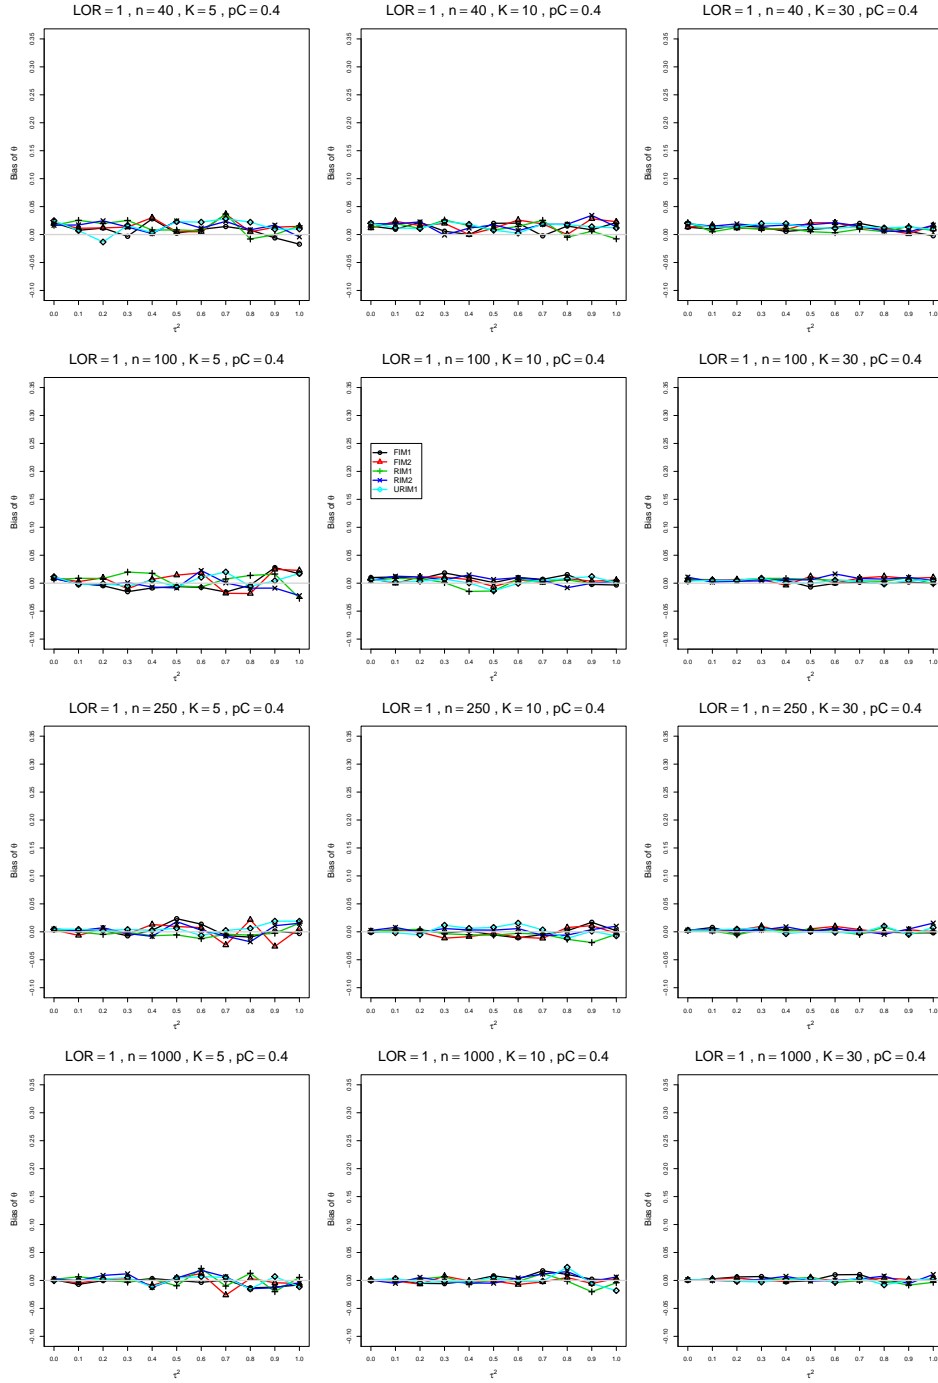

Figure A2.5.16: Bias of overall log-odds ratio  $\hat{\theta}_{FIM2}$  for  $\theta = 1$ ,  $p_C = 0.4$ ,  $\sigma^2 = 0.4$ , constant sample sizes  $n = 40, 100, 250, 1000$ . The data-generation mechanisms are FIM1 ( $\circ$ ), FIM2 ( $\triangle$ ), RIM1 ( $+$ ), RIM2 ( $\times$ ), and URIM1 ( $\diamond$ ).

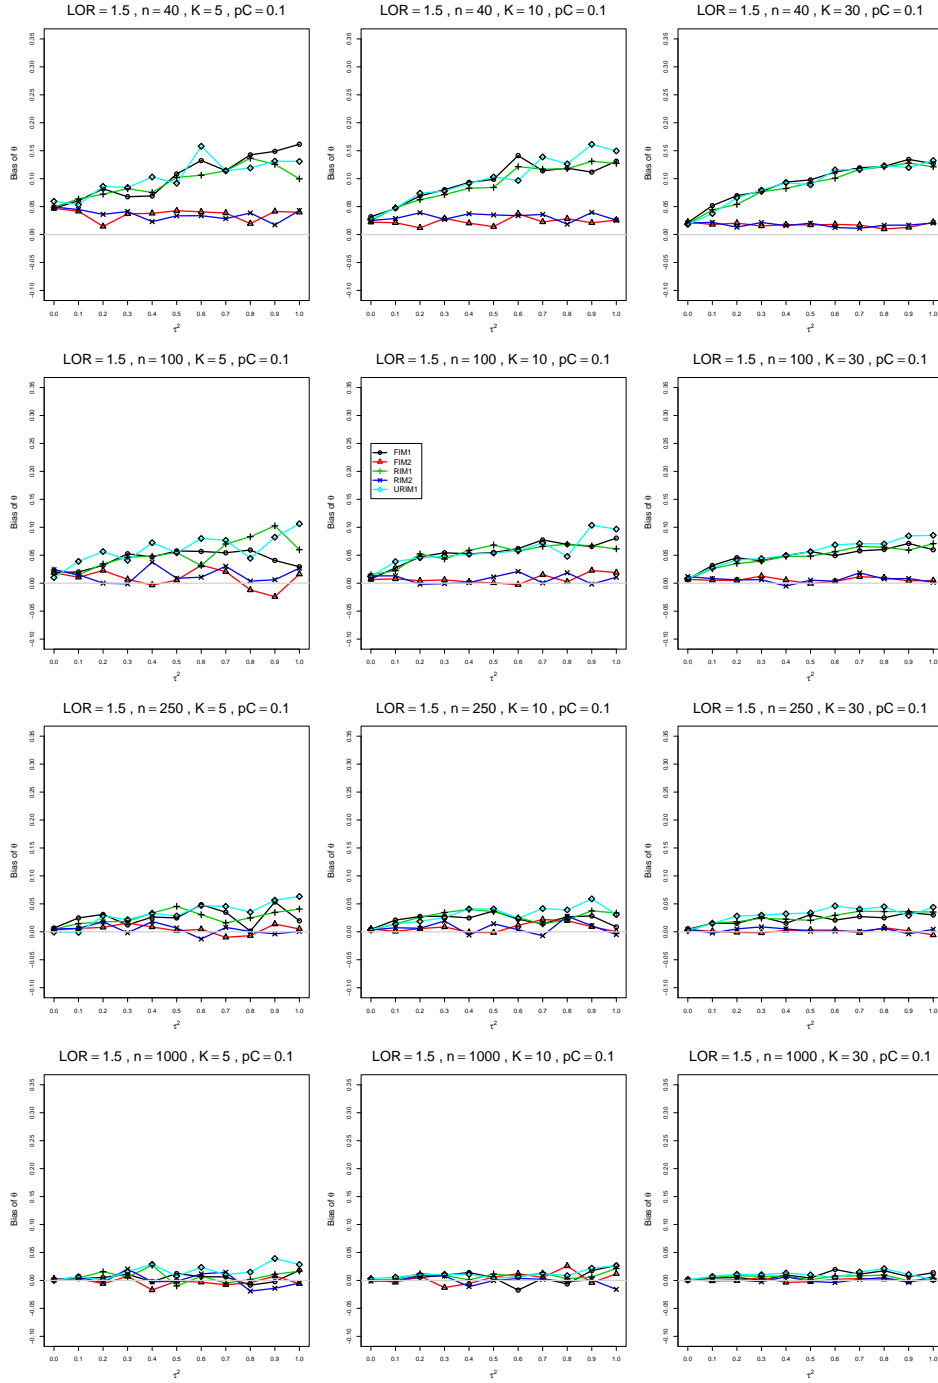

Figure A2.5.17: Bias of overall log-odds ratio  $\hat{\theta}_{FIM2}$  for  $\theta = 1.5$ ,  $p_C = 0.1$ ,  $\sigma^2 = 0.4$ , constant sample sizes  $n = 40, 100, 250, 1000$ . The data-generation mechanisms are FIM1 ( $\circ$ ), FIM2 ( $\triangle$ ), RIM1 ( $+$ ), RIM2 ( $\times$ ), and URIM1 ( $\diamond$ ).

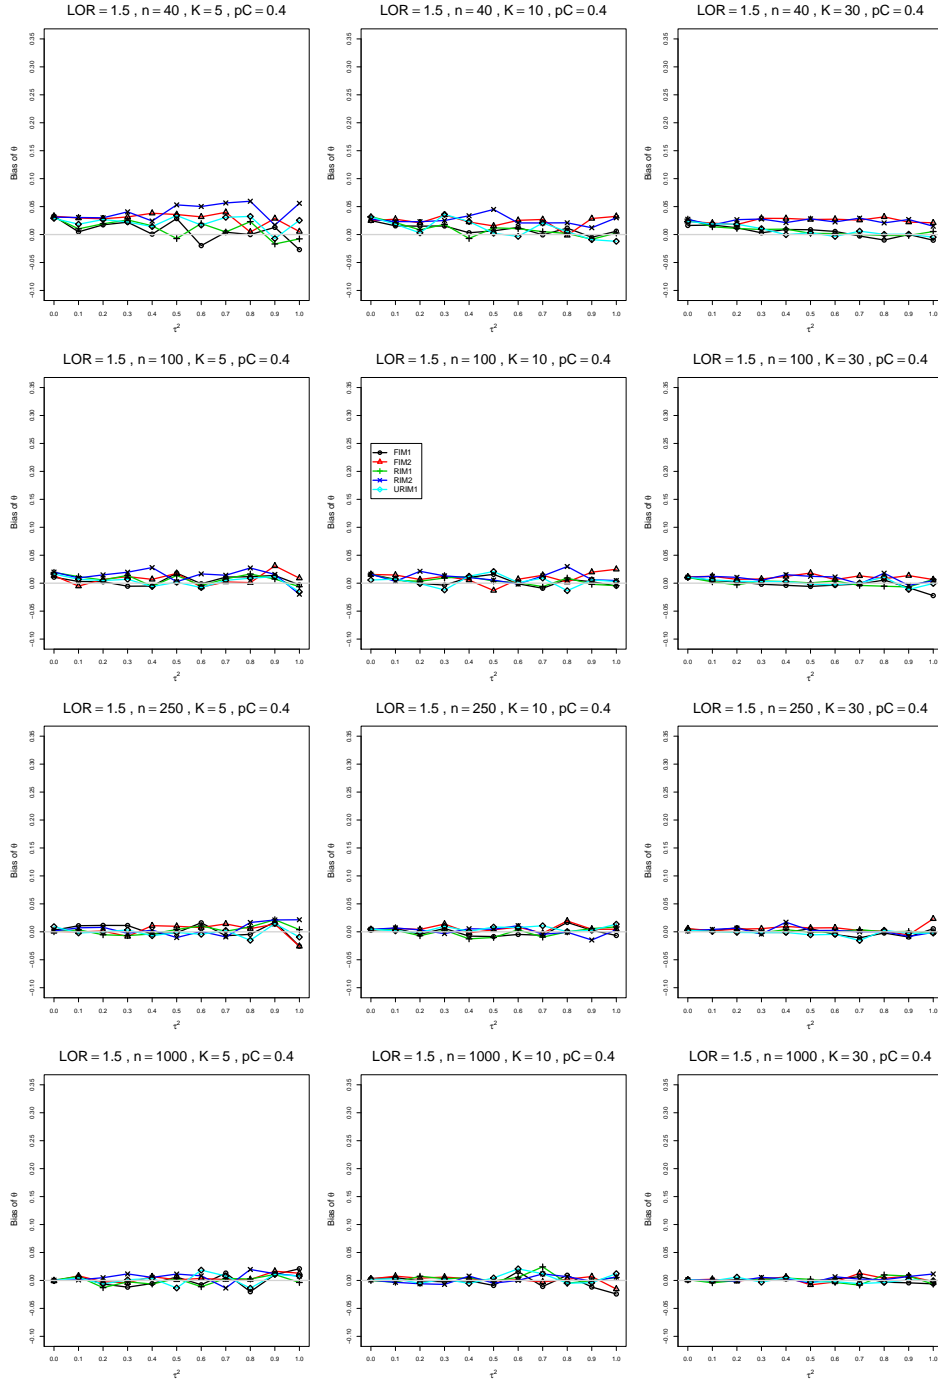

Figure A2.5.18: Bias of overall log-odds ratio  $\hat{\theta}_{FIM2}$  for  $\theta = 1.5$ ,  $p_C = 0.4$ ,  $\sigma^2 = 0.4$ , constant sample sizes  $n = 40, 100, 250, 1000$ . The data-generation mechanisms are FIM1 ( $\circ$ ), FIM2 ( $\triangle$ ), RIM1 ( $+$ ), RIM2 ( $\times$ ), and URIM1 ( $\diamond$ ).

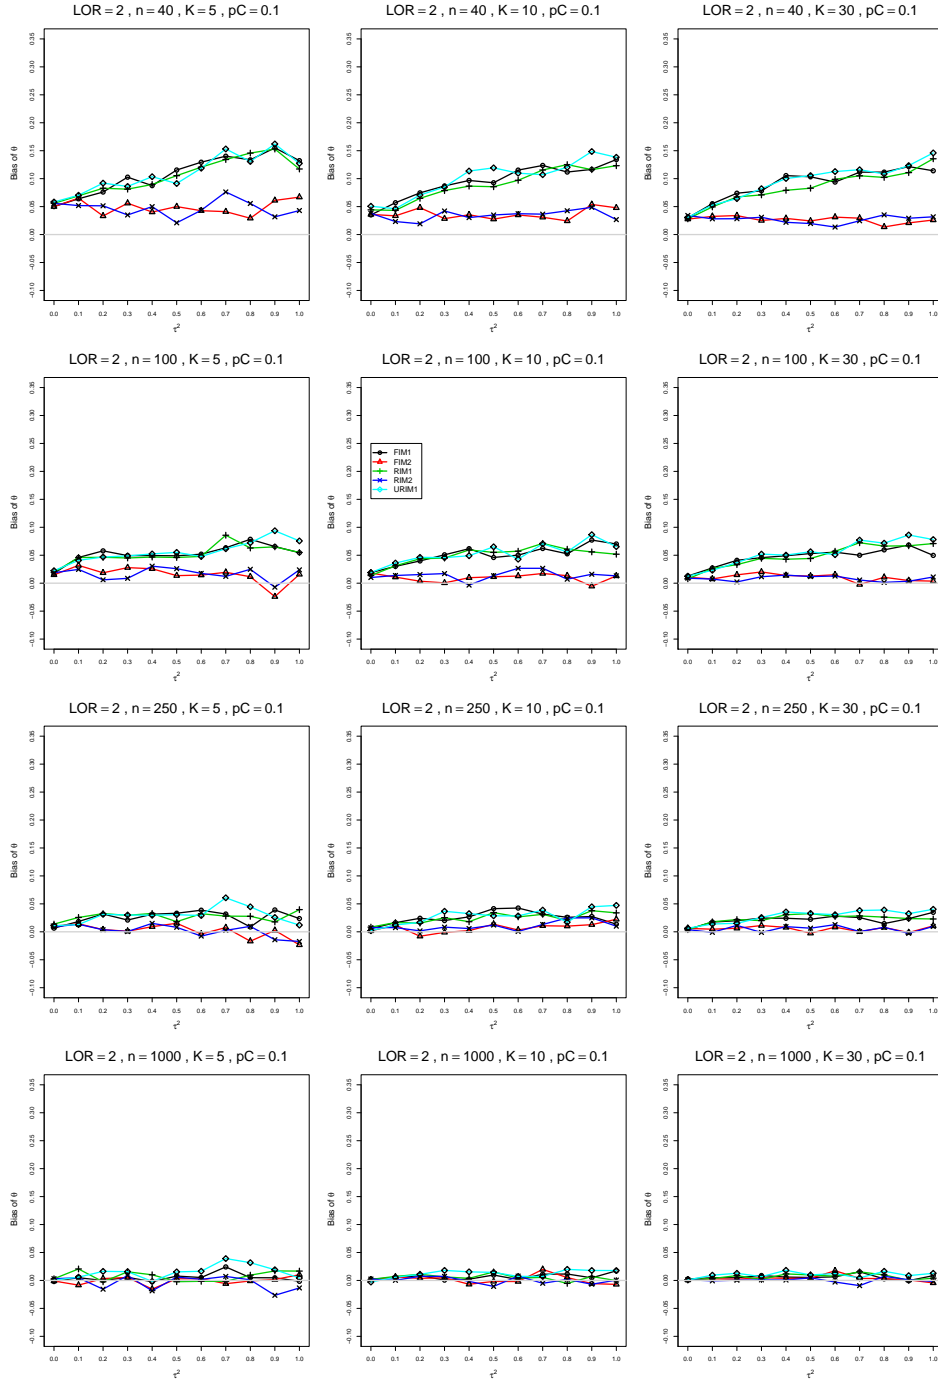

Figure A2.5.19: Bias of overall log-odds ratio  $\hat{\theta}_{FIM2}$  for  $\theta = 2$ ,  $p_C = 0.1$ ,  $\sigma^2 = 0.4$ , constant sample sizes  $n = 40, 100, 250, 1000$ . The data-generation mechanisms are FIM1 ( $\circ$ ), FIM2 ( $\triangle$ ), RIM1 ( $+$ ), RIM2 ( $\times$ ), and URIM1 ( $\diamond$ ).

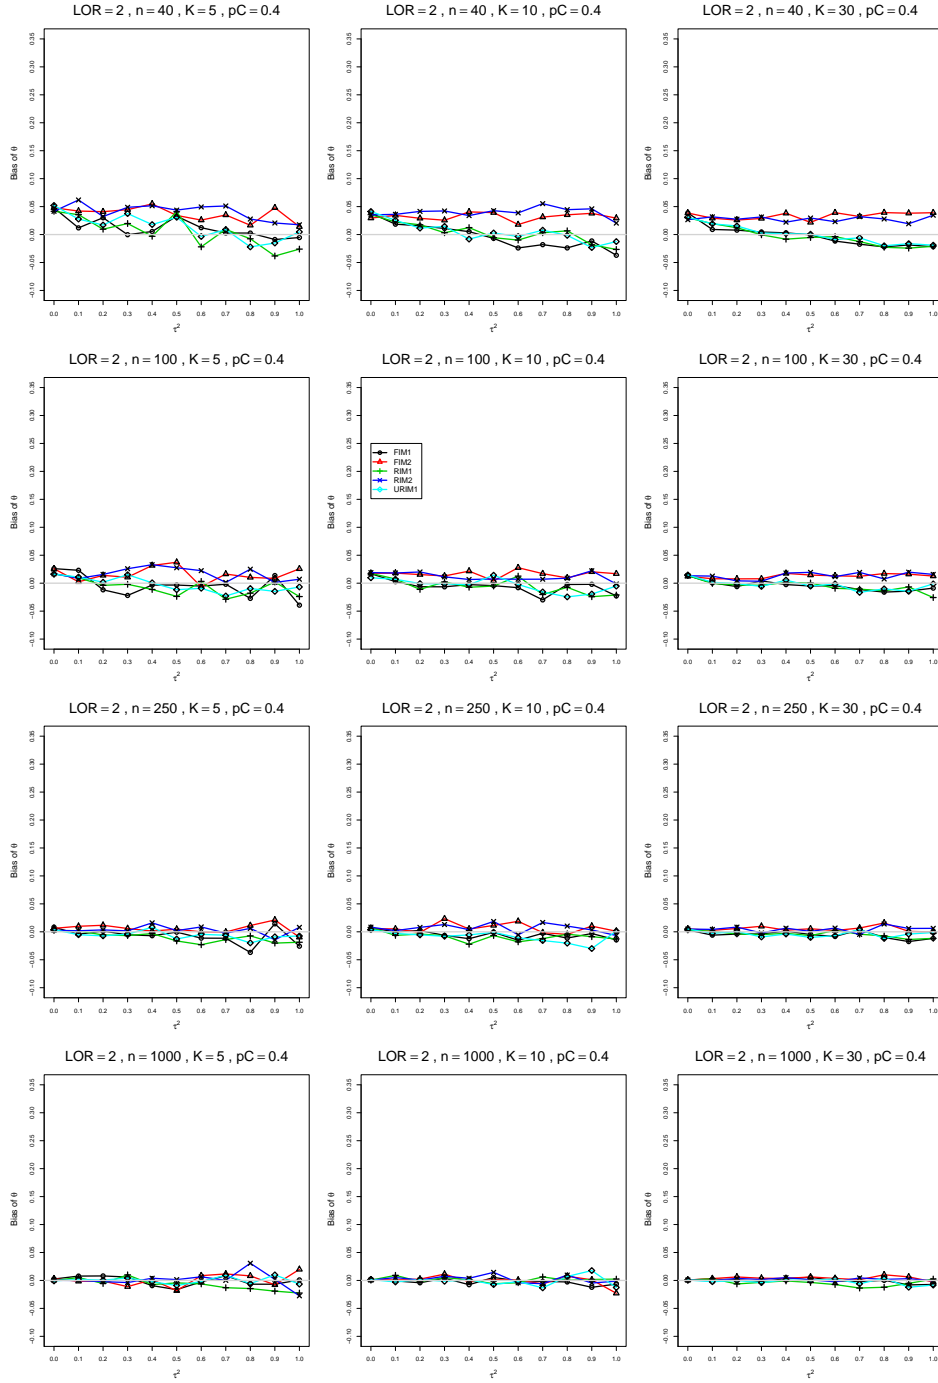

Figure A2.5.20: Bias of overall log-odds ratio  $\hat{\theta}_{FIM2}$  for  $\theta = 2$ ,  $p_C = 0.4$ ,  $\sigma^2 = 0.4$ , constant sample sizes  $n = 40, 100, 250, 1000$ . The data-generation mechanisms are FIM1 ( $\circ$ ), FIM2 ( $\triangle$ ), RIM1 ( $+$ ), RIM2 ( $\times$ ), and URIM1 ( $\diamond$ ).

## A2.6 Bias of $\hat{\theta}_{RIM2}$

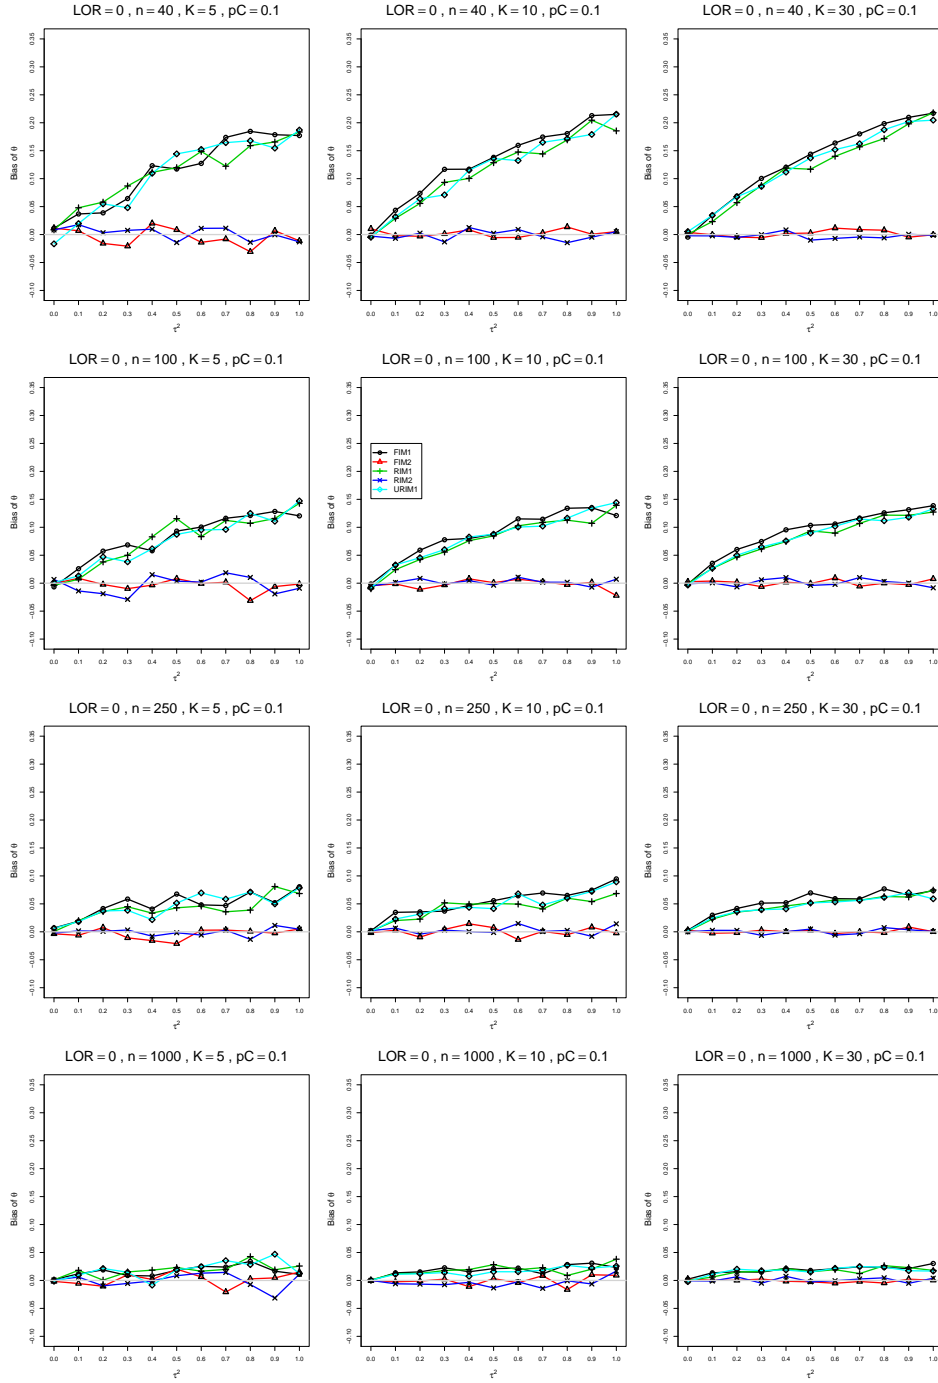

Figure A2.6.1: Bias of overall log-odds ratio  $\hat{\theta}_{RIM2}$  for  $\theta = 0$ ,  $p_C = 0.1$ ,  $\sigma^2 = 0.1$ , constant sample sizes  $n = 40, 100, 250, 1000$ . The data-generation mechanisms are FIM1 ( $\circ$ ), FIM2 ( $\triangle$ ), RIM1 ( $+$ ), RIM2 ( $\times$ ), and URIM1 ( $\diamond$ ).



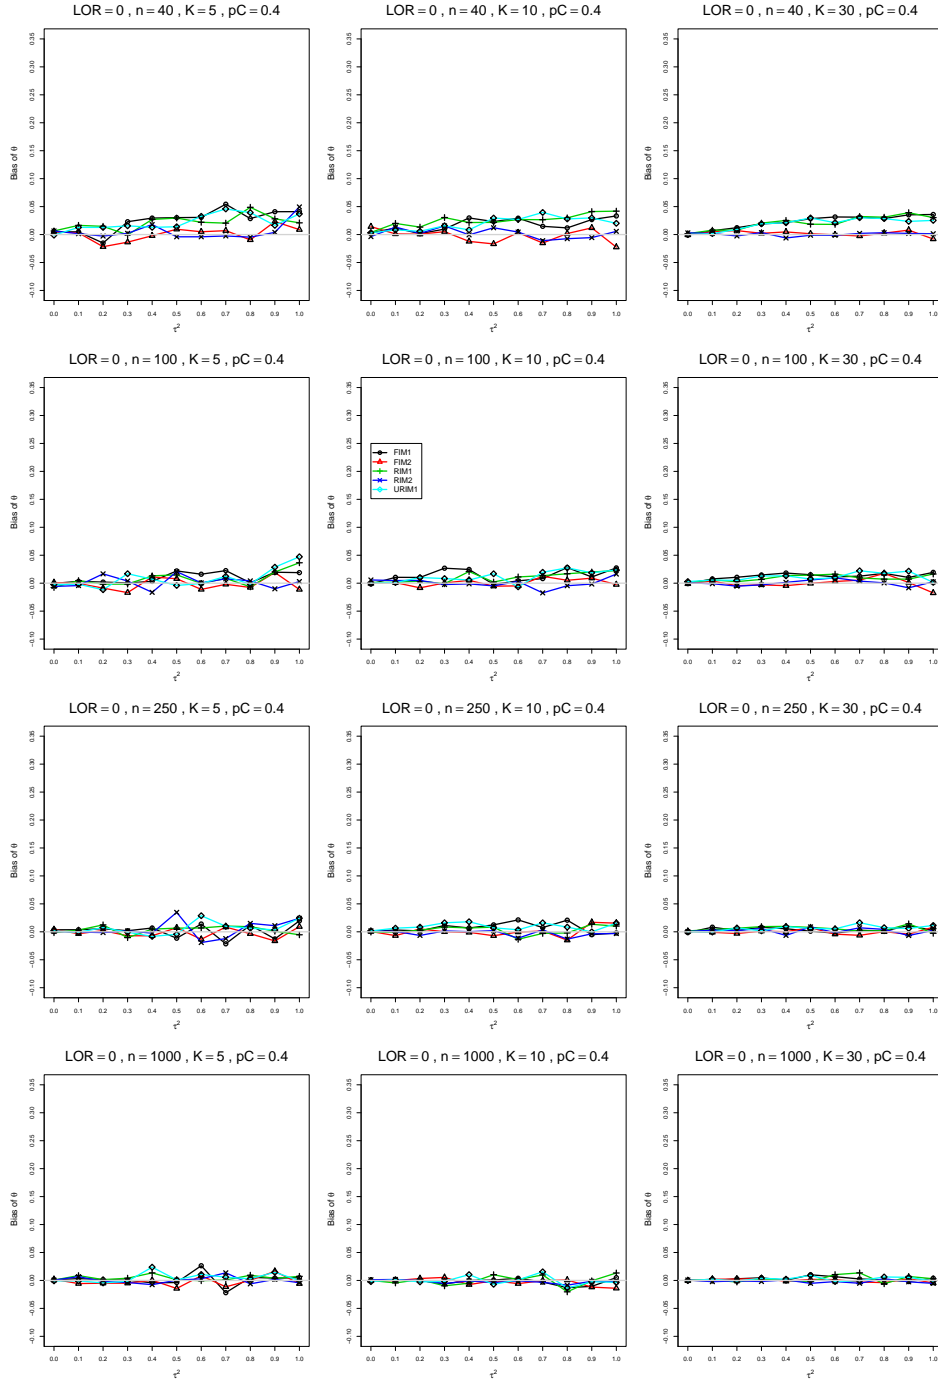

Figure A2.6.2: Bias of overall log-odds ratio  $\hat{\theta}_{RIM2}$  for  $\theta = 0$ ,  $p_C = 0.4$ ,  $\sigma^2 = 0.1$ , constant sample sizes  $n = 40, 100, 250, 1000$ . The data-generation mechanisms are FIM1 ( $\circ$ ), FIM2 ( $\triangle$ ), RIM1 ( $+$ ), RIM2 ( $\times$ ), and URIM1 ( $\diamond$ ).

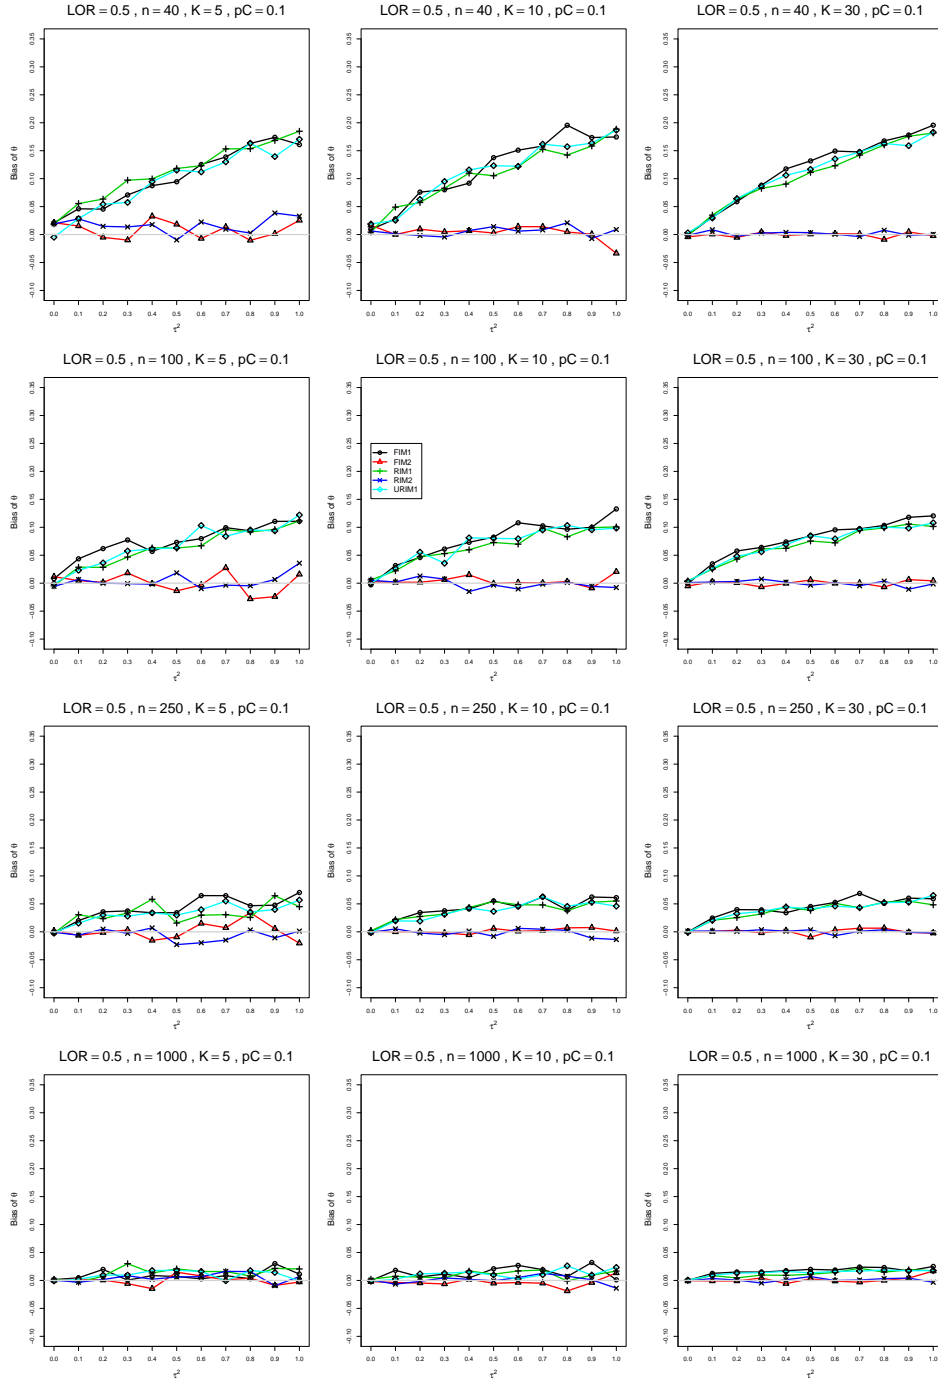

Figure A2.6.3: Bias of overall log-odds ratio  $\hat{\theta}_{RIM2}$  for  $\theta = 0.5$ ,  $p_C = 0.1$ ,  $\sigma^2 = 0.1$ , constant sample sizes  $n = 40, 100, 250, 1000$ . The data-generation mechanisms are FIM1 ( $\circ$ ), FIM2 ( $\triangle$ ), RIM1 ( $+$ ), RIM2 ( $\times$ ), and URIM1 ( $\diamond$ ).

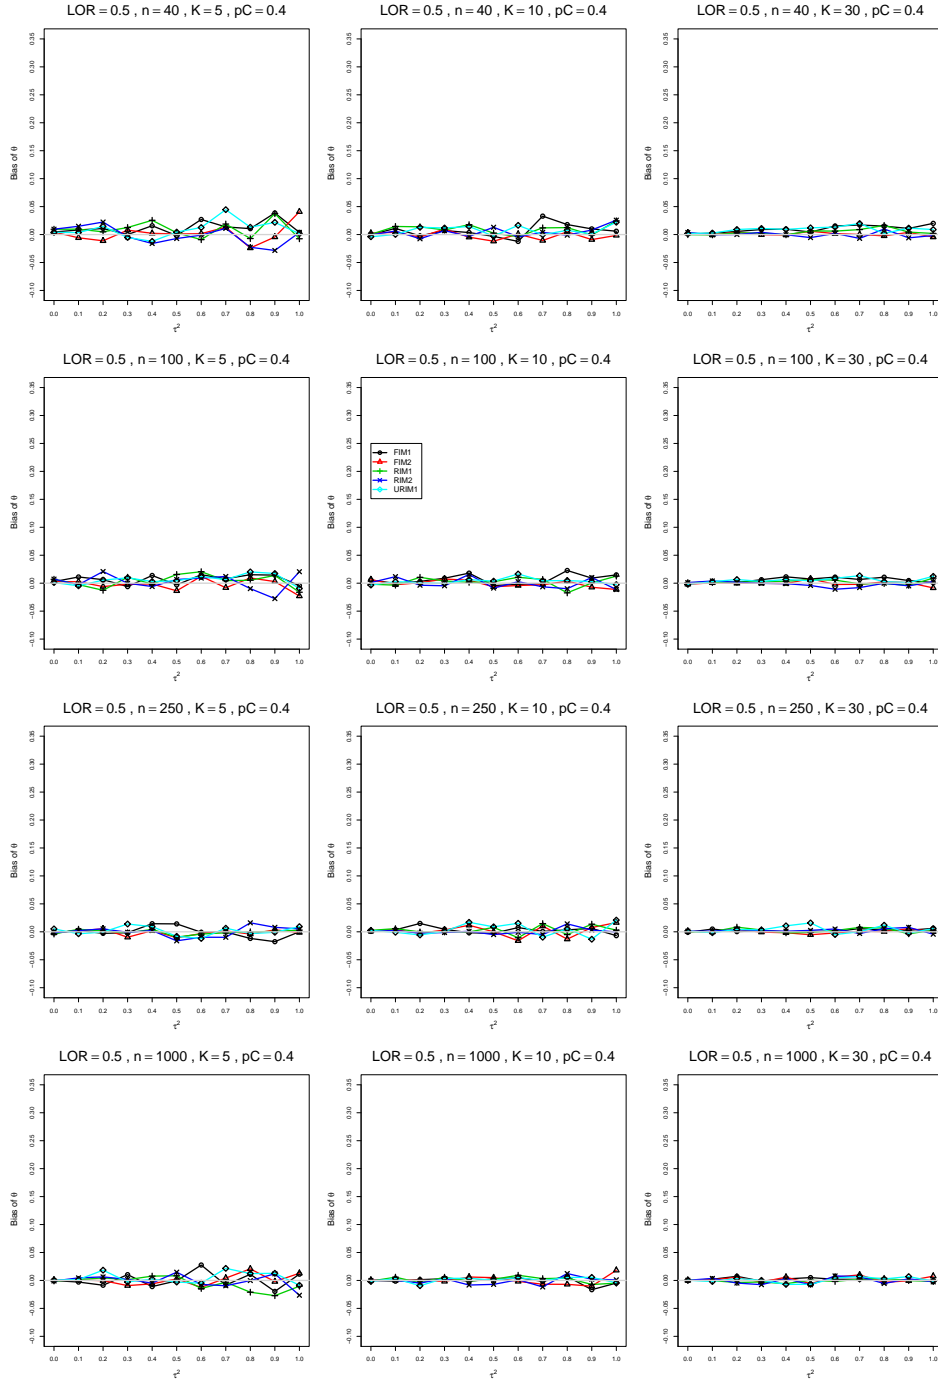

Figure A2.6.4: Bias of overall log-odds ratio  $\hat{\theta}_{RIM2}$  for  $\theta = 0.5$ ,  $p_C = 0.4$ ,  $\sigma^2 = 0.1$ , constant sample sizes  $n = 40, 100, 250, 1000$ . The data-generation mechanisms are FIM1 ( $\circ$ ), FIM2 ( $\triangle$ ), RIM1 ( $+$ ), RIM2 ( $\times$ ), and URIM1 ( $\diamond$ ).

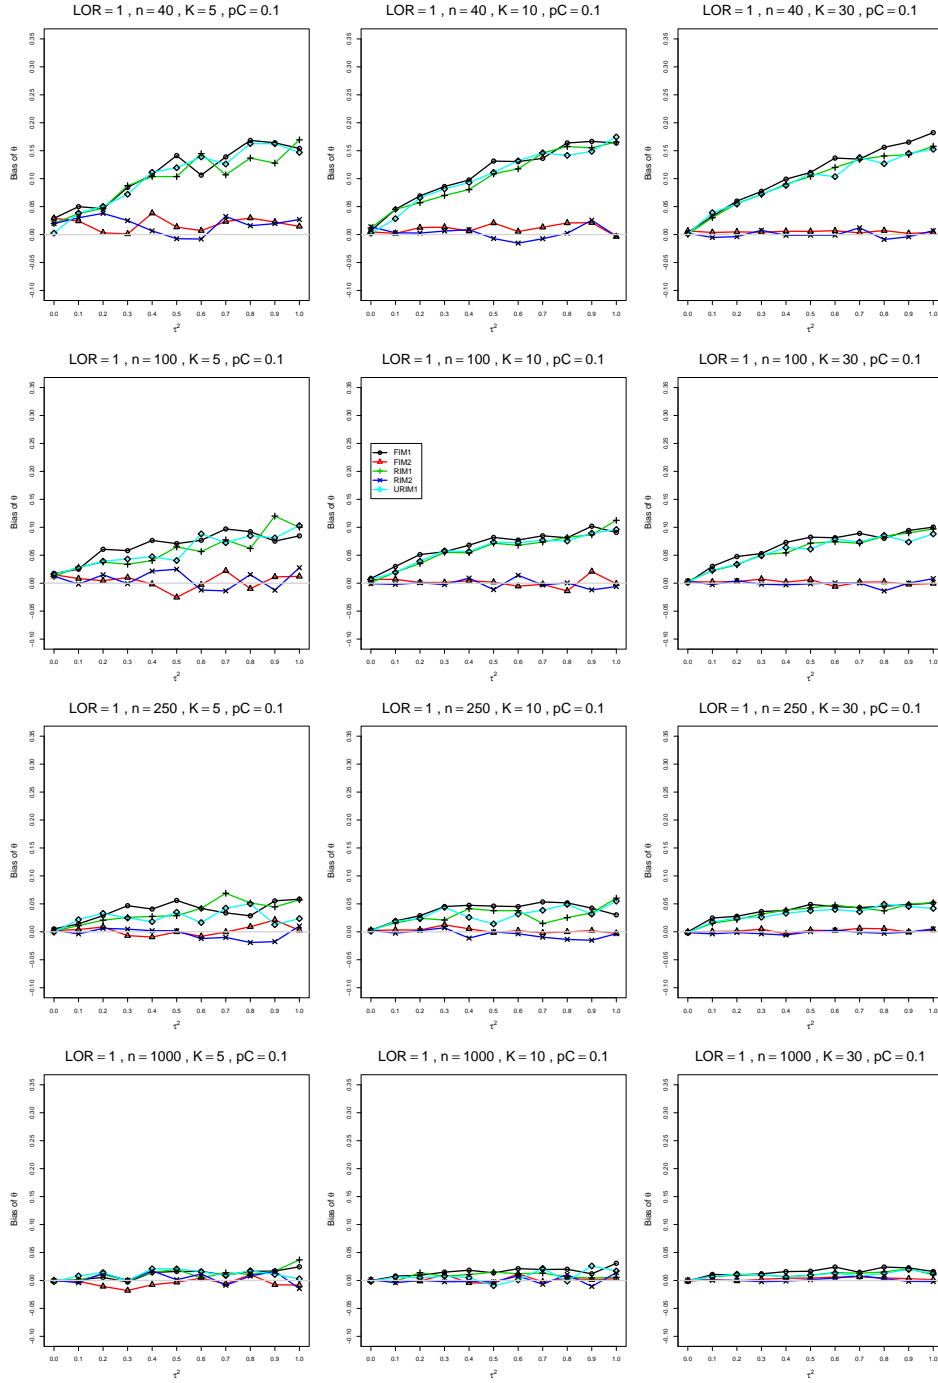

Figure A2.6.5: Bias of overall log-odds ratio  $\hat{\theta}_{RIM2}$  for  $\theta = 1$ ,  $p_C = 0.1$ ,  $\sigma^2 = 0.1$ , constant sample sizes  $n = 40, 100, 250, 1000$ . The data-generation mechanisms are FIM1 ( $\circ$ ), FIM2 ( $\triangle$ ), RIM1 ( $+$ ), RIM2 ( $\times$ ), and URIM1 ( $\diamond$ ).

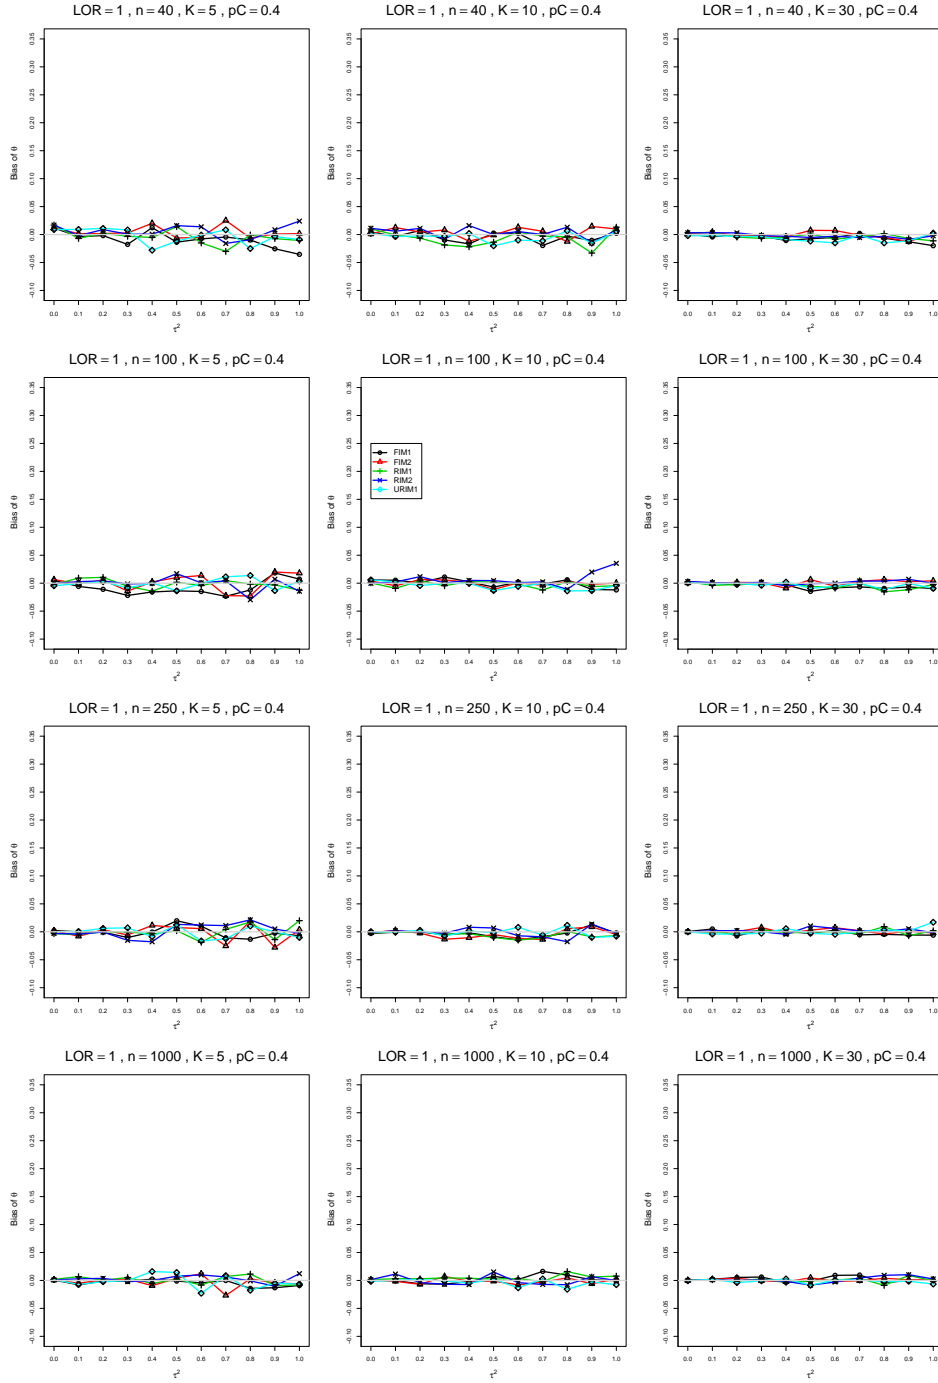

Figure A2.6.6: Bias of overall log-odds ratio  $\hat{\theta}_{RIM2}$  for  $\theta = 1$ ,  $p_C = 0.4$ ,  $\sigma^2 = 0.1$ , constant sample sizes  $n = 40, 100, 250, 1000$ . The data-generation mechanisms are FIM1 ( $\circ$ ), FIM2 ( $\triangle$ ), RIM1 ( $+$ ), RIM2 ( $\times$ ), and URIM1 ( $\diamond$ ).

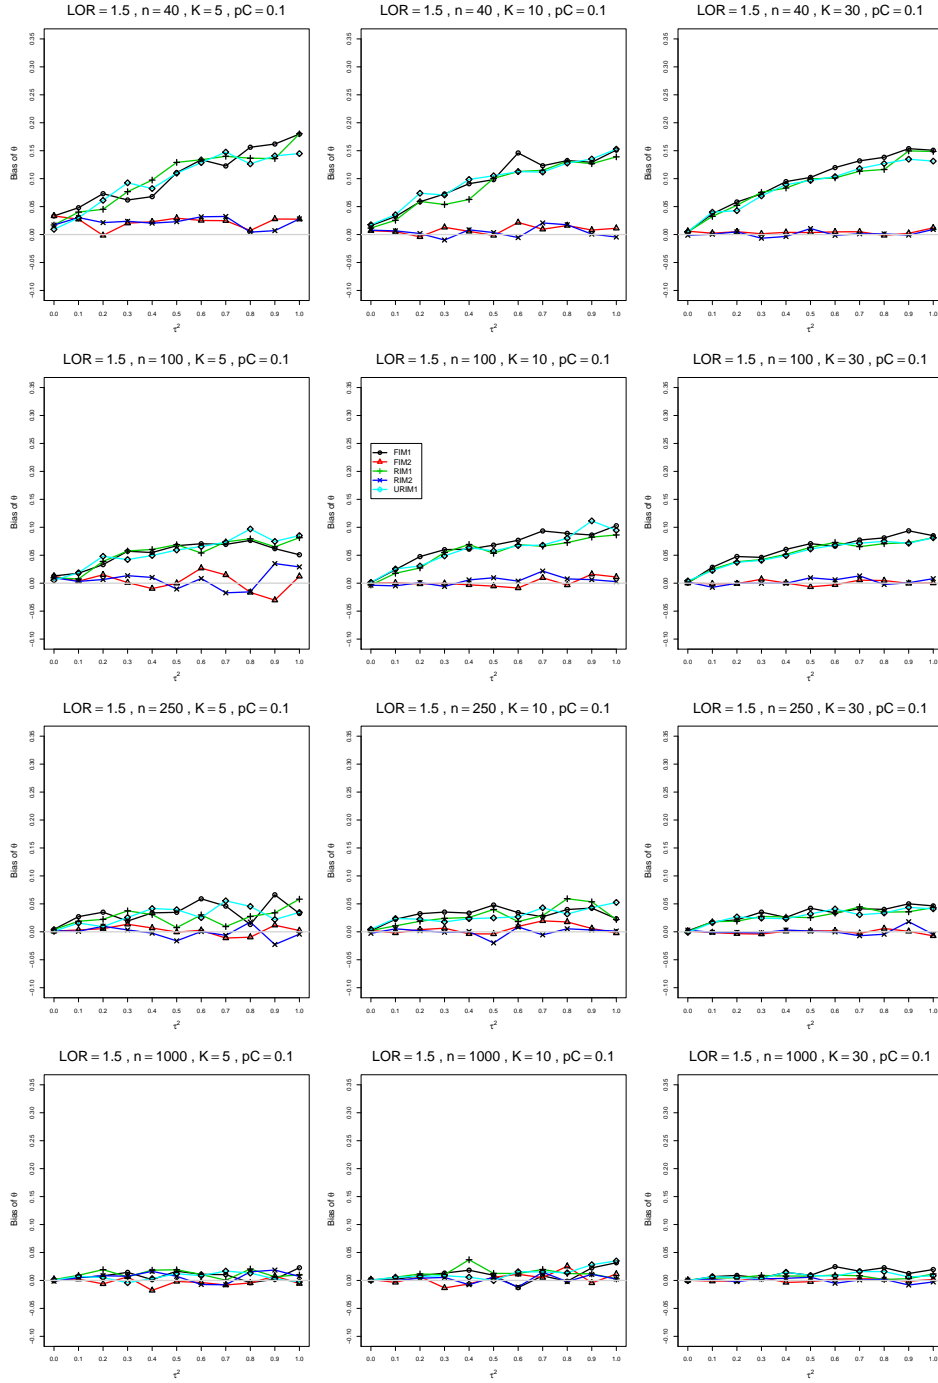

Figure A2.6.7: Bias of overall log-odds ratio  $\hat{\theta}_{RIM2}$  for  $\theta = 1.5$ ,  $p_C = 0.1$ ,  $\sigma^2 = 0.1$ , constant sample sizes  $n = 40, 100, 250, 1000$ . The data-generation mechanisms are FIM1 ( $\circ$ ), FIM2 ( $\triangle$ ), RIM1 ( $+$ ), RIM2 ( $\times$ ), and URIM1 ( $\diamond$ ).

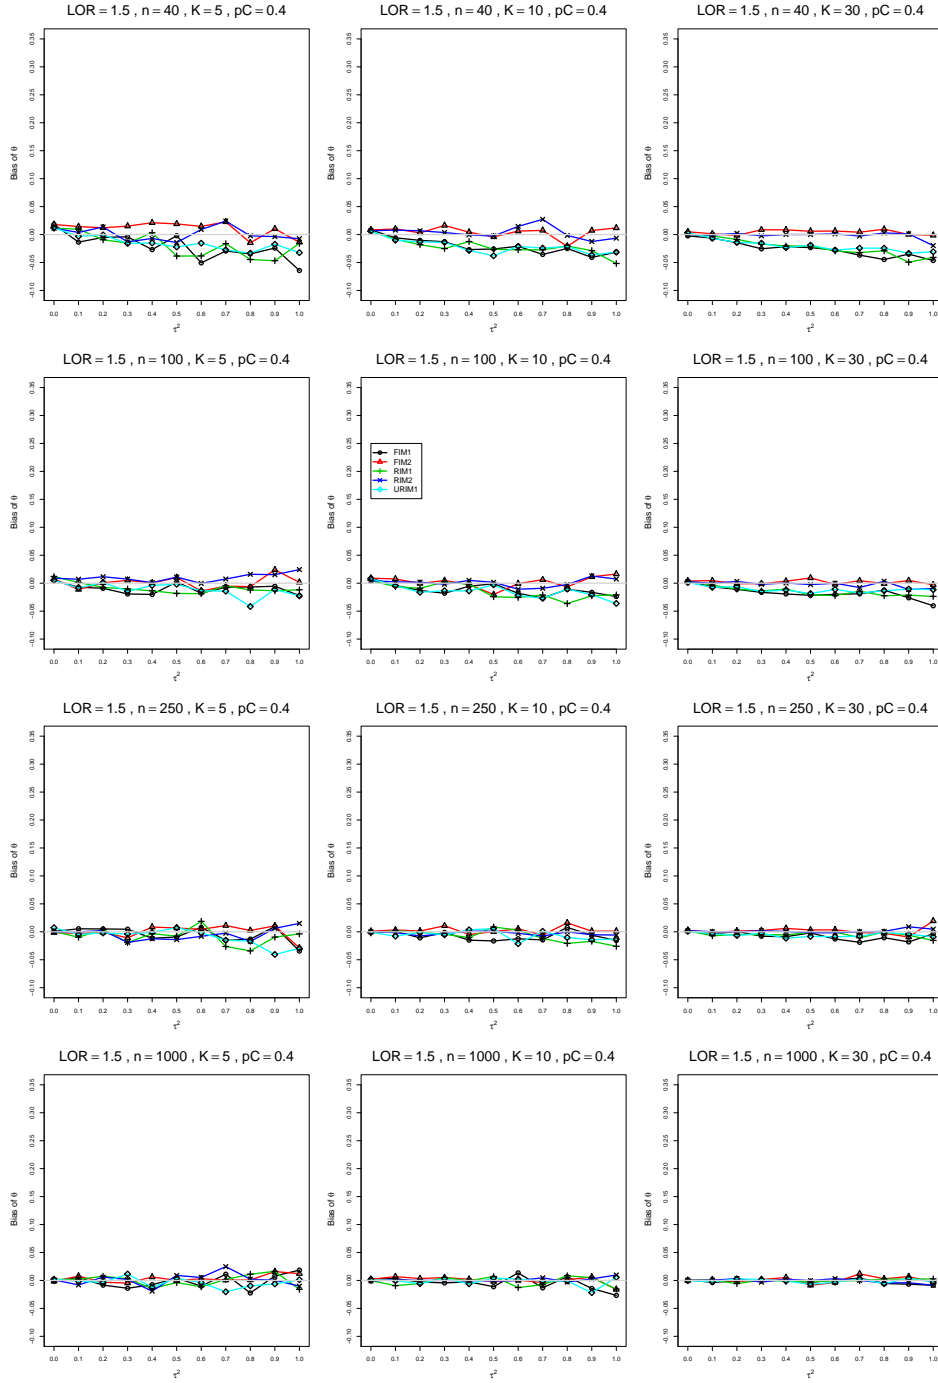

Figure A2.6.8: Bias of overall log-odds ratio  $\hat{\theta}_{RIM2}$  for  $\theta = 1.5$ ,  $p_C = 0.4$ ,  $\sigma^2 = 0.1$ , constant sample sizes  $n = 40, 100, 250, 1000$ . The data-generation mechanisms are FIM1 ( $\circ$ ), FIM2 ( $\triangle$ ), RIM1 ( $+$ ), RIM2 ( $\times$ ), and URIM1 ( $\diamond$ ).

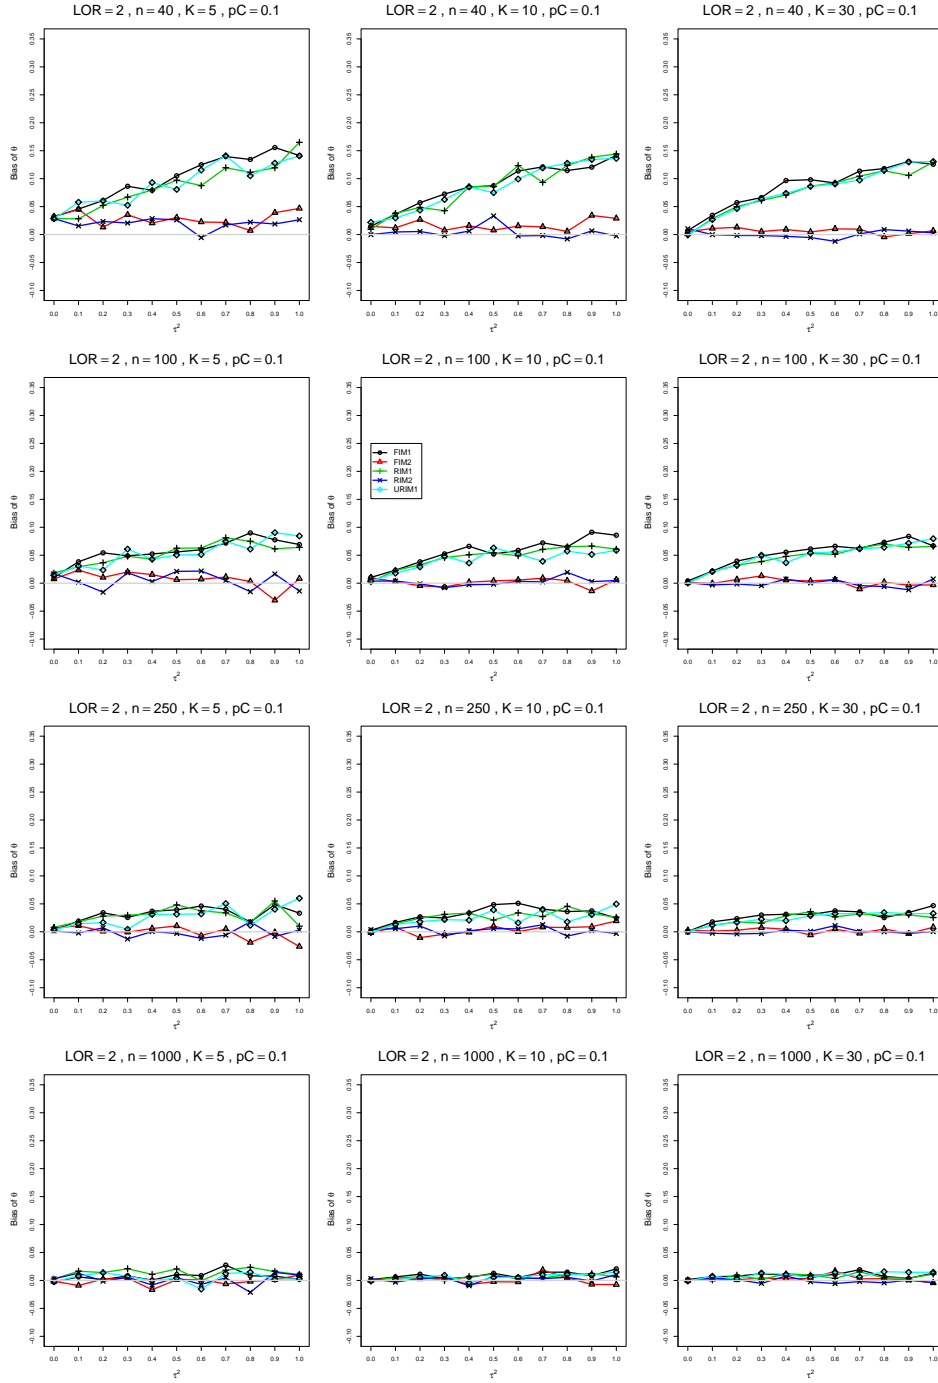

Figure A2.6.9: Bias of overall log-odds ratio  $\hat{\theta}_{RIM2}$  for  $\theta = 2$ ,  $p_C = 0.1$ ,  $\sigma^2 = 0.1$ , constant sample sizes  $n = 40, 100, 250, 1000$ . The data-generation mechanisms are FIM1 ( $\circ$ ), FIM2 ( $\triangle$ ), RIM1 ( $+$ ), RIM2 ( $\times$ ), and URIM1 ( $\diamond$ ).



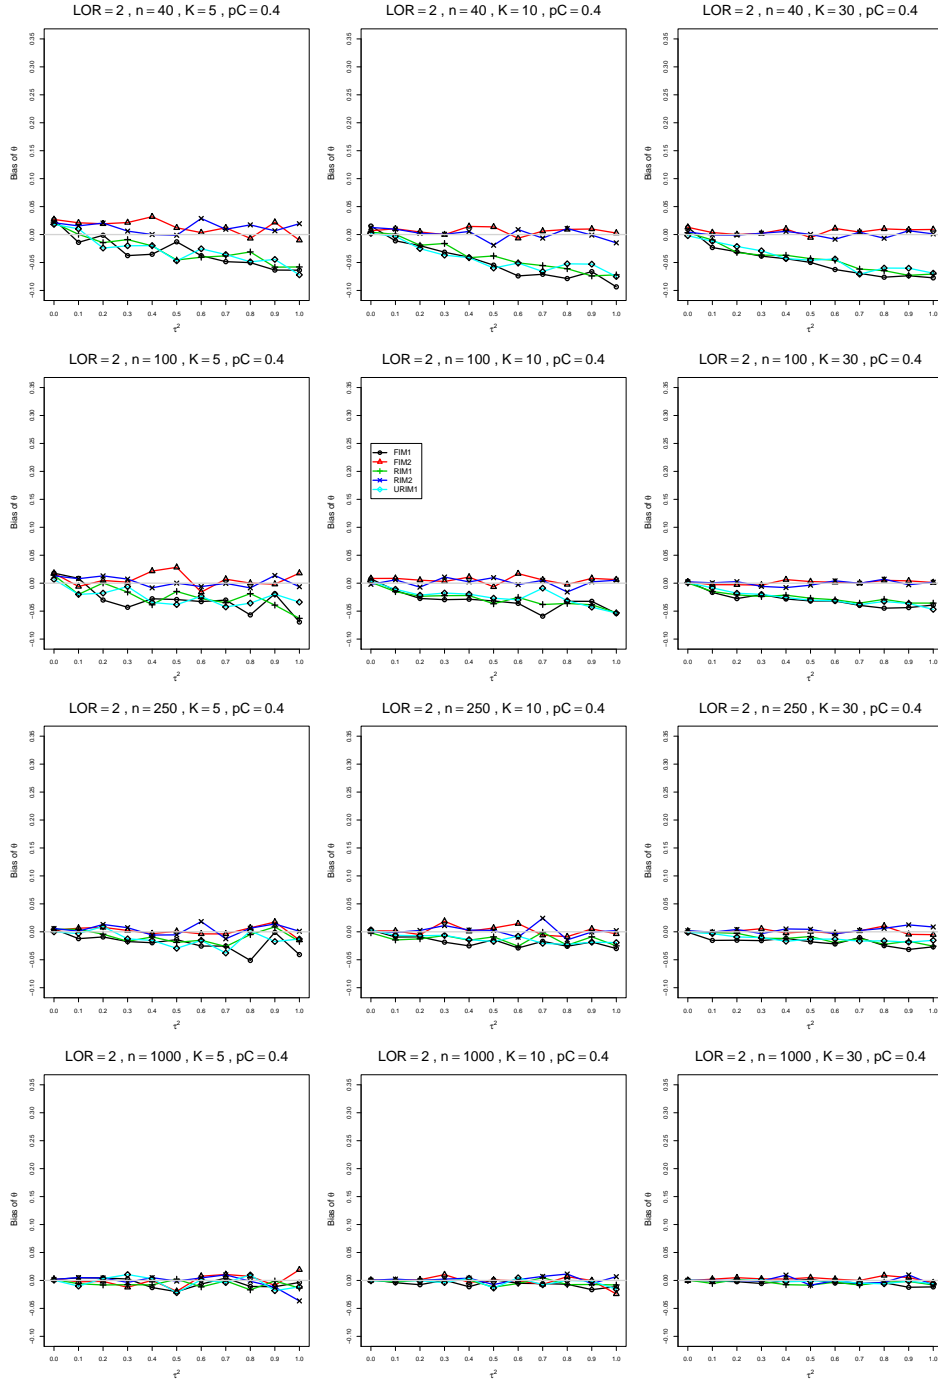

Figure A2.6.10: Bias of overall log-odds ratio  $\hat{\theta}_{RIM2}$  for  $\theta = 2$ ,  $p_C = 0.4$ ,  $\sigma^2 = 0.1$ , constant sample sizes  $n = 40, 100, 250, 1000$ . The data-generation mechanisms are FIM1 (○), FIM2 (△), RIM1 (+), RIM2 (×), and URIM1 (◇).

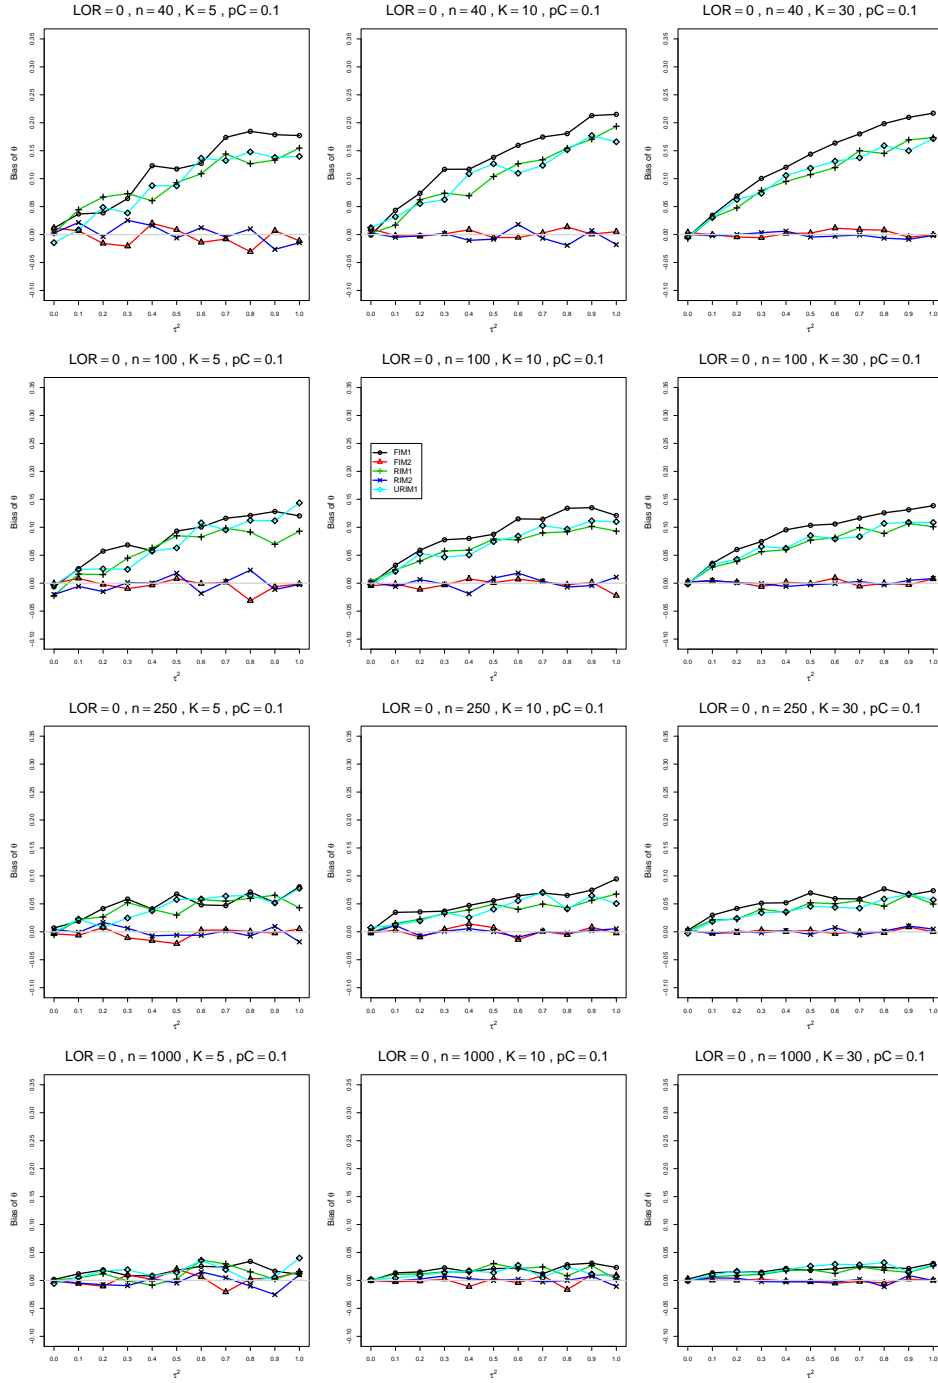

Figure A2.6.11: Bias of overall log-odds ratio  $\hat{\theta}_{RIM2}$  for  $\theta = 0$ ,  $p_C = 0.1$ ,  $\sigma^2 = 0.4$ , constant sample sizes  $n = 40, 100, 250, 1000$ . The data-generation mechanisms are FIM1 ( $\circ$ ), FIM2 ( $\triangle$ ), RIM1 ( $+$ ), RIM2 ( $\times$ ), and URIM1 ( $\diamond$ ).

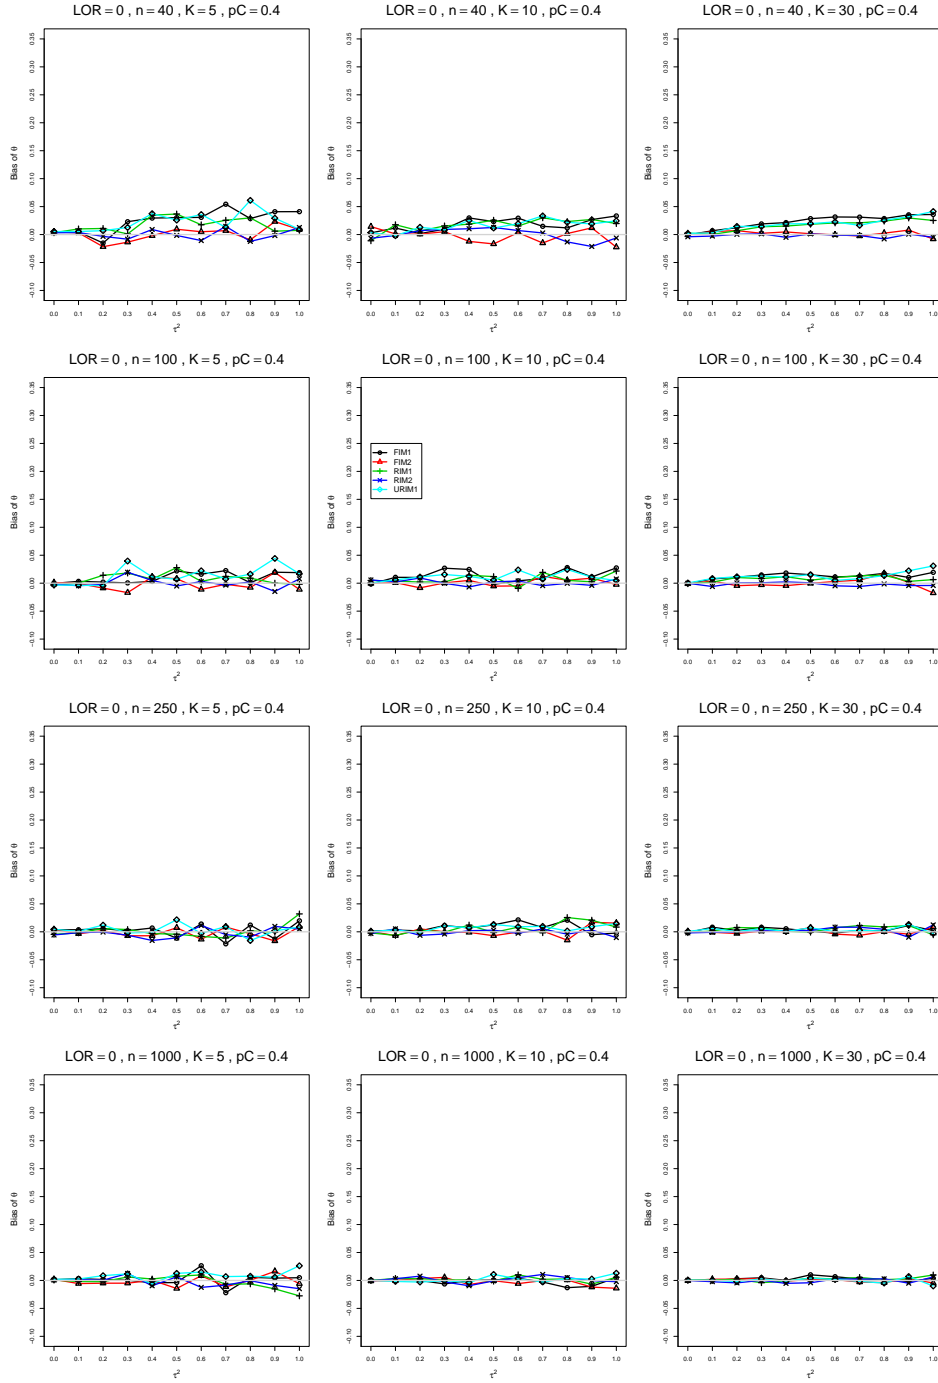

Figure A2.6.12: Bias of overall log-odds ratio  $\hat{\theta}_{RIM2}$  for  $\theta = 0$ ,  $p_C = 0.4$ ,  $\sigma^2 = 0.4$ , constant sample sizes  $n = 40, 100, 250, 1000$ . The data-generation mechanisms are FIM1 ( $\circ$ ), FIM2 ( $\triangle$ ), RIM1 ( $+$ ), RIM2 ( $\times$ ), and URIM1 ( $\diamond$ ).

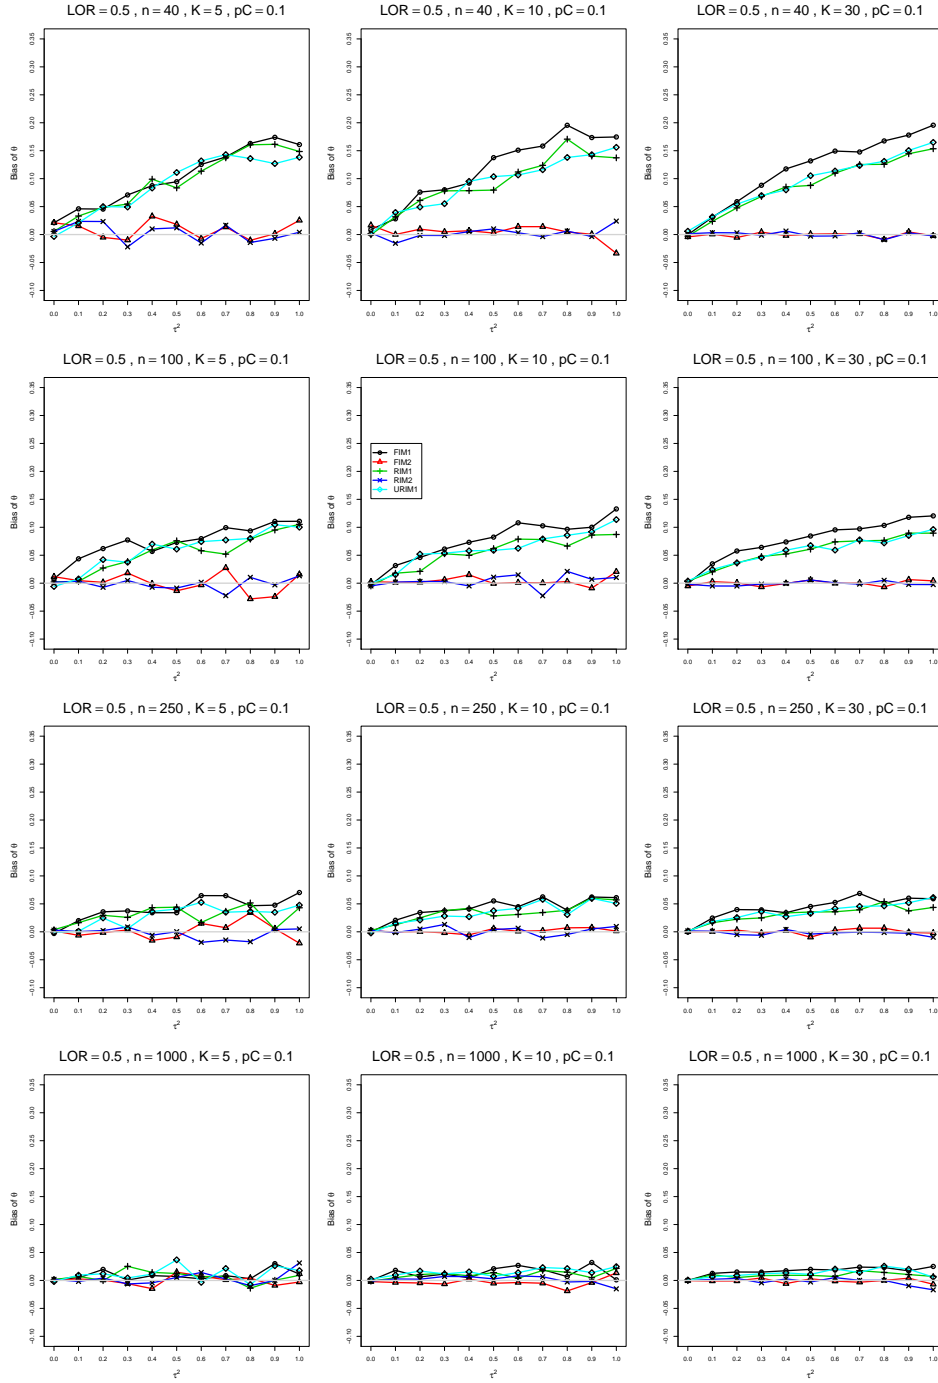

Figure A2.6.13: Bias of overall log-odds ratio  $\hat{\theta}_{RIM2}$  for  $\theta = 0.5$ ,  $p_C = 0.1$ ,  $\sigma^2 = 0.4$ , constant sample sizes  $n = 40, 100, 250, 1000$ . The data-generation mechanisms are FIM1 ( $\circ$ ), FIM2 ( $\triangle$ ), RIM1 ( $+$ ), RIM2 ( $\times$ ), and URIM1 ( $\diamond$ ).

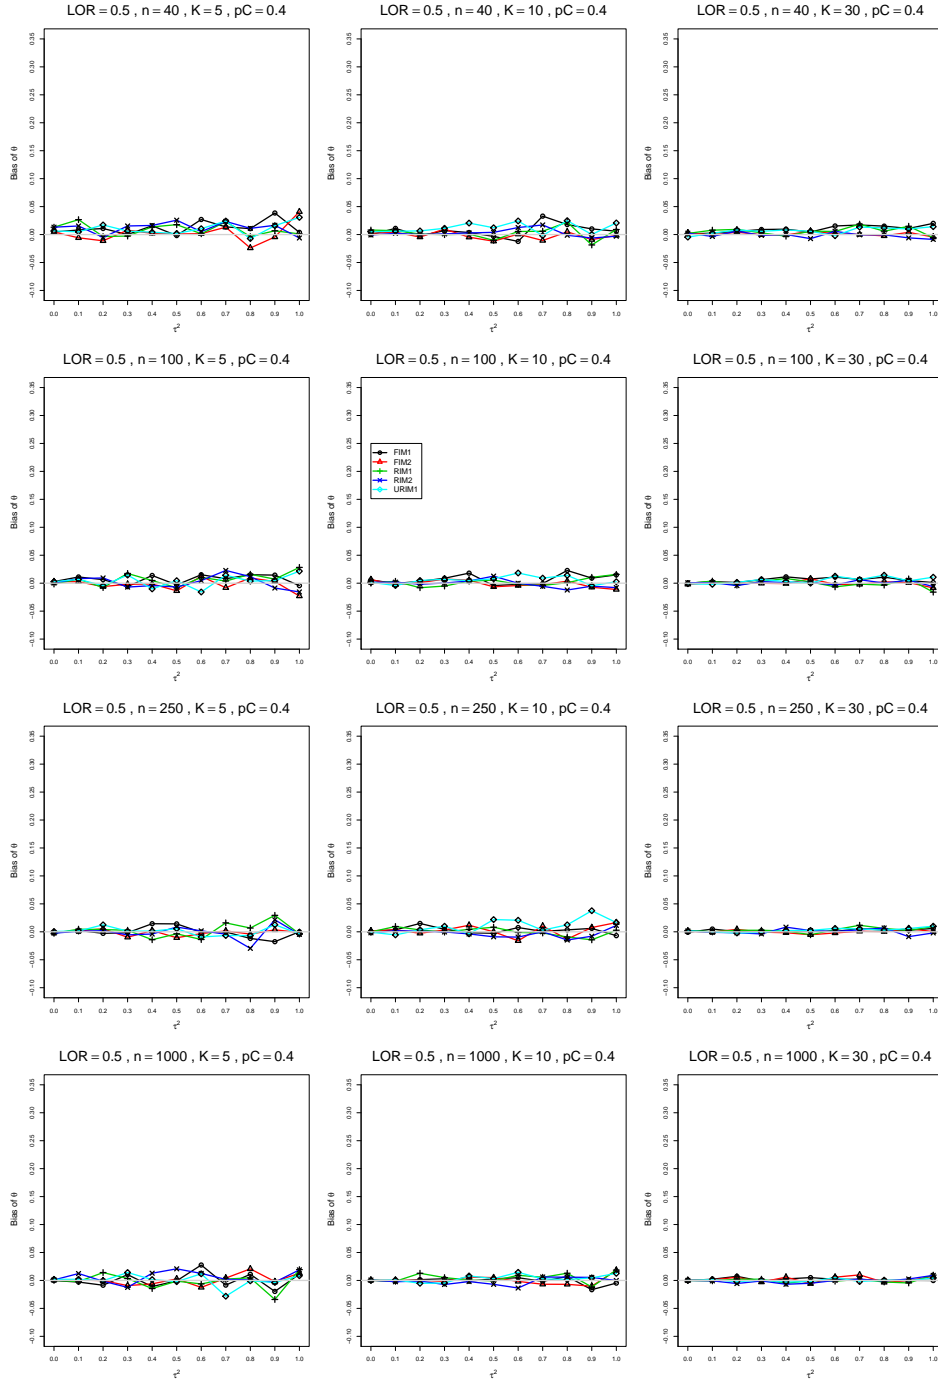

Figure A2.6.14: Bias of overall log-odds ratio  $\hat{\theta}_{RIM2}$  for  $\theta = 0.5$ ,  $p_C = 0.4$ ,  $\sigma^2 = 0.4$ , constant sample sizes  $n = 40, 100, 250, 1000$ . The data-generation mechanisms are FIM1 ( $\circ$ ), FIM2 ( $\triangle$ ), RIM1 ( $+$ ), RIM2 ( $\times$ ), and URIM1 ( $\diamond$ ).

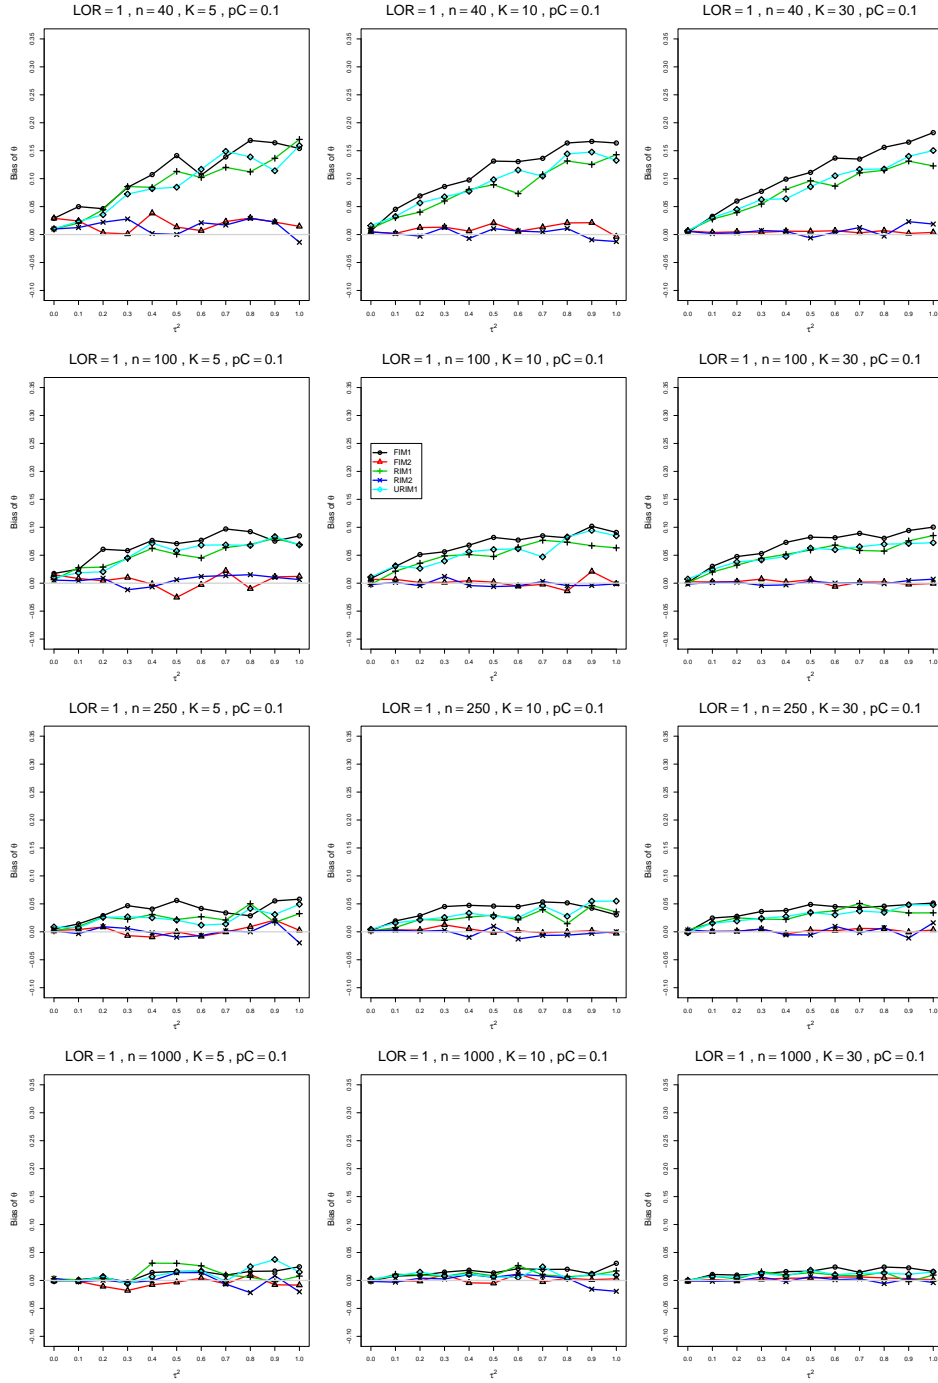

Figure A2.6.15: Bias of overall log-odds ratio  $\hat{\theta}_{RIM2}$  for  $\theta = 1$ ,  $p_C = 0.1$ ,  $\sigma^2 = 0.4$ , constant sample sizes  $n = 40, 100, 250, 1000$ . The data-generation mechanisms are FIM1 ( $\circ$ ), FIM2 ( $\triangle$ ), RIM1 ( $+$ ), RIM2 ( $\times$ ), and URIM1 ( $\diamond$ ).

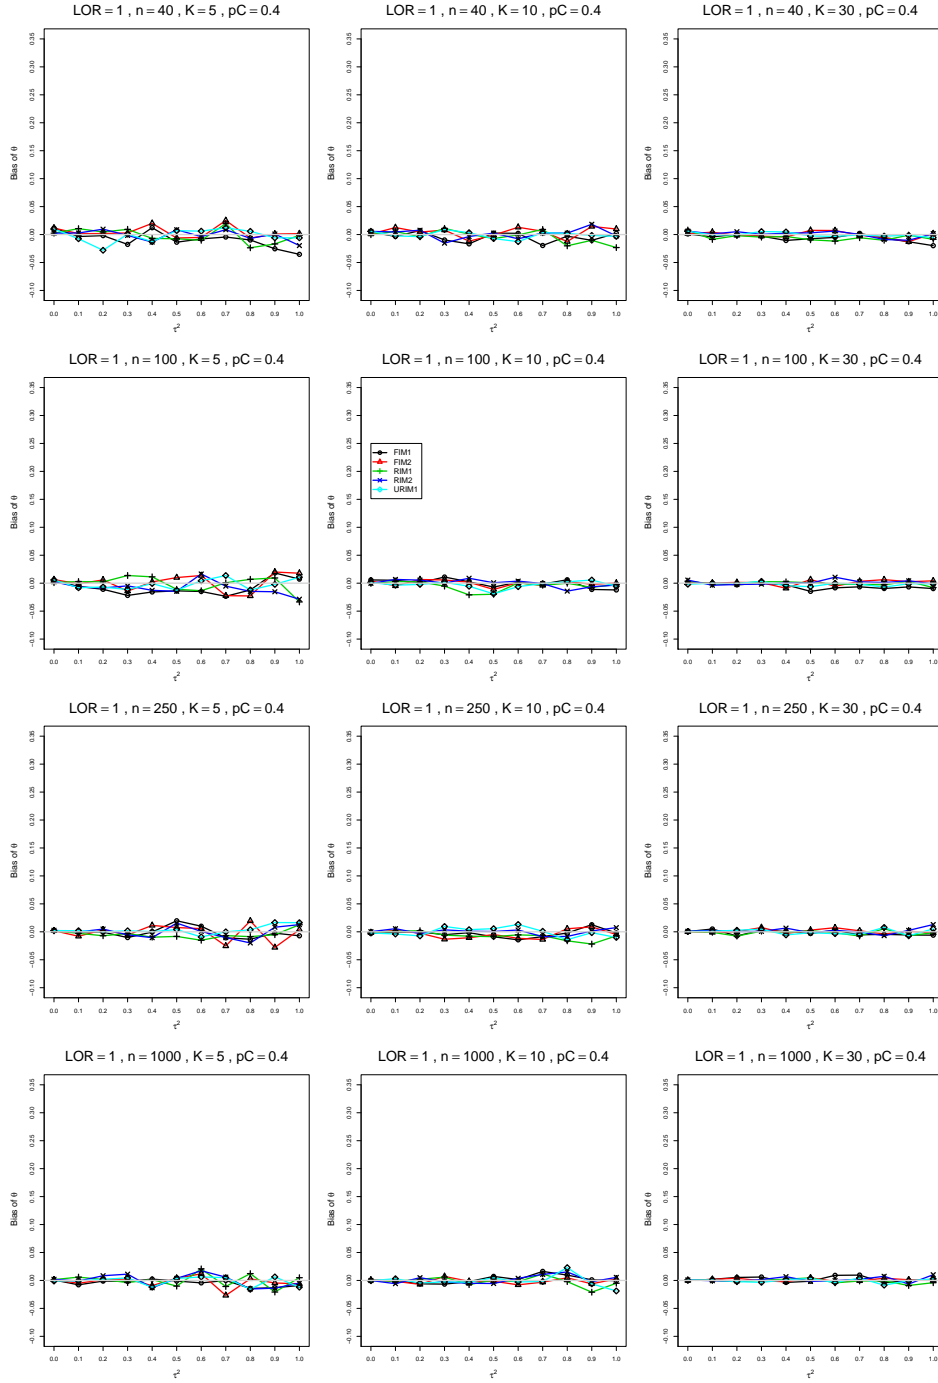

Figure A2.6.16: Bias of overall log-odds ratio  $\hat{\theta}_{RIM2}$  for  $\theta = 1$ ,  $p_C = 0.4$ ,  $\sigma^2 = 0.4$ , constant sample sizes  $n = 40, 100, 250, 1000$ . The data-generation mechanisms are FIM1 ( $\circ$ ), FIM2 ( $\triangle$ ), RIM1 ( $+$ ), RIM2 ( $\times$ ), and URIM1 ( $\diamond$ ).

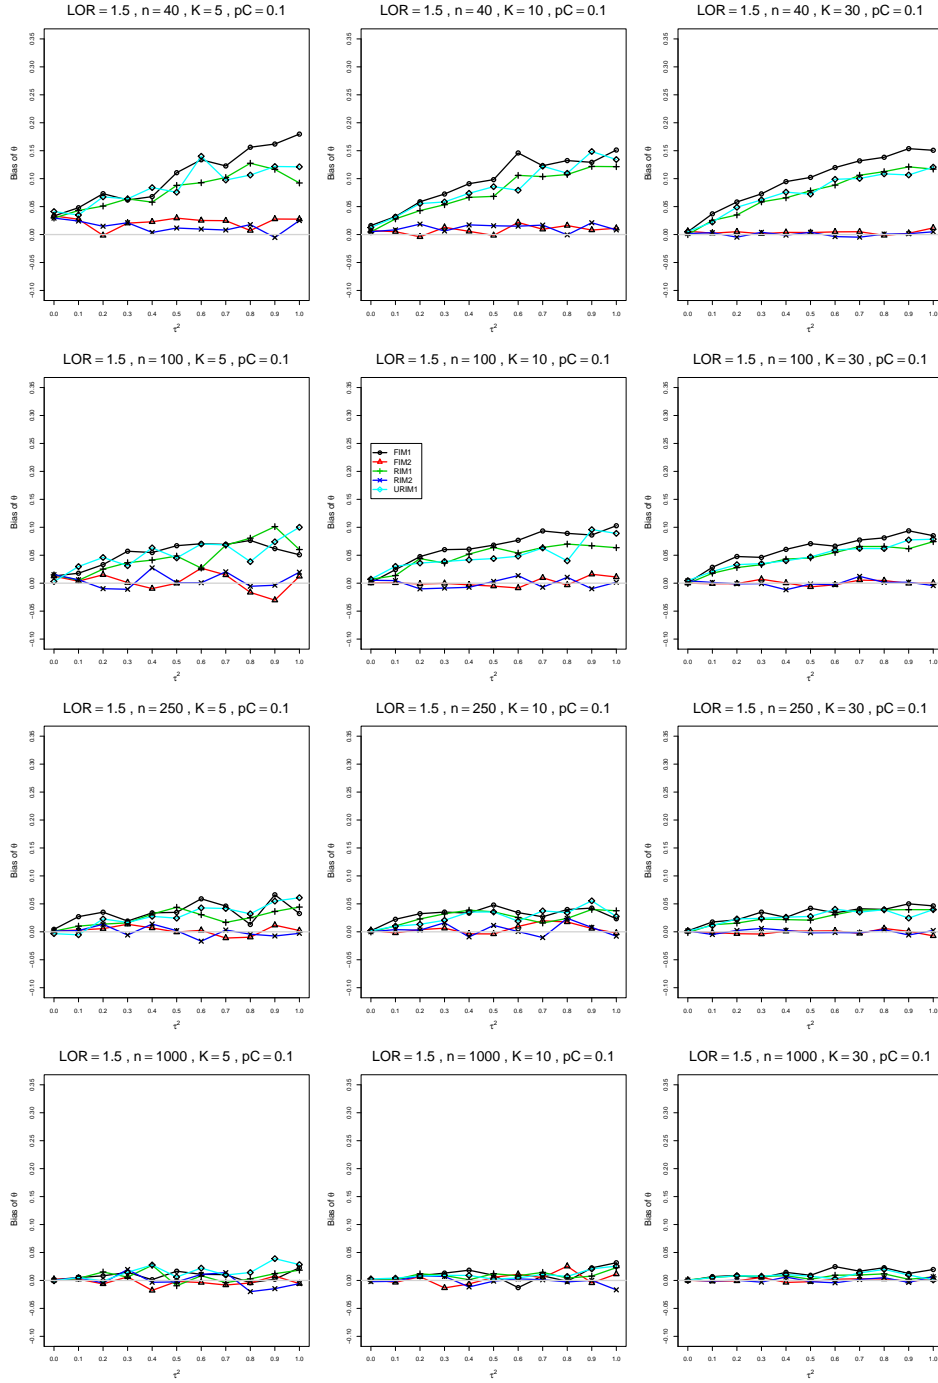

Figure A2.6.17: Bias of overall log-odds ratio  $\hat{\theta}_{RIM2}$  for  $\theta = 1.5$ ,  $p_C = 0.1$ ,  $\sigma^2 = 0.4$ , constant sample sizes  $n = 40, 100, 250, 1000$ . The data-generation mechanisms are FIM1 ( $\circ$ ), FIM2 ( $\triangle$ ), RIM1 ( $+$ ), RIM2 ( $\times$ ), and URIM1 ( $\diamond$ ).



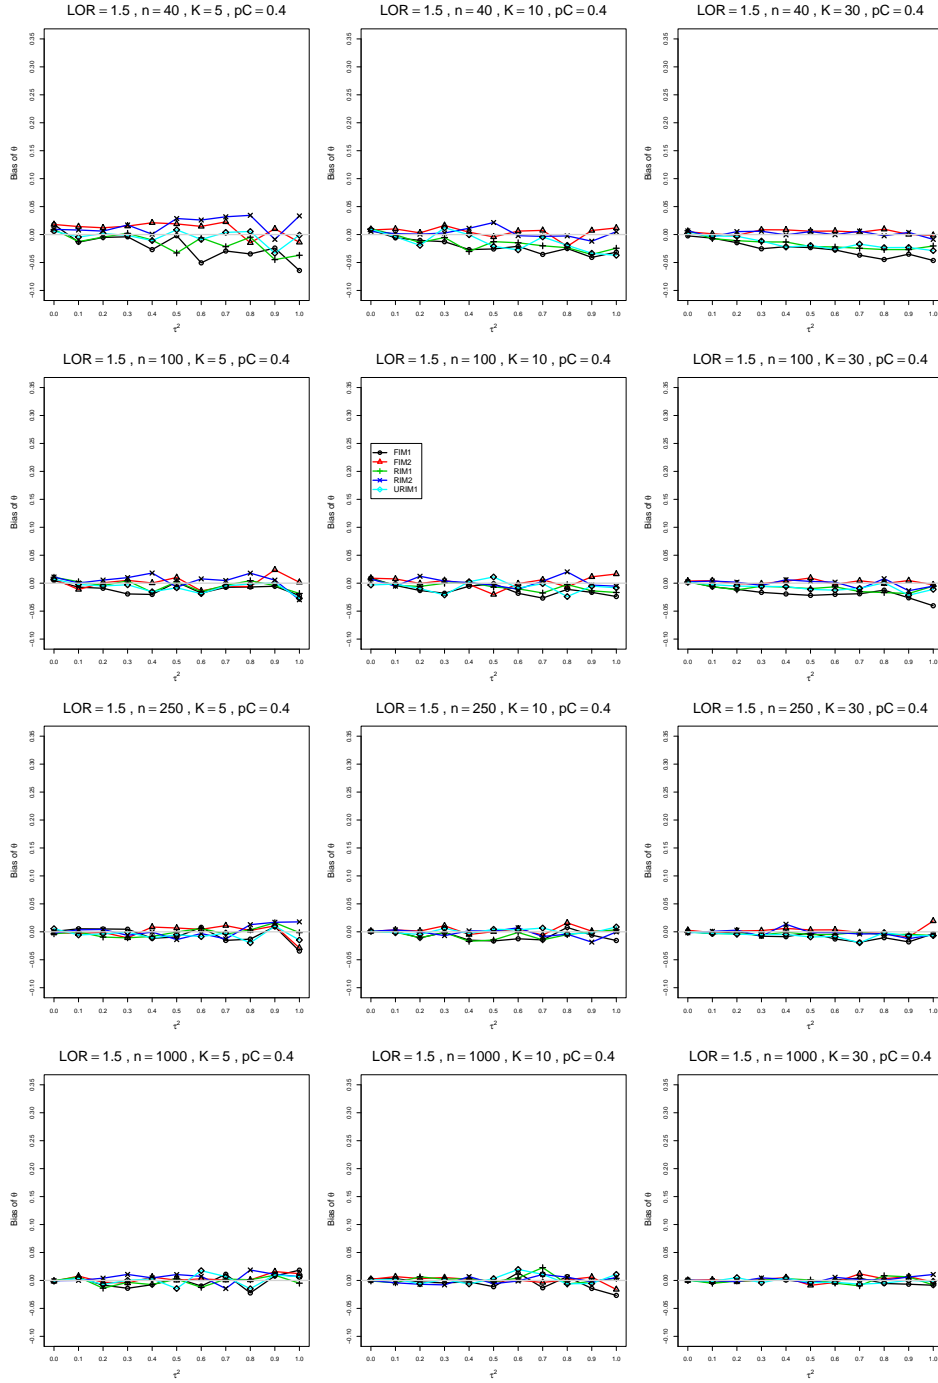

Figure A2.6.18: Bias of overall log-odds ratio  $\hat{\theta}_{RIM2}$  for  $\theta = 1.5$ ,  $p_C = 0.4$ ,  $\sigma^2 = 0.4$ , constant sample sizes  $n = 40, 100, 250, 1000$ . The data-generation mechanisms are FIM1 ( $\circ$ ), FIM2 ( $\triangle$ ), RIM1 ( $+$ ), RIM2 ( $\times$ ), and URIM1 ( $\diamond$ ).

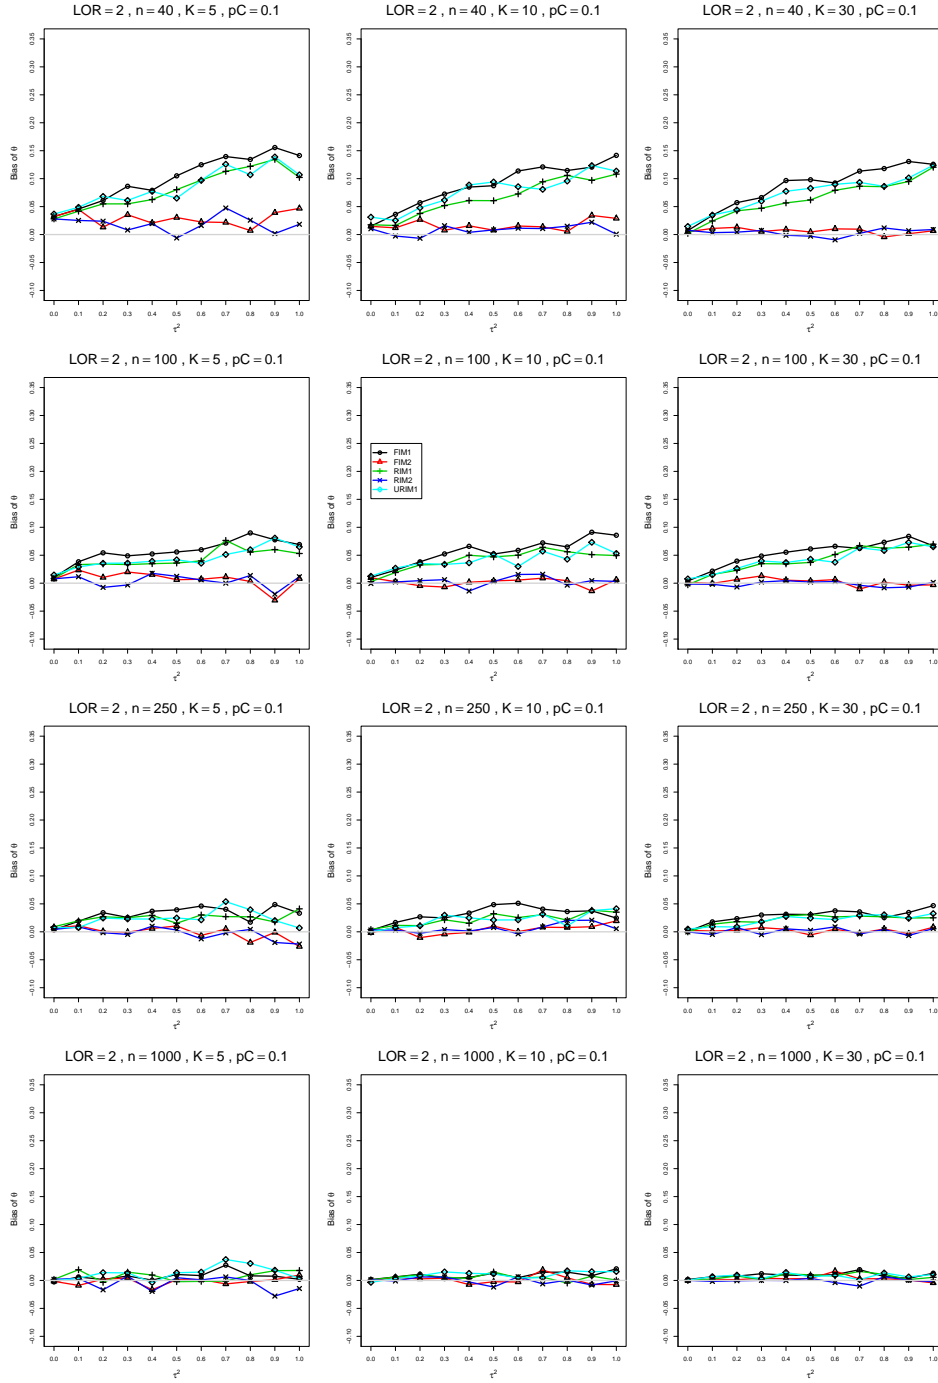

Figure A2.6.19: Bias of overall log-odds ratio  $\hat{\theta}_{RIM2}$  for  $\theta = 2$ ,  $p_C = 0.1$ ,  $\sigma^2 = 0.4$ , constant sample sizes  $n = 40, 100, 250, 1000$ . The data-generation mechanisms are FIM1 ( $\circ$ ), FIM2 ( $\triangle$ ), RIM1 ( $+$ ), RIM2 ( $\times$ ), and URIM1 ( $\diamond$ ).

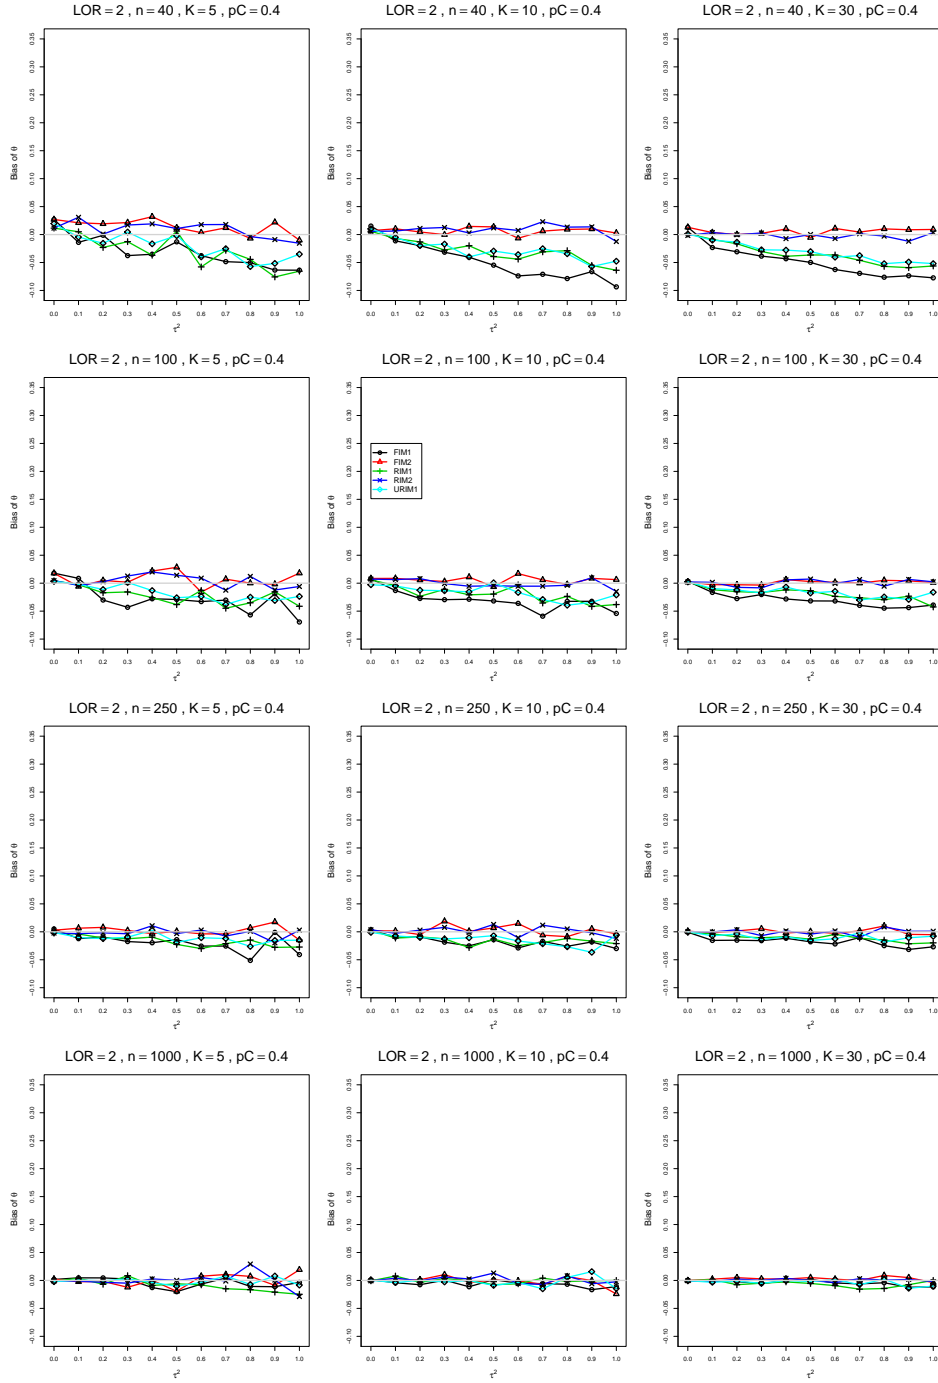

Figure A2.6.20: Bias of overall log-odds ratio  $\hat{\theta}_{RIM2}$  for  $\theta = 2$ ,  $p_C = 0.4$ ,  $\sigma^2 = 0.4$ , constant sample sizes  $n = 40, 100, 250, 1000$ . The data-generation mechanisms are FIM1 ( $\circ$ ), FIM2 ( $\triangle$ ), RIM1 ( $+$ ), RIM2 ( $\times$ ), and URIM1 ( $\diamond$ ).

## A2.7 Bias of $\hat{\theta}_{SW}$

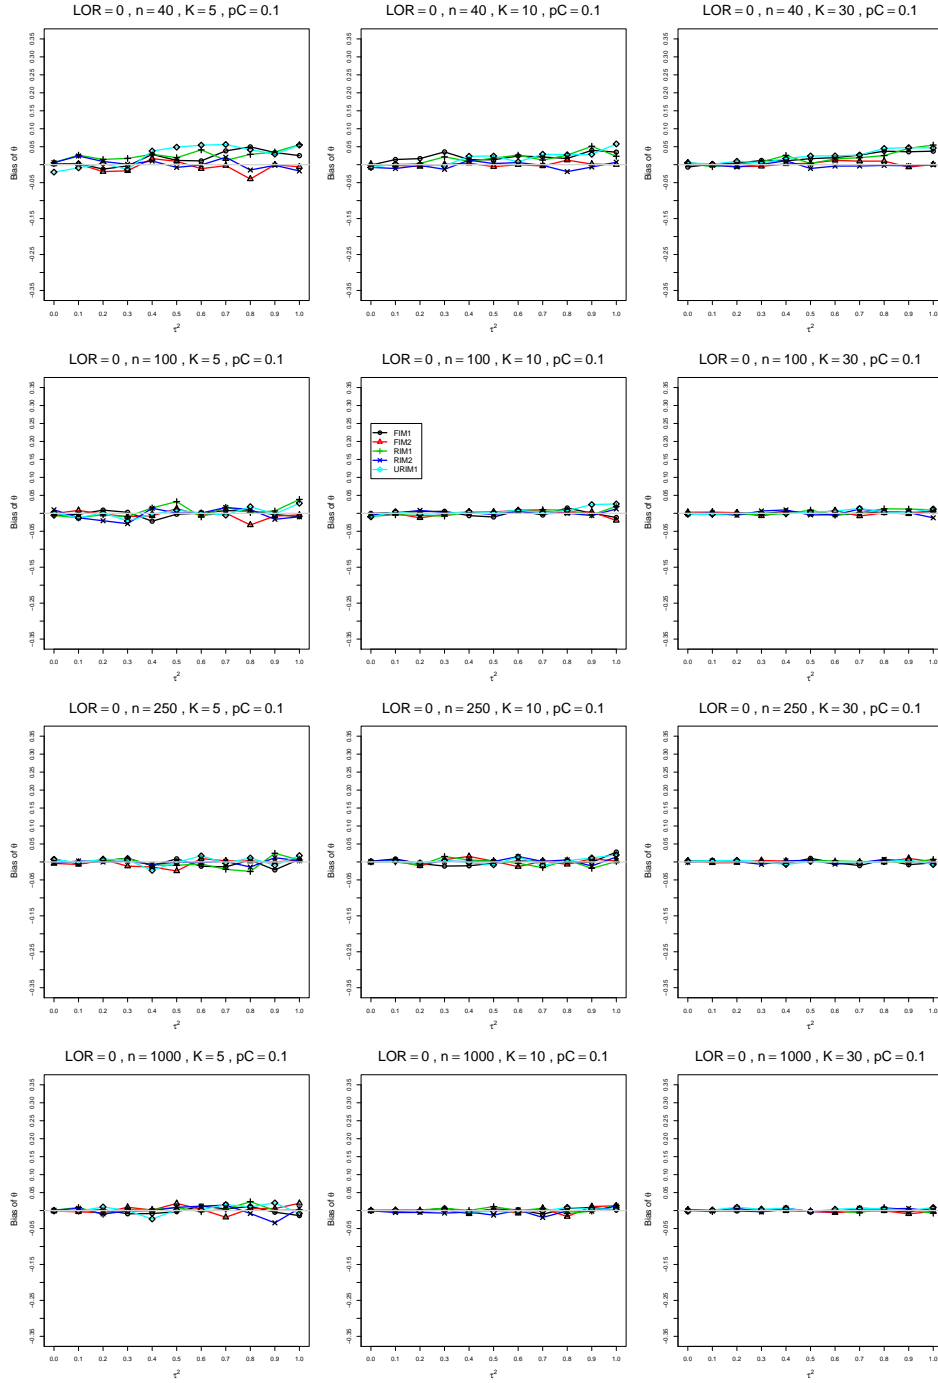

Figure A2.7.1: Bias of overall log-odds ratio  $\hat{\theta}_{SW}$  for  $\theta = 0$ ,  $p_C = 0.1$ ,  $\sigma^2 = 0.1$ , constant sample sizes  $n = 40, 100, 250, 1000$ . The data-generation mechanisms are FIM1 ( $\circ$ ), FIM2 ( $\triangle$ ), RIM1 ( $+$ ), RIM2 ( $\times$ ), and URIM1 ( $\diamond$ ).

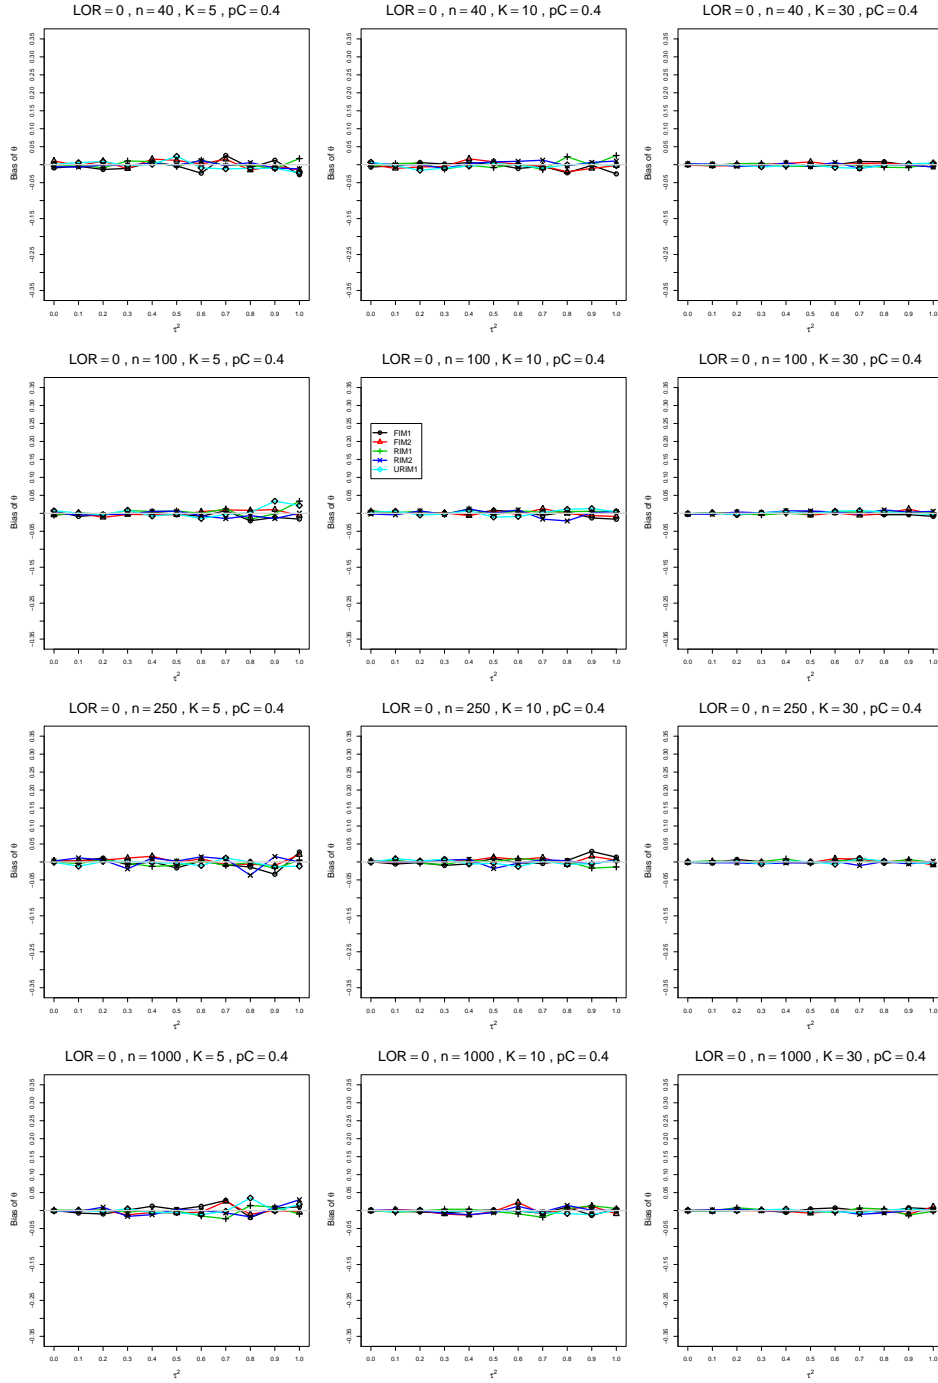

Figure A2.7.2: Bias of overall log-odds ratio  $\hat{\theta}_{SW}$  for  $\theta = 0$ ,  $p_C = 0.4$ ,  $\sigma^2 = 0.1$ , constant sample sizes  $n = 40, 100, 250, 1000$ . The data-generation mechanisms are FIM1 ( $\circ$ ), FIM2 ( $\triangle$ ), RIM1 ( $+$ ), RIM2 ( $\times$ ), and URIM1 ( $\diamond$ ).

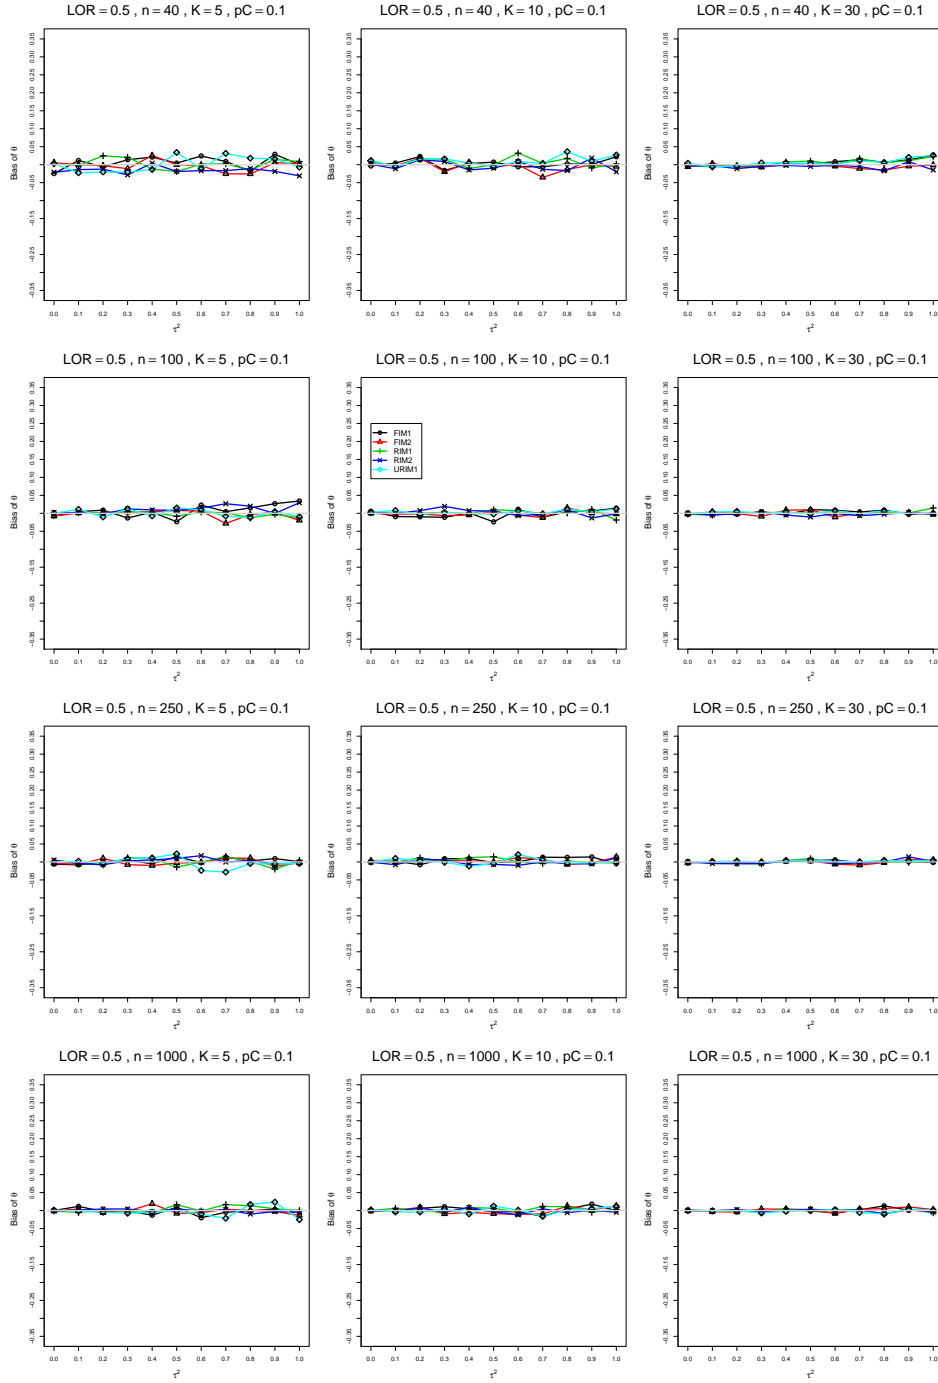

Figure A2.7.3: Bias of overall log-odds ratio  $\hat{\theta}_{SW}$  for  $\theta = 0.5$ ,  $p_C = 0.1$ ,  $\sigma^2 = 0.1$ , constant sample sizes  $n = 40, 100, 250, 1000$ . The data-generation mechanisms are FIM1 ( $\circ$ ), FIM2 ( $\triangle$ ), RIM1 ( $+$ ), RIM2 ( $\times$ ), and URIM1 ( $\diamond$ ).

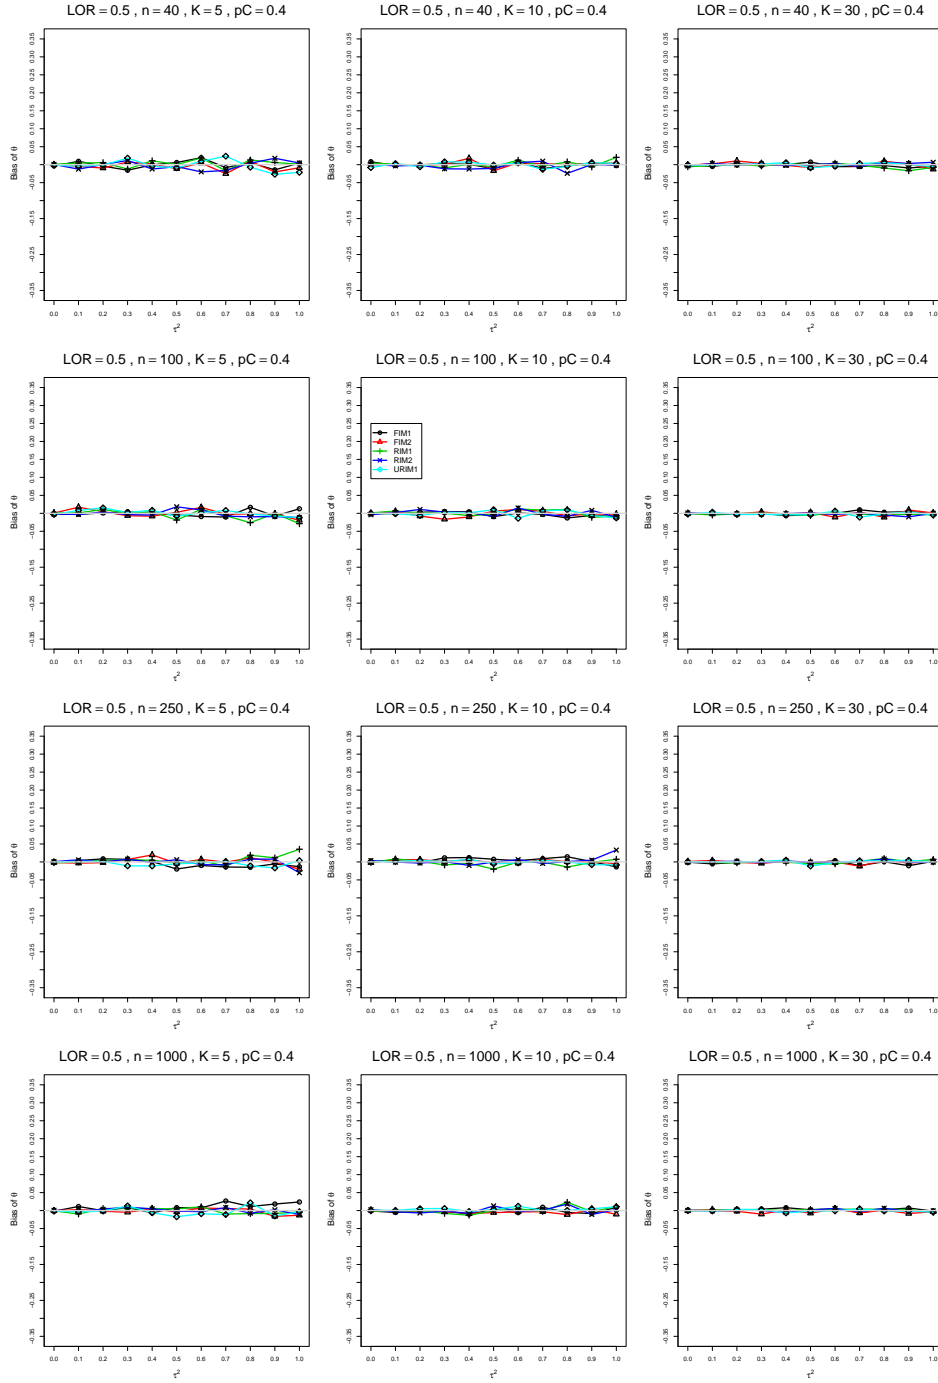

Figure A2.7.4: Bias of overall log-odds ratio  $\hat{\theta}_{SW}$  for  $\theta = 0.5$ ,  $p_C = 0.4$ ,  $\sigma^2 = 0.1$ , constant sample sizes  $n = 40, 100, 250, 1000$ . The data-generation mechanisms are FIM1 ( $\circ$ ), FIM2 ( $\triangle$ ), RIM1 ( $+$ ), RIM2 ( $\times$ ), and URIM1 ( $\diamond$ ).



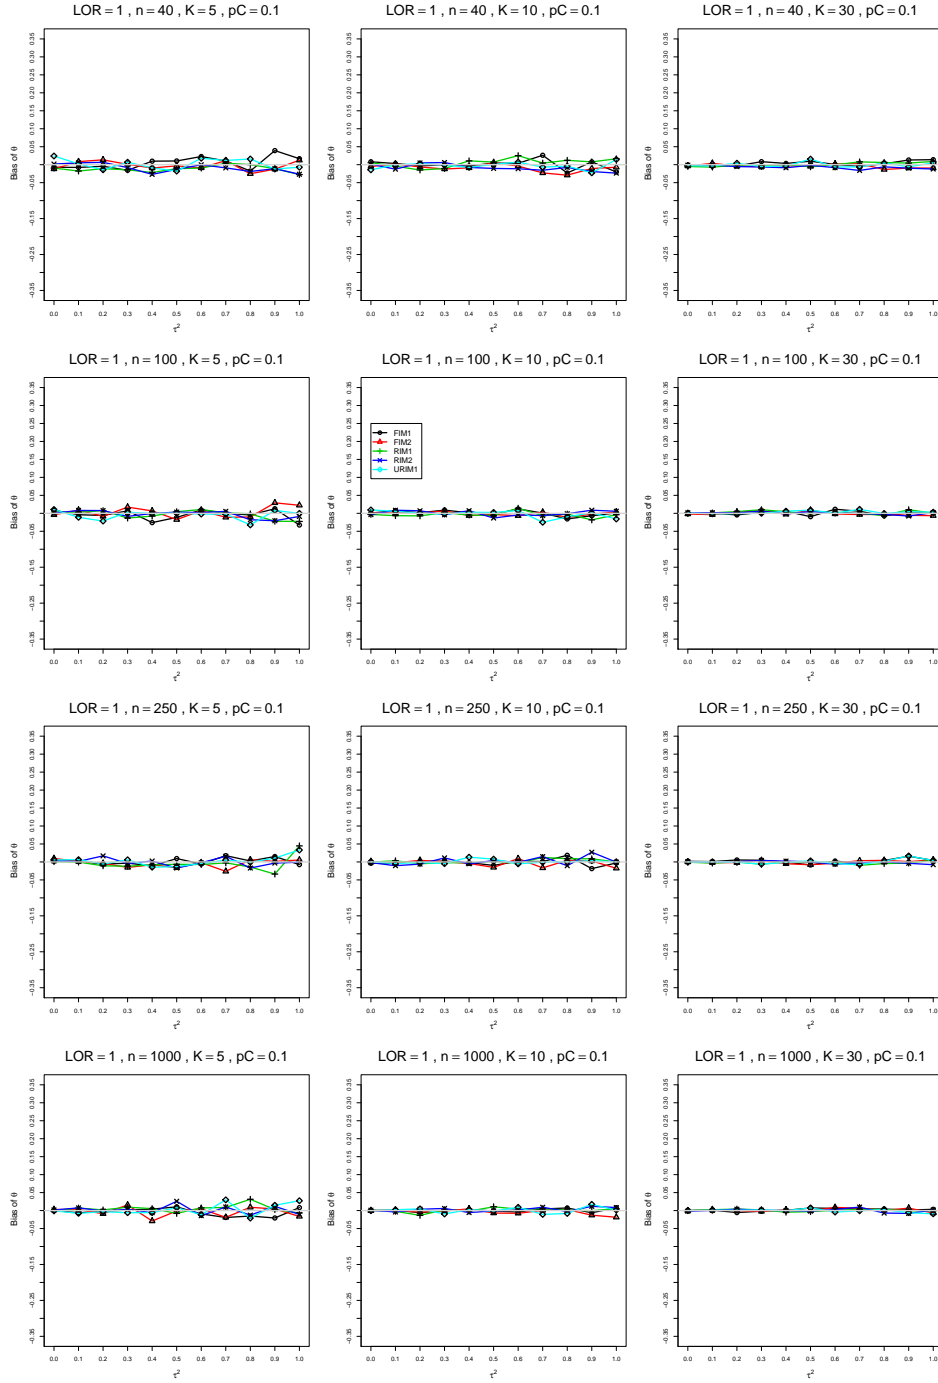

Figure A2.7.5: Bias of overall log-odds ratio  $\hat{\theta}_{SW}$  for  $\theta = 1$ ,  $p_C = 0.1$ ,  $\sigma^2 = 0.1$ , constant sample sizes  $n = 40, 100, 250, 1000$ . The data-generation mechanisms are FIM1 ( $\circ$ ), FIM2 ( $\triangle$ ), RIM1 ( $+$ ), RIM2 ( $\times$ ), and URIM1 ( $\diamond$ ).

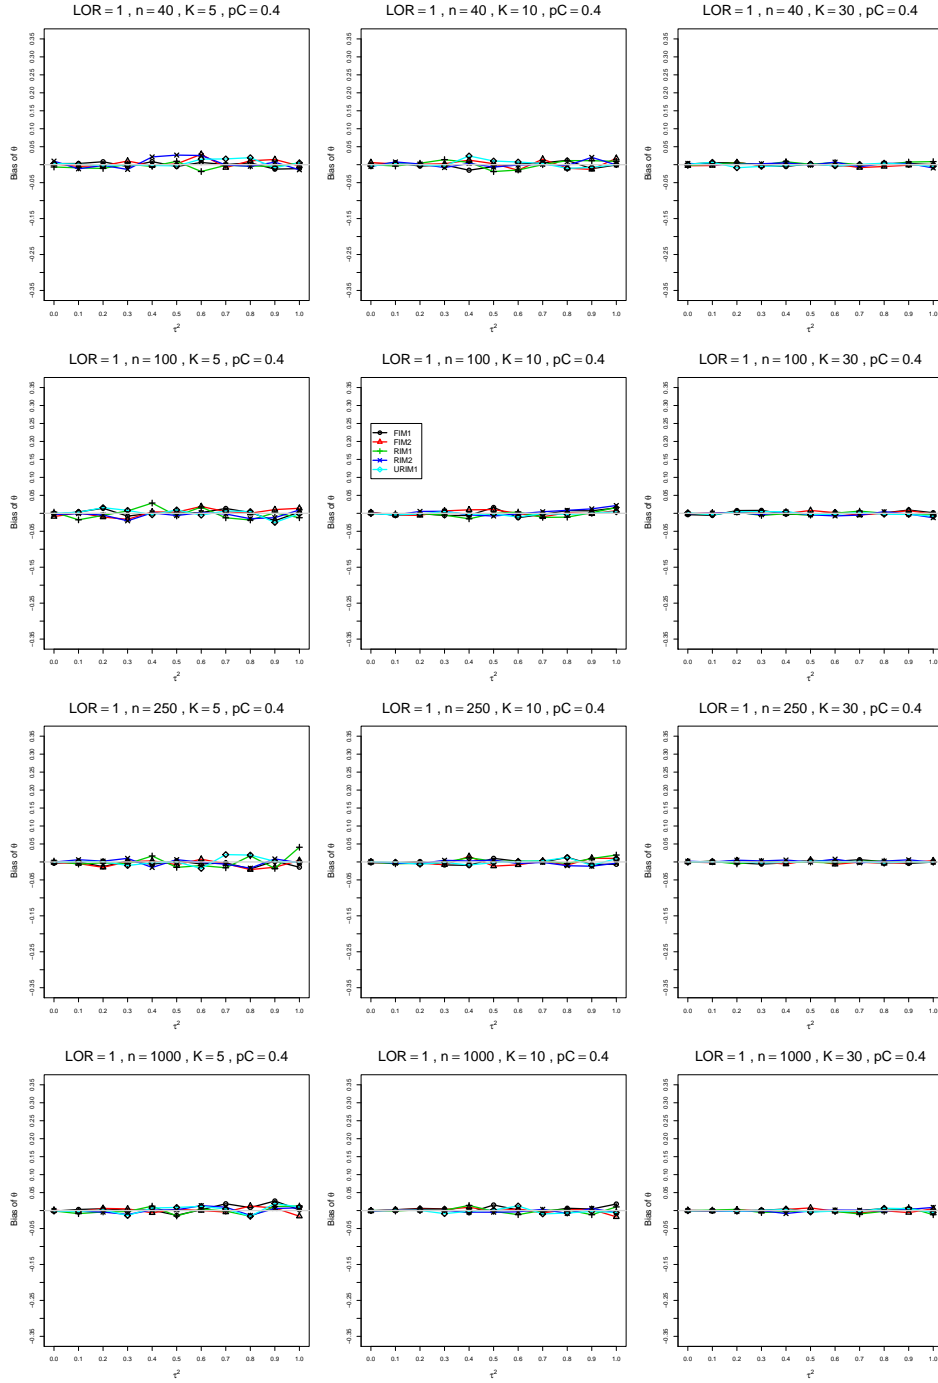

Figure A2.7.6: Bias of overall log-odds ratio  $\hat{\theta}_{SW}$  for  $\theta = 1$ ,  $p_C = 0.4$ ,  $\sigma^2 = 0.1$ , constant sample sizes  $n = 40, 100, 250, 1000$ . The data-generation mechanisms are FIM1 ( $\circ$ ), FIM2 ( $\triangle$ ), RIM1 ( $+$ ), RIM2 ( $\times$ ), and URIM1 ( $\diamond$ ).

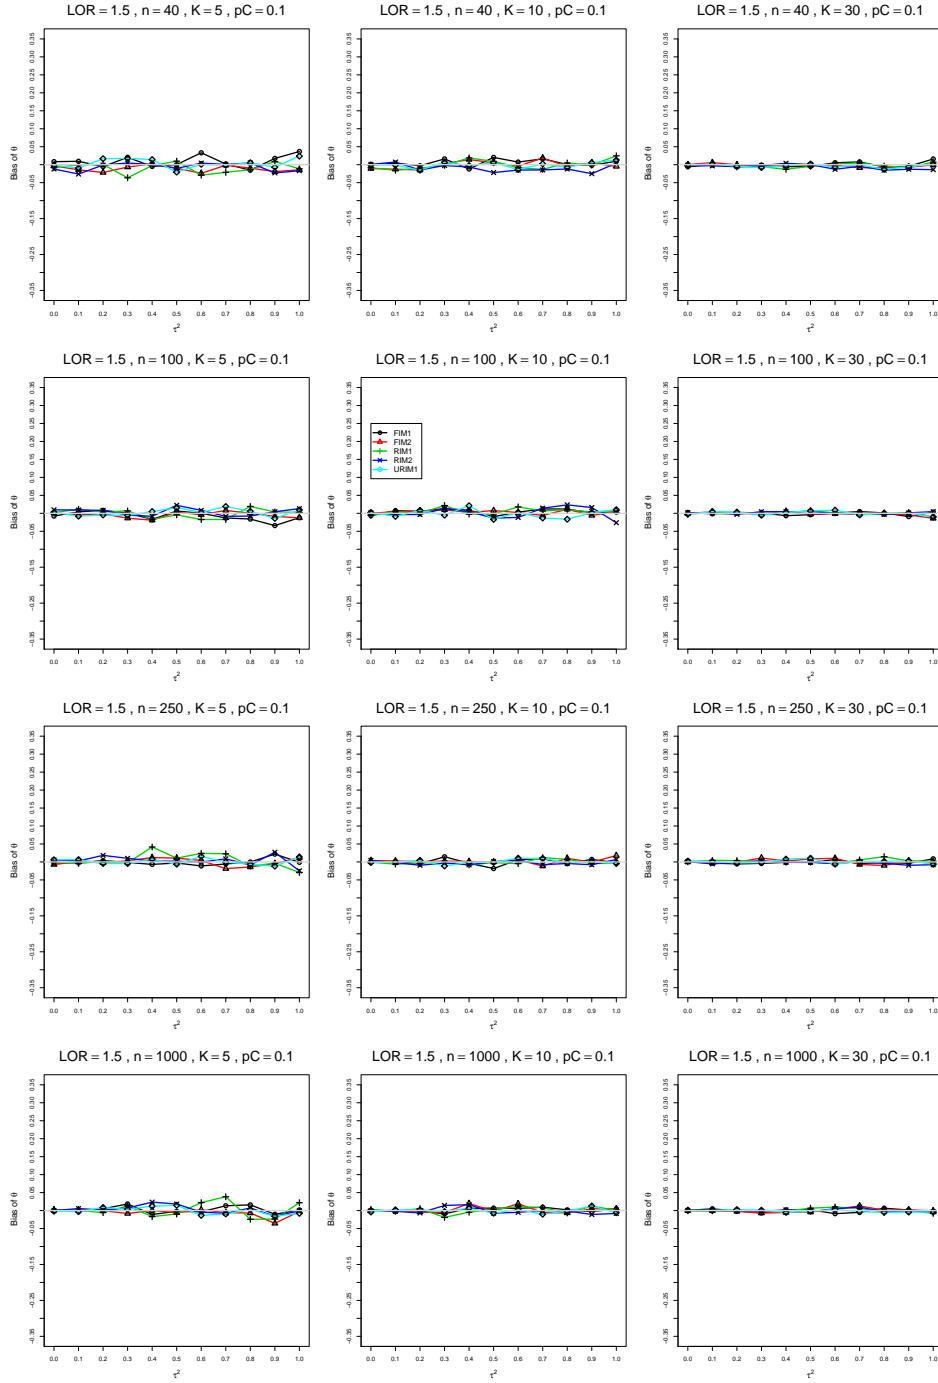

Figure A2.7.7: Bias of overall log-odds ratio  $\hat{\theta}_{SW}$  for  $\theta = 1.5$ ,  $p_C = 0.1$ ,  $\sigma^2 = 0.1$ , constant sample sizes  $n = 40, 100, 250, 1000$ . The data-generation mechanisms are FIM1 ( $\circ$ ), FIM2 ( $\triangle$ ), RIM1 ( $+$ ), RIM2 ( $\times$ ), and URIM1 ( $\diamond$ ).

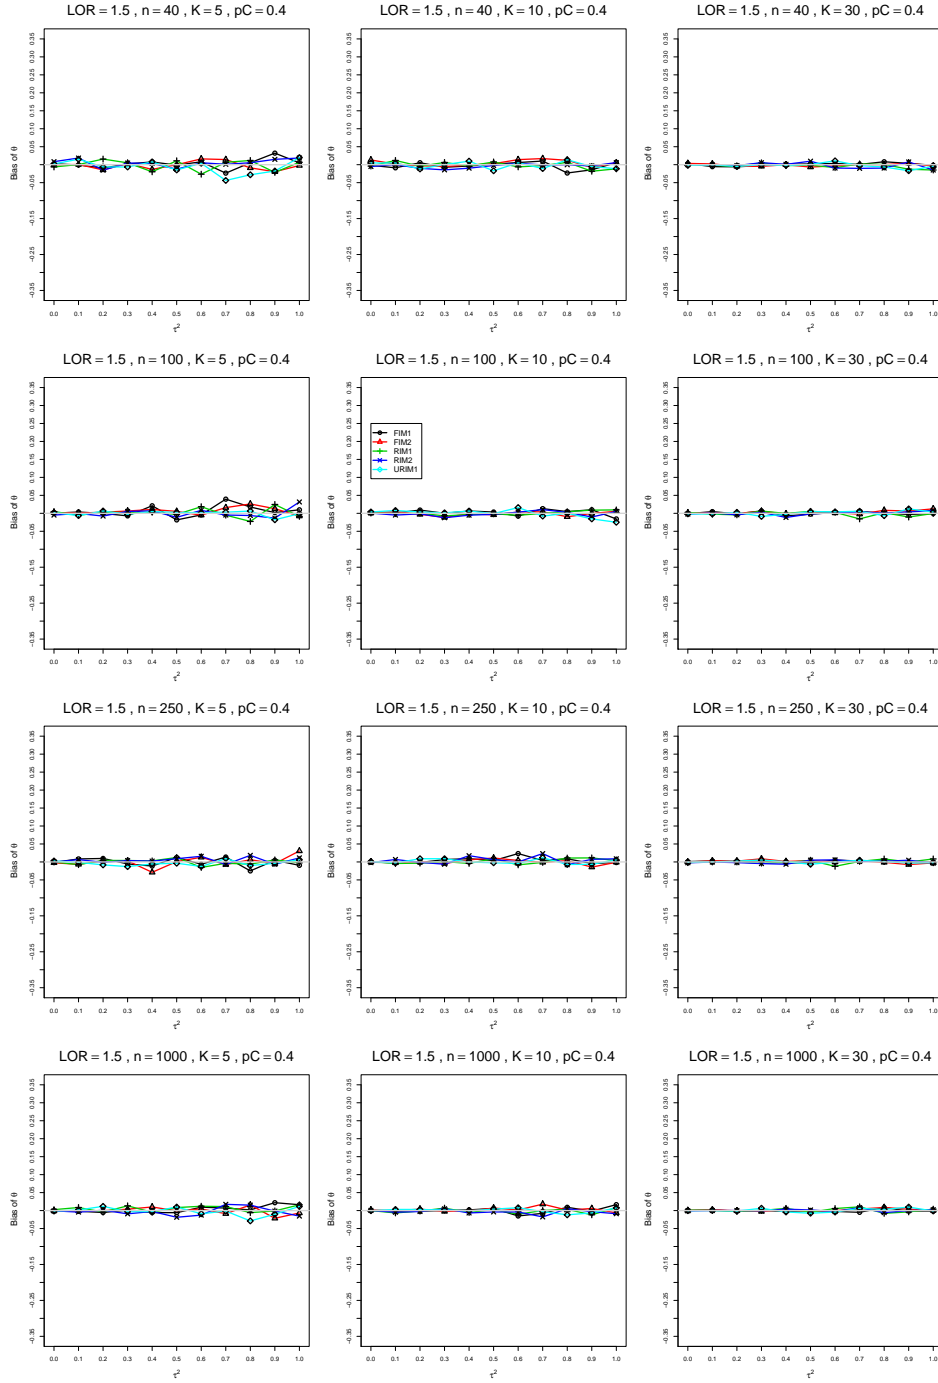

Figure A2.7.8: Bias of overall log-odds ratio  $\hat{\theta}_{SW}$  for  $\theta = 1.5$ ,  $p_C = 0.4$ ,  $\sigma^2 = 0.1$ , constant sample sizes  $n = 40, 100, 250, 1000$ . The data-generation mechanisms are FIM1 ( $\circ$ ), FIM2 ( $\triangle$ ), RIM1 ( $+$ ), RIM2 ( $\times$ ), and URIM1 ( $\diamond$ ).

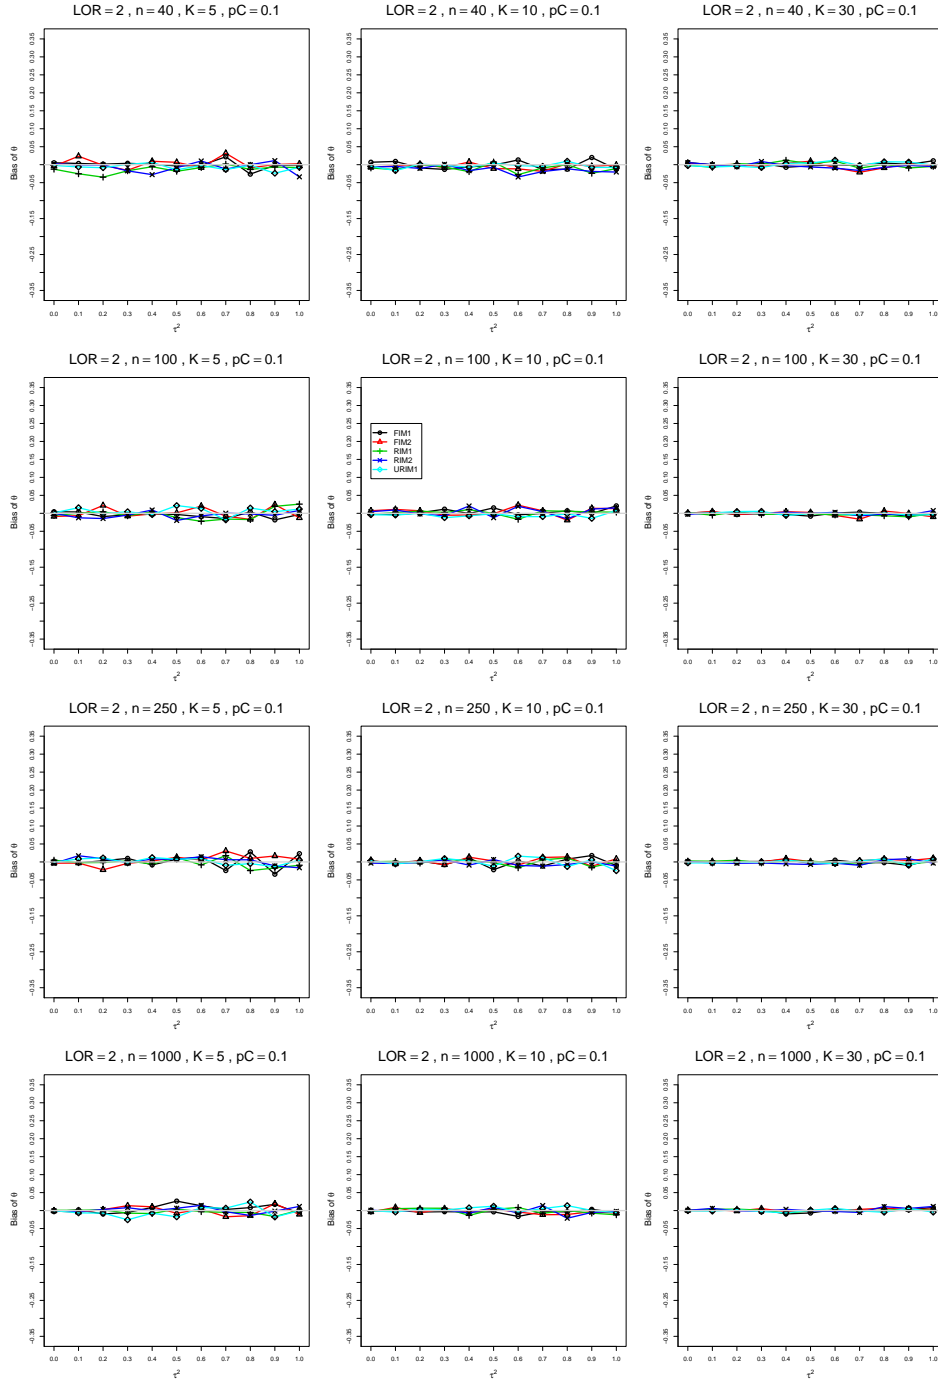

Figure A2.7.9: Bias of overall log-odds ratio  $\hat{\theta}_{SW}$  for  $\theta = 2$ ,  $p_C = 0.1$ ,  $\sigma^2 = 0.1$ , constant sample sizes  $n = 40, 100, 250, 1000$ . The data-generation mechanisms are FIM1 ( $\circ$ ), FIM2 ( $\triangle$ ), RIM1 ( $+$ ), RIM2 ( $\times$ ), and URIM1 ( $\diamond$ ).

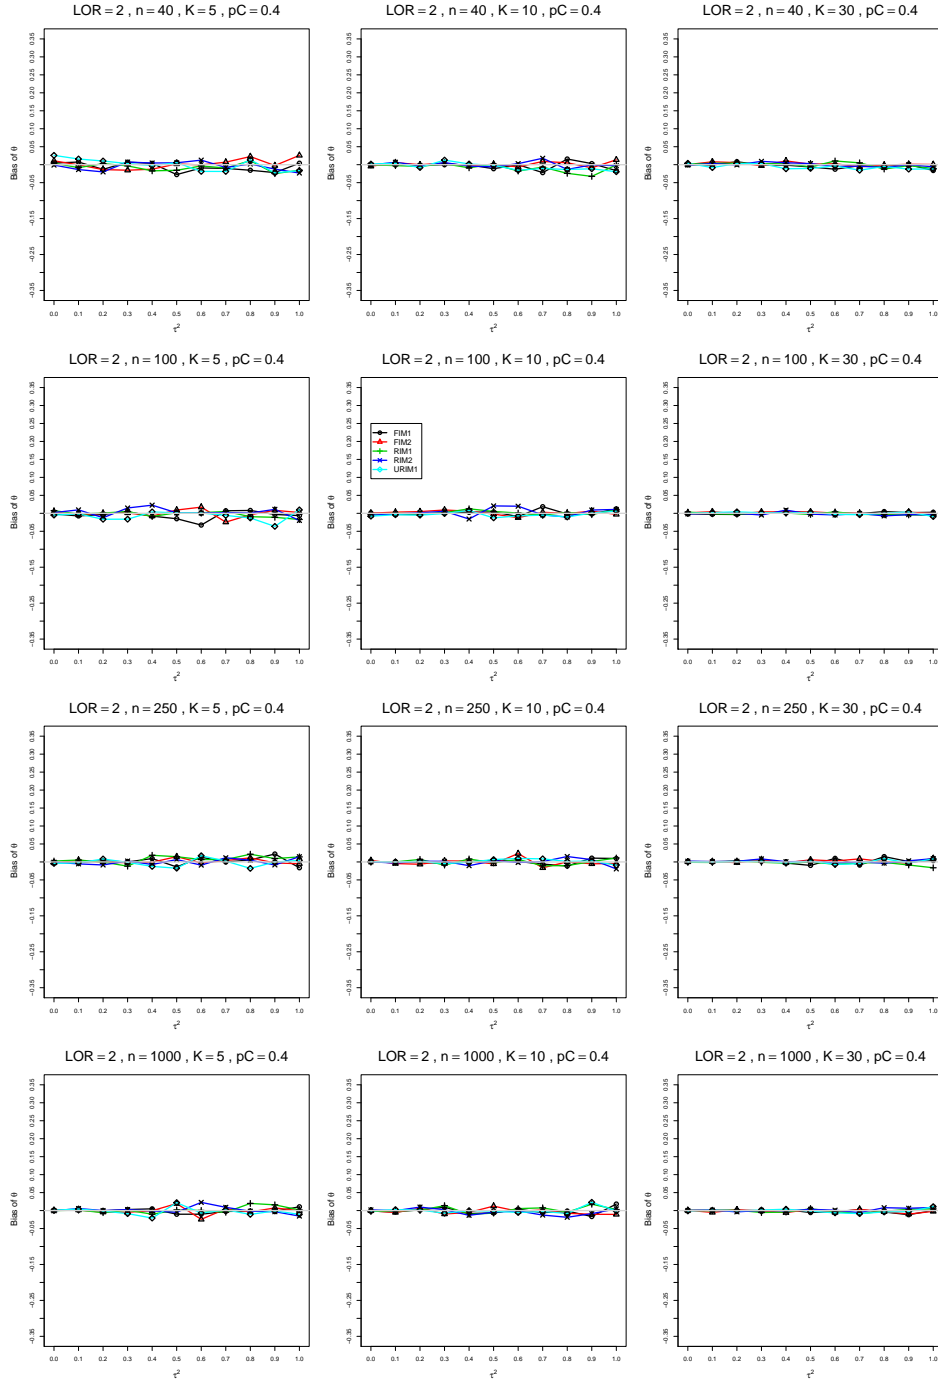

Figure A2.7.10: Bias of overall log-odds ratio  $\hat{\theta}_{SSW}$  for  $\theta = 2$ ,  $p_C = 0.4$ ,  $\sigma^2 = 0.1$ , constant sample sizes  $n = 40, 100, 250, 1000$ . The data-generation mechanisms are FIM1 ( $\circ$ ), FIM2 ( $\triangle$ ), RIM1 ( $+$ ), RIM2 ( $\times$ ), and URIM1 ( $\diamond$ ).

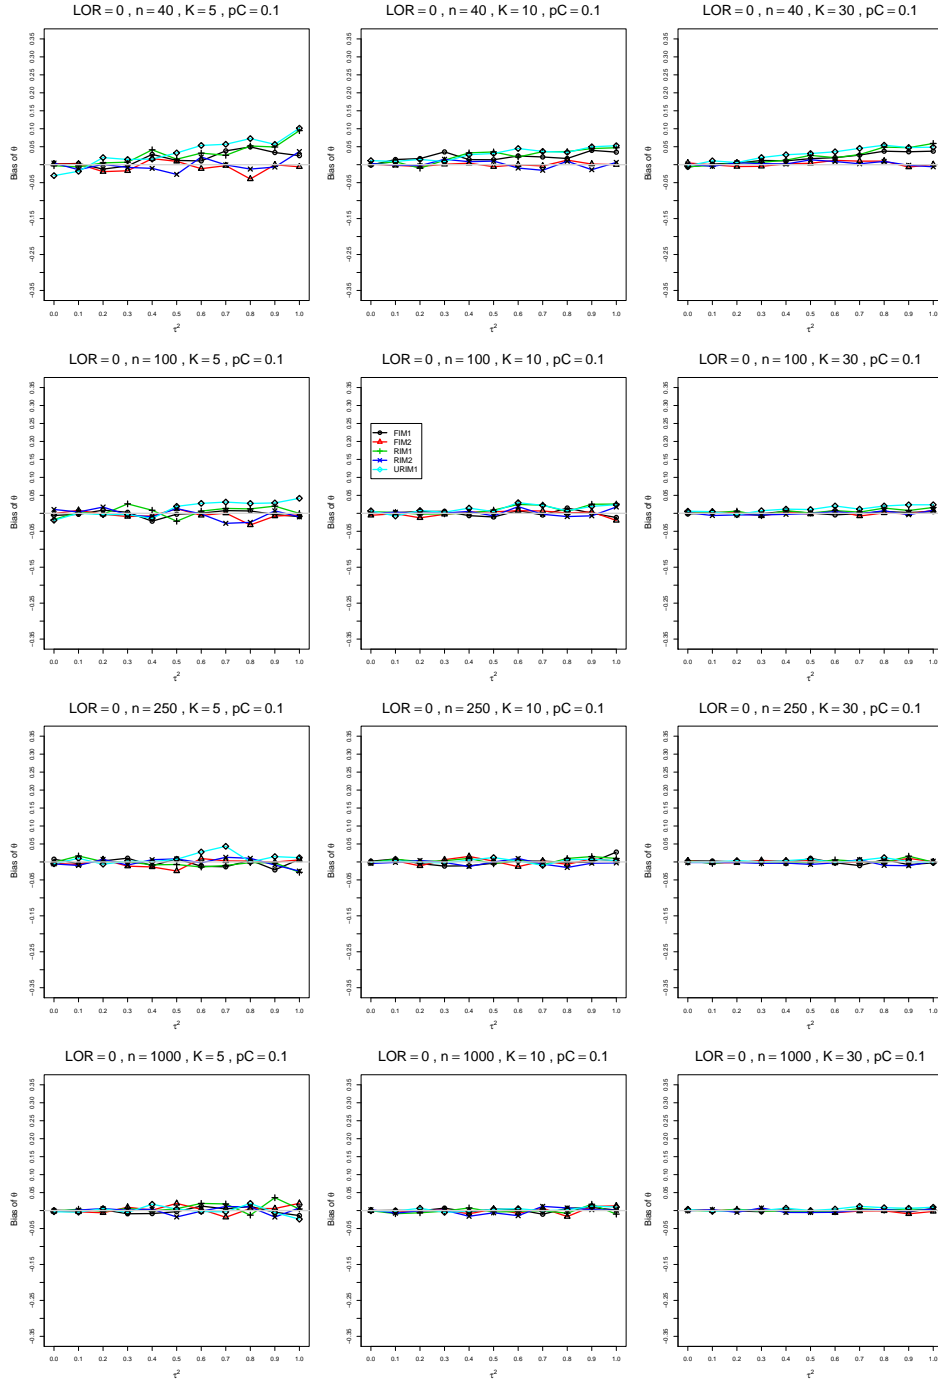

Figure A2.7.11: Bias of overall log-odds ratio  $\hat{\theta}_{SSW}$  for  $\theta = 0$ ,  $p_C = 0.1$ ,  $\sigma^2 = 0.4$ , constant sample sizes  $n = 40, 100, 250, 1000$ . The data-generation mechanisms are FIM1 ( $\circ$ ), FIM2 ( $\triangle$ ), RIM1 ( $+$ ), RIM2 ( $\times$ ), and URIM1 ( $\diamond$ ).

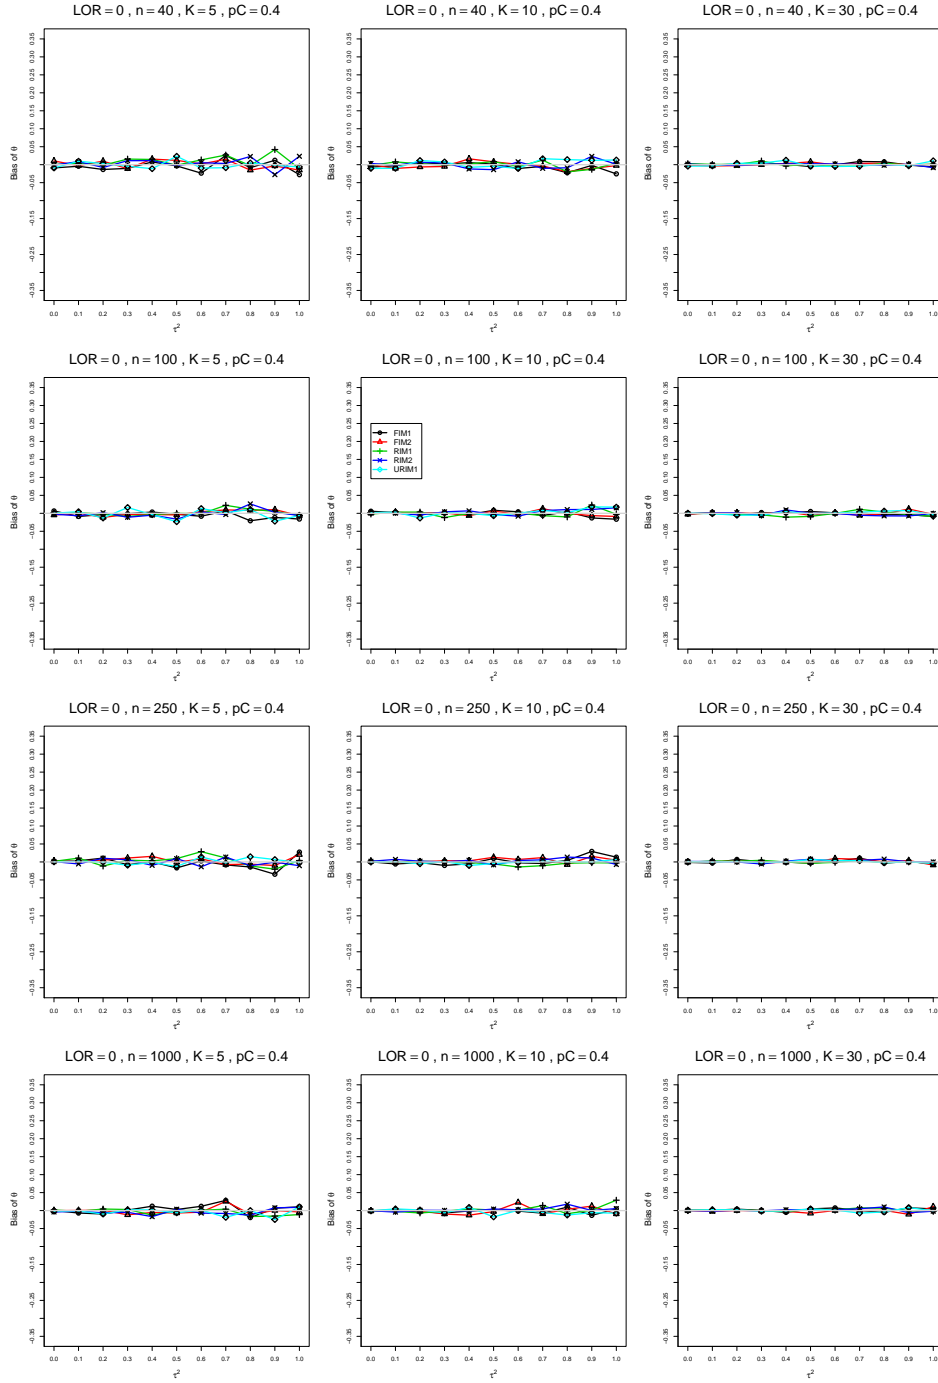

Figure A2.7.12: Bias of overall log-odds ratio  $\hat{\theta}_{SSW}$  for  $\theta = 0$ ,  $p_C = 0.4$ ,  $\sigma^2 = 0.4$ , constant sample sizes  $n = 40, 100, 250, 1000$ . The data-generation mechanisms are FIM1 ( $\circ$ ), FIM2 ( $\triangle$ ), RIM1 ( $+$ ), RIM2 ( $\times$ ), and URIM1 ( $\diamond$ ).



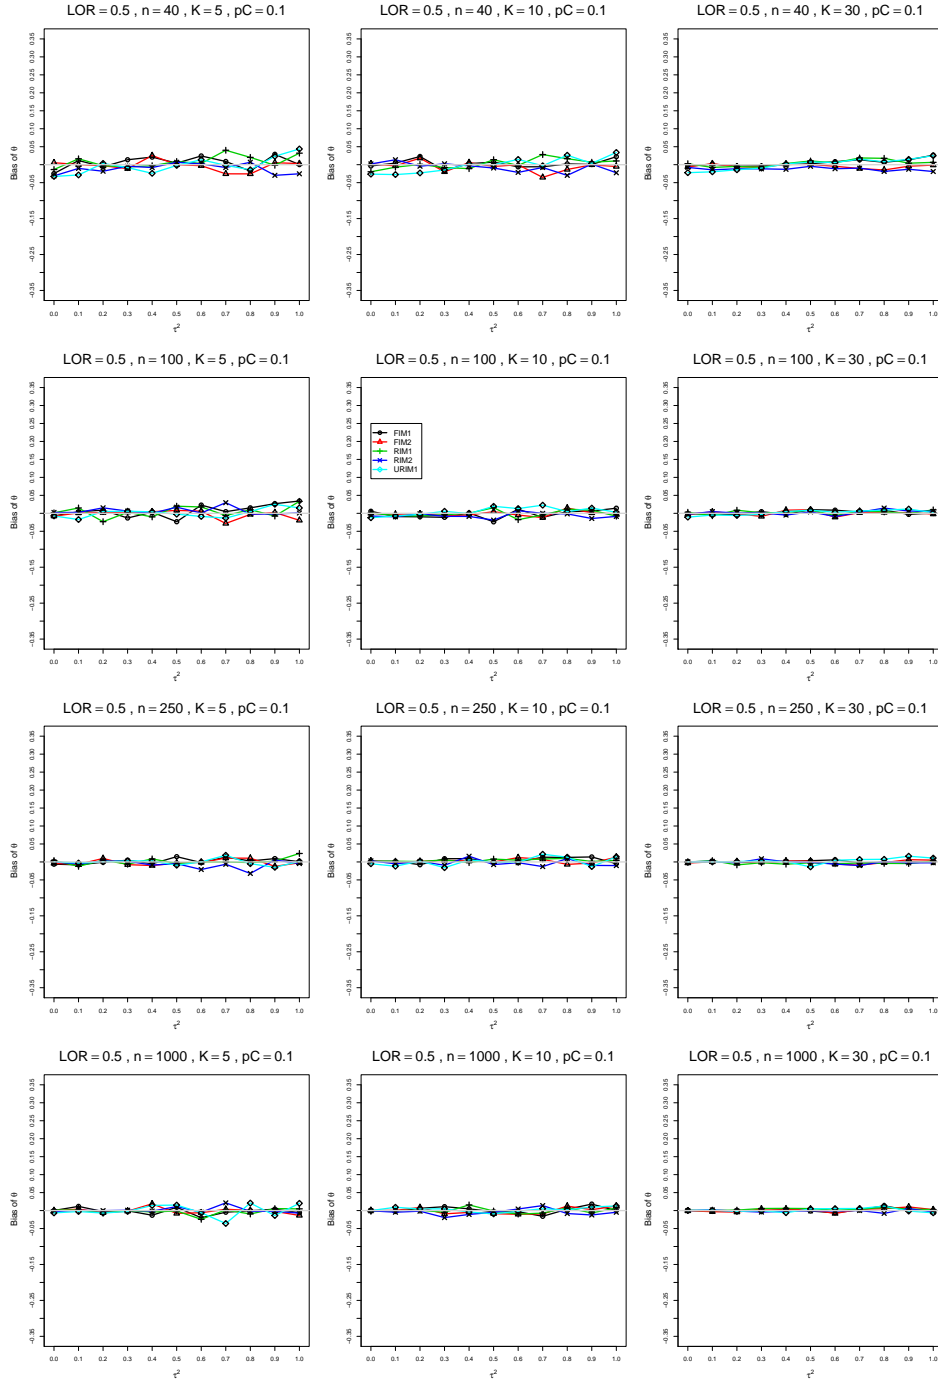

Figure A2.7.13: Bias of overall log-odds ratio  $\hat{\theta}_{SSW}$  for  $\theta = 0.5$ ,  $p_C = 0.1$ ,  $\sigma^2 = 0.4$ , constant sample sizes  $n = 40, 100, 250, 1000$ . The data-generation mechanisms are FIM1 ( $\circ$ ), FIM2 ( $\triangle$ ), RIM1 ( $+$ ), RIM2 ( $\times$ ), and URIM1 ( $\diamond$ ).

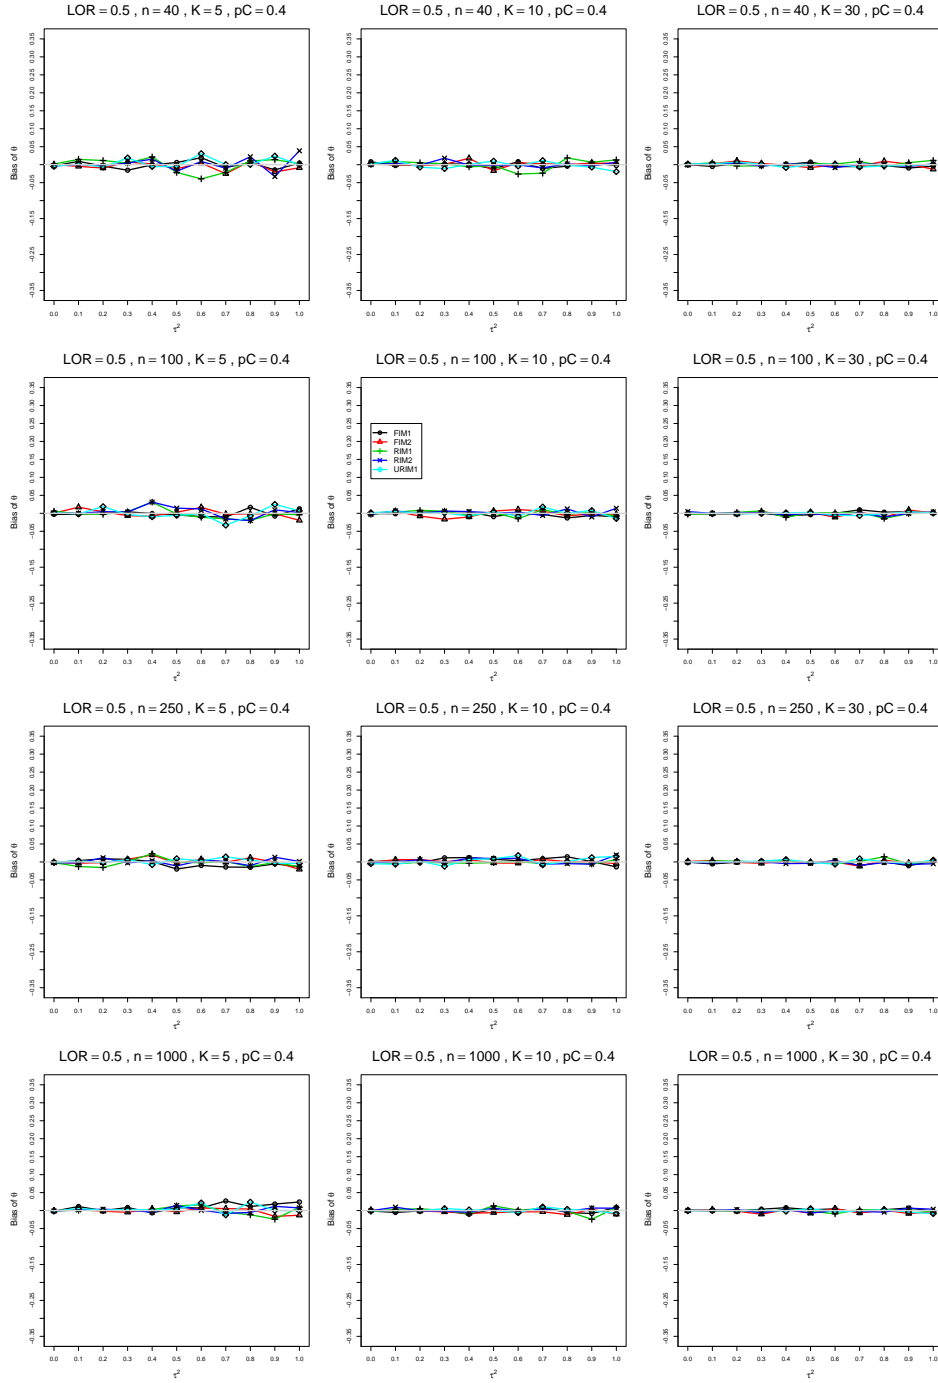

Figure A2.7.14: Bias of overall log-odds ratio  $\hat{\theta}_{SSW}$  for  $\theta = 0.5$ ,  $p_C = 0.4$ ,  $\sigma^2 = 0.4$ , constant sample sizes  $n = 40, 100, 250, 1000$ . The data-generation mechanisms are FIM1 ( $\circ$ ), FIM2 ( $\triangle$ ), RIM1 ( $+$ ), RIM2 ( $\times$ ), and URIM1 ( $\diamond$ ).

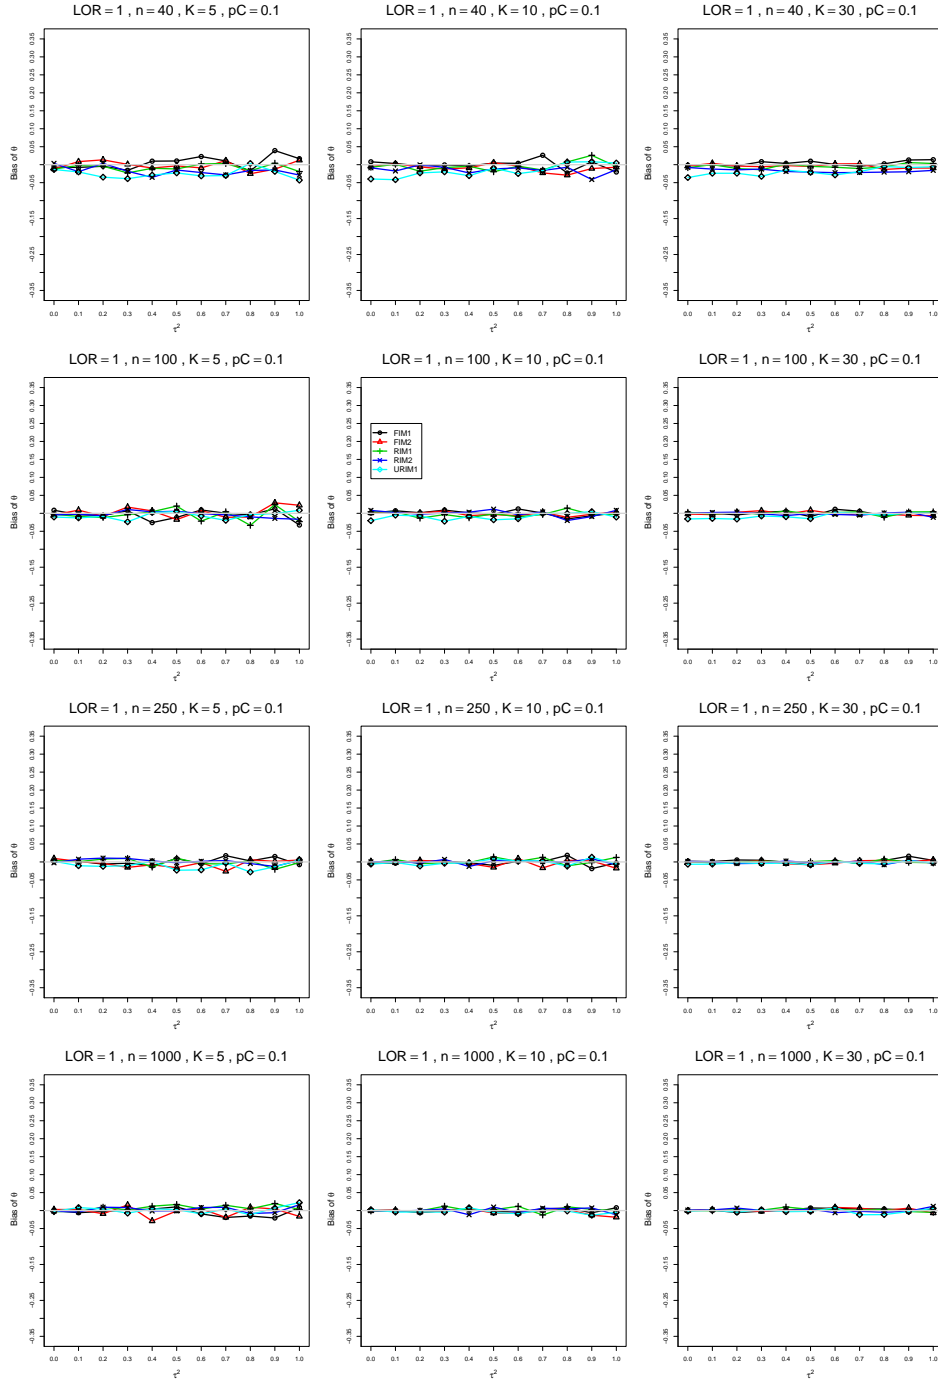

Figure A2.7.15: Bias of overall log-odds ratio  $\hat{\theta}_{SSW}$  for  $\theta = 1$ ,  $p_C = 0.1$ ,  $\sigma^2 = 0.4$ , constant sample sizes  $n = 40, 100, 250, 1000$ . The data-generation mechanisms are FIM1 ( $\circ$ ), FIM2 ( $\triangle$ ), RIM1 ( $+$ ), RIM2 ( $\times$ ), and URIM1 ( $\diamond$ ).

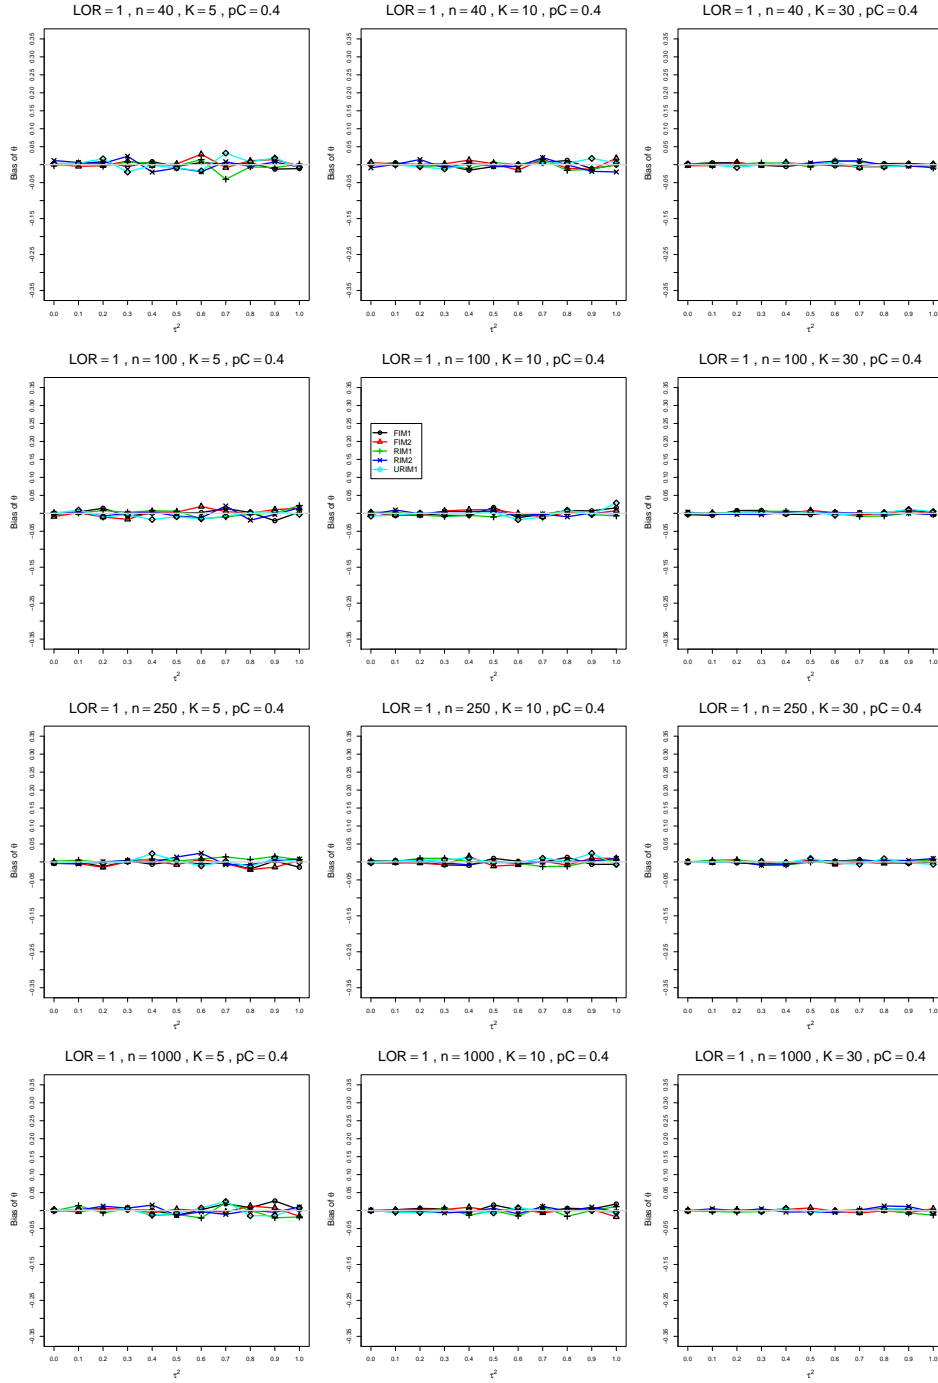

Figure A2.7.16: Bias of overall log-odds ratio  $\hat{\theta}_{SSW}$  for  $\theta = 1$ ,  $p_C = 0.4$ ,  $\sigma^2 = 0.4$ , constant sample sizes  $n = 40, 100, 250, 1000$ . The data-generation mechanisms are FIM1 ( $\circ$ ), FIM2 ( $\triangle$ ), RIM1 ( $+$ ), RIM2 ( $\times$ ), and URIM1 ( $\diamond$ ).

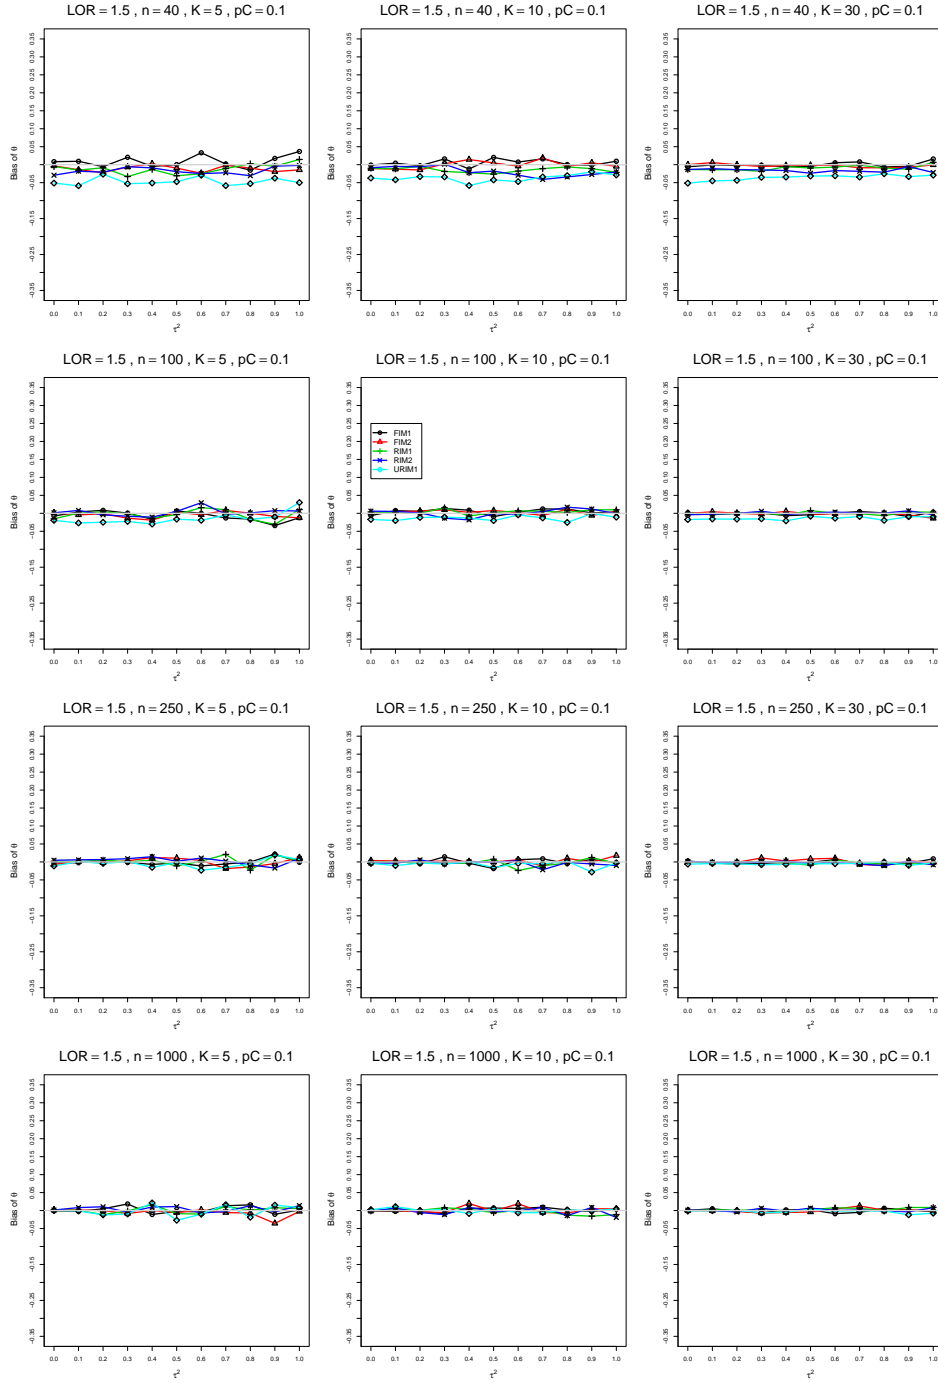

Figure A2.7.17: Bias of overall log-odds ratio  $\hat{\theta}_{SW}$  for  $\theta = 1.5$ ,  $p_C = 0.1$ ,  $\sigma^2 = 0.4$ , constant sample sizes  $n = 40, 100, 250, 1000$ . The data-generation mechanisms are FIM1 ( $\circ$ ), FIM2 ( $\triangle$ ), RIM1 ( $+$ ), RIM2 ( $\times$ ), and URIM1 ( $\diamond$ ).

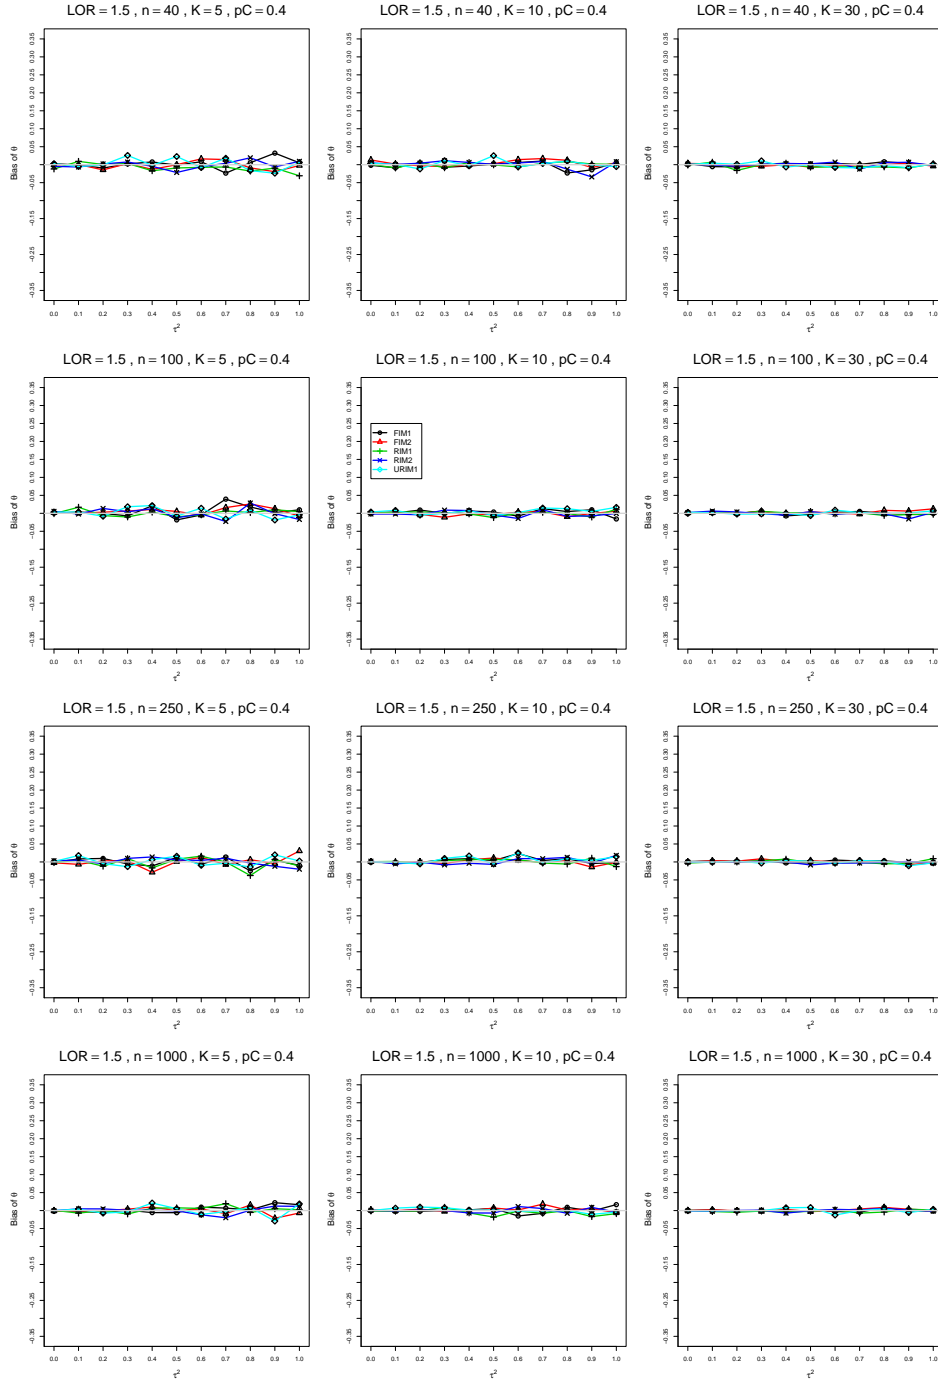

Figure A2.7.18: Bias of overall log-odds ratio  $\hat{\theta}_{SSW}$  for  $\theta = 1.5$ ,  $p_C = 0.4$ ,  $\sigma^2 = 0.4$ , constant sample sizes  $n = 40, 100, 250, 1000$ . The data-generation mechanisms are FIM1 ( $\circ$ ), FIM2 ( $\triangle$ ), RIM1 ( $+$ ), RIM2 ( $\times$ ), and URIM1 ( $\diamond$ ).

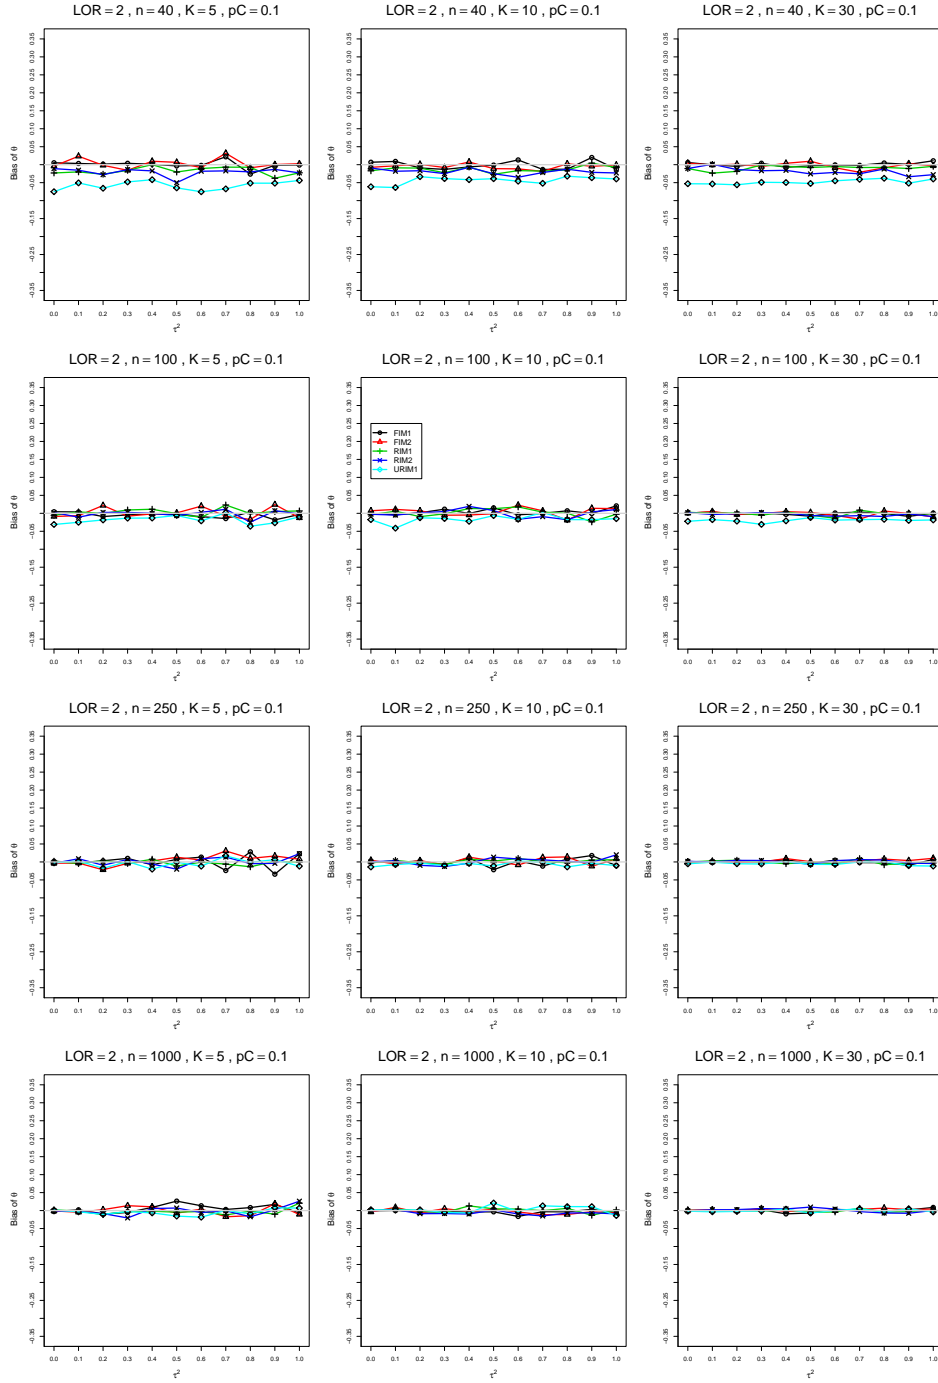

Figure A2.7.19: Bias of overall log-odds ratio  $\hat{\theta}_{SSW}$  for  $\theta = 2$ ,  $p_C = 0.1$ ,  $\sigma^2 = 0.4$ , constant sample sizes  $n = 40, 100, 250, 1000$ . The data-generation mechanisms are FIM1 ( $\circ$ ), FIM2 ( $\triangle$ ), RIM1 ( $+$ ), RIM2 ( $\times$ ), and URIM1 ( $\diamond$ ).

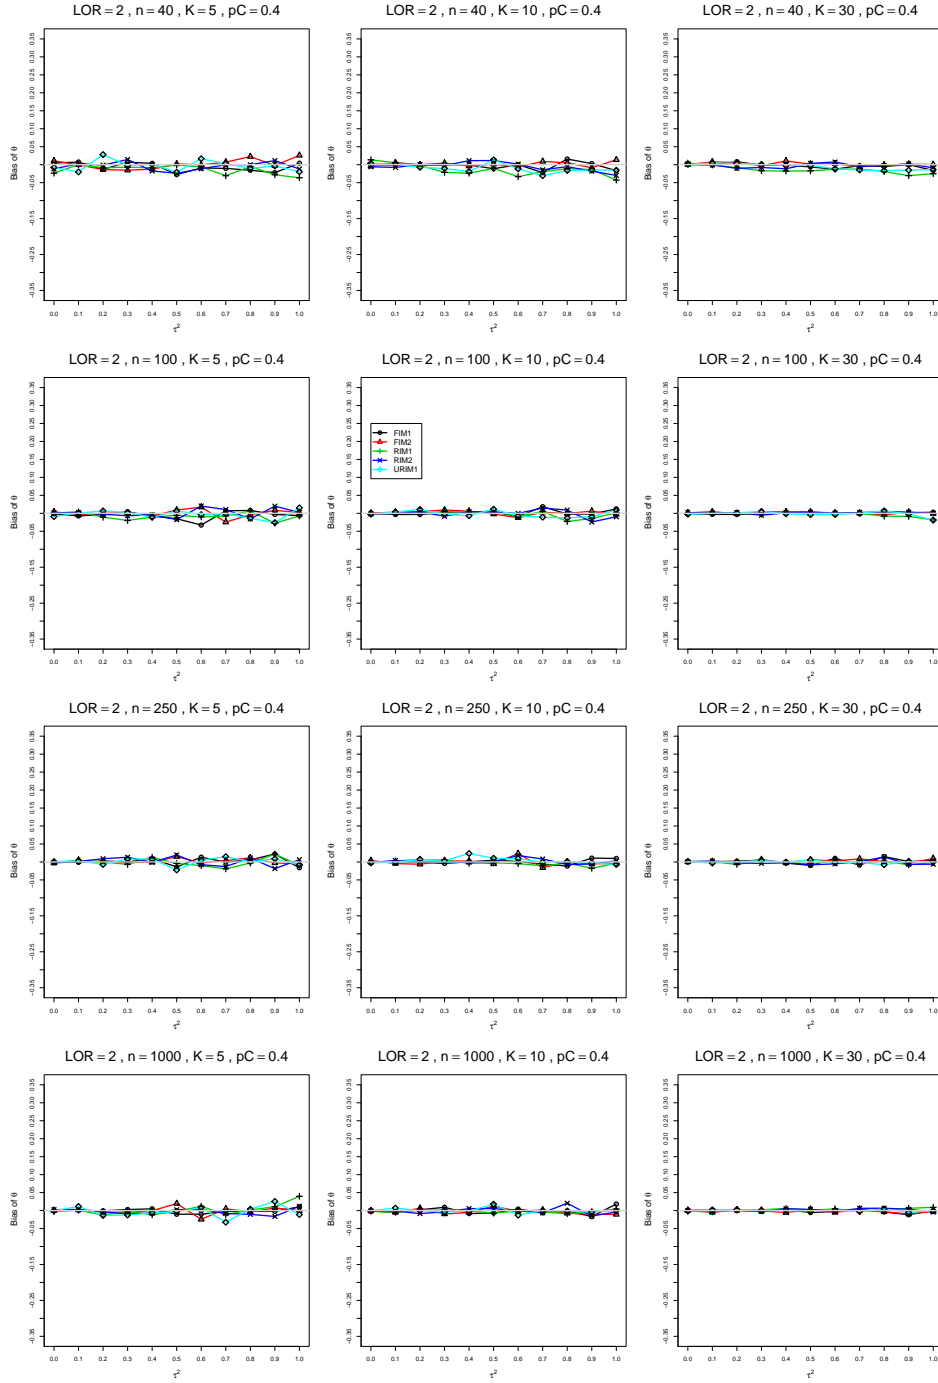

Figure A2.7.20: Bias of overall log-odds ratio  $\hat{\theta}_{SSW}$  for  $\theta = 2$ ,  $p_C = 0.4$ ,  $\sigma^2 = 0.4$ , constant sample sizes  $n = 40, 100, 250, 1000$ . The data-generation mechanisms are FIM1 ( $\circ$ ), FIM2 ( $\triangle$ ), RIM1 ( $+$ ), RIM2 ( $\times$ ), and URIM1 ( $\diamond$ ).



### A3: Coverage estimators of $\theta$ for log-odds-ratio

Each panel of a figure corresponds to a value of  $n$  ( $= 40, 100, 250, 1000$ ) and a value of  $K$  ( $= 5, 10, 30$ ) and has  $\tau^2 = 0.0(0.1)1.0$  on the horizontal axis.

The data-generation mechanisms are

- FIM1 - Fixed-intercept model with  $c = 0$
- FIM2 - Fixed-intercept model with  $c = 1/2$
- RIM1 - Random-intercept model with  $c = 0$
- RIM2 - Random-intercept model with  $c = 1/2$
- URIM1 - Random-intercept model with  $c = 0$  and  $p_{iC}$  is uniformly distributed on  $[p_{iC} - \sigma\sqrt{3}p_{iC}(1 - p_{iC}), p_{iC} + \sigma\sqrt{3}p_{iC}(1 - p_{iC})]$

The interval point estimators of  $\theta$  are

- $\hat{\theta}_{DL}$  - DerSimonian-Laird
- $\hat{\theta}_{REML}$  - Restricted maximum-likelihood
- $\hat{\theta}_{MP}$  - Mandel-Paule
- $\hat{\theta}_{KD}$  - Kulinskaya-Dollinger
- $\hat{\theta}_{FIM2}$  - Estimator of  $\theta$  in the FIM2 GLMM
- $\hat{\theta}_{RIM2}$  - Estimator of  $\theta$  in the RIM2 GLMM
- $\hat{\theta}_{SSW}$  - Estimator of  $\theta$  based on the Hartung-Knapp-Sidik-Jonkman with KD based modification and an interval based on the sample-size-weighted estimator

### A3.1 Coverage of $\hat{\theta}_{DL}$

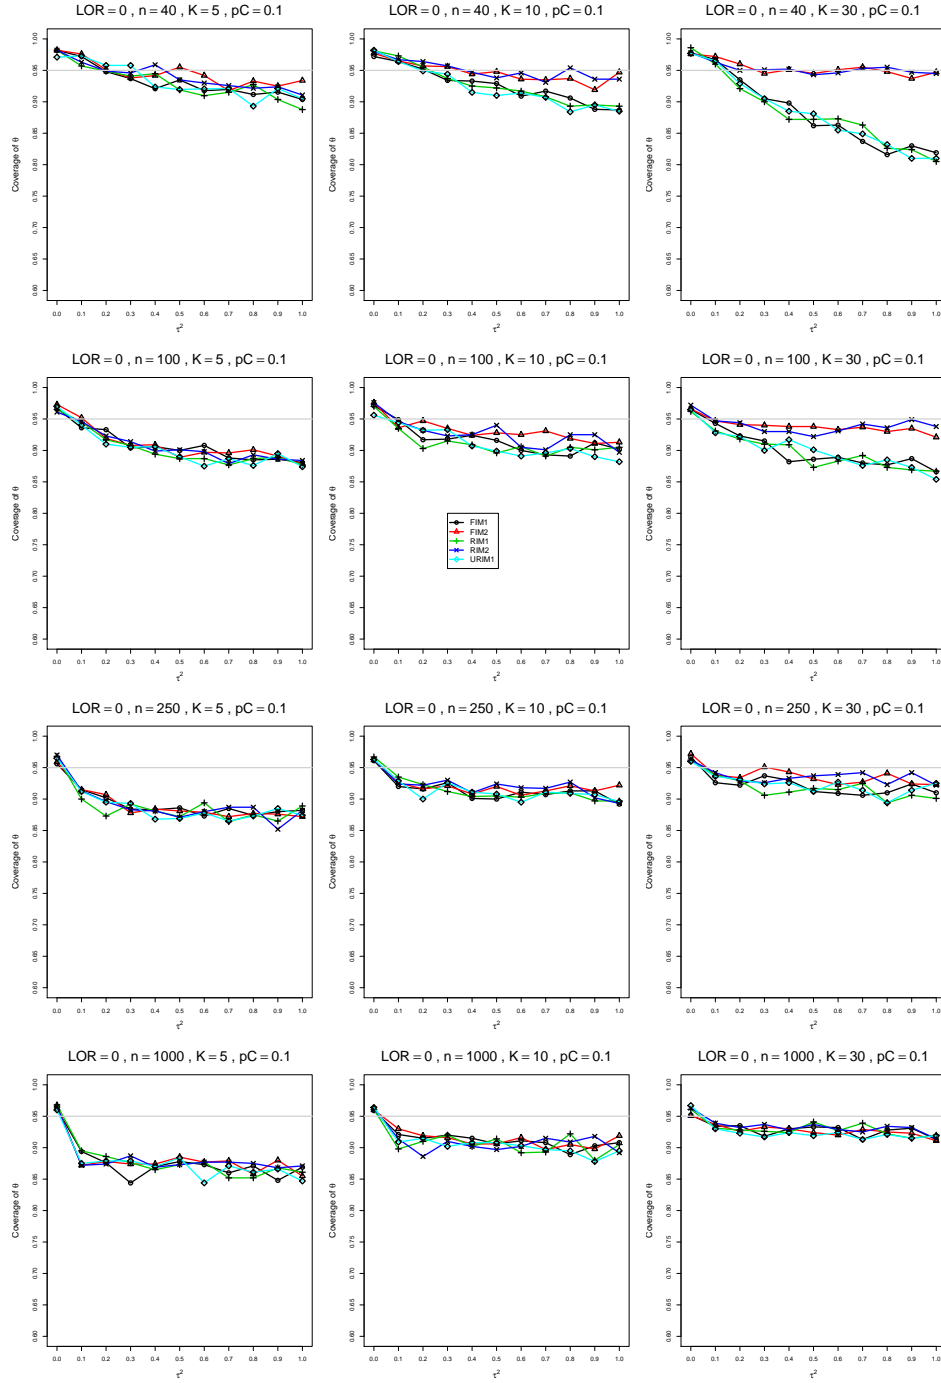

Figure A3.1.1: Coverage of the DerSimonian-Laird confidence interval for  $\theta = 0$ ,  $p_C = 0.1$ ,  $\sigma^2 = 0.1$ , constant sample sizes  $n = 40, 100, 250, 1000$ . The data-generation mechanisms are FIM1 ( $\circ$ ), FIM2 ( $\triangle$ ), RIM1 (+), RIM2 ( $\times$ ), and URIM1 ( $\diamond$ ).

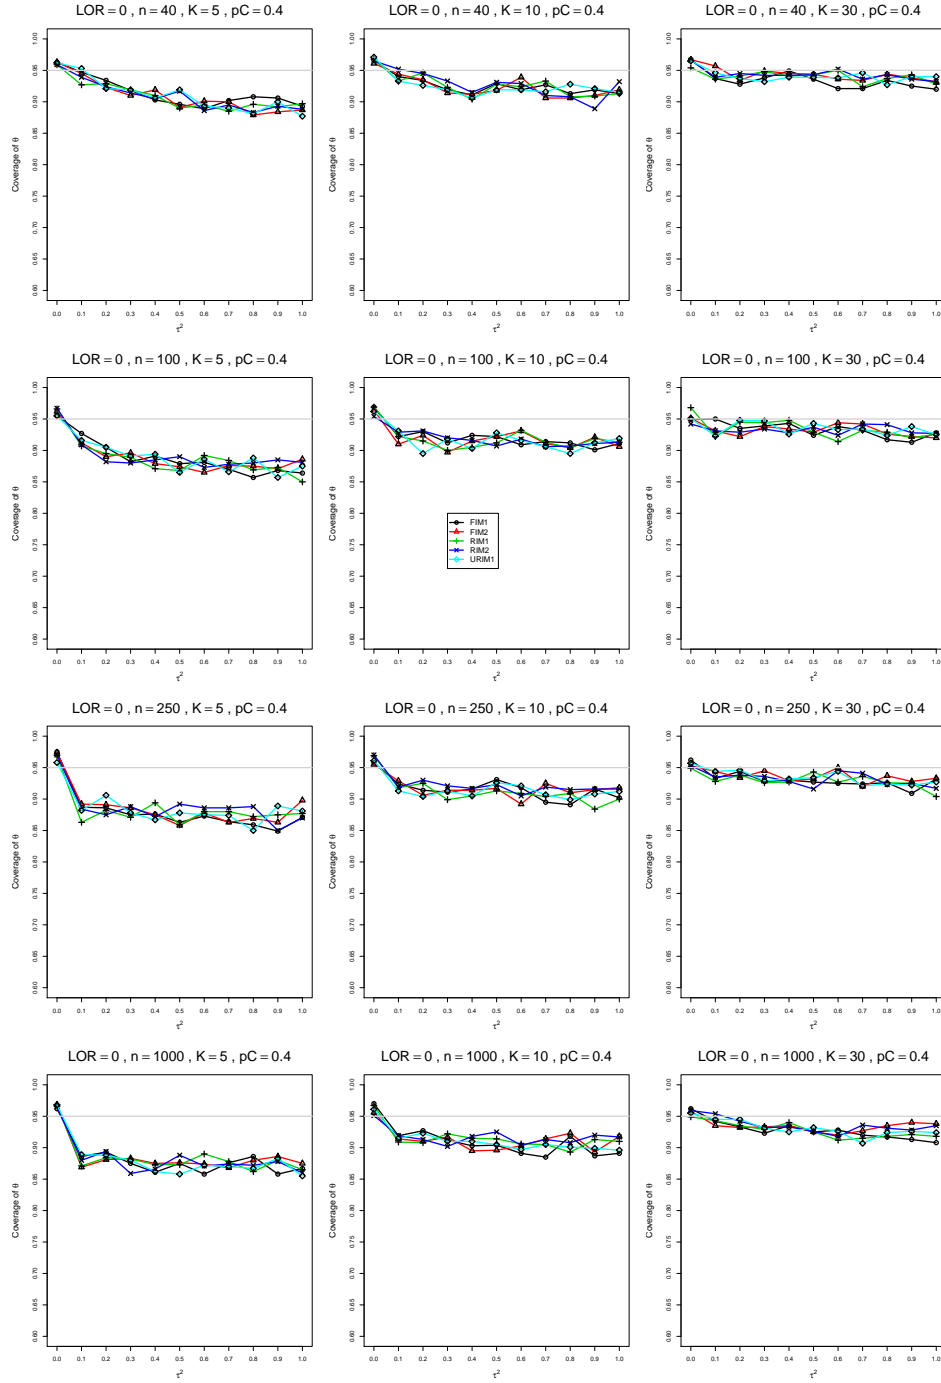

Figure A3.1.2: Coverage of the DerSimonian-Laird confidence interval for  $\theta = 0$ ,  $p_C = 0.4$ ,  $\sigma^2 = 0.1$ , constant sample sizes  $n = 40, 100, 250, 1000$ . The data-generation mechanisms are FIM1 ( $\circ$ ), FIM2 ( $\triangle$ ), RIM1 ( $+$ ), RIM2 ( $\times$ ), and URIM1 ( $\diamond$ ).

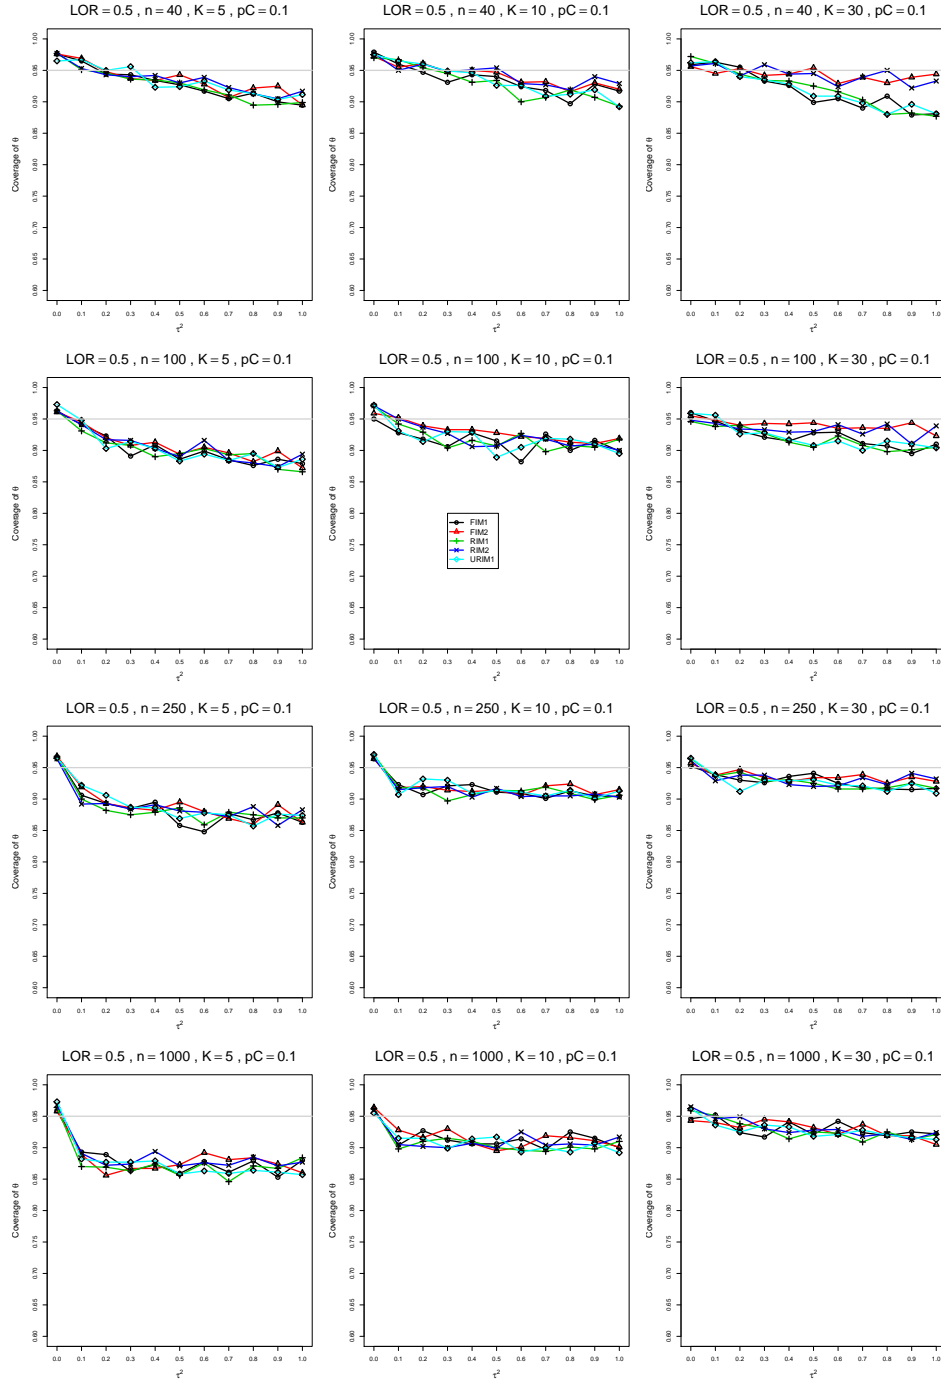

Figure A3.1.3: Coverage of the DerSimonian-Laird confidence interval for  $\theta = 0.5$ ,  $p_C = 0.1$ ,  $\sigma^2 = 0.1$ , constant sample sizes  $n = 40, 100, 250, 1000$ . The data-generation mechanisms are FIM1 ( $\circ$ ), FIM2 ( $\triangle$ ), RIM1 ( $+$ ), RIM2 ( $\times$ ), and URIM1 ( $\diamond$ ).

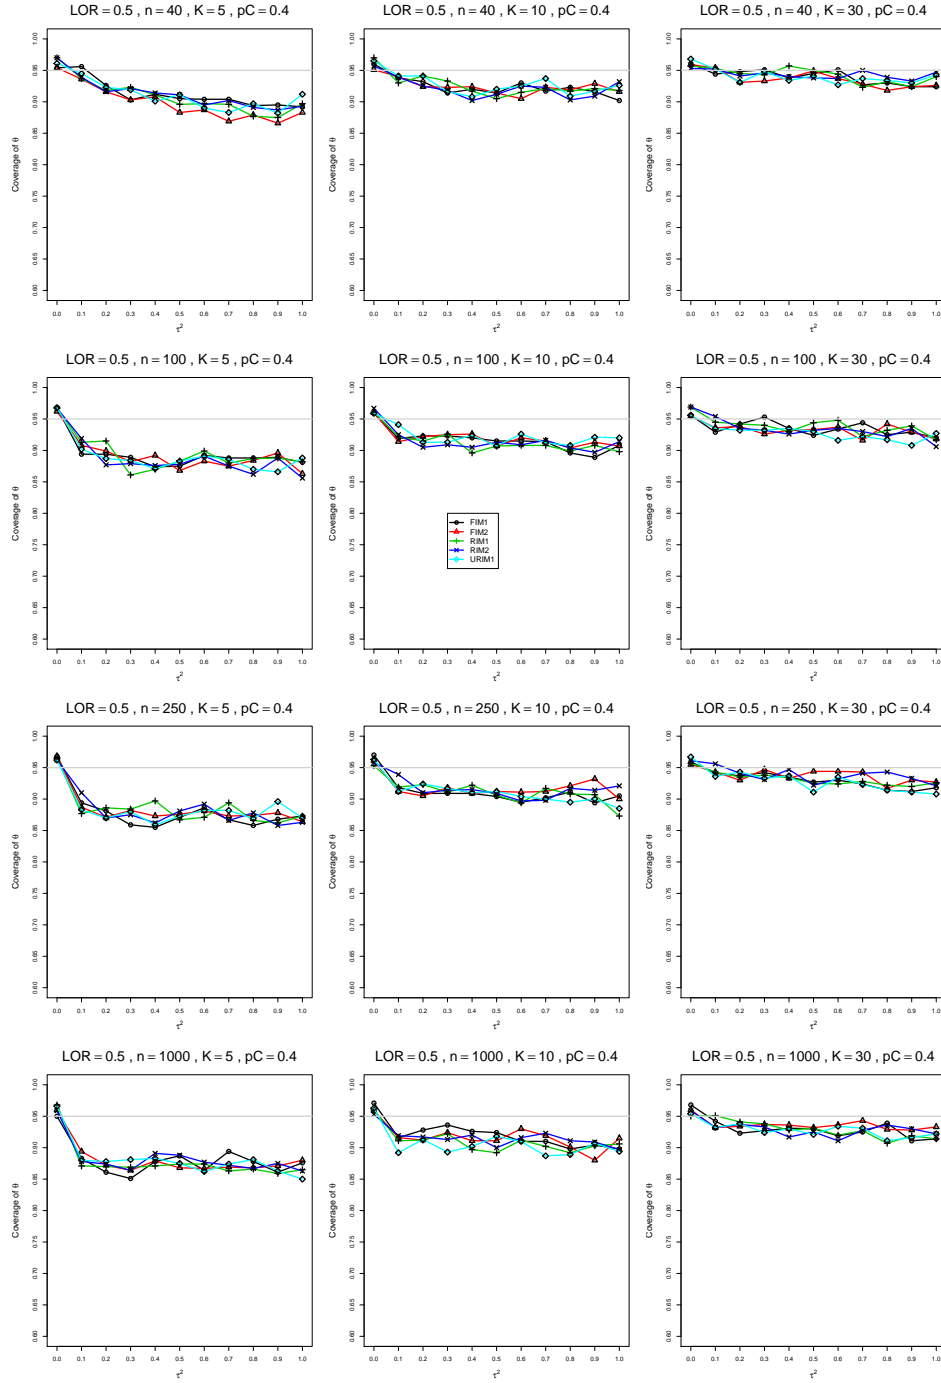

Figure A3.1.4: Coverage of the DerSimonian-Laird confidence interval for  $\theta = 0.5$ ,  $p_C = 0.4$ ,  $\sigma^2 = 0.1$ , constant sample sizes  $n = 40, 100, 250, 1000$ . The data-generation mechanisms are FIM1 ( $\circ$ ), FIM2 ( $\triangle$ ), RIM1 (+), RIM2 ( $\times$ ), and URIM1 ( $\diamond$ ).

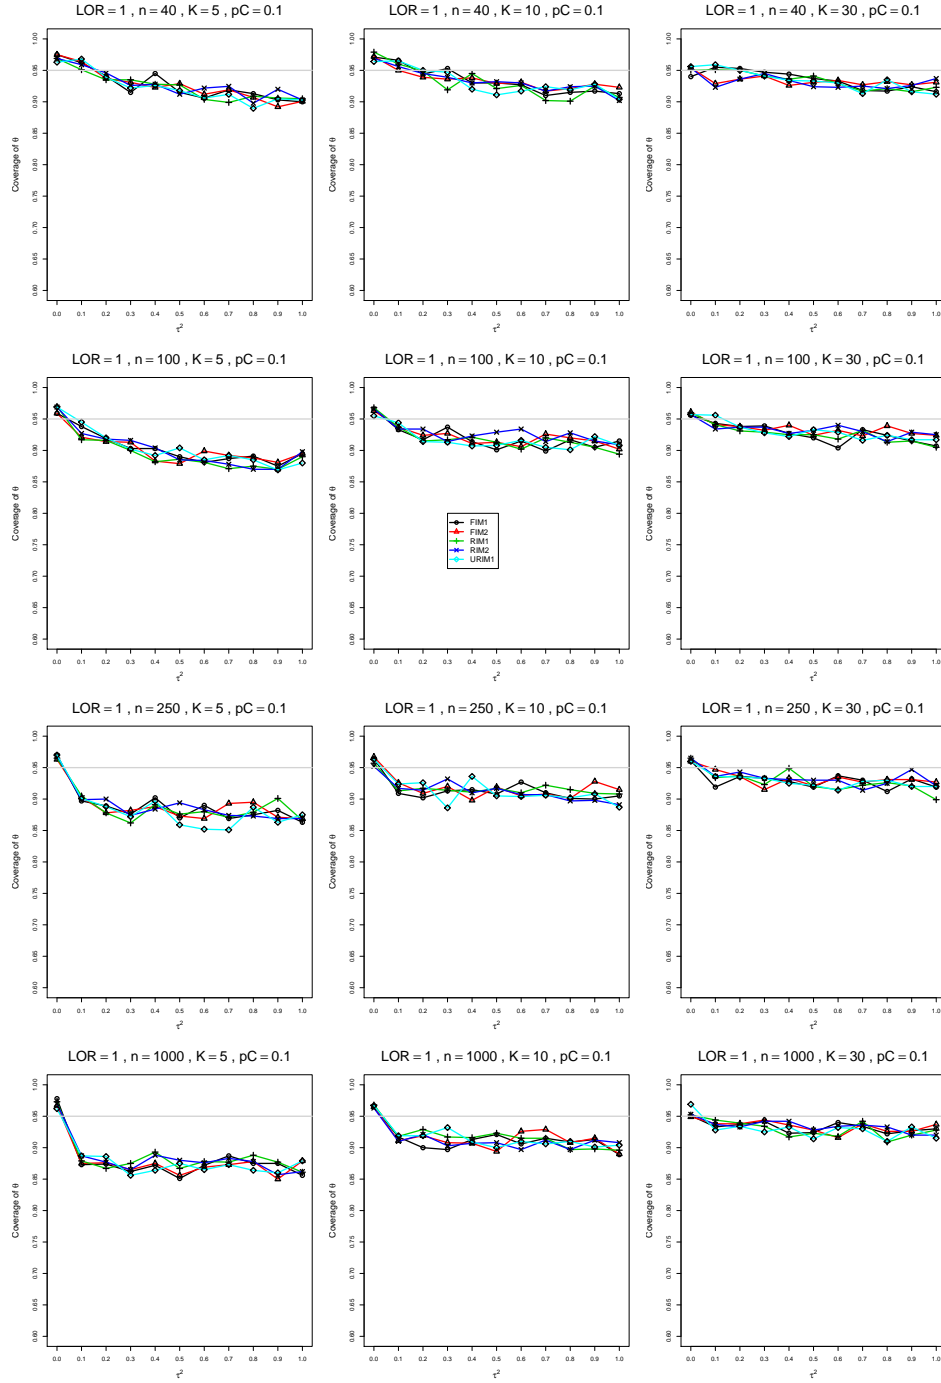

Figure A3.1.5: Coverage of the DerSimonian-Laird confidence interval for  $\theta = 1$ ,  $p_C = 0.1$ ,  $\sigma^2 = 0.1$ , constant sample sizes  $n = 40, 100, 250, 1000$ . The data-generation mechanisms are FIM1 ( $\circ$ ), FIM2 ( $\triangle$ ), RIM1 ( $+$ ), RIM2 ( $\times$ ), and URIM1 ( $\diamond$ ).

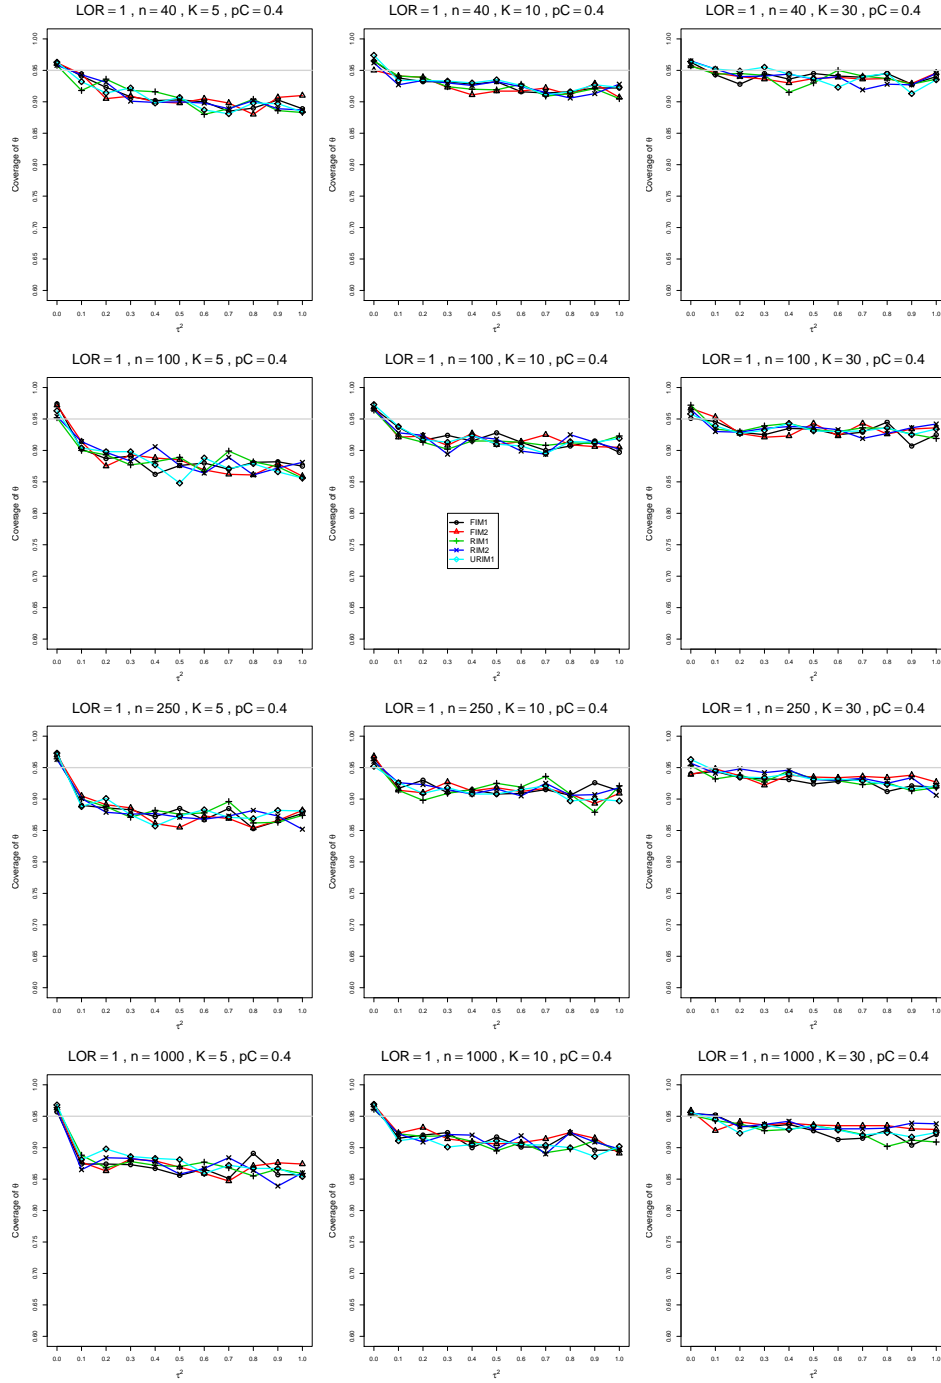

Figure A3.1.6: Coverage of the DerSimonian-Laird confidence interval for  $\theta = 1$ ,  $p_C = 0.4$ ,  $\sigma^2 = 0.1$ , constant sample sizes  $n = 40, 100, 250, 1000$ . The data-generation mechanisms are FIM1 ( $\circ$ ), FIM2 ( $\triangle$ ), RIM1 ( $+$ ), RIM2 ( $\times$ ), and URIM1 ( $\diamond$ ).



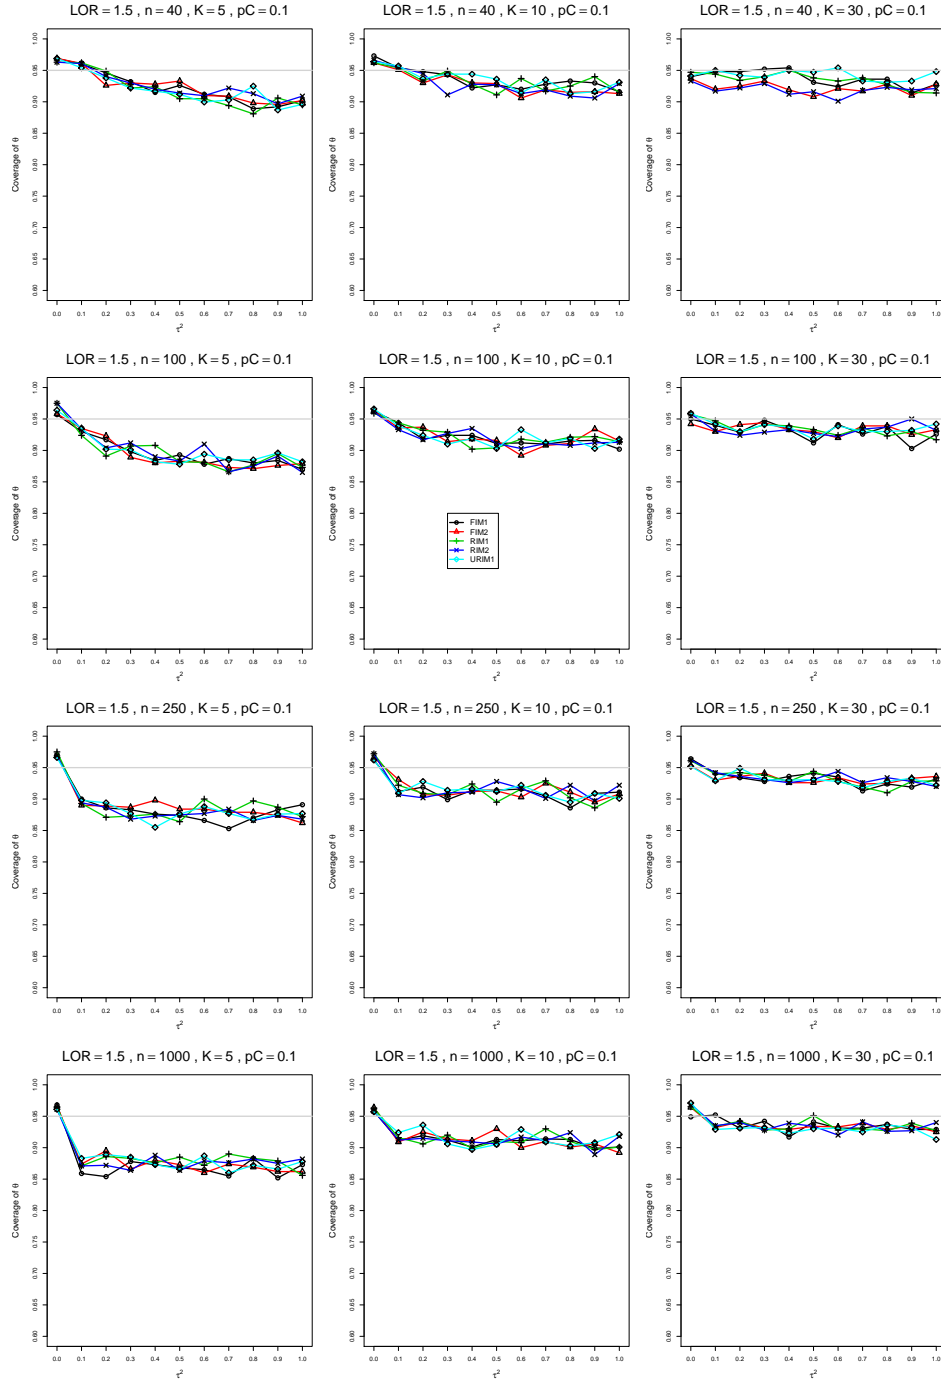

Figure A3.1.7: Coverage of the DerSimonian-Laird confidence interval for  $\theta = 1.5$ ,  $p_C = 0.1$ ,  $\sigma^2 = 0.1$ , constant sample sizes  $n = 40, 100, 250, 1000$ . The data-generation mechanisms are FIM1 ( $\circ$ ), FIM2 ( $\triangle$ ), RIM1 (+), RIM2 ( $\times$ ), and URIM1 ( $\diamond$ ).

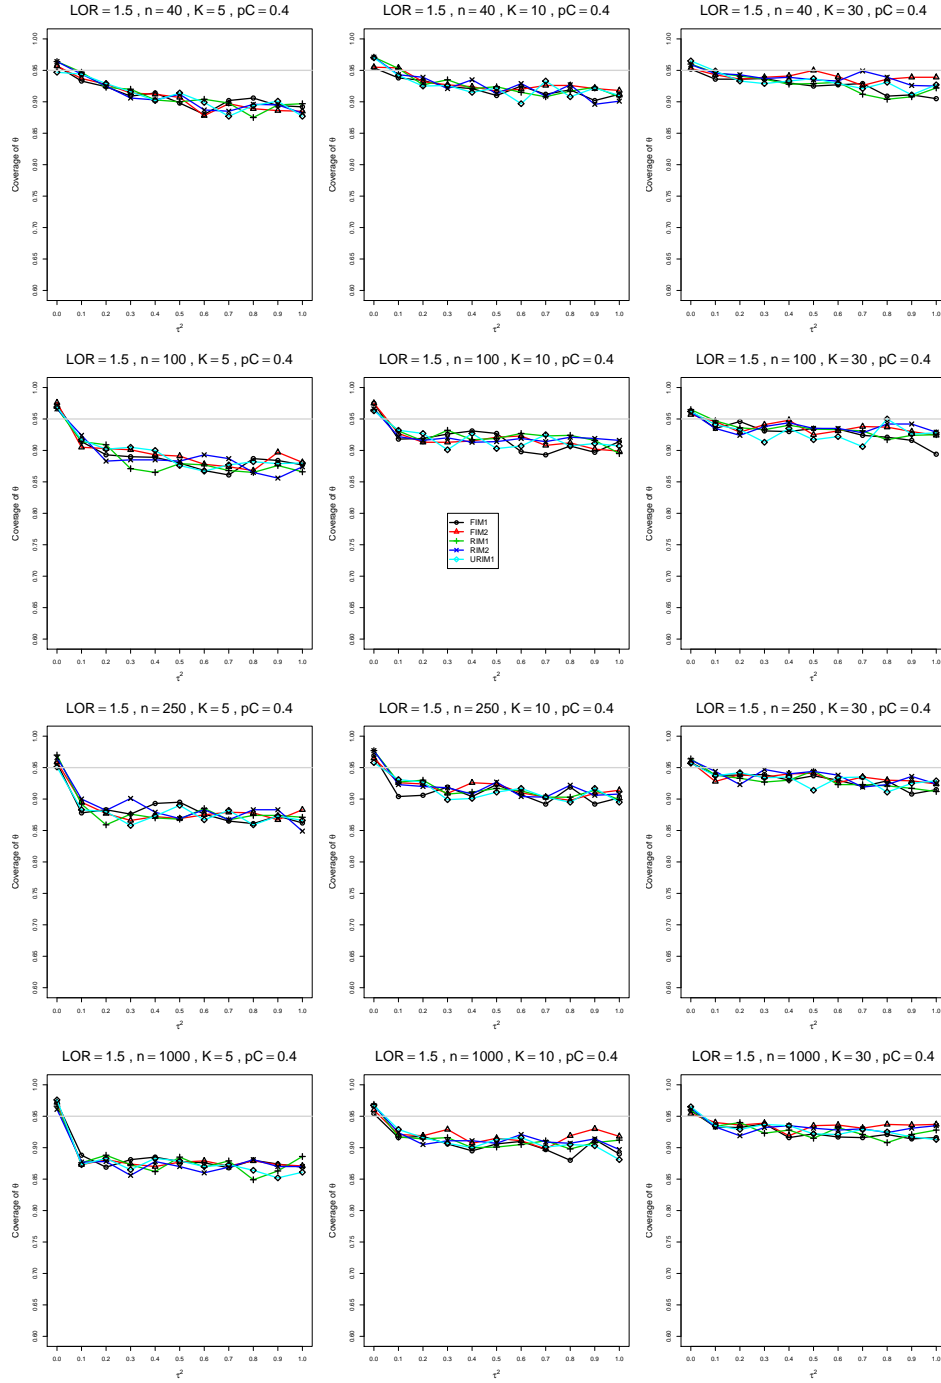

Figure A3.1.8: Coverage of the DerSimonian-Laird confidence interval for  $\theta = 1.5$ ,  $p_C = 0.4$ ,  $\sigma^2 = 0.1$ , constant sample sizes  $n = 40, 100, 250, 1000$ . The data-generation mechanisms are FIM1 ( $\circ$ ), FIM2 ( $\triangle$ ), RIM1 (+), RIM2 ( $\times$ ), and URIM1 ( $\diamond$ ).

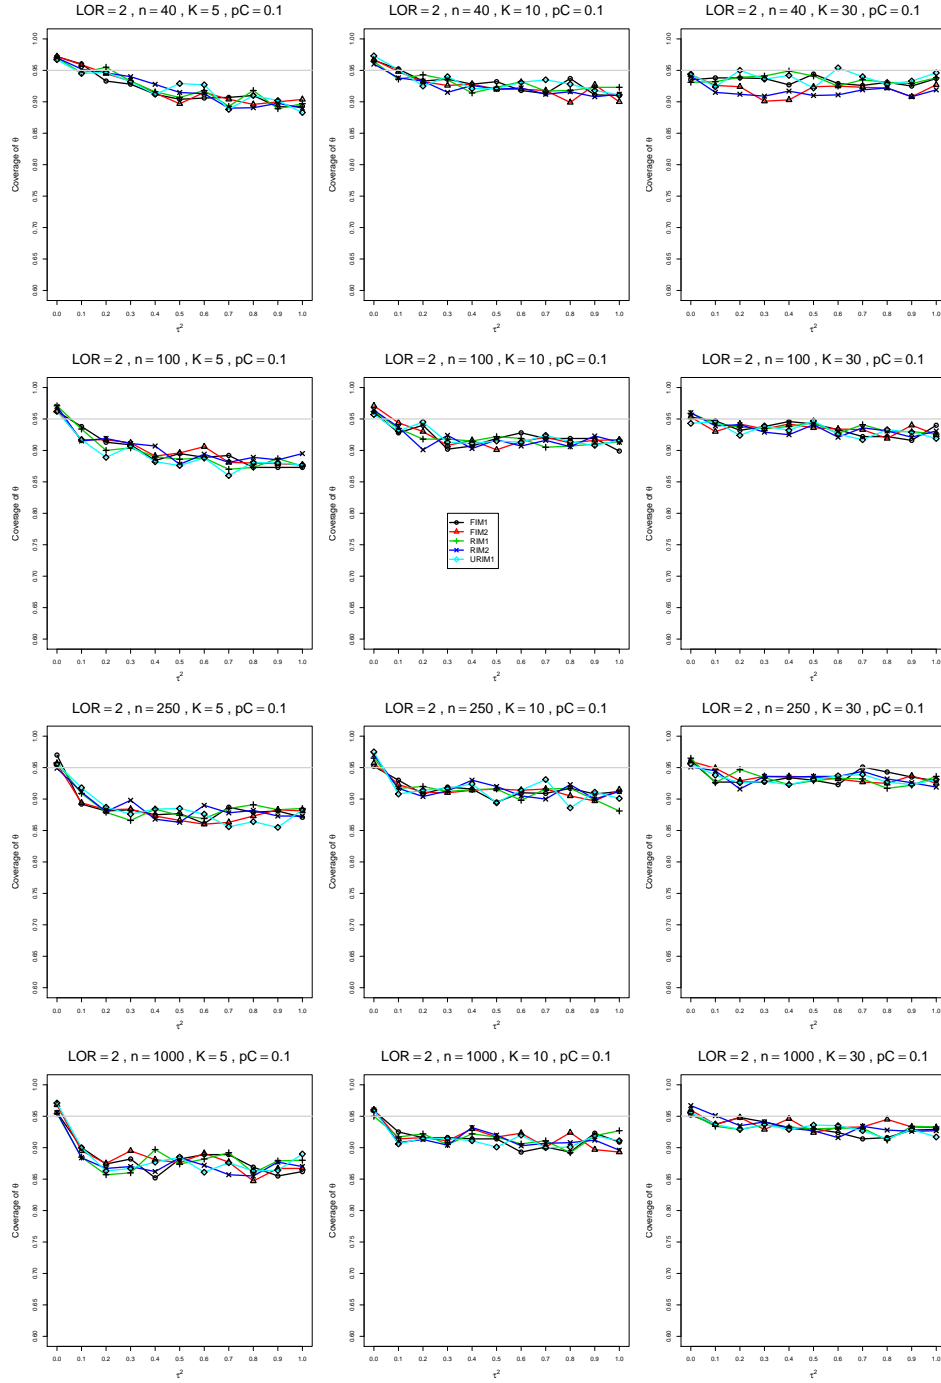

Figure A3.1.9: Coverage of the DerSimonian-Laird confidence interval for  $\theta = 2$ ,  $p_C = 0.1$ ,  $\sigma^2 = 0.1$ , constant sample sizes  $n = 40, 100, 250, 1000$ . The data-generation mechanisms are FIM1 ( $\circ$ ), FIM2 ( $\triangle$ ), RIM1 (+), RIM2 ( $\times$ ), and URIM1 ( $\diamond$ ).

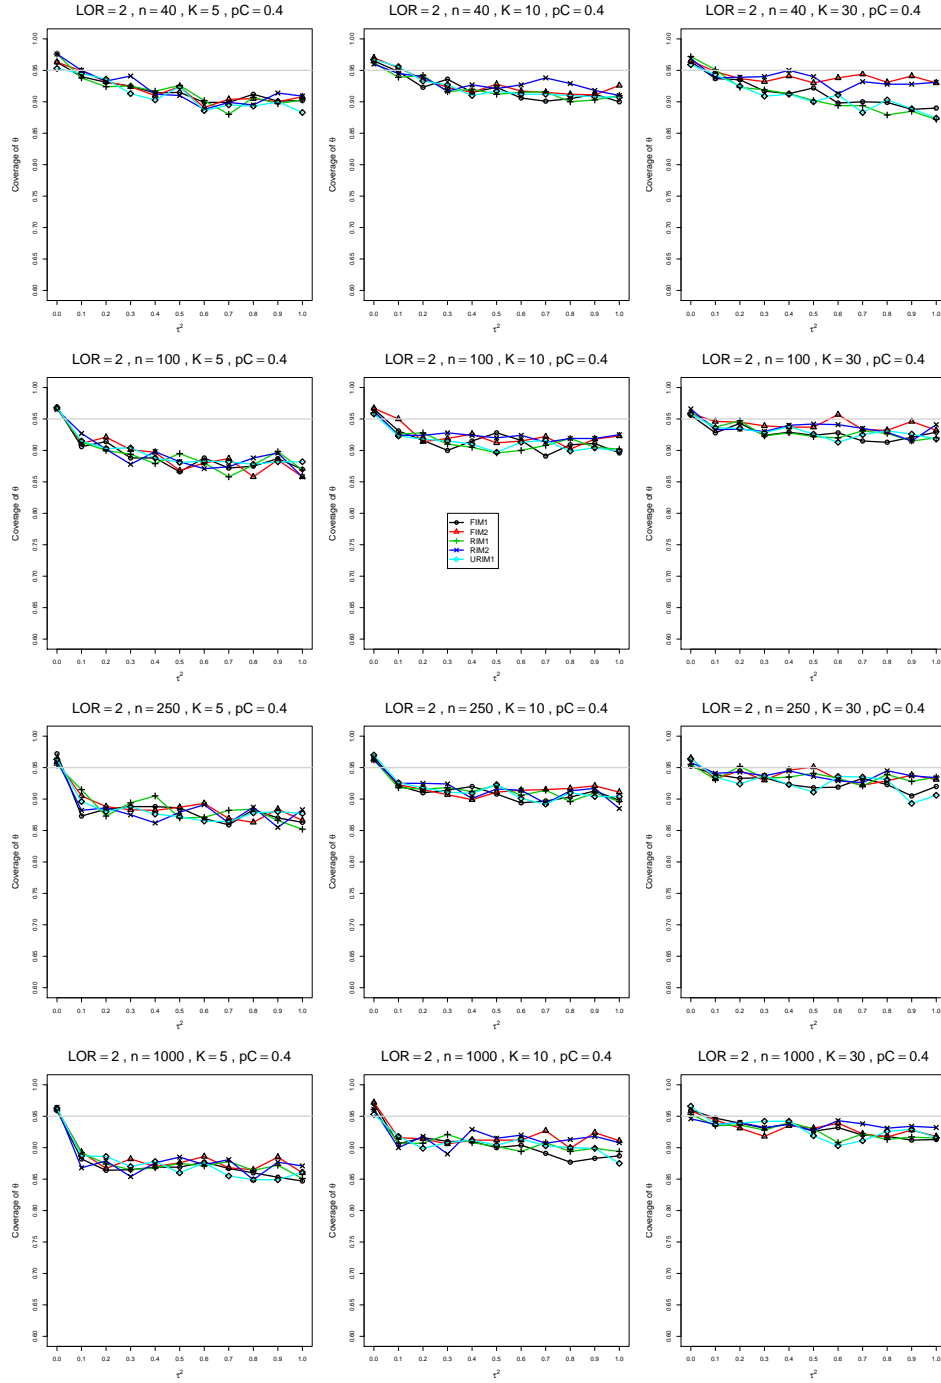

Figure A3.1.10: Coverage of the DerSimonian-Laird confidence interval for  $\theta = 2$ ,  $p_C = 0.4$ ,  $\sigma^2 = 0.1$ , constant sample sizes  $n = 40, 100, 250, 1000$ . The data-generation mechanisms are FIM1 ( $\circ$ ), FIM2 ( $\triangle$ ), RIM1 ( $+$ ), RIM2 ( $\times$ ), and URIM1 ( $\diamond$ ).

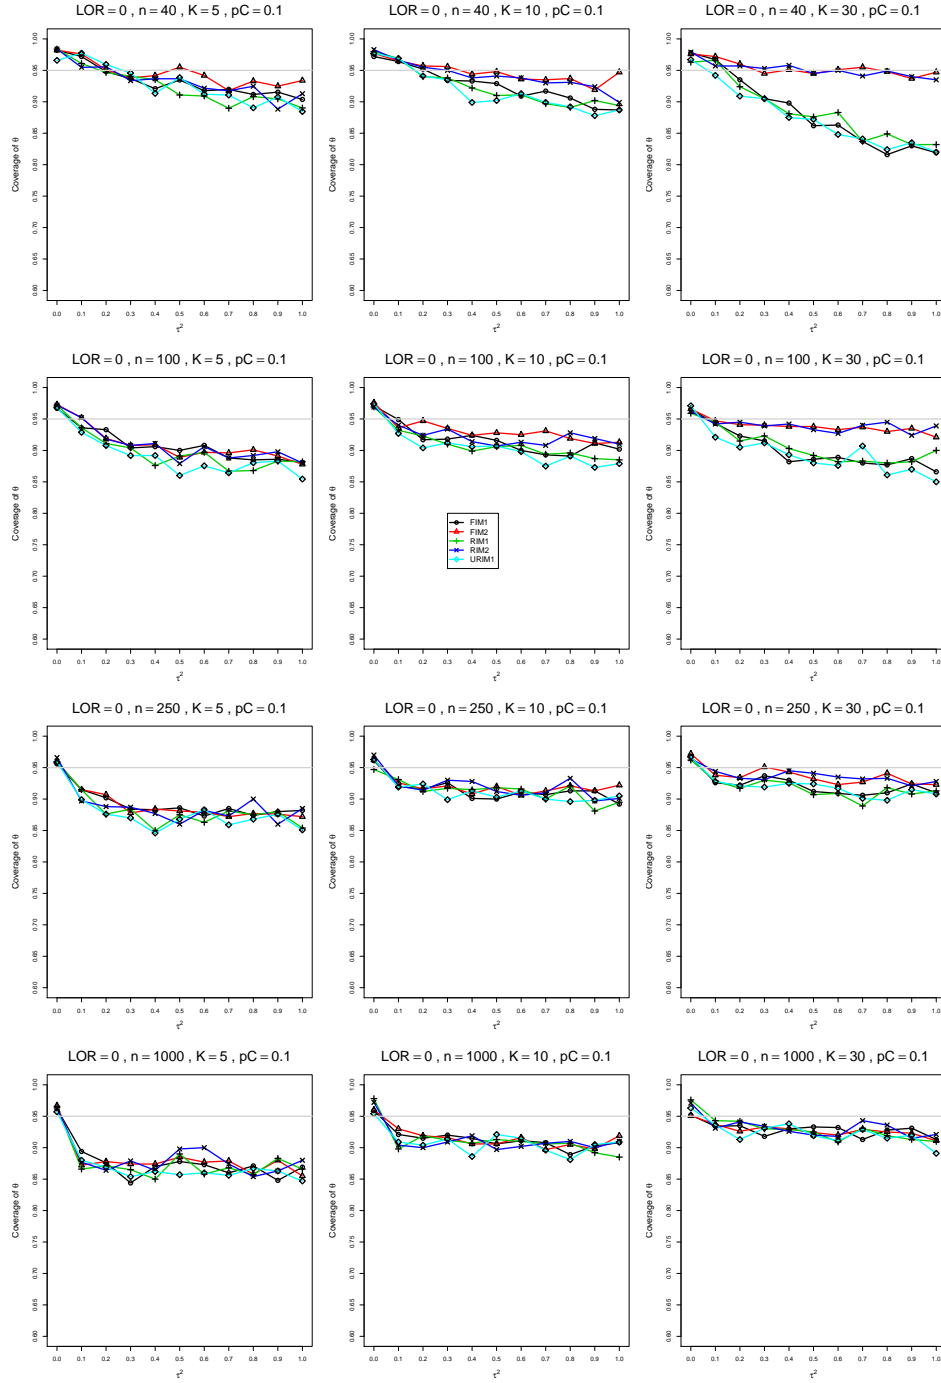

Figure A3.1.11: Coverage of the DerSimonian-Laird confidence interval for  $\theta = 0$ ,  $p_C = 0.1$ ,  $\sigma^2 = 0.4$ , constant sample sizes  $n = 40, 100, 250, 1000$ . The data-generation mechanisms are FIM1 ( $\circ$ ), FIM2 ( $\triangle$ ), RIM1 (+), RIM2 ( $\times$ ), and URIM1 ( $\diamond$ ).

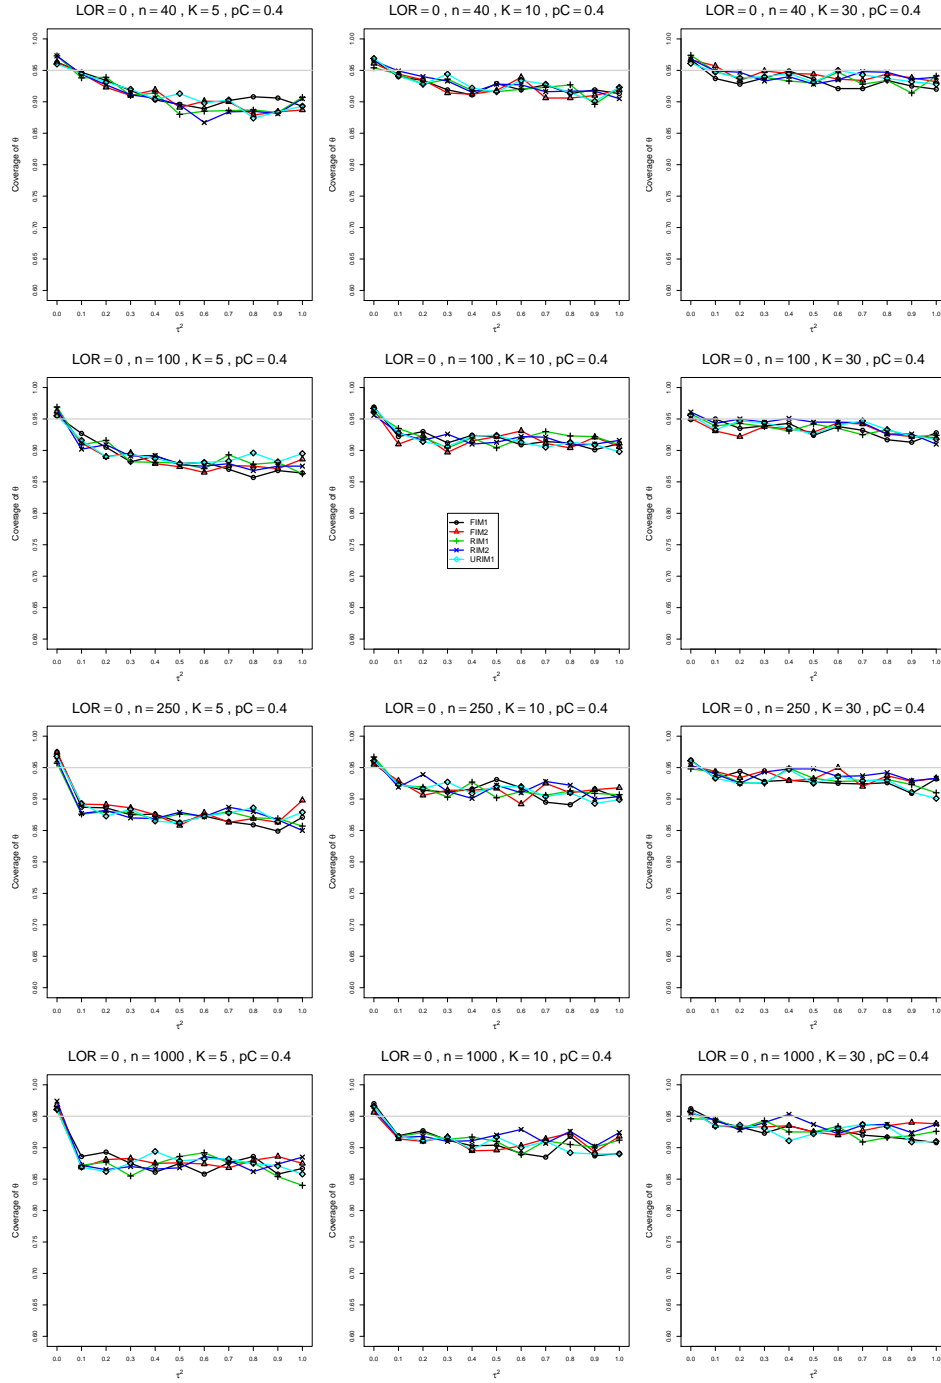

Figure A3.1.12: Coverage of the DerSimonian-Laird confidence interval for  $\theta = 0$ ,  $p_C = 0.4$ ,  $\sigma^2 = 0.4$ , constant sample sizes  $n = 40, 100, 250, 1000$ . The data-generation mechanisms are FIM1 ( $\circ$ ), FIM2 ( $\triangle$ ), RIM1 ( $+$ ), RIM2 ( $\times$ ), and URIM1 ( $\diamond$ ).

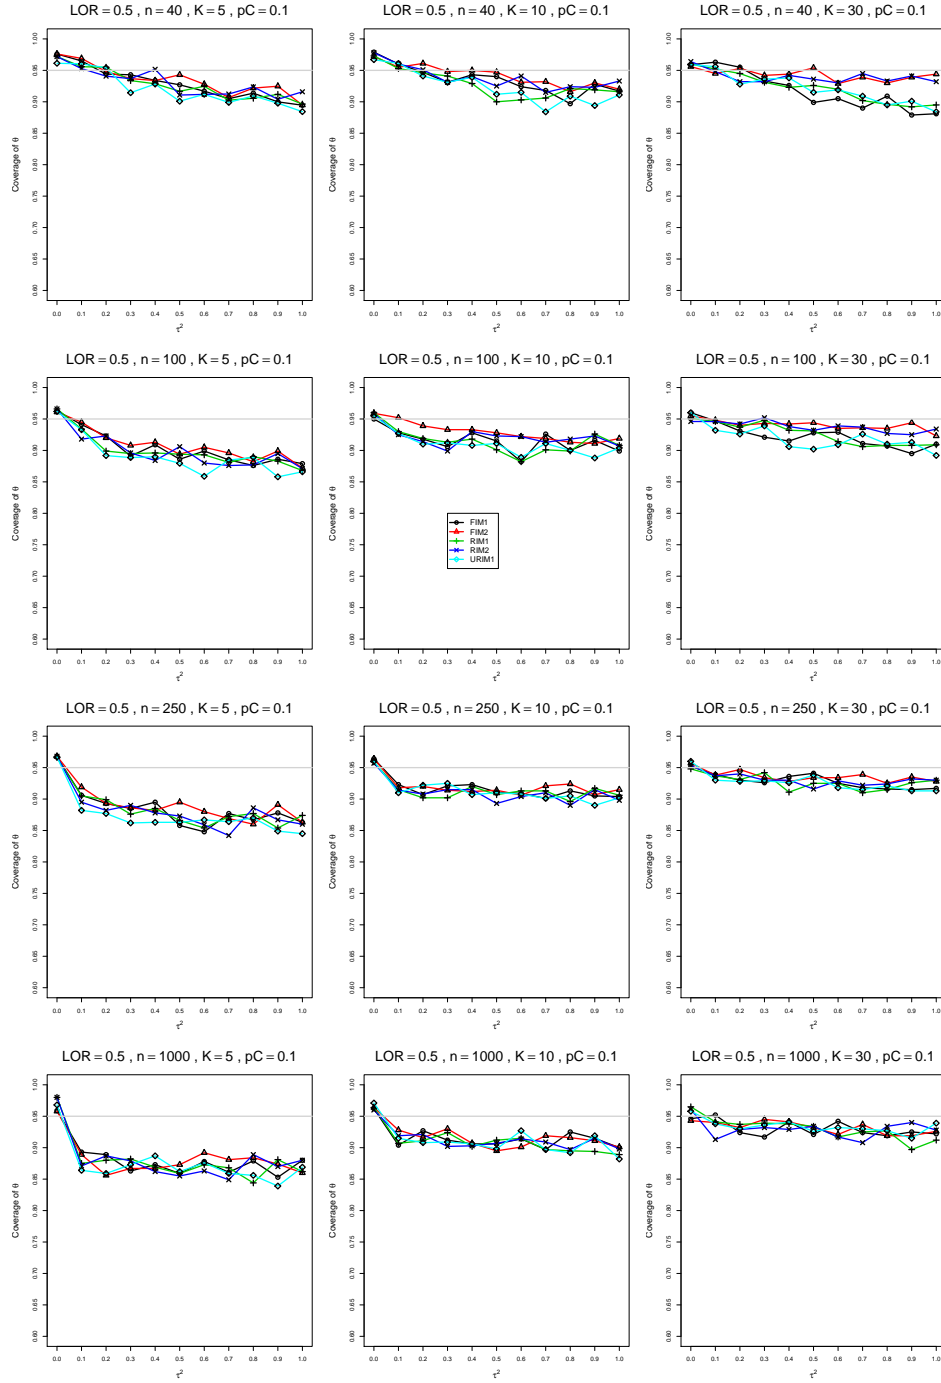

Figure A3.1.13: Coverage of the DerSimonian-Laird confidence interval for  $\theta = 0.5$ ,  $p_C = 0.1$ ,  $\sigma^2 = 0.4$ , constant sample sizes  $n = 40, 100, 250, 1000$ . The data-generation mechanisms are FIM1 ( $\circ$ ), FIM2 ( $\triangle$ ), RIM1 ( $+$ ), RIM2 ( $\times$ ), and URIM1 ( $\diamond$ ).

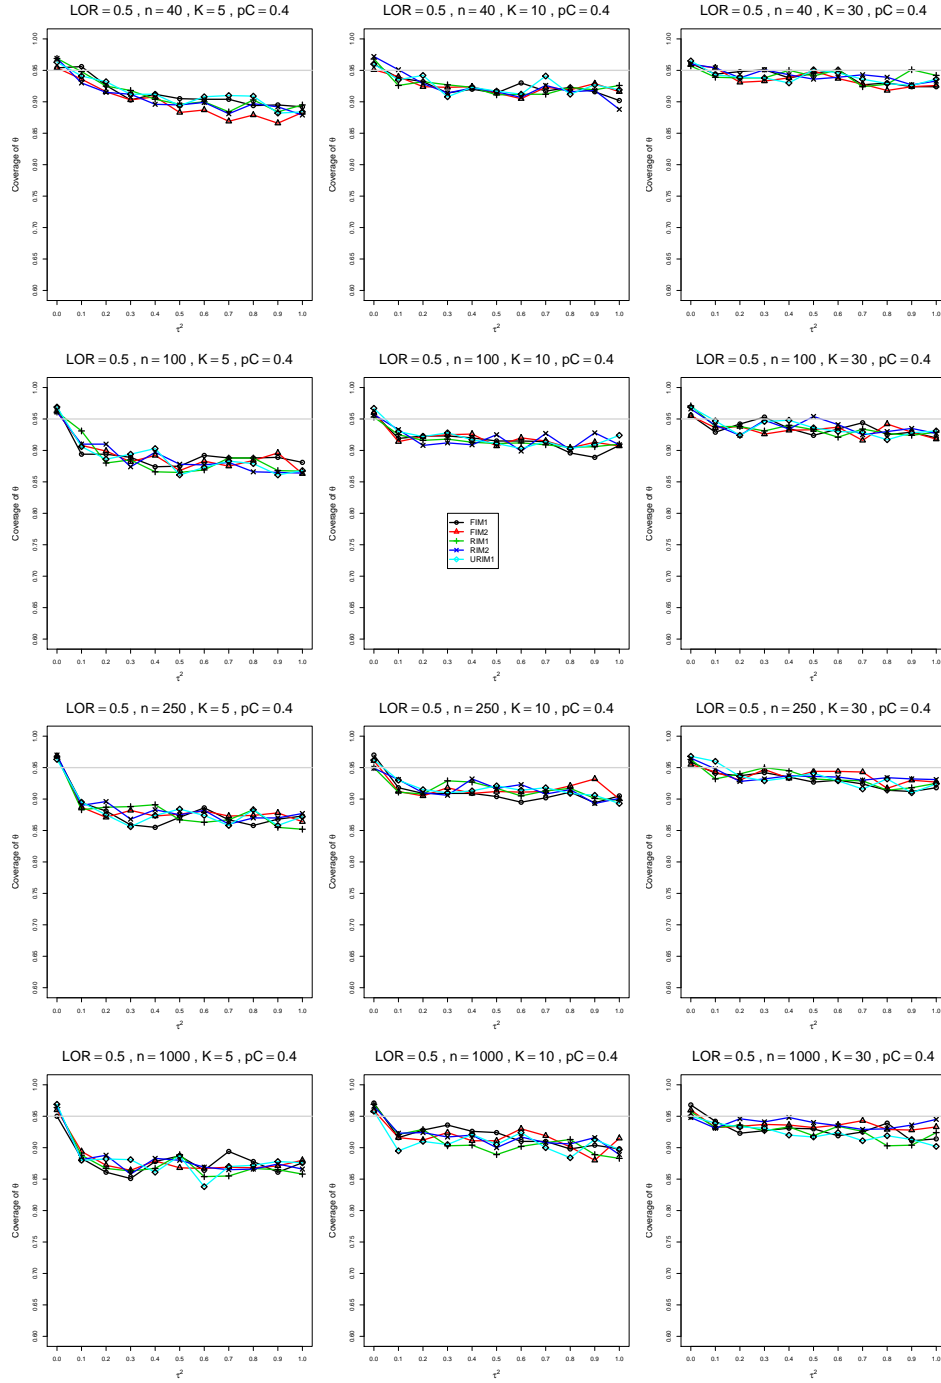

Figure A3.1.14: Coverage of the DerSimonian-Laird confidence interval for  $\theta = 0.5$ ,  $p_C = 0.4$ ,  $\sigma^2 = 0.4$ , constant sample sizes  $n = 40, 100, 250, 1000$ . The data-generation mechanisms are FIM1 (o), FIM2 ( $\triangle$ ), RIM1 (+), RIM2 ( $\times$ ), and URIM1 ( $\diamond$ ).



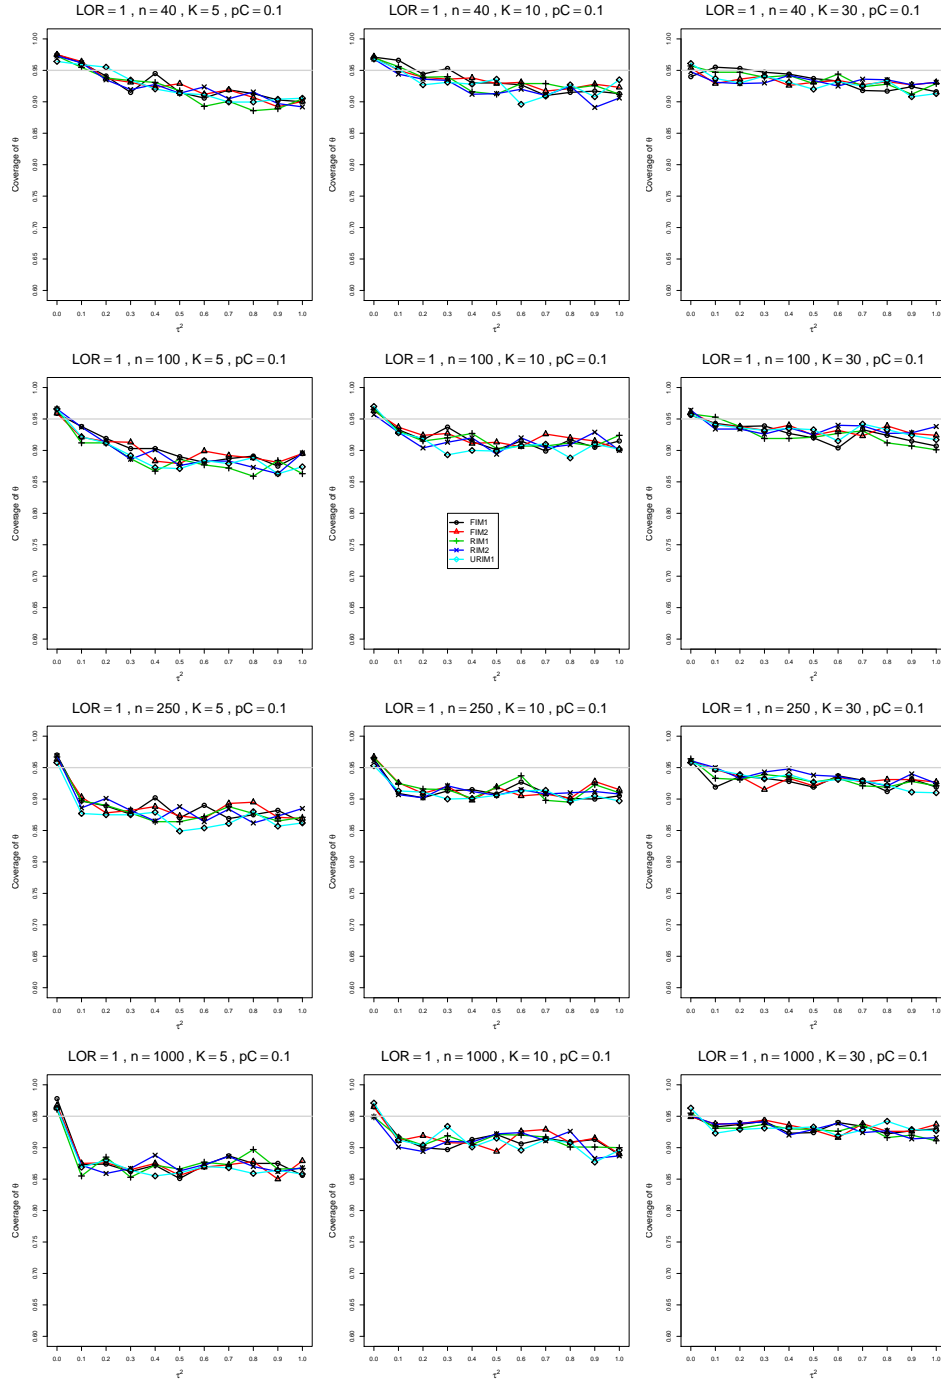

Figure A3.1.15: Coverage of the DerSimonian-Laird confidence interval for  $\theta = 1$ ,  $p_C = 0.1$ ,  $\sigma^2 = 0.4$ , constant sample sizes  $n = 40, 100, 250, 1000$ . The data-generation mechanisms are FIM1 ( $\circ$ ), FIM2 ( $\triangle$ ), RIM1 ( $+$ ), RIM2 ( $\times$ ), and URIM1 ( $\diamond$ ).

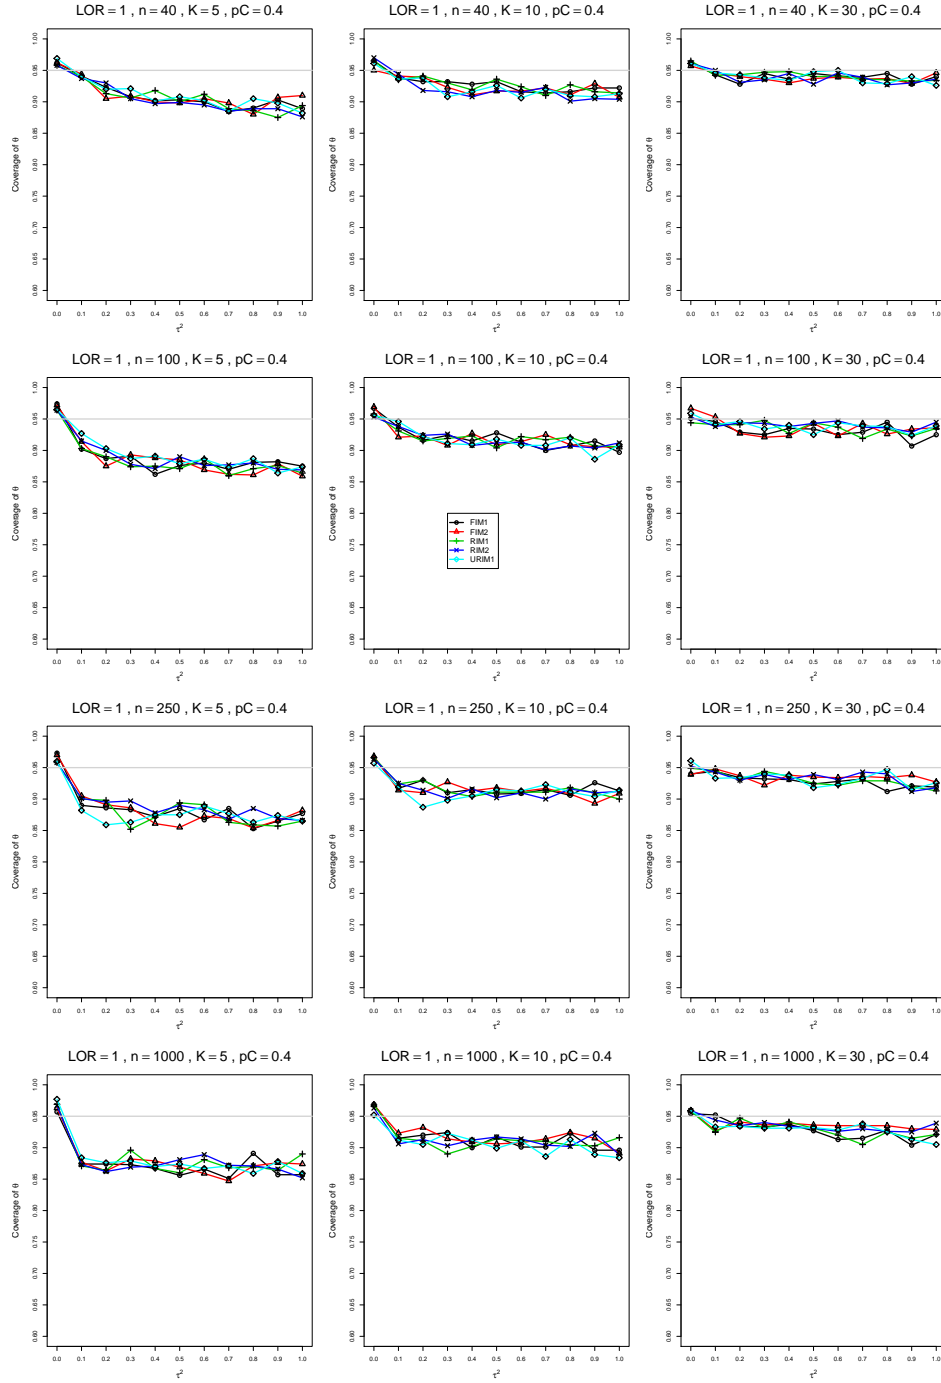

Figure A3.1.16: Coverage of the DerSimonian-Laird confidence interval for  $\theta = 1$ ,  $p_C = 0.4$ ,  $\sigma^2 = 0.4$ , constant sample sizes  $n = 40, 100, 250, 1000$ . The data-generation mechanisms are FIM1 ( $\circ$ ), FIM2 ( $\triangle$ ), RIM1 ( $+$ ), RIM2 ( $\times$ ), and URIM1 ( $\diamond$ ).

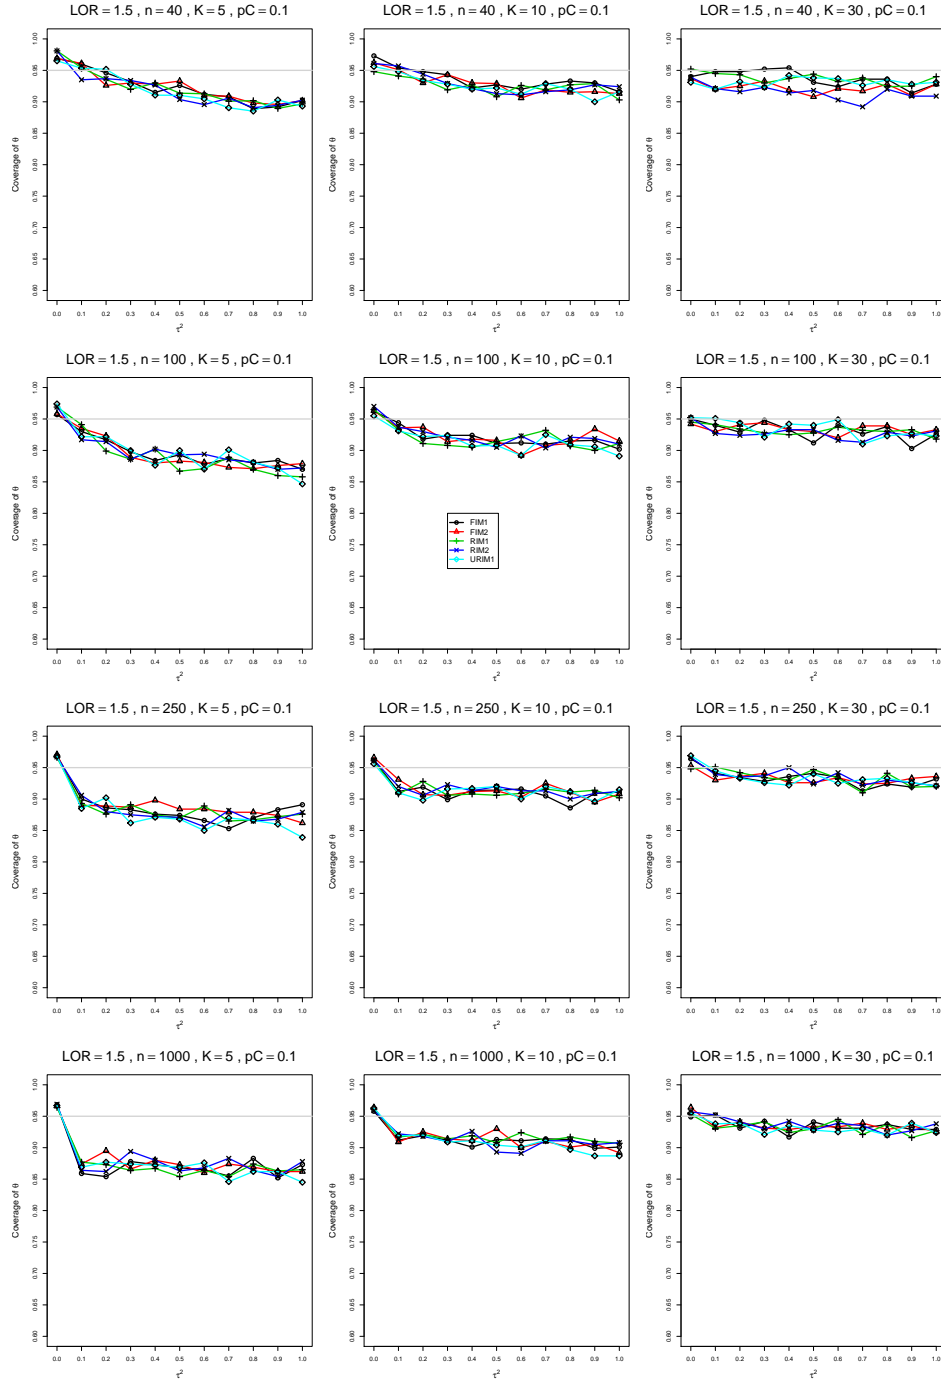

Figure A3.1.17: Coverage of the DerSimonian-Laird confidence interval for  $\theta = 1.5$ ,  $p_C = 0.1$ ,  $\sigma^2 = 0.4$ , constant sample sizes  $n = 40, 100, 250, 1000$ . The data-generation mechanisms are FIM1 ( $\circ$ ), FIM2 ( $\triangle$ ), RIM1 ( $+$ ), RIM2 ( $\times$ ), and URIM1 ( $\diamond$ ).

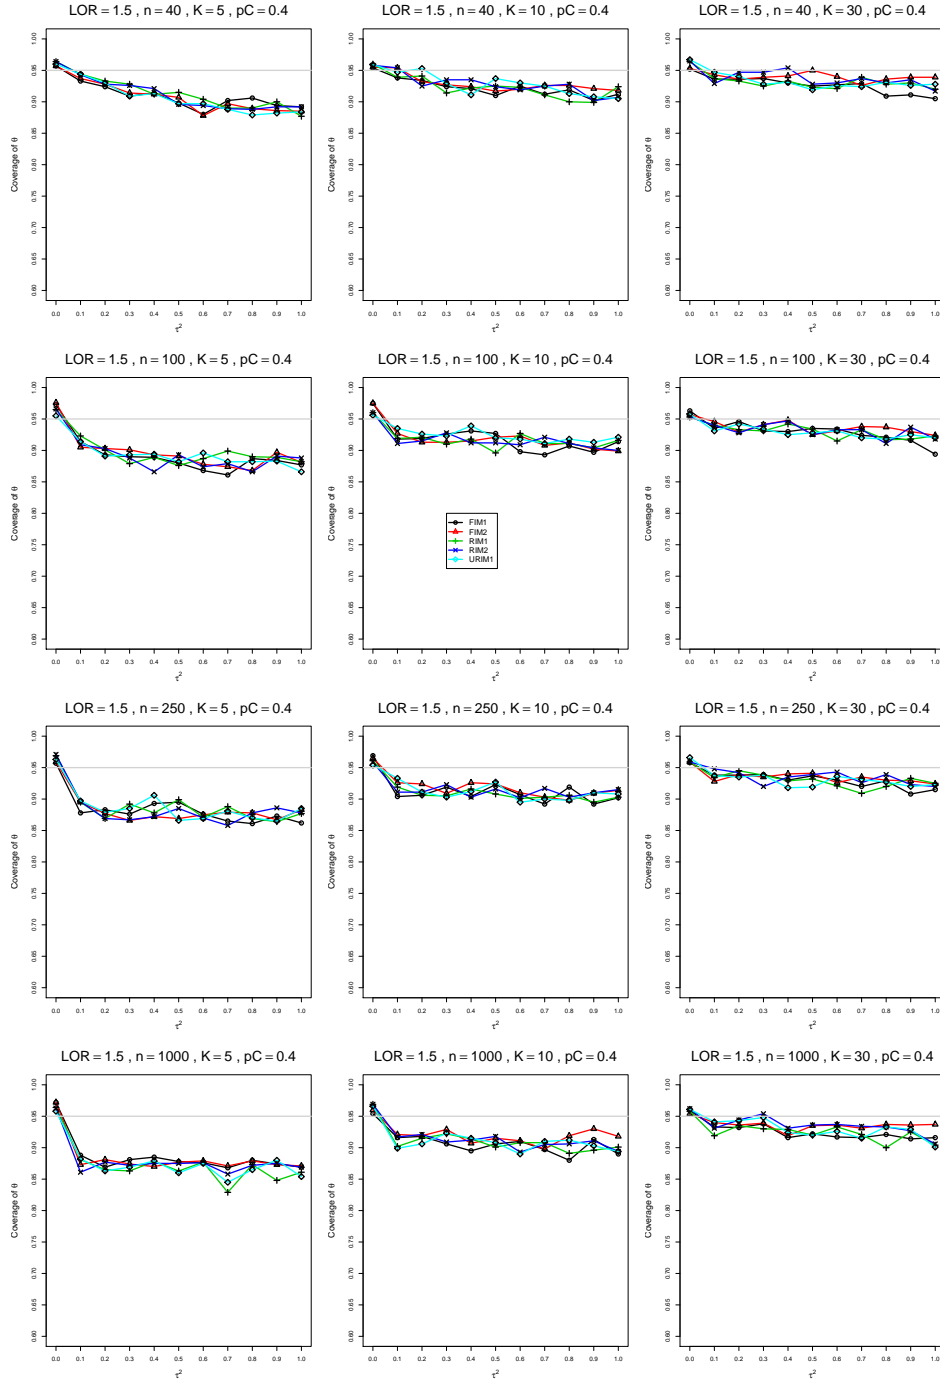

Figure A3.1.18: Coverage of the DerSimonian-Laird confidence interval for  $\theta = 1.5$ ,  $p_C = 0.4$ ,  $\sigma^2 = 0.4$ , constant sample sizes  $n = 40, 100, 250, 1000$ . The data-generation mechanisms are FIM1 ( $\circ$ ), FIM2 ( $\triangle$ ), RIM1 ( $+$ ), RIM2 ( $\times$ ), and URIM1 ( $\diamond$ ).

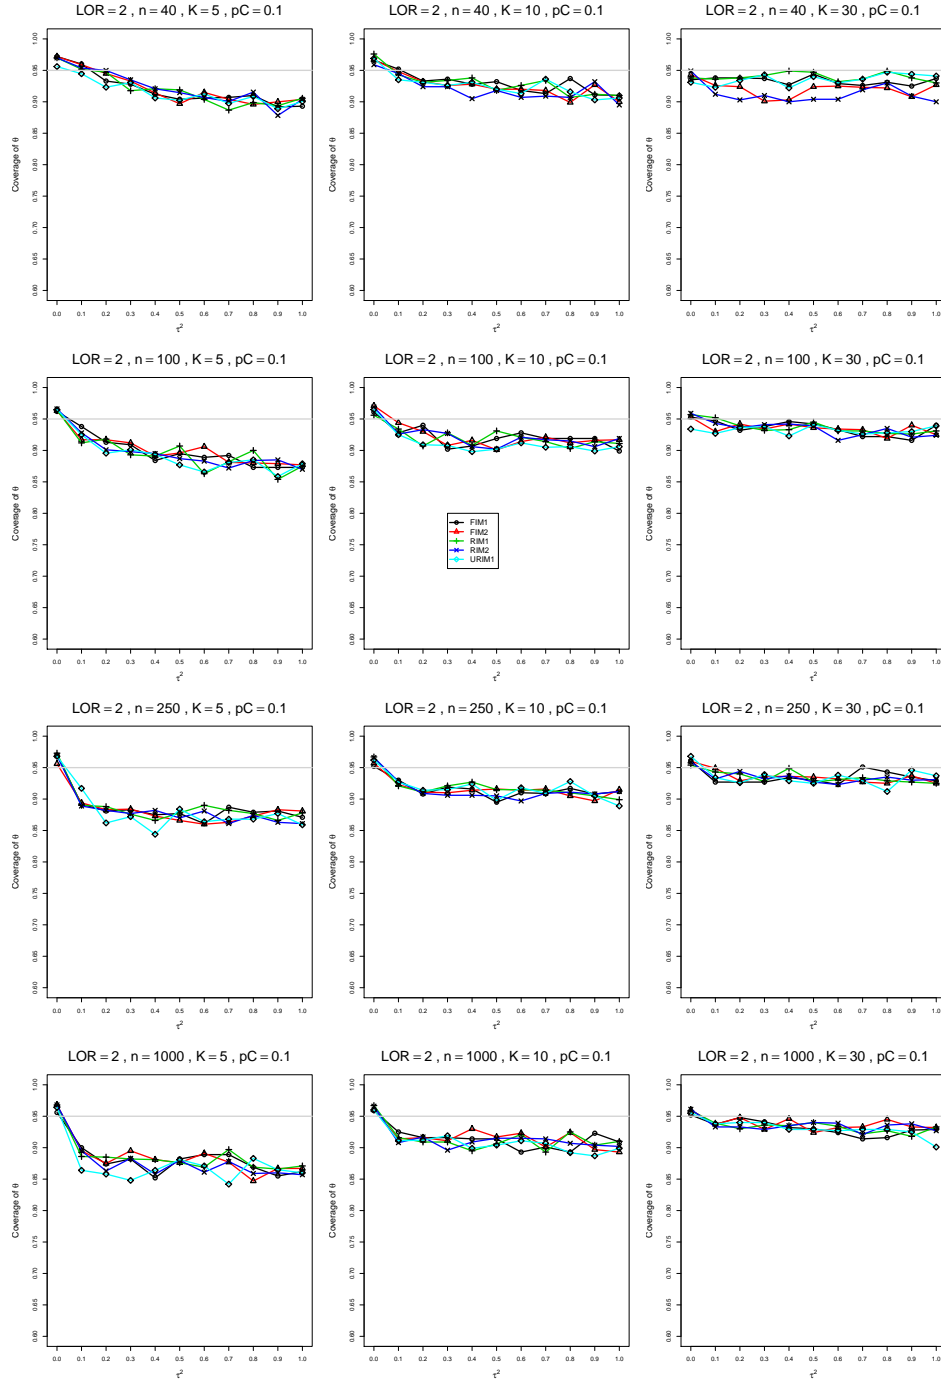

Figure A3.1.19: Coverage of the DerSimonian-Laird confidence interval for  $\theta = 2$ ,  $p_C = 0.1$ ,  $\sigma^2 = 0.4$ , constant sample sizes  $n = 40, 100, 250, 1000$ . The data-generation mechanisms are FIM1 ( $\circ$ ), FIM2 ( $\triangle$ ), RIM1 ( $+$ ), RIM2 ( $\times$ ), and URIM1 ( $\diamond$ ).

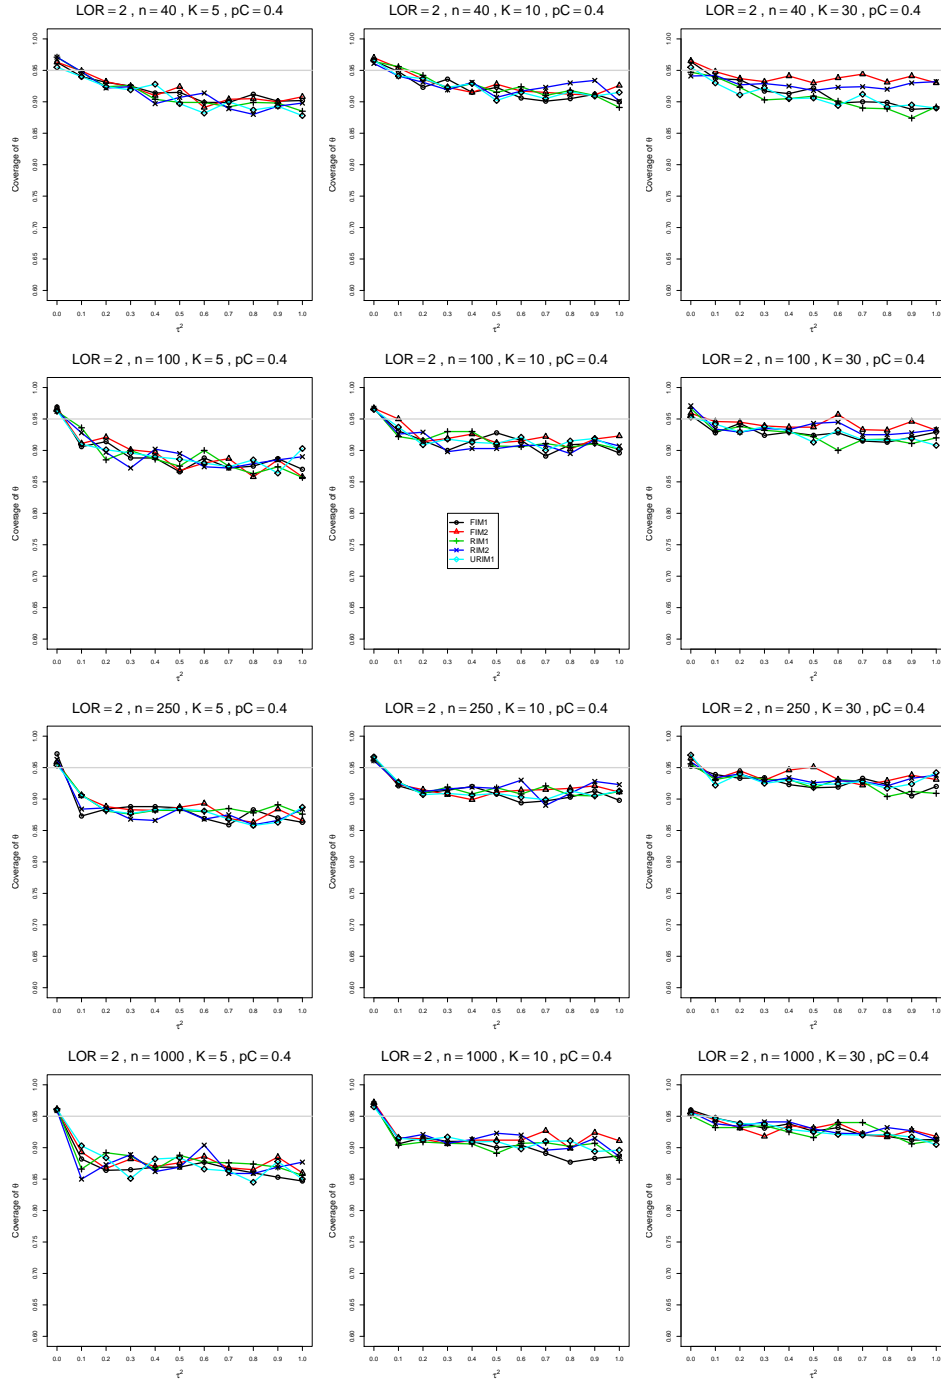

Figure A3.1.20: Coverage of the DerSimonian-Laird confidence interval for  $\theta = 2$ ,  $p_C = 0.4$ ,  $\sigma^2 = 0.4$ , constant sample sizes  $n = 40, 100, 250, 1000$ . The data-generation mechanisms are FIM1 ( $\circ$ ), FIM2 ( $\triangle$ ), RIM1 ( $+$ ), RIM2 ( $\times$ ), and URIM1 ( $\diamond$ ).

### A3.2 Coverage of $\hat{\theta}_{REML}$

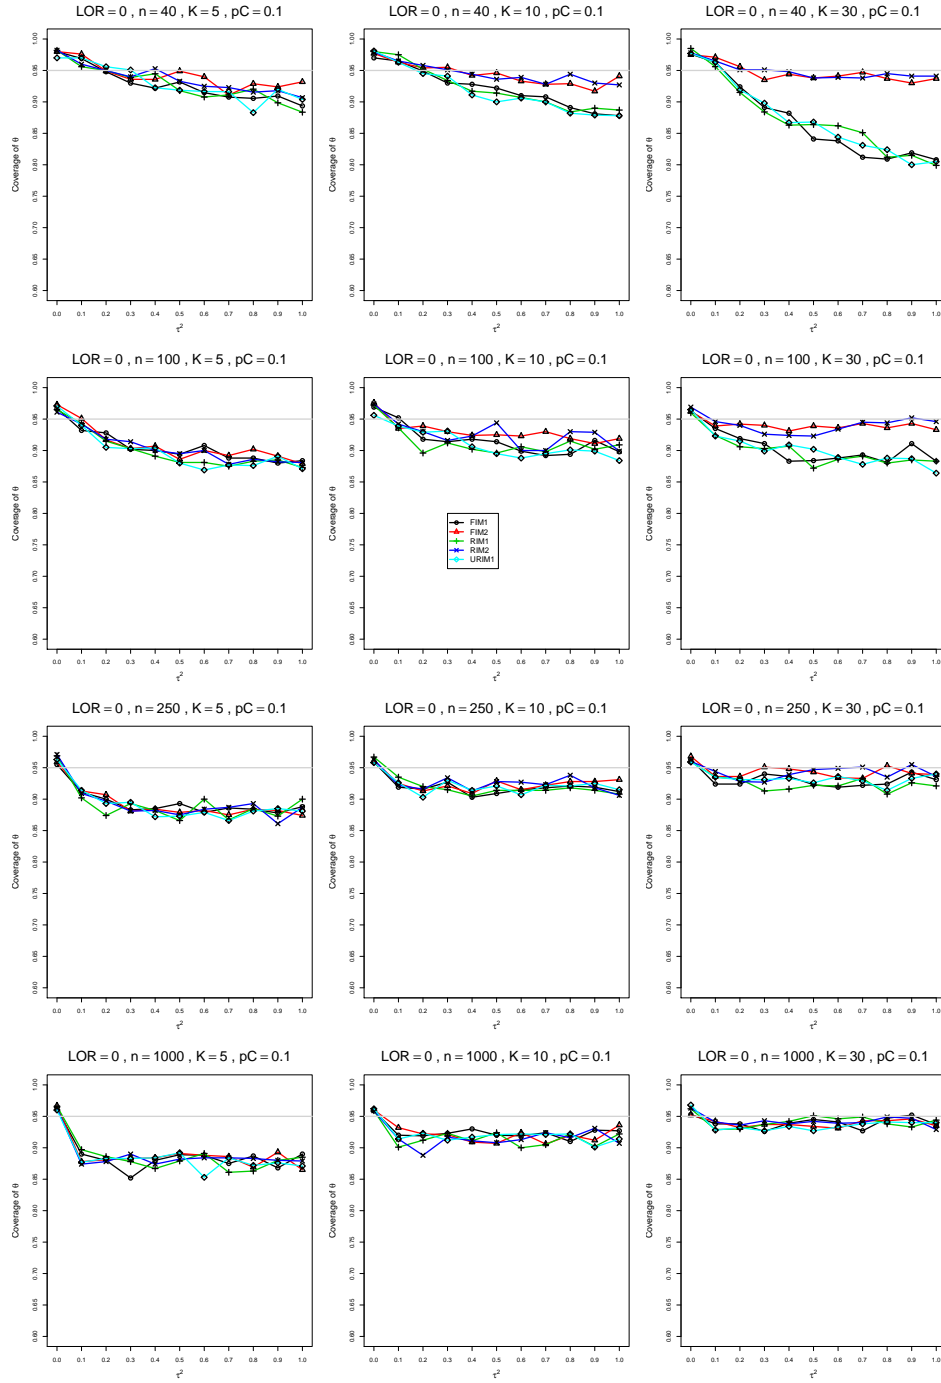

Figure A3.2.1: Coverage of the Restricted Maximum Likelihood confidence interval for  $\theta = 0$ ,  $p_C = 0.1$ ,  $\sigma^2 = 0.1$ , constant sample sizes  $n = 40, 100, 250, 1000$ . The data-generation mechanisms are FIM1 ( $\circ$ ), FIM2 ( $\triangle$ ), RIM1 ( $+$ ), RIM2 ( $\times$ ), and URIM1 ( $\diamond$ ).



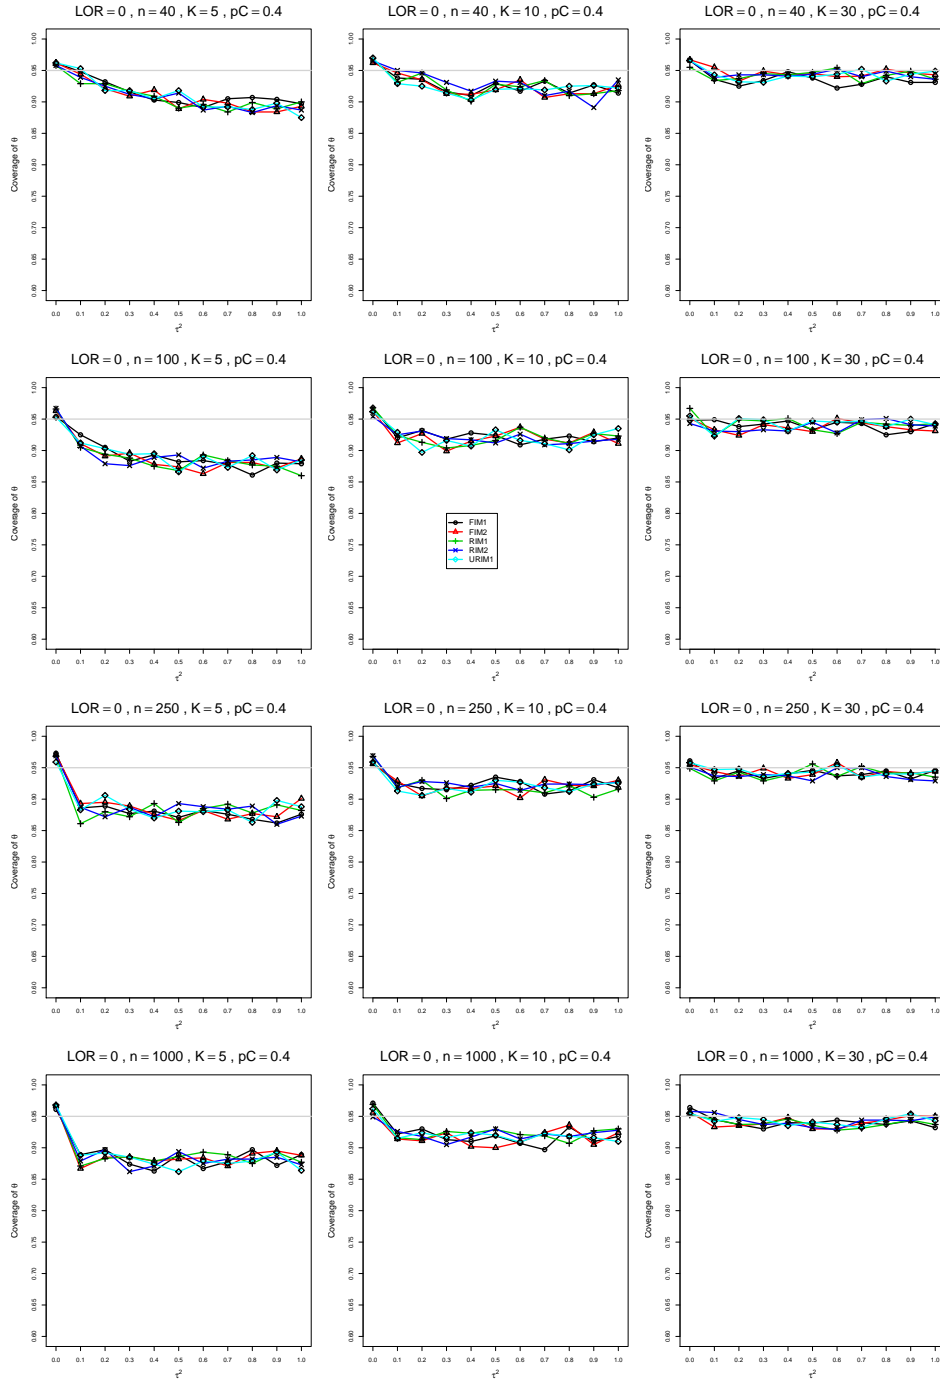

Figure A3.2.2: Coverage of the Restricted Maximum Likelihood confidence interval for  $\theta = 0$ ,  $p_C = 0.4$ ,  $\sigma^2 = 0.1$ , constant sample sizes  $n = 40, 100, 250, 1000$ . The data-generation mechanisms are FIM1 ( $\circ$ ), FIM2 ( $\triangle$ ), RIM1 ( $+$ ), RIM2 ( $\times$ ), and URIM1 ( $\diamond$ ).

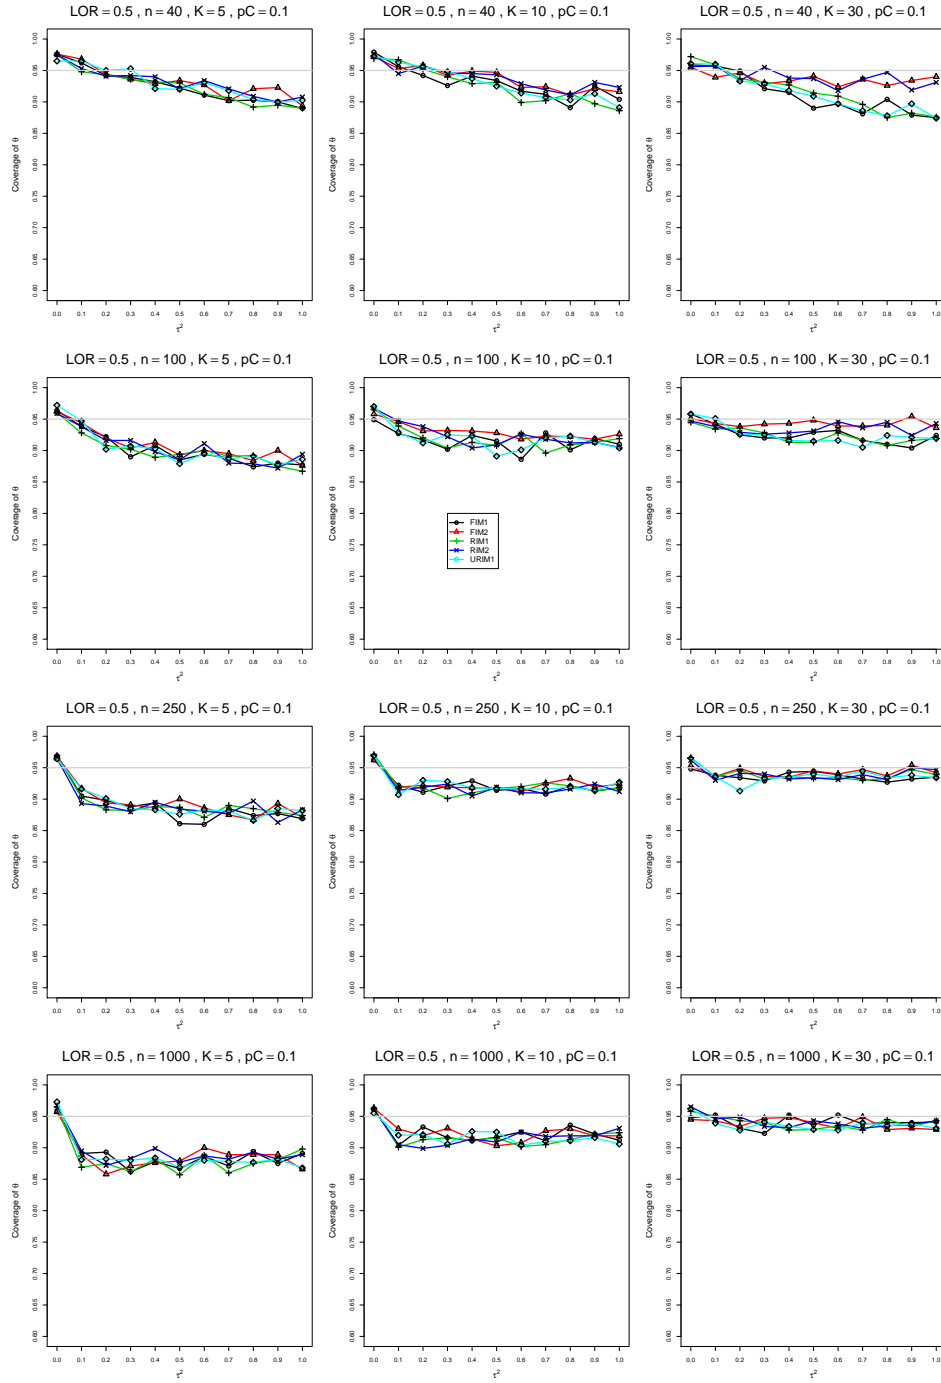

Figure A3.2.3: Coverage of the Restricted Maximum Likelihood confidence interval for  $\theta = 0.5$ ,  $p_C = 0.1$ ,  $\sigma^2 = 0.1$ , constant sample sizes  $n = 40, 100, 250, 1000$ . The data-generation mechanisms are FIM1 (o), FIM2 ( $\triangle$ ), RIM1 (+), RIM2 ( $\times$ ), and URIM1 ( $\diamond$ ).

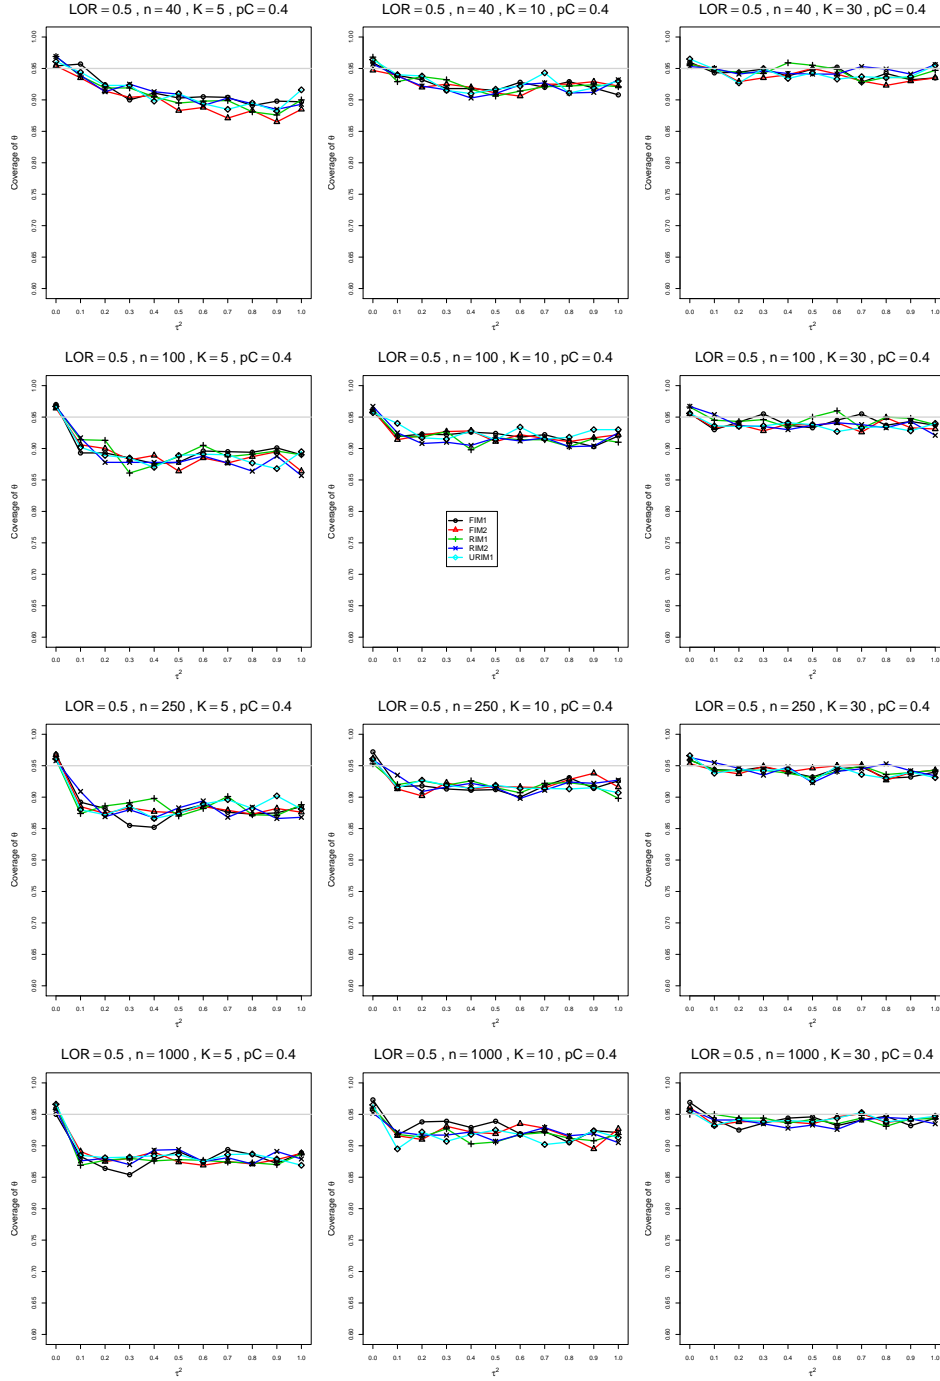

Figure A3.2.4: Coverage of the Restricted Maximum Likelihood confidence interval for  $\theta = 0.5$ ,  $p_C = 0.4$ ,  $\sigma^2 = 0.1$ , constant sample sizes  $n = 40, 100, 250, 1000$ . The data-generation mechanisms are FIM1 ( $\circ$ ), FIM2 ( $\triangle$ ), RIM1 ( $+$ ), RIM2 ( $\times$ ), and URIM1 ( $\diamond$ ).

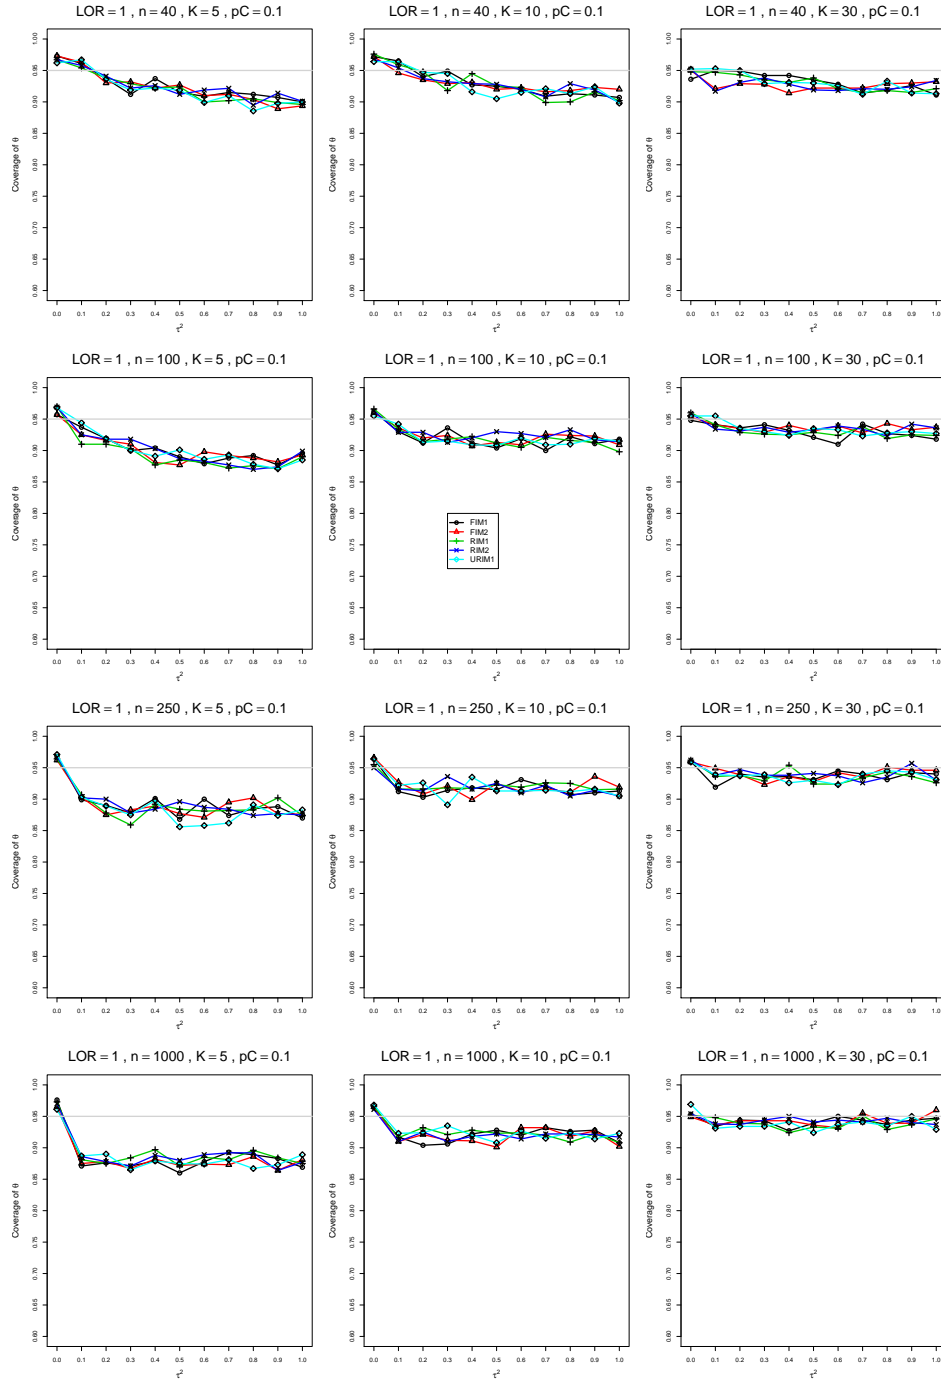

Figure A3.2.5: Coverage of the Restricted Maximum Likelihood confidence interval for  $\theta = 1$ ,  $p_C = 0.1$ ,  $\sigma^2 = 0.1$ , constant sample sizes  $n = 40, 100, 250, 1000$ . The data-generation mechanisms are FIM1 ( $\circ$ ), FIM2 ( $\triangle$ ), RIM1 ( $+$ ), RIM2 ( $\times$ ), and URIM1 ( $\diamond$ ).

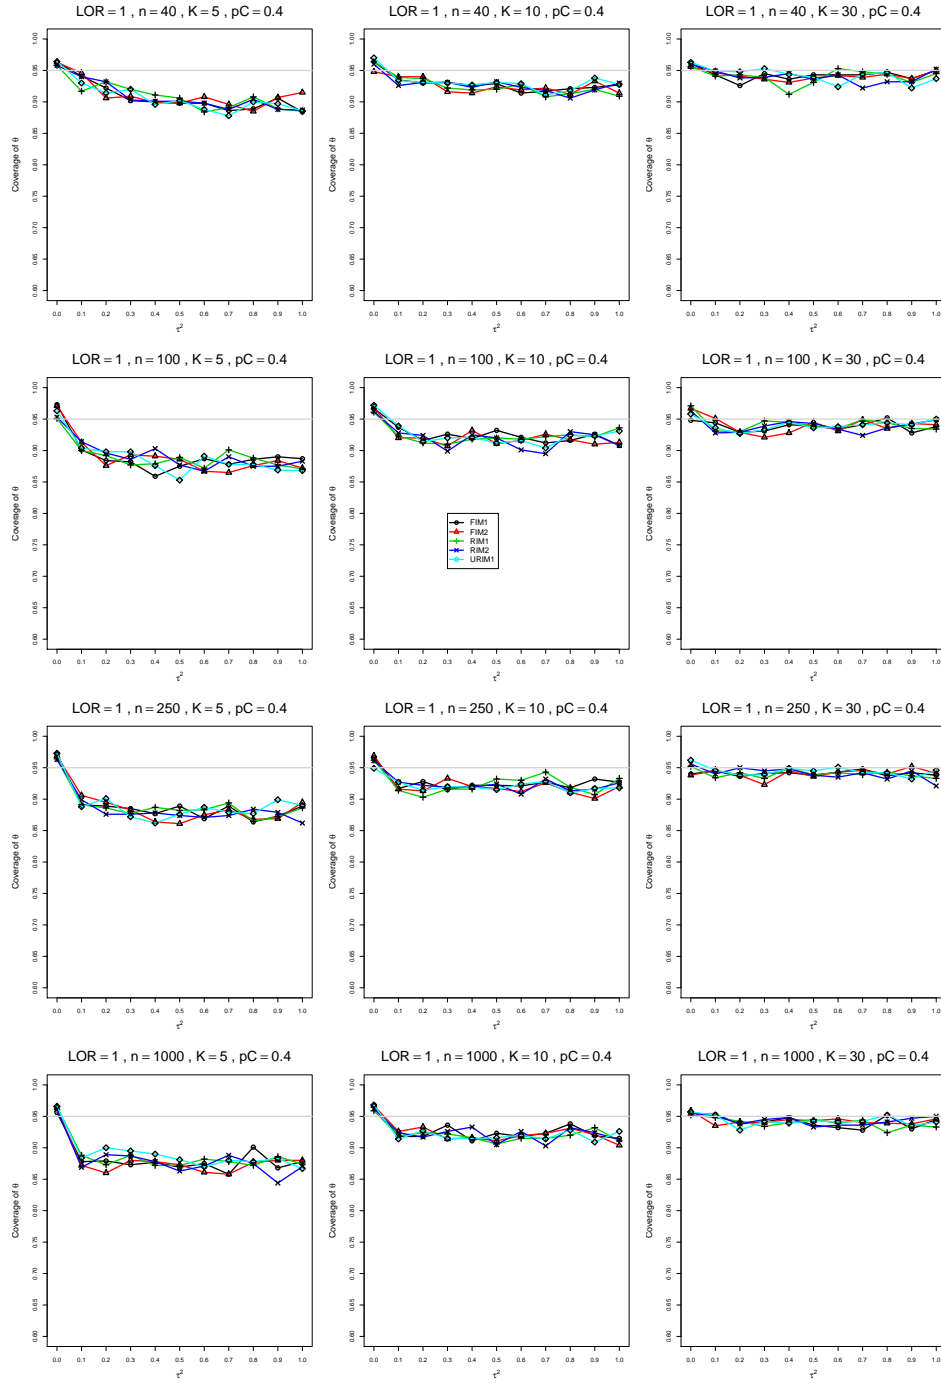

Figure A3.2.6: Coverage of the Restricted Maximum Likelihood confidence interval for  $\theta = 1$ ,  $p_C = 0.4$ ,  $\sigma^2 = 0.1$ , constant sample sizes  $n = 40, 100, 250, 1000$ . The data-generation mechanisms are FIM1 ( $\circ$ ), FIM2 ( $\triangle$ ), RIM1 ( $+$ ), RIM2 ( $\times$ ), and URIM1 ( $\diamond$ ).

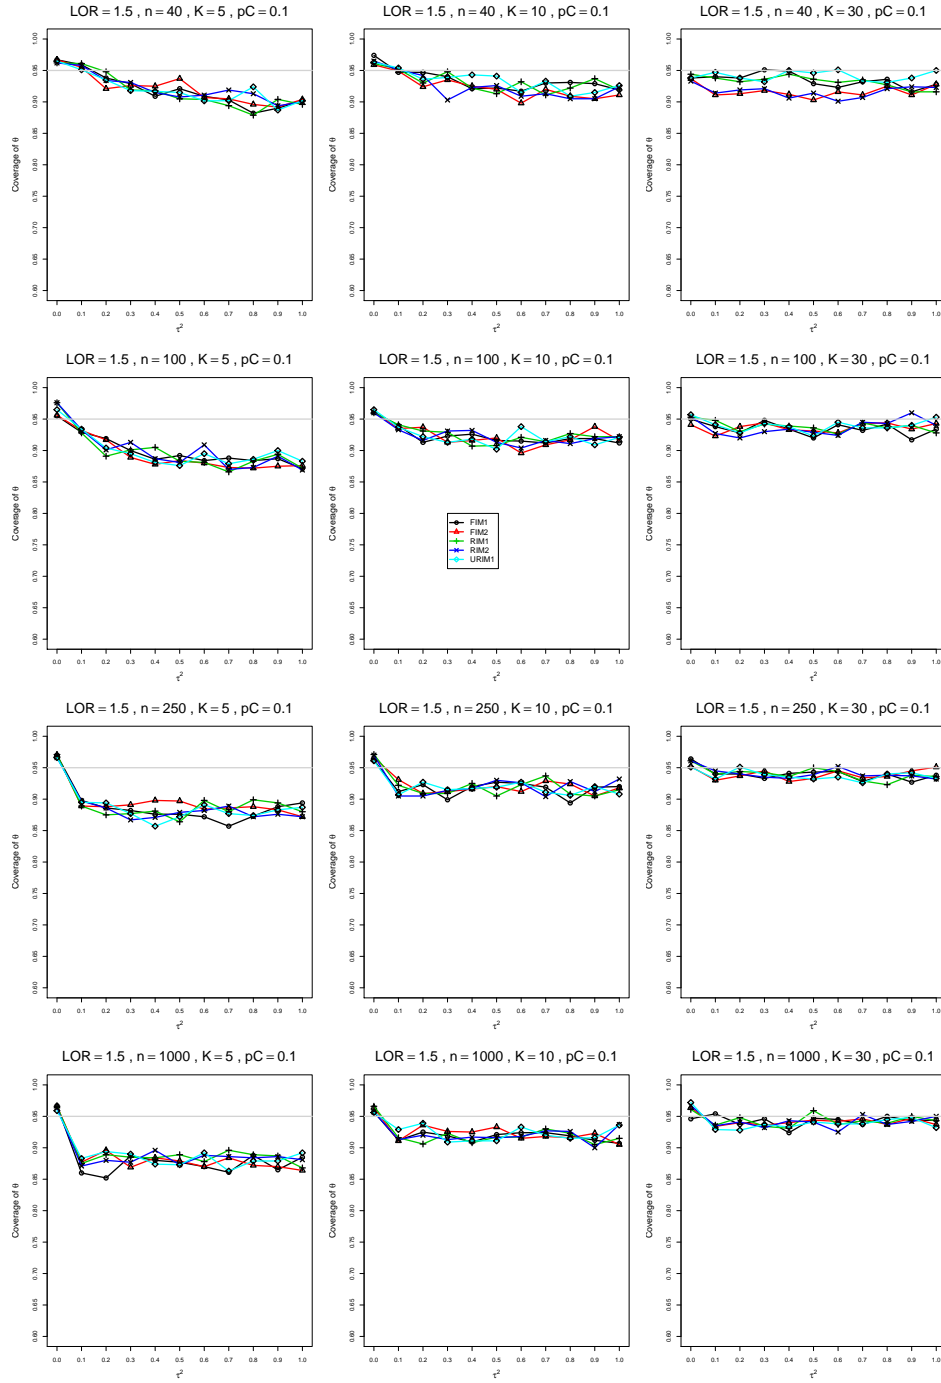

Figure A3.2.7: Coverage of the Restricted Maximum Likelihood confidence interval for  $\theta = 1.5$ ,  $p_C = 0.1$ ,  $\sigma^2 = 0.1$ , constant sample sizes  $n = 40, 100, 250, 1000$ . The data-generation mechanisms are FIM1 ( $\circ$ ), FIM2 ( $\triangle$ ), RIM1 ( $+$ ), RIM2 ( $\times$ ), and URIM1 ( $\diamond$ ).

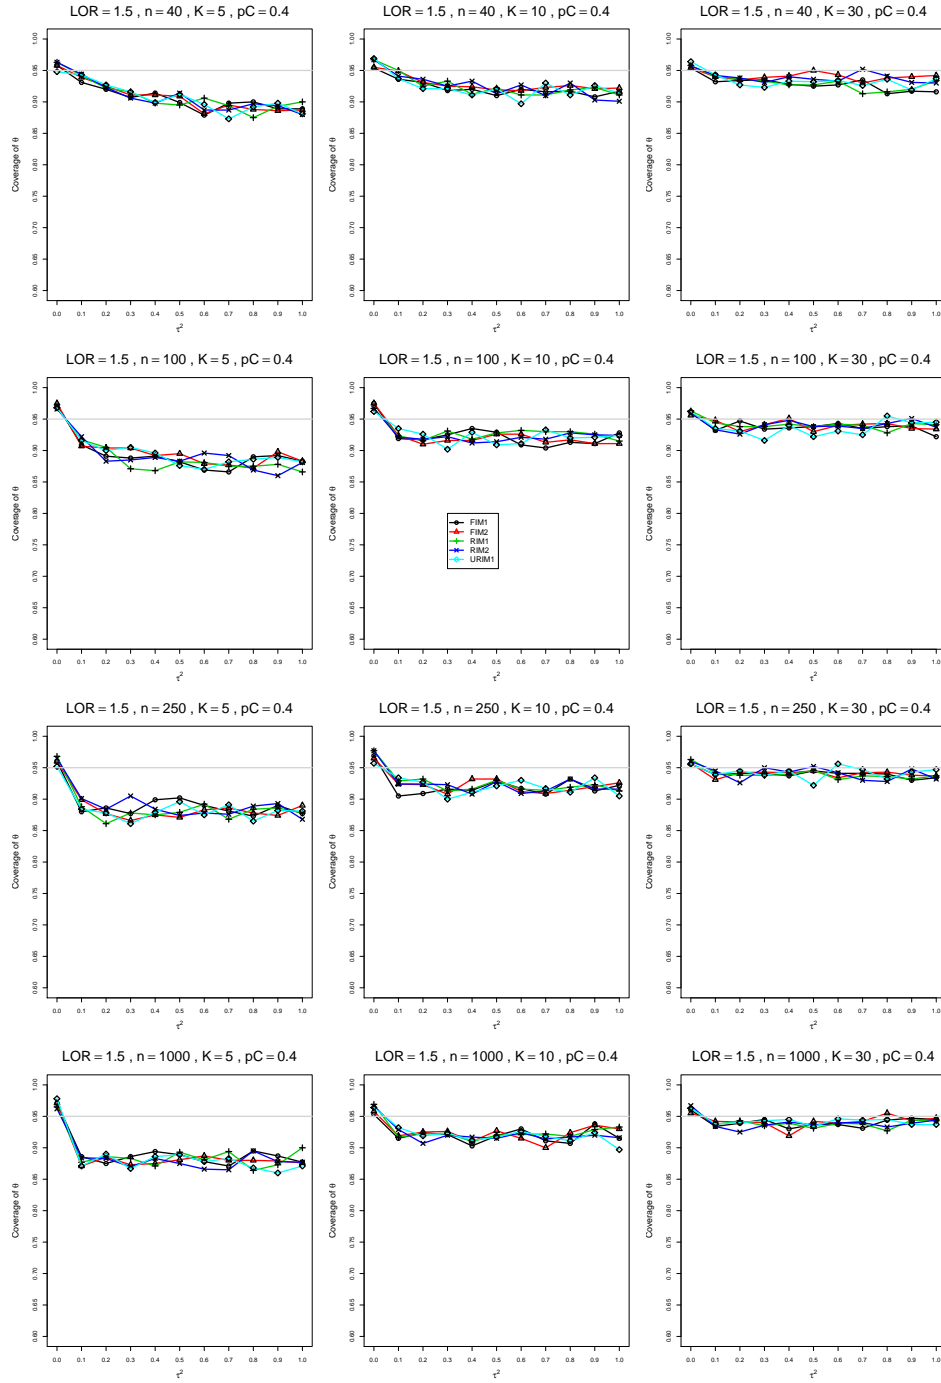

Figure A3.2.8: Coverage of the Restricted Maximum Likelihood confidence interval for  $\theta = 1.5$ ,  $p_C = 0.4$ ,  $\sigma^2 = 0.1$ , constant sample sizes  $n = 40, 100, 250, 1000$ . The data-generation mechanisms are FIM1 ( $\circ$ ), FIM2 ( $\triangle$ ), RIM1 ( $+$ ), RIM2 ( $\times$ ), and URIM1 ( $\diamond$ ).

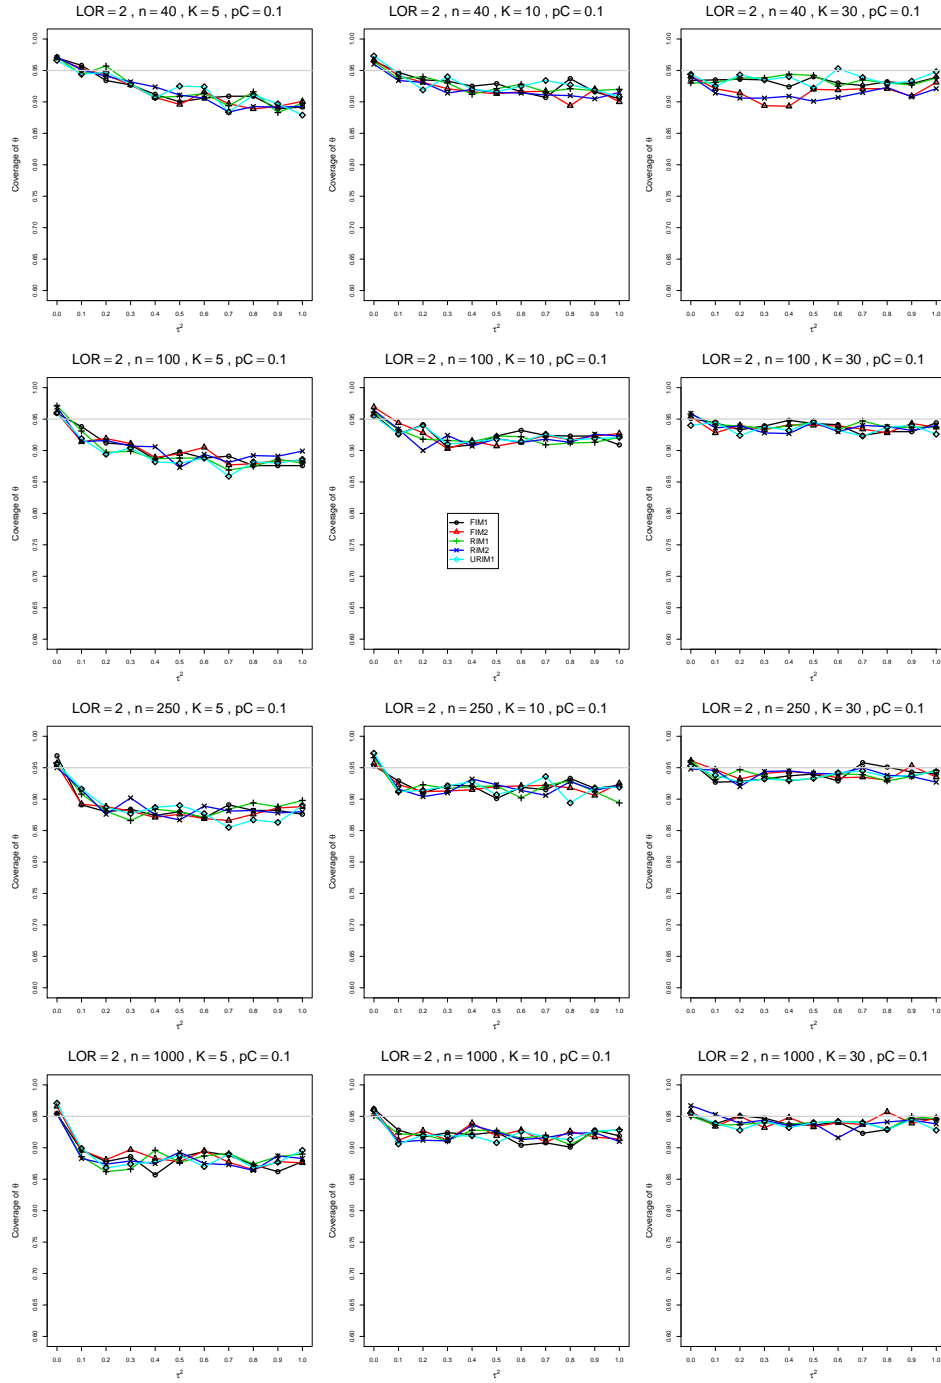

Figure A3.2.9: Coverage of the Restricted Maximum Likelihood confidence interval for  $\theta = 2$ ,  $p_C = 0.1$ ,  $\sigma^2 = 0.1$ , constant sample sizes  $n = 40, 100, 250, 1000$ . The data-generation mechanisms are FIM1 ( $\circ$ ), FIM2 ( $\triangle$ ), RIM1 (+), RIM2 ( $\times$ ), and URIM1 ( $\diamond$ ).



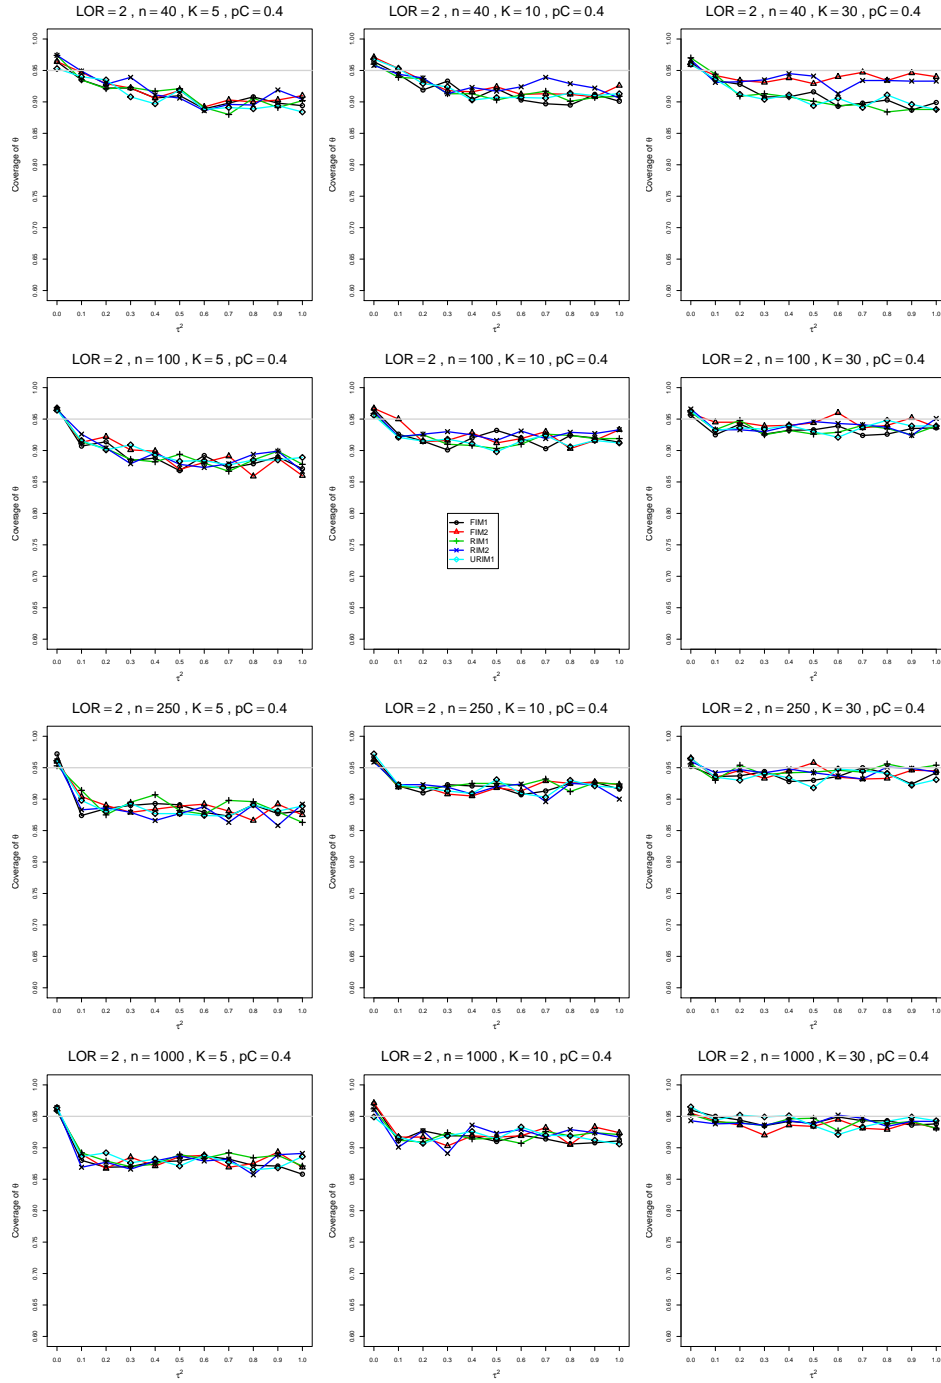

Figure A3.2.10: Coverage of the Restricted Maximum Likelihood confidence interval for  $\theta = 2$ ,  $p_C = 0.4$ ,  $\sigma^2 = 0.1$ , constant sample sizes  $n = 40, 100, 250, 1000$ . The data-generation mechanisms are FIM1 ( $\circ$ ), FIM2 ( $\triangle$ ), RIM1 (+), RIM2 ( $\times$ ), and URIM1 ( $\diamond$ ).

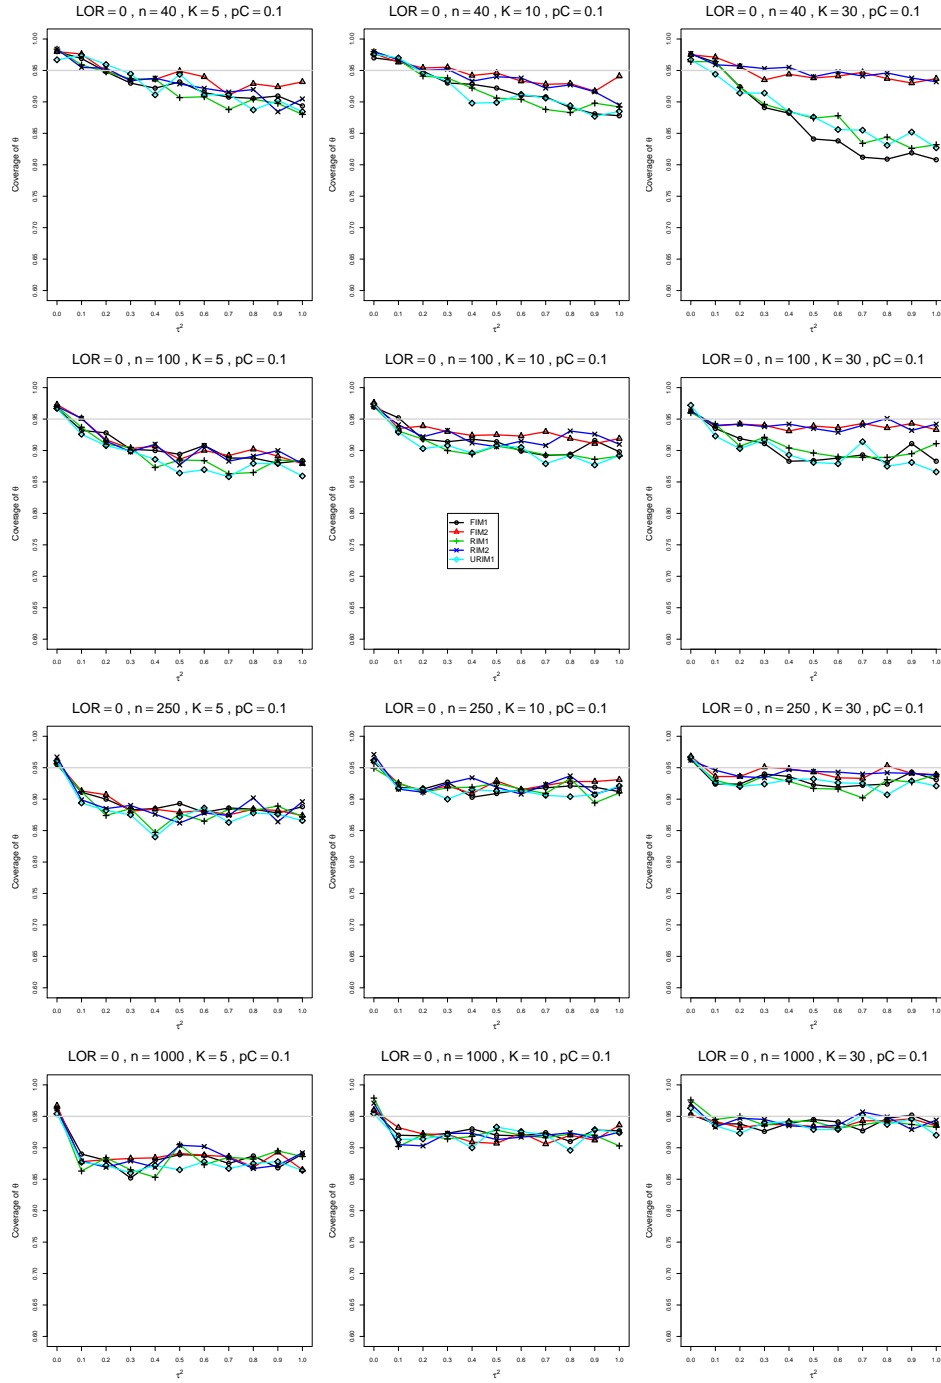

Figure A3.2.11: Coverage of the Restricted Maximum Likelihood confidence interval for  $\theta = 0$ ,  $p_C = 0.1$ ,  $\sigma^2 = 0.4$ , constant sample sizes  $n = 40, 100, 250, 1000$ . The data-generation mechanisms are FIM1 ( $\circ$ ), FIM2 ( $\triangle$ ), RIM1 (+), RIM2 ( $\times$ ), and URIM1 ( $\diamond$ ).

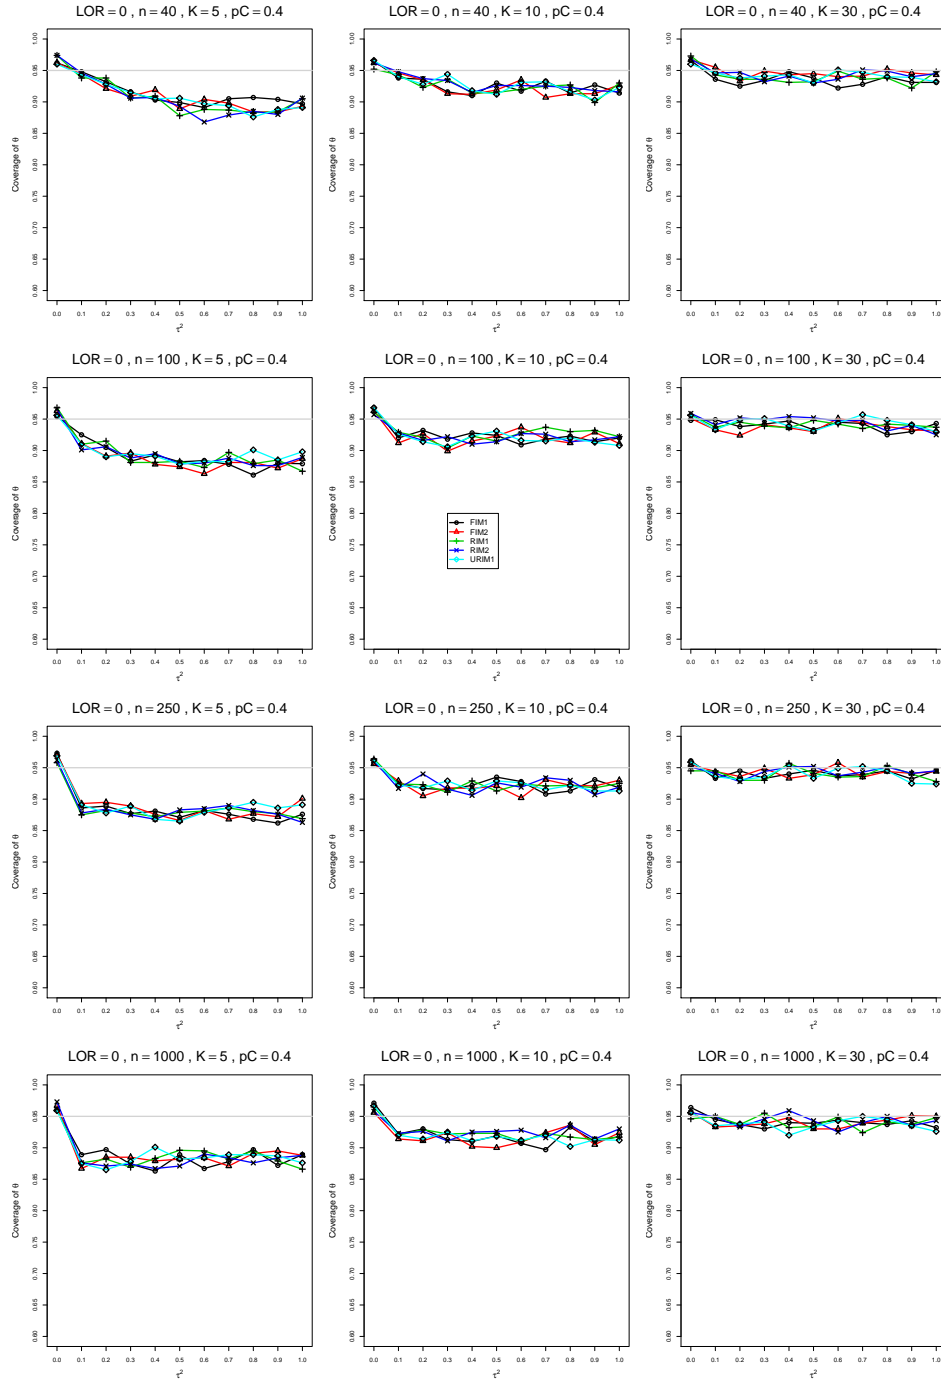

Figure A3.2.12: Coverage of the Restricted Maximum Likelihood confidence interval for  $\theta = 0$ ,  $p_C = 0.4$ ,  $\sigma^2 = 0.4$ , constant sample sizes  $n = 40, 100, 250, 1000$ . The data-generation mechanisms are FIM1 ( $\circ$ ), FIM2 ( $\triangle$ ), RIM1 ( $+$ ), RIM2 ( $\times$ ), and URIM1 ( $\diamond$ ).

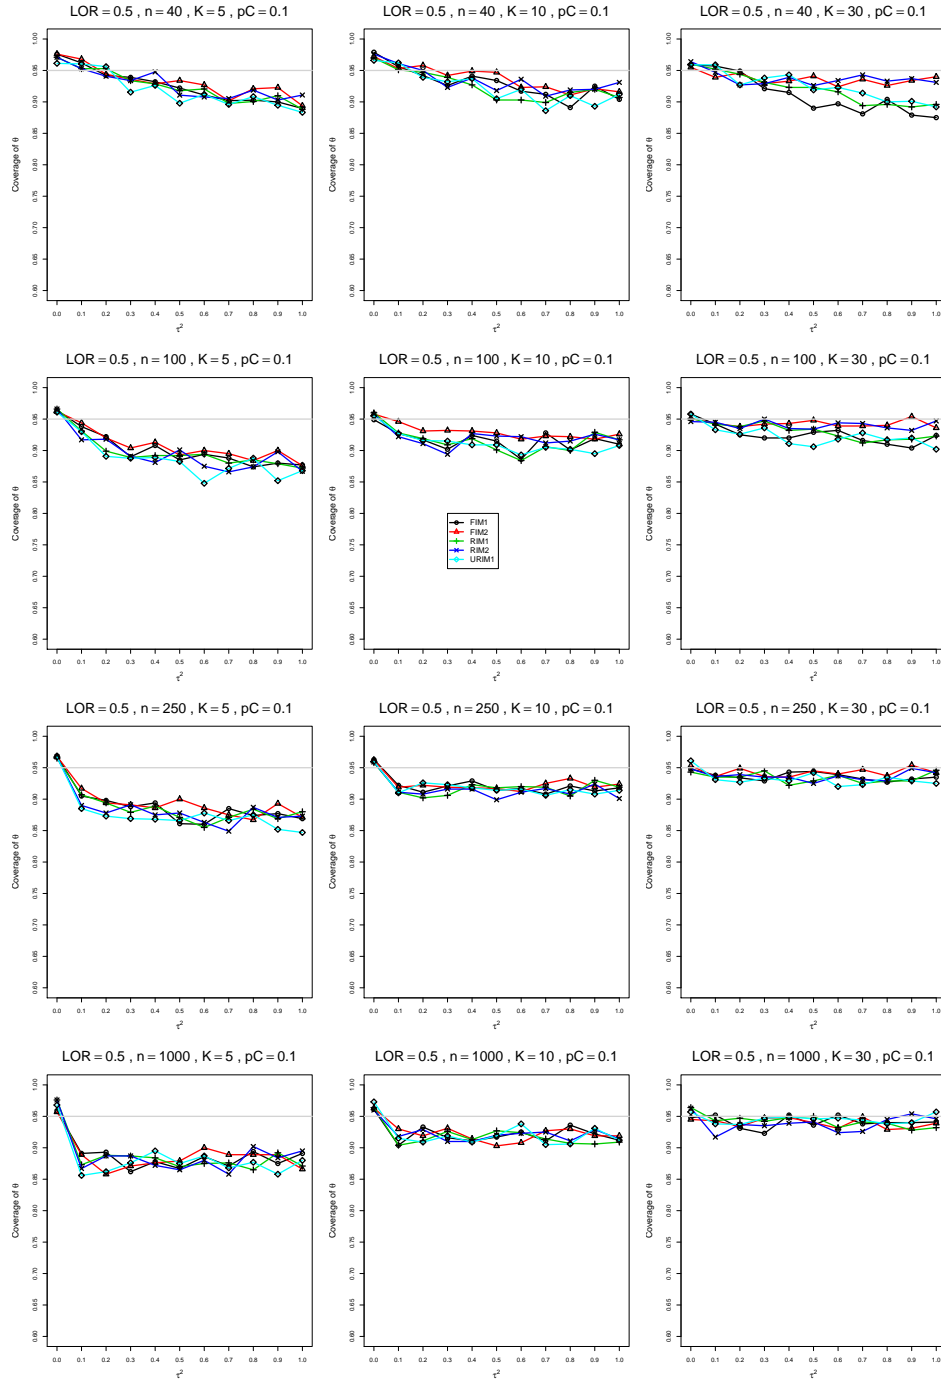

Figure A3.2.13: Coverage of the Restricted Maximum Likelihood confidence interval for  $\theta = 0.5$ ,  $p_C = 0.1$ ,  $\sigma^2 = 0.4$ , constant sample sizes  $n = 40, 100, 250, 1000$ . The data-generation mechanisms are FIM1 ( $\circ$ ), FIM2 ( $\triangle$ ), RIM1 ( $+$ ), RIM2 ( $\times$ ), and URIM1 ( $\diamond$ ).

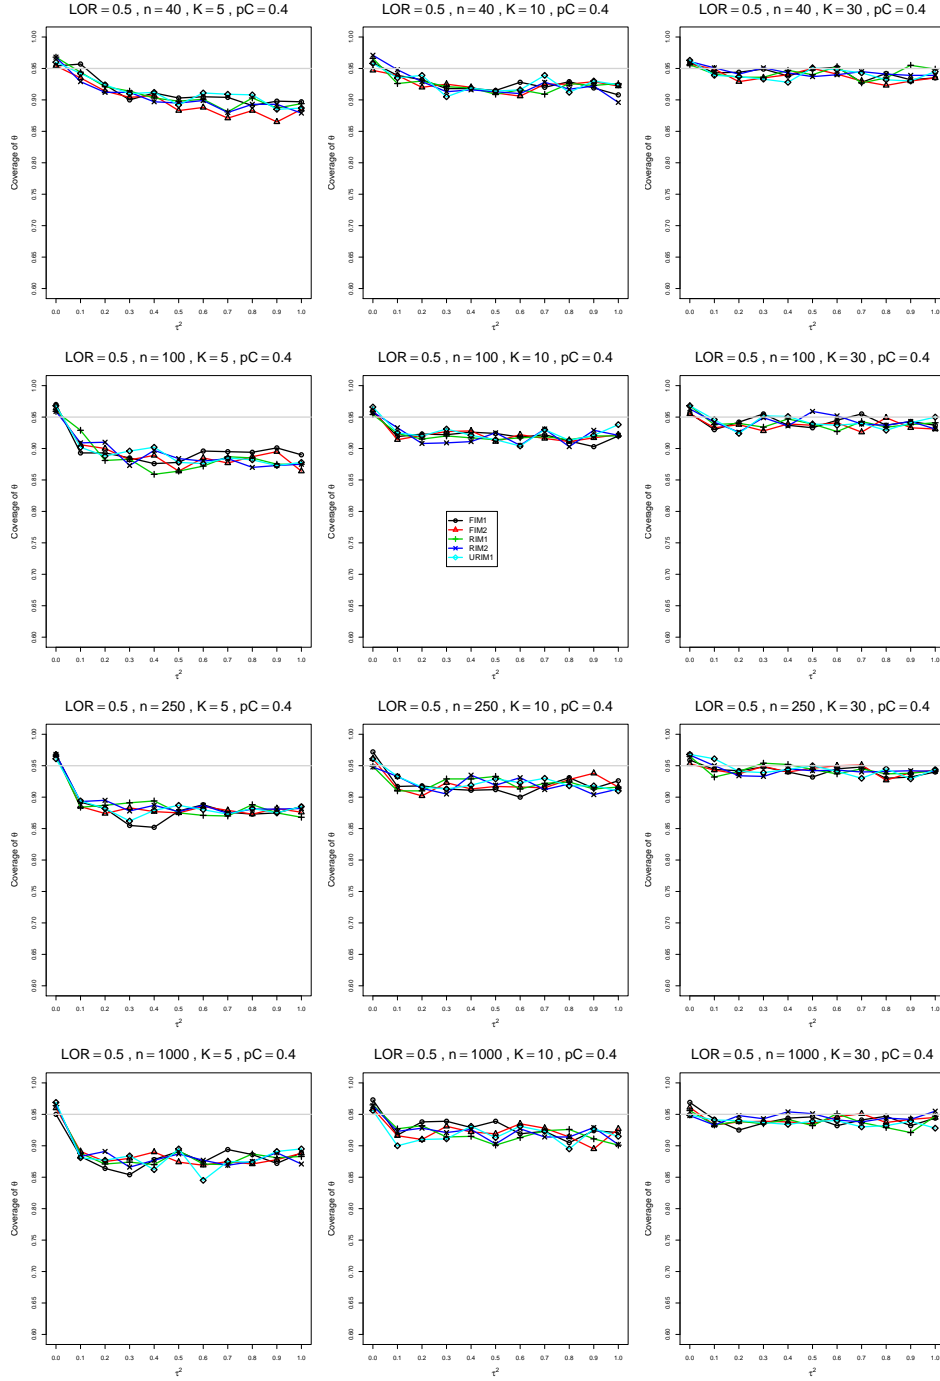

Figure A3.2.14: Coverage of the Restricted Maximum Likelihood confidence interval for  $\theta = 0.5$ ,  $p_C = 0.4$ ,  $\sigma^2 = 0.4$ , constant sample sizes  $n = 40, 100, 250, 1000$ . The data-generation mechanisms are FIM1 ( $\circ$ ), FIM2 ( $\triangle$ ), RIM1 ( $+$ ), RIM2 ( $\times$ ), and URIM1 ( $\diamond$ ).

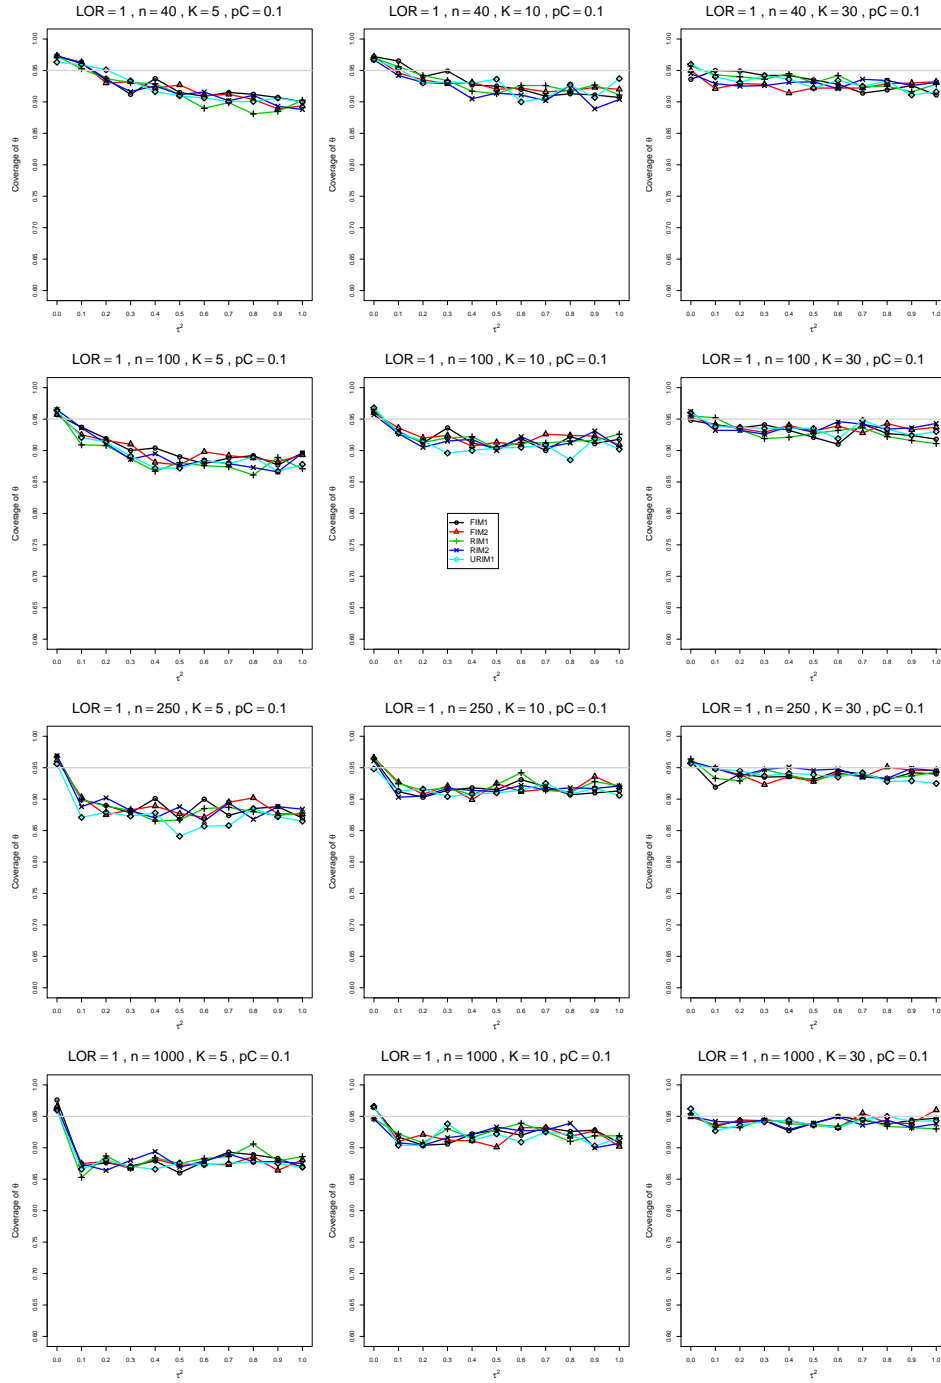

Figure A3.2.15: Coverage of the Restricted Maximum Likelihood confidence interval for  $\theta = 1$ ,  $p_C = 0.1$ ,  $\sigma^2 = 0.4$ , constant sample sizes  $n = 40, 100, 250, 1000$ . The data-generation mechanisms are FIM1 ( $\circ$ ), FIM2 ( $\triangle$ ), RIM1 (+), RIM2 ( $\times$ ), and URIM1 ( $\diamond$ ).

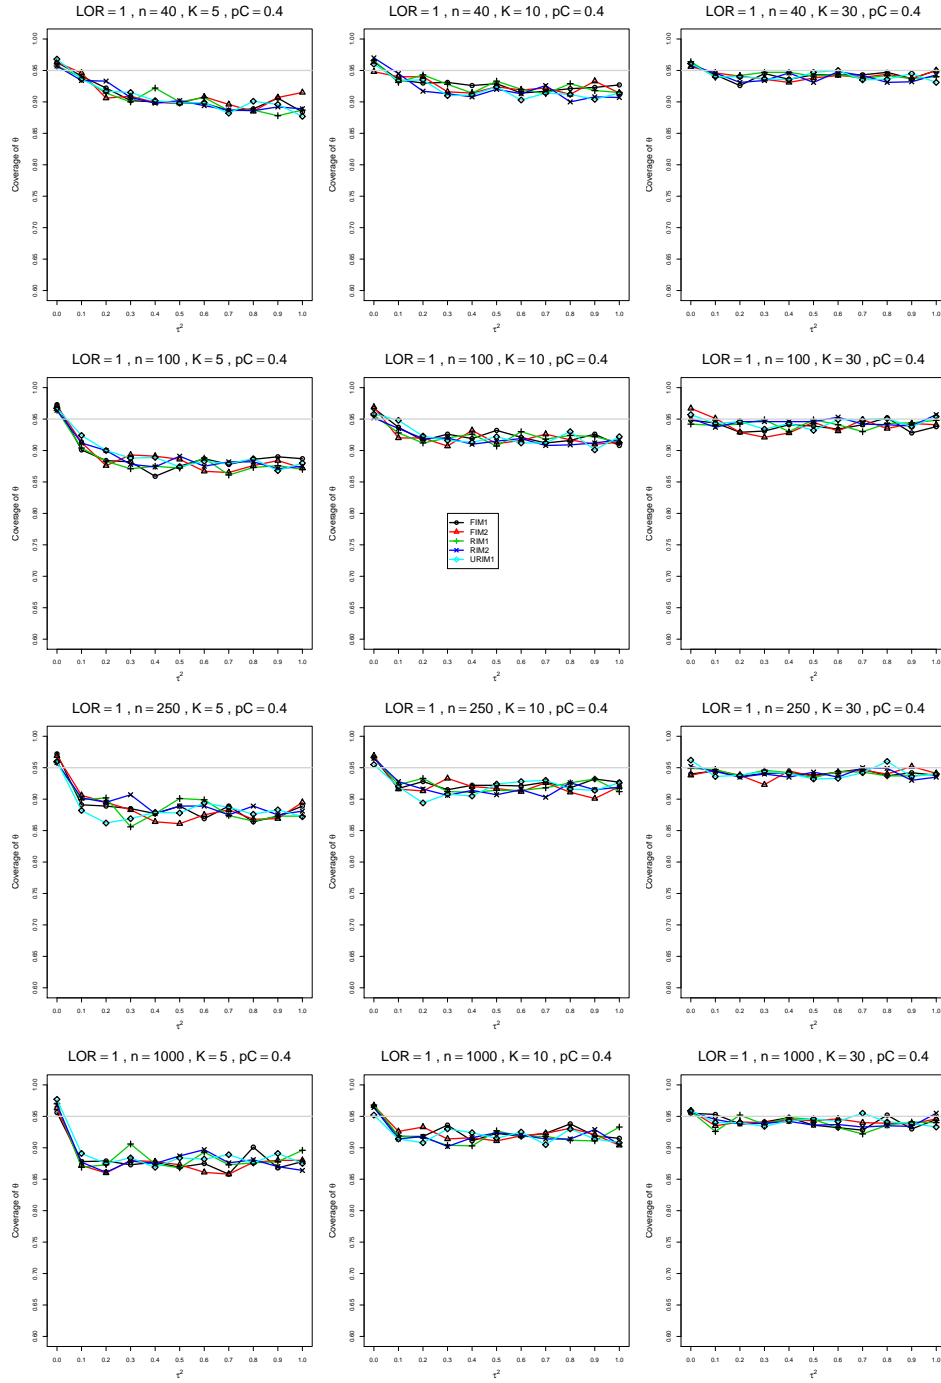

Figure A3.2.16: Coverage of the Restricted Maximum Likelihood confidence interval for  $\theta = 1$ ,  $p_C = 0.4$ ,  $\sigma^2 = 0.4$ , constant sample sizes  $n = 40, 100, 250, 1000$ . The data-generation mechanisms are FIM1 ( $\circ$ ), FIM2 ( $\triangle$ ), RIM1 ( $+$ ), RIM2 ( $\times$ ), and URIM1 ( $\diamond$ ).

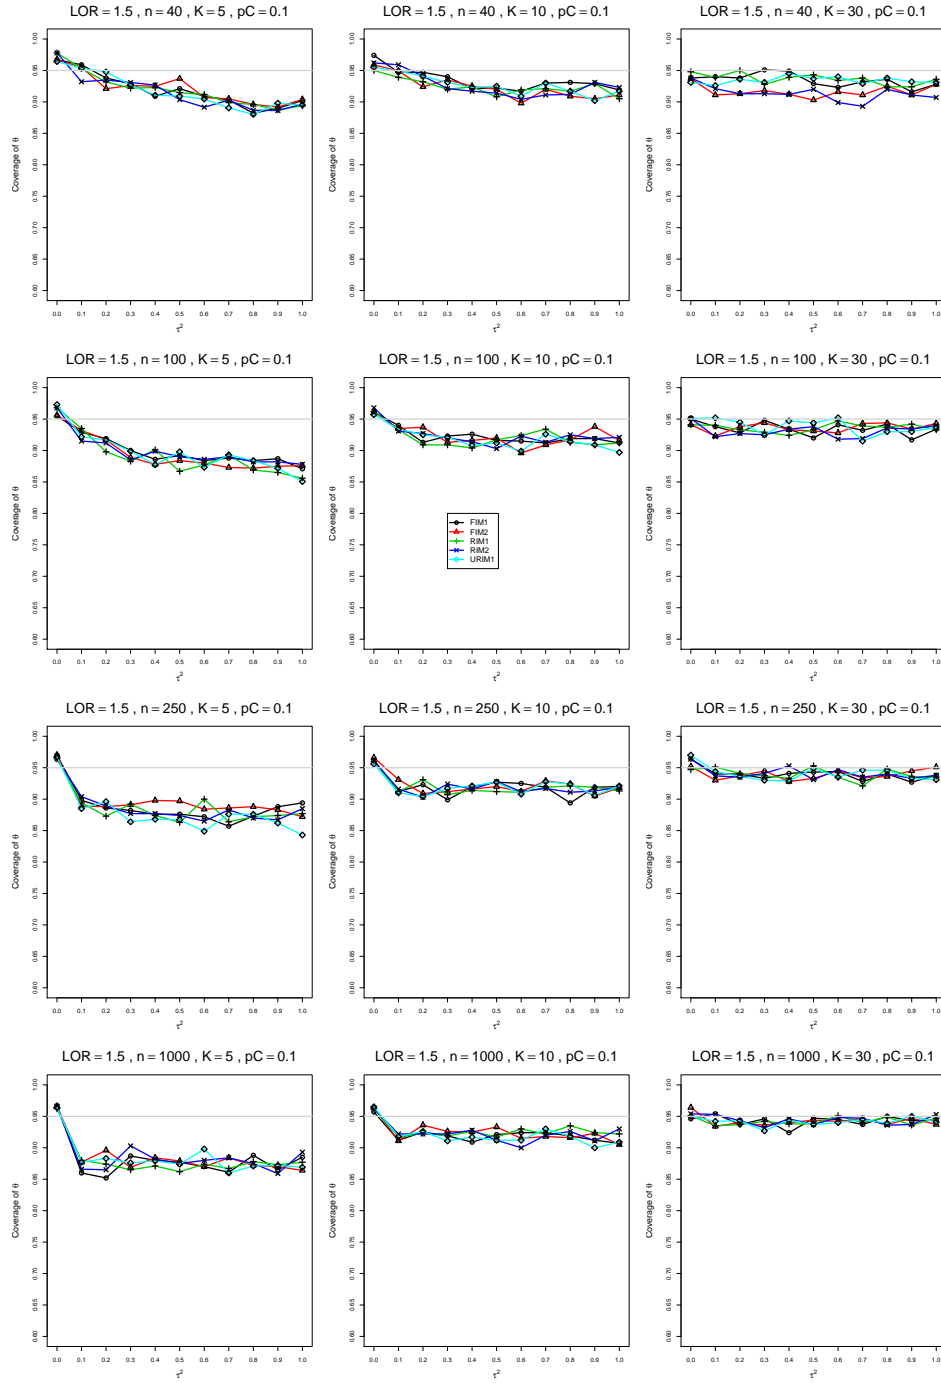

Figure A3.2.17: Coverage of the Restricted Maximum Likelihood confidence interval for  $\theta = 1.5$ ,  $p_C = 0.1$ ,  $\sigma^2 = 0.4$ , constant sample sizes  $n = 40, 100, 250, 1000$ . The data-generation mechanisms are FIM1 ( $\circ$ ), FIM2 ( $\triangle$ ), RIM1 ( $+$ ), RIM2 ( $\times$ ), and URIM1 ( $\diamond$ ).



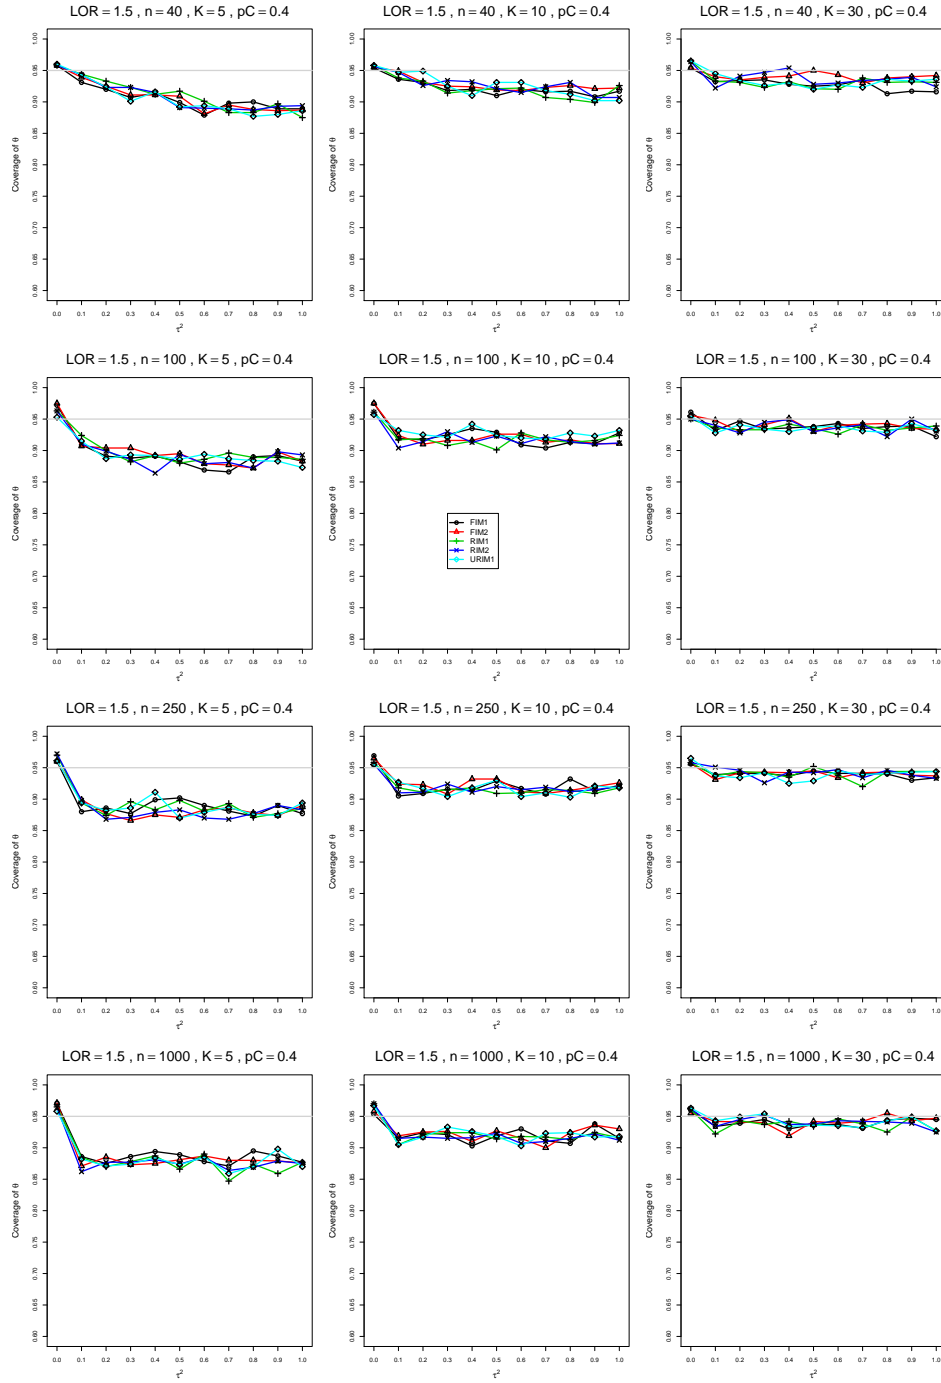

Figure A3.2.18: Coverage of the Restricted Maximum Likelihood confidence interval for  $\theta = 1.5$ ,  $p_C = 0.4$ ,  $\sigma^2 = 0.4$ , constant sample sizes  $n = 40, 100, 250, 1000$ . The data-generation mechanisms are FIM1 ( $\circ$ ), FIM2 ( $\triangle$ ), RIM1 ( $+$ ), RIM2 ( $\times$ ), and URIM1 ( $\diamond$ ).

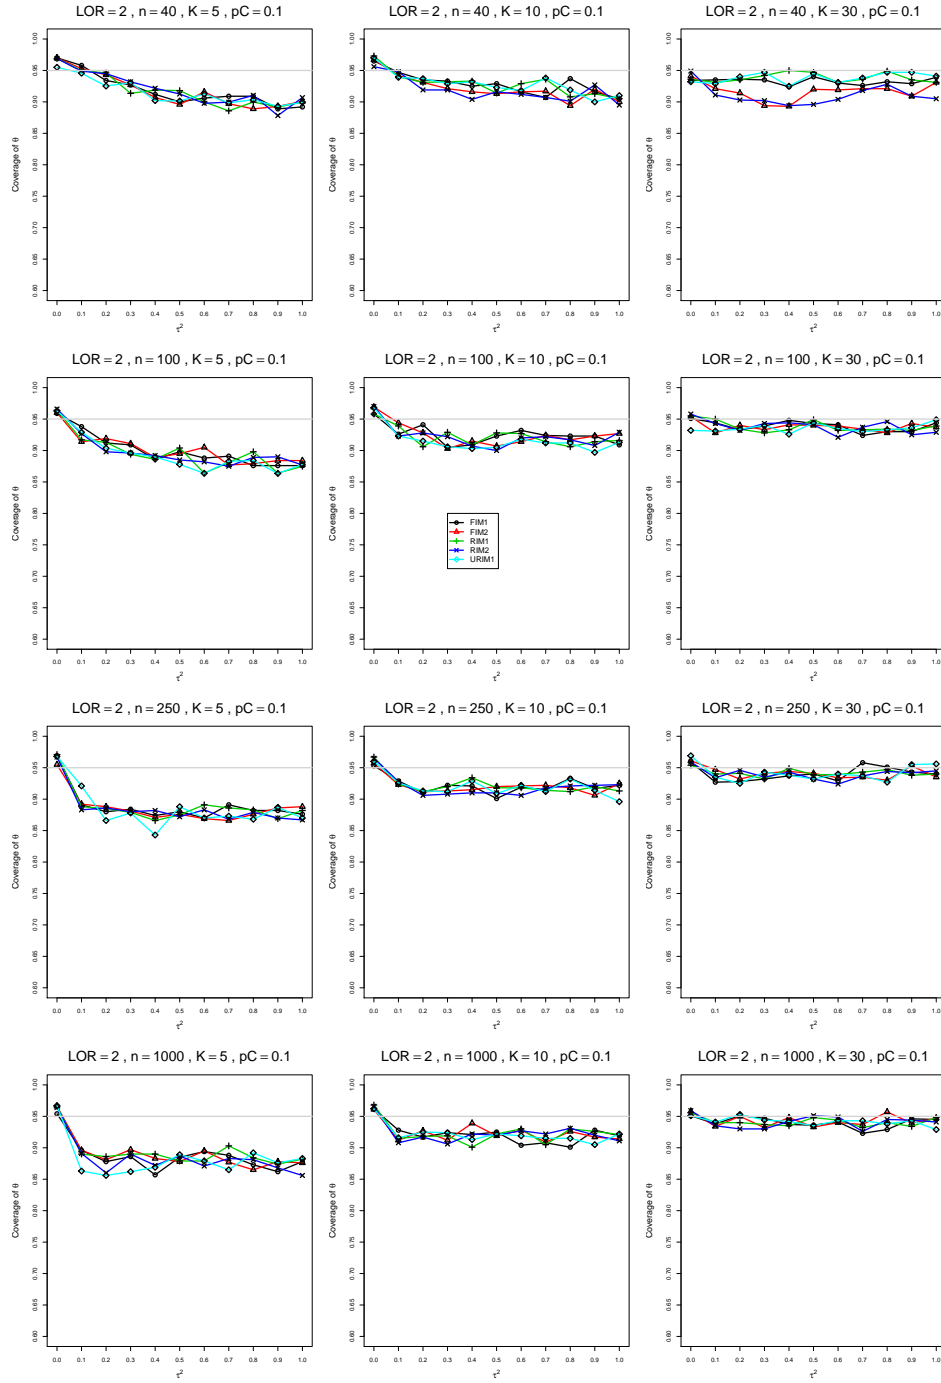

Figure A3.2.19: Coverage of the Restricted Maximum Likelihood confidence interval for  $\theta = 2$ ,  $p_C = 0.1$ ,  $\sigma^2 = 0.4$ , constant sample sizes  $n = 40, 100, 250, 1000$ . The data-generation mechanisms are FIM1 ( $\circ$ ), FIM2 ( $\triangle$ ), RIM1 ( $+$ ), RIM2 ( $\times$ ), and URIM1 ( $\diamond$ ).

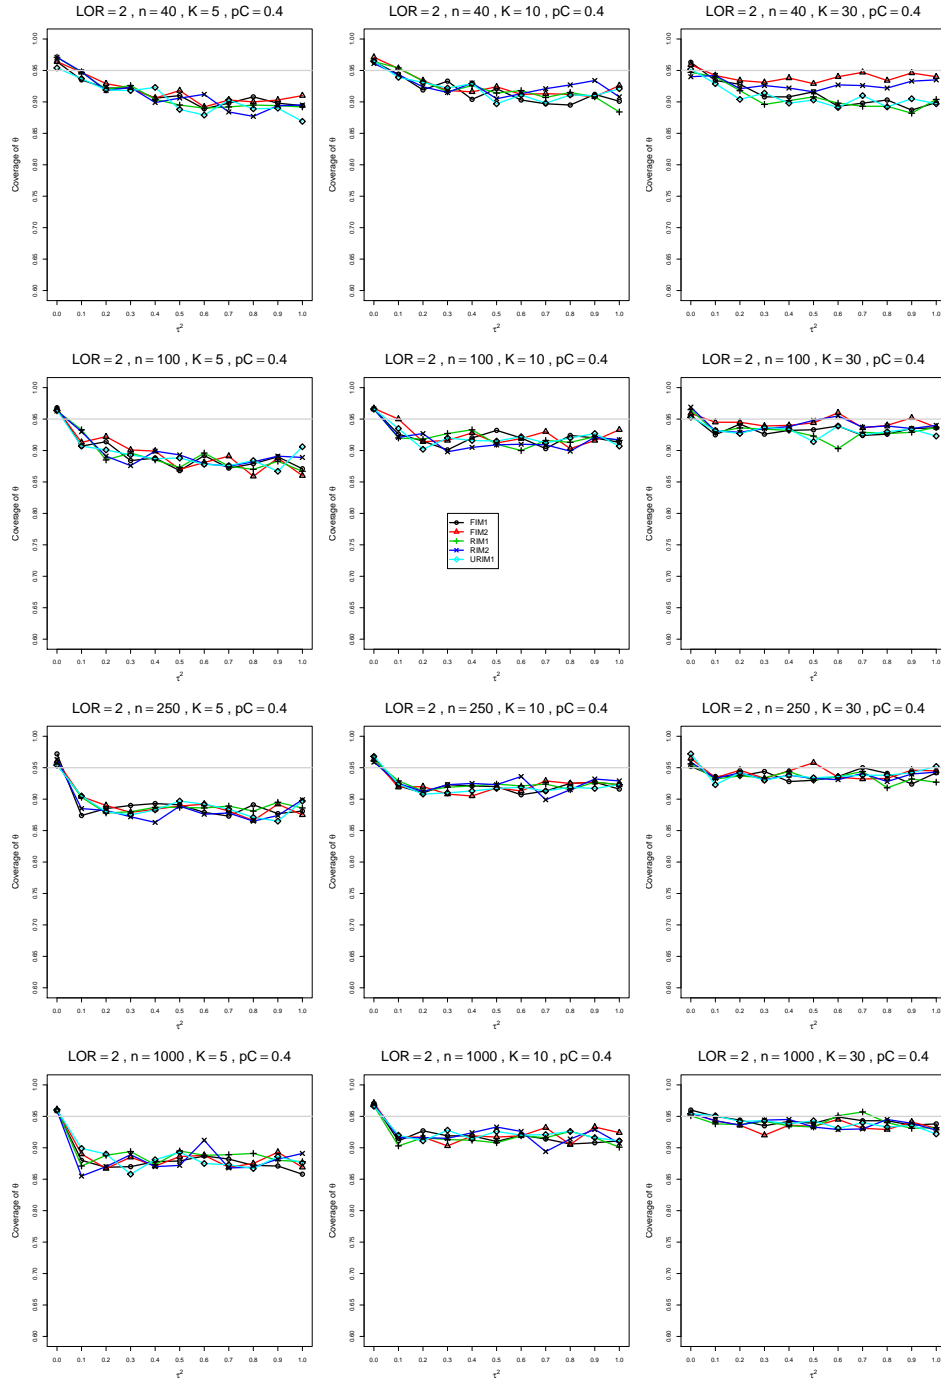

Figure A3.2.20: Coverage of the Restricted Maximum Likelihood confidence interval for  $\theta = 2$ ,  $p_C = 0.4$ ,  $\sigma^2 = 0.4$ , constant sample sizes  $n = 40, 100, 250, 1000$ . The data-generation mechanisms are FIM1 (○), FIM2 (△), RIM1 (+), RIM2 (×), and URIM1 (◇).

### A3.3 Coverage of $\hat{\theta}_{MP}$

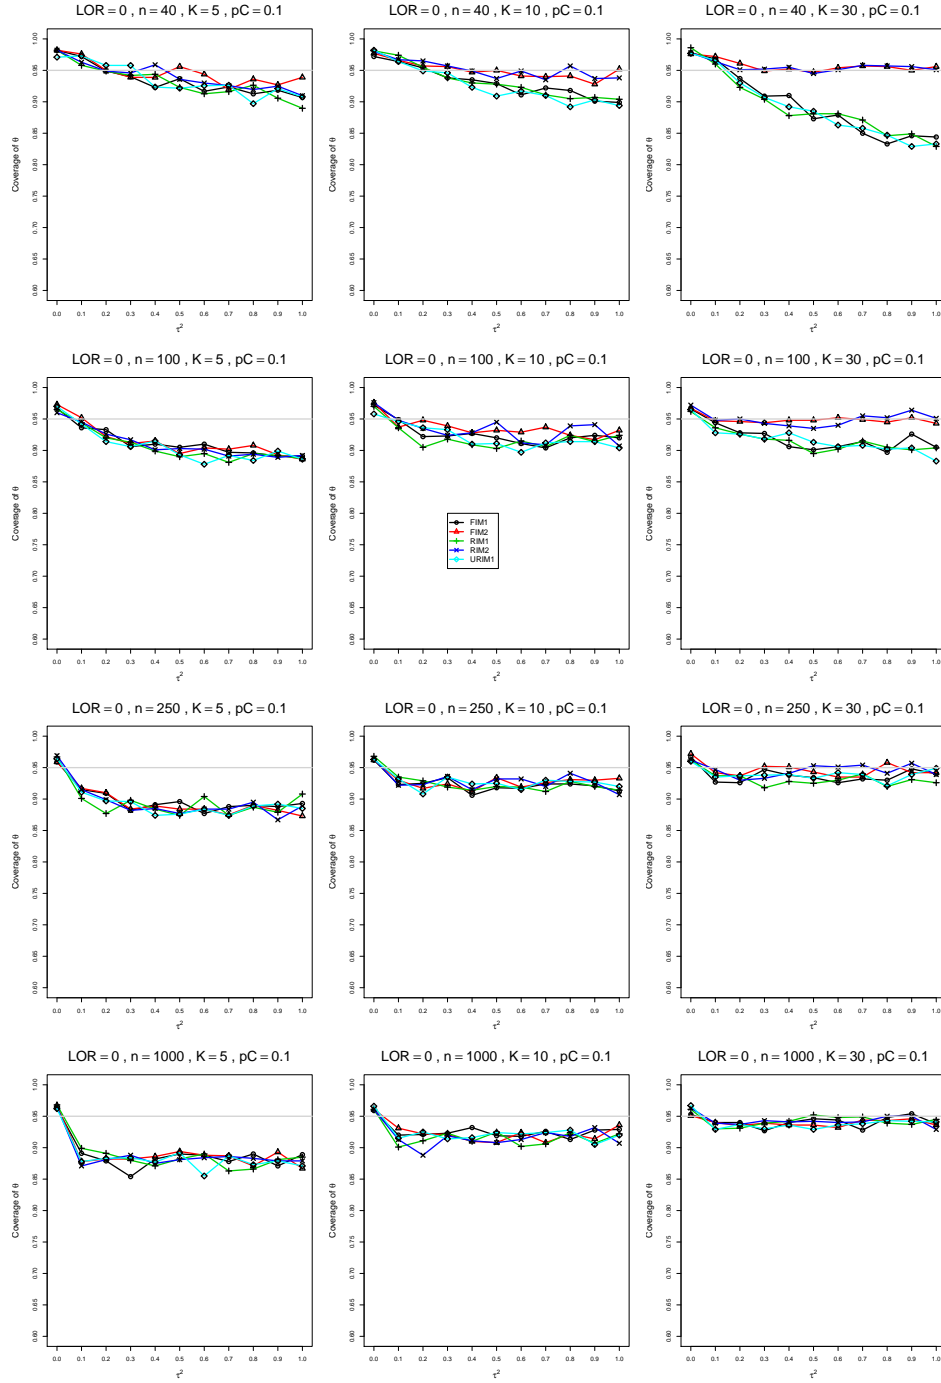

Figure A3.3.1: Coverage of the Mandel-Paule confidence interval for  $\theta = 0$ ,  $p_C = 0.1$ ,  $\sigma^2 = 0.1$ , constant sample sizes  $n = 40, 100, 250, 1000$ . The data-generation mechanisms are FIM1 ( $\circ$ ), FIM2 ( $\triangle$ ), RIM1 (+), RIM2 ( $\times$ ), and URIM1 ( $\diamond$ ).

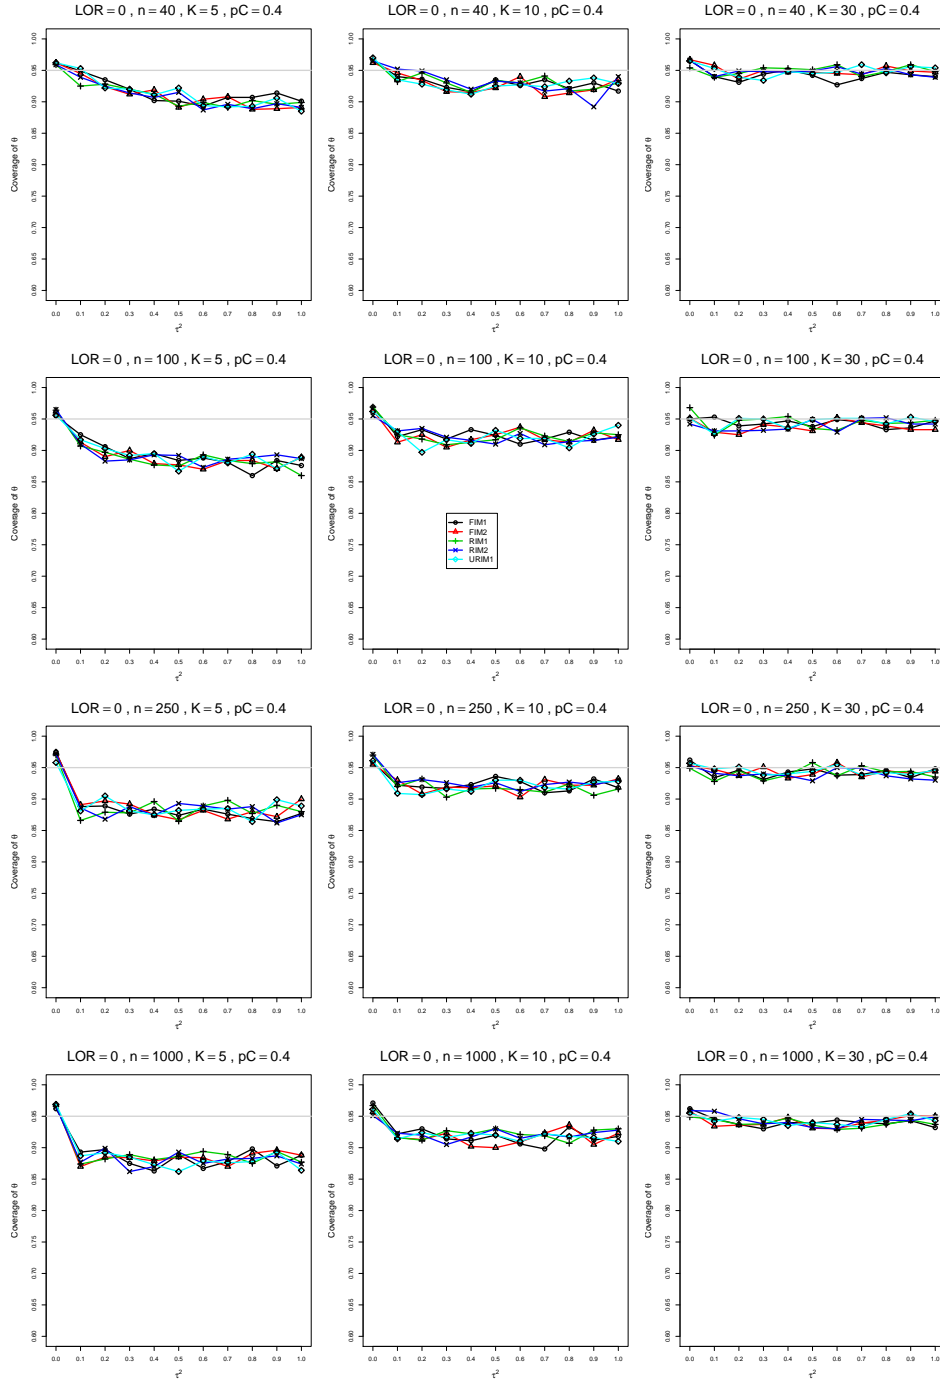

Figure A3.3.2: Coverage of the Mandel-Paule confidence interval for  $\theta = 0$ ,  $p_C = 0.4$ ,  $\sigma^2 = 0.1$ , constant sample sizes  $n = 40, 100, 250, 1000$ . The data-generation mechanisms are FIM1 ( $\circ$ ), FIM2 ( $\triangle$ ), RIM1 ( $+$ ), RIM2 ( $\times$ ), and URIM1 ( $\diamond$ ).

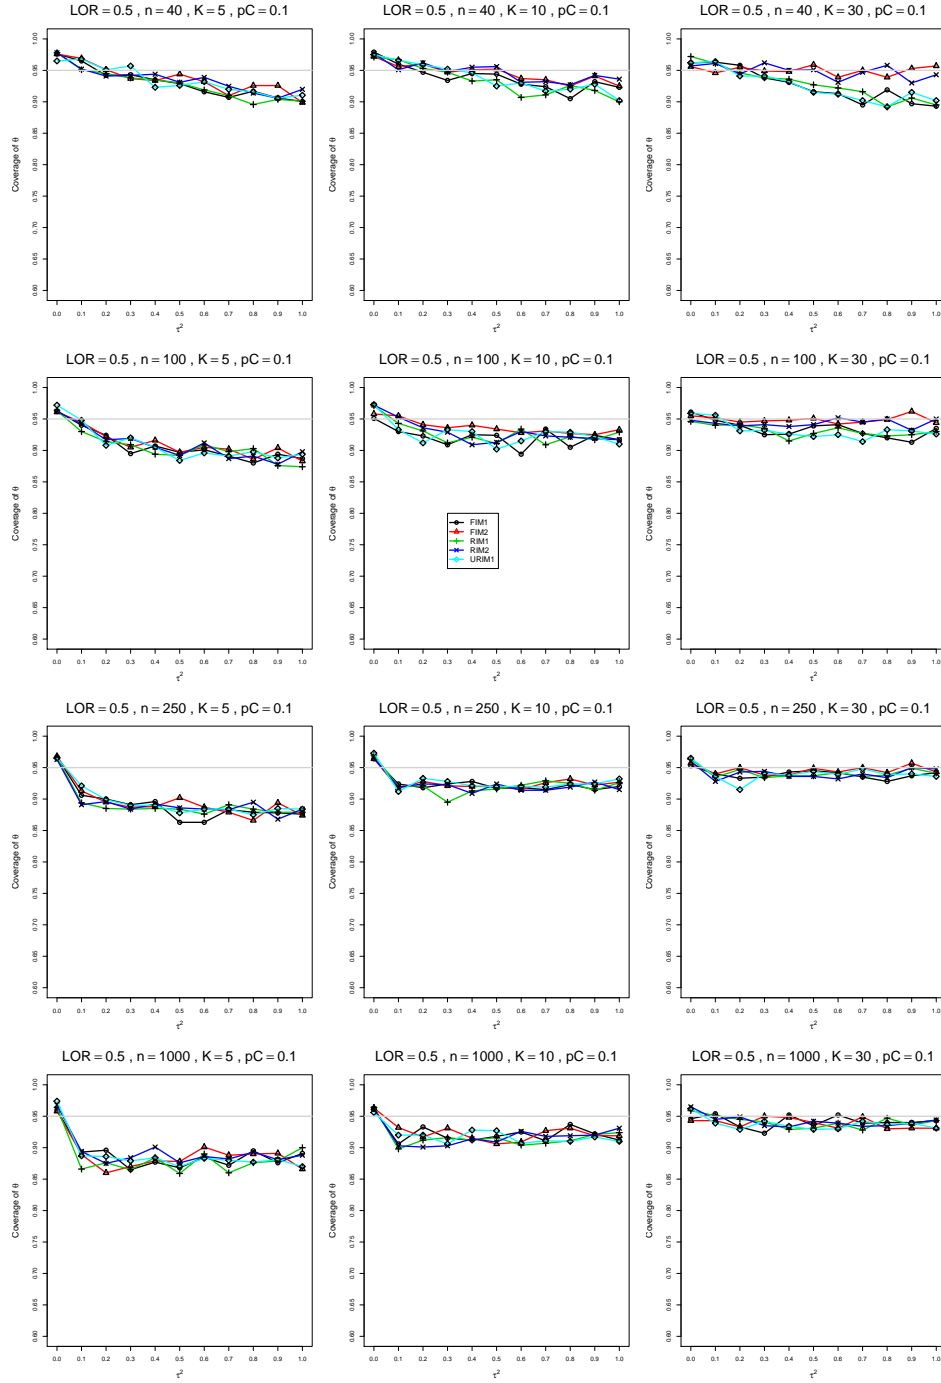

Figure A3.3.3: Coverage of the Mandel-Paula confidence interval for  $\theta = 0.5$ ,  $p_C = 0.1$ ,  $\sigma^2 = 0.1$ , constant sample sizes  $n = 40, 100, 250, 1000$ . The data-generation mechanisms are FIM1 ( $\circ$ ), FIM2 ( $\triangle$ ), RIM1 (+), RIM2 ( $\times$ ), and URIM1 ( $\diamond$ ).

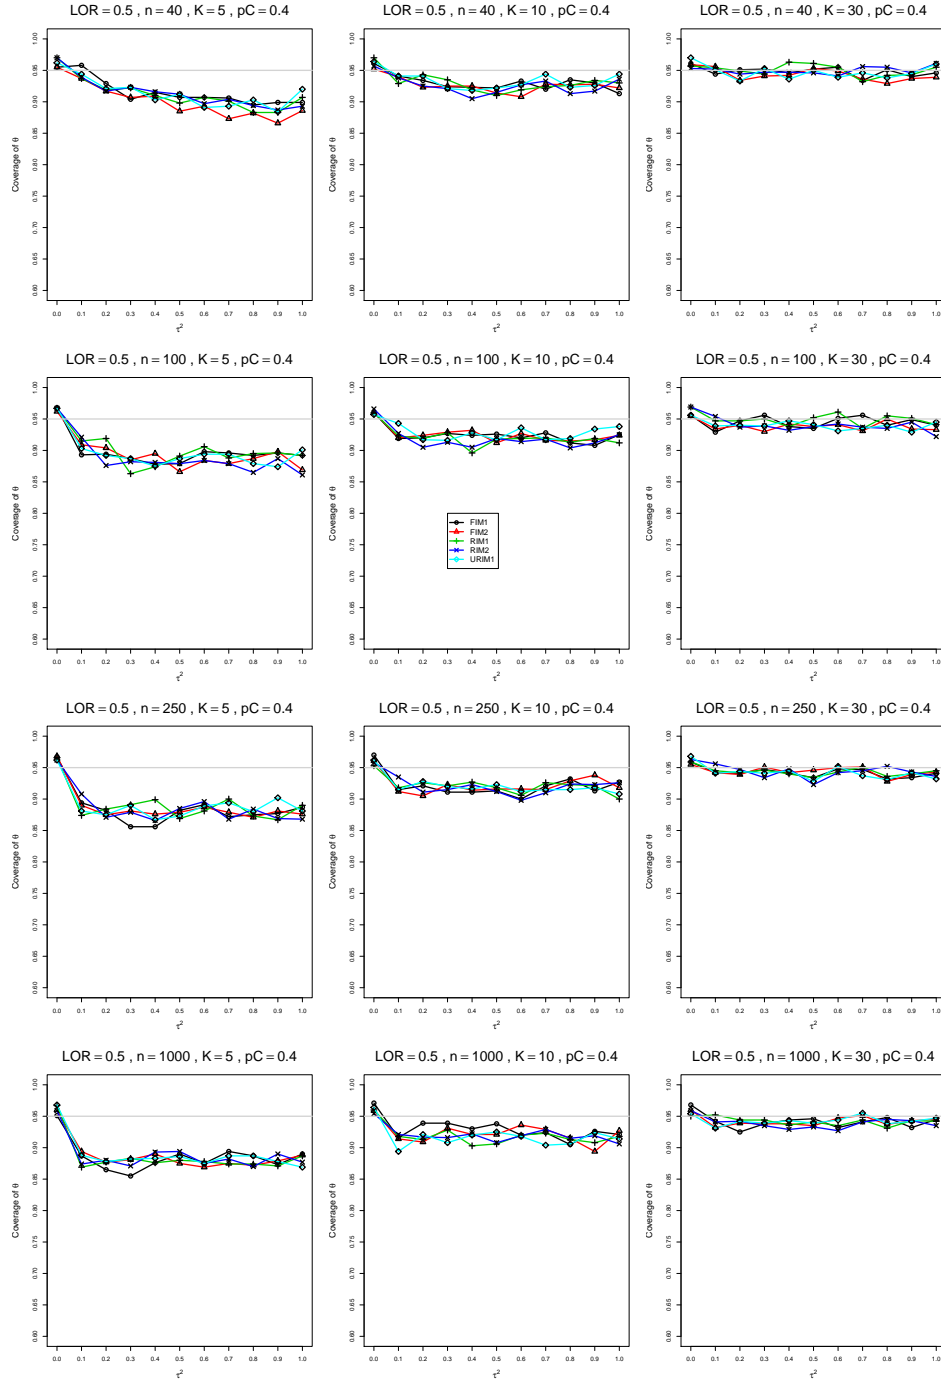

Figure A3.3.4: Coverage of the Mandel-Paule confidence interval for  $\theta = 0.5$ ,  $p_C = 0.4$ ,  $\sigma^2 = 0.1$ , constant sample sizes  $n = 40, 100, 250, 1000$ . The data-generation mechanisms are FIM1 ( $\circ$ ), FIM2 ( $\triangle$ ), RIM1 ( $+$ ), RIM2 ( $\times$ ), and URIM1 ( $\diamond$ ).



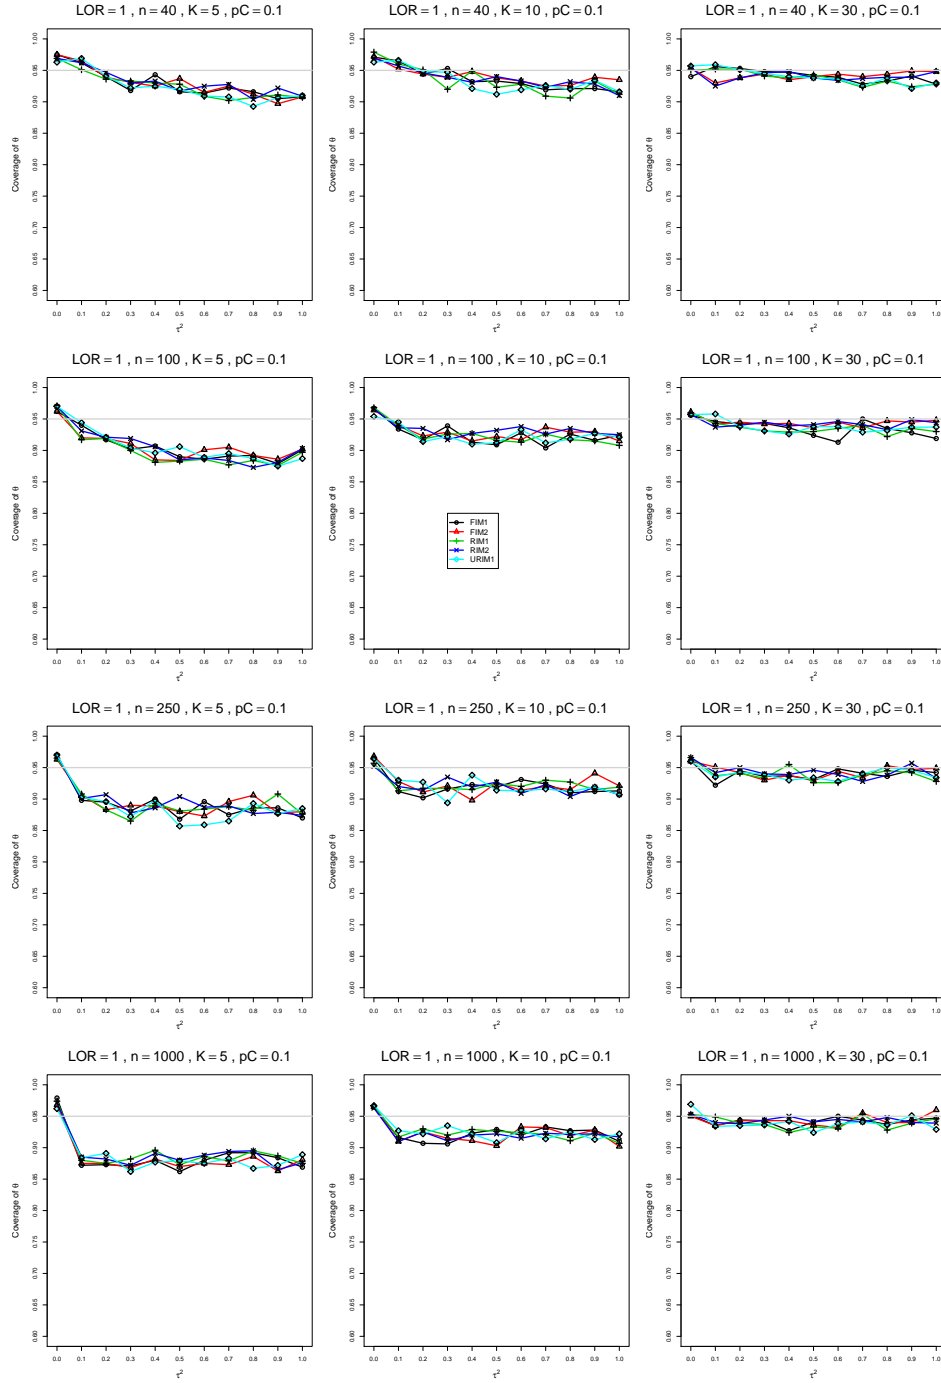

Figure A3.3.5: Coverage of the Mandel-Paule confidence interval for  $\theta = 1$ ,  $p_C = 0.1$ ,  $\sigma^2 = 0.1$ , constant sample sizes  $n = 40, 100, 250, 1000$ . The data-generation mechanisms are FIM1 ( $\circ$ ), FIM2 ( $\triangle$ ), RIM1 ( $+$ ), RIM2 ( $\times$ ), and URIM1 ( $\diamond$ ).

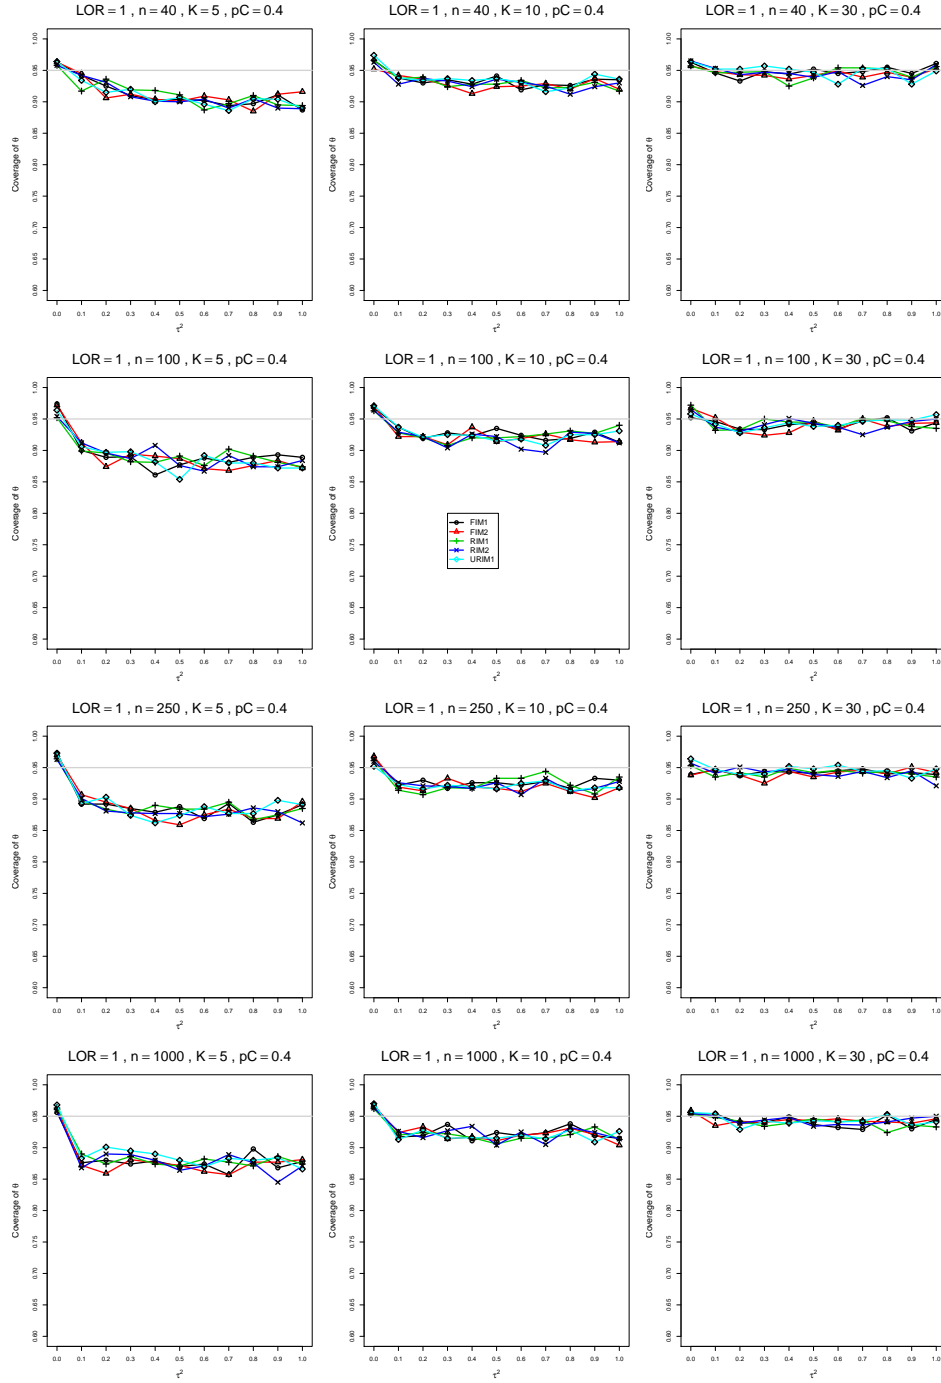

Figure A3.3.6: Coverage of the Mandel-Paule confidence interval for  $\theta = 1$ ,  $p_C = 0.4$ ,  $\sigma^2 = 0.1$ , constant sample sizes  $n = 40, 100, 250, 1000$ . The data-generation mechanisms are FIM1 ( $\circ$ ), FIM2 ( $\triangle$ ), RIM1 ( $+$ ), RIM2 ( $\times$ ), and URIM1 ( $\diamond$ ).

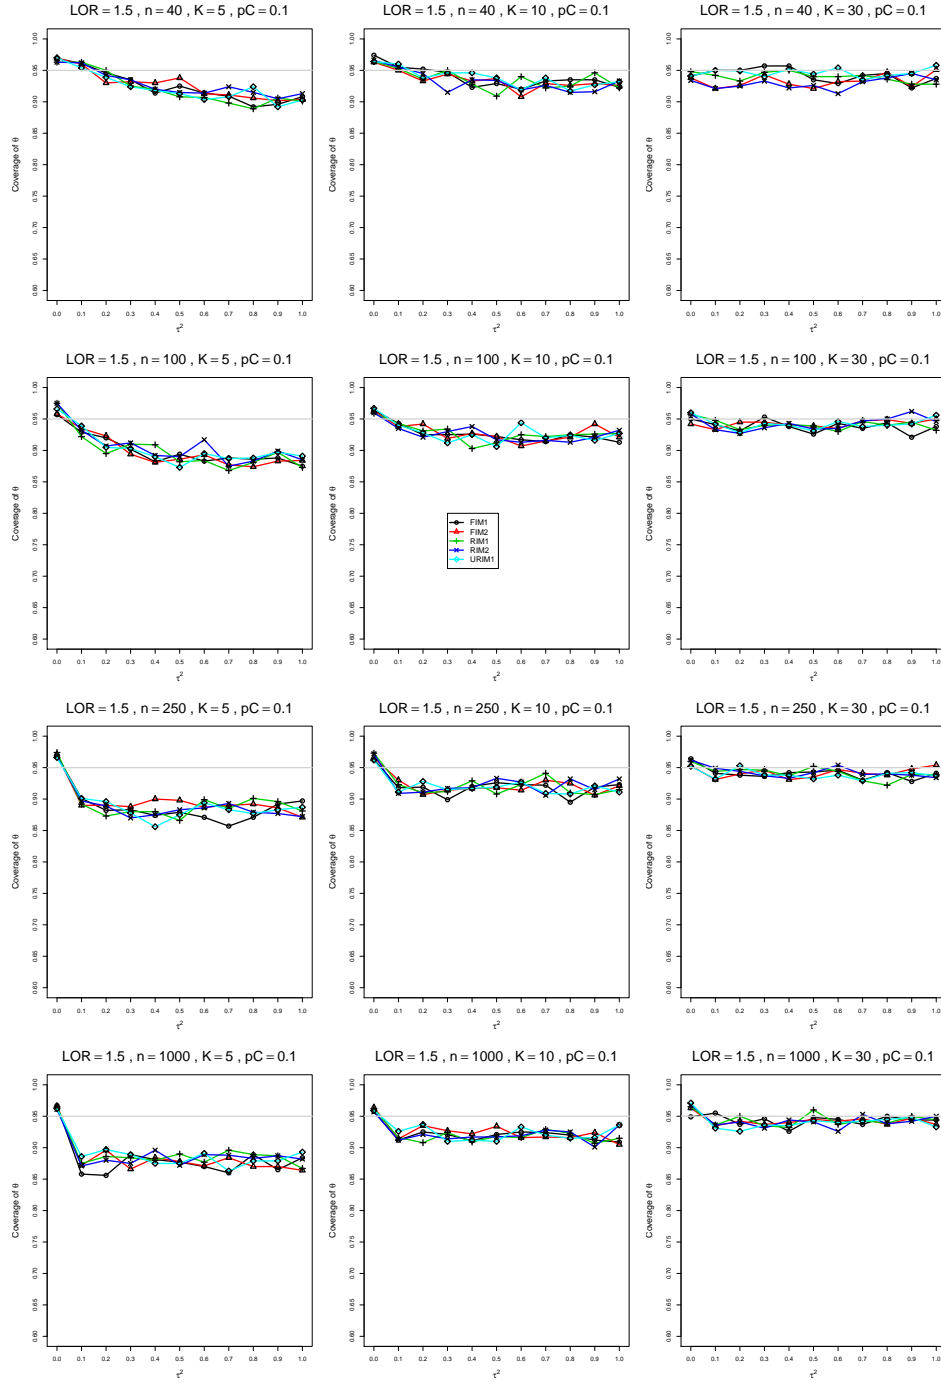

Figure A3.3.7: Coverage of the Mandel-Paula confidence interval for  $\theta = 1.5$ ,  $p_C = 0.1$ ,  $\sigma^2 = 0.1$ , constant sample sizes  $n = 40, 100, 250, 1000$ . The data-generation mechanisms are FIM1 ( $\circ$ ), FIM2 ( $\triangle$ ), RIM1 ( $+$ ), RIM2 ( $\times$ ), and URIM1 ( $\diamond$ ).

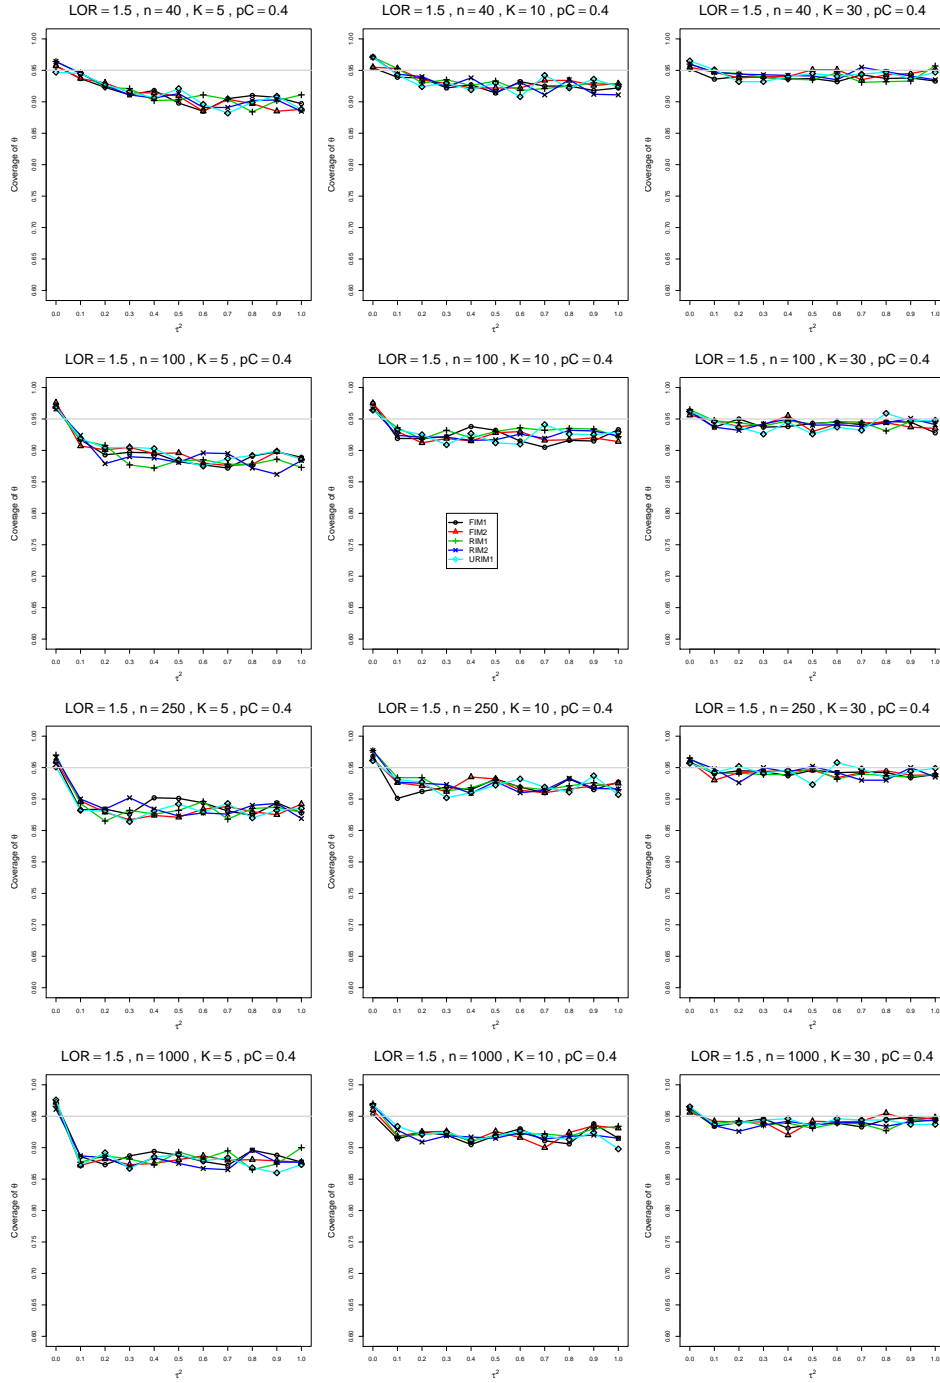

Figure A3.3.8: Coverage of the Mandel-Paula confidence interval for  $\theta = 1.5$ ,  $p_C = 0.4$ ,  $\sigma^2 = 0.1$ , constant sample sizes  $n = 40, 100, 250, 1000$ . The data-generation mechanisms are FIM1 ( $\circ$ ), FIM2 ( $\triangle$ ), RIM1 (+), RIM2 ( $\times$ ), and URIM1 ( $\diamond$ ).

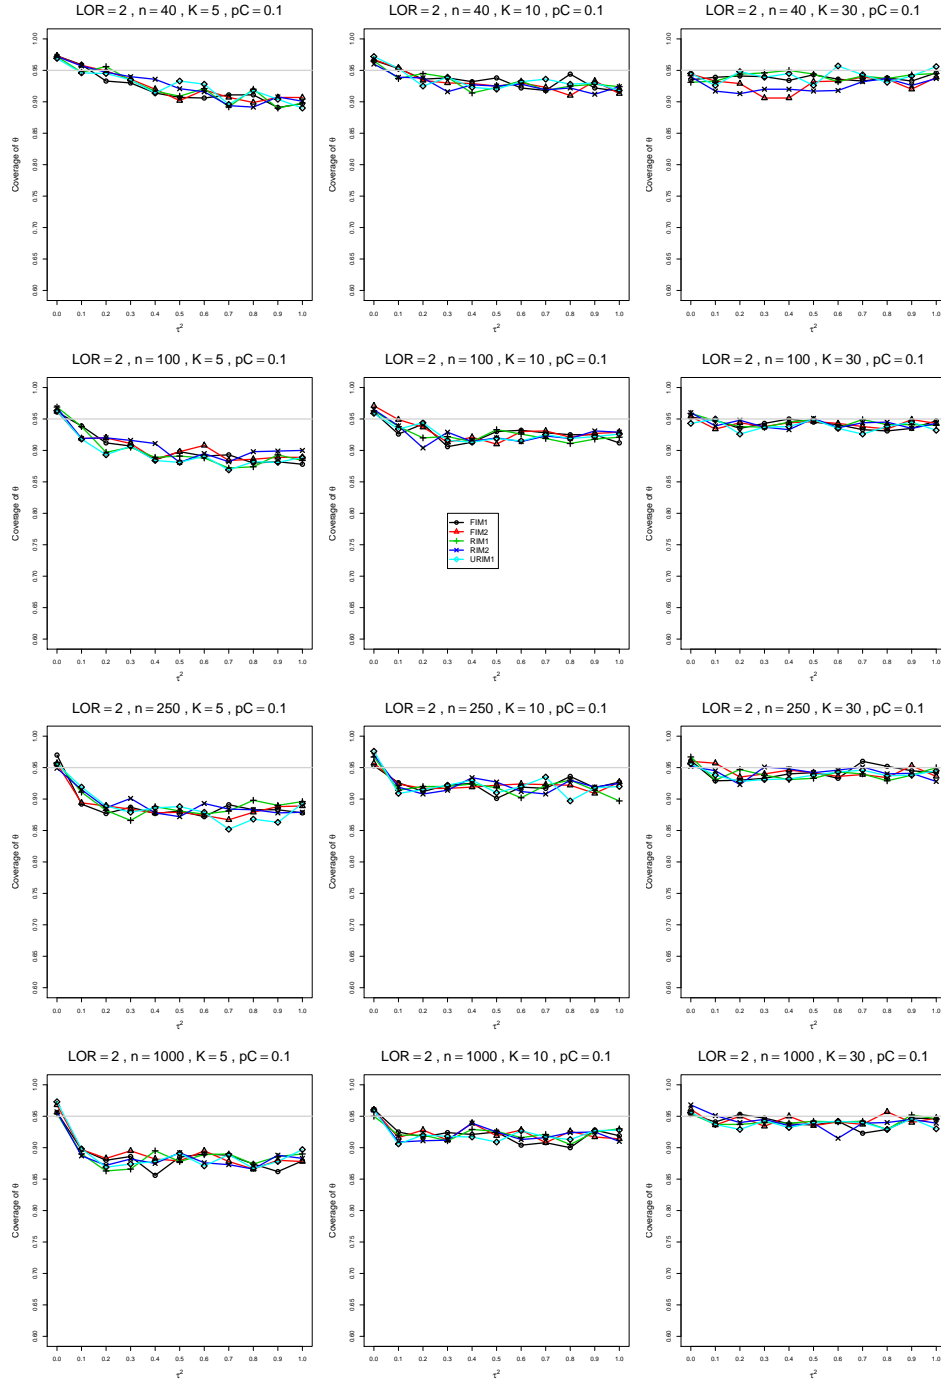

Figure A3.3.9: Coverage of the Mandel-Paule confidence interval for  $\theta = 2$ ,  $p_C = 0.1$ ,  $\sigma^2 = 0.1$ , constant sample sizes  $n = 40, 100, 250, 1000$ . The data-generation mechanisms are FIM1 ( $\circ$ ), FIM2 ( $\triangle$ ), RIM1 ( $+$ ), RIM2 ( $\times$ ), and URIM1 ( $\diamond$ ).

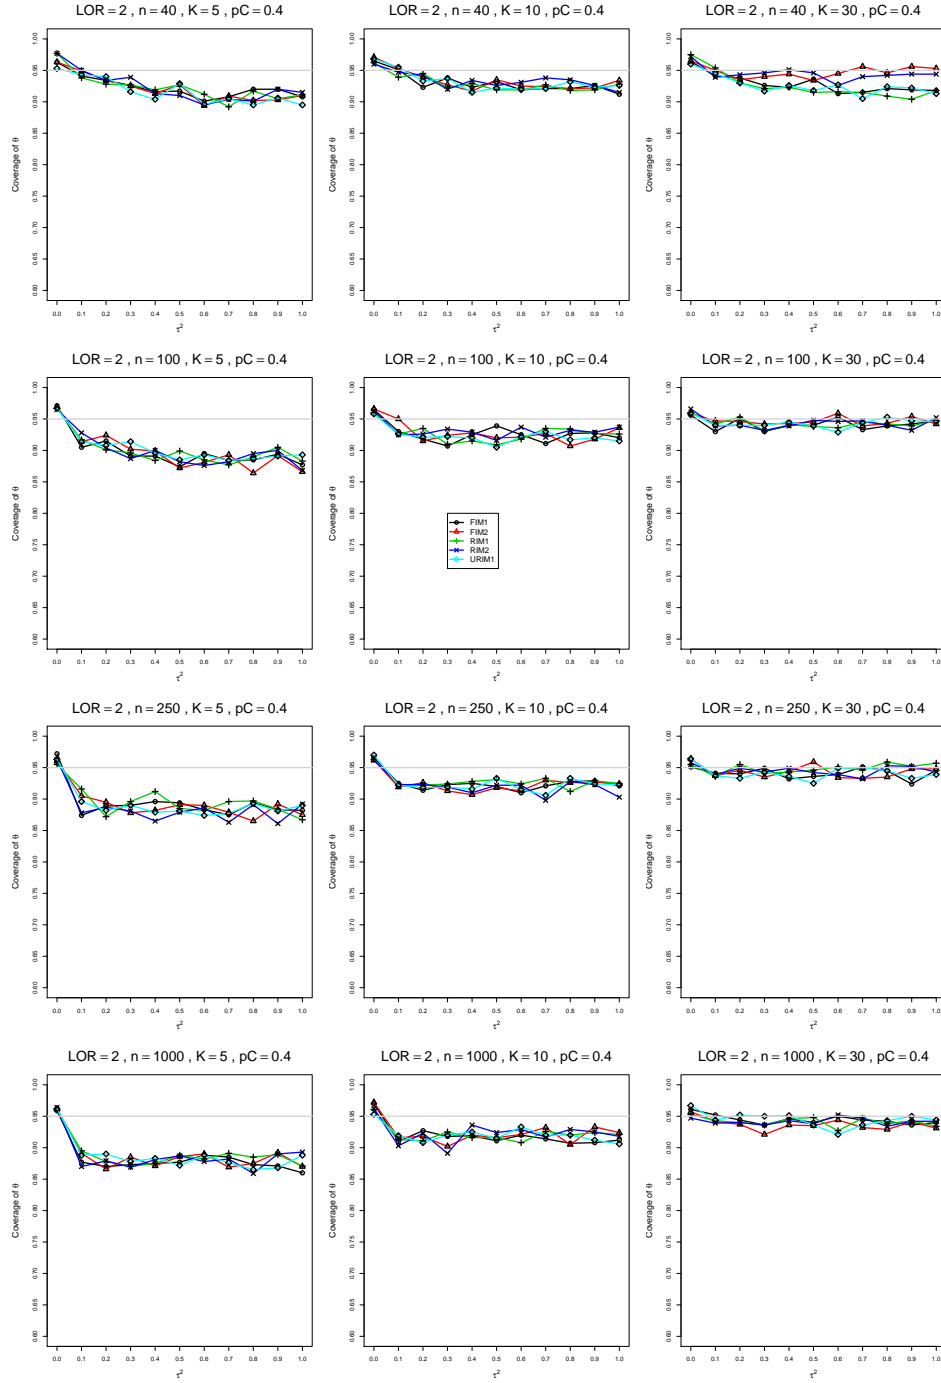

Figure A3.3.10: Coverage of the Mandel-Paule confidence interval for  $\theta = 2$ ,  $p_C = 0.4$ ,  $\sigma^2 = 0.1$ , constant sample sizes  $n = 40, 100, 250, 1000$ . The data-generation mechanisms are FIM1 ( $\circ$ ), FIM2 ( $\triangle$ ), RIM1 ( $+$ ), RIM2 ( $\times$ ), and URIM1 ( $\diamond$ ).

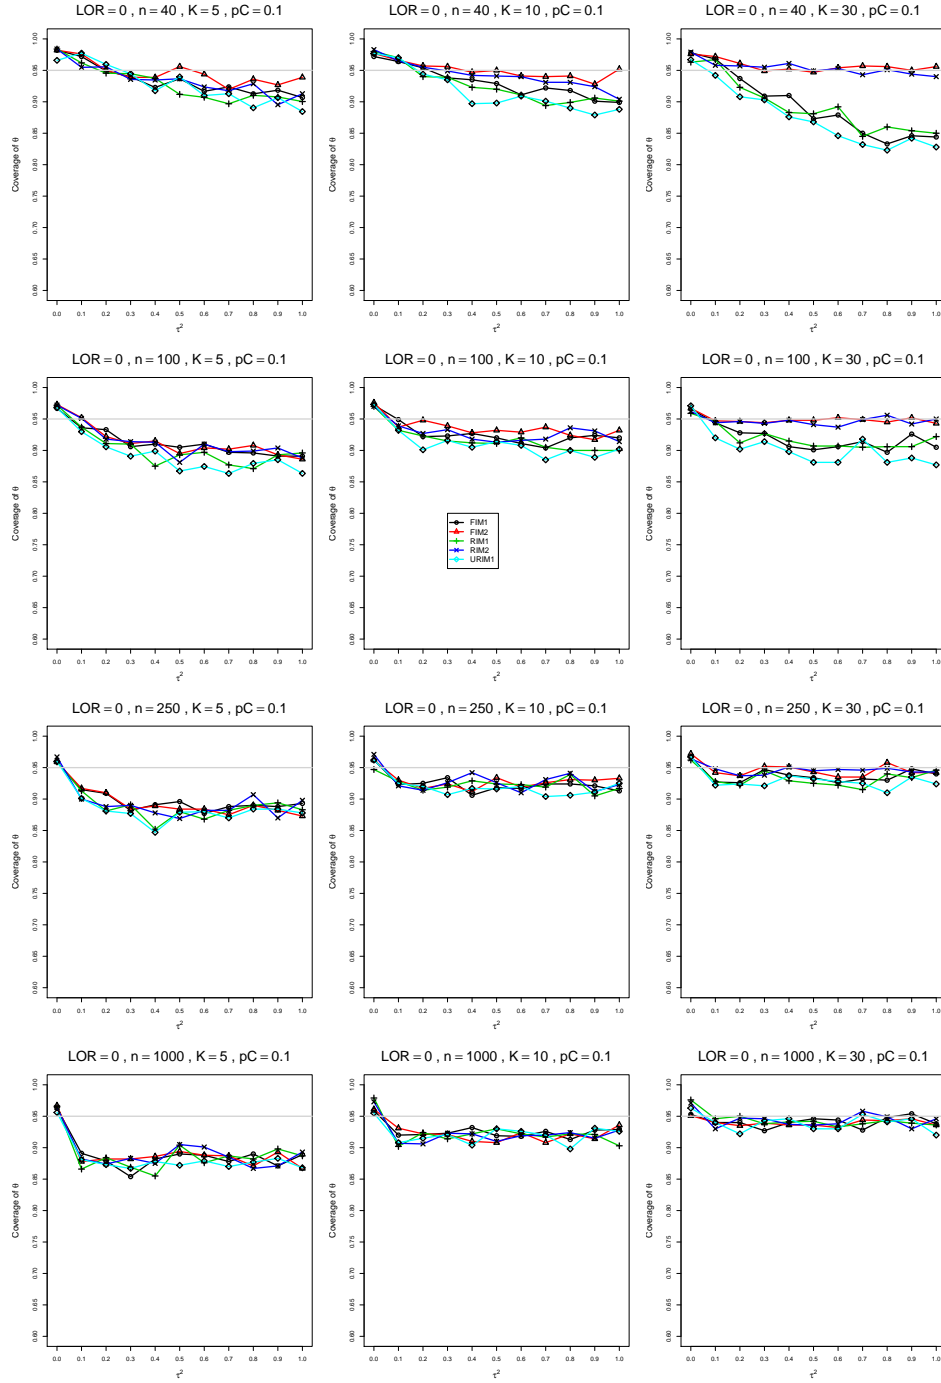

Figure A3.3.11: Coverage of the Mandel-Paulé confidence interval for  $\theta = 0$ ,  $p_C = 0.1$ ,  $\sigma^2 = 0.4$ , constant sample sizes  $n = 40, 100, 250, 1000$ . The data-generation mechanisms are FIM1 ( $\circ$ ), FIM2 ( $\triangle$ ), RIM1 ( $+$ ), RIM2 ( $\times$ ), and URIM1 ( $\diamond$ ).

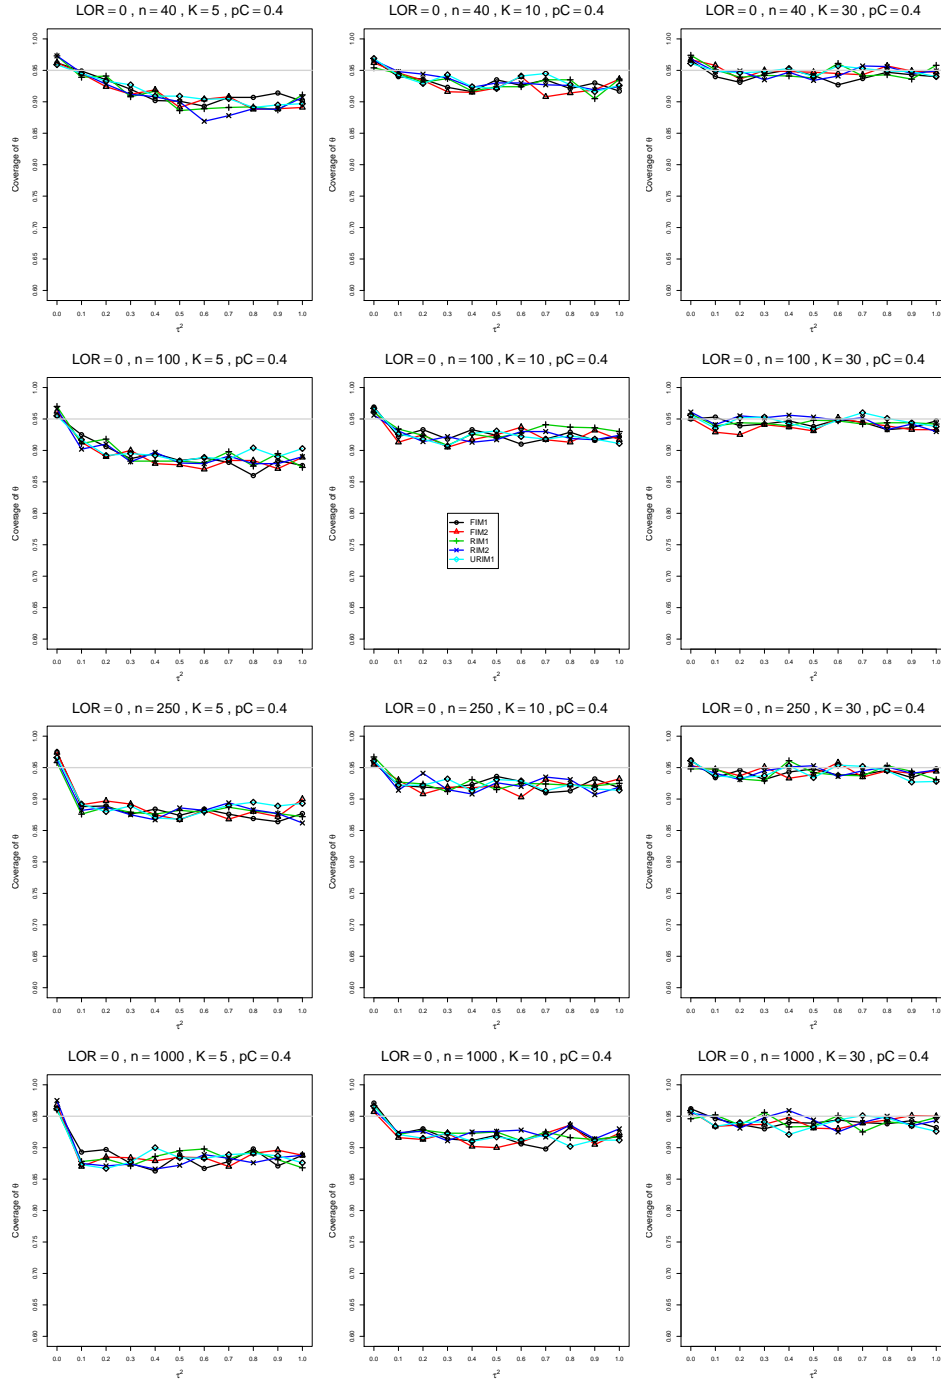

Figure A3.3.12: Coverage of the Mandel-Paulé confidence interval for  $\theta = 0$ ,  $p_C = 0.4$ ,  $\sigma^2 = 0.4$ , constant sample sizes  $n = 40, 100, 250, 1000$ . The data-generation mechanisms are FIM1 ( $\circ$ ), FIM2 ( $\triangle$ ), RIM1 ( $+$ ), RIM2 ( $\times$ ), and URIM1 ( $\diamond$ ).



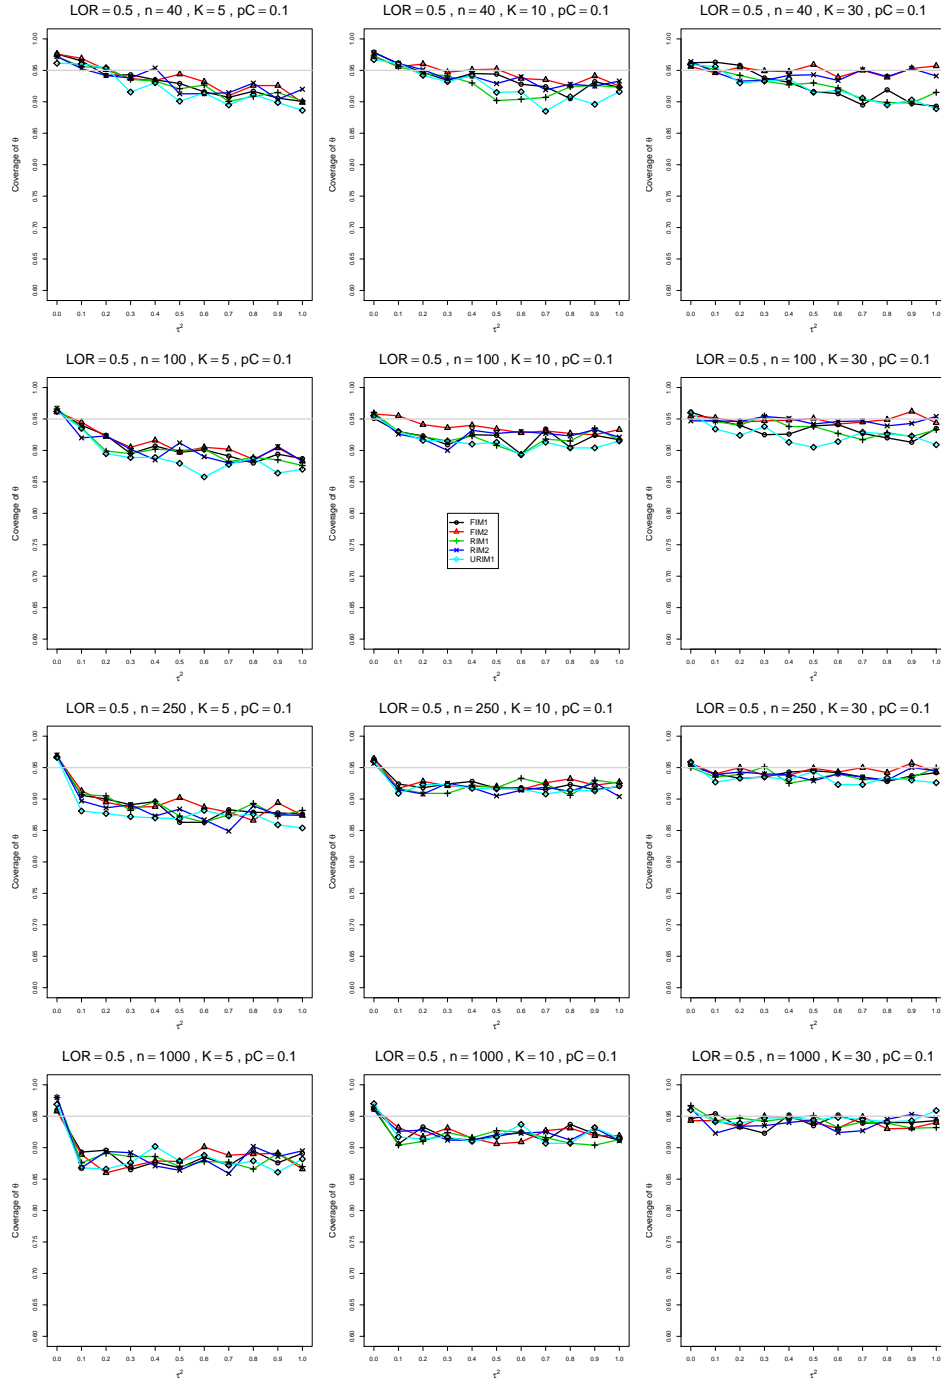

Figure A3.3.13: Coverage of the Mandel-Paule confidence interval for  $\theta = 0.5$ ,  $p_C = 0.1$ ,  $\sigma^2 = 0.4$ , constant sample sizes  $n = 40, 100, 250, 1000$ . The data-generation mechanisms are FIM1 ( $\circ$ ), FIM2 ( $\triangle$ ), RIM1 ( $+$ ), RIM2 ( $\times$ ), and URIM1 ( $\diamond$ ).

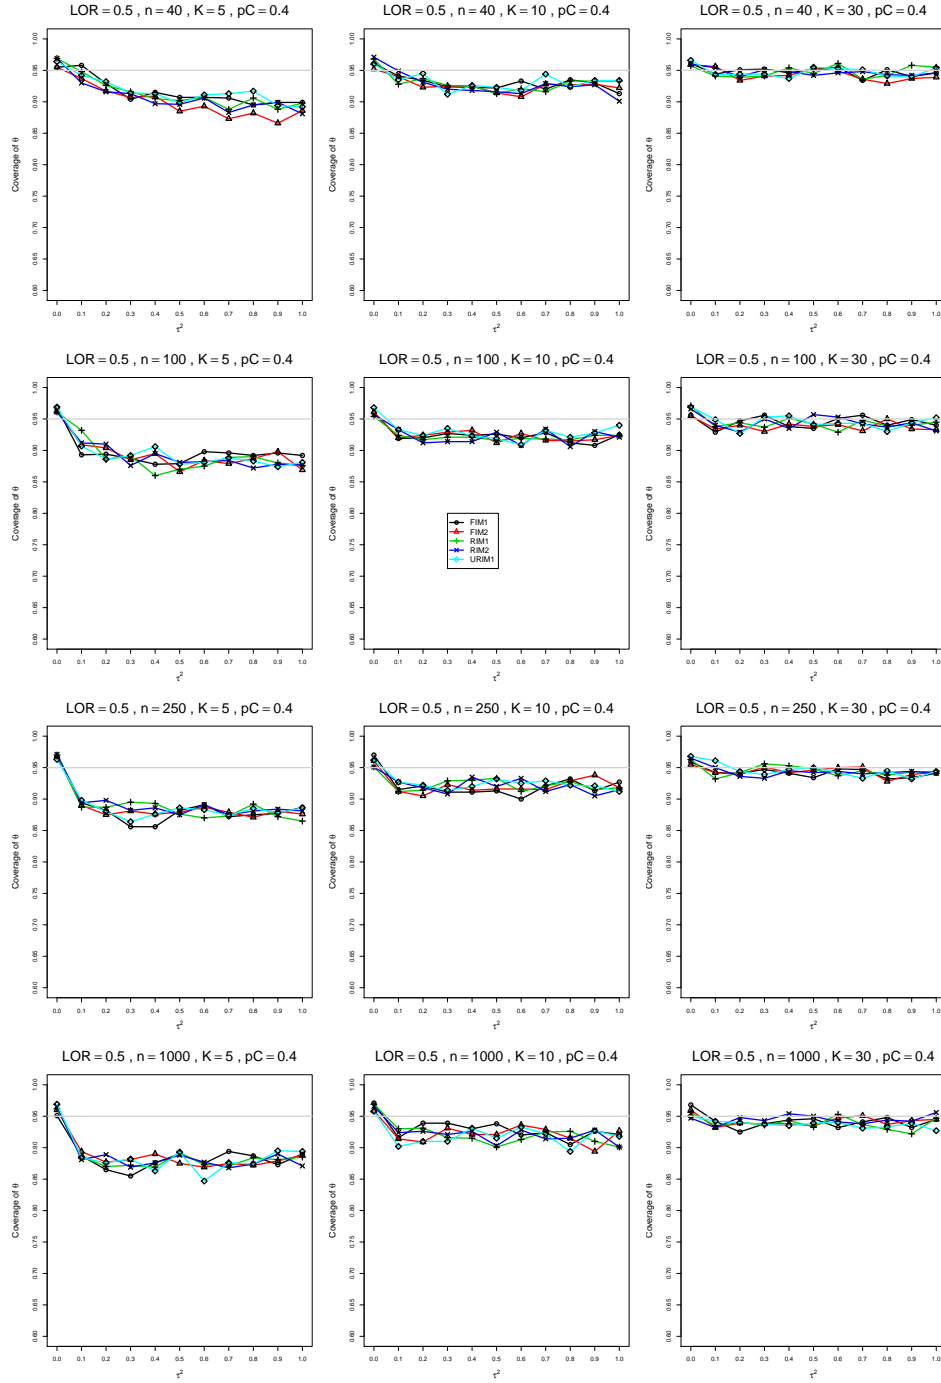

Figure A3.3.14: Coverage of the Mandel-Paule confidence interval for  $\theta = 0.5$ ,  $p_C = 0.4$ ,  $\sigma^2 = 0.4$ , constant sample sizes  $n = 40, 100, 250, 1000$ . The data-generation mechanisms are FIM1 ( $\circ$ ), FIM2 ( $\triangle$ ), RIM1 ( $+$ ), RIM2 ( $\times$ ), and URIM1 ( $\diamond$ ).

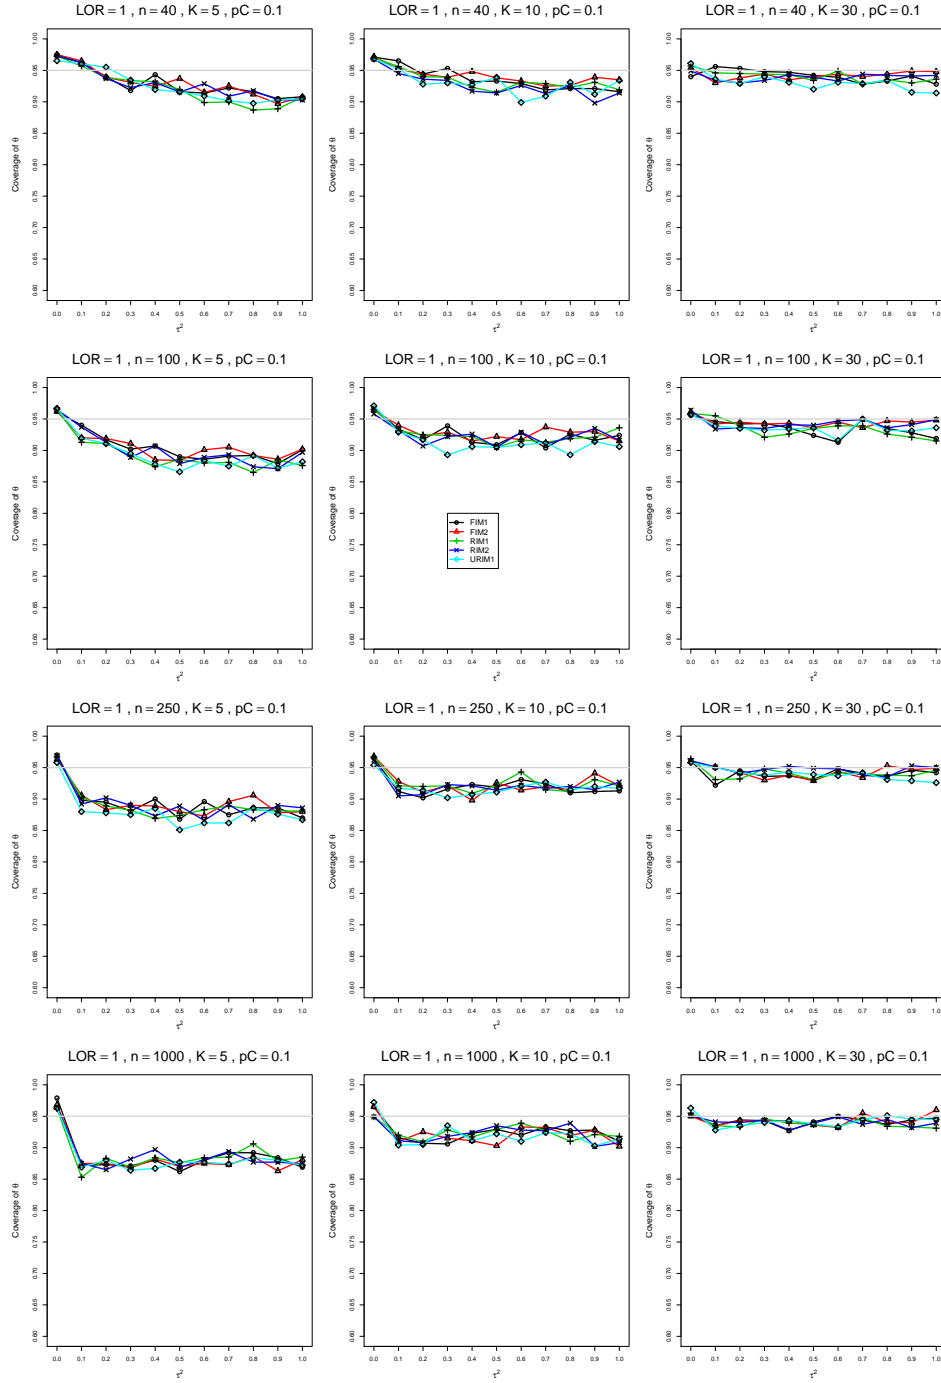

Figure A3.3.15: Coverage of the Mandel-Paule confidence interval for  $\theta = 1$ ,  $p_C = 0.1$ ,  $\sigma^2 = 0.4$ , constant sample sizes  $n = 40, 100, 250, 1000$ . The data-generation mechanisms are FIM1 ( $\circ$ ), FIM2 ( $\triangle$ ), RIM1 ( $+$ ), RIM2 ( $\times$ ), and URIM1 ( $\diamond$ ).

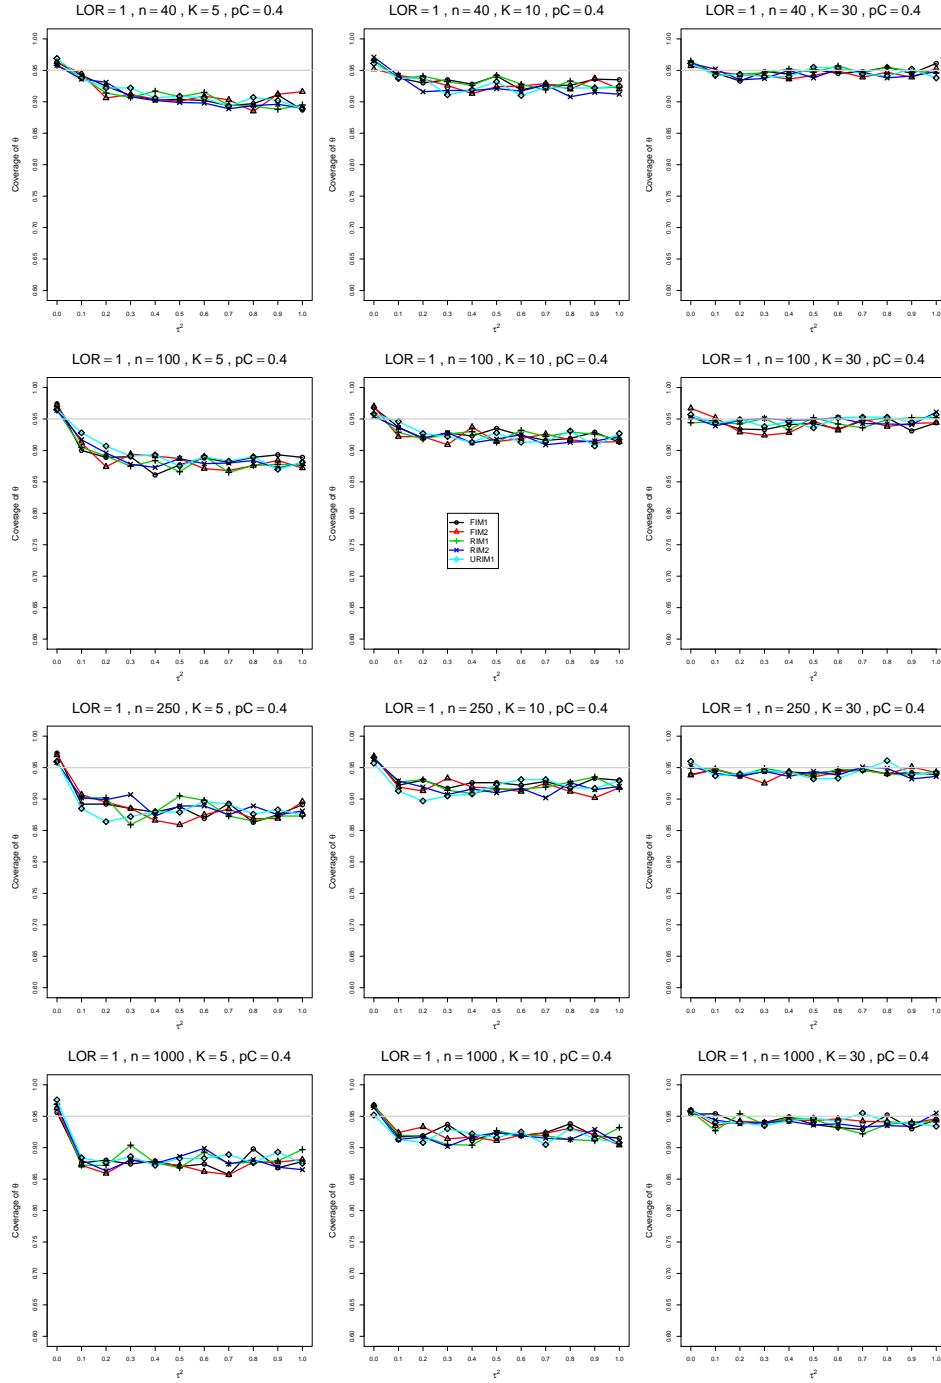

Figure A3.3.16: Coverage of the Mandel-Paule confidence interval for  $\theta = 1$ ,  $p_C = 0.4$ ,  $\sigma^2 = 0.4$ , constant sample sizes  $n = 40, 100, 250, 1000$ . The data-generation mechanisms are FIM1 ( $\circ$ ), FIM2 ( $\triangle$ ), RIM1 ( $+$ ), RIM2 ( $\times$ ), and URIM1 ( $\diamond$ ).

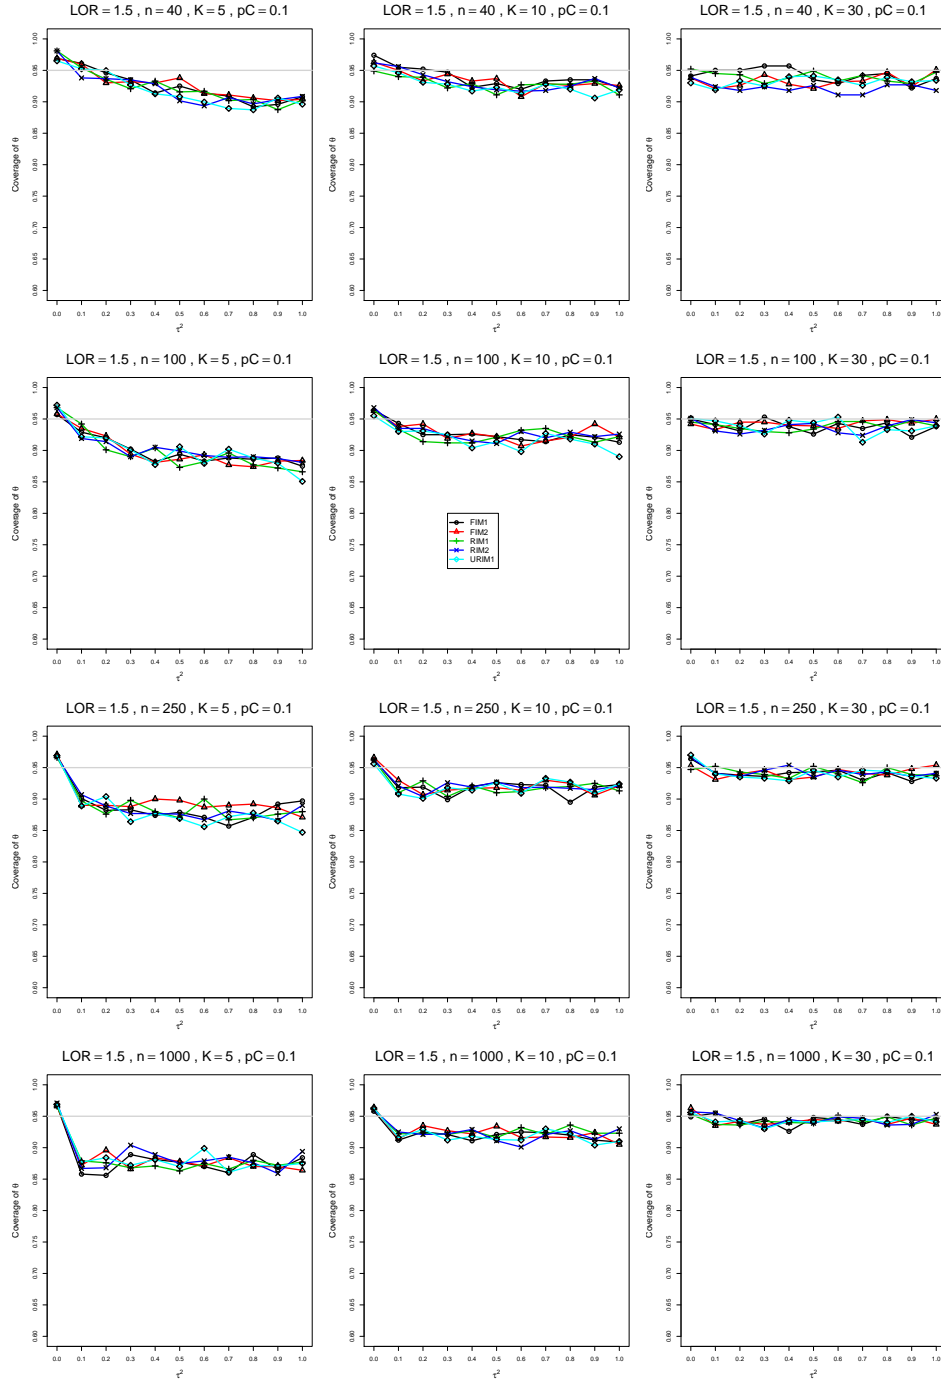

Figure A3.3.17: Coverage of the Mandel-Paule confidence interval for  $\theta = 1.5$ ,  $p_C = 0.1$ ,  $\sigma^2 = 0.4$ , constant sample sizes  $n = 40, 100, 250, 1000$ . The data-generation mechanisms are FIM1 ( $\circ$ ), FIM2 ( $\triangle$ ), RIM1 (+), RIM2 ( $\times$ ), and URIM1 ( $\diamond$ ).

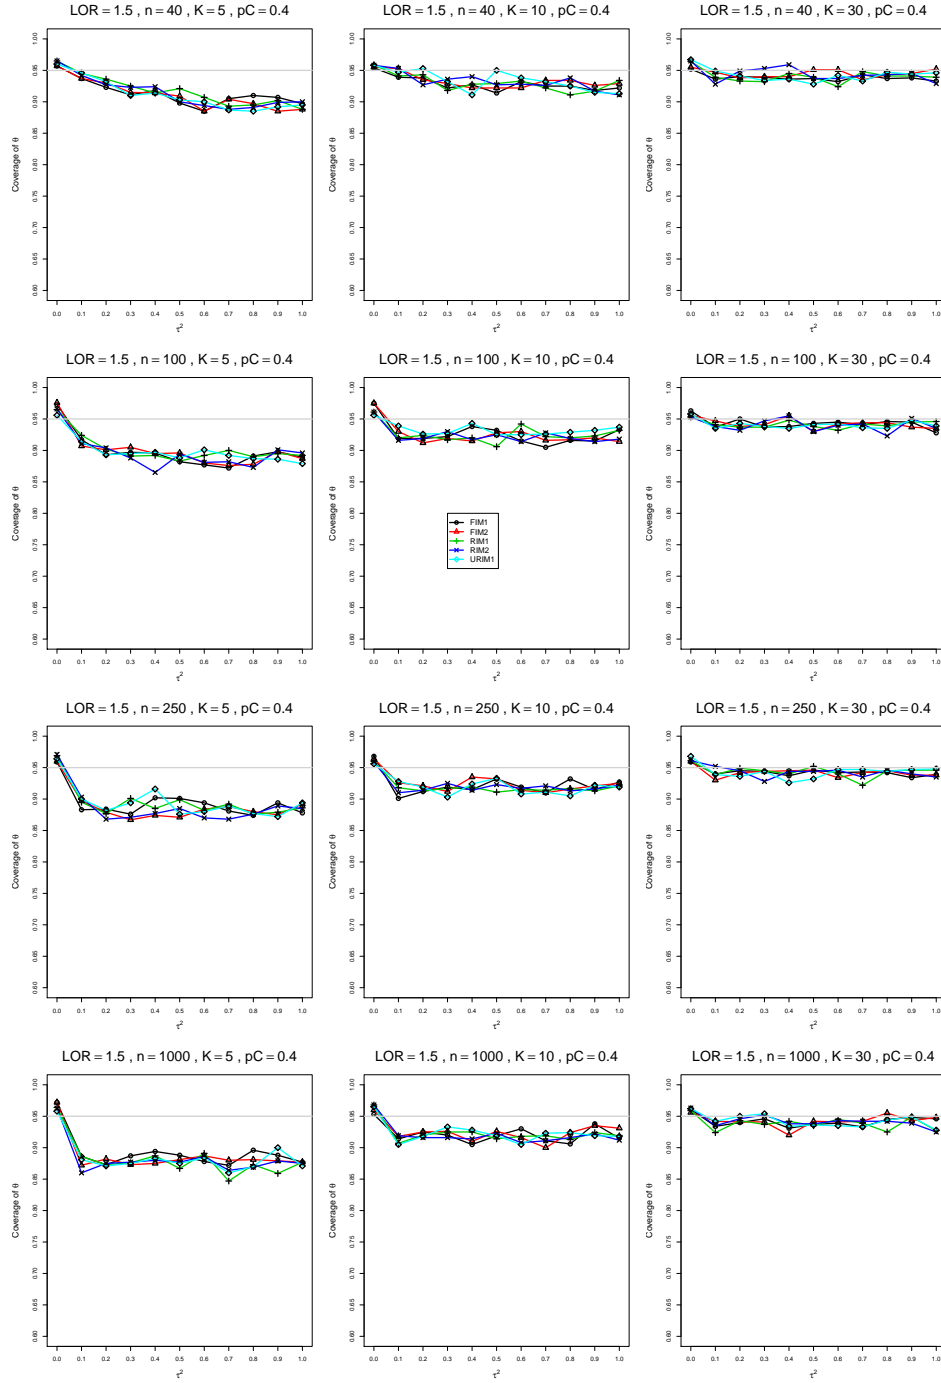

Figure A3.3.18: Coverage of the Mandel-Paule confidence interval for  $\theta = 1.5$ ,  $p_C = 0.4$ ,  $\sigma^2 = 0.4$ , constant sample sizes  $n = 40, 100, 250, 1000$ . The data-generation mechanisms are FIM1 ( $\circ$ ), FIM2 ( $\triangle$ ), RIM1 (+), RIM2 ( $\times$ ), and URIM1 ( $\diamond$ ).

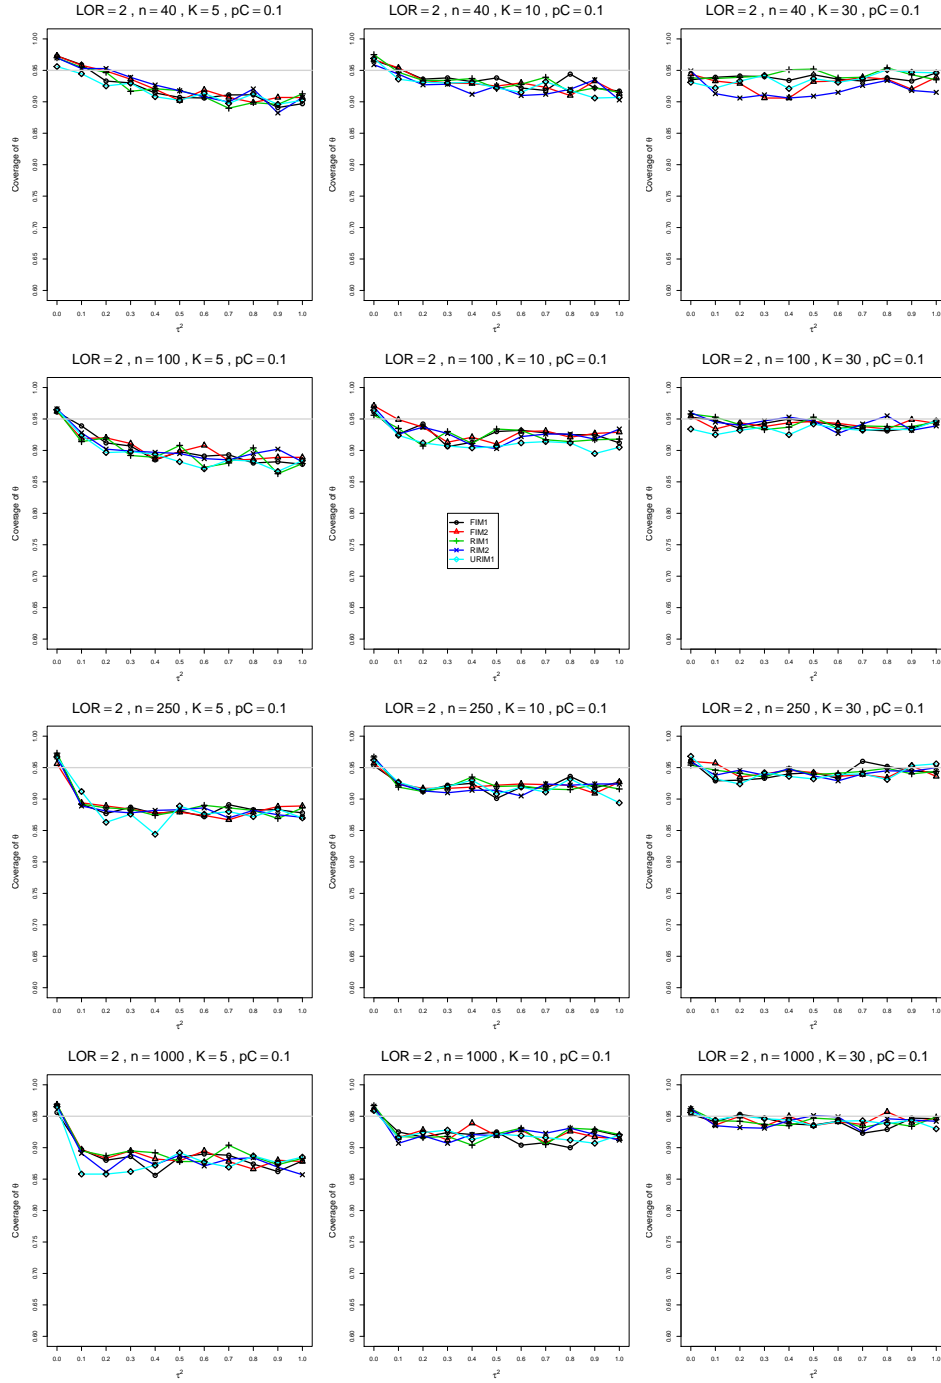

Figure A3.3.19: Coverage of the Mandel-Paulle confidence interval for  $\theta = 2$ ,  $p_C = 0.1$ ,  $\sigma^2 = 0.4$ , constant sample sizes  $n = 40, 100, 250, 1000$ . The data-generation mechanisms are FIM1 ( $\circ$ ), FIM2 ( $\triangle$ ), RIM1 ( $+$ ), RIM2 ( $\times$ ), and URIM1 ( $\diamond$ ).

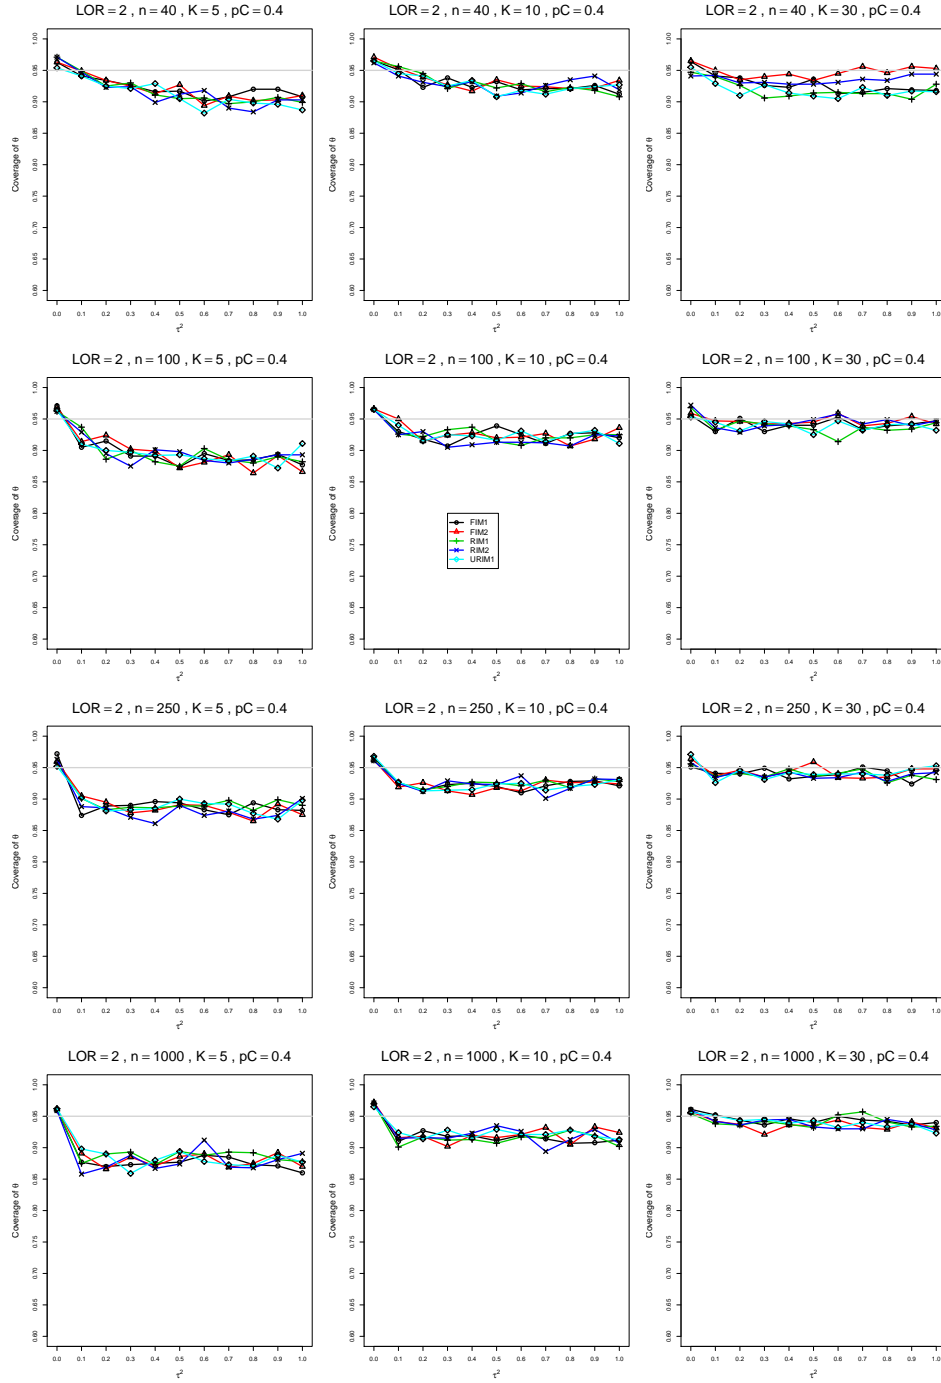

Figure A3.3.20: Coverage of the Mandel-Paule confidence interval for  $\theta = 2$ ,  $p_C = 0.4$ ,  $\sigma^2 = 0.4$ , constant sample sizes  $n = 40, 100, 250, 1000$ . The data-generation mechanisms are FIM1 ( $\circ$ ), FIM2 ( $\triangle$ ), RIM1 ( $+$ ), RIM2 ( $\times$ ), and URIM1 ( $\diamond$ ).



### A3.4 Coverage of $\hat{\theta}_{KD}$

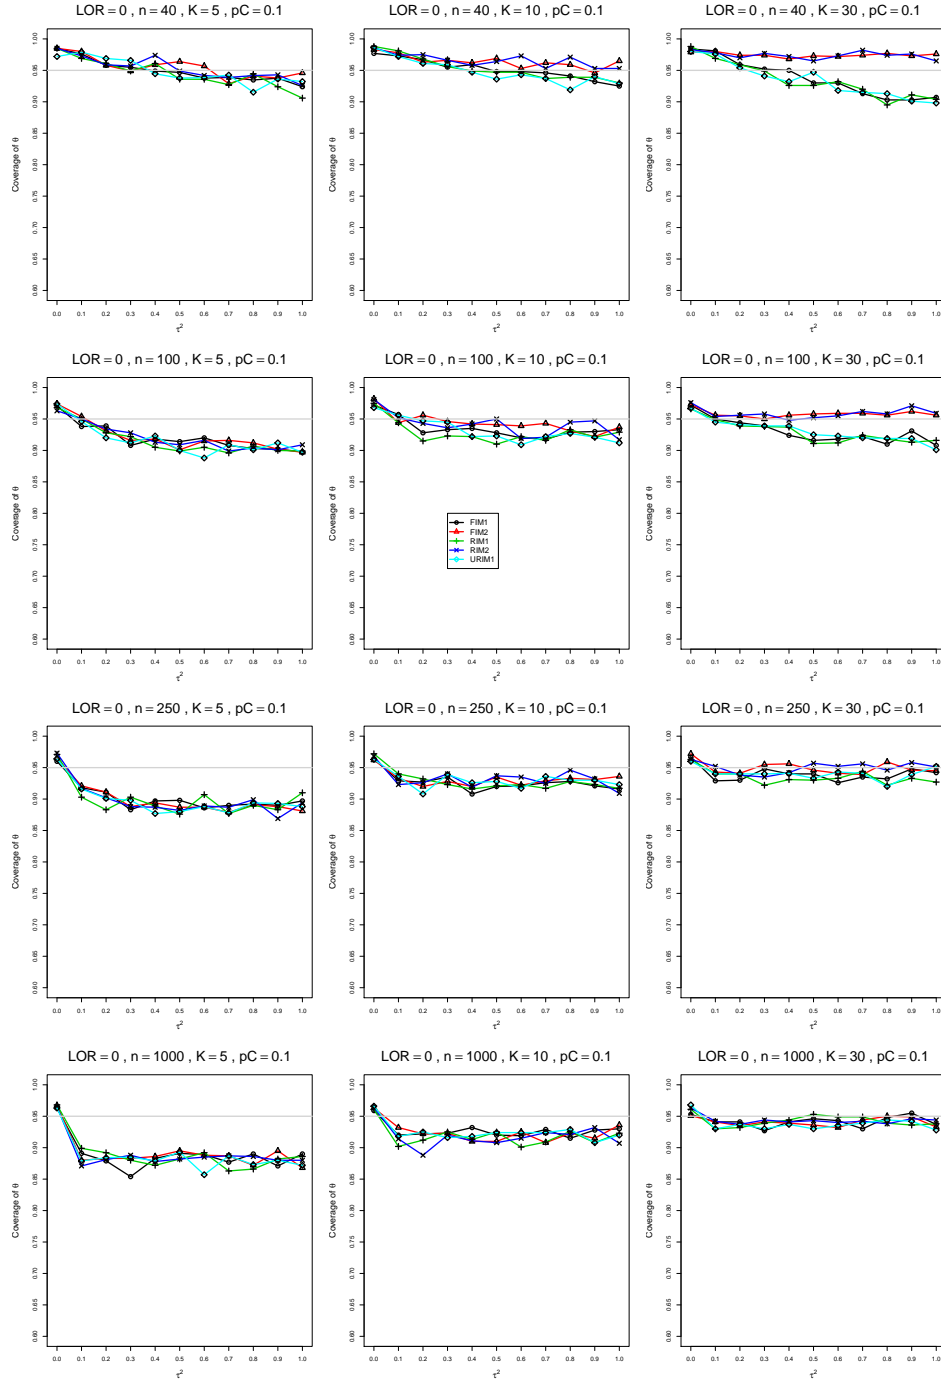

Figure A3.4.1: Coverage of the Kulinskaya-Dollinger confidence interval for  $\theta = 0$ ,  $p_C = 0.1$ ,  $\sigma^2 = 0.1$ , constant sample sizes  $n = 40, 100, 250, 1000$ . The data-generation mechanisms are FIM1 ( $\circ$ ), FIM2 ( $\triangle$ ), RIM1 ( $+$ ), RIM2 ( $\times$ ), and URIM1 ( $\diamond$ ).

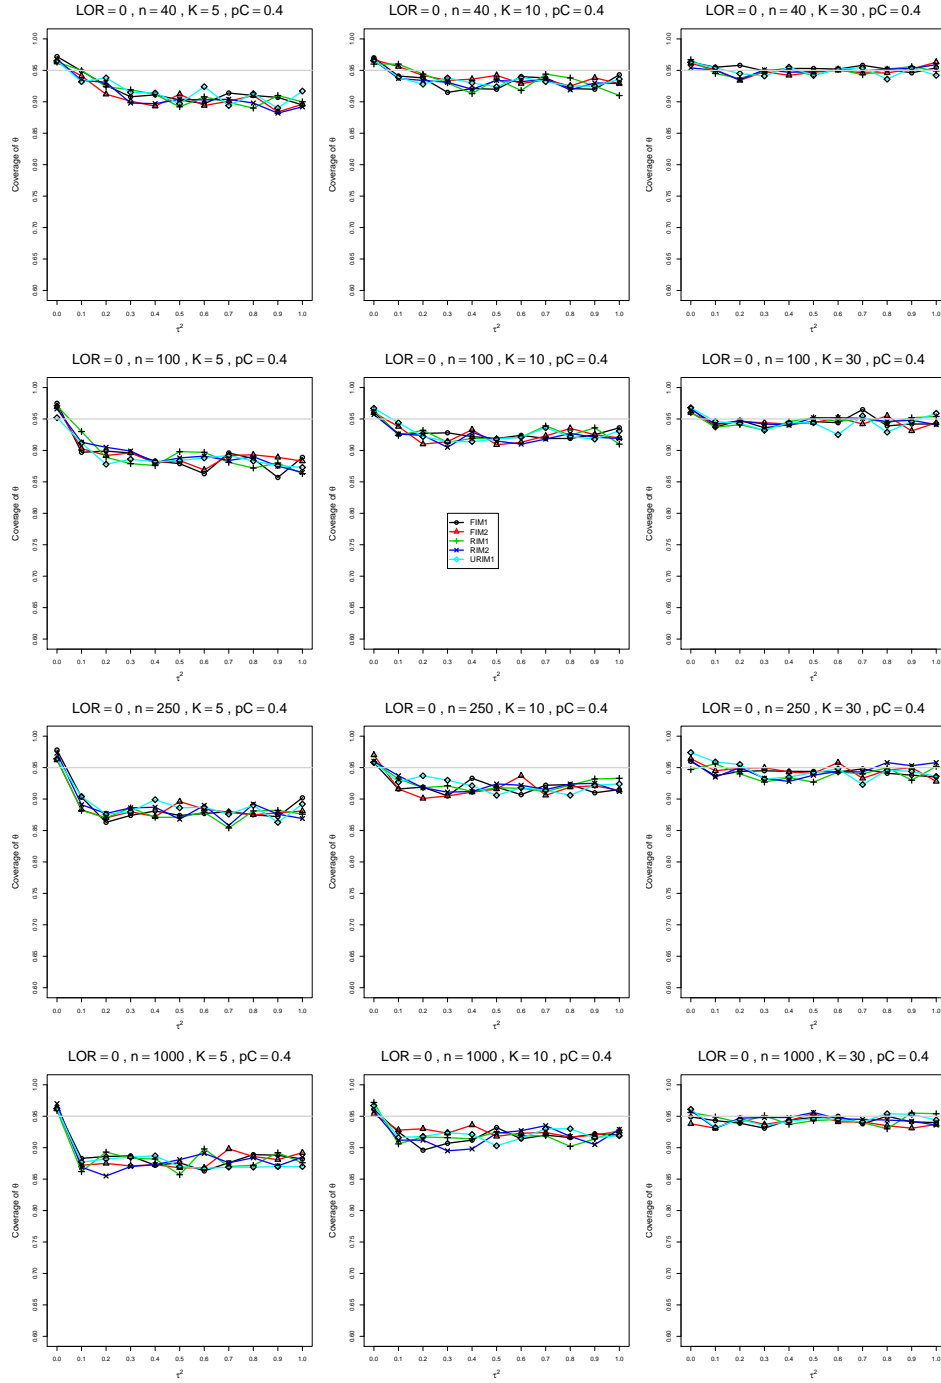

Figure A3.4.2: Coverage of the Kulinskaya-Dollinger confidence interval for  $\theta = 0$ ,  $p_C = 0.4$ ,  $\sigma^2 = 0.1$ , constant sample sizes  $n = 40, 100, 250, 1000$ . The data-generation mechanisms are FIM1 ( $\circ$ ), FIM2 ( $\triangle$ ), RIM1 ( $+$ ), RIM2 ( $\times$ ), and URIM1 ( $\diamond$ ).

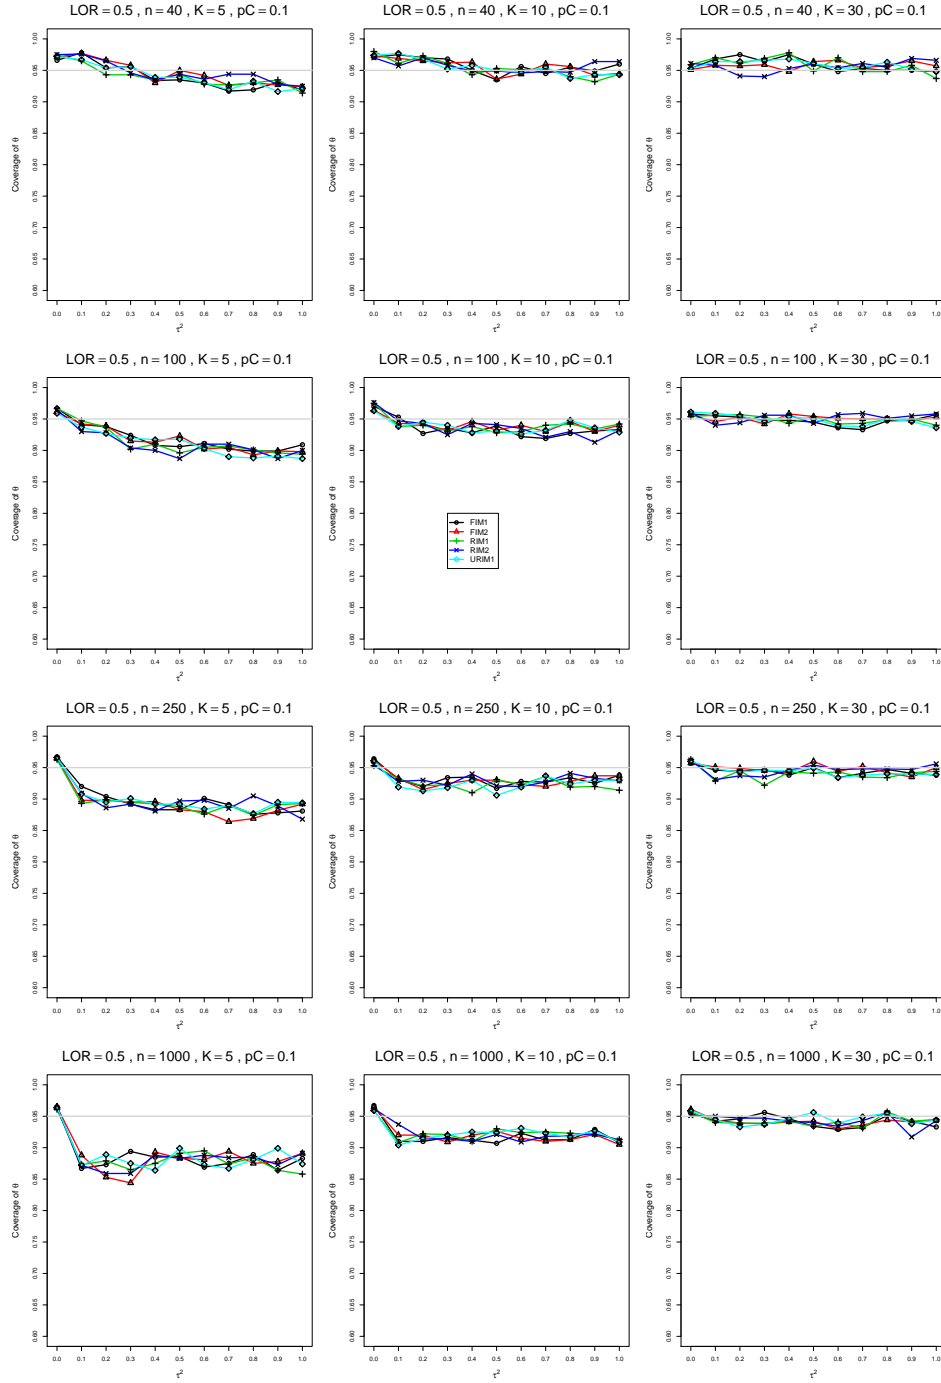

Figure A3.4.3: Coverage of the Kulinskaya-Dollinger confidence interval for  $\theta = 0.5$ ,  $p_C = 0.1$ ,  $\sigma^2 = 0.1$ , constant sample sizes  $n = 40, 100, 250, 1000$ . The data-generation mechanisms are FIM1 ( $\circ$ ), FIM2 ( $\triangle$ ), RIM1 (+), RIM2 ( $\times$ ), and URIM1 ( $\diamond$ ).

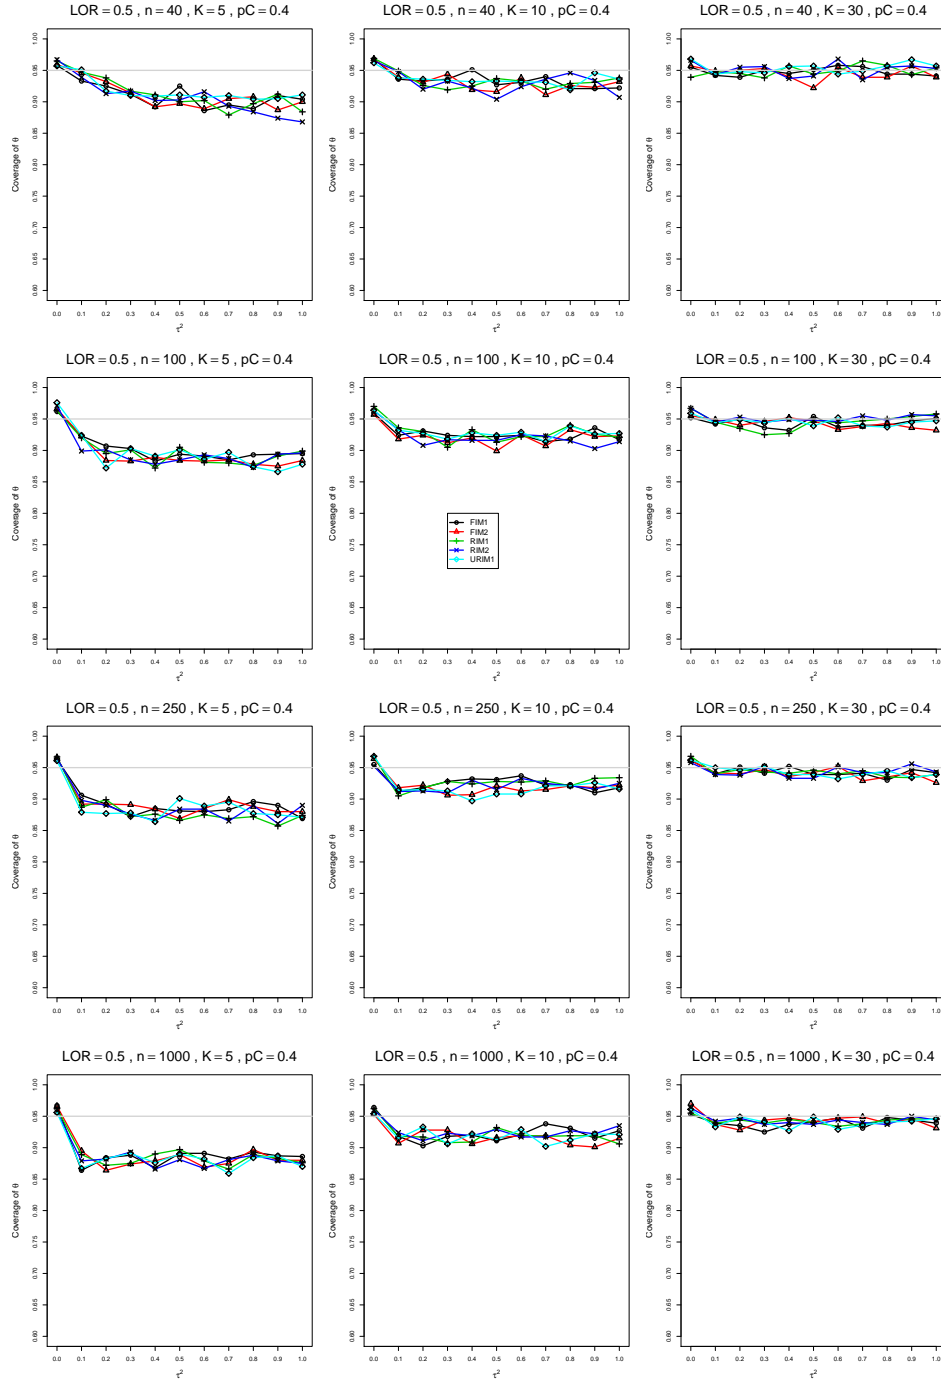

Figure A3.4.4: Coverage of the Kulinskaya-Dollinger confidence interval for  $\theta = 0.5$ ,  $p_C = 0.4$ ,  $\sigma^2 = 0.1$ , constant sample sizes  $n = 40, 100, 250, 1000$ . The data-generation mechanisms are FIM1 (o), FIM2 ( $\triangle$ ), RIM1 (+), RIM2 ( $\times$ ), and URIM1 ( $\diamond$ ).

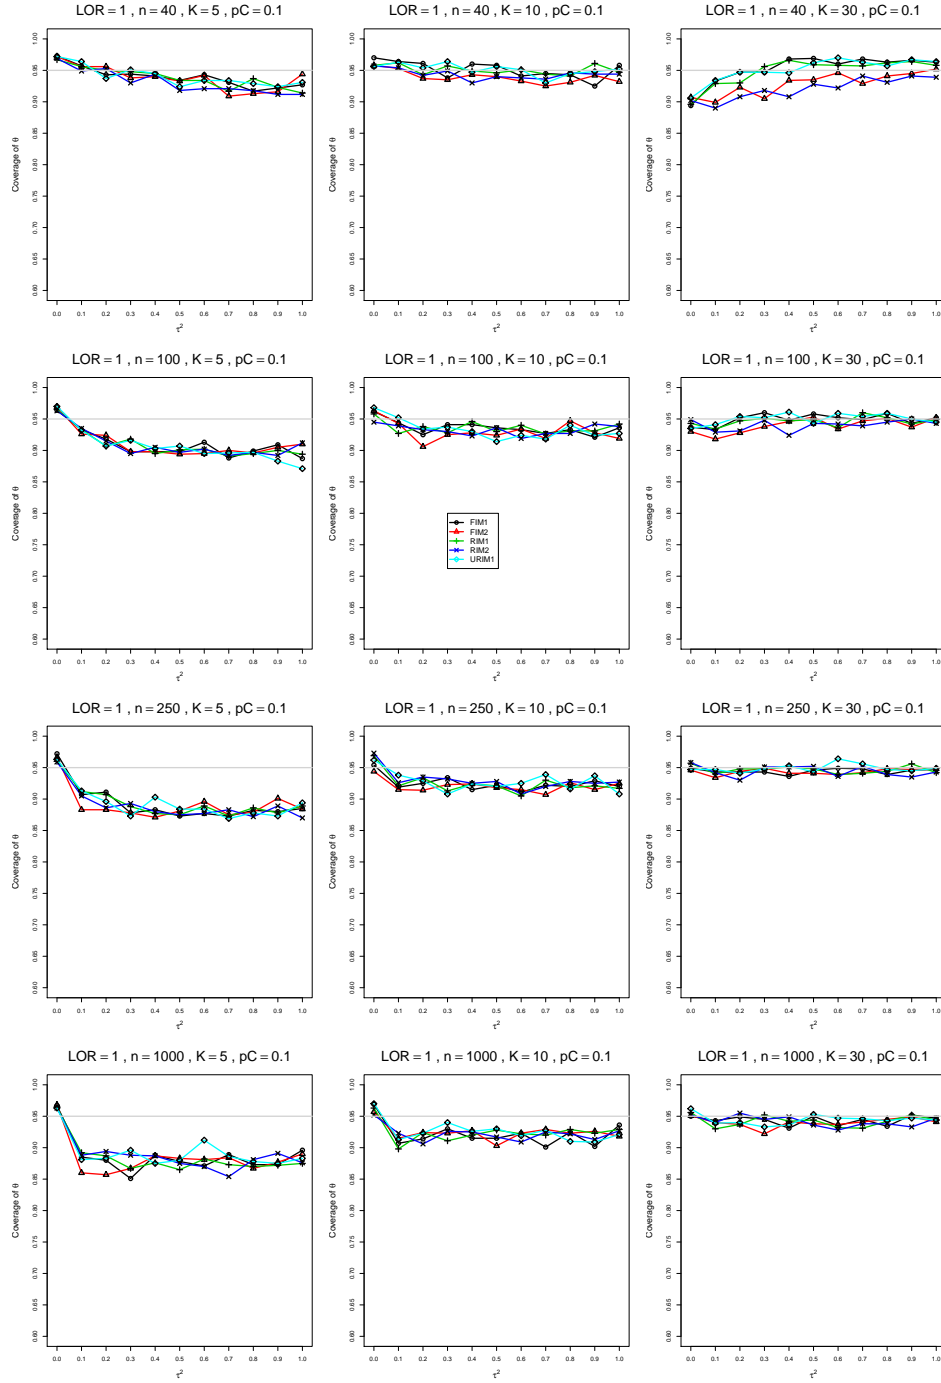

Figure A3.4.5: Coverage of the Kulinskaya-Dollinger confidence interval for  $\theta = 1$ ,  $p_C = 0.1$ ,  $\sigma^2 = 0.1$ , constant sample sizes  $n = 40, 100, 250, 1000$ . The data-generation mechanisms are FIM1 ( $\circ$ ), FIM2 ( $\triangle$ ), RIM1 ( $+$ ), RIM2 ( $\times$ ), and URIM1 ( $\diamond$ ).

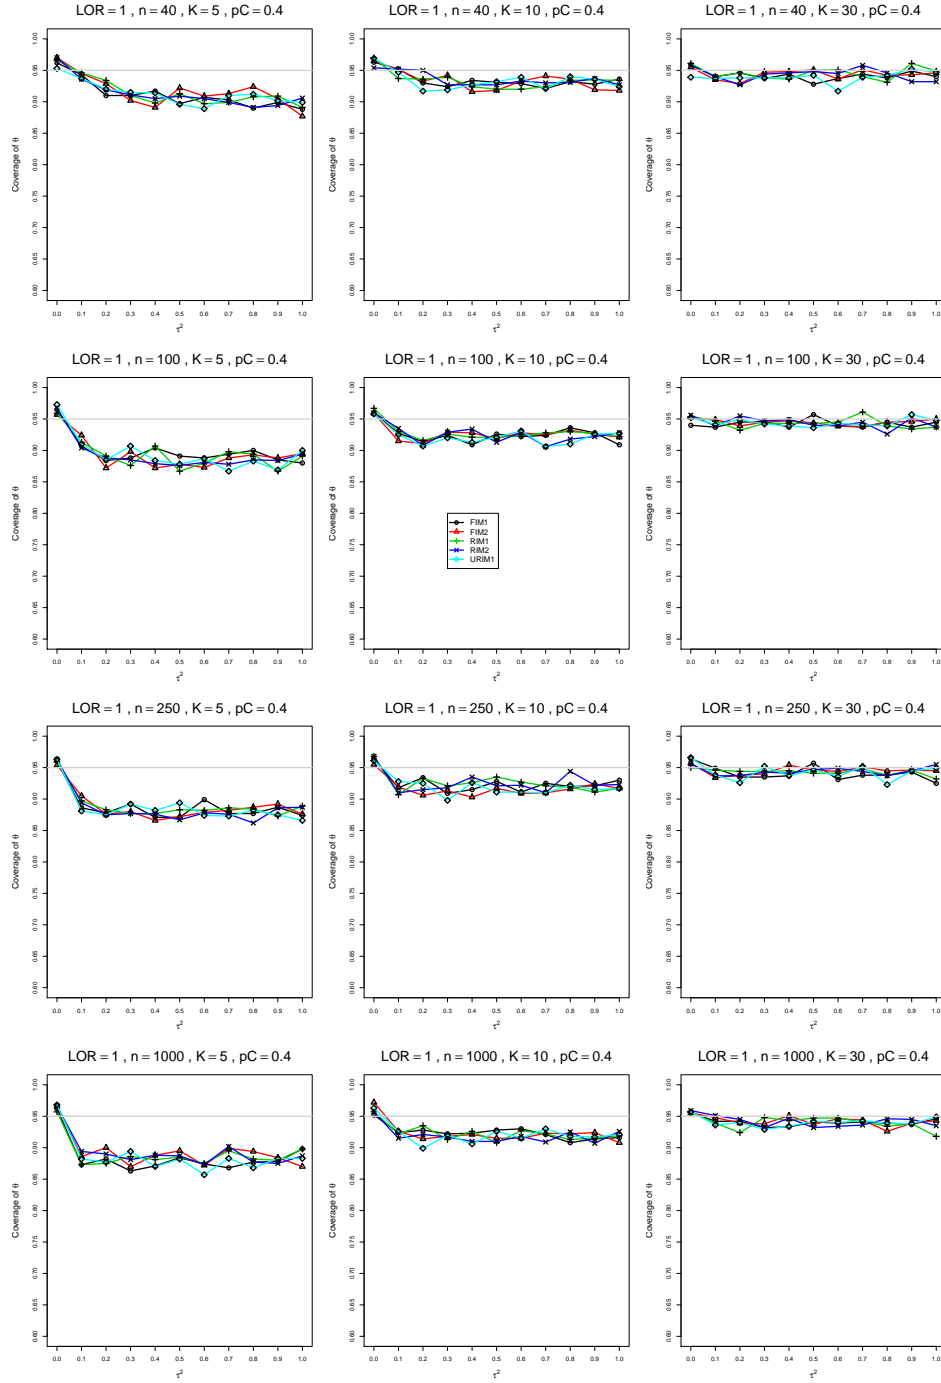

Figure A3.4.6: Coverage of the Kulinskaya-Dollinger confidence interval for  $\theta = 1$ ,  $p_C = 0.4$ ,  $\sigma^2 = 0.1$ , constant sample sizes  $n = 40, 100, 250, 1000$ . The data-generation mechanisms are FIM1 ( $\circ$ ), FIM2 ( $\triangle$ ), RIM1 ( $+$ ), RIM2 ( $\times$ ), and URIM1 ( $\diamond$ ).

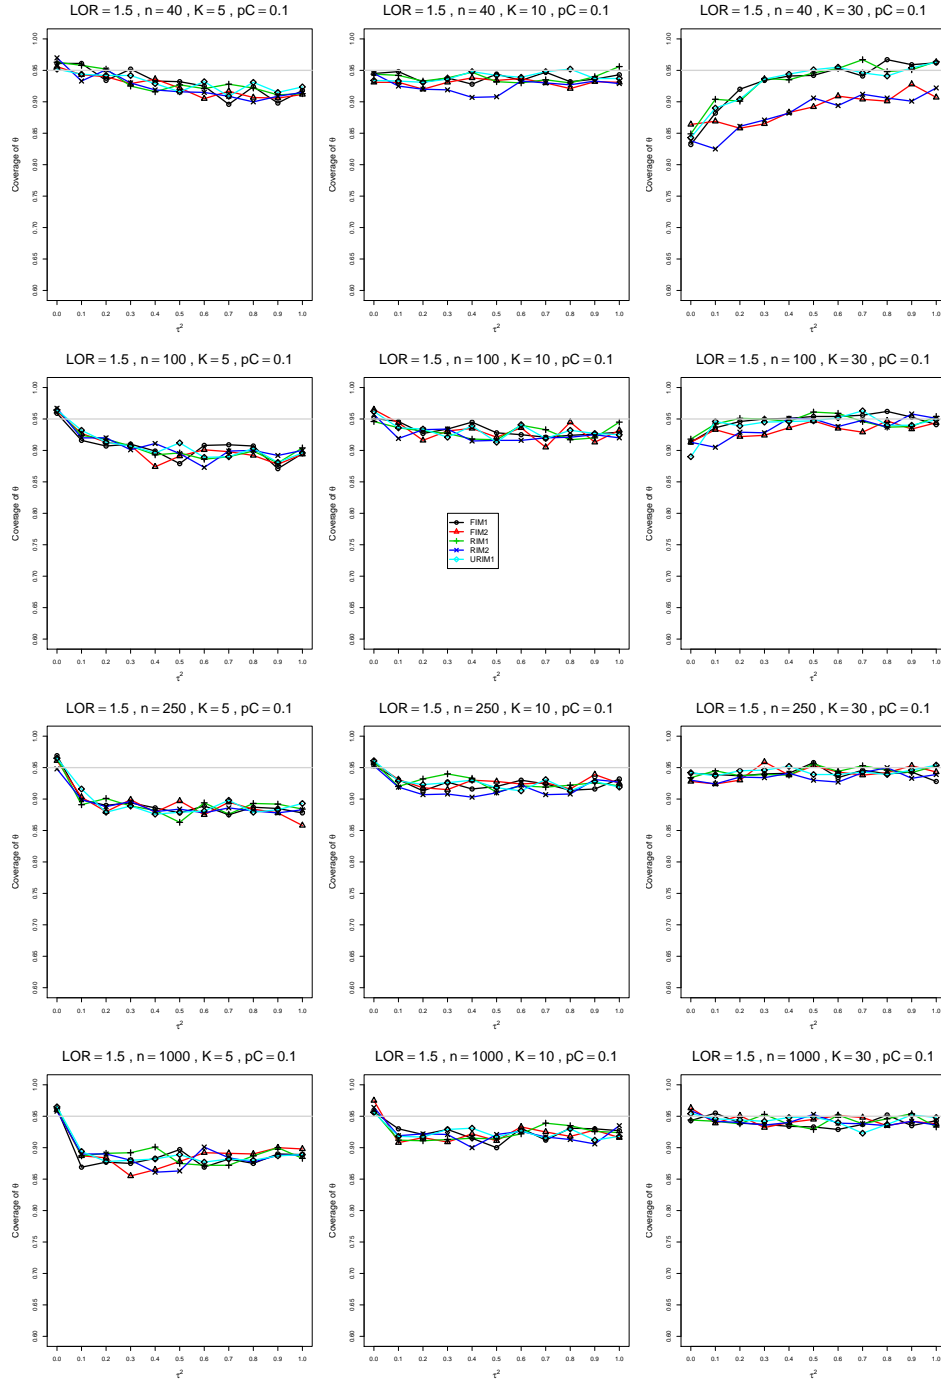

Figure A3.4.7: Coverage of the Kulinskaya-Dollinger confidence interval for  $\theta = 1.5$ ,  $p_C = 0.1$ ,  $\sigma^2 = 0.1$ , constant sample sizes  $n = 40, 100, 250, 1000$ . The data-generation mechanisms are FIM1 ( $\circ$ ), FIM2 ( $\triangle$ ), RIM1 (+), RIM2 ( $\times$ ), and URIM1 ( $\diamond$ ).



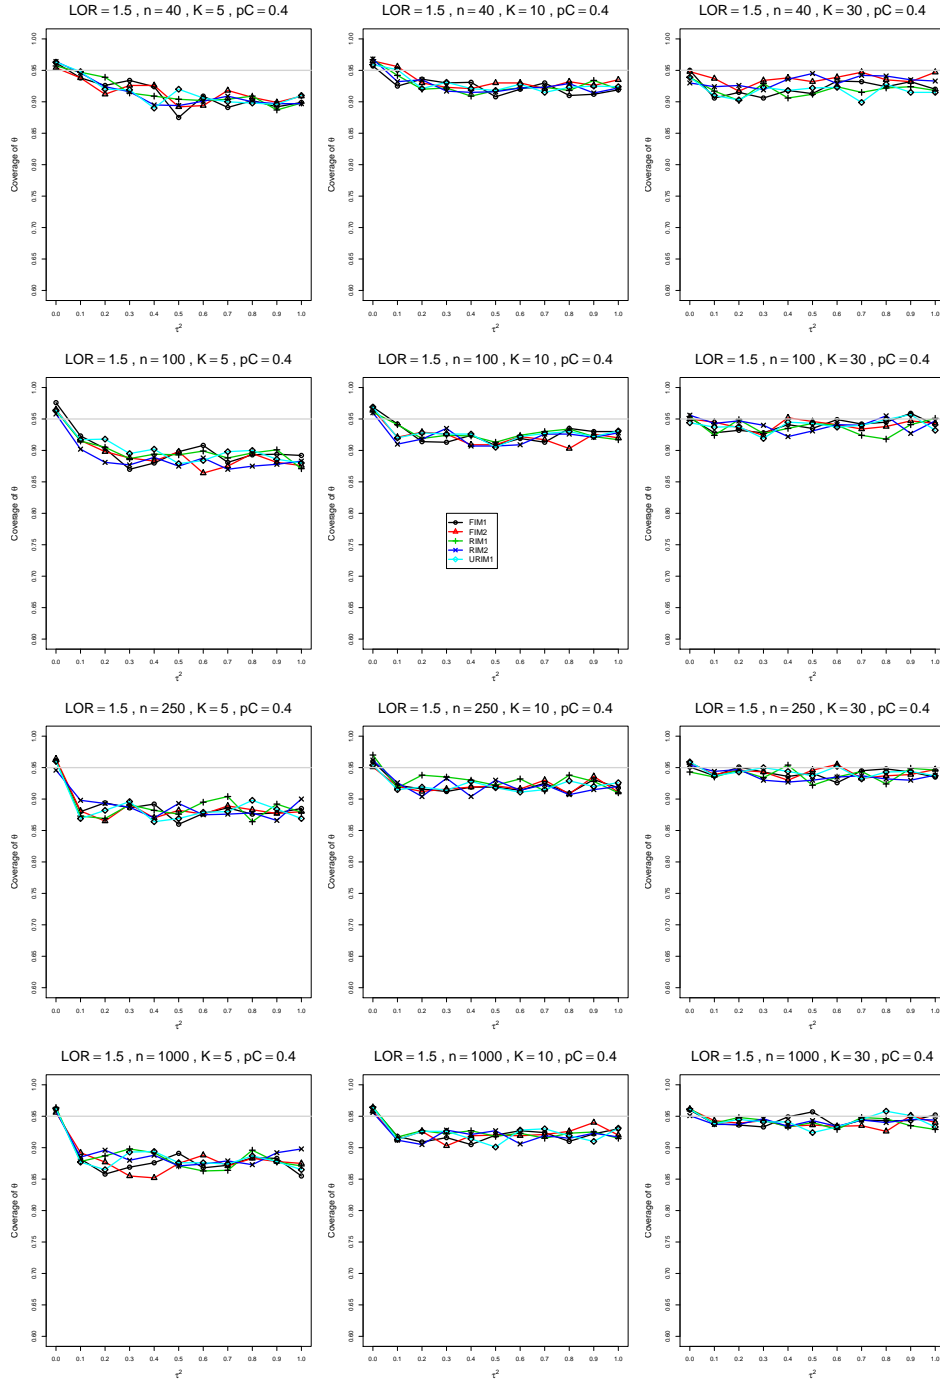

Figure A3.4.8: Coverage of the Kulinskaya-Dollinger confidence interval for  $\theta = 1.5$ ,  $p_C = 0.4$ ,  $\sigma^2 = 0.1$ , constant sample sizes  $n = 40, 100, 250, 1000$ . The data-generation mechanisms are FIM1 (o), FIM2 ( $\triangle$ ), RIM1 (+), RIM2 ( $\times$ ), and URIM1 ( $\diamond$ ).

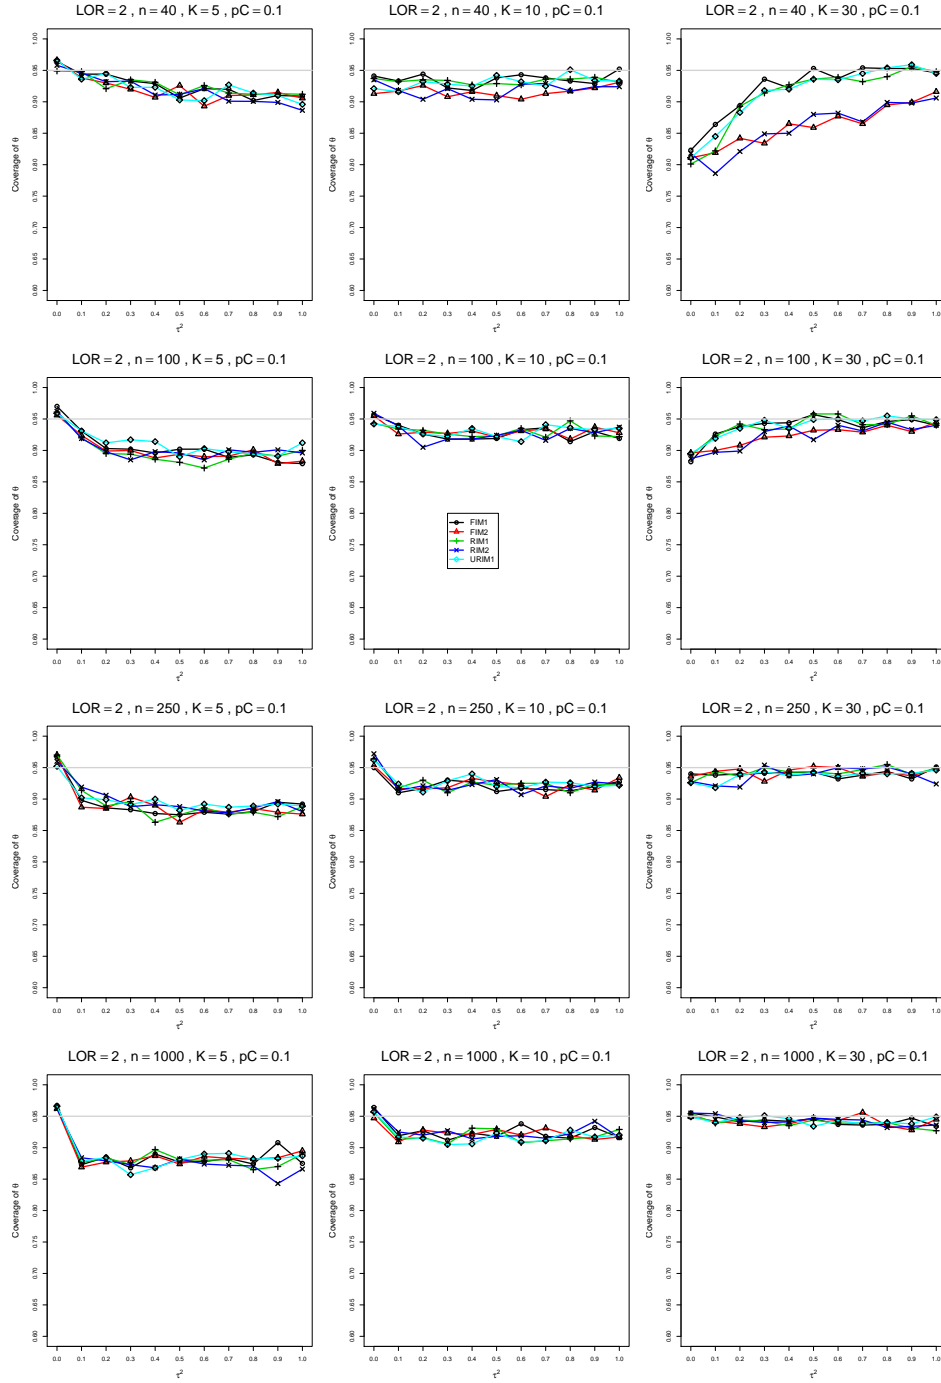

Figure A3.4.9: Coverage of the Kulinskaya-Dollinger confidence interval for  $\theta = 2$ ,  $p_C = 0.1$ ,  $\sigma^2 = 0.1$ , constant sample sizes  $n = 40, 100, 250, 1000$ . The data-generation mechanisms are FIM1 ( $\circ$ ), FIM2 ( $\triangle$ ), RIM1 ( $+$ ), RIM2 ( $\times$ ), and URIM1 ( $\diamond$ ).

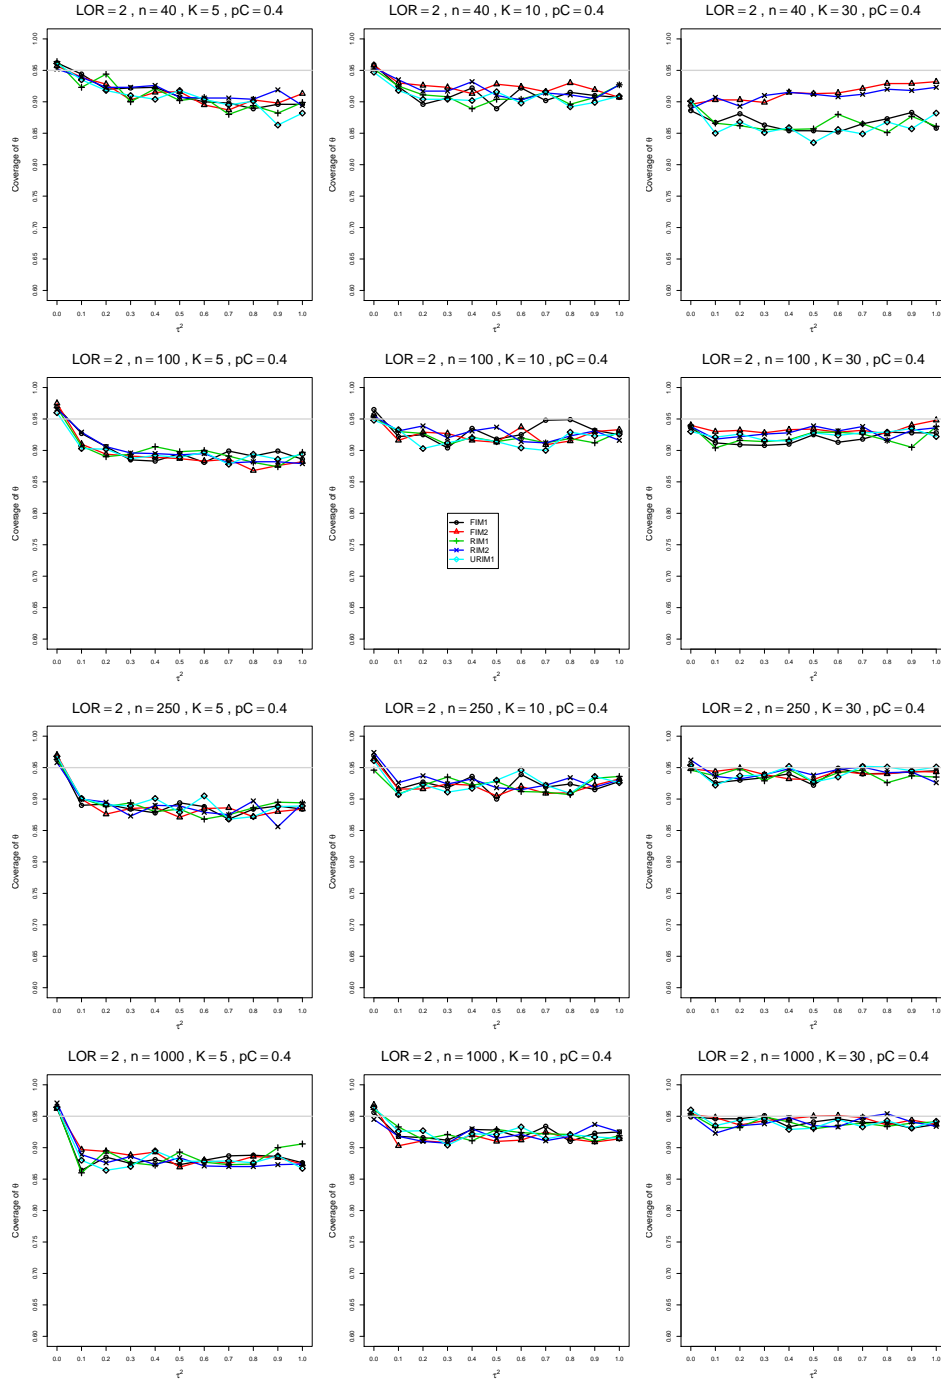

Figure A3.4.10: Coverage of the Kulinskaya-Dollinger confidence interval for  $\theta = 2$ ,  $p_C = 0.4$ ,  $\sigma^2 = 0.1$ , constant sample sizes  $n = 40, 100, 250, 1000$ . The data-generation mechanisms are FIM1 ( $\circ$ ), FIM2 ( $\triangle$ ), RIM1 ( $+$ ), RIM2 ( $\times$ ), and URIM1 ( $\diamond$ ).

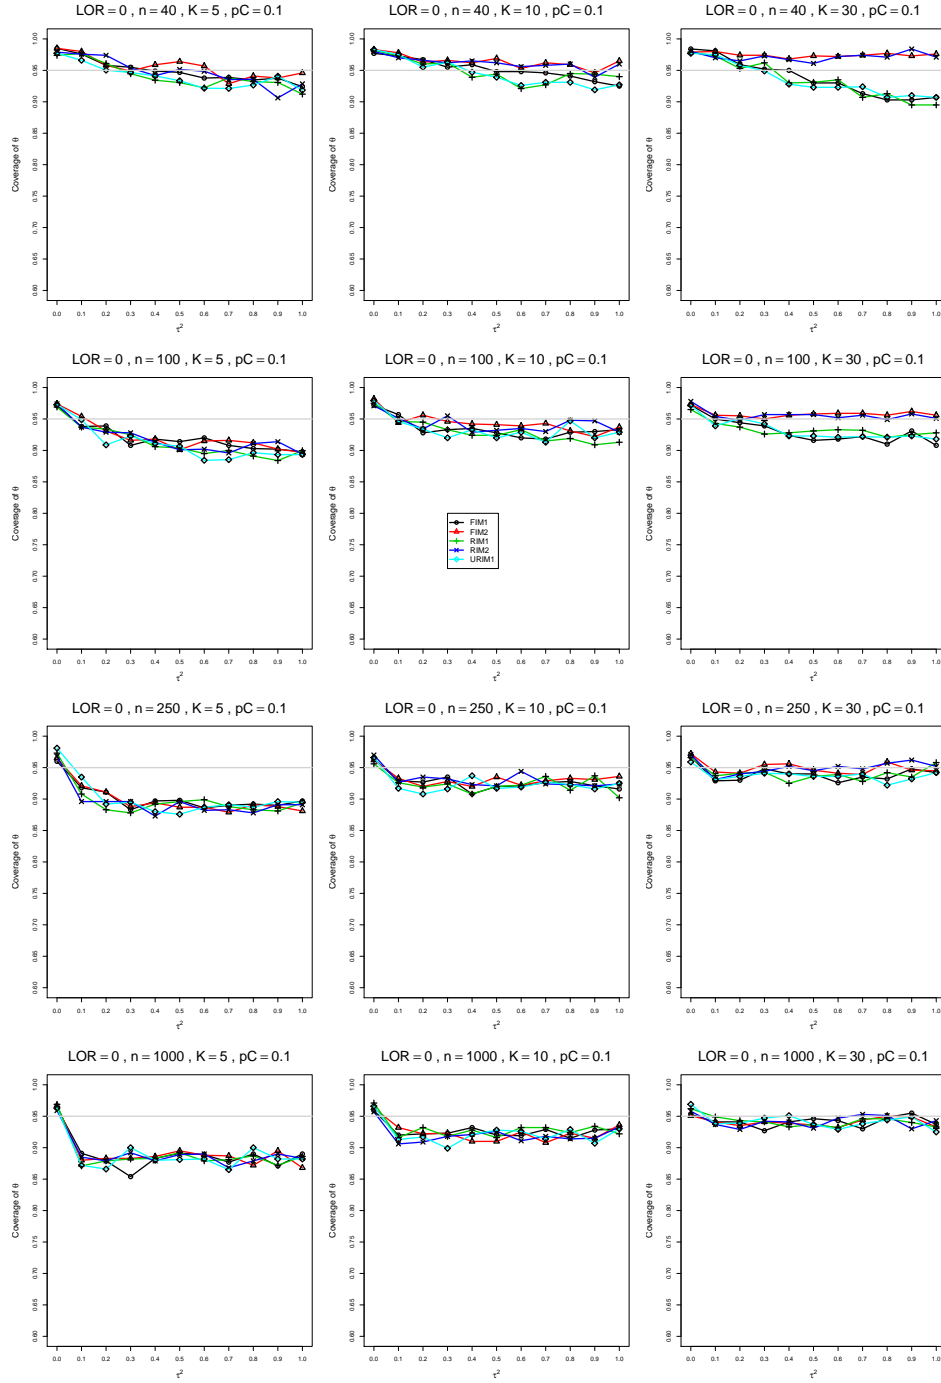

Figure A3.4.11: Coverage of the Kulinskaya-Dollinger confidence interval for  $\theta = 0$ ,  $p_C = 0.1$ ,  $\sigma^2 = 0.4$ , constant sample sizes  $n = 40, 100, 250, 1000$ . The data-generation mechanisms are FIM1 ( $\circ$ ), FIM2 ( $\triangle$ ), RIM1 ( $+$ ), RIM2 ( $\times$ ), and URIM1 ( $\diamond$ ).

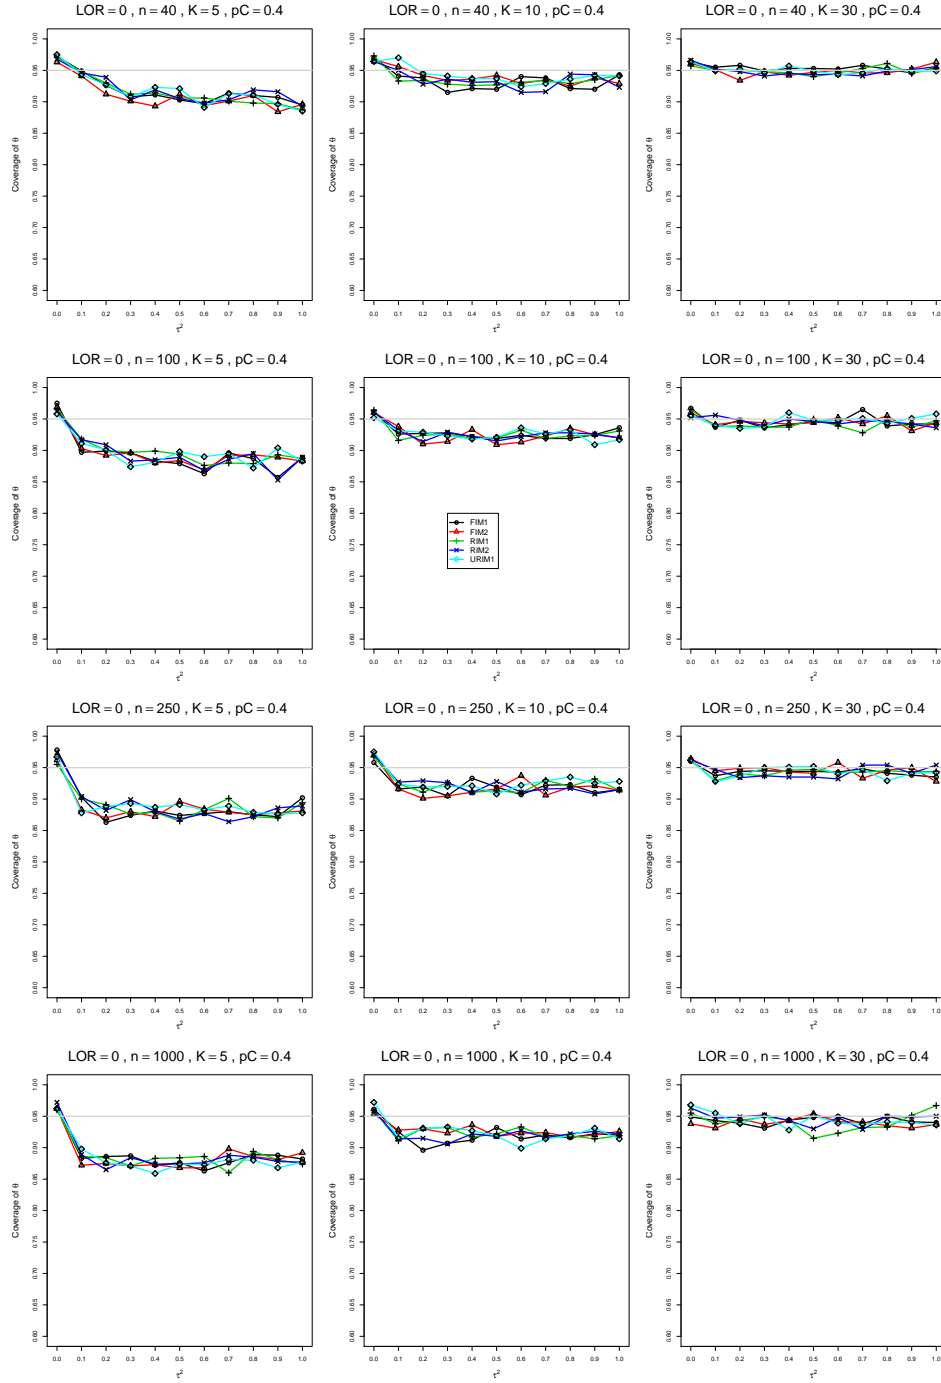

Figure A3.4.12: Coverage of the Kulinskaya-Dollinger confidence interval for  $\theta = 0$ ,  $p_C = 0.4$ ,  $\sigma^2 = 0.4$ , constant sample sizes  $n = 40, 100, 250, 1000$ . The data-generation mechanisms are FIM1 ( $\circ$ ), FIM2 ( $\triangle$ ), RIM1 ( $+$ ), RIM2 ( $\times$ ), and URIM1 ( $\diamond$ ).

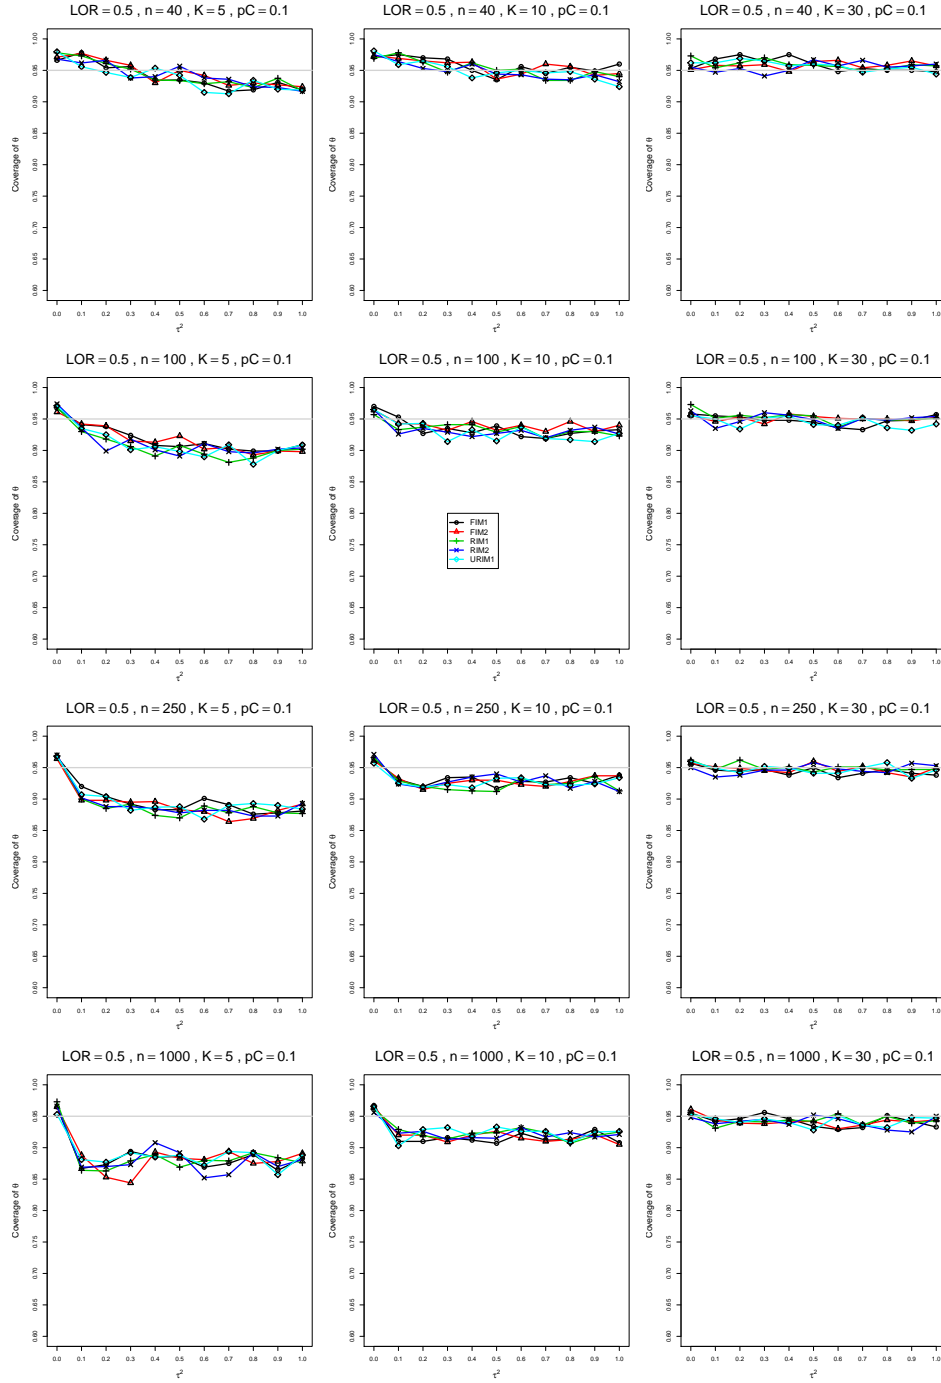

Figure A3.4.13: Coverage of the Kulinskaya-Dollinger confidence interval for  $\theta = 0.5$ ,  $p_C = 0.1$ ,  $\sigma^2 = 0.4$ , constant sample sizes  $n = 40, 100, 250, 1000$ . The data-generation mechanisms are FIM1 ( $\circ$ ), FIM2 ( $\triangle$ ), RIM1 (+), RIM2 ( $\times$ ), and URIM1 ( $\diamond$ ).

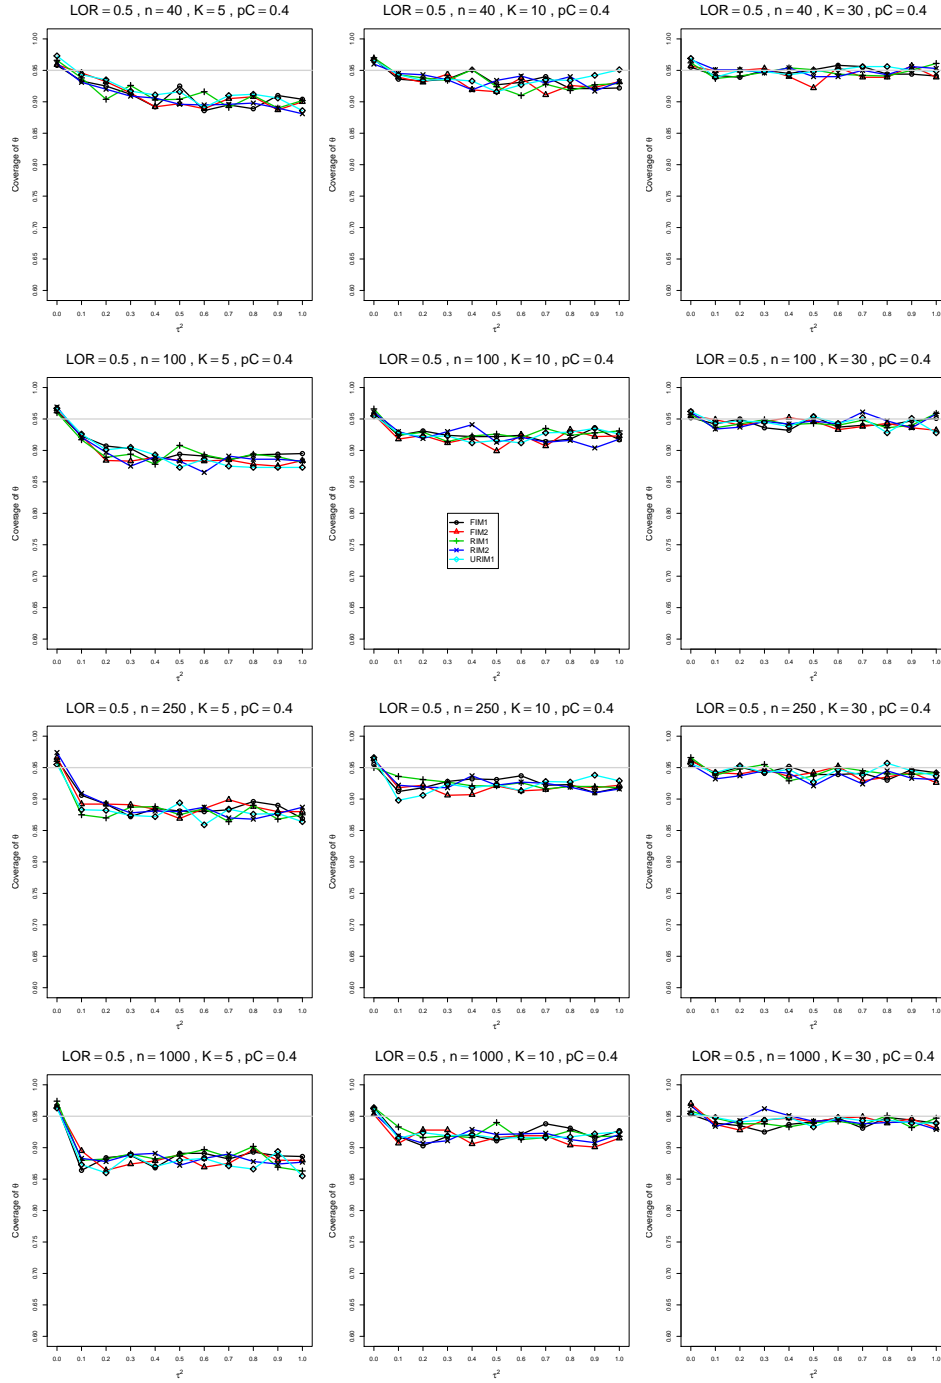

Figure A3.4.14: Coverage of the Kulinskaya-Dollinger confidence interval for  $\theta = 0.5$ ,  $p_C = 0.4$ ,  $\sigma^2 = 0.4$ , constant sample sizes  $n = 40, 100, 250, 1000$ . The data-generation mechanisms are FIM1 ( $\circ$ ), FIM2 ( $\triangle$ ), RIM1 ( $+$ ), RIM2 ( $\times$ ), and URIM1 ( $\diamond$ ).

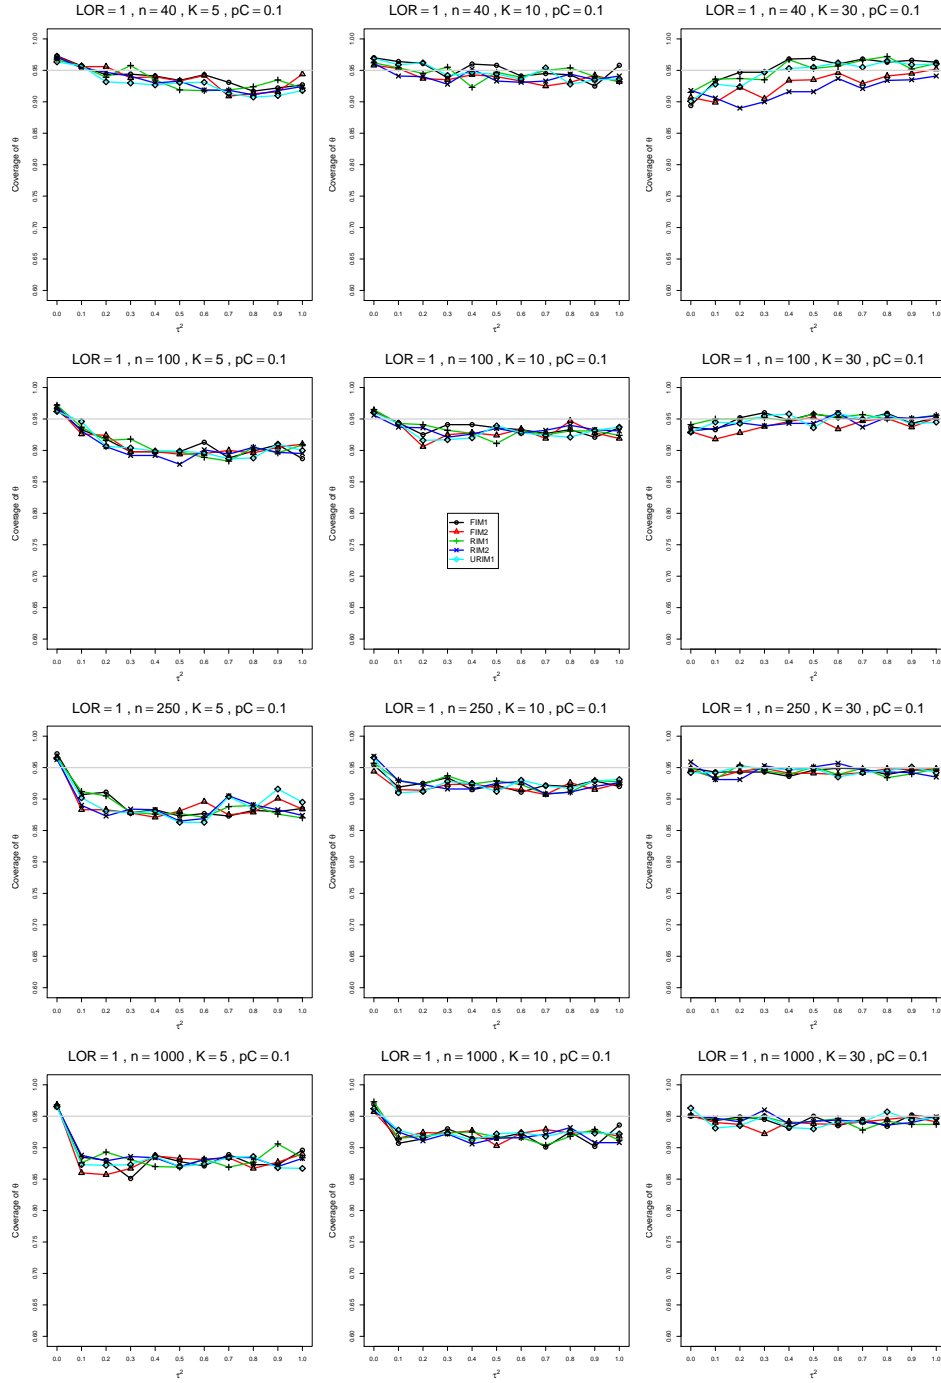

Figure A3.4.15: Coverage of the Kulinskaya-Dollinger confidence interval for  $\theta = 1$ ,  $p_C = 0.1$ ,  $\sigma^2 = 0.4$ , constant sample sizes  $n = 40, 100, 250, 1000$ . The data-generation mechanisms are FIM1 ( $\circ$ ), FIM2 ( $\triangle$ ), RIM1 ( $+$ ), RIM2 ( $\times$ ), and URIM1 ( $\diamond$ ).



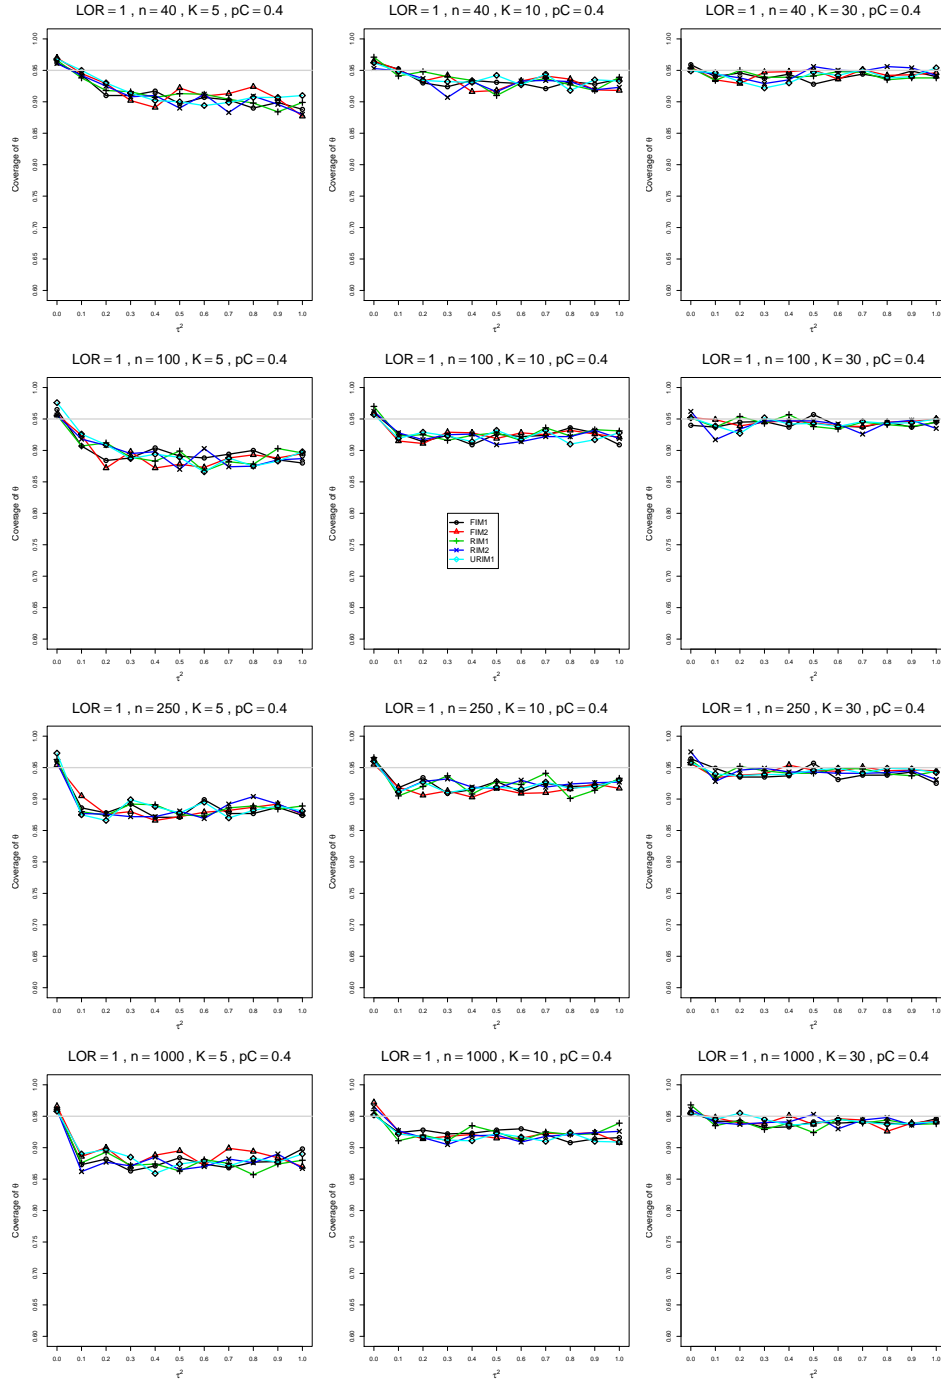

Figure A3.4.16: Coverage of the Kulinskaya-Dollinger confidence interval for  $\theta = 1$ ,  $p_C = 0.4$ ,  $\sigma^2 = 0.4$ , constant sample sizes  $n = 40, 100, 250, 1000$ . The data-generation mechanisms are FIM1 ( $\circ$ ), FIM2 ( $\triangle$ ), RIM1 ( $+$ ), RIM2 ( $\times$ ), and URIM1 ( $\diamond$ ).

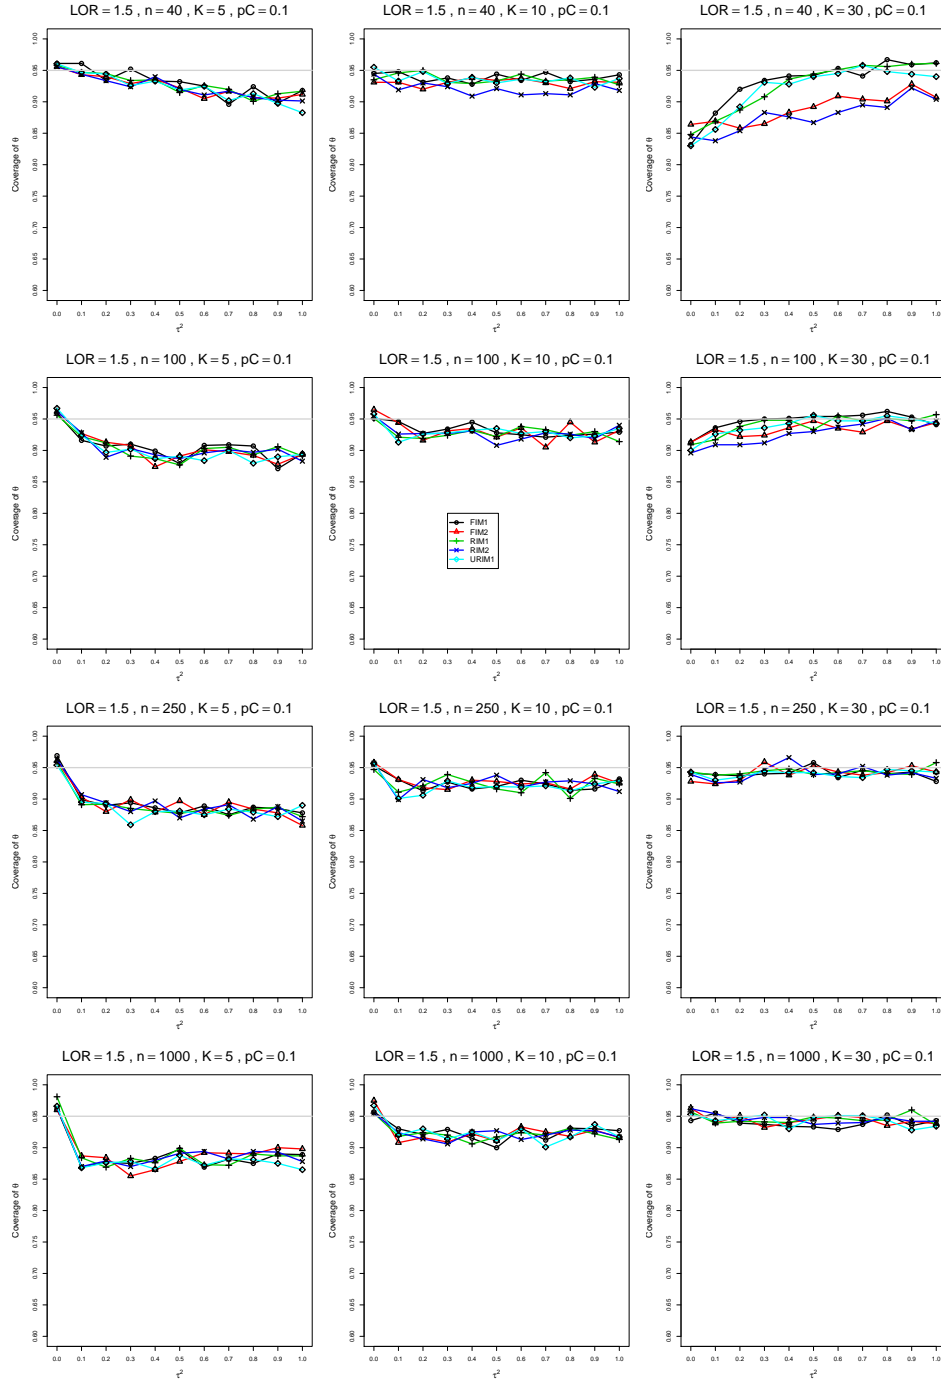

Figure A3.4.17: Coverage of the Kulinskaya-Dollinger confidence interval for  $\theta = 1.5$ ,  $p_C = 0.1$ ,  $\sigma^2 = 0.4$ , constant sample sizes  $n = 40, 100, 250, 1000$ . The data-generation mechanisms are FIM1 ( $\circ$ ), FIM2 ( $\triangle$ ), RIM1 ( $+$ ), RIM2 ( $\times$ ), and URIM1 ( $\diamond$ ).

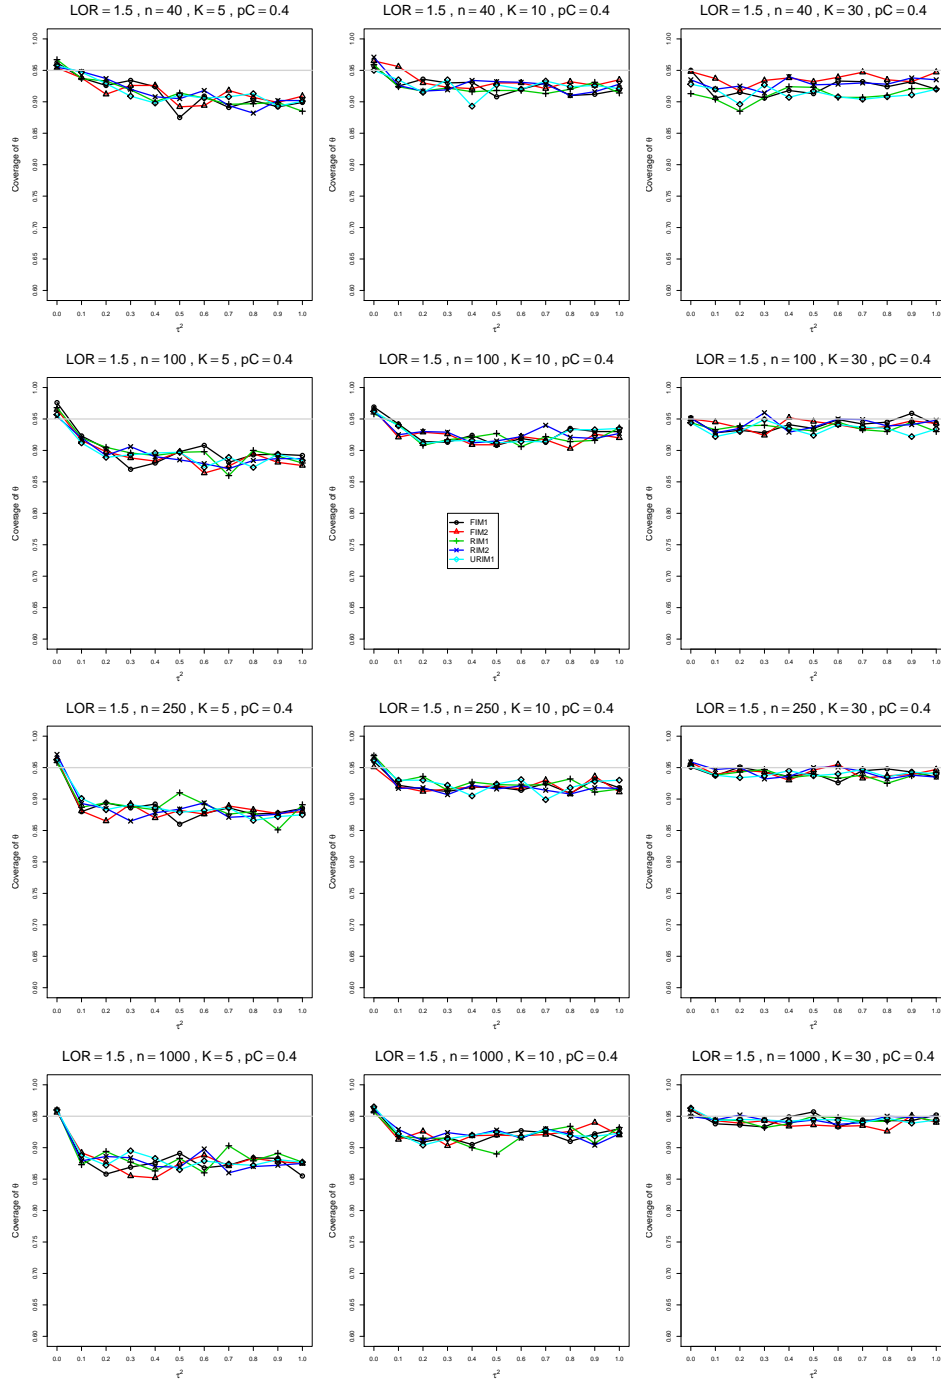

Figure A3.4.18: Coverage of the Kulinskaya-Dollinger confidence interval for  $\theta = 1.5$ ,  $p_C = 0.4$ ,  $\sigma^2 = 0.4$ , constant sample sizes  $n = 40, 100, 250, 1000$ . The data-generation mechanisms are FIM1 ( $\circ$ ), FIM2 ( $\triangle$ ), RIM1 (+), RIM2 ( $\times$ ), and URIM1 ( $\diamond$ ).

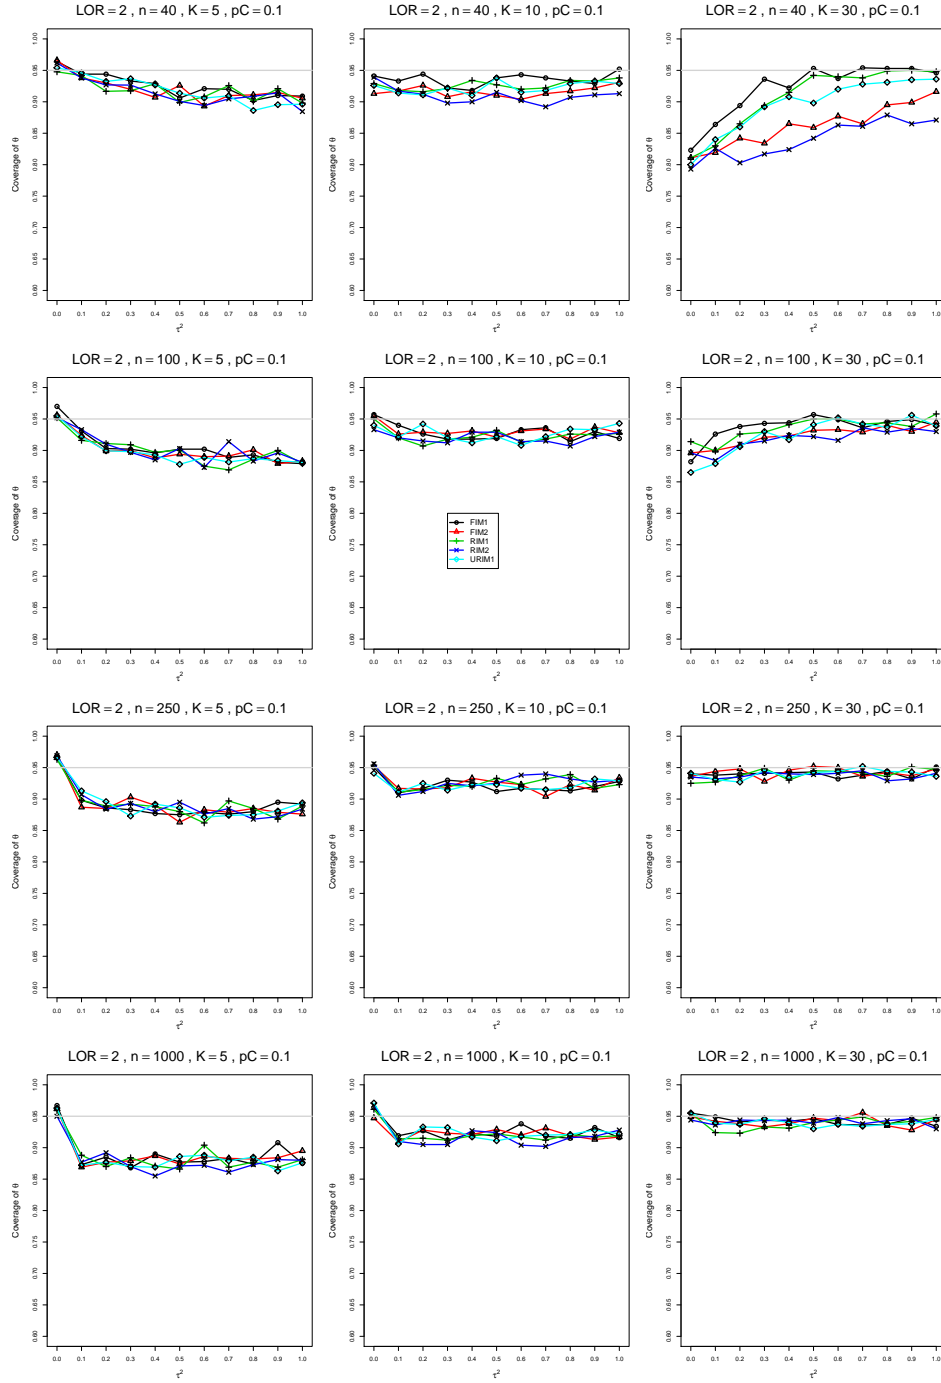

Figure A3.4.19: Coverage of the Kulinskaya-Dollinger confidence interval for  $\theta = 2$ ,  $p_C = 0.1$ ,  $\sigma^2 = 0.4$ , constant sample sizes  $n = 40, 100, 250, 1000$ . The data-generation mechanisms are FIM1 ( $\circ$ ), FIM2 ( $\triangle$ ), RIM1 ( $+$ ), RIM2 ( $\times$ ), and URIM1 ( $\diamond$ ).

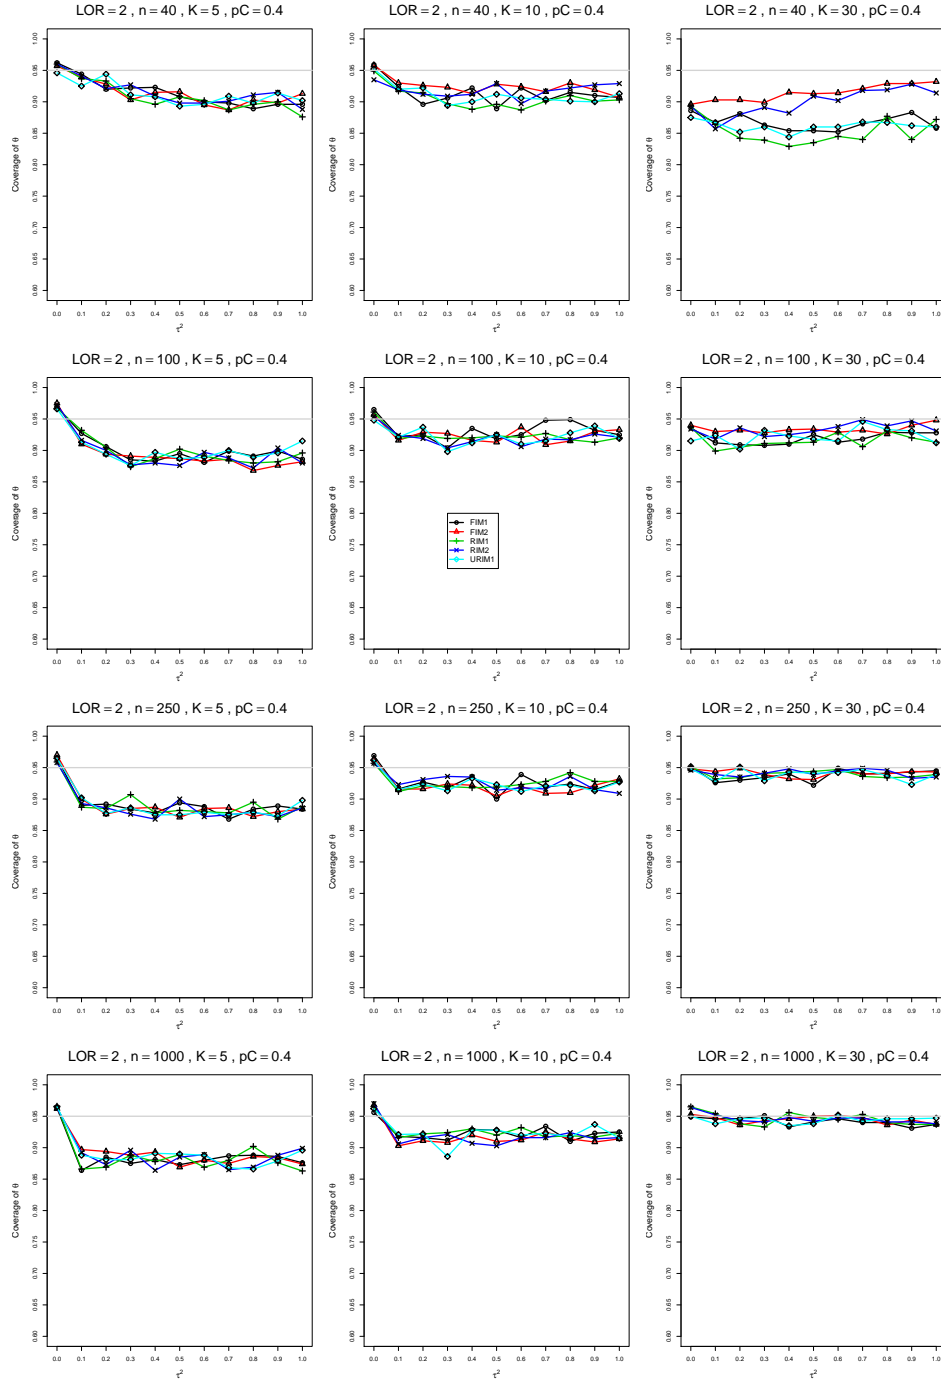

Figure A3.4.20: Coverage of the Kulinskaya-Dollinger confidence interval for  $\theta = 2$ ,  $p_C = 0.4$ ,  $\sigma^2 = 0.4$ , constant sample sizes  $n = 40, 100, 250, 1000$ . The data-generation mechanisms are FIM1 ( $\circ$ ), FIM2 ( $\triangle$ ), RIM1 ( $+$ ), RIM2 ( $\times$ ), and URIM1 ( $\diamond$ ).

### A3.5 Coverage of $\hat{\theta}_{FIM2}$

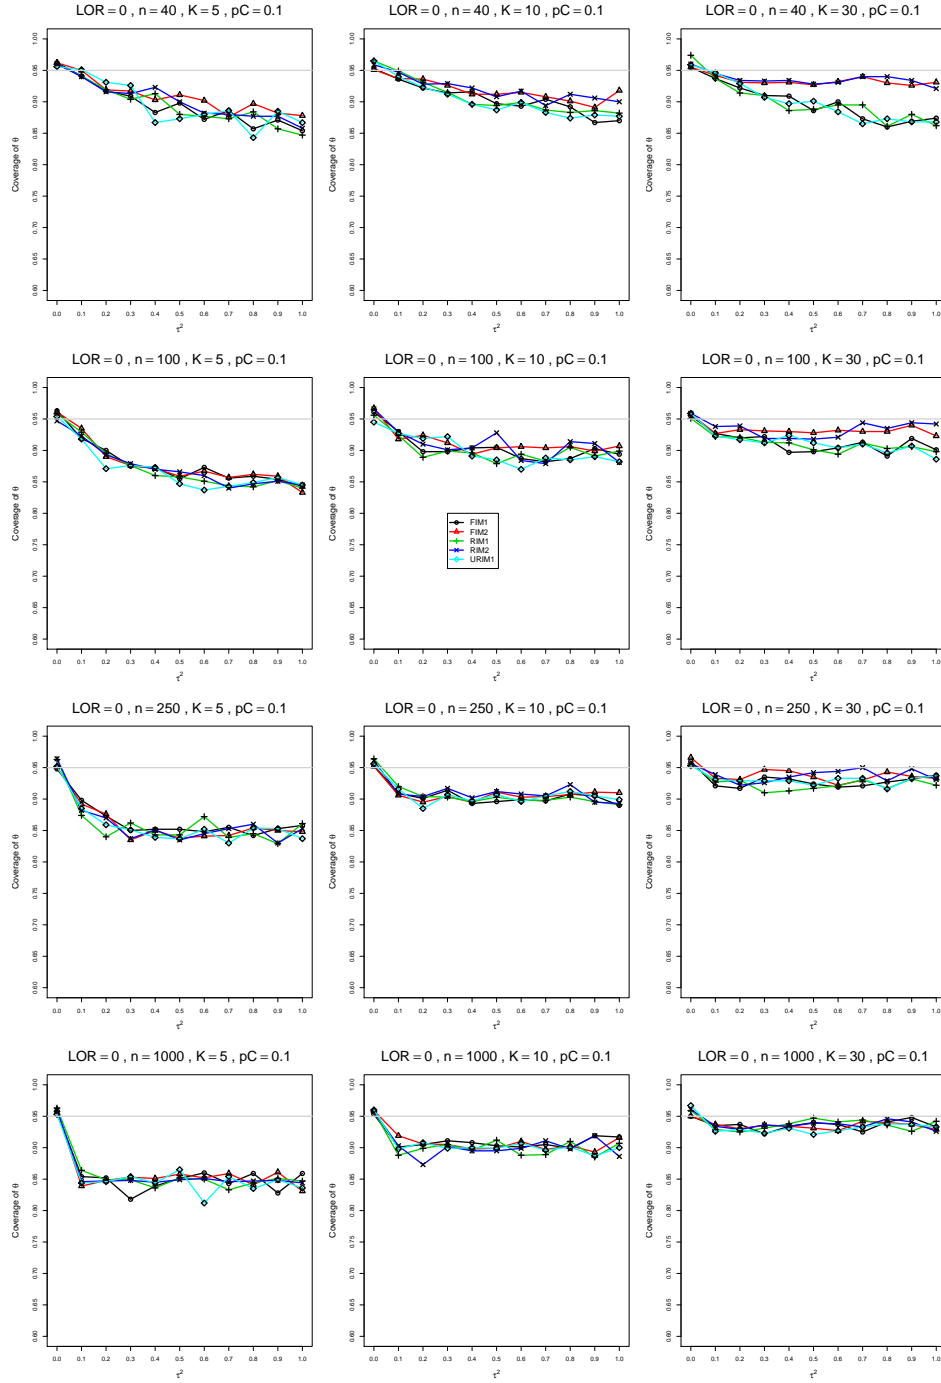

Figure A3.5.1: Coverage of the Fixed-intercept with  $c = 1/2$  confidence interval for  $\theta = 0$ ,  $p_C = 0.1$ ,  $\sigma^2 = 0.1$ , constant sample sizes  $n = 40, 100, 250, 1000$ . The data-generation mechanisms are FIM1 (o), FIM2 ( $\triangle$ ), RIM1 (+), RIM2 ( $\times$ ), and URIM1 ( $\diamond$ ).

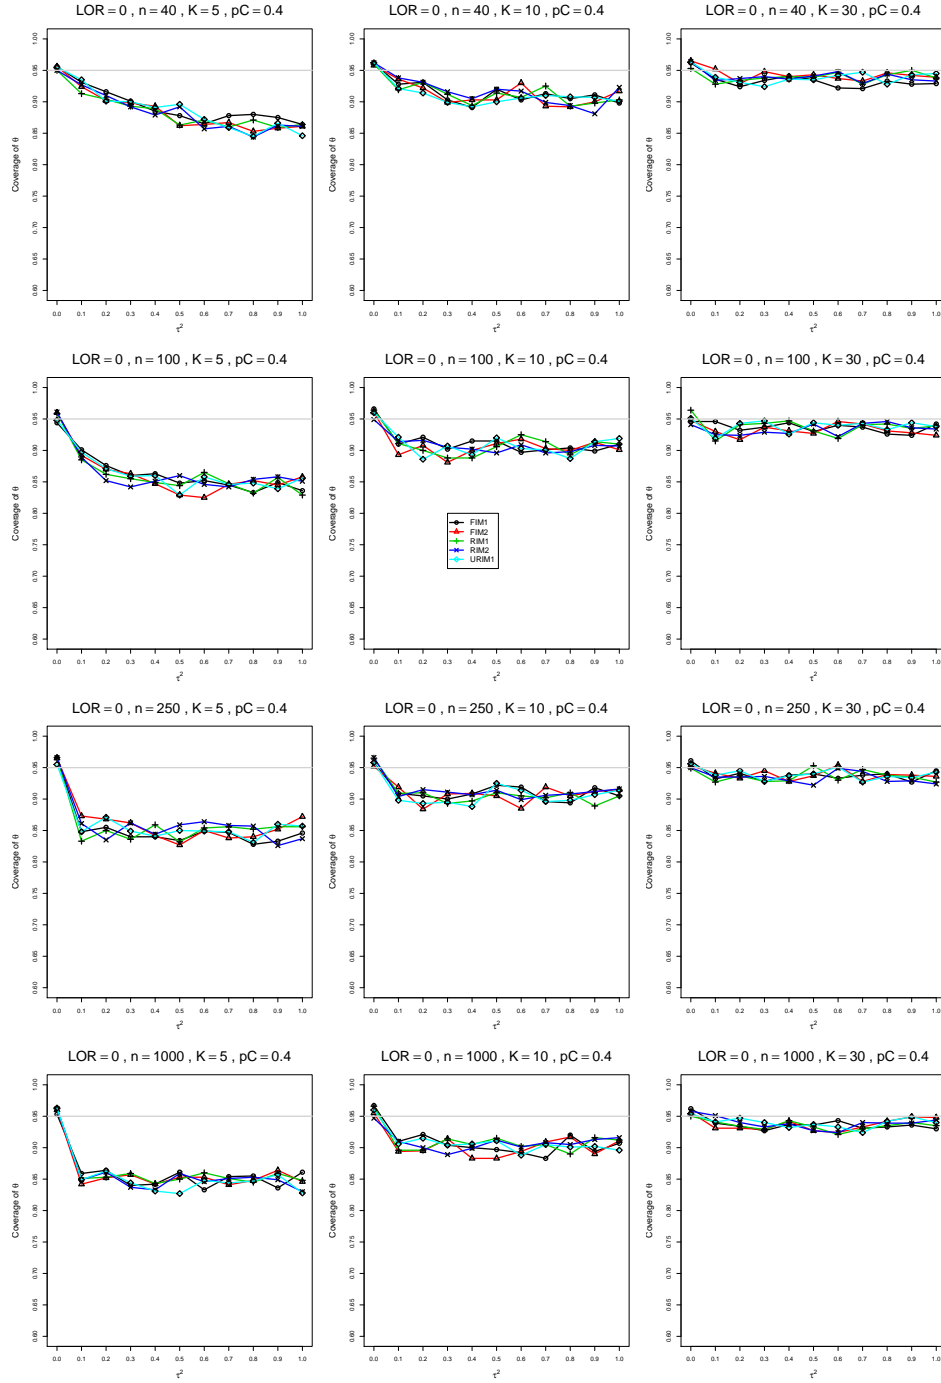

Figure A3.5.2: Coverage of the Fixed-intercept with  $c = 1/2$  confidence interval for  $\theta = 0$ ,  $p_C = 0.4$ ,  $\sigma^2 = 0.1$ , constant sample sizes  $n = 40, 100, 250, 1000$ . The data-generation mechanisms are FIM1 ( $\circ$ ), FIM2 ( $\triangle$ ), RIM1 ( $+$ ), RIM2 ( $\times$ ), and URIM1 ( $\diamond$ ).



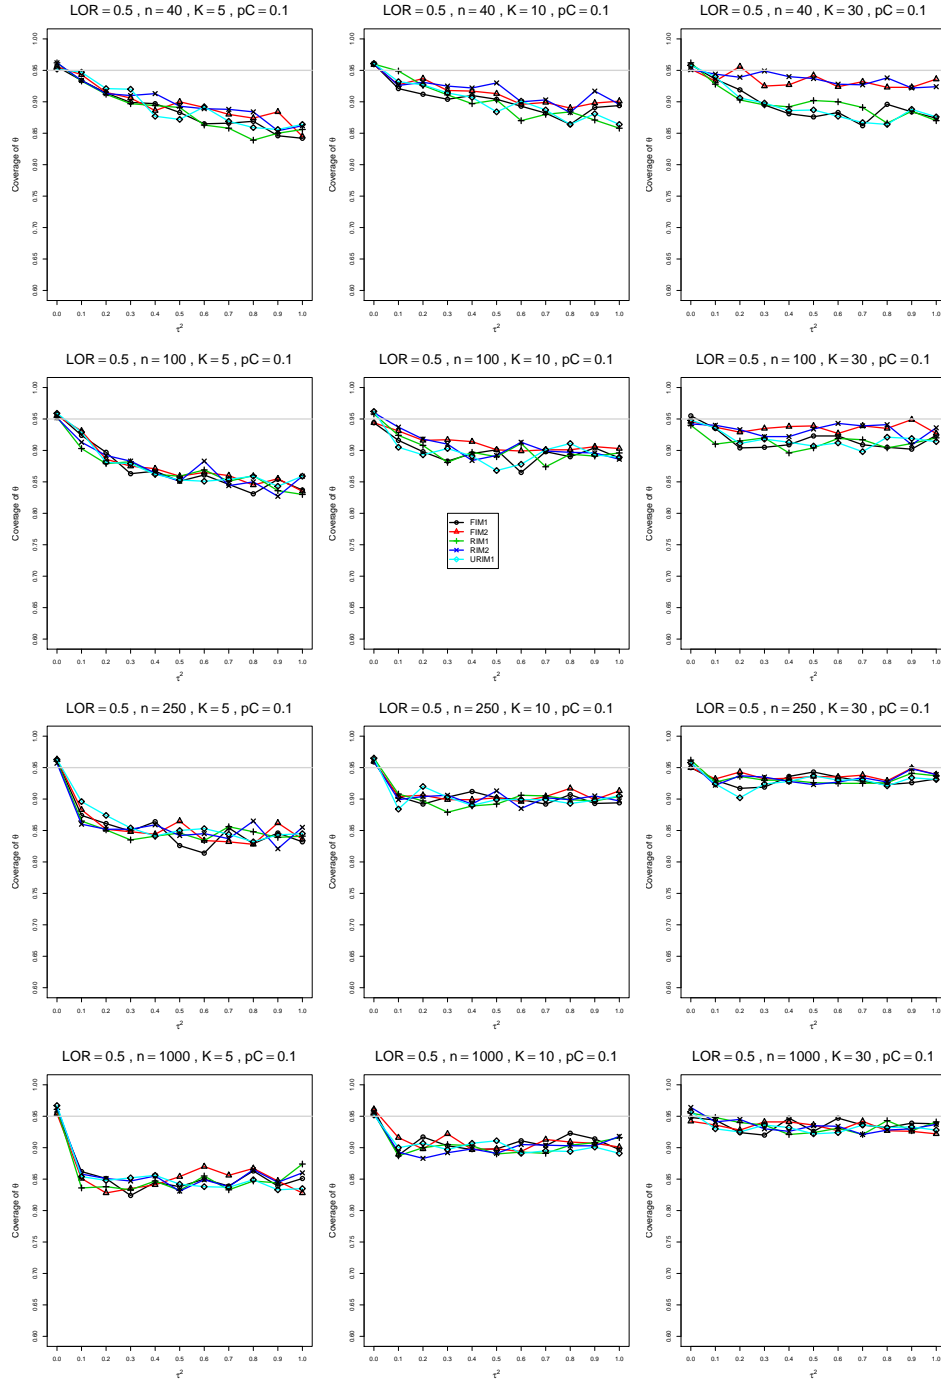

Figure A3.5.3: Coverage of the Fixed-intercept with  $c = 1/2$  confidence interval for  $\theta = 0.5$ ,  $p_C = 0.1$ ,  $\sigma^2 = 0.1$ , constant sample sizes  $n = 40, 100, 250, 1000$ . The data-generation mechanisms are FIM1 (o), FIM2 ( $\triangle$ ), RIM1 (+), RIM2 ( $\times$ ), and URIM1 ( $\diamond$ ).

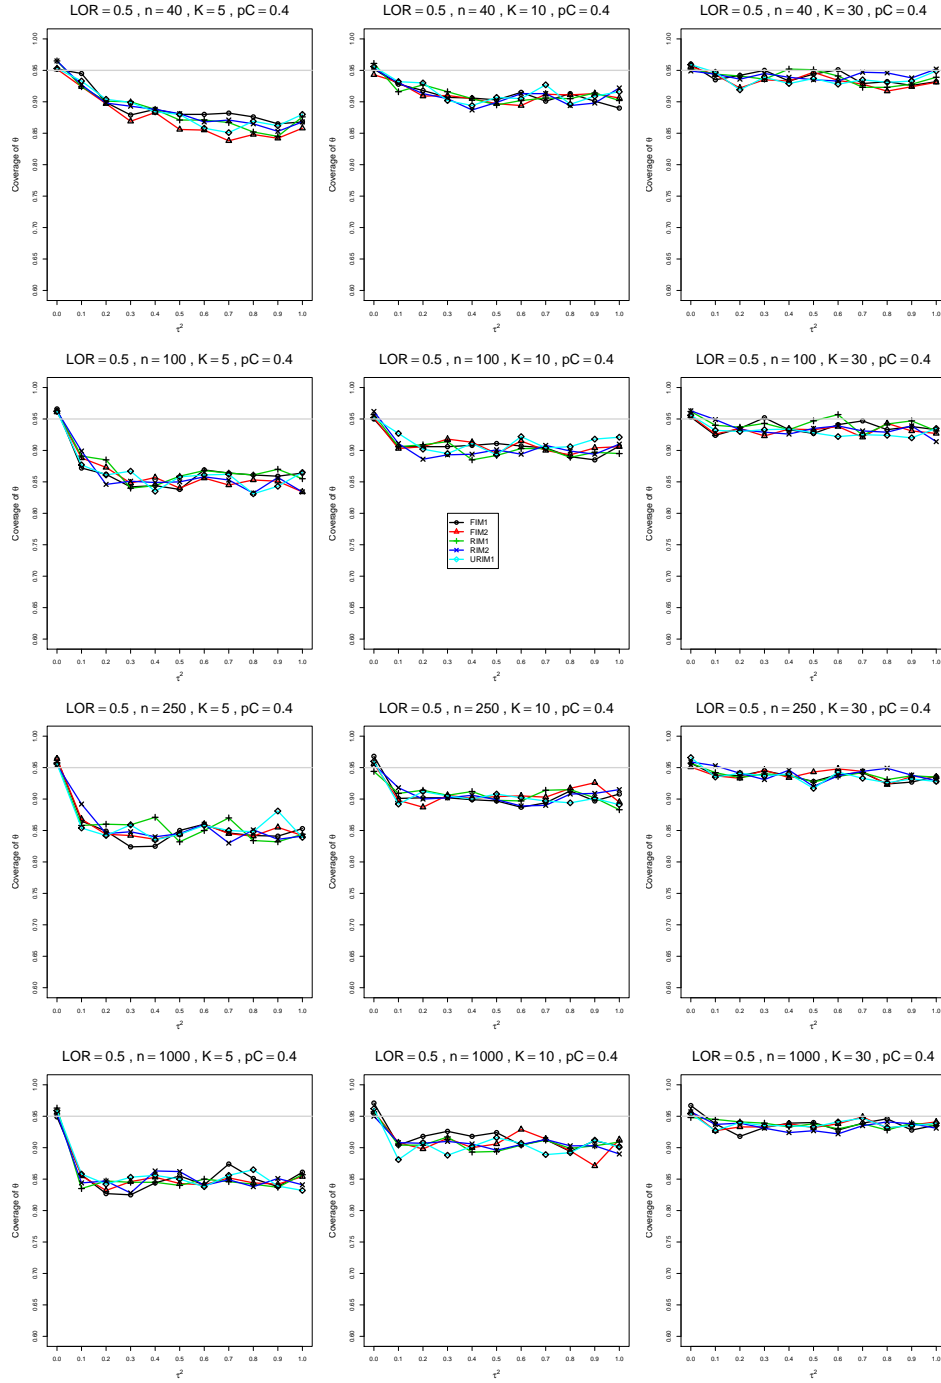

Figure A3.5.4: Coverage of the Fixed-intercept with  $c = 1/2$  confidence interval for  $\theta = 0.5$ ,  $p_C = 0.4$ ,  $\sigma^2 = 0.1$ , constant sample sizes  $n = 40, 100, 250, 1000$ . The data-generation mechanisms are FIM1 ( $\circ$ ), FIM2 ( $\triangle$ ), RIM1 ( $+$ ), RIM2 ( $\times$ ), and URIM1 ( $\diamond$ ).

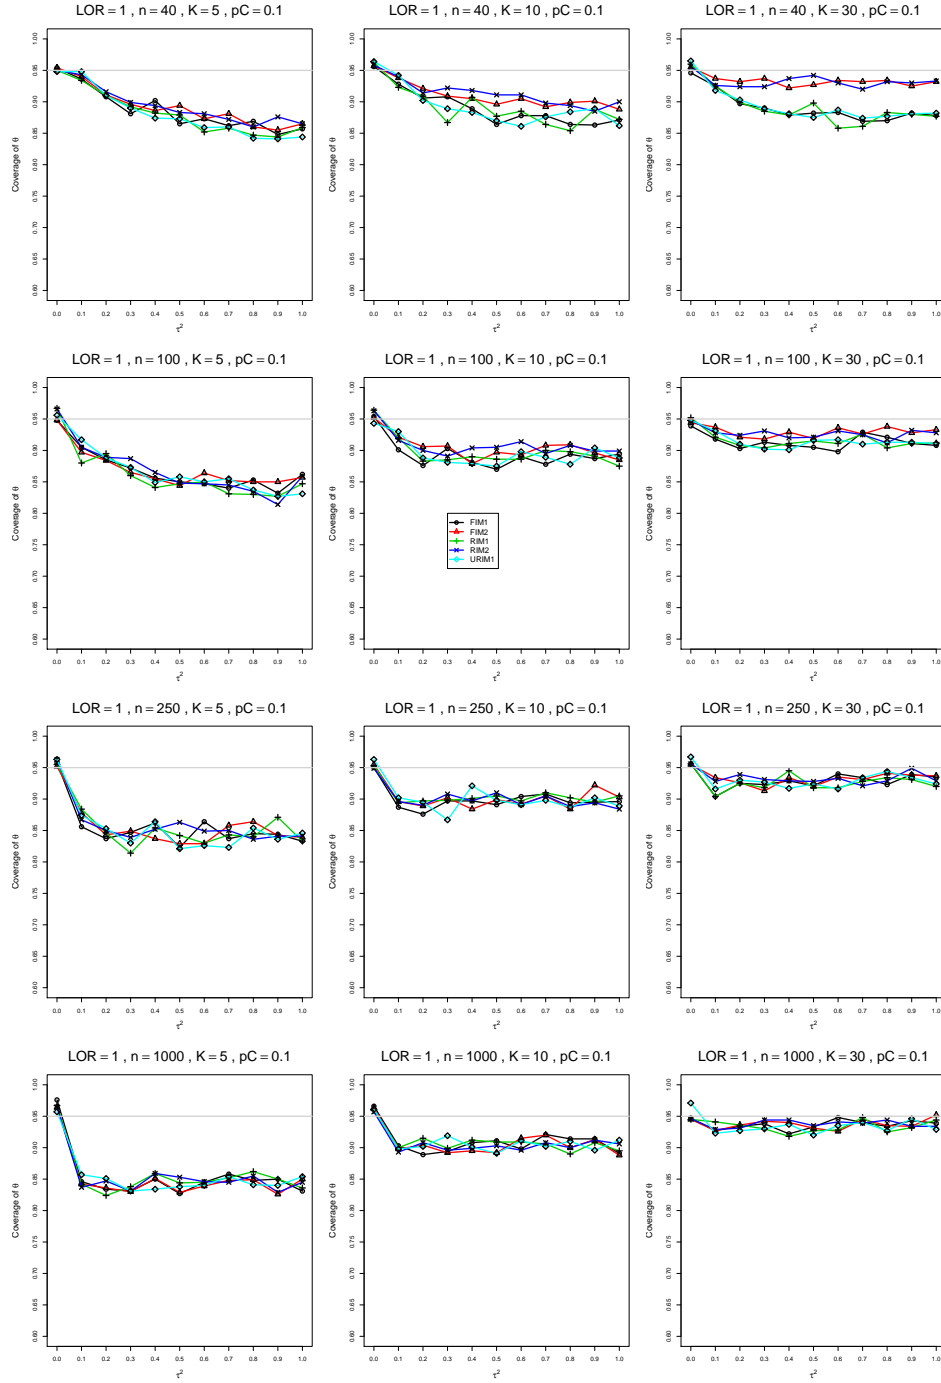

Figure A3.5.5: Coverage of the Fixed-intercept with  $c = 1/2$  confidence interval for  $\theta = 1$ ,  $p_C = 0.1$ ,  $\sigma^2 = 0.1$ , constant sample sizes  $n = 40, 100, 250, 1000$ . The data-generation mechanisms are FIM1 ( $\circ$ ), FIM2 ( $\triangle$ ), RIM1 ( $+$ ), RIM2 ( $\times$ ), and URIM1 ( $\diamond$ ).

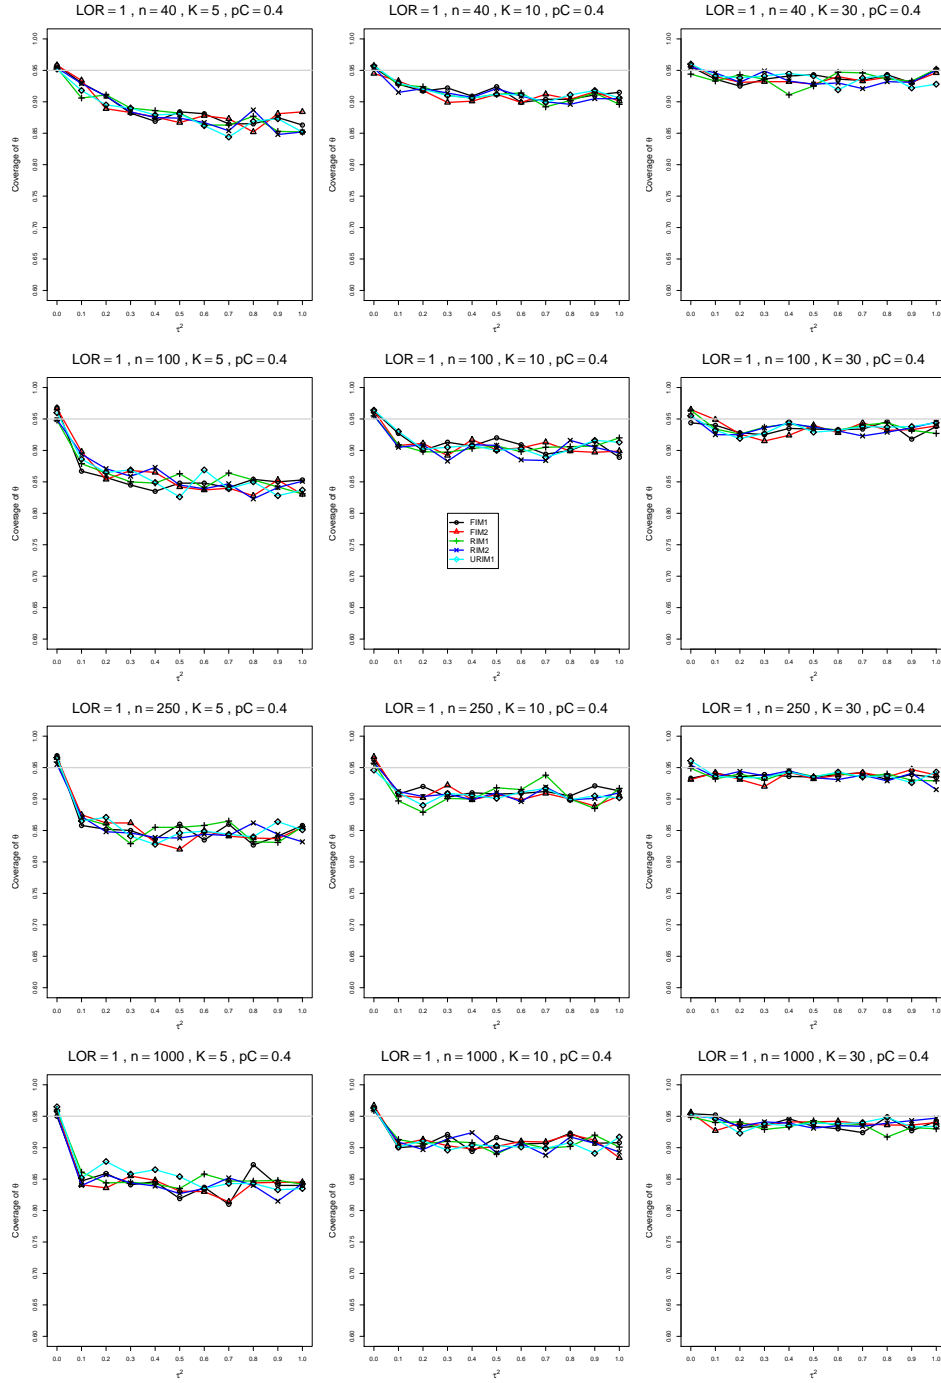

Figure A3.5.6: Coverage of the Fixed-intercept with  $c = 1/2$  confidence interval for  $\theta = 1$ ,  $p_C = 0.4$ ,  $\sigma^2 = 0.1$ , constant sample sizes  $n = 40, 100, 250, 1000$ . The data-generation mechanisms are FIM1 (o), FIM2 ( $\triangle$ ), RIM1 (+), RIM2 ( $\times$ ), and URIM1 ( $\diamond$ ).

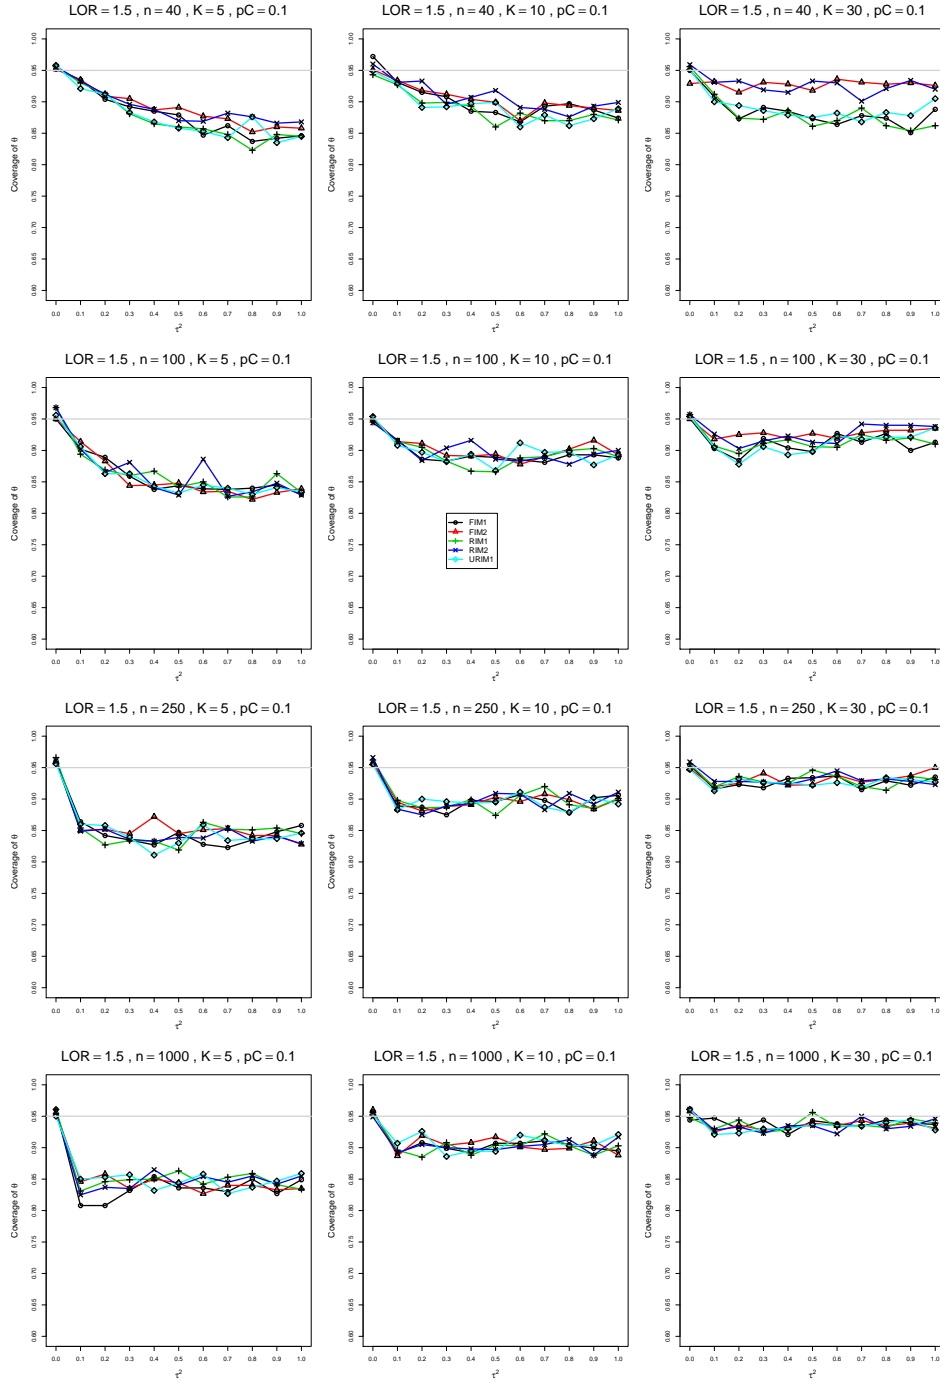

Figure A3.5.7: Coverage of the Fixed-intercept with  $c = 1/2$  confidence interval for  $\theta = 1.5$ ,  $p_C = 0.1$ ,  $\sigma^2 = 0.1$ , constant sample sizes  $n = 40, 100, 250, 1000$ . The data-generation mechanisms are FIM1 ( $\circ$ ), FIM2 ( $\triangle$ ), RIM1 (+), RIM2 ( $\times$ ), and URIM1 ( $\diamond$ ).

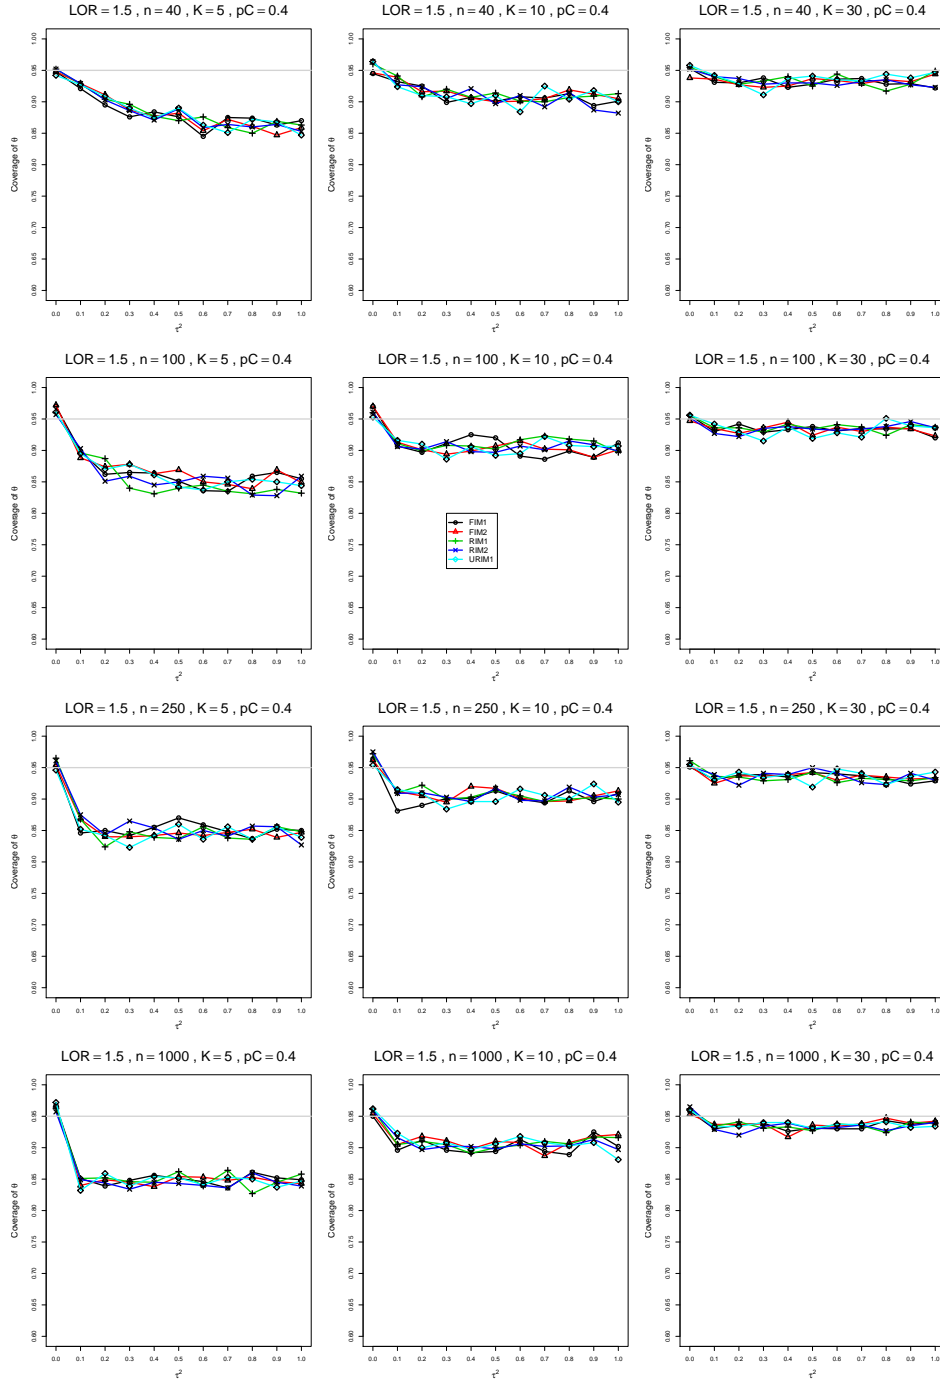

Figure A3.5.8: Coverage of the Fixed-intercept with  $c = 1/2$  confidence interval for  $\theta = 1.5$ ,  $p_C = 0.4$ ,  $\sigma^2 = 0.1$ , constant sample sizes  $n = 40, 100, 250, 1000$ . The data-generation mechanisms are FIM1 (o), FIM2 ( $\triangle$ ), RIM1 (+), RIM2 ( $\times$ ), and URIM1 ( $\diamond$ ).

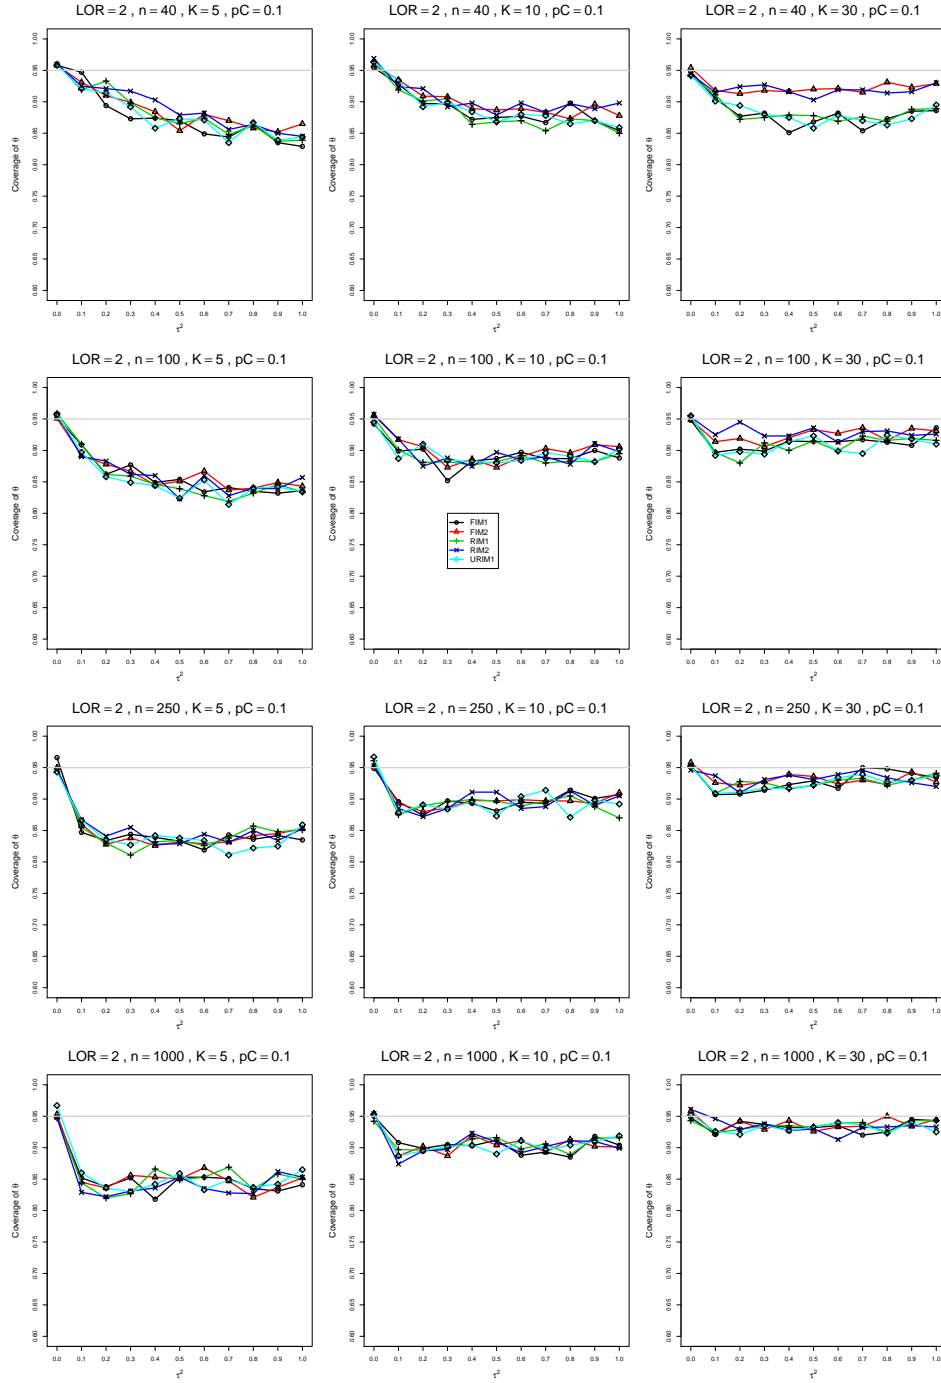

Figure A3.5.9: Coverage of the Fixed-intercept with  $c = 1/2$  confidence interval for  $\theta = 2$ ,  $p_C = 0.1$ ,  $\sigma^2 = 0.1$ , constant sample sizes  $n = 40, 100, 250, 1000$ . The data-generation mechanisms are FIM1 ( $\circ$ ), FIM2 ( $\triangle$ ), RIM1 ( $+$ ), RIM2 ( $\times$ ), and URIM1 ( $\diamond$ ).

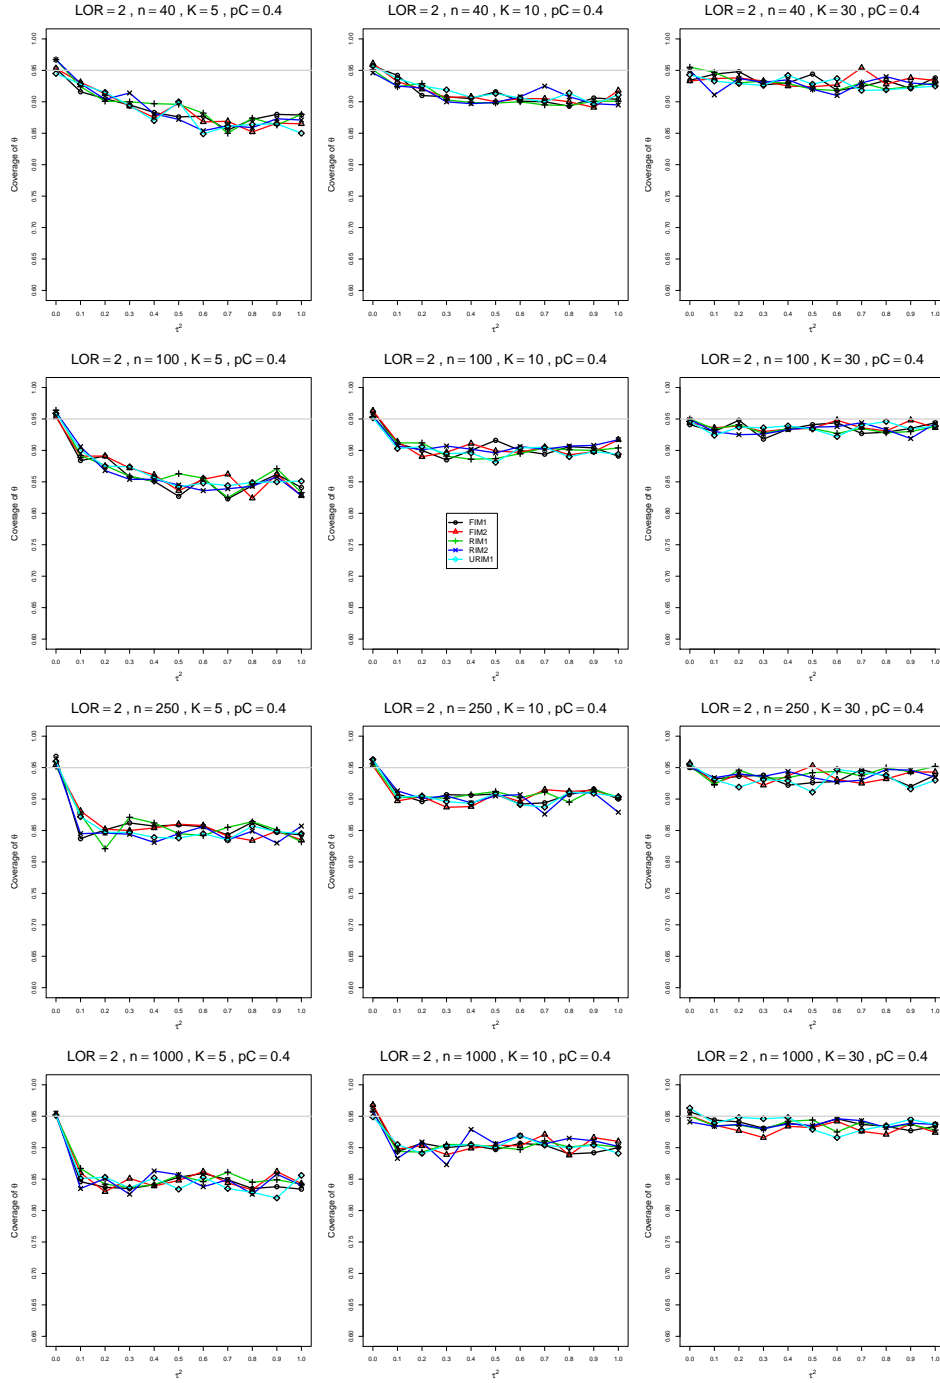

Figure A3.5.10: Coverage of the Fixed-intercept with  $c = 1/2$  confidence interval for  $\theta = 2$ ,  $p_C = 0.4$ ,  $\sigma^2 = 0.1$ , constant sample sizes  $n = 40, 100, 250, 1000$ . The data-generation mechanisms are FIM1 ( $\circ$ ), FIM2 ( $\triangle$ ), RIM1 ( $+$ ), RIM2 ( $\times$ ), and URIM1 ( $\diamond$ ).



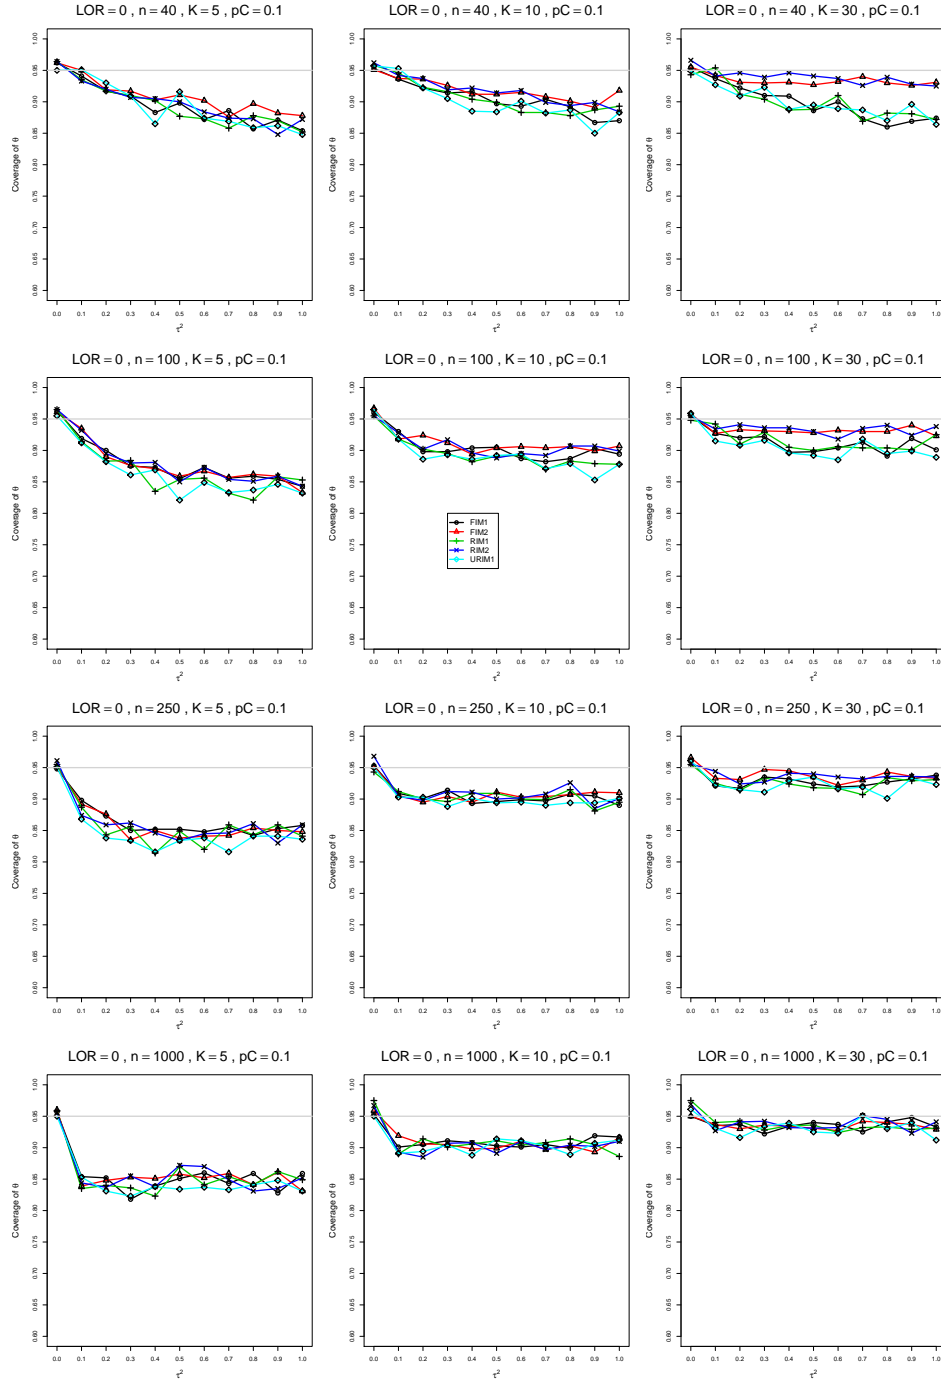

Figure A3.5.11: Coverage of the Fixed-intercept with  $c = 1/2$  confidence interval for  $\theta = 0$ ,  $p_C = 0.1$ ,  $\sigma^2 = 0.4$ , constant sample sizes  $n = 40, 100, 250, 1000$ . The data-generation mechanisms are FIM1 ( $\circ$ ), FIM2 ( $\triangle$ ), RIM1 ( $+$ ), RIM2 ( $\times$ ), and URIM1 ( $\diamond$ ).

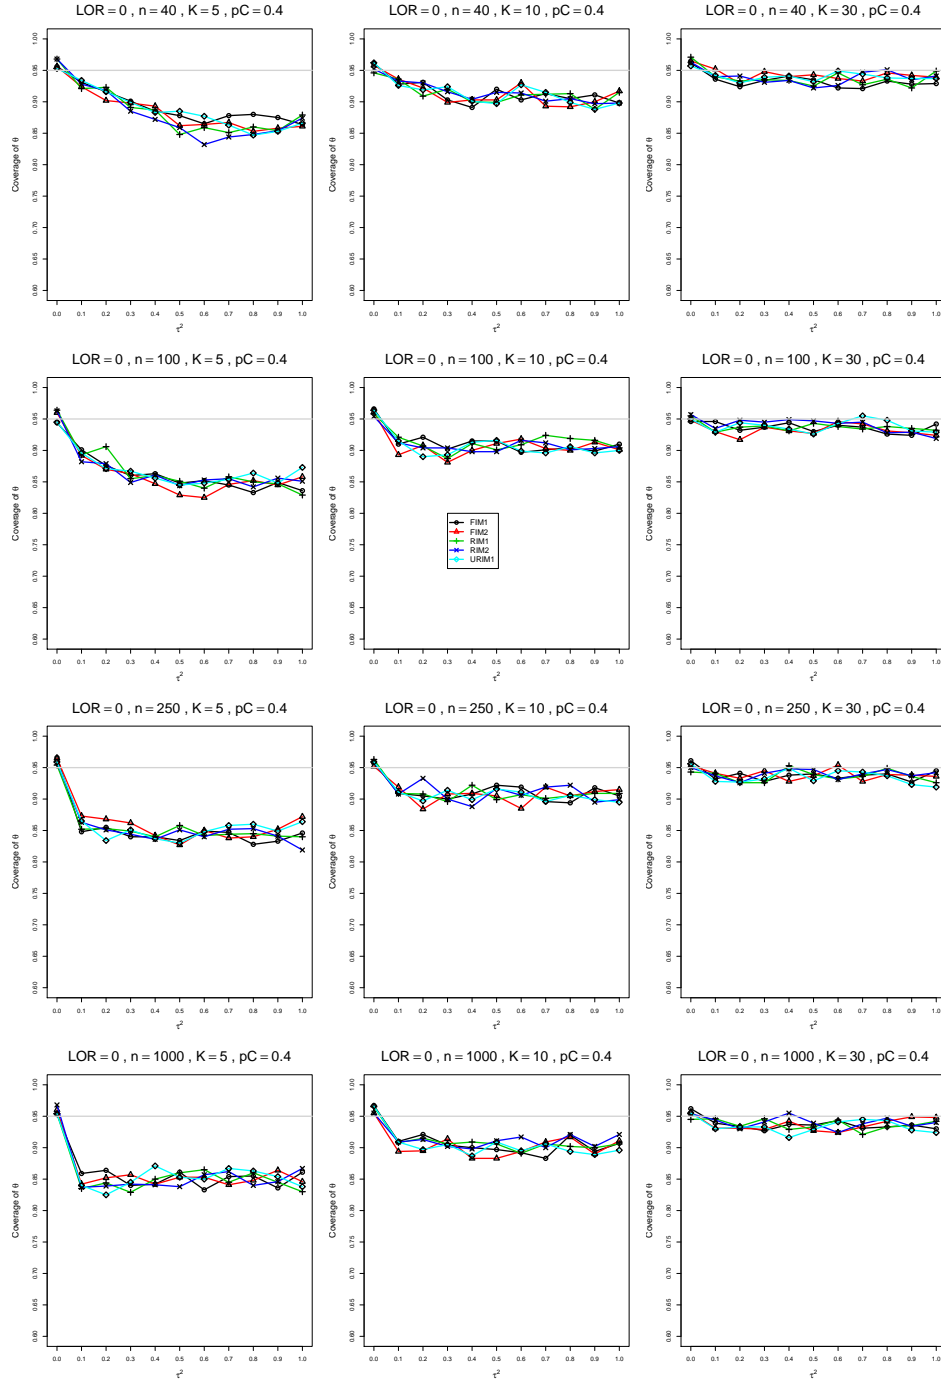

Figure A3.5.12: Coverage of the Fixed-intercept with  $c = 1/2$  confidence interval for  $\theta = 0$ ,  $p_C = 0.4$ ,  $\sigma^2 = 0.4$ , constant sample sizes  $n = 40, 100, 250, 1000$ . The data-generation mechanisms are FIM1 ( $\circ$ ), FIM2 ( $\triangle$ ), RIM1 ( $+$ ), RIM2 ( $\times$ ), and URIM1 ( $\diamond$ ).

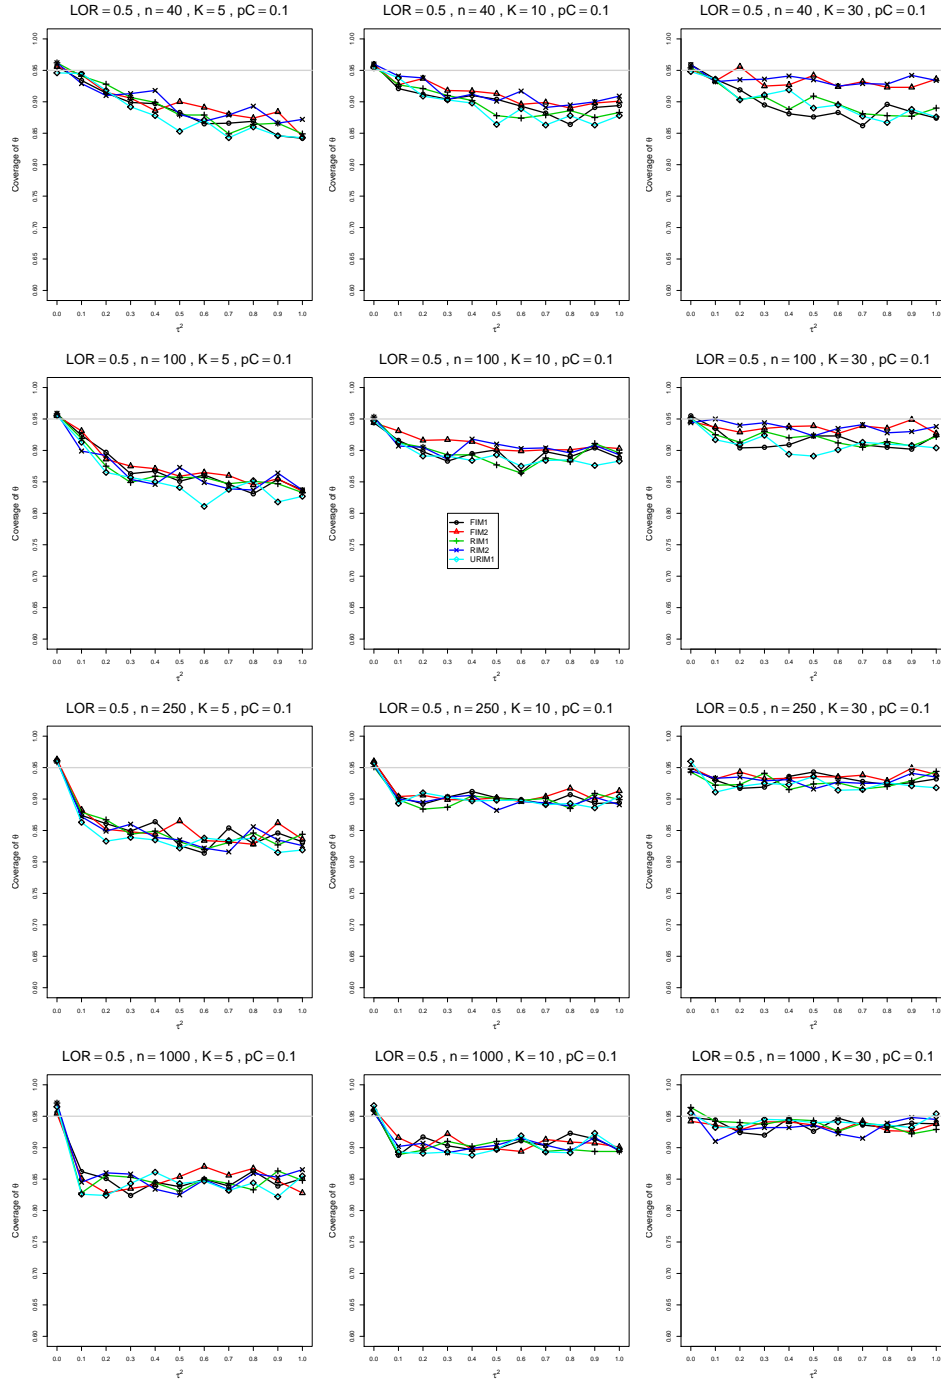

Figure A3.5.13: Coverage of the Fixed-intercept with  $c = 1/2$  confidence interval for  $\theta = 0.5$ ,  $p_C = 0.1$ ,  $\sigma^2 = 0.4$ , constant sample sizes  $n = 40, 100, 250, 1000$ . The data-generation mechanisms are FIM1 ( $\circ$ ), FIM2 ( $\triangle$ ), RIM1 ( $+$ ), RIM2 ( $\times$ ), and URIM1 ( $\diamond$ ).

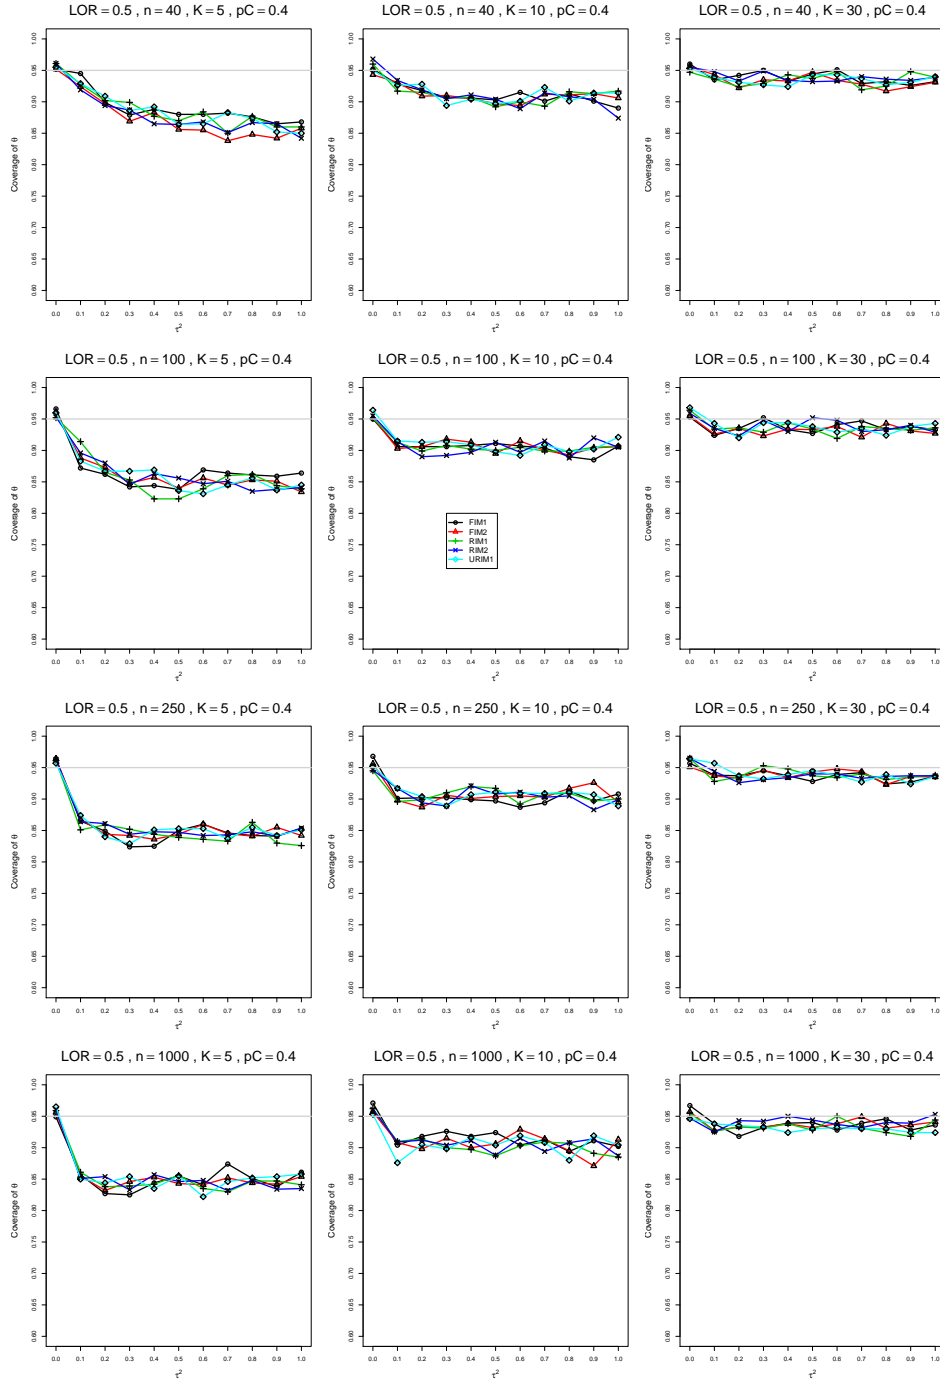

Figure A3.5.14: Coverage of the Fixed-intercept with  $c = 1/2$  confidence interval for  $\theta = 0.5$ ,  $p_C = 0.4$ ,  $\sigma^2 = 0.4$ , constant sample sizes  $n = 40, 100, 250, 1000$ . The data-generation mechanisms are FIM1 ( $\circ$ ), FIM2 ( $\triangle$ ), RIM1 ( $+$ ), RIM2 ( $\times$ ), and URIM1 ( $\diamond$ ).

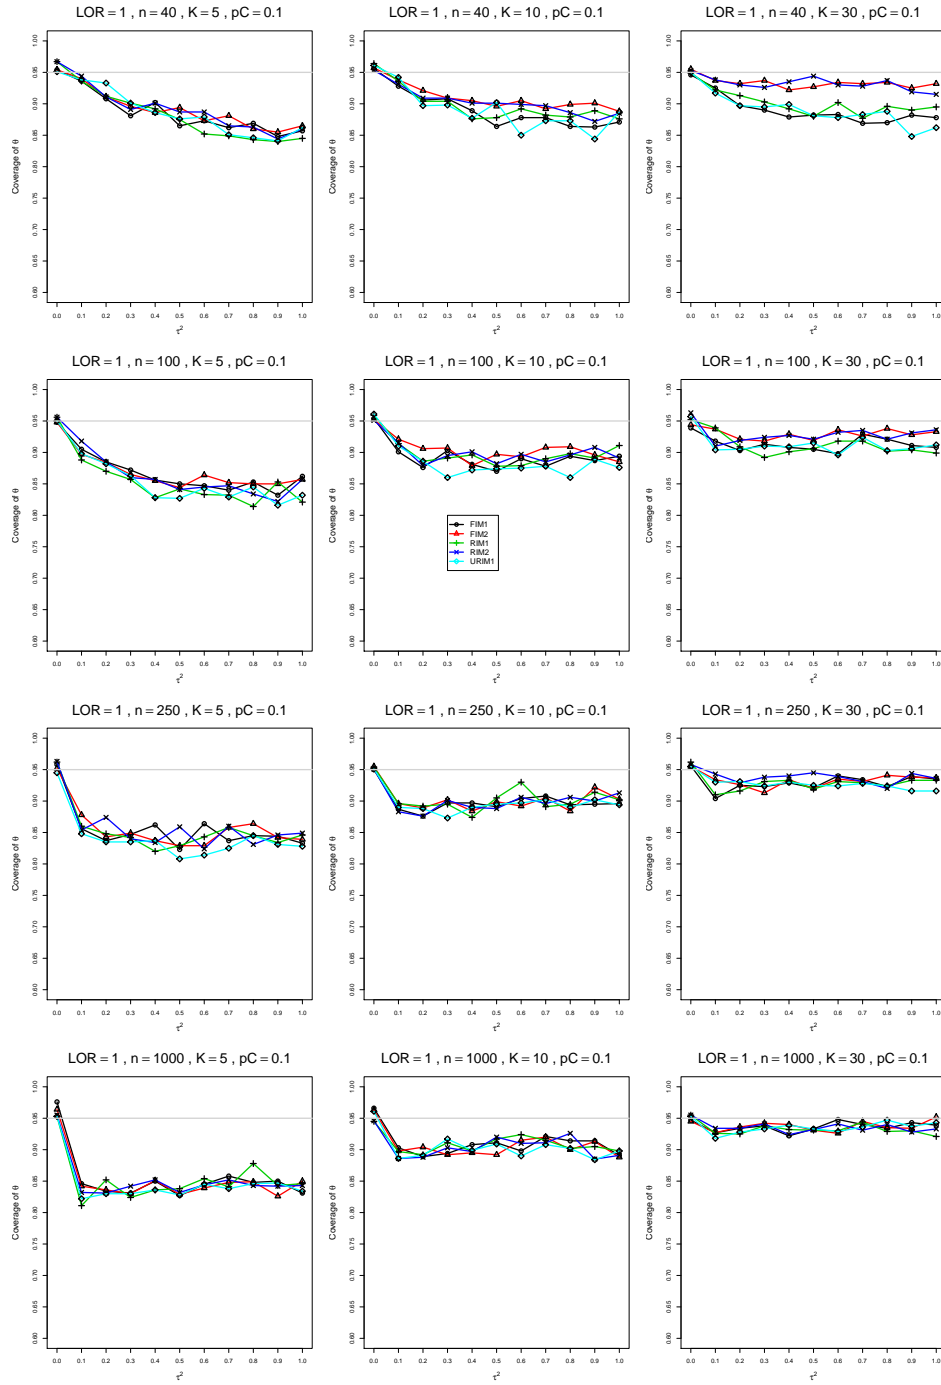

Figure A3.5.15: Coverage of the Fixed-intercept with  $c = 1/2$  confidence interval for  $\theta = 1$ ,  $p_C = 0.1$ ,  $\sigma^2 = 0.4$ , constant sample sizes  $n = 40, 100, 250, 1000$ . The data-generation mechanisms are FIM1 ( $\circ$ ), FIM2 ( $\triangle$ ), RIM1 ( $+$ ), RIM2 ( $\times$ ), and URIM1 ( $\diamond$ ).

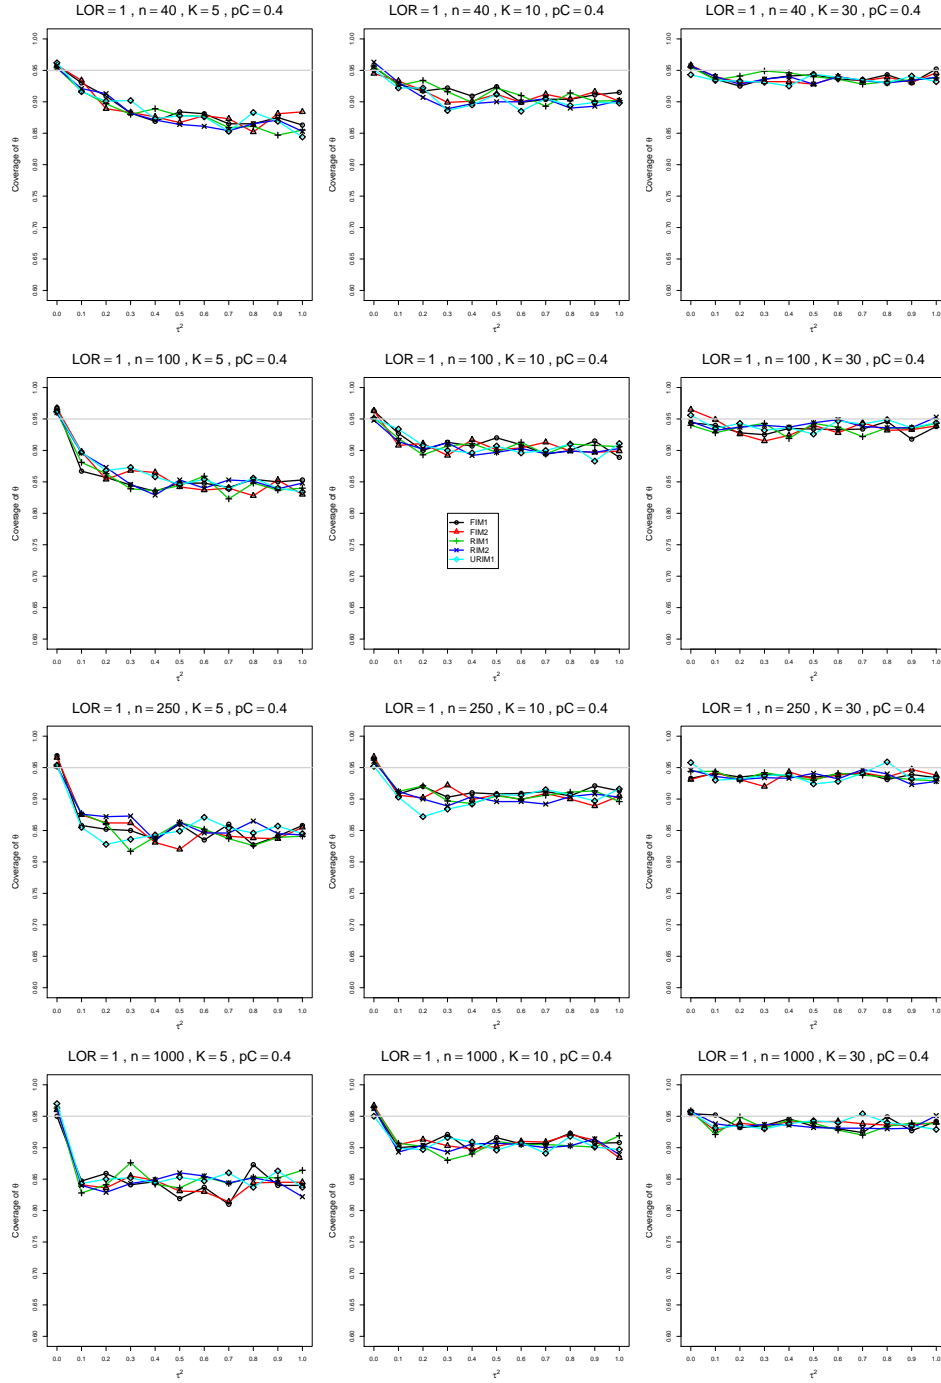

Figure A3.5.16: Coverage of the Fixed-intercept with  $c = 1/2$  confidence interval for  $\theta = 1$ ,  $p_C = 0.4$ ,  $\sigma^2 = 0.4$ , constant sample sizes  $n = 40, 100, 250, 1000$ . The data-generation mechanisms are FIM1 ( $\circ$ ), FIM2 ( $\triangle$ ), RIM1 ( $+$ ), RIM2 ( $\times$ ), and URIM1 ( $\diamond$ ).

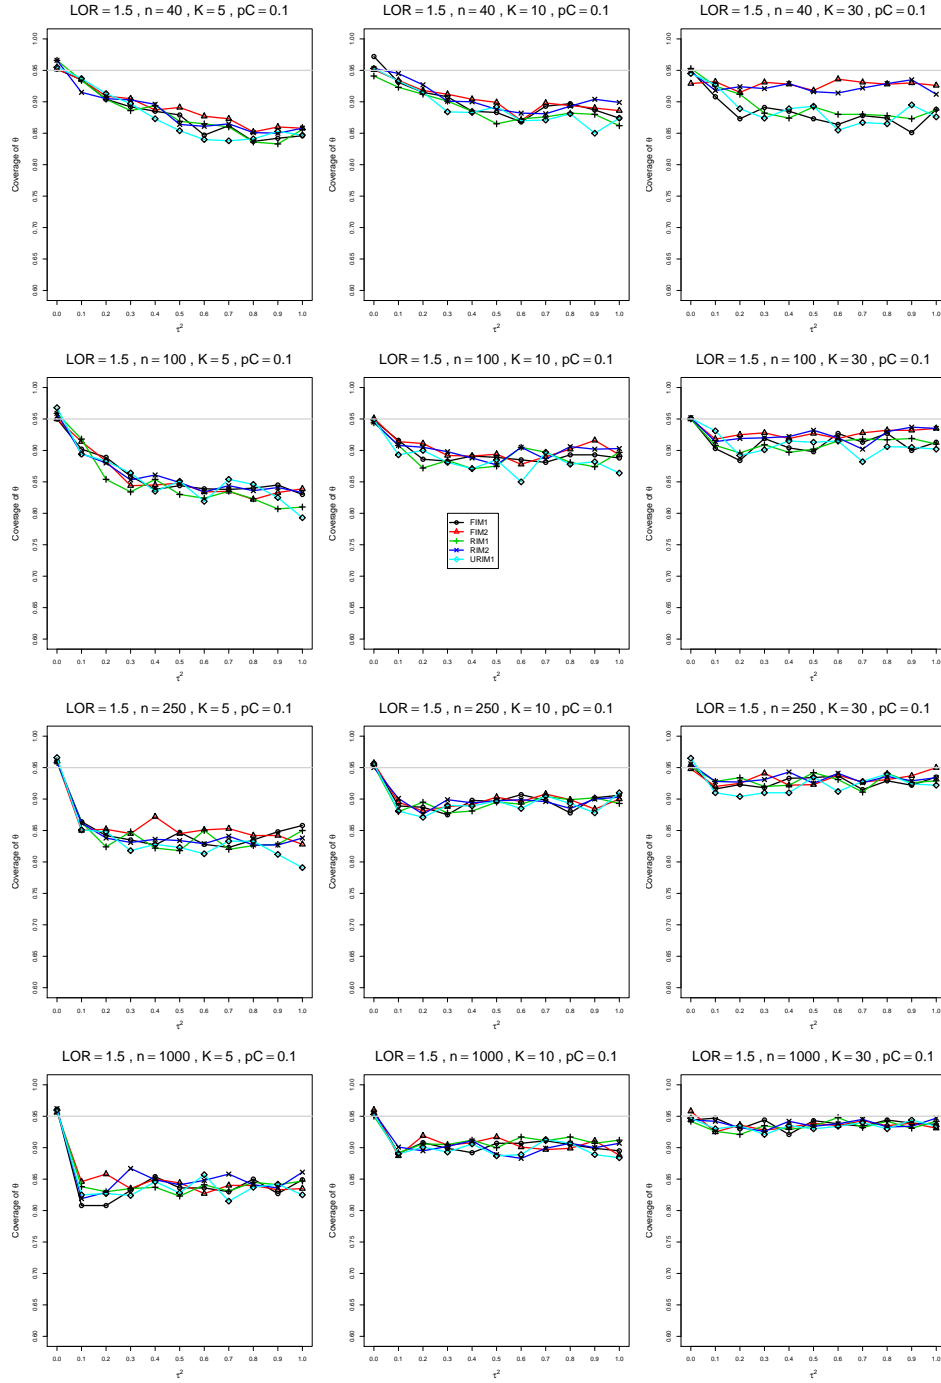

Figure A3.5.17: Coverage of the Fixed-intercept with  $c = 1/2$  confidence interval for  $\theta = 1.5$ ,  $p_C = 0.1$ ,  $\sigma^2 = 0.4$ , constant sample sizes  $n = 40, 100, 250, 1000$ . The data-generation mechanisms are FIM1 ( $\circ$ ), FIM2 ( $\triangle$ ), RIM1 ( $+$ ), RIM2 ( $\times$ ), and URIM1 ( $\diamond$ ).

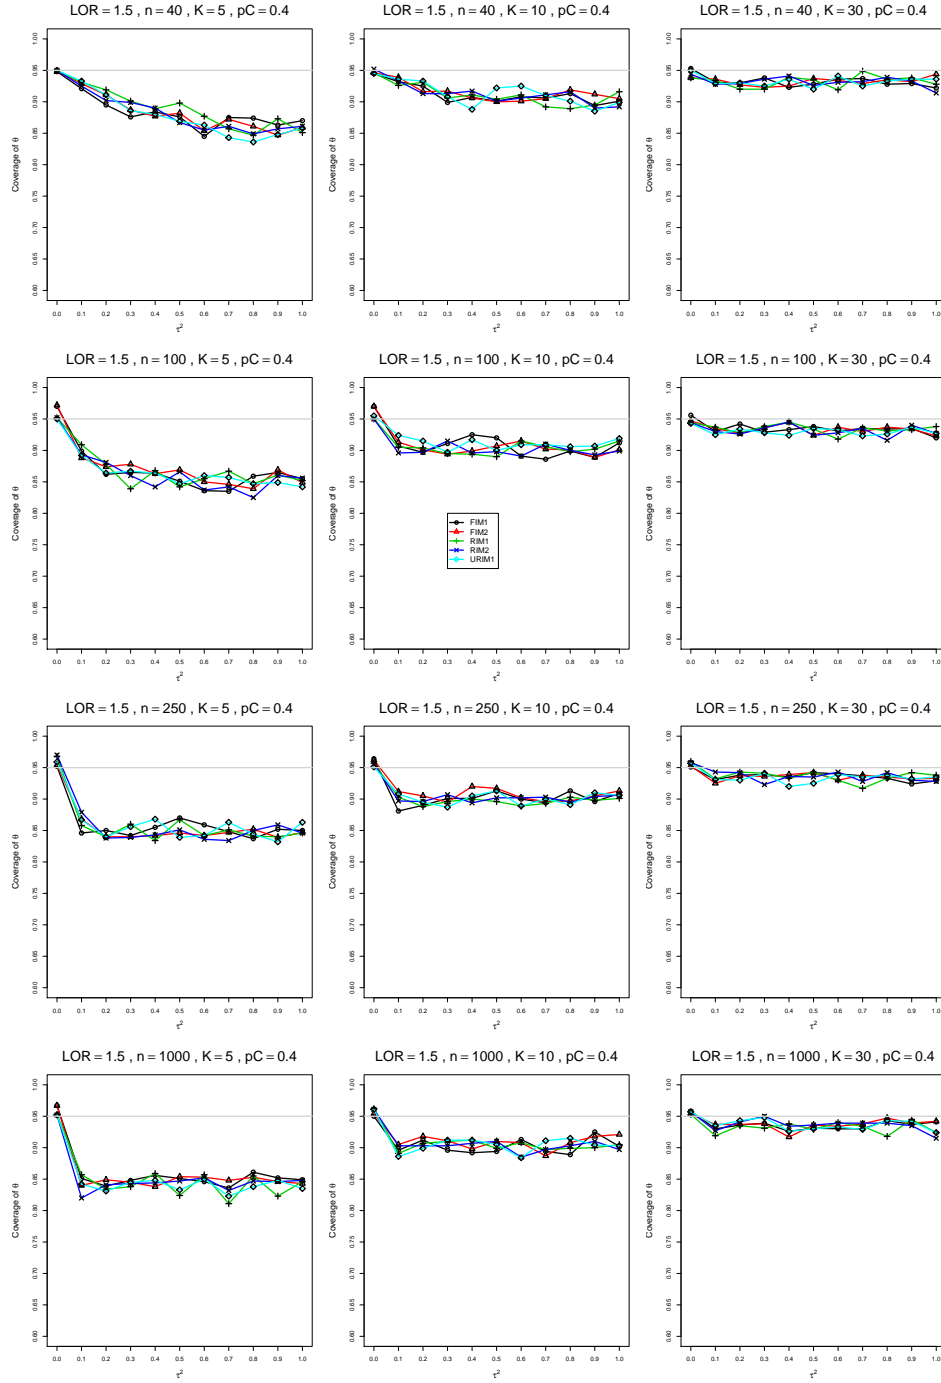

Figure A3.5.18: Coverage of the Fixed-intercept with  $c = 1/2$  confidence interval for  $\theta = 1.5$ ,  $p_C = 0.4$ ,  $\sigma^2 = 0.4$ , constant sample sizes  $n = 40, 100, 250, 1000$ . The data-generation mechanisms are FIM1 (o), FIM2 ( $\triangle$ ), RIM1 (+), RIM2 ( $\times$ ), and URIM1 ( $\diamond$ ).



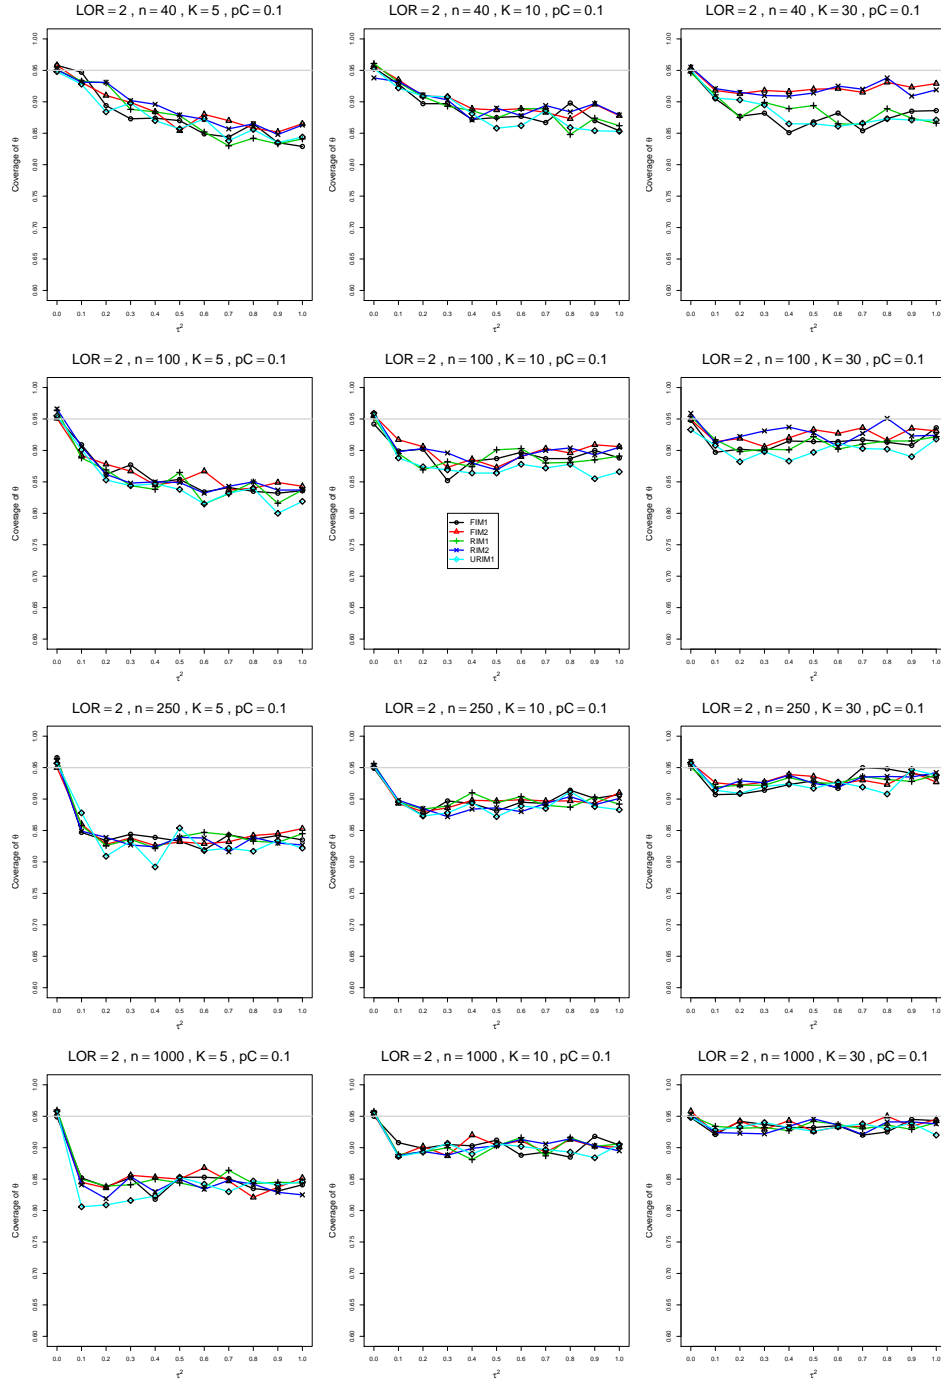

Figure A3.5.19: Coverage of the Fixed-intercept with  $c = 1/2$  confidence interval for  $\theta = 2$ ,  $p_C = 0.1$ ,  $\sigma^2 = 0.4$ , constant sample sizes  $n = 40, 100, 250, 1000$ . The data-generation mechanisms are FIM1 ( $\circ$ ), FIM2 ( $\triangle$ ), RIM1 (+), RIM2 ( $\times$ ), and URIM1 ( $\diamond$ ).

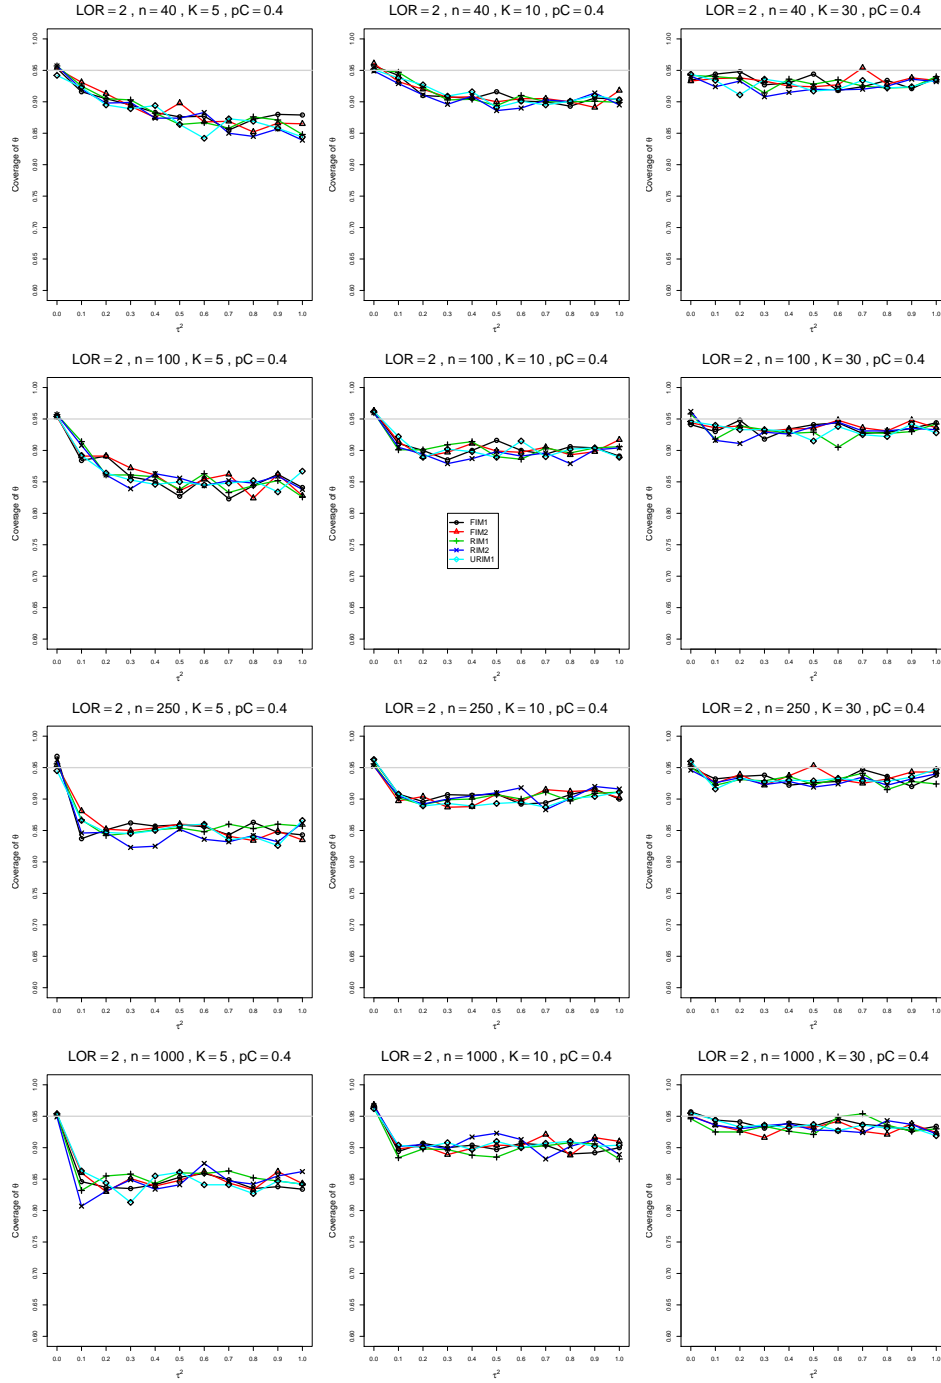

Figure A3.5.20: Coverage of the Fixed-intercept with  $c = 1/2$  confidence interval for  $\theta = 2$ ,  $p_C = 0.4$ ,  $\sigma^2 = 0.4$ , constant sample sizes  $n = 40, 100, 250, 1000$ . The data-generation mechanisms are FIM1 ( $\circ$ ), FIM2 ( $\triangle$ ), RIM1 ( $+$ ), RIM2 ( $\times$ ), and URIM1 ( $\diamond$ ).

### A3.6 Coverage of $\hat{\theta}_{RIM2}$

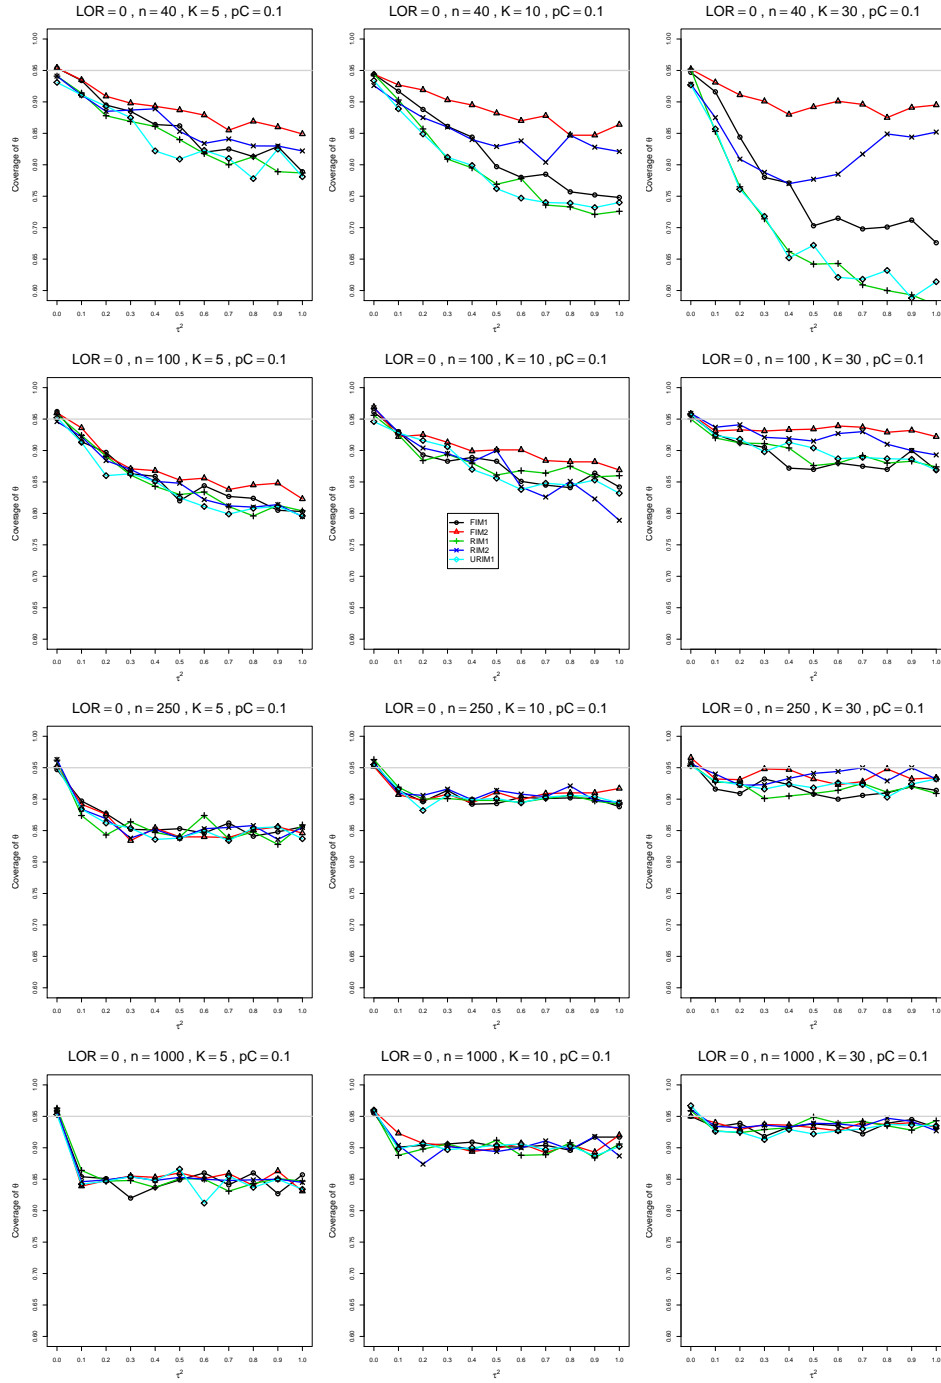

Figure A3.6.1: Coverage of the Random-intercept with  $c = 1/2$  confidence interval for  $\theta = 0$ ,  $p_C = 0.1$ ,  $\sigma^2 = 0.1$ , constant sample sizes  $n = 40, 100, 250, 1000$ . The data-generation mechanisms are FIM1 ( $\circ$ ), FIM2 ( $\triangle$ ), RIM1 ( $+$ ), RIM2 ( $\times$ ), and URIM1 ( $\diamond$ ).

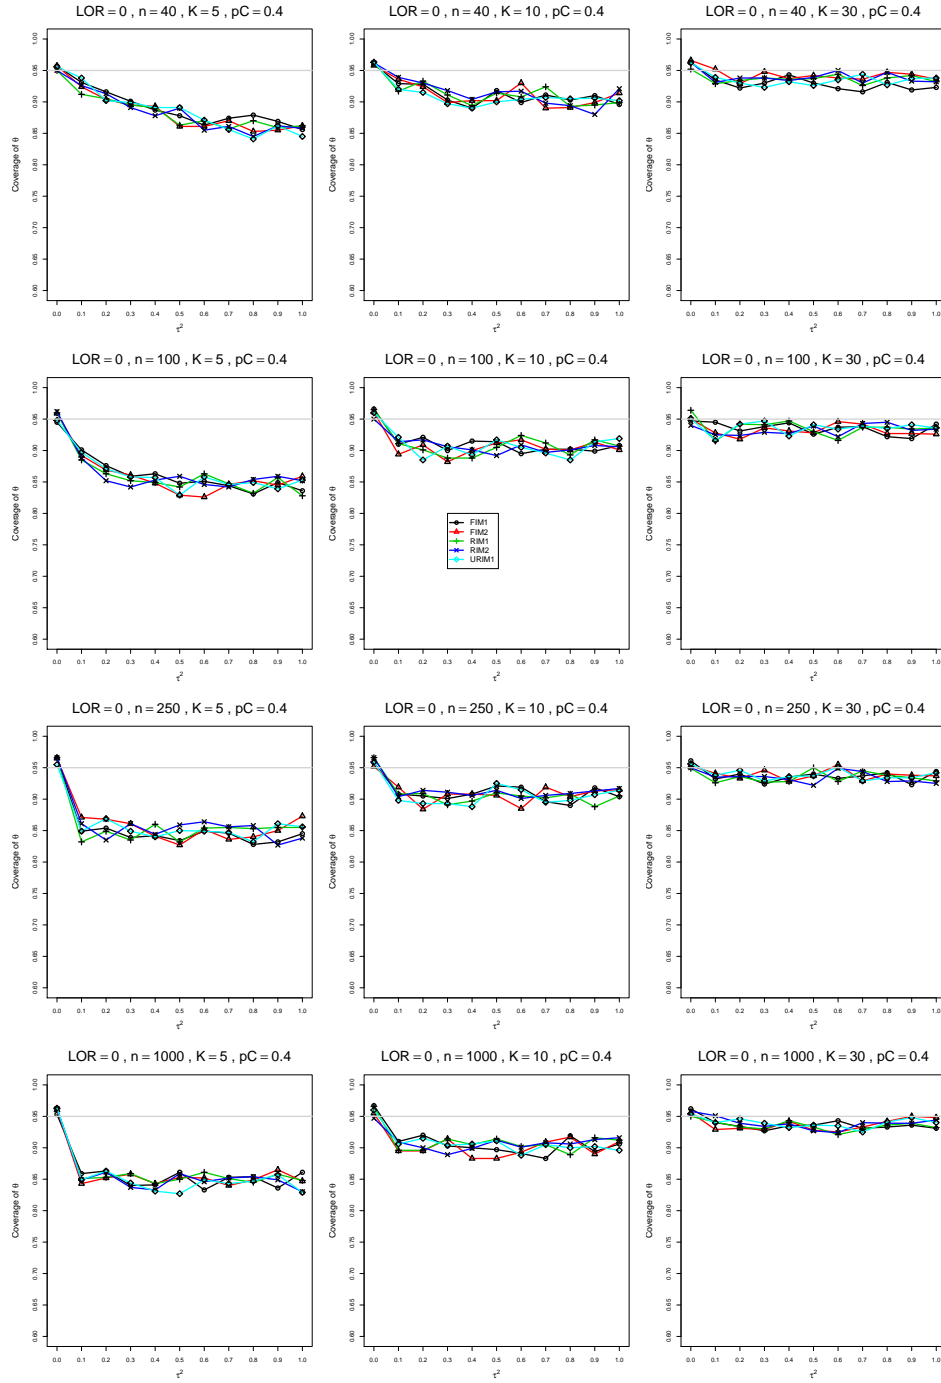

Figure A3.6.2: Coverage of the Random-intercept with  $c = 1/2$  confidence interval for  $\theta = 0$ ,  $p_C = 0.4$ ,  $\sigma^2 = 0.1$ , constant sample sizes  $n = 40, 100, 250, 1000$ . The data-generation mechanisms are FIM1 ( $\circ$ ), FIM2 ( $\triangle$ ), RIM1 ( $+$ ), RIM2 ( $\times$ ), and URIM1 ( $\diamond$ ).

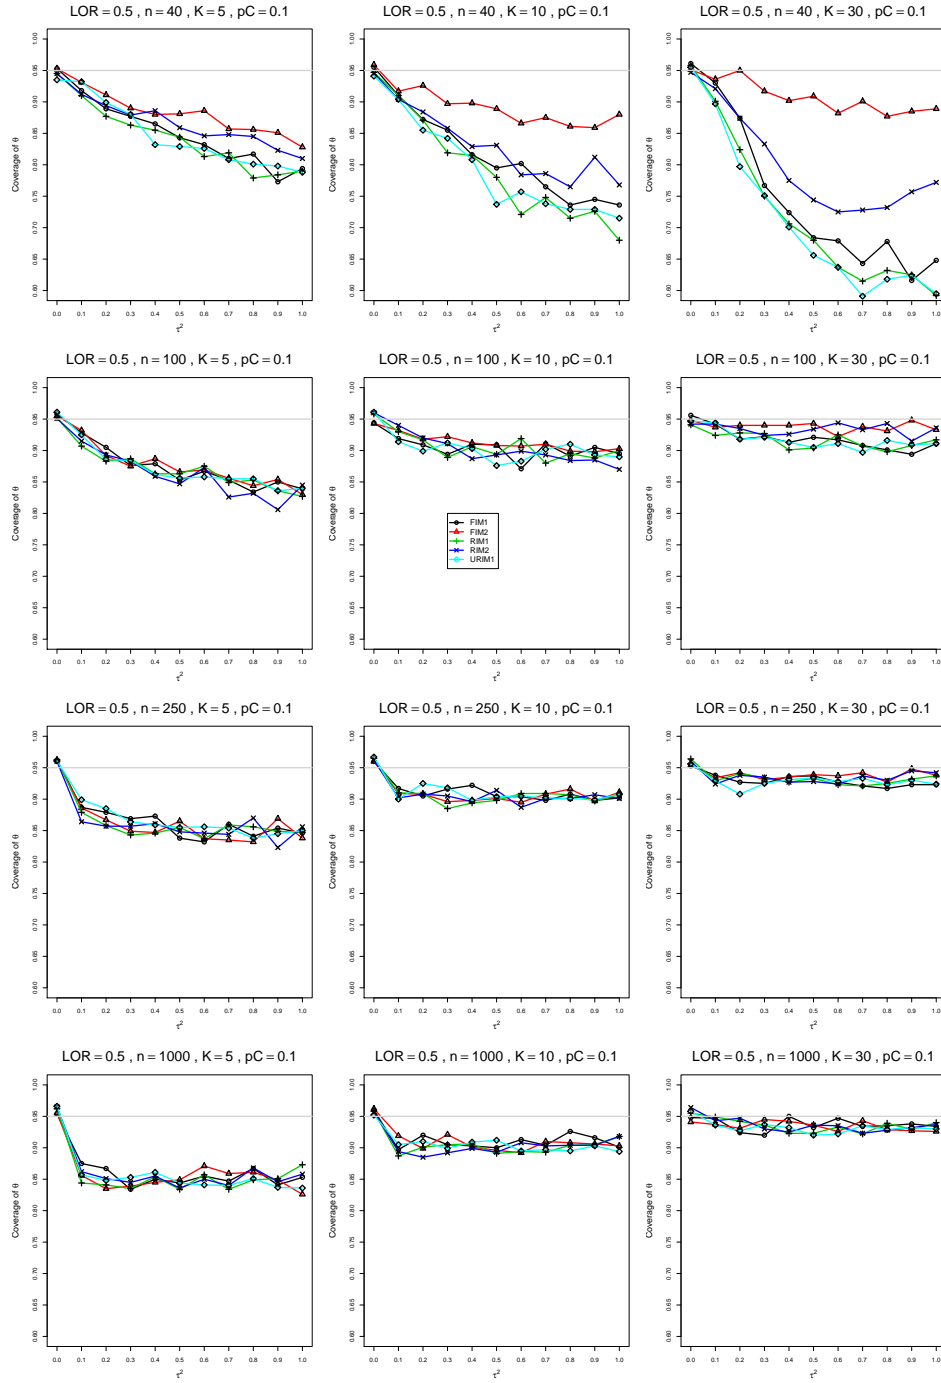

Figure A3.6.3: Coverage of the Random-intercept with  $c = 1/2$  confidence interval for  $\theta = 0.5$ ,  $p_C = 0.1$ ,  $\sigma^2 = 0.1$ , constant sample sizes  $n = 40, 100, 250, 1000$ . The data-generation mechanisms are FIM1 ( $\circ$ ), FIM2 ( $\triangle$ ), RIM1 ( $+$ ), RIM2 ( $\times$ ), and URIM1 ( $\diamond$ ).

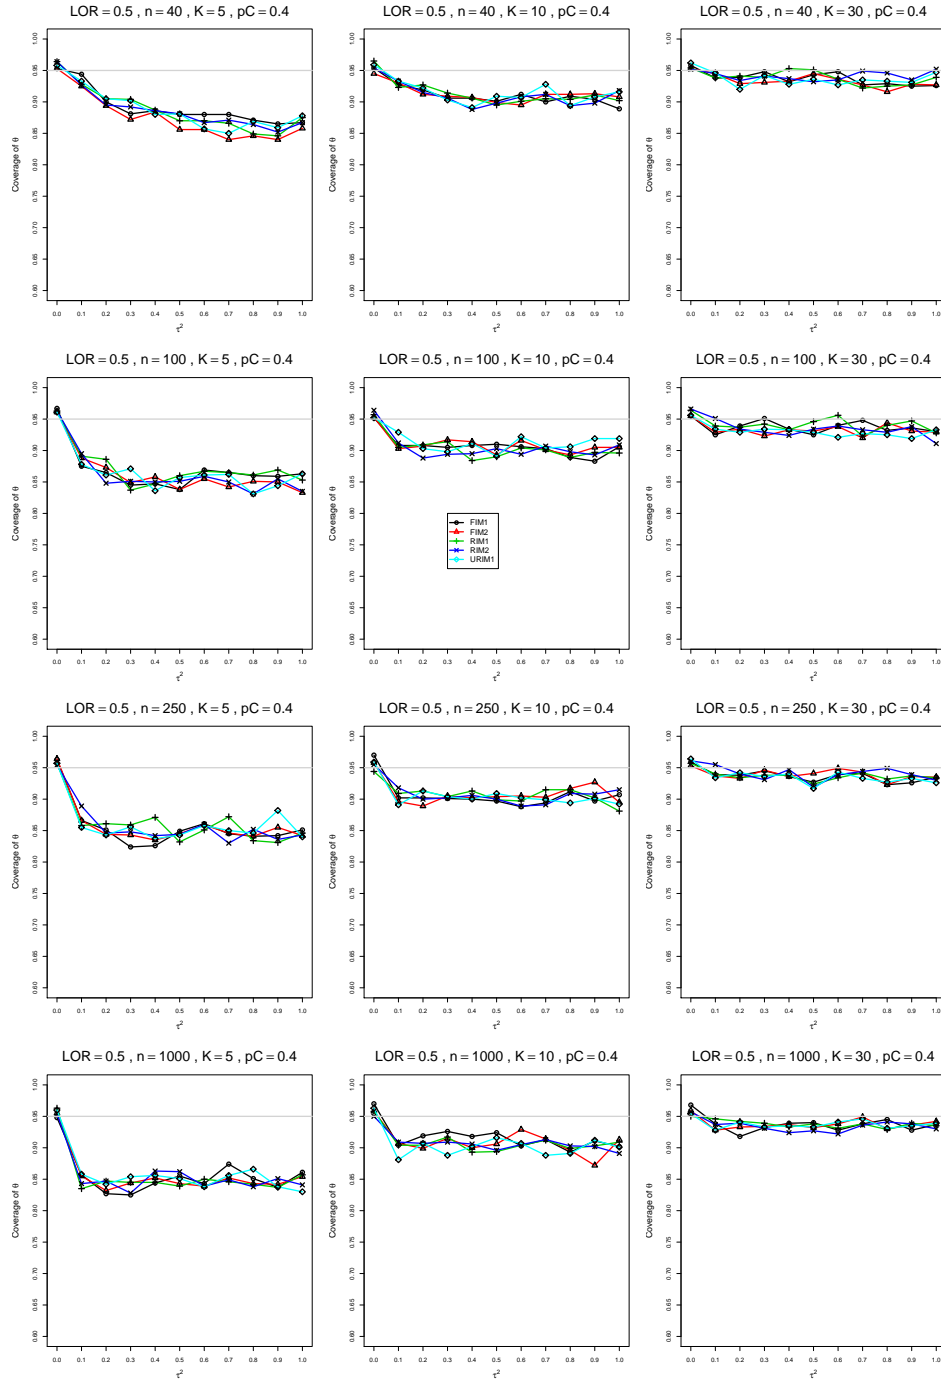

Figure A3.6.4: Coverage of the Random-intercept with  $c = 1/2$  confidence interval for  $\theta = 0.5$ ,  $p_C = 0.4$ ,  $\sigma^2 = 0.1$ , constant sample sizes  $n = 40, 100, 250, 1000$ . The data-generation mechanisms are FIM1 ( $\circ$ ), FIM2 ( $\triangle$ ), RIM1 ( $+$ ), RIM2 ( $\times$ ), and URIM1 ( $\diamond$ ).

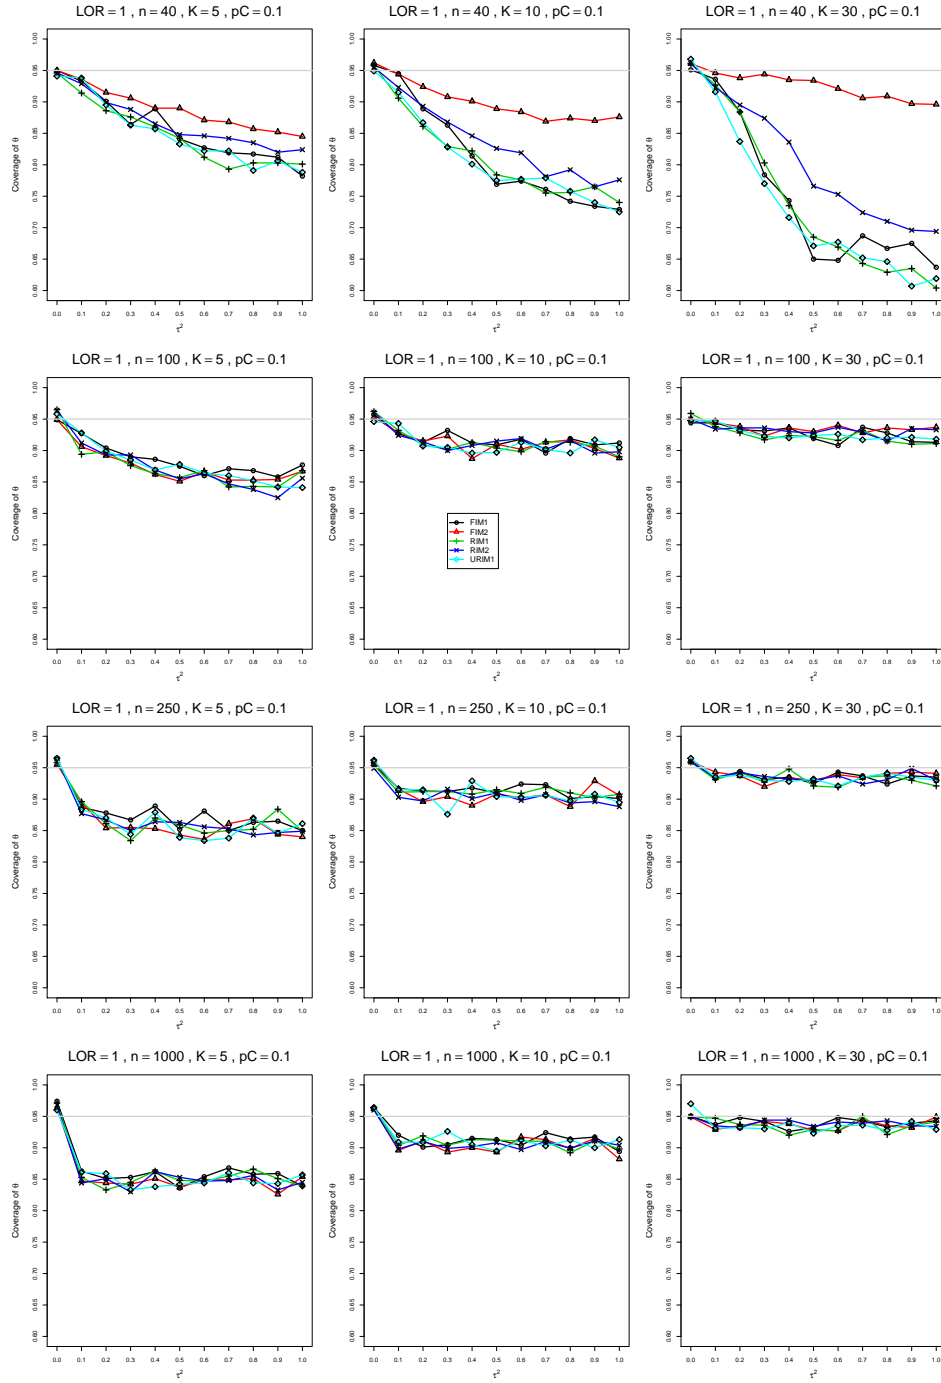

Figure A3.6.5: Coverage of the Random-intercept with  $c = 1/2$  confidence interval for  $\theta = 1$ ,  $p_C = 0.1$ ,  $\sigma^2 = 0.1$ , constant sample sizes  $n = 40, 100, 250, 1000$ . The data-generation mechanisms are FIM1 ( $\circ$ ), FIM2 ( $\triangle$ ), RIM1 ( $+$ ), RIM2 ( $\times$ ), and URIM1 ( $\diamond$ ).



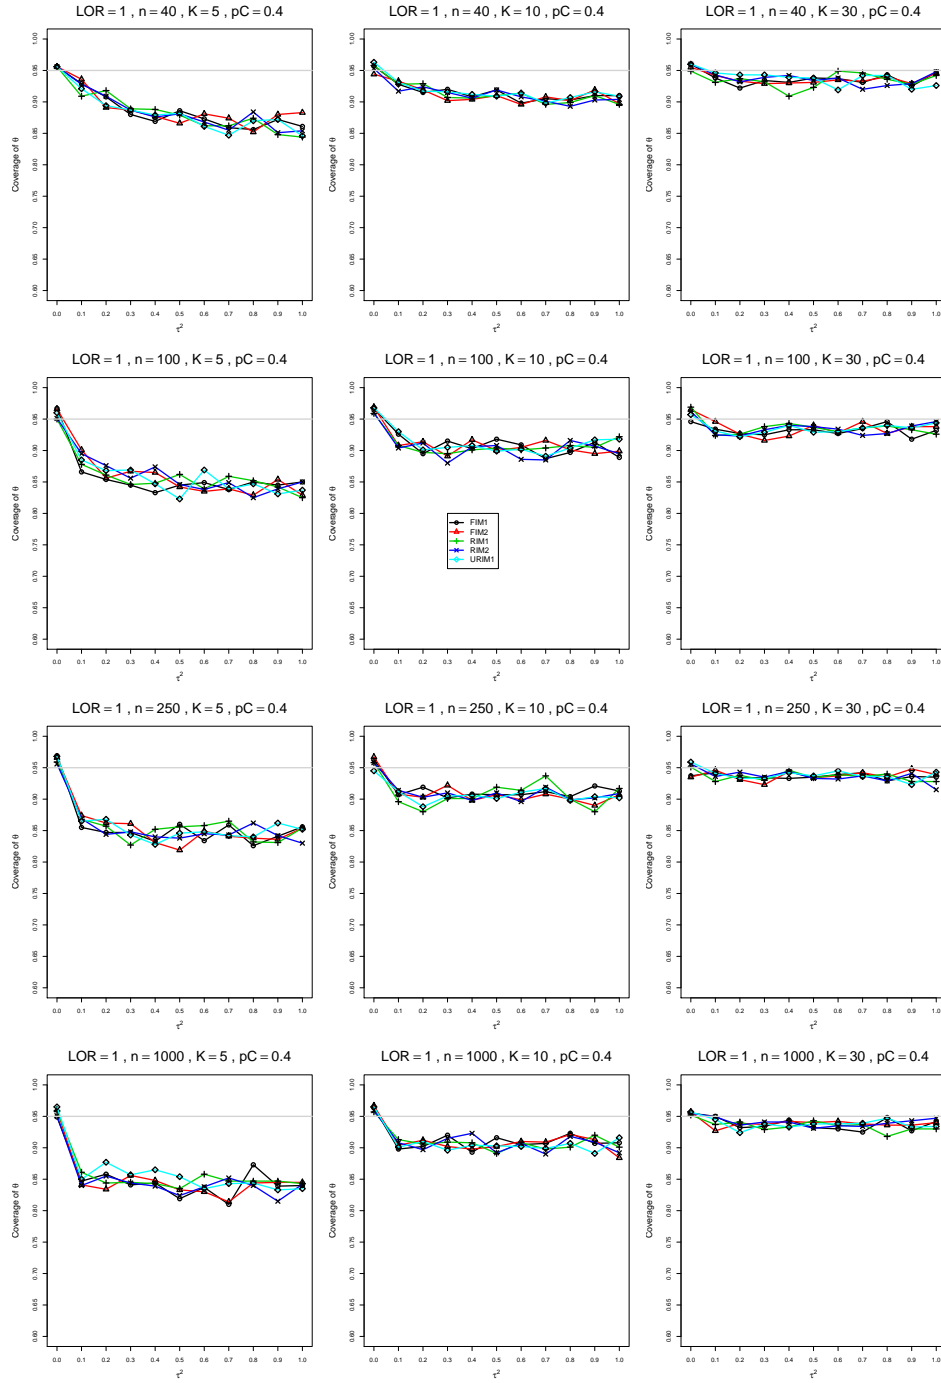

Figure A3.6.6: Coverage of the Random-intercept with  $c = 1/2$  confidence interval for  $\theta = 1$ ,  $p_C = 0.4$ ,  $\sigma^2 = 0.1$ , constant sample sizes  $n = 40, 100, 250, 1000$ . The data-generation mechanisms are FIM1 ( $\circ$ ), FIM2 ( $\triangle$ ), RIM1 ( $+$ ), RIM2 ( $\times$ ), and URIM1 ( $\diamond$ ).

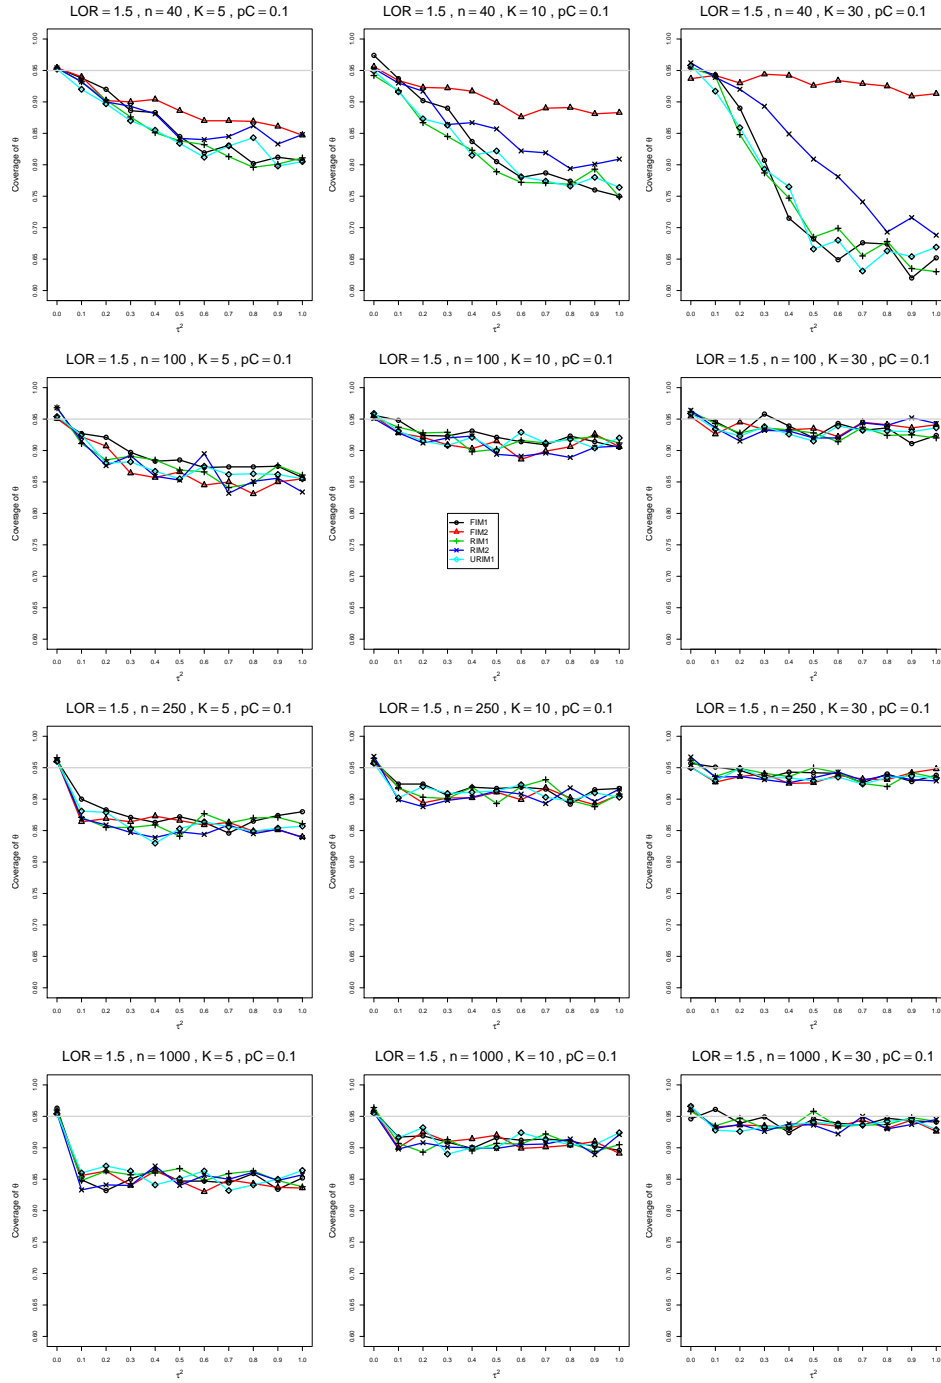

Figure A3.6.7: Coverage of the Random-intercept with  $c = 1/2$  confidence interval for  $\theta = 1.5$ ,  $p_C = 0.1$ ,  $\sigma^2 = 0.1$ , constant sample sizes  $n = 40, 100, 250, 1000$ . The data-generation mechanisms are FIM1 ( $\circ$ ), FIM2 ( $\triangle$ ), RIM1 ( $+$ ), RIM2 ( $\times$ ), and URIM1 ( $\diamond$ ).

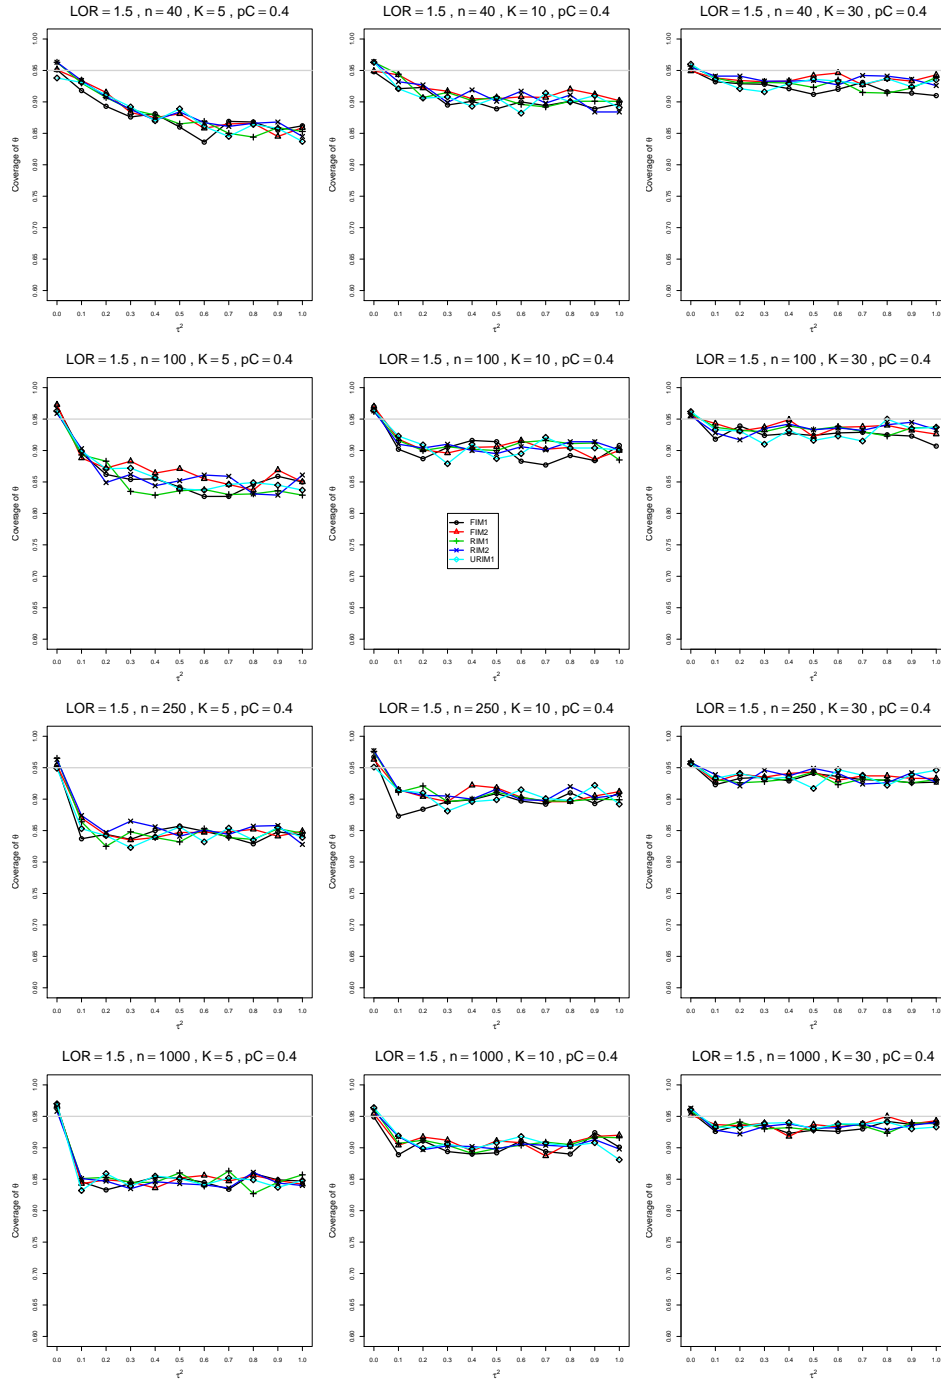

Figure A3.6.8: Coverage of the Random-intercept with  $c = 1/2$  confidence interval for  $\theta = 1.5$ ,  $p_C = 0.4$ ,  $\sigma^2 = 0.1$ , constant sample sizes  $n = 40, 100, 250, 1000$ . The data-generation mechanisms are FIM1 ( $\circ$ ), FIM2 ( $\triangle$ ), RIM1 ( $+$ ), RIM2 ( $\times$ ), and URIM1 ( $\diamond$ ).

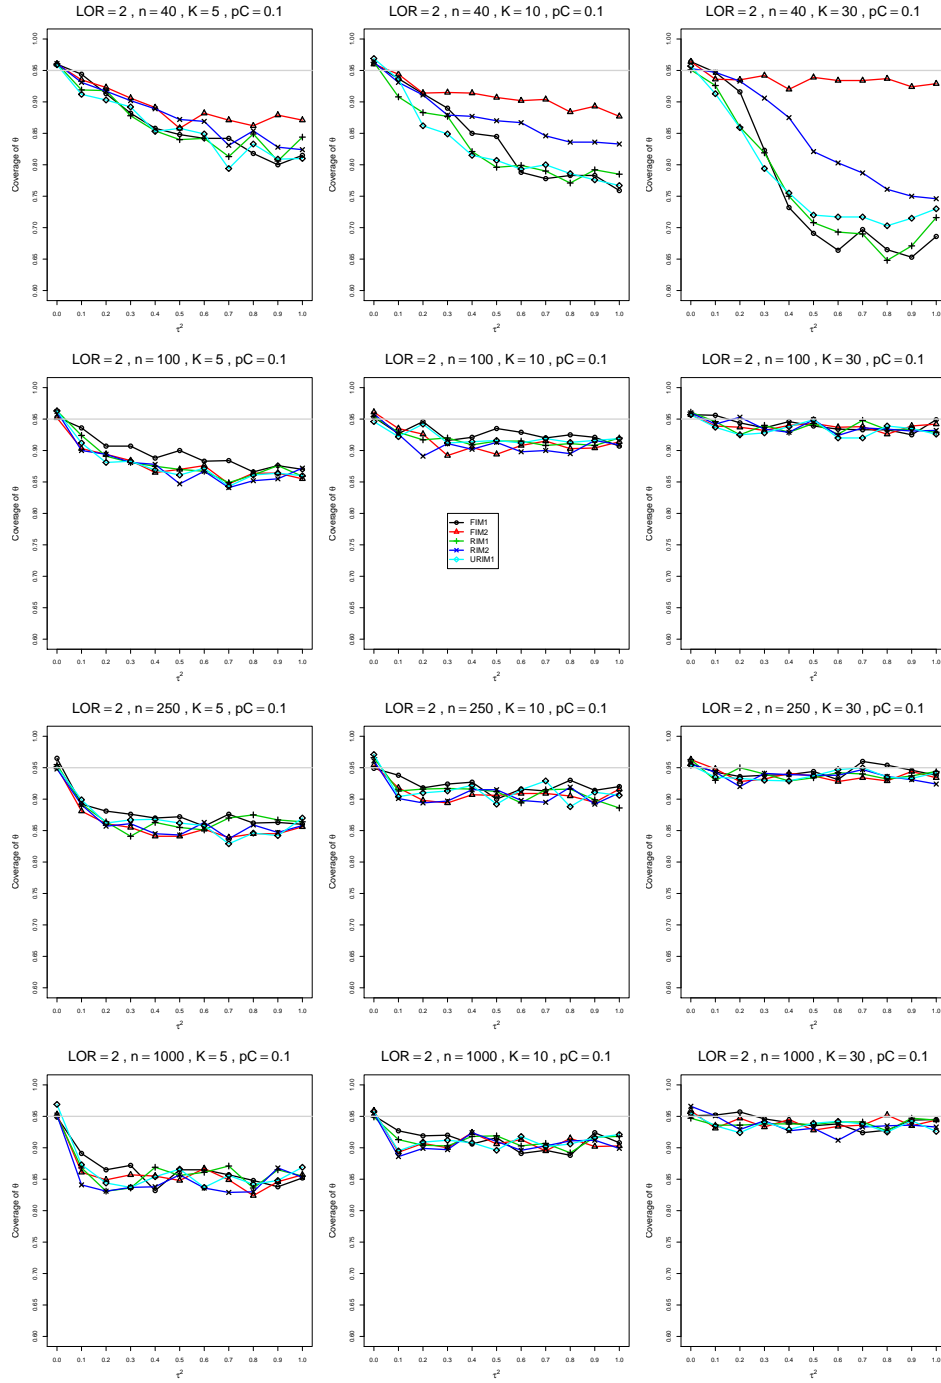

Figure A3.6.9: Coverage of the Random-intercept with  $c = 1/2$  confidence interval for  $\theta = 2$ ,  $p_C = 0.1$ ,  $\sigma^2 = 0.1$ , constant sample sizes  $n = 40, 100, 250, 1000$ . The data-generation mechanisms are FIM1 ( $\circ$ ), FIM2 ( $\triangle$ ), RIM1 ( $+$ ), RIM2 ( $\times$ ), and URIM1 ( $\diamond$ ).

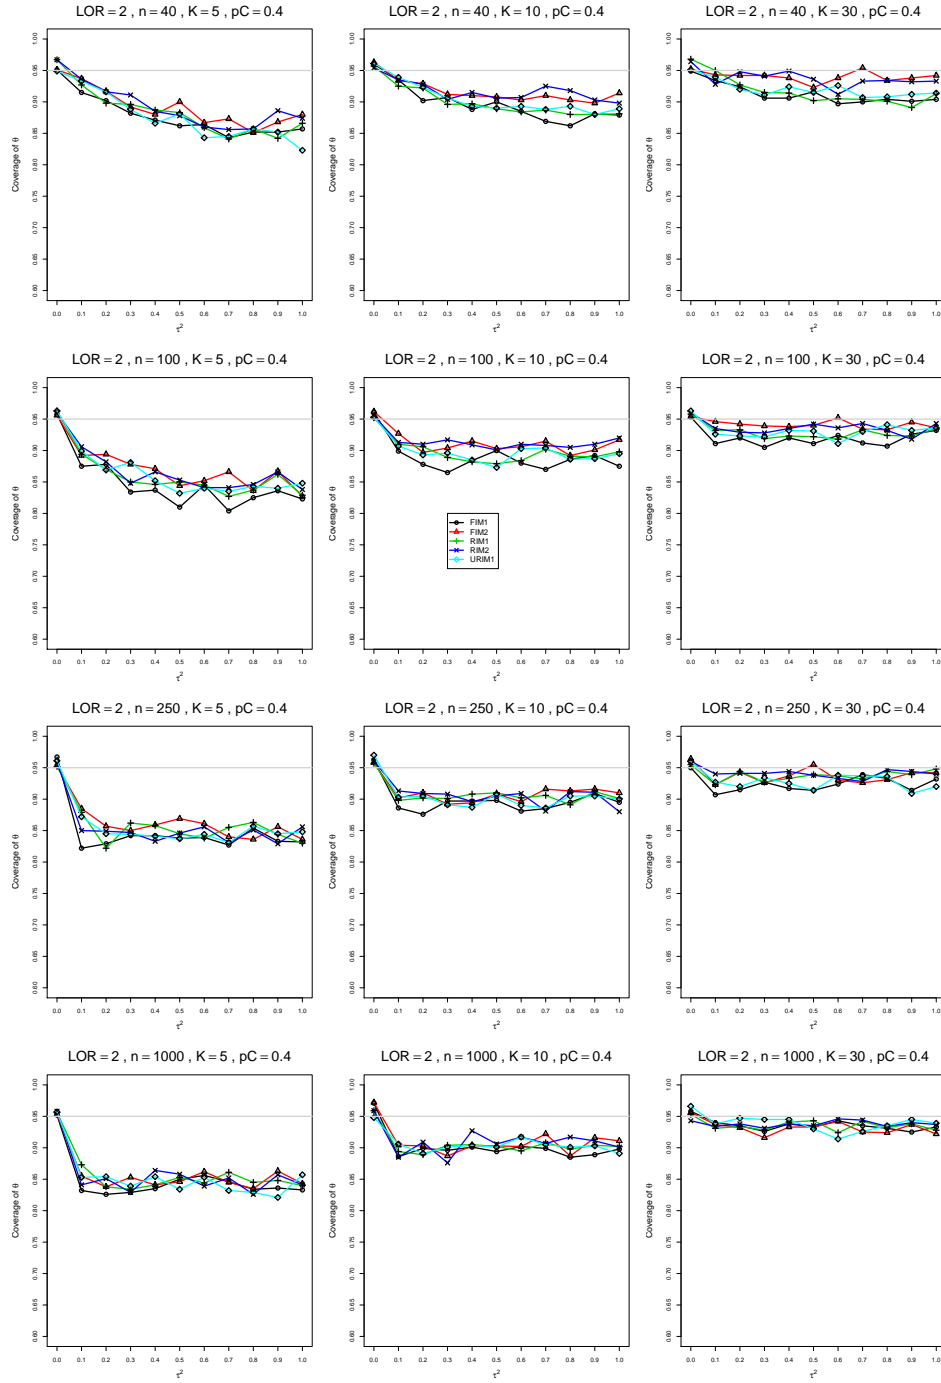

Figure A3.6.10: Coverage of the Random-intercept with  $c = 1/2$  confidence interval for  $\theta = 2$ ,  $p_C = 0.4$ ,  $\sigma^2 = 0.1$ , constant sample sizes  $n = 40, 100, 250, 1000$ . The data-generation mechanisms are FIM1 ( $\circ$ ), FIM2 ( $\triangle$ ), RIM1 ( $+$ ), RIM2 ( $\times$ ), and URIM1 ( $\diamond$ ).

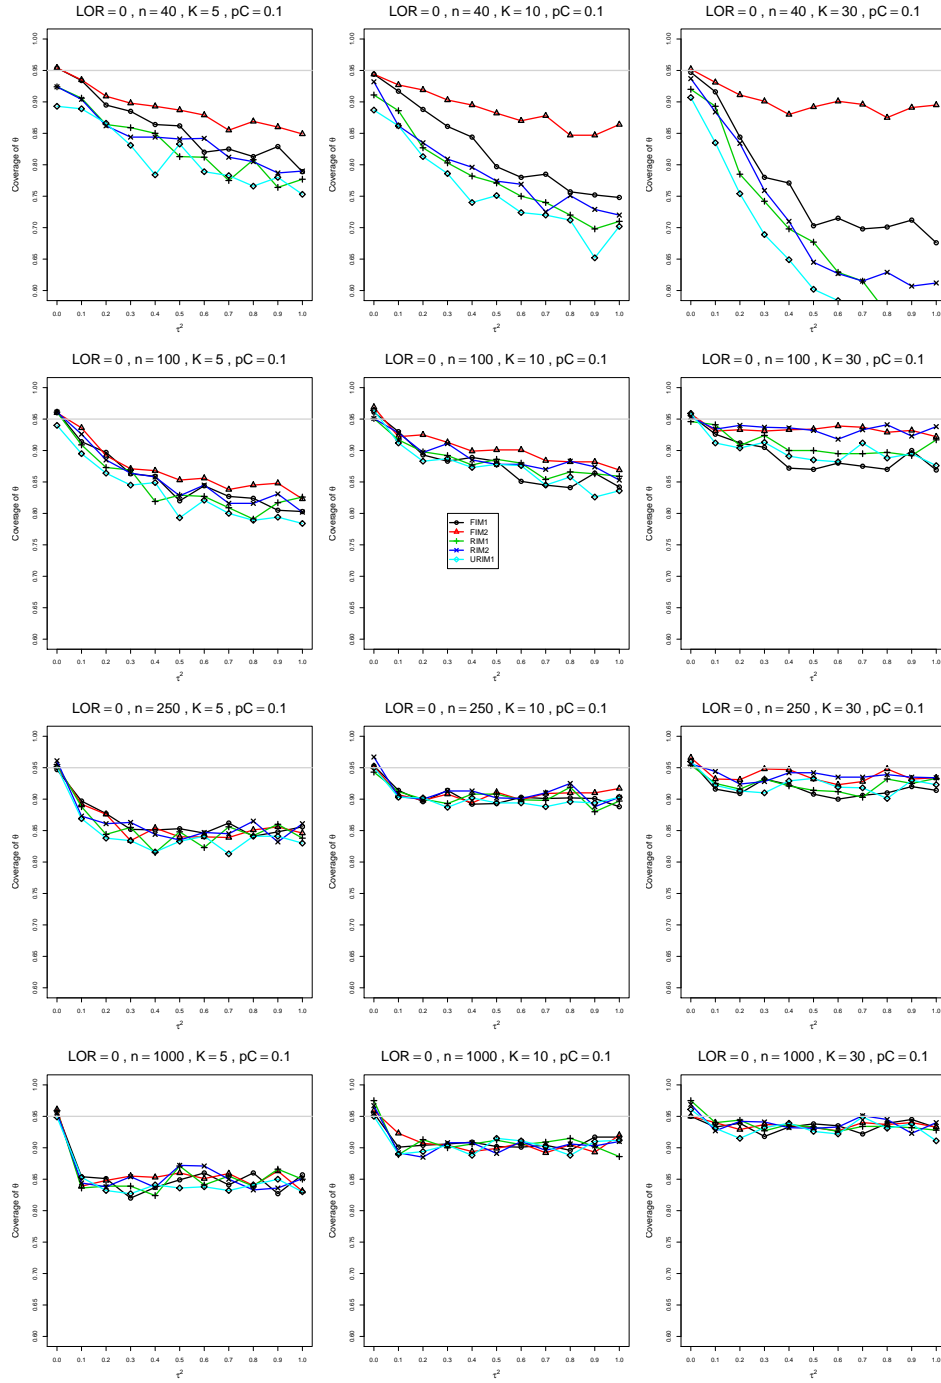

Figure A3.6.11: Coverage of the Random-intercept with  $c = 1/2$  confidence interval for  $\theta = 0$ ,  $p_C = 0.1$ ,  $\sigma^2 = 0.4$ , constant sample sizes  $n = 40, 100, 250, 1000$ . The data-generation mechanisms are FIM1 ( $\circ$ ), FIM2 ( $\triangle$ ), RIM1 ( $+$ ), RIM2 ( $\times$ ), and URIM1 ( $\diamond$ ).

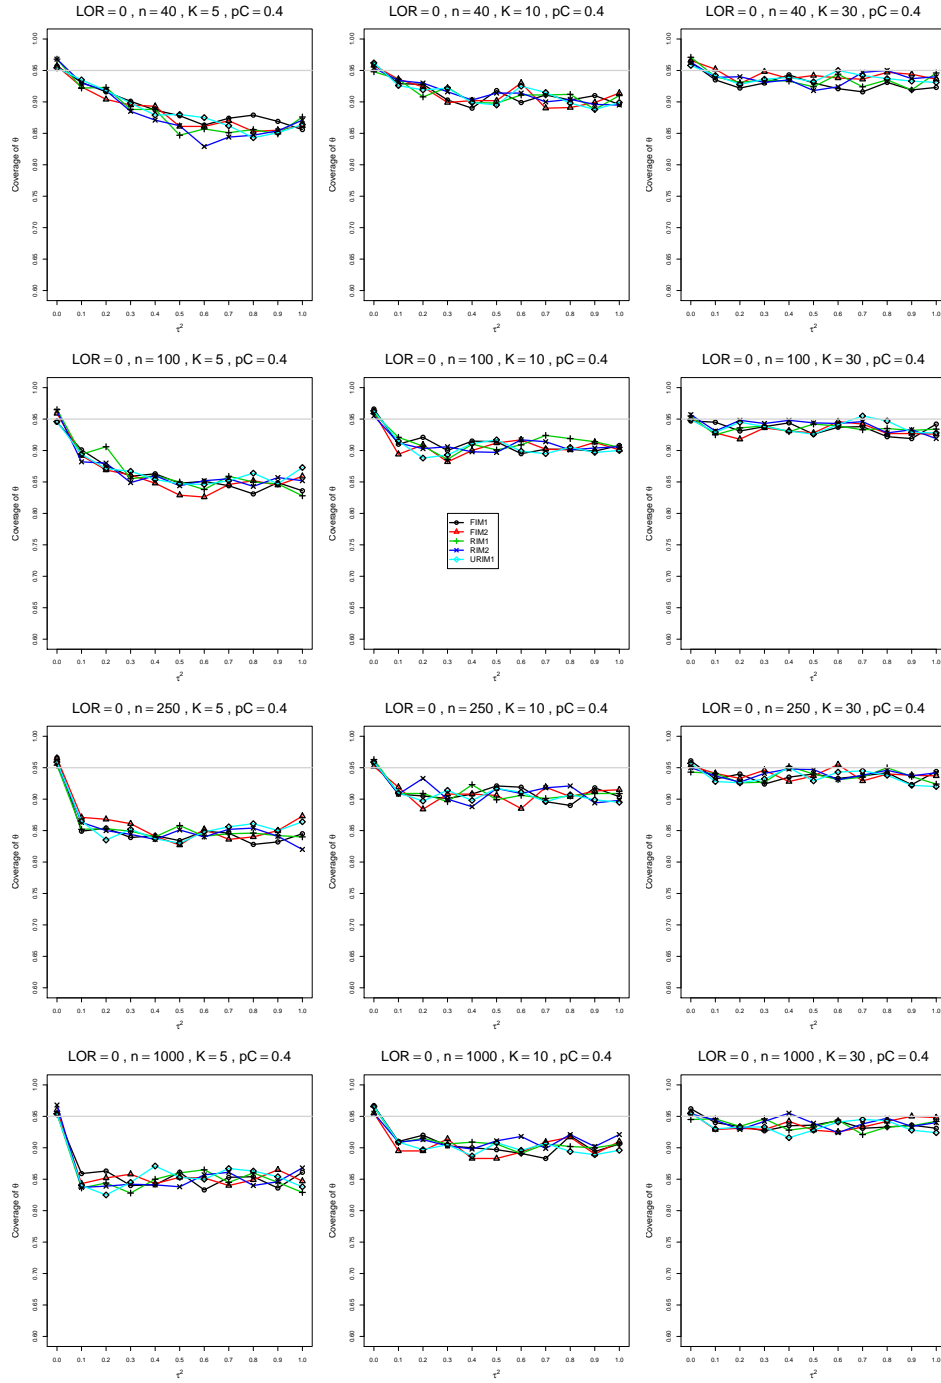

Figure A3.6.12: Coverage of the Random-intercept with  $c = 1/2$  confidence interval for  $\theta = 0$ ,  $p_C = 0.4$ ,  $\sigma^2 = 0.4$ , constant sample sizes  $n = 40, 100, 250, 1000$ . The data-generation mechanisms are FIM1 ( $\circ$ ), FIM2 ( $\triangle$ ), RIM1 (+), RIM2 ( $\times$ ), and URIM1 ( $\diamond$ ).

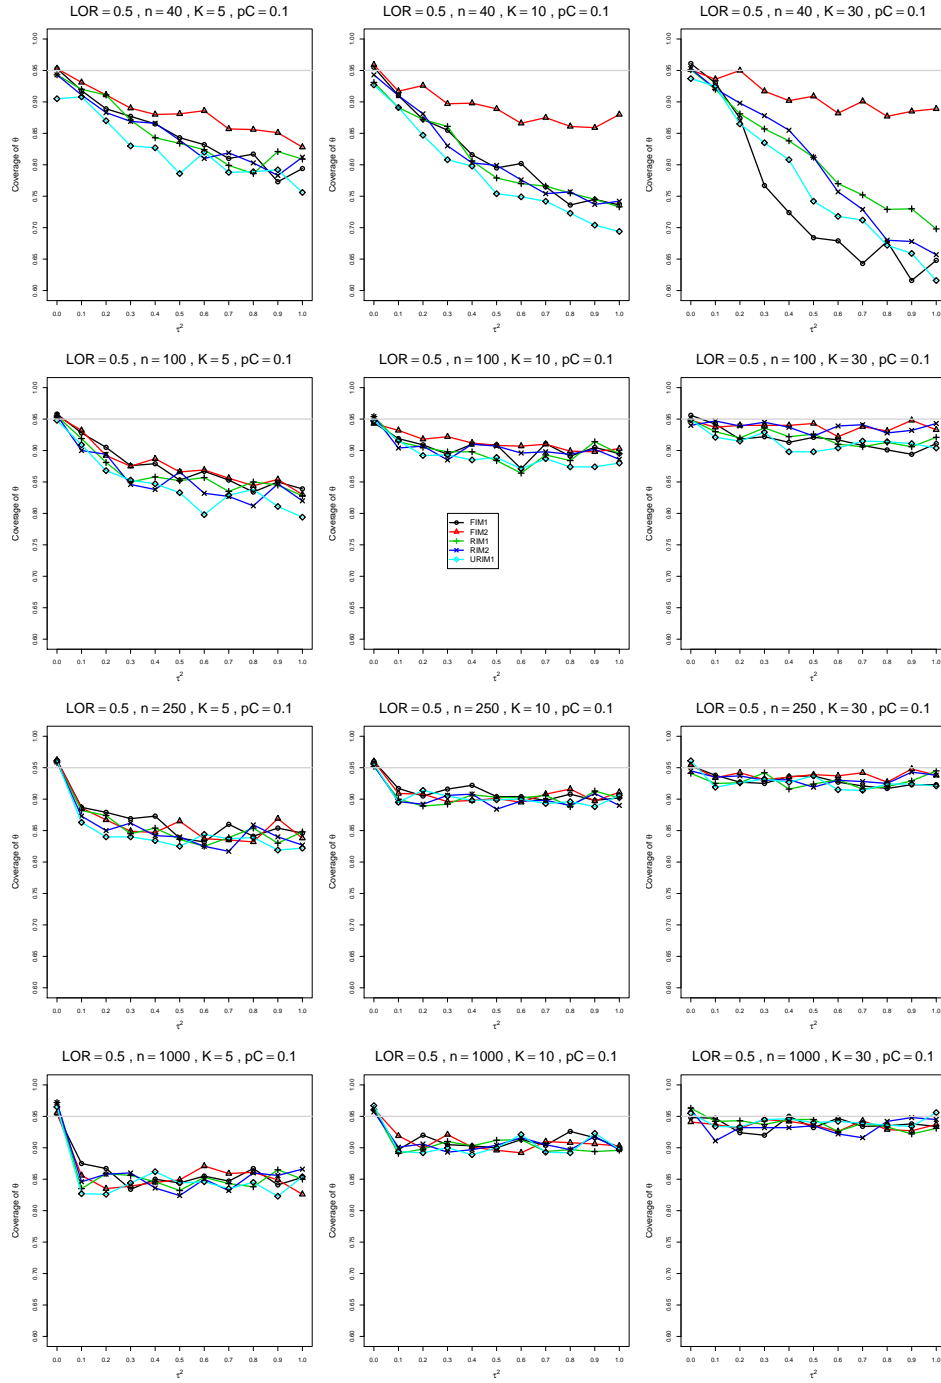

Figure A3.6.13: Coverage of the Random-intercept with  $c = 1/2$  confidence interval for  $\theta = 0.5$ ,  $p_C = 0.1$ ,  $\sigma^2 = 0.4$ , constant sample sizes  $n = 40, 100, 250, 1000$ . The data-generation mechanisms are FIM1 ( $\circ$ ), FIM2 ( $\triangle$ ), RIM1 ( $+$ ), RIM2 ( $\times$ ), and URIM1 ( $\diamond$ ).



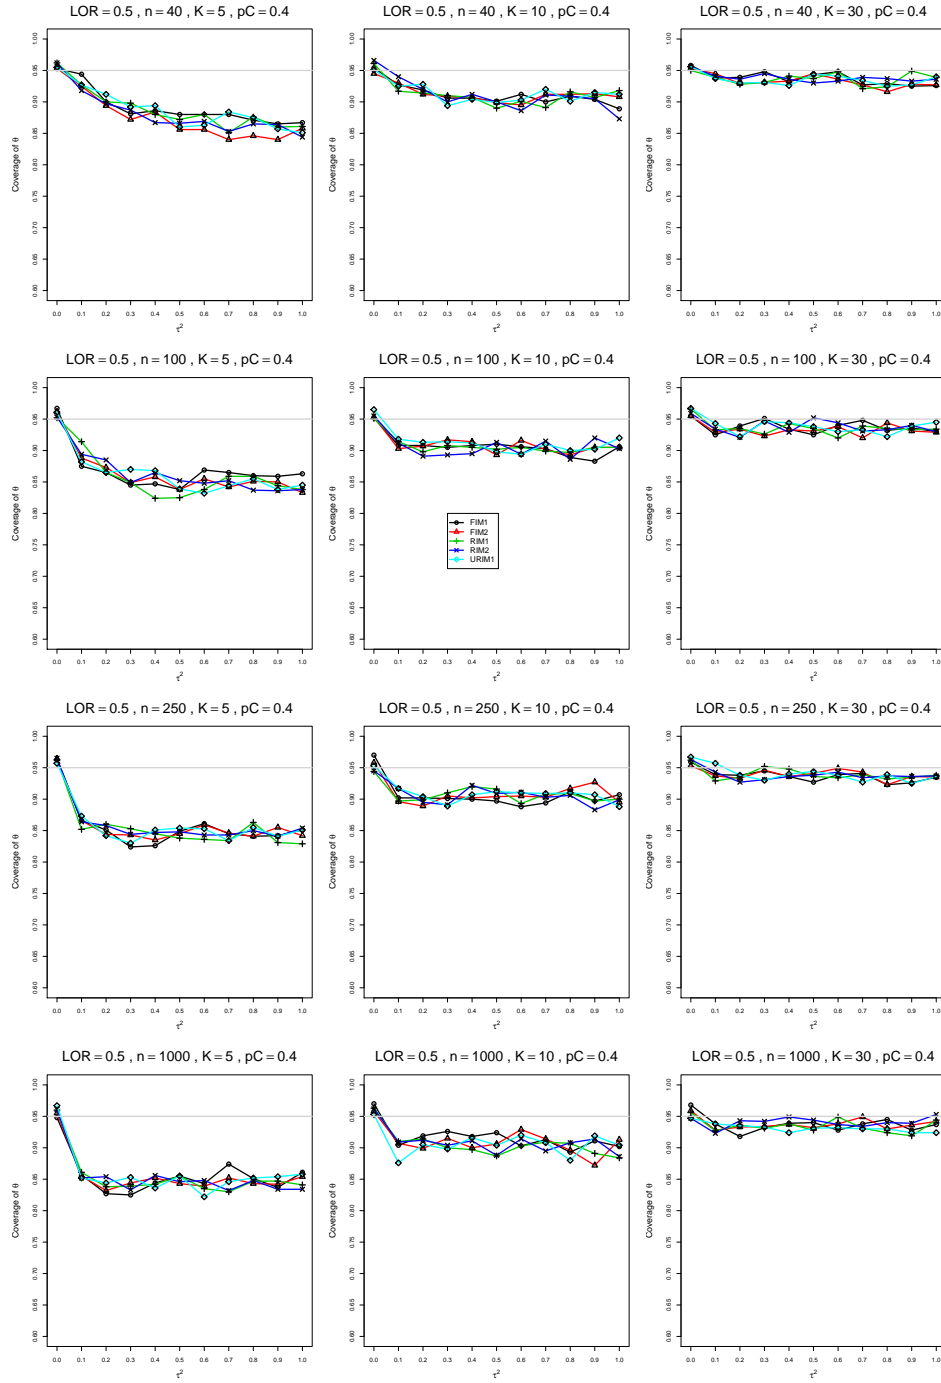

Figure A3.6.14: Coverage of the Random-intercept with  $c = 1/2$  confidence interval for  $\theta = 0.5$ ,  $p_C = 0.4$ ,  $\sigma^2 = 0.4$ , constant sample sizes  $n = 40, 100, 250, 1000$ . The data-generation mechanisms are FIM1 ( $\circ$ ), FIM2 ( $\triangle$ ), RIM1 ( $+$ ), RIM2 ( $\times$ ), and URIM1 ( $\diamond$ ).

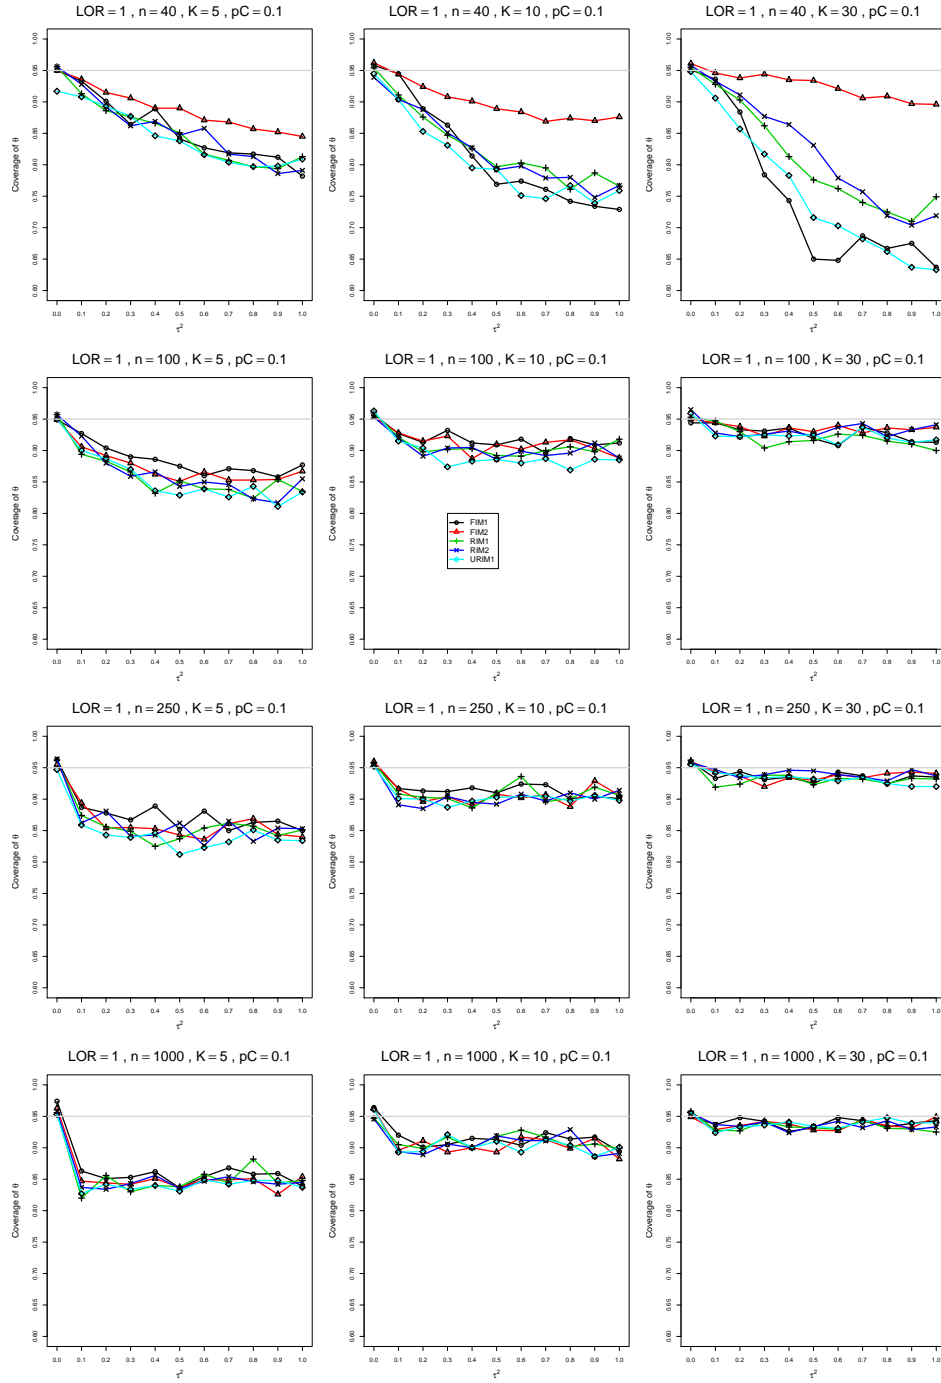

Figure A3.6.15: Coverage of the Random-intercept with  $c = 1/2$  confidence interval for  $\theta = 1$ ,  $p_C = 0.1$ ,  $\sigma^2 = 0.4$ , constant sample sizes  $n = 40, 100, 250, 1000$ . The data-generation mechanisms are FIM1 ( $\circ$ ), FIM2 ( $\triangle$ ), RIM1 ( $+$ ), RIM2 ( $\times$ ), and URIM1 ( $\diamond$ ).

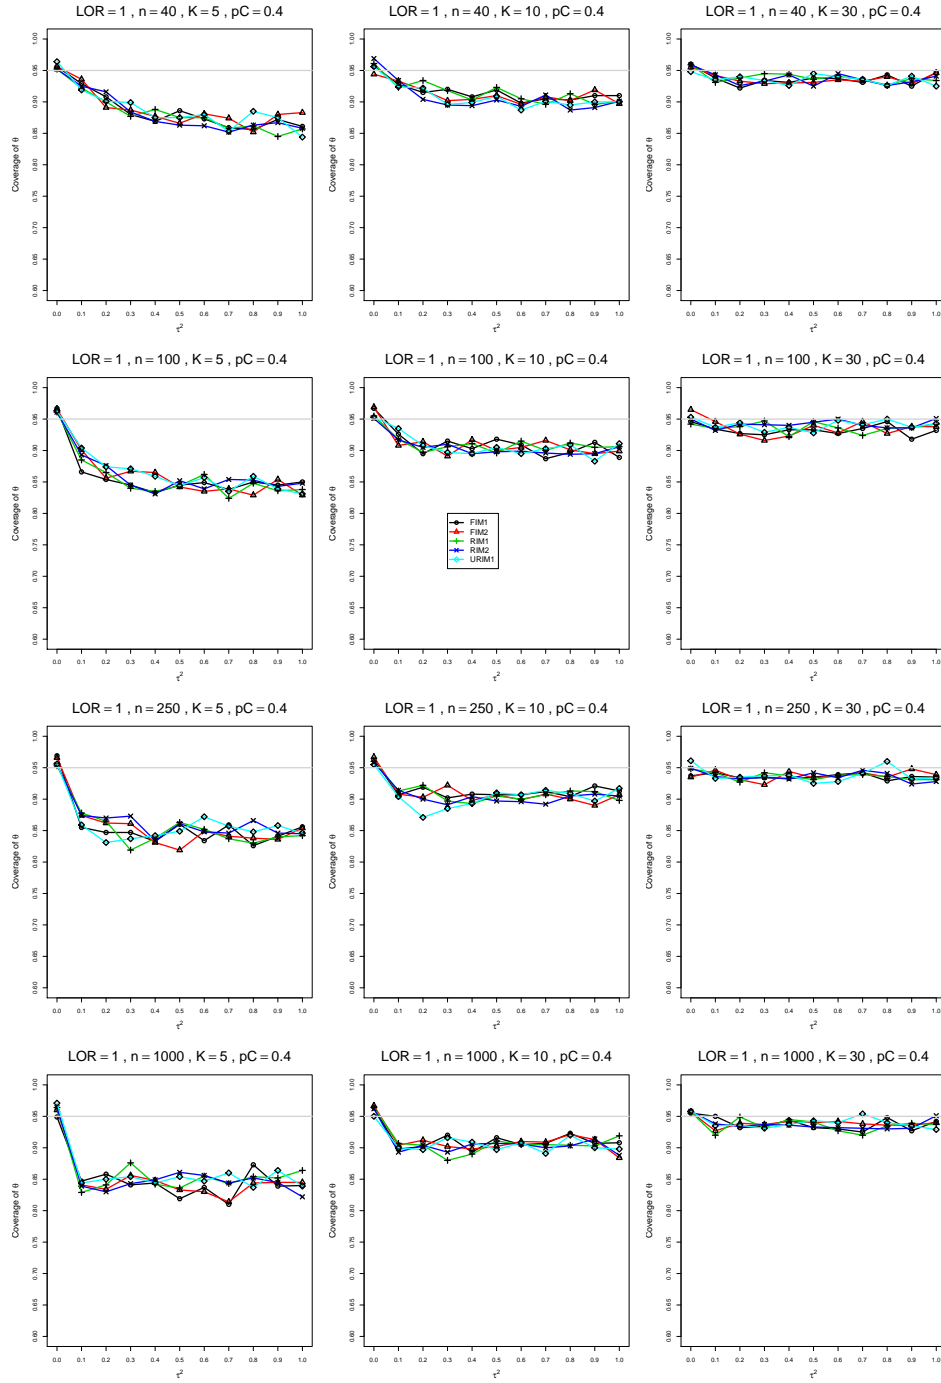

Figure A3.6.16: Coverage of the Random-intercept with  $c = 1/2$  confidence interval for  $\theta = 1$ ,  $p_C = 0.4$ ,  $\sigma^2 = 0.4$ , constant sample sizes  $n = 40, 100, 250, 1000$ . The data-generation mechanisms are FIM1 ( $\circ$ ), FIM2 ( $\triangle$ ), RIM1 ( $+$ ), RIM2 ( $\times$ ), and URIM1 ( $\diamond$ ).

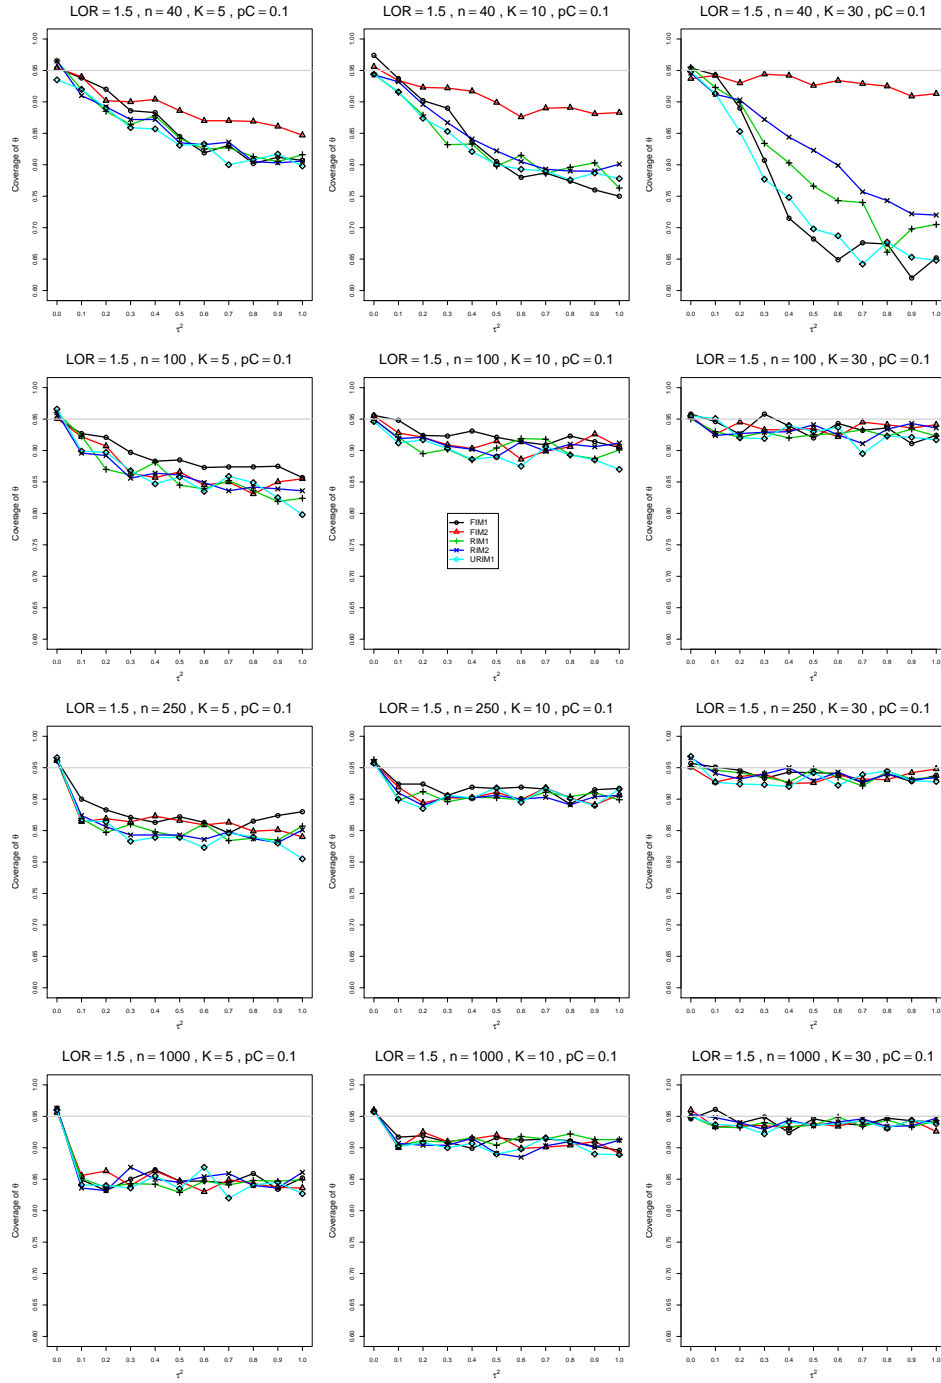

Figure A3.6.17: Coverage of the Random-intercept with  $c = 1/2$  confidence interval for  $\theta = 1.5$ ,  $p_C = 0.1$ ,  $\sigma^2 = 0.4$ , constant sample sizes  $n = 40, 100, 250, 1000$ . The data-generation mechanisms are FIM1 ( $\circ$ ), FIM2 ( $\triangle$ ), RIM1 ( $+$ ), RIM2 ( $\times$ ), and URIM1 ( $\diamond$ ).

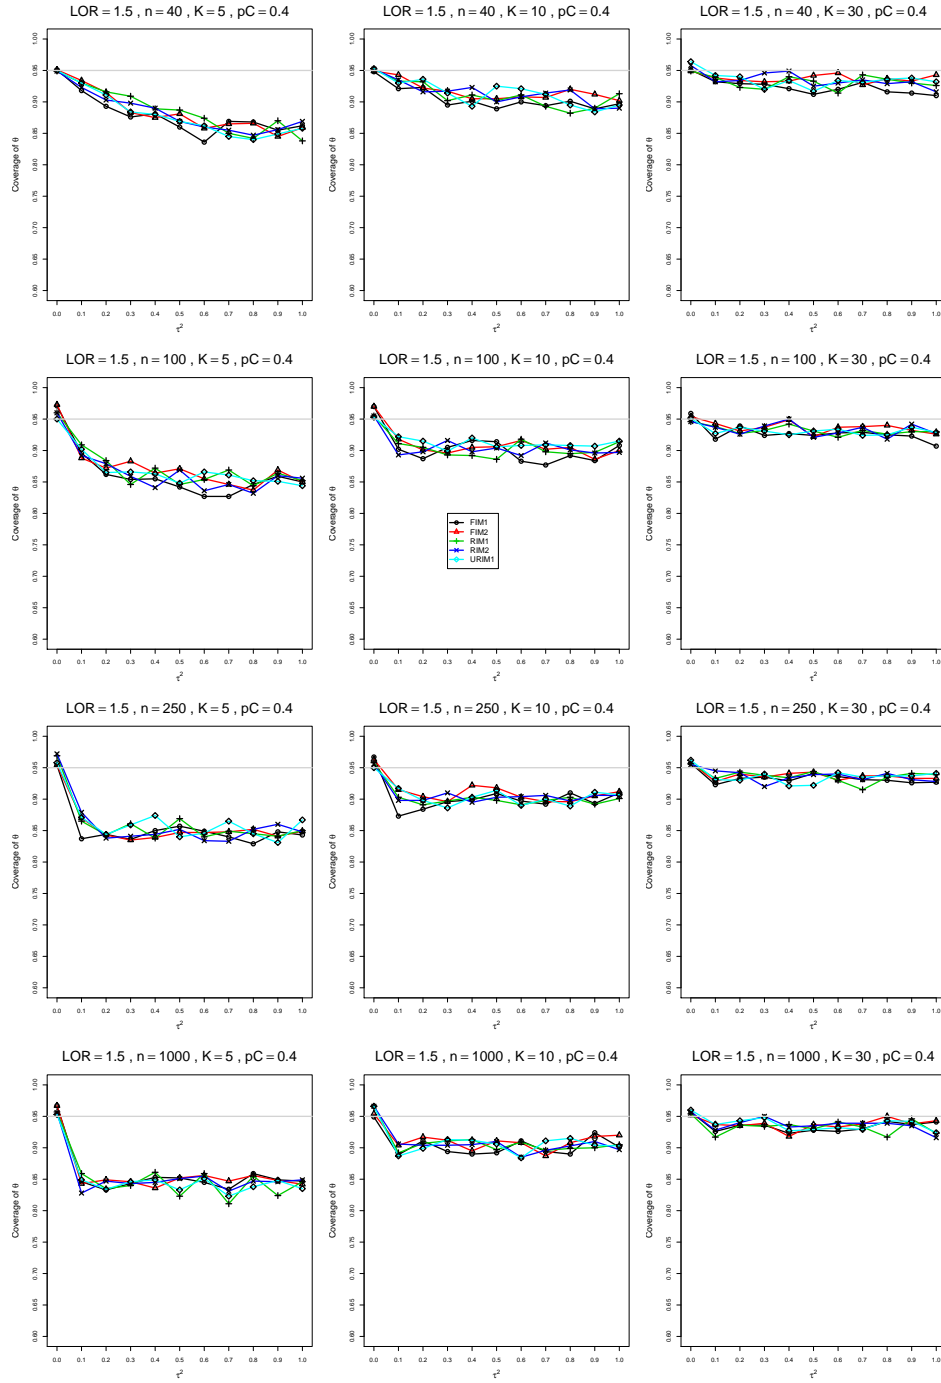

Figure A3.6.18: Coverage of the Random-intercept with  $c = 1/2$  confidence interval for  $\theta = 1.5$ ,  $p_C = 0.4$ ,  $\sigma^2 = 0.4$ , constant sample sizes  $n = 40, 100, 250, 1000$ . The data-generation mechanisms are FIM1 ( $\circ$ ), FIM2 ( $\triangle$ ), RIM1 ( $+$ ), RIM2 ( $\times$ ), and URIM1 ( $\diamond$ ).

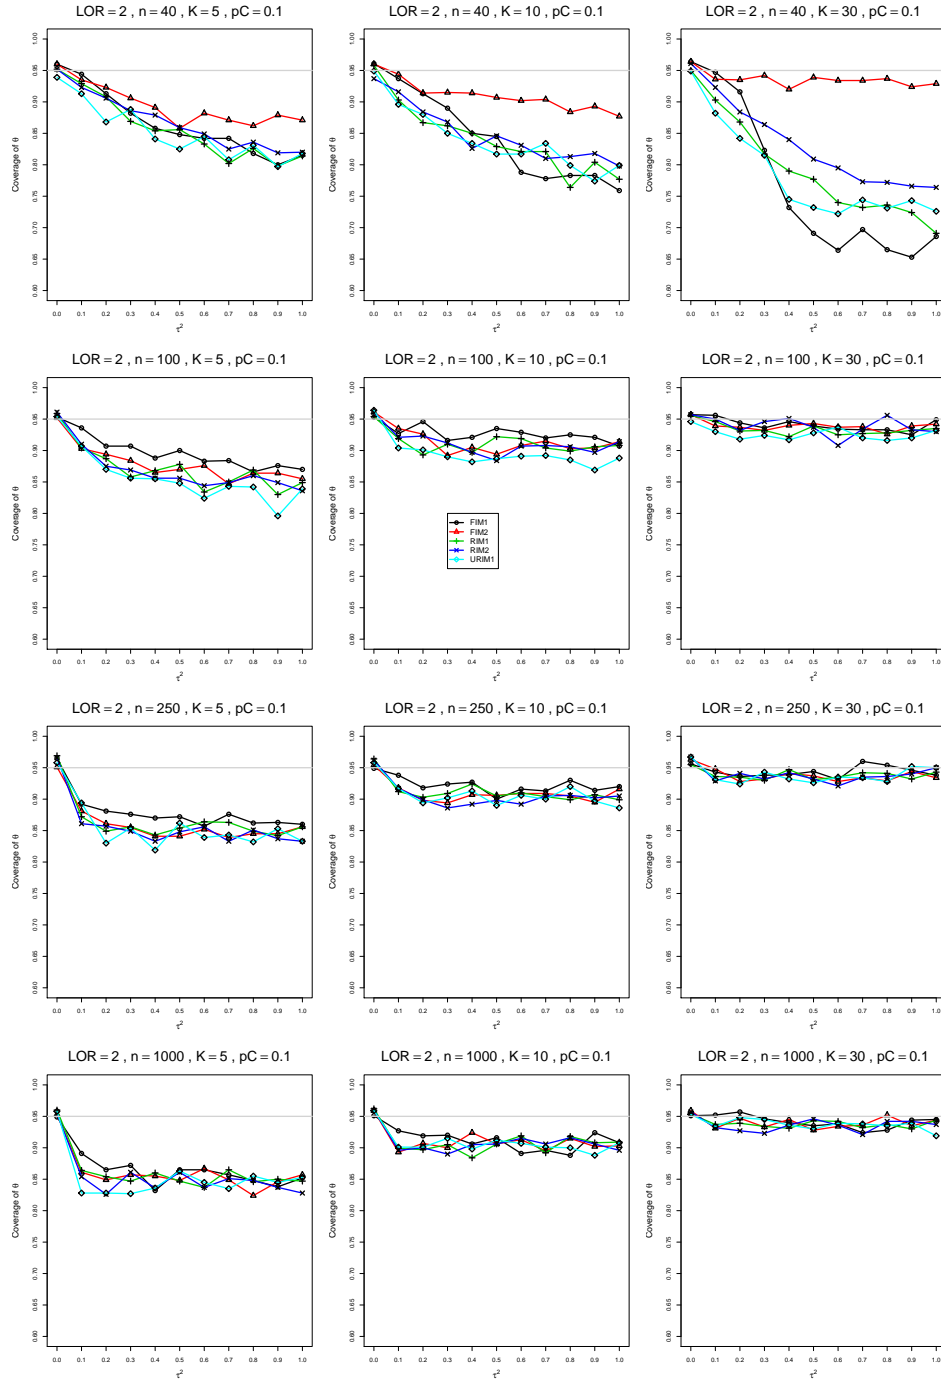

Figure A3.6.19: Coverage of the Random-intercept with  $c = 1/2$  confidence interval for  $\theta = 2$ ,  $p_C = 0.1$ ,  $\sigma^2 = 0.4$ , constant sample sizes  $n = 40, 100, 250, 1000$ . The data-generation mechanisms are FIM1 ( $\circ$ ), FIM2 ( $\triangle$ ), RIM1 ( $+$ ), RIM2 ( $\times$ ), and URIM1 ( $\diamond$ ).

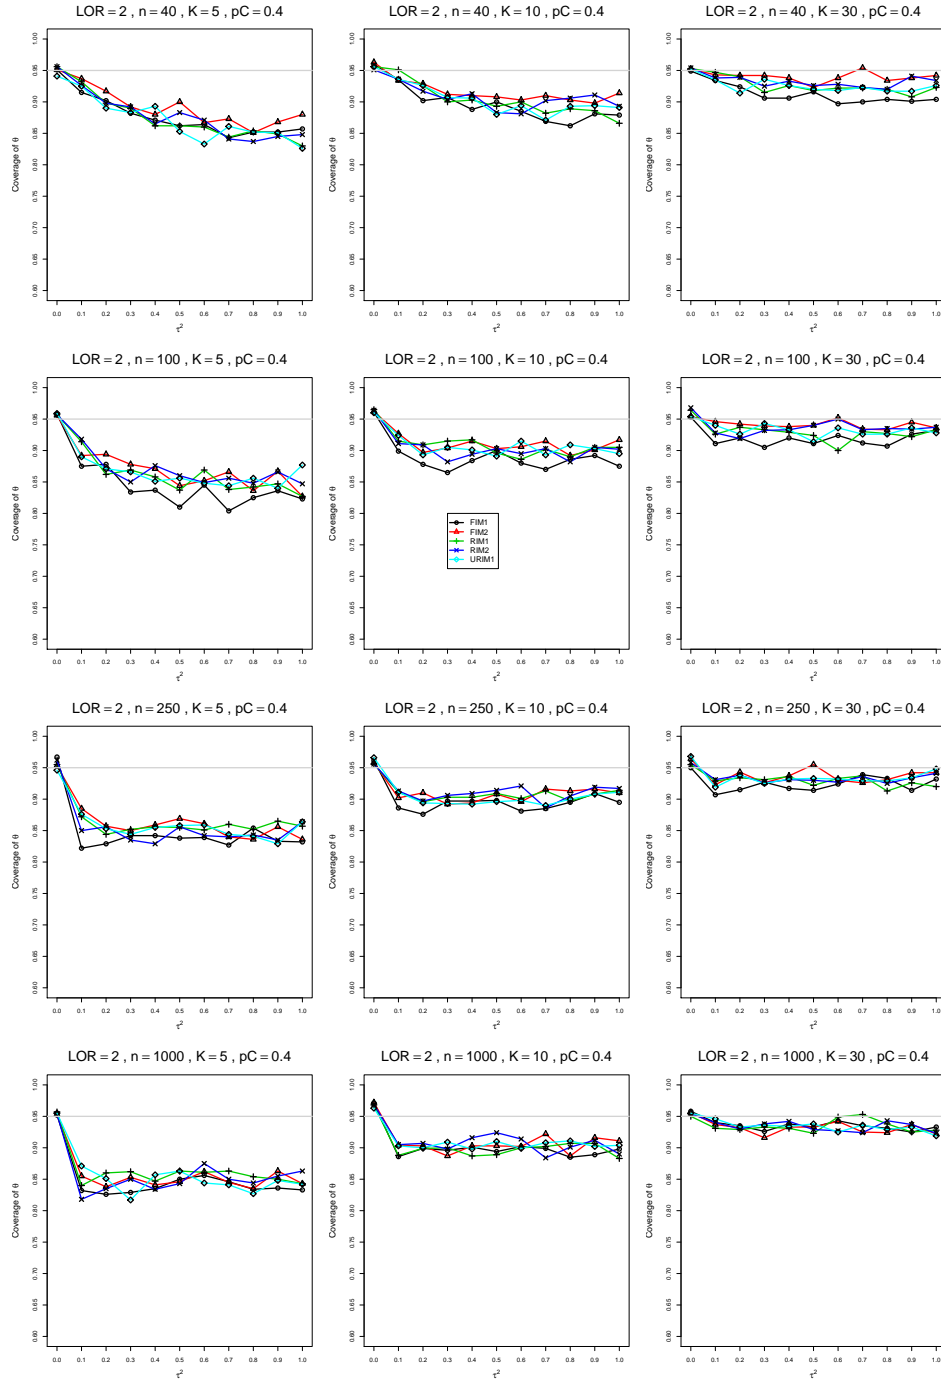

Figure A3.6.20: Coverage of the Random-intercept with  $c = 1/2$  confidence interval for  $\theta = 2$ ,  $p_C = 0.4$ ,  $\sigma^2 = 0.4$ , constant sample sizes  $n = 40, 100, 250, 1000$ . The data-generation mechanisms are FIM1 ( $\circ$ ), FIM2 ( $\triangle$ ), RIM1 (+), RIM2 ( $\times$ ), and URIM1 ( $\diamond$ ).

### A3.6 Coverage of $\hat{\theta}_{SW}$ with HkSJ and $\hat{tau}_{KD}^2$



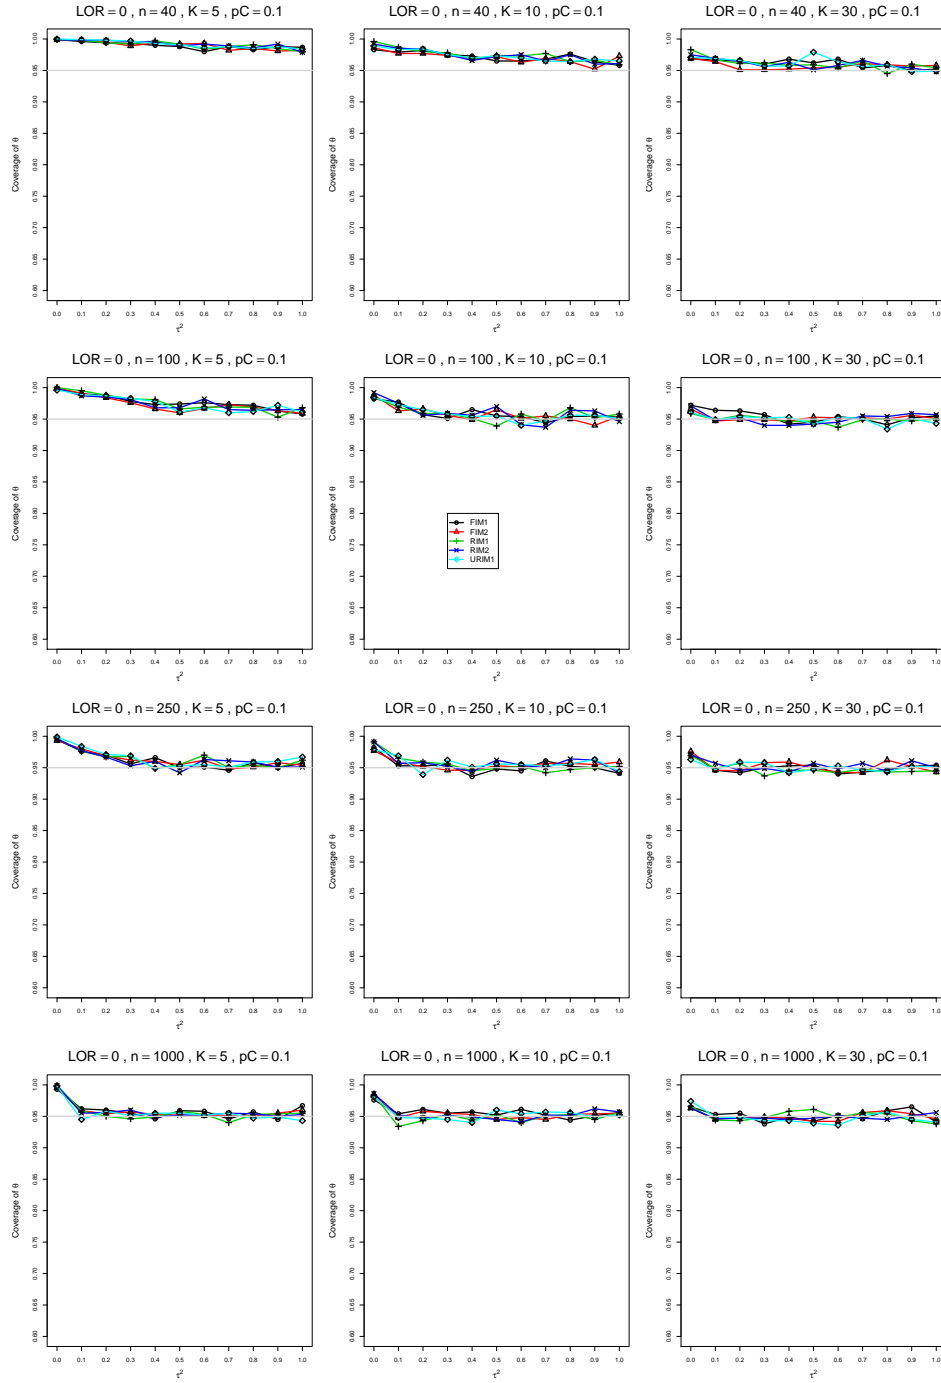

Figure A3.6.1: Coverage of the sample-size-weighted with Hartung-Knapp-Sidik-Jonkman (with KD) confidence interval for  $\theta = 0$ ,  $p_C = 0.1$ ,  $\sigma^2 = 0.1$ , constant sample sizes  $n = 40, 100, 250, 1000$ . The data-generation mechanisms are FIM1 ( $\circ$ ), FIM2 ( $\triangle$ ), RIM1 (+), RIM2 ( $\times$ ), and URIM1 ( $\diamond$ ).

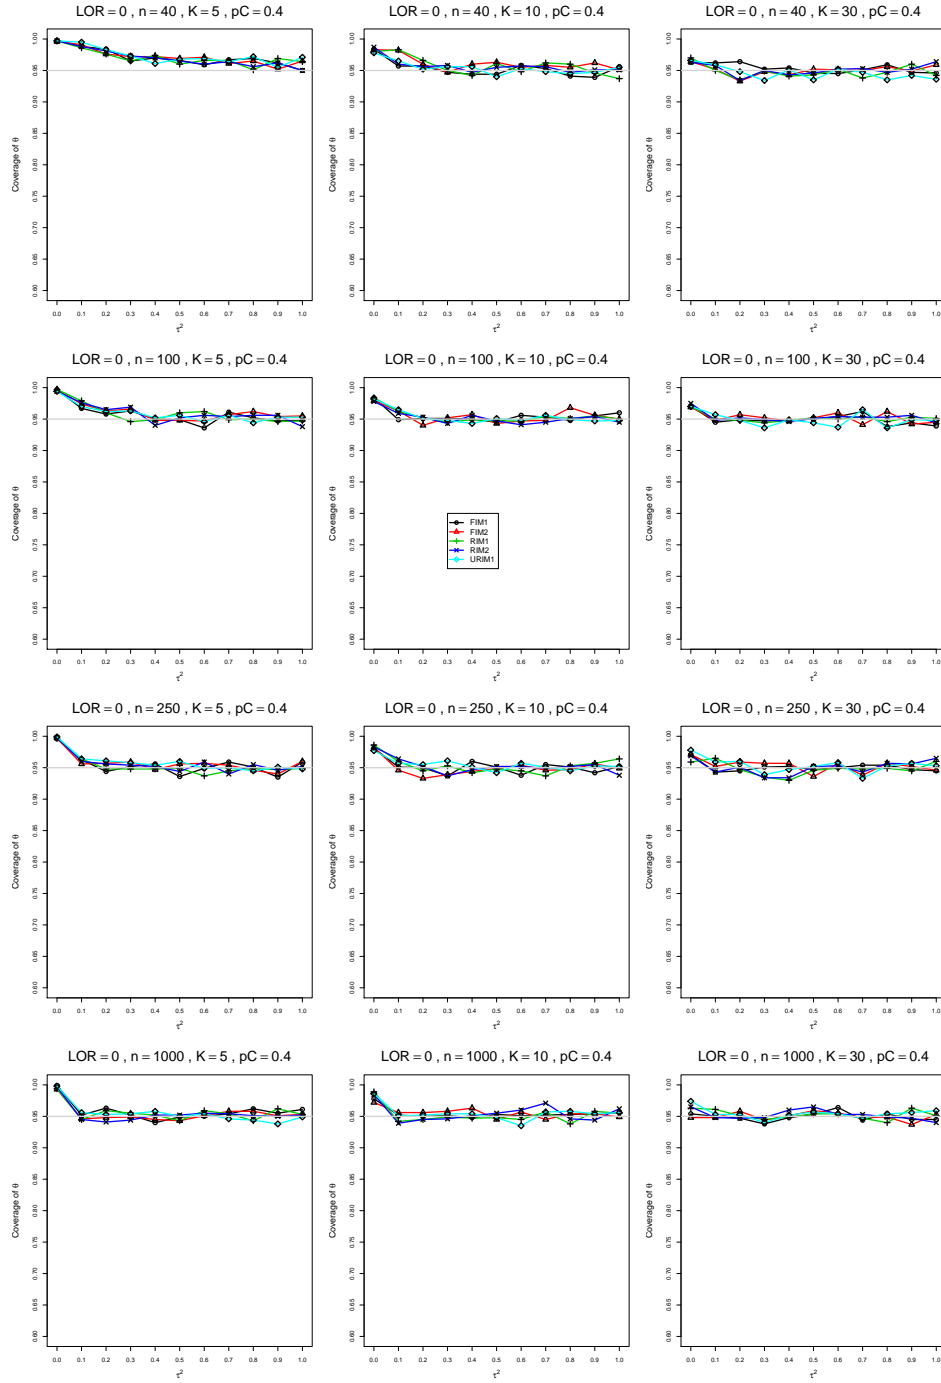

Figure A3.6.2: Coverage of the sample-size-weighted with Hartung-Knapp-Sidik-Jonkman (with KD) confidence interval for  $\theta = 0$ ,  $p_C = 0.4$ ,  $\sigma^2 = 0.1$ , constant sample sizes  $n = 40, 100, 250, 1000$ . The data-generation mechanisms are FIM1 ( $\circ$ ), FIM2 ( $\triangle$ ), RIM1 (+), RIM2 ( $\times$ ), and URIM1 ( $\diamond$ ).

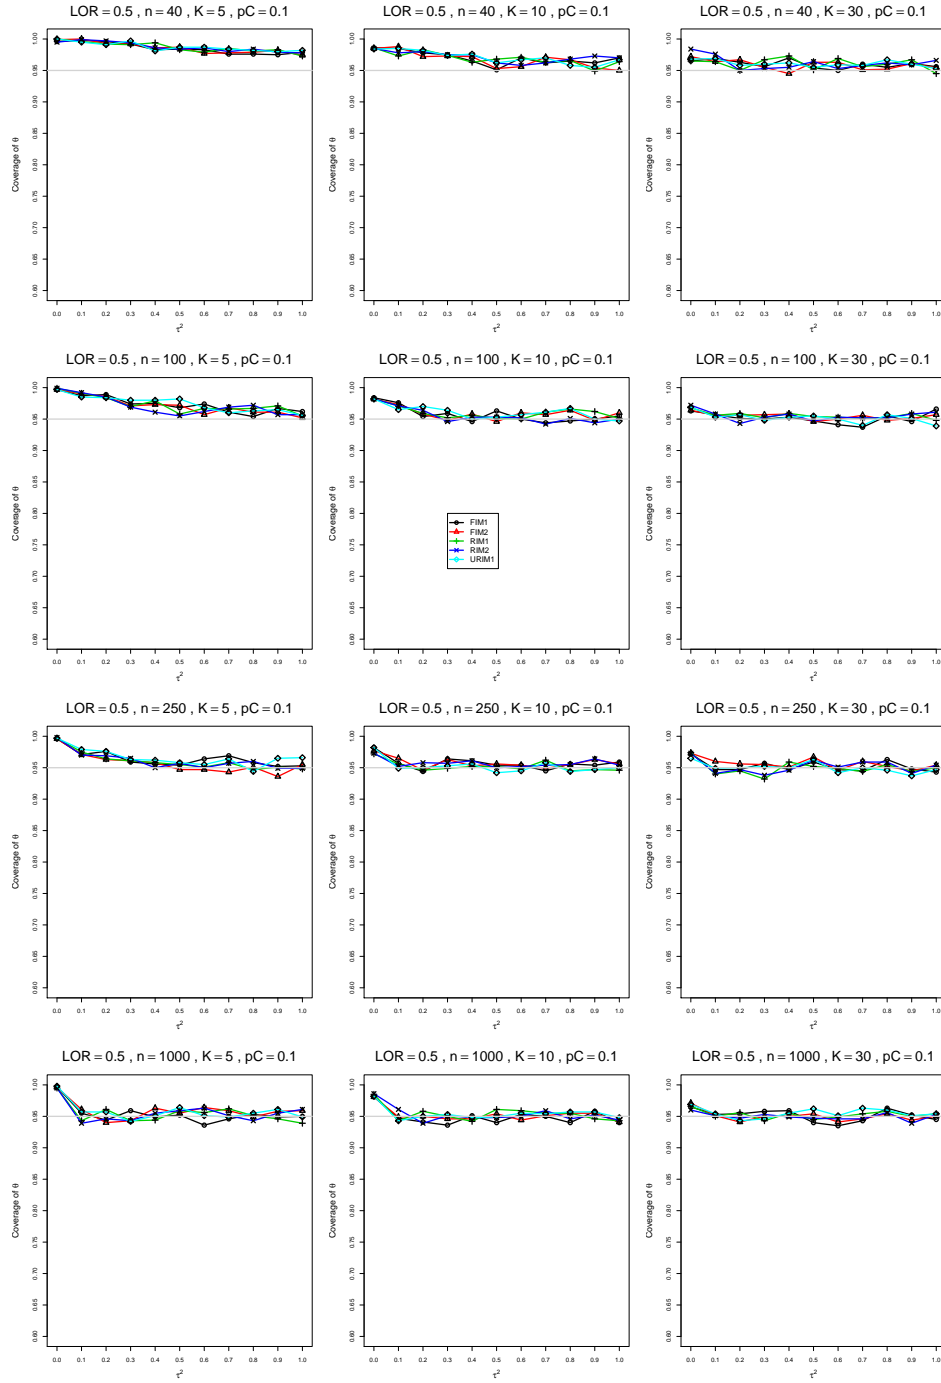

Figure A3.6.3: Coverage of the sample-size-weighted with Hartung-Knapp-Sidik-Jonkman (with KD) confidence interval for  $\theta = 0.5$ ,  $p_C = 0.1$ ,  $\sigma^2 = 0.1$ , constant sample sizes  $n = 40, 100, 250, 1000$ . The data-generation mechanisms are FIM1 ( $\circ$ ), FIM2 ( $\triangle$ ), RIM1 (+), RIM2 ( $\times$ ), and URIM1 ( $\diamond$ ).

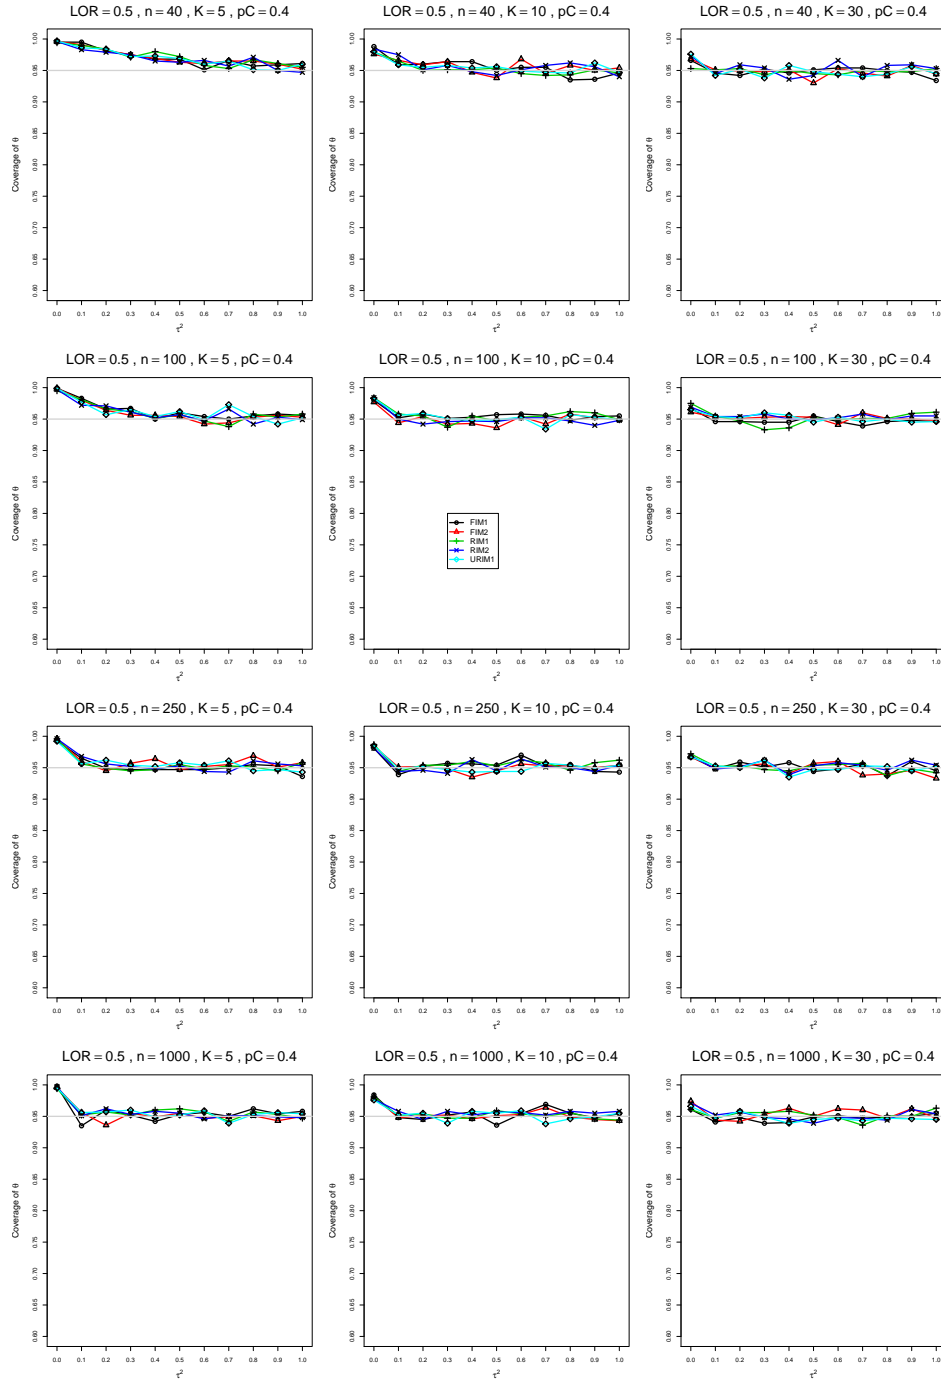

Figure A3.6.4: Coverage of the sample-size-weighted with Hartung-Knapp-Sidik-Jonkman (with KD) confidence interval for  $\theta = 0.5$ ,  $p_C = 0.4$ ,  $\sigma^2 = 0.1$ , constant sample sizes  $n = 40, 100, 250, 1000$ . The data-generation mechanisms are FIM1 ( $\circ$ ), FIM2 ( $\triangle$ ), RIM1 ( $+$ ), RIM2 ( $\times$ ), and URIM1 ( $\diamond$ ).

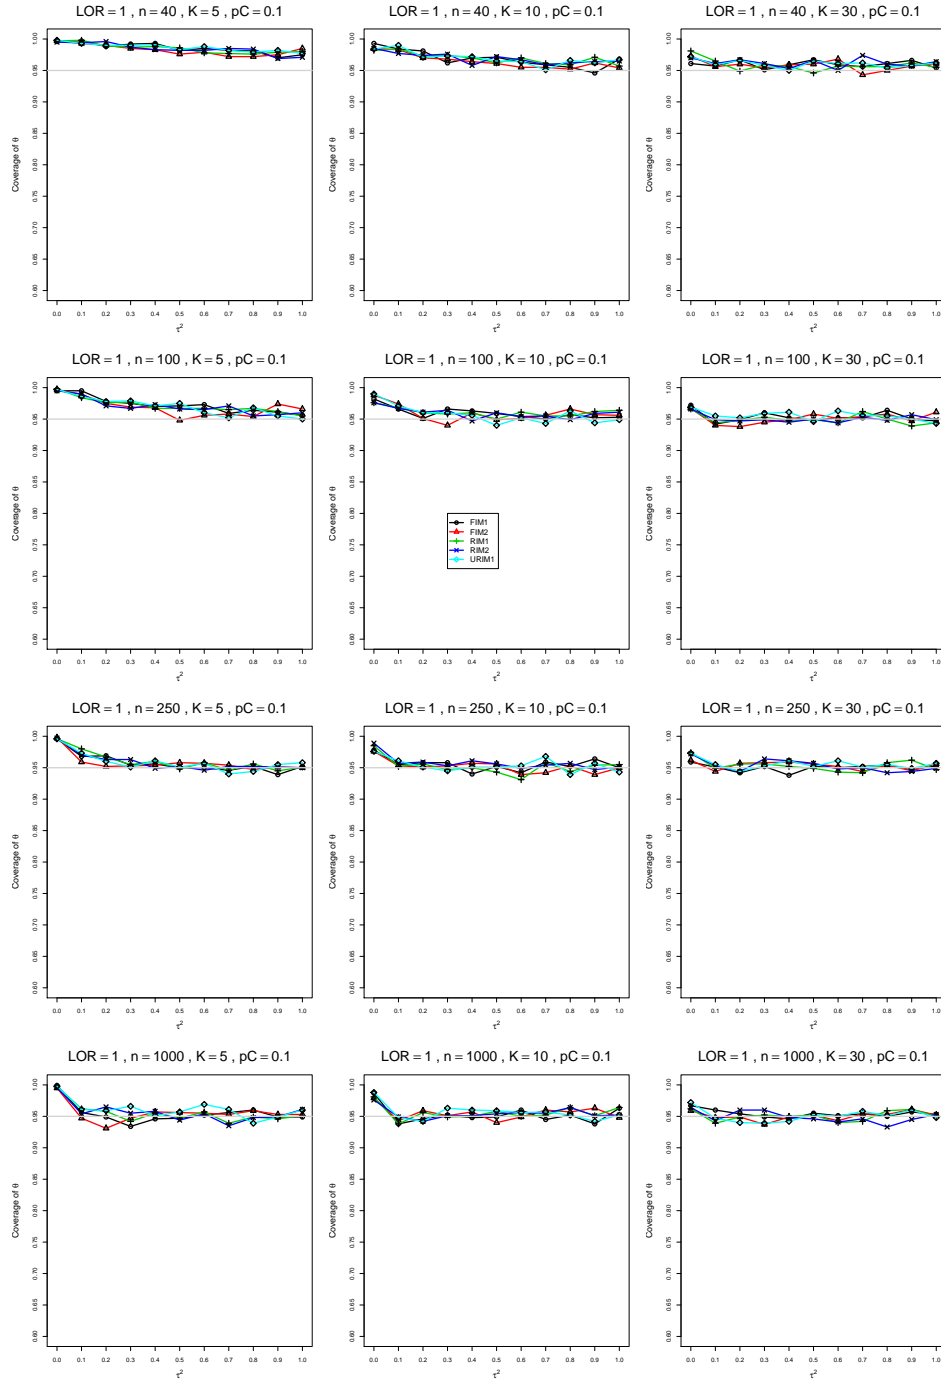

Figure A3.6.5: Coverage of the sample-size-weighted with Hartung-Knapp-Sidik-Jonkman (with KD) confidence interval for  $\theta = 1$ ,  $p_C = 0.1$ ,  $\sigma^2 = 0.1$ , constant sample sizes  $n = 40, 100, 250, 1000$ . The data-generation mechanisms are FIM1 ( $\circ$ ), FIM2 ( $\triangle$ ), RIM1 (+), RIM2 ( $\times$ ), and URIM1 ( $\diamond$ ).

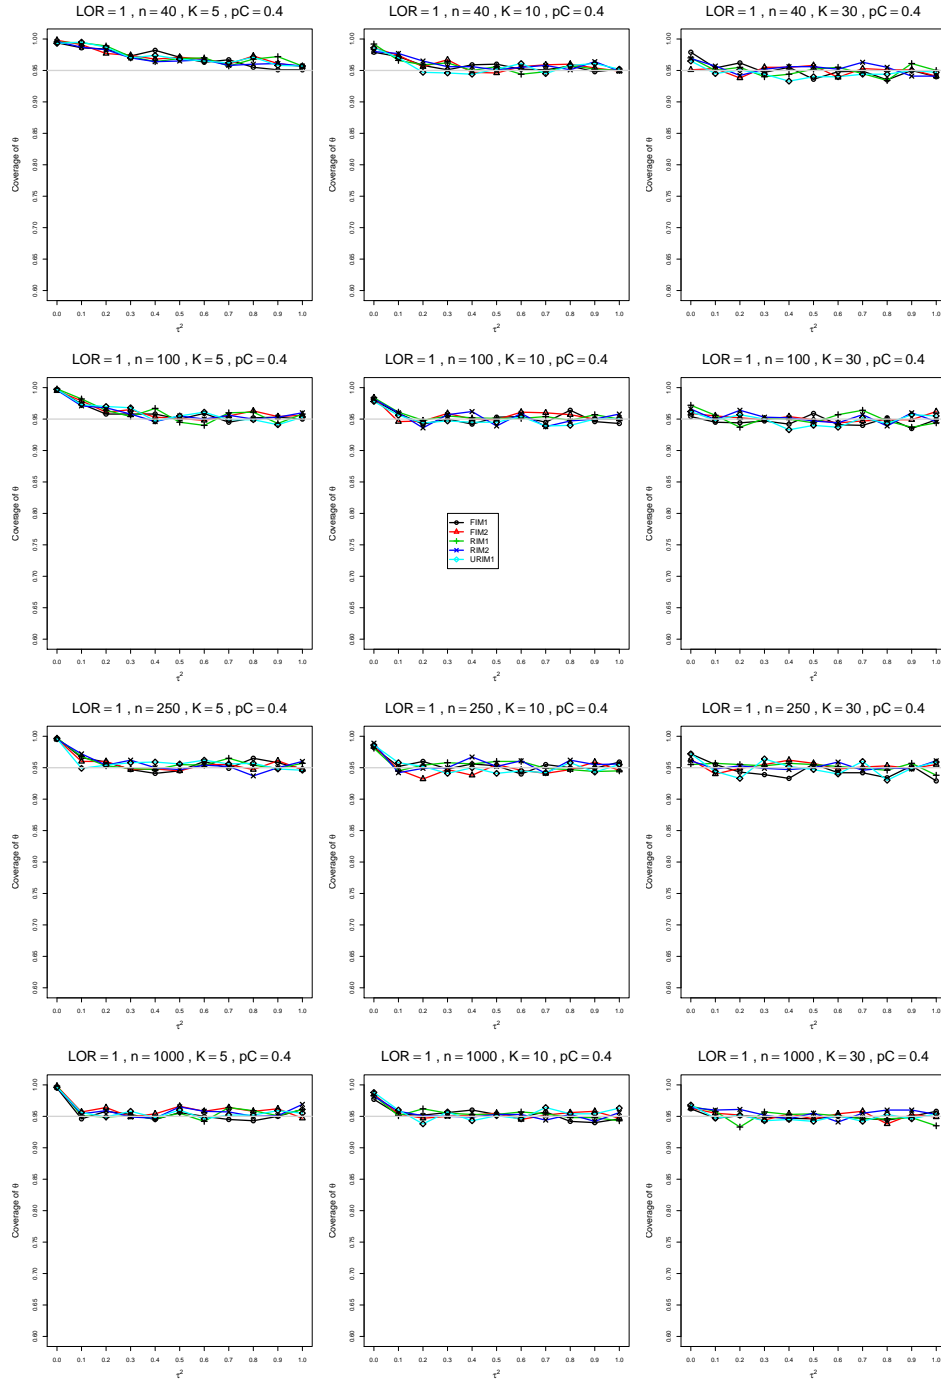

Figure A3.6.6: Coverage of the sample-size-weighted with Hartung-Knapp-Sidik-Jonkman (with KD) confidence interval for  $\theta = 1$ ,  $p_C = 0.4$ ,  $\sigma^2 = 0.1$ , constant sample sizes  $n = 40, 100, 250, 1000$ . The data-generation mechanisms are FIM1 ( $\circ$ ), FIM2 ( $\triangle$ ), RIM1 (+), RIM2 ( $\times$ ), and URIM1 ( $\diamond$ ).

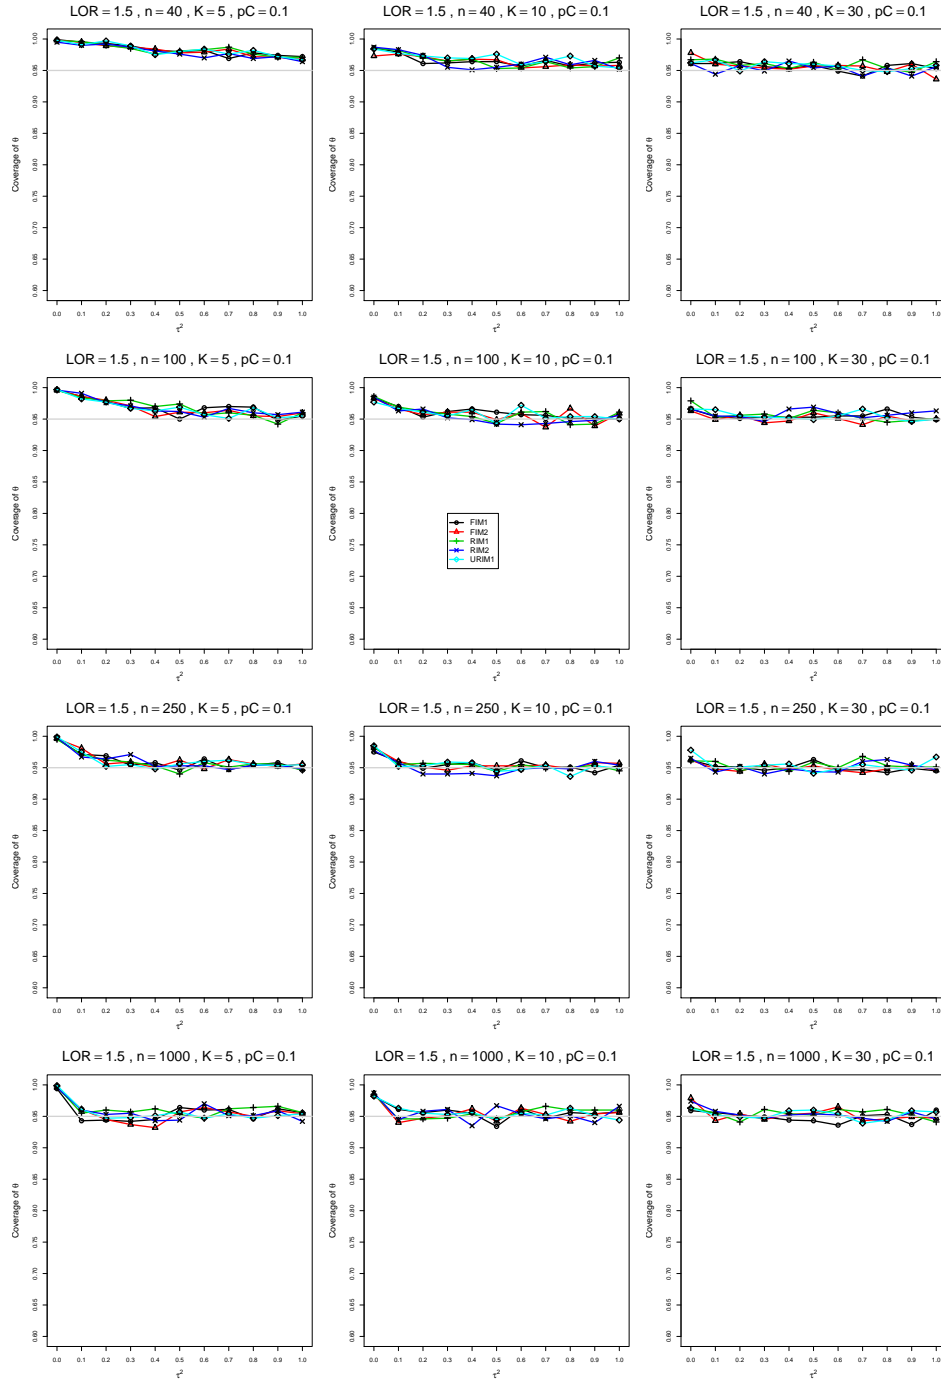

Figure A3.6.7: Coverage of the sample-size-weighted with Hartung-Knapp-Sidik-Jonkman (with KD) confidence interval for  $\theta = 1.5$ ,  $p_C = 0.1$ ,  $\sigma^2 = 0.1$ , constant sample sizes  $n = 40, 100, 250, 1000$ . The data-generation mechanisms are FIM1 ( $\circ$ ), FIM2 ( $\triangle$ ), RIM1 (+), RIM2 ( $\times$ ), and URIM1 ( $\diamond$ ).

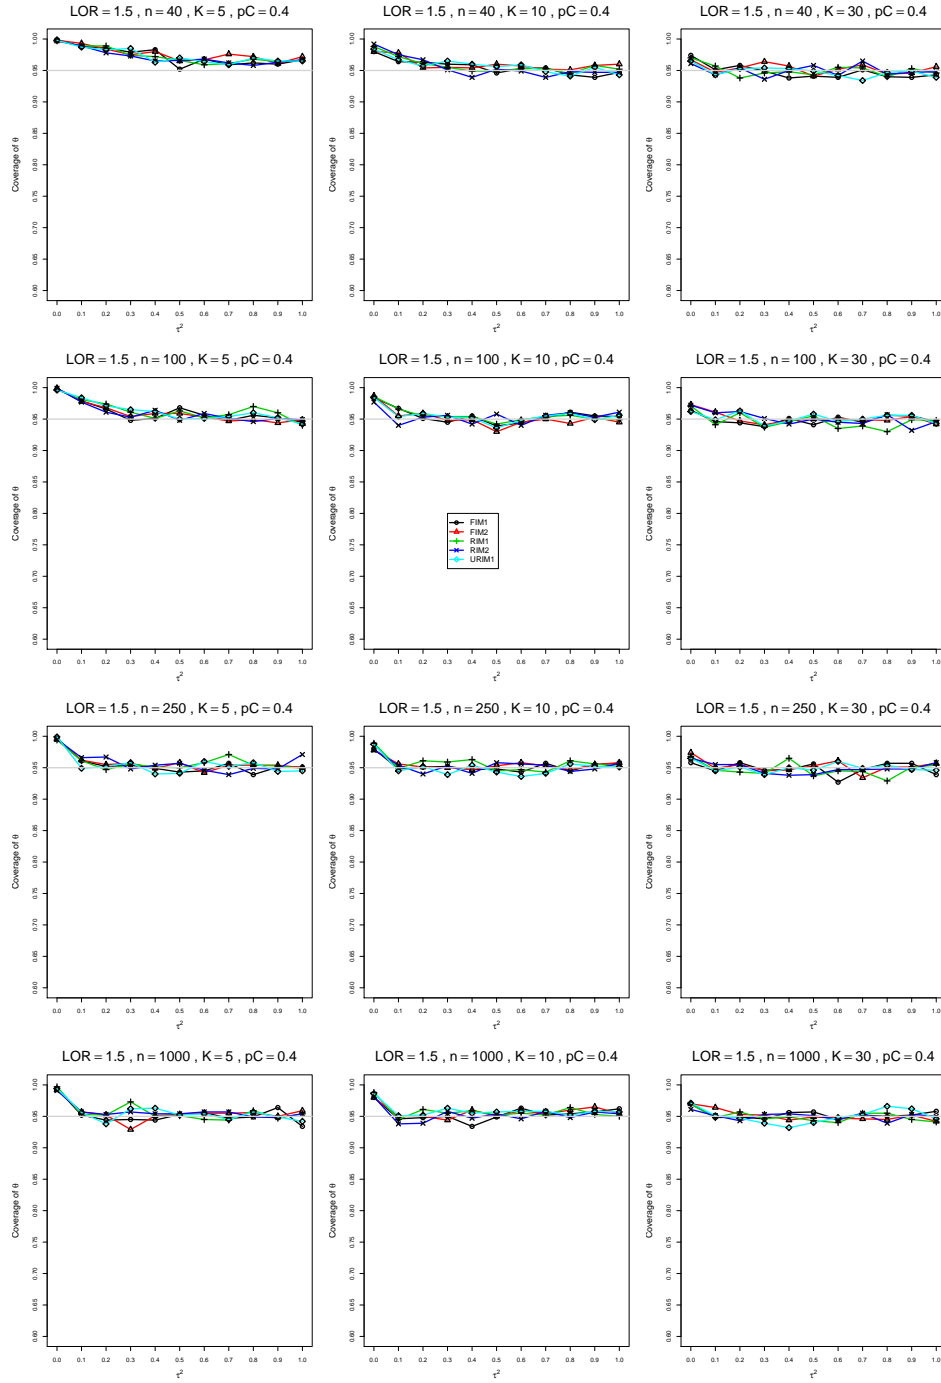

Figure A3.6.8: Coverage of the sample-size-weighted with Hartung-Knapp-Sidik-Jonkman (with KD) confidence interval for  $\theta = 1.5$ ,  $p_C = 0.4$ ,  $\sigma^2 = 0.1$ , constant sample sizes  $n = 40, 100, 250, 1000$ . The data-generation mechanisms are FIM1 ( $\circ$ ), FIM2 ( $\triangle$ ), RIM1 (+), RIM2 ( $\times$ ), and URIM1 ( $\diamond$ ).



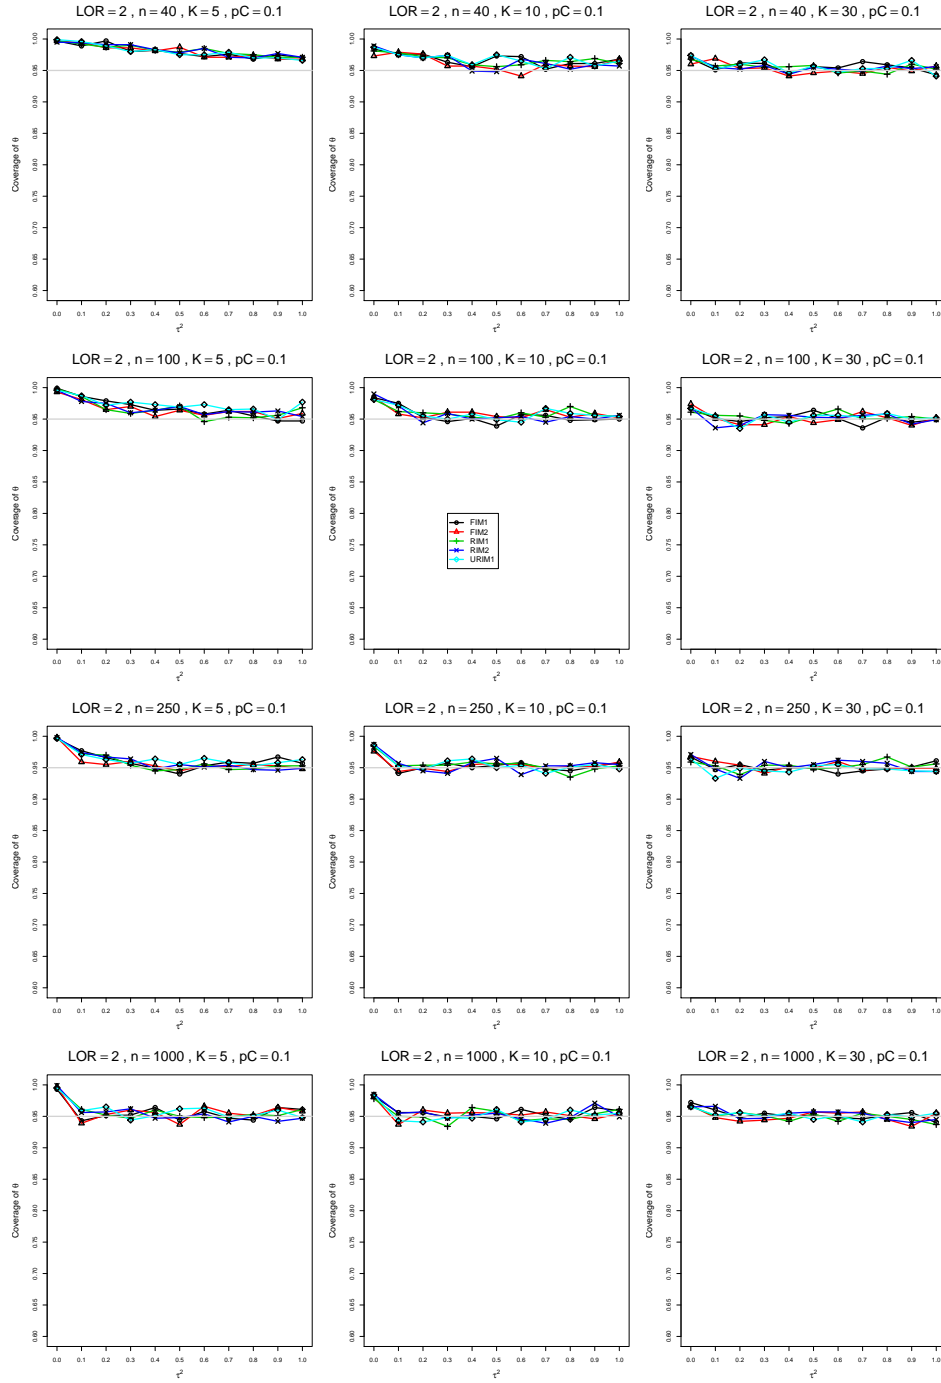

Figure A3.6.9: Coverage of the sample-size-weighted with Hartung-Knapp-Sidik-Jonkman (with KD) confidence interval for  $\theta = 2$ ,  $p_C = 0.1$ ,  $\sigma^2 = 0.1$ , constant sample sizes  $n = 40, 100, 250, 1000$ . The data-generation mechanisms are FIM1 ( $\circ$ ), FIM2 ( $\triangle$ ), RIM1 (+), RIM2 ( $\times$ ), and URIM1 ( $\diamond$ ).

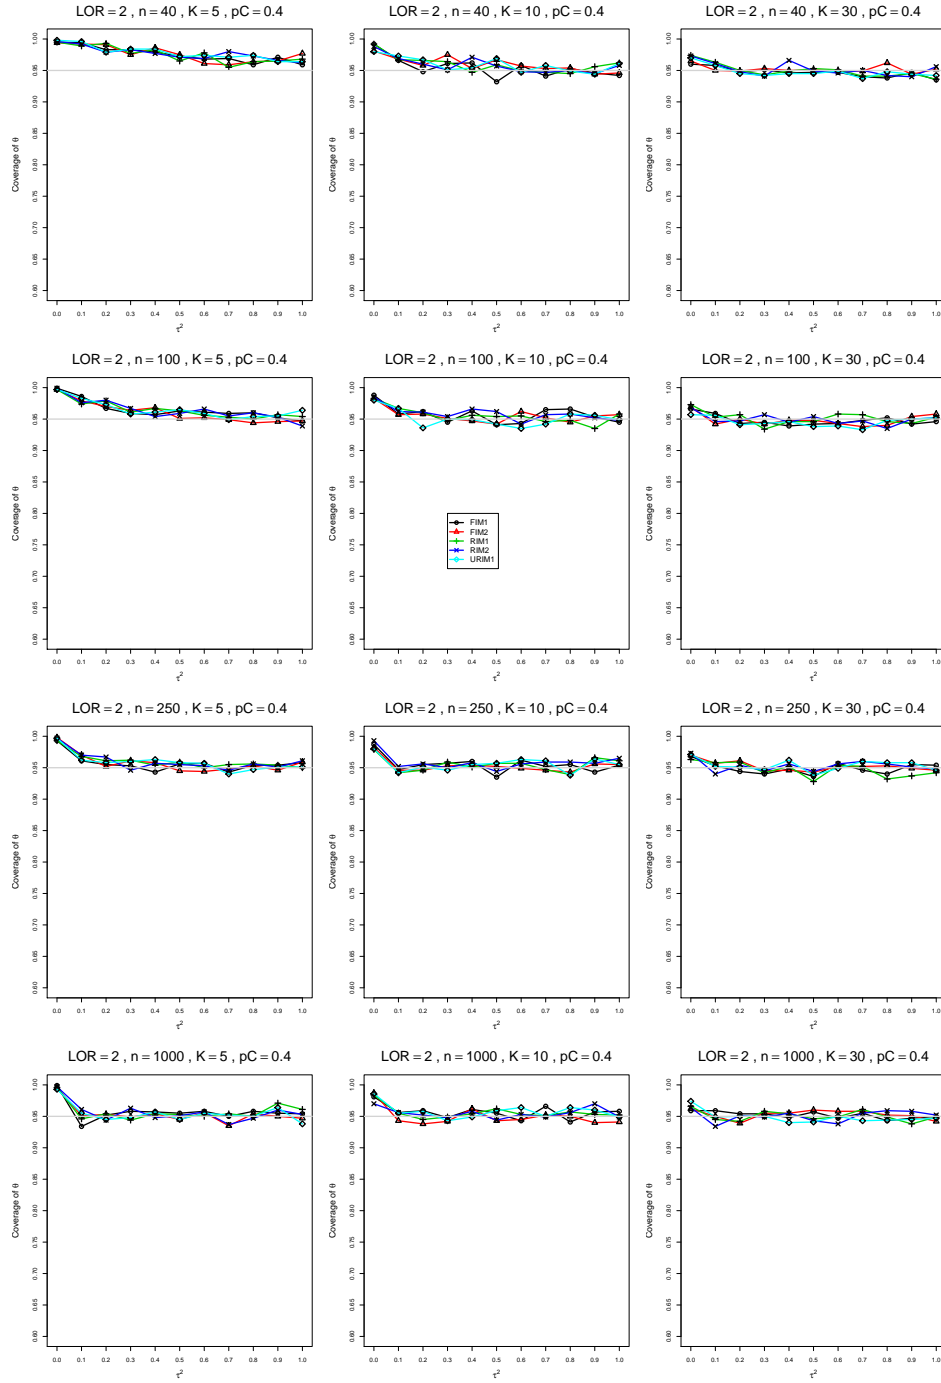

Figure A3.6.10: Coverage of the sample-size-weighted with Hartung-Knapp-Sidik-Jonkman (with KD) confidence interval for  $\theta = 2$ ,  $p_C = 0.4$ ,  $\sigma^2 = 0.1$ , constant sample sizes  $n = 40, 100, 250, 1000$ . The data-generation mechanisms are FIM1 ( $\circ$ ), FIM2 ( $\triangle$ ), RIM1 (+), RIM2 ( $\times$ ), and URIM1 ( $\diamond$ ).

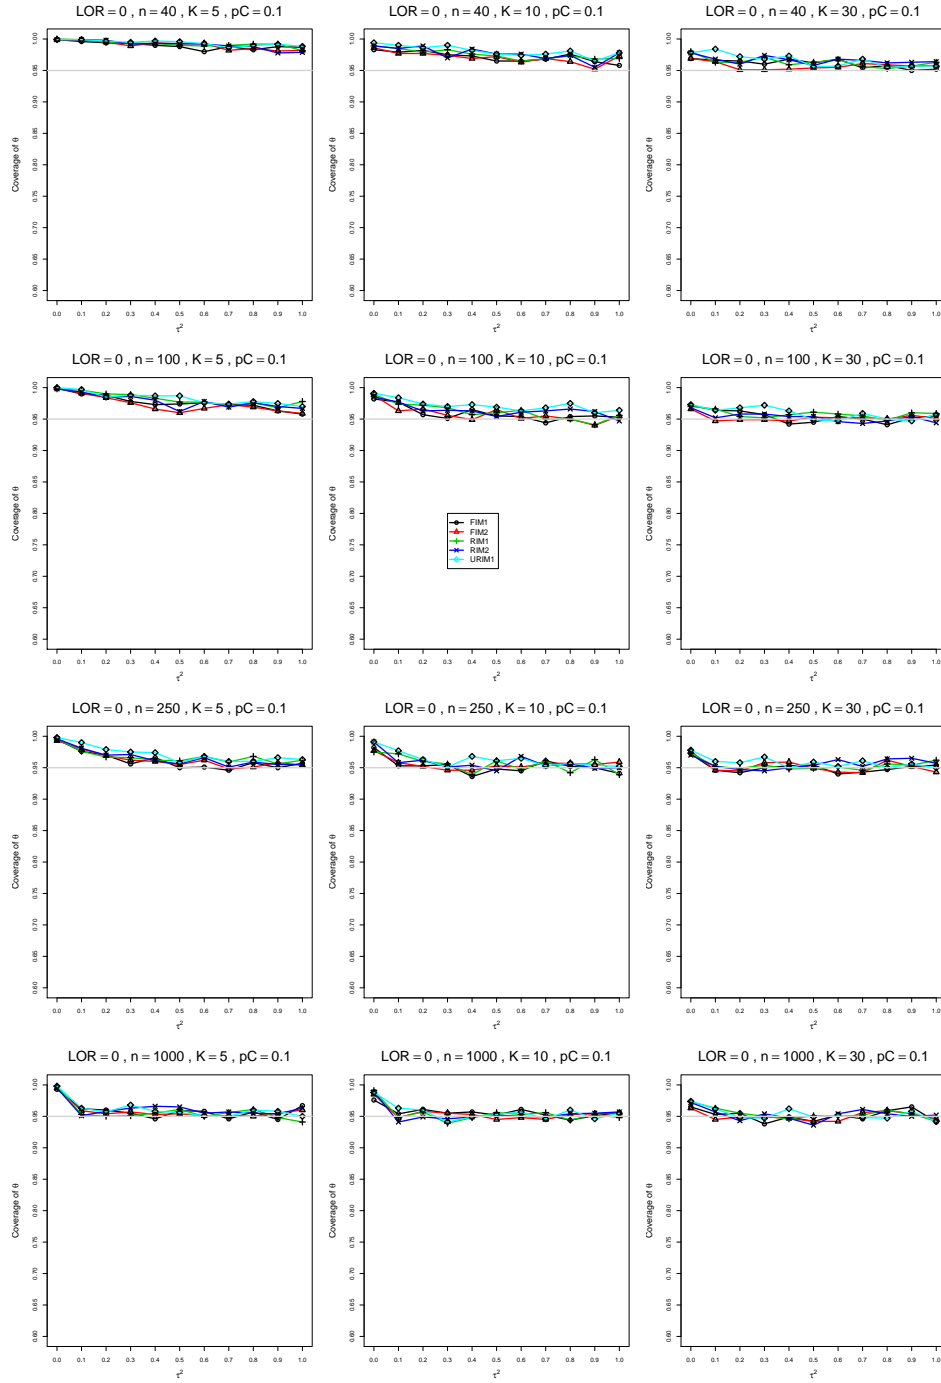

Figure A3.6.11: Coverage of the sample-size-weighted with Hartung-Knapp-Sidik-Jonkman (with KD) confidence interval for  $\theta = 0$ ,  $p_C = 0.1$ ,  $\sigma^2 = 0.4$ , constant sample sizes  $n = 40, 100, 250, 1000$ . The data-generation mechanisms are FIM1 ( $\circ$ ), FIM2 ( $\triangle$ ), RIM1 (+), RIM2 ( $\times$ ), and URIM1 ( $\diamond$ ).

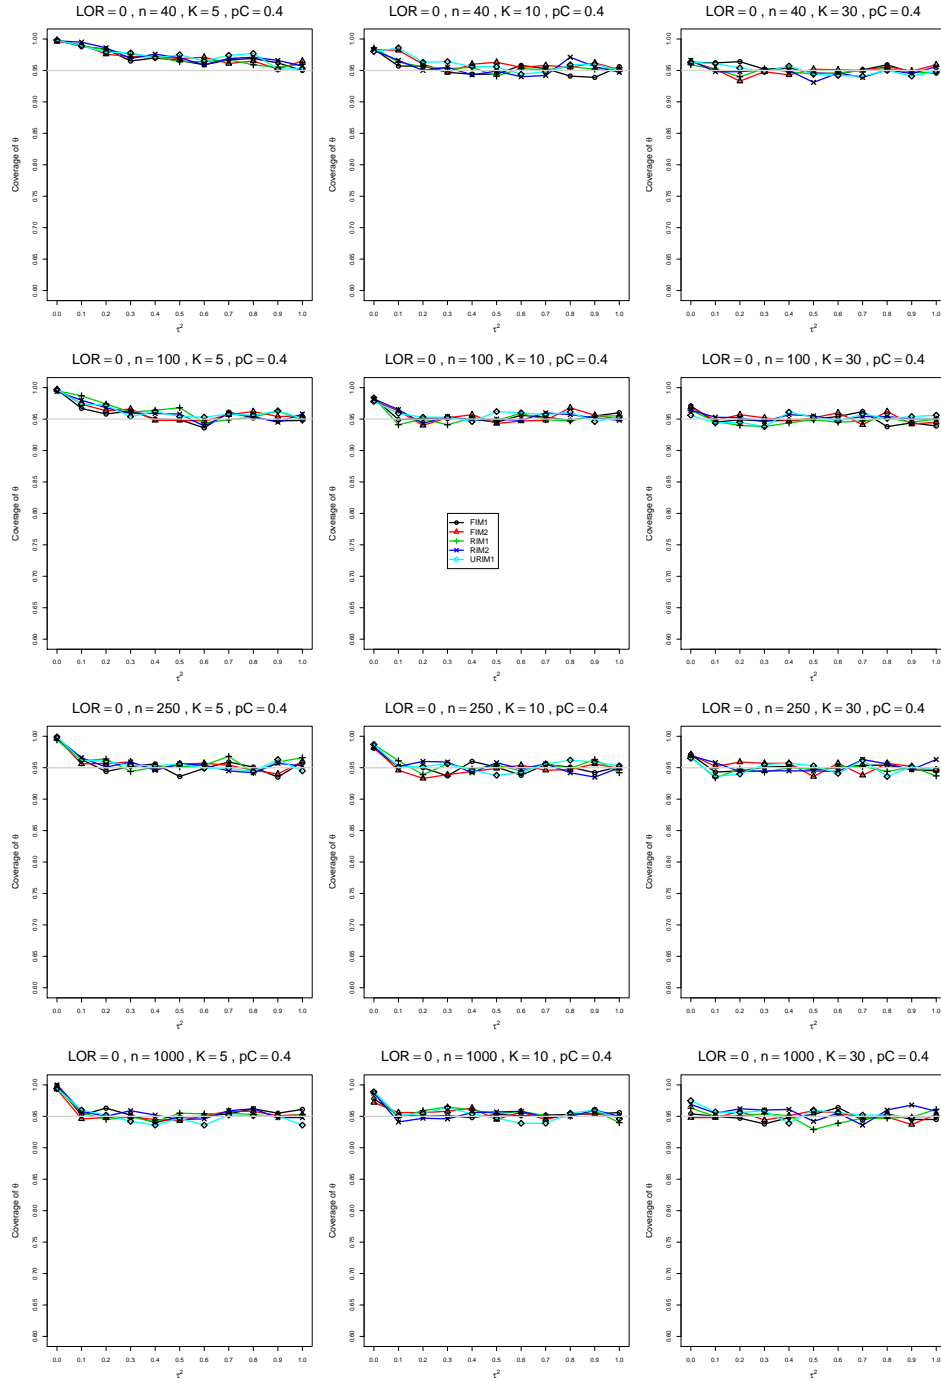

Figure A3.6.12: Coverage of the sample-size-weighted with Hartung-Knapp-Sidik-Jonkman (with KD) confidence interval for  $\theta = 0$ ,  $p_C = 0.4$ ,  $\sigma^2 = 0.4$ , constant sample sizes  $n = 40, 100, 250, 1000$ . The data-generation mechanisms are FIM1 ( $\circ$ ), FIM2 ( $\triangle$ ), RIM1 (+), RIM2 ( $\times$ ), and URIM1 ( $\diamond$ ).

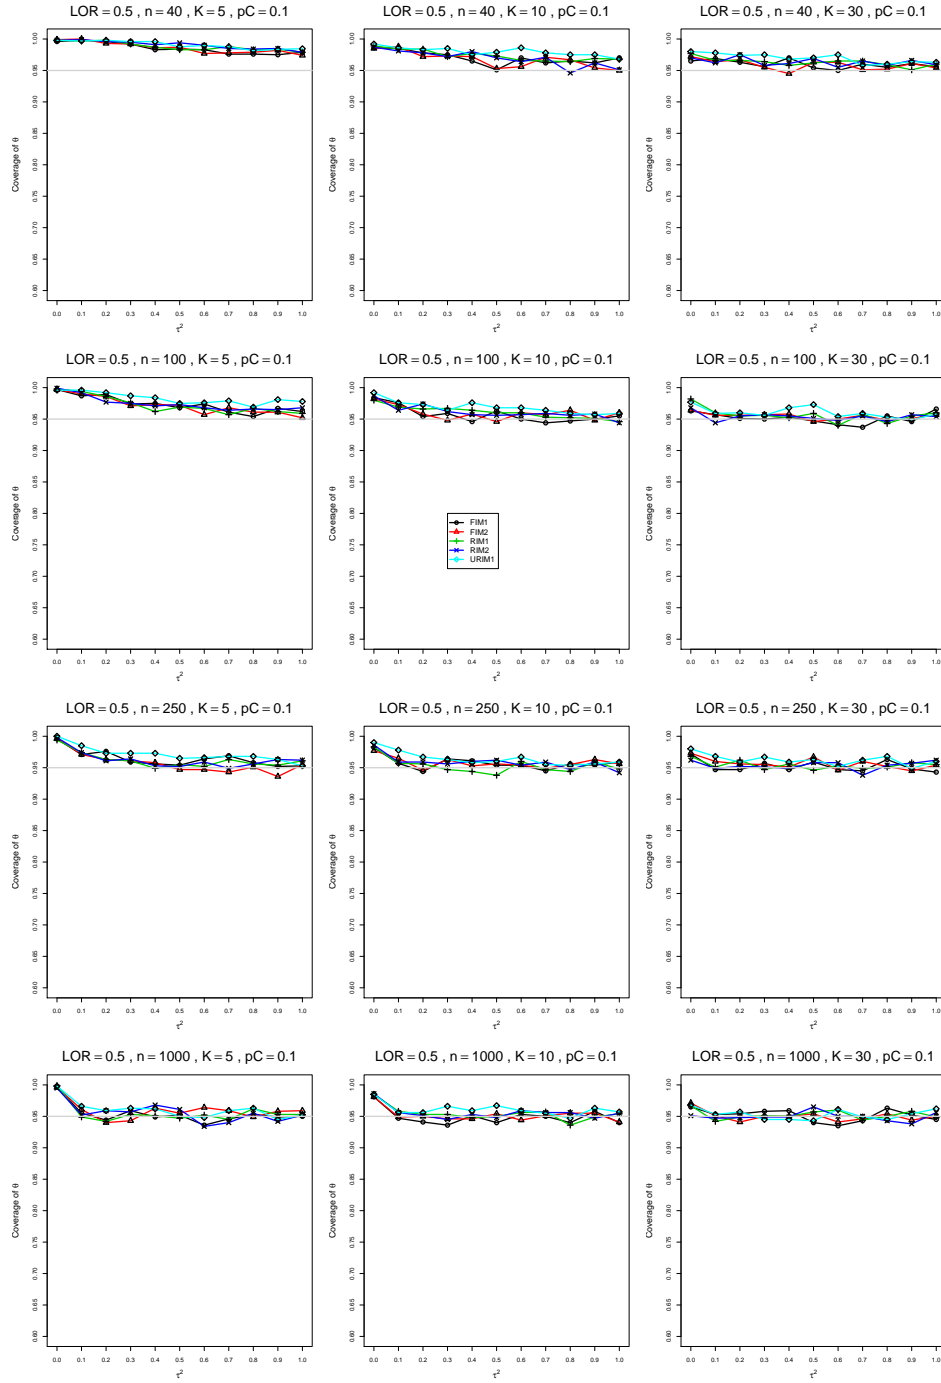

Figure A3.6.13: Coverage of the sample-size-weighted with Hartung-Knapp-Sidik-Jonkman (with KD) confidence interval for  $\theta = 0.5$ ,  $p_C = 0.1$ ,  $\sigma^2 = 0.4$ , constant sample sizes  $n = 40, 100, 250, 1000$ . The data-generation mechanisms are FIM1 ( $\circ$ ), FIM2 ( $\triangle$ ), RIM1 (+), RIM2 ( $\times$ ), and URIM1 ( $\diamond$ ).

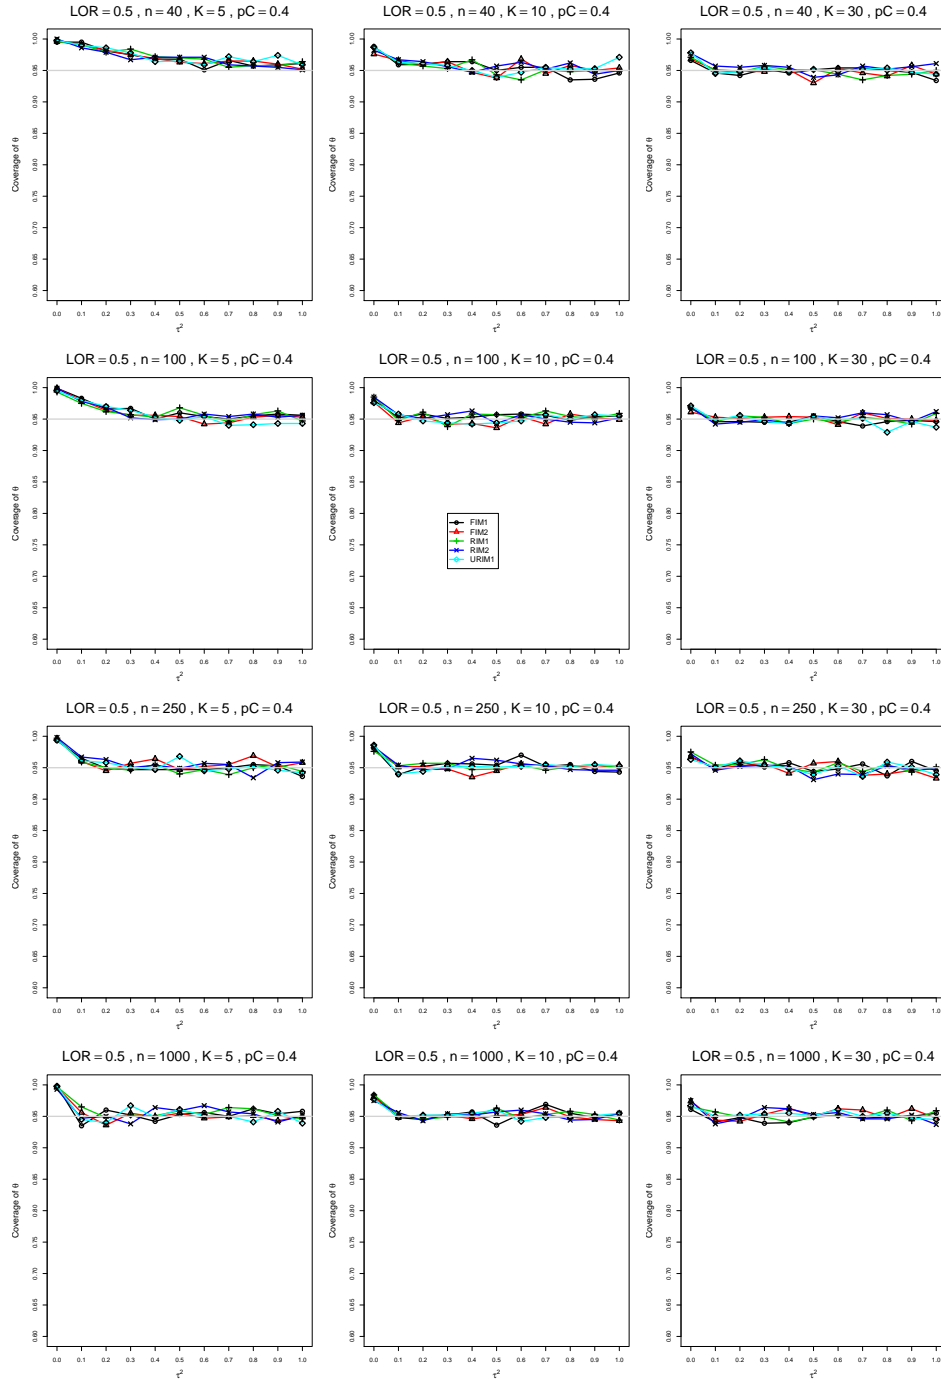

Figure A3.6.14: Coverage of the sample-size-weighted with Hartung-Knapp-Sidik-Jonkman (with KD) confidence interval for  $\theta = 0.5$ ,  $p_C = 0.4$ ,  $\sigma^2 = 0.4$ , constant sample sizes  $n = 40, 100, 250, 1000$ . The data-generation mechanisms are FIM1 ( $\circ$ ), FIM2 ( $\triangle$ ), RIM1 (+), RIM2 ( $\times$ ), and URIM1 ( $\diamond$ ).

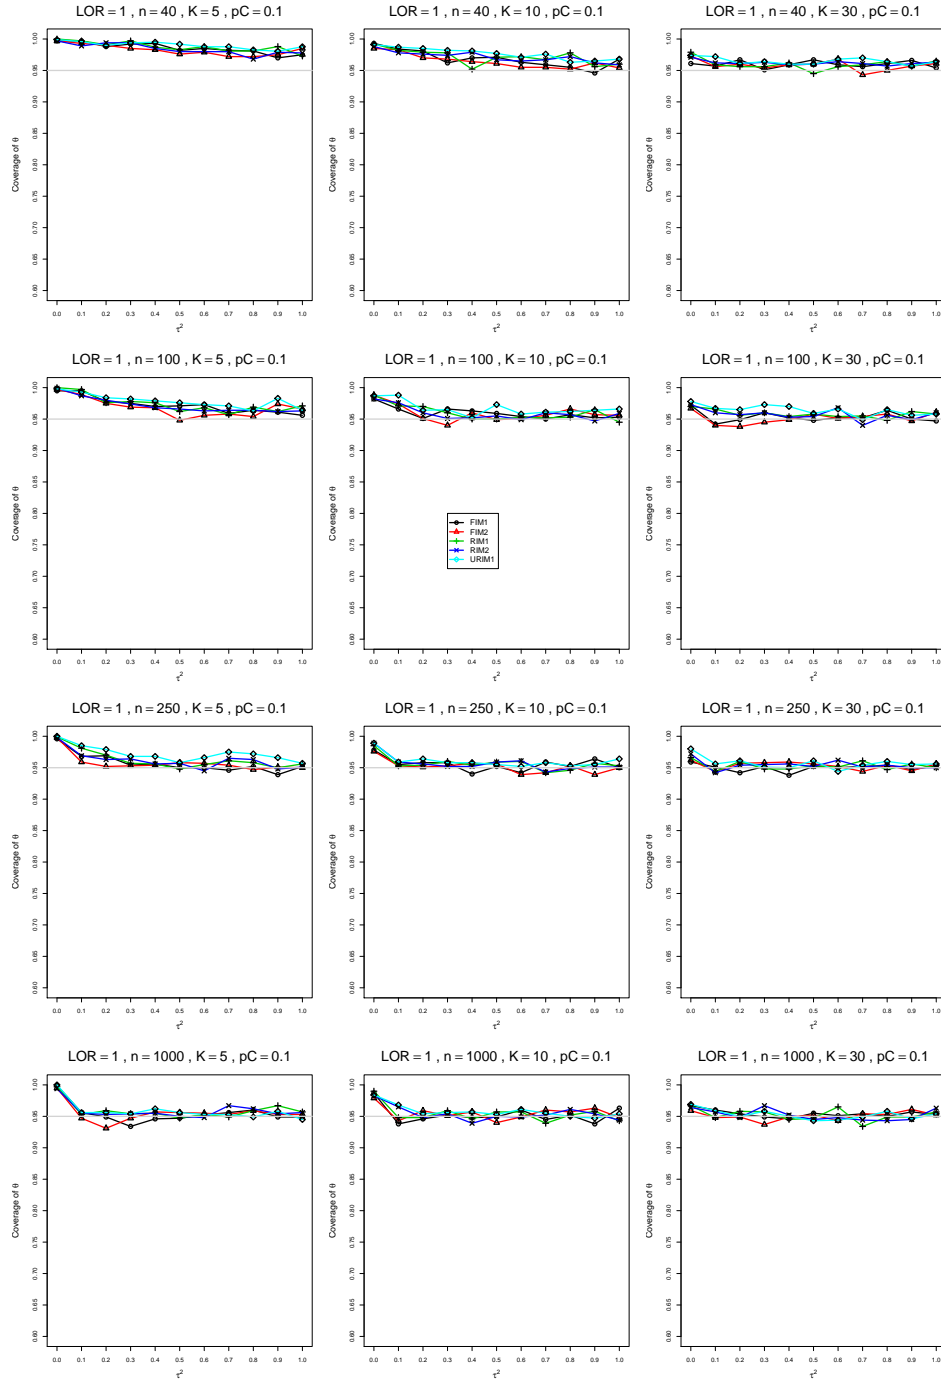

Figure A3.6.15: Coverage of the sample-size-weighted with Hartung-Knapp-Sidik-Jonkman (with KD) confidence interval for  $\theta = 1$ ,  $p_C = 0.1$ ,  $\sigma^2 = 0.4$ , constant sample sizes  $n = 40, 100, 250, 1000$ . The data-generation mechanisms are FIM1 ( $\circ$ ), FIM2 ( $\triangle$ ), RIM1 (+), RIM2 ( $\times$ ), and URIM1 ( $\diamond$ ).

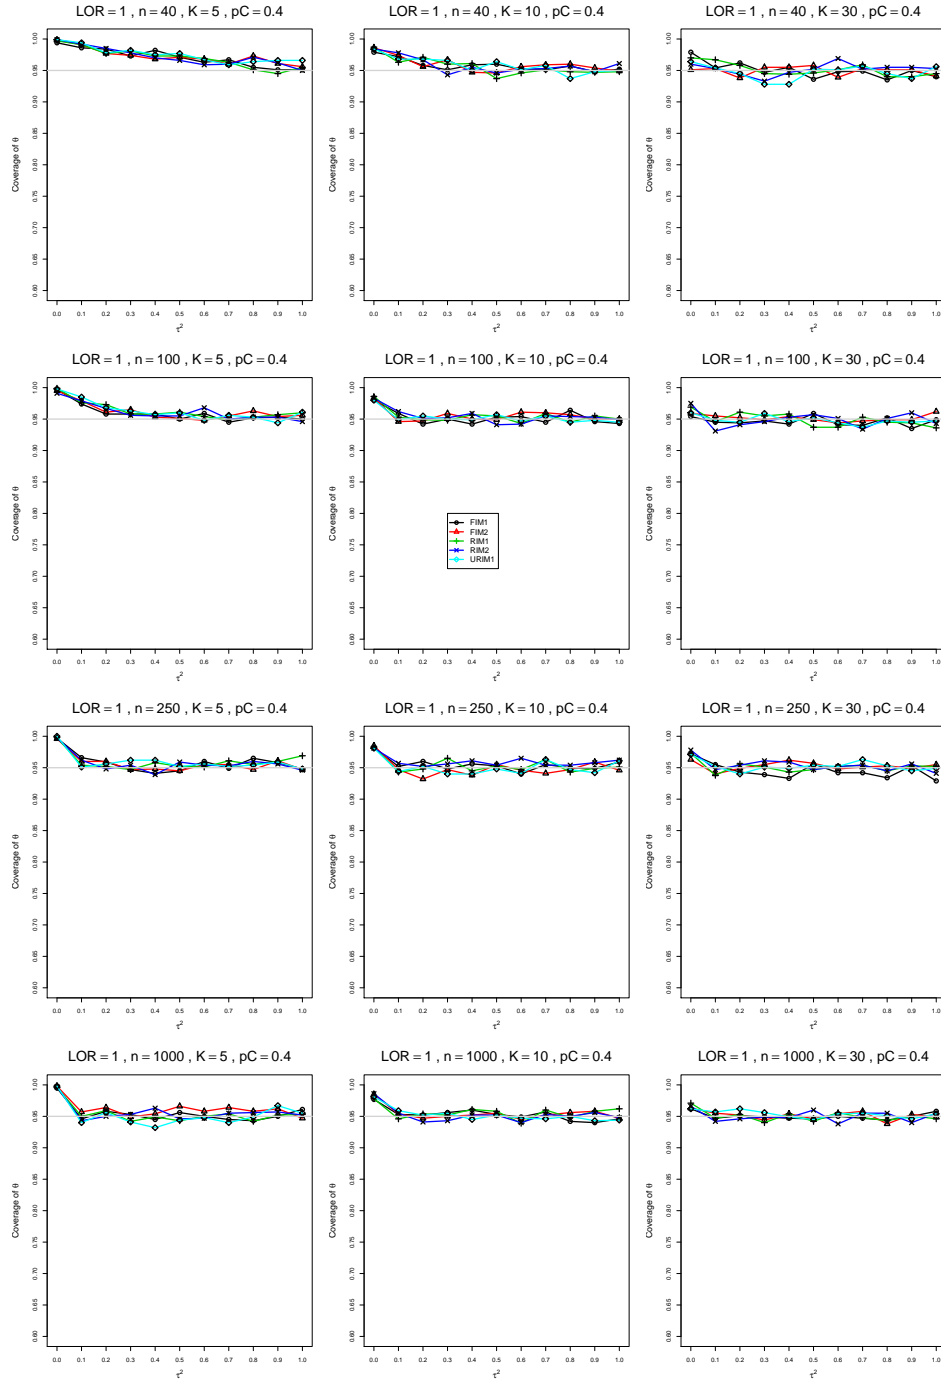

Figure A3.6.16: Coverage of the sample-size-weighted with Hartung-Knapp-Sidik-Jonkman (with KD) confidence interval for  $\theta = 1$ ,  $p_C = 0.4$ ,  $\sigma^2 = 0.4$ , constant sample sizes  $n = 40, 100, 250, 1000$ . The data-generation mechanisms are FIM1 ( $\circ$ ), FIM2 ( $\triangle$ ), RIM1 (+), RIM2 ( $\times$ ), and URIM1 ( $\diamond$ ).



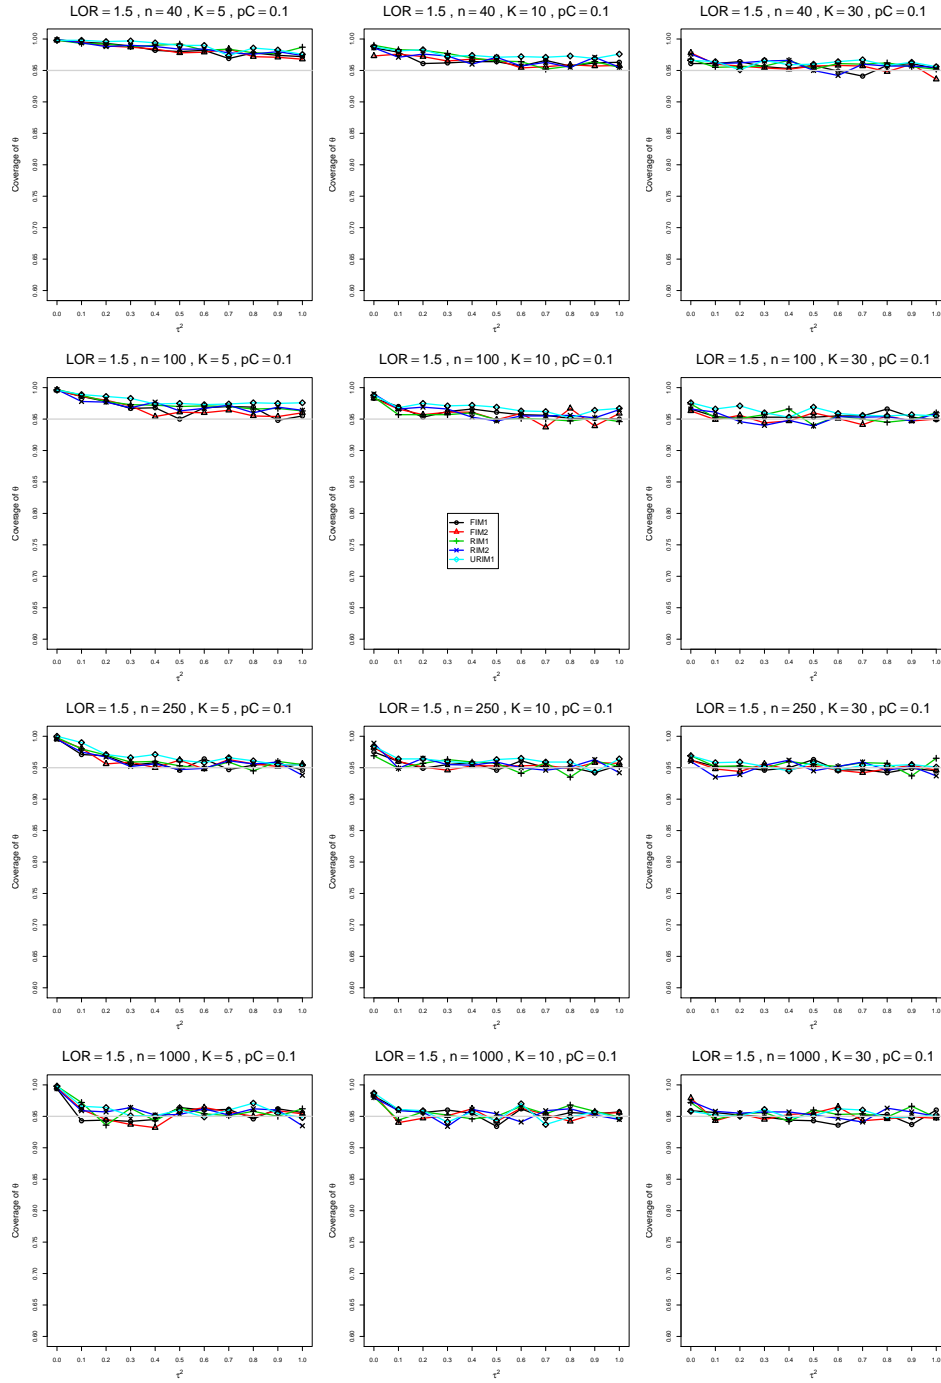

Figure A3.6.17: Coverage of the sample-size-weighted with Hartung-Knapp-Sidik-Jonkman (with KD) confidence interval for  $\theta = 1.5$ ,  $p_C = 0.1$ ,  $\sigma^2 = 0.4$ , constant sample sizes  $n = 40, 100, 250, 1000$ . The data-generation mechanisms are FIM1 ( $\circ$ ), FIM2 ( $\triangle$ ), RIM1 (+), RIM2 ( $\times$ ), and URIM1 ( $\diamond$ ).

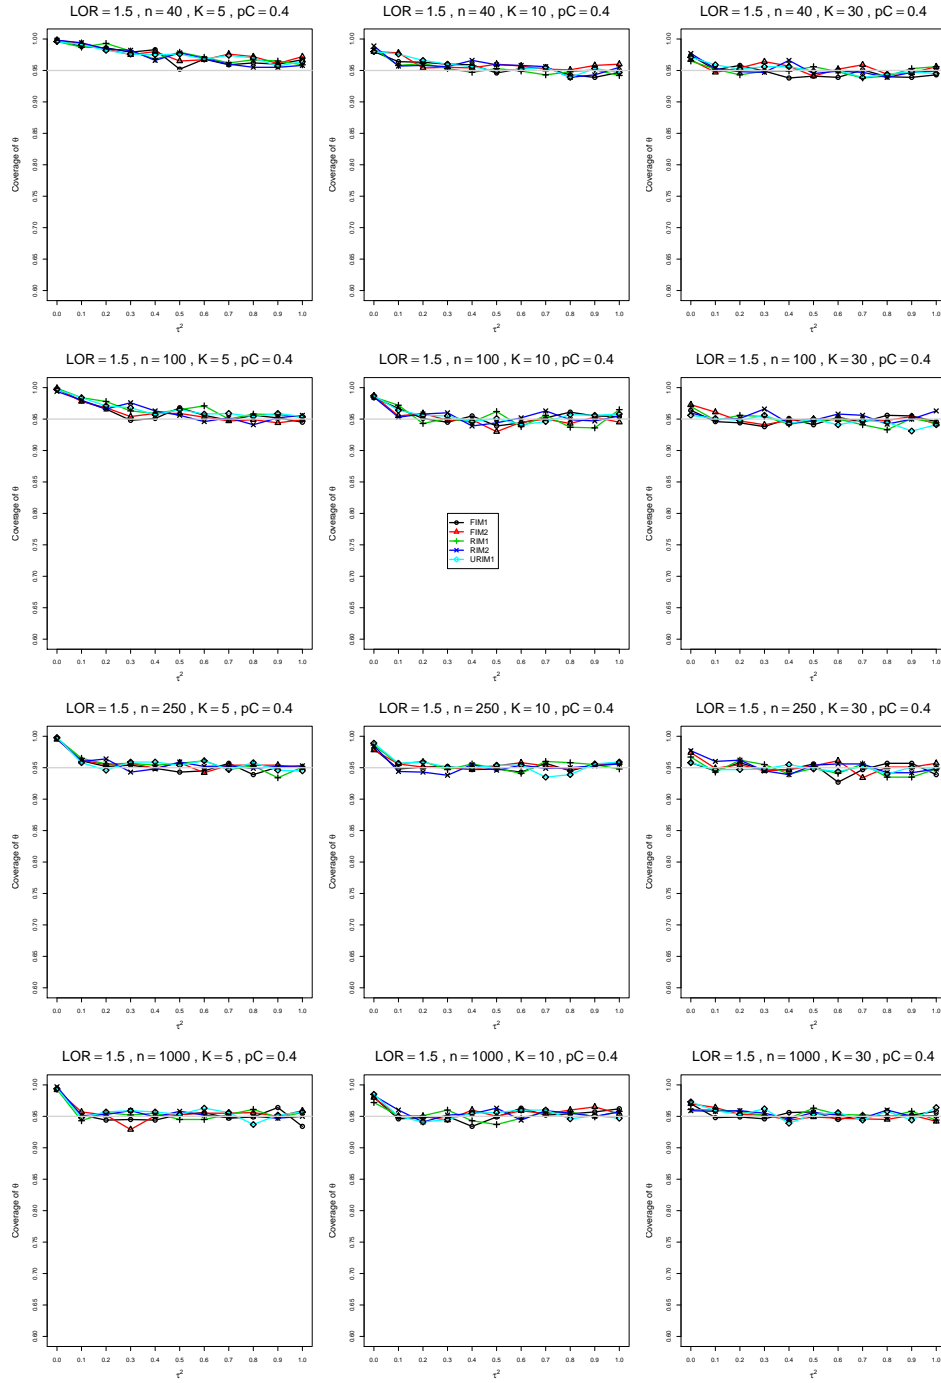

Figure A3.6.18: Coverage of the sample-size-weighted with Hartung-Knapp-Sidik-Jonkman (with KD) confidence interval for  $\theta = 1.5$ ,  $p_C = 0.4$ ,  $\sigma^2 = 0.4$ , constant sample sizes  $n = 40, 100, 250, 1000$ . The data-generation mechanisms are FIM1 ( $\circ$ ), FIM2 ( $\triangle$ ), RIM1 (+), RIM2 ( $\times$ ), and URIM1 ( $\diamond$ ).

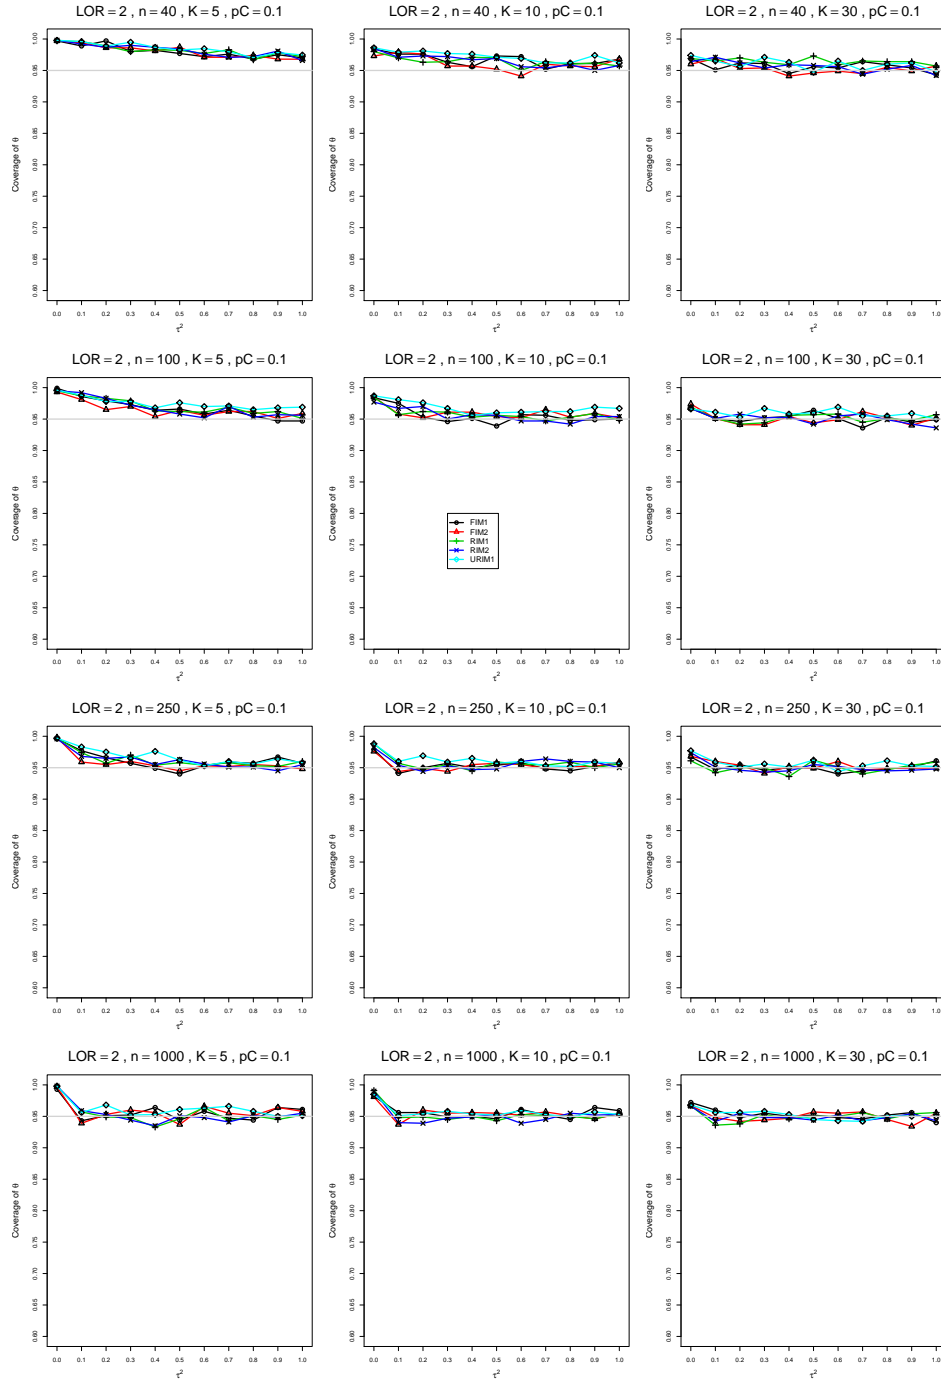

Figure A3.6.19: Coverage of the sample-size-weighted with Hartung-Knapp-Sidik-Jonkman (with KD) confidence interval for  $\theta = 2$ ,  $p_C = 0.1$ ,  $\sigma^2 = 0.4$ , constant sample sizes  $n = 40, 100, 250, 1000$ . The data-generation mechanisms are FIM1 ( $\circ$ ), FIM2 ( $\triangle$ ), RIM1 (+), RIM2 ( $\times$ ), and URIM1 ( $\diamond$ ).

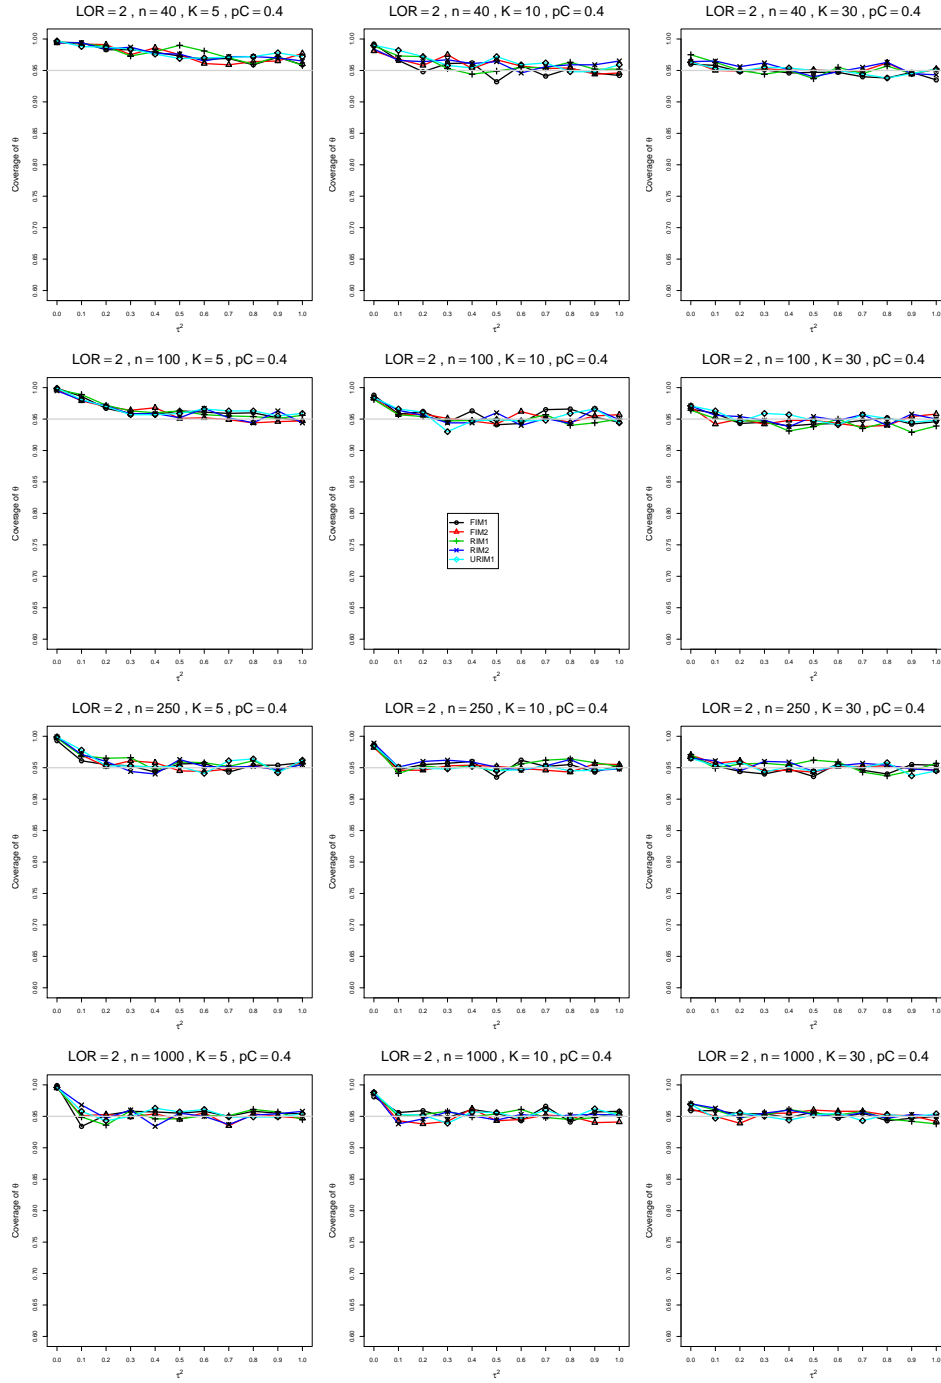

Figure A3.6.20: Coverage of the sample-size-weighted with Hartung-Knapp-Sidik-Jonkman (with KD) confidence interval for  $\theta = 2$ ,  $p_C = 0.4$ ,  $\sigma^2 = 0.4$ , constant sample sizes  $n = 40, 100, 250, 1000$ . The data-generation mechanisms are FIM1 ( $\circ$ ), FIM2 ( $\triangle$ ), RIM1 ( $+$ ), RIM2 ( $\times$ ), and URIM1 ( $\diamond$ ).
